# Supplementary material for: Diagnosis of two evaluation paths to density-based descriptors of molecular electronic transitions
Source: arXiv:1902.05840 ancillary file (2021-04-14)
Supplement: Supplementary file 1 [file Supplementary_Information.pdf]

# Diagnosis of two evaluation paths to density-based descriptors of molecular electronic transitions

## *Supplementary Information*

Gabriel Breuil,<sup>\*</sup> Kaltrina Shehu, Elise Lognon, Sylvain Pitié, Benjamin Lasorne, Thibaud Etienne<sup>†</sup>

Institut Charles Gerhardt – CNRS and Université de Montpellier

Place Eugène Bataillon – 34095 Montpellier, France

<sup>\*</sup> gabriel.breuil@umontpellier.fr

<sup>†</sup> thibaud.etienne@umontpellier.fr

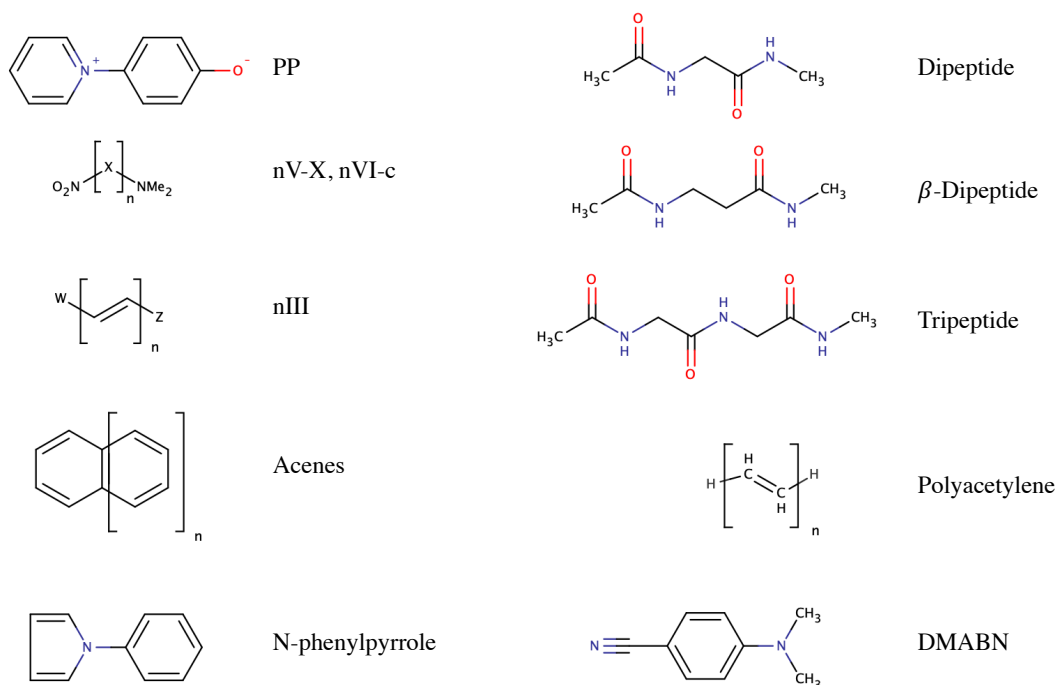

Figure S1: Sketch of the molecules investigated in this report. X can be a phenyl (nVI-c), a pyrrole (nV-NH), a furane (nV-O), a thiophene (nV-S), or a selenophene (nV-Se); W and Z can be replaced by a dimethylamino or a nitro group, with combinations giving the nIII-NMe<sub>2</sub>-NMe<sub>2</sub>, the nIII-NMe<sub>2</sub>-NO<sub>2</sub>, and the nIII-NO<sub>2</sub>-NO<sub>2</sub> series.

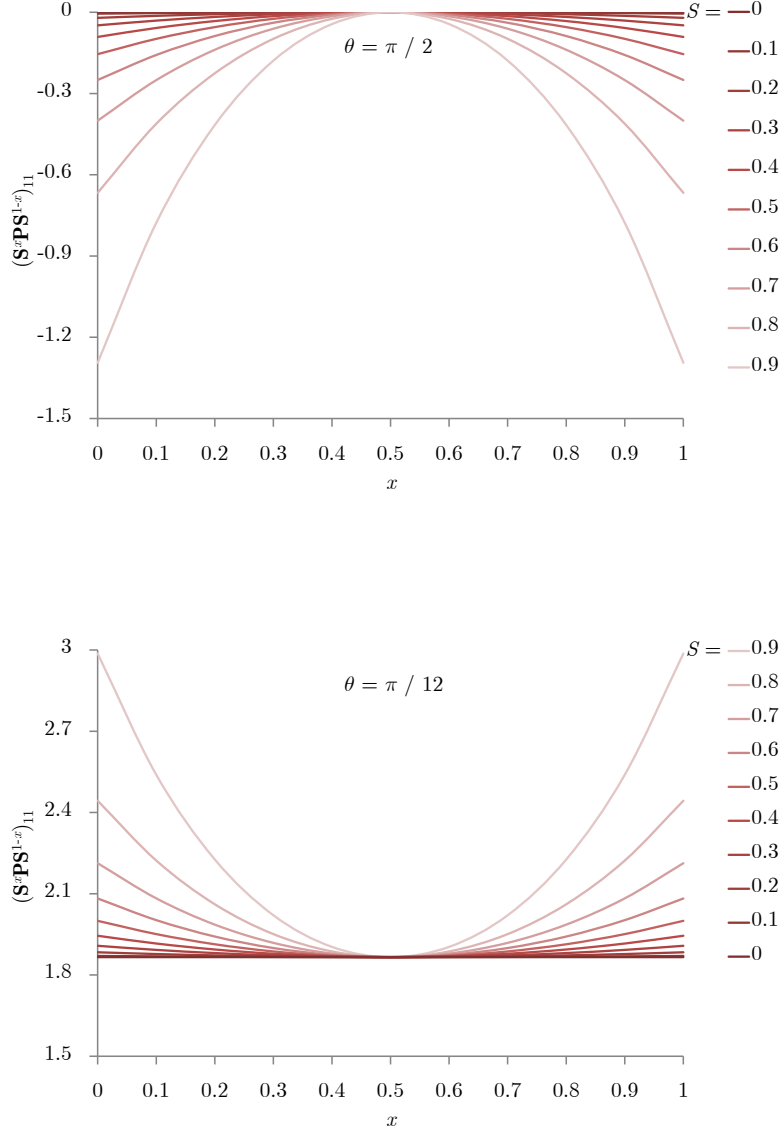

Figure S2: Illustration of two critical cases ( $\theta = \pi/2$  and  $\pi/12$ ) of the generalized orbital population analysis in the two-orbital model in appendix C.

| $n$                    | E-S | $\phi_S^\ell$ | $\phi_S$ | $\varphi^\ell$ | $\varphi$ | $\psi^\ell$ | $\psi$ |
|------------------------|-----|---------------|----------|----------------|-----------|-------------|--------|
| 1                      | 1   | 0.98          | 0.91     | 0.12           | 0.27      | 0.92        | 0.82   |
|                        | 2   | 0.98          | 0.97     | 0.13           | 0.16      | 0.92        | 0.90   |
|                        | 3   | 0.01          | 0.33     | 1.00           | 0.87      | 0.00        | 0.23   |
| 2                      | 1   | 0.98          | 0.90     | 0.10           | 0.29      | 0.93        | 0.80   |
|                        | 2   | 0.99          | 0.97     | 0.11           | 0.15      | 0.93        | 0.90   |
|                        | 3   | 0.98          | 0.91     | 0.13           | 0.26      | 0.91        | 0.82   |
| Continued on next page |     |               |          |                |           |             |        |

| $n$ | E-S | $\phi_S^\ell$ | $\phi_S$ | $\varphi^\ell$ | $\varphi$ | $\psi^\ell$ | $\psi$ |
|-----|-----|---------------|----------|----------------|-----------|-------------|--------|
| 3   | 1   | 0.99          | 0.90     | 0.09           | 0.27      | 0.94        | 0.81   |
|     | 2   | 0.99          | 0.97     | 0.11           | 0.15      | 0.93        | 0.90   |
|     | 3   | 0.97          | 0.91     | 0.21           | 0.29      | 0.86        | 0.80   |
| 4   | 1   | 0.99          | 0.90     | 0.08           | 0.27      | 0.95        | 0.81   |
|     | 2   | 0.95          | 0.90     | 0.24           | 0.30      | 0.85        | 0.80   |
|     | 3   | 0.94          | 0.89     | 0.27           | 0.35      | 0.82        | 0.76   |
| 5   | 1   | 0.99          | 0.90     | 0.08           | 0.26      | 0.95        | 0.82   |
|     | 2   | 0.96          | 0.90     | 0.26           | 0.32      | 0.83        | 0.78   |
|     | 3   | 0.94          | 0.89     | 0.25           | 0.35      | 0.83        | 0.76   |

Table S1: Reference ( $\phi_S$ ,  $\varphi$ ,  $\psi$ ) and approached ( $\phi_S^\ell$ ,  $\varphi^\ell$ ,  $\psi^\ell$ ) values of the topological descriptors for the three first excited-states (E-S) of acenes computed at the B3LYP/6-311++G(2d,p) level of theory.

| $n$ | E-S | $\phi_S^\ell$ | $\phi_S$ | $\varphi^\ell$ | $\varphi$ | $\psi^\ell$ | $\psi$ |
|-----|-----|---------------|----------|----------------|-----------|-------------|--------|
| 1   | 1   | 1.00          | 0.94     | 0.04           | 0.22      | 0.98        | 0.85   |
|     | 2   | 1.00          | 0.98     | 0.06           | 0.13      | 0.96        | 0.91   |
|     | 3   | 1.00          | 0.92     | 0.06           | 0.25      | 0.96        | 0.83   |
| 2   | 1   | 1.00          | 0.93     | 0.04           | 0.23      | 0.98        | 0.84   |
|     | 2   | 1.00          | 0.98     | 0.06           | 0.13      | 0.96        | 0.91   |
|     | 3   | 0.98          | 0.92     | 0.14           | 0.26      | 0.91        | 0.82   |
| 3   | 1   | 1.00          | 0.93     | 0.03           | 0.22      | 0.98        | 0.85   |
|     | 2   | 0.99          | 0.98     | 0.08           | 0.14      | 0.95        | 0.91   |
|     | 3   | 0.98          | 0.92     | 0.18           | 0.27      | 0.88        | 0.82   |
| 4   | 1   | 1.00          | 0.93     | 0.03           | 0.21      | 0.98        | 0.86   |
|     | 2   | 0.97          | 0.92     | 0.17           | 0.26      | 0.89        | 0.83   |
|     | 3   | 0.99          | 0.98     | 0.11           | 0.15      | 0.93        | 0.90   |
| 5   | 1   | 1.00          | 0.93     | 0.03           | 0.20      | 0.98        | 0.86   |
|     | 2   | 0.98          | 0.93     | 0.19           | 0.26      | 0.88        | 0.82   |
|     | 3   | 0.97          | 0.92     | 0.20           | 0.29      | 0.87        | 0.81   |

Table S2: Reference ( $\phi_S$ ,  $\varphi$ ,  $\psi$ ) and approached ( $\phi_S^\ell$ ,  $\varphi^\ell$ ,  $\psi^\ell$ ) values of the topological descriptors for the three first excited-states (E-S) of acenes computed at the B3LYP/6-31G level of theory.

| $n$ | E-S | $\phi_S^\ell$ | $\phi_S$ | $\varphi^\ell$ | $\varphi$ | $\psi^\ell$ | $\psi$ |
|-----|-----|---------------|----------|----------------|-----------|-------------|--------|
| 1   | 1   | 0.98          | 0.92     | 0.13           | 0.26      | 0.91        | 0.82   |
|     | 2   | 0.98          | 0.98     | 0.15           | 0.15      | 0.90        | 0.90   |
|     | 3   | 0.95          | 0.88     | 0.21           | 0.32      | 0.86        | 0.78   |
| 2   | 1   | 0.98          | 0.90     | 0.11           | 0.29      | 0.93        | 0.80   |
|     | 2   | 0.98          | 0.98     | 0.13           | 0.15      | 0.91        | 0.90   |
|     | 3   | 0.97          | 0.91     | 0.18           | 0.27      | 0.88        | 0.82   |
| 3   | 1   | 0.99          | 0.90     | 0.10           | 0.27      | 0.94        | 0.81   |
|     | 2   | 0.98          | 0.97     | 0.12           | 0.15      | 0.92        | 0.90   |
|     | 3   | 0.96          | 0.90     | 0.24           | 0.30      | 0.84        | 0.79   |
| 4   | 1   | 0.99          | 0.90     | 0.09           | 0.27      | 0.94        | 0.82   |
|     | 2   | 0.95          | 0.90     | 0.25           | 0.30      | 0.84        | 0.79   |
|     | 3   | 0.98          | 0.97     | 0.12           | 0.15      | 0.92        | 0.90   |
| 5   | 1   | 0.99          | 0.90     | 0.08           | 0.26      | 0.95        | 0.82   |
|     | 2   | 0.95          | 0.90     | 0.26           | 0.33      | 0.83        | 0.78   |
|     | 3   | 0.94          | 0.89     | 0.26           | 0.35      | 0.83        | 0.76   |

Table S3: Reference ( $\phi_S$ ,  $\varphi$ ,  $\psi$ ) and approached ( $\phi_S^\ell$ ,  $\varphi^\ell$ ,  $\psi^\ell$ ) values of the topological descriptors for the three first excited-states (E-S) of acenes computed at the B3LYP/cc-pVTZ level of theory.

| $n$ | E-S | $\phi_S^\ell$ | $\phi_S$ | $\varphi^\ell$ | $\varphi$ | $\psi^\ell$ | $\psi$ |
|-----|-----|---------------|----------|----------------|-----------|-------------|--------|
| 1   | 1   | 0.98          | 0.98     | 0.15           | 0.15      | 0.90        | 0.90   |
|     | 2   | 0.98          | 0.92     | 0.14           | 0.26      | 0.91        | 0.82   |
|     | 3   | 0.97          | 0.97     | 0.16           | 0.16      | 0.90        | 0.90   |
| 2   | 1   | 0.98          | 0.90     | 0.11           | 0.29      | 0.93        | 0.80   |
|     | 2   | 0.98          | 0.98     | 0.14           | 0.15      | 0.91        | 0.90   |
|     | 3   | 0.97          | 0.91     | 0.19           | 0.27      | 0.88        | 0.82   |
| 3   | 1   | 0.99          | 0.90     | 0.10           | 0.27      | 0.93        | 0.81   |
|     | 2   | 0.98          | 0.98     | 0.13           | 0.15      | 0.92        | 0.90   |
|     | 3   | 0.96          | 0.91     | 0.22           | 0.29      | 0.86        | 0.80   |
| 4   | 1   | 0.99          | 0.90     | 0.10           | 0.27      | 0.94        | 0.81   |
|     | 2   | 0.98          | 0.98     | 0.13           | 0.15      | 0.92        | 0.90   |

Continued on next page

| $n$ | E-S | $\phi_S^\ell$ | $\phi_S$ | $\varphi^\ell$ | $\varphi$ | $\psi^\ell$ | $\psi$ |
|-----|-----|---------------|----------|----------------|-----------|-------------|--------|
|     | 3   | 0.97          | 0.91     | 0.21           | 0.28      | 0.87        | 0.81   |
|     | 1   | 0.99          | 0.91     | 0.09           | 0.26      | 0.94        | 0.82   |
| 5   | 2   | 0.97          | 0.91     | 0.19           | 0.28      | 0.88        | 0.81   |
|     | 3   | 0.98          | 0.98     | 0.14           | 0.15      | 0.91        | 0.90   |

Table S4: Reference ( $\phi_S$ ,  $\varphi$ ,  $\psi$ ) and approached ( $\phi_S^\ell$ ,  $\varphi^\ell$ ,  $\psi^\ell$ ) values of the topological descriptors for the three first excited-states (E-S) of acenes computed at the CAM-B3LYP/cc-pVTZ level of theory.

| $n$ | E-S | $\phi_S^\ell$ | $\phi_S$ | $\varphi^\ell$ | $\varphi$ | $\psi^\ell$ | $\psi$ |
|-----|-----|---------------|----------|----------------|-----------|-------------|--------|
|     | 1   | 0.98          | 0.92     | 0.14           | 0.26      | 0.91        | 0.82   |
| 1   | 2   | 0.98          | 0.98     | 0.15           | 0.15      | 0.90        | 0.90   |
|     | 3   | 0.96          | 0.89     | 0.19           | 0.30      | 0.88        | 0.79   |
|     | 1   | 0.98          | 0.90     | 0.11           | 0.28      | 0.93        | 0.81   |
| 2   | 2   | 0.98          | 0.98     | 0.13           | 0.15      | 0.92        | 0.90   |
|     | 3   | 0.97          | 0.91     | 0.16           | 0.25      | 0.90        | 0.83   |
|     | 1   | 0.99          | 0.90     | 0.10           | 0.26      | 0.94        | 0.82   |
| 3   | 2   | 0.98          | 0.92     | 0.16           | 0.25      | 0.90        | 0.83   |
|     | 3   | 0.99          | 0.97     | 0.12           | 0.15      | 0.92        | 0.90   |
|     | 1   | 0.99          | 0.90     | 0.08           | 0.26      | 0.95        | 0.82   |
| 4   | 2   | 0.98          | 0.92     | 0.16           | 0.24      | 0.90        | 0.83   |
|     | 3   | 0.97          | 0.92     | 0.17           | 0.28      | 0.89        | 0.82   |
|     | 1   | 0.99          | 0.91     | 0.08           | 0.25      | 0.95        | 0.83   |
| 5   | 2   | 0.98          | 0.92     | 0.15           | 0.24      | 0.90        | 0.83   |
|     | 3   | 0.98          | 0.93     | 0.15           | 0.26      | 0.90        | 0.83   |

Table S5: Reference ( $\phi_S$ ,  $\varphi$ ,  $\psi$ ) and approached ( $\phi_S^\ell$ ,  $\varphi^\ell$ ,  $\psi^\ell$ ) values of the topological descriptors for the three first excited-states (E-S) of acenes computed at the PBE/cc-pVTZ level of theory.

| E-S | $\phi_S^\ell$ | $\phi_S$ | $\varphi^\ell$ | $\varphi$ | $\psi^\ell$ | $\psi$ |
|-----|---------------|----------|----------------|-----------|-------------|--------|
| 1   | 0.35          | 0.47     | 0.89           | 0.77      | 0.24        | 0.35   |
| 2   | 0.36          | 0.47     | 0.87           | 0.78      | 0.25        | 0.35   |
| 3   | 0.38          | 0.45     | 0.83           | 0.80      | 0.27        | 0.32   |

Table S6: Reference ( $\phi_S$ ,  $\varphi$ ,  $\psi$ ) and approached ( $\phi_S^\ell$ ,  $\varphi^\ell$ ,  $\psi^\ell$ ) values of the topological descriptors for the three first excited-states (E-S) of beta-dipeptide computed at the B3LYP/cc-pVTZ level of theory.

| E-S | $\phi_S^\ell$ | $\phi_S$ | $\varphi^\ell$ | $\varphi$ | $\psi^\ell$ | $\psi$ |
|-----|---------------|----------|----------------|-----------|-------------|--------|
| 1   | 0.35          | 0.47     | 0.89           | 0.77      | 0.24        | 0.35   |
| 2   | 0.35          | 0.47     | 0.88           | 0.78      | 0.24        | 0.35   |
| 3   | 0.29          | 0.39     | 0.88           | 0.84      | 0.21        | 0.28   |

Table S7: Reference ( $\phi_S$ ,  $\varphi$ ,  $\psi$ ) and approached ( $\phi_S^\ell$ ,  $\varphi^\ell$ ,  $\psi^\ell$ ) values of the topological descriptors for the three first excited-states (E-S) of beta-dipeptide computed at the CAM-B3LYP/cc-pVTZ level of theory.

| E-S | $\phi_S^\ell$ | $\phi_S$ | $\varphi^\ell$ | $\varphi$ | $\psi^\ell$ | $\psi$ |
|-----|---------------|----------|----------------|-----------|-------------|--------|
| 1   | 0.34          | 0.41     | 0.87           | 0.82      | 0.24        | 0.30   |
| 2   | 0.33          | 0.40     | 0.89           | 0.82      | 0.22        | 0.29   |
| 3   | 0.39          | 0.50     | 0.87           | 0.76      | 0.27        | 0.37   |

Table S8: Reference ( $\phi_S$ ,  $\varphi$ ,  $\psi$ ) and approached ( $\phi_S^\ell$ ,  $\varphi^\ell$ ,  $\psi^\ell$ ) values of the topological descriptors for the three first excited-states (E-S) of beta-dipeptide computed at the PBE/cc-pVTZ level of theory.

| E-S | $\phi_S^\ell$ | $\phi_S$ | $\varphi^\ell$ | $\varphi$ | $\psi^\ell$ | $\psi$ |
|-----|---------------|----------|----------------|-----------|-------------|--------|
| 1   | 0.08          | 0.71     | 0.99           | 0.57      | 0.05        | 0.57   |
| 2   | 0.12          | 0.71     | 0.99           | 0.57      | 0.08        | 0.57   |
| 3   | 0.84          | 0.80     | 0.43           | 0.50      | 0.70        | 0.65   |

Table S9: Reference ( $\phi_S$ ,  $\varphi$ ,  $\psi$ ) and approached ( $\phi_S^\ell$ ,  $\varphi^\ell$ ,  $\psi^\ell$ ) values of the topological descriptors for the three first excited-states (E-S) of CO computed at the B3LYP/*d*-aug-cc-pVTZ level of theory.

| E-S | $\phi_S^\ell$ | $\phi_S$ | $\varphi^\ell$ | $\varphi$ | $\psi^\ell$ | $\psi$ |
|-----|---------------|----------|----------------|-----------|-------------|--------|
| 1   | 0.12          | 0.71     | 0.99           | 0.57      | 0.08        | 0.57   |
| 2   | 0.08          | 0.71     | 0.99           | 0.57      | 0.05        | 0.57   |
| 3   | 0.84          | 0.81     | 0.43           | 0.50      | 0.70        | 0.65   |

Table S10: Reference ( $\phi_S$ ,  $\varphi$ ,  $\psi$ ) and approached ( $\phi_S^\ell$ ,  $\varphi^\ell$ ,  $\psi^\ell$ ) values of the topological descriptors for the three first excited-states (E-S) of CO computed at the CAM-B3LYP/*d*-aug-cc-pVTZ level of theory.

| E-S | $\phi_S^\ell$ | $\phi_S$ | $\varphi^\ell$ | $\varphi$ | $\psi^\ell$ | $\psi$ |
|-----|---------------|----------|----------------|-----------|-------------|--------|
| 1   | 0.12          | 0.71     | 0.99           | 0.58      | 0.08        | 0.56   |
| 2   | 0.07          | 0.70     | 0.99           | 0.58      | 0.05        | 0.56   |
| 3   | 0.36          | 0.28     | 0.89           | 0.92      | 0.25        | 0.19   |

Table S11: Reference ( $\phi_S$ ,  $\varphi$ ,  $\psi$ ) and approached ( $\phi_S^\ell$ ,  $\varphi^\ell$ ,  $\psi^\ell$ ) values of the topological descriptors for the three first excited-states (E-S) of CO computed at the PBE/*d*-aug-cc-pVTZ level of theory.

| E-S | $\phi_S^\ell$ | $\phi_S$ | $\varphi^\ell$ | $\varphi$ | $\psi^\ell$ | $\psi$ |
|-----|---------------|----------|----------------|-----------|-------------|--------|
| 1   | 0.13          | 0.47     | 0.97           | 0.78      | 0.08        | 0.34   |
| 2   | 0.11          | 0.46     | 0.98           | 0.78      | 0.07        | 0.34   |
| 3   | 0.30          | 0.32     | 0.85           | 0.87      | 0.22        | 0.22   |

Table S12: Reference ( $\phi_S$ ,  $\varphi$ ,  $\psi$ ) and approached ( $\phi_S^\ell$ ,  $\varphi^\ell$ ,  $\psi^\ell$ ) values of the topological descriptors for the three first excited-states (E-S) of dipeptide computed at the B3LYP/cc-pVTZ level of theory.

| E-S | $\phi_S^\ell$ | $\phi_S$ | $\varphi^\ell$ | $\varphi$ | $\psi^\ell$ | $\psi$ |
|-----|---------------|----------|----------------|-----------|-------------|--------|
| 1   | 0.12          | 0.47     | 0.97           | 0.78      | 0.08        | 0.34   |
| 2   | 0.11          | 0.47     | 0.98           | 0.78      | 0.07        | 0.35   |
| 3   | 0.31          | 0.47     | 0.91           | 0.78      | 0.21        | 0.34   |

Table S13: Reference ( $\phi_S$ ,  $\varphi$ ,  $\psi$ ) and approached ( $\phi_S^\ell$ ,  $\varphi^\ell$ ,  $\psi^\ell$ ) values of the topological descriptors for the three first excited-states (E-S) of dipeptide computed at the CAM-B3LYP/cc-pVTZ level of theory.

| E-S | $\phi_S^\ell$ | $\phi_S$ | $\varphi^\ell$ | $\varphi$ | $\psi^\ell$ | $\psi$ |
|-----|---------------|----------|----------------|-----------|-------------|--------|
| 1   | 0.06          | 0.16     | 0.99           | 0.96      | 0.04        | 0.11   |
| 2   | 0.24          | 0.24     | 0.88           | 0.91      | 0.17        | 0.17   |
| 3   | 0.11          | 0.13     | 0.96           | 0.96      | 0.08        | 0.09   |

Table S14: Reference ( $\phi_S$ ,  $\varphi$ ,  $\psi$ ) and approached ( $\phi_S^\ell$ ,  $\varphi^\ell$ ,  $\psi^\ell$ ) values of the topological descriptors for the three first excited-states (E-S) of dipeptide computed at the PBE/cc-pVTZ level of theory.

| E-S | $\phi_S^\ell$ | $\phi_S$ | $\varphi^\ell$ | $\varphi$ | $\psi^\ell$ | $\psi$ |
|-----|---------------|----------|----------------|-----------|-------------|--------|
| 1   | 0.34          | 0.35     | 0.86           | 0.86      | 0.24        | 0.25   |
| 2   | 0.26          | 0.31     | 0.89           | 0.87      | 0.18        | 0.22   |
| 3   | 0.19          | 0.21     | 0.93           | 0.93      | 0.13        | 0.14   |

Table S15: Reference ( $\phi_S$ ,  $\varphi$ ,  $\psi$ ) and approached ( $\phi_S^\ell$ ,  $\varphi^\ell$ ,  $\psi^\ell$ ) values of the topological descriptors for the three first excited-states (E-S) of DMABN computed at the B3LYP/cc-pVTZ level of theory.

| E-S | $\phi_S^\ell$ | $\phi_S$ | $\varphi^\ell$ | $\varphi$ | $\psi^\ell$ | $\psi$ |
|-----|---------------|----------|----------------|-----------|-------------|--------|
| 1   | 0.40          | 0.43     | 0.84           | 0.82      | 0.28        | 0.31   |
| 2   | 0.89          | 0.83     | 0.32           | 0.41      | 0.78        | 0.71   |
| 3   | 0.39          | 0.43     | 0.82           | 0.80      | 0.28        | 0.32   |

Table S16: Reference ( $\phi_S$ ,  $\varphi$ ,  $\psi$ ) and approached ( $\phi_S^\ell$ ,  $\varphi^\ell$ ,  $\psi^\ell$ ) values of the topological descriptors for the three first excited-states (E-S) of DMABN computed at the CAM-B3LYP/cc-pVTZ level of theory.

| E-S | $\phi_S^\ell$ | $\phi_S$ | $\varphi^\ell$ | $\varphi$ | $\psi^\ell$ | $\psi$ |
|-----|---------------|----------|----------------|-----------|-------------|--------|
| 1   | 0.17          | 0.18     | 0.94           | 0.95      | 0.12        | 0.12   |
| 2   | 0.10          | 0.11     | 0.98           | 0.97      | 0.07        | 0.07   |
| 3   | 0.30          | 0.32     | 0.87           | 0.87      | 0.21        | 0.22   |

Table S17: Reference ( $\phi_S$ ,  $\varphi$ ,  $\psi$ ) and approached ( $\phi_S^\ell$ ,  $\varphi^\ell$ ,  $\psi^\ell$ ) values of the topological descriptors for the three first excited-states (E-S) of DMABN computed at the PBE/cc-pVTZ level of theory.



| E-S | $\phi_S^\ell$ | $\phi_S$ | $\varphi^\ell$ | $\varphi$ | $\psi^\ell$ | $\psi$ |
|-----|---------------|----------|----------------|-----------|-------------|--------|
| 1   | 0.70          | 0.52     | 0.58           | 0.74      | 0.56        | 0.39   |
| 2   | 0.18          | 0.40     | 0.97           | 0.83      | 0.12        | 0.29   |
| 3   | 0.08          | 0.58     | 0.99           | 0.69      | 0.05        | 0.45   |

Table S18: Reference ( $\phi_S$ ,  $\varphi$ ,  $\psi$ ) and approached ( $\phi_S^\ell$ ,  $\varphi^\ell$ ,  $\psi^\ell$ ) values of the topological descriptors for the three first excited-states (E-S) of H<sub>2</sub>CO computed at the B3LYP/cc-pVTZ level of theory.

| E-S | $\phi_S^\ell$ | $\phi_S$ | $\varphi^\ell$ | $\varphi$ | $\psi^\ell$ | $\psi$ |
|-----|---------------|----------|----------------|-----------|-------------|--------|
| 1   | 0.70          | 0.52     | 0.58           | 0.73      | 0.56        | 0.39   |
| 2   | 0.18          | 0.41     | 0.97           | 0.82      | 0.12        | 0.30   |
| 3   | 0.08          | 0.58     | 0.99           | 0.69      | 0.05        | 0.45   |

Table S19: Reference ( $\phi_S$ ,  $\varphi$ ,  $\psi$ ) and approached ( $\phi_S^\ell$ ,  $\varphi^\ell$ ,  $\psi^\ell$ ) values of the topological descriptors for the three first excited-states (E-S) of H<sub>2</sub>CO computed at the CAM-B3LYP/cc-pVTZ level of theory.

| E-S | $\phi_S^\ell$ | $\phi_S$ | $\varphi^\ell$ | $\varphi$ | $\psi^\ell$ | $\psi$ |
|-----|---------------|----------|----------------|-----------|-------------|--------|
| 1   | 0.70          | 0.52     | 0.57           | 0.73      | 0.57        | 0.39   |
| 2   | 0.19          | 0.39     | 0.97           | 0.83      | 0.12        | 0.28   |
| 3   | 0.52          | 0.56     | 0.82           | 0.75      | 0.36        | 0.41   |

Table S20: Reference ( $\phi_S$ ,  $\varphi$ ,  $\psi$ ) and approached ( $\phi_S^\ell$ ,  $\varphi^\ell$ ,  $\psi^\ell$ ) values of the topological descriptors for the three first excited-states (E-S) of H<sub>2</sub>CO computed at the PBE/cc-pVTZ level of theory.

| E-S | $\phi_S^\ell$ | $\phi_S$ | $\varphi^\ell$ | $\varphi$ | $\psi^\ell$ | $\psi$ |
|-----|---------------|----------|----------------|-----------|-------------|--------|
| 1   | 0.38          | 0.48     | 0.81           | 0.77      | 0.28        | 0.35   |
| 2   | 0.18          | 0.48     | 0.95           | 0.77      | 0.12        | 0.35   |
| 3   | 0.59          | 0.67     | 0.74           | 0.63      | 0.43        | 0.52   |

Table S21: Reference ( $\phi_S$ ,  $\varphi$ ,  $\psi$ ) and approached ( $\phi_S^\ell$ ,  $\varphi^\ell$ ,  $\psi^\ell$ ) values of the topological descriptors for the three first excited-states (E-S) of HCl computed at the B3LYP/cc-pVTZ level of theory.

| E-S | $\phi_S^\ell$ | $\phi_S$ | $\varphi^\ell$ | $\varphi$ | $\psi^\ell$ | $\psi$ |
|-----|---------------|----------|----------------|-----------|-------------|--------|
| 1   | 0.39          | 0.49     | 0.81           | 0.77      | 0.29        | 0.36   |
| 2   | 0.18          | 0.48     | 0.95           | 0.77      | 0.12        | 0.36   |
| 3   | 0.60          | 0.68     | 0.74           | 0.63      | 0.44        | 0.52   |

Table S22: Reference ( $\phi_S$ ,  $\varphi$ ,  $\psi$ ) and approached ( $\phi_S^\ell$ ,  $\varphi^\ell$ ,  $\psi^\ell$ ) values of the topological descriptors for the three first excited-states (E-S) of HCl computed at the CAM-B3LYP/cc-pVTZ level of theory.

| E-S | $\phi_S^\ell$ | $\phi_S$ | $\varphi^\ell$ | $\varphi$ | $\psi^\ell$ | $\psi$ |
|-----|---------------|----------|----------------|-----------|-------------|--------|
| 1   | 0.38          | 0.47     | 0.82           | 0.77      | 0.28        | 0.35   |
| 2   | 0.20          | 0.47     | 0.93           | 0.77      | 0.14        | 0.35   |
| 3   | 0.58          | 0.66     | 0.75           | 0.64      | 0.42        | 0.51   |

Table S23: Reference ( $\phi_S$ ,  $\varphi$ ,  $\psi$ ) and approached ( $\phi_S^\ell$ ,  $\varphi^\ell$ ,  $\psi^\ell$ ) values of the topological descriptors for the three first excited-states (E-S) of HCl computed at the PBE/cc-pVTZ level of theory.

| E-S | $\phi_S^\ell$ | $\phi_S$ | $\varphi^\ell$ | $\varphi$ | $\psi^\ell$ | $\psi$ |
|-----|---------------|----------|----------------|-----------|-------------|--------|
| 1   | 0.97          | 0.91     | 0.18           | 0.30      | 0.88        | 0.80   |
| 2   | 0.06          | 0.69     | 1.00           | 0.59      | 0.04        | 0.55   |
| 3   | 0.14          | 0.69     | 0.99           | 0.59      | 0.09        | 0.55   |

Table S24: Reference ( $\phi_S$ ,  $\varphi$ ,  $\psi$ ) and approached ( $\phi_S^\ell$ ,  $\varphi^\ell$ ,  $\psi^\ell$ ) values of the topological descriptors for the three first excited-states (E-S) of N<sub>2</sub> computed at the B3LYP/*d*-aug-cc-pVTZ level of theory.

| E-S | $\phi_S^\ell$ | $\phi_S$ | $\varphi^\ell$ | $\varphi$ | $\psi^\ell$ | $\psi$ |
|-----|---------------|----------|----------------|-----------|-------------|--------|
| 1   | 0.97          | 0.91     | 0.18           | 0.30      | 0.88        | 0.80   |
| 2   | 0.15          | 0.69     | 0.99           | 0.59      | 0.09        | 0.55   |
| 3   | 0.06          | 0.69     | 1.00           | 0.59      | 0.04        | 0.55   |

Table S25: Reference ( $\phi_S$ ,  $\varphi$ ,  $\psi$ ) and approached ( $\phi_S^\ell$ ,  $\varphi^\ell$ ,  $\psi^\ell$ ) values of the topological descriptors for the three first excited-states (E-S) of N<sub>2</sub> computed at the CAM-B3LYP/*d*-aug-cc-pVTZ level of theory.

| E-S | $\phi_S^\ell$ | $\phi_S$ | $\varphi^\ell$ | $\varphi$ | $\psi^\ell$ | $\psi$ |
|-----|---------------|----------|----------------|-----------|-------------|--------|
| 1   | 0.05          | 0.69     | 1.00           | 0.59      | 0.03        | 0.55   |
| 2   | 0.14          | 0.69     | 0.99           | 0.59      | 0.09        | 0.55   |
| 3   | 0.97          | 0.91     | 0.18           | 0.29      | 0.88        | 0.80   |

Table S26: Reference ( $\phi_S$ ,  $\varphi$ ,  $\psi$ ) and approached ( $\phi_S^\ell$ ,  $\varphi^\ell$ ,  $\psi^\ell$ ) values of the topological descriptors for the three first excited-states (E-S) of N<sub>2</sub> computed at the PBE/*d*-aug-cc-pVTZ level of theory.

| <i>n</i> | E-S | $\phi_S^\ell$ | $\phi_S$ | $\varphi^\ell$ | $\varphi$ | $\psi^\ell$ | $\psi$ |
|----------|-----|---------------|----------|----------------|-----------|-------------|--------|
| 1        | 1   | 0.56          | 0.57     | 0.77           | 0.75      | 0.40        | 0.41   |
|          | 2   | 0.07          | 0.49     | 0.99           | 0.75      | 0.05        | 0.37   |
|          | 3   | 0.37          | 0.40     | 0.86           | 0.82      | 0.26        | 0.29   |
| 3        | 1   | 0.47          | 0.48     | 0.82           | 0.81      | 0.33        | 0.34   |
|          | 2   | 0.73          | 0.73     | 0.54           | 0.56      | 0.60        | 0.58   |
|          | 3   | 0.62          | 0.63     | 0.67           | 0.66      | 0.48        | 0.49   |
| 4        | 1   | 0.39          | 0.39     | 0.86           | 0.86      | 0.27        | 0.27   |
|          | 2   | 0.60          | 0.60     | 0.72           | 0.71      | 0.44        | 0.44   |
|          | 3   | 0.75          | 0.71     | 0.52           | 0.58      | 0.61        | 0.57   |
| 5        | 1   | 0.33          | 0.34     | 0.89           | 0.89      | 0.23        | 0.23   |
|          | 2   | 0.52          | 0.53     | 0.78           | 0.77      | 0.38        | 0.38   |
|          | 3   | 0.75          | 0.71     | 0.52           | 0.58      | 0.61        | 0.56   |

Table S27: Reference ( $\phi_S$ ,  $\varphi$ ,  $\psi$ ) and approached ( $\phi_S^\ell$ ,  $\varphi^\ell$ ,  $\psi^\ell$ ) values of the topological descriptors for the three first excited-states (E-S) of nV-NH in linear configuration (i.e., with heteroatom on the top of alternating spacer subunits) computed at the PBE0/6-311++G(2d,p) level of theory.

| <i>n</i> | E-S | $\phi_S^\ell$ | $\phi_S$ | $\varphi^\ell$ | $\varphi$ | $\psi^\ell$ | $\psi$ |
|----------|-----|---------------|----------|----------------|-----------|-------------|--------|
| 1        | 1   | 0.67          | 0.69     | 0.66           | 0.64      | 0.50        | 0.53   |
|          | 2   | 0.13          | 0.48     | 0.98           | 0.76      | 0.08        | 0.36   |
|          | 3   | 0.20          | 0.34     | 0.95           | 0.87      | 0.13        | 0.23   |
| 2        | 1   | 0.54          | 0.57     | 0.78           | 0.75      | 0.39        | 0.41   |
|          | 2   | 0.32          | 0.37     | 0.89           | 0.85      | 0.22        | 0.26   |

Continued on next page

| $n$ | E-S | $\phi_S^\ell$ | $\phi_S$ | $\varphi^\ell$ | $\varphi$ | $\psi^\ell$ | $\psi$ |
|-----|-----|---------------|----------|----------------|-----------|-------------|--------|
|     | 3   | 0.14          | 0.50     | 0.98           | 0.75      | 0.09        | 0.38   |
|     | 1   | 0.46          | 0.48     | 0.82           | 0.81      | 0.33        | 0.34   |
| 3   | 2   | 0.29          | 0.32     | 0.90           | 0.87      | 0.20        | 0.23   |
|     | 3   | 0.70          | 0.70     | 0.59           | 0.60      | 0.55        | 0.55   |
|     | 1   | 0.38          | 0.40     | 0.86           | 0.86      | 0.27        | 0.28   |
| 4   | 2   | 0.59          | 0.59     | 0.72           | 0.71      | 0.44        | 0.44   |
|     | 3   | 0.21          | 0.25     | 0.94           | 0.92      | 0.14        | 0.17   |
|     | 1   | 0.28          | 0.29     | 0.92           | 0.91      | 0.19        | 0.20   |
| 5   | 2   | 0.53          | 0.53     | 0.77           | 0.77      | 0.38        | 0.39   |
|     | 3   | 0.18          | 0.21     | 0.95           | 0.93      | 0.12        | 0.14   |

Table S28: Reference ( $\phi_S$ ,  $\varphi$ ,  $\psi$ ) and approached ( $\phi_S^\ell$ ,  $\varphi^\ell$ ,  $\psi^\ell$ ) values of the topological descriptors for the three first excited-states (E-S) of nV-NH in crowned configuration (i.e., with heteroatom on the top of each spacer subunit) computed at the PBE0/6-311++G(2d,p) level of theory.

| $n$ | E-S | $\vartheta^\ell$ | $\vartheta_{d,m}$ | $\vartheta_{a,m}$ | $\vartheta_{d,f}$ | $\vartheta_{a,f}$ |
|-----|-----|------------------|-------------------|-------------------|-------------------|-------------------|
|     | 1   | 1.00             | 1.00              | 0.93              | 1.00              | 0.92              |
| 1   | 2   | 1.00             | 1.00              | 0.89              | 1.00              | 0.88              |
|     | 3   | 1.00             | 1.00              | 0.92              | 1.00              | 0.92              |
|     | 1   | 1.00             | 1.00              | 0.88              | 1.00              | 0.88              |
| 2   | 2   | 1.00             | 1.00              | 0.87              | 1.00              | 0.87              |
|     | 3   | 1.00             | 1.00              | 0.90              | 1.00              | 0.89              |
|     | 1   | 1.00             | 1.00              | 0.89              | 1.00              | 0.89              |
| 3   | 2   | 1.01             | 1.01              | 0.92              | 1.01              | 0.92              |
|     | 3   | 1.00             | 1.00              | 0.95              | 1.00              | 0.95              |
|     | 1   | 1.04             | 1.04              | 1.01              | 1.04              | 1.01              |
| 4   | 2   | 1.00             | 1.00              | 0.89              | 1.00              | 0.89              |
|     | 3   | 1.01             | 1.01              | 0.92              | 1.01              | 0.92              |
|     | 1   | 1.05             | 1.05              | 1.04              | 1.05              | 1.04              |
| 5   | 2   | 1.00             | 1.00              | 0.89              | 1.00              | 0.89              |
|     | 3   | 1.00             | 1.00              | 0.90              | 1.00              | 0.89              |

Table S29: Reference ( $\vartheta^\ell$ ), and Cartesian grid detachment (d) and attachment (a) density integrals

( $\vartheta$ ) obtained with a medium (m) and a fine (f) grid for the three first excited-states (E-S) of nIII-NMe<sub>2</sub>-NMe<sub>2</sub> computed at the PBE0/6-311++G(2d,p) level of theory.

| $n$ | E-S | $\phi_S^\ell$ | $\phi_S$ | $\varphi^\ell$ | $\varphi$ | $\psi^\ell$ | $\psi$ |
|-----|-----|---------------|----------|----------------|-----------|-------------|--------|
| 1   | 1   | 0.29          | 0.35     | 0.91           | 0.87      | 0.20        | 0.24   |
|     | 2   | 0.31          | 0.32     | 0.89           | 0.88      | 0.21        | 0.22   |
|     | 3   | 0.33          | 0.30     | 0.88           | 0.89      | 0.23        | 0.21   |
| 2   | 1   | 0.28          | 0.37     | 0.93           | 0.85      | 0.18        | 0.26   |
|     | 2   | 0.21          | 0.29     | 0.95           | 0.90      | 0.14        | 0.20   |
|     | 3   | 0.15          | 0.28     | 0.97           | 0.90      | 0.10        | 0.19   |
| 3   | 1   | 0.18          | 0.30     | 0.96           | 0.89      | 0.12        | 0.21   |
|     | 2   | 0.53          | 0.55     | 0.75           | 0.73      | 0.39        | 0.41   |
|     | 3   | 0.29          | 0.34     | 0.92           | 0.87      | 0.19        | 0.24   |
| 4   | 1   | 0.84          | 0.78     | 0.37           | 0.48      | 0.73        | 0.65   |
|     | 2   | 0.20          | 0.30     | 0.96           | 0.90      | 0.13        | 0.21   |
|     | 3   | 0.48          | 0.49     | 0.78           | 0.77      | 0.35        | 0.36   |
| 5   | 1   | 0.91          | 0.83     | 0.31           | 0.44      | 0.79        | 0.69   |
|     | 2   | 0.27          | 0.34     | 0.93           | 0.89      | 0.18        | 0.24   |
|     | 3   | 0.29          | 0.36     | 0.92           | 0.87      | 0.19        | 0.25   |

Table S30: Reference ( $\phi_S$ ,  $\varphi$ ,  $\psi$ ) and approached ( $\phi_S^\ell$ ,  $\varphi^\ell$ ,  $\psi^\ell$ ) values of the topological descriptors for the three first excited-states (E-S) of nIII-NMe<sub>2</sub>-NMe<sub>2</sub> computed at the PBE0/6-311++G(2d,p) level of theory.

| $n$ | E-S | $\vartheta^\ell$ | $\vartheta_{d,m}$ | $\vartheta_{a,m}$ | $\vartheta_{d,f}$ | $\vartheta_{a,f}$ |
|-----|-----|------------------|-------------------|-------------------|-------------------|-------------------|
| 1   | 1   | 1.00             | 1.00              | 1.00              | 1.00              | 1.00              |
|     | 2   | 1.03             | 1.03              | 1.03              | 1.03              | 1.03              |
|     | 3   | 1.00             | 1.00              | 1.00              | 1.00              | 1.00              |
| 2   | 1   | 1.04             | 1.04              | 1.04              | 1.04              | 1.04              |
|     | 2   | 1.00             | 1.00              | 1.00              | 1.00              | 1.00              |
|     | 3   | 1.00             | 1.00              | 1.00              | 1.00              | 1.00              |
| 3   | 1   | 1.05             | 1.05              | 1.05              | 1.05              | 1.05              |

Continued on next page

| $n$ | E-S | $\vartheta^\ell$ | $\vartheta_{d,m}$ | $\vartheta_{a,m}$ | $\vartheta_{d,f}$ | $\vartheta_{a,f}$ |
|-----|-----|------------------|-------------------|-------------------|-------------------|-------------------|
| 3   | 2   | 1.00             | 1.00              | 1.00              | 1.00              | 1.00              |
|     | 3   | 1.00             | 1.00              | 1.00              | 1.00              | 1.00              |
| 4   | 1   | 1.06             | 1.06              | 1.06              | 1.06              | 1.06              |
|     | 2   | 1.00             | 1.00              | 1.00              | 1.00              | 1.00              |
|     | 3   | 1.01             | 1.01              | 0.96              | 1.01              | 0.96              |
| 5   | 1   | 1.06             | 1.06              | 1.06              | 1.06              | 1.06              |
|     | 2   | 1.00             | 1.00              | 1.00              | 1.00              | 1.00              |
|     | 3   | 1.02             | 1.02              | 1.01              | 1.02              | 1.01              |

Table S31: Reference ( $\vartheta^\ell$ ), and Cartesian grid detachment (d) and attachment (a) density integrals ( $\vartheta$ ) obtained with a medium (m) and a fine (f) grid for the three first excited-states (E-S) of nIII-NMe<sub>2</sub>-NO<sub>2</sub> computed at the PBE0/6-311++G(2d,p) level of theory.

| $n$ | E-S | $\phi_S^\ell$ | $\phi_S$ | $\varphi^\ell$ | $\varphi$ | $\psi^\ell$ | $\psi$ |
|-----|-----|---------------|----------|----------------|-----------|-------------|--------|
| 1   | 1   | 0.14          | 0.48     | 0.98           | 0.76      | 0.09        | 0.36   |
|     | 2   | 0.60          | 0.65     | 0.70           | 0.65      | 0.45        | 0.50   |
|     | 3   | 0.17          | 0.54     | 0.97           | 0.73      | 0.11        | 0.41   |
| 2   | 1   | 0.60          | 0.67     | 0.71           | 0.65      | 0.45        | 0.51   |
|     | 2   | 0.09          | 0.49     | 0.99           | 0.76      | 0.06        | 0.36   |
|     | 3   | 0.09          | 0.51     | 0.99           | 0.74      | 0.06        | 0.39   |
| 3   | 1   | 0.62          | 0.67     | 0.68           | 0.64      | 0.47        | 0.52   |
|     | 2   | 0.13          | 0.46     | 0.98           | 0.77      | 0.08        | 0.34   |
|     | 3   | 0.13          | 0.51     | 0.98           | 0.74      | 0.08        | 0.38   |
| 4   | 1   | 0.63          | 0.68     | 0.66           | 0.62      | 0.49        | 0.53   |
|     | 2   | 0.06          | 0.45     | 0.99           | 0.78      | 0.04        | 0.34   |
|     | 3   | 0.63          | 0.68     | 0.63           | 0.61      | 0.50        | 0.53   |
| 5   | 1   | 0.64          | 0.68     | 0.64           | 0.62      | 0.50        | 0.53   |
|     | 2   | 0.12          | 0.45     | 0.98           | 0.78      | 0.08        | 0.33   |
|     | 3   | 0.87          | 0.86     | 0.40           | 0.42      | 0.72        | 0.71   |

Table S32: Reference ( $\phi_S$ ,  $\varphi$ ,  $\psi$ ) and approached ( $\phi_S^\ell$ ,  $\varphi^\ell$ ,  $\psi^\ell$ ) values of the topological descriptors for the three first excited-states (E-S) of nIII-NMe<sub>2</sub>-NO<sub>2</sub> computed at the PBE0/6-311++G(2d,p) level of theory.

| $n$ | E-S | $\vartheta^\ell$ | $\vartheta_{d,m}$ | $\vartheta_{a,m}$ | $\vartheta_{d,f}$ | $\vartheta_{a,f}$ |
|-----|-----|------------------|-------------------|-------------------|-------------------|-------------------|
| 1   | 1   | 1.00             | 1.00              | 1.00              | 1.00              | 1.00              |
|     | 2   | 1.00             | 1.00              | 1.00              | 1.00              | 1.00              |
|     | 3   | 1.00             | 1.00              | 1.00              | 1.00              | 1.00              |
| 2   | 1   | 1.00             | 1.00              | 1.00              | 1.00              | 1.00              |
|     | 2   | 1.00             | 1.00              | 1.00              | 1.00              | 1.00              |
|     | 3   | 1.00             | 1.00              | 1.00              | 1.00              | 1.00              |
| 3   | 1   | 1.00             | 1.00              | 1.00              | 1.00              | 1.00              |
|     | 2   | 1.00             | 1.00              | 1.00              | 1.00              | 1.00              |
|     | 3   | 1.05             | 1.05              | 1.05              | 1.05              | 1.05              |
| 4   | 1   | 1.06             | 1.06              | 1.06              | 1.06              | 1.06              |
|     | 2   | 1.00             | 1.00              | 1.00              | 1.00              | 1.00              |
|     | 3   | 1.00             | 1.00              | 1.00              | 1.00              | 1.00              |
| 5   | 1   | 1.06             | 1.06              | 1.06              | 1.06              | 1.06              |
|     | 2   | 1.00             | 1.00              | 1.00              | 1.00              | 1.00              |
|     | 3   | 1.00             | 1.00              | 1.00              | 1.00              | 1.00              |

Table S33: Reference ( $\vartheta^\ell$ ), and Cartesian grid detachment (d) and attachment (a) density integrals ( $\vartheta$ ) obtained with a medium (m) and a fine (f) grid for the three first excited-states (E-S) of nIII-NO<sub>2</sub>-NO<sub>2</sub> computed at the PBE0/6-311++G(2d,p) level of theory.

| $n$ | E-S | $\phi_S^\ell$ | $\phi_S$ | $\varphi^\ell$ | $\varphi$ | $\psi^\ell$ | $\psi$ |
|-----|-----|---------------|----------|----------------|-----------|-------------|--------|
| 1   | 1   | 0.04          | 0.51     | 1.00           | 0.74      | 0.02        | 0.38   |
|     | 2   | 0.04          | 0.52     | 1.00           | 0.74      | 0.02        | 0.39   |
|     | 3   | 0.05          | 0.54     | 1.00           | 0.73      | 0.03        | 0.41   |
| 2   | 1   | 0.08          | 0.49     | 0.99           | 0.75      | 0.05        | 0.37   |
|     | 2   | 0.08          | 0.49     | 0.99           | 0.76      | 0.05        | 0.36   |
|     | 3   | 0.09          | 0.56     | 0.99           | 0.71      | 0.06        | 0.43   |
| 3   | 1   | 0.08          | 0.48     | 0.99           | 0.77      | 0.05        | 0.35   |
|     | 2   | 0.08          | 0.47     | 0.99           | 0.77      | 0.05        | 0.35   |
|     | 3   | 0.84          | 0.78     | 0.45           | 0.51      | 0.69        | 0.63   |
| 1   | 1   | 0.86          | 0.80     | 0.42           | 0.49      | 0.71        | 0.65   |

Continued on next page

| $n$ | E-S | $\phi_S^\ell$ | $\phi_S$ | $\varphi^\ell$ | $\varphi$ | $\psi^\ell$ | $\psi$ |
|-----|-----|---------------|----------|----------------|-----------|-------------|--------|
| 4   | 2   | 0.07          | 0.46     | 0.99           | 0.78      | 0.05        | 0.34   |
|     | 3   | 0.07          | 0.46     | 0.99           | 0.78      | 0.05        | 0.34   |
| 5   | 1   | 0.88          | 0.80     | 0.38           | 0.47      | 0.74        | 0.66   |
|     | 2   | 0.07          | 0.45     | 0.99           | 0.78      | 0.05        | 0.33   |
|     | 3   | 0.07          | 0.45     | 0.99           | 0.78      | 0.05        | 0.33   |

Table S34: Reference ( $\phi_S$ ,  $\varphi$ ,  $\psi$ ) and approached ( $\phi_S^\ell$ ,  $\varphi^\ell$ ,  $\psi^\ell$ ) values of the topological descriptors for the three first excited-states (E-S) of nIII-NO<sub>2</sub>-NO<sub>2</sub> computed at the PBE0/6-311++G(2d,p) level of theory.

| $n$ | E-S | $\phi_S^\ell$ | $\phi_S$ | $\varphi^\ell$ | $\varphi$ | $\psi^\ell$ | $\psi$ |
|-----|-----|---------------|----------|----------------|-----------|-------------|--------|
| 1   | 1   | 0.55          | 0.60     | 0.77           | 0.73      | 0.40        | 0.44   |
|     | 2   | 0.09          | 0.49     | 0.99           | 0.75      | 0.06        | 0.37   |
|     | 3   | 0.82          | 0.84     | 0.43           | 0.43      | 0.69        | 0.70   |
| 3   | 1   | 0.41          | 0.45     | 0.84           | 0.83      | 0.29        | 0.32   |
|     | 2   | 0.47          | 0.50     | 0.81           | 0.75      | 0.34        | 0.37   |
|     | 3   | 0.74          | 0.75     | 0.54           | 0.53      | 0.60        | 0.61   |
| 4   | 1   | 0.31          | 0.33     | 0.89           | 0.89      | 0.22        | 0.23   |
|     | 2   | 0.54          | 0.55     | 0.63           | 0.71      | 0.45        | 0.42   |
|     | 3   | 0.72          | 0.70     | 0.52           | 0.56      | 0.60        | 0.57   |
| 5   | 1   | 0.23          | 0.23     | 0.92           | 0.93      | 0.16        | 0.16   |
|     | 2   | 0.66          | 0.63     | 0.61           | 0.65      | 0.53        | 0.49   |
|     | 3   | 0.68          | 0.65     | 0.56           | 0.63      | 0.56        | 0.51   |

Table S35: Reference ( $\phi_S$ ,  $\varphi$ ,  $\psi$ ) and approached ( $\phi_S^\ell$ ,  $\varphi^\ell$ ,  $\psi^\ell$ ) values of the topological descriptors for the three first excited-states (E-S) of nVI-c computed at the PBE0/6-311++G(2d,p) level of theory.

| $n$ | E-S | $\phi_S^\ell$ | $\phi_S$ | $\varphi^\ell$ | $\varphi$ | $\psi^\ell$ | $\psi$ |
|-----|-----|---------------|----------|----------------|-----------|-------------|--------|
| 1   | 1   | 0.57          | 0.60     | 0.74           | 0.72      | 0.42        | 0.44   |

Continued on next page



| $n$ | E-S | $\phi_S^\ell$ | $\phi_S$ | $\varphi^\ell$ | $\varphi$ | $\psi^\ell$ | $\psi$ |
|-----|-----|---------------|----------|----------------|-----------|-------------|--------|
| 2   | 2   | 0.12          | 0.48     | 0.98           | 0.76      | 0.08        | 0.36   |
|     | 3   | 0.67          | 0.71     | 0.56           | 0.56      | 0.55        | 0.57   |
| 3   | 1   | 0.51          | 0.53     | 0.77           | 0.77      | 0.37        | 0.39   |
|     | 2   | 0.80          | 0.78     | 0.47           | 0.51      | 0.66        | 0.63   |
|     | 3   | 0.69          | 0.69     | 0.60           | 0.61      | 0.54        | 0.54   |
| 4   | 1   | 0.46          | 0.47     | 0.82           | 0.81      | 0.32        | 0.34   |
|     | 2   | 0.79          | 0.77     | 0.46           | 0.52      | 0.66        | 0.62   |
|     | 3   | 0.67          | 0.66     | 0.62           | 0.63      | 0.53        | 0.52   |
| 5   | 1   | 0.41          | 0.42     | 0.83           | 0.84      | 0.29        | 0.30   |
|     | 2   | 0.77          | 0.75     | 0.47           | 0.53      | 0.65        | 0.61   |
|     | 3   | 0.66          | 0.65     | 0.61           | 0.63      | 0.53        | 0.51   |

Table S36: Reference ( $\phi_S$ ,  $\varphi$ ,  $\psi$ ) and approached ( $\phi_S^\ell$ ,  $\varphi^\ell$ ,  $\psi^\ell$ ) values of the topological descriptors for the three first excited-states (E-S) of nV-O in linear configuration (i.e., with heteroatom on the top of alternating spacer subunits) computed at the PBE0/6-311++G(2d,p) level of theory.

| $n$ | E-S | $\phi_S^\ell$ | $\phi_S$ | $\varphi^\ell$ | $\varphi$ | $\psi^\ell$ | $\psi$ |
|-----|-----|---------------|----------|----------------|-----------|-------------|--------|
| 1   | 1   | 0.65          | 0.68     | 0.68           | 0.65      | 0.49        | 0.51   |
|     | 2   | 0.12          | 0.48     | 0.98           | 0.76      | 0.08        | 0.36   |
|     | 3   | 0.12          | 0.52     | 0.99           | 0.74      | 0.08        | 0.39   |
| 2   | 1   | 0.56          | 0.61     | 0.74           | 0.71      | 0.42        | 0.45   |
|     | 2   | 0.11          | 0.48     | 0.99           | 0.76      | 0.07        | 0.36   |
|     | 3   | 0.74          | 0.75     | 0.53           | 0.54      | 0.60        | 0.60   |
| 3   | 1   | 0.50          | 0.54     | 0.79           | 0.77      | 0.36        | 0.39   |
|     | 2   | 0.79          | 0.78     | 0.48           | 0.51      | 0.65        | 0.63   |
|     | 3   | 0.70          | 0.70     | 0.59           | 0.60      | 0.55        | 0.55   |
| 4   | 1   | 0.41          | 0.44     | 0.85           | 0.83      | 0.28        | 0.31   |
|     | 2   | 0.77          | 0.76     | 0.48           | 0.52      | 0.65        | 0.62   |
|     | 3   | 0.66          | 0.67     | 0.60           | 0.62      | 0.53        | 0.53   |
| 5   | 1   | 0.33          | 0.37     | 0.90           | 0.88      | 0.23        | 0.25   |
|     | 2   | 0.75          | 0.74     | 0.49           | 0.54      | 0.63        | 0.59   |
|     | 3   | 0.62          | 0.62     | 0.63           | 0.65      | 0.50        | 0.48   |

Table S37: Reference ( $\phi_S$ ,  $\varphi$ ,  $\psi$ ) and approached ( $\phi_S^\ell$ ,  $\varphi^\ell$ ,  $\psi^\ell$ ) values of the topological descriptors for

the three first excited-states (E-S) of nV-O in crowned configuration (i.e., with heteroatom on the top of each spacer subunit) computed at the PBE0/6-311++G(2d,p) level of theory.

| $n$ | E-S | $\phi_S^\ell$ | $\phi_S$ | $\varphi^\ell$ | $\varphi$ | $\psi^\ell$ | $\psi$ |
|-----|-----|---------------|----------|----------------|-----------|-------------|--------|
| 1   | 1   | 0.97          | 0.89     | 0.15           | 0.32      | 0.90        | 0.78   |
|     | 2   | 0.95          | 0.92     | 0.23           | 0.29      | 0.85        | 0.80   |
|     | 3   | 0.53          | 0.60     | 0.79           | 0.70      | 0.37        | 0.45   |
| 3   | 1   | 0.98          | 0.88     | 0.12           | 0.32      | 0.92        | 0.78   |
|     | 2   | 0.97          | 0.94     | 0.17           | 0.26      | 0.89        | 0.83   |
|     | 3   | 0.07          | 0.34     | 1.00           | 0.86      | 0.04        | 0.24   |
| 4   | 1   | 0.98          | 0.88     | 0.10           | 0.32      | 0.93        | 0.78   |
|     | 2   | 0.98          | 0.94     | 0.15           | 0.26      | 0.90        | 0.83   |
|     | 3   | 0.04          | 0.33     | 1.00           | 0.87      | 0.03        | 0.23   |
| 5   | 1   | 0.99          | 0.87     | 0.09           | 0.33      | 0.94        | 0.77   |
|     | 2   | 0.98          | 0.93     | 0.13           | 0.26      | 0.92        | 0.83   |
|     | 3   | 0.97          | 0.93     | 0.17           | 0.28      | 0.89        | 0.81   |

Table S38: Reference ( $\phi_S$ ,  $\varphi$ ,  $\psi$ ) and approached ( $\phi_S^\ell$ ,  $\varphi^\ell$ ,  $\psi^\ell$ ) values of the topological descriptors for the three first excited-states (E-S) of polyacetylene (PA) computed at the B3LYP/cc-pVTZ level of theory.

| $n$ | E-S | $\phi_S^\ell$ | $\phi_S$ | $\varphi^\ell$ | $\varphi$ | $\psi^\ell$ | $\psi$ |
|-----|-----|---------------|----------|----------------|-----------|-------------|--------|
| 1   | 1   | 0.97          | 0.88     | 0.15           | 0.32      | 0.90        | 0.78   |
|     | 2   | 0.72          | 0.80     | 0.59           | 0.48      | 0.56        | 0.65   |
|     | 3   | 0.70          | 0.72     | 0.58           | 0.55      | 0.56        | 0.58   |
| 3   | 1   | 0.98          | 0.88     | 0.13           | 0.33      | 0.92        | 0.77   |
|     | 2   | 0.97          | 0.93     | 0.19           | 0.27      | 0.88        | 0.82   |
|     | 3   | 0.10          | 0.35     | 0.99           | 0.85      | 0.06        | 0.25   |
| 4   | 1   | 0.98          | 0.87     | 0.11           | 0.33      | 0.93        | 0.77   |
|     | 2   | 0.97          | 0.93     | 0.20           | 0.28      | 0.87        | 0.81   |
|     | 3   | 0.05          | 0.34     | 1.00           | 0.86      | 0.04        | 0.24   |
| 5   | 1   | 0.99          | 0.87     | 0.10           | 0.34      | 0.94        | 0.76   |

Continued on next page

| $n$ | E-S | $\phi_S^\ell$ | $\phi_S$ | $\varphi^\ell$ | $\varphi$ | $\psi^\ell$ | $\psi$ |
|-----|-----|---------------|----------|----------------|-----------|-------------|--------|
| 5   | 2   | 0.97          | 0.92     | 0.20           | 0.30      | 0.87        | 0.80   |
|     | 3   | 0.95          | 0.89     | 0.24           | 0.35      | 0.84        | 0.76   |

Table S39: Reference ( $\phi_S$ ,  $\varphi$ ,  $\psi$ ) and approached ( $\phi_S^\ell$ ,  $\varphi^\ell$ ,  $\psi^\ell$ ) values of the topological descriptors for the three first excited-states (E-S) of polyacetylene (PA) computed at the CAM-B3LYP/cc-pVTZ level of theory.

| $n$ | E-S  | $\phi_S^\ell$ | $\phi_S$ | $\varphi^\ell$ | $\varphi$ | $\psi^\ell$ | $\psi$ |
|-----|------|---------------|----------|----------------|-----------|-------------|--------|
| 1   | 0.97 | 0.90          | 0.16     | 0.30           | 0.90      | 0.79        |        |
| 2   | 0.96 | 0.93          | 0.22     | 0.28           | 0.85      | 0.82        |        |
| 3   | 0.16 | 0.56          | 0.98     | 0.71           | 0.10      | 0.43        |        |
| 1   | 0.98 | 0.89          | 0.12     | 0.30           | 0.92      | 0.79        |        |
| 2   | 0.97 | 0.94          | 0.18     | 0.25           | 0.88      | 0.84        |        |
| 3   | 0.52 | 0.72          | 0.79     | 0.59           | 0.37      | 0.56        |        |
| 1   | 0.98 | 0.89          | 0.10     | 0.31           | 0.94      | 0.79        |        |
| 2   | 0.98 | 0.94          | 0.15     | 0.25           | 0.90      | 0.84        |        |
| 3   | 0.96 | 0.92          | 0.21     | 0.27           | 0.86      | 0.82        |        |
| 1   | 0.99 | 0.88          | 0.09     | 0.31           | 0.94      | 0.79        |        |
| 2   | 0.98 | 0.94          | 0.13     | 0.25           | 0.92      | 0.84        |        |
| 3   | 0.96 | 0.93          | 0.24     | 0.28           | 0.84      | 0.81        |        |

Table S40: Reference ( $\phi_S$ ,  $\varphi$ ,  $\psi$ ) and approached ( $\phi_S^\ell$ ,  $\varphi^\ell$ ,  $\psi^\ell$ ) values of the topological descriptors for the three first excited-states (E-S) of polyacetylene (PA) computed at the PBE/cc-pVTZ level of theory.

| E-S | $\phi_S^\ell$ | $\phi_S$ | $\varphi^\ell$ | $\varphi$ | $\psi^\ell$ | $\psi$ |
|-----|---------------|----------|----------------|-----------|-------------|--------|
| 1   | 0.34          | 0.35     | 0.90           | 0.88      | 0.23        | 0.24   |
| 2   | 0.09          | 0.11     | 0.99           | 0.98      | 0.06        | 0.07   |
| 3   | 0.66          | 0.70     | 0.62           | 0.59      | 0.52        | 0.55   |

Table S41: Reference ( $\phi_S$ ,  $\varphi$ ,  $\psi$ ) and approached ( $\phi_S^\ell$ ,  $\varphi^\ell$ ,  $\psi^\ell$ ) values of the topological descriptors for the three first excited-states (E-S) of N-phenylpyrrole computed at the B3LYP/cc-pVTZ level of theory.

| E-S | $\phi_S^\ell$ | $\phi_S$ | $\varphi^\ell$ | $\varphi$ | $\psi^\ell$ | $\psi$ |
|-----|---------------|----------|----------------|-----------|-------------|--------|
| 1   | 0.88          | 0.89     | 0.36           | 0.35      | 0.75        | 0.76   |
| 2   | 0.56          | 0.55     | 0.75           | 0.75      | 0.41        | 0.41   |
| 3   | 0.81          | 0.79     | 0.47           | 0.51      | 0.67        | 0.64   |

Table S42: Reference ( $\phi_S$ ,  $\varphi$ ,  $\psi$ ) and approached ( $\phi_S^\ell$ ,  $\varphi^\ell$ ,  $\psi^\ell$ ) values of the topological descriptors for the three first excited-states (E-S) of N-phenylpyrrole computed at the CAM-B3LYP/cc-pVTZ level of theory.

| E-S | $\phi_S^\ell$ | $\phi_S$ | $\varphi^\ell$ | $\varphi$ | $\psi^\ell$ | $\psi$ |
|-----|---------------|----------|----------------|-----------|-------------|--------|
| 1   | 0.08          | 0.10     | 0.99           | 0.98      | 0.05        | 0.06   |
| 2   | 0.26          | 0.28     | 0.93           | 0.92      | 0.17        | 0.19   |
| 3   | 0.43          | 0.48     | 0.83           | 0.79      | 0.31        | 0.35   |

Table S43: Reference ( $\phi_S$ ,  $\varphi$ ,  $\psi$ ) and approached ( $\phi_S^\ell$ ,  $\varphi^\ell$ ,  $\psi^\ell$ ) values of the topological descriptors for the three first excited-states (E-S) of N-phenylpyrrole computed at the PBE/cc-pVTZ level of theory.

| $n$ | E-S | $\phi_S^\ell$ | $\phi_S$ | $\varphi^\ell$ | $\varphi$ | $\psi^\ell$ | $\psi$ |
|-----|-----|---------------|----------|----------------|-----------|-------------|--------|
| 1   | 1   | 0.66          | 0.68     | 0.65           | 0.63      | 0.51        | 0.52   |
|     | 2   | 0.27          | 0.52     | 0.93           | 0.74      | 0.18        | 0.39   |
|     | 3   | 0.48          | 0.60     | 0.77           | 0.68      | 0.36        | 0.46   |
| 3   | 1   | 0.61          | 0.62     | 0.69           | 0.69      | 0.46        | 0.47   |
|     | 2   | 0.80          | 0.79     | 0.45           | 0.49      | 0.67        | 0.65   |
|     | 3   | 0.75          | 0.74     | 0.56           | 0.56      | 0.59        | 0.59   |
| 4   | 1   | 0.56          | 0.57     | 0.72           | 0.73      | 0.42        | 0.42   |
|     | 2   | 0.80          | 0.78     | 0.45           | 0.50      | 0.67        | 0.64   |
|     | 3   | 0.76          | 0.74     | 0.53           | 0.56      | 0.61        | 0.59   |
| 5   | 1   | 0.53          | 0.53     | 0.75           | 0.76      | 0.39        | 0.39   |
|     | 2   | 0.78          | 0.76     | 0.46           | 0.52      | 0.66        | 0.62   |
|     | 3   | 0.74          | 0.72     | 0.53           | 0.57      | 0.60        | 0.58   |

Table S44: Reference ( $\phi_S$ ,  $\varphi$ ,  $\psi$ ) and approached ( $\phi_S^\ell$ ,  $\varphi^\ell$ ,  $\psi^\ell$ ) values of the topological descriptors for the three first excited-states (E-S) of nV-Se in linear configuration (i.e., with heteroatom on the top of alternating spacer subunits) computed at the PBE0/6-311++G(2d,p) level of theory.

| $n$ | E-S | $\phi_S^\ell$ | $\phi_S$ | $\varphi^\ell$ | $\varphi$ | $\psi^\ell$ | $\psi$ |
|-----|-----|---------------|----------|----------------|-----------|-------------|--------|
| 1   | 1   | 0.68          | 0.72     | 0.65           | 0.61      | 0.52        | 0.55   |
|     | 2   | 0.10          | 0.48     | 0.99           | 0.76      | 0.06        | 0.36   |
|     | 3   | 0.51          | 0.54     | 0.76           | 0.74      | 0.37        | 0.40   |
| 2   | 1   | 0.61          | 0.64     | 0.69           | 0.67      | 0.46        | 0.49   |
|     | 2   | 0.39          | 0.48     | 0.85           | 0.77      | 0.27        | 0.35   |
|     | 3   | 0.51          | 0.51     | 0.79           | 0.74      | 0.36        | 0.38   |
| 3   | 1   | 0.55          | 0.56     | 0.75           | 0.74      | 0.40        | 0.41   |
|     | 2   | 0.71          | 0.71     | 0.56           | 0.57      | 0.58        | 0.57   |
|     | 3   | 0.49          | 0.56     | 0.76           | 0.71      | 0.36        | 0.42   |
| 4   | 1   | 0.50          | 0.50     | 0.78           | 0.78      | 0.36        | 0.36   |
|     | 2   | 0.74          | 0.73     | 0.51           | 0.56      | 0.62        | 0.58   |
|     | 3   | 0.68          | 0.70     | 0.61           | 0.60      | 0.53        | 0.55   |
| 5   | 1   | 0.44          | 0.44     | 0.81           | 0.82      | 0.32        | 0.31   |
|     | 2   | 0.73          | 0.71     | 0.51           | 0.57      | 0.61        | 0.57   |
|     | 3   | 0.70          | 0.68     | 0.56           | 0.60      | 0.57        | 0.54   |

Table S45: Reference ( $\phi_S$ ,  $\varphi$ ,  $\psi$ ) and approached ( $\phi_S^\ell$ ,  $\varphi^\ell$ ,  $\psi^\ell$ ) values of the topological descriptors for the three first excited-states (E-S) of nV-Se in crowned configuration (i.e., with heteroatom on the top of each spacer subunit) computed at the PBE0/6-311++G(2d,p) level of theory.

| $n$ | E-S | $\phi_S^\ell$ | $\phi_S$ | $\varphi^\ell$ | $\varphi$ | $\psi^\ell$ | $\psi$ |
|-----|-----|---------------|----------|----------------|-----------|-------------|--------|
| 1   | 1   | 0.63          | 0.65     | 0.69           | 0.67      | 0.47        | 0.49   |
|     | 2   | 0.25          | 0.49     | 0.94           | 0.76      | 0.16        | 0.37   |
|     | 3   | 0.77          | 0.77     | 0.52           | 0.53      | 0.62        | 0.62   |
| 3   | 1   | 0.56          | 0.58     | 0.74           | 0.73      | 0.41        | 0.43   |
|     | 2   | 0.78          | 0.77     | 0.47           | 0.52      | 0.65        | 0.62   |
|     | 3   | 0.74          | 0.73     | 0.55           | 0.57      | 0.59        | 0.57   |
| 4   | 1   | 0.51          | 0.52     | 0.77           | 0.77      | 0.37        | 0.38   |
|     | 2   | 0.77          | 0.75     | 0.48           | 0.53      | 0.65        | 0.61   |
|     | 3   | 0.72          | 0.70     | 0.57           | 0.59      | 0.57        | 0.56   |
| 5   | 1   | 0.47          | 0.47     | 0.79           | 0.80      | 0.34        | 0.34   |
|     | 2   | 0.76          | 0.73     | 0.49           | 0.55      | 0.63        | 0.59   |
|     | 3   | 0.70          | 0.68     | 0.57           | 0.60      | 0.56        | 0.54   |

Table S46: Reference ( $\phi_S$ ,  $\varphi$ ,  $\psi$ ) and approached ( $\phi_S^\ell$ ,  $\varphi^\ell$ ,  $\psi^\ell$ ) values of the topological descriptors for

the three first excited-states (E-S) of nV-S in linear configuration (i.e., with heteroatom on the top of alternating spacer subunits) computed at the PBE0/6-311++G(2d,p) level of theory.

| $n$ | E-S | $\phi_S^\ell$ | $\phi_S$ | $\varphi^\ell$ | $\varphi$ | $\psi^\ell$ | $\psi$ |
|-----|-----|---------------|----------|----------------|-----------|-------------|--------|
| 1   | 1   | 0.67          | 0.70     | 0.66           | 0.63      | 0.51        | 0.54   |
|     | 2   | 0.10          | 0.48     | 0.99           | 0.76      | 0.06        | 0.36   |
|     | 3   | 0.10          | 0.52     | 0.99           | 0.74      | 0.06        | 0.39   |
| 2   | 1   | 0.62          | 0.64     | 0.69           | 0.68      | 0.46        | 0.48   |
|     | 2   | 0.32          | 0.50     | 0.91           | 0.75      | 0.22        | 0.38   |
|     | 3   | 0.58          | 0.64     | 0.67           | 0.64      | 0.45        | 0.50   |
| 3   | 1   | 0.55          | 0.57     | 0.75           | 0.74      | 0.40        | 0.42   |
|     | 2   | 0.78          | 0.77     | 0.47           | 0.51      | 0.66        | 0.63   |
|     | 3   | 0.74          | 0.73     | 0.53           | 0.57      | 0.60        | 0.58   |
| 4   | 1   | 0.49          | 0.50     | 0.78           | 0.79      | 0.36        | 0.36   |
|     | 2   | 0.77          | 0.75     | 0.47           | 0.53      | 0.65        | 0.61   |
|     | 3   | 0.72          | 0.71     | 0.55           | 0.59      | 0.58        | 0.56   |
| 5   | 1   | 0.44          | 0.44     | 0.81           | 0.82      | 0.32        | 0.31   |
|     | 2   | 0.75          | 0.72     | 0.49           | 0.56      | 0.63        | 0.58   |
|     | 3   | 0.70          | 0.68     | 0.56           | 0.60      | 0.57        | 0.54   |

Table S47: Reference ( $\phi_S$ ,  $\varphi$ ,  $\psi$ ) and approached ( $\phi_S^\ell$ ,  $\varphi^\ell$ ,  $\psi^\ell$ ) values of the topological descriptors for the three first excited-states (E-S) of nV-S in crowned configuration (i.e., with heteroatom on the top of each spacer subunit) computed at the PBE0/6-311++G(2d,p) level of theory.

| E-S | $\phi_S^\ell$ | $\phi_S$ | $\varphi^\ell$ | $\varphi$ | $\psi^\ell$ | $\psi$ |
|-----|---------------|----------|----------------|-----------|-------------|--------|
| 1   | 0.21          | 0.47     | 0.94           | 0.78      | 0.14        | 0.34   |
| 2   | 0.16          | 0.46     | 0.95           | 0.78      | 0.11        | 0.34   |
| 3   | 0.15          | 0.47     | 0.95           | 0.78      | 0.10        | 0.35   |

Table S48: Reference ( $\phi_S$ ,  $\varphi$ ,  $\psi$ ) and approached ( $\phi_S^\ell$ ,  $\varphi^\ell$ ,  $\psi^\ell$ ) values of the topological descriptors for the three first excited-states (E-S) of tripeptide computed at the B3LYP/cc-pVTZ level of theory.

| E-S | $\phi_S^\ell$ | $\phi_S$ | $\varphi^\ell$ | $\varphi$ | $\psi^\ell$ | $\psi$ |
|-----|---------------|----------|----------------|-----------|-------------|--------|
| 1   | 0.20          | 0.47     | 0.94           | 0.78      | 0.14        | 0.35   |
| 2   | 0.16          | 0.47     | 0.95           | 0.78      | 0.10        | 0.35   |
| 3   | 0.14          | 0.47     | 0.95           | 0.77      | 0.10        | 0.35   |

Table S49: Reference ( $\phi_S$ ,  $\varphi$ ,  $\psi$ ) and approached ( $\phi_S^\ell$ ,  $\varphi^\ell$ ,  $\psi^\ell$ ) values of the topological descriptors for the three first excited-states (E-S) of tripeptide computed at the CAM-B3LYP/cc-pVTZ level of theory.

| E-S | $\phi_S^\ell$ | $\phi_S$ | $\varphi^\ell$ | $\varphi$ | $\psi^\ell$ | $\psi$ |
|-----|---------------|----------|----------------|-----------|-------------|--------|
| 1   | 0.03          | 0.06     | 0.99           | 0.98      | 0.02        | 0.04   |
| 2   | 0.08          | 0.16     | 0.98           | 0.96      | 0.05        | 0.11   |
| 3   | 0.12          | 0.12     | 0.97           | 0.96      | 0.08        | 0.08   |

Table S50: Reference ( $\phi_S$ ,  $\varphi$ ,  $\psi$ ) and approached ( $\phi_S^\ell$ ,  $\varphi^\ell$ ,  $\psi^\ell$ ) values of the topological descriptors for the three first excited-states (E-S) of tripeptide computed at the PBE/cc-pVTZ level of theory.

| $\alpha$ | $\phi_S^\ell$ | $\phi_S$ | $\varphi^\ell$ | $\varphi$ | $\psi^\ell$ | $\psi$ |
|----------|---------------|----------|----------------|-----------|-------------|--------|
| 0        | 0.43          | 0.33     | 0.82           | 0.86      | 0.31        | 0.23   |
| 1        | 0.43          | 0.33     | 0.82           | 0.86      | 0.31        | 0.23   |
| 2        | 0.43          | 0.33     | 0.82           | 0.86      | 0.31        | 0.23   |
| 3        | 0.43          | 0.33     | 0.82           | 0.86      | 0.31        | 0.23   |
| 4        | 0.43          | 0.33     | 0.82           | 0.86      | 0.31        | 0.23   |
| 5        | 0.42          | 0.33     | 0.82           | 0.86      | 0.30        | 0.23   |
| 6        | 0.42          | 0.33     | 0.82           | 0.86      | 0.30        | 0.23   |
| 7        | 0.42          | 0.33     | 0.82           | 0.86      | 0.30        | 0.23   |
| 8        | 0.41          | 0.33     | 0.82           | 0.86      | 0.30        | 0.23   |
| 9        | 0.41          | 0.33     | 0.83           | 0.86      | 0.29        | 0.23   |
| 10       | 0.40          | 0.33     | 0.83           | 0.86      | 0.29        | 0.23   |
| 11       | 0.40          | 0.33     | 0.83           | 0.86      | 0.29        | 0.23   |
| 12       | 0.39          | 0.33     | 0.83           | 0.86      | 0.28        | 0.23   |
| 13       | 0.39          | 0.33     | 0.84           | 0.86      | 0.28        | 0.23   |
| 14       | 0.38          | 0.33     | 0.84           | 0.86      | 0.27        | 0.23   |
| 15       | 0.37          | 0.33     | 0.84           | 0.86      | 0.26        | 0.23   |
| 16       | 0.37          | 0.33     | 0.84           | 0.86      | 0.26        | 0.23   |
| 17       | 0.36          | 0.33     | 0.85           | 0.86      | 0.26        | 0.23   |
| 18       | 0.35          | 0.33     | 0.85           | 0.86      | 0.25        | 0.23   |
| 19       | 0.34          | 0.32     | 0.85           | 0.86      | 0.24        | 0.23   |
| 20       | 0.33          | 0.32     | 0.85           | 0.86      | 0.24        | 0.23   |
| 21       | 0.32          | 0.32     | 0.86           | 0.86      | 0.23        | 0.23   |
| 22       | 0.31          | 0.32     | 0.86           | 0.86      | 0.22        | 0.23   |
| 23       | 0.30          | 0.32     | 0.86           | 0.86      | 0.21        | 0.23   |
| 24       | 0.29          | 0.32     | 0.86           | 0.86      | 0.21        | 0.23   |
| 25       | 0.28          | 0.32     | 0.87           | 0.86      | 0.20        | 0.23   |
| 26       | 0.27          | 0.32     | 0.87           | 0.86      | 0.19        | 0.23   |
| 27       | 0.26          | 0.32     | 0.88           | 0.87      | 0.18        | 0.22   |
| 28       | 0.25          | 0.32     | 0.89           | 0.87      | 0.17        | 0.22   |
| 29       | 0.24          | 0.32     | 0.90           | 0.87      | 0.17        | 0.22   |
| 30       | 0.23          | 0.32     | 0.91           | 0.87      | 0.16        | 0.22   |
| 31       | 0.22          | 0.32     | 0.92           | 0.87      | 0.15        | 0.22   |

Continued on next page



| $\alpha$ | $\phi_S^\ell$ | $\phi_S$ | $\varphi^\ell$ | $\varphi$ | $\psi^\ell$ | $\psi$ |
|----------|---------------|----------|----------------|-----------|-------------|--------|
| 32       | 0.20          | 0.31     | 0.93           | 0.87      | 0.13        | 0.22   |
| 33       | 0.19          | 0.31     | 0.94           | 0.87      | 0.13        | 0.22   |
| 34       | 0.18          | 0.31     | 0.94           | 0.87      | 0.12        | 0.22   |
| 35       | 0.17          | 0.31     | 0.95           | 0.87      | 0.11        | 0.22   |
| 36       | 0.16          | 0.31     | 0.96           | 0.87      | 0.11        | 0.22   |
| 37       | 0.15          | 0.31     | 0.96           | 0.87      | 0.10        | 0.22   |
| 38       | 0.14          | 0.31     | 0.97           | 0.87      | 0.09        | 0.22   |
| 39       | 0.13          | 0.30     | 0.97           | 0.88      | 0.08        | 0.21   |
| 40       | 0.12          | 0.30     | 0.98           | 0.88      | 0.08        | 0.21   |
| 41       | 0.11          | 0.30     | 0.98           | 0.88      | 0.07        | 0.21   |
| 42       | 0.10          | 0.30     | 0.98           | 0.88      | 0.06        | 0.21   |
| 43       | 0.09          | 0.30     | 0.99           | 0.88      | 0.06        | 0.21   |
| 44       | 0.08          | 0.29     | 0.99           | 0.88      | 0.05        | 0.20   |
| 45       | 0.07          | 0.29     | 0.99           | 0.88      | 0.04        | 0.20   |
| 46       | 0.07          | 0.29     | 0.99           | 0.88      | 0.04        | 0.20   |
| 47       | 0.08          | 0.29     | 0.99           | 0.88      | 0.05        | 0.20   |
| 48       | 0.09          | 0.29     | 0.99           | 0.89      | 0.06        | 0.20   |
| 49       | 0.10          | 0.28     | 0.98           | 0.89      | 0.06        | 0.19   |
| 50       | 0.11          | 0.28     | 0.98           | 0.89      | 0.07        | 0.19   |
| 51       | 0.12          | 0.28     | 0.98           | 0.89      | 0.08        | 0.19   |
| 52       | 0.13          | 0.28     | 0.97           | 0.89      | 0.08        | 0.19   |
| 53       | 0.14          | 0.27     | 0.97           | 0.89      | 0.09        | 0.19   |
| 54       | 0.15          | 0.27     | 0.96           | 0.89      | 0.10        | 0.19   |
| 55       | 0.16          | 0.27     | 0.96           | 0.89      | 0.11        | 0.19   |
| 56       | 0.17          | 0.27     | 0.95           | 0.89      | 0.11        | 0.19   |
| 57       | 0.18          | 0.26     | 0.94           | 0.90      | 0.12        | 0.18   |
| 58       | 0.19          | 0.26     | 0.94           | 0.90      | 0.13        | 0.18   |
| 59       | 0.20          | 0.26     | 0.93           | 0.90      | 0.13        | 0.18   |
| 60       | 0.20          | 0.26     | 0.92           | 0.90      | 0.14        | 0.18   |
| 61       | 0.21          | 0.25     | 0.91           | 0.90      | 0.14        | 0.17   |
| 62       | 0.22          | 0.25     | 0.90           | 0.90      | 0.15        | 0.17   |
| 63       | 0.23          | 0.25     | 0.90           | 0.90      | 0.16        | 0.17   |

Continued on next page

| $\alpha$ | $\phi_S^\ell$ | $\phi_S$ | $\varphi^\ell$ | $\varphi$ | $\psi^\ell$ | $\psi$ |
|----------|---------------|----------|----------------|-----------|-------------|--------|
| 64       | 0.23          | 0.24     | 0.90           | 0.91      | 0.16        | 0.16   |
| 65       | 0.24          | 0.24     | 0.91           | 0.91      | 0.16        | 0.16   |
| 66       | 0.24          | 0.24     | 0.91           | 0.91      | 0.16        | 0.16   |
| 67       | 0.25          | 0.23     | 0.91           | 0.91      | 0.17        | 0.16   |
| 68       | 0.25          | 0.23     | 0.91           | 0.91      | 0.17        | 0.16   |
| 69       | 0.26          | 0.23     | 0.91           | 0.91      | 0.18        | 0.16   |
| 70       | 0.26          | 0.23     | 0.91           | 0.91      | 0.18        | 0.16   |
| 71       | 0.27          | 0.23     | 0.91           | 0.91      | 0.18        | 0.16   |
| 72       | 0.28          | 0.23     | 0.91           | 0.92      | 0.19        | 0.16   |
| 73       | 0.28          | 0.23     | 0.91           | 0.92      | 0.19        | 0.16   |
| 74       | 0.29          | 0.24     | 0.91           | 0.92      | 0.20        | 0.16   |
| 75       | 0.31          | 0.25     | 0.91           | 0.92      | 0.21        | 0.17   |
| 76       | 0.33          | 0.27     | 0.91           | 0.91      | 0.22        | 0.18   |
| 77       | 0.36          | 0.30     | 0.90           | 0.90      | 0.24        | 0.20   |
| 78       | 0.42          | 0.36     | 0.87           | 0.88      | 0.29        | 0.25   |
| 79       | 0.50          | 0.46     | 0.84           | 0.84      | 0.34        | 0.32   |
| 80       | 0.54          | 0.53     | 0.82           | 0.81      | 0.37        | 0.37   |
| 81       | 0.55          | 0.55     | 0.81           | 0.80      | 0.38        | 0.38   |
| 82       | 0.56          | 0.56     | 0.82           | 0.80      | 0.38        | 0.39   |
| 83       | 0.55          | 0.55     | 0.82           | 0.81      | 0.38        | 0.38   |
| 84       | 0.54          | 0.55     | 0.83           | 0.81      | 0.37        | 0.38   |
| 85       | 0.54          | 0.54     | 0.83           | 0.82      | 0.37        | 0.37   |
| 86       | 0.52          | 0.53     | 0.84           | 0.83      | 0.35        | 0.36   |
| 87       | 0.51          | 0.52     | 0.85           | 0.83      | 0.34        | 0.36   |
| 88       | 0.50          | 0.50     | 0.86           | 0.84      | 0.34        | 0.34   |
| 89       | 0.48          | 0.49     | 0.87           | 0.85      | 0.32        | 0.33   |
| 90       | 0.13          | 0.17     | 0.98           | 0.96      | 0.08        | 0.11   |

Table S51: Reference ( $\phi_S$ ,  $\varphi$ ,  $\psi$ ) and approached ( $\phi_S^\ell$ ,  $\varphi^\ell$ ,  $\psi^\ell$ ) values of the topological descriptors for the first excited-state of the pyridinium-phenolate (PP), computed at the B3LYP/3-21G level of theory.  $\alpha$  is the pyridinium-phenolate central twist angle amplitude.

| $\alpha$ | $\phi_S^\ell$ | $\phi_S$ | $\varphi^\ell$ | $\varphi$ | $\psi^\ell$ | $\psi$ |
|----------|---------------|----------|----------------|-----------|-------------|--------|
| 0        | 0.41          | 0.31     | 0.83           | 0.87      | 0.29        | 0.22   |
| 1        | 0.41          | 0.31     | 0.83           | 0.87      | 0.29        | 0.22   |
| 2        | 0.41          | 0.31     | 0.83           | 0.87      | 0.29        | 0.22   |
| 3        | 0.41          | 0.31     | 0.84           | 0.87      | 0.29        | 0.22   |
| 4        | 0.41          | 0.31     | 0.84           | 0.87      | 0.29        | 0.22   |
| 5        | 0.41          | 0.31     | 0.84           | 0.87      | 0.29        | 0.22   |
| 6        | 0.40          | 0.31     | 0.84           | 0.87      | 0.28        | 0.22   |
| 7        | 0.40          | 0.31     | 0.84           | 0.87      | 0.28        | 0.22   |
| 8        | 0.40          | 0.32     | 0.84           | 0.87      | 0.28        | 0.22   |
| 9        | 0.39          | 0.32     | 0.85           | 0.87      | 0.27        | 0.22   |
| 10       | 0.39          | 0.32     | 0.85           | 0.87      | 0.27        | 0.22   |
| 11       | 0.39          | 0.32     | 0.85           | 0.87      | 0.27        | 0.22   |
| 12       | 0.38          | 0.32     | 0.85           | 0.87      | 0.27        | 0.22   |
| 13       | 0.38          | 0.32     | 0.85           | 0.87      | 0.27        | 0.22   |
| 14       | 0.37          | 0.32     | 0.86           | 0.87      | 0.26        | 0.22   |
| 15       | 0.37          | 0.32     | 0.86           | 0.87      | 0.26        | 0.22   |
| 16       | 0.36          | 0.33     | 0.86           | 0.87      | 0.25        | 0.23   |
| 17       | 0.36          | 0.33     | 0.86           | 0.87      | 0.25        | 0.23   |
| 18       | 0.35          | 0.33     | 0.86           | 0.87      | 0.25        | 0.23   |
| 19       | 0.35          | 0.33     | 0.87           | 0.87      | 0.24        | 0.23   |
| 20       | 0.34          | 0.33     | 0.87           | 0.87      | 0.24        | 0.23   |
| 21       | 0.33          | 0.33     | 0.87           | 0.87      | 0.23        | 0.23   |
| 22       | 0.33          | 0.33     | 0.87           | 0.87      | 0.23        | 0.23   |
| 23       | 0.32          | 0.33     | 0.87           | 0.87      | 0.22        | 0.23   |
| 24       | 0.31          | 0.33     | 0.88           | 0.87      | 0.22        | 0.23   |
| 25       | 0.31          | 0.33     | 0.88           | 0.87      | 0.22        | 0.23   |
| 26       | 0.30          | 0.33     | 0.88           | 0.87      | 0.21        | 0.23   |
| 27       | 0.29          | 0.33     | 0.88           | 0.87      | 0.20        | 0.23   |
| 28       | 0.28          | 0.33     | 0.88           | 0.87      | 0.20        | 0.23   |
| 29       | 0.28          | 0.33     | 0.88           | 0.87      | 0.20        | 0.23   |
| 30       | 0.27          | 0.33     | 0.88           | 0.87      | 0.19        | 0.23   |
| 31       | 0.26          | 0.33     | 0.89           | 0.87      | 0.18        | 0.23   |

Continued on next page

| $\alpha$ | $\phi_S^\ell$ | $\phi_S$ | $\varphi^\ell$ | $\varphi$ | $\psi^\ell$ | $\psi$ |
|----------|---------------|----------|----------------|-----------|-------------|--------|
| 32       | 0.25          | 0.33     | 0.89           | 0.87      | 0.17        | 0.23   |
| 33       | 0.25          | 0.33     | 0.90           | 0.87      | 0.17        | 0.23   |
| 34       | 0.24          | 0.33     | 0.90           | 0.87      | 0.17        | 0.23   |
| 35       | 0.23          | 0.33     | 0.91           | 0.87      | 0.16        | 0.23   |
| 36       | 0.23          | 0.33     | 0.92           | 0.87      | 0.16        | 0.23   |
| 37       | 0.22          | 0.33     | 0.92           | 0.88      | 0.15        | 0.23   |
| 38       | 0.21          | 0.33     | 0.93           | 0.88      | 0.14        | 0.23   |
| 39       | 0.20          | 0.33     | 0.93           | 0.88      | 0.13        | 0.23   |
| 40       | 0.20          | 0.33     | 0.93           | 0.88      | 0.13        | 0.23   |
| 41       | 0.19          | 0.33     | 0.94           | 0.88      | 0.13        | 0.23   |
| 42       | 0.19          | 0.33     | 0.94           | 0.88      | 0.13        | 0.23   |
| 43       | 0.18          | 0.33     | 0.94           | 0.88      | 0.12        | 0.23   |
| 44       | 0.18          | 0.33     | 0.94           | 0.88      | 0.12        | 0.23   |
| 45       | 0.18          | 0.33     | 0.94           | 0.88      | 0.12        | 0.23   |
| 46       | 0.18          | 0.33     | 0.94           | 0.88      | 0.12        | 0.23   |
| 47       | 0.18          | 0.33     | 0.94           | 0.88      | 0.12        | 0.23   |
| 48       | 0.19          | 0.33     | 0.94           | 0.88      | 0.13        | 0.23   |
| 49       | 0.19          | 0.33     | 0.94           | 0.88      | 0.13        | 0.23   |
| 50       | 0.20          | 0.34     | 0.93           | 0.88      | 0.13        | 0.23   |
| 51       | 0.21          | 0.34     | 0.93           | 0.88      | 0.14        | 0.23   |
| 52       | 0.23          | 0.35     | 0.92           | 0.88      | 0.16        | 0.24   |
| 53       | 0.24          | 0.36     | 0.92           | 0.88      | 0.16        | 0.25   |
| 54       | 0.27          | 0.37     | 0.91           | 0.87      | 0.18        | 0.26   |
| 55       | 0.29          | 0.38     | 0.90           | 0.86      | 0.20        | 0.26   |
| 56       | 0.33          | 0.41     | 0.89           | 0.85      | 0.23        | 0.29   |
| 57       | 0.38          | 0.44     | 0.86           | 0.84      | 0.26        | 0.31   |
| 58       | 0.45          | 0.49     | 0.82           | 0.81      | 0.32        | 0.35   |
| 59       | 0.52          | 0.54     | 0.79           | 0.79      | 0.37        | 0.38   |
| 60       | 0.57          | 0.58     | 0.78           | 0.77      | 0.40        | 0.41   |
| 61       | 0.59          | 0.61     | 0.77           | 0.76      | 0.42        | 0.43   |
| 62       | 0.60          | 0.61     | 0.77           | 0.75      | 0.42        | 0.43   |
| 63       | 0.61          | 0.61     | 0.77           | 0.76      | 0.43        | 0.43   |

Continued on next page

| $\alpha$ | $\phi_S^\ell$ | $\phi_S$ | $\varphi^\ell$ | $\varphi$ | $\psi^\ell$ | $\psi$ |
|----------|---------------|----------|----------------|-----------|-------------|--------|
| 64       | 0.60          | 0.61     | 0.77           | 0.76      | 0.42        | 0.43   |
| 65       | 0.60          | 0.61     | 0.78           | 0.76      | 0.42        | 0.43   |
| 66       | 0.60          | 0.60     | 0.78           | 0.77      | 0.42        | 0.42   |
| 67       | 0.59          | 0.60     | 0.78           | 0.77      | 0.41        | 0.42   |
| 68       | 0.59          | 0.59     | 0.79           | 0.78      | 0.41        | 0.41   |
| 69       | 0.58          | 0.59     | 0.79           | 0.78      | 0.40        | 0.41   |
| 70       | 0.57          | 0.58     | 0.80           | 0.78      | 0.39        | 0.41   |
| 71       | 0.57          | 0.58     | 0.80           | 0.79      | 0.39        | 0.40   |
| 72       | 0.56          | 0.57     | 0.81           | 0.80      | 0.39        | 0.39   |
| 73       | 0.55          | 0.56     | 0.81           | 0.80      | 0.38        | 0.39   |
| 74       | 0.54          | 0.55     | 0.82           | 0.81      | 0.37        | 0.38   |
| 75       | 0.54          | 0.55     | 0.82           | 0.81      | 0.37        | 0.38   |
| 76       | 0.53          | 0.54     | 0.83           | 0.82      | 0.36        | 0.37   |
| 77       | 0.52          | 0.53     | 0.84           | 0.82      | 0.35        | 0.37   |
| 78       | 0.51          | 0.52     | 0.84           | 0.83      | 0.35        | 0.36   |
| 79       | 0.50          | 0.51     | 0.85           | 0.84      | 0.34        | 0.35   |
| 80       | 0.49          | 0.50     | 0.85           | 0.84      | 0.33        | 0.34   |
| 81       | 0.47          | 0.48     | 0.86           | 0.85      | 0.32        | 0.33   |
| 82       | 0.46          | 0.47     | 0.87           | 0.86      | 0.31        | 0.32   |
| 83       | 0.45          | 0.46     | 0.88           | 0.86      | 0.30        | 0.31   |
| 84       | 0.43          | 0.44     | 0.89           | 0.87      | 0.29        | 0.30   |
| 85       | 0.41          | 0.42     | 0.89           | 0.88      | 0.27        | 0.28   |
| 86       | 0.39          | 0.40     | 0.90           | 0.89      | 0.26        | 0.27   |
| 87       | 0.36          | 0.38     | 0.91           | 0.90      | 0.24        | 0.25   |
| 88       | 0.33          | 0.35     | 0.93           | 0.91      | 0.22        | 0.23   |
| 89       | 0.28          | 0.31     | 0.94           | 0.93      | 0.18        | 0.20   |
| 90       | 0.12          | 0.14     | 0.98           | 0.96      | 0.08        | 0.09   |

Table S52: Reference ( $\phi_S$ ,  $\varphi$ ,  $\psi$ ) and approached ( $\phi_S^\ell$ ,  $\varphi^\ell$ ,  $\psi^\ell$ ) values of the topological descriptors for the first excited-state of the pyridinium-phenolate (PP), computed at the B3LYP/6-311++G(2d,p) level of theory.  $\alpha$  is the pyridinium-phenolate central twist angle amplitude.

| $\alpha$ | $\phi_S^\ell$ | $\phi_S$ | $\varphi^\ell$ | $\varphi$ | $\psi^\ell$ | $\psi$ |
|----------|---------------|----------|----------------|-----------|-------------|--------|
| 0        | 0.41          | 0.31     | 0.83           | 0.87      | 0.29        | 0.22   |
| 1        | 0.41          | 0.31     | 0.83           | 0.87      | 0.29        | 0.22   |
| 2        | 0.41          | 0.31     | 0.84           | 0.87      | 0.29        | 0.22   |
| 3        | 0.40          | 0.31     | 0.84           | 0.87      | 0.28        | 0.22   |
| 4        | 0.40          | 0.31     | 0.84           | 0.87      | 0.28        | 0.22   |
| 5        | 0.40          | 0.31     | 0.84           | 0.87      | 0.28        | 0.22   |
| 6        | 0.40          | 0.32     | 0.84           | 0.87      | 0.28        | 0.22   |
| 7        | 0.40          | 0.32     | 0.84           | 0.87      | 0.28        | 0.22   |
| 8        | 0.39          | 0.32     | 0.84           | 0.87      | 0.28        | 0.22   |
| 9        | 0.39          | 0.32     | 0.85           | 0.87      | 0.27        | 0.22   |
| 10       | 0.39          | 0.32     | 0.85           | 0.87      | 0.27        | 0.22   |
| 11       | 0.38          | 0.32     | 0.85           | 0.87      | 0.27        | 0.22   |
| 12       | 0.38          | 0.32     | 0.85           | 0.87      | 0.27        | 0.22   |
| 13       | 0.37          | 0.32     | 0.85           | 0.87      | 0.26        | 0.22   |
| 14       | 0.37          | 0.32     | 0.86           | 0.87      | 0.26        | 0.22   |
| 15       | 0.36          | 0.32     | 0.86           | 0.87      | 0.25        | 0.22   |
| 16       | 0.36          | 0.33     | 0.86           | 0.87      | 0.25        | 0.23   |
| 17       | 0.35          | 0.33     | 0.86           | 0.87      | 0.25        | 0.23   |
| 18       | 0.35          | 0.33     | 0.87           | 0.87      | 0.24        | 0.23   |
| 19       | 0.34          | 0.33     | 0.87           | 0.87      | 0.24        | 0.23   |
| 20       | 0.33          | 0.33     | 0.87           | 0.87      | 0.23        | 0.23   |
| 21       | 0.33          | 0.33     | 0.87           | 0.87      | 0.23        | 0.23   |
| 22       | 0.32          | 0.33     | 0.87           | 0.87      | 0.22        | 0.23   |
| 23       | 0.31          | 0.33     | 0.88           | 0.87      | 0.22        | 0.23   |
| 24       | 0.31          | 0.33     | 0.88           | 0.87      | 0.22        | 0.23   |
| 25       | 0.30          | 0.33     | 0.88           | 0.87      | 0.21        | 0.23   |
| 26       | 0.29          | 0.33     | 0.88           | 0.87      | 0.20        | 0.23   |
| 27       | 0.28          | 0.33     | 0.88           | 0.87      | 0.20        | 0.23   |
| 28       | 0.28          | 0.33     | 0.88           | 0.87      | 0.20        | 0.23   |
| 29       | 0.27          | 0.33     | 0.89           | 0.87      | 0.19        | 0.23   |
| 30       | 0.26          | 0.33     | 0.89           | 0.87      | 0.18        | 0.23   |
| 31       | 0.25          | 0.33     | 0.89           | 0.87      | 0.17        | 0.23   |

Continued on next page

| $\alpha$ | $\phi_S^\ell$ | $\phi_S$ | $\varphi^\ell$ | $\varphi$ | $\psi^\ell$ | $\psi$ |
|----------|---------------|----------|----------------|-----------|-------------|--------|
| 32       | 0.25          | 0.33     | 0.90           | 0.87      | 0.17        | 0.23   |
| 33       | 0.24          | 0.33     | 0.90           | 0.87      | 0.17        | 0.23   |
| 34       | 0.23          | 0.33     | 0.91           | 0.87      | 0.16        | 0.23   |
| 35       | 0.23          | 0.33     | 0.91           | 0.87      | 0.16        | 0.23   |
| 36       | 0.22          | 0.33     | 0.92           | 0.87      | 0.15        | 0.23   |
| 37       | 0.21          | 0.33     | 0.93           | 0.88      | 0.14        | 0.23   |
| 38       | 0.20          | 0.33     | 0.93           | 0.88      | 0.13        | 0.23   |
| 39       | 0.20          | 0.33     | 0.93           | 0.88      | 0.13        | 0.23   |
| 40       | 0.19          | 0.33     | 0.94           | 0.88      | 0.13        | 0.23   |
| 41       | 0.18          | 0.33     | 0.94           | 0.88      | 0.12        | 0.23   |
| 42       | 0.18          | 0.33     | 0.94           | 0.88      | 0.12        | 0.23   |
| 43       | 0.17          | 0.33     | 0.94           | 0.88      | 0.11        | 0.23   |
| 44       | 0.17          | 0.33     | 0.95           | 0.88      | 0.11        | 0.23   |
| 45       | 0.17          | 0.33     | 0.95           | 0.88      | 0.11        | 0.23   |
| 46       | 0.17          | 0.33     | 0.95           | 0.88      | 0.11        | 0.23   |
| 47       | 0.17          | 0.33     | 0.94           | 0.88      | 0.11        | 0.23   |
| 48       | 0.18          | 0.33     | 0.94           | 0.88      | 0.12        | 0.23   |
| 49       | 0.18          | 0.33     | 0.94           | 0.88      | 0.12        | 0.23   |
| 50       | 0.19          | 0.33     | 0.94           | 0.88      | 0.13        | 0.23   |
| 51       | 0.20          | 0.33     | 0.93           | 0.88      | 0.13        | 0.23   |
| 52       | 0.21          | 0.34     | 0.93           | 0.88      | 0.14        | 0.23   |
| 53       | 0.23          | 0.35     | 0.92           | 0.88      | 0.16        | 0.24   |
| 54       | 0.25          | 0.35     | 0.92           | 0.88      | 0.17        | 0.24   |
| 55       | 0.27          | 0.37     | 0.91           | 0.87      | 0.18        | 0.26   |
| 56       | 0.30          | 0.38     | 0.90           | 0.86      | 0.20        | 0.26   |
| 57       | 0.34          | 0.41     | 0.89           | 0.85      | 0.23        | 0.29   |
| 58       | 0.40          | 0.45     | 0.86           | 0.83      | 0.28        | 0.32   |
| 59       | 0.47          | 0.50     | 0.81           | 0.81      | 0.33        | 0.35   |
| 60       | 0.54          | 0.56     | 0.79           | 0.78      | 0.38        | 0.40   |
| 61       | 0.58          | 0.59     | 0.77           | 0.76      | 0.41        | 0.42   |
| 62       | 0.60          | 0.61     | 0.76           | 0.76      | 0.43        | 0.43   |
| 63       | 0.61          | 0.61     | 0.77           | 0.75      | 0.43        | 0.43   |

Continued on next page

| $\alpha$ | $\phi_S^\ell$ | $\phi_S$ | $\varphi^\ell$ | $\varphi$ | $\psi^\ell$ | $\psi$ |
|----------|---------------|----------|----------------|-----------|-------------|--------|
| 64       | 0.61          | 0.61     | 0.77           | 0.76      | 0.43        | 0.43   |
| 65       | 0.61          | 0.61     | 0.77           | 0.76      | 0.43        | 0.43   |
| 66       | 0.60          | 0.61     | 0.78           | 0.76      | 0.42        | 0.43   |
| 67       | 0.60          | 0.60     | 0.78           | 0.77      | 0.42        | 0.42   |
| 68       | 0.59          | 0.60     | 0.79           | 0.77      | 0.41        | 0.42   |
| 69       | 0.59          | 0.59     | 0.79           | 0.78      | 0.41        | 0.41   |
| 70       | 0.58          | 0.59     | 0.80           | 0.78      | 0.40        | 0.41   |
| 71       | 0.57          | 0.58     | 0.80           | 0.79      | 0.39        | 0.40   |
| 72       | 0.57          | 0.57     | 0.81           | 0.79      | 0.39        | 0.40   |
| 73       | 0.56          | 0.56     | 0.81           | 0.80      | 0.39        | 0.39   |
| 74       | 0.55          | 0.56     | 0.82           | 0.80      | 0.38        | 0.39   |
| 75       | 0.54          | 0.55     | 0.82           | 0.81      | 0.37        | 0.38   |
| 76       | 0.53          | 0.54     | 0.83           | 0.81      | 0.36        | 0.37   |
| 77       | 0.52          | 0.53     | 0.84           | 0.82      | 0.35        | 0.37   |
| 78       | 0.51          | 0.52     | 0.84           | 0.83      | 0.35        | 0.36   |
| 79       | 0.50          | 0.51     | 0.85           | 0.83      | 0.34        | 0.35   |
| 80       | 0.49          | 0.50     | 0.86           | 0.84      | 0.33        | 0.34   |
| 81       | 0.48          | 0.49     | 0.86           | 0.85      | 0.32        | 0.33   |
| 82       | 0.46          | 0.48     | 0.87           | 0.85      | 0.31        | 0.33   |
| 83       | 0.45          | 0.46     | 0.88           | 0.86      | 0.30        | 0.31   |
| 84       | 0.43          | 0.45     | 0.89           | 0.87      | 0.29        | 0.30   |
| 85       | 0.41          | 0.43     | 0.90           | 0.88      | 0.27        | 0.29   |
| 86       | 0.39          | 0.41     | 0.91           | 0.89      | 0.26        | 0.27   |
| 87       | 0.37          | 0.39     | 0.92           | 0.90      | 0.24        | 0.26   |
| 88       | 0.33          | 0.36     | 0.93           | 0.91      | 0.22        | 0.24   |
| 89       | 0.29          | 0.32     | 0.95           | 0.92      | 0.19        | 0.21   |
| 90       | 0.11          | 0.14     | 0.99           | 0.96      | 0.07        | 0.09   |

Table S53: Reference ( $\phi_S$ ,  $\varphi$ ,  $\psi$ ) and approached ( $\phi_S^\ell$ ,  $\varphi^\ell$ ,  $\psi^\ell$ ) values of the topological descriptors for the first excited-state of the pyridinium-phenolate (PP), computed at the B3LYP/6-311++G(d,p) level of theory.  $\alpha$  is the pyridinium-phenolate central twist angle amplitude.



| $\alpha$ | $\phi_S^\ell$ | $\phi_S$ | $\varphi^\ell$ | $\varphi$ | $\psi^\ell$ | $\psi$ |
|----------|---------------|----------|----------------|-----------|-------------|--------|
| 0        | 0.41          | 0.31     | 0.83           | 0.87      | 0.29        | 0.22   |
| 1        | 0.41          | 0.31     | 0.83           | 0.87      | 0.29        | 0.22   |
| 2        | 0.41          | 0.31     | 0.84           | 0.87      | 0.29        | 0.22   |
| 3        | 0.40          | 0.31     | 0.84           | 0.87      | 0.28        | 0.22   |
| 4        | 0.40          | 0.31     | 0.84           | 0.87      | 0.28        | 0.22   |
| 5        | 0.40          | 0.31     | 0.84           | 0.87      | 0.28        | 0.22   |
| 6        | 0.40          | 0.32     | 0.84           | 0.87      | 0.28        | 0.22   |
| 7        | 0.40          | 0.32     | 0.84           | 0.87      | 0.28        | 0.22   |
| 8        | 0.39          | 0.32     | 0.84           | 0.87      | 0.28        | 0.22   |
| 9        | 0.39          | 0.32     | 0.85           | 0.87      | 0.27        | 0.22   |
| 10       | 0.39          | 0.32     | 0.85           | 0.87      | 0.27        | 0.22   |
| 11       | 0.38          | 0.32     | 0.85           | 0.87      | 0.27        | 0.22   |
| 12       | 0.38          | 0.32     | 0.85           | 0.87      | 0.27        | 0.22   |
| 13       | 0.37          | 0.32     | 0.85           | 0.87      | 0.26        | 0.22   |
| 14       | 0.37          | 0.32     | 0.86           | 0.87      | 0.26        | 0.22   |
| 15       | 0.36          | 0.32     | 0.86           | 0.87      | 0.25        | 0.22   |
| 16       | 0.36          | 0.33     | 0.86           | 0.87      | 0.25        | 0.23   |
| 17       | 0.35          | 0.33     | 0.86           | 0.87      | 0.25        | 0.23   |
| 18       | 0.35          | 0.33     | 0.87           | 0.87      | 0.24        | 0.23   |
| 19       | 0.34          | 0.33     | 0.87           | 0.87      | 0.24        | 0.23   |
| 20       | 0.33          | 0.33     | 0.87           | 0.87      | 0.23        | 0.23   |
| 21       | 0.33          | 0.33     | 0.87           | 0.87      | 0.23        | 0.23   |
| 22       | 0.32          | 0.33     | 0.87           | 0.87      | 0.22        | 0.23   |
| 23       | 0.31          | 0.33     | 0.88           | 0.87      | 0.22        | 0.23   |
| 24       | 0.31          | 0.33     | 0.88           | 0.87      | 0.22        | 0.23   |
| 25       | 0.30          | 0.33     | 0.88           | 0.87      | 0.21        | 0.23   |
| 26       | 0.29          | 0.33     | 0.88           | 0.87      | 0.20        | 0.23   |
| 27       | 0.28          | 0.33     | 0.88           | 0.87      | 0.20        | 0.23   |
| 28       | 0.28          | 0.33     | 0.88           | 0.87      | 0.20        | 0.23   |
| 29       | 0.27          | 0.33     | 0.89           | 0.87      | 0.19        | 0.23   |
| 30       | 0.26          | 0.33     | 0.89           | 0.87      | 0.18        | 0.23   |
| 31       | 0.25          | 0.33     | 0.89           | 0.87      | 0.17        | 0.23   |

Continued on next page

| $\alpha$ | $\phi_S^\ell$ | $\phi_S$ | $\varphi^\ell$ | $\varphi$ | $\psi^\ell$ | $\psi$ |
|----------|---------------|----------|----------------|-----------|-------------|--------|
| 32       | 0.25          | 0.33     | 0.90           | 0.87      | 0.17        | 0.23   |
| 33       | 0.24          | 0.33     | 0.90           | 0.87      | 0.17        | 0.23   |
| 34       | 0.23          | 0.33     | 0.91           | 0.87      | 0.16        | 0.23   |
| 35       | 0.23          | 0.33     | 0.91           | 0.87      | 0.16        | 0.23   |
| 36       | 0.22          | 0.33     | 0.92           | 0.87      | 0.15        | 0.23   |
| 37       | 0.21          | 0.33     | 0.93           | 0.88      | 0.14        | 0.23   |
| 38       | 0.20          | 0.33     | 0.93           | 0.88      | 0.13        | 0.23   |
| 39       | 0.20          | 0.33     | 0.93           | 0.88      | 0.13        | 0.23   |
| 40       | 0.19          | 0.33     | 0.94           | 0.88      | 0.13        | 0.23   |
| 41       | 0.18          | 0.33     | 0.94           | 0.88      | 0.12        | 0.23   |
| 42       | 0.18          | 0.33     | 0.94           | 0.88      | 0.12        | 0.23   |
| 43       | 0.17          | 0.33     | 0.94           | 0.88      | 0.11        | 0.23   |
| 44       | 0.17          | 0.33     | 0.95           | 0.88      | 0.11        | 0.23   |
| 45       | 0.17          | 0.33     | 0.95           | 0.88      | 0.11        | 0.23   |
| 46       | 0.17          | 0.33     | 0.95           | 0.88      | 0.11        | 0.23   |
| 47       | 0.17          | 0.33     | 0.95           | 0.88      | 0.11        | 0.23   |
| 48       | 0.18          | 0.33     | 0.94           | 0.88      | 0.12        | 0.23   |
| 49       | 0.18          | 0.33     | 0.94           | 0.88      | 0.12        | 0.23   |
| 50       | 0.19          | 0.33     | 0.94           | 0.88      | 0.13        | 0.23   |
| 51       | 0.20          | 0.33     | 0.93           | 0.88      | 0.13        | 0.23   |
| 52       | 0.21          | 0.34     | 0.93           | 0.88      | 0.14        | 0.23   |
| 53       | 0.23          | 0.35     | 0.92           | 0.88      | 0.16        | 0.24   |
| 54       | 0.25          | 0.35     | 0.92           | 0.88      | 0.17        | 0.24   |
| 55       | 0.27          | 0.37     | 0.91           | 0.87      | 0.18        | 0.26   |
| 56       | 0.30          | 0.38     | 0.90           | 0.86      | 0.20        | 0.26   |
| 57       | 0.34          | 0.41     | 0.89           | 0.85      | 0.23        | 0.29   |
| 58       | 0.39          | 0.45     | 0.86           | 0.83      | 0.27        | 0.32   |
| 59       | 0.47          | 0.50     | 0.81           | 0.81      | 0.33        | 0.35   |
| 60       | 0.54          | 0.56     | 0.79           | 0.78      | 0.38        | 0.40   |
| 61       | 0.58          | 0.59     | 0.77           | 0.76      | 0.41        | 0.42   |
| 62       | 0.60          | 0.61     | 0.76           | 0.76      | 0.43        | 0.43   |
| 63       | 0.61          | 0.61     | 0.77           | 0.75      | 0.43        | 0.43   |

Continued on next page

| $\alpha$ | $\phi_S^\ell$ | $\phi_S$ | $\varphi^\ell$ | $\varphi$ | $\psi^\ell$ | $\psi$ |
|----------|---------------|----------|----------------|-----------|-------------|--------|
| 64       | 0.61          | 0.61     | 0.77           | 0.76      | 0.43        | 0.43   |
| 65       | 0.61          | 0.61     | 0.77           | 0.76      | 0.43        | 0.43   |
| 66       | 0.60          | 0.61     | 0.78           | 0.76      | 0.42        | 0.43   |
| 67       | 0.60          | 0.60     | 0.78           | 0.77      | 0.42        | 0.42   |
| 68       | 0.59          | 0.60     | 0.79           | 0.77      | 0.41        | 0.42   |
| 69       | 0.59          | 0.59     | 0.79           | 0.78      | 0.41        | 0.41   |
| 70       | 0.58          | 0.59     | 0.80           | 0.78      | 0.40        | 0.41   |
| 71       | 0.57          | 0.58     | 0.80           | 0.79      | 0.39        | 0.40   |
| 72       | 0.57          | 0.57     | 0.81           | 0.79      | 0.39        | 0.40   |
| 73       | 0.56          | 0.56     | 0.81           | 0.80      | 0.39        | 0.39   |
| 74       | 0.55          | 0.56     | 0.82           | 0.80      | 0.38        | 0.39   |
| 75       | 0.54          | 0.55     | 0.82           | 0.81      | 0.37        | 0.38   |
| 76       | 0.53          | 0.54     | 0.83           | 0.81      | 0.36        | 0.37   |
| 77       | 0.52          | 0.53     | 0.84           | 0.82      | 0.35        | 0.37   |
| 78       | 0.51          | 0.52     | 0.84           | 0.83      | 0.35        | 0.36   |
| 79       | 0.50          | 0.51     | 0.85           | 0.83      | 0.34        | 0.35   |
| 80       | 0.49          | 0.50     | 0.86           | 0.84      | 0.33        | 0.34   |
| 81       | 0.48          | 0.49     | 0.86           | 0.85      | 0.32        | 0.33   |
| 82       | 0.46          | 0.48     | 0.87           | 0.85      | 0.31        | 0.33   |
| 83       | 0.45          | 0.46     | 0.88           | 0.86      | 0.30        | 0.31   |
| 84       | 0.43          | 0.45     | 0.89           | 0.87      | 0.29        | 0.30   |
| 85       | 0.41          | 0.43     | 0.90           | 0.88      | 0.27        | 0.29   |
| 86       | 0.39          | 0.41     | 0.91           | 0.89      | 0.26        | 0.27   |
| 87       | 0.37          | 0.39     | 0.92           | 0.90      | 0.24        | 0.26   |
| 88       | 0.33          | 0.36     | 0.93           | 0.91      | 0.22        | 0.24   |
| 89       | 0.29          | 0.32     | 0.95           | 0.92      | 0.19        | 0.21   |
| 90       | 0.11          | 0.14     | 0.99           | 0.96      | 0.07        | 0.09   |

Table S54: Reference ( $\phi_S$ ,  $\varphi$ ,  $\psi$ ) and approached ( $\phi_S^\ell$ ,  $\varphi^\ell$ ,  $\psi^\ell$ ) values of the topological descriptors for the first excited-state of the pyridinium-phenolate (PP), computed at the B3LYP/6-311+G(d,p) level of theory.  $\alpha$  is the pyridinium-phenolate central twist angle amplitude.

| $\alpha$ | $\phi_S^\ell$ | $\phi_S$ | $\varphi^\ell$ | $\varphi$ | $\psi^\ell$ | $\psi$ |
|----------|---------------|----------|----------------|-----------|-------------|--------|
| 0        | 0.40          | 0.31     | 0.84           | 0.87      | 0.28        | 0.22   |
| 1        | 0.40          | 0.31     | 0.84           | 0.87      | 0.28        | 0.22   |
| 2        | 0.40          | 0.31     | 0.84           | 0.87      | 0.28        | 0.22   |
| 3        | 0.40          | 0.31     | 0.84           | 0.87      | 0.28        | 0.22   |
| 4        | 0.40          | 0.31     | 0.84           | 0.87      | 0.28        | 0.22   |
| 5        | 0.40          | 0.31     | 0.84           | 0.87      | 0.28        | 0.22   |
| 6        | 0.40          | 0.31     | 0.84           | 0.87      | 0.28        | 0.22   |
| 7        | 0.39          | 0.31     | 0.85           | 0.87      | 0.27        | 0.22   |
| 8        | 0.39          | 0.31     | 0.85           | 0.87      | 0.27        | 0.22   |
| 9        | 0.39          | 0.32     | 0.85           | 0.87      | 0.27        | 0.22   |
| 10       | 0.38          | 0.32     | 0.85           | 0.87      | 0.27        | 0.22   |
| 11       | 0.38          | 0.32     | 0.85           | 0.87      | 0.27        | 0.22   |
| 12       | 0.37          | 0.32     | 0.85           | 0.87      | 0.26        | 0.22   |
| 13       | 0.37          | 0.32     | 0.86           | 0.87      | 0.26        | 0.22   |
| 14       | 0.37          | 0.32     | 0.86           | 0.87      | 0.26        | 0.22   |
| 15       | 0.36          | 0.32     | 0.86           | 0.87      | 0.25        | 0.22   |
| 16       | 0.35          | 0.32     | 0.86           | 0.87      | 0.25        | 0.22   |
| 17       | 0.35          | 0.32     | 0.87           | 0.87      | 0.24        | 0.22   |
| 18       | 0.34          | 0.32     | 0.87           | 0.87      | 0.24        | 0.22   |
| 19       | 0.34          | 0.33     | 0.87           | 0.87      | 0.24        | 0.23   |
| 20       | 0.33          | 0.33     | 0.87           | 0.87      | 0.23        | 0.23   |
| 21       | 0.32          | 0.33     | 0.87           | 0.87      | 0.22        | 0.23   |
| 22       | 0.32          | 0.33     | 0.88           | 0.87      | 0.22        | 0.23   |
| 23       | 0.31          | 0.33     | 0.88           | 0.87      | 0.22        | 0.23   |
| 24       | 0.30          | 0.33     | 0.88           | 0.87      | 0.21        | 0.23   |
| 25       | 0.30          | 0.33     | 0.88           | 0.87      | 0.21        | 0.23   |
| 26       | 0.29          | 0.33     | 0.88           | 0.87      | 0.20        | 0.23   |
| 27       | 0.28          | 0.33     | 0.88           | 0.87      | 0.20        | 0.23   |
| 28       | 0.27          | 0.33     | 0.89           | 0.87      | 0.19        | 0.23   |
| 29       | 0.27          | 0.33     | 0.89           | 0.87      | 0.19        | 0.23   |
| 30       | 0.26          | 0.33     | 0.89           | 0.87      | 0.18        | 0.23   |
| 31       | 0.25          | 0.33     | 0.89           | 0.87      | 0.17        | 0.23   |

Continued on next page

| $\alpha$ | $\phi_S^\ell$ | $\phi_S$ | $\varphi^\ell$ | $\varphi$ | $\psi^\ell$ | $\psi$ |
|----------|---------------|----------|----------------|-----------|-------------|--------|
| 32       | 0.25          | 0.33     | 0.90           | 0.87      | 0.17        | 0.23   |
| 33       | 0.24          | 0.33     | 0.90           | 0.87      | 0.17        | 0.23   |
| 34       | 0.23          | 0.33     | 0.91           | 0.87      | 0.16        | 0.23   |
| 35       | 0.22          | 0.33     | 0.92           | 0.87      | 0.15        | 0.23   |
| 36       | 0.22          | 0.33     | 0.92           | 0.88      | 0.15        | 0.23   |
| 37       | 0.21          | 0.33     | 0.93           | 0.88      | 0.14        | 0.23   |
| 38       | 0.20          | 0.33     | 0.93           | 0.88      | 0.13        | 0.23   |
| 39       | 0.20          | 0.33     | 0.93           | 0.88      | 0.13        | 0.23   |
| 40       | 0.19          | 0.33     | 0.94           | 0.88      | 0.13        | 0.23   |
| 41       | 0.18          | 0.33     | 0.94           | 0.88      | 0.12        | 0.23   |
| 42       | 0.18          | 0.33     | 0.94           | 0.88      | 0.12        | 0.23   |
| 43       | 0.17          | 0.33     | 0.94           | 0.88      | 0.11        | 0.23   |
| 44       | 0.17          | 0.33     | 0.95           | 0.88      | 0.11        | 0.23   |
| 45       | 0.17          | 0.33     | 0.95           | 0.88      | 0.11        | 0.23   |
| 46       | 0.17          | 0.33     | 0.95           | 0.88      | 0.11        | 0.23   |
| 47       | 0.17          | 0.33     | 0.94           | 0.88      | 0.11        | 0.23   |
| 48       | 0.18          | 0.33     | 0.94           | 0.88      | 0.12        | 0.23   |
| 49       | 0.19          | 0.33     | 0.94           | 0.88      | 0.13        | 0.23   |
| 50       | 0.20          | 0.33     | 0.93           | 0.88      | 0.13        | 0.23   |
| 51       | 0.21          | 0.34     | 0.93           | 0.88      | 0.14        | 0.23   |
| 52       | 0.22          | 0.34     | 0.92           | 0.88      | 0.15        | 0.23   |
| 53       | 0.24          | 0.35     | 0.92           | 0.88      | 0.16        | 0.24   |
| 54       | 0.26          | 0.36     | 0.91           | 0.87      | 0.18        | 0.25   |
| 55       | 0.29          | 0.38     | 0.91           | 0.87      | 0.20        | 0.26   |
| 56       | 0.32          | 0.40     | 0.89           | 0.86      | 0.22        | 0.28   |
| 57       | 0.37          | 0.44     | 0.87           | 0.84      | 0.26        | 0.31   |
| 58       | 0.44          | 0.48     | 0.82           | 0.82      | 0.31        | 0.34   |
| 59       | 0.51          | 0.54     | 0.80           | 0.79      | 0.36        | 0.38   |
| 60       | 0.57          | 0.58     | 0.78           | 0.77      | 0.40        | 0.41   |
| 61       | 0.60          | 0.61     | 0.77           | 0.76      | 0.42        | 0.43   |
| 62       | 0.61          | 0.61     | 0.76           | 0.75      | 0.43        | 0.43   |
| 63       | 0.61          | 0.62     | 0.77           | 0.75      | 0.43        | 0.44   |

Continued on next page

| $\alpha$ | $\phi_S^\ell$ | $\phi_S$ | $\varphi^\ell$ | $\varphi$ | $\psi^\ell$ | $\psi$ |
|----------|---------------|----------|----------------|-----------|-------------|--------|
| 64       | 0.61          | 0.61     | 0.77           | 0.76      | 0.43        | 0.43   |
| 65       | 0.61          | 0.61     | 0.77           | 0.76      | 0.43        | 0.43   |
| 66       | 0.60          | 0.61     | 0.78           | 0.77      | 0.42        | 0.43   |
| 67       | 0.60          | 0.60     | 0.78           | 0.77      | 0.42        | 0.42   |
| 68       | 0.59          | 0.60     | 0.79           | 0.77      | 0.41        | 0.42   |
| 69       | 0.58          | 0.59     | 0.79           | 0.78      | 0.40        | 0.41   |
| 70       | 0.58          | 0.58     | 0.80           | 0.78      | 0.40        | 0.41   |
| 71       | 0.57          | 0.58     | 0.80           | 0.79      | 0.39        | 0.40   |
| 72       | 0.56          | 0.57     | 0.81           | 0.79      | 0.39        | 0.40   |
| 73       | 0.56          | 0.56     | 0.81           | 0.80      | 0.39        | 0.39   |
| 74       | 0.55          | 0.55     | 0.82           | 0.80      | 0.38        | 0.38   |
| 75       | 0.54          | 0.55     | 0.83           | 0.81      | 0.37        | 0.38   |
| 76       | 0.53          | 0.54     | 0.83           | 0.82      | 0.36        | 0.37   |
| 77       | 0.52          | 0.53     | 0.84           | 0.82      | 0.35        | 0.37   |
| 78       | 0.51          | 0.52     | 0.84           | 0.83      | 0.35        | 0.36   |
| 79       | 0.50          | 0.51     | 0.85           | 0.83      | 0.34        | 0.35   |
| 80       | 0.49          | 0.50     | 0.86           | 0.84      | 0.33        | 0.34   |
| 81       | 0.48          | 0.49     | 0.86           | 0.85      | 0.32        | 0.33   |
| 82       | 0.46          | 0.47     | 0.87           | 0.86      | 0.31        | 0.32   |
| 83       | 0.45          | 0.46     | 0.88           | 0.86      | 0.30        | 0.31   |
| 84       | 0.43          | 0.44     | 0.89           | 0.87      | 0.29        | 0.30   |
| 85       | 0.41          | 0.43     | 0.90           | 0.88      | 0.27        | 0.29   |
| 86       | 0.39          | 0.41     | 0.91           | 0.89      | 0.26        | 0.27   |
| 87       | 0.36          | 0.38     | 0.92           | 0.90      | 0.24        | 0.25   |
| 88       | 0.33          | 0.35     | 0.93           | 0.91      | 0.22        | 0.23   |
| 89       | 0.28          | 0.31     | 0.95           | 0.93      | 0.18        | 0.20   |
| 90       | 0.10          | 0.14     | 0.99           | 0.96      | 0.06        | 0.09   |

Table S55: Reference ( $\phi_S$ ,  $\varphi$ ,  $\psi$ ) and approached ( $\phi_S^\ell$ ,  $\varphi^\ell$ ,  $\psi^\ell$ ) values of the topological descriptors for the first excited-state of the pyridinium-phenolate (PP), computed at the B3LYP/6-311+G(d) level of theory.  $\alpha$  is the pyridinium-phenolate central twist angle amplitude.

| $\alpha$ | $\phi_S^\ell$ | $\phi_S$ | $\varphi^\ell$ | $\varphi$ | $\psi^\ell$ | $\psi$ |
|----------|---------------|----------|----------------|-----------|-------------|--------|
| 0        | 0.41          | 0.31     | 0.83           | 0.86      | 0.29        | 0.22   |
| 1        | 0.41          | 0.31     | 0.83           | 0.86      | 0.29        | 0.22   |
| 2        | 0.41          | 0.31     | 0.83           | 0.86      | 0.29        | 0.22   |
| 3        | 0.41          | 0.31     | 0.83           | 0.86      | 0.29        | 0.22   |
| 4        | 0.41          | 0.31     | 0.83           | 0.86      | 0.29        | 0.22   |
| 5        | 0.41          | 0.31     | 0.84           | 0.86      | 0.29        | 0.22   |
| 6        | 0.40          | 0.32     | 0.84           | 0.86      | 0.28        | 0.23   |
| 7        | 0.40          | 0.32     | 0.84           | 0.86      | 0.28        | 0.23   |
| 8        | 0.40          | 0.32     | 0.84           | 0.86      | 0.28        | 0.23   |
| 9        | 0.39          | 0.32     | 0.84           | 0.86      | 0.28        | 0.23   |
| 10       | 0.39          | 0.32     | 0.84           | 0.86      | 0.28        | 0.23   |
| 11       | 0.38          | 0.32     | 0.85           | 0.86      | 0.27        | 0.23   |
| 12       | 0.38          | 0.32     | 0.85           | 0.87      | 0.27        | 0.22   |
| 13       | 0.37          | 0.32     | 0.85           | 0.87      | 0.26        | 0.22   |
| 14       | 0.37          | 0.32     | 0.85           | 0.87      | 0.26        | 0.22   |
| 15       | 0.36          | 0.32     | 0.85           | 0.87      | 0.26        | 0.22   |
| 16       | 0.36          | 0.32     | 0.86           | 0.87      | 0.25        | 0.22   |
| 17       | 0.35          | 0.32     | 0.86           | 0.87      | 0.25        | 0.22   |
| 18       | 0.34          | 0.32     | 0.86           | 0.87      | 0.24        | 0.22   |
| 19       | 0.33          | 0.32     | 0.86           | 0.87      | 0.23        | 0.22   |
| 20       | 0.33          | 0.32     | 0.87           | 0.87      | 0.23        | 0.22   |
| 21       | 0.32          | 0.32     | 0.87           | 0.87      | 0.22        | 0.22   |
| 22       | 0.31          | 0.32     | 0.87           | 0.87      | 0.22        | 0.22   |
| 23       | 0.30          | 0.32     | 0.87           | 0.87      | 0.21        | 0.22   |
| 24       | 0.29          | 0.32     | 0.88           | 0.87      | 0.20        | 0.22   |
| 25       | 0.28          | 0.32     | 0.88           | 0.87      | 0.20        | 0.22   |
| 26       | 0.27          | 0.32     | 0.88           | 0.87      | 0.19        | 0.22   |
| 27       | 0.27          | 0.32     | 0.88           | 0.87      | 0.19        | 0.22   |
| 28       | 0.26          | 0.32     | 0.89           | 0.87      | 0.18        | 0.22   |
| 29       | 0.25          | 0.32     | 0.89           | 0.87      | 0.17        | 0.22   |
| 30       | 0.24          | 0.32     | 0.90           | 0.87      | 0.17        | 0.22   |
| 31       | 0.23          | 0.31     | 0.91           | 0.87      | 0.16        | 0.22   |

Continued on next page

| $\alpha$ | $\phi_S^\ell$ | $\phi_S$ | $\varphi^\ell$ | $\varphi$ | $\psi^\ell$ | $\psi$ |
|----------|---------------|----------|----------------|-----------|-------------|--------|
| 32       | 0.22          | 0.31     | 0.91           | 0.87      | 0.15        | 0.22   |
| 33       | 0.21          | 0.31     | 0.92           | 0.88      | 0.14        | 0.22   |
| 34       | 0.20          | 0.31     | 0.93           | 0.88      | 0.13        | 0.22   |
| 35       | 0.19          | 0.31     | 0.94           | 0.88      | 0.13        | 0.22   |
| 36       | 0.18          | 0.31     | 0.94           | 0.88      | 0.12        | 0.22   |
| 37       | 0.17          | 0.31     | 0.95           | 0.88      | 0.11        | 0.22   |
| 38       | 0.16          | 0.31     | 0.96           | 0.88      | 0.11        | 0.22   |
| 39       | 0.15          | 0.31     | 0.96           | 0.88      | 0.10        | 0.22   |
| 40       | 0.14          | 0.30     | 0.97           | 0.88      | 0.09        | 0.21   |
| 41       | 0.14          | 0.30     | 0.97           | 0.88      | 0.09        | 0.21   |
| 42       | 0.13          | 0.30     | 0.97           | 0.88      | 0.08        | 0.21   |
| 43       | 0.12          | 0.30     | 0.98           | 0.89      | 0.08        | 0.21   |
| 44       | 0.11          | 0.30     | 0.98           | 0.89      | 0.07        | 0.21   |
| 45       | 0.10          | 0.30     | 0.98           | 0.89      | 0.06        | 0.21   |
| 46       | 0.10          | 0.29     | 0.98           | 0.89      | 0.06        | 0.20   |
| 47       | 0.10          | 0.29     | 0.98           | 0.89      | 0.06        | 0.20   |
| 48       | 0.11          | 0.29     | 0.98           | 0.89      | 0.07        | 0.20   |
| 49       | 0.11          | 0.29     | 0.98           | 0.89      | 0.07        | 0.20   |
| 50       | 0.12          | 0.28     | 0.98           | 0.89      | 0.08        | 0.19   |
| 51       | 0.13          | 0.28     | 0.97           | 0.89      | 0.08        | 0.19   |
| 52       | 0.14          | 0.28     | 0.97           | 0.90      | 0.09        | 0.19   |
| 53       | 0.15          | 0.28     | 0.97           | 0.90      | 0.10        | 0.19   |
| 54       | 0.16          | 0.28     | 0.96           | 0.90      | 0.11        | 0.19   |
| 55       | 0.17          | 0.27     | 0.96           | 0.90      | 0.11        | 0.19   |
| 56       | 0.18          | 0.27     | 0.95           | 0.90      | 0.12        | 0.19   |
| 57       | 0.19          | 0.27     | 0.95           | 0.90      | 0.13        | 0.19   |
| 58       | 0.20          | 0.27     | 0.94           | 0.90      | 0.13        | 0.19   |
| 59       | 0.20          | 0.27     | 0.93           | 0.91      | 0.13        | 0.18   |
| 60       | 0.21          | 0.26     | 0.93           | 0.91      | 0.14        | 0.18   |
| 61       | 0.22          | 0.26     | 0.92           | 0.91      | 0.15        | 0.18   |
| 62       | 0.23          | 0.26     | 0.91           | 0.91      | 0.16        | 0.18   |
| 63       | 0.23          | 0.26     | 0.91           | 0.91      | 0.16        | 0.18   |

Continued on next page



| $\alpha$ | $\phi_S^\ell$ | $\phi_S$ | $\varphi^\ell$ | $\varphi$ | $\psi^\ell$ | $\psi$ |
|----------|---------------|----------|----------------|-----------|-------------|--------|
| 64       | 0.24          | 0.26     | 0.90           | 0.91      | 0.17        | 0.18   |
| 65       | 0.25          | 0.26     | 0.90           | 0.91      | 0.17        | 0.18   |
| 66       | 0.26          | 0.27     | 0.90           | 0.91      | 0.18        | 0.18   |
| 67       | 0.61          | 0.61     | 0.77           | 0.76      | 0.43        | 0.43   |
| 68       | 0.61          | 0.61     | 0.77           | 0.76      | 0.43        | 0.43   |
| 69       | 0.61          | 0.61     | 0.78           | 0.76      | 0.42        | 0.43   |
| 70       | 0.60          | 0.60     | 0.78           | 0.77      | 0.42        | 0.42   |
| 71       | 0.59          | 0.60     | 0.79           | 0.77      | 0.41        | 0.42   |
| 72       | 0.59          | 0.59     | 0.79           | 0.78      | 0.41        | 0.41   |
| 73       | 0.58          | 0.58     | 0.80           | 0.78      | 0.40        | 0.41   |
| 74       | 0.57          | 0.58     | 0.80           | 0.79      | 0.39        | 0.40   |
| 75       | 0.57          | 0.57     | 0.81           | 0.80      | 0.39        | 0.39   |
| 76       | 0.56          | 0.56     | 0.81           | 0.80      | 0.39        | 0.39   |
| 77       | 0.55          | 0.55     | 0.82           | 0.81      | 0.38        | 0.38   |
| 78       | 0.54          | 0.54     | 0.83           | 0.81      | 0.37        | 0.37   |
| 79       | 0.53          | 0.54     | 0.83           | 0.82      | 0.36        | 0.37   |
| 80       | 0.52          | 0.53     | 0.84           | 0.82      | 0.35        | 0.37   |
| 81       | 0.51          | 0.52     | 0.85           | 0.83      | 0.34        | 0.36   |
| 82       | 0.50          | 0.50     | 0.85           | 0.84      | 0.34        | 0.34   |
| 83       | 0.48          | 0.49     | 0.86           | 0.85      | 0.32        | 0.33   |
| 84       | 0.47          | 0.48     | 0.87           | 0.85      | 0.32        | 0.33   |
| 85       | 0.45          | 0.46     | 0.88           | 0.86      | 0.30        | 0.31   |
| 86       | 0.43          | 0.45     | 0.89           | 0.87      | 0.29        | 0.30   |
| 87       | 0.41          | 0.43     | 0.90           | 0.88      | 0.27        | 0.29   |
| 88       | 0.39          | 0.40     | 0.91           | 0.89      | 0.26        | 0.27   |
| 89       | 0.35          | 0.37     | 0.92           | 0.90      | 0.23        | 0.25   |
| 90       | 0.10          | 0.15     | 0.99           | 0.96      | 0.06        | 0.10   |

Table S56: Reference ( $\phi_S$ ,  $\varphi$ ,  $\psi$ ) and approached ( $\phi_S^\ell$ ,  $\varphi^\ell$ ,  $\psi^\ell$ ) values of the topological descriptors for the first excited-state of the pyridinium-phenolate (PP), computed at the B3LYP/6-311G(d) level of theory.  $\alpha$  is the pyridinium-phenolate central twist angle amplitude.

| $\alpha$ | $\phi_S^\ell$ | $\phi_S$ | $\varphi^\ell$ | $\varphi$ | $\psi^\ell$ | $\psi$ |
|----------|---------------|----------|----------------|-----------|-------------|--------|
| 0        | 0.41          | 0.31     | 0.83           | 0.87      | 0.29        | 0.22   |
| 1        | 0.41          | 0.31     | 0.83           | 0.87      | 0.29        | 0.22   |
| 2        | 0.41          | 0.31     | 0.83           | 0.87      | 0.29        | 0.22   |
| 3        | 0.41          | 0.31     | 0.83           | 0.87      | 0.29        | 0.22   |
| 4        | 0.40          | 0.31     | 0.83           | 0.87      | 0.29        | 0.22   |
| 5        | 0.40          | 0.32     | 0.84           | 0.87      | 0.28        | 0.22   |
| 6        | 0.40          | 0.32     | 0.84           | 0.87      | 0.28        | 0.22   |
| 7        | 0.40          | 0.32     | 0.84           | 0.87      | 0.28        | 0.22   |
| 8        | 0.39          | 0.32     | 0.84           | 0.87      | 0.28        | 0.22   |
| 9        | 0.39          | 0.32     | 0.84           | 0.87      | 0.28        | 0.22   |
| 10       | 0.39          | 0.32     | 0.85           | 0.87      | 0.27        | 0.22   |
| 11       | 0.38          | 0.32     | 0.85           | 0.87      | 0.27        | 0.22   |
| 12       | 0.38          | 0.32     | 0.85           | 0.87      | 0.27        | 0.22   |
| 13       | 0.37          | 0.32     | 0.85           | 0.87      | 0.26        | 0.22   |
| 14       | 0.37          | 0.32     | 0.85           | 0.87      | 0.26        | 0.22   |
| 15       | 0.36          | 0.32     | 0.86           | 0.87      | 0.25        | 0.22   |
| 16       | 0.36          | 0.32     | 0.86           | 0.87      | 0.25        | 0.22   |
| 17       | 0.35          | 0.33     | 0.86           | 0.87      | 0.25        | 0.23   |
| 18       | 0.35          | 0.33     | 0.86           | 0.87      | 0.25        | 0.23   |
| 19       | 0.34          | 0.33     | 0.86           | 0.87      | 0.24        | 0.23   |
| 20       | 0.33          | 0.33     | 0.87           | 0.87      | 0.23        | 0.23   |
| 21       | 0.33          | 0.33     | 0.87           | 0.87      | 0.23        | 0.23   |
| 22       | 0.32          | 0.33     | 0.87           | 0.87      | 0.22        | 0.23   |
| 23       | 0.31          | 0.33     | 0.87           | 0.87      | 0.22        | 0.23   |
| 24       | 0.31          | 0.33     | 0.88           | 0.87      | 0.22        | 0.23   |
| 25       | 0.30          | 0.33     | 0.88           | 0.87      | 0.21        | 0.23   |
| 26       | 0.29          | 0.33     | 0.88           | 0.87      | 0.20        | 0.23   |
| 27       | 0.28          | 0.33     | 0.88           | 0.87      | 0.20        | 0.23   |
| 28       | 0.28          | 0.33     | 0.88           | 0.87      | 0.20        | 0.23   |
| 29       | 0.27          | 0.33     | 0.88           | 0.87      | 0.19        | 0.23   |
| 30       | 0.26          | 0.33     | 0.88           | 0.87      | 0.18        | 0.23   |
| 31       | 0.26          | 0.33     | 0.89           | 0.87      | 0.18        | 0.23   |

Continued on next page

| $\alpha$ | $\phi_S^\ell$ | $\phi_S$ | $\varphi^\ell$ | $\varphi$ | $\psi^\ell$ | $\psi$ |
|----------|---------------|----------|----------------|-----------|-------------|--------|
| 32       | 0.25          | 0.33     | 0.89           | 0.87      | 0.17        | 0.23   |
| 33       | 0.24          | 0.33     | 0.90           | 0.87      | 0.17        | 0.23   |
| 34       | 0.24          | 0.33     | 0.91           | 0.87      | 0.16        | 0.23   |
| 35       | 0.23          | 0.33     | 0.91           | 0.87      | 0.16        | 0.23   |
| 36       | 0.22          | 0.33     | 0.92           | 0.87      | 0.15        | 0.23   |
| 37       | 0.22          | 0.33     | 0.92           | 0.87      | 0.15        | 0.23   |
| 38       | 0.21          | 0.33     | 0.93           | 0.88      | 0.14        | 0.23   |
| 39       | 0.20          | 0.33     | 0.93           | 0.88      | 0.13        | 0.23   |
| 40       | 0.20          | 0.33     | 0.93           | 0.88      | 0.13        | 0.23   |
| 41       | 0.19          | 0.33     | 0.94           | 0.88      | 0.13        | 0.23   |
| 42       | 0.19          | 0.33     | 0.94           | 0.88      | 0.13        | 0.23   |
| 43       | 0.18          | 0.33     | 0.94           | 0.88      | 0.12        | 0.23   |
| 44       | 0.18          | 0.33     | 0.94           | 0.88      | 0.12        | 0.23   |
| 45       | 0.18          | 0.33     | 0.94           | 0.88      | 0.12        | 0.23   |
| 46       | 0.18          | 0.33     | 0.94           | 0.88      | 0.12        | 0.23   |
| 47       | 0.18          | 0.33     | 0.94           | 0.88      | 0.12        | 0.23   |
| 48       | 0.19          | 0.33     | 0.94           | 0.88      | 0.13        | 0.23   |
| 49       | 0.19          | 0.34     | 0.93           | 0.88      | 0.13        | 0.23   |
| 50       | 0.20          | 0.34     | 0.93           | 0.88      | 0.13        | 0.23   |
| 51       | 0.21          | 0.34     | 0.92           | 0.88      | 0.14        | 0.23   |
| 52       | 0.22          | 0.35     | 0.92           | 0.88      | 0.15        | 0.24   |
| 53       | 0.24          | 0.35     | 0.92           | 0.88      | 0.16        | 0.24   |
| 54       | 0.25          | 0.36     | 0.92           | 0.87      | 0.17        | 0.25   |
| 55       | 0.27          | 0.37     | 0.91           | 0.87      | 0.18        | 0.26   |
| 56       | 0.29          | 0.38     | 0.91           | 0.87      | 0.20        | 0.26   |
| 57       | 0.31          | 0.39     | 0.90           | 0.86      | 0.21        | 0.27   |
| 58       | 0.35          | 0.41     | 0.89           | 0.85      | 0.24        | 0.29   |
| 59       | 0.38          | 0.44     | 0.87           | 0.84      | 0.26        | 0.31   |
| 60       | 0.43          | 0.47     | 0.84           | 0.83      | 0.30        | 0.33   |
| 61       | 0.48          | 0.51     | 0.81           | 0.81      | 0.34        | 0.36   |
| 62       | 0.53          | 0.55     | 0.80           | 0.79      | 0.37        | 0.39   |
| 63       | 0.56          | 0.57     | 0.79           | 0.78      | 0.39        | 0.40   |

Continued on next page

| $\alpha$ | $\phi_S^\ell$ | $\phi_S$ | $\varphi^\ell$ | $\varphi$ | $\psi^\ell$ | $\psi$ |
|----------|---------------|----------|----------------|-----------|-------------|--------|
| 64       | 0.58          | 0.59     | 0.78           | 0.77      | 0.41        | 0.42   |
| 65       | 0.59          | 0.60     | 0.78           | 0.77      | 0.41        | 0.42   |
| 66       | 0.60          | 0.60     | 0.78           | 0.77      | 0.42        | 0.42   |
| 67       | 0.60          | 0.60     | 0.78           | 0.77      | 0.42        | 0.42   |
| 68       | 0.59          | 0.60     | 0.78           | 0.77      | 0.41        | 0.42   |
| 69       | 0.59          | 0.59     | 0.79           | 0.78      | 0.41        | 0.41   |
| 70       | 0.58          | 0.59     | 0.79           | 0.78      | 0.40        | 0.41   |
| 71       | 0.58          | 0.58     | 0.80           | 0.79      | 0.40        | 0.40   |
| 72       | 0.57          | 0.58     | 0.80           | 0.79      | 0.39        | 0.40   |
| 73       | 0.57          | 0.57     | 0.81           | 0.80      | 0.39        | 0.39   |
| 74       | 0.56          | 0.56     | 0.81           | 0.80      | 0.39        | 0.39   |
| 75       | 0.55          | 0.55     | 0.82           | 0.81      | 0.38        | 0.38   |
| 76       | 0.54          | 0.55     | 0.83           | 0.81      | 0.37        | 0.38   |
| 77       | 0.53          | 0.54     | 0.83           | 0.82      | 0.36        | 0.37   |
| 78       | 0.52          | 0.53     | 0.84           | 0.82      | 0.35        | 0.37   |
| 79       | 0.51          | 0.52     | 0.85           | 0.83      | 0.34        | 0.36   |
| 80       | 0.50          | 0.51     | 0.85           | 0.84      | 0.34        | 0.35   |
| 81       | 0.49          | 0.50     | 0.86           | 0.84      | 0.33        | 0.34   |
| 82       | 0.48          | 0.49     | 0.87           | 0.85      | 0.32        | 0.33   |
| 83       | 0.46          | 0.47     | 0.88           | 0.86      | 0.31        | 0.32   |
| 84       | 0.45          | 0.46     | 0.88           | 0.87      | 0.30        | 0.31   |
| 85       | 0.43          | 0.44     | 0.89           | 0.87      | 0.29        | 0.30   |
| 86       | 0.41          | 0.42     | 0.90           | 0.88      | 0.27        | 0.28   |
| 87       | 0.38          | 0.40     | 0.91           | 0.89      | 0.25        | 0.27   |
| 88       | 0.35          | 0.37     | 0.93           | 0.91      | 0.23        | 0.25   |
| 89       | 0.32          | 0.34     | 0.94           | 0.92      | 0.21        | 0.23   |
| 90       | 0.09          | 0.13     | 0.99           | 0.97      | 0.06        | 0.08   |

Table S57: Reference ( $\phi_S$ ,  $\varphi$ ,  $\psi$ ) and approached ( $\phi_S^\ell$ ,  $\varphi^\ell$ ,  $\psi^\ell$ ) values of the topological descriptors for the first excited-state of the pyridinium-phenolate (PP), computed at the B3LYP/6-311+G level of theory.  $\alpha$  is the pyridinium-phenolate central twist angle amplitude.

| $\alpha$ | $\phi_S^\ell$ | $\phi_S$ | $\varphi^\ell$ | $\varphi$ | $\psi^\ell$ | $\psi$ |
|----------|---------------|----------|----------------|-----------|-------------|--------|
| 0        | 0.42          | 0.32     | 0.83           | 0.86      | 0.30        | 0.23   |
| 1        | 0.42          | 0.32     | 0.83           | 0.86      | 0.30        | 0.23   |
| 2        | 0.42          | 0.32     | 0.83           | 0.86      | 0.30        | 0.23   |
| 3        | 0.41          | 0.32     | 0.83           | 0.86      | 0.29        | 0.23   |
| 4        | 0.41          | 0.32     | 0.83           | 0.86      | 0.29        | 0.23   |
| 5        | 0.41          | 0.32     | 0.83           | 0.86      | 0.29        | 0.23   |
| 6        | 0.41          | 0.32     | 0.83           | 0.86      | 0.29        | 0.23   |
| 7        | 0.40          | 0.32     | 0.83           | 0.86      | 0.29        | 0.23   |
| 8        | 0.40          | 0.32     | 0.84           | 0.86      | 0.28        | 0.23   |
| 9        | 0.40          | 0.32     | 0.84           | 0.86      | 0.28        | 0.23   |
| 10       | 0.39          | 0.32     | 0.84           | 0.86      | 0.28        | 0.23   |
| 11       | 0.39          | 0.32     | 0.84           | 0.86      | 0.28        | 0.23   |
| 12       | 0.38          | 0.32     | 0.84           | 0.86      | 0.27        | 0.23   |
| 13       | 0.38          | 0.32     | 0.84           | 0.86      | 0.27        | 0.23   |
| 14       | 0.37          | 0.32     | 0.85           | 0.86      | 0.26        | 0.23   |
| 15       | 0.37          | 0.32     | 0.85           | 0.87      | 0.26        | 0.22   |
| 16       | 0.36          | 0.32     | 0.85           | 0.87      | 0.26        | 0.22   |
| 17       | 0.35          | 0.32     | 0.85           | 0.87      | 0.25        | 0.22   |
| 18       | 0.35          | 0.32     | 0.86           | 0.87      | 0.25        | 0.22   |
| 19       | 0.34          | 0.32     | 0.86           | 0.87      | 0.24        | 0.22   |
| 20       | 0.33          | 0.32     | 0.86           | 0.87      | 0.23        | 0.22   |
| 21       | 0.32          | 0.32     | 0.86           | 0.87      | 0.23        | 0.22   |
| 22       | 0.31          | 0.32     | 0.87           | 0.87      | 0.22        | 0.22   |
| 23       | 0.31          | 0.32     | 0.87           | 0.87      | 0.22        | 0.22   |
| 24       | 0.30          | 0.32     | 0.87           | 0.87      | 0.21        | 0.22   |
| 25       | 0.29          | 0.32     | 0.87           | 0.87      | 0.20        | 0.22   |
| 26       | 0.28          | 0.32     | 0.87           | 0.87      | 0.20        | 0.22   |
| 27       | 0.27          | 0.32     | 0.88           | 0.87      | 0.19        | 0.22   |
| 28       | 0.26          | 0.32     | 0.88           | 0.87      | 0.18        | 0.22   |
| 29       | 0.25          | 0.32     | 0.89           | 0.87      | 0.17        | 0.22   |
| 30       | 0.24          | 0.32     | 0.89           | 0.87      | 0.17        | 0.22   |
| 31       | 0.24          | 0.32     | 0.90           | 0.87      | 0.17        | 0.22   |

Continued on next page

| $\alpha$ | $\phi_S^\ell$ | $\phi_S$ | $\varphi^\ell$ | $\varphi$ | $\psi^\ell$ | $\psi$ |
|----------|---------------|----------|----------------|-----------|-------------|--------|
| 32       | 0.23          | 0.32     | 0.91           | 0.87      | 0.16        | 0.22   |
| 33       | 0.22          | 0.32     | 0.92           | 0.87      | 0.15        | 0.22   |
| 34       | 0.21          | 0.32     | 0.93           | 0.87      | 0.14        | 0.22   |
| 35       | 0.20          | 0.32     | 0.93           | 0.88      | 0.13        | 0.22   |
| 36       | 0.19          | 0.32     | 0.94           | 0.88      | 0.13        | 0.22   |
| 37       | 0.18          | 0.31     | 0.94           | 0.88      | 0.12        | 0.22   |
| 38       | 0.18          | 0.31     | 0.95           | 0.88      | 0.12        | 0.22   |
| 39       | 0.17          | 0.31     | 0.95           | 0.88      | 0.11        | 0.22   |
| 40       | 0.16          | 0.31     | 0.96           | 0.88      | 0.11        | 0.22   |
| 41       | 0.15          | 0.31     | 0.96           | 0.88      | 0.10        | 0.22   |
| 42       | 0.14          | 0.31     | 0.97           | 0.88      | 0.09        | 0.22   |
| 43       | 0.13          | 0.31     | 0.97           | 0.88      | 0.08        | 0.22   |
| 44       | 0.13          | 0.31     | 0.97           | 0.88      | 0.08        | 0.22   |
| 45       | 0.12          | 0.31     | 0.97           | 0.88      | 0.08        | 0.22   |
| 46       | 0.12          | 0.30     | 0.97           | 0.89      | 0.08        | 0.21   |
| 47       | 0.12          | 0.30     | 0.97           | 0.89      | 0.08        | 0.21   |
| 48       | 0.12          | 0.30     | 0.97           | 0.89      | 0.08        | 0.21   |
| 49       | 0.13          | 0.30     | 0.97           | 0.89      | 0.08        | 0.21   |
| 50       | 0.13          | 0.30     | 0.97           | 0.89      | 0.08        | 0.21   |
| 51       | 0.14          | 0.30     | 0.97           | 0.89      | 0.09        | 0.21   |
| 52       | 0.15          | 0.30     | 0.96           | 0.89      | 0.10        | 0.21   |
| 53       | 0.16          | 0.29     | 0.96           | 0.89      | 0.11        | 0.20   |
| 54       | 0.17          | 0.29     | 0.96           | 0.89      | 0.11        | 0.20   |
| 55       | 0.18          | 0.29     | 0.95           | 0.89      | 0.12        | 0.20   |
| 56       | 0.19          | 0.29     | 0.95           | 0.89      | 0.13        | 0.20   |
| 57       | 0.20          | 0.29     | 0.94           | 0.90      | 0.13        | 0.20   |
| 58       | 0.22          | 0.29     | 0.93           | 0.90      | 0.15        | 0.20   |
| 59       | 0.23          | 0.29     | 0.93           | 0.90      | 0.15        | 0.20   |
| 60       | 0.24          | 0.30     | 0.92           | 0.90      | 0.16        | 0.20   |
| 61       | 0.25          | 0.30     | 0.91           | 0.90      | 0.17        | 0.20   |
| 62       | 0.26          | 0.30     | 0.91           | 0.90      | 0.18        | 0.20   |
| 63       | 0.27          | 0.31     | 0.90           | 0.89      | 0.19        | 0.21   |

Continued on next page

| $\alpha$ | $\phi_S^\ell$ | $\phi_S$ | $\varphi^\ell$ | $\varphi$ | $\psi^\ell$ | $\psi$ |
|----------|---------------|----------|----------------|-----------|-------------|--------|
| 64       | 0.29          | 0.32     | 0.90           | 0.89      | 0.20        | 0.22   |
| 65       | 0.31          | 0.34     | 0.89           | 0.88      | 0.21        | 0.23   |
| 66       | 0.34          | 0.37     | 0.89           | 0.87      | 0.23        | 0.26   |
| 67       | 0.40          | 0.43     | 0.87           | 0.85      | 0.27        | 0.30   |
| 68       | 0.50          | 0.52     | 0.81           | 0.81      | 0.35        | 0.36   |
| 69       | 0.57          | 0.58     | 0.79           | 0.78      | 0.40        | 0.41   |
| 70       | 0.60          | 0.59     | 0.78           | 0.77      | 0.42        | 0.42   |
| 71       | 0.60          | 0.60     | 0.78           | 0.77      | 0.42        | 0.42   |
| 72       | 0.59          | 0.59     | 0.79           | 0.78      | 0.41        | 0.41   |
| 73       | 0.59          | 0.59     | 0.79           | 0.78      | 0.41        | 0.41   |
| 74       | 0.58          | 0.58     | 0.80           | 0.79      | 0.40        | 0.40   |
| 75       | 0.58          | 0.58     | 0.81           | 0.79      | 0.40        | 0.40   |
| 76       | 0.57          | 0.57     | 0.81           | 0.80      | 0.39        | 0.39   |
| 77       | 0.56          | 0.56     | 0.82           | 0.80      | 0.38        | 0.39   |
| 78       | 0.55          | 0.55     | 0.82           | 0.81      | 0.38        | 0.38   |
| 79       | 0.54          | 0.54     | 0.83           | 0.81      | 0.37        | 0.37   |
| 80       | 0.53          | 0.53     | 0.84           | 0.82      | 0.36        | 0.37   |
| 81       | 0.52          | 0.52     | 0.84           | 0.83      | 0.35        | 0.36   |
| 82       | 0.51          | 0.51     | 0.85           | 0.83      | 0.34        | 0.35   |
| 83       | 0.50          | 0.50     | 0.86           | 0.84      | 0.34        | 0.34   |
| 84       | 0.48          | 0.49     | 0.87           | 0.85      | 0.32        | 0.33   |
| 85       | 0.47          | 0.48     | 0.88           | 0.86      | 0.31        | 0.32   |
| 86       | 0.45          | 0.46     | 0.88           | 0.87      | 0.30        | 0.31   |
| 87       | 0.43          | 0.44     | 0.89           | 0.87      | 0.29        | 0.30   |
| 88       | 0.41          | 0.42     | 0.91           | 0.88      | 0.27        | 0.28   |
| 89       | 0.38          | 0.40     | 0.92           | 0.90      | 0.25        | 0.27   |
| 90       | 0.08          | 0.13     | 0.99           | 0.97      | 0.05        | 0.08   |

Table S58: Reference ( $\phi_S$ ,  $\varphi$ ,  $\psi$ ) and approached ( $\phi_S^\ell$ ,  $\varphi^\ell$ ,  $\psi^\ell$ ) values of the topological descriptors for the first excited-state of the pyridinium-phenolate (PP), computed at the B3LYP/6-311G level of theory.  $\alpha$  is the pyridinium-phenolate central twist angle amplitude.

| $\alpha$ | $\phi_S^\ell$ | $\phi_S$ | $\varphi^\ell$ | $\varphi$ | $\psi^\ell$ | $\psi$ |
|----------|---------------|----------|----------------|-----------|-------------|--------|
| 0        | 0.41          | 0.31     | 0.83           | 0.87      | 0.29        | 0.22   |
| 1        | 0.41          | 0.31     | 0.83           | 0.87      | 0.29        | 0.22   |
| 2        | 0.41          | 0.31     | 0.83           | 0.87      | 0.29        | 0.22   |
| 3        | 0.41          | 0.31     | 0.84           | 0.87      | 0.29        | 0.22   |
| 4        | 0.41          | 0.31     | 0.84           | 0.87      | 0.29        | 0.22   |
| 5        | 0.40          | 0.31     | 0.84           | 0.87      | 0.28        | 0.22   |
| 6        | 0.40          | 0.31     | 0.84           | 0.87      | 0.28        | 0.22   |
| 7        | 0.40          | 0.31     | 0.84           | 0.87      | 0.28        | 0.22   |
| 8        | 0.40          | 0.32     | 0.85           | 0.87      | 0.28        | 0.22   |
| 9        | 0.39          | 0.32     | 0.85           | 0.87      | 0.27        | 0.22   |
| 10       | 0.39          | 0.32     | 0.85           | 0.87      | 0.27        | 0.22   |
| 11       | 0.39          | 0.32     | 0.85           | 0.87      | 0.27        | 0.22   |
| 12       | 0.38          | 0.32     | 0.85           | 0.87      | 0.27        | 0.22   |
| 13       | 0.38          | 0.32     | 0.85           | 0.87      | 0.27        | 0.22   |
| 14       | 0.37          | 0.32     | 0.86           | 0.87      | 0.26        | 0.22   |
| 15       | 0.37          | 0.32     | 0.86           | 0.87      | 0.26        | 0.22   |
| 16       | 0.36          | 0.32     | 0.86           | 0.87      | 0.25        | 0.22   |
| 17       | 0.36          | 0.32     | 0.86           | 0.87      | 0.25        | 0.22   |
| 18       | 0.35          | 0.33     | 0.87           | 0.87      | 0.24        | 0.23   |
| 19       | 0.34          | 0.33     | 0.87           | 0.87      | 0.24        | 0.23   |
| 20       | 0.34          | 0.33     | 0.87           | 0.87      | 0.24        | 0.23   |
| 21       | 0.33          | 0.33     | 0.87           | 0.87      | 0.23        | 0.23   |
| 22       | 0.32          | 0.33     | 0.87           | 0.87      | 0.22        | 0.23   |
| 23       | 0.32          | 0.33     | 0.88           | 0.87      | 0.22        | 0.23   |
| 24       | 0.31          | 0.33     | 0.88           | 0.87      | 0.22        | 0.23   |
| 25       | 0.30          | 0.33     | 0.88           | 0.87      | 0.21        | 0.23   |
| 26       | 0.29          | 0.33     | 0.88           | 0.87      | 0.20        | 0.23   |
| 27       | 0.29          | 0.33     | 0.88           | 0.87      | 0.20        | 0.23   |
| 28       | 0.28          | 0.33     | 0.88           | 0.87      | 0.20        | 0.23   |
| 29       | 0.27          | 0.33     | 0.89           | 0.87      | 0.19        | 0.23   |
| 30       | 0.27          | 0.33     | 0.89           | 0.87      | 0.19        | 0.23   |
| 31       | 0.26          | 0.33     | 0.89           | 0.87      | 0.18        | 0.23   |

Continued on next page



| $\alpha$ | $\phi_S^\ell$ | $\phi_S$ | $\varphi^\ell$ | $\varphi$ | $\psi^\ell$ | $\psi$ |
|----------|---------------|----------|----------------|-----------|-------------|--------|
| 32       | 0.25          | 0.33     | 0.90           | 0.87      | 0.17        | 0.23   |
| 33       | 0.24          | 0.33     | 0.90           | 0.87      | 0.17        | 0.23   |
| 34       | 0.24          | 0.33     | 0.91           | 0.87      | 0.16        | 0.23   |
| 35       | 0.23          | 0.33     | 0.91           | 0.88      | 0.16        | 0.23   |
| 36       | 0.22          | 0.33     | 0.92           | 0.88      | 0.15        | 0.23   |
| 37       | 0.21          | 0.33     | 0.93           | 0.88      | 0.14        | 0.23   |
| 38       | 0.21          | 0.33     | 0.93           | 0.88      | 0.14        | 0.23   |
| 39       | 0.20          | 0.33     | 0.93           | 0.88      | 0.13        | 0.23   |
| 40       | 0.19          | 0.33     | 0.94           | 0.88      | 0.13        | 0.23   |
| 41       | 0.19          | 0.33     | 0.94           | 0.88      | 0.13        | 0.23   |
| 42       | 0.18          | 0.32     | 0.94           | 0.88      | 0.12        | 0.22   |
| 43       | 0.17          | 0.33     | 0.94           | 0.88      | 0.11        | 0.23   |
| 44       | 0.17          | 0.33     | 0.95           | 0.88      | 0.11        | 0.23   |
| 45       | 0.17          | 0.33     | 0.95           | 0.88      | 0.11        | 0.23   |
| 46       | 0.17          | 0.33     | 0.95           | 0.88      | 0.11        | 0.23   |
| 47       | 0.17          | 0.33     | 0.94           | 0.88      | 0.11        | 0.23   |
| 48       | 0.18          | 0.33     | 0.94           | 0.88      | 0.12        | 0.23   |
| 49       | 0.19          | 0.33     | 0.94           | 0.88      | 0.13        | 0.23   |
| 50       | 0.19          | 0.33     | 0.94           | 0.88      | 0.13        | 0.23   |
| 51       | 0.21          | 0.33     | 0.93           | 0.88      | 0.14        | 0.23   |
| 52       | 0.22          | 0.34     | 0.92           | 0.88      | 0.15        | 0.23   |
| 53       | 0.23          | 0.35     | 0.92           | 0.88      | 0.16        | 0.24   |
| 54       | 0.25          | 0.36     | 0.92           | 0.88      | 0.17        | 0.25   |
| 55       | 0.28          | 0.37     | 0.91           | 0.87      | 0.19        | 0.26   |
| 56       | 0.32          | 0.40     | 0.90           | 0.86      | 0.22        | 0.28   |
| 57       | 0.37          | 0.43     | 0.87           | 0.84      | 0.26        | 0.30   |
| 58       | 0.44          | 0.48     | 0.83           | 0.82      | 0.31        | 0.34   |
| 59       | 0.51          | 0.54     | 0.80           | 0.79      | 0.36        | 0.38   |
| 60       | 0.57          | 0.59     | 0.78           | 0.77      | 0.40        | 0.42   |
| 61       | 0.60          | 0.61     | 0.77           | 0.76      | 0.42        | 0.43   |
| 62       | 0.60          | 0.61     | 0.77           | 0.76      | 0.42        | 0.43   |
| 63       | 0.61          | 0.61     | 0.77           | 0.76      | 0.43        | 0.43   |

Continued on next page

| $\alpha$ | $\phi_S^\ell$ | $\phi_S$ | $\varphi^\ell$ | $\varphi$ | $\psi^\ell$ | $\psi$ |
|----------|---------------|----------|----------------|-----------|-------------|--------|
| 64       | 0.60          | 0.61     | 0.78           | 0.76      | 0.42        | 0.43   |
| 65       | 0.60          | 0.61     | 0.78           | 0.76      | 0.42        | 0.43   |
| 66       | 0.59          | 0.60     | 0.78           | 0.77      | 0.41        | 0.42   |
| 67       | 0.59          | 0.60     | 0.79           | 0.77      | 0.41        | 0.42   |
| 68       | 0.58          | 0.59     | 0.79           | 0.78      | 0.40        | 0.41   |
| 69       | 0.58          | 0.59     | 0.80           | 0.78      | 0.40        | 0.41   |
| 70       | 0.57          | 0.58     | 0.80           | 0.79      | 0.39        | 0.40   |
| 71       | 0.57          | 0.57     | 0.81           | 0.79      | 0.39        | 0.40   |
| 72       | 0.56          | 0.57     | 0.81           | 0.80      | 0.39        | 0.39   |
| 73       | 0.55          | 0.56     | 0.82           | 0.80      | 0.38        | 0.39   |
| 74       | 0.54          | 0.55     | 0.82           | 0.81      | 0.37        | 0.38   |
| 75       | 0.53          | 0.54     | 0.83           | 0.81      | 0.36        | 0.37   |
| 76       | 0.53          | 0.53     | 0.83           | 0.82      | 0.36        | 0.37   |
| 77       | 0.52          | 0.52     | 0.84           | 0.82      | 0.35        | 0.36   |
| 78       | 0.51          | 0.51     | 0.85           | 0.83      | 0.34        | 0.35   |
| 79       | 0.50          | 0.50     | 0.85           | 0.84      | 0.34        | 0.34   |
| 80       | 0.48          | 0.49     | 0.86           | 0.84      | 0.32        | 0.34   |
| 81       | 0.47          | 0.48     | 0.87           | 0.85      | 0.32        | 0.33   |
| 82       | 0.46          | 0.47     | 0.87           | 0.86      | 0.31        | 0.32   |
| 83       | 0.44          | 0.45     | 0.88           | 0.87      | 0.30        | 0.30   |
| 84       | 0.43          | 0.44     | 0.89           | 0.87      | 0.29        | 0.30   |
| 85       | 0.41          | 0.42     | 0.90           | 0.88      | 0.27        | 0.28   |
| 86       | 0.38          | 0.40     | 0.91           | 0.89      | 0.25        | 0.27   |
| 87       | 0.36          | 0.37     | 0.92           | 0.90      | 0.24        | 0.25   |
| 88       | 0.32          | 0.34     | 0.93           | 0.91      | 0.21        | 0.23   |
| 89       | 0.28          | 0.30     | 0.95           | 0.93      | 0.18        | 0.20   |
| 90       | 0.12          | 0.15     | 0.98           | 0.96      | 0.08        | 0.10   |

Table S59: Reference ( $\phi_S$ ,  $\varphi$ ,  $\psi$ ) and approached ( $\phi_S^\ell$ ,  $\varphi^\ell$ ,  $\psi^\ell$ ) values of the topological descriptors for the first excited-state of the pyridinium-phenolate (PP), computed at the B3LYP/6-31++G(2d,p) level of theory.  $\alpha$  is the pyridinium-phenolate central twist angle amplitude.

| $\alpha$ | $\phi_S^\ell$ | $\phi_S$ | $\varphi^\ell$ | $\varphi$ | $\psi^\ell$ | $\psi$ |
|----------|---------------|----------|----------------|-----------|-------------|--------|
| 0        | 0.40          | 0.31     | 0.84           | 0.87      | 0.28        | 0.22   |
| 1        | 0.40          | 0.31     | 0.84           | 0.87      | 0.28        | 0.22   |
| 2        | 0.40          | 0.31     | 0.84           | 0.87      | 0.28        | 0.22   |
| 3        | 0.40          | 0.31     | 0.84           | 0.87      | 0.28        | 0.22   |
| 4        | 0.40          | 0.31     | 0.84           | 0.87      | 0.28        | 0.22   |
| 5        | 0.40          | 0.31     | 0.84           | 0.87      | 0.28        | 0.22   |
| 6        | 0.40          | 0.31     | 0.84           | 0.87      | 0.28        | 0.22   |
| 7        | 0.39          | 0.32     | 0.85           | 0.87      | 0.27        | 0.22   |
| 8        | 0.39          | 0.32     | 0.85           | 0.87      | 0.27        | 0.22   |
| 9        | 0.39          | 0.32     | 0.85           | 0.87      | 0.27        | 0.22   |
| 10       | 0.38          | 0.32     | 0.85           | 0.87      | 0.27        | 0.22   |
| 11       | 0.38          | 0.32     | 0.85           | 0.87      | 0.27        | 0.22   |
| 12       | 0.37          | 0.32     | 0.85           | 0.87      | 0.26        | 0.22   |
| 13       | 0.37          | 0.32     | 0.86           | 0.87      | 0.26        | 0.22   |
| 14       | 0.37          | 0.32     | 0.86           | 0.87      | 0.26        | 0.22   |
| 15       | 0.36          | 0.32     | 0.86           | 0.87      | 0.25        | 0.22   |
| 16       | 0.35          | 0.32     | 0.86           | 0.87      | 0.25        | 0.22   |
| 17       | 0.35          | 0.33     | 0.87           | 0.87      | 0.24        | 0.23   |
| 18       | 0.34          | 0.33     | 0.87           | 0.87      | 0.24        | 0.23   |
| 19       | 0.34          | 0.33     | 0.87           | 0.87      | 0.24        | 0.23   |
| 20       | 0.33          | 0.33     | 0.87           | 0.87      | 0.23        | 0.23   |
| 21       | 0.32          | 0.33     | 0.88           | 0.87      | 0.22        | 0.23   |
| 22       | 0.32          | 0.33     | 0.88           | 0.87      | 0.22        | 0.23   |
| 23       | 0.31          | 0.33     | 0.88           | 0.87      | 0.22        | 0.23   |
| 24       | 0.30          | 0.33     | 0.88           | 0.87      | 0.21        | 0.23   |
| 25       | 0.30          | 0.33     | 0.88           | 0.87      | 0.21        | 0.23   |
| 26       | 0.29          | 0.33     | 0.88           | 0.87      | 0.20        | 0.23   |
| 27       | 0.28          | 0.33     | 0.89           | 0.87      | 0.19        | 0.23   |
| 28       | 0.27          | 0.33     | 0.89           | 0.87      | 0.19        | 0.23   |
| 29       | 0.27          | 0.33     | 0.89           | 0.87      | 0.19        | 0.23   |
| 30       | 0.26          | 0.33     | 0.89           | 0.87      | 0.18        | 0.23   |
| 31       | 0.25          | 0.33     | 0.89           | 0.87      | 0.17        | 0.23   |

Continued on next page

| $\alpha$ | $\phi_S^\ell$ | $\phi_S$ | $\varphi^\ell$ | $\varphi$ | $\psi^\ell$ | $\psi$ |
|----------|---------------|----------|----------------|-----------|-------------|--------|
| 32       | 0.25          | 0.33     | 0.90           | 0.87      | 0.17        | 0.23   |
| 33       | 0.24          | 0.33     | 0.90           | 0.87      | 0.17        | 0.23   |
| 34       | 0.23          | 0.33     | 0.91           | 0.87      | 0.16        | 0.23   |
| 35       | 0.23          | 0.33     | 0.92           | 0.87      | 0.16        | 0.23   |
| 36       | 0.22          | 0.33     | 0.92           | 0.88      | 0.15        | 0.23   |
| 37       | 0.21          | 0.33     | 0.93           | 0.88      | 0.14        | 0.23   |
| 38       | 0.20          | 0.33     | 0.93           | 0.88      | 0.13        | 0.23   |
| 39       | 0.20          | 0.33     | 0.93           | 0.88      | 0.13        | 0.23   |
| 40       | 0.19          | 0.33     | 0.94           | 0.88      | 0.13        | 0.23   |
| 41       | 0.18          | 0.33     | 0.94           | 0.88      | 0.12        | 0.23   |
| 42       | 0.18          | 0.33     | 0.94           | 0.88      | 0.12        | 0.23   |
| 43       | 0.18          | 0.33     | 0.94           | 0.88      | 0.12        | 0.23   |
| 44       | 0.17          | 0.33     | 0.95           | 0.88      | 0.11        | 0.23   |
| 45       | 0.17          | 0.33     | 0.95           | 0.88      | 0.11        | 0.23   |
| 46       | 0.17          | 0.33     | 0.94           | 0.88      | 0.11        | 0.23   |
| 47       | 0.18          | 0.33     | 0.94           | 0.88      | 0.12        | 0.23   |
| 48       | 0.18          | 0.33     | 0.94           | 0.88      | 0.12        | 0.23   |
| 49       | 0.19          | 0.33     | 0.94           | 0.88      | 0.13        | 0.23   |
| 50       | 0.20          | 0.33     | 0.93           | 0.88      | 0.13        | 0.23   |
| 51       | 0.21          | 0.34     | 0.93           | 0.88      | 0.14        | 0.23   |
| 52       | 0.22          | 0.34     | 0.92           | 0.88      | 0.15        | 0.23   |
| 53       | 0.24          | 0.35     | 0.92           | 0.88      | 0.16        | 0.24   |
| 54       | 0.26          | 0.36     | 0.91           | 0.87      | 0.18        | 0.25   |
| 55       | 0.28          | 0.37     | 0.91           | 0.87      | 0.19        | 0.26   |
| 56       | 0.32          | 0.39     | 0.90           | 0.86      | 0.22        | 0.27   |
| 57       | 0.36          | 0.43     | 0.88           | 0.85      | 0.25        | 0.30   |
| 58       | 0.43          | 0.47     | 0.84           | 0.82      | 0.30        | 0.33   |
| 59       | 0.50          | 0.53     | 0.80           | 0.80      | 0.36        | 0.37   |
| 60       | 0.56          | 0.58     | 0.78           | 0.77      | 0.40        | 0.41   |
| 61       | 0.60          | 0.60     | 0.77           | 0.76      | 0.42        | 0.43   |
| 62       | 0.61          | 0.61     | 0.76           | 0.76      | 0.43        | 0.43   |
| 63       | 0.61          | 0.61     | 0.77           | 0.76      | 0.43        | 0.43   |

Continued on next page

| $\alpha$ | $\phi_S^\ell$ | $\phi_S$ | $\varphi^\ell$ | $\varphi$ | $\psi^\ell$ | $\psi$ |
|----------|---------------|----------|----------------|-----------|-------------|--------|
| 64       | 0.61          | 0.61     | 0.77           | 0.76      | 0.43        | 0.43   |
| 65       | 0.61          | 0.61     | 0.77           | 0.76      | 0.43        | 0.43   |
| 66       | 0.60          | 0.61     | 0.78           | 0.77      | 0.42        | 0.43   |
| 67       | 0.60          | 0.60     | 0.78           | 0.77      | 0.42        | 0.42   |
| 68       | 0.59          | 0.59     | 0.79           | 0.78      | 0.41        | 0.41   |
| 69       | 0.59          | 0.59     | 0.79           | 0.78      | 0.41        | 0.41   |
| 70       | 0.58          | 0.58     | 0.80           | 0.78      | 0.40        | 0.41   |
| 71       | 0.57          | 0.58     | 0.80           | 0.79      | 0.39        | 0.40   |
| 72       | 0.57          | 0.57     | 0.81           | 0.79      | 0.39        | 0.40   |
| 73       | 0.56          | 0.56     | 0.81           | 0.80      | 0.39        | 0.39   |
| 74       | 0.55          | 0.55     | 0.82           | 0.81      | 0.38        | 0.38   |
| 75       | 0.54          | 0.55     | 0.82           | 0.81      | 0.37        | 0.38   |
| 76       | 0.53          | 0.54     | 0.83           | 0.82      | 0.36        | 0.37   |
| 77       | 0.52          | 0.53     | 0.84           | 0.82      | 0.35        | 0.37   |
| 78       | 0.51          | 0.52     | 0.84           | 0.83      | 0.35        | 0.36   |
| 79       | 0.50          | 0.51     | 0.85           | 0.84      | 0.34        | 0.35   |
| 80       | 0.49          | 0.50     | 0.86           | 0.84      | 0.33        | 0.34   |
| 81       | 0.48          | 0.49     | 0.86           | 0.85      | 0.32        | 0.33   |
| 82       | 0.46          | 0.47     | 0.87           | 0.86      | 0.31        | 0.32   |
| 83       | 0.45          | 0.46     | 0.88           | 0.86      | 0.30        | 0.31   |
| 84       | 0.43          | 0.44     | 0.89           | 0.87      | 0.29        | 0.30   |
| 85       | 0.41          | 0.42     | 0.90           | 0.88      | 0.27        | 0.28   |
| 86       | 0.39          | 0.40     | 0.91           | 0.89      | 0.26        | 0.27   |
| 87       | 0.36          | 0.38     | 0.92           | 0.90      | 0.24        | 0.25   |
| 88       | 0.33          | 0.35     | 0.93           | 0.91      | 0.22        | 0.23   |
| 89       | 0.29          | 0.31     | 0.94           | 0.93      | 0.19        | 0.20   |
| 90       | 0.11          | 0.14     | 0.98           | 0.96      | 0.07        | 0.09   |

Table S60: Reference ( $\phi_S$ ,  $\varphi$ ,  $\psi$ ) and approached ( $\phi_S^\ell$ ,  $\varphi^\ell$ ,  $\psi^\ell$ ) values of the topological descriptors for the first excited-state of the pyridinium-phenolate (PP), computed at the B3LYP/6-31++G(d,p) level of theory.  $\alpha$  is the pyridinium-phenolate central twist angle amplitude.

| $\alpha$ | $\phi_S^\ell$ | $\phi_S$ | $\varphi^\ell$ | $\varphi$ | $\psi^\ell$ | $\psi$ |
|----------|---------------|----------|----------------|-----------|-------------|--------|
| 0        | 0.40          | 0.31     | 0.84           | 0.87      | 0.28        | 0.22   |
| 1        | 0.40          | 0.31     | 0.84           | 0.87      | 0.28        | 0.22   |
| 2        | 0.40          | 0.31     | 0.84           | 0.87      | 0.28        | 0.22   |
| 3        | 0.40          | 0.31     | 0.84           | 0.87      | 0.28        | 0.22   |
| 4        | 0.40          | 0.31     | 0.84           | 0.87      | 0.28        | 0.22   |
| 5        | 0.40          | 0.31     | 0.84           | 0.87      | 0.28        | 0.22   |
| 6        | 0.40          | 0.31     | 0.84           | 0.87      | 0.28        | 0.22   |
| 7        | 0.39          | 0.32     | 0.85           | 0.87      | 0.27        | 0.22   |
| 8        | 0.39          | 0.32     | 0.85           | 0.87      | 0.27        | 0.22   |
| 9        | 0.39          | 0.32     | 0.85           | 0.87      | 0.27        | 0.22   |
| 10       | 0.38          | 0.32     | 0.85           | 0.87      | 0.27        | 0.22   |
| 11       | 0.38          | 0.32     | 0.85           | 0.87      | 0.27        | 0.22   |
| 12       | 0.37          | 0.32     | 0.85           | 0.87      | 0.26        | 0.22   |
| 13       | 0.37          | 0.32     | 0.86           | 0.87      | 0.26        | 0.22   |
| 14       | 0.37          | 0.32     | 0.86           | 0.87      | 0.26        | 0.22   |
| 15       | 0.36          | 0.32     | 0.86           | 0.87      | 0.25        | 0.22   |
| 16       | 0.35          | 0.32     | 0.86           | 0.87      | 0.25        | 0.22   |
| 17       | 0.35          | 0.33     | 0.87           | 0.87      | 0.24        | 0.23   |
| 18       | 0.34          | 0.33     | 0.87           | 0.87      | 0.24        | 0.23   |
| 19       | 0.34          | 0.33     | 0.87           | 0.87      | 0.24        | 0.23   |
| 20       | 0.33          | 0.33     | 0.87           | 0.87      | 0.23        | 0.23   |
| 21       | 0.32          | 0.33     | 0.88           | 0.87      | 0.22        | 0.23   |
| 22       | 0.32          | 0.33     | 0.88           | 0.87      | 0.22        | 0.23   |
| 23       | 0.31          | 0.33     | 0.88           | 0.87      | 0.22        | 0.23   |
| 24       | 0.30          | 0.33     | 0.88           | 0.87      | 0.21        | 0.23   |
| 25       | 0.30          | 0.33     | 0.88           | 0.87      | 0.21        | 0.23   |
| 26       | 0.29          | 0.33     | 0.88           | 0.87      | 0.20        | 0.23   |
| 27       | 0.28          | 0.33     | 0.89           | 0.87      | 0.19        | 0.23   |
| 28       | 0.27          | 0.33     | 0.89           | 0.87      | 0.19        | 0.23   |
| 29       | 0.27          | 0.33     | 0.89           | 0.87      | 0.19        | 0.23   |
| 30       | 0.26          | 0.33     | 0.89           | 0.87      | 0.18        | 0.23   |
| 31       | 0.25          | 0.33     | 0.89           | 0.87      | 0.17        | 0.23   |

Continued on next page

| $\alpha$ | $\phi_S^\ell$ | $\phi_S$ | $\varphi^\ell$ | $\varphi$ | $\psi^\ell$ | $\psi$ |
|----------|---------------|----------|----------------|-----------|-------------|--------|
| 32       | 0.25          | 0.33     | 0.90           | 0.87      | 0.17        | 0.23   |
| 33       | 0.24          | 0.33     | 0.90           | 0.87      | 0.17        | 0.23   |
| 34       | 0.23          | 0.33     | 0.91           | 0.87      | 0.16        | 0.23   |
| 35       | 0.22          | 0.33     | 0.92           | 0.87      | 0.15        | 0.23   |
| 36       | 0.22          | 0.33     | 0.92           | 0.88      | 0.15        | 0.23   |
| 37       | 0.21          | 0.33     | 0.93           | 0.88      | 0.14        | 0.23   |
| 38       | 0.20          | 0.33     | 0.93           | 0.88      | 0.13        | 0.23   |
| 39       | 0.20          | 0.33     | 0.93           | 0.88      | 0.13        | 0.23   |
| 40       | 0.19          | 0.33     | 0.94           | 0.88      | 0.13        | 0.23   |
| 41       | 0.18          | 0.33     | 0.94           | 0.88      | 0.12        | 0.23   |
| 42       | 0.18          | 0.33     | 0.94           | 0.88      | 0.12        | 0.23   |
| 43       | 0.18          | 0.33     | 0.94           | 0.88      | 0.12        | 0.23   |
| 44       | 0.17          | 0.33     | 0.95           | 0.88      | 0.11        | 0.23   |
| 45       | 0.17          | 0.33     | 0.95           | 0.88      | 0.11        | 0.23   |
| 46       | 0.17          | 0.33     | 0.94           | 0.88      | 0.11        | 0.23   |
| 47       | 0.18          | 0.33     | 0.94           | 0.88      | 0.12        | 0.23   |
| 48       | 0.18          | 0.33     | 0.94           | 0.88      | 0.12        | 0.23   |
| 49       | 0.19          | 0.33     | 0.94           | 0.88      | 0.13        | 0.23   |
| 50       | 0.20          | 0.33     | 0.93           | 0.88      | 0.13        | 0.23   |
| 51       | 0.21          | 0.34     | 0.93           | 0.88      | 0.14        | 0.23   |
| 52       | 0.22          | 0.34     | 0.92           | 0.88      | 0.15        | 0.23   |
| 53       | 0.24          | 0.35     | 0.92           | 0.88      | 0.16        | 0.24   |
| 54       | 0.26          | 0.36     | 0.91           | 0.87      | 0.18        | 0.25   |
| 55       | 0.28          | 0.37     | 0.91           | 0.87      | 0.19        | 0.26   |
| 56       | 0.32          | 0.40     | 0.90           | 0.86      | 0.22        | 0.28   |
| 57       | 0.36          | 0.43     | 0.87           | 0.85      | 0.25        | 0.30   |
| 58       | 0.43          | 0.47     | 0.83           | 0.82      | 0.30        | 0.33   |
| 59       | 0.50          | 0.53     | 0.80           | 0.80      | 0.36        | 0.37   |
| 60       | 0.56          | 0.58     | 0.78           | 0.77      | 0.40        | 0.41   |
| 61       | 0.60          | 0.60     | 0.77           | 0.76      | 0.42        | 0.43   |
| 62       | 0.61          | 0.61     | 0.76           | 0.75      | 0.43        | 0.43   |
| 63       | 0.61          | 0.61     | 0.77           | 0.76      | 0.43        | 0.43   |

Continued on next page

| $\alpha$ | $\phi_S^\ell$ | $\phi_S$ | $\varphi^\ell$ | $\varphi$ | $\psi^\ell$ | $\psi$ |
|----------|---------------|----------|----------------|-----------|-------------|--------|
| 64       | 0.61          | 0.61     | 0.77           | 0.76      | 0.43        | 0.43   |
| 65       | 0.61          | 0.61     | 0.77           | 0.76      | 0.43        | 0.43   |
| 66       | 0.60          | 0.61     | 0.78           | 0.77      | 0.42        | 0.43   |
| 67       | 0.60          | 0.60     | 0.78           | 0.77      | 0.42        | 0.42   |
| 68       | 0.59          | 0.59     | 0.79           | 0.78      | 0.41        | 0.41   |
| 69       | 0.59          | 0.59     | 0.79           | 0.78      | 0.41        | 0.41   |
| 70       | 0.58          | 0.58     | 0.80           | 0.78      | 0.40        | 0.41   |
| 71       | 0.57          | 0.58     | 0.80           | 0.79      | 0.39        | 0.40   |
| 72       | 0.57          | 0.57     | 0.81           | 0.79      | 0.39        | 0.40   |
| 73       | 0.56          | 0.56     | 0.81           | 0.80      | 0.39        | 0.39   |
| 74       | 0.55          | 0.55     | 0.82           | 0.81      | 0.38        | 0.38   |
| 75       | 0.54          | 0.55     | 0.82           | 0.81      | 0.37        | 0.38   |
| 76       | 0.53          | 0.54     | 0.83           | 0.82      | 0.36        | 0.37   |
| 77       | 0.52          | 0.53     | 0.84           | 0.82      | 0.35        | 0.37   |
| 78       | 0.51          | 0.52     | 0.84           | 0.83      | 0.35        | 0.36   |
| 79       | 0.50          | 0.51     | 0.85           | 0.84      | 0.34        | 0.35   |
| 80       | 0.49          | 0.50     | 0.86           | 0.84      | 0.33        | 0.34   |
| 81       | 0.48          | 0.49     | 0.86           | 0.85      | 0.32        | 0.33   |
| 82       | 0.46          | 0.47     | 0.87           | 0.86      | 0.31        | 0.32   |
| 83       | 0.45          | 0.46     | 0.88           | 0.86      | 0.30        | 0.31   |
| 84       | 0.43          | 0.44     | 0.89           | 0.87      | 0.29        | 0.30   |
| 85       | 0.41          | 0.42     | 0.90           | 0.88      | 0.27        | 0.28   |
| 86       | 0.39          | 0.40     | 0.91           | 0.89      | 0.26        | 0.27   |
| 87       | 0.36          | 0.38     | 0.92           | 0.90      | 0.24        | 0.25   |
| 88       | 0.33          | 0.35     | 0.93           | 0.91      | 0.22        | 0.23   |
| 89       | 0.29          | 0.31     | 0.94           | 0.93      | 0.19        | 0.20   |
| 90       | 0.11          | 0.14     | 0.98           | 0.96      | 0.07        | 0.09   |

Table S61: Reference ( $\phi_S$ ,  $\varphi$ ,  $\psi$ ) and approached ( $\phi_S^\ell$ ,  $\varphi^\ell$ ,  $\psi^\ell$ ) values of the topological descriptors for the first excited-state of the pyridinium-phenolate (PP), computed at the B3LYP/6-31+G(d,p) level of theory.  $\alpha$  is the pyridinium-phenolate central twist angle amplitude.



| $\alpha$ | $\phi_S^\ell$ | $\phi_S$ | $\varphi^\ell$ | $\varphi$ | $\psi^\ell$ | $\psi$ |
|----------|---------------|----------|----------------|-----------|-------------|--------|
| 0        | 0.40          | 0.31     | 0.84           | 0.87      | 0.28        | 0.22   |
| 1        | 0.40          | 0.31     | 0.84           | 0.87      | 0.28        | 0.22   |
| 2        | 0.40          | 0.31     | 0.84           | 0.87      | 0.28        | 0.22   |
| 3        | 0.40          | 0.31     | 0.84           | 0.87      | 0.28        | 0.22   |
| 4        | 0.40          | 0.31     | 0.84           | 0.87      | 0.28        | 0.22   |
| 5        | 0.40          | 0.31     | 0.84           | 0.87      | 0.28        | 0.22   |
| 6        | 0.39          | 0.31     | 0.84           | 0.87      | 0.28        | 0.22   |
| 7        | 0.39          | 0.31     | 0.85           | 0.87      | 0.27        | 0.22   |
| 8        | 0.39          | 0.31     | 0.85           | 0.87      | 0.27        | 0.22   |
| 9        | 0.39          | 0.32     | 0.85           | 0.87      | 0.27        | 0.22   |
| 10       | 0.38          | 0.32     | 0.85           | 0.87      | 0.27        | 0.22   |
| 11       | 0.38          | 0.32     | 0.85           | 0.87      | 0.27        | 0.22   |
| 12       | 0.37          | 0.32     | 0.86           | 0.87      | 0.26        | 0.22   |
| 13       | 0.37          | 0.32     | 0.86           | 0.87      | 0.26        | 0.22   |
| 14       | 0.36          | 0.32     | 0.86           | 0.87      | 0.25        | 0.22   |
| 15       | 0.36          | 0.32     | 0.86           | 0.87      | 0.25        | 0.22   |
| 16       | 0.35          | 0.32     | 0.86           | 0.87      | 0.25        | 0.22   |
| 17       | 0.35          | 0.32     | 0.87           | 0.87      | 0.24        | 0.22   |
| 18       | 0.34          | 0.32     | 0.87           | 0.87      | 0.24        | 0.22   |
| 19       | 0.34          | 0.32     | 0.87           | 0.87      | 0.24        | 0.22   |
| 20       | 0.33          | 0.33     | 0.87           | 0.87      | 0.23        | 0.23   |
| 21       | 0.32          | 0.33     | 0.88           | 0.87      | 0.22        | 0.23   |
| 22       | 0.32          | 0.33     | 0.88           | 0.87      | 0.22        | 0.23   |
| 23       | 0.31          | 0.33     | 0.88           | 0.87      | 0.22        | 0.23   |
| 24       | 0.30          | 0.33     | 0.88           | 0.87      | 0.21        | 0.23   |
| 25       | 0.29          | 0.33     | 0.88           | 0.87      | 0.20        | 0.23   |
| 26       | 0.29          | 0.33     | 0.89           | 0.87      | 0.20        | 0.23   |
| 27       | 0.28          | 0.33     | 0.89           | 0.87      | 0.19        | 0.23   |
| 28       | 0.27          | 0.33     | 0.89           | 0.87      | 0.19        | 0.23   |
| 29       | 0.26          | 0.33     | 0.89           | 0.87      | 0.18        | 0.23   |
| 30       | 0.26          | 0.33     | 0.89           | 0.87      | 0.18        | 0.23   |
| 31       | 0.25          | 0.33     | 0.89           | 0.87      | 0.17        | 0.23   |

Continued on next page

| $\alpha$ | $\phi_S^\ell$ | $\phi_S$ | $\varphi^\ell$ | $\varphi$ | $\psi^\ell$ | $\psi$ |
|----------|---------------|----------|----------------|-----------|-------------|--------|
| 32       | 0.24          | 0.33     | 0.90           | 0.87      | 0.17        | 0.23   |
| 33       | 0.24          | 0.33     | 0.91           | 0.87      | 0.16        | 0.23   |
| 34       | 0.23          | 0.33     | 0.91           | 0.87      | 0.16        | 0.23   |
| 35       | 0.22          | 0.33     | 0.92           | 0.88      | 0.15        | 0.23   |
| 36       | 0.22          | 0.33     | 0.92           | 0.88      | 0.15        | 0.23   |
| 37       | 0.21          | 0.33     | 0.93           | 0.88      | 0.14        | 0.23   |
| 38       | 0.20          | 0.33     | 0.93           | 0.88      | 0.13        | 0.23   |
| 39       | 0.20          | 0.33     | 0.94           | 0.88      | 0.13        | 0.23   |
| 40       | 0.19          | 0.32     | 0.94           | 0.88      | 0.13        | 0.22   |
| 41       | 0.18          | 0.32     | 0.94           | 0.88      | 0.12        | 0.22   |
| 42       | 0.18          | 0.32     | 0.94           | 0.88      | 0.12        | 0.22   |
| 43       | 0.17          | 0.32     | 0.95           | 0.88      | 0.11        | 0.22   |
| 44       | 0.17          | 0.32     | 0.95           | 0.88      | 0.11        | 0.22   |
| 45       | 0.17          | 0.33     | 0.95           | 0.88      | 0.11        | 0.23   |
| 46       | 0.17          | 0.33     | 0.95           | 0.88      | 0.11        | 0.23   |
| 47       | 0.18          | 0.33     | 0.94           | 0.88      | 0.12        | 0.23   |
| 48       | 0.18          | 0.33     | 0.94           | 0.88      | 0.12        | 0.23   |
| 49       | 0.19          | 0.33     | 0.94           | 0.88      | 0.13        | 0.23   |
| 50       | 0.20          | 0.33     | 0.93           | 0.88      | 0.13        | 0.23   |
| 51       | 0.21          | 0.34     | 0.93           | 0.88      | 0.14        | 0.23   |
| 52       | 0.22          | 0.34     | 0.92           | 0.88      | 0.15        | 0.23   |
| 53       | 0.24          | 0.35     | 0.92           | 0.88      | 0.16        | 0.24   |
| 54       | 0.26          | 0.36     | 0.91           | 0.87      | 0.18        | 0.25   |
| 55       | 0.29          | 0.38     | 0.91           | 0.87      | 0.20        | 0.26   |
| 56       | 0.33          | 0.40     | 0.89           | 0.86      | 0.23        | 0.28   |
| 57       | 0.38          | 0.44     | 0.87           | 0.84      | 0.26        | 0.31   |
| 58       | 0.45          | 0.49     | 0.82           | 0.82      | 0.32        | 0.34   |
| 59       | 0.52          | 0.54     | 0.79           | 0.79      | 0.37        | 0.38   |
| 60       | 0.57          | 0.59     | 0.78           | 0.77      | 0.40        | 0.42   |
| 61       | 0.60          | 0.61     | 0.76           | 0.76      | 0.43        | 0.43   |
| 62       | 0.61          | 0.61     | 0.76           | 0.75      | 0.43        | 0.43   |
| 63       | 0.61          | 0.62     | 0.77           | 0.76      | 0.43        | 0.44   |

Continued on next page

| $\alpha$ | $\phi_S^\ell$ | $\phi_S$ | $\varphi^\ell$ | $\varphi$ | $\psi^\ell$ | $\psi$ |
|----------|---------------|----------|----------------|-----------|-------------|--------|
| 64       | 0.61          | 0.61     | 0.77           | 0.76      | 0.43        | 0.43   |
| 65       | 0.61          | 0.61     | 0.77           | 0.76      | 0.43        | 0.43   |
| 66       | 0.60          | 0.60     | 0.78           | 0.77      | 0.42        | 0.42   |
| 67       | 0.60          | 0.60     | 0.78           | 0.77      | 0.42        | 0.42   |
| 68       | 0.59          | 0.59     | 0.79           | 0.78      | 0.41        | 0.41   |
| 69       | 0.58          | 0.59     | 0.79           | 0.78      | 0.40        | 0.41   |
| 70       | 0.58          | 0.58     | 0.80           | 0.79      | 0.40        | 0.40   |
| 71       | 0.57          | 0.57     | 0.80           | 0.79      | 0.39        | 0.40   |
| 72       | 0.56          | 0.57     | 0.81           | 0.80      | 0.39        | 0.39   |
| 73       | 0.56          | 0.56     | 0.81           | 0.80      | 0.39        | 0.39   |
| 74       | 0.55          | 0.55     | 0.82           | 0.81      | 0.38        | 0.38   |
| 75       | 0.54          | 0.54     | 0.82           | 0.81      | 0.37        | 0.37   |
| 76       | 0.53          | 0.54     | 0.83           | 0.82      | 0.36        | 0.37   |
| 77       | 0.52          | 0.53     | 0.84           | 0.82      | 0.35        | 0.37   |
| 78       | 0.51          | 0.52     | 0.84           | 0.83      | 0.35        | 0.36   |
| 79       | 0.50          | 0.51     | 0.85           | 0.84      | 0.34        | 0.35   |
| 80       | 0.49          | 0.50     | 0.86           | 0.84      | 0.33        | 0.34   |
| 81       | 0.48          | 0.48     | 0.86           | 0.85      | 0.32        | 0.33   |
| 82       | 0.46          | 0.47     | 0.87           | 0.86      | 0.31        | 0.32   |
| 83       | 0.45          | 0.46     | 0.88           | 0.86      | 0.30        | 0.31   |
| 84       | 0.43          | 0.44     | 0.89           | 0.87      | 0.29        | 0.30   |
| 85       | 0.41          | 0.42     | 0.90           | 0.88      | 0.27        | 0.28   |
| 86       | 0.39          | 0.40     | 0.91           | 0.89      | 0.26        | 0.27   |
| 87       | 0.36          | 0.38     | 0.92           | 0.90      | 0.24        | 0.25   |
| 88       | 0.33          | 0.35     | 0.93           | 0.91      | 0.22        | 0.23   |
| 89       | 0.28          | 0.31     | 0.95           | 0.93      | 0.18        | 0.20   |
| 90       | 0.11          | 0.14     | 0.98           | 0.96      | 0.07        | 0.09   |

Table S62: Reference ( $\phi_S$ ,  $\varphi$ ,  $\psi$ ) and approached ( $\phi_S^\ell$ ,  $\varphi^\ell$ ,  $\psi^\ell$ ) values of the topological descriptors for the first excited-state of the pyridinium-phenolate (PP), computed at the B3LYP/6-31+G(d) level of theory.  $\alpha$  is the pyridinium-phenolate central twist angle amplitude.

| $\alpha$ | $\phi_S^\ell$ | $\phi_S$ | $\varphi^\ell$ | $\varphi$ | $\psi^\ell$ | $\psi$ |
|----------|---------------|----------|----------------|-----------|-------------|--------|
| 0        | 0.42          | 0.31     | 0.83           | 0.86      | 0.30        | 0.22   |
| 1        | 0.42          | 0.31     | 0.83           | 0.86      | 0.30        | 0.22   |
| 2        | 0.41          | 0.31     | 0.83           | 0.86      | 0.29        | 0.22   |
| 3        | 0.41          | 0.31     | 0.83           | 0.86      | 0.29        | 0.22   |
| 4        | 0.41          | 0.32     | 0.83           | 0.86      | 0.29        | 0.23   |
| 5        | 0.41          | 0.32     | 0.84           | 0.86      | 0.29        | 0.23   |
| 6        | 0.41          | 0.32     | 0.84           | 0.86      | 0.29        | 0.23   |
| 7        | 0.40          | 0.32     | 0.84           | 0.86      | 0.28        | 0.23   |
| 8        | 0.40          | 0.32     | 0.84           | 0.86      | 0.28        | 0.23   |
| 9        | 0.39          | 0.32     | 0.84           | 0.86      | 0.28        | 0.23   |
| 10       | 0.39          | 0.32     | 0.84           | 0.86      | 0.28        | 0.23   |
| 11       | 0.38          | 0.32     | 0.85           | 0.86      | 0.27        | 0.23   |
| 12       | 0.38          | 0.32     | 0.85           | 0.86      | 0.27        | 0.23   |
| 13       | 0.37          | 0.32     | 0.85           | 0.87      | 0.26        | 0.22   |
| 14       | 0.37          | 0.32     | 0.85           | 0.87      | 0.26        | 0.22   |
| 15       | 0.36          | 0.32     | 0.85           | 0.87      | 0.26        | 0.22   |
| 16       | 0.35          | 0.32     | 0.86           | 0.87      | 0.25        | 0.22   |
| 17       | 0.35          | 0.32     | 0.86           | 0.87      | 0.25        | 0.22   |
| 18       | 0.34          | 0.32     | 0.86           | 0.87      | 0.24        | 0.22   |
| 19       | 0.33          | 0.32     | 0.86           | 0.87      | 0.23        | 0.22   |
| 20       | 0.32          | 0.32     | 0.87           | 0.87      | 0.22        | 0.22   |
| 21       | 0.31          | 0.32     | 0.87           | 0.87      | 0.22        | 0.22   |
| 22       | 0.30          | 0.32     | 0.87           | 0.87      | 0.21        | 0.22   |
| 23       | 0.30          | 0.31     | 0.87           | 0.87      | 0.21        | 0.22   |
| 24       | 0.29          | 0.31     | 0.88           | 0.87      | 0.20        | 0.22   |
| 25       | 0.28          | 0.31     | 0.88           | 0.87      | 0.20        | 0.22   |
| 26       | 0.27          | 0.31     | 0.88           | 0.87      | 0.19        | 0.22   |
| 27       | 0.26          | 0.31     | 0.88           | 0.87      | 0.18        | 0.22   |
| 28       | 0.25          | 0.31     | 0.89           | 0.87      | 0.17        | 0.22   |
| 29       | 0.24          | 0.31     | 0.90           | 0.87      | 0.17        | 0.22   |
| 30       | 0.23          | 0.31     | 0.91           | 0.87      | 0.16        | 0.22   |
| 31       | 0.22          | 0.31     | 0.92           | 0.87      | 0.15        | 0.22   |

Continued on next page

| $\alpha$ | $\phi_S^\ell$ | $\phi_S$ | $\varphi^\ell$ | $\varphi$ | $\psi^\ell$ | $\psi$ |
|----------|---------------|----------|----------------|-----------|-------------|--------|
| 32       | 0.21          | 0.31     | 0.92           | 0.88      | 0.14        | 0.22   |
| 33       | 0.20          | 0.31     | 0.93           | 0.88      | 0.13        | 0.22   |
| 34       | 0.19          | 0.30     | 0.94           | 0.88      | 0.13        | 0.21   |
| 35       | 0.18          | 0.30     | 0.95           | 0.88      | 0.12        | 0.21   |
| 36       | 0.17          | 0.30     | 0.95           | 0.88      | 0.11        | 0.21   |
| 37       | 0.16          | 0.30     | 0.96           | 0.88      | 0.11        | 0.21   |
| 38       | 0.15          | 0.30     | 0.97           | 0.88      | 0.10        | 0.21   |
| 39       | 0.14          | 0.30     | 0.97           | 0.88      | 0.09        | 0.21   |
| 40       | 0.13          | 0.30     | 0.97           | 0.88      | 0.08        | 0.21   |
| 41       | 0.12          | 0.29     | 0.98           | 0.88      | 0.08        | 0.20   |
| 42       | 0.11          | 0.29     | 0.98           | 0.89      | 0.07        | 0.20   |
| 43       | 0.10          | 0.29     | 0.98           | 0.89      | 0.06        | 0.20   |
| 44       | 0.09          | 0.29     | 0.99           | 0.89      | 0.06        | 0.20   |
| 45       | 0.09          | 0.29     | 0.99           | 0.89      | 0.06        | 0.20   |
| 46       | 0.08          | 0.28     | 0.99           | 0.89      | 0.05        | 0.19   |
| 47       | 0.09          | 0.28     | 0.99           | 0.89      | 0.06        | 0.19   |
| 48       | 0.09          | 0.28     | 0.99           | 0.89      | 0.06        | 0.19   |
| 49       | 0.10          | 0.28     | 0.98           | 0.89      | 0.06        | 0.19   |
| 50       | 0.11          | 0.27     | 0.98           | 0.89      | 0.07        | 0.19   |
| 51       | 0.12          | 0.27     | 0.98           | 0.90      | 0.08        | 0.19   |
| 52       | 0.13          | 0.27     | 0.98           | 0.90      | 0.08        | 0.19   |
| 53       | 0.14          | 0.27     | 0.97           | 0.90      | 0.09        | 0.19   |
| 54       | 0.15          | 0.26     | 0.97           | 0.90      | 0.10        | 0.18   |
| 55       | 0.16          | 0.26     | 0.96           | 0.90      | 0.11        | 0.18   |
| 56       | 0.17          | 0.26     | 0.95           | 0.90      | 0.11        | 0.18   |
| 57       | 0.18          | 0.25     | 0.95           | 0.90      | 0.12        | 0.17   |
| 58       | 0.19          | 0.25     | 0.94           | 0.91      | 0.13        | 0.17   |
| 59       | 0.19          | 0.25     | 0.93           | 0.91      | 0.13        | 0.17   |
| 60       | 0.20          | 0.24     | 0.92           | 0.91      | 0.14        | 0.16   |
| 61       | 0.21          | 0.24     | 0.92           | 0.91      | 0.14        | 0.16   |
| 62       | 0.21          | 0.24     | 0.92           | 0.91      | 0.14        | 0.16   |
| 63       | 0.22          | 0.23     | 0.92           | 0.91      | 0.15        | 0.16   |

Continued on next page

| $\alpha$ | $\phi_S^\ell$ | $\phi_S$ | $\varphi^\ell$ | $\varphi$ | $\psi^\ell$ | $\psi$ |
|----------|---------------|----------|----------------|-----------|-------------|--------|
| 64       | 0.22          | 0.23     | 0.92           | 0.91      | 0.15        | 0.16   |
| 65       | 0.23          | 0.22     | 0.92           | 0.92      | 0.16        | 0.15   |
| 66       | 0.23          | 0.22     | 0.92           | 0.92      | 0.16        | 0.15   |
| 67       | 0.24          | 0.22     | 0.92           | 0.92      | 0.16        | 0.15   |
| 68       | 0.26          | 0.23     | 0.92           | 0.92      | 0.18        | 0.16   |
| 69       | 0.29          | 0.25     | 0.92           | 0.92      | 0.19        | 0.17   |
| 70       | 0.34          | 0.30     | 0.90           | 0.90      | 0.23        | 0.20   |
| 71       | 0.47          | 0.42     | 0.85           | 0.86      | 0.32        | 0.29   |
| 72       | 0.56          | 0.54     | 0.80           | 0.80      | 0.39        | 0.38   |
| 73       | 0.58          | 0.57     | 0.80           | 0.79      | 0.40        | 0.40   |
| 74       | 0.58          | 0.58     | 0.79           | 0.79      | 0.40        | 0.40   |
| 75       | 0.58          | 0.57     | 0.80           | 0.79      | 0.40        | 0.40   |
| 76       | 0.57          | 0.57     | 0.80           | 0.79      | 0.39        | 0.40   |
| 77       | 0.56          | 0.56     | 0.81           | 0.80      | 0.39        | 0.39   |
| 78       | 0.56          | 0.56     | 0.81           | 0.80      | 0.39        | 0.39   |
| 79       | 0.55          | 0.55     | 0.82           | 0.81      | 0.38        | 0.38   |
| 80       | 0.54          | 0.54     | 0.83           | 0.81      | 0.37        | 0.37   |
| 81       | 0.53          | 0.53     | 0.83           | 0.82      | 0.36        | 0.37   |
| 82       | 0.52          | 0.52     | 0.84           | 0.83      | 0.35        | 0.36   |
| 83       | 0.51          | 0.51     | 0.85           | 0.83      | 0.34        | 0.35   |
| 84       | 0.49          | 0.50     | 0.86           | 0.84      | 0.33        | 0.34   |
| 85       | 0.48          | 0.49     | 0.86           | 0.85      | 0.32        | 0.33   |
| 86       | 0.46          | 0.47     | 0.87           | 0.86      | 0.31        | 0.32   |
| 87       | 0.45          | 0.45     | 0.88           | 0.87      | 0.30        | 0.30   |
| 88       | 0.43          | 0.43     | 0.89           | 0.88      | 0.29        | 0.29   |
| 89       | 0.40          | 0.41     | 0.90           | 0.89      | 0.27        | 0.27   |
| 90       | 0.11          | 0.15     | 0.98           | 0.96      | 0.07        | 0.10   |

Table S63: Reference ( $\phi_S$ ,  $\varphi$ ,  $\psi$ ) and approached ( $\phi_S^\ell$ ,  $\varphi^\ell$ ,  $\psi^\ell$ ) values of the topological descriptors for the first excited-state of the pyridinium-phenolate (PP), computed at the B3LYP/6-31G(d) level of theory.  $\alpha$  is the pyridinium-phenolate central twist angle amplitude.

| $\alpha$ | $\phi_S^\ell$ | $\phi_S$ | $\varphi^\ell$ | $\varphi$ | $\psi^\ell$ | $\psi$ |
|----------|---------------|----------|----------------|-----------|-------------|--------|
| 0        | 0.41          | 0.31     | 0.83           | 0.87      | 0.29        | 0.22   |
| 1        | 0.41          | 0.31     | 0.83           | 0.87      | 0.29        | 0.22   |
| 2        | 0.41          | 0.31     | 0.83           | 0.87      | 0.29        | 0.22   |
| 3        | 0.41          | 0.31     | 0.83           | 0.87      | 0.29        | 0.22   |
| 4        | 0.40          | 0.31     | 0.83           | 0.87      | 0.29        | 0.22   |
| 5        | 0.40          | 0.32     | 0.83           | 0.87      | 0.29        | 0.22   |
| 6        | 0.40          | 0.32     | 0.84           | 0.87      | 0.28        | 0.22   |
| 7        | 0.40          | 0.32     | 0.84           | 0.87      | 0.28        | 0.22   |
| 8        | 0.39          | 0.32     | 0.84           | 0.87      | 0.28        | 0.22   |
| 9        | 0.39          | 0.32     | 0.84           | 0.87      | 0.28        | 0.22   |
| 10       | 0.39          | 0.32     | 0.85           | 0.87      | 0.27        | 0.22   |
| 11       | 0.38          | 0.32     | 0.85           | 0.87      | 0.27        | 0.22   |
| 12       | 0.38          | 0.32     | 0.85           | 0.87      | 0.27        | 0.22   |
| 13       | 0.37          | 0.32     | 0.85           | 0.87      | 0.26        | 0.22   |
| 14       | 0.37          | 0.32     | 0.85           | 0.87      | 0.26        | 0.22   |
| 15       | 0.36          | 0.32     | 0.86           | 0.87      | 0.25        | 0.22   |
| 16       | 0.36          | 0.32     | 0.86           | 0.87      | 0.25        | 0.22   |
| 17       | 0.35          | 0.33     | 0.86           | 0.87      | 0.25        | 0.23   |
| 18       | 0.34          | 0.33     | 0.86           | 0.87      | 0.24        | 0.23   |
| 19       | 0.34          | 0.33     | 0.87           | 0.87      | 0.24        | 0.23   |
| 20       | 0.33          | 0.33     | 0.87           | 0.87      | 0.23        | 0.23   |
| 21       | 0.33          | 0.33     | 0.87           | 0.87      | 0.23        | 0.23   |
| 22       | 0.32          | 0.33     | 0.87           | 0.87      | 0.22        | 0.23   |
| 23       | 0.31          | 0.33     | 0.88           | 0.87      | 0.22        | 0.23   |
| 24       | 0.30          | 0.33     | 0.88           | 0.87      | 0.21        | 0.23   |
| 25       | 0.30          | 0.33     | 0.88           | 0.87      | 0.21        | 0.23   |
| 26       | 0.29          | 0.33     | 0.88           | 0.87      | 0.20        | 0.23   |
| 27       | 0.28          | 0.33     | 0.88           | 0.87      | 0.20        | 0.23   |
| 28       | 0.28          | 0.33     | 0.88           | 0.87      | 0.20        | 0.23   |
| 29       | 0.27          | 0.33     | 0.88           | 0.87      | 0.19        | 0.23   |
| 30       | 0.26          | 0.33     | 0.89           | 0.87      | 0.18        | 0.23   |
| 31       | 0.26          | 0.33     | 0.89           | 0.87      | 0.18        | 0.23   |

Continued on next page

| $\alpha$ | $\phi_S^\ell$ | $\phi_S$ | $\varphi^\ell$ | $\varphi$ | $\psi^\ell$ | $\psi$ |
|----------|---------------|----------|----------------|-----------|-------------|--------|
| 32       | 0.25          | 0.33     | 0.90           | 0.87      | 0.17        | 0.23   |
| 33       | 0.24          | 0.33     | 0.90           | 0.87      | 0.17        | 0.23   |
| 34       | 0.24          | 0.33     | 0.91           | 0.87      | 0.16        | 0.23   |
| 35       | 0.23          | 0.33     | 0.91           | 0.87      | 0.16        | 0.23   |
| 36       | 0.22          | 0.33     | 0.92           | 0.87      | 0.15        | 0.23   |
| 37       | 0.22          | 0.33     | 0.92           | 0.87      | 0.15        | 0.23   |
| 38       | 0.21          | 0.33     | 0.93           | 0.88      | 0.14        | 0.23   |
| 39       | 0.20          | 0.33     | 0.93           | 0.88      | 0.13        | 0.23   |
| 40       | 0.20          | 0.33     | 0.93           | 0.88      | 0.13        | 0.23   |
| 41       | 0.19          | 0.33     | 0.94           | 0.88      | 0.13        | 0.23   |
| 42       | 0.19          | 0.33     | 0.94           | 0.88      | 0.13        | 0.23   |
| 43       | 0.18          | 0.33     | 0.94           | 0.88      | 0.12        | 0.23   |
| 44       | 0.18          | 0.33     | 0.94           | 0.88      | 0.12        | 0.23   |
| 45       | 0.18          | 0.33     | 0.94           | 0.88      | 0.12        | 0.23   |
| 46       | 0.18          | 0.33     | 0.94           | 0.88      | 0.12        | 0.23   |
| 47       | 0.18          | 0.33     | 0.94           | 0.88      | 0.12        | 0.23   |
| 48       | 0.19          | 0.33     | 0.94           | 0.88      | 0.13        | 0.23   |
| 49       | 0.19          | 0.33     | 0.93           | 0.88      | 0.13        | 0.23   |
| 50       | 0.20          | 0.34     | 0.93           | 0.88      | 0.13        | 0.23   |
| 51       | 0.21          | 0.34     | 0.93           | 0.88      | 0.14        | 0.23   |
| 52       | 0.22          | 0.34     | 0.92           | 0.88      | 0.15        | 0.23   |
| 53       | 0.23          | 0.35     | 0.92           | 0.88      | 0.16        | 0.24   |
| 54       | 0.25          | 0.36     | 0.92           | 0.87      | 0.17        | 0.25   |
| 55       | 0.27          | 0.37     | 0.91           | 0.87      | 0.18        | 0.26   |
| 56       | 0.29          | 0.38     | 0.91           | 0.87      | 0.20        | 0.26   |
| 57       | 0.32          | 0.39     | 0.90           | 0.86      | 0.22        | 0.27   |
| 58       | 0.35          | 0.42     | 0.88           | 0.85      | 0.24        | 0.29   |
| 59       | 0.39          | 0.44     | 0.86           | 0.84      | 0.27        | 0.31   |
| 60       | 0.44          | 0.48     | 0.83           | 0.82      | 0.31        | 0.34   |
| 61       | 0.50          | 0.52     | 0.80           | 0.80      | 0.36        | 0.37   |
| 62       | 0.54          | 0.56     | 0.79           | 0.78      | 0.38        | 0.40   |
| 63       | 0.57          | 0.58     | 0.78           | 0.77      | 0.40        | 0.41   |

Continued on next page



| $\alpha$ | $\phi_S^\ell$ | $\phi_S$ | $\varphi^\ell$ | $\varphi$ | $\psi^\ell$ | $\psi$ |
|----------|---------------|----------|----------------|-----------|-------------|--------|
| 64       | 0.59          | 0.59     | 0.77           | 0.77      | 0.42        | 0.42   |
| 65       | 0.60          | 0.60     | 0.77           | 0.77      | 0.42        | 0.42   |
| 66       | 0.60          | 0.60     | 0.78           | 0.77      | 0.42        | 0.42   |
| 67       | 0.60          | 0.60     | 0.78           | 0.77      | 0.42        | 0.42   |
| 68       | 0.59          | 0.60     | 0.78           | 0.77      | 0.41        | 0.42   |
| 69       | 0.59          | 0.59     | 0.79           | 0.78      | 0.41        | 0.41   |
| 70       | 0.58          | 0.59     | 0.79           | 0.78      | 0.40        | 0.41   |
| 71       | 0.58          | 0.58     | 0.80           | 0.79      | 0.40        | 0.40   |
| 72       | 0.57          | 0.57     | 0.80           | 0.79      | 0.39        | 0.40   |
| 73       | 0.56          | 0.57     | 0.81           | 0.80      | 0.39        | 0.39   |
| 74       | 0.56          | 0.56     | 0.82           | 0.80      | 0.38        | 0.39   |
| 75       | 0.55          | 0.55     | 0.82           | 0.81      | 0.38        | 0.38   |
| 76       | 0.54          | 0.54     | 0.83           | 0.81      | 0.37        | 0.37   |
| 77       | 0.53          | 0.54     | 0.83           | 0.82      | 0.36        | 0.37   |
| 78       | 0.52          | 0.53     | 0.84           | 0.83      | 0.35        | 0.36   |
| 79       | 0.51          | 0.52     | 0.85           | 0.83      | 0.34        | 0.36   |
| 80       | 0.50          | 0.51     | 0.85           | 0.84      | 0.34        | 0.35   |
| 81       | 0.49          | 0.50     | 0.86           | 0.84      | 0.33        | 0.34   |
| 82       | 0.48          | 0.48     | 0.87           | 0.85      | 0.32        | 0.33   |
| 83       | 0.46          | 0.47     | 0.88           | 0.86      | 0.31        | 0.32   |
| 84       | 0.44          | 0.46     | 0.88           | 0.87      | 0.30        | 0.31   |
| 85       | 0.43          | 0.44     | 0.89           | 0.88      | 0.29        | 0.30   |
| 86       | 0.41          | 0.42     | 0.90           | 0.88      | 0.27        | 0.28   |
| 87       | 0.38          | 0.40     | 0.91           | 0.89      | 0.25        | 0.27   |
| 88       | 0.35          | 0.37     | 0.93           | 0.91      | 0.23        | 0.25   |
| 89       | 0.31          | 0.34     | 0.94           | 0.92      | 0.20        | 0.23   |
| 90       | 0.09          | 0.13     | 0.99           | 0.97      | 0.06        | 0.08   |

Table S64: Reference ( $\phi_S$ ,  $\varphi$ ,  $\psi$ ) and approached ( $\phi_S^\ell$ ,  $\varphi^\ell$ ,  $\psi^\ell$ ) values of the topological descriptors for the first excited-state of the pyridinium-phenolate (PP), computed at the B3LYP/6-31+G level of theory.  $\alpha$  is the pyridinium-phenolate central twist angle amplitude.

| $\alpha$ | $\phi_S^\ell$ | $\phi_S$ | $\varphi^\ell$ | $\varphi$ | $\psi^\ell$ | $\psi$ |
|----------|---------------|----------|----------------|-----------|-------------|--------|
| 0        | 0.42          | 0.32     | 0.83           | 0.86      | 0.30        | 0.23   |
| 1        | 0.42          | 0.32     | 0.83           | 0.86      | 0.30        | 0.23   |
| 2        | 0.42          | 0.32     | 0.83           | 0.86      | 0.30        | 0.23   |
| 3        | 0.42          | 0.32     | 0.83           | 0.86      | 0.30        | 0.23   |
| 4        | 0.42          | 0.32     | 0.83           | 0.86      | 0.30        | 0.23   |
| 5        | 0.41          | 0.32     | 0.83           | 0.86      | 0.29        | 0.23   |
| 6        | 0.41          | 0.32     | 0.83           | 0.86      | 0.29        | 0.23   |
| 7        | 0.41          | 0.32     | 0.83           | 0.86      | 0.29        | 0.23   |
| 8        | 0.40          | 0.32     | 0.83           | 0.86      | 0.29        | 0.23   |
| 9        | 0.40          | 0.32     | 0.83           | 0.86      | 0.29        | 0.23   |
| 10       | 0.39          | 0.32     | 0.84           | 0.86      | 0.28        | 0.23   |
| 11       | 0.39          | 0.32     | 0.84           | 0.86      | 0.28        | 0.23   |
| 12       | 0.38          | 0.32     | 0.84           | 0.86      | 0.27        | 0.23   |
| 13       | 0.38          | 0.32     | 0.84           | 0.86      | 0.27        | 0.23   |
| 14       | 0.37          | 0.32     | 0.85           | 0.86      | 0.26        | 0.23   |
| 15       | 0.37          | 0.32     | 0.85           | 0.86      | 0.26        | 0.23   |
| 16       | 0.36          | 0.32     | 0.85           | 0.86      | 0.26        | 0.23   |
| 17       | 0.35          | 0.32     | 0.85           | 0.86      | 0.25        | 0.23   |
| 18       | 0.34          | 0.32     | 0.86           | 0.87      | 0.24        | 0.22   |
| 19       | 0.34          | 0.32     | 0.86           | 0.87      | 0.24        | 0.22   |
| 20       | 0.33          | 0.32     | 0.86           | 0.87      | 0.23        | 0.22   |
| 21       | 0.32          | 0.32     | 0.86           | 0.87      | 0.23        | 0.22   |
| 22       | 0.31          | 0.32     | 0.87           | 0.87      | 0.22        | 0.22   |
| 23       | 0.30          | 0.32     | 0.87           | 0.87      | 0.21        | 0.22   |
| 24       | 0.29          | 0.32     | 0.87           | 0.87      | 0.20        | 0.22   |
| 25       | 0.28          | 0.32     | 0.87           | 0.87      | 0.20        | 0.22   |
| 26       | 0.27          | 0.32     | 0.88           | 0.87      | 0.19        | 0.22   |
| 27       | 0.26          | 0.32     | 0.88           | 0.87      | 0.18        | 0.22   |
| 28       | 0.25          | 0.32     | 0.89           | 0.87      | 0.17        | 0.22   |
| 29       | 0.24          | 0.31     | 0.89           | 0.87      | 0.17        | 0.22   |
| 30       | 0.23          | 0.31     | 0.90           | 0.87      | 0.16        | 0.22   |
| 31       | 0.22          | 0.31     | 0.91           | 0.87      | 0.15        | 0.22   |

Continued on next page

| $\alpha$ | $\phi_S^\ell$ | $\phi_S$ | $\varphi^\ell$ | $\varphi$ | $\psi^\ell$ | $\psi$ |
|----------|---------------|----------|----------------|-----------|-------------|--------|
| 32       | 0.21          | 0.31     | 0.92           | 0.87      | 0.14        | 0.22   |
| 33       | 0.20          | 0.31     | 0.93           | 0.87      | 0.13        | 0.22   |
| 34       | 0.19          | 0.31     | 0.94           | 0.87      | 0.13        | 0.22   |
| 35       | 0.19          | 0.31     | 0.94           | 0.88      | 0.13        | 0.22   |
| 36       | 0.18          | 0.31     | 0.95           | 0.88      | 0.12        | 0.22   |
| 37       | 0.17          | 0.31     | 0.95           | 0.88      | 0.11        | 0.22   |
| 38       | 0.16          | 0.31     | 0.96           | 0.88      | 0.11        | 0.22   |
| 39       | 0.15          | 0.30     | 0.97           | 0.88      | 0.10        | 0.21   |
| 40       | 0.14          | 0.30     | 0.97           | 0.88      | 0.09        | 0.21   |
| 41       | 0.13          | 0.30     | 0.97           | 0.88      | 0.08        | 0.21   |
| 42       | 0.12          | 0.30     | 0.98           | 0.88      | 0.08        | 0.21   |
| 43       | 0.11          | 0.30     | 0.98           | 0.88      | 0.07        | 0.21   |
| 44       | 0.10          | 0.30     | 0.98           | 0.88      | 0.06        | 0.21   |
| 45       | 0.10          | 0.29     | 0.98           | 0.89      | 0.06        | 0.20   |
| 46       | 0.10          | 0.29     | 0.98           | 0.89      | 0.06        | 0.20   |
| 47       | 0.10          | 0.29     | 0.98           | 0.89      | 0.06        | 0.20   |
| 48       | 0.10          | 0.29     | 0.98           | 0.89      | 0.06        | 0.20   |
| 49       | 0.11          | 0.29     | 0.98           | 0.89      | 0.07        | 0.20   |
| 50       | 0.12          | 0.28     | 0.98           | 0.89      | 0.08        | 0.19   |
| 51       | 0.13          | 0.28     | 0.98           | 0.89      | 0.08        | 0.19   |
| 52       | 0.14          | 0.28     | 0.97           | 0.89      | 0.09        | 0.19   |
| 53       | 0.15          | 0.28     | 0.97           | 0.90      | 0.10        | 0.19   |
| 54       | 0.16          | 0.28     | 0.96           | 0.90      | 0.11        | 0.19   |
| 55       | 0.17          | 0.27     | 0.96           | 0.90      | 0.11        | 0.19   |
| 56       | 0.18          | 0.27     | 0.95           | 0.90      | 0.12        | 0.19   |
| 57       | 0.19          | 0.27     | 0.95           | 0.90      | 0.13        | 0.19   |
| 58       | 0.20          | 0.27     | 0.94           | 0.90      | 0.13        | 0.19   |
| 59       | 0.20          | 0.27     | 0.93           | 0.90      | 0.13        | 0.19   |
| 60       | 0.21          | 0.26     | 0.93           | 0.90      | 0.14        | 0.18   |
| 61       | 0.22          | 0.26     | 0.92           | 0.91      | 0.15        | 0.18   |
| 62       | 0.23          | 0.26     | 0.91           | 0.91      | 0.16        | 0.18   |
| 63       | 0.23          | 0.26     | 0.90           | 0.91      | 0.16        | 0.18   |

Continued on next page

| $\alpha$ | $\phi_S^\ell$ | $\phi_S$ | $\varphi^\ell$ | $\varphi$ | $\psi^\ell$ | $\psi$ |
|----------|---------------|----------|----------------|-----------|-------------|--------|
| 64       | 0.24          | 0.26     | 0.90           | 0.91      | 0.17        | 0.18   |
| 65       | 0.25          | 0.25     | 0.90           | 0.91      | 0.17        | 0.17   |
| 66       | 0.25          | 0.25     | 0.90           | 0.91      | 0.17        | 0.17   |
| 67       | 0.26          | 0.25     | 0.90           | 0.91      | 0.18        | 0.17   |
| 68       | 0.27          | 0.25     | 0.90           | 0.91      | 0.19        | 0.17   |
| 69       | 0.27          | 0.25     | 0.90           | 0.91      | 0.19        | 0.17   |
| 70       | 0.28          | 0.25     | 0.90           | 0.91      | 0.19        | 0.17   |
| 71       | 0.30          | 0.27     | 0.89           | 0.91      | 0.21        | 0.18   |
| 72       | 0.34          | 0.32     | 0.88           | 0.90      | 0.23        | 0.22   |
| 73       | 0.59          | 0.59     | 0.79           | 0.78      | 0.41        | 0.41   |
| 74       | 0.60          | 0.60     | 0.79           | 0.78      | 0.41        | 0.42   |
| 75       | 0.59          | 0.59     | 0.79           | 0.78      | 0.41        | 0.41   |
| 76       | 0.59          | 0.58     | 0.80           | 0.79      | 0.40        | 0.40   |
| 77       | 0.58          | 0.58     | 0.80           | 0.79      | 0.40        | 0.40   |
| 78       | 0.57          | 0.57     | 0.81           | 0.80      | 0.39        | 0.39   |
| 79       | 0.56          | 0.56     | 0.82           | 0.80      | 0.38        | 0.39   |
| 80       | 0.55          | 0.55     | 0.82           | 0.81      | 0.38        | 0.38   |
| 81       | 0.54          | 0.54     | 0.83           | 0.82      | 0.37        | 0.37   |
| 82       | 0.53          | 0.53     | 0.84           | 0.82      | 0.36        | 0.37   |
| 83       | 0.52          | 0.52     | 0.84           | 0.83      | 0.35        | 0.36   |
| 84       | 0.51          | 0.51     | 0.85           | 0.84      | 0.34        | 0.35   |
| 85       | 0.49          | 0.50     | 0.86           | 0.84      | 0.33        | 0.34   |
| 86       | 0.48          | 0.49     | 0.87           | 0.85      | 0.32        | 0.33   |
| 87       | 0.46          | 0.47     | 0.88           | 0.86      | 0.31        | 0.32   |
| 88       | 0.44          | 0.45     | 0.89           | 0.87      | 0.29        | 0.30   |
| 89       | 0.42          | 0.43     | 0.90           | 0.88      | 0.28        | 0.29   |
| 90       | 0.09          | 0.14     | 0.99           | 0.97      | 0.06        | 0.09   |

Table S65: Reference ( $\phi_S$ ,  $\varphi$ ,  $\psi$ ) and approached ( $\phi_S^\ell$ ,  $\varphi^\ell$ ,  $\psi^\ell$ ) values of the topological descriptors for the first excited-state of the pyridinium-phenolate (PP), computed at the B3LYP/6-31G level of theory.  $\alpha$  is the pyridinium-phenolate central twist angle amplitude.

| $\alpha$ | $\phi_S^\ell$ | $\phi_S$ | $\varphi^\ell$ | $\varphi$ | $\psi^\ell$ | $\psi$ |
|----------|---------------|----------|----------------|-----------|-------------|--------|
| 0        | 0.71          | 0.74     | 0.63           | 0.60      | 0.54        | 0.57   |
| 1        | 0.71          | 0.74     | 0.64           | 0.60      | 0.53        | 0.57   |
| 2        | 0.71          | 0.74     | 0.64           | 0.60      | 0.53        | 0.57   |
| 3        | 0.71          | 0.74     | 0.64           | 0.60      | 0.53        | 0.57   |
| 4        | 0.70          | 0.73     | 0.64           | 0.61      | 0.53        | 0.56   |
| 5        | 0.70          | 0.73     | 0.64           | 0.61      | 0.53        | 0.56   |
| 6        | 0.70          | 0.73     | 0.64           | 0.61      | 0.53        | 0.56   |
| 7        | 0.70          | 0.73     | 0.64           | 0.61      | 0.53        | 0.56   |
| 8        | 0.70          | 0.73     | 0.64           | 0.61      | 0.53        | 0.56   |
| 9        | 0.70          | 0.72     | 0.65           | 0.61      | 0.52        | 0.55   |
| 10       | 0.69          | 0.72     | 0.65           | 0.62      | 0.52        | 0.55   |
| 11       | 0.69          | 0.72     | 0.65           | 0.62      | 0.52        | 0.55   |
| 12       | 0.69          | 0.72     | 0.66           | 0.62      | 0.51        | 0.55   |
| 13       | 0.69          | 0.72     | 0.66           | 0.62      | 0.51        | 0.55   |
| 14       | 0.69          | 0.72     | 0.66           | 0.62      | 0.51        | 0.55   |
| 15       | 0.69          | 0.72     | 0.66           | 0.63      | 0.51        | 0.54   |
| 16       | 0.69          | 0.71     | 0.66           | 0.63      | 0.51        | 0.54   |
| 17       | 0.69          | 0.71     | 0.66           | 0.63      | 0.51        | 0.54   |
| 18       | 0.69          | 0.71     | 0.67           | 0.63      | 0.51        | 0.54   |
| 19       | 0.69          | 0.71     | 0.67           | 0.63      | 0.51        | 0.54   |
| 20       | 0.69          | 0.71     | 0.67           | 0.64      | 0.51        | 0.53   |
| 21       | 0.69          | 0.71     | 0.67           | 0.64      | 0.51        | 0.53   |
| 22       | 0.68          | 0.71     | 0.67           | 0.64      | 0.50        | 0.53   |
| 23       | 0.68          | 0.71     | 0.67           | 0.64      | 0.50        | 0.53   |
| 24       | 0.68          | 0.70     | 0.67           | 0.64      | 0.50        | 0.53   |
| 25       | 0.68          | 0.70     | 0.68           | 0.65      | 0.50        | 0.52   |
| 26       | 0.68          | 0.70     | 0.68           | 0.65      | 0.50        | 0.52   |
| 27       | 0.68          | 0.70     | 0.68           | 0.65      | 0.50        | 0.52   |
| 28       | 0.68          | 0.70     | 0.68           | 0.65      | 0.50        | 0.52   |
| 29       | 0.68          | 0.70     | 0.68           | 0.66      | 0.50        | 0.52   |
| 30       | 0.68          | 0.70     | 0.68           | 0.66      | 0.50        | 0.52   |
| 31       | 0.68          | 0.69     | 0.69           | 0.66      | 0.50        | 0.51   |

Continued on next page

| $\alpha$ | $\phi_S^\ell$ | $\phi_S$ | $\varphi^\ell$ | $\varphi$ | $\psi^\ell$ | $\psi$ |
|----------|---------------|----------|----------------|-----------|-------------|--------|
| 32       | 0.68          | 0.69     | 0.69           | 0.67      | 0.50        | 0.51   |
| 33       | 0.67          | 0.69     | 0.69           | 0.67      | 0.49        | 0.51   |
| 34       | 0.67          | 0.69     | 0.69           | 0.67      | 0.49        | 0.51   |
| 35       | 0.67          | 0.69     | 0.70           | 0.68      | 0.49        | 0.50   |
| 36       | 0.67          | 0.68     | 0.70           | 0.68      | 0.49        | 0.50   |
| 37       | 0.67          | 0.68     | 0.70           | 0.68      | 0.49        | 0.50   |
| 38       | 0.66          | 0.68     | 0.71           | 0.69      | 0.48        | 0.50   |
| 39       | 0.66          | 0.67     | 0.71           | 0.69      | 0.48        | 0.49   |
| 40       | 0.66          | 0.67     | 0.71           | 0.69      | 0.48        | 0.49   |
| 41       | 0.66          | 0.67     | 0.72           | 0.70      | 0.47        | 0.49   |
| 42       | 0.65          | 0.67     | 0.72           | 0.70      | 0.47        | 0.49   |
| 43       | 0.65          | 0.66     | 0.73           | 0.71      | 0.46        | 0.48   |
| 44       | 0.65          | 0.66     | 0.73           | 0.71      | 0.46        | 0.48   |
| 45       | 0.64          | 0.65     | 0.73           | 0.71      | 0.46        | 0.47   |
| 46       | 0.64          | 0.65     | 0.74           | 0.72      | 0.45        | 0.47   |
| 47       | 0.64          | 0.65     | 0.74           | 0.72      | 0.45        | 0.47   |
| 48       | 0.63          | 0.64     | 0.75           | 0.73      | 0.44        | 0.46   |
| 49       | 0.63          | 0.64     | 0.75           | 0.73      | 0.44        | 0.46   |
| 50       | 0.62          | 0.63     | 0.76           | 0.74      | 0.44        | 0.45   |
| 51       | 0.62          | 0.63     | 0.76           | 0.74      | 0.44        | 0.45   |
| 52       | 0.61          | 0.62     | 0.76           | 0.74      | 0.43        | 0.44   |
| 53       | 0.61          | 0.62     | 0.77           | 0.75      | 0.43        | 0.44   |
| 54       | 0.60          | 0.61     | 0.77           | 0.75      | 0.42        | 0.43   |
| 55       | 0.60          | 0.61     | 0.78           | 0.76      | 0.42        | 0.43   |
| 56       | 0.59          | 0.60     | 0.78           | 0.76      | 0.41        | 0.43   |
| 57       | 0.59          | 0.60     | 0.79           | 0.77      | 0.41        | 0.42   |
| 58       | 0.58          | 0.59     | 0.79           | 0.77      | 0.40        | 0.42   |
| 59       | 0.58          | 0.59     | 0.80           | 0.78      | 0.40        | 0.41   |
| 60       | 0.57          | 0.58     | 0.80           | 0.78      | 0.39        | 0.41   |
| 61       | 0.56          | 0.57     | 0.81           | 0.79      | 0.39        | 0.40   |
| 62       | 0.55          | 0.57     | 0.81           | 0.79      | 0.38        | 0.40   |
| 63       | 0.55          | 0.56     | 0.82           | 0.80      | 0.38        | 0.39   |

Continued on next page

| $\alpha$ | $\phi_S^\ell$ | $\phi_S$ | $\varphi^\ell$ | $\varphi$ | $\psi^\ell$ | $\psi$ |
|----------|---------------|----------|----------------|-----------|-------------|--------|
| 64       | 0.54          | 0.55     | 0.83           | 0.80      | 0.37        | 0.38   |
| 65       | 0.53          | 0.54     | 0.83           | 0.81      | 0.36        | 0.37   |
| 66       | 0.52          | 0.54     | 0.84           | 0.82      | 0.35        | 0.37   |
| 67       | 0.51          | 0.53     | 0.84           | 0.82      | 0.35        | 0.37   |
| 68       | 0.50          | 0.52     | 0.85           | 0.83      | 0.34        | 0.36   |
| 69       | 0.50          | 0.51     | 0.86           | 0.83      | 0.34        | 0.35   |
| 70       | 0.48          | 0.50     | 0.86           | 0.84      | 0.32        | 0.34   |
| 71       | 0.47          | 0.49     | 0.87           | 0.85      | 0.32        | 0.33   |
| 72       | 0.46          | 0.48     | 0.87           | 0.85      | 0.31        | 0.33   |
| 73       | 0.45          | 0.47     | 0.88           | 0.86      | 0.30        | 0.32   |
| 74       | 0.44          | 0.46     | 0.89           | 0.86      | 0.29        | 0.31   |
| 75       | 0.42          | 0.44     | 0.89           | 0.87      | 0.28        | 0.30   |
| 76       | 0.41          | 0.43     | 0.90           | 0.88      | 0.27        | 0.29   |
| 77       | 0.39          | 0.42     | 0.91           | 0.88      | 0.26        | 0.28   |
| 78       | 0.38          | 0.40     | 0.92           | 0.89      | 0.25        | 0.27   |
| 79       | 0.36          | 0.39     | 0.92           | 0.90      | 0.24        | 0.26   |
| 80       | 0.34          | 0.37     | 0.93           | 0.90      | 0.22        | 0.25   |
| 81       | 0.32          | 0.35     | 0.94           | 0.91      | 0.21        | 0.23   |
| 82       | 0.30          | 0.33     | 0.95           | 0.92      | 0.19        | 0.22   |
| 83       | 0.27          | 0.31     | 0.95           | 0.93      | 0.18        | 0.20   |
| 84       | 0.25          | 0.29     | 0.96           | 0.93      | 0.16        | 0.19   |
| 85       | 0.22          | 0.26     | 0.97           | 0.94      | 0.14        | 0.17   |
| 86       | 0.18          | 0.24     | 0.98           | 0.95      | 0.12        | 0.16   |
| 87       | 0.15          | 0.21     | 0.98           | 0.95      | 0.10        | 0.14   |
| 88       | 0.12          | 0.18     | 0.99           | 0.96      | 0.08        | 0.12   |
| 89       | 0.10          | 0.16     | 0.99           | 0.96      | 0.06        | 0.11   |
| 90       | 0.09          | 0.15     | 0.99           | 0.96      | 0.06        | 0.10   |

Table S66: Reference ( $\phi_S$ ,  $\varphi$ ,  $\psi$ ) and approached ( $\phi_S^\ell$ ,  $\varphi^\ell$ ,  $\psi^\ell$ ) values of the topological descriptors for the first excited-state of the pyridinium-phenolate (PP), computed at the CAM-B3LYP/3-21G level of theory.  $\alpha$  is the pyridinium-phenolate central twist angle amplitude.

| $\alpha$ | $\phi_S^\ell$ | $\phi_S$ | $\varphi^\ell$ | $\varphi$ | $\psi^\ell$ | $\psi$ |
|----------|---------------|----------|----------------|-----------|-------------|--------|
| 0        | 0.66          | 0.70     | 0.66           | 0.63      | 0.50        | 0.53   |
| 1        | 0.66          | 0.70     | 0.66           | 0.63      | 0.50        | 0.53   |
| 2        | 0.66          | 0.70     | 0.66           | 0.63      | 0.50        | 0.53   |
| 3        | 0.66          | 0.70     | 0.66           | 0.63      | 0.50        | 0.53   |
| 4        | 0.66          | 0.70     | 0.66           | 0.63      | 0.50        | 0.53   |
| 5        | 0.66          | 0.70     | 0.67           | 0.63      | 0.50        | 0.53   |
| 6        | 0.66          | 0.70     | 0.67           | 0.63      | 0.50        | 0.53   |
| 7        | 0.66          | 0.70     | 0.67           | 0.63      | 0.50        | 0.53   |
| 8        | 0.66          | 0.70     | 0.67           | 0.64      | 0.50        | 0.53   |
| 9        | 0.66          | 0.70     | 0.67           | 0.64      | 0.50        | 0.53   |
| 10       | 0.66          | 0.70     | 0.67           | 0.64      | 0.50        | 0.53   |
| 11       | 0.65          | 0.70     | 0.67           | 0.64      | 0.49        | 0.53   |
| 12       | 0.65          | 0.70     | 0.67           | 0.64      | 0.49        | 0.53   |
| 13       | 0.65          | 0.70     | 0.67           | 0.64      | 0.49        | 0.53   |
| 14       | 0.65          | 0.69     | 0.68           | 0.64      | 0.49        | 0.52   |
| 15       | 0.65          | 0.69     | 0.68           | 0.65      | 0.49        | 0.52   |
| 16       | 0.65          | 0.69     | 0.68           | 0.65      | 0.49        | 0.52   |
| 17       | 0.65          | 0.69     | 0.68           | 0.65      | 0.49        | 0.52   |
| 18       | 0.65          | 0.69     | 0.68           | 0.65      | 0.49        | 0.52   |
| 19       | 0.65          | 0.69     | 0.69           | 0.66      | 0.48        | 0.51   |
| 20       | 0.64          | 0.68     | 0.69           | 0.66      | 0.48        | 0.51   |
| 21       | 0.64          | 0.68     | 0.69           | 0.66      | 0.48        | 0.51   |
| 22       | 0.64          | 0.68     | 0.69           | 0.66      | 0.48        | 0.51   |
| 23       | 0.64          | 0.68     | 0.70           | 0.67      | 0.47        | 0.50   |
| 24       | 0.64          | 0.68     | 0.70           | 0.67      | 0.47        | 0.50   |
| 25       | 0.64          | 0.67     | 0.70           | 0.67      | 0.47        | 0.50   |
| 26       | 0.63          | 0.67     | 0.70           | 0.68      | 0.47        | 0.50   |
| 27       | 0.63          | 0.67     | 0.71           | 0.68      | 0.46        | 0.50   |
| 28       | 0.63          | 0.67     | 0.71           | 0.68      | 0.46        | 0.50   |
| 29       | 0.63          | 0.67     | 0.71           | 0.68      | 0.46        | 0.50   |
| 30       | 0.63          | 0.66     | 0.72           | 0.69      | 0.46        | 0.49   |
| 31       | 0.62          | 0.66     | 0.72           | 0.69      | 0.45        | 0.49   |

Continued on next page



| $\alpha$ | $\phi_S^\ell$ | $\phi_S$ | $\varphi^\ell$ | $\varphi$ | $\psi^\ell$ | $\psi$ |
|----------|---------------|----------|----------------|-----------|-------------|--------|
| 32       | 0.62          | 0.66     | 0.72           | 0.70      | 0.45        | 0.48   |
| 33       | 0.62          | 0.65     | 0.73           | 0.70      | 0.45        | 0.48   |
| 34       | 0.62          | 0.65     | 0.73           | 0.70      | 0.45        | 0.48   |
| 35       | 0.61          | 0.65     | 0.73           | 0.71      | 0.44        | 0.47   |
| 36       | 0.61          | 0.64     | 0.74           | 0.71      | 0.44        | 0.47   |
| 37       | 0.61          | 0.64     | 0.74           | 0.71      | 0.44        | 0.47   |
| 38       | 0.61          | 0.64     | 0.75           | 0.72      | 0.43        | 0.46   |
| 39       | 0.60          | 0.63     | 0.75           | 0.72      | 0.43        | 0.46   |
| 40       | 0.60          | 0.63     | 0.75           | 0.73      | 0.43        | 0.45   |
| 41       | 0.60          | 0.63     | 0.76           | 0.73      | 0.43        | 0.45   |
| 42       | 0.59          | 0.62     | 0.76           | 0.73      | 0.42        | 0.45   |
| 43       | 0.59          | 0.62     | 0.77           | 0.74      | 0.42        | 0.44   |
| 44       | 0.58          | 0.61     | 0.77           | 0.74      | 0.41        | 0.44   |
| 45       | 0.58          | 0.61     | 0.77           | 0.75      | 0.41        | 0.43   |
| 46       | 0.58          | 0.60     | 0.78           | 0.75      | 0.41        | 0.43   |
| 47       | 0.57          | 0.60     | 0.78           | 0.76      | 0.40        | 0.43   |
| 48       | 0.57          | 0.59     | 0.79           | 0.76      | 0.40        | 0.42   |
| 49       | 0.56          | 0.59     | 0.79           | 0.77      | 0.39        | 0.42   |
| 50       | 0.56          | 0.58     | 0.80           | 0.77      | 0.39        | 0.41   |
| 51       | 0.55          | 0.58     | 0.80           | 0.78      | 0.38        | 0.41   |
| 52       | 0.55          | 0.57     | 0.80           | 0.78      | 0.38        | 0.40   |
| 53       | 0.54          | 0.57     | 0.81           | 0.78      | 0.37        | 0.40   |
| 54       | 0.53          | 0.56     | 0.81           | 0.79      | 0.37        | 0.39   |
| 55       | 0.53          | 0.55     | 0.82           | 0.79      | 0.37        | 0.39   |
| 56       | 0.52          | 0.55     | 0.82           | 0.80      | 0.36        | 0.38   |
| 57       | 0.52          | 0.54     | 0.83           | 0.80      | 0.36        | 0.38   |
| 58       | 0.51          | 0.53     | 0.83           | 0.81      | 0.35        | 0.37   |
| 59       | 0.50          | 0.53     | 0.84           | 0.81      | 0.34        | 0.37   |
| 60       | 0.49          | 0.52     | 0.84           | 0.82      | 0.34        | 0.36   |
| 61       | 0.49          | 0.51     | 0.85           | 0.83      | 0.33        | 0.35   |
| 62       | 0.48          | 0.50     | 0.85           | 0.83      | 0.33        | 0.35   |
| 63       | 0.47          | 0.50     | 0.86           | 0.84      | 0.32        | 0.34   |

Continued on next page

| $\alpha$ | $\phi_S^\ell$ | $\phi_S$ | $\varphi^\ell$ | $\varphi$ | $\psi^\ell$ | $\psi$ |
|----------|---------------|----------|----------------|-----------|-------------|--------|
| 64       | 0.46          | 0.49     | 0.86           | 0.84      | 0.31        | 0.34   |
| 65       | 0.45          | 0.48     | 0.87           | 0.85      | 0.30        | 0.33   |
| 66       | 0.45          | 0.47     | 0.87           | 0.85      | 0.30        | 0.32   |
| 67       | 0.44          | 0.46     | 0.88           | 0.86      | 0.30        | 0.31   |
| 68       | 0.43          | 0.45     | 0.88           | 0.86      | 0.29        | 0.31   |
| 69       | 0.42          | 0.44     | 0.89           | 0.87      | 0.28        | 0.30   |
| 70       | 0.41          | 0.43     | 0.90           | 0.87      | 0.27        | 0.29   |
| 71       | 0.39          | 0.42     | 0.90           | 0.88      | 0.26        | 0.28   |
| 72       | 0.38          | 0.41     | 0.91           | 0.88      | 0.25        | 0.28   |
| 73       | 0.37          | 0.39     | 0.91           | 0.89      | 0.25        | 0.26   |
| 74       | 0.36          | 0.38     | 0.92           | 0.90      | 0.24        | 0.25   |
| 75       | 0.34          | 0.37     | 0.92           | 0.90      | 0.23        | 0.25   |
| 76       | 0.33          | 0.35     | 0.93           | 0.91      | 0.22        | 0.23   |
| 77       | 0.32          | 0.34     | 0.93           | 0.91      | 0.21        | 0.23   |
| 78       | 0.30          | 0.33     | 0.94           | 0.92      | 0.20        | 0.22   |
| 79       | 0.29          | 0.31     | 0.94           | 0.92      | 0.19        | 0.21   |
| 80       | 0.27          | 0.30     | 0.94           | 0.93      | 0.18        | 0.20   |
| 81       | 0.25          | 0.28     | 0.95           | 0.93      | 0.16        | 0.19   |
| 82       | 0.24          | 0.26     | 0.95           | 0.94      | 0.16        | 0.17   |
| 83       | 0.22          | 0.25     | 0.96           | 0.94      | 0.14        | 0.17   |
| 84       | 0.20          | 0.23     | 0.96           | 0.94      | 0.13        | 0.15   |
| 85       | 0.19          | 0.22     | 0.96           | 0.95      | 0.12        | 0.14   |
| 86       | 0.17          | 0.20     | 0.97           | 0.95      | 0.11        | 0.13   |
| 87       | 0.16          | 0.19     | 0.97           | 0.95      | 0.10        | 0.13   |
| 88       | 0.15          | 0.17     | 0.97           | 0.95      | 0.10        | 0.11   |
| 89       | 0.14          | 0.16     | 0.97           | 0.96      | 0.09        | 0.11   |
| 90       | 0.13          | 0.16     | 0.97           | 0.96      | 0.08        | 0.11   |

Table S67: Reference ( $\phi_S$ ,  $\varphi$ ,  $\psi$ ) and approached ( $\phi_S^\ell$ ,  $\varphi^\ell$ ,  $\psi^\ell$ ) values of the topological descriptors for the first excited-state of the pyridinium-phenolate (PP), computed at the CAM-B3LYP/6-311++G(2d,p) level of theory.  $\alpha$  is the pyridinium-phenolate central twist angle amplitude.

| $\alpha$ | $\phi_S^\ell$ | $\phi_S$ | $\varphi^\ell$ | $\varphi$ | $\psi^\ell$ | $\psi$ |
|----------|---------------|----------|----------------|-----------|-------------|--------|
| 0        | 0.66          | 0.71     | 0.66           | 0.63      | 0.50        | 0.54   |
| 1        | 0.66          | 0.71     | 0.66           | 0.63      | 0.50        | 0.54   |
| 2        | 0.66          | 0.71     | 0.66           | 0.63      | 0.50        | 0.54   |
| 3        | 0.66          | 0.71     | 0.66           | 0.63      | 0.50        | 0.54   |
| 4        | 0.66          | 0.71     | 0.66           | 0.63      | 0.50        | 0.54   |
| 5        | 0.66          | 0.71     | 0.66           | 0.63      | 0.50        | 0.54   |
| 6        | 0.66          | 0.71     | 0.66           | 0.63      | 0.50        | 0.54   |
| 7        | 0.66          | 0.70     | 0.66           | 0.63      | 0.50        | 0.53   |
| 8        | 0.66          | 0.70     | 0.67           | 0.63      | 0.50        | 0.53   |
| 9        | 0.66          | 0.70     | 0.67           | 0.63      | 0.50        | 0.53   |
| 10       | 0.65          | 0.70     | 0.67           | 0.64      | 0.49        | 0.53   |
| 11       | 0.65          | 0.70     | 0.67           | 0.64      | 0.49        | 0.53   |
| 12       | 0.65          | 0.70     | 0.67           | 0.64      | 0.49        | 0.53   |
| 13       | 0.65          | 0.70     | 0.67           | 0.64      | 0.49        | 0.53   |
| 14       | 0.65          | 0.70     | 0.67           | 0.64      | 0.49        | 0.53   |
| 15       | 0.65          | 0.70     | 0.67           | 0.64      | 0.49        | 0.53   |
| 16       | 0.65          | 0.69     | 0.68           | 0.65      | 0.49        | 0.52   |
| 17       | 0.65          | 0.69     | 0.68           | 0.65      | 0.49        | 0.52   |
| 18       | 0.65          | 0.69     | 0.68           | 0.65      | 0.49        | 0.52   |
| 19       | 0.65          | 0.69     | 0.68           | 0.65      | 0.49        | 0.52   |
| 20       | 0.64          | 0.69     | 0.69           | 0.66      | 0.48        | 0.51   |
| 21       | 0.64          | 0.69     | 0.69           | 0.66      | 0.48        | 0.51   |
| 22       | 0.64          | 0.68     | 0.69           | 0.66      | 0.48        | 0.51   |
| 23       | 0.64          | 0.68     | 0.69           | 0.66      | 0.48        | 0.51   |
| 24       | 0.64          | 0.68     | 0.70           | 0.67      | 0.47        | 0.50   |
| 25       | 0.64          | 0.68     | 0.70           | 0.67      | 0.47        | 0.50   |
| 26       | 0.64          | 0.67     | 0.70           | 0.67      | 0.47        | 0.50   |
| 27       | 0.63          | 0.67     | 0.70           | 0.68      | 0.47        | 0.50   |
| 28       | 0.63          | 0.67     | 0.71           | 0.68      | 0.46        | 0.50   |
| 29       | 0.63          | 0.67     | 0.71           | 0.68      | 0.46        | 0.50   |
| 30       | 0.63          | 0.66     | 0.71           | 0.69      | 0.46        | 0.49   |
| 31       | 0.63          | 0.66     | 0.72           | 0.69      | 0.46        | 0.49   |

Continued on next page

| $\alpha$ | $\phi_S^\ell$ | $\phi_S$ | $\varphi^\ell$ | $\varphi$ | $\psi^\ell$ | $\psi$ |
|----------|---------------|----------|----------------|-----------|-------------|--------|
| 32       | 0.63          | 0.66     | 0.72           | 0.69      | 0.46        | 0.49   |
| 33       | 0.62          | 0.66     | 0.72           | 0.70      | 0.45        | 0.48   |
| 34       | 0.62          | 0.65     | 0.73           | 0.70      | 0.45        | 0.48   |
| 35       | 0.62          | 0.65     | 0.73           | 0.70      | 0.45        | 0.48   |
| 36       | 0.62          | 0.65     | 0.73           | 0.71      | 0.45        | 0.47   |
| 37       | 0.61          | 0.64     | 0.74           | 0.71      | 0.44        | 0.47   |
| 38       | 0.61          | 0.64     | 0.74           | 0.72      | 0.44        | 0.46   |
| 39       | 0.61          | 0.64     | 0.75           | 0.72      | 0.43        | 0.46   |
| 40       | 0.60          | 0.63     | 0.75           | 0.72      | 0.43        | 0.46   |
| 41       | 0.60          | 0.63     | 0.75           | 0.73      | 0.43        | 0.45   |
| 42       | 0.60          | 0.62     | 0.76           | 0.73      | 0.43        | 0.45   |
| 43       | 0.59          | 0.62     | 0.76           | 0.74      | 0.42        | 0.44   |
| 44       | 0.59          | 0.62     | 0.77           | 0.74      | 0.42        | 0.44   |
| 45       | 0.58          | 0.61     | 0.77           | 0.75      | 0.41        | 0.43   |
| 46       | 0.58          | 0.61     | 0.78           | 0.75      | 0.41        | 0.43   |
| 47       | 0.58          | 0.60     | 0.78           | 0.76      | 0.41        | 0.43   |
| 48       | 0.57          | 0.60     | 0.78           | 0.76      | 0.40        | 0.43   |
| 49       | 0.57          | 0.59     | 0.79           | 0.76      | 0.40        | 0.42   |
| 50       | 0.56          | 0.59     | 0.79           | 0.77      | 0.39        | 0.42   |
| 51       | 0.56          | 0.58     | 0.80           | 0.77      | 0.39        | 0.41   |
| 52       | 0.55          | 0.57     | 0.80           | 0.78      | 0.38        | 0.40   |
| 53       | 0.54          | 0.57     | 0.81           | 0.78      | 0.37        | 0.40   |
| 54       | 0.54          | 0.56     | 0.81           | 0.79      | 0.37        | 0.39   |
| 55       | 0.53          | 0.56     | 0.82           | 0.79      | 0.37        | 0.39   |
| 56       | 0.53          | 0.55     | 0.82           | 0.80      | 0.37        | 0.38   |
| 57       | 0.52          | 0.54     | 0.83           | 0.80      | 0.36        | 0.38   |
| 58       | 0.51          | 0.54     | 0.83           | 0.81      | 0.35        | 0.37   |
| 59       | 0.51          | 0.53     | 0.84           | 0.81      | 0.35        | 0.37   |
| 60       | 0.50          | 0.52     | 0.84           | 0.82      | 0.34        | 0.36   |
| 61       | 0.49          | 0.51     | 0.85           | 0.82      | 0.33        | 0.35   |
| 62       | 0.48          | 0.51     | 0.85           | 0.83      | 0.33        | 0.35   |
| 63       | 0.47          | 0.50     | 0.86           | 0.83      | 0.32        | 0.35   |

Continued on next page

| $\alpha$ | $\phi_S^\ell$ | $\phi_S$ | $\varphi^\ell$ | $\varphi$ | $\psi^\ell$ | $\psi$ |
|----------|---------------|----------|----------------|-----------|-------------|--------|
| 64       | 0.46          | 0.49     | 0.86           | 0.84      | 0.31        | 0.34   |
| 65       | 0.46          | 0.48     | 0.87           | 0.85      | 0.31        | 0.33   |
| 66       | 0.45          | 0.47     | 0.87           | 0.85      | 0.30        | 0.32   |
| 67       | 0.44          | 0.46     | 0.88           | 0.86      | 0.30        | 0.31   |
| 68       | 0.43          | 0.45     | 0.89           | 0.86      | 0.29        | 0.31   |
| 69       | 0.42          | 0.44     | 0.89           | 0.87      | 0.28        | 0.30   |
| 70       | 0.40          | 0.43     | 0.90           | 0.87      | 0.27        | 0.29   |
| 71       | 0.39          | 0.42     | 0.90           | 0.88      | 0.26        | 0.28   |
| 72       | 0.38          | 0.41     | 0.91           | 0.88      | 0.25        | 0.28   |
| 73       | 0.37          | 0.40     | 0.91           | 0.89      | 0.25        | 0.27   |
| 74       | 0.35          | 0.38     | 0.92           | 0.89      | 0.23        | 0.26   |
| 75       | 0.34          | 0.37     | 0.93           | 0.90      | 0.22        | 0.25   |
| 76       | 0.33          | 0.36     | 0.93           | 0.91      | 0.22        | 0.24   |
| 77       | 0.31          | 0.34     | 0.94           | 0.91      | 0.20        | 0.23   |
| 78       | 0.29          | 0.33     | 0.94           | 0.92      | 0.19        | 0.22   |
| 79       | 0.28          | 0.31     | 0.95           | 0.92      | 0.18        | 0.21   |
| 80       | 0.26          | 0.30     | 0.95           | 0.93      | 0.17        | 0.20   |
| 81       | 0.24          | 0.28     | 0.96           | 0.93      | 0.16        | 0.19   |
| 82       | 0.23          | 0.27     | 0.96           | 0.94      | 0.15        | 0.18   |
| 83       | 0.21          | 0.25     | 0.97           | 0.94      | 0.14        | 0.17   |
| 84       | 0.19          | 0.23     | 0.97           | 0.94      | 0.12        | 0.15   |
| 85       | 0.18          | 0.22     | 0.97           | 0.95      | 0.12        | 0.14   |
| 86       | 0.16          | 0.20     | 0.98           | 0.95      | 0.10        | 0.13   |
| 87       | 0.15          | 0.19     | 0.98           | 0.95      | 0.10        | 0.13   |
| 88       | 0.13          | 0.17     | 0.98           | 0.95      | 0.08        | 0.11   |
| 89       | 0.12          | 0.16     | 0.98           | 0.96      | 0.08        | 0.11   |
| 90       | 0.12          | 0.16     | 0.98           | 0.96      | 0.08        | 0.11   |

Table S68: Reference ( $\phi_S$ ,  $\varphi$ ,  $\psi$ ) and approached ( $\phi_S^\ell$ ,  $\varphi^\ell$ ,  $\psi^\ell$ ) values of the topological descriptors for the first excited-state of the pyridinium-phenolate (PP), computed at the CAM-B3LYP/6-311++G(d,p) level of theory.  $\alpha$  is the pyridinium-phenolate central twist angle amplitude.

| $\alpha$ | $\phi_S^\ell$ | $\phi_S$ | $\varphi^\ell$ | $\varphi$ | $\psi^\ell$ | $\psi$ |
|----------|---------------|----------|----------------|-----------|-------------|--------|
| 0        | 0.66          | 0.71     | 0.66           | 0.63      | 0.50        | 0.54   |
| 1        | 0.66          | 0.71     | 0.66           | 0.63      | 0.50        | 0.54   |
| 2        | 0.66          | 0.71     | 0.66           | 0.63      | 0.50        | 0.54   |
| 3        | 0.66          | 0.71     | 0.66           | 0.63      | 0.50        | 0.54   |
| 4        | 0.66          | 0.71     | 0.66           | 0.63      | 0.50        | 0.54   |
| 5        | 0.66          | 0.71     | 0.66           | 0.63      | 0.50        | 0.54   |
| 6        | 0.66          | 0.71     | 0.66           | 0.63      | 0.50        | 0.54   |
| 7        | 0.66          | 0.70     | 0.66           | 0.63      | 0.50        | 0.53   |
| 8        | 0.66          | 0.70     | 0.67           | 0.63      | 0.50        | 0.53   |
| 9        | 0.66          | 0.70     | 0.67           | 0.63      | 0.50        | 0.53   |
| 10       | 0.65          | 0.70     | 0.67           | 0.64      | 0.49        | 0.53   |
| 11       | 0.65          | 0.70     | 0.67           | 0.64      | 0.49        | 0.53   |
| 12       | 0.65          | 0.70     | 0.67           | 0.64      | 0.49        | 0.53   |
| 13       | 0.65          | 0.70     | 0.67           | 0.64      | 0.49        | 0.53   |
| 14       | 0.65          | 0.70     | 0.67           | 0.64      | 0.49        | 0.53   |
| 15       | 0.65          | 0.70     | 0.67           | 0.64      | 0.49        | 0.53   |
| 16       | 0.65          | 0.69     | 0.68           | 0.65      | 0.49        | 0.52   |
| 17       | 0.65          | 0.69     | 0.68           | 0.65      | 0.49        | 0.52   |
| 18       | 0.65          | 0.69     | 0.68           | 0.65      | 0.49        | 0.52   |
| 19       | 0.65          | 0.69     | 0.68           | 0.65      | 0.49        | 0.52   |
| 20       | 0.64          | 0.69     | 0.69           | 0.66      | 0.48        | 0.51   |
| 21       | 0.64          | 0.69     | 0.69           | 0.66      | 0.48        | 0.51   |
| 22       | 0.64          | 0.68     | 0.69           | 0.66      | 0.48        | 0.51   |
| 23       | 0.64          | 0.68     | 0.69           | 0.66      | 0.48        | 0.51   |
| 24       | 0.64          | 0.68     | 0.70           | 0.67      | 0.47        | 0.50   |
| 25       | 0.64          | 0.68     | 0.70           | 0.67      | 0.47        | 0.50   |
| 26       | 0.64          | 0.67     | 0.70           | 0.67      | 0.47        | 0.50   |
| 27       | 0.63          | 0.67     | 0.70           | 0.68      | 0.47        | 0.50   |
| 28       | 0.63          | 0.67     | 0.71           | 0.68      | 0.46        | 0.50   |
| 29       | 0.63          | 0.67     | 0.71           | 0.68      | 0.46        | 0.50   |
| 30       | 0.63          | 0.66     | 0.71           | 0.69      | 0.46        | 0.49   |
| 31       | 0.63          | 0.66     | 0.72           | 0.69      | 0.46        | 0.49   |

Continued on next page

| $\alpha$ | $\phi_S^\ell$ | $\phi_S$ | $\varphi^\ell$ | $\varphi$ | $\psi^\ell$ | $\psi$ |
|----------|---------------|----------|----------------|-----------|-------------|--------|
| 32       | 0.63          | 0.66     | 0.72           | 0.69      | 0.46        | 0.49   |
| 33       | 0.62          | 0.66     | 0.72           | 0.70      | 0.45        | 0.48   |
| 34       | 0.62          | 0.65     | 0.73           | 0.70      | 0.45        | 0.48   |
| 35       | 0.62          | 0.65     | 0.73           | 0.70      | 0.45        | 0.48   |
| 36       | 0.62          | 0.65     | 0.73           | 0.71      | 0.45        | 0.47   |
| 37       | 0.61          | 0.64     | 0.74           | 0.71      | 0.44        | 0.47   |
| 38       | 0.61          | 0.64     | 0.74           | 0.72      | 0.44        | 0.46   |
| 39       | 0.61          | 0.64     | 0.75           | 0.72      | 0.43        | 0.46   |
| 40       | 0.60          | 0.63     | 0.75           | 0.72      | 0.43        | 0.46   |
| 41       | 0.60          | 0.63     | 0.75           | 0.73      | 0.43        | 0.45   |
| 42       | 0.60          | 0.62     | 0.76           | 0.73      | 0.43        | 0.45   |
| 43       | 0.59          | 0.62     | 0.76           | 0.74      | 0.42        | 0.44   |
| 44       | 0.59          | 0.62     | 0.77           | 0.74      | 0.42        | 0.44   |
| 45       | 0.58          | 0.61     | 0.77           | 0.75      | 0.41        | 0.43   |
| 46       | 0.58          | 0.61     | 0.78           | 0.75      | 0.41        | 0.43   |
| 47       | 0.57          | 0.60     | 0.78           | 0.76      | 0.40        | 0.43   |
| 48       | 0.57          | 0.60     | 0.78           | 0.76      | 0.40        | 0.43   |
| 49       | 0.57          | 0.59     | 0.79           | 0.76      | 0.40        | 0.42   |
| 50       | 0.56          | 0.59     | 0.79           | 0.77      | 0.39        | 0.42   |
| 51       | 0.56          | 0.58     | 0.80           | 0.77      | 0.39        | 0.41   |
| 52       | 0.55          | 0.57     | 0.80           | 0.78      | 0.38        | 0.40   |
| 53       | 0.54          | 0.57     | 0.81           | 0.78      | 0.37        | 0.40   |
| 54       | 0.54          | 0.56     | 0.81           | 0.79      | 0.37        | 0.39   |
| 55       | 0.53          | 0.56     | 0.82           | 0.79      | 0.37        | 0.39   |
| 56       | 0.53          | 0.55     | 0.82           | 0.80      | 0.37        | 0.38   |
| 57       | 0.52          | 0.54     | 0.83           | 0.80      | 0.36        | 0.38   |
| 58       | 0.51          | 0.54     | 0.83           | 0.81      | 0.35        | 0.37   |
| 59       | 0.51          | 0.53     | 0.84           | 0.81      | 0.35        | 0.37   |
| 60       | 0.50          | 0.52     | 0.84           | 0.82      | 0.34        | 0.36   |
| 61       | 0.49          | 0.51     | 0.85           | 0.82      | 0.33        | 0.35   |
| 62       | 0.48          | 0.51     | 0.85           | 0.83      | 0.33        | 0.35   |
| 63       | 0.47          | 0.50     | 0.86           | 0.83      | 0.32        | 0.35   |

Continued on next page

| $\alpha$ | $\phi_S^\ell$ | $\phi_S$ | $\varphi^\ell$ | $\varphi$ | $\psi^\ell$ | $\psi$ |
|----------|---------------|----------|----------------|-----------|-------------|--------|
| 64       | 0.46          | 0.49     | 0.86           | 0.84      | 0.31        | 0.34   |
| 65       | 0.46          | 0.48     | 0.87           | 0.85      | 0.31        | 0.33   |
| 66       | 0.45          | 0.47     | 0.87           | 0.85      | 0.30        | 0.32   |
| 67       | 0.44          | 0.46     | 0.88           | 0.86      | 0.30        | 0.31   |
| 68       | 0.43          | 0.45     | 0.89           | 0.86      | 0.29        | 0.31   |
| 69       | 0.42          | 0.44     | 0.89           | 0.87      | 0.28        | 0.30   |
| 70       | 0.40          | 0.43     | 0.90           | 0.87      | 0.27        | 0.29   |
| 71       | 0.39          | 0.42     | 0.90           | 0.88      | 0.26        | 0.28   |
| 72       | 0.38          | 0.41     | 0.91           | 0.88      | 0.25        | 0.28   |
| 73       | 0.37          | 0.40     | 0.91           | 0.89      | 0.25        | 0.27   |
| 74       | 0.35          | 0.38     | 0.92           | 0.89      | 0.23        | 0.26   |
| 75       | 0.34          | 0.37     | 0.93           | 0.90      | 0.22        | 0.25   |
| 76       | 0.33          | 0.36     | 0.93           | 0.91      | 0.22        | 0.24   |
| 77       | 0.31          | 0.34     | 0.94           | 0.91      | 0.20        | 0.23   |
| 78       | 0.30          | 0.33     | 0.94           | 0.92      | 0.20        | 0.22   |
| 79       | 0.28          | 0.31     | 0.95           | 0.92      | 0.18        | 0.21   |
| 80       | 0.26          | 0.30     | 0.95           | 0.93      | 0.17        | 0.20   |
| 81       | 0.24          | 0.28     | 0.96           | 0.93      | 0.16        | 0.19   |
| 82       | 0.23          | 0.27     | 0.96           | 0.94      | 0.15        | 0.18   |
| 83       | 0.21          | 0.25     | 0.97           | 0.94      | 0.14        | 0.17   |
| 84       | 0.19          | 0.23     | 0.97           | 0.94      | 0.12        | 0.15   |
| 85       | 0.18          | 0.22     | 0.97           | 0.95      | 0.12        | 0.14   |
| 86       | 0.16          | 0.20     | 0.98           | 0.95      | 0.10        | 0.13   |
| 87       | 0.15          | 0.19     | 0.98           | 0.95      | 0.10        | 0.13   |
| 88       | 0.13          | 0.17     | 0.98           | 0.95      | 0.08        | 0.11   |
| 89       | 0.12          | 0.16     | 0.98           | 0.96      | 0.08        | 0.11   |
| 90       | 0.12          | 0.16     | 0.98           | 0.96      | 0.08        | 0.11   |

Table S69: Reference ( $\phi_S$ ,  $\varphi$ ,  $\psi$ ) and approached ( $\phi_S^\ell$ ,  $\varphi^\ell$ ,  $\psi^\ell$ ) values of the topological descriptors for the first excited-state of the pyridinium-phenolate (PP), computed at the CAM-B3LYP/6-311+G(d,p) level of theory.  $\alpha$  is the pyridinium-phenolate central twist angle amplitude.



| $\alpha$ | $\phi_S^\ell$ | $\phi_S$ | $\varphi^\ell$ | $\varphi$ | $\psi^\ell$ | $\psi$ |
|----------|---------------|----------|----------------|-----------|-------------|--------|
| 0        | 0.66          | 0.71     | 0.66           | 0.63      | 0.50        | 0.54   |
| 1        | 0.66          | 0.71     | 0.66           | 0.63      | 0.50        | 0.54   |
| 2        | 0.66          | 0.71     | 0.66           | 0.63      | 0.50        | 0.54   |
| 3        | 0.66          | 0.71     | 0.66           | 0.63      | 0.50        | 0.54   |
| 4        | 0.66          | 0.71     | 0.66           | 0.63      | 0.50        | 0.54   |
| 5        | 0.66          | 0.71     | 0.66           | 0.63      | 0.50        | 0.54   |
| 6        | 0.66          | 0.70     | 0.66           | 0.63      | 0.50        | 0.53   |
| 7        | 0.66          | 0.70     | 0.67           | 0.63      | 0.50        | 0.53   |
| 8        | 0.66          | 0.70     | 0.67           | 0.63      | 0.50        | 0.53   |
| 9        | 0.65          | 0.70     | 0.67           | 0.64      | 0.49        | 0.53   |
| 10       | 0.65          | 0.70     | 0.67           | 0.64      | 0.49        | 0.53   |
| 11       | 0.65          | 0.70     | 0.67           | 0.64      | 0.49        | 0.53   |
| 12       | 0.65          | 0.70     | 0.67           | 0.64      | 0.49        | 0.53   |
| 13       | 0.65          | 0.70     | 0.67           | 0.64      | 0.49        | 0.53   |
| 14       | 0.65          | 0.70     | 0.67           | 0.64      | 0.49        | 0.53   |
| 15       | 0.65          | 0.69     | 0.68           | 0.65      | 0.49        | 0.52   |
| 16       | 0.65          | 0.69     | 0.68           | 0.65      | 0.49        | 0.52   |
| 17       | 0.65          | 0.69     | 0.68           | 0.65      | 0.49        | 0.52   |
| 18       | 0.65          | 0.69     | 0.68           | 0.65      | 0.49        | 0.52   |
| 19       | 0.65          | 0.69     | 0.68           | 0.66      | 0.49        | 0.51   |
| 20       | 0.64          | 0.69     | 0.69           | 0.66      | 0.48        | 0.51   |
| 21       | 0.64          | 0.68     | 0.69           | 0.66      | 0.48        | 0.51   |
| 22       | 0.64          | 0.68     | 0.69           | 0.66      | 0.48        | 0.51   |
| 23       | 0.64          | 0.68     | 0.69           | 0.67      | 0.48        | 0.50   |
| 24       | 0.64          | 0.68     | 0.70           | 0.67      | 0.47        | 0.50   |
| 25       | 0.64          | 0.68     | 0.70           | 0.67      | 0.47        | 0.50   |
| 26       | 0.64          | 0.67     | 0.70           | 0.67      | 0.47        | 0.50   |
| 27       | 0.63          | 0.67     | 0.71           | 0.68      | 0.46        | 0.50   |
| 28       | 0.63          | 0.67     | 0.71           | 0.68      | 0.46        | 0.50   |
| 29       | 0.63          | 0.67     | 0.71           | 0.68      | 0.46        | 0.50   |
| 30       | 0.63          | 0.66     | 0.71           | 0.69      | 0.46        | 0.49   |
| 31       | 0.63          | 0.66     | 0.72           | 0.69      | 0.46        | 0.49   |

Continued on next page

| $\alpha$ | $\phi_S^\ell$ | $\phi_S$ | $\varphi^\ell$ | $\varphi$ | $\psi^\ell$ | $\psi$ |
|----------|---------------|----------|----------------|-----------|-------------|--------|
| 32       | 0.62          | 0.66     | 0.72           | 0.70      | 0.45        | 0.48   |
| 33       | 0.62          | 0.65     | 0.72           | 0.70      | 0.45        | 0.48   |
| 34       | 0.62          | 0.65     | 0.73           | 0.70      | 0.45        | 0.48   |
| 35       | 0.62          | 0.65     | 0.73           | 0.71      | 0.45        | 0.47   |
| 36       | 0.61          | 0.65     | 0.74           | 0.71      | 0.44        | 0.47   |
| 37       | 0.61          | 0.64     | 0.74           | 0.71      | 0.44        | 0.47   |
| 38       | 0.61          | 0.64     | 0.74           | 0.72      | 0.44        | 0.46   |
| 39       | 0.60          | 0.63     | 0.75           | 0.72      | 0.43        | 0.46   |
| 40       | 0.60          | 0.63     | 0.75           | 0.73      | 0.43        | 0.45   |
| 41       | 0.60          | 0.63     | 0.76           | 0.73      | 0.43        | 0.45   |
| 42       | 0.59          | 0.62     | 0.76           | 0.73      | 0.42        | 0.45   |
| 43       | 0.59          | 0.62     | 0.76           | 0.74      | 0.42        | 0.44   |
| 44       | 0.59          | 0.61     | 0.77           | 0.74      | 0.42        | 0.44   |
| 45       | 0.58          | 0.61     | 0.77           | 0.75      | 0.41        | 0.43   |
| 46       | 0.58          | 0.60     | 0.78           | 0.75      | 0.41        | 0.43   |
| 47       | 0.57          | 0.60     | 0.78           | 0.76      | 0.40        | 0.43   |
| 48       | 0.57          | 0.59     | 0.79           | 0.76      | 0.40        | 0.42   |
| 49       | 0.56          | 0.59     | 0.79           | 0.77      | 0.39        | 0.42   |
| 50       | 0.56          | 0.58     | 0.79           | 0.77      | 0.39        | 0.41   |
| 51       | 0.55          | 0.58     | 0.80           | 0.78      | 0.38        | 0.41   |
| 52       | 0.55          | 0.57     | 0.80           | 0.78      | 0.38        | 0.40   |
| 53       | 0.54          | 0.57     | 0.81           | 0.78      | 0.37        | 0.40   |
| 54       | 0.54          | 0.56     | 0.81           | 0.79      | 0.37        | 0.39   |
| 55       | 0.53          | 0.55     | 0.82           | 0.79      | 0.37        | 0.39   |
| 56       | 0.52          | 0.55     | 0.82           | 0.80      | 0.36        | 0.38   |
| 57       | 0.52          | 0.54     | 0.83           | 0.80      | 0.36        | 0.38   |
| 58       | 0.51          | 0.53     | 0.83           | 0.81      | 0.35        | 0.37   |
| 59       | 0.50          | 0.53     | 0.84           | 0.81      | 0.34        | 0.37   |
| 60       | 0.50          | 0.52     | 0.84           | 0.82      | 0.34        | 0.36   |
| 61       | 0.49          | 0.51     | 0.85           | 0.83      | 0.33        | 0.35   |
| 62       | 0.48          | 0.50     | 0.85           | 0.83      | 0.33        | 0.35   |
| 63       | 0.47          | 0.50     | 0.86           | 0.84      | 0.32        | 0.34   |

Continued on next page

| $\alpha$ | $\phi_S^\ell$ | $\phi_S$ | $\varphi^\ell$ | $\varphi$ | $\psi^\ell$ | $\psi$ |
|----------|---------------|----------|----------------|-----------|-------------|--------|
| 64       | 0.46          | 0.49     | 0.86           | 0.84      | 0.31        | 0.34   |
| 65       | 0.45          | 0.48     | 0.87           | 0.85      | 0.30        | 0.33   |
| 66       | 0.44          | 0.47     | 0.88           | 0.85      | 0.30        | 0.32   |
| 67       | 0.43          | 0.46     | 0.88           | 0.86      | 0.29        | 0.31   |
| 68       | 0.42          | 0.45     | 0.89           | 0.86      | 0.28        | 0.31   |
| 69       | 0.41          | 0.44     | 0.89           | 0.87      | 0.27        | 0.30   |
| 70       | 0.40          | 0.43     | 0.90           | 0.87      | 0.27        | 0.29   |
| 71       | 0.39          | 0.42     | 0.90           | 0.88      | 0.26        | 0.28   |
| 72       | 0.38          | 0.41     | 0.91           | 0.88      | 0.25        | 0.28   |
| 73       | 0.37          | 0.39     | 0.92           | 0.89      | 0.24        | 0.26   |
| 74       | 0.35          | 0.38     | 0.92           | 0.90      | 0.23        | 0.25   |
| 75       | 0.34          | 0.37     | 0.93           | 0.90      | 0.22        | 0.25   |
| 76       | 0.32          | 0.35     | 0.93           | 0.91      | 0.21        | 0.23   |
| 77       | 0.31          | 0.34     | 0.94           | 0.91      | 0.20        | 0.23   |
| 78       | 0.29          | 0.33     | 0.94           | 0.92      | 0.19        | 0.22   |
| 79       | 0.28          | 0.31     | 0.95           | 0.92      | 0.18        | 0.21   |
| 80       | 0.26          | 0.30     | 0.95           | 0.93      | 0.17        | 0.20   |
| 81       | 0.24          | 0.28     | 0.96           | 0.93      | 0.16        | 0.19   |
| 82       | 0.23          | 0.26     | 0.96           | 0.94      | 0.15        | 0.17   |
| 83       | 0.21          | 0.25     | 0.97           | 0.94      | 0.14        | 0.17   |
| 84       | 0.19          | 0.23     | 0.97           | 0.94      | 0.12        | 0.15   |
| 85       | 0.17          | 0.21     | 0.97           | 0.95      | 0.11        | 0.14   |
| 86       | 0.16          | 0.20     | 0.98           | 0.95      | 0.10        | 0.13   |
| 87       | 0.14          | 0.18     | 0.98           | 0.95      | 0.09        | 0.12   |
| 88       | 0.13          | 0.17     | 0.98           | 0.96      | 0.08        | 0.11   |
| 89       | 0.12          | 0.16     | 0.98           | 0.96      | 0.08        | 0.11   |
| 90       | 0.12          | 0.16     | 0.98           | 0.96      | 0.08        | 0.11   |

Table S70: Reference ( $\phi_S$ ,  $\varphi$ ,  $\psi$ ) and approached ( $\phi_S^\ell$ ,  $\varphi^\ell$ ,  $\psi^\ell$ ) values of the topological descriptors for the first excited-state of the pyridinium-phenolate (PP), computed at the CAM-B3LYP/6-311+G(d) level of theory.  $\alpha$  is the pyridinium-phenolate central twist angle amplitude.

| $\alpha$ | $\phi_S^\ell$ | $\phi_S$ | $\varphi^\ell$ | $\varphi$ | $\psi^\ell$ | $\psi$ |
|----------|---------------|----------|----------------|-----------|-------------|--------|
| 0        | 0.68          | 0.72     | 0.65           | 0.62      | 0.51        | 0.55   |
| 1        | 0.68          | 0.72     | 0.65           | 0.62      | 0.51        | 0.55   |
| 2        | 0.68          | 0.72     | 0.65           | 0.62      | 0.51        | 0.55   |
| 3        | 0.68          | 0.72     | 0.65           | 0.62      | 0.51        | 0.55   |
| 4        | 0.68          | 0.72     | 0.65           | 0.62      | 0.51        | 0.55   |
| 5        | 0.68          | 0.72     | 0.65           | 0.62      | 0.51        | 0.55   |
| 6        | 0.68          | 0.72     | 0.65           | 0.62      | 0.51        | 0.55   |
| 7        | 0.68          | 0.72     | 0.66           | 0.62      | 0.51        | 0.55   |
| 8        | 0.68          | 0.72     | 0.66           | 0.62      | 0.51        | 0.55   |
| 9        | 0.68          | 0.72     | 0.66           | 0.62      | 0.51        | 0.55   |
| 10       | 0.68          | 0.72     | 0.66           | 0.62      | 0.51        | 0.55   |
| 11       | 0.68          | 0.72     | 0.66           | 0.62      | 0.51        | 0.55   |
| 12       | 0.68          | 0.72     | 0.66           | 0.63      | 0.51        | 0.54   |
| 13       | 0.68          | 0.71     | 0.66           | 0.63      | 0.51        | 0.54   |
| 14       | 0.67          | 0.71     | 0.66           | 0.63      | 0.50        | 0.54   |
| 15       | 0.67          | 0.71     | 0.67           | 0.63      | 0.50        | 0.54   |
| 16       | 0.67          | 0.71     | 0.67           | 0.63      | 0.50        | 0.54   |
| 17       | 0.67          | 0.71     | 0.67           | 0.64      | 0.50        | 0.53   |
| 18       | 0.67          | 0.71     | 0.67           | 0.64      | 0.50        | 0.53   |
| 19       | 0.67          | 0.71     | 0.67           | 0.64      | 0.50        | 0.53   |
| 20       | 0.67          | 0.70     | 0.68           | 0.64      | 0.50        | 0.53   |
| 21       | 0.67          | 0.70     | 0.68           | 0.65      | 0.50        | 0.52   |
| 22       | 0.66          | 0.70     | 0.68           | 0.65      | 0.49        | 0.52   |
| 23       | 0.66          | 0.70     | 0.68           | 0.65      | 0.49        | 0.52   |
| 24       | 0.66          | 0.70     | 0.69           | 0.66      | 0.49        | 0.52   |
| 25       | 0.66          | 0.69     | 0.69           | 0.66      | 0.49        | 0.51   |
| 26       | 0.66          | 0.69     | 0.69           | 0.66      | 0.49        | 0.51   |
| 27       | 0.66          | 0.69     | 0.69           | 0.66      | 0.49        | 0.51   |
| 28       | 0.65          | 0.69     | 0.70           | 0.67      | 0.48        | 0.51   |
| 29       | 0.65          | 0.68     | 0.70           | 0.67      | 0.48        | 0.50   |
| 30       | 0.65          | 0.68     | 0.70           | 0.67      | 0.48        | 0.50   |
| 31       | 0.65          | 0.68     | 0.71           | 0.68      | 0.47        | 0.50   |

Continued on next page

| $\alpha$ | $\phi_S^\ell$ | $\phi_S$ | $\varphi^\ell$ | $\varphi$ | $\psi^\ell$ | $\psi$ |
|----------|---------------|----------|----------------|-----------|-------------|--------|
| 32       | 0.65          | 0.67     | 0.71           | 0.68      | 0.47        | 0.50   |
| 33       | 0.64          | 0.67     | 0.71           | 0.69      | 0.47        | 0.49   |
| 34       | 0.64          | 0.67     | 0.72           | 0.69      | 0.46        | 0.49   |
| 35       | 0.64          | 0.67     | 0.72           | 0.69      | 0.46        | 0.49   |
| 36       | 0.64          | 0.66     | 0.72           | 0.70      | 0.46        | 0.48   |
| 37       | 0.63          | 0.66     | 0.73           | 0.70      | 0.45        | 0.48   |
| 38       | 0.63          | 0.66     | 0.73           | 0.70      | 0.45        | 0.48   |
| 39       | 0.63          | 0.65     | 0.74           | 0.71      | 0.45        | 0.47   |
| 40       | 0.62          | 0.65     | 0.74           | 0.71      | 0.44        | 0.47   |
| 41       | 0.62          | 0.64     | 0.74           | 0.72      | 0.44        | 0.46   |
| 42       | 0.62          | 0.64     | 0.75           | 0.72      | 0.44        | 0.46   |
| 43       | 0.61          | 0.64     | 0.75           | 0.73      | 0.43        | 0.46   |
| 44       | 0.61          | 0.63     | 0.76           | 0.73      | 0.43        | 0.45   |
| 45       | 0.61          | 0.63     | 0.76           | 0.73      | 0.43        | 0.45   |
| 46       | 0.60          | 0.62     | 0.77           | 0.74      | 0.42        | 0.44   |
| 47       | 0.60          | 0.62     | 0.77           | 0.74      | 0.42        | 0.44   |
| 48       | 0.59          | 0.61     | 0.77           | 0.75      | 0.42        | 0.43   |
| 49       | 0.59          | 0.61     | 0.78           | 0.75      | 0.41        | 0.43   |
| 50       | 0.58          | 0.60     | 0.78           | 0.76      | 0.41        | 0.43   |
| 51       | 0.58          | 0.60     | 0.79           | 0.76      | 0.40        | 0.43   |
| 52       | 0.57          | 0.59     | 0.79           | 0.77      | 0.40        | 0.42   |
| 53       | 0.57          | 0.59     | 0.80           | 0.77      | 0.39        | 0.42   |
| 54       | 0.56          | 0.58     | 0.80           | 0.78      | 0.39        | 0.41   |
| 55       | 0.55          | 0.57     | 0.81           | 0.78      | 0.38        | 0.40   |
| 56       | 0.55          | 0.57     | 0.81           | 0.79      | 0.38        | 0.40   |
| 57       | 0.54          | 0.56     | 0.82           | 0.79      | 0.37        | 0.39   |
| 58       | 0.54          | 0.55     | 0.82           | 0.80      | 0.37        | 0.38   |
| 59       | 0.53          | 0.55     | 0.83           | 0.80      | 0.36        | 0.38   |
| 60       | 0.52          | 0.54     | 0.83           | 0.81      | 0.36        | 0.37   |
| 61       | 0.51          | 0.53     | 0.84           | 0.81      | 0.35        | 0.37   |
| 62       | 0.51          | 0.52     | 0.84           | 0.82      | 0.35        | 0.36   |
| 63       | 0.50          | 0.52     | 0.85           | 0.82      | 0.34        | 0.36   |

Continued on next page

| $\alpha$ | $\phi_S^\ell$ | $\phi_S$ | $\varphi^\ell$ | $\varphi$ | $\psi^\ell$ | $\psi$ |
|----------|---------------|----------|----------------|-----------|-------------|--------|
| 64       | 0.49          | 0.51     | 0.85           | 0.83      | 0.33        | 0.35   |
| 65       | 0.48          | 0.50     | 0.86           | 0.83      | 0.32        | 0.35   |
| 66       | 0.47          | 0.49     | 0.86           | 0.84      | 0.32        | 0.34   |
| 67       | 0.46          | 0.48     | 0.87           | 0.85      | 0.31        | 0.33   |
| 68       | 0.45          | 0.47     | 0.88           | 0.85      | 0.30        | 0.32   |
| 69       | 0.44          | 0.46     | 0.88           | 0.86      | 0.30        | 0.31   |
| 70       | 0.43          | 0.45     | 0.89           | 0.86      | 0.29        | 0.31   |
| 71       | 0.42          | 0.44     | 0.89           | 0.87      | 0.28        | 0.30   |
| 72       | 0.40          | 0.43     | 0.90           | 0.87      | 0.27        | 0.29   |
| 73       | 0.39          | 0.42     | 0.91           | 0.88      | 0.26        | 0.28   |
| 74       | 0.38          | 0.40     | 0.91           | 0.89      | 0.25        | 0.27   |
| 75       | 0.36          | 0.39     | 0.92           | 0.89      | 0.24        | 0.26   |
| 76       | 0.35          | 0.38     | 0.93           | 0.90      | 0.23        | 0.25   |
| 77       | 0.33          | 0.36     | 0.93           | 0.90      | 0.22        | 0.24   |
| 78       | 0.32          | 0.35     | 0.94           | 0.91      | 0.21        | 0.23   |
| 79       | 0.30          | 0.33     | 0.94           | 0.92      | 0.20        | 0.22   |
| 80       | 0.28          | 0.32     | 0.95           | 0.92      | 0.18        | 0.21   |
| 81       | 0.26          | 0.30     | 0.95           | 0.93      | 0.17        | 0.20   |
| 82       | 0.24          | 0.28     | 0.96           | 0.93      | 0.16        | 0.19   |
| 83       | 0.22          | 0.26     | 0.96           | 0.94      | 0.14        | 0.17   |
| 84       | 0.20          | 0.24     | 0.97           | 0.94      | 0.13        | 0.16   |
| 85       | 0.18          | 0.23     | 0.97           | 0.95      | 0.12        | 0.15   |
| 86       | 0.16          | 0.21     | 0.98           | 0.95      | 0.10        | 0.14   |
| 87       | 0.14          | 0.19     | 0.98           | 0.95      | 0.09        | 0.13   |
| 88       | 0.13          | 0.18     | 0.98           | 0.95      | 0.08        | 0.12   |
| 89       | 0.11          | 0.16     | 0.98           | 0.96      | 0.07        | 0.11   |
| 90       | 0.11          | 0.16     | 0.99           | 0.96      | 0.07        | 0.11   |

Table S71: Reference ( $\phi_S$ ,  $\varphi$ ,  $\psi$ ) and approached ( $\phi_S^\ell$ ,  $\varphi^\ell$ ,  $\psi^\ell$ ) values of the topological descriptors for the first excited-state of the pyridinium-phenolate (PP), computed at the CAM-B3LYP/6-311G(d) level of theory.  $\alpha$  is the pyridinium-phenolate central twist angle amplitude.

| $\alpha$ | $\phi_S^\ell$ | $\phi_S$ | $\varphi^\ell$ | $\varphi$ | $\psi^\ell$ | $\psi$ |
|----------|---------------|----------|----------------|-----------|-------------|--------|
| 0        | 0.66          | 0.70     | 0.66           | 0.63      | 0.50        | 0.53   |
| 1        | 0.66          | 0.70     | 0.66           | 0.63      | 0.50        | 0.53   |
| 2        | 0.66          | 0.70     | 0.66           | 0.63      | 0.50        | 0.53   |
| 3        | 0.66          | 0.70     | 0.66           | 0.63      | 0.50        | 0.53   |
| 4        | 0.66          | 0.70     | 0.66           | 0.63      | 0.50        | 0.53   |
| 5        | 0.66          | 0.70     | 0.66           | 0.63      | 0.50        | 0.53   |
| 6        | 0.66          | 0.70     | 0.66           | 0.64      | 0.50        | 0.53   |
| 7        | 0.66          | 0.70     | 0.66           | 0.64      | 0.50        | 0.53   |
| 8        | 0.66          | 0.70     | 0.66           | 0.64      | 0.50        | 0.53   |
| 9        | 0.66          | 0.70     | 0.67           | 0.64      | 0.50        | 0.53   |
| 10       | 0.66          | 0.70     | 0.67           | 0.64      | 0.50        | 0.53   |
| 11       | 0.66          | 0.70     | 0.67           | 0.64      | 0.50        | 0.53   |
| 12       | 0.66          | 0.69     | 0.67           | 0.64      | 0.50        | 0.52   |
| 13       | 0.66          | 0.69     | 0.67           | 0.65      | 0.50        | 0.52   |
| 14       | 0.65          | 0.69     | 0.67           | 0.65      | 0.49        | 0.52   |
| 15       | 0.65          | 0.69     | 0.67           | 0.65      | 0.49        | 0.52   |
| 16       | 0.65          | 0.69     | 0.68           | 0.65      | 0.49        | 0.52   |
| 17       | 0.65          | 0.69     | 0.68           | 0.65      | 0.49        | 0.52   |
| 18       | 0.65          | 0.69     | 0.68           | 0.66      | 0.49        | 0.51   |
| 19       | 0.65          | 0.68     | 0.68           | 0.66      | 0.49        | 0.51   |
| 20       | 0.65          | 0.68     | 0.68           | 0.66      | 0.49        | 0.51   |
| 21       | 0.65          | 0.68     | 0.69           | 0.66      | 0.48        | 0.51   |
| 22       | 0.65          | 0.68     | 0.69           | 0.67      | 0.48        | 0.50   |
| 23       | 0.64          | 0.68     | 0.69           | 0.67      | 0.48        | 0.50   |
| 24       | 0.64          | 0.68     | 0.70           | 0.67      | 0.47        | 0.50   |
| 25       | 0.64          | 0.67     | 0.70           | 0.67      | 0.47        | 0.50   |
| 26       | 0.64          | 0.67     | 0.70           | 0.68      | 0.47        | 0.50   |
| 27       | 0.64          | 0.67     | 0.70           | 0.68      | 0.47        | 0.50   |
| 28       | 0.64          | 0.67     | 0.71           | 0.68      | 0.47        | 0.50   |
| 29       | 0.63          | 0.66     | 0.71           | 0.69      | 0.46        | 0.49   |
| 30       | 0.63          | 0.66     | 0.71           | 0.69      | 0.46        | 0.49   |
| 31       | 0.63          | 0.66     | 0.71           | 0.69      | 0.46        | 0.49   |

Continued on next page

| $\alpha$ | $\phi_S^\ell$ | $\phi_S$ | $\varphi^\ell$ | $\varphi$ | $\psi^\ell$ | $\psi$ |
|----------|---------------|----------|----------------|-----------|-------------|--------|
| 32       | 0.63          | 0.66     | 0.72           | 0.70      | 0.46        | 0.48   |
| 33       | 0.63          | 0.65     | 0.72           | 0.70      | 0.46        | 0.48   |
| 34       | 0.62          | 0.65     | 0.73           | 0.71      | 0.45        | 0.47   |
| 35       | 0.62          | 0.65     | 0.73           | 0.71      | 0.45        | 0.47   |
| 36       | 0.62          | 0.64     | 0.73           | 0.71      | 0.45        | 0.47   |
| 37       | 0.62          | 0.64     | 0.74           | 0.72      | 0.44        | 0.46   |
| 38       | 0.61          | 0.64     | 0.74           | 0.72      | 0.44        | 0.46   |
| 39       | 0.61          | 0.63     | 0.74           | 0.72      | 0.44        | 0.46   |
| 40       | 0.61          | 0.63     | 0.75           | 0.73      | 0.43        | 0.45   |
| 41       | 0.60          | 0.63     | 0.75           | 0.73      | 0.43        | 0.45   |
| 42       | 0.60          | 0.62     | 0.76           | 0.74      | 0.43        | 0.44   |
| 43       | 0.60          | 0.62     | 0.76           | 0.74      | 0.43        | 0.44   |
| 44       | 0.59          | 0.61     | 0.76           | 0.74      | 0.42        | 0.44   |
| 45       | 0.59          | 0.61     | 0.77           | 0.75      | 0.42        | 0.43   |
| 46       | 0.58          | 0.60     | 0.77           | 0.75      | 0.41        | 0.43   |
| 47       | 0.58          | 0.60     | 0.78           | 0.76      | 0.41        | 0.43   |
| 48       | 0.58          | 0.60     | 0.78           | 0.76      | 0.41        | 0.43   |
| 49       | 0.57          | 0.59     | 0.79           | 0.77      | 0.40        | 0.42   |
| 50       | 0.57          | 0.58     | 0.79           | 0.77      | 0.40        | 0.41   |
| 51       | 0.56          | 0.58     | 0.80           | 0.78      | 0.39        | 0.41   |
| 52       | 0.55          | 0.57     | 0.80           | 0.78      | 0.38        | 0.40   |
| 53       | 0.55          | 0.57     | 0.81           | 0.79      | 0.38        | 0.40   |
| 54       | 0.54          | 0.56     | 0.81           | 0.79      | 0.37        | 0.39   |
| 55       | 0.54          | 0.56     | 0.81           | 0.80      | 0.37        | 0.39   |
| 56       | 0.53          | 0.55     | 0.82           | 0.80      | 0.37        | 0.38   |
| 57       | 0.52          | 0.54     | 0.82           | 0.81      | 0.36        | 0.37   |
| 58       | 0.52          | 0.54     | 0.83           | 0.81      | 0.36        | 0.37   |
| 59       | 0.51          | 0.53     | 0.83           | 0.82      | 0.35        | 0.37   |
| 60       | 0.50          | 0.52     | 0.84           | 0.82      | 0.34        | 0.36   |
| 61       | 0.49          | 0.51     | 0.85           | 0.83      | 0.33        | 0.35   |
| 62       | 0.49          | 0.51     | 0.85           | 0.83      | 0.33        | 0.35   |
| 63       | 0.48          | 0.50     | 0.86           | 0.84      | 0.32        | 0.34   |

Continued on next page



| $\alpha$ | $\phi_S^\ell$ | $\phi_S$ | $\varphi^\ell$ | $\varphi$ | $\psi^\ell$ | $\psi$ |
|----------|---------------|----------|----------------|-----------|-------------|--------|
| 64       | 0.47          | 0.49     | 0.86           | 0.84      | 0.32        | 0.34   |
| 65       | 0.46          | 0.48     | 0.87           | 0.85      | 0.31        | 0.33   |
| 66       | 0.45          | 0.47     | 0.87           | 0.85      | 0.30        | 0.32   |
| 67       | 0.44          | 0.46     | 0.88           | 0.86      | 0.30        | 0.31   |
| 68       | 0.43          | 0.45     | 0.89           | 0.86      | 0.29        | 0.31   |
| 69       | 0.42          | 0.44     | 0.89           | 0.87      | 0.28        | 0.30   |
| 70       | 0.41          | 0.43     | 0.90           | 0.87      | 0.27        | 0.29   |
| 71       | 0.40          | 0.42     | 0.90           | 0.88      | 0.27        | 0.28   |
| 72       | 0.38          | 0.41     | 0.91           | 0.88      | 0.25        | 0.28   |
| 73       | 0.37          | 0.40     | 0.92           | 0.89      | 0.24        | 0.27   |
| 74       | 0.36          | 0.39     | 0.92           | 0.90      | 0.24        | 0.26   |
| 75       | 0.34          | 0.37     | 0.93           | 0.90      | 0.22        | 0.25   |
| 76       | 0.33          | 0.36     | 0.93           | 0.91      | 0.22        | 0.24   |
| 77       | 0.31          | 0.34     | 0.94           | 0.91      | 0.20        | 0.23   |
| 78       | 0.30          | 0.33     | 0.94           | 0.92      | 0.20        | 0.22   |
| 79       | 0.28          | 0.31     | 0.95           | 0.92      | 0.18        | 0.21   |
| 80       | 0.26          | 0.30     | 0.95           | 0.93      | 0.17        | 0.20   |
| 81       | 0.24          | 0.28     | 0.96           | 0.93      | 0.16        | 0.19   |
| 82       | 0.22          | 0.26     | 0.96           | 0.94      | 0.14        | 0.17   |
| 83       | 0.21          | 0.25     | 0.97           | 0.94      | 0.14        | 0.17   |
| 84       | 0.19          | 0.23     | 0.97           | 0.95      | 0.12        | 0.15   |
| 85       | 0.17          | 0.21     | 0.98           | 0.95      | 0.11        | 0.14   |
| 86       | 0.15          | 0.19     | 0.98           | 0.95      | 0.10        | 0.13   |
| 87       | 0.14          | 0.18     | 0.98           | 0.96      | 0.09        | 0.12   |
| 88       | 0.12          | 0.16     | 0.99           | 0.96      | 0.08        | 0.11   |
| 89       | 0.11          | 0.15     | 0.99           | 0.96      | 0.07        | 0.10   |
| 90       | 0.10          | 0.15     | 0.99           | 0.96      | 0.06        | 0.10   |

Table S72: Reference ( $\phi_S$ ,  $\varphi$ ,  $\psi$ ) and approached ( $\phi_S^\ell$ ,  $\varphi^\ell$ ,  $\psi^\ell$ ) values of the topological descriptors for the first excited-state of the pyridinium-phenolate (PP), computed at the CAM-B3LYP/6-311+G level of theory.  $\alpha$  is the pyridinium-phenolate central twist angle amplitude.

| $\alpha$ | $\phi_S^\ell$ | $\phi_S$ | $\varphi^\ell$ | $\varphi$ | $\psi^\ell$ | $\psi$ |
|----------|---------------|----------|----------------|-----------|-------------|--------|
| 0        | 0.69          | 0.72     | 0.65           | 0.62      | 0.52        | 0.55   |
| 1        | 0.69          | 0.72     | 0.65           | 0.62      | 0.52        | 0.55   |
| 2        | 0.69          | 0.72     | 0.65           | 0.62      | 0.52        | 0.55   |
| 3        | 0.69          | 0.72     | 0.65           | 0.62      | 0.52        | 0.55   |
| 4        | 0.69          | 0.72     | 0.65           | 0.62      | 0.52        | 0.55   |
| 5        | 0.69          | 0.72     | 0.65           | 0.62      | 0.52        | 0.55   |
| 6        | 0.68          | 0.72     | 0.65           | 0.62      | 0.51        | 0.55   |
| 7        | 0.68          | 0.72     | 0.65           | 0.62      | 0.51        | 0.55   |
| 8        | 0.68          | 0.72     | 0.65           | 0.63      | 0.51        | 0.54   |
| 9        | 0.68          | 0.71     | 0.66           | 0.63      | 0.51        | 0.54   |
| 10       | 0.68          | 0.71     | 0.66           | 0.63      | 0.51        | 0.54   |
| 11       | 0.68          | 0.71     | 0.66           | 0.63      | 0.51        | 0.54   |
| 12       | 0.68          | 0.71     | 0.66           | 0.63      | 0.51        | 0.54   |
| 13       | 0.68          | 0.71     | 0.66           | 0.63      | 0.51        | 0.54   |
| 14       | 0.68          | 0.71     | 0.66           | 0.63      | 0.51        | 0.54   |
| 15       | 0.68          | 0.71     | 0.66           | 0.64      | 0.51        | 0.53   |
| 16       | 0.68          | 0.71     | 0.67           | 0.64      | 0.50        | 0.53   |
| 17       | 0.67          | 0.70     | 0.67           | 0.64      | 0.50        | 0.53   |
| 18       | 0.67          | 0.70     | 0.67           | 0.64      | 0.50        | 0.53   |
| 19       | 0.67          | 0.70     | 0.67           | 0.65      | 0.50        | 0.52   |
| 20       | 0.67          | 0.70     | 0.67           | 0.65      | 0.50        | 0.52   |
| 21       | 0.67          | 0.70     | 0.68           | 0.65      | 0.50        | 0.52   |
| 22       | 0.67          | 0.70     | 0.68           | 0.65      | 0.50        | 0.52   |
| 23       | 0.67          | 0.69     | 0.68           | 0.66      | 0.50        | 0.51   |
| 24       | 0.66          | 0.69     | 0.68           | 0.66      | 0.49        | 0.51   |
| 25       | 0.66          | 0.69     | 0.69           | 0.66      | 0.49        | 0.51   |
| 26       | 0.66          | 0.69     | 0.69           | 0.67      | 0.49        | 0.51   |
| 27       | 0.66          | 0.68     | 0.69           | 0.67      | 0.49        | 0.50   |
| 28       | 0.66          | 0.68     | 0.70           | 0.67      | 0.48        | 0.50   |
| 29       | 0.66          | 0.68     | 0.70           | 0.68      | 0.48        | 0.50   |
| 30       | 0.65          | 0.68     | 0.70           | 0.68      | 0.48        | 0.50   |
| 31       | 0.65          | 0.67     | 0.70           | 0.68      | 0.48        | 0.50   |

Continued on next page

| $\alpha$ | $\phi_S^\ell$ | $\phi_S$ | $\varphi^\ell$ | $\varphi$ | $\psi^\ell$ | $\psi$ |
|----------|---------------|----------|----------------|-----------|-------------|--------|
| 32       | 0.65          | 0.67     | 0.71           | 0.69      | 0.47        | 0.49   |
| 33       | 0.65          | 0.67     | 0.71           | 0.69      | 0.47        | 0.49   |
| 34       | 0.65          | 0.67     | 0.71           | 0.69      | 0.47        | 0.49   |
| 35       | 0.64          | 0.66     | 0.72           | 0.70      | 0.46        | 0.48   |
| 36       | 0.64          | 0.66     | 0.72           | 0.70      | 0.46        | 0.48   |
| 37       | 0.64          | 0.66     | 0.72           | 0.70      | 0.46        | 0.48   |
| 38       | 0.64          | 0.65     | 0.73           | 0.71      | 0.46        | 0.47   |
| 39       | 0.63          | 0.65     | 0.73           | 0.71      | 0.45        | 0.47   |
| 40       | 0.63          | 0.65     | 0.74           | 0.72      | 0.45        | 0.47   |
| 41       | 0.63          | 0.64     | 0.74           | 0.72      | 0.45        | 0.46   |
| 42       | 0.62          | 0.64     | 0.74           | 0.72      | 0.44        | 0.46   |
| 43       | 0.62          | 0.63     | 0.75           | 0.73      | 0.44        | 0.45   |
| 44       | 0.62          | 0.63     | 0.75           | 0.73      | 0.44        | 0.45   |
| 45       | 0.61          | 0.63     | 0.76           | 0.74      | 0.43        | 0.45   |
| 46       | 0.61          | 0.62     | 0.76           | 0.74      | 0.43        | 0.44   |
| 47       | 0.60          | 0.62     | 0.77           | 0.75      | 0.42        | 0.44   |
| 48       | 0.60          | 0.61     | 0.77           | 0.75      | 0.42        | 0.43   |
| 49       | 0.59          | 0.61     | 0.78           | 0.75      | 0.41        | 0.43   |
| 50       | 0.59          | 0.60     | 0.78           | 0.76      | 0.41        | 0.43   |
| 51       | 0.58          | 0.60     | 0.78           | 0.76      | 0.41        | 0.43   |
| 52       | 0.58          | 0.59     | 0.79           | 0.77      | 0.40        | 0.42   |
| 53       | 0.57          | 0.59     | 0.79           | 0.77      | 0.40        | 0.42   |
| 54       | 0.57          | 0.58     | 0.80           | 0.78      | 0.39        | 0.41   |
| 55       | 0.56          | 0.57     | 0.80           | 0.78      | 0.39        | 0.40   |
| 56       | 0.55          | 0.57     | 0.81           | 0.79      | 0.38        | 0.40   |
| 57       | 0.55          | 0.56     | 0.81           | 0.79      | 0.38        | 0.39   |
| 58       | 0.54          | 0.56     | 0.82           | 0.80      | 0.37        | 0.39   |
| 59       | 0.53          | 0.55     | 0.82           | 0.80      | 0.37        | 0.38   |
| 60       | 0.53          | 0.54     | 0.83           | 0.81      | 0.36        | 0.37   |
| 61       | 0.52          | 0.53     | 0.83           | 0.81      | 0.36        | 0.37   |
| 62       | 0.51          | 0.53     | 0.84           | 0.82      | 0.35        | 0.37   |
| 63       | 0.50          | 0.52     | 0.85           | 0.82      | 0.34        | 0.36   |

Continued on next page

| $\alpha$ | $\phi_S^\ell$ | $\phi_S$ | $\varphi^\ell$ | $\varphi$ | $\psi^\ell$ | $\psi$ |
|----------|---------------|----------|----------------|-----------|-------------|--------|
| 64       | 0.49          | 0.51     | 0.85           | 0.83      | 0.33        | 0.35   |
| 65       | 0.48          | 0.50     | 0.86           | 0.84      | 0.32        | 0.34   |
| 66       | 0.48          | 0.49     | 0.86           | 0.84      | 0.32        | 0.34   |
| 67       | 0.47          | 0.48     | 0.87           | 0.85      | 0.32        | 0.33   |
| 68       | 0.46          | 0.47     | 0.88           | 0.85      | 0.31        | 0.32   |
| 69       | 0.44          | 0.46     | 0.88           | 0.86      | 0.30        | 0.31   |
| 70       | 0.43          | 0.45     | 0.89           | 0.86      | 0.29        | 0.31   |
| 71       | 0.42          | 0.44     | 0.89           | 0.87      | 0.28        | 0.30   |
| 72       | 0.41          | 0.43     | 0.90           | 0.88      | 0.27        | 0.29   |
| 73       | 0.40          | 0.42     | 0.91           | 0.88      | 0.26        | 0.28   |
| 74       | 0.38          | 0.41     | 0.91           | 0.89      | 0.25        | 0.27   |
| 75       | 0.37          | 0.39     | 0.92           | 0.89      | 0.24        | 0.26   |
| 76       | 0.35          | 0.38     | 0.93           | 0.90      | 0.23        | 0.25   |
| 77       | 0.34          | 0.37     | 0.93           | 0.90      | 0.22        | 0.25   |
| 78       | 0.32          | 0.35     | 0.94           | 0.91      | 0.21        | 0.23   |
| 79       | 0.30          | 0.33     | 0.94           | 0.92      | 0.20        | 0.22   |
| 80       | 0.28          | 0.32     | 0.95           | 0.92      | 0.18        | 0.21   |
| 81       | 0.26          | 0.30     | 0.96           | 0.93      | 0.17        | 0.20   |
| 82       | 0.24          | 0.28     | 0.96           | 0.93      | 0.16        | 0.19   |
| 83       | 0.22          | 0.26     | 0.97           | 0.94      | 0.14        | 0.17   |
| 84       | 0.20          | 0.24     | 0.97           | 0.94      | 0.13        | 0.16   |
| 85       | 0.18          | 0.22     | 0.98           | 0.95      | 0.12        | 0.14   |
| 86       | 0.16          | 0.20     | 0.98           | 0.95      | 0.10        | 0.13   |
| 87       | 0.13          | 0.19     | 0.99           | 0.96      | 0.08        | 0.12   |
| 88       | 0.12          | 0.17     | 0.99           | 0.96      | 0.08        | 0.11   |
| 89       | 0.10          | 0.15     | 0.99           | 0.96      | 0.06        | 0.10   |
| 90       | 0.09          | 0.15     | 0.99           | 0.96      | 0.06        | 0.10   |

Table S73: Reference ( $\phi_S$ ,  $\varphi$ ,  $\psi$ ) and approached ( $\phi_S^\ell$ ,  $\varphi^\ell$ ,  $\psi^\ell$ ) values of the topological descriptors for the first excited-state of the pyridinium-phenolate (PP), computed at the CAM-B3LYP/6-311G level of theory.  $\alpha$  is the pyridinium-phenolate central twist angle amplitude.

| $\alpha$ | $\phi_S^\ell$ | $\phi_S$ | $\varphi^\ell$ | $\varphi$ | $\psi^\ell$ | $\psi$ |
|----------|---------------|----------|----------------|-----------|-------------|--------|
| 0        | 0.66          | 0.70     | 0.67           | 0.63      | 0.50        | 0.53   |
| 1        | 0.66          | 0.70     | 0.67           | 0.63      | 0.50        | 0.53   |
| 2        | 0.66          | 0.70     | 0.67           | 0.63      | 0.50        | 0.53   |
| 3        | 0.66          | 0.70     | 0.67           | 0.63      | 0.50        | 0.53   |
| 4        | 0.66          | 0.70     | 0.67           | 0.63      | 0.50        | 0.53   |
| 5        | 0.66          | 0.70     | 0.67           | 0.63      | 0.50        | 0.53   |
| 6        | 0.66          | 0.70     | 0.67           | 0.63      | 0.50        | 0.53   |
| 7        | 0.66          | 0.70     | 0.67           | 0.64      | 0.50        | 0.53   |
| 8        | 0.65          | 0.70     | 0.67           | 0.64      | 0.49        | 0.53   |
| 9        | 0.65          | 0.70     | 0.67           | 0.64      | 0.49        | 0.53   |
| 10       | 0.65          | 0.70     | 0.67           | 0.64      | 0.49        | 0.53   |
| 11       | 0.65          | 0.70     | 0.67           | 0.64      | 0.49        | 0.53   |
| 12       | 0.65          | 0.70     | 0.68           | 0.64      | 0.49        | 0.53   |
| 13       | 0.65          | 0.69     | 0.68           | 0.64      | 0.49        | 0.52   |
| 14       | 0.65          | 0.69     | 0.68           | 0.65      | 0.49        | 0.52   |
| 15       | 0.65          | 0.69     | 0.68           | 0.65      | 0.49        | 0.52   |
| 16       | 0.65          | 0.69     | 0.68           | 0.65      | 0.49        | 0.52   |
| 17       | 0.65          | 0.69     | 0.68           | 0.65      | 0.49        | 0.52   |
| 18       | 0.65          | 0.69     | 0.69           | 0.65      | 0.48        | 0.52   |
| 19       | 0.64          | 0.69     | 0.69           | 0.66      | 0.48        | 0.51   |
| 20       | 0.64          | 0.68     | 0.69           | 0.66      | 0.48        | 0.51   |
| 21       | 0.64          | 0.68     | 0.69           | 0.66      | 0.48        | 0.51   |
| 22       | 0.64          | 0.68     | 0.70           | 0.66      | 0.47        | 0.51   |
| 23       | 0.64          | 0.68     | 0.70           | 0.67      | 0.47        | 0.50   |
| 24       | 0.64          | 0.68     | 0.70           | 0.67      | 0.47        | 0.50   |
| 25       | 0.64          | 0.67     | 0.70           | 0.67      | 0.47        | 0.50   |
| 26       | 0.63          | 0.67     | 0.71           | 0.68      | 0.46        | 0.50   |
| 27       | 0.63          | 0.67     | 0.71           | 0.68      | 0.46        | 0.50   |
| 28       | 0.63          | 0.67     | 0.71           | 0.68      | 0.46        | 0.50   |
| 29       | 0.63          | 0.66     | 0.72           | 0.69      | 0.46        | 0.49   |
| 30       | 0.63          | 0.66     | 0.72           | 0.69      | 0.46        | 0.49   |
| 31       | 0.62          | 0.66     | 0.72           | 0.69      | 0.45        | 0.49   |

Continued on next page

| $\alpha$ | $\phi_S^\ell$ | $\phi_S$ | $\varphi^\ell$ | $\varphi$ | $\psi^\ell$ | $\psi$ |
|----------|---------------|----------|----------------|-----------|-------------|--------|
| 32       | 0.62          | 0.66     | 0.72           | 0.70      | 0.45        | 0.48   |
| 33       | 0.62          | 0.65     | 0.73           | 0.70      | 0.45        | 0.48   |
| 34       | 0.62          | 0.65     | 0.73           | 0.70      | 0.45        | 0.48   |
| 35       | 0.61          | 0.65     | 0.74           | 0.71      | 0.44        | 0.47   |
| 36       | 0.61          | 0.64     | 0.74           | 0.71      | 0.44        | 0.47   |
| 37       | 0.61          | 0.64     | 0.74           | 0.72      | 0.44        | 0.46   |
| 38       | 0.60          | 0.64     | 0.75           | 0.72      | 0.43        | 0.46   |
| 39       | 0.60          | 0.63     | 0.75           | 0.72      | 0.43        | 0.46   |
| 40       | 0.60          | 0.63     | 0.76           | 0.73      | 0.43        | 0.45   |
| 41       | 0.59          | 0.62     | 0.76           | 0.73      | 0.42        | 0.45   |
| 42       | 0.59          | 0.62     | 0.76           | 0.74      | 0.42        | 0.44   |
| 43       | 0.59          | 0.62     | 0.77           | 0.74      | 0.42        | 0.44   |
| 44       | 0.58          | 0.61     | 0.77           | 0.74      | 0.41        | 0.44   |
| 45       | 0.58          | 0.61     | 0.78           | 0.75      | 0.41        | 0.43   |
| 46       | 0.57          | 0.60     | 0.78           | 0.75      | 0.40        | 0.43   |
| 47       | 0.57          | 0.60     | 0.79           | 0.76      | 0.40        | 0.43   |
| 48       | 0.57          | 0.59     | 0.79           | 0.76      | 0.40        | 0.42   |
| 49       | 0.56          | 0.59     | 0.79           | 0.77      | 0.39        | 0.42   |
| 50       | 0.56          | 0.58     | 0.80           | 0.77      | 0.39        | 0.41   |
| 51       | 0.55          | 0.58     | 0.80           | 0.78      | 0.38        | 0.41   |
| 52       | 0.54          | 0.57     | 0.81           | 0.78      | 0.37        | 0.40   |
| 53       | 0.54          | 0.56     | 0.81           | 0.79      | 0.37        | 0.39   |
| 54       | 0.53          | 0.56     | 0.82           | 0.79      | 0.37        | 0.39   |
| 55       | 0.53          | 0.55     | 0.82           | 0.80      | 0.37        | 0.38   |
| 56       | 0.52          | 0.55     | 0.83           | 0.80      | 0.36        | 0.38   |
| 57       | 0.51          | 0.54     | 0.83           | 0.81      | 0.35        | 0.37   |
| 58       | 0.51          | 0.53     | 0.83           | 0.81      | 0.35        | 0.37   |
| 59       | 0.50          | 0.52     | 0.84           | 0.82      | 0.34        | 0.36   |
| 60       | 0.49          | 0.52     | 0.84           | 0.82      | 0.34        | 0.36   |
| 61       | 0.49          | 0.51     | 0.85           | 0.83      | 0.33        | 0.35   |
| 62       | 0.48          | 0.50     | 0.85           | 0.83      | 0.33        | 0.35   |
| 63       | 0.47          | 0.49     | 0.86           | 0.84      | 0.32        | 0.34   |

Continued on next page

| $\alpha$ | $\phi_S^\ell$ | $\phi_S$ | $\varphi^\ell$ | $\varphi$ | $\psi^\ell$ | $\psi$ |
|----------|---------------|----------|----------------|-----------|-------------|--------|
| 64       | 0.46          | 0.48     | 0.87           | 0.84      | 0.31        | 0.33   |
| 65       | 0.45          | 0.48     | 0.87           | 0.85      | 0.30        | 0.33   |
| 66       | 0.44          | 0.47     | 0.88           | 0.85      | 0.30        | 0.32   |
| 67       | 0.43          | 0.46     | 0.88           | 0.86      | 0.29        | 0.31   |
| 68       | 0.42          | 0.45     | 0.89           | 0.86      | 0.28        | 0.31   |
| 69       | 0.41          | 0.44     | 0.89           | 0.87      | 0.27        | 0.30   |
| 70       | 0.40          | 0.43     | 0.90           | 0.87      | 0.27        | 0.29   |
| 71       | 0.39          | 0.42     | 0.90           | 0.88      | 0.26        | 0.28   |
| 72       | 0.38          | 0.40     | 0.91           | 0.89      | 0.25        | 0.27   |
| 73       | 0.37          | 0.39     | 0.91           | 0.89      | 0.25        | 0.26   |
| 74       | 0.35          | 0.38     | 0.92           | 0.90      | 0.23        | 0.25   |
| 75       | 0.34          | 0.37     | 0.92           | 0.90      | 0.23        | 0.25   |
| 76       | 0.33          | 0.35     | 0.93           | 0.91      | 0.22        | 0.23   |
| 77       | 0.31          | 0.34     | 0.93           | 0.91      | 0.20        | 0.23   |
| 78       | 0.30          | 0.32     | 0.94           | 0.92      | 0.20        | 0.21   |
| 79       | 0.28          | 0.31     | 0.94           | 0.92      | 0.18        | 0.21   |
| 80       | 0.27          | 0.29     | 0.95           | 0.93      | 0.18        | 0.19   |
| 81       | 0.25          | 0.28     | 0.95           | 0.93      | 0.16        | 0.19   |
| 82       | 0.23          | 0.26     | 0.96           | 0.94      | 0.15        | 0.17   |
| 83       | 0.21          | 0.25     | 0.96           | 0.94      | 0.14        | 0.17   |
| 84       | 0.20          | 0.23     | 0.96           | 0.94      | 0.13        | 0.15   |
| 85       | 0.18          | 0.21     | 0.97           | 0.95      | 0.12        | 0.14   |
| 86       | 0.17          | 0.20     | 0.97           | 0.95      | 0.11        | 0.13   |
| 87       | 0.15          | 0.19     | 0.97           | 0.95      | 0.10        | 0.13   |
| 88       | 0.14          | 0.17     | 0.97           | 0.95      | 0.09        | 0.11   |
| 89       | 0.13          | 0.16     | 0.97           | 0.95      | 0.08        | 0.11   |
| 90       | 0.13          | 0.16     | 0.97           | 0.96      | 0.08        | 0.11   |

Table S74: Reference ( $\phi_S$ ,  $\varphi$ ,  $\psi$ ) and approached ( $\phi_S^\ell$ ,  $\varphi^\ell$ ,  $\psi^\ell$ ) values of the topological descriptors for the first excited-state of the pyridinium-phenolate (PP), computed at the CAM-B3LYP/6-31++G(2d,p) level of theory.  $\alpha$  is the pyridinium-phenolate central twist angle amplitude.

| $\alpha$ | $\phi_S^\ell$ | $\phi_S$ | $\varphi^\ell$ | $\varphi$ | $\psi^\ell$ | $\psi$ |
|----------|---------------|----------|----------------|-----------|-------------|--------|
| 0        | 0.66          | 0.71     | 0.66           | 0.63      | 0.50        | 0.54   |
| 1        | 0.66          | 0.71     | 0.66           | 0.63      | 0.50        | 0.54   |
| 2        | 0.66          | 0.71     | 0.66           | 0.63      | 0.50        | 0.54   |
| 3        | 0.66          | 0.71     | 0.66           | 0.63      | 0.50        | 0.54   |
| 4        | 0.66          | 0.71     | 0.66           | 0.63      | 0.50        | 0.54   |
| 5        | 0.66          | 0.70     | 0.66           | 0.63      | 0.50        | 0.53   |
| 6        | 0.66          | 0.70     | 0.66           | 0.63      | 0.50        | 0.53   |
| 7        | 0.66          | 0.70     | 0.66           | 0.63      | 0.50        | 0.53   |
| 8        | 0.66          | 0.70     | 0.67           | 0.63      | 0.50        | 0.53   |
| 9        | 0.65          | 0.70     | 0.67           | 0.64      | 0.49        | 0.53   |
| 10       | 0.65          | 0.70     | 0.67           | 0.64      | 0.49        | 0.53   |
| 11       | 0.65          | 0.70     | 0.67           | 0.64      | 0.49        | 0.53   |
| 12       | 0.65          | 0.70     | 0.67           | 0.64      | 0.49        | 0.53   |
| 13       | 0.65          | 0.70     | 0.67           | 0.64      | 0.49        | 0.53   |
| 14       | 0.65          | 0.70     | 0.67           | 0.64      | 0.49        | 0.53   |
| 15       | 0.65          | 0.69     | 0.68           | 0.65      | 0.49        | 0.52   |
| 16       | 0.65          | 0.69     | 0.68           | 0.65      | 0.49        | 0.52   |
| 17       | 0.65          | 0.69     | 0.68           | 0.65      | 0.49        | 0.52   |
| 18       | 0.65          | 0.69     | 0.68           | 0.65      | 0.49        | 0.52   |
| 19       | 0.65          | 0.69     | 0.68           | 0.66      | 0.49        | 0.51   |
| 20       | 0.64          | 0.69     | 0.69           | 0.66      | 0.48        | 0.51   |
| 21       | 0.64          | 0.68     | 0.69           | 0.66      | 0.48        | 0.51   |
| 22       | 0.64          | 0.68     | 0.69           | 0.66      | 0.48        | 0.51   |
| 23       | 0.64          | 0.68     | 0.69           | 0.67      | 0.48        | 0.50   |
| 24       | 0.64          | 0.68     | 0.70           | 0.67      | 0.47        | 0.50   |
| 25       | 0.64          | 0.68     | 0.70           | 0.67      | 0.47        | 0.50   |
| 26       | 0.64          | 0.67     | 0.70           | 0.67      | 0.47        | 0.50   |
| 27       | 0.64          | 0.67     | 0.70           | 0.68      | 0.47        | 0.50   |
| 28       | 0.63          | 0.67     | 0.71           | 0.68      | 0.46        | 0.50   |
| 29       | 0.63          | 0.67     | 0.71           | 0.68      | 0.46        | 0.50   |
| 30       | 0.63          | 0.66     | 0.71           | 0.69      | 0.46        | 0.49   |
| 31       | 0.63          | 0.66     | 0.72           | 0.69      | 0.46        | 0.49   |

Continued on next page



| $\alpha$ | $\phi_S^\ell$ | $\phi_S$ | $\varphi^\ell$ | $\varphi$ | $\psi^\ell$ | $\psi$ |
|----------|---------------|----------|----------------|-----------|-------------|--------|
| 32       | 0.63          | 0.66     | 0.72           | 0.70      | 0.46        | 0.48   |
| 33       | 0.62          | 0.65     | 0.72           | 0.70      | 0.45        | 0.48   |
| 34       | 0.62          | 0.65     | 0.73           | 0.70      | 0.45        | 0.48   |
| 35       | 0.62          | 0.65     | 0.73           | 0.71      | 0.45        | 0.47   |
| 36       | 0.62          | 0.64     | 0.73           | 0.71      | 0.45        | 0.47   |
| 37       | 0.61          | 0.64     | 0.74           | 0.71      | 0.44        | 0.47   |
| 38       | 0.61          | 0.64     | 0.74           | 0.72      | 0.44        | 0.46   |
| 39       | 0.61          | 0.63     | 0.75           | 0.72      | 0.43        | 0.46   |
| 40       | 0.60          | 0.63     | 0.75           | 0.73      | 0.43        | 0.45   |
| 41       | 0.60          | 0.63     | 0.75           | 0.73      | 0.43        | 0.45   |
| 42       | 0.60          | 0.62     | 0.76           | 0.73      | 0.43        | 0.45   |
| 43       | 0.59          | 0.62     | 0.76           | 0.74      | 0.42        | 0.44   |
| 44       | 0.59          | 0.61     | 0.77           | 0.74      | 0.42        | 0.44   |
| 45       | 0.58          | 0.61     | 0.77           | 0.75      | 0.41        | 0.43   |
| 46       | 0.58          | 0.60     | 0.78           | 0.75      | 0.41        | 0.43   |
| 47       | 0.58          | 0.60     | 0.78           | 0.76      | 0.41        | 0.43   |
| 48       | 0.57          | 0.59     | 0.78           | 0.76      | 0.40        | 0.42   |
| 49       | 0.57          | 0.59     | 0.79           | 0.77      | 0.40        | 0.42   |
| 50       | 0.56          | 0.58     | 0.79           | 0.77      | 0.39        | 0.41   |
| 51       | 0.56          | 0.58     | 0.80           | 0.78      | 0.39        | 0.41   |
| 52       | 0.55          | 0.57     | 0.80           | 0.78      | 0.38        | 0.40   |
| 53       | 0.54          | 0.57     | 0.81           | 0.78      | 0.37        | 0.40   |
| 54       | 0.54          | 0.56     | 0.81           | 0.79      | 0.37        | 0.39   |
| 55       | 0.53          | 0.55     | 0.82           | 0.79      | 0.37        | 0.39   |
| 56       | 0.53          | 0.55     | 0.82           | 0.80      | 0.37        | 0.38   |
| 57       | 0.52          | 0.54     | 0.82           | 0.80      | 0.36        | 0.38   |
| 58       | 0.51          | 0.53     | 0.83           | 0.81      | 0.35        | 0.37   |
| 59       | 0.51          | 0.53     | 0.83           | 0.82      | 0.35        | 0.37   |
| 60       | 0.50          | 0.52     | 0.84           | 0.82      | 0.34        | 0.36   |
| 61       | 0.49          | 0.51     | 0.84           | 0.83      | 0.34        | 0.35   |
| 62       | 0.48          | 0.50     | 0.85           | 0.83      | 0.33        | 0.35   |
| 63       | 0.47          | 0.50     | 0.86           | 0.84      | 0.32        | 0.34   |

Continued on next page

| $\alpha$ | $\phi_S^\ell$ | $\phi_S$ | $\varphi^\ell$ | $\varphi$ | $\psi^\ell$ | $\psi$ |
|----------|---------------|----------|----------------|-----------|-------------|--------|
| 64       | 0.47          | 0.49     | 0.86           | 0.84      | 0.32        | 0.34   |
| 65       | 0.46          | 0.48     | 0.87           | 0.85      | 0.31        | 0.33   |
| 66       | 0.45          | 0.47     | 0.87           | 0.85      | 0.30        | 0.32   |
| 67       | 0.44          | 0.46     | 0.88           | 0.86      | 0.30        | 0.31   |
| 68       | 0.43          | 0.45     | 0.88           | 0.86      | 0.29        | 0.31   |
| 69       | 0.42          | 0.44     | 0.89           | 0.87      | 0.28        | 0.30   |
| 70       | 0.41          | 0.43     | 0.90           | 0.87      | 0.27        | 0.29   |
| 71       | 0.39          | 0.42     | 0.90           | 0.88      | 0.26        | 0.28   |
| 72       | 0.38          | 0.41     | 0.91           | 0.88      | 0.25        | 0.28   |
| 73       | 0.37          | 0.39     | 0.91           | 0.89      | 0.25        | 0.26   |
| 74       | 0.36          | 0.38     | 0.92           | 0.90      | 0.24        | 0.25   |
| 75       | 0.34          | 0.37     | 0.92           | 0.90      | 0.23        | 0.25   |
| 76       | 0.33          | 0.35     | 0.93           | 0.91      | 0.22        | 0.23   |
| 77       | 0.31          | 0.34     | 0.93           | 0.91      | 0.20        | 0.23   |
| 78       | 0.30          | 0.33     | 0.94           | 0.92      | 0.20        | 0.22   |
| 79       | 0.28          | 0.31     | 0.94           | 0.92      | 0.18        | 0.21   |
| 80       | 0.26          | 0.30     | 0.95           | 0.93      | 0.17        | 0.20   |
| 81       | 0.25          | 0.28     | 0.95           | 0.93      | 0.16        | 0.19   |
| 82       | 0.23          | 0.26     | 0.96           | 0.94      | 0.15        | 0.17   |
| 83       | 0.21          | 0.25     | 0.96           | 0.94      | 0.14        | 0.17   |
| 84       | 0.19          | 0.23     | 0.96           | 0.94      | 0.12        | 0.15   |
| 85       | 0.18          | 0.22     | 0.97           | 0.95      | 0.12        | 0.14   |
| 86       | 0.16          | 0.20     | 0.97           | 0.95      | 0.10        | 0.13   |
| 87       | 0.15          | 0.19     | 0.97           | 0.95      | 0.10        | 0.13   |
| 88       | 0.14          | 0.17     | 0.98           | 0.95      | 0.09        | 0.11   |
| 89       | 0.13          | 0.16     | 0.98           | 0.96      | 0.08        | 0.11   |
| 90       | 0.12          | 0.16     | 0.98           | 0.96      | 0.08        | 0.11   |

Table S75: Reference ( $\phi_S$ ,  $\varphi$ ,  $\psi$ ) and approached ( $\phi_S^\ell$ ,  $\varphi^\ell$ ,  $\psi^\ell$ ) values of the topological descriptors for the first excited-state of the pyridinium-phenolate (PP), computed at the CAM-B3LYP/6-31++G(d,p) level of theory.  $\alpha$  is the pyridinium-phenolate central twist angle amplitude.

| $\alpha$ | $\phi_S^\ell$ | $\phi_S$ | $\varphi^\ell$ | $\varphi$ | $\psi^\ell$ | $\psi$ |
|----------|---------------|----------|----------------|-----------|-------------|--------|
| 0        | 0.66          | 0.71     | 0.66           | 0.63      | 0.50        | 0.54   |
| 1        | 0.66          | 0.71     | 0.66           | 0.63      | 0.50        | 0.54   |
| 2        | 0.66          | 0.71     | 0.66           | 0.63      | 0.50        | 0.54   |
| 3        | 0.66          | 0.71     | 0.66           | 0.63      | 0.50        | 0.54   |
| 4        | 0.66          | 0.71     | 0.66           | 0.63      | 0.50        | 0.54   |
| 5        | 0.66          | 0.70     | 0.66           | 0.63      | 0.50        | 0.54   |
| 6        | 0.66          | 0.70     | 0.66           | 0.63      | 0.50        | 0.53   |
| 7        | 0.66          | 0.70     | 0.66           | 0.63      | 0.50        | 0.53   |
| 8        | 0.66          | 0.70     | 0.67           | 0.63      | 0.50        | 0.53   |
| 9        | 0.66          | 0.70     | 0.67           | 0.64      | 0.49        | 0.53   |
| 10       | 0.65          | 0.70     | 0.67           | 0.64      | 0.49        | 0.53   |
| 11       | 0.65          | 0.70     | 0.67           | 0.64      | 0.49        | 0.53   |
| 12       | 0.65          | 0.70     | 0.67           | 0.64      | 0.49        | 0.53   |
| 13       | 0.65          | 0.70     | 0.67           | 0.64      | 0.49        | 0.53   |
| 14       | 0.65          | 0.70     | 0.67           | 0.64      | 0.49        | 0.52   |
| 15       | 0.65          | 0.69     | 0.68           | 0.65      | 0.49        | 0.52   |
| 16       | 0.65          | 0.69     | 0.68           | 0.65      | 0.49        | 0.52   |
| 17       | 0.65          | 0.69     | 0.68           | 0.65      | 0.49        | 0.52   |
| 18       | 0.65          | 0.69     | 0.68           | 0.65      | 0.48        | 0.52   |
| 19       | 0.65          | 0.69     | 0.68           | 0.66      | 0.48        | 0.52   |
| 20       | 0.65          | 0.69     | 0.69           | 0.66      | 0.48        | 0.51   |
| 21       | 0.64          | 0.68     | 0.69           | 0.66      | 0.48        | 0.51   |
| 22       | 0.64          | 0.68     | 0.69           | 0.66      | 0.48        | 0.51   |
| 23       | 0.64          | 0.68     | 0.69           | 0.67      | 0.48        | 0.51   |
| 24       | 0.64          | 0.68     | 0.70           | 0.67      | 0.47        | 0.50   |
| 25       | 0.64          | 0.68     | 0.70           | 0.67      | 0.47        | 0.50   |
| 26       | 0.64          | 0.67     | 0.70           | 0.67      | 0.47        | 0.50   |
| 27       | 0.64          | 0.67     | 0.70           | 0.68      | 0.47        | 0.50   |
| 28       | 0.63          | 0.67     | 0.71           | 0.68      | 0.46        | 0.49   |
| 29       | 0.63          | 0.67     | 0.71           | 0.68      | 0.46        | 0.49   |
| 30       | 0.63          | 0.66     | 0.71           | 0.69      | 0.46        | 0.49   |
| 31       | 0.63          | 0.66     | 0.72           | 0.69      | 0.46        | 0.49   |

Continued on next page

| $\alpha$ | $\phi_S^\ell$ | $\phi_S$ | $\varphi^\ell$ | $\varphi$ | $\psi^\ell$ | $\psi$ |
|----------|---------------|----------|----------------|-----------|-------------|--------|
| 32       | 0.63          | 0.66     | 0.72           | 0.70      | 0.46        | 0.48   |
| 33       | 0.62          | 0.65     | 0.72           | 0.70      | 0.45        | 0.48   |
| 34       | 0.62          | 0.65     | 0.73           | 0.70      | 0.45        | 0.48   |
| 35       | 0.62          | 0.65     | 0.73           | 0.71      | 0.45        | 0.47   |
| 36       | 0.62          | 0.64     | 0.73           | 0.71      | 0.44        | 0.47   |
| 37       | 0.61          | 0.64     | 0.74           | 0.71      | 0.44        | 0.47   |
| 38       | 0.61          | 0.64     | 0.74           | 0.72      | 0.44        | 0.46   |
| 39       | 0.61          | 0.63     | 0.75           | 0.72      | 0.43        | 0.46   |
| 40       | 0.60          | 0.63     | 0.75           | 0.73      | 0.43        | 0.46   |
| 41       | 0.60          | 0.63     | 0.75           | 0.73      | 0.43        | 0.45   |
| 42       | 0.60          | 0.62     | 0.76           | 0.73      | 0.42        | 0.45   |
| 43       | 0.59          | 0.62     | 0.76           | 0.74      | 0.42        | 0.44   |
| 44       | 0.59          | 0.61     | 0.77           | 0.74      | 0.42        | 0.44   |
| 45       | 0.58          | 0.61     | 0.77           | 0.75      | 0.41        | 0.44   |
| 46       | 0.58          | 0.60     | 0.78           | 0.75      | 0.41        | 0.43   |
| 47       | 0.57          | 0.60     | 0.78           | 0.76      | 0.40        | 0.43   |
| 48       | 0.57          | 0.59     | 0.78           | 0.76      | 0.40        | 0.42   |
| 49       | 0.57          | 0.59     | 0.79           | 0.77      | 0.40        | 0.42   |
| 50       | 0.56          | 0.58     | 0.79           | 0.77      | 0.39        | 0.41   |
| 51       | 0.56          | 0.58     | 0.80           | 0.78      | 0.39        | 0.41   |
| 52       | 0.55          | 0.57     | 0.80           | 0.78      | 0.38        | 0.40   |
| 53       | 0.54          | 0.57     | 0.81           | 0.78      | 0.38        | 0.40   |
| 54       | 0.54          | 0.56     | 0.81           | 0.79      | 0.37        | 0.39   |
| 55       | 0.53          | 0.55     | 0.82           | 0.79      | 0.37        | 0.39   |
| 56       | 0.53          | 0.55     | 0.82           | 0.80      | 0.36        | 0.38   |
| 57       | 0.52          | 0.54     | 0.82           | 0.80      | 0.36        | 0.38   |
| 58       | 0.51          | 0.53     | 0.83           | 0.81      | 0.35        | 0.37   |
| 59       | 0.51          | 0.53     | 0.83           | 0.81      | 0.35        | 0.37   |
| 60       | 0.50          | 0.52     | 0.84           | 0.82      | 0.34        | 0.36   |
| 61       | 0.49          | 0.51     | 0.84           | 0.83      | 0.34        | 0.35   |
| 62       | 0.48          | 0.50     | 0.85           | 0.83      | 0.33        | 0.35   |
| 63       | 0.47          | 0.50     | 0.86           | 0.84      | 0.32        | 0.34   |

Continued on next page

| $\alpha$ | $\phi_S^\ell$ | $\phi_S$ | $\varphi^\ell$ | $\varphi$ | $\psi^\ell$ | $\psi$ |
|----------|---------------|----------|----------------|-----------|-------------|--------|
| 64       | 0.47          | 0.49     | 0.86           | 0.84      | 0.32        | 0.33   |
| 65       | 0.46          | 0.48     | 0.87           | 0.85      | 0.31        | 0.33   |
| 66       | 0.45          | 0.47     | 0.87           | 0.85      | 0.30        | 0.32   |
| 67       | 0.44          | 0.46     | 0.88           | 0.86      | 0.29        | 0.31   |
| 68       | 0.43          | 0.45     | 0.88           | 0.86      | 0.29        | 0.31   |
| 69       | 0.42          | 0.44     | 0.89           | 0.87      | 0.28        | 0.30   |
| 70       | 0.41          | 0.43     | 0.89           | 0.87      | 0.27        | 0.29   |
| 71       | 0.39          | 0.42     | 0.90           | 0.88      | 0.26        | 0.28   |
| 72       | 0.38          | 0.41     | 0.91           | 0.88      | 0.25        | 0.27   |
| 73       | 0.37          | 0.39     | 0.91           | 0.89      | 0.24        | 0.27   |
| 74       | 0.36          | 0.38     | 0.92           | 0.90      | 0.24        | 0.26   |
| 75       | 0.34          | 0.37     | 0.92           | 0.90      | 0.23        | 0.25   |
| 76       | 0.33          | 0.35     | 0.93           | 0.91      | 0.22        | 0.24   |
| 77       | 0.31          | 0.34     | 0.93           | 0.91      | 0.21        | 0.23   |
| 78       | 0.30          | 0.33     | 0.94           | 0.92      | 0.20        | 0.22   |
| 79       | 0.28          | 0.31     | 0.94           | 0.92      | 0.18        | 0.21   |
| 80       | 0.26          | 0.30     | 0.95           | 0.93      | 0.17        | 0.20   |
| 81       | 0.25          | 0.28     | 0.95           | 0.93      | 0.16        | 0.19   |
| 82       | 0.23          | 0.26     | 0.96           | 0.94      | 0.15        | 0.18   |
| 83       | 0.21          | 0.25     | 0.96           | 0.94      | 0.14        | 0.16   |
| 84       | 0.20          | 0.23     | 0.96           | 0.94      | 0.13        | 0.15   |
| 85       | 0.18          | 0.22     | 0.97           | 0.95      | 0.12        | 0.14   |
| 86       | 0.17          | 0.20     | 0.97           | 0.95      | 0.11        | 0.13   |
| 87       | 0.15          | 0.19     | 0.97           | 0.95      | 0.10        | 0.12   |
| 88       | 0.14          | 0.17     | 0.97           | 0.95      | 0.09        | 0.11   |
| 89       | 0.13          | 0.16     | 0.98           | 0.96      | 0.08        | 0.11   |
| 90       | 0.12          | 0.16     | 0.98           | 0.96      | 0.08        | 0.11   |

Table S76: Reference ( $\phi_S$ ,  $\varphi$ ,  $\psi$ ) and approached ( $\phi_S^\ell$ ,  $\varphi^\ell$ ,  $\psi^\ell$ ) values of the topological descriptors for the first excited-state of the pyridinium-phenolate (PP), computed at the CAM-B3LYP/6-31+G(d,p) level of theory.  $\alpha$  is the pyridinium-phenolate central twist angle amplitude.

| $\alpha$ | $\phi_S^\ell$ | $\phi_S$ | $\varphi^\ell$ | $\varphi$ | $\psi^\ell$ | $\psi$ |
|----------|---------------|----------|----------------|-----------|-------------|--------|
| 0        | 0.66          | 0.71     | 0.66           | 0.63      | 0.50        | 0.54   |
| 1        | 0.66          | 0.71     | 0.66           | 0.63      | 0.50        | 0.54   |
| 2        | 0.66          | 0.71     | 0.66           | 0.63      | 0.50        | 0.54   |
| 3        | 0.66          | 0.71     | 0.66           | 0.63      | 0.50        | 0.54   |
| 4        | 0.66          | 0.71     | 0.66           | 0.63      | 0.50        | 0.54   |
| 5        | 0.66          | 0.70     | 0.66           | 0.63      | 0.50        | 0.53   |
| 6        | 0.66          | 0.70     | 0.66           | 0.63      | 0.50        | 0.53   |
| 7        | 0.66          | 0.70     | 0.67           | 0.63      | 0.50        | 0.53   |
| 8        | 0.66          | 0.70     | 0.67           | 0.64      | 0.50        | 0.53   |
| 9        | 0.65          | 0.70     | 0.67           | 0.64      | 0.49        | 0.53   |
| 10       | 0.65          | 0.70     | 0.67           | 0.64      | 0.49        | 0.53   |
| 11       | 0.65          | 0.70     | 0.67           | 0.64      | 0.49        | 0.53   |
| 12       | 0.65          | 0.70     | 0.67           | 0.64      | 0.49        | 0.53   |
| 13       | 0.65          | 0.70     | 0.67           | 0.64      | 0.49        | 0.53   |
| 14       | 0.65          | 0.70     | 0.67           | 0.64      | 0.49        | 0.53   |
| 15       | 0.65          | 0.69     | 0.68           | 0.65      | 0.49        | 0.52   |
| 16       | 0.65          | 0.69     | 0.68           | 0.65      | 0.49        | 0.52   |
| 17       | 0.65          | 0.69     | 0.68           | 0.65      | 0.49        | 0.52   |
| 18       | 0.65          | 0.69     | 0.68           | 0.65      | 0.49        | 0.52   |
| 19       | 0.65          | 0.69     | 0.68           | 0.66      | 0.49        | 0.51   |
| 20       | 0.64          | 0.69     | 0.69           | 0.66      | 0.48        | 0.51   |
| 21       | 0.64          | 0.68     | 0.69           | 0.66      | 0.48        | 0.51   |
| 22       | 0.64          | 0.68     | 0.69           | 0.66      | 0.48        | 0.51   |
| 23       | 0.64          | 0.68     | 0.69           | 0.67      | 0.48        | 0.50   |
| 24       | 0.64          | 0.68     | 0.70           | 0.67      | 0.47        | 0.50   |
| 25       | 0.64          | 0.68     | 0.70           | 0.67      | 0.47        | 0.50   |
| 26       | 0.64          | 0.67     | 0.70           | 0.68      | 0.47        | 0.50   |
| 27       | 0.63          | 0.67     | 0.71           | 0.68      | 0.46        | 0.50   |
| 28       | 0.63          | 0.67     | 0.71           | 0.68      | 0.46        | 0.50   |
| 29       | 0.63          | 0.67     | 0.71           | 0.69      | 0.46        | 0.49   |
| 30       | 0.63          | 0.66     | 0.71           | 0.69      | 0.46        | 0.49   |
| 31       | 0.63          | 0.66     | 0.72           | 0.69      | 0.46        | 0.49   |

Continued on next page

| $\alpha$ | $\phi_S^\ell$ | $\phi_S$ | $\varphi^\ell$ | $\varphi$ | $\psi^\ell$ | $\psi$ |
|----------|---------------|----------|----------------|-----------|-------------|--------|
| 32       | 0.63          | 0.66     | 0.72           | 0.70      | 0.46        | 0.48   |
| 33       | 0.62          | 0.65     | 0.72           | 0.70      | 0.45        | 0.48   |
| 34       | 0.62          | 0.65     | 0.73           | 0.70      | 0.45        | 0.48   |
| 35       | 0.62          | 0.65     | 0.73           | 0.71      | 0.45        | 0.47   |
| 36       | 0.62          | 0.64     | 0.73           | 0.71      | 0.45        | 0.47   |
| 37       | 0.61          | 0.64     | 0.74           | 0.71      | 0.44        | 0.47   |
| 38       | 0.61          | 0.64     | 0.74           | 0.72      | 0.44        | 0.46   |
| 39       | 0.61          | 0.63     | 0.75           | 0.72      | 0.43        | 0.46   |
| 40       | 0.60          | 0.63     | 0.75           | 0.73      | 0.43        | 0.45   |
| 41       | 0.60          | 0.63     | 0.75           | 0.73      | 0.43        | 0.45   |
| 42       | 0.60          | 0.62     | 0.76           | 0.74      | 0.43        | 0.44   |
| 43       | 0.59          | 0.62     | 0.76           | 0.74      | 0.42        | 0.44   |
| 44       | 0.59          | 0.61     | 0.77           | 0.74      | 0.42        | 0.44   |
| 45       | 0.58          | 0.61     | 0.77           | 0.75      | 0.41        | 0.43   |
| 46       | 0.58          | 0.60     | 0.78           | 0.75      | 0.41        | 0.43   |
| 47       | 0.57          | 0.60     | 0.78           | 0.76      | 0.40        | 0.43   |
| 48       | 0.57          | 0.59     | 0.79           | 0.76      | 0.40        | 0.42   |
| 49       | 0.57          | 0.59     | 0.79           | 0.77      | 0.40        | 0.42   |
| 50       | 0.56          | 0.58     | 0.79           | 0.77      | 0.39        | 0.41   |
| 51       | 0.56          | 0.58     | 0.80           | 0.78      | 0.39        | 0.41   |
| 52       | 0.55          | 0.57     | 0.80           | 0.78      | 0.38        | 0.40   |
| 53       | 0.54          | 0.57     | 0.81           | 0.79      | 0.37        | 0.40   |
| 54       | 0.54          | 0.56     | 0.81           | 0.79      | 0.37        | 0.39   |
| 55       | 0.53          | 0.55     | 0.82           | 0.80      | 0.37        | 0.38   |
| 56       | 0.53          | 0.55     | 0.82           | 0.80      | 0.37        | 0.38   |
| 57       | 0.52          | 0.54     | 0.83           | 0.81      | 0.36        | 0.37   |
| 58       | 0.51          | 0.53     | 0.83           | 0.81      | 0.35        | 0.37   |
| 59       | 0.51          | 0.53     | 0.84           | 0.82      | 0.35        | 0.37   |
| 60       | 0.50          | 0.52     | 0.84           | 0.82      | 0.34        | 0.36   |
| 61       | 0.49          | 0.51     | 0.85           | 0.83      | 0.33        | 0.35   |
| 62       | 0.48          | 0.50     | 0.85           | 0.83      | 0.33        | 0.35   |
| 63       | 0.47          | 0.50     | 0.86           | 0.84      | 0.32        | 0.34   |

Continued on next page

| $\alpha$ | $\phi_S^\ell$ | $\phi_S$ | $\varphi^\ell$ | $\varphi$ | $\psi^\ell$ | $\psi$ |
|----------|---------------|----------|----------------|-----------|-------------|--------|
| 64       | 0.47          | 0.49     | 0.86           | 0.84      | 0.32        | 0.34   |
| 65       | 0.46          | 0.48     | 0.87           | 0.85      | 0.31        | 0.33   |
| 66       | 0.45          | 0.47     | 0.87           | 0.85      | 0.30        | 0.32   |
| 67       | 0.44          | 0.46     | 0.88           | 0.86      | 0.30        | 0.31   |
| 68       | 0.43          | 0.45     | 0.88           | 0.86      | 0.29        | 0.31   |
| 69       | 0.42          | 0.44     | 0.89           | 0.87      | 0.28        | 0.30   |
| 70       | 0.40          | 0.43     | 0.90           | 0.87      | 0.27        | 0.29   |
| 71       | 0.39          | 0.42     | 0.90           | 0.88      | 0.26        | 0.28   |
| 72       | 0.38          | 0.41     | 0.91           | 0.89      | 0.25        | 0.27   |
| 73       | 0.37          | 0.39     | 0.91           | 0.89      | 0.25        | 0.26   |
| 74       | 0.36          | 0.38     | 0.92           | 0.90      | 0.24        | 0.25   |
| 75       | 0.34          | 0.37     | 0.92           | 0.90      | 0.23        | 0.25   |
| 76       | 0.33          | 0.35     | 0.93           | 0.91      | 0.22        | 0.23   |
| 77       | 0.31          | 0.34     | 0.93           | 0.91      | 0.20        | 0.23   |
| 78       | 0.30          | 0.33     | 0.94           | 0.92      | 0.20        | 0.22   |
| 79       | 0.28          | 0.31     | 0.94           | 0.92      | 0.18        | 0.21   |
| 80       | 0.26          | 0.30     | 0.95           | 0.93      | 0.17        | 0.20   |
| 81       | 0.25          | 0.28     | 0.95           | 0.93      | 0.16        | 0.19   |
| 82       | 0.23          | 0.26     | 0.96           | 0.94      | 0.15        | 0.17   |
| 83       | 0.21          | 0.25     | 0.96           | 0.94      | 0.14        | 0.17   |
| 84       | 0.20          | 0.23     | 0.96           | 0.94      | 0.13        | 0.15   |
| 85       | 0.18          | 0.21     | 0.97           | 0.95      | 0.12        | 0.14   |
| 86       | 0.16          | 0.20     | 0.97           | 0.95      | 0.10        | 0.13   |
| 87       | 0.15          | 0.18     | 0.97           | 0.95      | 0.10        | 0.12   |
| 88       | 0.14          | 0.17     | 0.97           | 0.95      | 0.09        | 0.11   |
| 89       | 0.13          | 0.16     | 0.98           | 0.96      | 0.08        | 0.11   |
| 90       | 0.12          | 0.16     | 0.98           | 0.96      | 0.08        | 0.11   |

Table S77: Reference ( $\phi_S$ ,  $\varphi$ ,  $\psi$ ) and approached ( $\phi_S^\ell$ ,  $\varphi^\ell$ ,  $\psi^\ell$ ) values of the topological descriptors for the first excited-state of the pyridinium-phenolate (PP), computed at the CAM-B3LYP/6-31+G(d) level of theory.  $\alpha$  is the pyridinium-phenolate central twist angle amplitude.



| $\alpha$ | $\phi_S^\ell$ | $\phi_S$ | $\varphi^\ell$ | $\varphi$ | $\psi^\ell$ | $\psi$ |
|----------|---------------|----------|----------------|-----------|-------------|--------|
| 0        | 0.69          | 0.73     | 0.65           | 0.61      | 0.52        | 0.56   |
| 1        | 0.69          | 0.73     | 0.65           | 0.61      | 0.52        | 0.56   |
| 2        | 0.69          | 0.73     | 0.65           | 0.61      | 0.52        | 0.56   |
| 3        | 0.69          | 0.73     | 0.65           | 0.61      | 0.52        | 0.56   |
| 4        | 0.69          | 0.73     | 0.65           | 0.61      | 0.52        | 0.56   |
| 5        | 0.69          | 0.73     | 0.65           | 0.61      | 0.52        | 0.56   |
| 6        | 0.69          | 0.73     | 0.65           | 0.62      | 0.52        | 0.55   |
| 7        | 0.69          | 0.73     | 0.65           | 0.62      | 0.52        | 0.55   |
| 8        | 0.69          | 0.72     | 0.65           | 0.62      | 0.52        | 0.55   |
| 9        | 0.69          | 0.72     | 0.65           | 0.62      | 0.52        | 0.55   |
| 10       | 0.69          | 0.72     | 0.66           | 0.62      | 0.51        | 0.55   |
| 11       | 0.69          | 0.72     | 0.66           | 0.62      | 0.51        | 0.55   |
| 12       | 0.68          | 0.72     | 0.66           | 0.62      | 0.51        | 0.55   |
| 13       | 0.68          | 0.72     | 0.66           | 0.62      | 0.51        | 0.55   |
| 14       | 0.68          | 0.72     | 0.66           | 0.63      | 0.51        | 0.54   |
| 15       | 0.68          | 0.72     | 0.66           | 0.63      | 0.51        | 0.54   |
| 16       | 0.68          | 0.71     | 0.66           | 0.63      | 0.51        | 0.54   |
| 17       | 0.68          | 0.71     | 0.67           | 0.63      | 0.50        | 0.54   |
| 18       | 0.68          | 0.71     | 0.67           | 0.64      | 0.50        | 0.53   |
| 19       | 0.68          | 0.71     | 0.67           | 0.64      | 0.50        | 0.53   |
| 20       | 0.67          | 0.71     | 0.67           | 0.64      | 0.50        | 0.53   |
| 21       | 0.67          | 0.71     | 0.67           | 0.64      | 0.50        | 0.53   |
| 22       | 0.67          | 0.70     | 0.68           | 0.65      | 0.50        | 0.52   |
| 23       | 0.67          | 0.70     | 0.68           | 0.65      | 0.50        | 0.52   |
| 24       | 0.67          | 0.70     | 0.68           | 0.65      | 0.50        | 0.52   |
| 25       | 0.67          | 0.70     | 0.68           | 0.65      | 0.50        | 0.52   |
| 26       | 0.67          | 0.70     | 0.69           | 0.66      | 0.49        | 0.52   |
| 27       | 0.66          | 0.69     | 0.69           | 0.66      | 0.49        | 0.51   |
| 28       | 0.66          | 0.69     | 0.69           | 0.66      | 0.49        | 0.51   |
| 29       | 0.66          | 0.69     | 0.70           | 0.67      | 0.48        | 0.51   |
| 30       | 0.66          | 0.69     | 0.70           | 0.67      | 0.48        | 0.51   |
| 31       | 0.66          | 0.68     | 0.70           | 0.67      | 0.48        | 0.50   |

Continued on next page

| $\alpha$ | $\phi_S^\ell$ | $\phi_S$ | $\varphi^\ell$ | $\varphi$ | $\psi^\ell$ | $\psi$ |
|----------|---------------|----------|----------------|-----------|-------------|--------|
| 32       | 0.66          | 0.68     | 0.70           | 0.68      | 0.48        | 0.50   |
| 33       | 0.65          | 0.68     | 0.71           | 0.68      | 0.47        | 0.50   |
| 34       | 0.65          | 0.68     | 0.71           | 0.68      | 0.47        | 0.50   |
| 35       | 0.65          | 0.67     | 0.71           | 0.69      | 0.47        | 0.49   |
| 36       | 0.65          | 0.67     | 0.72           | 0.69      | 0.47        | 0.49   |
| 37       | 0.64          | 0.67     | 0.72           | 0.70      | 0.46        | 0.49   |
| 38       | 0.64          | 0.66     | 0.73           | 0.70      | 0.46        | 0.48   |
| 39       | 0.64          | 0.66     | 0.73           | 0.70      | 0.46        | 0.48   |
| 40       | 0.63          | 0.66     | 0.73           | 0.71      | 0.45        | 0.48   |
| 41       | 0.63          | 0.65     | 0.74           | 0.71      | 0.45        | 0.47   |
| 42       | 0.63          | 0.65     | 0.74           | 0.72      | 0.45        | 0.47   |
| 43       | 0.62          | 0.64     | 0.75           | 0.72      | 0.44        | 0.46   |
| 44       | 0.62          | 0.64     | 0.75           | 0.73      | 0.44        | 0.46   |
| 45       | 0.62          | 0.64     | 0.75           | 0.73      | 0.44        | 0.46   |
| 46       | 0.61          | 0.63     | 0.76           | 0.73      | 0.43        | 0.45   |
| 47       | 0.61          | 0.63     | 0.76           | 0.74      | 0.43        | 0.45   |
| 48       | 0.60          | 0.62     | 0.77           | 0.74      | 0.42        | 0.44   |
| 49       | 0.60          | 0.62     | 0.77           | 0.75      | 0.42        | 0.44   |
| 50       | 0.59          | 0.61     | 0.78           | 0.75      | 0.41        | 0.43   |
| 51       | 0.59          | 0.61     | 0.78           | 0.76      | 0.41        | 0.43   |
| 52       | 0.58          | 0.60     | 0.78           | 0.76      | 0.41        | 0.43   |
| 53       | 0.58          | 0.60     | 0.79           | 0.77      | 0.40        | 0.42   |
| 54       | 0.57          | 0.59     | 0.79           | 0.77      | 0.40        | 0.42   |
| 55       | 0.57          | 0.58     | 0.80           | 0.78      | 0.39        | 0.41   |
| 56       | 0.56          | 0.58     | 0.80           | 0.78      | 0.39        | 0.41   |
| 57       | 0.56          | 0.57     | 0.81           | 0.79      | 0.39        | 0.40   |
| 58       | 0.55          | 0.56     | 0.81           | 0.79      | 0.38        | 0.39   |
| 59       | 0.54          | 0.56     | 0.82           | 0.80      | 0.37        | 0.39   |
| 60       | 0.54          | 0.55     | 0.82           | 0.80      | 0.37        | 0.38   |
| 61       | 0.53          | 0.54     | 0.83           | 0.81      | 0.36        | 0.37   |
| 62       | 0.52          | 0.54     | 0.83           | 0.81      | 0.36        | 0.37   |
| 63       | 0.51          | 0.53     | 0.84           | 0.82      | 0.35        | 0.37   |

Continued on next page

| $\alpha$ | $\phi_S^\ell$ | $\phi_S$ | $\varphi^\ell$ | $\varphi$ | $\psi^\ell$ | $\psi$ |
|----------|---------------|----------|----------------|-----------|-------------|--------|
| 64       | 0.51          | 0.52     | 0.84           | 0.82      | 0.35        | 0.36   |
| 65       | 0.50          | 0.51     | 0.85           | 0.83      | 0.34        | 0.35   |
| 66       | 0.49          | 0.50     | 0.85           | 0.83      | 0.33        | 0.35   |
| 67       | 0.48          | 0.49     | 0.86           | 0.84      | 0.32        | 0.34   |
| 68       | 0.47          | 0.48     | 0.87           | 0.85      | 0.32        | 0.33   |
| 69       | 0.46          | 0.47     | 0.87           | 0.85      | 0.31        | 0.32   |
| 70       | 0.45          | 0.46     | 0.88           | 0.86      | 0.30        | 0.31   |
| 71       | 0.44          | 0.45     | 0.88           | 0.86      | 0.30        | 0.31   |
| 72       | 0.42          | 0.44     | 0.89           | 0.87      | 0.28        | 0.30   |
| 73       | 0.41          | 0.43     | 0.90           | 0.87      | 0.27        | 0.29   |
| 74       | 0.40          | 0.42     | 0.90           | 0.88      | 0.27        | 0.28   |
| 75       | 0.38          | 0.40     | 0.91           | 0.89      | 0.25        | 0.27   |
| 76       | 0.37          | 0.39     | 0.91           | 0.89      | 0.25        | 0.26   |
| 77       | 0.35          | 0.38     | 0.92           | 0.90      | 0.23        | 0.25   |
| 78       | 0.34          | 0.36     | 0.93           | 0.91      | 0.22        | 0.24   |
| 79       | 0.32          | 0.35     | 0.93           | 0.91      | 0.21        | 0.23   |
| 80       | 0.30          | 0.33     | 0.94           | 0.92      | 0.20        | 0.22   |
| 81       | 0.28          | 0.31     | 0.94           | 0.92      | 0.18        | 0.21   |
| 82       | 0.26          | 0.29     | 0.95           | 0.93      | 0.17        | 0.19   |
| 83       | 0.24          | 0.27     | 0.96           | 0.93      | 0.16        | 0.18   |
| 84       | 0.22          | 0.25     | 0.96           | 0.94      | 0.14        | 0.17   |
| 85       | 0.19          | 0.23     | 0.97           | 0.94      | 0.12        | 0.15   |
| 86       | 0.17          | 0.21     | 0.97           | 0.95      | 0.11        | 0.14   |
| 87       | 0.15          | 0.19     | 0.98           | 0.95      | 0.10        | 0.13   |
| 88       | 0.13          | 0.18     | 0.98           | 0.96      | 0.08        | 0.12   |
| 89       | 0.12          | 0.16     | 0.98           | 0.96      | 0.08        | 0.11   |
| 90       | 0.11          | 0.16     | 0.98           | 0.96      | 0.07        | 0.11   |

Table S78: Reference ( $\phi_S$ ,  $\varphi$ ,  $\psi$ ) and approached ( $\phi_S^\ell$ ,  $\varphi^\ell$ ,  $\psi^\ell$ ) values of the topological descriptors for the first excited-state of the pyridinium-phenolate (PP), computed at the CAM-B3LYP/6-31G(d) level of theory.  $\alpha$  is the pyridinium-phenolate central twist angle amplitude.

| $\alpha$ | $\phi_S^\ell$ | $\phi_S$ | $\varphi^\ell$ | $\varphi$ | $\psi^\ell$ | $\psi$ |
|----------|---------------|----------|----------------|-----------|-------------|--------|
| 0        | 0.66          | 0.70     | 0.66           | 0.63      | 0.50        | 0.53   |
| 1        | 0.66          | 0.70     | 0.66           | 0.63      | 0.50        | 0.53   |
| 2        | 0.66          | 0.70     | 0.66           | 0.63      | 0.50        | 0.53   |
| 3        | 0.66          | 0.70     | 0.66           | 0.63      | 0.50        | 0.53   |
| 4        | 0.66          | 0.70     | 0.66           | 0.63      | 0.50        | 0.53   |
| 5        | 0.66          | 0.70     | 0.66           | 0.63      | 0.50        | 0.53   |
| 6        | 0.66          | 0.70     | 0.66           | 0.64      | 0.50        | 0.53   |
| 7        | 0.66          | 0.70     | 0.66           | 0.64      | 0.50        | 0.53   |
| 8        | 0.66          | 0.70     | 0.66           | 0.64      | 0.50        | 0.53   |
| 9        | 0.66          | 0.70     | 0.67           | 0.64      | 0.50        | 0.53   |
| 10       | 0.66          | 0.70     | 0.67           | 0.64      | 0.50        | 0.53   |
| 11       | 0.66          | 0.70     | 0.67           | 0.64      | 0.50        | 0.53   |
| 12       | 0.66          | 0.69     | 0.67           | 0.64      | 0.50        | 0.52   |
| 13       | 0.65          | 0.69     | 0.67           | 0.65      | 0.49        | 0.52   |
| 14       | 0.65          | 0.69     | 0.67           | 0.65      | 0.49        | 0.52   |
| 15       | 0.65          | 0.69     | 0.67           | 0.65      | 0.49        | 0.52   |
| 16       | 0.65          | 0.69     | 0.68           | 0.65      | 0.49        | 0.52   |
| 17       | 0.65          | 0.69     | 0.68           | 0.65      | 0.49        | 0.52   |
| 18       | 0.65          | 0.69     | 0.68           | 0.66      | 0.49        | 0.51   |
| 19       | 0.65          | 0.68     | 0.68           | 0.66      | 0.49        | 0.51   |
| 20       | 0.65          | 0.68     | 0.68           | 0.66      | 0.49        | 0.51   |
| 21       | 0.65          | 0.68     | 0.69           | 0.66      | 0.48        | 0.51   |
| 22       | 0.64          | 0.68     | 0.69           | 0.67      | 0.48        | 0.50   |
| 23       | 0.64          | 0.68     | 0.69           | 0.67      | 0.48        | 0.50   |
| 24       | 0.64          | 0.67     | 0.69           | 0.67      | 0.48        | 0.50   |
| 25       | 0.64          | 0.67     | 0.70           | 0.67      | 0.47        | 0.50   |
| 26       | 0.64          | 0.67     | 0.70           | 0.68      | 0.47        | 0.50   |
| 27       | 0.64          | 0.67     | 0.70           | 0.68      | 0.47        | 0.50   |
| 28       | 0.64          | 0.67     | 0.71           | 0.68      | 0.47        | 0.50   |
| 29       | 0.63          | 0.66     | 0.71           | 0.69      | 0.46        | 0.49   |
| 30       | 0.63          | 0.66     | 0.71           | 0.69      | 0.46        | 0.49   |
| 31       | 0.63          | 0.66     | 0.71           | 0.69      | 0.46        | 0.49   |

Continued on next page

| $\alpha$ | $\phi_S^\ell$ | $\phi_S$ | $\varphi^\ell$ | $\varphi$ | $\psi^\ell$ | $\psi$ |
|----------|---------------|----------|----------------|-----------|-------------|--------|
| 32       | 0.63          | 0.66     | 0.72           | 0.70      | 0.46        | 0.48   |
| 33       | 0.63          | 0.65     | 0.72           | 0.70      | 0.46        | 0.48   |
| 34       | 0.62          | 0.65     | 0.72           | 0.70      | 0.45        | 0.48   |
| 35       | 0.62          | 0.65     | 0.73           | 0.71      | 0.45        | 0.47   |
| 36       | 0.62          | 0.64     | 0.73           | 0.71      | 0.45        | 0.47   |
| 37       | 0.62          | 0.64     | 0.74           | 0.72      | 0.44        | 0.46   |
| 38       | 0.61          | 0.64     | 0.74           | 0.72      | 0.44        | 0.46   |
| 39       | 0.61          | 0.63     | 0.74           | 0.72      | 0.44        | 0.46   |
| 40       | 0.61          | 0.63     | 0.75           | 0.73      | 0.43        | 0.45   |
| 41       | 0.60          | 0.63     | 0.75           | 0.73      | 0.43        | 0.45   |
| 42       | 0.60          | 0.62     | 0.76           | 0.74      | 0.43        | 0.44   |
| 43       | 0.60          | 0.62     | 0.76           | 0.74      | 0.43        | 0.44   |
| 44       | 0.59          | 0.61     | 0.77           | 0.74      | 0.42        | 0.44   |
| 45       | 0.59          | 0.61     | 0.77           | 0.75      | 0.42        | 0.43   |
| 46       | 0.58          | 0.60     | 0.77           | 0.75      | 0.41        | 0.43   |
| 47       | 0.58          | 0.60     | 0.78           | 0.76      | 0.41        | 0.43   |
| 48       | 0.57          | 0.59     | 0.78           | 0.76      | 0.40        | 0.42   |
| 49       | 0.57          | 0.59     | 0.79           | 0.77      | 0.40        | 0.42   |
| 50       | 0.56          | 0.58     | 0.79           | 0.77      | 0.39        | 0.41   |
| 51       | 0.56          | 0.58     | 0.80           | 0.78      | 0.39        | 0.41   |
| 52       | 0.55          | 0.57     | 0.80           | 0.78      | 0.38        | 0.40   |
| 53       | 0.55          | 0.57     | 0.81           | 0.79      | 0.38        | 0.40   |
| 54       | 0.54          | 0.56     | 0.81           | 0.79      | 0.37        | 0.39   |
| 55       | 0.54          | 0.56     | 0.81           | 0.80      | 0.37        | 0.39   |
| 56       | 0.53          | 0.55     | 0.82           | 0.80      | 0.37        | 0.38   |
| 57       | 0.52          | 0.54     | 0.82           | 0.81      | 0.36        | 0.37   |
| 58       | 0.52          | 0.54     | 0.83           | 0.81      | 0.36        | 0.37   |
| 59       | 0.51          | 0.53     | 0.83           | 0.82      | 0.35        | 0.37   |
| 60       | 0.50          | 0.52     | 0.84           | 0.82      | 0.34        | 0.36   |
| 61       | 0.49          | 0.51     | 0.84           | 0.83      | 0.34        | 0.35   |
| 62       | 0.49          | 0.51     | 0.85           | 0.83      | 0.33        | 0.35   |
| 63       | 0.48          | 0.50     | 0.86           | 0.84      | 0.32        | 0.34   |

Continued on next page

| $\alpha$ | $\phi_S^\ell$ | $\phi_S$ | $\varphi^\ell$ | $\varphi$ | $\psi^\ell$ | $\psi$ |
|----------|---------------|----------|----------------|-----------|-------------|--------|
| 64       | 0.47          | 0.49     | 0.86           | 0.84      | 0.32        | 0.34   |
| 65       | 0.46          | 0.48     | 0.87           | 0.85      | 0.31        | 0.33   |
| 66       | 0.45          | 0.47     | 0.87           | 0.85      | 0.30        | 0.32   |
| 67       | 0.44          | 0.46     | 0.88           | 0.86      | 0.30        | 0.31   |
| 68       | 0.43          | 0.45     | 0.89           | 0.86      | 0.29        | 0.31   |
| 69       | 0.42          | 0.44     | 0.89           | 0.87      | 0.28        | 0.30   |
| 70       | 0.41          | 0.43     | 0.90           | 0.87      | 0.27        | 0.29   |
| 71       | 0.40          | 0.42     | 0.90           | 0.88      | 0.27        | 0.28   |
| 72       | 0.38          | 0.41     | 0.91           | 0.89      | 0.25        | 0.27   |
| 73       | 0.37          | 0.40     | 0.91           | 0.89      | 0.25        | 0.27   |
| 74       | 0.36          | 0.38     | 0.92           | 0.90      | 0.24        | 0.25   |
| 75       | 0.34          | 0.37     | 0.93           | 0.90      | 0.22        | 0.25   |
| 76       | 0.33          | 0.36     | 0.93           | 0.91      | 0.22        | 0.24   |
| 77       | 0.31          | 0.34     | 0.94           | 0.91      | 0.20        | 0.23   |
| 78       | 0.30          | 0.33     | 0.94           | 0.92      | 0.20        | 0.22   |
| 79       | 0.28          | 0.31     | 0.95           | 0.92      | 0.18        | 0.21   |
| 80       | 0.26          | 0.30     | 0.95           | 0.93      | 0.17        | 0.20   |
| 81       | 0.24          | 0.28     | 0.96           | 0.93      | 0.16        | 0.19   |
| 82       | 0.22          | 0.26     | 0.96           | 0.94      | 0.14        | 0.17   |
| 83       | 0.21          | 0.25     | 0.97           | 0.94      | 0.14        | 0.17   |
| 84       | 0.19          | 0.23     | 0.97           | 0.95      | 0.12        | 0.15   |
| 85       | 0.17          | 0.21     | 0.98           | 0.95      | 0.11        | 0.14   |
| 86       | 0.16          | 0.20     | 0.98           | 0.95      | 0.10        | 0.13   |
| 87       | 0.14          | 0.18     | 0.98           | 0.96      | 0.09        | 0.12   |
| 88       | 0.12          | 0.17     | 0.99           | 0.96      | 0.08        | 0.11   |
| 89       | 0.11          | 0.15     | 0.99           | 0.96      | 0.07        | 0.10   |
| 90       | 0.11          | 0.15     | 0.99           | 0.96      | 0.07        | 0.10   |

Table S79: Reference ( $\phi_S$ ,  $\varphi$ ,  $\psi$ ) and approached ( $\phi_S^\ell$ ,  $\varphi^\ell$ ,  $\psi^\ell$ ) values of the topological descriptors for the first excited-state of the pyridinium-phenolate (PP), computed at the CAM-B3LYP/6-31+G level of theory.  $\alpha$  is the pyridinium-phenolate central twist angle amplitude.

| $\alpha$ | $\phi_S^\ell$ | $\phi_S$ | $\varphi^\ell$ | $\varphi$ | $\psi^\ell$ | $\psi$ |
|----------|---------------|----------|----------------|-----------|-------------|--------|
| 0        | 0.69          | 0.73     | 0.65           | 0.62      | 0.52        | 0.55   |
| 1        | 0.69          | 0.73     | 0.65           | 0.62      | 0.52        | 0.55   |
| 2        | 0.69          | 0.73     | 0.65           | 0.62      | 0.52        | 0.55   |
| 3        | 0.69          | 0.72     | 0.65           | 0.62      | 0.52        | 0.55   |
| 4        | 0.69          | 0.72     | 0.65           | 0.62      | 0.52        | 0.55   |
| 5        | 0.69          | 0.72     | 0.65           | 0.62      | 0.52        | 0.55   |
| 6        | 0.69          | 0.72     | 0.65           | 0.62      | 0.52        | 0.55   |
| 7        | 0.69          | 0.72     | 0.65           | 0.62      | 0.52        | 0.55   |
| 8        | 0.69          | 0.72     | 0.65           | 0.62      | 0.52        | 0.55   |
| 9        | 0.69          | 0.72     | 0.65           | 0.62      | 0.52        | 0.55   |
| 10       | 0.69          | 0.72     | 0.65           | 0.62      | 0.52        | 0.55   |
| 11       | 0.69          | 0.72     | 0.65           | 0.62      | 0.52        | 0.55   |
| 12       | 0.69          | 0.72     | 0.66           | 0.63      | 0.51        | 0.54   |
| 13       | 0.69          | 0.72     | 0.66           | 0.63      | 0.51        | 0.54   |
| 14       | 0.69          | 0.71     | 0.66           | 0.63      | 0.51        | 0.54   |
| 15       | 0.68          | 0.71     | 0.66           | 0.63      | 0.51        | 0.54   |
| 16       | 0.68          | 0.71     | 0.66           | 0.63      | 0.51        | 0.54   |
| 17       | 0.68          | 0.71     | 0.66           | 0.64      | 0.51        | 0.53   |
| 18       | 0.68          | 0.71     | 0.67           | 0.64      | 0.50        | 0.53   |
| 19       | 0.68          | 0.71     | 0.67           | 0.64      | 0.50        | 0.53   |
| 20       | 0.68          | 0.71     | 0.67           | 0.64      | 0.50        | 0.53   |
| 21       | 0.68          | 0.70     | 0.67           | 0.65      | 0.50        | 0.52   |
| 22       | 0.68          | 0.70     | 0.67           | 0.65      | 0.50        | 0.52   |
| 23       | 0.67          | 0.70     | 0.68           | 0.65      | 0.50        | 0.52   |
| 24       | 0.67          | 0.70     | 0.68           | 0.65      | 0.50        | 0.52   |
| 25       | 0.67          | 0.70     | 0.68           | 0.66      | 0.50        | 0.52   |
| 26       | 0.67          | 0.69     | 0.68           | 0.66      | 0.50        | 0.51   |
| 27       | 0.67          | 0.69     | 0.69           | 0.66      | 0.49        | 0.51   |
| 28       | 0.67          | 0.69     | 0.69           | 0.67      | 0.49        | 0.51   |
| 29       | 0.66          | 0.69     | 0.69           | 0.67      | 0.49        | 0.51   |
| 30       | 0.66          | 0.68     | 0.70           | 0.67      | 0.48        | 0.50   |
| 31       | 0.66          | 0.68     | 0.70           | 0.68      | 0.48        | 0.50   |

Continued on next page

| $\alpha$ | $\phi_S^\ell$ | $\phi_S$ | $\varphi^\ell$ | $\varphi$ | $\psi^\ell$ | $\psi$ |
|----------|---------------|----------|----------------|-----------|-------------|--------|
| 32       | 0.66          | 0.68     | 0.70           | 0.68      | 0.48        | 0.50   |
| 33       | 0.66          | 0.68     | 0.71           | 0.68      | 0.48        | 0.50   |
| 34       | 0.66          | 0.67     | 0.71           | 0.69      | 0.48        | 0.49   |
| 35       | 0.65          | 0.67     | 0.71           | 0.69      | 0.47        | 0.49   |
| 36       | 0.65          | 0.67     | 0.71           | 0.69      | 0.47        | 0.49   |
| 37       | 0.65          | 0.67     | 0.72           | 0.70      | 0.47        | 0.49   |
| 38       | 0.65          | 0.66     | 0.72           | 0.70      | 0.47        | 0.48   |
| 39       | 0.64          | 0.66     | 0.73           | 0.71      | 0.46        | 0.48   |
| 40       | 0.64          | 0.66     | 0.73           | 0.71      | 0.46        | 0.48   |
| 41       | 0.64          | 0.65     | 0.73           | 0.71      | 0.46        | 0.47   |
| 42       | 0.63          | 0.65     | 0.74           | 0.72      | 0.45        | 0.47   |
| 43       | 0.63          | 0.64     | 0.74           | 0.72      | 0.45        | 0.46   |
| 44       | 0.63          | 0.64     | 0.75           | 0.73      | 0.44        | 0.46   |
| 45       | 0.62          | 0.64     | 0.75           | 0.73      | 0.44        | 0.46   |
| 46       | 0.62          | 0.63     | 0.75           | 0.73      | 0.44        | 0.45   |
| 47       | 0.61          | 0.63     | 0.76           | 0.74      | 0.43        | 0.45   |
| 48       | 0.61          | 0.62     | 0.76           | 0.74      | 0.43        | 0.44   |
| 49       | 0.61          | 0.62     | 0.77           | 0.75      | 0.43        | 0.44   |
| 50       | 0.60          | 0.61     | 0.77           | 0.75      | 0.42        | 0.43   |
| 51       | 0.60          | 0.61     | 0.78           | 0.76      | 0.42        | 0.43   |
| 52       | 0.59          | 0.60     | 0.78           | 0.76      | 0.41        | 0.43   |
| 53       | 0.58          | 0.60     | 0.79           | 0.77      | 0.40        | 0.42   |
| 54       | 0.58          | 0.59     | 0.79           | 0.77      | 0.40        | 0.42   |
| 55       | 0.57          | 0.59     | 0.80           | 0.78      | 0.39        | 0.41   |
| 56       | 0.57          | 0.58     | 0.80           | 0.78      | 0.39        | 0.41   |
| 57       | 0.56          | 0.57     | 0.81           | 0.79      | 0.39        | 0.40   |
| 58       | 0.56          | 0.57     | 0.81           | 0.79      | 0.39        | 0.40   |
| 59       | 0.55          | 0.56     | 0.82           | 0.80      | 0.38        | 0.39   |
| 60       | 0.54          | 0.55     | 0.82           | 0.80      | 0.37        | 0.38   |
| 61       | 0.53          | 0.55     | 0.83           | 0.81      | 0.36        | 0.38   |
| 62       | 0.53          | 0.54     | 0.83           | 0.81      | 0.36        | 0.37   |
| 63       | 0.52          | 0.53     | 0.84           | 0.82      | 0.35        | 0.37   |

Continued on next page



| $\alpha$ | $\phi_S^\ell$ | $\phi_S$ | $\varphi^\ell$ | $\varphi$ | $\psi^\ell$ | $\psi$ |
|----------|---------------|----------|----------------|-----------|-------------|--------|
| 64       | 0.51          | 0.52     | 0.84           | 0.82      | 0.35        | 0.36   |
| 65       | 0.50          | 0.52     | 0.85           | 0.83      | 0.34        | 0.36   |
| 66       | 0.49          | 0.51     | 0.85           | 0.83      | 0.33        | 0.35   |
| 67       | 0.48          | 0.50     | 0.86           | 0.84      | 0.32        | 0.34   |
| 68       | 0.47          | 0.49     | 0.87           | 0.84      | 0.32        | 0.34   |
| 69       | 0.46          | 0.48     | 0.87           | 0.85      | 0.31        | 0.33   |
| 70       | 0.45          | 0.47     | 0.88           | 0.86      | 0.30        | 0.32   |
| 71       | 0.44          | 0.46     | 0.89           | 0.86      | 0.29        | 0.31   |
| 72       | 0.43          | 0.45     | 0.89           | 0.87      | 0.29        | 0.30   |
| 73       | 0.41          | 0.44     | 0.90           | 0.87      | 0.27        | 0.30   |
| 74       | 0.40          | 0.42     | 0.90           | 0.88      | 0.27        | 0.28   |
| 75       | 0.39          | 0.41     | 0.91           | 0.89      | 0.26        | 0.27   |
| 76       | 0.37          | 0.40     | 0.92           | 0.89      | 0.24        | 0.27   |
| 77       | 0.36          | 0.38     | 0.92           | 0.90      | 0.24        | 0.25   |
| 78       | 0.34          | 0.37     | 0.93           | 0.90      | 0.22        | 0.25   |
| 79       | 0.32          | 0.35     | 0.94           | 0.91      | 0.21        | 0.23   |
| 80       | 0.30          | 0.33     | 0.94           | 0.92      | 0.20        | 0.22   |
| 81       | 0.28          | 0.32     | 0.95           | 0.92      | 0.18        | 0.21   |
| 82       | 0.26          | 0.30     | 0.96           | 0.93      | 0.17        | 0.20   |
| 83       | 0.24          | 0.28     | 0.96           | 0.94      | 0.16        | 0.18   |
| 84       | 0.21          | 0.26     | 0.97           | 0.94      | 0.14        | 0.17   |
| 85       | 0.19          | 0.23     | 0.98           | 0.95      | 0.12        | 0.15   |
| 86       | 0.16          | 0.21     | 0.98           | 0.95      | 0.10        | 0.14   |
| 87       | 0.14          | 0.19     | 0.99           | 0.96      | 0.09        | 0.12   |
| 88       | 0.12          | 0.17     | 0.99           | 0.96      | 0.08        | 0.11   |
| 89       | 0.10          | 0.16     | 0.99           | 0.96      | 0.06        | 0.11   |
| 90       | 0.09          | 0.15     | 0.99           | 0.96      | 0.06        | 0.10   |

Table S80: Reference ( $\phi_S$ ,  $\varphi$ ,  $\psi$ ) and approached ( $\phi_S^\ell$ ,  $\varphi^\ell$ ,  $\psi^\ell$ ) values of the topological descriptors for the first excited-state of the pyridinium-phenolate (PP), computed at the CAM-B3LYP/6-31G level of theory.  $\alpha$  is the pyridinium-phenolate central twist angle amplitude.

| $\alpha$ | $\phi_S^\ell$ | $\phi_S$ | $\varphi^\ell$ | $\varphi$ | $\psi^\ell$ | $\psi$ |
|----------|---------------|----------|----------------|-----------|-------------|--------|
| 0        | 0.62          | 0.67     | 0.71           | 0.67      | 0.46        | 0.50   |
| 1        | 0.62          | 0.67     | 0.71           | 0.67      | 0.46        | 0.50   |
| 2        | 0.62          | 0.67     | 0.71           | 0.67      | 0.46        | 0.50   |
| 3        | 0.62          | 0.67     | 0.71           | 0.68      | 0.46        | 0.50   |
| 4        | 0.62          | 0.67     | 0.71           | 0.68      | 0.46        | 0.50   |
| 5        | 0.62          | 0.66     | 0.71           | 0.68      | 0.46        | 0.49   |
| 6        | 0.62          | 0.66     | 0.71           | 0.68      | 0.46        | 0.49   |
| 7        | 0.61          | 0.66     | 0.71           | 0.68      | 0.45        | 0.49   |
| 8        | 0.61          | 0.66     | 0.72           | 0.68      | 0.45        | 0.49   |
| 9        | 0.61          | 0.66     | 0.72           | 0.68      | 0.45        | 0.49   |
| 10       | 0.61          | 0.66     | 0.72           | 0.68      | 0.45        | 0.49   |
| 11       | 0.61          | 0.66     | 0.72           | 0.68      | 0.45        | 0.49   |
| 12       | 0.61          | 0.66     | 0.72           | 0.68      | 0.45        | 0.49   |
| 13       | 0.61          | 0.66     | 0.72           | 0.69      | 0.45        | 0.49   |
| 14       | 0.61          | 0.65     | 0.72           | 0.69      | 0.45        | 0.48   |
| 15       | 0.60          | 0.65     | 0.72           | 0.69      | 0.44        | 0.48   |
| 16       | 0.60          | 0.65     | 0.73           | 0.69      | 0.44        | 0.48   |
| 17       | 0.60          | 0.65     | 0.73           | 0.70      | 0.44        | 0.48   |
| 18       | 0.60          | 0.65     | 0.73           | 0.70      | 0.44        | 0.48   |
| 19       | 0.60          | 0.64     | 0.73           | 0.70      | 0.44        | 0.47   |
| 20       | 0.60          | 0.64     | 0.74           | 0.70      | 0.43        | 0.47   |
| 21       | 0.59          | 0.64     | 0.74           | 0.71      | 0.43        | 0.47   |
| 22       | 0.59          | 0.63     | 0.74           | 0.71      | 0.43        | 0.46   |
| 23       | 0.59          | 0.63     | 0.74           | 0.71      | 0.43        | 0.46   |
| 24       | 0.59          | 0.63     | 0.75           | 0.72      | 0.42        | 0.46   |
| 25       | 0.58          | 0.63     | 0.75           | 0.72      | 0.42        | 0.46   |
| 26       | 0.58          | 0.62     | 0.75           | 0.72      | 0.42        | 0.45   |
| 27       | 0.58          | 0.62     | 0.76           | 0.73      | 0.41        | 0.45   |
| 28       | 0.57          | 0.62     | 0.76           | 0.73      | 0.41        | 0.45   |
| 29       | 0.57          | 0.61     | 0.76           | 0.73      | 0.41        | 0.44   |
| 30       | 0.57          | 0.61     | 0.77           | 0.74      | 0.41        | 0.44   |
| 31       | 0.56          | 0.60     | 0.77           | 0.74      | 0.40        | 0.43   |

Continued on next page

| $\alpha$ | $\phi_S^\ell$ | $\phi_S$ | $\varphi^\ell$ | $\varphi$ | $\psi^\ell$ | $\psi$ |
|----------|---------------|----------|----------------|-----------|-------------|--------|
| 32       | 0.56          | 0.60     | 0.78           | 0.74      | 0.40        | 0.43   |
| 33       | 0.56          | 0.59     | 0.78           | 0.75      | 0.40        | 0.42   |
| 34       | 0.55          | 0.59     | 0.78           | 0.75      | 0.39        | 0.42   |
| 35       | 0.55          | 0.59     | 0.79           | 0.76      | 0.39        | 0.42   |
| 36       | 0.54          | 0.58     | 0.79           | 0.76      | 0.38        | 0.41   |
| 37       | 0.54          | 0.58     | 0.80           | 0.77      | 0.38        | 0.41   |
| 38       | 0.53          | 0.57     | 0.80           | 0.77      | 0.37        | 0.41   |
| 39       | 0.53          | 0.56     | 0.80           | 0.77      | 0.37        | 0.40   |
| 40       | 0.52          | 0.56     | 0.81           | 0.78      | 0.36        | 0.40   |
| 41       | 0.52          | 0.55     | 0.81           | 0.78      | 0.36        | 0.39   |
| 42       | 0.51          | 0.55     | 0.82           | 0.79      | 0.35        | 0.39   |
| 43       | 0.51          | 0.54     | 0.82           | 0.79      | 0.35        | 0.38   |
| 44       | 0.50          | 0.54     | 0.83           | 0.80      | 0.35        | 0.38   |
| 45       | 0.49          | 0.53     | 0.83           | 0.80      | 0.34        | 0.37   |
| 46       | 0.49          | 0.52     | 0.84           | 0.81      | 0.34        | 0.36   |
| 47       | 0.48          | 0.52     | 0.84           | 0.81      | 0.33        | 0.36   |
| 48       | 0.47          | 0.51     | 0.85           | 0.82      | 0.32        | 0.35   |
| 49       | 0.47          | 0.50     | 0.85           | 0.82      | 0.32        | 0.35   |
| 50       | 0.46          | 0.49     | 0.86           | 0.83      | 0.31        | 0.34   |
| 51       | 0.45          | 0.49     | 0.86           | 0.83      | 0.31        | 0.34   |
| 52       | 0.45          | 0.48     | 0.87           | 0.84      | 0.30        | 0.33   |
| 53       | 0.44          | 0.47     | 0.87           | 0.84      | 0.30        | 0.32   |
| 54       | 0.43          | 0.46     | 0.88           | 0.85      | 0.29        | 0.32   |
| 55       | 0.42          | 0.46     | 0.88           | 0.85      | 0.28        | 0.32   |
| 56       | 0.41          | 0.45     | 0.88           | 0.86      | 0.28        | 0.31   |
| 57       | 0.40          | 0.44     | 0.89           | 0.86      | 0.27        | 0.30   |
| 58       | 0.40          | 0.43     | 0.89           | 0.87      | 0.27        | 0.29   |
| 59       | 0.39          | 0.42     | 0.90           | 0.87      | 0.26        | 0.29   |
| 60       | 0.38          | 0.41     | 0.90           | 0.88      | 0.25        | 0.28   |
| 61       | 0.37          | 0.40     | 0.91           | 0.88      | 0.25        | 0.27   |
| 62       | 0.36          | 0.40     | 0.91           | 0.89      | 0.24        | 0.27   |
| 63       | 0.35          | 0.39     | 0.92           | 0.89      | 0.23        | 0.26   |

Continued on next page

| $\alpha$ | $\phi_S^\ell$ | $\phi_S$ | $\varphi^\ell$ | $\varphi$ | $\psi^\ell$ | $\psi$ |
|----------|---------------|----------|----------------|-----------|-------------|--------|
| 64       | 0.34          | 0.38     | 0.92           | 0.89      | 0.23        | 0.26   |
| 65       | 0.33          | 0.37     | 0.93           | 0.90      | 0.22        | 0.25   |
| 66       | 0.32          | 0.36     | 0.93           | 0.90      | 0.21        | 0.24   |
| 67       | 0.31          | 0.35     | 0.94           | 0.91      | 0.20        | 0.23   |
| 68       | 0.30          | 0.34     | 0.94           | 0.91      | 0.20        | 0.23   |
| 69       | 0.29          | 0.33     | 0.95           | 0.91      | 0.19        | 0.22   |
| 70       | 0.27          | 0.32     | 0.95           | 0.92      | 0.18        | 0.21   |
| 71       | 0.26          | 0.31     | 0.95           | 0.92      | 0.17        | 0.21   |
| 72       | 0.25          | 0.30     | 0.96           | 0.92      | 0.16        | 0.20   |
| 73       | 0.24          | 0.29     | 0.96           | 0.93      | 0.16        | 0.19   |
| 74       | 0.23          | 0.28     | 0.96           | 0.93      | 0.15        | 0.19   |
| 75       | 0.22          | 0.27     | 0.97           | 0.93      | 0.14        | 0.18   |
| 76       | 0.21          | 0.26     | 0.97           | 0.94      | 0.14        | 0.17   |
| 77       | 0.20          | 0.25     | 0.97           | 0.94      | 0.13        | 0.17   |
| 78       | 0.19          | 0.24     | 0.97           | 0.94      | 0.12        | 0.16   |
| 79       | 0.18          | 0.23     | 0.98           | 0.94      | 0.12        | 0.15   |
| 80       | 0.17          | 0.22     | 0.98           | 0.95      | 0.11        | 0.14   |
| 81       | 0.16          | 0.21     | 0.98           | 0.95      | 0.10        | 0.14   |
| 82       | 0.15          | 0.20     | 0.98           | 0.95      | 0.10        | 0.13   |
| 83       | 0.14          | 0.20     | 0.98           | 0.95      | 0.09        | 0.13   |
| 84       | 0.13          | 0.19     | 0.98           | 0.95      | 0.08        | 0.13   |
| 85       | 0.13          | 0.18     | 0.98           | 0.95      | 0.08        | 0.12   |
| 86       | 0.12          | 0.17     | 0.98           | 0.95      | 0.08        | 0.11   |
| 87       | 0.11          | 0.17     | 0.99           | 0.95      | 0.07        | 0.11   |
| 88       | 0.10          | 0.16     | 0.99           | 0.96      | 0.06        | 0.11   |
| 89       | 0.10          | 0.16     | 0.99           | 0.96      | 0.06        | 0.11   |
| 90       | 0.10          | 0.16     | 0.99           | 0.96      | 0.06        | 0.11   |

Table S81: Reference ( $\phi_S$ ,  $\varphi$ ,  $\psi$ ) and approached ( $\phi_S^\ell$ ,  $\varphi^\ell$ ,  $\psi^\ell$ ) values of the topological descriptors for the first excited-state of the pyridinium-phenolate (PP), computed at the CIS/3-21G level of theory.  $\alpha$  is the pyridinium-phenolate central twist angle amplitude.

| $\alpha$ | $\phi_S^\ell$ | $\phi_S$ | $\varphi^\ell$ | $\varphi$ | $\psi^\ell$ | $\psi$ |
|----------|---------------|----------|----------------|-----------|-------------|--------|
| 0        | 0.60          | 0.65     | 0.70           | 0.68      | 0.45        | 0.49   |
| 1        | 0.60          | 0.65     | 0.70           | 0.68      | 0.45        | 0.49   |
| 2        | 0.60          | 0.65     | 0.70           | 0.68      | 0.45        | 0.49   |
| 3        | 0.60          | 0.65     | 0.70           | 0.68      | 0.45        | 0.49   |
| 4        | 0.60          | 0.65     | 0.70           | 0.68      | 0.45        | 0.49   |
| 5        | 0.60          | 0.65     | 0.71           | 0.68      | 0.45        | 0.49   |
| 6        | 0.60          | 0.64     | 0.71           | 0.68      | 0.45        | 0.48   |
| 7        | 0.60          | 0.64     | 0.71           | 0.68      | 0.45        | 0.48   |
| 8        | 0.60          | 0.64     | 0.71           | 0.68      | 0.45        | 0.48   |
| 9        | 0.60          | 0.64     | 0.71           | 0.69      | 0.45        | 0.48   |
| 10       | 0.60          | 0.64     | 0.71           | 0.69      | 0.45        | 0.48   |
| 11       | 0.60          | 0.64     | 0.71           | 0.69      | 0.45        | 0.48   |
| 12       | 0.60          | 0.64     | 0.71           | 0.69      | 0.45        | 0.48   |
| 13       | 0.59          | 0.64     | 0.71           | 0.69      | 0.44        | 0.48   |
| 14       | 0.59          | 0.63     | 0.72           | 0.69      | 0.44        | 0.47   |
| 15       | 0.59          | 0.63     | 0.72           | 0.70      | 0.44        | 0.47   |
| 16       | 0.59          | 0.63     | 0.72           | 0.70      | 0.44        | 0.47   |
| 17       | 0.59          | 0.63     | 0.72           | 0.70      | 0.44        | 0.47   |
| 18       | 0.58          | 0.63     | 0.73           | 0.70      | 0.43        | 0.47   |
| 19       | 0.58          | 0.62     | 0.73           | 0.71      | 0.43        | 0.46   |
| 20       | 0.58          | 0.62     | 0.73           | 0.71      | 0.43        | 0.46   |
| 21       | 0.58          | 0.62     | 0.74           | 0.71      | 0.42        | 0.46   |
| 22       | 0.58          | 0.62     | 0.74           | 0.71      | 0.42        | 0.46   |
| 23       | 0.57          | 0.61     | 0.74           | 0.72      | 0.42        | 0.45   |
| 24       | 0.57          | 0.61     | 0.74           | 0.72      | 0.42        | 0.45   |
| 25       | 0.57          | 0.61     | 0.75           | 0.72      | 0.41        | 0.45   |
| 26       | 0.56          | 0.60     | 0.75           | 0.73      | 0.41        | 0.44   |
| 27       | 0.56          | 0.60     | 0.75           | 0.73      | 0.41        | 0.44   |
| 28       | 0.56          | 0.60     | 0.76           | 0.73      | 0.40        | 0.44   |
| 29       | 0.55          | 0.59     | 0.76           | 0.74      | 0.40        | 0.43   |
| 30       | 0.55          | 0.59     | 0.76           | 0.74      | 0.40        | 0.43   |
| 31       | 0.55          | 0.58     | 0.77           | 0.74      | 0.39        | 0.42   |

Continued on next page

| $\alpha$ | $\phi_S^\ell$ | $\phi_S$ | $\varphi^\ell$ | $\varphi$ | $\psi^\ell$ | $\psi$ |
|----------|---------------|----------|----------------|-----------|-------------|--------|
| 32       | 0.54          | 0.58     | 0.77           | 0.75      | 0.39        | 0.42   |
| 33       | 0.54          | 0.58     | 0.78           | 0.75      | 0.39        | 0.42   |
| 34       | 0.53          | 0.57     | 0.78           | 0.76      | 0.38        | 0.41   |
| 35       | 0.53          | 0.57     | 0.78           | 0.76      | 0.38        | 0.41   |
| 36       | 0.52          | 0.56     | 0.79           | 0.76      | 0.37        | 0.40   |
| 37       | 0.52          | 0.56     | 0.79           | 0.77      | 0.37        | 0.40   |
| 38       | 0.51          | 0.55     | 0.80           | 0.77      | 0.36        | 0.39   |
| 39       | 0.51          | 0.55     | 0.80           | 0.78      | 0.36        | 0.39   |
| 40       | 0.50          | 0.54     | 0.81           | 0.78      | 0.35        | 0.39   |
| 41       | 0.50          | 0.54     | 0.81           | 0.79      | 0.35        | 0.38   |
| 42       | 0.49          | 0.53     | 0.82           | 0.79      | 0.34        | 0.38   |
| 43       | 0.48          | 0.52     | 0.82           | 0.80      | 0.34        | 0.37   |
| 44       | 0.48          | 0.52     | 0.83           | 0.80      | 0.33        | 0.37   |
| 45       | 0.47          | 0.51     | 0.83           | 0.81      | 0.33        | 0.36   |
| 46       | 0.47          | 0.51     | 0.83           | 0.81      | 0.33        | 0.36   |
| 47       | 0.46          | 0.50     | 0.84           | 0.81      | 0.32        | 0.35   |
| 48       | 0.45          | 0.49     | 0.84           | 0.82      | 0.31        | 0.34   |
| 49       | 0.45          | 0.49     | 0.85           | 0.82      | 0.31        | 0.34   |
| 50       | 0.44          | 0.48     | 0.85           | 0.83      | 0.30        | 0.33   |
| 51       | 0.44          | 0.47     | 0.86           | 0.83      | 0.30        | 0.33   |
| 52       | 0.43          | 0.46     | 0.86           | 0.84      | 0.30        | 0.32   |
| 53       | 0.42          | 0.46     | 0.87           | 0.84      | 0.29        | 0.32   |
| 54       | 0.42          | 0.45     | 0.87           | 0.85      | 0.29        | 0.31   |
| 55       | 0.41          | 0.44     | 0.88           | 0.85      | 0.28        | 0.30   |
| 56       | 0.40          | 0.43     | 0.88           | 0.86      | 0.27        | 0.30   |
| 57       | 0.40          | 0.43     | 0.88           | 0.86      | 0.27        | 0.30   |
| 58       | 0.39          | 0.42     | 0.89           | 0.87      | 0.26        | 0.29   |
| 59       | 0.38          | 0.41     | 0.89           | 0.87      | 0.26        | 0.28   |
| 60       | 0.37          | 0.40     | 0.90           | 0.88      | 0.25        | 0.27   |
| 61       | 0.37          | 0.39     | 0.90           | 0.88      | 0.25        | 0.27   |
| 62       | 0.36          | 0.38     | 0.91           | 0.88      | 0.24        | 0.26   |
| 63       | 0.35          | 0.38     | 0.91           | 0.89      | 0.23        | 0.26   |

Continued on next page

| $\alpha$ | $\phi_S^\ell$ | $\phi_S$ | $\varphi^\ell$ | $\varphi$ | $\psi^\ell$ | $\psi$ |
|----------|---------------|----------|----------------|-----------|-------------|--------|
| 64       | 0.34          | 0.37     | 0.91           | 0.89      | 0.23        | 0.25   |
| 65       | 0.33          | 0.36     | 0.92           | 0.90      | 0.22        | 0.24   |
| 66       | 0.33          | 0.35     | 0.92           | 0.90      | 0.22        | 0.24   |
| 67       | 0.32          | 0.34     | 0.93           | 0.90      | 0.21        | 0.23   |
| 68       | 0.31          | 0.33     | 0.93           | 0.91      | 0.20        | 0.22   |
| 69       | 0.30          | 0.32     | 0.93           | 0.91      | 0.20        | 0.22   |
| 70       | 0.29          | 0.31     | 0.93           | 0.91      | 0.19        | 0.21   |
| 71       | 0.28          | 0.30     | 0.94           | 0.92      | 0.18        | 0.20   |
| 72       | 0.27          | 0.29     | 0.94           | 0.92      | 0.18        | 0.19   |
| 73       | 0.26          | 0.29     | 0.94           | 0.92      | 0.17        | 0.19   |
| 74       | 0.26          | 0.28     | 0.94           | 0.93      | 0.17        | 0.19   |
| 75       | 0.25          | 0.27     | 0.95           | 0.93      | 0.16        | 0.18   |
| 76       | 0.24          | 0.26     | 0.95           | 0.93      | 0.16        | 0.17   |
| 77       | 0.23          | 0.25     | 0.95           | 0.93      | 0.15        | 0.17   |
| 78       | 0.22          | 0.24     | 0.95           | 0.94      | 0.14        | 0.16   |
| 79       | 0.21          | 0.23     | 0.95           | 0.94      | 0.14        | 0.15   |
| 80       | 0.20          | 0.23     | 0.95           | 0.94      | 0.13        | 0.15   |
| 81       | 0.20          | 0.22     | 0.96           | 0.94      | 0.13        | 0.15   |
| 82       | 0.19          | 0.21     | 0.96           | 0.94      | 0.12        | 0.14   |
| 83       | 0.18          | 0.20     | 0.96           | 0.94      | 0.12        | 0.13   |
| 84       | 0.18          | 0.20     | 0.96           | 0.95      | 0.12        | 0.13   |
| 85       | 0.17          | 0.19     | 0.96           | 0.95      | 0.11        | 0.13   |
| 86       | 0.16          | 0.18     | 0.96           | 0.95      | 0.11        | 0.12   |
| 87       | 0.16          | 0.18     | 0.96           | 0.95      | 0.11        | 0.12   |
| 88       | 0.15          | 0.17     | 0.96           | 0.95      | 0.10        | 0.11   |
| 89       | 0.15          | 0.17     | 0.96           | 0.95      | 0.10        | 0.11   |
| 90       | 0.15          | 0.17     | 0.96           | 0.95      | 0.10        | 0.11   |

Table S82: Reference ( $\phi_S$ ,  $\varphi$ ,  $\psi$ ) and approached ( $\phi_S^\ell$ ,  $\varphi^\ell$ ,  $\psi^\ell$ ) values of the topological descriptors for the first excited-state of the pyridinium-phenolate (PP), computed at the CIS/6-311++G(2d,p) level of theory.  $\alpha$  is the pyridinium-phenolate central twist angle amplitude.

| $\alpha$ | $\phi_S^\ell$ | $\phi_S$ | $\varphi^\ell$ | $\varphi$ | $\psi^\ell$ | $\psi$ |
|----------|---------------|----------|----------------|-----------|-------------|--------|
| 0        | 0.59          | 0.65     | 0.71           | 0.68      | 0.44        | 0.49   |
| 1        | 0.59          | 0.65     | 0.71           | 0.68      | 0.44        | 0.49   |
| 2        | 0.59          | 0.65     | 0.71           | 0.68      | 0.44        | 0.49   |
| 3        | 0.59          | 0.65     | 0.71           | 0.68      | 0.44        | 0.49   |
| 4        | 0.59          | 0.64     | 0.71           | 0.68      | 0.44        | 0.48   |
| 5        | 0.59          | 0.64     | 0.71           | 0.68      | 0.44        | 0.48   |
| 6        | 0.59          | 0.64     | 0.71           | 0.69      | 0.44        | 0.48   |
| 7        | 0.59          | 0.64     | 0.71           | 0.69      | 0.44        | 0.48   |
| 8        | 0.59          | 0.64     | 0.71           | 0.69      | 0.44        | 0.48   |
| 9        | 0.59          | 0.64     | 0.71           | 0.69      | 0.44        | 0.48   |
| 10       | 0.59          | 0.64     | 0.71           | 0.69      | 0.44        | 0.48   |
| 11       | 0.59          | 0.64     | 0.72           | 0.69      | 0.44        | 0.48   |
| 12       | 0.59          | 0.64     | 0.72           | 0.69      | 0.44        | 0.48   |
| 13       | 0.58          | 0.63     | 0.72           | 0.70      | 0.43        | 0.47   |
| 14       | 0.58          | 0.63     | 0.72           | 0.70      | 0.43        | 0.47   |
| 15       | 0.58          | 0.63     | 0.72           | 0.70      | 0.43        | 0.47   |
| 16       | 0.58          | 0.63     | 0.73           | 0.70      | 0.43        | 0.47   |
| 17       | 0.58          | 0.63     | 0.73           | 0.70      | 0.43        | 0.47   |
| 18       | 0.58          | 0.62     | 0.73           | 0.71      | 0.43        | 0.46   |
| 19       | 0.57          | 0.62     | 0.73           | 0.71      | 0.42        | 0.46   |
| 20       | 0.57          | 0.62     | 0.74           | 0.71      | 0.42        | 0.46   |
| 21       | 0.57          | 0.62     | 0.74           | 0.71      | 0.42        | 0.46   |
| 22       | 0.57          | 0.61     | 0.74           | 0.72      | 0.42        | 0.45   |
| 23       | 0.56          | 0.61     | 0.75           | 0.72      | 0.41        | 0.45   |
| 24       | 0.56          | 0.61     | 0.75           | 0.72      | 0.41        | 0.45   |
| 25       | 0.56          | 0.60     | 0.75           | 0.73      | 0.41        | 0.44   |
| 26       | 0.56          | 0.60     | 0.76           | 0.73      | 0.40        | 0.44   |
| 27       | 0.55          | 0.60     | 0.76           | 0.73      | 0.40        | 0.44   |
| 28       | 0.55          | 0.59     | 0.76           | 0.74      | 0.40        | 0.43   |
| 29       | 0.55          | 0.59     | 0.77           | 0.74      | 0.39        | 0.43   |
| 30       | 0.54          | 0.59     | 0.77           | 0.74      | 0.39        | 0.43   |
| 31       | 0.54          | 0.58     | 0.77           | 0.75      | 0.39        | 0.42   |

Continued on next page



| $\alpha$ | $\phi_S^\ell$ | $\phi_S$ | $\varphi^\ell$ | $\varphi$ | $\psi^\ell$ | $\psi$ |
|----------|---------------|----------|----------------|-----------|-------------|--------|
| 32       | 0.53          | 0.58     | 0.78           | 0.75      | 0.38        | 0.42   |
| 33       | 0.53          | 0.57     | 0.78           | 0.76      | 0.38        | 0.41   |
| 34       | 0.53          | 0.57     | 0.78           | 0.76      | 0.38        | 0.41   |
| 35       | 0.52          | 0.57     | 0.79           | 0.76      | 0.37        | 0.41   |
| 36       | 0.52          | 0.56     | 0.79           | 0.77      | 0.37        | 0.40   |
| 37       | 0.51          | 0.56     | 0.80           | 0.77      | 0.36        | 0.40   |
| 38       | 0.51          | 0.55     | 0.80           | 0.78      | 0.36        | 0.39   |
| 39       | 0.50          | 0.55     | 0.80           | 0.78      | 0.36        | 0.39   |
| 40       | 0.50          | 0.54     | 0.81           | 0.79      | 0.35        | 0.38   |
| 41       | 0.49          | 0.53     | 0.81           | 0.79      | 0.35        | 0.38   |
| 42       | 0.49          | 0.53     | 0.82           | 0.79      | 0.34        | 0.38   |
| 43       | 0.48          | 0.52     | 0.82           | 0.80      | 0.34        | 0.37   |
| 44       | 0.47          | 0.52     | 0.83           | 0.80      | 0.33        | 0.37   |
| 45       | 0.47          | 0.51     | 0.83           | 0.81      | 0.33        | 0.36   |
| 46       | 0.46          | 0.50     | 0.84           | 0.81      | 0.32        | 0.35   |
| 47       | 0.46          | 0.50     | 0.84           | 0.82      | 0.32        | 0.35   |
| 48       | 0.45          | 0.49     | 0.85           | 0.82      | 0.31        | 0.34   |
| 49       | 0.44          | 0.48     | 0.85           | 0.83      | 0.30        | 0.33   |
| 50       | 0.44          | 0.48     | 0.86           | 0.83      | 0.30        | 0.33   |
| 51       | 0.43          | 0.47     | 0.86           | 0.84      | 0.30        | 0.32   |
| 52       | 0.42          | 0.46     | 0.86           | 0.84      | 0.29        | 0.32   |
| 53       | 0.42          | 0.46     | 0.87           | 0.85      | 0.29        | 0.32   |
| 54       | 0.41          | 0.45     | 0.87           | 0.85      | 0.28        | 0.31   |
| 55       | 0.40          | 0.44     | 0.88           | 0.85      | 0.27        | 0.30   |
| 56       | 0.40          | 0.43     | 0.88           | 0.86      | 0.27        | 0.30   |
| 57       | 0.39          | 0.42     | 0.89           | 0.86      | 0.26        | 0.29   |
| 58       | 0.38          | 0.42     | 0.89           | 0.87      | 0.26        | 0.29   |
| 59       | 0.37          | 0.41     | 0.90           | 0.87      | 0.25        | 0.28   |
| 60       | 0.36          | 0.40     | 0.90           | 0.88      | 0.24        | 0.27   |
| 61       | 0.36          | 0.39     | 0.91           | 0.88      | 0.24        | 0.27   |
| 62       | 0.35          | 0.38     | 0.91           | 0.89      | 0.23        | 0.26   |
| 63       | 0.34          | 0.37     | 0.92           | 0.89      | 0.23        | 0.25   |

Continued on next page

| $\alpha$ | $\phi_S^\ell$ | $\phi_S$ | $\varphi^\ell$ | $\varphi$ | $\psi^\ell$ | $\psi$ |
|----------|---------------|----------|----------------|-----------|-------------|--------|
| 64       | 0.33          | 0.36     | 0.92           | 0.89      | 0.22        | 0.24   |
| 65       | 0.32          | 0.36     | 0.92           | 0.90      | 0.21        | 0.24   |
| 66       | 0.31          | 0.35     | 0.93           | 0.90      | 0.20        | 0.24   |
| 67       | 0.30          | 0.34     | 0.93           | 0.91      | 0.20        | 0.23   |
| 68       | 0.30          | 0.33     | 0.94           | 0.91      | 0.20        | 0.22   |
| 69       | 0.29          | 0.32     | 0.94           | 0.91      | 0.19        | 0.22   |
| 70       | 0.28          | 0.31     | 0.94           | 0.92      | 0.18        | 0.21   |
| 71       | 0.27          | 0.30     | 0.95           | 0.92      | 0.18        | 0.20   |
| 72       | 0.26          | 0.29     | 0.95           | 0.92      | 0.17        | 0.19   |
| 73       | 0.25          | 0.28     | 0.95           | 0.92      | 0.16        | 0.19   |
| 74       | 0.24          | 0.27     | 0.95           | 0.93      | 0.16        | 0.18   |
| 75       | 0.23          | 0.27     | 0.96           | 0.93      | 0.15        | 0.18   |
| 76       | 0.22          | 0.26     | 0.96           | 0.93      | 0.14        | 0.17   |
| 77       | 0.22          | 0.25     | 0.96           | 0.94      | 0.14        | 0.17   |
| 78       | 0.21          | 0.24     | 0.96           | 0.94      | 0.14        | 0.16   |
| 79       | 0.20          | 0.23     | 0.96           | 0.94      | 0.13        | 0.15   |
| 80       | 0.19          | 0.22     | 0.97           | 0.94      | 0.12        | 0.15   |
| 81       | 0.18          | 0.22     | 0.97           | 0.94      | 0.12        | 0.15   |
| 82       | 0.18          | 0.21     | 0.97           | 0.94      | 0.12        | 0.14   |
| 83       | 0.17          | 0.20     | 0.97           | 0.95      | 0.11        | 0.13   |
| 84       | 0.16          | 0.19     | 0.97           | 0.95      | 0.10        | 0.13   |
| 85       | 0.16          | 0.19     | 0.97           | 0.95      | 0.10        | 0.13   |
| 86       | 0.15          | 0.18     | 0.97           | 0.95      | 0.10        | 0.12   |
| 87       | 0.14          | 0.18     | 0.97           | 0.95      | 0.09        | 0.12   |
| 88       | 0.14          | 0.17     | 0.97           | 0.95      | 0.09        | 0.11   |
| 89       | 0.13          | 0.17     | 0.97           | 0.95      | 0.08        | 0.11   |
| 90       | 0.13          | 0.17     | 0.97           | 0.95      | 0.08        | 0.11   |

Table S83: Reference ( $\phi_S$ ,  $\varphi$ ,  $\psi$ ) and approached ( $\phi_S^\ell$ ,  $\varphi^\ell$ ,  $\psi^\ell$ ) values of the topological descriptors for the first excited-state of the pyridinium-phenolate (PP), computed at the CIS/6-311++G(d,p) level of theory.  $\alpha$  is the pyridinium-phenolate central twist angle amplitude.

| $\alpha$ | $\phi_S^\ell$ | $\phi_S$ | $\varphi^\ell$ | $\varphi$ | $\psi^\ell$ | $\psi$ |
|----------|---------------|----------|----------------|-----------|-------------|--------|
| 0        | 0.59          | 0.65     | 0.71           | 0.68      | 0.44        | 0.49   |
| 1        | 0.59          | 0.65     | 0.71           | 0.68      | 0.44        | 0.49   |
| 2        | 0.59          | 0.65     | 0.71           | 0.68      | 0.44        | 0.49   |
| 3        | 0.59          | 0.65     | 0.71           | 0.68      | 0.44        | 0.49   |
| 4        | 0.59          | 0.64     | 0.71           | 0.68      | 0.44        | 0.48   |
| 5        | 0.59          | 0.64     | 0.71           | 0.68      | 0.44        | 0.48   |
| 6        | 0.59          | 0.64     | 0.71           | 0.69      | 0.44        | 0.48   |
| 7        | 0.59          | 0.64     | 0.71           | 0.69      | 0.44        | 0.48   |
| 8        | 0.59          | 0.64     | 0.71           | 0.69      | 0.44        | 0.48   |
| 9        | 0.59          | 0.64     | 0.71           | 0.69      | 0.44        | 0.48   |
| 10       | 0.59          | 0.64     | 0.71           | 0.69      | 0.44        | 0.48   |
| 11       | 0.59          | 0.64     | 0.72           | 0.69      | 0.44        | 0.48   |
| 12       | 0.59          | 0.64     | 0.72           | 0.69      | 0.44        | 0.48   |
| 13       | 0.58          | 0.63     | 0.72           | 0.70      | 0.43        | 0.47   |
| 14       | 0.58          | 0.63     | 0.72           | 0.70      | 0.43        | 0.47   |
| 15       | 0.58          | 0.63     | 0.72           | 0.70      | 0.43        | 0.47   |
| 16       | 0.58          | 0.63     | 0.73           | 0.70      | 0.43        | 0.47   |
| 17       | 0.58          | 0.63     | 0.73           | 0.70      | 0.43        | 0.47   |
| 18       | 0.58          | 0.62     | 0.73           | 0.71      | 0.43        | 0.46   |
| 19       | 0.57          | 0.62     | 0.73           | 0.71      | 0.42        | 0.46   |
| 20       | 0.57          | 0.62     | 0.74           | 0.71      | 0.42        | 0.46   |
| 21       | 0.57          | 0.62     | 0.74           | 0.71      | 0.42        | 0.46   |
| 22       | 0.57          | 0.61     | 0.74           | 0.72      | 0.42        | 0.45   |
| 23       | 0.56          | 0.61     | 0.75           | 0.72      | 0.41        | 0.45   |
| 24       | 0.56          | 0.61     | 0.75           | 0.72      | 0.41        | 0.45   |
| 25       | 0.56          | 0.60     | 0.75           | 0.73      | 0.41        | 0.44   |
| 26       | 0.56          | 0.60     | 0.75           | 0.73      | 0.41        | 0.44   |
| 27       | 0.55          | 0.60     | 0.76           | 0.73      | 0.40        | 0.44   |
| 28       | 0.55          | 0.59     | 0.76           | 0.74      | 0.40        | 0.43   |
| 29       | 0.55          | 0.59     | 0.76           | 0.74      | 0.40        | 0.43   |
| 30       | 0.54          | 0.59     | 0.77           | 0.74      | 0.39        | 0.43   |
| 31       | 0.54          | 0.58     | 0.77           | 0.75      | 0.39        | 0.42   |

Continued on next page

| $\alpha$ | $\phi_S^\ell$ | $\phi_S$ | $\varphi^\ell$ | $\varphi$ | $\psi^\ell$ | $\psi$ |
|----------|---------------|----------|----------------|-----------|-------------|--------|
| 32       | 0.53          | 0.58     | 0.78           | 0.75      | 0.38        | 0.42   |
| 33       | 0.53          | 0.57     | 0.78           | 0.76      | 0.38        | 0.41   |
| 34       | 0.53          | 0.57     | 0.78           | 0.76      | 0.38        | 0.41   |
| 35       | 0.52          | 0.57     | 0.79           | 0.76      | 0.37        | 0.41   |
| 36       | 0.52          | 0.56     | 0.79           | 0.77      | 0.37        | 0.40   |
| 37       | 0.51          | 0.56     | 0.79           | 0.77      | 0.36        | 0.40   |
| 38       | 0.51          | 0.55     | 0.80           | 0.78      | 0.36        | 0.39   |
| 39       | 0.50          | 0.55     | 0.80           | 0.78      | 0.36        | 0.39   |
| 40       | 0.50          | 0.54     | 0.81           | 0.79      | 0.35        | 0.38   |
| 41       | 0.49          | 0.53     | 0.81           | 0.79      | 0.35        | 0.38   |
| 42       | 0.49          | 0.53     | 0.82           | 0.79      | 0.34        | 0.38   |
| 43       | 0.48          | 0.52     | 0.82           | 0.80      | 0.34        | 0.37   |
| 44       | 0.47          | 0.52     | 0.83           | 0.80      | 0.33        | 0.37   |
| 45       | 0.47          | 0.51     | 0.83           | 0.81      | 0.33        | 0.36   |
| 46       | 0.46          | 0.50     | 0.84           | 0.81      | 0.32        | 0.35   |
| 47       | 0.46          | 0.50     | 0.84           | 0.82      | 0.32        | 0.35   |
| 48       | 0.45          | 0.49     | 0.85           | 0.82      | 0.31        | 0.34   |
| 49       | 0.44          | 0.48     | 0.85           | 0.83      | 0.30        | 0.33   |
| 50       | 0.44          | 0.48     | 0.85           | 0.83      | 0.30        | 0.33   |
| 51       | 0.43          | 0.47     | 0.86           | 0.84      | 0.30        | 0.32   |
| 52       | 0.42          | 0.46     | 0.86           | 0.84      | 0.29        | 0.32   |
| 53       | 0.42          | 0.46     | 0.87           | 0.85      | 0.29        | 0.32   |
| 54       | 0.41          | 0.45     | 0.87           | 0.85      | 0.28        | 0.31   |
| 55       | 0.40          | 0.44     | 0.88           | 0.85      | 0.27        | 0.30   |
| 56       | 0.40          | 0.43     | 0.88           | 0.86      | 0.27        | 0.30   |
| 57       | 0.39          | 0.42     | 0.89           | 0.86      | 0.26        | 0.29   |
| 58       | 0.38          | 0.42     | 0.89           | 0.87      | 0.26        | 0.29   |
| 59       | 0.37          | 0.41     | 0.90           | 0.87      | 0.25        | 0.28   |
| 60       | 0.37          | 0.40     | 0.90           | 0.88      | 0.25        | 0.27   |
| 61       | 0.36          | 0.39     | 0.91           | 0.88      | 0.24        | 0.27   |
| 62       | 0.35          | 0.38     | 0.91           | 0.89      | 0.23        | 0.26   |
| 63       | 0.34          | 0.37     | 0.92           | 0.89      | 0.23        | 0.25   |

Continued on next page

| $\alpha$ | $\phi_S^\ell$ | $\phi_S$ | $\varphi^\ell$ | $\varphi$ | $\psi^\ell$ | $\psi$ |
|----------|---------------|----------|----------------|-----------|-------------|--------|
| 64       | 0.33          | 0.36     | 0.92           | 0.89      | 0.22        | 0.24   |
| 65       | 0.32          | 0.36     | 0.92           | 0.90      | 0.21        | 0.24   |
| 66       | 0.31          | 0.35     | 0.93           | 0.90      | 0.20        | 0.24   |
| 67       | 0.31          | 0.34     | 0.93           | 0.91      | 0.20        | 0.23   |
| 68       | 0.30          | 0.33     | 0.94           | 0.91      | 0.20        | 0.22   |
| 69       | 0.29          | 0.32     | 0.94           | 0.91      | 0.19        | 0.22   |
| 70       | 0.28          | 0.31     | 0.94           | 0.92      | 0.18        | 0.21   |
| 71       | 0.27          | 0.30     | 0.94           | 0.92      | 0.18        | 0.20   |
| 72       | 0.26          | 0.29     | 0.95           | 0.92      | 0.17        | 0.19   |
| 73       | 0.25          | 0.28     | 0.95           | 0.92      | 0.16        | 0.19   |
| 74       | 0.24          | 0.27     | 0.95           | 0.93      | 0.16        | 0.18   |
| 75       | 0.23          | 0.27     | 0.96           | 0.93      | 0.15        | 0.18   |
| 76       | 0.23          | 0.26     | 0.96           | 0.93      | 0.15        | 0.17   |
| 77       | 0.22          | 0.25     | 0.96           | 0.94      | 0.14        | 0.17   |
| 78       | 0.21          | 0.24     | 0.96           | 0.94      | 0.14        | 0.16   |
| 79       | 0.20          | 0.23     | 0.96           | 0.94      | 0.13        | 0.15   |
| 80       | 0.19          | 0.22     | 0.96           | 0.94      | 0.12        | 0.15   |
| 81       | 0.19          | 0.22     | 0.97           | 0.94      | 0.12        | 0.15   |
| 82       | 0.18          | 0.21     | 0.97           | 0.94      | 0.12        | 0.14   |
| 83       | 0.17          | 0.20     | 0.97           | 0.95      | 0.11        | 0.13   |
| 84       | 0.17          | 0.19     | 0.97           | 0.95      | 0.11        | 0.13   |
| 85       | 0.16          | 0.19     | 0.97           | 0.95      | 0.10        | 0.13   |
| 86       | 0.15          | 0.18     | 0.97           | 0.95      | 0.10        | 0.12   |
| 87       | 0.15          | 0.18     | 0.97           | 0.95      | 0.10        | 0.12   |
| 88       | 0.14          | 0.17     | 0.97           | 0.95      | 0.09        | 0.11   |
| 89       | 0.14          | 0.17     | 0.97           | 0.95      | 0.09        | 0.11   |
| 90       | 0.14          | 0.17     | 0.97           | 0.95      | 0.09        | 0.11   |

Table S84: Reference ( $\phi_S$ ,  $\varphi$ ,  $\psi$ ) and approached ( $\phi_S^\ell$ ,  $\varphi^\ell$ ,  $\psi^\ell$ ) values of the topological descriptors for the first excited-state of the pyridinium-phenolate (PP), computed at the CIS/6-311+G(d,p) level of theory.  $\alpha$  is the pyridinium-phenolate central twist angle amplitude.

| $\alpha$ | $\phi_S^\ell$ | $\phi_S$ | $\varphi^\ell$ | $\varphi$ | $\psi^\ell$ | $\psi$ |
|----------|---------------|----------|----------------|-----------|-------------|--------|
| 0        | 0.59          | 0.65     | 0.71           | 0.68      | 0.44        | 0.49   |
| 1        | 0.59          | 0.65     | 0.71           | 0.68      | 0.44        | 0.49   |
| 2        | 0.59          | 0.65     | 0.71           | 0.68      | 0.44        | 0.49   |
| 3        | 0.59          | 0.64     | 0.71           | 0.68      | 0.44        | 0.48   |
| 4        | 0.59          | 0.64     | 0.71           | 0.68      | 0.44        | 0.48   |
| 5        | 0.59          | 0.64     | 0.71           | 0.69      | 0.44        | 0.48   |
| 6        | 0.59          | 0.64     | 0.71           | 0.69      | 0.44        | 0.48   |
| 7        | 0.59          | 0.64     | 0.71           | 0.69      | 0.44        | 0.48   |
| 8        | 0.59          | 0.64     | 0.71           | 0.69      | 0.44        | 0.48   |
| 9        | 0.59          | 0.64     | 0.71           | 0.69      | 0.44        | 0.48   |
| 10       | 0.59          | 0.64     | 0.72           | 0.69      | 0.44        | 0.48   |
| 11       | 0.59          | 0.64     | 0.72           | 0.69      | 0.44        | 0.48   |
| 12       | 0.59          | 0.63     | 0.72           | 0.69      | 0.44        | 0.47   |
| 13       | 0.58          | 0.63     | 0.72           | 0.70      | 0.43        | 0.47   |
| 14       | 0.58          | 0.63     | 0.72           | 0.70      | 0.43        | 0.47   |
| 15       | 0.58          | 0.63     | 0.72           | 0.70      | 0.43        | 0.47   |
| 16       | 0.58          | 0.63     | 0.73           | 0.70      | 0.43        | 0.47   |
| 17       | 0.58          | 0.63     | 0.73           | 0.70      | 0.43        | 0.47   |
| 18       | 0.58          | 0.62     | 0.73           | 0.71      | 0.43        | 0.46   |
| 19       | 0.57          | 0.62     | 0.73           | 0.71      | 0.42        | 0.46   |
| 20       | 0.57          | 0.62     | 0.74           | 0.71      | 0.42        | 0.46   |
| 21       | 0.57          | 0.62     | 0.74           | 0.71      | 0.42        | 0.46   |
| 22       | 0.57          | 0.61     | 0.74           | 0.72      | 0.42        | 0.45   |
| 23       | 0.56          | 0.61     | 0.75           | 0.72      | 0.41        | 0.45   |
| 24       | 0.56          | 0.61     | 0.75           | 0.72      | 0.41        | 0.45   |
| 25       | 0.56          | 0.60     | 0.75           | 0.73      | 0.41        | 0.44   |
| 26       | 0.56          | 0.60     | 0.76           | 0.73      | 0.40        | 0.44   |
| 27       | 0.55          | 0.60     | 0.76           | 0.73      | 0.40        | 0.44   |
| 28       | 0.55          | 0.59     | 0.76           | 0.74      | 0.40        | 0.43   |
| 29       | 0.55          | 0.59     | 0.77           | 0.74      | 0.39        | 0.43   |
| 30       | 0.54          | 0.59     | 0.77           | 0.74      | 0.39        | 0.43   |
| 31       | 0.54          | 0.58     | 0.77           | 0.75      | 0.39        | 0.42   |

Continued on next page

| $\alpha$ | $\phi_S^\ell$ | $\phi_S$ | $\varphi^\ell$ | $\varphi$ | $\psi^\ell$ | $\psi$ |
|----------|---------------|----------|----------------|-----------|-------------|--------|
| 32       | 0.53          | 0.58     | 0.78           | 0.75      | 0.38        | 0.42   |
| 33       | 0.53          | 0.57     | 0.78           | 0.76      | 0.38        | 0.41   |
| 34       | 0.53          | 0.57     | 0.78           | 0.76      | 0.38        | 0.41   |
| 35       | 0.52          | 0.56     | 0.79           | 0.76      | 0.37        | 0.40   |
| 36       | 0.52          | 0.56     | 0.79           | 0.77      | 0.37        | 0.40   |
| 37       | 0.51          | 0.55     | 0.80           | 0.77      | 0.36        | 0.39   |
| 38       | 0.51          | 0.55     | 0.80           | 0.78      | 0.36        | 0.39   |
| 39       | 0.50          | 0.54     | 0.80           | 0.78      | 0.36        | 0.39   |
| 40       | 0.50          | 0.54     | 0.81           | 0.79      | 0.35        | 0.38   |
| 41       | 0.49          | 0.53     | 0.81           | 0.79      | 0.35        | 0.38   |
| 42       | 0.48          | 0.53     | 0.82           | 0.79      | 0.34        | 0.38   |
| 43       | 0.48          | 0.52     | 0.82           | 0.80      | 0.34        | 0.37   |
| 44       | 0.47          | 0.52     | 0.83           | 0.80      | 0.33        | 0.37   |
| 45       | 0.47          | 0.51     | 0.83           | 0.81      | 0.33        | 0.36   |
| 46       | 0.46          | 0.50     | 0.84           | 0.81      | 0.32        | 0.35   |
| 47       | 0.45          | 0.50     | 0.84           | 0.82      | 0.31        | 0.35   |
| 48       | 0.45          | 0.49     | 0.85           | 0.82      | 0.31        | 0.34   |
| 49       | 0.44          | 0.48     | 0.85           | 0.83      | 0.30        | 0.33   |
| 50       | 0.44          | 0.48     | 0.86           | 0.83      | 0.30        | 0.33   |
| 51       | 0.43          | 0.47     | 0.86           | 0.84      | 0.30        | 0.32   |
| 52       | 0.42          | 0.46     | 0.86           | 0.84      | 0.29        | 0.32   |
| 53       | 0.42          | 0.45     | 0.87           | 0.85      | 0.29        | 0.31   |
| 54       | 0.41          | 0.45     | 0.87           | 0.85      | 0.28        | 0.31   |
| 55       | 0.40          | 0.44     | 0.88           | 0.86      | 0.27        | 0.30   |
| 56       | 0.40          | 0.43     | 0.88           | 0.86      | 0.27        | 0.30   |
| 57       | 0.39          | 0.42     | 0.89           | 0.86      | 0.26        | 0.29   |
| 58       | 0.38          | 0.42     | 0.89           | 0.87      | 0.26        | 0.29   |
| 59       | 0.37          | 0.41     | 0.90           | 0.87      | 0.25        | 0.28   |
| 60       | 0.36          | 0.40     | 0.90           | 0.88      | 0.24        | 0.27   |
| 61       | 0.36          | 0.39     | 0.91           | 0.88      | 0.24        | 0.27   |
| 62       | 0.35          | 0.38     | 0.91           | 0.89      | 0.23        | 0.26   |
| 63       | 0.34          | 0.37     | 0.92           | 0.89      | 0.23        | 0.25   |

Continued on next page

| $\alpha$ | $\phi_S^\ell$ | $\phi_S$ | $\varphi^\ell$ | $\varphi$ | $\psi^\ell$ | $\psi$ |
|----------|---------------|----------|----------------|-----------|-------------|--------|
| 64       | 0.33          | 0.36     | 0.92           | 0.89      | 0.22        | 0.24   |
| 65       | 0.32          | 0.36     | 0.92           | 0.90      | 0.21        | 0.24   |
| 66       | 0.31          | 0.35     | 0.93           | 0.90      | 0.20        | 0.24   |
| 67       | 0.31          | 0.34     | 0.93           | 0.91      | 0.20        | 0.23   |
| 68       | 0.30          | 0.33     | 0.94           | 0.91      | 0.20        | 0.22   |
| 69       | 0.29          | 0.32     | 0.94           | 0.91      | 0.19        | 0.22   |
| 70       | 0.28          | 0.31     | 0.94           | 0.92      | 0.18        | 0.21   |
| 71       | 0.27          | 0.30     | 0.95           | 0.92      | 0.18        | 0.20   |
| 72       | 0.26          | 0.29     | 0.95           | 0.92      | 0.17        | 0.19   |
| 73       | 0.25          | 0.28     | 0.95           | 0.93      | 0.16        | 0.19   |
| 74       | 0.24          | 0.27     | 0.95           | 0.93      | 0.16        | 0.18   |
| 75       | 0.23          | 0.27     | 0.96           | 0.93      | 0.15        | 0.18   |
| 76       | 0.23          | 0.26     | 0.96           | 0.93      | 0.15        | 0.17   |
| 77       | 0.22          | 0.25     | 0.96           | 0.94      | 0.14        | 0.17   |
| 78       | 0.21          | 0.24     | 0.96           | 0.94      | 0.14        | 0.16   |
| 79       | 0.20          | 0.23     | 0.96           | 0.94      | 0.13        | 0.15   |
| 80       | 0.19          | 0.22     | 0.97           | 0.94      | 0.12        | 0.15   |
| 81       | 0.18          | 0.22     | 0.97           | 0.94      | 0.12        | 0.15   |
| 82       | 0.18          | 0.21     | 0.97           | 0.94      | 0.12        | 0.14   |
| 83       | 0.17          | 0.20     | 0.97           | 0.95      | 0.11        | 0.13   |
| 84       | 0.16          | 0.19     | 0.97           | 0.95      | 0.10        | 0.13   |
| 85       | 0.16          | 0.19     | 0.97           | 0.95      | 0.10        | 0.13   |
| 86       | 0.15          | 0.18     | 0.97           | 0.95      | 0.10        | 0.12   |
| 87       | 0.14          | 0.17     | 0.97           | 0.95      | 0.09        | 0.11   |
| 88       | 0.14          | 0.17     | 0.97           | 0.95      | 0.09        | 0.11   |
| 89       | 0.13          | 0.17     | 0.97           | 0.95      | 0.08        | 0.11   |
| 90       | 0.13          | 0.16     | 0.97           | 0.95      | 0.08        | 0.11   |

Table S85: Reference ( $\phi_S$ ,  $\varphi$ ,  $\psi$ ) and approached ( $\phi_S^\ell$ ,  $\varphi^\ell$ ,  $\psi^\ell$ ) values of the topological descriptors for the first excited-state of the pyridinium-phenolate (PP), computed at the CIS/6-311+G(d) level of theory.  $\alpha$  is the pyridinium-phenolate central twist angle amplitude.



| $\alpha$ | $\phi_S^\ell$ | $\phi_S$ | $\varphi^\ell$ | $\varphi$ | $\psi^\ell$ | $\psi$ |
|----------|---------------|----------|----------------|-----------|-------------|--------|
| 0        | 0.62          | 0.67     | 0.71           | 0.67      | 0.46        | 0.50   |
| 1        | 0.62          | 0.67     | 0.71           | 0.67      | 0.46        | 0.50   |
| 2        | 0.62          | 0.67     | 0.71           | 0.67      | 0.46        | 0.50   |
| 3        | 0.62          | 0.67     | 0.71           | 0.67      | 0.46        | 0.50   |
| 4        | 0.62          | 0.67     | 0.71           | 0.67      | 0.46        | 0.50   |
| 5        | 0.62          | 0.67     | 0.71           | 0.67      | 0.46        | 0.50   |
| 6        | 0.62          | 0.67     | 0.71           | 0.67      | 0.46        | 0.50   |
| 7        | 0.62          | 0.67     | 0.71           | 0.67      | 0.46        | 0.50   |
| 8        | 0.62          | 0.66     | 0.71           | 0.67      | 0.46        | 0.50   |
| 9        | 0.61          | 0.66     | 0.71           | 0.68      | 0.45        | 0.49   |
| 10       | 0.61          | 0.66     | 0.71           | 0.68      | 0.45        | 0.49   |
| 11       | 0.61          | 0.66     | 0.71           | 0.68      | 0.45        | 0.49   |
| 12       | 0.61          | 0.66     | 0.72           | 0.68      | 0.45        | 0.49   |
| 13       | 0.61          | 0.66     | 0.72           | 0.68      | 0.45        | 0.49   |
| 14       | 0.61          | 0.65     | 0.72           | 0.69      | 0.45        | 0.48   |
| 15       | 0.61          | 0.65     | 0.72           | 0.69      | 0.45        | 0.48   |
| 16       | 0.60          | 0.65     | 0.72           | 0.69      | 0.44        | 0.48   |
| 17       | 0.60          | 0.65     | 0.73           | 0.69      | 0.44        | 0.48   |
| 18       | 0.60          | 0.65     | 0.73           | 0.69      | 0.44        | 0.48   |
| 19       | 0.60          | 0.64     | 0.73           | 0.70      | 0.44        | 0.47   |
| 20       | 0.60          | 0.64     | 0.73           | 0.70      | 0.44        | 0.47   |
| 21       | 0.59          | 0.64     | 0.74           | 0.70      | 0.43        | 0.47   |
| 22       | 0.59          | 0.63     | 0.74           | 0.71      | 0.43        | 0.46   |
| 23       | 0.59          | 0.63     | 0.74           | 0.71      | 0.43        | 0.46   |
| 24       | 0.59          | 0.63     | 0.75           | 0.71      | 0.42        | 0.46   |
| 25       | 0.58          | 0.63     | 0.75           | 0.72      | 0.42        | 0.46   |
| 26       | 0.58          | 0.62     | 0.75           | 0.72      | 0.42        | 0.45   |
| 27       | 0.58          | 0.62     | 0.76           | 0.72      | 0.41        | 0.45   |
| 28       | 0.57          | 0.61     | 0.76           | 0.73      | 0.41        | 0.44   |
| 29       | 0.57          | 0.61     | 0.76           | 0.73      | 0.41        | 0.44   |
| 30       | 0.57          | 0.61     | 0.77           | 0.73      | 0.41        | 0.44   |
| 31       | 0.56          | 0.60     | 0.77           | 0.74      | 0.40        | 0.43   |

Continued on next page

| $\alpha$ | $\phi_S^\ell$ | $\phi_S$ | $\varphi^\ell$ | $\varphi$ | $\psi^\ell$ | $\psi$ |
|----------|---------------|----------|----------------|-----------|-------------|--------|
| 32       | 0.56          | 0.60     | 0.77           | 0.74      | 0.40        | 0.43   |
| 33       | 0.55          | 0.59     | 0.78           | 0.75      | 0.39        | 0.42   |
| 34       | 0.55          | 0.59     | 0.78           | 0.75      | 0.39        | 0.42   |
| 35       | 0.55          | 0.58     | 0.79           | 0.75      | 0.39        | 0.42   |
| 36       | 0.54          | 0.58     | 0.79           | 0.76      | 0.38        | 0.41   |
| 37       | 0.54          | 0.57     | 0.80           | 0.76      | 0.38        | 0.41   |
| 38       | 0.53          | 0.57     | 0.80           | 0.77      | 0.37        | 0.41   |
| 39       | 0.53          | 0.56     | 0.80           | 0.77      | 0.37        | 0.40   |
| 40       | 0.52          | 0.56     | 0.81           | 0.78      | 0.36        | 0.40   |
| 41       | 0.51          | 0.55     | 0.81           | 0.78      | 0.36        | 0.39   |
| 42       | 0.51          | 0.54     | 0.82           | 0.79      | 0.35        | 0.38   |
| 43       | 0.50          | 0.54     | 0.82           | 0.79      | 0.35        | 0.38   |
| 44       | 0.50          | 0.53     | 0.83           | 0.80      | 0.35        | 0.37   |
| 45       | 0.49          | 0.53     | 0.83           | 0.80      | 0.34        | 0.37   |
| 46       | 0.48          | 0.52     | 0.84           | 0.81      | 0.33        | 0.36   |
| 47       | 0.48          | 0.51     | 0.84           | 0.81      | 0.33        | 0.36   |
| 48       | 0.47          | 0.51     | 0.85           | 0.82      | 0.32        | 0.35   |
| 49       | 0.46          | 0.50     | 0.85           | 0.82      | 0.32        | 0.35   |
| 50       | 0.46          | 0.49     | 0.85           | 0.83      | 0.32        | 0.34   |
| 51       | 0.45          | 0.48     | 0.86           | 0.83      | 0.31        | 0.33   |
| 52       | 0.44          | 0.48     | 0.86           | 0.84      | 0.30        | 0.33   |
| 53       | 0.44          | 0.47     | 0.87           | 0.84      | 0.30        | 0.32   |
| 54       | 0.43          | 0.46     | 0.87           | 0.85      | 0.29        | 0.32   |
| 55       | 0.42          | 0.45     | 0.88           | 0.85      | 0.28        | 0.31   |
| 56       | 0.41          | 0.44     | 0.88           | 0.85      | 0.28        | 0.30   |
| 57       | 0.41          | 0.44     | 0.89           | 0.86      | 0.27        | 0.30   |
| 58       | 0.40          | 0.43     | 0.89           | 0.86      | 0.27        | 0.30   |
| 59       | 0.39          | 0.42     | 0.90           | 0.87      | 0.26        | 0.29   |
| 60       | 0.38          | 0.41     | 0.90           | 0.87      | 0.25        | 0.28   |
| 61       | 0.37          | 0.40     | 0.91           | 0.88      | 0.25        | 0.27   |
| 62       | 0.36          | 0.39     | 0.91           | 0.88      | 0.24        | 0.27   |
| 63       | 0.35          | 0.38     | 0.92           | 0.89      | 0.23        | 0.26   |

Continued on next page

| $\alpha$ | $\phi_S^\ell$ | $\phi_S$ | $\varphi^\ell$ | $\varphi$ | $\psi^\ell$ | $\psi$ |
|----------|---------------|----------|----------------|-----------|-------------|--------|
| 64       | 0.34          | 0.37     | 0.92           | 0.89      | 0.23        | 0.25   |
| 65       | 0.33          | 0.37     | 0.93           | 0.89      | 0.22        | 0.25   |
| 66       | 0.32          | 0.36     | 0.93           | 0.90      | 0.21        | 0.24   |
| 67       | 0.31          | 0.35     | 0.93           | 0.90      | 0.20        | 0.24   |
| 68       | 0.30          | 0.34     | 0.94           | 0.91      | 0.20        | 0.23   |
| 69       | 0.29          | 0.33     | 0.94           | 0.91      | 0.19        | 0.22   |
| 70       | 0.28          | 0.32     | 0.94           | 0.91      | 0.18        | 0.22   |
| 71       | 0.27          | 0.31     | 0.95           | 0.92      | 0.18        | 0.21   |
| 72       | 0.26          | 0.30     | 0.95           | 0.92      | 0.17        | 0.20   |
| 73       | 0.25          | 0.29     | 0.95           | 0.92      | 0.16        | 0.19   |
| 74       | 0.24          | 0.28     | 0.96           | 0.93      | 0.16        | 0.19   |
| 75       | 0.23          | 0.27     | 0.96           | 0.93      | 0.15        | 0.18   |
| 76       | 0.22          | 0.26     | 0.96           | 0.93      | 0.14        | 0.17   |
| 77       | 0.21          | 0.25     | 0.96           | 0.93      | 0.14        | 0.17   |
| 78       | 0.20          | 0.24     | 0.97           | 0.94      | 0.13        | 0.16   |
| 79       | 0.19          | 0.24     | 0.97           | 0.94      | 0.12        | 0.16   |
| 80       | 0.18          | 0.23     | 0.97           | 0.94      | 0.12        | 0.15   |
| 81       | 0.17          | 0.22     | 0.97           | 0.94      | 0.11        | 0.15   |
| 82       | 0.17          | 0.21     | 0.97           | 0.94      | 0.11        | 0.14   |
| 83       | 0.16          | 0.20     | 0.97           | 0.95      | 0.10        | 0.13   |
| 84       | 0.15          | 0.20     | 0.97           | 0.95      | 0.10        | 0.13   |
| 85       | 0.14          | 0.19     | 0.98           | 0.95      | 0.09        | 0.13   |
| 86       | 0.13          | 0.18     | 0.98           | 0.95      | 0.08        | 0.12   |
| 87       | 0.13          | 0.18     | 0.98           | 0.95      | 0.08        | 0.12   |
| 88       | 0.12          | 0.17     | 0.98           | 0.95      | 0.08        | 0.11   |
| 89       | 0.12          | 0.17     | 0.98           | 0.95      | 0.08        | 0.11   |
| 90       | 0.11          | 0.17     | 0.98           | 0.95      | 0.07        | 0.11   |

Table S86: Reference ( $\phi_S$ ,  $\varphi$ ,  $\psi$ ) and approached ( $\phi_S^\ell$ ,  $\varphi^\ell$ ,  $\psi^\ell$ ) values of the topological descriptors for the first excited-state of the pyridinium-phenolate (PP), computed at the CIS/6-311G(d) level of theory.  $\alpha$  is the pyridinium-phenolate central twist angle amplitude.

| $\alpha$ | $\phi_S^\ell$ | $\phi_S$ | $\varphi^\ell$ | $\varphi$ | $\psi^\ell$ | $\psi$ |
|----------|---------------|----------|----------------|-----------|-------------|--------|
| 0        | 0.59          | 0.63     | 0.72           | 0.69      | 0.44        | 0.47   |
| 1        | 0.59          | 0.63     | 0.72           | 0.69      | 0.44        | 0.47   |
| 2        | 0.59          | 0.63     | 0.72           | 0.69      | 0.44        | 0.47   |
| 3        | 0.59          | 0.63     | 0.72           | 0.69      | 0.44        | 0.47   |
| 4        | 0.58          | 0.63     | 0.72           | 0.69      | 0.43        | 0.47   |
| 5        | 0.58          | 0.63     | 0.72           | 0.70      | 0.43        | 0.47   |
| 6        | 0.58          | 0.63     | 0.72           | 0.70      | 0.43        | 0.47   |
| 7        | 0.58          | 0.63     | 0.72           | 0.70      | 0.43        | 0.47   |
| 8        | 0.58          | 0.63     | 0.72           | 0.70      | 0.43        | 0.47   |
| 9        | 0.58          | 0.63     | 0.72           | 0.70      | 0.43        | 0.47   |
| 10       | 0.58          | 0.63     | 0.72           | 0.70      | 0.43        | 0.47   |
| 11       | 0.58          | 0.62     | 0.72           | 0.70      | 0.43        | 0.46   |
| 12       | 0.58          | 0.62     | 0.72           | 0.70      | 0.43        | 0.46   |
| 13       | 0.58          | 0.62     | 0.73           | 0.71      | 0.43        | 0.46   |
| 14       | 0.57          | 0.62     | 0.73           | 0.71      | 0.42        | 0.46   |
| 15       | 0.57          | 0.62     | 0.73           | 0.71      | 0.42        | 0.46   |
| 16       | 0.57          | 0.62     | 0.73           | 0.71      | 0.42        | 0.46   |
| 17       | 0.57          | 0.61     | 0.73           | 0.71      | 0.42        | 0.45   |
| 18       | 0.57          | 0.61     | 0.74           | 0.72      | 0.42        | 0.45   |
| 19       | 0.57          | 0.61     | 0.74           | 0.72      | 0.42        | 0.45   |
| 20       | 0.56          | 0.61     | 0.74           | 0.72      | 0.41        | 0.45   |
| 21       | 0.56          | 0.60     | 0.75           | 0.72      | 0.41        | 0.44   |
| 22       | 0.56          | 0.60     | 0.75           | 0.73      | 0.41        | 0.44   |
| 23       | 0.56          | 0.60     | 0.75           | 0.73      | 0.41        | 0.44   |
| 24       | 0.55          | 0.59     | 0.75           | 0.73      | 0.40        | 0.43   |
| 25       | 0.55          | 0.59     | 0.76           | 0.74      | 0.40        | 0.43   |
| 26       | 0.55          | 0.59     | 0.76           | 0.74      | 0.40        | 0.43   |
| 27       | 0.54          | 0.59     | 0.76           | 0.74      | 0.39        | 0.43   |
| 28       | 0.54          | 0.58     | 0.77           | 0.75      | 0.39        | 0.42   |
| 29       | 0.54          | 0.58     | 0.77           | 0.75      | 0.39        | 0.42   |
| 30       | 0.53          | 0.57     | 0.77           | 0.75      | 0.38        | 0.41   |
| 31       | 0.53          | 0.57     | 0.78           | 0.76      | 0.38        | 0.41   |

Continued on next page

| $\alpha$ | $\phi_S^\ell$ | $\phi_S$ | $\varphi^\ell$ | $\varphi$ | $\psi^\ell$ | $\psi$ |
|----------|---------------|----------|----------------|-----------|-------------|--------|
| 32       | 0.53          | 0.57     | 0.78           | 0.76      | 0.38        | 0.41   |
| 33       | 0.52          | 0.56     | 0.79           | 0.77      | 0.37        | 0.40   |
| 34       | 0.52          | 0.56     | 0.79           | 0.77      | 0.37        | 0.40   |
| 35       | 0.51          | 0.55     | 0.79           | 0.77      | 0.36        | 0.39   |
| 36       | 0.51          | 0.55     | 0.80           | 0.78      | 0.36        | 0.39   |
| 37       | 0.51          | 0.54     | 0.80           | 0.78      | 0.36        | 0.39   |
| 38       | 0.50          | 0.54     | 0.81           | 0.79      | 0.35        | 0.38   |
| 39       | 0.50          | 0.53     | 0.81           | 0.79      | 0.35        | 0.38   |
| 40       | 0.49          | 0.53     | 0.81           | 0.79      | 0.35        | 0.38   |
| 41       | 0.48          | 0.52     | 0.82           | 0.80      | 0.34        | 0.37   |
| 42       | 0.48          | 0.52     | 0.82           | 0.80      | 0.34        | 0.37   |
| 43       | 0.47          | 0.51     | 0.83           | 0.81      | 0.33        | 0.36   |
| 44       | 0.47          | 0.50     | 0.83           | 0.81      | 0.33        | 0.35   |
| 45       | 0.46          | 0.50     | 0.84           | 0.82      | 0.32        | 0.35   |
| 46       | 0.45          | 0.49     | 0.84           | 0.82      | 0.31        | 0.34   |
| 47       | 0.45          | 0.49     | 0.85           | 0.83      | 0.31        | 0.34   |
| 48       | 0.44          | 0.48     | 0.85           | 0.83      | 0.30        | 0.33   |
| 49       | 0.44          | 0.47     | 0.86           | 0.83      | 0.30        | 0.33   |
| 50       | 0.43          | 0.47     | 0.86           | 0.84      | 0.30        | 0.32   |
| 51       | 0.42          | 0.46     | 0.86           | 0.84      | 0.29        | 0.32   |
| 52       | 0.42          | 0.45     | 0.87           | 0.85      | 0.29        | 0.31   |
| 53       | 0.41          | 0.44     | 0.87           | 0.85      | 0.28        | 0.30   |
| 54       | 0.40          | 0.44     | 0.88           | 0.86      | 0.27        | 0.30   |
| 55       | 0.40          | 0.43     | 0.88           | 0.86      | 0.27        | 0.30   |
| 56       | 0.39          | 0.42     | 0.89           | 0.87      | 0.26        | 0.29   |
| 57       | 0.38          | 0.41     | 0.89           | 0.87      | 0.26        | 0.28   |
| 58       | 0.37          | 0.41     | 0.90           | 0.87      | 0.25        | 0.28   |
| 59       | 0.36          | 0.40     | 0.90           | 0.88      | 0.24        | 0.27   |
| 60       | 0.36          | 0.39     | 0.91           | 0.88      | 0.24        | 0.27   |
| 61       | 0.35          | 0.38     | 0.91           | 0.89      | 0.23        | 0.26   |
| 62       | 0.34          | 0.37     | 0.92           | 0.89      | 0.23        | 0.25   |
| 63       | 0.33          | 0.36     | 0.92           | 0.90      | 0.22        | 0.24   |

Continued on next page

| $\alpha$ | $\phi_S^\ell$ | $\phi_S$ | $\varphi^\ell$ | $\varphi$ | $\psi^\ell$ | $\psi$ |
|----------|---------------|----------|----------------|-----------|-------------|--------|
| 64       | 0.32          | 0.36     | 0.93           | 0.90      | 0.21        | 0.24   |
| 65       | 0.31          | 0.35     | 0.93           | 0.90      | 0.20        | 0.24   |
| 66       | 0.30          | 0.34     | 0.93           | 0.91      | 0.20        | 0.23   |
| 67       | 0.30          | 0.33     | 0.94           | 0.91      | 0.20        | 0.22   |
| 68       | 0.29          | 0.32     | 0.94           | 0.91      | 0.19        | 0.22   |
| 69       | 0.28          | 0.31     | 0.94           | 0.92      | 0.18        | 0.21   |
| 70       | 0.27          | 0.30     | 0.95           | 0.92      | 0.18        | 0.20   |
| 71       | 0.26          | 0.29     | 0.95           | 0.92      | 0.17        | 0.19   |
| 72       | 0.25          | 0.28     | 0.95           | 0.93      | 0.16        | 0.19   |
| 73       | 0.24          | 0.27     | 0.96           | 0.93      | 0.16        | 0.18   |
| 74       | 0.23          | 0.27     | 0.96           | 0.93      | 0.15        | 0.18   |
| 75       | 0.22          | 0.26     | 0.96           | 0.93      | 0.14        | 0.17   |
| 76       | 0.21          | 0.25     | 0.96           | 0.94      | 0.14        | 0.17   |
| 77       | 0.21          | 0.24     | 0.97           | 0.94      | 0.14        | 0.16   |
| 78       | 0.20          | 0.23     | 0.97           | 0.94      | 0.13        | 0.15   |
| 79       | 0.19          | 0.22     | 0.97           | 0.94      | 0.12        | 0.15   |
| 80       | 0.18          | 0.21     | 0.97           | 0.95      | 0.12        | 0.14   |
| 81       | 0.18          | 0.21     | 0.97           | 0.95      | 0.12        | 0.14   |
| 82       | 0.17          | 0.20     | 0.97           | 0.95      | 0.11        | 0.13   |
| 83       | 0.16          | 0.19     | 0.97           | 0.95      | 0.10        | 0.13   |
| 84       | 0.16          | 0.18     | 0.97           | 0.95      | 0.10        | 0.12   |
| 85       | 0.15          | 0.18     | 0.98           | 0.95      | 0.10        | 0.12   |
| 86       | 0.14          | 0.17     | 0.98           | 0.95      | 0.09        | 0.11   |
| 87       | 0.14          | 0.17     | 0.98           | 0.95      | 0.09        | 0.11   |
| 88       | 0.13          | 0.16     | 0.98           | 0.95      | 0.08        | 0.11   |
| 89       | 0.13          | 0.16     | 0.98           | 0.95      | 0.08        | 0.11   |
| 90       | 0.13          | 0.15     | 0.98           | 0.95      | 0.08        | 0.10   |

Table S87: Reference ( $\phi_S$ ,  $\varphi$ ,  $\psi$ ) and approached ( $\phi_S^\ell$ ,  $\varphi^\ell$ ,  $\psi^\ell$ ) values of the topological descriptors for the first excited-state of the pyridinium-phenolate (PP), computed at the CIS/6-311+G level of theory.  $\alpha$  is the pyridinium-phenolate central twist angle amplitude.

| $\alpha$ | $\phi_S^\ell$ | $\phi_S$ | $\varphi^\ell$ | $\varphi$ | $\psi^\ell$ | $\psi$ |
|----------|---------------|----------|----------------|-----------|-------------|--------|
| 0        | 0.61          | 0.65     | 0.72           | 0.68      | 0.45        | 0.49   |
| 1        | 0.61          | 0.65     | 0.72           | 0.68      | 0.45        | 0.49   |
| 2        | 0.61          | 0.65     | 0.72           | 0.68      | 0.45        | 0.49   |
| 3        | 0.61          | 0.65     | 0.72           | 0.68      | 0.45        | 0.49   |
| 4        | 0.61          | 0.65     | 0.72           | 0.68      | 0.45        | 0.49   |
| 5        | 0.61          | 0.65     | 0.72           | 0.68      | 0.45        | 0.49   |
| 6        | 0.61          | 0.65     | 0.72           | 0.69      | 0.45        | 0.48   |
| 7        | 0.61          | 0.65     | 0.72           | 0.69      | 0.45        | 0.48   |
| 8        | 0.61          | 0.65     | 0.72           | 0.69      | 0.45        | 0.48   |
| 9        | 0.60          | 0.65     | 0.72           | 0.69      | 0.44        | 0.48   |
| 10       | 0.60          | 0.65     | 0.72           | 0.69      | 0.44        | 0.48   |
| 11       | 0.60          | 0.65     | 0.72           | 0.69      | 0.44        | 0.48   |
| 12       | 0.60          | 0.64     | 0.72           | 0.69      | 0.44        | 0.48   |
| 13       | 0.60          | 0.64     | 0.73           | 0.70      | 0.44        | 0.47   |
| 14       | 0.60          | 0.64     | 0.73           | 0.70      | 0.44        | 0.47   |
| 15       | 0.60          | 0.64     | 0.73           | 0.70      | 0.44        | 0.47   |
| 16       | 0.59          | 0.64     | 0.73           | 0.70      | 0.43        | 0.47   |
| 17       | 0.59          | 0.63     | 0.73           | 0.70      | 0.43        | 0.47   |
| 18       | 0.59          | 0.63     | 0.74           | 0.71      | 0.43        | 0.46   |
| 19       | 0.59          | 0.63     | 0.74           | 0.71      | 0.43        | 0.46   |
| 20       | 0.59          | 0.63     | 0.74           | 0.71      | 0.43        | 0.46   |
| 21       | 0.58          | 0.62     | 0.74           | 0.71      | 0.42        | 0.46   |
| 22       | 0.58          | 0.62     | 0.75           | 0.72      | 0.42        | 0.45   |
| 23       | 0.58          | 0.62     | 0.75           | 0.72      | 0.42        | 0.45   |
| 24       | 0.58          | 0.61     | 0.75           | 0.72      | 0.42        | 0.45   |
| 25       | 0.57          | 0.61     | 0.76           | 0.73      | 0.41        | 0.44   |
| 26       | 0.57          | 0.61     | 0.76           | 0.73      | 0.41        | 0.44   |
| 27       | 0.57          | 0.60     | 0.76           | 0.73      | 0.41        | 0.44   |
| 28       | 0.56          | 0.60     | 0.77           | 0.74      | 0.40        | 0.43   |
| 29       | 0.56          | 0.60     | 0.77           | 0.74      | 0.40        | 0.43   |
| 30       | 0.56          | 0.59     | 0.77           | 0.75      | 0.40        | 0.42   |
| 31       | 0.55          | 0.59     | 0.78           | 0.75      | 0.39        | 0.42   |

Continued on next page

| $\alpha$ | $\phi_S^\ell$ | $\phi_S$ | $\varphi^\ell$ | $\varphi$ | $\psi^\ell$ | $\psi$ |
|----------|---------------|----------|----------------|-----------|-------------|--------|
| 32       | 0.55          | 0.58     | 0.78           | 0.75      | 0.39        | 0.42   |
| 33       | 0.55          | 0.58     | 0.78           | 0.76      | 0.39        | 0.41   |
| 34       | 0.54          | 0.57     | 0.79           | 0.76      | 0.38        | 0.41   |
| 35       | 0.54          | 0.57     | 0.79           | 0.77      | 0.38        | 0.41   |
| 36       | 0.53          | 0.57     | 0.80           | 0.77      | 0.37        | 0.41   |
| 37       | 0.53          | 0.56     | 0.80           | 0.77      | 0.37        | 0.40   |
| 38       | 0.52          | 0.55     | 0.81           | 0.78      | 0.36        | 0.39   |
| 39       | 0.52          | 0.55     | 0.81           | 0.78      | 0.36        | 0.39   |
| 40       | 0.51          | 0.54     | 0.81           | 0.79      | 0.36        | 0.38   |
| 41       | 0.51          | 0.54     | 0.82           | 0.79      | 0.35        | 0.38   |
| 42       | 0.50          | 0.53     | 0.82           | 0.80      | 0.35        | 0.37   |
| 43       | 0.49          | 0.53     | 0.83           | 0.80      | 0.34        | 0.37   |
| 44       | 0.49          | 0.52     | 0.83           | 0.81      | 0.34        | 0.36   |
| 45       | 0.48          | 0.51     | 0.84           | 0.81      | 0.33        | 0.36   |
| 46       | 0.48          | 0.51     | 0.84           | 0.82      | 0.33        | 0.35   |
| 47       | 0.47          | 0.50     | 0.85           | 0.82      | 0.32        | 0.35   |
| 48       | 0.46          | 0.49     | 0.85           | 0.82      | 0.32        | 0.34   |
| 49       | 0.46          | 0.49     | 0.86           | 0.83      | 0.31        | 0.34   |
| 50       | 0.45          | 0.48     | 0.86           | 0.83      | 0.31        | 0.33   |
| 51       | 0.44          | 0.47     | 0.86           | 0.84      | 0.30        | 0.32   |
| 52       | 0.44          | 0.46     | 0.87           | 0.84      | 0.30        | 0.32   |
| 53       | 0.43          | 0.46     | 0.87           | 0.85      | 0.29        | 0.32   |
| 54       | 0.42          | 0.45     | 0.88           | 0.85      | 0.28        | 0.31   |
| 55       | 0.41          | 0.44     | 0.88           | 0.86      | 0.28        | 0.30   |
| 56       | 0.40          | 0.43     | 0.89           | 0.86      | 0.27        | 0.30   |
| 57       | 0.40          | 0.43     | 0.89           | 0.87      | 0.27        | 0.29   |
| 58       | 0.39          | 0.42     | 0.90           | 0.87      | 0.26        | 0.29   |
| 59       | 0.38          | 0.41     | 0.90           | 0.88      | 0.25        | 0.28   |
| 60       | 0.37          | 0.40     | 0.91           | 0.88      | 0.25        | 0.27   |
| 61       | 0.36          | 0.39     | 0.91           | 0.88      | 0.24        | 0.27   |
| 62       | 0.35          | 0.38     | 0.92           | 0.89      | 0.23        | 0.26   |
| 63       | 0.34          | 0.37     | 0.92           | 0.89      | 0.23        | 0.25   |

Continued on next page



| $\alpha$ | $\phi_S^\ell$ | $\phi_S$ | $\varphi^\ell$ | $\varphi$ | $\psi^\ell$ | $\psi$ |
|----------|---------------|----------|----------------|-----------|-------------|--------|
| 64       | 0.33          | 0.36     | 0.93           | 0.90      | 0.22        | 0.24   |
| 65       | 0.32          | 0.36     | 0.93           | 0.90      | 0.21        | 0.24   |
| 66       | 0.31          | 0.35     | 0.93           | 0.90      | 0.20        | 0.24   |
| 67       | 0.30          | 0.34     | 0.94           | 0.91      | 0.20        | 0.23   |
| 68       | 0.29          | 0.33     | 0.94           | 0.91      | 0.19        | 0.22   |
| 69       | 0.28          | 0.32     | 0.95           | 0.92      | 0.18        | 0.21   |
| 70       | 0.27          | 0.31     | 0.95           | 0.92      | 0.18        | 0.21   |
| 71       | 0.26          | 0.30     | 0.95           | 0.92      | 0.17        | 0.20   |
| 72       | 0.25          | 0.29     | 0.96           | 0.93      | 0.16        | 0.19   |
| 73       | 0.24          | 0.28     | 0.96           | 0.93      | 0.16        | 0.19   |
| 74       | 0.23          | 0.27     | 0.96           | 0.93      | 0.15        | 0.18   |
| 75       | 0.22          | 0.26     | 0.97           | 0.93      | 0.14        | 0.17   |
| 76       | 0.21          | 0.25     | 0.97           | 0.94      | 0.14        | 0.17   |
| 77       | 0.20          | 0.24     | 0.97           | 0.94      | 0.13        | 0.16   |
| 78       | 0.19          | 0.23     | 0.97           | 0.94      | 0.12        | 0.15   |
| 79       | 0.18          | 0.23     | 0.97           | 0.94      | 0.12        | 0.15   |
| 80       | 0.17          | 0.22     | 0.98           | 0.95      | 0.11        | 0.14   |
| 81       | 0.16          | 0.21     | 0.98           | 0.95      | 0.10        | 0.14   |
| 82       | 0.16          | 0.20     | 0.98           | 0.95      | 0.10        | 0.13   |
| 83       | 0.15          | 0.19     | 0.98           | 0.95      | 0.10        | 0.13   |
| 84       | 0.14          | 0.19     | 0.98           | 0.95      | 0.09        | 0.13   |
| 85       | 0.14          | 0.18     | 0.98           | 0.95      | 0.09        | 0.12   |
| 86       | 0.13          | 0.17     | 0.98           | 0.95      | 0.08        | 0.11   |
| 87       | 0.12          | 0.17     | 0.98           | 0.95      | 0.08        | 0.11   |
| 88       | 0.12          | 0.16     | 0.98           | 0.95      | 0.08        | 0.11   |
| 89       | 0.11          | 0.16     | 0.98           | 0.95      | 0.07        | 0.11   |
| 90       | 0.11          | 0.16     | 0.98           | 0.95      | 0.07        | 0.11   |

Table S88: Reference ( $\phi_S$ ,  $\varphi$ ,  $\psi$ ) and approached ( $\phi_S^\ell$ ,  $\varphi^\ell$ ,  $\psi^\ell$ ) values of the topological descriptors for the first excited-state of the pyridinium-phenolate (PP), computed at the CIS/6-311G level of theory.  $\alpha$  is the pyridinium-phenolate central twist angle amplitude.

| $\alpha$ | $\phi_S^\ell$ | $\phi_S$ | $\varphi^\ell$ | $\varphi$ | $\psi^\ell$ | $\psi$ |
|----------|---------------|----------|----------------|-----------|-------------|--------|
| 0        | 0.60          | 0.65     | 0.71           | 0.68      | 0.45        | 0.49   |
| 1        | 0.60          | 0.65     | 0.71           | 0.68      | 0.45        | 0.49   |
| 2        | 0.60          | 0.65     | 0.71           | 0.68      | 0.45        | 0.49   |
| 3        | 0.60          | 0.65     | 0.71           | 0.68      | 0.45        | 0.49   |
| 4        | 0.60          | 0.65     | 0.71           | 0.68      | 0.45        | 0.49   |
| 5        | 0.60          | 0.65     | 0.71           | 0.68      | 0.45        | 0.49   |
| 6        | 0.60          | 0.64     | 0.71           | 0.68      | 0.45        | 0.48   |
| 7        | 0.60          | 0.64     | 0.71           | 0.68      | 0.45        | 0.48   |
| 8        | 0.60          | 0.64     | 0.71           | 0.68      | 0.45        | 0.48   |
| 9        | 0.60          | 0.64     | 0.71           | 0.69      | 0.45        | 0.48   |
| 10       | 0.60          | 0.64     | 0.71           | 0.69      | 0.45        | 0.48   |
| 11       | 0.59          | 0.64     | 0.71           | 0.69      | 0.44        | 0.48   |
| 12       | 0.59          | 0.64     | 0.72           | 0.69      | 0.44        | 0.48   |
| 13       | 0.59          | 0.64     | 0.72           | 0.69      | 0.44        | 0.48   |
| 14       | 0.59          | 0.63     | 0.72           | 0.69      | 0.44        | 0.47   |
| 15       | 0.59          | 0.63     | 0.72           | 0.70      | 0.44        | 0.47   |
| 16       | 0.59          | 0.63     | 0.72           | 0.70      | 0.44        | 0.47   |
| 17       | 0.58          | 0.63     | 0.73           | 0.70      | 0.43        | 0.47   |
| 18       | 0.58          | 0.63     | 0.73           | 0.70      | 0.43        | 0.47   |
| 19       | 0.58          | 0.62     | 0.73           | 0.71      | 0.43        | 0.46   |
| 20       | 0.58          | 0.62     | 0.73           | 0.71      | 0.43        | 0.46   |
| 21       | 0.58          | 0.62     | 0.74           | 0.71      | 0.42        | 0.46   |
| 22       | 0.57          | 0.62     | 0.74           | 0.71      | 0.42        | 0.46   |
| 23       | 0.57          | 0.61     | 0.74           | 0.72      | 0.42        | 0.45   |
| 24       | 0.57          | 0.61     | 0.75           | 0.72      | 0.41        | 0.45   |
| 25       | 0.56          | 0.61     | 0.75           | 0.72      | 0.41        | 0.45   |
| 26       | 0.56          | 0.60     | 0.75           | 0.73      | 0.41        | 0.44   |
| 27       | 0.56          | 0.60     | 0.76           | 0.73      | 0.40        | 0.44   |
| 28       | 0.55          | 0.60     | 0.76           | 0.73      | 0.40        | 0.44   |
| 29       | 0.55          | 0.59     | 0.76           | 0.74      | 0.40        | 0.43   |
| 30       | 0.55          | 0.59     | 0.77           | 0.74      | 0.39        | 0.43   |
| 31       | 0.54          | 0.58     | 0.77           | 0.74      | 0.39        | 0.42   |

Continued on next page

| $\alpha$ | $\phi_S^\ell$ | $\phi_S$ | $\varphi^\ell$ | $\varphi$ | $\psi^\ell$ | $\psi$ |
|----------|---------------|----------|----------------|-----------|-------------|--------|
| 32       | 0.54          | 0.58     | 0.77           | 0.75      | 0.39        | 0.42   |
| 33       | 0.54          | 0.58     | 0.78           | 0.75      | 0.39        | 0.42   |
| 34       | 0.53          | 0.57     | 0.78           | 0.76      | 0.38        | 0.41   |
| 35       | 0.53          | 0.57     | 0.78           | 0.76      | 0.38        | 0.41   |
| 36       | 0.52          | 0.56     | 0.79           | 0.77      | 0.37        | 0.40   |
| 37       | 0.52          | 0.56     | 0.79           | 0.77      | 0.37        | 0.40   |
| 38       | 0.51          | 0.55     | 0.80           | 0.77      | 0.36        | 0.39   |
| 39       | 0.51          | 0.55     | 0.80           | 0.78      | 0.36        | 0.39   |
| 40       | 0.50          | 0.54     | 0.81           | 0.78      | 0.35        | 0.39   |
| 41       | 0.49          | 0.54     | 0.81           | 0.79      | 0.35        | 0.38   |
| 42       | 0.49          | 0.53     | 0.82           | 0.79      | 0.34        | 0.38   |
| 43       | 0.48          | 0.52     | 0.82           | 0.80      | 0.34        | 0.37   |
| 44       | 0.48          | 0.52     | 0.83           | 0.80      | 0.33        | 0.37   |
| 45       | 0.47          | 0.51     | 0.83           | 0.81      | 0.33        | 0.36   |
| 46       | 0.46          | 0.51     | 0.84           | 0.81      | 0.32        | 0.36   |
| 47       | 0.46          | 0.50     | 0.84           | 0.82      | 0.32        | 0.35   |
| 48       | 0.45          | 0.49     | 0.84           | 0.82      | 0.31        | 0.34   |
| 49       | 0.45          | 0.49     | 0.85           | 0.82      | 0.31        | 0.34   |
| 50       | 0.44          | 0.48     | 0.85           | 0.83      | 0.30        | 0.33   |
| 51       | 0.43          | 0.47     | 0.86           | 0.83      | 0.30        | 0.33   |
| 52       | 0.43          | 0.46     | 0.86           | 0.84      | 0.30        | 0.32   |
| 53       | 0.42          | 0.46     | 0.87           | 0.84      | 0.29        | 0.32   |
| 54       | 0.41          | 0.45     | 0.87           | 0.85      | 0.28        | 0.31   |
| 55       | 0.41          | 0.44     | 0.88           | 0.85      | 0.28        | 0.30   |
| 56       | 0.40          | 0.43     | 0.88           | 0.86      | 0.27        | 0.30   |
| 57       | 0.39          | 0.43     | 0.89           | 0.86      | 0.26        | 0.30   |
| 58       | 0.39          | 0.42     | 0.89           | 0.87      | 0.26        | 0.29   |
| 59       | 0.38          | 0.41     | 0.90           | 0.87      | 0.25        | 0.28   |
| 60       | 0.37          | 0.40     | 0.90           | 0.88      | 0.25        | 0.27   |
| 61       | 0.36          | 0.39     | 0.90           | 0.88      | 0.24        | 0.27   |
| 62       | 0.35          | 0.38     | 0.91           | 0.88      | 0.23        | 0.26   |
| 63       | 0.35          | 0.38     | 0.91           | 0.89      | 0.23        | 0.26   |

Continued on next page

| $\alpha$ | $\phi_S^\ell$ | $\phi_S$ | $\varphi^\ell$ | $\varphi$ | $\psi^\ell$ | $\psi$ |
|----------|---------------|----------|----------------|-----------|-------------|--------|
| 64       | 0.34          | 0.37     | 0.92           | 0.89      | 0.23        | 0.25   |
| 65       | 0.33          | 0.36     | 0.92           | 0.90      | 0.22        | 0.24   |
| 66       | 0.32          | 0.35     | 0.92           | 0.90      | 0.21        | 0.24   |
| 67       | 0.31          | 0.34     | 0.93           | 0.90      | 0.20        | 0.23   |
| 68       | 0.30          | 0.33     | 0.93           | 0.91      | 0.20        | 0.22   |
| 69       | 0.29          | 0.32     | 0.93           | 0.91      | 0.19        | 0.22   |
| 70       | 0.29          | 0.31     | 0.94           | 0.91      | 0.19        | 0.21   |
| 71       | 0.28          | 0.30     | 0.94           | 0.92      | 0.18        | 0.20   |
| 72       | 0.27          | 0.29     | 0.94           | 0.92      | 0.18        | 0.19   |
| 73       | 0.26          | 0.29     | 0.94           | 0.92      | 0.17        | 0.19   |
| 74       | 0.25          | 0.28     | 0.95           | 0.93      | 0.16        | 0.19   |
| 75       | 0.24          | 0.27     | 0.95           | 0.93      | 0.16        | 0.18   |
| 76       | 0.23          | 0.26     | 0.95           | 0.93      | 0.15        | 0.17   |
| 77       | 0.22          | 0.25     | 0.95           | 0.93      | 0.14        | 0.17   |
| 78       | 0.22          | 0.24     | 0.95           | 0.94      | 0.14        | 0.16   |
| 79       | 0.21          | 0.23     | 0.96           | 0.94      | 0.14        | 0.15   |
| 80       | 0.20          | 0.23     | 0.96           | 0.94      | 0.13        | 0.15   |
| 81       | 0.19          | 0.22     | 0.96           | 0.94      | 0.12        | 0.15   |
| 82       | 0.19          | 0.21     | 0.96           | 0.94      | 0.12        | 0.14   |
| 83       | 0.18          | 0.20     | 0.96           | 0.94      | 0.12        | 0.13   |
| 84       | 0.17          | 0.20     | 0.96           | 0.95      | 0.11        | 0.13   |
| 85       | 0.17          | 0.19     | 0.96           | 0.95      | 0.11        | 0.13   |
| 86       | 0.16          | 0.18     | 0.96           | 0.95      | 0.11        | 0.12   |
| 87       | 0.15          | 0.18     | 0.96           | 0.95      | 0.10        | 0.12   |
| 88       | 0.15          | 0.17     | 0.96           | 0.95      | 0.10        | 0.11   |
| 89       | 0.15          | 0.17     | 0.96           | 0.95      | 0.10        | 0.11   |
| 90       | 0.15          | 0.17     | 0.96           | 0.95      | 0.10        | 0.11   |

Table S89: Reference ( $\phi_S$ ,  $\varphi$ ,  $\psi$ ) and approached ( $\phi_S^\ell$ ,  $\varphi^\ell$ ,  $\psi^\ell$ ) values of the topological descriptors for the first excited-state of the pyridinium-phenolate (PP), computed at the CIS/6-31++G(2d,p) level of theory.  $\alpha$  is the pyridinium-phenolate central twist angle amplitude.

| $\alpha$ | $\phi_S^\ell$ | $\phi_S$ | $\varphi^\ell$ | $\varphi$ | $\psi^\ell$ | $\psi$ |
|----------|---------------|----------|----------------|-----------|-------------|--------|
| 0        | 0.59          | 0.65     | 0.71           | 0.68      | 0.44        | 0.49   |
| 1        | 0.59          | 0.65     | 0.71           | 0.68      | 0.44        | 0.49   |
| 2        | 0.59          | 0.65     | 0.71           | 0.68      | 0.44        | 0.49   |
| 3        | 0.59          | 0.65     | 0.71           | 0.68      | 0.44        | 0.49   |
| 4        | 0.59          | 0.64     | 0.71           | 0.68      | 0.44        | 0.48   |
| 5        | 0.59          | 0.64     | 0.71           | 0.68      | 0.44        | 0.48   |
| 6        | 0.59          | 0.64     | 0.71           | 0.69      | 0.44        | 0.48   |
| 7        | 0.59          | 0.64     | 0.71           | 0.69      | 0.44        | 0.48   |
| 8        | 0.59          | 0.64     | 0.71           | 0.69      | 0.44        | 0.48   |
| 9        | 0.59          | 0.64     | 0.71           | 0.69      | 0.44        | 0.48   |
| 10       | 0.59          | 0.64     | 0.71           | 0.69      | 0.44        | 0.48   |
| 11       | 0.59          | 0.64     | 0.72           | 0.69      | 0.44        | 0.48   |
| 12       | 0.59          | 0.64     | 0.72           | 0.69      | 0.44        | 0.48   |
| 13       | 0.59          | 0.63     | 0.72           | 0.70      | 0.44        | 0.47   |
| 14       | 0.58          | 0.63     | 0.72           | 0.70      | 0.43        | 0.47   |
| 15       | 0.58          | 0.63     | 0.72           | 0.70      | 0.43        | 0.47   |
| 16       | 0.58          | 0.63     | 0.72           | 0.70      | 0.43        | 0.47   |
| 17       | 0.58          | 0.63     | 0.73           | 0.70      | 0.43        | 0.47   |
| 18       | 0.58          | 0.62     | 0.73           | 0.71      | 0.43        | 0.46   |
| 19       | 0.57          | 0.62     | 0.73           | 0.71      | 0.42        | 0.46   |
| 20       | 0.57          | 0.62     | 0.74           | 0.71      | 0.42        | 0.46   |
| 21       | 0.57          | 0.62     | 0.74           | 0.71      | 0.42        | 0.46   |
| 22       | 0.57          | 0.61     | 0.74           | 0.72      | 0.42        | 0.45   |
| 23       | 0.57          | 0.61     | 0.74           | 0.72      | 0.42        | 0.45   |
| 24       | 0.56          | 0.61     | 0.75           | 0.72      | 0.41        | 0.45   |
| 25       | 0.56          | 0.60     | 0.75           | 0.73      | 0.41        | 0.44   |
| 26       | 0.56          | 0.60     | 0.75           | 0.73      | 0.41        | 0.44   |
| 27       | 0.55          | 0.60     | 0.76           | 0.73      | 0.40        | 0.44   |
| 28       | 0.55          | 0.59     | 0.76           | 0.74      | 0.40        | 0.43   |
| 29       | 0.55          | 0.59     | 0.76           | 0.74      | 0.40        | 0.43   |
| 30       | 0.54          | 0.59     | 0.77           | 0.74      | 0.39        | 0.43   |
| 31       | 0.54          | 0.58     | 0.77           | 0.75      | 0.39        | 0.42   |

Continued on next page

| $\alpha$ | $\phi_S^\ell$ | $\phi_S$ | $\varphi^\ell$ | $\varphi$ | $\psi^\ell$ | $\psi$ |
|----------|---------------|----------|----------------|-----------|-------------|--------|
| 32       | 0.54          | 0.58     | 0.77           | 0.75      | 0.39        | 0.42   |
| 33       | 0.53          | 0.57     | 0.78           | 0.76      | 0.38        | 0.41   |
| 34       | 0.53          | 0.57     | 0.78           | 0.76      | 0.38        | 0.41   |
| 35       | 0.52          | 0.57     | 0.79           | 0.76      | 0.37        | 0.41   |
| 36       | 0.52          | 0.56     | 0.79           | 0.77      | 0.37        | 0.40   |
| 37       | 0.51          | 0.56     | 0.79           | 0.77      | 0.36        | 0.40   |
| 38       | 0.51          | 0.55     | 0.80           | 0.78      | 0.36        | 0.39   |
| 39       | 0.50          | 0.55     | 0.80           | 0.78      | 0.36        | 0.39   |
| 40       | 0.50          | 0.54     | 0.81           | 0.79      | 0.35        | 0.38   |
| 41       | 0.49          | 0.53     | 0.81           | 0.79      | 0.35        | 0.38   |
| 42       | 0.49          | 0.53     | 0.82           | 0.79      | 0.34        | 0.38   |
| 43       | 0.48          | 0.52     | 0.82           | 0.80      | 0.34        | 0.37   |
| 44       | 0.47          | 0.52     | 0.83           | 0.80      | 0.33        | 0.37   |
| 45       | 0.47          | 0.51     | 0.83           | 0.81      | 0.33        | 0.36   |
| 46       | 0.46          | 0.50     | 0.83           | 0.81      | 0.32        | 0.35   |
| 47       | 0.46          | 0.50     | 0.84           | 0.82      | 0.32        | 0.35   |
| 48       | 0.45          | 0.49     | 0.84           | 0.82      | 0.31        | 0.34   |
| 49       | 0.44          | 0.48     | 0.85           | 0.83      | 0.30        | 0.33   |
| 50       | 0.44          | 0.48     | 0.85           | 0.83      | 0.30        | 0.33   |
| 51       | 0.43          | 0.47     | 0.86           | 0.84      | 0.30        | 0.32   |
| 52       | 0.42          | 0.46     | 0.86           | 0.84      | 0.29        | 0.32   |
| 53       | 0.42          | 0.46     | 0.87           | 0.85      | 0.29        | 0.32   |
| 54       | 0.41          | 0.45     | 0.87           | 0.85      | 0.28        | 0.31   |
| 55       | 0.40          | 0.44     | 0.87           | 0.85      | 0.27        | 0.30   |
| 56       | 0.40          | 0.43     | 0.88           | 0.86      | 0.27        | 0.30   |
| 57       | 0.39          | 0.42     | 0.88           | 0.86      | 0.27        | 0.29   |
| 58       | 0.38          | 0.42     | 0.89           | 0.87      | 0.26        | 0.29   |
| 59       | 0.37          | 0.41     | 0.89           | 0.87      | 0.25        | 0.28   |
| 60       | 0.37          | 0.40     | 0.90           | 0.88      | 0.25        | 0.27   |
| 61       | 0.36          | 0.39     | 0.90           | 0.88      | 0.24        | 0.27   |
| 62       | 0.35          | 0.38     | 0.91           | 0.89      | 0.23        | 0.26   |
| 63       | 0.34          | 0.37     | 0.91           | 0.89      | 0.23        | 0.25   |

Continued on next page

| $\alpha$ | $\phi_S^\ell$ | $\phi_S$ | $\varphi^\ell$ | $\varphi$ | $\psi^\ell$ | $\psi$ |
|----------|---------------|----------|----------------|-----------|-------------|--------|
| 64       | 0.33          | 0.36     | 0.92           | 0.89      | 0.22        | 0.24   |
| 65       | 0.32          | 0.36     | 0.92           | 0.90      | 0.21        | 0.24   |
| 66       | 0.32          | 0.35     | 0.92           | 0.90      | 0.21        | 0.24   |
| 67       | 0.31          | 0.34     | 0.93           | 0.91      | 0.20        | 0.23   |
| 68       | 0.30          | 0.33     | 0.93           | 0.91      | 0.20        | 0.22   |
| 69       | 0.29          | 0.32     | 0.93           | 0.91      | 0.19        | 0.22   |
| 70       | 0.28          | 0.31     | 0.94           | 0.92      | 0.18        | 0.21   |
| 71       | 0.27          | 0.30     | 0.94           | 0.92      | 0.18        | 0.20   |
| 72       | 0.26          | 0.29     | 0.94           | 0.92      | 0.17        | 0.19   |
| 73       | 0.25          | 0.28     | 0.95           | 0.92      | 0.16        | 0.19   |
| 74       | 0.25          | 0.28     | 0.95           | 0.93      | 0.16        | 0.19   |
| 75       | 0.24          | 0.27     | 0.95           | 0.93      | 0.16        | 0.18   |
| 76       | 0.23          | 0.26     | 0.95           | 0.93      | 0.15        | 0.17   |
| 77       | 0.22          | 0.25     | 0.95           | 0.93      | 0.14        | 0.17   |
| 78       | 0.21          | 0.24     | 0.96           | 0.94      | 0.14        | 0.16   |
| 79       | 0.21          | 0.23     | 0.96           | 0.94      | 0.14        | 0.15   |
| 80       | 0.20          | 0.22     | 0.96           | 0.94      | 0.13        | 0.15   |
| 81       | 0.19          | 0.22     | 0.96           | 0.94      | 0.12        | 0.15   |
| 82       | 0.18          | 0.21     | 0.96           | 0.94      | 0.12        | 0.14   |
| 83       | 0.18          | 0.20     | 0.96           | 0.95      | 0.12        | 0.13   |
| 84       | 0.17          | 0.19     | 0.96           | 0.95      | 0.11        | 0.13   |
| 85       | 0.16          | 0.19     | 0.96           | 0.95      | 0.11        | 0.13   |
| 86       | 0.16          | 0.18     | 0.96           | 0.95      | 0.11        | 0.12   |
| 87       | 0.15          | 0.18     | 0.97           | 0.95      | 0.10        | 0.12   |
| 88       | 0.14          | 0.17     | 0.97           | 0.95      | 0.09        | 0.11   |
| 89       | 0.14          | 0.17     | 0.97           | 0.95      | 0.09        | 0.11   |
| 90       | 0.14          | 0.17     | 0.97           | 0.95      | 0.09        | 0.11   |

Table S90: Reference ( $\phi_S$ ,  $\varphi$ ,  $\psi$ ) and approached ( $\phi_S^\ell$ ,  $\varphi^\ell$ ,  $\psi^\ell$ ) values of the topological descriptors for the first excited-state of the pyridinium-phenolate (PP), computed at the CIS/6-31++G(d,p) level of theory.  $\alpha$  is the pyridinium-phenolate central twist angle amplitude.

| $\alpha$ | $\phi_S^\ell$ | $\phi_S$ | $\varphi^\ell$ | $\varphi$ | $\psi^\ell$ | $\psi$ |
|----------|---------------|----------|----------------|-----------|-------------|--------|
| 0        | 0.59          | 0.65     | 0.71           | 0.68      | 0.44        | 0.49   |
| 1        | 0.59          | 0.65     | 0.71           | 0.68      | 0.44        | 0.49   |
| 2        | 0.59          | 0.65     | 0.71           | 0.68      | 0.44        | 0.49   |
| 3        | 0.59          | 0.65     | 0.71           | 0.68      | 0.44        | 0.49   |
| 4        | 0.59          | 0.64     | 0.71           | 0.68      | 0.44        | 0.48   |
| 5        | 0.59          | 0.64     | 0.71           | 0.68      | 0.44        | 0.48   |
| 6        | 0.59          | 0.64     | 0.71           | 0.69      | 0.44        | 0.48   |
| 7        | 0.59          | 0.64     | 0.71           | 0.69      | 0.44        | 0.48   |
| 8        | 0.59          | 0.64     | 0.71           | 0.69      | 0.44        | 0.48   |
| 9        | 0.59          | 0.64     | 0.71           | 0.69      | 0.44        | 0.48   |
| 10       | 0.59          | 0.64     | 0.71           | 0.69      | 0.44        | 0.48   |
| 11       | 0.59          | 0.64     | 0.72           | 0.69      | 0.44        | 0.48   |
| 12       | 0.59          | 0.64     | 0.72           | 0.69      | 0.44        | 0.48   |
| 13       | 0.59          | 0.63     | 0.72           | 0.70      | 0.44        | 0.47   |
| 14       | 0.58          | 0.63     | 0.72           | 0.70      | 0.43        | 0.47   |
| 15       | 0.58          | 0.63     | 0.72           | 0.70      | 0.43        | 0.47   |
| 16       | 0.58          | 0.63     | 0.72           | 0.70      | 0.43        | 0.47   |
| 17       | 0.58          | 0.63     | 0.73           | 0.70      | 0.43        | 0.47   |
| 18       | 0.58          | 0.62     | 0.73           | 0.71      | 0.43        | 0.46   |
| 19       | 0.57          | 0.62     | 0.73           | 0.71      | 0.42        | 0.46   |
| 20       | 0.57          | 0.62     | 0.73           | 0.71      | 0.42        | 0.46   |
| 21       | 0.57          | 0.62     | 0.74           | 0.71      | 0.42        | 0.46   |
| 22       | 0.57          | 0.61     | 0.74           | 0.72      | 0.42        | 0.45   |
| 23       | 0.57          | 0.61     | 0.74           | 0.72      | 0.42        | 0.45   |
| 24       | 0.56          | 0.61     | 0.75           | 0.72      | 0.41        | 0.45   |
| 25       | 0.56          | 0.60     | 0.75           | 0.73      | 0.41        | 0.44   |
| 26       | 0.56          | 0.60     | 0.75           | 0.73      | 0.41        | 0.44   |
| 27       | 0.55          | 0.60     | 0.76           | 0.73      | 0.40        | 0.44   |
| 28       | 0.55          | 0.59     | 0.76           | 0.74      | 0.40        | 0.43   |
| 29       | 0.55          | 0.59     | 0.76           | 0.74      | 0.40        | 0.43   |
| 30       | 0.54          | 0.59     | 0.77           | 0.74      | 0.39        | 0.43   |
| 31       | 0.54          | 0.58     | 0.77           | 0.75      | 0.39        | 0.42   |

Continued on next page



| $\alpha$ | $\phi_S^\ell$ | $\phi_S$ | $\varphi^\ell$ | $\varphi$ | $\psi^\ell$ | $\psi$ |
|----------|---------------|----------|----------------|-----------|-------------|--------|
| 32       | 0.54          | 0.58     | 0.77           | 0.75      | 0.39        | 0.42   |
| 33       | 0.53          | 0.57     | 0.78           | 0.76      | 0.38        | 0.41   |
| 34       | 0.53          | 0.57     | 0.78           | 0.76      | 0.38        | 0.41   |
| 35       | 0.52          | 0.57     | 0.78           | 0.76      | 0.37        | 0.41   |
| 36       | 0.52          | 0.56     | 0.79           | 0.77      | 0.37        | 0.40   |
| 37       | 0.51          | 0.56     | 0.79           | 0.77      | 0.36        | 0.40   |
| 38       | 0.51          | 0.55     | 0.80           | 0.78      | 0.36        | 0.39   |
| 39       | 0.50          | 0.55     | 0.80           | 0.78      | 0.36        | 0.39   |
| 40       | 0.50          | 0.54     | 0.81           | 0.79      | 0.35        | 0.38   |
| 41       | 0.49          | 0.53     | 0.81           | 0.79      | 0.35        | 0.38   |
| 42       | 0.49          | 0.53     | 0.82           | 0.79      | 0.34        | 0.38   |
| 43       | 0.48          | 0.52     | 0.82           | 0.80      | 0.34        | 0.37   |
| 44       | 0.47          | 0.52     | 0.83           | 0.80      | 0.33        | 0.37   |
| 45       | 0.47          | 0.51     | 0.83           | 0.81      | 0.33        | 0.36   |
| 46       | 0.46          | 0.50     | 0.83           | 0.81      | 0.32        | 0.35   |
| 47       | 0.46          | 0.50     | 0.84           | 0.82      | 0.32        | 0.35   |
| 48       | 0.45          | 0.49     | 0.84           | 0.82      | 0.31        | 0.34   |
| 49       | 0.44          | 0.48     | 0.85           | 0.83      | 0.30        | 0.33   |
| 50       | 0.44          | 0.48     | 0.85           | 0.83      | 0.30        | 0.33   |
| 51       | 0.43          | 0.47     | 0.86           | 0.84      | 0.30        | 0.32   |
| 52       | 0.42          | 0.46     | 0.86           | 0.84      | 0.29        | 0.32   |
| 53       | 0.42          | 0.46     | 0.87           | 0.85      | 0.29        | 0.32   |
| 54       | 0.41          | 0.45     | 0.87           | 0.85      | 0.28        | 0.31   |
| 55       | 0.40          | 0.44     | 0.87           | 0.85      | 0.27        | 0.30   |
| 56       | 0.40          | 0.43     | 0.88           | 0.86      | 0.27        | 0.30   |
| 57       | 0.39          | 0.42     | 0.88           | 0.86      | 0.27        | 0.29   |
| 58       | 0.38          | 0.42     | 0.89           | 0.87      | 0.26        | 0.29   |
| 59       | 0.37          | 0.41     | 0.89           | 0.87      | 0.25        | 0.28   |
| 60       | 0.37          | 0.40     | 0.90           | 0.88      | 0.25        | 0.27   |
| 61       | 0.36          | 0.39     | 0.90           | 0.88      | 0.24        | 0.27   |
| 62       | 0.35          | 0.38     | 0.91           | 0.89      | 0.23        | 0.26   |
| 63       | 0.34          | 0.37     | 0.91           | 0.89      | 0.23        | 0.25   |

Continued on next page

| $\alpha$ | $\phi_S^\ell$ | $\phi_S$ | $\varphi^\ell$ | $\varphi$ | $\psi^\ell$ | $\psi$ |
|----------|---------------|----------|----------------|-----------|-------------|--------|
| 64       | 0.33          | 0.36     | 0.92           | 0.89      | 0.22        | 0.24   |
| 65       | 0.33          | 0.36     | 0.92           | 0.90      | 0.22        | 0.24   |
| 66       | 0.32          | 0.35     | 0.92           | 0.90      | 0.21        | 0.24   |
| 67       | 0.31          | 0.34     | 0.93           | 0.91      | 0.20        | 0.23   |
| 68       | 0.30          | 0.33     | 0.93           | 0.91      | 0.20        | 0.22   |
| 69       | 0.29          | 0.32     | 0.93           | 0.91      | 0.19        | 0.22   |
| 70       | 0.28          | 0.31     | 0.94           | 0.92      | 0.18        | 0.21   |
| 71       | 0.27          | 0.30     | 0.94           | 0.92      | 0.18        | 0.20   |
| 72       | 0.27          | 0.29     | 0.94           | 0.92      | 0.18        | 0.19   |
| 73       | 0.26          | 0.28     | 0.95           | 0.92      | 0.17        | 0.19   |
| 74       | 0.25          | 0.28     | 0.95           | 0.93      | 0.16        | 0.19   |
| 75       | 0.24          | 0.27     | 0.95           | 0.93      | 0.16        | 0.18   |
| 76       | 0.23          | 0.26     | 0.95           | 0.93      | 0.15        | 0.17   |
| 77       | 0.22          | 0.25     | 0.95           | 0.94      | 0.14        | 0.17   |
| 78       | 0.22          | 0.24     | 0.96           | 0.94      | 0.14        | 0.16   |
| 79       | 0.21          | 0.23     | 0.96           | 0.94      | 0.14        | 0.15   |
| 80       | 0.20          | 0.22     | 0.96           | 0.94      | 0.13        | 0.15   |
| 81       | 0.19          | 0.22     | 0.96           | 0.94      | 0.12        | 0.15   |
| 82       | 0.19          | 0.21     | 0.96           | 0.94      | 0.12        | 0.14   |
| 83       | 0.18          | 0.20     | 0.96           | 0.95      | 0.12        | 0.13   |
| 84       | 0.17          | 0.19     | 0.96           | 0.95      | 0.11        | 0.13   |
| 85       | 0.17          | 0.19     | 0.96           | 0.95      | 0.11        | 0.13   |
| 86       | 0.16          | 0.18     | 0.96           | 0.95      | 0.11        | 0.12   |
| 87       | 0.15          | 0.18     | 0.96           | 0.95      | 0.10        | 0.12   |
| 88       | 0.15          | 0.17     | 0.96           | 0.95      | 0.10        | 0.11   |
| 89       | 0.14          | 0.17     | 0.96           | 0.95      | 0.09        | 0.11   |
| 90       | 0.14          | 0.17     | 0.96           | 0.95      | 0.09        | 0.11   |

Table S91: Reference ( $\phi_S$ ,  $\varphi$ ,  $\psi$ ) and approached ( $\phi_S^\ell$ ,  $\varphi^\ell$ ,  $\psi^\ell$ ) values of the topological descriptors for the first excited-state of the pyridinium-phenolate (PP), computed at the CIS/6-31+G(d,p) level of theory.  $\alpha$  is the pyridinium-phenolate central twist angle amplitude.

| $\alpha$ | $\phi_S^\ell$ | $\phi_S$ | $\varphi^\ell$ | $\varphi$ | $\psi^\ell$ | $\psi$ |
|----------|---------------|----------|----------------|-----------|-------------|--------|
| 0        | 0.59          | 0.65     | 0.71           | 0.68      | 0.44        | 0.49   |
| 1        | 0.59          | 0.65     | 0.71           | 0.68      | 0.44        | 0.49   |
| 2        | 0.59          | 0.65     | 0.71           | 0.68      | 0.44        | 0.49   |
| 3        | 0.59          | 0.65     | 0.71           | 0.68      | 0.44        | 0.49   |
| 4        | 0.59          | 0.64     | 0.71           | 0.68      | 0.44        | 0.48   |
| 5        | 0.59          | 0.64     | 0.71           | 0.68      | 0.44        | 0.48   |
| 6        | 0.59          | 0.64     | 0.71           | 0.69      | 0.44        | 0.48   |
| 7        | 0.59          | 0.64     | 0.71           | 0.69      | 0.44        | 0.48   |
| 8        | 0.59          | 0.64     | 0.71           | 0.69      | 0.44        | 0.48   |
| 9        | 0.59          | 0.64     | 0.71           | 0.69      | 0.44        | 0.48   |
| 10       | 0.59          | 0.64     | 0.71           | 0.69      | 0.44        | 0.48   |
| 11       | 0.59          | 0.64     | 0.72           | 0.69      | 0.44        | 0.48   |
| 12       | 0.59          | 0.64     | 0.72           | 0.69      | 0.44        | 0.48   |
| 13       | 0.59          | 0.63     | 0.72           | 0.70      | 0.44        | 0.47   |
| 14       | 0.58          | 0.63     | 0.72           | 0.70      | 0.43        | 0.47   |
| 15       | 0.58          | 0.63     | 0.72           | 0.70      | 0.43        | 0.47   |
| 16       | 0.58          | 0.63     | 0.72           | 0.70      | 0.43        | 0.47   |
| 17       | 0.58          | 0.63     | 0.73           | 0.70      | 0.43        | 0.47   |
| 18       | 0.58          | 0.62     | 0.73           | 0.71      | 0.43        | 0.46   |
| 19       | 0.57          | 0.62     | 0.73           | 0.71      | 0.42        | 0.46   |
| 20       | 0.57          | 0.62     | 0.74           | 0.71      | 0.42        | 0.46   |
| 21       | 0.57          | 0.62     | 0.74           | 0.71      | 0.42        | 0.46   |
| 22       | 0.57          | 0.61     | 0.74           | 0.72      | 0.42        | 0.45   |
| 23       | 0.57          | 0.61     | 0.74           | 0.72      | 0.42        | 0.45   |
| 24       | 0.56          | 0.61     | 0.75           | 0.72      | 0.41        | 0.45   |
| 25       | 0.56          | 0.60     | 0.75           | 0.73      | 0.41        | 0.44   |
| 26       | 0.56          | 0.60     | 0.75           | 0.73      | 0.41        | 0.44   |
| 27       | 0.55          | 0.60     | 0.76           | 0.73      | 0.40        | 0.44   |
| 28       | 0.55          | 0.59     | 0.76           | 0.74      | 0.40        | 0.43   |
| 29       | 0.55          | 0.59     | 0.76           | 0.74      | 0.40        | 0.43   |
| 30       | 0.54          | 0.59     | 0.77           | 0.74      | 0.39        | 0.43   |
| 31       | 0.54          | 0.58     | 0.77           | 0.75      | 0.39        | 0.42   |

Continued on next page

| $\alpha$ | $\phi_S^\ell$ | $\phi_S$ | $\varphi^\ell$ | $\varphi$ | $\psi^\ell$ | $\psi$ |
|----------|---------------|----------|----------------|-----------|-------------|--------|
| 32       | 0.54          | 0.58     | 0.77           | 0.75      | 0.39        | 0.42   |
| 33       | 0.53          | 0.57     | 0.78           | 0.76      | 0.38        | 0.41   |
| 34       | 0.53          | 0.57     | 0.78           | 0.76      | 0.38        | 0.41   |
| 35       | 0.52          | 0.57     | 0.78           | 0.76      | 0.37        | 0.41   |
| 36       | 0.52          | 0.56     | 0.79           | 0.77      | 0.37        | 0.40   |
| 37       | 0.51          | 0.56     | 0.79           | 0.77      | 0.36        | 0.40   |
| 38       | 0.51          | 0.55     | 0.80           | 0.78      | 0.36        | 0.39   |
| 39       | 0.50          | 0.55     | 0.80           | 0.78      | 0.36        | 0.39   |
| 40       | 0.50          | 0.54     | 0.81           | 0.79      | 0.35        | 0.38   |
| 41       | 0.49          | 0.53     | 0.81           | 0.79      | 0.35        | 0.38   |
| 42       | 0.49          | 0.53     | 0.82           | 0.79      | 0.34        | 0.38   |
| 43       | 0.48          | 0.52     | 0.82           | 0.80      | 0.34        | 0.37   |
| 44       | 0.47          | 0.52     | 0.83           | 0.80      | 0.33        | 0.37   |
| 45       | 0.47          | 0.51     | 0.83           | 0.81      | 0.33        | 0.36   |
| 46       | 0.46          | 0.50     | 0.83           | 0.81      | 0.32        | 0.35   |
| 47       | 0.46          | 0.50     | 0.84           | 0.82      | 0.32        | 0.35   |
| 48       | 0.45          | 0.49     | 0.84           | 0.82      | 0.31        | 0.34   |
| 49       | 0.44          | 0.48     | 0.85           | 0.83      | 0.30        | 0.33   |
| 50       | 0.44          | 0.48     | 0.85           | 0.83      | 0.30        | 0.33   |
| 51       | 0.43          | 0.47     | 0.86           | 0.84      | 0.30        | 0.32   |
| 52       | 0.42          | 0.46     | 0.86           | 0.84      | 0.29        | 0.32   |
| 53       | 0.42          | 0.46     | 0.87           | 0.85      | 0.29        | 0.32   |
| 54       | 0.41          | 0.45     | 0.87           | 0.85      | 0.28        | 0.31   |
| 55       | 0.40          | 0.44     | 0.87           | 0.85      | 0.27        | 0.30   |
| 56       | 0.40          | 0.43     | 0.88           | 0.86      | 0.27        | 0.30   |
| 57       | 0.39          | 0.42     | 0.88           | 0.86      | 0.27        | 0.29   |
| 58       | 0.38          | 0.42     | 0.89           | 0.87      | 0.26        | 0.29   |
| 59       | 0.37          | 0.41     | 0.89           | 0.87      | 0.25        | 0.28   |
| 60       | 0.37          | 0.40     | 0.90           | 0.88      | 0.25        | 0.27   |
| 61       | 0.36          | 0.39     | 0.90           | 0.88      | 0.24        | 0.27   |
| 62       | 0.35          | 0.38     | 0.91           | 0.89      | 0.23        | 0.26   |
| 63       | 0.34          | 0.37     | 0.91           | 0.89      | 0.23        | 0.25   |

Continued on next page

| $\alpha$ | $\phi_S^\ell$ | $\phi_S$ | $\varphi^\ell$ | $\varphi$ | $\psi^\ell$ | $\psi$ |
|----------|---------------|----------|----------------|-----------|-------------|--------|
| 64       | 0.33          | 0.36     | 0.92           | 0.89      | 0.22        | 0.24   |
| 65       | 0.33          | 0.36     | 0.92           | 0.90      | 0.22        | 0.24   |
| 66       | 0.32          | 0.35     | 0.92           | 0.90      | 0.21        | 0.24   |
| 67       | 0.31          | 0.34     | 0.93           | 0.91      | 0.20        | 0.23   |
| 68       | 0.30          | 0.33     | 0.93           | 0.91      | 0.20        | 0.22   |
| 69       | 0.29          | 0.32     | 0.93           | 0.91      | 0.19        | 0.22   |
| 70       | 0.28          | 0.31     | 0.94           | 0.92      | 0.18        | 0.21   |
| 71       | 0.27          | 0.30     | 0.94           | 0.92      | 0.18        | 0.20   |
| 72       | 0.27          | 0.29     | 0.94           | 0.92      | 0.18        | 0.19   |
| 73       | 0.26          | 0.28     | 0.95           | 0.92      | 0.17        | 0.19   |
| 74       | 0.25          | 0.27     | 0.95           | 0.93      | 0.16        | 0.18   |
| 75       | 0.24          | 0.27     | 0.95           | 0.93      | 0.16        | 0.18   |
| 76       | 0.23          | 0.26     | 0.95           | 0.93      | 0.15        | 0.17   |
| 77       | 0.22          | 0.25     | 0.95           | 0.94      | 0.14        | 0.17   |
| 78       | 0.22          | 0.24     | 0.96           | 0.94      | 0.14        | 0.16   |
| 79       | 0.21          | 0.23     | 0.96           | 0.94      | 0.14        | 0.15   |
| 80       | 0.20          | 0.22     | 0.96           | 0.94      | 0.13        | 0.15   |
| 81       | 0.19          | 0.22     | 0.96           | 0.94      | 0.12        | 0.15   |
| 82       | 0.19          | 0.21     | 0.96           | 0.94      | 0.12        | 0.14   |
| 83       | 0.18          | 0.20     | 0.96           | 0.95      | 0.12        | 0.13   |
| 84       | 0.17          | 0.19     | 0.96           | 0.95      | 0.11        | 0.13   |
| 85       | 0.16          | 0.19     | 0.96           | 0.95      | 0.11        | 0.13   |
| 86       | 0.16          | 0.18     | 0.96           | 0.95      | 0.11        | 0.12   |
| 87       | 0.15          | 0.17     | 0.96           | 0.95      | 0.10        | 0.11   |
| 88       | 0.15          | 0.17     | 0.96           | 0.95      | 0.10        | 0.11   |
| 89       | 0.14          | 0.17     | 0.96           | 0.95      | 0.09        | 0.11   |
| 90       | 0.14          | 0.16     | 0.96           | 0.95      | 0.09        | 0.11   |

Table S92: Reference ( $\phi_S$ ,  $\varphi$ ,  $\psi$ ) and approached ( $\phi_S^\ell$ ,  $\varphi^\ell$ ,  $\psi^\ell$ ) values of the topological descriptors for the first excited-state of the pyridinium-phenolate (PP), computed at the CIS/6-31+G(d) level of theory.  $\alpha$  is the pyridinium-phenolate central twist angle amplitude.

| $\alpha$ | $\phi_S^\ell$ | $\phi_S$ | $\varphi^\ell$ | $\varphi$ | $\psi^\ell$ | $\psi$ |
|----------|---------------|----------|----------------|-----------|-------------|--------|
| 0        | 0.62          | 0.67     | 0.71           | 0.67      | 0.46        | 0.50   |
| 1        | 0.62          | 0.67     | 0.71           | 0.67      | 0.46        | 0.50   |
| 2        | 0.62          | 0.67     | 0.71           | 0.67      | 0.46        | 0.50   |
| 3        | 0.62          | 0.67     | 0.71           | 0.67      | 0.46        | 0.50   |
| 4        | 0.62          | 0.67     | 0.71           | 0.67      | 0.46        | 0.50   |
| 5        | 0.62          | 0.67     | 0.71           | 0.67      | 0.46        | 0.50   |
| 6        | 0.62          | 0.67     | 0.71           | 0.67      | 0.46        | 0.50   |
| 7        | 0.62          | 0.67     | 0.71           | 0.67      | 0.46        | 0.50   |
| 8        | 0.62          | 0.67     | 0.71           | 0.67      | 0.46        | 0.50   |
| 9        | 0.62          | 0.67     | 0.71           | 0.67      | 0.46        | 0.50   |
| 10       | 0.62          | 0.67     | 0.71           | 0.67      | 0.46        | 0.50   |
| 11       | 0.62          | 0.66     | 0.71           | 0.68      | 0.46        | 0.49   |
| 12       | 0.61          | 0.66     | 0.72           | 0.68      | 0.45        | 0.49   |
| 13       | 0.61          | 0.66     | 0.72           | 0.68      | 0.45        | 0.49   |
| 14       | 0.61          | 0.66     | 0.72           | 0.68      | 0.45        | 0.49   |
| 15       | 0.61          | 0.66     | 0.72           | 0.68      | 0.45        | 0.49   |
| 16       | 0.61          | 0.66     | 0.72           | 0.69      | 0.45        | 0.49   |
| 17       | 0.61          | 0.65     | 0.72           | 0.69      | 0.45        | 0.48   |
| 18       | 0.60          | 0.65     | 0.73           | 0.69      | 0.44        | 0.48   |
| 19       | 0.60          | 0.65     | 0.73           | 0.69      | 0.44        | 0.48   |
| 20       | 0.60          | 0.65     | 0.73           | 0.70      | 0.44        | 0.48   |
| 21       | 0.60          | 0.64     | 0.73           | 0.70      | 0.44        | 0.47   |
| 22       | 0.60          | 0.64     | 0.74           | 0.70      | 0.43        | 0.47   |
| 23       | 0.59          | 0.64     | 0.74           | 0.71      | 0.43        | 0.47   |
| 24       | 0.59          | 0.63     | 0.74           | 0.71      | 0.43        | 0.46   |
| 25       | 0.59          | 0.63     | 0.75           | 0.71      | 0.42        | 0.46   |
| 26       | 0.59          | 0.63     | 0.75           | 0.72      | 0.42        | 0.46   |
| 27       | 0.58          | 0.62     | 0.75           | 0.72      | 0.42        | 0.45   |
| 28       | 0.58          | 0.62     | 0.76           | 0.72      | 0.41        | 0.45   |
| 29       | 0.58          | 0.62     | 0.76           | 0.73      | 0.41        | 0.45   |
| 30       | 0.57          | 0.61     | 0.76           | 0.73      | 0.41        | 0.44   |
| 31       | 0.57          | 0.61     | 0.77           | 0.74      | 0.41        | 0.44   |

Continued on next page

| $\alpha$ | $\phi_S^\ell$ | $\phi_S$ | $\varphi^\ell$ | $\varphi$ | $\psi^\ell$ | $\psi$ |
|----------|---------------|----------|----------------|-----------|-------------|--------|
| 32       | 0.56          | 0.60     | 0.77           | 0.74      | 0.40        | 0.43   |
| 33       | 0.56          | 0.60     | 0.78           | 0.74      | 0.40        | 0.43   |
| 34       | 0.56          | 0.59     | 0.78           | 0.75      | 0.40        | 0.42   |
| 35       | 0.55          | 0.59     | 0.78           | 0.75      | 0.39        | 0.42   |
| 36       | 0.55          | 0.58     | 0.79           | 0.76      | 0.39        | 0.41   |
| 37       | 0.54          | 0.58     | 0.79           | 0.76      | 0.38        | 0.41   |
| 38       | 0.54          | 0.57     | 0.80           | 0.77      | 0.38        | 0.41   |
| 39       | 0.53          | 0.57     | 0.80           | 0.77      | 0.37        | 0.41   |
| 40       | 0.53          | 0.56     | 0.81           | 0.78      | 0.37        | 0.40   |
| 41       | 0.52          | 0.56     | 0.81           | 0.78      | 0.36        | 0.40   |
| 42       | 0.51          | 0.55     | 0.82           | 0.78      | 0.35        | 0.39   |
| 43       | 0.51          | 0.54     | 0.82           | 0.79      | 0.35        | 0.38   |
| 44       | 0.50          | 0.54     | 0.83           | 0.79      | 0.35        | 0.38   |
| 45       | 0.50          | 0.53     | 0.83           | 0.80      | 0.35        | 0.37   |
| 46       | 0.49          | 0.52     | 0.84           | 0.80      | 0.34        | 0.37   |
| 47       | 0.48          | 0.52     | 0.84           | 0.81      | 0.33        | 0.36   |
| 48       | 0.48          | 0.51     | 0.84           | 0.81      | 0.33        | 0.36   |
| 49       | 0.47          | 0.50     | 0.85           | 0.82      | 0.32        | 0.35   |
| 50       | 0.46          | 0.50     | 0.85           | 0.82      | 0.32        | 0.35   |
| 51       | 0.46          | 0.49     | 0.86           | 0.83      | 0.31        | 0.34   |
| 52       | 0.45          | 0.48     | 0.86           | 0.83      | 0.31        | 0.33   |
| 53       | 0.44          | 0.47     | 0.87           | 0.84      | 0.30        | 0.32   |
| 54       | 0.43          | 0.46     | 0.87           | 0.84      | 0.29        | 0.32   |
| 55       | 0.43          | 0.46     | 0.87           | 0.85      | 0.29        | 0.32   |
| 56       | 0.42          | 0.45     | 0.88           | 0.85      | 0.28        | 0.31   |
| 57       | 0.41          | 0.44     | 0.88           | 0.86      | 0.28        | 0.30   |
| 58       | 0.40          | 0.43     | 0.89           | 0.86      | 0.27        | 0.30   |
| 59       | 0.39          | 0.42     | 0.89           | 0.87      | 0.26        | 0.29   |
| 60       | 0.39          | 0.41     | 0.90           | 0.87      | 0.26        | 0.28   |
| 61       | 0.38          | 0.41     | 0.90           | 0.88      | 0.25        | 0.28   |
| 62       | 0.37          | 0.40     | 0.91           | 0.88      | 0.25        | 0.27   |
| 63       | 0.36          | 0.39     | 0.91           | 0.89      | 0.24        | 0.26   |

Continued on next page

| $\alpha$ | $\phi_S^\ell$ | $\phi_S$ | $\varphi^\ell$ | $\varphi$ | $\psi^\ell$ | $\psi$ |
|----------|---------------|----------|----------------|-----------|-------------|--------|
| 64       | 0.35          | 0.38     | 0.92           | 0.89      | 0.23        | 0.26   |
| 65       | 0.34          | 0.37     | 0.92           | 0.89      | 0.23        | 0.25   |
| 66       | 0.33          | 0.36     | 0.92           | 0.90      | 0.22        | 0.24   |
| 67       | 0.32          | 0.35     | 0.93           | 0.90      | 0.21        | 0.24   |
| 68       | 0.31          | 0.34     | 0.93           | 0.91      | 0.20        | 0.23   |
| 69       | 0.30          | 0.33     | 0.94           | 0.91      | 0.20        | 0.22   |
| 70       | 0.29          | 0.32     | 0.94           | 0.91      | 0.19        | 0.22   |
| 71       | 0.28          | 0.31     | 0.94           | 0.92      | 0.18        | 0.21   |
| 72       | 0.27          | 0.30     | 0.95           | 0.92      | 0.18        | 0.20   |
| 73       | 0.26          | 0.29     | 0.95           | 0.92      | 0.17        | 0.19   |
| 74       | 0.25          | 0.28     | 0.95           | 0.93      | 0.16        | 0.19   |
| 75       | 0.24          | 0.27     | 0.95           | 0.93      | 0.16        | 0.18   |
| 76       | 0.23          | 0.26     | 0.96           | 0.93      | 0.15        | 0.17   |
| 77       | 0.22          | 0.25     | 0.96           | 0.93      | 0.14        | 0.17   |
| 78       | 0.21          | 0.24     | 0.96           | 0.94      | 0.14        | 0.16   |
| 79       | 0.20          | 0.24     | 0.96           | 0.94      | 0.13        | 0.16   |
| 80       | 0.19          | 0.23     | 0.96           | 0.94      | 0.12        | 0.15   |
| 81       | 0.18          | 0.22     | 0.97           | 0.94      | 0.12        | 0.15   |
| 82       | 0.17          | 0.21     | 0.97           | 0.94      | 0.11        | 0.14   |
| 83       | 0.17          | 0.20     | 0.97           | 0.95      | 0.11        | 0.13   |
| 84       | 0.16          | 0.19     | 0.97           | 0.95      | 0.10        | 0.13   |
| 85       | 0.15          | 0.19     | 0.97           | 0.95      | 0.10        | 0.13   |
| 86       | 0.14          | 0.18     | 0.97           | 0.95      | 0.09        | 0.12   |
| 87       | 0.13          | 0.18     | 0.97           | 0.95      | 0.08        | 0.12   |
| 88       | 0.13          | 0.17     | 0.97           | 0.95      | 0.08        | 0.11   |
| 89       | 0.12          | 0.17     | 0.97           | 0.95      | 0.08        | 0.11   |
| 90       | 0.12          | 0.16     | 0.97           | 0.95      | 0.08        | 0.11   |

Table S93: Reference ( $\phi_S$ ,  $\varphi$ ,  $\psi$ ) and approached ( $\phi_S^\ell$ ,  $\varphi^\ell$ ,  $\psi^\ell$ ) values of the topological descriptors for the first excited-state of the pyridinium-phenolate (PP), computed at the CIS/6-31G(d) level of theory.  $\alpha$  is the pyridinium-phenolate central twist angle amplitude.



| $\alpha$ | $\phi_S^\ell$ | $\phi_S$ | $\varphi^\ell$ | $\varphi$ | $\psi^\ell$ | $\psi$ |
|----------|---------------|----------|----------------|-----------|-------------|--------|
| 0        | 0.59          | 0.63     | 0.71           | 0.69      | 0.44        | 0.47   |
| 1        | 0.59          | 0.63     | 0.71           | 0.69      | 0.44        | 0.47   |
| 2        | 0.59          | 0.63     | 0.71           | 0.69      | 0.44        | 0.47   |
| 3        | 0.59          | 0.63     | 0.72           | 0.69      | 0.44        | 0.47   |
| 4        | 0.59          | 0.63     | 0.72           | 0.69      | 0.44        | 0.47   |
| 5        | 0.59          | 0.63     | 0.72           | 0.69      | 0.44        | 0.47   |
| 6        | 0.58          | 0.63     | 0.72           | 0.70      | 0.43        | 0.47   |
| 7        | 0.58          | 0.63     | 0.72           | 0.70      | 0.43        | 0.47   |
| 8        | 0.58          | 0.63     | 0.72           | 0.70      | 0.43        | 0.47   |
| 9        | 0.58          | 0.63     | 0.72           | 0.70      | 0.43        | 0.47   |
| 10       | 0.58          | 0.63     | 0.72           | 0.70      | 0.43        | 0.47   |
| 11       | 0.58          | 0.62     | 0.72           | 0.70      | 0.43        | 0.46   |
| 12       | 0.58          | 0.62     | 0.72           | 0.70      | 0.43        | 0.46   |
| 13       | 0.58          | 0.62     | 0.73           | 0.71      | 0.43        | 0.46   |
| 14       | 0.58          | 0.62     | 0.73           | 0.71      | 0.43        | 0.46   |
| 15       | 0.57          | 0.62     | 0.73           | 0.71      | 0.42        | 0.46   |
| 16       | 0.57          | 0.62     | 0.73           | 0.71      | 0.42        | 0.46   |
| 17       | 0.57          | 0.61     | 0.73           | 0.71      | 0.42        | 0.45   |
| 18       | 0.57          | 0.61     | 0.74           | 0.72      | 0.42        | 0.45   |
| 19       | 0.57          | 0.61     | 0.74           | 0.72      | 0.42        | 0.45   |
| 20       | 0.56          | 0.61     | 0.74           | 0.72      | 0.41        | 0.45   |
| 21       | 0.56          | 0.60     | 0.74           | 0.72      | 0.41        | 0.44   |
| 22       | 0.56          | 0.60     | 0.75           | 0.73      | 0.41        | 0.44   |
| 23       | 0.56          | 0.60     | 0.75           | 0.73      | 0.41        | 0.44   |
| 24       | 0.55          | 0.60     | 0.75           | 0.73      | 0.40        | 0.44   |
| 25       | 0.55          | 0.59     | 0.76           | 0.74      | 0.40        | 0.43   |
| 26       | 0.55          | 0.59     | 0.76           | 0.74      | 0.40        | 0.43   |
| 27       | 0.54          | 0.59     | 0.76           | 0.74      | 0.39        | 0.43   |
| 28       | 0.54          | 0.58     | 0.77           | 0.75      | 0.39        | 0.42   |
| 29       | 0.54          | 0.58     | 0.77           | 0.75      | 0.39        | 0.42   |
| 30       | 0.53          | 0.57     | 0.77           | 0.75      | 0.38        | 0.41   |
| 31       | 0.53          | 0.57     | 0.78           | 0.76      | 0.38        | 0.41   |

Continued on next page

| $\alpha$ | $\phi_S^\ell$ | $\phi_S$ | $\varphi^\ell$ | $\varphi$ | $\psi^\ell$ | $\psi$ |
|----------|---------------|----------|----------------|-----------|-------------|--------|
| 32       | 0.53          | 0.57     | 0.78           | 0.76      | 0.38        | 0.41   |
| 33       | 0.52          | 0.56     | 0.78           | 0.76      | 0.37        | 0.40   |
| 34       | 0.52          | 0.56     | 0.79           | 0.77      | 0.37        | 0.40   |
| 35       | 0.51          | 0.55     | 0.79           | 0.77      | 0.36        | 0.39   |
| 36       | 0.51          | 0.55     | 0.80           | 0.78      | 0.36        | 0.39   |
| 37       | 0.50          | 0.54     | 0.80           | 0.78      | 0.36        | 0.39   |
| 38       | 0.50          | 0.54     | 0.80           | 0.79      | 0.36        | 0.38   |
| 39       | 0.49          | 0.53     | 0.81           | 0.79      | 0.35        | 0.38   |
| 40       | 0.49          | 0.53     | 0.81           | 0.79      | 0.35        | 0.38   |
| 41       | 0.48          | 0.52     | 0.82           | 0.80      | 0.34        | 0.37   |
| 42       | 0.48          | 0.52     | 0.82           | 0.80      | 0.34        | 0.37   |
| 43       | 0.47          | 0.51     | 0.83           | 0.81      | 0.33        | 0.36   |
| 44       | 0.46          | 0.51     | 0.83           | 0.81      | 0.32        | 0.36   |
| 45       | 0.46          | 0.50     | 0.84           | 0.82      | 0.32        | 0.35   |
| 46       | 0.45          | 0.49     | 0.84           | 0.82      | 0.31        | 0.34   |
| 47       | 0.45          | 0.49     | 0.85           | 0.83      | 0.31        | 0.34   |
| 48       | 0.44          | 0.48     | 0.85           | 0.83      | 0.30        | 0.33   |
| 49       | 0.43          | 0.47     | 0.85           | 0.83      | 0.30        | 0.33   |
| 50       | 0.43          | 0.47     | 0.86           | 0.84      | 0.30        | 0.32   |
| 51       | 0.42          | 0.46     | 0.86           | 0.84      | 0.29        | 0.32   |
| 52       | 0.41          | 0.45     | 0.87           | 0.85      | 0.28        | 0.31   |
| 53       | 0.41          | 0.44     | 0.87           | 0.85      | 0.28        | 0.30   |
| 54       | 0.40          | 0.44     | 0.88           | 0.86      | 0.27        | 0.30   |
| 55       | 0.39          | 0.43     | 0.88           | 0.86      | 0.27        | 0.30   |
| 56       | 0.39          | 0.42     | 0.89           | 0.87      | 0.26        | 0.29   |
| 57       | 0.38          | 0.41     | 0.89           | 0.87      | 0.26        | 0.28   |
| 58       | 0.37          | 0.41     | 0.90           | 0.87      | 0.25        | 0.28   |
| 59       | 0.36          | 0.40     | 0.90           | 0.88      | 0.24        | 0.27   |
| 60       | 0.35          | 0.39     | 0.91           | 0.88      | 0.23        | 0.27   |
| 61       | 0.35          | 0.38     | 0.91           | 0.89      | 0.23        | 0.26   |
| 62       | 0.34          | 0.37     | 0.92           | 0.89      | 0.23        | 0.25   |
| 63       | 0.33          | 0.36     | 0.92           | 0.90      | 0.22        | 0.24   |

Continued on next page

| $\alpha$ | $\phi_S^\ell$ | $\phi_S$ | $\varphi^\ell$ | $\varphi$ | $\psi^\ell$ | $\psi$ |
|----------|---------------|----------|----------------|-----------|-------------|--------|
| 64       | 0.32          | 0.36     | 0.92           | 0.90      | 0.21        | 0.24   |
| 65       | 0.31          | 0.35     | 0.93           | 0.90      | 0.20        | 0.24   |
| 66       | 0.30          | 0.34     | 0.93           | 0.91      | 0.20        | 0.23   |
| 67       | 0.29          | 0.33     | 0.94           | 0.91      | 0.19        | 0.22   |
| 68       | 0.29          | 0.32     | 0.94           | 0.91      | 0.19        | 0.22   |
| 69       | 0.28          | 0.31     | 0.94           | 0.92      | 0.18        | 0.21   |
| 70       | 0.27          | 0.30     | 0.95           | 0.92      | 0.18        | 0.20   |
| 71       | 0.26          | 0.29     | 0.95           | 0.92      | 0.17        | 0.19   |
| 72       | 0.25          | 0.28     | 0.95           | 0.93      | 0.16        | 0.19   |
| 73       | 0.24          | 0.27     | 0.96           | 0.93      | 0.16        | 0.18   |
| 74       | 0.23          | 0.27     | 0.96           | 0.93      | 0.15        | 0.18   |
| 75       | 0.23          | 0.26     | 0.96           | 0.93      | 0.15        | 0.17   |
| 76       | 0.22          | 0.25     | 0.96           | 0.94      | 0.14        | 0.17   |
| 77       | 0.21          | 0.24     | 0.96           | 0.94      | 0.14        | 0.16   |
| 78       | 0.20          | 0.23     | 0.97           | 0.94      | 0.13        | 0.15   |
| 79       | 0.19          | 0.22     | 0.97           | 0.94      | 0.12        | 0.15   |
| 80       | 0.19          | 0.21     | 0.97           | 0.95      | 0.12        | 0.14   |
| 81       | 0.18          | 0.21     | 0.97           | 0.95      | 0.12        | 0.14   |
| 82       | 0.17          | 0.20     | 0.97           | 0.95      | 0.11        | 0.13   |
| 83       | 0.17          | 0.19     | 0.97           | 0.95      | 0.11        | 0.13   |
| 84       | 0.16          | 0.18     | 0.97           | 0.95      | 0.10        | 0.12   |
| 85       | 0.15          | 0.18     | 0.97           | 0.95      | 0.10        | 0.12   |
| 86       | 0.14          | 0.17     | 0.97           | 0.95      | 0.09        | 0.11   |
| 87       | 0.14          | 0.17     | 0.97           | 0.95      | 0.09        | 0.11   |
| 88       | 0.13          | 0.16     | 0.98           | 0.95      | 0.08        | 0.11   |
| 89       | 0.13          | 0.16     | 0.98           | 0.95      | 0.08        | 0.11   |
| 90       | 0.12          | 0.16     | 0.98           | 0.95      | 0.08        | 0.11   |

Table S94: Reference ( $\phi_S$ ,  $\varphi$ ,  $\psi$ ) and approached ( $\phi_S^\ell$ ,  $\varphi^\ell$ ,  $\psi^\ell$ ) values of the topological descriptors for the first excited-state of the pyridinium-phenolate (PP), computed at the CIS/6-31+G level of theory.  $\alpha$  is the pyridinium-phenolate central twist angle amplitude.

| $\alpha$ | $\phi_S^\ell$ | $\phi_S$ | $\varphi^\ell$ | $\varphi$ | $\psi^\ell$ | $\psi$ |
|----------|---------------|----------|----------------|-----------|-------------|--------|
| 0        | 0.61          | 0.66     | 0.71           | 0.68      | 0.45        | 0.49   |
| 1        | 0.61          | 0.66     | 0.71           | 0.68      | 0.45        | 0.49   |
| 2        | 0.61          | 0.66     | 0.71           | 0.68      | 0.45        | 0.49   |
| 3        | 0.61          | 0.66     | 0.71           | 0.68      | 0.45        | 0.49   |
| 4        | 0.61          | 0.66     | 0.72           | 0.68      | 0.45        | 0.49   |
| 5        | 0.61          | 0.66     | 0.72           | 0.68      | 0.45        | 0.49   |
| 6        | 0.61          | 0.66     | 0.72           | 0.68      | 0.45        | 0.49   |
| 7        | 0.61          | 0.66     | 0.72           | 0.68      | 0.45        | 0.49   |
| 8        | 0.61          | 0.65     | 0.72           | 0.69      | 0.45        | 0.48   |
| 9        | 0.61          | 0.65     | 0.72           | 0.69      | 0.45        | 0.48   |
| 10       | 0.61          | 0.65     | 0.72           | 0.69      | 0.45        | 0.48   |
| 11       | 0.61          | 0.65     | 0.72           | 0.69      | 0.45        | 0.48   |
| 12       | 0.60          | 0.65     | 0.72           | 0.69      | 0.44        | 0.48   |
| 13       | 0.60          | 0.65     | 0.72           | 0.69      | 0.44        | 0.48   |
| 14       | 0.60          | 0.65     | 0.73           | 0.69      | 0.44        | 0.48   |
| 15       | 0.60          | 0.64     | 0.73           | 0.70      | 0.44        | 0.47   |
| 16       | 0.60          | 0.64     | 0.73           | 0.70      | 0.44        | 0.47   |
| 17       | 0.60          | 0.64     | 0.73           | 0.70      | 0.44        | 0.47   |
| 18       | 0.59          | 0.64     | 0.73           | 0.70      | 0.43        | 0.47   |
| 19       | 0.59          | 0.63     | 0.74           | 0.71      | 0.43        | 0.46   |
| 20       | 0.59          | 0.63     | 0.74           | 0.71      | 0.43        | 0.46   |
| 21       | 0.59          | 0.63     | 0.74           | 0.71      | 0.43        | 0.46   |
| 22       | 0.59          | 0.63     | 0.75           | 0.71      | 0.42        | 0.46   |
| 23       | 0.58          | 0.62     | 0.75           | 0.72      | 0.42        | 0.45   |
| 24       | 0.58          | 0.62     | 0.75           | 0.72      | 0.42        | 0.45   |
| 25       | 0.58          | 0.62     | 0.75           | 0.72      | 0.42        | 0.45   |
| 26       | 0.57          | 0.61     | 0.76           | 0.73      | 0.41        | 0.44   |
| 27       | 0.57          | 0.61     | 0.76           | 0.73      | 0.41        | 0.44   |
| 28       | 0.57          | 0.61     | 0.76           | 0.73      | 0.41        | 0.44   |
| 29       | 0.57          | 0.60     | 0.77           | 0.74      | 0.41        | 0.43   |
| 30       | 0.56          | 0.60     | 0.77           | 0.74      | 0.40        | 0.43   |
| 31       | 0.56          | 0.59     | 0.78           | 0.75      | 0.40        | 0.42   |

Continued on next page

| $\alpha$ | $\phi_S^\ell$ | $\phi_S$ | $\varphi^\ell$ | $\varphi$ | $\psi^\ell$ | $\psi$ |
|----------|---------------|----------|----------------|-----------|-------------|--------|
| 32       | 0.55          | 0.59     | 0.78           | 0.75      | 0.39        | 0.42   |
| 33       | 0.55          | 0.59     | 0.78           | 0.75      | 0.39        | 0.42   |
| 34       | 0.55          | 0.58     | 0.79           | 0.76      | 0.39        | 0.41   |
| 35       | 0.54          | 0.58     | 0.79           | 0.76      | 0.38        | 0.41   |
| 36       | 0.54          | 0.57     | 0.80           | 0.77      | 0.38        | 0.41   |
| 37       | 0.53          | 0.57     | 0.80           | 0.77      | 0.37        | 0.41   |
| 38       | 0.53          | 0.56     | 0.80           | 0.78      | 0.37        | 0.40   |
| 39       | 0.52          | 0.55     | 0.81           | 0.78      | 0.36        | 0.39   |
| 40       | 0.52          | 0.55     | 0.81           | 0.79      | 0.36        | 0.39   |
| 41       | 0.51          | 0.54     | 0.82           | 0.79      | 0.35        | 0.38   |
| 42       | 0.51          | 0.54     | 0.82           | 0.79      | 0.35        | 0.38   |
| 43       | 0.50          | 0.53     | 0.83           | 0.80      | 0.35        | 0.37   |
| 44       | 0.49          | 0.53     | 0.83           | 0.80      | 0.34        | 0.37   |
| 45       | 0.49          | 0.52     | 0.84           | 0.81      | 0.34        | 0.36   |
| 46       | 0.48          | 0.51     | 0.84           | 0.81      | 0.33        | 0.36   |
| 47       | 0.47          | 0.51     | 0.85           | 0.82      | 0.32        | 0.35   |
| 48       | 0.47          | 0.50     | 0.85           | 0.82      | 0.32        | 0.35   |
| 49       | 0.46          | 0.49     | 0.86           | 0.83      | 0.31        | 0.34   |
| 50       | 0.45          | 0.48     | 0.86           | 0.83      | 0.31        | 0.33   |
| 51       | 0.45          | 0.48     | 0.86           | 0.84      | 0.31        | 0.33   |
| 52       | 0.44          | 0.47     | 0.87           | 0.84      | 0.30        | 0.32   |
| 53       | 0.43          | 0.46     | 0.87           | 0.85      | 0.29        | 0.32   |
| 54       | 0.42          | 0.45     | 0.88           | 0.85      | 0.28        | 0.31   |
| 55       | 0.42          | 0.45     | 0.88           | 0.86      | 0.28        | 0.31   |
| 56       | 0.41          | 0.44     | 0.89           | 0.86      | 0.27        | 0.30   |
| 57       | 0.40          | 0.43     | 0.89           | 0.87      | 0.27        | 0.29   |
| 58       | 0.39          | 0.42     | 0.90           | 0.87      | 0.26        | 0.29   |
| 59       | 0.38          | 0.41     | 0.90           | 0.88      | 0.25        | 0.28   |
| 60       | 0.37          | 0.40     | 0.91           | 0.88      | 0.25        | 0.27   |
| 61       | 0.36          | 0.39     | 0.91           | 0.88      | 0.24        | 0.27   |
| 62       | 0.35          | 0.39     | 0.92           | 0.89      | 0.23        | 0.26   |
| 63       | 0.35          | 0.38     | 0.92           | 0.89      | 0.23        | 0.26   |

Continued on next page

| $\alpha$ | $\phi_S^\ell$ | $\phi_S$ | $\varphi^\ell$ | $\varphi$ | $\psi^\ell$ | $\psi$ |
|----------|---------------|----------|----------------|-----------|-------------|--------|
| 64       | 0.34          | 0.37     | 0.93           | 0.90      | 0.22        | 0.25   |
| 65       | 0.33          | 0.36     | 0.93           | 0.90      | 0.22        | 0.24   |
| 66       | 0.32          | 0.35     | 0.93           | 0.90      | 0.21        | 0.24   |
| 67       | 0.31          | 0.34     | 0.94           | 0.91      | 0.20        | 0.23   |
| 68       | 0.30          | 0.33     | 0.94           | 0.91      | 0.20        | 0.22   |
| 69       | 0.29          | 0.32     | 0.95           | 0.92      | 0.19        | 0.21   |
| 70       | 0.27          | 0.31     | 0.95           | 0.92      | 0.18        | 0.21   |
| 71       | 0.26          | 0.30     | 0.95           | 0.92      | 0.17        | 0.20   |
| 72       | 0.25          | 0.29     | 0.96           | 0.93      | 0.16        | 0.19   |
| 73       | 0.24          | 0.28     | 0.96           | 0.93      | 0.16        | 0.19   |
| 74       | 0.23          | 0.27     | 0.96           | 0.93      | 0.15        | 0.18   |
| 75       | 0.22          | 0.26     | 0.97           | 0.93      | 0.14        | 0.17   |
| 76       | 0.21          | 0.25     | 0.97           | 0.94      | 0.14        | 0.17   |
| 77       | 0.20          | 0.24     | 0.97           | 0.94      | 0.13        | 0.16   |
| 78       | 0.19          | 0.24     | 0.97           | 0.94      | 0.12        | 0.16   |
| 79       | 0.18          | 0.23     | 0.97           | 0.94      | 0.12        | 0.15   |
| 80       | 0.18          | 0.22     | 0.98           | 0.95      | 0.12        | 0.14   |
| 81       | 0.17          | 0.21     | 0.98           | 0.95      | 0.11        | 0.14   |
| 82       | 0.16          | 0.20     | 0.98           | 0.95      | 0.10        | 0.13   |
| 83       | 0.15          | 0.19     | 0.98           | 0.95      | 0.10        | 0.13   |
| 84       | 0.14          | 0.18     | 0.98           | 0.95      | 0.09        | 0.12   |
| 85       | 0.13          | 0.18     | 0.98           | 0.95      | 0.08        | 0.12   |
| 86       | 0.13          | 0.17     | 0.98           | 0.95      | 0.08        | 0.11   |
| 87       | 0.12          | 0.17     | 0.98           | 0.95      | 0.08        | 0.11   |
| 88       | 0.11          | 0.16     | 0.98           | 0.96      | 0.07        | 0.11   |
| 89       | 0.10          | 0.16     | 0.98           | 0.96      | 0.06        | 0.11   |
| 90       | 0.10          | 0.15     | 0.98           | 0.96      | 0.06        | 0.10   |

Table S95: Reference ( $\phi_S$ ,  $\varphi$ ,  $\psi$ ) and approached ( $\phi_S^\ell$ ,  $\varphi^\ell$ ,  $\psi^\ell$ ) values of the topological descriptors for the first excited-state of the pyridinium-phenolate (PP), computed at the CIS/6-31G level of theory.  $\alpha$  is the pyridinium-phenolate central twist angle amplitude.

| $\alpha$ | $\phi_S^\ell$ | $\phi_S$ | $\varphi^\ell$ | $\varphi$ | $\psi^\ell$ | $\psi$ |
|----------|---------------|----------|----------------|-----------|-------------|--------|
| 0        | 0.66          | 0.70     | 0.67           | 0.63      | 0.50        | 0.53   |
| 1        | 0.66          | 0.70     | 0.67           | 0.63      | 0.50        | 0.53   |
| 2        | 0.66          | 0.70     | 0.67           | 0.63      | 0.50        | 0.53   |
| 3        | 0.66          | 0.70     | 0.67           | 0.63      | 0.50        | 0.53   |
| 4        | 0.66          | 0.70     | 0.67           | 0.63      | 0.50        | 0.53   |
| 5        | 0.66          | 0.70     | 0.67           | 0.63      | 0.50        | 0.53   |
| 6        | 0.66          | 0.70     | 0.67           | 0.63      | 0.50        | 0.53   |
| 7        | 0.66          | 0.70     | 0.67           | 0.63      | 0.50        | 0.53   |
| 8        | 0.66          | 0.70     | 0.67           | 0.64      | 0.50        | 0.53   |
| 9        | 0.66          | 0.70     | 0.67           | 0.64      | 0.50        | 0.53   |
| 10       | 0.65          | 0.70     | 0.67           | 0.64      | 0.49        | 0.53   |
| 11       | 0.65          | 0.70     | 0.68           | 0.64      | 0.49        | 0.53   |
| 12       | 0.65          | 0.70     | 0.68           | 0.64      | 0.49        | 0.53   |
| 13       | 0.65          | 0.69     | 0.68           | 0.64      | 0.49        | 0.52   |
| 14       | 0.65          | 0.69     | 0.68           | 0.64      | 0.49        | 0.52   |
| 15       | 0.65          | 0.69     | 0.68           | 0.65      | 0.49        | 0.52   |
| 16       | 0.65          | 0.69     | 0.68           | 0.65      | 0.49        | 0.52   |
| 17       | 0.65          | 0.69     | 0.69           | 0.65      | 0.48        | 0.52   |
| 18       | 0.65          | 0.69     | 0.69           | 0.65      | 0.48        | 0.52   |
| 19       | 0.64          | 0.69     | 0.69           | 0.66      | 0.48        | 0.51   |
| 20       | 0.64          | 0.68     | 0.69           | 0.66      | 0.48        | 0.51   |
| 21       | 0.64          | 0.68     | 0.69           | 0.66      | 0.48        | 0.51   |
| 22       | 0.64          | 0.68     | 0.70           | 0.66      | 0.47        | 0.51   |
| 23       | 0.64          | 0.68     | 0.70           | 0.67      | 0.47        | 0.50   |
| 24       | 0.64          | 0.67     | 0.70           | 0.67      | 0.47        | 0.50   |
| 25       | 0.63          | 0.67     | 0.71           | 0.67      | 0.46        | 0.50   |
| 26       | 0.63          | 0.67     | 0.71           | 0.68      | 0.46        | 0.50   |
| 27       | 0.63          | 0.67     | 0.71           | 0.68      | 0.46        | 0.50   |
| 28       | 0.63          | 0.66     | 0.71           | 0.68      | 0.46        | 0.49   |
| 29       | 0.63          | 0.66     | 0.72           | 0.69      | 0.46        | 0.49   |
| 30       | 0.62          | 0.66     | 0.72           | 0.69      | 0.45        | 0.49   |
| 31       | 0.62          | 0.66     | 0.72           | 0.69      | 0.45        | 0.49   |

Continued on next page

| $\alpha$ | $\phi_S^\ell$ | $\phi_S$ | $\varphi^\ell$ | $\varphi$ | $\psi^\ell$ | $\psi$ |
|----------|---------------|----------|----------------|-----------|-------------|--------|
| 32       | 0.62          | 0.65     | 0.73           | 0.70      | 0.45        | 0.48   |
| 33       | 0.62          | 0.65     | 0.73           | 0.70      | 0.45        | 0.48   |
| 34       | 0.61          | 0.65     | 0.74           | 0.71      | 0.44        | 0.47   |
| 35       | 0.61          | 0.64     | 0.74           | 0.71      | 0.44        | 0.47   |
| 36       | 0.61          | 0.64     | 0.74           | 0.71      | 0.44        | 0.47   |
| 37       | 0.61          | 0.63     | 0.75           | 0.72      | 0.43        | 0.46   |
| 38       | 0.60          | 0.63     | 0.75           | 0.72      | 0.43        | 0.46   |
| 39       | 0.60          | 0.63     | 0.76           | 0.73      | 0.43        | 0.45   |
| 40       | 0.59          | 0.62     | 0.76           | 0.73      | 0.42        | 0.45   |
| 41       | 0.59          | 0.62     | 0.76           | 0.74      | 0.42        | 0.44   |
| 42       | 0.59          | 0.61     | 0.77           | 0.74      | 0.42        | 0.44   |
| 43       | 0.58          | 0.61     | 0.77           | 0.75      | 0.41        | 0.43   |
| 44       | 0.58          | 0.60     | 0.78           | 0.75      | 0.41        | 0.43   |
| 45       | 0.57          | 0.60     | 0.78           | 0.75      | 0.40        | 0.43   |
| 46       | 0.57          | 0.59     | 0.79           | 0.76      | 0.40        | 0.42   |
| 47       | 0.56          | 0.59     | 0.79           | 0.76      | 0.39        | 0.42   |
| 48       | 0.56          | 0.58     | 0.80           | 0.77      | 0.39        | 0.41   |
| 49       | 0.55          | 0.58     | 0.80           | 0.77      | 0.38        | 0.41   |
| 50       | 0.54          | 0.57     | 0.81           | 0.78      | 0.37        | 0.40   |
| 51       | 0.54          | 0.56     | 0.81           | 0.78      | 0.37        | 0.40   |
| 52       | 0.53          | 0.56     | 0.82           | 0.79      | 0.37        | 0.39   |
| 53       | 0.53          | 0.55     | 0.82           | 0.80      | 0.37        | 0.38   |
| 54       | 0.52          | 0.54     | 0.83           | 0.80      | 0.36        | 0.38   |
| 55       | 0.51          | 0.54     | 0.83           | 0.81      | 0.35        | 0.37   |
| 56       | 0.50          | 0.53     | 0.84           | 0.81      | 0.34        | 0.37   |
| 57       | 0.50          | 0.52     | 0.84           | 0.82      | 0.34        | 0.36   |
| 58       | 0.49          | 0.51     | 0.85           | 0.82      | 0.33        | 0.35   |
| 59       | 0.48          | 0.51     | 0.85           | 0.83      | 0.33        | 0.35   |
| 60       | 0.47          | 0.50     | 0.86           | 0.83      | 0.32        | 0.35   |
| 61       | 0.46          | 0.49     | 0.87           | 0.84      | 0.31        | 0.34   |
| 62       | 0.45          | 0.48     | 0.87           | 0.84      | 0.30        | 0.33   |
| 63       | 0.44          | 0.47     | 0.88           | 0.85      | 0.30        | 0.32   |

Continued on next page



| $\alpha$ | $\phi_S^\ell$ | $\phi_S$ | $\varphi^\ell$ | $\varphi$ | $\psi^\ell$ | $\psi$ |
|----------|---------------|----------|----------------|-----------|-------------|--------|
| 64       | 0.43          | 0.46     | 0.88           | 0.85      | 0.29        | 0.32   |
| 65       | 0.42          | 0.45     | 0.89           | 0.86      | 0.28        | 0.31   |
| 66       | 0.41          | 0.44     | 0.89           | 0.87      | 0.27        | 0.30   |
| 67       | 0.40          | 0.43     | 0.90           | 0.87      | 0.27        | 0.29   |
| 68       | 0.39          | 0.42     | 0.91           | 0.88      | 0.26        | 0.28   |
| 69       | 0.38          | 0.41     | 0.91           | 0.88      | 0.25        | 0.28   |
| 70       | 0.37          | 0.40     | 0.92           | 0.89      | 0.24        | 0.27   |
| 71       | 0.35          | 0.39     | 0.92           | 0.89      | 0.23        | 0.26   |
| 72       | 0.34          | 0.38     | 0.93           | 0.90      | 0.22        | 0.25   |
| 73       | 0.33          | 0.36     | 0.93           | 0.90      | 0.22        | 0.24   |
| 74       | 0.31          | 0.35     | 0.94           | 0.91      | 0.20        | 0.23   |
| 75       | 0.30          | 0.34     | 0.94           | 0.91      | 0.20        | 0.23   |
| 76       | 0.28          | 0.33     | 0.95           | 0.92      | 0.18        | 0.22   |
| 77       | 0.27          | 0.31     | 0.95           | 0.92      | 0.18        | 0.21   |
| 78       | 0.25          | 0.30     | 0.96           | 0.93      | 0.16        | 0.20   |
| 79       | 0.24          | 0.28     | 0.96           | 0.93      | 0.16        | 0.19   |
| 80       | 0.22          | 0.27     | 0.97           | 0.93      | 0.14        | 0.18   |
| 81       | 0.21          | 0.26     | 0.97           | 0.94      | 0.14        | 0.17   |
| 82       | 0.19          | 0.24     | 0.97           | 0.94      | 0.12        | 0.16   |
| 83       | 0.18          | 0.23     | 0.98           | 0.95      | 0.12        | 0.15   |
| 84       | 0.16          | 0.22     | 0.98           | 0.95      | 0.10        | 0.14   |
| 85       | 0.15          | 0.20     | 0.98           | 0.95      | 0.10        | 0.13   |
| 86       | 0.14          | 0.19     | 0.98           | 0.95      | 0.09        | 0.13   |
| 87       | 0.12          | 0.18     | 0.99           | 0.95      | 0.08        | 0.12   |
| 88       | 0.11          | 0.17     | 0.99           | 0.96      | 0.07        | 0.11   |
| 89       | 0.11          | 0.17     | 0.99           | 0.96      | 0.07        | 0.11   |
| 90       | 0.10          | 0.17     | 0.99           | 0.96      | 0.06        | 0.11   |

Table S96: Reference ( $\phi_S$ ,  $\varphi$ ,  $\psi$ ) and approached ( $\phi_S^\ell$ ,  $\varphi^\ell$ ,  $\psi^\ell$ ) values of the topological descriptors for the first excited-state of the pyridinium-phenolate (PP), computed at the LC-wHPBE/3-21G level of theory.  $\alpha$  is the pyridinium-phenolate central twist angle amplitude.

| $\alpha$ | $\phi_S^\ell$ | $\phi_S$ | $\varphi^\ell$ | $\varphi$ | $\psi^\ell$ | $\psi$ |
|----------|---------------|----------|----------------|-----------|-------------|--------|
| 0        | 0.63          | 0.68     | 0.69           | 0.65      | 0.47        | 0.51   |
| 0        | 0.65          | 0.63     | 0.68           | 1.00      | 0.49        | 0.36   |
| 1        | 0.65          | 0.63     | 0.68           | 2.00      | 0.49        | 0.19   |
| 2        | 0.65          | 0.63     | 0.68           | 3.00      | 0.49        | 0.13   |
| 3        | 0.65          | 0.63     | 0.68           | 4.00      | 0.49        | 0.10   |
| 4        | 0.65          | 0.63     | 0.68           | 5.00      | 0.49        | 0.08   |
| 5        | 0.65          | 0.62     | 0.68           | 6.00      | 0.49        | 0.07   |
| 6        | 0.65          | 0.62     | 0.68           | 7.00      | 0.49        | 0.06   |
| 7        | 0.66          | 0.62     | 0.68           | 8.00      | 0.49        | 0.05   |
| 8        | 0.66          | 0.62     | 0.67           | 9.00      | 0.49        | 0.04   |
| 9        | 0.66          | 0.62     | 0.67           | 10.00     | 0.49        | 0.04   |
| 10       | 0.66          | 0.62     | 0.67           | 11.00     | 0.49        | 0.04   |
| 11       | 0.66          | 0.62     | 0.67           | 12.00     | 0.49        | 0.03   |
| 12       | 0.66          | 0.62     | 0.67           | 13.00     | 0.50        | 0.03   |
| 13       | 0.66          | 0.62     | 0.67           | 14.00     | 0.50        | 0.03   |
| 14       | 0.67          | 0.62     | 0.67           | 15.00     | 0.50        | 0.03   |
| 15       | 0.67          | 0.62     | 0.67           | 16.00     | 0.50        | 0.02   |
| 16       | 0.67          | 0.61     | 0.66           | 17.00     | 0.50        | 0.02   |
| 17       | 0.67          | 0.61     | 0.66           | 18.00     | 0.50        | 0.02   |
| 18       | 0.67          | 0.61     | 0.66           | 19.00     | 0.51        | 0.02   |
| 19       | 0.68          | 0.61     | 0.66           | 20.00     | 0.51        | 0.02   |
| 20       | 0.68          | 0.61     | 0.66           | 21.00     | 0.51        | 0.02   |
| 21       | 0.68          | 0.61     | 0.65           | 22.00     | 0.51        | 0.02   |
| 22       | 0.68          | 0.60     | 0.65           | 23.00     | 0.52        | 0.02   |
| 23       | 0.69          | 0.60     | 0.65           | 24.00     | 0.52        | 0.02   |
| 24       | 0.69          | 0.60     | 0.65           | 25.00     | 0.52        | 0.02   |
| 25       | 0.69          | 0.60     | 0.64           | 26.00     | 0.52        | 0.01   |
| 26       | 0.70          | 0.59     | 0.64           | 27.00     | 0.53        | 0.01   |
| 27       | 0.70          | 0.59     | 0.64           | 28.00     | 0.53        | 0.01   |
| 28       | 0.70          | 0.59     | 0.64           | 29.00     | 0.53        | 0.01   |
| 29       | 0.71          | 0.59     | 0.63           | 30.00     | 0.54        | 0.01   |
| 30       | 0.71          | 0.58     | 0.63           | 31.00     | 0.54        | 0.01   |

Continued on next page

| $\alpha$ | $\phi_S^\ell$ | $\phi_S$ | $\varphi^\ell$ | $\varphi$ | $\psi^\ell$ | $\psi$ |
|----------|---------------|----------|----------------|-----------|-------------|--------|
| 31       | 0.71          | 0.58     | 0.63           | 32.00     | 0.54        | 0.01   |
| 32       | 0.72          | 0.58     | 0.62           | 33.00     | 0.55        | 0.01   |
| 33       | 0.72          | 0.57     | 0.62           | 34.00     | 0.55        | 0.01   |
| 34       | 0.73          | 0.57     | 0.61           | 35.00     | 0.55        | 0.01   |
| 35       | 0.73          | 0.57     | 0.61           | 36.00     | 0.56        | 0.01   |
| 36       | 0.73          | 0.56     | 0.61           | 37.00     | 0.56        | 0.01   |
| 37       | 0.74          | 0.56     | 0.60           | 38.00     | 0.56        | 0.01   |
| 38       | 0.74          | 0.56     | 0.60           | 39.00     | 0.57        | 0.01   |
| 39       | 0.75          | 0.55     | 0.59           | 40.00     | 0.57        | 0.01   |
| 40       | 0.75          | 0.55     | 0.59           | 41.00     | 0.58        | 0.01   |
| 41       | 0.76          | 0.54     | 0.58           | 42.00     | 0.58        | 0.01   |
| 42       | 0.76          | 0.54     | 0.58           | 43.00     | 0.59        | 0.01   |
| 43       | 0.77          | 0.53     | 0.57           | 44.00     | 0.59        | 0.01   |
| 44       | 0.77          | 0.53     | 0.57           | 45.00     | 0.60        | 0.01   |
| 45       | 0.78          | 0.52     | 0.56           | 46.00     | 0.60        | 0.01   |
| 46       | 0.78          | 0.52     | 0.56           | 47.00     | 0.61        | 0.01   |
| 47       | 0.78          | 0.51     | 0.55           | 48.00     | 0.61        | 0.01   |
| 48       | 0.79          | 0.51     | 0.54           | 49.00     | 0.62        | 0.01   |
| 49       | 0.79          | 0.50     | 0.54           | 50.00     | 0.62        | 0.01   |
| 50       | 0.80          | 0.49     | 0.53           | 51.00     | 0.63        | 0.01   |
| 51       | 0.80          | 0.49     | 0.52           | 52.00     | 0.63        | 0.01   |
| 52       | 0.81          | 0.48     | 0.52           | 53.00     | 0.64        | 0.01   |
| 53       | 0.81          | 0.48     | 0.51           | 54.00     | 0.64        | 0.01   |
| 54       | 0.82          | 0.47     | 0.50           | 55.00     | 0.65        | 0.01   |
| 55       | 0.83          | 0.46     | 0.50           | 56.00     | 0.66        | 0.01   |
| 56       | 0.83          | 0.45     | 0.49           | 57.00     | 0.66        | 0.01   |
| 57       | 0.84          | 0.45     | 0.48           | 58.00     | 0.67        | 0.00   |
| 58       | 0.84          | 0.44     | 0.47           | 59.00     | 0.67        | 0.00   |
| 59       | 0.85          | 0.43     | 0.46           | 60.00     | 0.68        | 0.00   |
| 60       | 0.85          | 0.42     | 0.46           | 61.00     | 0.69        | 0.00   |
| 61       | 0.86          | 0.41     | 0.45           | 62.00     | 0.69        | 0.00   |
| 62       | 0.86          | 0.41     | 0.44           | 63.00     | 0.70        | 0.00   |

Continued on next page

| $\alpha$ | $\phi_S^\ell$ | $\phi_S$ | $\varphi^\ell$ | $\varphi$ | $\psi^\ell$ | $\psi$ |
|----------|---------------|----------|----------------|-----------|-------------|--------|
| 63       | 0.87          | 0.40     | 0.43           | 64.00     | 0.71        | 0.00   |
| 64       | 0.87          | 0.39     | 0.42           | 65.00     | 0.71        | 0.00   |
| 65       | 0.88          | 0.38     | 0.41           | 66.00     | 0.72        | 0.00   |
| 66       | 0.88          | 0.37     | 0.40           | 67.00     | 0.73        | 0.00   |
| 67       | 0.88          | 0.36     | 0.39           | 68.00     | 0.73        | 0.00   |
| 68       | 0.89          | 0.35     | 0.38           | 69.00     | 0.74        | 0.00   |
| 69       | 0.89          | 0.34     | 0.37           | 70.00     | 0.75        | 0.00   |
| 70       | 0.90          | 0.33     | 0.36           | 71.00     | 0.76        | 0.00   |
| 71       | 0.90          | 0.32     | 0.35           | 72.00     | 0.76        | 0.00   |
| 72       | 0.91          | 0.31     | 0.34           | 73.00     | 0.77        | 0.00   |
| 73       | 0.91          | 0.29     | 0.33           | 74.00     | 0.78        | 0.00   |
| 74       | 0.91          | 0.28     | 0.32           | 75.00     | 0.79        | 0.00   |
| 75       | 0.92          | 0.27     | 0.31           | 76.00     | 0.79        | 0.00   |
| 76       | 0.92          | 0.26     | 0.30           | 77.00     | 0.80        | 0.00   |
| 77       | 0.93          | 0.25     | 0.29           | 78.00     | 0.81        | 0.00   |
| 78       | 0.93          | 0.24     | 0.28           | 79.00     | 0.82        | 0.00   |
| 79       | 0.93          | 0.23     | 0.26           | 80.00     | 0.82        | 0.00   |
| 80       | 0.93          | 0.22     | 0.25           | 81.00     | 0.83        | 0.00   |
| 81       | 0.94          | 0.20     | 0.24           | 82.00     | 0.84        | 0.00   |
| 82       | 0.94          | 0.19     | 0.23           | 83.00     | 0.84        | 0.00   |
| 83       | 0.94          | 0.19     | 0.22           | 84.00     | 0.85        | 0.00   |
| 84       | 0.94          | 0.18     | 0.21           | 85.00     | 0.86        | 0.00   |
| 85       | 0.94          | 0.17     | 0.21           | 86.00     | 0.86        | 0.00   |
| 86       | 0.95          | 0.16     | 0.20           | 87.00     | 0.87        | 0.00   |
| 87       | 0.95          | 0.16     | 0.19           | 88.00     | 0.87        | 0.00   |
| 88       | 0.95          | 0.15     | 0.18           | 89.00     | 0.88        | 0.00   |
| 89       | 0.95          | 0.15     | 0.18           | 90.00     | 0.88        | 0.00   |

Table S97: Reference ( $\phi_S$ ,  $\varphi$ ,  $\psi$ ) and approached ( $\phi_S^\ell$ ,  $\varphi^\ell$ ,  $\psi^\ell$ ) values of the topological descriptors for the first excited-state of the pyridinium-phenolate (PP), computed at the LC-wHPBE/6-311++G(2d,p) level of theory.  $\alpha$  is the pyridinium-phenolate central twist angle amplitude.

| $\alpha$ | $\phi_S^\ell$ | $\phi_S$ | $\varphi^\ell$ | $\varphi$ | $\psi^\ell$ | $\psi$ |
|----------|---------------|----------|----------------|-----------|-------------|--------|
| 0        | 0.62          | 0.68     | 0.69           | 0.65      | 0.47        | 0.51   |
| 1        | 0.62          | 0.68     | 0.69           | 0.65      | 0.47        | 0.51   |
| 2        | 0.62          | 0.68     | 0.69           | 0.65      | 0.47        | 0.51   |
| 3        | 0.62          | 0.68     | 0.69           | 0.65      | 0.47        | 0.51   |
| 4        | 0.62          | 0.68     | 0.69           | 0.65      | 0.47        | 0.51   |
| 5        | 0.62          | 0.68     | 0.69           | 0.65      | 0.47        | 0.51   |
| 6        | 0.62          | 0.68     | 0.69           | 0.65      | 0.47        | 0.51   |
| 7        | 0.62          | 0.68     | 0.69           | 0.66      | 0.47        | 0.51   |
| 8        | 0.62          | 0.68     | 0.69           | 0.66      | 0.47        | 0.51   |
| 9        | 0.62          | 0.67     | 0.69           | 0.66      | 0.47        | 0.50   |
| 10       | 0.62          | 0.67     | 0.69           | 0.66      | 0.47        | 0.50   |
| 11       | 0.61          | 0.67     | 0.70           | 0.66      | 0.46        | 0.50   |
| 12       | 0.61          | 0.67     | 0.70           | 0.66      | 0.46        | 0.50   |
| 13       | 0.61          | 0.67     | 0.70           | 0.66      | 0.46        | 0.50   |
| 14       | 0.61          | 0.67     | 0.70           | 0.67      | 0.46        | 0.50   |
| 15       | 0.61          | 0.67     | 0.70           | 0.67      | 0.46        | 0.50   |
| 16       | 0.61          | 0.66     | 0.70           | 0.67      | 0.46        | 0.50   |
| 17       | 0.61          | 0.66     | 0.71           | 0.67      | 0.45        | 0.50   |
| 18       | 0.61          | 0.66     | 0.71           | 0.67      | 0.45        | 0.50   |
| 19       | 0.61          | 0.66     | 0.71           | 0.68      | 0.45        | 0.49   |
| 20       | 0.60          | 0.66     | 0.71           | 0.68      | 0.45        | 0.49   |
| 21       | 0.60          | 0.65     | 0.72           | 0.68      | 0.44        | 0.49   |
| 22       | 0.60          | 0.65     | 0.72           | 0.69      | 0.44        | 0.48   |
| 23       | 0.60          | 0.65     | 0.72           | 0.69      | 0.44        | 0.48   |
| 24       | 0.60          | 0.65     | 0.72           | 0.69      | 0.44        | 0.48   |
| 25       | 0.60          | 0.64     | 0.73           | 0.69      | 0.44        | 0.48   |
| 26       | 0.59          | 0.64     | 0.73           | 0.70      | 0.43        | 0.47   |
| 27       | 0.59          | 0.64     | 0.73           | 0.70      | 0.43        | 0.47   |
| 28       | 0.59          | 0.64     | 0.74           | 0.70      | 0.43        | 0.47   |
| 29       | 0.59          | 0.63     | 0.74           | 0.71      | 0.43        | 0.46   |
| 30       | 0.58          | 0.63     | 0.74           | 0.71      | 0.42        | 0.46   |
| 31       | 0.58          | 0.63     | 0.75           | 0.72      | 0.42        | 0.46   |

Continued on next page

| $\alpha$ | $\phi_S^\ell$ | $\phi_S$ | $\varphi^\ell$ | $\varphi$ | $\psi^\ell$ | $\psi$ |
|----------|---------------|----------|----------------|-----------|-------------|--------|
| 32       | 0.58          | 0.62     | 0.75           | 0.72      | 0.42        | 0.45   |
| 33       | 0.58          | 0.62     | 0.75           | 0.72      | 0.42        | 0.45   |
| 34       | 0.57          | 0.61     | 0.76           | 0.73      | 0.41        | 0.44   |
| 35       | 0.57          | 0.61     | 0.76           | 0.73      | 0.41        | 0.44   |
| 36       | 0.57          | 0.61     | 0.76           | 0.74      | 0.41        | 0.44   |
| 37       | 0.56          | 0.60     | 0.77           | 0.74      | 0.40        | 0.43   |
| 38       | 0.56          | 0.60     | 0.77           | 0.74      | 0.40        | 0.43   |
| 39       | 0.55          | 0.59     | 0.78           | 0.75      | 0.39        | 0.42   |
| 40       | 0.55          | 0.59     | 0.78           | 0.75      | 0.39        | 0.42   |
| 41       | 0.55          | 0.58     | 0.79           | 0.76      | 0.39        | 0.41   |
| 42       | 0.54          | 0.58     | 0.79           | 0.76      | 0.38        | 0.41   |
| 43       | 0.54          | 0.57     | 0.80           | 0.77      | 0.38        | 0.41   |
| 44       | 0.53          | 0.57     | 0.80           | 0.77      | 0.37        | 0.41   |
| 45       | 0.53          | 0.56     | 0.80           | 0.78      | 0.37        | 0.40   |
| 46       | 0.52          | 0.56     | 0.81           | 0.78      | 0.36        | 0.40   |
| 47       | 0.52          | 0.55     | 0.81           | 0.79      | 0.36        | 0.39   |
| 48       | 0.51          | 0.54     | 0.82           | 0.79      | 0.35        | 0.38   |
| 49       | 0.50          | 0.54     | 0.82           | 0.80      | 0.35        | 0.38   |
| 50       | 0.50          | 0.53     | 0.83           | 0.80      | 0.35        | 0.37   |
| 51       | 0.49          | 0.52     | 0.83           | 0.81      | 0.34        | 0.36   |
| 52       | 0.49          | 0.52     | 0.84           | 0.81      | 0.34        | 0.36   |
| 53       | 0.48          | 0.51     | 0.84           | 0.82      | 0.33        | 0.35   |
| 54       | 0.47          | 0.50     | 0.85           | 0.82      | 0.32        | 0.35   |
| 55       | 0.47          | 0.50     | 0.85           | 0.83      | 0.32        | 0.35   |
| 56       | 0.46          | 0.49     | 0.86           | 0.83      | 0.31        | 0.34   |
| 57       | 0.45          | 0.48     | 0.86           | 0.84      | 0.31        | 0.33   |
| 58       | 0.44          | 0.47     | 0.87           | 0.84      | 0.30        | 0.32   |
| 59       | 0.43          | 0.46     | 0.87           | 0.85      | 0.29        | 0.32   |
| 60       | 0.43          | 0.46     | 0.88           | 0.85      | 0.29        | 0.32   |
| 61       | 0.42          | 0.45     | 0.88           | 0.86      | 0.28        | 0.31   |
| 62       | 0.41          | 0.44     | 0.89           | 0.86      | 0.27        | 0.30   |
| 63       | 0.40          | 0.43     | 0.89           | 0.87      | 0.27        | 0.29   |

Continued on next page

| $\alpha$ | $\phi_S^\ell$ | $\phi_S$ | $\varphi^\ell$ | $\varphi$ | $\psi^\ell$ | $\psi$ |
|----------|---------------|----------|----------------|-----------|-------------|--------|
| 64       | 0.39          | 0.42     | 0.90           | 0.87      | 0.26        | 0.29   |
| 65       | 0.38          | 0.41     | 0.90           | 0.88      | 0.25        | 0.28   |
| 66       | 0.37          | 0.40     | 0.91           | 0.88      | 0.25        | 0.27   |
| 67       | 0.36          | 0.39     | 0.91           | 0.89      | 0.24        | 0.26   |
| 68       | 0.35          | 0.38     | 0.92           | 0.89      | 0.23        | 0.26   |
| 69       | 0.34          | 0.37     | 0.92           | 0.89      | 0.23        | 0.25   |
| 70       | 0.33          | 0.36     | 0.93           | 0.90      | 0.22        | 0.24   |
| 71       | 0.32          | 0.35     | 0.93           | 0.90      | 0.21        | 0.24   |
| 72       | 0.31          | 0.34     | 0.94           | 0.91      | 0.20        | 0.23   |
| 73       | 0.29          | 0.33     | 0.94           | 0.91      | 0.19        | 0.22   |
| 74       | 0.28          | 0.32     | 0.94           | 0.92      | 0.18        | 0.21   |
| 75       | 0.27          | 0.31     | 0.95           | 0.92      | 0.18        | 0.21   |
| 76       | 0.26          | 0.30     | 0.95           | 0.92      | 0.17        | 0.20   |
| 77       | 0.25          | 0.28     | 0.96           | 0.93      | 0.16        | 0.19   |
| 78       | 0.23          | 0.27     | 0.96           | 0.93      | 0.15        | 0.18   |
| 79       | 0.22          | 0.26     | 0.96           | 0.93      | 0.14        | 0.17   |
| 80       | 0.21          | 0.25     | 0.96           | 0.94      | 0.14        | 0.17   |
| 81       | 0.20          | 0.24     | 0.97           | 0.94      | 0.13        | 0.16   |
| 82       | 0.19          | 0.23     | 0.97           | 0.94      | 0.12        | 0.15   |
| 83       | 0.18          | 0.22     | 0.97           | 0.94      | 0.12        | 0.15   |
| 84       | 0.17          | 0.21     | 0.97           | 0.94      | 0.11        | 0.14   |
| 85       | 0.17          | 0.20     | 0.97           | 0.95      | 0.11        | 0.13   |
| 86       | 0.16          | 0.20     | 0.97           | 0.95      | 0.10        | 0.13   |
| 87       | 0.15          | 0.19     | 0.97           | 0.95      | 0.10        | 0.13   |
| 88       | 0.14          | 0.18     | 0.97           | 0.95      | 0.09        | 0.12   |
| 89       | 0.14          | 0.18     | 0.97           | 0.95      | 0.09        | 0.12   |
| 90       | 0.14          | 0.18     | 0.97           | 0.95      | 0.09        | 0.12   |

Table S98: Reference ( $\phi_S$ ,  $\varphi$ ,  $\psi$ ) and approached ( $\phi_S^\ell$ ,  $\varphi^\ell$ ,  $\psi^\ell$ ) values of the topological descriptors for the first excited-state of the pyridinium-phenolate (PP), computed at the LC-wHPBE/6-311++G(d,p) level of theory.  $\alpha$  is the pyridinium-phenolate central twist angle amplitude.

| $\alpha$ | $\phi_S^\ell$ | $\phi_S$ | $\varphi^\ell$ | $\varphi$ | $\psi^\ell$ | $\psi$ |
|----------|---------------|----------|----------------|-----------|-------------|--------|
| 0        | 0.62          | 0.68     | 0.69           | 0.65      | 0.47        | 0.51   |
| 1        | 0.62          | 0.68     | 0.69           | 0.65      | 0.47        | 0.51   |
| 2        | 0.62          | 0.68     | 0.69           | 0.65      | 0.47        | 0.51   |
| 3        | 0.62          | 0.68     | 0.69           | 0.65      | 0.47        | 0.51   |
| 4        | 0.62          | 0.68     | 0.69           | 0.65      | 0.47        | 0.51   |
| 5        | 0.62          | 0.68     | 0.69           | 0.65      | 0.47        | 0.51   |
| 6        | 0.62          | 0.68     | 0.69           | 0.65      | 0.47        | 0.51   |
| 7        | 0.62          | 0.68     | 0.69           | 0.66      | 0.47        | 0.51   |
| 8        | 0.62          | 0.68     | 0.69           | 0.66      | 0.47        | 0.51   |
| 9        | 0.62          | 0.67     | 0.69           | 0.66      | 0.47        | 0.50   |
| 10       | 0.62          | 0.67     | 0.69           | 0.66      | 0.47        | 0.50   |
| 11       | 0.61          | 0.67     | 0.70           | 0.66      | 0.46        | 0.50   |
| 12       | 0.61          | 0.67     | 0.70           | 0.66      | 0.46        | 0.50   |
| 13       | 0.61          | 0.67     | 0.70           | 0.66      | 0.46        | 0.50   |
| 14       | 0.61          | 0.67     | 0.70           | 0.67      | 0.46        | 0.50   |
| 15       | 0.61          | 0.67     | 0.70           | 0.67      | 0.46        | 0.50   |
| 16       | 0.61          | 0.66     | 0.70           | 0.67      | 0.46        | 0.50   |
| 17       | 0.61          | 0.66     | 0.71           | 0.67      | 0.45        | 0.50   |
| 18       | 0.61          | 0.66     | 0.71           | 0.67      | 0.45        | 0.50   |
| 19       | 0.61          | 0.66     | 0.71           | 0.68      | 0.45        | 0.49   |
| 20       | 0.60          | 0.66     | 0.71           | 0.68      | 0.45        | 0.49   |
| 21       | 0.60          | 0.65     | 0.72           | 0.68      | 0.44        | 0.49   |
| 22       | 0.60          | 0.65     | 0.72           | 0.69      | 0.44        | 0.48   |
| 23       | 0.60          | 0.65     | 0.72           | 0.69      | 0.44        | 0.48   |
| 24       | 0.60          | 0.65     | 0.72           | 0.69      | 0.44        | 0.48   |
| 25       | 0.60          | 0.64     | 0.73           | 0.69      | 0.44        | 0.48   |
| 26       | 0.59          | 0.64     | 0.73           | 0.70      | 0.43        | 0.47   |
| 27       | 0.59          | 0.64     | 0.73           | 0.70      | 0.43        | 0.47   |
| 28       | 0.59          | 0.64     | 0.74           | 0.70      | 0.43        | 0.47   |
| 29       | 0.59          | 0.63     | 0.74           | 0.71      | 0.43        | 0.46   |
| 30       | 0.58          | 0.63     | 0.74           | 0.71      | 0.42        | 0.46   |
| 31       | 0.58          | 0.63     | 0.75           | 0.72      | 0.42        | 0.46   |

Continued on next page



| $\alpha$ | $\phi_S^\ell$ | $\phi_S$ | $\varphi^\ell$ | $\varphi$ | $\psi^\ell$ | $\psi$ |
|----------|---------------|----------|----------------|-----------|-------------|--------|
| 32       | 0.58          | 0.62     | 0.75           | 0.72      | 0.42        | 0.45   |
| 33       | 0.58          | 0.62     | 0.75           | 0.72      | 0.42        | 0.45   |
| 34       | 0.57          | 0.61     | 0.76           | 0.73      | 0.41        | 0.44   |
| 35       | 0.57          | 0.61     | 0.76           | 0.73      | 0.41        | 0.44   |
| 36       | 0.57          | 0.61     | 0.76           | 0.74      | 0.41        | 0.44   |
| 37       | 0.56          | 0.60     | 0.77           | 0.74      | 0.40        | 0.43   |
| 38       | 0.56          | 0.60     | 0.77           | 0.74      | 0.40        | 0.43   |
| 39       | 0.55          | 0.59     | 0.78           | 0.75      | 0.39        | 0.42   |
| 40       | 0.55          | 0.59     | 0.78           | 0.75      | 0.39        | 0.42   |
| 41       | 0.55          | 0.58     | 0.79           | 0.76      | 0.39        | 0.41   |
| 42       | 0.54          | 0.58     | 0.79           | 0.76      | 0.38        | 0.41   |
| 43       | 0.54          | 0.57     | 0.80           | 0.77      | 0.38        | 0.41   |
| 44       | 0.53          | 0.57     | 0.80           | 0.77      | 0.37        | 0.41   |
| 45       | 0.53          | 0.56     | 0.80           | 0.78      | 0.37        | 0.40   |
| 46       | 0.52          | 0.56     | 0.81           | 0.78      | 0.36        | 0.40   |
| 47       | 0.52          | 0.55     | 0.81           | 0.79      | 0.36        | 0.39   |
| 48       | 0.51          | 0.54     | 0.82           | 0.79      | 0.35        | 0.38   |
| 49       | 0.50          | 0.54     | 0.82           | 0.80      | 0.35        | 0.38   |
| 50       | 0.50          | 0.53     | 0.83           | 0.80      | 0.35        | 0.37   |
| 51       | 0.49          | 0.52     | 0.83           | 0.81      | 0.34        | 0.36   |
| 52       | 0.49          | 0.52     | 0.84           | 0.81      | 0.34        | 0.36   |
| 53       | 0.48          | 0.51     | 0.84           | 0.82      | 0.33        | 0.35   |
| 54       | 0.47          | 0.50     | 0.85           | 0.82      | 0.32        | 0.35   |
| 55       | 0.47          | 0.50     | 0.85           | 0.83      | 0.32        | 0.35   |
| 56       | 0.46          | 0.49     | 0.86           | 0.83      | 0.31        | 0.34   |
| 57       | 0.45          | 0.48     | 0.86           | 0.84      | 0.31        | 0.33   |
| 58       | 0.44          | 0.47     | 0.87           | 0.84      | 0.30        | 0.32   |
| 59       | 0.43          | 0.46     | 0.87           | 0.85      | 0.29        | 0.32   |
| 60       | 0.43          | 0.46     | 0.88           | 0.85      | 0.29        | 0.32   |
| 61       | 0.42          | 0.45     | 0.88           | 0.86      | 0.28        | 0.31   |
| 62       | 0.41          | 0.44     | 0.89           | 0.86      | 0.27        | 0.30   |
| 63       | 0.40          | 0.43     | 0.89           | 0.87      | 0.27        | 0.29   |

Continued on next page

| $\alpha$ | $\phi_S^\ell$ | $\phi_S$ | $\varphi^\ell$ | $\varphi$ | $\psi^\ell$ | $\psi$ |
|----------|---------------|----------|----------------|-----------|-------------|--------|
| 64       | 0.39          | 0.42     | 0.90           | 0.87      | 0.26        | 0.29   |
| 65       | 0.38          | 0.41     | 0.90           | 0.88      | 0.25        | 0.28   |
| 66       | 0.37          | 0.40     | 0.91           | 0.88      | 0.25        | 0.27   |
| 67       | 0.36          | 0.39     | 0.91           | 0.89      | 0.24        | 0.26   |
| 68       | 0.35          | 0.38     | 0.92           | 0.89      | 0.23        | 0.26   |
| 69       | 0.34          | 0.37     | 0.92           | 0.89      | 0.23        | 0.25   |
| 70       | 0.33          | 0.36     | 0.93           | 0.90      | 0.22        | 0.24   |
| 71       | 0.32          | 0.35     | 0.93           | 0.90      | 0.21        | 0.24   |
| 72       | 0.31          | 0.34     | 0.94           | 0.91      | 0.20        | 0.23   |
| 73       | 0.29          | 0.33     | 0.94           | 0.91      | 0.19        | 0.22   |
| 74       | 0.28          | 0.32     | 0.94           | 0.92      | 0.18        | 0.21   |
| 75       | 0.27          | 0.31     | 0.95           | 0.92      | 0.18        | 0.21   |
| 76       | 0.26          | 0.30     | 0.95           | 0.92      | 0.17        | 0.20   |
| 77       | 0.25          | 0.28     | 0.95           | 0.93      | 0.16        | 0.19   |
| 78       | 0.24          | 0.27     | 0.96           | 0.93      | 0.16        | 0.18   |
| 79       | 0.22          | 0.26     | 0.96           | 0.93      | 0.14        | 0.17   |
| 80       | 0.21          | 0.25     | 0.96           | 0.94      | 0.14        | 0.17   |
| 81       | 0.20          | 0.24     | 0.97           | 0.94      | 0.13        | 0.16   |
| 82       | 0.19          | 0.23     | 0.97           | 0.94      | 0.12        | 0.15   |
| 83       | 0.18          | 0.22     | 0.97           | 0.94      | 0.12        | 0.15   |
| 84       | 0.18          | 0.21     | 0.97           | 0.94      | 0.12        | 0.14   |
| 85       | 0.17          | 0.20     | 0.97           | 0.95      | 0.11        | 0.13   |
| 86       | 0.16          | 0.20     | 0.97           | 0.95      | 0.10        | 0.13   |
| 87       | 0.15          | 0.19     | 0.97           | 0.95      | 0.10        | 0.13   |
| 88       | 0.14          | 0.18     | 0.97           | 0.95      | 0.09        | 0.12   |
| 89       | 0.14          | 0.18     | 0.97           | 0.95      | 0.09        | 0.12   |
| 90       | 0.14          | 0.18     | 0.97           | 0.95      | 0.09        | 0.12   |

Table S99: Reference ( $\phi_S$ ,  $\varphi$ ,  $\psi$ ) and approached ( $\phi_S^\ell$ ,  $\varphi^\ell$ ,  $\psi^\ell$ ) values of the topological descriptors for the first excited-state of the pyridinium-phenolate (PP), computed at the LC-wHPBE/6-311+G(d,p) level of theory.  $\alpha$  is the pyridinium-phenolate central twist angle amplitude.

| $\alpha$ | $\phi_S^\ell$ | $\phi_S$ | $\varphi^\ell$ | $\varphi$ | $\psi^\ell$ | $\psi$ |
|----------|---------------|----------|----------------|-----------|-------------|--------|
| 0        | 0.62          | 0.68     | 0.69           | 0.65      | 0.47        | 0.51   |
| 1        | 0.62          | 0.68     | 0.69           | 0.65      | 0.47        | 0.51   |
| 2        | 0.62          | 0.68     | 0.69           | 0.65      | 0.47        | 0.51   |
| 3        | 0.62          | 0.68     | 0.69           | 0.65      | 0.47        | 0.51   |
| 4        | 0.62          | 0.68     | 0.69           | 0.65      | 0.47        | 0.51   |
| 5        | 0.62          | 0.68     | 0.69           | 0.65      | 0.47        | 0.51   |
| 6        | 0.62          | 0.68     | 0.69           | 0.66      | 0.47        | 0.51   |
| 7        | 0.62          | 0.68     | 0.69           | 0.66      | 0.47        | 0.51   |
| 8        | 0.62          | 0.67     | 0.69           | 0.66      | 0.47        | 0.50   |
| 9        | 0.62          | 0.67     | 0.69           | 0.66      | 0.47        | 0.50   |
| 10       | 0.62          | 0.67     | 0.70           | 0.66      | 0.46        | 0.50   |
| 11       | 0.61          | 0.67     | 0.70           | 0.66      | 0.46        | 0.50   |
| 12       | 0.61          | 0.67     | 0.70           | 0.66      | 0.46        | 0.50   |
| 13       | 0.61          | 0.67     | 0.70           | 0.67      | 0.46        | 0.50   |
| 14       | 0.61          | 0.67     | 0.70           | 0.67      | 0.46        | 0.50   |
| 15       | 0.61          | 0.67     | 0.70           | 0.67      | 0.46        | 0.50   |
| 16       | 0.61          | 0.66     | 0.70           | 0.67      | 0.46        | 0.50   |
| 17       | 0.61          | 0.66     | 0.71           | 0.67      | 0.45        | 0.50   |
| 18       | 0.61          | 0.66     | 0.71           | 0.68      | 0.45        | 0.49   |
| 19       | 0.61          | 0.66     | 0.71           | 0.68      | 0.45        | 0.49   |
| 20       | 0.60          | 0.66     | 0.71           | 0.68      | 0.45        | 0.49   |
| 21       | 0.60          | 0.65     | 0.72           | 0.68      | 0.44        | 0.49   |
| 22       | 0.60          | 0.65     | 0.72           | 0.69      | 0.44        | 0.48   |
| 23       | 0.60          | 0.65     | 0.72           | 0.69      | 0.44        | 0.48   |
| 24       | 0.60          | 0.65     | 0.72           | 0.69      | 0.44        | 0.48   |
| 25       | 0.59          | 0.64     | 0.73           | 0.70      | 0.43        | 0.47   |
| 26       | 0.59          | 0.64     | 0.73           | 0.70      | 0.43        | 0.47   |
| 27       | 0.59          | 0.64     | 0.73           | 0.70      | 0.43        | 0.47   |
| 28       | 0.59          | 0.63     | 0.74           | 0.71      | 0.43        | 0.46   |
| 29       | 0.59          | 0.63     | 0.74           | 0.71      | 0.43        | 0.46   |
| 30       | 0.58          | 0.63     | 0.74           | 0.71      | 0.42        | 0.46   |
| 31       | 0.58          | 0.62     | 0.75           | 0.72      | 0.42        | 0.45   |

Continued on next page

| $\alpha$ | $\phi_S^\ell$ | $\phi_S$ | $\varphi^\ell$ | $\varphi$ | $\psi^\ell$ | $\psi$ |
|----------|---------------|----------|----------------|-----------|-------------|--------|
| 32       | 0.58          | 0.62     | 0.75           | 0.72      | 0.42        | 0.45   |
| 33       | 0.58          | 0.62     | 0.75           | 0.72      | 0.42        | 0.45   |
| 34       | 0.57          | 0.61     | 0.76           | 0.73      | 0.41        | 0.44   |
| 35       | 0.57          | 0.61     | 0.76           | 0.73      | 0.41        | 0.44   |
| 36       | 0.57          | 0.61     | 0.76           | 0.74      | 0.41        | 0.44   |
| 37       | 0.56          | 0.60     | 0.77           | 0.74      | 0.40        | 0.43   |
| 38       | 0.56          | 0.60     | 0.77           | 0.74      | 0.40        | 0.43   |
| 39       | 0.55          | 0.59     | 0.78           | 0.75      | 0.39        | 0.42   |
| 40       | 0.55          | 0.59     | 0.78           | 0.75      | 0.39        | 0.42   |
| 41       | 0.54          | 0.58     | 0.79           | 0.76      | 0.38        | 0.41   |
| 42       | 0.54          | 0.58     | 0.79           | 0.76      | 0.38        | 0.41   |
| 43       | 0.53          | 0.57     | 0.80           | 0.77      | 0.37        | 0.41   |
| 44       | 0.53          | 0.57     | 0.80           | 0.77      | 0.37        | 0.41   |
| 45       | 0.52          | 0.56     | 0.81           | 0.78      | 0.36        | 0.40   |
| 46       | 0.52          | 0.56     | 0.81           | 0.78      | 0.36        | 0.40   |
| 47       | 0.51          | 0.55     | 0.82           | 0.79      | 0.35        | 0.39   |
| 48       | 0.51          | 0.54     | 0.82           | 0.79      | 0.35        | 0.38   |
| 49       | 0.50          | 0.54     | 0.82           | 0.80      | 0.35        | 0.38   |
| 50       | 0.50          | 0.53     | 0.83           | 0.80      | 0.35        | 0.37   |
| 51       | 0.49          | 0.52     | 0.83           | 0.81      | 0.34        | 0.36   |
| 52       | 0.48          | 0.52     | 0.84           | 0.81      | 0.33        | 0.36   |
| 53       | 0.48          | 0.51     | 0.84           | 0.82      | 0.33        | 0.35   |
| 54       | 0.47          | 0.50     | 0.85           | 0.82      | 0.32        | 0.35   |
| 55       | 0.46          | 0.50     | 0.85           | 0.83      | 0.32        | 0.35   |
| 56       | 0.46          | 0.49     | 0.86           | 0.83      | 0.31        | 0.34   |
| 57       | 0.45          | 0.48     | 0.86           | 0.84      | 0.31        | 0.33   |
| 58       | 0.44          | 0.47     | 0.87           | 0.84      | 0.30        | 0.32   |
| 59       | 0.43          | 0.46     | 0.87           | 0.85      | 0.29        | 0.32   |
| 60       | 0.42          | 0.45     | 0.88           | 0.85      | 0.28        | 0.31   |
| 61       | 0.42          | 0.45     | 0.88           | 0.86      | 0.28        | 0.31   |
| 62       | 0.41          | 0.44     | 0.89           | 0.86      | 0.27        | 0.30   |
| 63       | 0.40          | 0.43     | 0.89           | 0.87      | 0.27        | 0.29   |

Continued on next page

| $\alpha$ | $\phi_S^\ell$ | $\phi_S$ | $\varphi^\ell$ | $\varphi$ | $\psi^\ell$ | $\psi$ |
|----------|---------------|----------|----------------|-----------|-------------|--------|
| 64       | 0.39          | 0.42     | 0.90           | 0.87      | 0.26        | 0.29   |
| 65       | 0.38          | 0.41     | 0.91           | 0.88      | 0.25        | 0.28   |
| 66       | 0.37          | 0.40     | 0.91           | 0.88      | 0.25        | 0.27   |
| 67       | 0.36          | 0.39     | 0.92           | 0.89      | 0.24        | 0.26   |
| 68       | 0.35          | 0.38     | 0.92           | 0.89      | 0.23        | 0.26   |
| 69       | 0.34          | 0.37     | 0.92           | 0.90      | 0.23        | 0.25   |
| 70       | 0.33          | 0.36     | 0.93           | 0.90      | 0.22        | 0.24   |
| 71       | 0.32          | 0.35     | 0.93           | 0.90      | 0.21        | 0.24   |
| 72       | 0.31          | 0.34     | 0.94           | 0.91      | 0.20        | 0.23   |
| 73       | 0.29          | 0.33     | 0.94           | 0.91      | 0.19        | 0.22   |
| 74       | 0.28          | 0.32     | 0.95           | 0.92      | 0.18        | 0.21   |
| 75       | 0.27          | 0.31     | 0.95           | 0.92      | 0.18        | 0.21   |
| 76       | 0.26          | 0.29     | 0.95           | 0.92      | 0.17        | 0.19   |
| 77       | 0.25          | 0.28     | 0.96           | 0.93      | 0.16        | 0.19   |
| 78       | 0.24          | 0.27     | 0.96           | 0.93      | 0.16        | 0.18   |
| 79       | 0.22          | 0.26     | 0.96           | 0.93      | 0.14        | 0.17   |
| 80       | 0.21          | 0.25     | 0.96           | 0.94      | 0.14        | 0.17   |
| 81       | 0.20          | 0.24     | 0.97           | 0.94      | 0.13        | 0.16   |
| 82       | 0.19          | 0.23     | 0.97           | 0.94      | 0.12        | 0.15   |
| 83       | 0.18          | 0.22     | 0.97           | 0.94      | 0.12        | 0.15   |
| 84       | 0.17          | 0.21     | 0.97           | 0.94      | 0.11        | 0.14   |
| 85       | 0.16          | 0.20     | 0.97           | 0.95      | 0.10        | 0.13   |
| 86       | 0.16          | 0.20     | 0.97           | 0.95      | 0.10        | 0.13   |
| 87       | 0.15          | 0.19     | 0.97           | 0.95      | 0.10        | 0.13   |
| 88       | 0.14          | 0.18     | 0.97           | 0.95      | 0.09        | 0.12   |
| 89       | 0.14          | 0.18     | 0.98           | 0.95      | 0.09        | 0.12   |
| 90       | 0.14          | 0.18     | 0.98           | 0.95      | 0.09        | 0.12   |

Table S100: Reference ( $\phi_S$ ,  $\varphi$ ,  $\psi$ ) and approached ( $\phi_S^\ell$ ,  $\varphi^\ell$ ,  $\psi^\ell$ ) values of the topological descriptors for the first excited-state of the pyridinium-phenolate (PP), computed at the LC-wHPBE/6-311+G(d) level of theory.  $\alpha$  is the pyridinium-phenolate central twist angle amplitude.

| $\alpha$ | $\phi_S^\ell$ | $\phi_S$ | $\varphi^\ell$ | $\varphi$ | $\psi^\ell$ | $\psi$ |
|----------|---------------|----------|----------------|-----------|-------------|--------|
| 0        | 0.64          | 0.69     | 0.68           | 0.64      | 0.48        | 0.52   |
| 1        | 0.64          | 0.69     | 0.68           | 0.64      | 0.48        | 0.52   |
| 2        | 0.64          | 0.69     | 0.68           | 0.64      | 0.48        | 0.52   |
| 3        | 0.64          | 0.69     | 0.68           | 0.64      | 0.48        | 0.52   |
| 4        | 0.64          | 0.69     | 0.68           | 0.64      | 0.48        | 0.52   |
| 5        | 0.64          | 0.69     | 0.68           | 0.64      | 0.48        | 0.52   |
| 6        | 0.64          | 0.69     | 0.69           | 0.64      | 0.48        | 0.52   |
| 7        | 0.64          | 0.69     | 0.69           | 0.65      | 0.48        | 0.52   |
| 8        | 0.64          | 0.69     | 0.69           | 0.65      | 0.48        | 0.52   |
| 9        | 0.64          | 0.69     | 0.69           | 0.65      | 0.48        | 0.52   |
| 10       | 0.64          | 0.69     | 0.69           | 0.65      | 0.48        | 0.52   |
| 11       | 0.63          | 0.69     | 0.69           | 0.65      | 0.47        | 0.52   |
| 12       | 0.63          | 0.69     | 0.69           | 0.65      | 0.47        | 0.52   |
| 13       | 0.63          | 0.68     | 0.69           | 0.65      | 0.47        | 0.51   |
| 14       | 0.63          | 0.68     | 0.69           | 0.66      | 0.47        | 0.51   |
| 15       | 0.63          | 0.68     | 0.70           | 0.66      | 0.47        | 0.51   |
| 16       | 0.63          | 0.68     | 0.70           | 0.66      | 0.47        | 0.51   |
| 17       | 0.63          | 0.68     | 0.70           | 0.66      | 0.47        | 0.51   |
| 18       | 0.63          | 0.68     | 0.70           | 0.66      | 0.47        | 0.51   |
| 19       | 0.62          | 0.67     | 0.70           | 0.67      | 0.46        | 0.50   |
| 20       | 0.62          | 0.67     | 0.71           | 0.67      | 0.46        | 0.50   |
| 21       | 0.62          | 0.67     | 0.71           | 0.67      | 0.46        | 0.50   |
| 22       | 0.62          | 0.67     | 0.71           | 0.68      | 0.46        | 0.50   |
| 23       | 0.62          | 0.66     | 0.72           | 0.68      | 0.45        | 0.49   |
| 24       | 0.62          | 0.66     | 0.72           | 0.68      | 0.45        | 0.49   |
| 25       | 0.61          | 0.66     | 0.72           | 0.68      | 0.45        | 0.49   |
| 26       | 0.61          | 0.66     | 0.72           | 0.69      | 0.45        | 0.49   |
| 27       | 0.61          | 0.65     | 0.73           | 0.69      | 0.44        | 0.48   |
| 28       | 0.61          | 0.65     | 0.73           | 0.70      | 0.44        | 0.48   |
| 29       | 0.60          | 0.65     | 0.73           | 0.70      | 0.44        | 0.48   |
| 30       | 0.60          | 0.64     | 0.74           | 0.70      | 0.43        | 0.47   |
| 31       | 0.60          | 0.64     | 0.74           | 0.71      | 0.43        | 0.47   |

Continued on next page

| $\alpha$ | $\phi_S^\ell$ | $\phi_S$ | $\varphi^\ell$ | $\varphi$ | $\psi^\ell$ | $\psi$ |
|----------|---------------|----------|----------------|-----------|-------------|--------|
| 32       | 0.60          | 0.64     | 0.74           | 0.71      | 0.43        | 0.47   |
| 33       | 0.59          | 0.63     | 0.75           | 0.71      | 0.42        | 0.46   |
| 34       | 0.59          | 0.63     | 0.75           | 0.72      | 0.42        | 0.46   |
| 35       | 0.59          | 0.62     | 0.76           | 0.72      | 0.42        | 0.45   |
| 36       | 0.58          | 0.62     | 0.76           | 0.73      | 0.41        | 0.45   |
| 37       | 0.58          | 0.62     | 0.76           | 0.73      | 0.41        | 0.45   |
| 38       | 0.58          | 0.61     | 0.77           | 0.74      | 0.41        | 0.44   |
| 39       | 0.57          | 0.61     | 0.77           | 0.74      | 0.41        | 0.44   |
| 40       | 0.57          | 0.60     | 0.78           | 0.74      | 0.40        | 0.43   |
| 41       | 0.56          | 0.60     | 0.78           | 0.75      | 0.40        | 0.43   |
| 42       | 0.56          | 0.59     | 0.79           | 0.75      | 0.39        | 0.42   |
| 43       | 0.55          | 0.59     | 0.79           | 0.76      | 0.39        | 0.42   |
| 44       | 0.55          | 0.58     | 0.80           | 0.76      | 0.38        | 0.41   |
| 45       | 0.54          | 0.58     | 0.80           | 0.77      | 0.38        | 0.41   |
| 46       | 0.54          | 0.57     | 0.81           | 0.77      | 0.37        | 0.41   |
| 47       | 0.53          | 0.56     | 0.81           | 0.78      | 0.37        | 0.40   |
| 48       | 0.53          | 0.56     | 0.81           | 0.78      | 0.37        | 0.40   |
| 49       | 0.52          | 0.55     | 0.82           | 0.79      | 0.36        | 0.39   |
| 50       | 0.52          | 0.55     | 0.82           | 0.79      | 0.36        | 0.39   |
| 51       | 0.51          | 0.54     | 0.83           | 0.80      | 0.35        | 0.38   |
| 52       | 0.50          | 0.53     | 0.83           | 0.80      | 0.35        | 0.37   |
| 53       | 0.50          | 0.52     | 0.84           | 0.81      | 0.34        | 0.36   |
| 54       | 0.49          | 0.52     | 0.84           | 0.81      | 0.34        | 0.36   |
| 55       | 0.48          | 0.51     | 0.85           | 0.82      | 0.33        | 0.35   |
| 56       | 0.47          | 0.50     | 0.85           | 0.82      | 0.32        | 0.35   |
| 57       | 0.47          | 0.49     | 0.86           | 0.83      | 0.32        | 0.34   |
| 58       | 0.46          | 0.49     | 0.86           | 0.83      | 0.31        | 0.34   |
| 59       | 0.45          | 0.48     | 0.87           | 0.84      | 0.30        | 0.33   |
| 60       | 0.44          | 0.47     | 0.87           | 0.85      | 0.30        | 0.32   |
| 61       | 0.43          | 0.46     | 0.88           | 0.85      | 0.29        | 0.32   |
| 62       | 0.42          | 0.45     | 0.88           | 0.86      | 0.28        | 0.31   |
| 63       | 0.41          | 0.44     | 0.89           | 0.86      | 0.27        | 0.30   |

Continued on next page

| $\alpha$ | $\phi_S^\ell$ | $\phi_S$ | $\varphi^\ell$ | $\varphi$ | $\psi^\ell$ | $\psi$ |
|----------|---------------|----------|----------------|-----------|-------------|--------|
| 64       | 0.40          | 0.43     | 0.90           | 0.87      | 0.27        | 0.29   |
| 65       | 0.39          | 0.42     | 0.90           | 0.87      | 0.26        | 0.29   |
| 66       | 0.38          | 0.41     | 0.91           | 0.88      | 0.25        | 0.28   |
| 67       | 0.37          | 0.40     | 0.91           | 0.88      | 0.25        | 0.27   |
| 68       | 0.36          | 0.39     | 0.92           | 0.89      | 0.24        | 0.26   |
| 69       | 0.35          | 0.38     | 0.92           | 0.89      | 0.23        | 0.26   |
| 70       | 0.34          | 0.37     | 0.93           | 0.90      | 0.22        | 0.25   |
| 71       | 0.33          | 0.36     | 0.93           | 0.90      | 0.22        | 0.24   |
| 72       | 0.32          | 0.35     | 0.94           | 0.90      | 0.21        | 0.24   |
| 73       | 0.30          | 0.34     | 0.94           | 0.91      | 0.20        | 0.23   |
| 74       | 0.29          | 0.33     | 0.94           | 0.91      | 0.19        | 0.22   |
| 75       | 0.28          | 0.32     | 0.95           | 0.92      | 0.18        | 0.21   |
| 76       | 0.27          | 0.30     | 0.95           | 0.92      | 0.18        | 0.20   |
| 77       | 0.25          | 0.29     | 0.96           | 0.92      | 0.16        | 0.19   |
| 78       | 0.24          | 0.28     | 0.96           | 0.93      | 0.16        | 0.19   |
| 79       | 0.23          | 0.27     | 0.96           | 0.93      | 0.15        | 0.18   |
| 80       | 0.21          | 0.26     | 0.97           | 0.93      | 0.14        | 0.17   |
| 81       | 0.20          | 0.25     | 0.97           | 0.94      | 0.13        | 0.17   |
| 82       | 0.19          | 0.24     | 0.97           | 0.94      | 0.12        | 0.16   |
| 83       | 0.18          | 0.23     | 0.97           | 0.94      | 0.12        | 0.15   |
| 84       | 0.17          | 0.22     | 0.97           | 0.94      | 0.11        | 0.15   |
| 85       | 0.16          | 0.21     | 0.98           | 0.95      | 0.10        | 0.14   |
| 86       | 0.15          | 0.20     | 0.98           | 0.95      | 0.10        | 0.13   |
| 87       | 0.14          | 0.19     | 0.98           | 0.95      | 0.09        | 0.13   |
| 88       | 0.13          | 0.18     | 0.98           | 0.95      | 0.08        | 0.12   |
| 89       | 0.13          | 0.18     | 0.98           | 0.95      | 0.08        | 0.12   |
| 90       | 0.12          | 0.18     | 0.98           | 0.95      | 0.08        | 0.12   |

Table S101: Reference ( $\phi_S$ ,  $\varphi$ ,  $\psi$ ) and approached ( $\phi_S^\ell$ ,  $\varphi^\ell$ ,  $\psi^\ell$ ) values of the topological descriptors for the first excited-state of the pyridinium-phenolate (PP), computed at the LC-wHPBE/6-311G(d) level of theory.  $\alpha$  is the pyridinium-phenolate central twist angle amplitude.



| $\alpha$ | $\phi_S^\ell$ | $\phi_S$ | $\varphi^\ell$ | $\varphi$ | $\psi^\ell$ | $\psi$ |
|----------|---------------|----------|----------------|-----------|-------------|--------|
| 0        | 0.62          | 0.67     | 0.69           | 0.66      | 0.47        | 0.50   |
| 1        | 0.62          | 0.67     | 0.69           | 0.66      | 0.47        | 0.50   |
| 2        | 0.62          | 0.67     | 0.69           | 0.66      | 0.47        | 0.50   |
| 3        | 0.62          | 0.67     | 0.69           | 0.66      | 0.47        | 0.50   |
| 4        | 0.62          | 0.67     | 0.69           | 0.66      | 0.47        | 0.50   |
| 5        | 0.62          | 0.67     | 0.69           | 0.66      | 0.47        | 0.50   |
| 6        | 0.62          | 0.67     | 0.69           | 0.66      | 0.47        | 0.50   |
| 7        | 0.62          | 0.67     | 0.69           | 0.66      | 0.47        | 0.50   |
| 8        | 0.62          | 0.67     | 0.69           | 0.67      | 0.47        | 0.50   |
| 9        | 0.61          | 0.66     | 0.69           | 0.67      | 0.46        | 0.50   |
| 10       | 0.61          | 0.66     | 0.70           | 0.67      | 0.46        | 0.50   |
| 11       | 0.61          | 0.66     | 0.70           | 0.67      | 0.46        | 0.50   |
| 12       | 0.61          | 0.66     | 0.70           | 0.67      | 0.46        | 0.50   |
| 13       | 0.61          | 0.66     | 0.70           | 0.67      | 0.46        | 0.50   |
| 14       | 0.61          | 0.66     | 0.70           | 0.67      | 0.46        | 0.50   |
| 15       | 0.61          | 0.66     | 0.70           | 0.68      | 0.46        | 0.49   |
| 16       | 0.61          | 0.65     | 0.71           | 0.68      | 0.45        | 0.49   |
| 17       | 0.61          | 0.65     | 0.71           | 0.68      | 0.45        | 0.49   |
| 18       | 0.61          | 0.65     | 0.71           | 0.68      | 0.45        | 0.49   |
| 19       | 0.60          | 0.65     | 0.71           | 0.69      | 0.45        | 0.48   |
| 20       | 0.60          | 0.65     | 0.71           | 0.69      | 0.45        | 0.48   |
| 21       | 0.60          | 0.65     | 0.72           | 0.69      | 0.44        | 0.48   |
| 22       | 0.60          | 0.64     | 0.72           | 0.69      | 0.44        | 0.48   |
| 23       | 0.60          | 0.64     | 0.72           | 0.70      | 0.44        | 0.47   |
| 24       | 0.60          | 0.64     | 0.73           | 0.70      | 0.44        | 0.47   |
| 25       | 0.59          | 0.64     | 0.73           | 0.70      | 0.43        | 0.47   |
| 26       | 0.59          | 0.63     | 0.73           | 0.71      | 0.43        | 0.46   |
| 27       | 0.59          | 0.63     | 0.73           | 0.71      | 0.43        | 0.46   |
| 28       | 0.59          | 0.63     | 0.74           | 0.71      | 0.43        | 0.46   |
| 29       | 0.59          | 0.62     | 0.74           | 0.72      | 0.43        | 0.45   |
| 30       | 0.58          | 0.62     | 0.74           | 0.72      | 0.42        | 0.45   |
| 31       | 0.58          | 0.62     | 0.75           | 0.72      | 0.42        | 0.45   |

Continued on next page

| $\alpha$ | $\phi_S^\ell$ | $\phi_S$ | $\varphi^\ell$ | $\varphi$ | $\psi^\ell$ | $\psi$ |
|----------|---------------|----------|----------------|-----------|-------------|--------|
| 32       | 0.58          | 0.61     | 0.75           | 0.73      | 0.42        | 0.44   |
| 33       | 0.58          | 0.61     | 0.75           | 0.73      | 0.42        | 0.44   |
| 34       | 0.57          | 0.61     | 0.76           | 0.73      | 0.41        | 0.44   |
| 35       | 0.57          | 0.60     | 0.76           | 0.74      | 0.41        | 0.43   |
| 36       | 0.57          | 0.60     | 0.76           | 0.74      | 0.41        | 0.43   |
| 37       | 0.56          | 0.59     | 0.77           | 0.75      | 0.40        | 0.42   |
| 38       | 0.56          | 0.59     | 0.77           | 0.75      | 0.40        | 0.42   |
| 39       | 0.55          | 0.59     | 0.78           | 0.75      | 0.39        | 0.42   |
| 40       | 0.55          | 0.58     | 0.78           | 0.76      | 0.39        | 0.41   |
| 41       | 0.55          | 0.58     | 0.79           | 0.76      | 0.39        | 0.41   |
| 42       | 0.54          | 0.57     | 0.79           | 0.77      | 0.38        | 0.41   |
| 43       | 0.54          | 0.57     | 0.80           | 0.77      | 0.38        | 0.41   |
| 44       | 0.53          | 0.56     | 0.80           | 0.78      | 0.37        | 0.40   |
| 45       | 0.53          | 0.56     | 0.81           | 0.78      | 0.37        | 0.40   |
| 46       | 0.52          | 0.55     | 0.81           | 0.79      | 0.36        | 0.39   |
| 47       | 0.51          | 0.54     | 0.81           | 0.79      | 0.36        | 0.38   |
| 48       | 0.51          | 0.54     | 0.82           | 0.80      | 0.35        | 0.38   |
| 49       | 0.50          | 0.53     | 0.82           | 0.80      | 0.35        | 0.37   |
| 50       | 0.50          | 0.53     | 0.83           | 0.81      | 0.35        | 0.37   |
| 51       | 0.49          | 0.52     | 0.83           | 0.81      | 0.34        | 0.36   |
| 52       | 0.48          | 0.51     | 0.84           | 0.82      | 0.33        | 0.35   |
| 53       | 0.48          | 0.51     | 0.84           | 0.82      | 0.33        | 0.35   |
| 54       | 0.47          | 0.50     | 0.85           | 0.83      | 0.32        | 0.35   |
| 55       | 0.46          | 0.49     | 0.85           | 0.83      | 0.32        | 0.34   |
| 56       | 0.46          | 0.48     | 0.86           | 0.84      | 0.31        | 0.33   |
| 57       | 0.45          | 0.48     | 0.86           | 0.84      | 0.31        | 0.33   |
| 58       | 0.44          | 0.47     | 0.87           | 0.85      | 0.30        | 0.32   |
| 59       | 0.43          | 0.46     | 0.87           | 0.85      | 0.29        | 0.32   |
| 60       | 0.42          | 0.45     | 0.88           | 0.86      | 0.28        | 0.31   |
| 61       | 0.41          | 0.44     | 0.88           | 0.86      | 0.28        | 0.30   |
| 62       | 0.40          | 0.43     | 0.89           | 0.87      | 0.27        | 0.29   |
| 63       | 0.40          | 0.43     | 0.90           | 0.87      | 0.27        | 0.29   |

Continued on next page

| $\alpha$ | $\phi_S^\ell$ | $\phi_S$ | $\varphi^\ell$ | $\varphi$ | $\psi^\ell$ | $\psi$ |
|----------|---------------|----------|----------------|-----------|-------------|--------|
| 64       | 0.39          | 0.42     | 0.90           | 0.88      | 0.26        | 0.28   |
| 65       | 0.38          | 0.41     | 0.91           | 0.88      | 0.25        | 0.28   |
| 66       | 0.37          | 0.40     | 0.91           | 0.88      | 0.25        | 0.27   |
| 67       | 0.36          | 0.39     | 0.92           | 0.89      | 0.24        | 0.26   |
| 68       | 0.35          | 0.38     | 0.92           | 0.89      | 0.23        | 0.26   |
| 69       | 0.33          | 0.37     | 0.93           | 0.90      | 0.22        | 0.25   |
| 70       | 0.32          | 0.36     | 0.93           | 0.90      | 0.21        | 0.24   |
| 71       | 0.31          | 0.35     | 0.94           | 0.91      | 0.20        | 0.23   |
| 72       | 0.30          | 0.33     | 0.94           | 0.91      | 0.20        | 0.22   |
| 73       | 0.29          | 0.32     | 0.95           | 0.92      | 0.19        | 0.21   |
| 74       | 0.28          | 0.31     | 0.95           | 0.92      | 0.18        | 0.21   |
| 75       | 0.26          | 0.30     | 0.95           | 0.92      | 0.17        | 0.20   |
| 76       | 0.25          | 0.29     | 0.96           | 0.93      | 0.16        | 0.19   |
| 77       | 0.24          | 0.28     | 0.96           | 0.93      | 0.16        | 0.19   |
| 78       | 0.23          | 0.27     | 0.96           | 0.93      | 0.15        | 0.18   |
| 79       | 0.22          | 0.26     | 0.97           | 0.94      | 0.14        | 0.17   |
| 80       | 0.20          | 0.25     | 0.97           | 0.94      | 0.13        | 0.17   |
| 81       | 0.19          | 0.23     | 0.97           | 0.94      | 0.12        | 0.15   |
| 82       | 0.18          | 0.22     | 0.97           | 0.94      | 0.12        | 0.15   |
| 83       | 0.17          | 0.21     | 0.97           | 0.95      | 0.11        | 0.14   |
| 84       | 0.16          | 0.20     | 0.98           | 0.95      | 0.10        | 0.13   |
| 85       | 0.16          | 0.19     | 0.98           | 0.95      | 0.10        | 0.13   |
| 86       | 0.15          | 0.19     | 0.98           | 0.95      | 0.10        | 0.13   |
| 87       | 0.14          | 0.18     | 0.98           | 0.95      | 0.09        | 0.12   |
| 88       | 0.13          | 0.17     | 0.98           | 0.95      | 0.08        | 0.11   |
| 89       | 0.13          | 0.17     | 0.98           | 0.95      | 0.08        | 0.11   |
| 90       | 0.12          | 0.17     | 0.98           | 0.95      | 0.08        | 0.11   |

Table S102: Reference ( $\phi_S$ ,  $\varphi$ ,  $\psi$ ) and approached ( $\phi_S^\ell$ ,  $\varphi^\ell$ ,  $\psi^\ell$ ) values of the topological descriptors for the first excited-state of the pyridinium-phenolate (PP), computed at the LC-wHPBE/6-311+G level of theory.  $\alpha$  is the pyridinium-phenolate central twist angle amplitude.

| $\alpha$ | $\phi_S^\ell$ | $\phi_S$ | $\varphi^\ell$ | $\varphi$ | $\psi^\ell$ | $\psi$ |
|----------|---------------|----------|----------------|-----------|-------------|--------|
| 0        | 0.64          | 0.68     | 0.68           | 0.65      | 0.48        | 0.51   |
| 1        | 0.64          | 0.68     | 0.68           | 0.65      | 0.48        | 0.51   |
| 2        | 0.64          | 0.68     | 0.68           | 0.65      | 0.48        | 0.51   |
| 3        | 0.64          | 0.68     | 0.68           | 0.65      | 0.48        | 0.51   |
| 4        | 0.64          | 0.68     | 0.68           | 0.65      | 0.48        | 0.51   |
| 5        | 0.64          | 0.68     | 0.69           | 0.65      | 0.48        | 0.51   |
| 6        | 0.64          | 0.68     | 0.69           | 0.65      | 0.48        | 0.51   |
| 7        | 0.64          | 0.68     | 0.69           | 0.65      | 0.48        | 0.51   |
| 8        | 0.64          | 0.68     | 0.69           | 0.65      | 0.48        | 0.51   |
| 9        | 0.64          | 0.68     | 0.69           | 0.66      | 0.48        | 0.51   |
| 10       | 0.63          | 0.68     | 0.69           | 0.66      | 0.47        | 0.51   |
| 11       | 0.63          | 0.68     | 0.69           | 0.66      | 0.47        | 0.51   |
| 12       | 0.63          | 0.68     | 0.69           | 0.66      | 0.47        | 0.51   |
| 13       | 0.63          | 0.67     | 0.69           | 0.66      | 0.47        | 0.50   |
| 14       | 0.63          | 0.67     | 0.70           | 0.66      | 0.47        | 0.50   |
| 15       | 0.63          | 0.67     | 0.70           | 0.67      | 0.47        | 0.50   |
| 16       | 0.63          | 0.67     | 0.70           | 0.67      | 0.47        | 0.50   |
| 17       | 0.63          | 0.67     | 0.70           | 0.67      | 0.47        | 0.50   |
| 18       | 0.62          | 0.67     | 0.70           | 0.67      | 0.46        | 0.50   |
| 19       | 0.62          | 0.66     | 0.71           | 0.67      | 0.46        | 0.50   |
| 20       | 0.62          | 0.66     | 0.71           | 0.68      | 0.46        | 0.49   |
| 21       | 0.62          | 0.66     | 0.71           | 0.68      | 0.46        | 0.49   |
| 22       | 0.62          | 0.66     | 0.71           | 0.68      | 0.46        | 0.49   |
| 23       | 0.62          | 0.66     | 0.72           | 0.69      | 0.45        | 0.49   |
| 24       | 0.61          | 0.65     | 0.72           | 0.69      | 0.45        | 0.48   |
| 25       | 0.61          | 0.65     | 0.72           | 0.69      | 0.45        | 0.48   |
| 26       | 0.61          | 0.65     | 0.73           | 0.70      | 0.44        | 0.48   |
| 27       | 0.61          | 0.64     | 0.73           | 0.70      | 0.44        | 0.47   |
| 28       | 0.61          | 0.64     | 0.73           | 0.70      | 0.44        | 0.47   |
| 29       | 0.60          | 0.64     | 0.73           | 0.71      | 0.44        | 0.47   |
| 30       | 0.60          | 0.64     | 0.74           | 0.71      | 0.43        | 0.47   |
| 31       | 0.60          | 0.63     | 0.74           | 0.71      | 0.43        | 0.46   |

Continued on next page

| $\alpha$ | $\phi_S^\ell$ | $\phi_S$ | $\varphi^\ell$ | $\varphi$ | $\psi^\ell$ | $\psi$ |
|----------|---------------|----------|----------------|-----------|-------------|--------|
| 32       | 0.60          | 0.63     | 0.74           | 0.72      | 0.43        | 0.46   |
| 33       | 0.59          | 0.62     | 0.75           | 0.72      | 0.42        | 0.45   |
| 34       | 0.59          | 0.62     | 0.75           | 0.72      | 0.42        | 0.45   |
| 35       | 0.59          | 0.62     | 0.76           | 0.73      | 0.42        | 0.45   |
| 36       | 0.58          | 0.61     | 0.76           | 0.73      | 0.41        | 0.44   |
| 37       | 0.58          | 0.61     | 0.76           | 0.74      | 0.41        | 0.44   |
| 38       | 0.58          | 0.60     | 0.77           | 0.74      | 0.41        | 0.43   |
| 39       | 0.57          | 0.60     | 0.77           | 0.75      | 0.41        | 0.43   |
| 40       | 0.57          | 0.60     | 0.78           | 0.75      | 0.40        | 0.43   |
| 41       | 0.56          | 0.59     | 0.78           | 0.75      | 0.40        | 0.42   |
| 42       | 0.56          | 0.59     | 0.79           | 0.76      | 0.39        | 0.42   |
| 43       | 0.55          | 0.58     | 0.79           | 0.76      | 0.39        | 0.41   |
| 44       | 0.55          | 0.58     | 0.80           | 0.77      | 0.38        | 0.41   |
| 45       | 0.54          | 0.57     | 0.80           | 0.77      | 0.38        | 0.41   |
| 46       | 0.54          | 0.56     | 0.80           | 0.78      | 0.38        | 0.40   |
| 47       | 0.53          | 0.56     | 0.81           | 0.78      | 0.37        | 0.40   |
| 48       | 0.53          | 0.55     | 0.81           | 0.79      | 0.37        | 0.39   |
| 49       | 0.52          | 0.55     | 0.82           | 0.79      | 0.36        | 0.39   |
| 50       | 0.52          | 0.54     | 0.82           | 0.80      | 0.36        | 0.38   |
| 51       | 0.51          | 0.53     | 0.83           | 0.80      | 0.35        | 0.37   |
| 52       | 0.50          | 0.53     | 0.83           | 0.81      | 0.35        | 0.37   |
| 53       | 0.50          | 0.52     | 0.84           | 0.81      | 0.34        | 0.36   |
| 54       | 0.49          | 0.51     | 0.84           | 0.82      | 0.34        | 0.35   |
| 55       | 0.48          | 0.51     | 0.85           | 0.82      | 0.33        | 0.35   |
| 56       | 0.47          | 0.50     | 0.85           | 0.83      | 0.32        | 0.35   |
| 57       | 0.47          | 0.49     | 0.86           | 0.83      | 0.32        | 0.34   |
| 58       | 0.46          | 0.48     | 0.86           | 0.84      | 0.31        | 0.33   |
| 59       | 0.45          | 0.47     | 0.87           | 0.84      | 0.30        | 0.32   |
| 60       | 0.44          | 0.47     | 0.87           | 0.85      | 0.30        | 0.32   |
| 61       | 0.43          | 0.46     | 0.88           | 0.85      | 0.29        | 0.32   |
| 62       | 0.42          | 0.45     | 0.89           | 0.86      | 0.28        | 0.31   |
| 63       | 0.41          | 0.44     | 0.89           | 0.86      | 0.27        | 0.30   |

Continued on next page

| $\alpha$ | $\phi_S^\ell$ | $\phi_S$ | $\varphi^\ell$ | $\varphi$ | $\psi^\ell$ | $\psi$ |
|----------|---------------|----------|----------------|-----------|-------------|--------|
| 64       | 0.40          | 0.43     | 0.90           | 0.87      | 0.27        | 0.29   |
| 65       | 0.39          | 0.42     | 0.90           | 0.87      | 0.26        | 0.29   |
| 66       | 0.38          | 0.41     | 0.91           | 0.88      | 0.25        | 0.28   |
| 67       | 0.37          | 0.40     | 0.91           | 0.88      | 0.25        | 0.27   |
| 68       | 0.36          | 0.39     | 0.92           | 0.89      | 0.24        | 0.26   |
| 69       | 0.35          | 0.38     | 0.92           | 0.89      | 0.23        | 0.26   |
| 70       | 0.34          | 0.37     | 0.93           | 0.90      | 0.22        | 0.25   |
| 71       | 0.32          | 0.36     | 0.93           | 0.90      | 0.21        | 0.24   |
| 72       | 0.31          | 0.35     | 0.94           | 0.91      | 0.20        | 0.23   |
| 73       | 0.30          | 0.34     | 0.94           | 0.91      | 0.20        | 0.23   |
| 74       | 0.29          | 0.32     | 0.95           | 0.92      | 0.19        | 0.21   |
| 75       | 0.27          | 0.31     | 0.95           | 0.92      | 0.18        | 0.21   |
| 76       | 0.26          | 0.30     | 0.96           | 0.92      | 0.17        | 0.20   |
| 77       | 0.25          | 0.29     | 0.96           | 0.93      | 0.16        | 0.19   |
| 78       | 0.23          | 0.28     | 0.96           | 0.93      | 0.15        | 0.19   |
| 79       | 0.22          | 0.26     | 0.97           | 0.94      | 0.14        | 0.17   |
| 80       | 0.21          | 0.25     | 0.97           | 0.94      | 0.14        | 0.17   |
| 81       | 0.19          | 0.24     | 0.97           | 0.94      | 0.12        | 0.16   |
| 82       | 0.18          | 0.23     | 0.98           | 0.94      | 0.12        | 0.15   |
| 83       | 0.17          | 0.22     | 0.98           | 0.95      | 0.11        | 0.14   |
| 84       | 0.16          | 0.21     | 0.98           | 0.95      | 0.10        | 0.14   |
| 85       | 0.15          | 0.20     | 0.98           | 0.95      | 0.10        | 0.13   |
| 86       | 0.14          | 0.19     | 0.98           | 0.95      | 0.09        | 0.13   |
| 87       | 0.13          | 0.18     | 0.98           | 0.95      | 0.08        | 0.12   |
| 88       | 0.12          | 0.17     | 0.98           | 0.95      | 0.08        | 0.11   |
| 89       | 0.11          | 0.17     | 0.98           | 0.95      | 0.07        | 0.11   |
| 90       | 0.11          | 0.17     | 0.99           | 0.95      | 0.07        | 0.11   |

Table S103: Reference ( $\phi_S$ ,  $\varphi$ ,  $\psi$ ) and approached ( $\phi_S^\ell$ ,  $\varphi^\ell$ ,  $\psi^\ell$ ) values of the topological descriptors for the first excited-state of the pyridinium-phenolate (PP), computed at the LC-wHPBE/6-311G level of theory.  $\alpha$  is the pyridinium-phenolate central twist angle amplitude.

| $\alpha$ | $\phi_S^\ell$ | $\phi_S$ | $\varphi^\ell$ | $\varphi$ | $\psi^\ell$ | $\psi$ |
|----------|---------------|----------|----------------|-----------|-------------|--------|
| 0        | 0.62          | 0.68     | 0.69           | 0.65      | 0.47        | 0.51   |
| 1        | 0.62          | 0.68     | 0.69           | 0.65      | 0.47        | 0.51   |
| 2        | 0.62          | 0.68     | 0.69           | 0.65      | 0.47        | 0.51   |
| 3        | 0.62          | 0.68     | 0.69           | 0.65      | 0.47        | 0.51   |
| 4        | 0.62          | 0.68     | 0.69           | 0.65      | 0.47        | 0.51   |
| 5        | 0.62          | 0.68     | 0.69           | 0.65      | 0.47        | 0.51   |
| 6        | 0.62          | 0.68     | 0.69           | 0.65      | 0.47        | 0.51   |
| 7        | 0.62          | 0.68     | 0.69           | 0.66      | 0.47        | 0.51   |
| 8        | 0.62          | 0.67     | 0.69           | 0.66      | 0.47        | 0.50   |
| 9        | 0.62          | 0.67     | 0.69           | 0.66      | 0.47        | 0.50   |
| 10       | 0.62          | 0.67     | 0.70           | 0.66      | 0.46        | 0.50   |
| 11       | 0.62          | 0.67     | 0.70           | 0.66      | 0.46        | 0.50   |
| 12       | 0.62          | 0.67     | 0.70           | 0.66      | 0.46        | 0.50   |
| 13       | 0.62          | 0.67     | 0.70           | 0.66      | 0.46        | 0.50   |
| 14       | 0.62          | 0.67     | 0.70           | 0.67      | 0.46        | 0.50   |
| 15       | 0.61          | 0.67     | 0.70           | 0.67      | 0.46        | 0.50   |
| 16       | 0.61          | 0.66     | 0.70           | 0.67      | 0.46        | 0.50   |
| 17       | 0.61          | 0.66     | 0.71           | 0.67      | 0.45        | 0.50   |
| 18       | 0.61          | 0.66     | 0.71           | 0.67      | 0.45        | 0.50   |
| 19       | 0.61          | 0.66     | 0.71           | 0.68      | 0.45        | 0.49   |
| 20       | 0.61          | 0.66     | 0.71           | 0.68      | 0.45        | 0.49   |
| 21       | 0.61          | 0.65     | 0.72           | 0.68      | 0.45        | 0.49   |
| 22       | 0.60          | 0.65     | 0.72           | 0.68      | 0.44        | 0.49   |
| 23       | 0.60          | 0.65     | 0.72           | 0.69      | 0.44        | 0.48   |
| 24       | 0.60          | 0.65     | 0.72           | 0.69      | 0.44        | 0.48   |
| 25       | 0.60          | 0.64     | 0.73           | 0.69      | 0.44        | 0.48   |
| 26       | 0.60          | 0.64     | 0.73           | 0.70      | 0.44        | 0.47   |
| 27       | 0.59          | 0.64     | 0.73           | 0.70      | 0.43        | 0.47   |
| 28       | 0.59          | 0.63     | 0.74           | 0.70      | 0.43        | 0.47   |
| 29       | 0.59          | 0.63     | 0.74           | 0.71      | 0.43        | 0.46   |
| 30       | 0.59          | 0.63     | 0.74           | 0.71      | 0.43        | 0.46   |
| 31       | 0.58          | 0.62     | 0.75           | 0.71      | 0.42        | 0.46   |

Continued on next page

| $\alpha$ | $\phi_S^\ell$ | $\phi_S$ | $\varphi^\ell$ | $\varphi$ | $\psi^\ell$ | $\psi$ |
|----------|---------------|----------|----------------|-----------|-------------|--------|
| 32       | 0.58          | 0.62     | 0.75           | 0.72      | 0.42        | 0.45   |
| 33       | 0.58          | 0.62     | 0.75           | 0.72      | 0.42        | 0.45   |
| 34       | 0.57          | 0.61     | 0.76           | 0.73      | 0.41        | 0.44   |
| 35       | 0.57          | 0.61     | 0.76           | 0.73      | 0.41        | 0.44   |
| 36       | 0.57          | 0.61     | 0.76           | 0.73      | 0.41        | 0.44   |
| 37       | 0.56          | 0.60     | 0.77           | 0.74      | 0.40        | 0.43   |
| 38       | 0.56          | 0.60     | 0.77           | 0.74      | 0.40        | 0.43   |
| 39       | 0.55          | 0.59     | 0.78           | 0.75      | 0.39        | 0.42   |
| 40       | 0.55          | 0.59     | 0.78           | 0.75      | 0.39        | 0.42   |
| 41       | 0.55          | 0.58     | 0.79           | 0.76      | 0.39        | 0.41   |
| 42       | 0.54          | 0.58     | 0.79           | 0.76      | 0.38        | 0.41   |
| 43       | 0.54          | 0.57     | 0.80           | 0.77      | 0.38        | 0.41   |
| 44       | 0.53          | 0.57     | 0.80           | 0.77      | 0.37        | 0.41   |
| 45       | 0.53          | 0.56     | 0.81           | 0.78      | 0.37        | 0.40   |
| 46       | 0.52          | 0.56     | 0.81           | 0.78      | 0.36        | 0.40   |
| 47       | 0.52          | 0.55     | 0.81           | 0.79      | 0.36        | 0.39   |
| 48       | 0.51          | 0.54     | 0.82           | 0.79      | 0.35        | 0.38   |
| 49       | 0.50          | 0.54     | 0.82           | 0.80      | 0.35        | 0.38   |
| 50       | 0.50          | 0.53     | 0.83           | 0.80      | 0.35        | 0.37   |
| 51       | 0.49          | 0.52     | 0.83           | 0.81      | 0.34        | 0.36   |
| 52       | 0.49          | 0.52     | 0.84           | 0.81      | 0.34        | 0.36   |
| 53       | 0.48          | 0.51     | 0.84           | 0.82      | 0.33        | 0.35   |
| 54       | 0.47          | 0.50     | 0.85           | 0.82      | 0.32        | 0.35   |
| 55       | 0.47          | 0.50     | 0.85           | 0.83      | 0.32        | 0.35   |
| 56       | 0.46          | 0.49     | 0.86           | 0.83      | 0.31        | 0.34   |
| 57       | 0.45          | 0.48     | 0.86           | 0.84      | 0.31        | 0.33   |
| 58       | 0.44          | 0.47     | 0.87           | 0.84      | 0.30        | 0.32   |
| 59       | 0.44          | 0.46     | 0.87           | 0.85      | 0.30        | 0.32   |
| 60       | 0.43          | 0.46     | 0.88           | 0.85      | 0.29        | 0.32   |
| 61       | 0.42          | 0.45     | 0.88           | 0.86      | 0.28        | 0.31   |
| 62       | 0.41          | 0.44     | 0.89           | 0.86      | 0.27        | 0.30   |
| 63       | 0.40          | 0.43     | 0.89           | 0.87      | 0.27        | 0.29   |

Continued on next page



| $\alpha$ | $\phi_S^\ell$ | $\phi_S$ | $\varphi^\ell$ | $\varphi$ | $\psi^\ell$ | $\psi$ |
|----------|---------------|----------|----------------|-----------|-------------|--------|
| 64       | 0.39          | 0.42     | 0.90           | 0.87      | 0.26        | 0.29   |
| 65       | 0.38          | 0.41     | 0.90           | 0.88      | 0.25        | 0.28   |
| 66       | 0.38          | 0.40     | 0.91           | 0.88      | 0.25        | 0.27   |
| 67       | 0.37          | 0.39     | 0.91           | 0.88      | 0.25        | 0.27   |
| 68       | 0.36          | 0.38     | 0.92           | 0.89      | 0.24        | 0.26   |
| 69       | 0.35          | 0.37     | 0.92           | 0.89      | 0.23        | 0.25   |
| 70       | 0.33          | 0.36     | 0.92           | 0.90      | 0.22        | 0.24   |
| 71       | 0.32          | 0.35     | 0.93           | 0.90      | 0.21        | 0.24   |
| 72       | 0.31          | 0.34     | 0.93           | 0.91      | 0.20        | 0.23   |
| 73       | 0.30          | 0.33     | 0.94           | 0.91      | 0.20        | 0.22   |
| 74       | 0.29          | 0.32     | 0.94           | 0.91      | 0.19        | 0.22   |
| 75       | 0.28          | 0.31     | 0.94           | 0.92      | 0.18        | 0.21   |
| 76       | 0.27          | 0.30     | 0.94           | 0.92      | 0.18        | 0.20   |
| 77       | 0.26          | 0.29     | 0.95           | 0.93      | 0.17        | 0.19   |
| 78       | 0.24          | 0.27     | 0.95           | 0.93      | 0.16        | 0.18   |
| 79       | 0.23          | 0.26     | 0.95           | 0.93      | 0.15        | 0.17   |
| 80       | 0.22          | 0.25     | 0.96           | 0.93      | 0.14        | 0.17   |
| 81       | 0.21          | 0.24     | 0.96           | 0.94      | 0.14        | 0.16   |
| 82       | 0.20          | 0.23     | 0.96           | 0.94      | 0.13        | 0.15   |
| 83       | 0.19          | 0.22     | 0.96           | 0.94      | 0.12        | 0.15   |
| 84       | 0.18          | 0.21     | 0.96           | 0.94      | 0.12        | 0.14   |
| 85       | 0.17          | 0.21     | 0.96           | 0.94      | 0.11        | 0.14   |
| 86       | 0.17          | 0.20     | 0.96           | 0.95      | 0.11        | 0.13   |
| 87       | 0.16          | 0.19     | 0.97           | 0.95      | 0.10        | 0.13   |
| 88       | 0.15          | 0.18     | 0.97           | 0.95      | 0.10        | 0.12   |
| 89       | 0.15          | 0.18     | 0.97           | 0.95      | 0.10        | 0.12   |
| 90       | 0.15          | 0.18     | 0.97           | 0.95      | 0.10        | 0.12   |

Table S104: Reference ( $\phi_S$ ,  $\varphi$ ,  $\psi$ ) and approached ( $\phi_S^\ell$ ,  $\varphi^\ell$ ,  $\psi^\ell$ ) values of the topological descriptors for the first excited-state of the pyridinium-phenolate (PP), computed at the LC-wHPBE/6-31++G(2d,p) level of theory.  $\alpha$  is the pyridinium-phenolate central twist angle amplitude.

| $\alpha$ | $\phi_S^\ell$ | $\phi_S$ | $\varphi^\ell$ | $\varphi$ | $\psi^\ell$ | $\psi$ |
|----------|---------------|----------|----------------|-----------|-------------|--------|
| 0        | 0.62          | 0.68     | 0.69           | 0.65      | 0.47        | 0.51   |
| 1        | 0.62          | 0.68     | 0.69           | 0.65      | 0.47        | 0.51   |
| 2        | 0.62          | 0.68     | 0.69           | 0.65      | 0.47        | 0.51   |
| 3        | 0.62          | 0.68     | 0.69           | 0.65      | 0.47        | 0.51   |
| 4        | 0.62          | 0.68     | 0.69           | 0.65      | 0.47        | 0.51   |
| 5        | 0.62          | 0.68     | 0.69           | 0.65      | 0.47        | 0.51   |
| 6        | 0.62          | 0.68     | 0.69           | 0.65      | 0.47        | 0.51   |
| 7        | 0.62          | 0.68     | 0.69           | 0.66      | 0.47        | 0.51   |
| 8        | 0.62          | 0.67     | 0.69           | 0.66      | 0.47        | 0.50   |
| 9        | 0.62          | 0.67     | 0.69           | 0.66      | 0.47        | 0.50   |
| 10       | 0.62          | 0.67     | 0.69           | 0.66      | 0.47        | 0.50   |
| 11       | 0.62          | 0.67     | 0.69           | 0.66      | 0.47        | 0.50   |
| 12       | 0.61          | 0.67     | 0.70           | 0.66      | 0.46        | 0.50   |
| 13       | 0.61          | 0.67     | 0.70           | 0.66      | 0.46        | 0.50   |
| 14       | 0.61          | 0.67     | 0.70           | 0.67      | 0.46        | 0.50   |
| 15       | 0.61          | 0.67     | 0.70           | 0.67      | 0.46        | 0.50   |
| 16       | 0.61          | 0.66     | 0.70           | 0.67      | 0.46        | 0.50   |
| 17       | 0.61          | 0.66     | 0.70           | 0.67      | 0.46        | 0.50   |
| 18       | 0.61          | 0.66     | 0.71           | 0.68      | 0.45        | 0.49   |
| 19       | 0.61          | 0.66     | 0.71           | 0.68      | 0.45        | 0.49   |
| 20       | 0.61          | 0.66     | 0.71           | 0.68      | 0.45        | 0.49   |
| 21       | 0.60          | 0.65     | 0.71           | 0.68      | 0.45        | 0.49   |
| 22       | 0.60          | 0.65     | 0.72           | 0.69      | 0.44        | 0.48   |
| 23       | 0.60          | 0.65     | 0.72           | 0.69      | 0.44        | 0.48   |
| 24       | 0.60          | 0.65     | 0.72           | 0.69      | 0.44        | 0.48   |
| 25       | 0.60          | 0.64     | 0.73           | 0.69      | 0.44        | 0.48   |
| 26       | 0.59          | 0.64     | 0.73           | 0.70      | 0.43        | 0.47   |
| 27       | 0.59          | 0.64     | 0.73           | 0.70      | 0.43        | 0.47   |
| 28       | 0.59          | 0.63     | 0.73           | 0.70      | 0.43        | 0.47   |
| 29       | 0.59          | 0.63     | 0.74           | 0.71      | 0.43        | 0.46   |
| 30       | 0.59          | 0.63     | 0.74           | 0.71      | 0.43        | 0.46   |
| 31       | 0.58          | 0.62     | 0.74           | 0.72      | 0.42        | 0.45   |

Continued on next page

| $\alpha$ | $\phi_S^\ell$ | $\phi_S$ | $\varphi^\ell$ | $\varphi$ | $\psi^\ell$ | $\psi$ |
|----------|---------------|----------|----------------|-----------|-------------|--------|
| 32       | 0.58          | 0.62     | 0.75           | 0.72      | 0.42        | 0.45   |
| 33       | 0.58          | 0.62     | 0.75           | 0.72      | 0.42        | 0.45   |
| 34       | 0.57          | 0.61     | 0.75           | 0.73      | 0.41        | 0.44   |
| 35       | 0.57          | 0.61     | 0.76           | 0.73      | 0.41        | 0.44   |
| 36       | 0.57          | 0.61     | 0.76           | 0.74      | 0.41        | 0.44   |
| 37       | 0.56          | 0.60     | 0.77           | 0.74      | 0.40        | 0.43   |
| 38       | 0.56          | 0.60     | 0.77           | 0.74      | 0.40        | 0.43   |
| 39       | 0.56          | 0.59     | 0.77           | 0.75      | 0.40        | 0.42   |
| 40       | 0.55          | 0.59     | 0.78           | 0.75      | 0.39        | 0.42   |
| 41       | 0.55          | 0.58     | 0.78           | 0.76      | 0.39        | 0.41   |
| 42       | 0.54          | 0.58     | 0.79           | 0.76      | 0.38        | 0.41   |
| 43       | 0.54          | 0.57     | 0.79           | 0.77      | 0.38        | 0.41   |
| 44       | 0.53          | 0.57     | 0.80           | 0.77      | 0.37        | 0.41   |
| 45       | 0.53          | 0.56     | 0.80           | 0.78      | 0.37        | 0.40   |
| 46       | 0.52          | 0.56     | 0.81           | 0.78      | 0.36        | 0.40   |
| 47       | 0.52          | 0.55     | 0.81           | 0.79      | 0.36        | 0.39   |
| 48       | 0.51          | 0.54     | 0.82           | 0.79      | 0.35        | 0.38   |
| 49       | 0.51          | 0.54     | 0.82           | 0.80      | 0.35        | 0.38   |
| 50       | 0.50          | 0.53     | 0.83           | 0.80      | 0.35        | 0.37   |
| 51       | 0.49          | 0.52     | 0.83           | 0.81      | 0.34        | 0.36   |
| 52       | 0.49          | 0.52     | 0.83           | 0.81      | 0.34        | 0.36   |
| 53       | 0.48          | 0.51     | 0.84           | 0.82      | 0.33        | 0.35   |
| 54       | 0.47          | 0.50     | 0.84           | 0.82      | 0.32        | 0.35   |
| 55       | 0.47          | 0.50     | 0.85           | 0.83      | 0.32        | 0.35   |
| 56       | 0.46          | 0.49     | 0.85           | 0.83      | 0.32        | 0.34   |
| 57       | 0.45          | 0.48     | 0.86           | 0.84      | 0.31        | 0.33   |
| 58       | 0.44          | 0.47     | 0.86           | 0.84      | 0.30        | 0.32   |
| 59       | 0.44          | 0.46     | 0.87           | 0.85      | 0.30        | 0.32   |
| 60       | 0.43          | 0.46     | 0.87           | 0.85      | 0.29        | 0.32   |
| 61       | 0.42          | 0.45     | 0.88           | 0.86      | 0.28        | 0.31   |
| 62       | 0.41          | 0.44     | 0.88           | 0.86      | 0.28        | 0.30   |
| 63       | 0.40          | 0.43     | 0.89           | 0.87      | 0.27        | 0.29   |

Continued on next page

| $\alpha$ | $\phi_S^\ell$ | $\phi_S$ | $\varphi^\ell$ | $\varphi$ | $\psi^\ell$ | $\psi$ |
|----------|---------------|----------|----------------|-----------|-------------|--------|
| 64       | 0.39          | 0.42     | 0.90           | 0.87      | 0.26        | 0.29   |
| 65       | 0.38          | 0.41     | 0.90           | 0.88      | 0.25        | 0.28   |
| 66       | 0.37          | 0.40     | 0.91           | 0.88      | 0.25        | 0.27   |
| 67       | 0.36          | 0.39     | 0.91           | 0.89      | 0.24        | 0.26   |
| 68       | 0.35          | 0.38     | 0.92           | 0.89      | 0.23        | 0.26   |
| 69       | 0.34          | 0.37     | 0.92           | 0.89      | 0.23        | 0.25   |
| 70       | 0.33          | 0.36     | 0.92           | 0.90      | 0.22        | 0.24   |
| 71       | 0.32          | 0.35     | 0.93           | 0.90      | 0.21        | 0.24   |
| 72       | 0.31          | 0.34     | 0.93           | 0.91      | 0.20        | 0.23   |
| 73       | 0.30          | 0.33     | 0.94           | 0.91      | 0.20        | 0.22   |
| 74       | 0.29          | 0.32     | 0.94           | 0.92      | 0.19        | 0.21   |
| 75       | 0.27          | 0.31     | 0.94           | 0.92      | 0.18        | 0.21   |
| 76       | 0.26          | 0.30     | 0.95           | 0.92      | 0.17        | 0.20   |
| 77       | 0.25          | 0.28     | 0.95           | 0.93      | 0.16        | 0.19   |
| 78       | 0.24          | 0.27     | 0.95           | 0.93      | 0.16        | 0.18   |
| 79       | 0.23          | 0.26     | 0.95           | 0.93      | 0.15        | 0.17   |
| 80       | 0.22          | 0.25     | 0.96           | 0.94      | 0.14        | 0.17   |
| 81       | 0.21          | 0.24     | 0.96           | 0.94      | 0.14        | 0.16   |
| 82       | 0.20          | 0.23     | 0.96           | 0.94      | 0.13        | 0.15   |
| 83       | 0.19          | 0.22     | 0.96           | 0.94      | 0.12        | 0.15   |
| 84       | 0.18          | 0.21     | 0.96           | 0.94      | 0.12        | 0.14   |
| 85       | 0.17          | 0.20     | 0.97           | 0.95      | 0.11        | 0.13   |
| 86       | 0.16          | 0.20     | 0.97           | 0.95      | 0.10        | 0.13   |
| 87       | 0.15          | 0.19     | 0.97           | 0.95      | 0.10        | 0.13   |
| 88       | 0.15          | 0.18     | 0.97           | 0.95      | 0.10        | 0.12   |
| 89       | 0.14          | 0.18     | 0.97           | 0.95      | 0.09        | 0.12   |
| 90       | 0.14          | 0.18     | 0.97           | 0.95      | 0.09        | 0.12   |

Table S105: Reference ( $\phi_S$ ,  $\varphi$ ,  $\psi$ ) and approached ( $\phi_S^\ell$ ,  $\varphi^\ell$ ,  $\psi^\ell$ ) values of the topological descriptors for the first excited-state of the pyridinium-phenolate (PP), computed at the LC-wHPBE/6-31++G(d,p) level of theory.  $\alpha$  is the pyridinium-phenolate central twist angle amplitude.

| $\alpha$ | $\phi_S^\ell$ | $\phi_S$ | $\varphi^\ell$ | $\varphi$ | $\psi^\ell$ | $\psi$ |
|----------|---------------|----------|----------------|-----------|-------------|--------|
| 0        | 0.62          | 0.68     | 0.69           | 0.65      | 0.47        | 0.51   |
| 0        | 0.65          | 0.62     | 0.68           | 1.00      | 0.49        | 0.35   |
| 1        | 0.65          | 0.62     | 0.68           | 2.00      | 0.49        | 0.19   |
| 2        | 0.65          | 0.62     | 0.68           | 3.00      | 0.49        | 0.13   |
| 3        | 0.65          | 0.62     | 0.68           | 4.00      | 0.49        | 0.10   |
| 4        | 0.65          | 0.62     | 0.68           | 5.00      | 0.49        | 0.08   |
| 5        | 0.65          | 0.62     | 0.68           | 6.00      | 0.49        | 0.07   |
| 6        | 0.65          | 0.62     | 0.68           | 7.00      | 0.49        | 0.06   |
| 7        | 0.66          | 0.62     | 0.68           | 8.00      | 0.49        | 0.05   |
| 8        | 0.66          | 0.62     | 0.67           | 9.00      | 0.49        | 0.04   |
| 9        | 0.66          | 0.62     | 0.67           | 10.00     | 0.49        | 0.04   |
| 10       | 0.66          | 0.62     | 0.67           | 11.00     | 0.49        | 0.04   |
| 11       | 0.66          | 0.61     | 0.67           | 12.00     | 0.50        | 0.03   |
| 12       | 0.66          | 0.61     | 0.67           | 13.00     | 0.50        | 0.03   |
| 13       | 0.66          | 0.61     | 0.67           | 14.00     | 0.50        | 0.03   |
| 14       | 0.67          | 0.61     | 0.67           | 15.00     | 0.50        | 0.03   |
| 15       | 0.67          | 0.61     | 0.67           | 16.00     | 0.50        | 0.02   |
| 16       | 0.67          | 0.61     | 0.66           | 17.00     | 0.50        | 0.02   |
| 17       | 0.67          | 0.61     | 0.66           | 18.00     | 0.50        | 0.02   |
| 18       | 0.68          | 0.61     | 0.66           | 19.00     | 0.51        | 0.02   |
| 19       | 0.68          | 0.61     | 0.66           | 20.00     | 0.51        | 0.02   |
| 20       | 0.68          | 0.60     | 0.66           | 21.00     | 0.51        | 0.02   |
| 21       | 0.68          | 0.60     | 0.65           | 22.00     | 0.51        | 0.02   |
| 22       | 0.69          | 0.60     | 0.65           | 23.00     | 0.52        | 0.02   |
| 23       | 0.69          | 0.60     | 0.65           | 24.00     | 0.52        | 0.02   |
| 24       | 0.69          | 0.60     | 0.65           | 25.00     | 0.52        | 0.02   |
| 25       | 0.69          | 0.59     | 0.64           | 26.00     | 0.52        | 0.01   |
| 26       | 0.70          | 0.59     | 0.64           | 27.00     | 0.53        | 0.01   |
| 27       | 0.70          | 0.59     | 0.64           | 28.00     | 0.53        | 0.01   |
| 28       | 0.70          | 0.59     | 0.64           | 29.00     | 0.53        | 0.01   |
| 29       | 0.71          | 0.59     | 0.63           | 30.00     | 0.54        | 0.01   |
| 30       | 0.71          | 0.58     | 0.63           | 31.00     | 0.54        | 0.01   |

Continued on next page

| $\alpha$ | $\phi_S^\ell$ | $\phi_S$ | $\varphi^\ell$ | $\varphi$ | $\psi^\ell$ | $\psi$ |
|----------|---------------|----------|----------------|-----------|-------------|--------|
| 31       | 0.72          | 0.58     | 0.62           | 32.00     | 0.54        | 0.01   |
| 32       | 0.72          | 0.58     | 0.62           | 33.00     | 0.55        | 0.01   |
| 33       | 0.72          | 0.57     | 0.62           | 34.00     | 0.55        | 0.01   |
| 34       | 0.73          | 0.57     | 0.61           | 35.00     | 0.55        | 0.01   |
| 35       | 0.73          | 0.57     | 0.61           | 36.00     | 0.56        | 0.01   |
| 36       | 0.74          | 0.56     | 0.61           | 37.00     | 0.56        | 0.01   |
| 37       | 0.74          | 0.56     | 0.60           | 38.00     | 0.57        | 0.01   |
| 38       | 0.74          | 0.56     | 0.60           | 39.00     | 0.57        | 0.01   |
| 39       | 0.75          | 0.55     | 0.59           | 40.00     | 0.57        | 0.01   |
| 40       | 0.75          | 0.55     | 0.59           | 41.00     | 0.58        | 0.01   |
| 41       | 0.76          | 0.54     | 0.58           | 42.00     | 0.58        | 0.01   |
| 42       | 0.76          | 0.54     | 0.58           | 43.00     | 0.59        | 0.01   |
| 43       | 0.77          | 0.53     | 0.57           | 44.00     | 0.59        | 0.01   |
| 44       | 0.77          | 0.53     | 0.57           | 45.00     | 0.60        | 0.01   |
| 45       | 0.78          | 0.52     | 0.56           | 46.00     | 0.60        | 0.01   |
| 46       | 0.78          | 0.52     | 0.56           | 47.00     | 0.61        | 0.01   |
| 47       | 0.79          | 0.51     | 0.55           | 48.00     | 0.61        | 0.01   |
| 48       | 0.79          | 0.50     | 0.54           | 49.00     | 0.62        | 0.01   |
| 49       | 0.80          | 0.50     | 0.54           | 50.00     | 0.62        | 0.01   |
| 50       | 0.80          | 0.49     | 0.53           | 51.00     | 0.63        | 0.01   |
| 51       | 0.81          | 0.49     | 0.52           | 52.00     | 0.63        | 0.01   |
| 52       | 0.81          | 0.48     | 0.52           | 53.00     | 0.64        | 0.01   |
| 53       | 0.82          | 0.47     | 0.51           | 54.00     | 0.64        | 0.01   |
| 54       | 0.82          | 0.47     | 0.50           | 55.00     | 0.65        | 0.01   |
| 55       | 0.83          | 0.46     | 0.50           | 56.00     | 0.66        | 0.01   |
| 56       | 0.83          | 0.45     | 0.49           | 57.00     | 0.66        | 0.01   |
| 57       | 0.84          | 0.44     | 0.48           | 58.00     | 0.67        | 0.00   |
| 58       | 0.84          | 0.44     | 0.47           | 59.00     | 0.67        | 0.00   |
| 59       | 0.85          | 0.43     | 0.46           | 60.00     | 0.68        | 0.00   |
| 60       | 0.85          | 0.42     | 0.46           | 61.00     | 0.69        | 0.00   |
| 61       | 0.86          | 0.41     | 0.45           | 62.00     | 0.69        | 0.00   |
| 62       | 0.86          | 0.40     | 0.44           | 63.00     | 0.70        | 0.00   |

Continued on next page

| $\alpha$ | $\phi_S^\ell$ | $\phi_S$ | $\varphi^\ell$ | $\varphi$ | $\psi^\ell$ | $\psi$ |
|----------|---------------|----------|----------------|-----------|-------------|--------|
| 63       | 0.87          | 0.39     | 0.43           | 64.00     | 0.71        | 0.00   |
| 64       | 0.87          | 0.38     | 0.42           | 65.00     | 0.71        | 0.00   |
| 65       | 0.88          | 0.37     | 0.41           | 66.00     | 0.72        | 0.00   |
| 66       | 0.88          | 0.36     | 0.40           | 67.00     | 0.73        | 0.00   |
| 67       | 0.89          | 0.35     | 0.39           | 68.00     | 0.74        | 0.00   |
| 68       | 0.89          | 0.34     | 0.38           | 69.00     | 0.74        | 0.00   |
| 69       | 0.89          | 0.33     | 0.37           | 70.00     | 0.75        | 0.00   |
| 70       | 0.90          | 0.32     | 0.36           | 71.00     | 0.76        | 0.00   |
| 71       | 0.90          | 0.31     | 0.35           | 72.00     | 0.76        | 0.00   |
| 72       | 0.91          | 0.30     | 0.34           | 73.00     | 0.77        | 0.00   |
| 73       | 0.91          | 0.29     | 0.33           | 74.00     | 0.78        | 0.00   |
| 74       | 0.92          | 0.27     | 0.32           | 75.00     | 0.79        | 0.00   |
| 75       | 0.92          | 0.26     | 0.31           | 76.00     | 0.79        | 0.00   |
| 76       | 0.92          | 0.25     | 0.30           | 77.00     | 0.80        | 0.00   |
| 77       | 0.93          | 0.24     | 0.28           | 78.00     | 0.81        | 0.00   |
| 78       | 0.93          | 0.23     | 0.27           | 79.00     | 0.82        | 0.00   |
| 79       | 0.93          | 0.22     | 0.26           | 80.00     | 0.82        | 0.00   |
| 80       | 0.94          | 0.21     | 0.25           | 81.00     | 0.83        | 0.00   |
| 81       | 0.94          | 0.20     | 0.24           | 82.00     | 0.84        | 0.00   |
| 82       | 0.94          | 0.19     | 0.23           | 83.00     | 0.85        | 0.00   |
| 83       | 0.94          | 0.18     | 0.22           | 84.00     | 0.85        | 0.00   |
| 84       | 0.94          | 0.17     | 0.21           | 85.00     | 0.86        | 0.00   |
| 85       | 0.95          | 0.16     | 0.20           | 86.00     | 0.86        | 0.00   |
| 86       | 0.95          | 0.16     | 0.20           | 87.00     | 0.87        | 0.00   |
| 87       | 0.95          | 0.15     | 0.19           | 88.00     | 0.87        | 0.00   |
| 88       | 0.95          | 0.14     | 0.18           | 89.00     | 0.88        | 0.00   |
| 89       | 0.95          | 0.14     | 0.18           | 90.00     | 0.88        | 0.00   |

Table S106: Reference  $(\phi_S, \varphi, \psi)$  and approached  $(\phi_S^\ell, \varphi^\ell, \psi^\ell)$  values of the topological descriptors for the first excited-state of the pyridinium-phenolate (PP), computed at the LC-wHPBE/6-31+G(d,p) level of theory.  $\alpha$  is the pyridinium-phenolate central twist angle amplitude.

| $\alpha$ | $\phi_S^\ell$ | $\phi_S$ | $\varphi^\ell$ | $\varphi$ | $\psi^\ell$ | $\psi$ |
|----------|---------------|----------|----------------|-----------|-------------|--------|
| 0        | 0.62          | 0.68     | 0.69           | 0.65      | 0.47        | 0.51   |
| 1        | 0.62          | 0.68     | 0.69           | 0.65      | 0.47        | 0.51   |
| 2        | 0.62          | 0.68     | 0.69           | 0.65      | 0.47        | 0.51   |
| 3        | 0.62          | 0.68     | 0.69           | 0.65      | 0.47        | 0.51   |
| 4        | 0.62          | 0.68     | 0.69           | 0.65      | 0.47        | 0.51   |
| 5        | 0.62          | 0.68     | 0.69           | 0.65      | 0.47        | 0.51   |
| 6        | 0.62          | 0.68     | 0.69           | 0.66      | 0.47        | 0.51   |
| 7        | 0.62          | 0.68     | 0.69           | 0.66      | 0.47        | 0.51   |
| 8        | 0.62          | 0.67     | 0.69           | 0.66      | 0.47        | 0.50   |
| 9        | 0.62          | 0.67     | 0.69           | 0.66      | 0.47        | 0.50   |
| 10       | 0.62          | 0.67     | 0.69           | 0.66      | 0.47        | 0.50   |
| 11       | 0.62          | 0.67     | 0.70           | 0.66      | 0.46        | 0.50   |
| 12       | 0.61          | 0.67     | 0.70           | 0.66      | 0.46        | 0.50   |
| 13       | 0.61          | 0.67     | 0.70           | 0.67      | 0.46        | 0.50   |
| 14       | 0.61          | 0.67     | 0.70           | 0.67      | 0.46        | 0.50   |
| 15       | 0.61          | 0.67     | 0.70           | 0.67      | 0.46        | 0.50   |
| 16       | 0.61          | 0.66     | 0.70           | 0.67      | 0.46        | 0.50   |
| 17       | 0.61          | 0.66     | 0.70           | 0.67      | 0.46        | 0.50   |
| 18       | 0.61          | 0.66     | 0.71           | 0.68      | 0.45        | 0.49   |
| 19       | 0.61          | 0.66     | 0.71           | 0.68      | 0.45        | 0.49   |
| 20       | 0.61          | 0.66     | 0.71           | 0.68      | 0.45        | 0.49   |
| 21       | 0.60          | 0.65     | 0.71           | 0.68      | 0.45        | 0.49   |
| 22       | 0.60          | 0.65     | 0.72           | 0.69      | 0.44        | 0.48   |
| 23       | 0.60          | 0.65     | 0.72           | 0.69      | 0.44        | 0.48   |
| 24       | 0.60          | 0.65     | 0.72           | 0.69      | 0.44        | 0.48   |
| 25       | 0.60          | 0.64     | 0.73           | 0.70      | 0.44        | 0.47   |
| 26       | 0.59          | 0.64     | 0.73           | 0.70      | 0.43        | 0.47   |
| 27       | 0.59          | 0.64     | 0.73           | 0.70      | 0.43        | 0.47   |
| 28       | 0.59          | 0.63     | 0.74           | 0.70      | 0.43        | 0.47   |
| 29       | 0.59          | 0.63     | 0.74           | 0.71      | 0.43        | 0.46   |
| 30       | 0.59          | 0.63     | 0.74           | 0.71      | 0.43        | 0.46   |
| 31       | 0.58          | 0.62     | 0.74           | 0.72      | 0.42        | 0.45   |

Continued on next page



| $\alpha$ | $\phi_S^\ell$ | $\phi_S$ | $\varphi^\ell$ | $\varphi$ | $\psi^\ell$ | $\psi$ |
|----------|---------------|----------|----------------|-----------|-------------|--------|
| 32       | 0.58          | 0.62     | 0.75           | 0.72      | 0.42        | 0.45   |
| 33       | 0.58          | 0.62     | 0.75           | 0.72      | 0.42        | 0.45   |
| 34       | 0.57          | 0.61     | 0.75           | 0.73      | 0.41        | 0.44   |
| 35       | 0.57          | 0.61     | 0.76           | 0.73      | 0.41        | 0.44   |
| 36       | 0.57          | 0.61     | 0.76           | 0.74      | 0.41        | 0.44   |
| 37       | 0.56          | 0.60     | 0.77           | 0.74      | 0.40        | 0.43   |
| 38       | 0.56          | 0.60     | 0.77           | 0.74      | 0.40        | 0.43   |
| 39       | 0.56          | 0.59     | 0.78           | 0.75      | 0.40        | 0.42   |
| 40       | 0.55          | 0.59     | 0.78           | 0.75      | 0.39        | 0.42   |
| 41       | 0.55          | 0.58     | 0.78           | 0.76      | 0.39        | 0.41   |
| 42       | 0.54          | 0.58     | 0.79           | 0.76      | 0.38        | 0.41   |
| 43       | 0.54          | 0.57     | 0.79           | 0.77      | 0.38        | 0.41   |
| 44       | 0.53          | 0.57     | 0.80           | 0.77      | 0.37        | 0.41   |
| 45       | 0.53          | 0.56     | 0.80           | 0.78      | 0.37        | 0.40   |
| 46       | 0.52          | 0.56     | 0.81           | 0.78      | 0.36        | 0.40   |
| 47       | 0.52          | 0.55     | 0.81           | 0.79      | 0.36        | 0.39   |
| 48       | 0.51          | 0.54     | 0.82           | 0.79      | 0.35        | 0.38   |
| 49       | 0.50          | 0.54     | 0.82           | 0.80      | 0.35        | 0.38   |
| 50       | 0.50          | 0.53     | 0.83           | 0.80      | 0.35        | 0.37   |
| 51       | 0.49          | 0.52     | 0.83           | 0.81      | 0.34        | 0.36   |
| 52       | 0.49          | 0.52     | 0.84           | 0.81      | 0.34        | 0.36   |
| 53       | 0.48          | 0.51     | 0.84           | 0.82      | 0.33        | 0.35   |
| 54       | 0.47          | 0.50     | 0.84           | 0.82      | 0.32        | 0.35   |
| 55       | 0.47          | 0.50     | 0.85           | 0.83      | 0.32        | 0.35   |
| 56       | 0.46          | 0.49     | 0.85           | 0.83      | 0.32        | 0.34   |
| 57       | 0.45          | 0.48     | 0.86           | 0.84      | 0.31        | 0.33   |
| 58       | 0.44          | 0.47     | 0.86           | 0.84      | 0.30        | 0.32   |
| 59       | 0.43          | 0.46     | 0.87           | 0.85      | 0.29        | 0.32   |
| 60       | 0.43          | 0.46     | 0.87           | 0.85      | 0.29        | 0.32   |
| 61       | 0.42          | 0.45     | 0.88           | 0.86      | 0.28        | 0.31   |
| 62       | 0.41          | 0.44     | 0.88           | 0.86      | 0.28        | 0.30   |
| 63       | 0.40          | 0.43     | 0.89           | 0.87      | 0.27        | 0.29   |

Continued on next page

| $\alpha$ | $\phi_S^\ell$ | $\phi_S$ | $\varphi^\ell$ | $\varphi$ | $\psi^\ell$ | $\psi$ |
|----------|---------------|----------|----------------|-----------|-------------|--------|
| 64       | 0.39          | 0.42     | 0.90           | 0.87      | 0.26        | 0.29   |
| 65       | 0.38          | 0.41     | 0.90           | 0.88      | 0.25        | 0.28   |
| 66       | 0.37          | 0.40     | 0.91           | 0.88      | 0.25        | 0.27   |
| 67       | 0.36          | 0.39     | 0.91           | 0.89      | 0.24        | 0.26   |
| 68       | 0.35          | 0.38     | 0.92           | 0.89      | 0.23        | 0.26   |
| 69       | 0.34          | 0.37     | 0.92           | 0.89      | 0.23        | 0.25   |
| 70       | 0.33          | 0.36     | 0.92           | 0.90      | 0.22        | 0.24   |
| 71       | 0.32          | 0.35     | 0.93           | 0.90      | 0.21        | 0.24   |
| 72       | 0.31          | 0.34     | 0.93           | 0.91      | 0.20        | 0.23   |
| 73       | 0.30          | 0.33     | 0.94           | 0.91      | 0.20        | 0.22   |
| 74       | 0.29          | 0.32     | 0.94           | 0.92      | 0.19        | 0.21   |
| 75       | 0.27          | 0.31     | 0.94           | 0.92      | 0.18        | 0.21   |
| 76       | 0.26          | 0.30     | 0.95           | 0.92      | 0.17        | 0.20   |
| 77       | 0.25          | 0.28     | 0.95           | 0.93      | 0.16        | 0.19   |
| 78       | 0.24          | 0.27     | 0.95           | 0.93      | 0.16        | 0.18   |
| 79       | 0.23          | 0.26     | 0.95           | 0.93      | 0.15        | 0.17   |
| 80       | 0.22          | 0.25     | 0.96           | 0.94      | 0.14        | 0.17   |
| 81       | 0.21          | 0.24     | 0.96           | 0.94      | 0.14        | 0.16   |
| 82       | 0.20          | 0.23     | 0.96           | 0.94      | 0.13        | 0.15   |
| 83       | 0.19          | 0.22     | 0.96           | 0.94      | 0.12        | 0.15   |
| 84       | 0.18          | 0.21     | 0.96           | 0.94      | 0.12        | 0.14   |
| 85       | 0.17          | 0.20     | 0.97           | 0.95      | 0.11        | 0.13   |
| 86       | 0.16          | 0.20     | 0.97           | 0.95      | 0.10        | 0.13   |
| 87       | 0.16          | 0.19     | 0.97           | 0.95      | 0.10        | 0.13   |
| 88       | 0.15          | 0.18     | 0.97           | 0.95      | 0.10        | 0.12   |
| 89       | 0.14          | 0.18     | 0.97           | 0.95      | 0.09        | 0.12   |
| 90       | 0.14          | 0.18     | 0.97           | 0.95      | 0.09        | 0.12   |

Table S107: Reference ( $\phi_S$ ,  $\varphi$ ,  $\psi$ ) and approached ( $\phi_S^\ell$ ,  $\varphi^\ell$ ,  $\psi^\ell$ ) values of the topological descriptors for the first excited-state of the pyridinium-phenolate (PP), computed at the LC-wHPBE/6-31+G(d) level of theory.  $\alpha$  is the pyridinium-phenolate central twist angle amplitude.

| $\alpha$ | $\phi_S^\ell$ | $\phi_S$ | $\varphi^\ell$ | $\varphi$ | $\psi^\ell$ | $\psi$ |
|----------|---------------|----------|----------------|-----------|-------------|--------|
| 0        | 0.65          | 0.70     | 0.68           | 0.64      | 0.49        | 0.53   |
| 1        | 0.65          | 0.70     | 0.68           | 0.64      | 0.49        | 0.53   |
| 2        | 0.65          | 0.70     | 0.68           | 0.64      | 0.49        | 0.53   |
| 3        | 0.65          | 0.70     | 0.68           | 0.64      | 0.49        | 0.53   |
| 4        | 0.65          | 0.70     | 0.68           | 0.64      | 0.49        | 0.53   |
| 5        | 0.65          | 0.70     | 0.68           | 0.64      | 0.49        | 0.53   |
| 6        | 0.64          | 0.70     | 0.68           | 0.64      | 0.48        | 0.53   |
| 7        | 0.64          | 0.70     | 0.68           | 0.64      | 0.48        | 0.53   |
| 8        | 0.64          | 0.69     | 0.68           | 0.64      | 0.48        | 0.52   |
| 9        | 0.64          | 0.69     | 0.68           | 0.64      | 0.48        | 0.52   |
| 10       | 0.64          | 0.69     | 0.69           | 0.64      | 0.48        | 0.52   |
| 11       | 0.64          | 0.69     | 0.69           | 0.65      | 0.48        | 0.52   |
| 12       | 0.64          | 0.69     | 0.69           | 0.65      | 0.48        | 0.52   |
| 13       | 0.64          | 0.69     | 0.69           | 0.65      | 0.48        | 0.52   |
| 14       | 0.64          | 0.69     | 0.69           | 0.65      | 0.48        | 0.52   |
| 15       | 0.64          | 0.69     | 0.69           | 0.65      | 0.48        | 0.52   |
| 16       | 0.64          | 0.68     | 0.69           | 0.66      | 0.48        | 0.51   |
| 17       | 0.63          | 0.68     | 0.70           | 0.66      | 0.47        | 0.51   |
| 18       | 0.63          | 0.68     | 0.70           | 0.66      | 0.47        | 0.51   |
| 19       | 0.63          | 0.68     | 0.70           | 0.66      | 0.47        | 0.51   |
| 20       | 0.63          | 0.68     | 0.70           | 0.67      | 0.47        | 0.50   |
| 21       | 0.63          | 0.67     | 0.71           | 0.67      | 0.46        | 0.50   |
| 22       | 0.63          | 0.67     | 0.71           | 0.67      | 0.46        | 0.50   |
| 23       | 0.62          | 0.67     | 0.71           | 0.67      | 0.46        | 0.50   |
| 24       | 0.62          | 0.67     | 0.71           | 0.68      | 0.46        | 0.50   |
| 25       | 0.62          | 0.66     | 0.72           | 0.68      | 0.45        | 0.49   |
| 26       | 0.62          | 0.66     | 0.72           | 0.68      | 0.45        | 0.49   |
| 27       | 0.62          | 0.66     | 0.72           | 0.69      | 0.45        | 0.49   |
| 28       | 0.61          | 0.66     | 0.73           | 0.69      | 0.44        | 0.49   |
| 29       | 0.61          | 0.65     | 0.73           | 0.69      | 0.44        | 0.48   |
| 30       | 0.61          | 0.65     | 0.73           | 0.70      | 0.44        | 0.48   |
| 31       | 0.61          | 0.65     | 0.74           | 0.70      | 0.44        | 0.48   |

Continued on next page

| $\alpha$ | $\phi_S^\ell$ | $\phi_S$ | $\varphi^\ell$ | $\varphi$ | $\psi^\ell$ | $\psi$ |
|----------|---------------|----------|----------------|-----------|-------------|--------|
| 32       | 0.61          | 0.64     | 0.74           | 0.71      | 0.44        | 0.47   |
| 33       | 0.60          | 0.64     | 0.74           | 0.71      | 0.43        | 0.47   |
| 34       | 0.60          | 0.63     | 0.75           | 0.71      | 0.43        | 0.46   |
| 35       | 0.60          | 0.63     | 0.75           | 0.72      | 0.43        | 0.46   |
| 36       | 0.59          | 0.63     | 0.75           | 0.72      | 0.42        | 0.46   |
| 37       | 0.59          | 0.62     | 0.76           | 0.73      | 0.42        | 0.45   |
| 38       | 0.59          | 0.62     | 0.76           | 0.73      | 0.42        | 0.45   |
| 39       | 0.58          | 0.61     | 0.77           | 0.74      | 0.41        | 0.44   |
| 40       | 0.58          | 0.61     | 0.77           | 0.74      | 0.41        | 0.44   |
| 41       | 0.57          | 0.60     | 0.78           | 0.74      | 0.40        | 0.43   |
| 42       | 0.57          | 0.60     | 0.78           | 0.75      | 0.40        | 0.43   |
| 43       | 0.56          | 0.59     | 0.79           | 0.75      | 0.39        | 0.42   |
| 44       | 0.56          | 0.59     | 0.79           | 0.76      | 0.39        | 0.42   |
| 45       | 0.55          | 0.58     | 0.80           | 0.76      | 0.38        | 0.41   |
| 46       | 0.55          | 0.58     | 0.80           | 0.77      | 0.38        | 0.41   |
| 47       | 0.54          | 0.57     | 0.80           | 0.77      | 0.38        | 0.41   |
| 48       | 0.54          | 0.57     | 0.81           | 0.78      | 0.37        | 0.40   |
| 49       | 0.53          | 0.56     | 0.81           | 0.78      | 0.37        | 0.40   |
| 50       | 0.53          | 0.55     | 0.82           | 0.79      | 0.37        | 0.39   |
| 51       | 0.52          | 0.55     | 0.82           | 0.79      | 0.36        | 0.39   |
| 52       | 0.51          | 0.54     | 0.83           | 0.80      | 0.35        | 0.38   |
| 53       | 0.51          | 0.53     | 0.83           | 0.80      | 0.35        | 0.37   |
| 54       | 0.50          | 0.53     | 0.84           | 0.81      | 0.34        | 0.37   |
| 55       | 0.49          | 0.52     | 0.84           | 0.82      | 0.34        | 0.36   |
| 56       | 0.48          | 0.51     | 0.85           | 0.82      | 0.33        | 0.35   |
| 57       | 0.48          | 0.50     | 0.85           | 0.83      | 0.33        | 0.35   |
| 58       | 0.47          | 0.49     | 0.86           | 0.83      | 0.32        | 0.34   |
| 59       | 0.46          | 0.49     | 0.86           | 0.84      | 0.31        | 0.34   |
| 60       | 0.45          | 0.48     | 0.87           | 0.84      | 0.30        | 0.33   |
| 61       | 0.44          | 0.47     | 0.87           | 0.85      | 0.30        | 0.32   |
| 62       | 0.44          | 0.46     | 0.88           | 0.85      | 0.30        | 0.32   |
| 63       | 0.43          | 0.45     | 0.88           | 0.86      | 0.29        | 0.31   |

Continued on next page

| $\alpha$ | $\phi_S^\ell$ | $\phi_S$ | $\varphi^\ell$ | $\varphi$ | $\psi^\ell$ | $\psi$ |
|----------|---------------|----------|----------------|-----------|-------------|--------|
| 64       | 0.42          | 0.44     | 0.89           | 0.86      | 0.28        | 0.30   |
| 65       | 0.41          | 0.43     | 0.89           | 0.87      | 0.27        | 0.29   |
| 66       | 0.40          | 0.42     | 0.90           | 0.87      | 0.27        | 0.29   |
| 67       | 0.39          | 0.41     | 0.90           | 0.88      | 0.26        | 0.28   |
| 68       | 0.38          | 0.40     | 0.91           | 0.88      | 0.25        | 0.27   |
| 69       | 0.36          | 0.39     | 0.91           | 0.89      | 0.24        | 0.26   |
| 70       | 0.35          | 0.38     | 0.92           | 0.89      | 0.23        | 0.26   |
| 71       | 0.34          | 0.37     | 0.92           | 0.90      | 0.23        | 0.25   |
| 72       | 0.33          | 0.36     | 0.93           | 0.90      | 0.22        | 0.24   |
| 73       | 0.32          | 0.35     | 0.93           | 0.91      | 0.21        | 0.23   |
| 74       | 0.30          | 0.33     | 0.94           | 0.91      | 0.20        | 0.22   |
| 75       | 0.29          | 0.32     | 0.94           | 0.92      | 0.19        | 0.21   |
| 76       | 0.28          | 0.31     | 0.95           | 0.92      | 0.18        | 0.21   |
| 77       | 0.26          | 0.30     | 0.95           | 0.92      | 0.17        | 0.20   |
| 78       | 0.25          | 0.29     | 0.95           | 0.93      | 0.16        | 0.19   |
| 79       | 0.24          | 0.27     | 0.96           | 0.93      | 0.16        | 0.18   |
| 80       | 0.22          | 0.26     | 0.96           | 0.93      | 0.14        | 0.17   |
| 81       | 0.21          | 0.25     | 0.96           | 0.94      | 0.14        | 0.17   |
| 82       | 0.20          | 0.24     | 0.96           | 0.94      | 0.13        | 0.16   |
| 83       | 0.19          | 0.23     | 0.97           | 0.94      | 0.12        | 0.15   |
| 84       | 0.17          | 0.22     | 0.97           | 0.94      | 0.11        | 0.15   |
| 85       | 0.16          | 0.21     | 0.97           | 0.95      | 0.10        | 0.14   |
| 86       | 0.15          | 0.20     | 0.97           | 0.95      | 0.10        | 0.13   |
| 87       | 0.14          | 0.19     | 0.97           | 0.95      | 0.09        | 0.13   |
| 88       | 0.14          | 0.18     | 0.97           | 0.95      | 0.09        | 0.12   |
| 89       | 0.13          | 0.18     | 0.97           | 0.95      | 0.08        | 0.12   |
| 90       | 0.13          | 0.17     | 0.97           | 0.95      | 0.08        | 0.11   |

Table S108: Reference ( $\phi_S$ ,  $\varphi$ ,  $\psi$ ) and approached ( $\phi_S^\ell$ ,  $\varphi^\ell$ ,  $\psi^\ell$ ) values of the topological descriptors for the first excited-state of the pyridinium-phenolate (PP), computed at the LC-wHPBE/6-31G(d) level of theory.  $\alpha$  is the pyridinium-phenolate central twist angle amplitude.

| $\alpha$ | $\phi_S^\ell$ | $\phi_S$ | $\varphi^\ell$ | $\varphi$ | $\psi^\ell$ | $\psi$ |
|----------|---------------|----------|----------------|-----------|-------------|--------|
| 0        | 0.62          | 0.67     | 0.69           | 0.66      | 0.47        | 0.50   |
| 1        | 0.62          | 0.67     | 0.69           | 0.66      | 0.47        | 0.50   |
| 2        | 0.62          | 0.67     | 0.69           | 0.66      | 0.47        | 0.50   |
| 3        | 0.62          | 0.67     | 0.69           | 0.66      | 0.47        | 0.50   |
| 4        | 0.62          | 0.67     | 0.69           | 0.66      | 0.47        | 0.50   |
| 5        | 0.62          | 0.67     | 0.69           | 0.66      | 0.47        | 0.50   |
| 6        | 0.62          | 0.67     | 0.69           | 0.66      | 0.47        | 0.50   |
| 7        | 0.62          | 0.67     | 0.69           | 0.66      | 0.47        | 0.50   |
| 8        | 0.62          | 0.67     | 0.69           | 0.66      | 0.47        | 0.50   |
| 9        | 0.62          | 0.67     | 0.69           | 0.67      | 0.47        | 0.50   |
| 10       | 0.61          | 0.66     | 0.69           | 0.67      | 0.46        | 0.50   |
| 11       | 0.61          | 0.66     | 0.70           | 0.67      | 0.46        | 0.50   |
| 12       | 0.61          | 0.66     | 0.70           | 0.67      | 0.46        | 0.50   |
| 13       | 0.61          | 0.66     | 0.70           | 0.67      | 0.46        | 0.50   |
| 14       | 0.61          | 0.66     | 0.70           | 0.67      | 0.46        | 0.50   |
| 15       | 0.61          | 0.66     | 0.70           | 0.68      | 0.46        | 0.49   |
| 16       | 0.61          | 0.66     | 0.70           | 0.68      | 0.46        | 0.49   |
| 17       | 0.61          | 0.65     | 0.71           | 0.68      | 0.45        | 0.49   |
| 18       | 0.61          | 0.65     | 0.71           | 0.68      | 0.45        | 0.49   |
| 19       | 0.61          | 0.65     | 0.71           | 0.68      | 0.45        | 0.49   |
| 20       | 0.60          | 0.65     | 0.71           | 0.69      | 0.45        | 0.48   |
| 21       | 0.60          | 0.65     | 0.72           | 0.69      | 0.44        | 0.48   |
| 22       | 0.60          | 0.64     | 0.72           | 0.69      | 0.44        | 0.48   |
| 23       | 0.60          | 0.64     | 0.72           | 0.69      | 0.44        | 0.48   |
| 24       | 0.60          | 0.64     | 0.72           | 0.70      | 0.44        | 0.47   |
| 25       | 0.59          | 0.64     | 0.73           | 0.70      | 0.43        | 0.47   |
| 26       | 0.59          | 0.63     | 0.73           | 0.70      | 0.43        | 0.47   |
| 27       | 0.59          | 0.63     | 0.73           | 0.71      | 0.43        | 0.46   |
| 28       | 0.59          | 0.63     | 0.74           | 0.71      | 0.43        | 0.46   |
| 29       | 0.59          | 0.62     | 0.74           | 0.71      | 0.43        | 0.46   |
| 30       | 0.58          | 0.62     | 0.74           | 0.72      | 0.42        | 0.45   |
| 31       | 0.58          | 0.62     | 0.75           | 0.72      | 0.42        | 0.45   |

Continued on next page

| $\alpha$ | $\phi_S^\ell$ | $\phi_S$ | $\varphi^\ell$ | $\varphi$ | $\psi^\ell$ | $\psi$ |
|----------|---------------|----------|----------------|-----------|-------------|--------|
| 32       | 0.58          | 0.61     | 0.75           | 0.73      | 0.42        | 0.44   |
| 33       | 0.58          | 0.61     | 0.75           | 0.73      | 0.42        | 0.44   |
| 34       | 0.57          | 0.61     | 0.76           | 0.73      | 0.41        | 0.44   |
| 35       | 0.57          | 0.60     | 0.76           | 0.74      | 0.41        | 0.43   |
| 36       | 0.57          | 0.60     | 0.76           | 0.74      | 0.41        | 0.43   |
| 37       | 0.56          | 0.60     | 0.77           | 0.75      | 0.40        | 0.43   |
| 38       | 0.56          | 0.59     | 0.77           | 0.75      | 0.40        | 0.42   |
| 39       | 0.55          | 0.59     | 0.78           | 0.75      | 0.39        | 0.42   |
| 40       | 0.55          | 0.58     | 0.78           | 0.76      | 0.39        | 0.41   |
| 41       | 0.55          | 0.58     | 0.79           | 0.76      | 0.39        | 0.41   |
| 42       | 0.54          | 0.57     | 0.79           | 0.77      | 0.38        | 0.41   |
| 43       | 0.54          | 0.57     | 0.80           | 0.77      | 0.38        | 0.41   |
| 44       | 0.53          | 0.56     | 0.80           | 0.78      | 0.37        | 0.40   |
| 45       | 0.53          | 0.56     | 0.80           | 0.78      | 0.37        | 0.40   |
| 46       | 0.52          | 0.55     | 0.81           | 0.79      | 0.36        | 0.39   |
| 47       | 0.51          | 0.55     | 0.81           | 0.79      | 0.36        | 0.39   |
| 48       | 0.51          | 0.54     | 0.82           | 0.80      | 0.35        | 0.38   |
| 49       | 0.50          | 0.53     | 0.82           | 0.80      | 0.35        | 0.37   |
| 50       | 0.50          | 0.53     | 0.83           | 0.81      | 0.35        | 0.37   |
| 51       | 0.49          | 0.52     | 0.83           | 0.81      | 0.34        | 0.36   |
| 52       | 0.48          | 0.51     | 0.84           | 0.82      | 0.33        | 0.35   |
| 53       | 0.48          | 0.51     | 0.84           | 0.82      | 0.33        | 0.35   |
| 54       | 0.47          | 0.50     | 0.85           | 0.83      | 0.32        | 0.35   |
| 55       | 0.46          | 0.49     | 0.85           | 0.83      | 0.32        | 0.34   |
| 56       | 0.45          | 0.48     | 0.86           | 0.84      | 0.31        | 0.33   |
| 57       | 0.45          | 0.48     | 0.86           | 0.84      | 0.31        | 0.33   |
| 58       | 0.44          | 0.47     | 0.87           | 0.85      | 0.30        | 0.32   |
| 59       | 0.43          | 0.46     | 0.87           | 0.85      | 0.29        | 0.32   |
| 60       | 0.42          | 0.45     | 0.88           | 0.86      | 0.28        | 0.31   |
| 61       | 0.41          | 0.44     | 0.88           | 0.86      | 0.28        | 0.30   |
| 62       | 0.40          | 0.43     | 0.89           | 0.87      | 0.27        | 0.29   |
| 63       | 0.40          | 0.43     | 0.89           | 0.87      | 0.27        | 0.29   |

Continued on next page

| $\alpha$ | $\phi_S^\ell$ | $\phi_S$ | $\varphi^\ell$ | $\varphi$ | $\psi^\ell$ | $\psi$ |
|----------|---------------|----------|----------------|-----------|-------------|--------|
| 64       | 0.39          | 0.42     | 0.90           | 0.88      | 0.26        | 0.28   |
| 65       | 0.38          | 0.41     | 0.91           | 0.88      | 0.25        | 0.28   |
| 66       | 0.37          | 0.40     | 0.91           | 0.88      | 0.25        | 0.27   |
| 67       | 0.36          | 0.39     | 0.92           | 0.89      | 0.24        | 0.26   |
| 68       | 0.34          | 0.38     | 0.92           | 0.89      | 0.23        | 0.26   |
| 69       | 0.33          | 0.37     | 0.93           | 0.90      | 0.22        | 0.25   |
| 70       | 0.32          | 0.36     | 0.93           | 0.90      | 0.21        | 0.24   |
| 71       | 0.31          | 0.35     | 0.94           | 0.91      | 0.20        | 0.23   |
| 72       | 0.30          | 0.34     | 0.94           | 0.91      | 0.20        | 0.23   |
| 73       | 0.29          | 0.32     | 0.94           | 0.92      | 0.19        | 0.21   |
| 74       | 0.28          | 0.31     | 0.95           | 0.92      | 0.18        | 0.21   |
| 75       | 0.26          | 0.30     | 0.95           | 0.92      | 0.17        | 0.20   |
| 76       | 0.25          | 0.29     | 0.96           | 0.93      | 0.16        | 0.19   |
| 77       | 0.24          | 0.28     | 0.96           | 0.93      | 0.16        | 0.19   |
| 78       | 0.23          | 0.27     | 0.96           | 0.93      | 0.15        | 0.18   |
| 79       | 0.22          | 0.26     | 0.97           | 0.94      | 0.14        | 0.17   |
| 80       | 0.21          | 0.25     | 0.97           | 0.94      | 0.14        | 0.17   |
| 81       | 0.20          | 0.23     | 0.97           | 0.94      | 0.13        | 0.15   |
| 82       | 0.19          | 0.22     | 0.97           | 0.94      | 0.12        | 0.15   |
| 83       | 0.18          | 0.21     | 0.97           | 0.95      | 0.12        | 0.14   |
| 84       | 0.17          | 0.20     | 0.98           | 0.95      | 0.11        | 0.13   |
| 85       | 0.16          | 0.19     | 0.98           | 0.95      | 0.10        | 0.13   |
| 86       | 0.15          | 0.19     | 0.98           | 0.95      | 0.10        | 0.13   |
| 87       | 0.14          | 0.18     | 0.98           | 0.95      | 0.09        | 0.12   |
| 88       | 0.13          | 0.17     | 0.98           | 0.95      | 0.08        | 0.11   |
| 89       | 0.13          | 0.17     | 0.98           | 0.95      | 0.08        | 0.11   |
| 90       | 0.13          | 0.17     | 0.98           | 0.95      | 0.08        | 0.11   |

Table S109: Reference ( $\phi_S$ ,  $\varphi$ ,  $\psi$ ) and approached ( $\phi_S^\ell$ ,  $\varphi^\ell$ ,  $\psi^\ell$ ) values of the topological descriptors for the first excited-state of the pyridinium-phenolate (PP), computed at the LC-wHPBE/6-31+G level of theory.  $\alpha$  is the pyridinium-phenolate central twist angle amplitude.



| $\alpha$ | $\phi_S^\ell$ | $\phi_S$ | $\varphi^\ell$ | $\varphi$ | $\psi^\ell$ | $\psi$ |
|----------|---------------|----------|----------------|-----------|-------------|--------|
| 0        | 0.65          | 0.69     | 0.68           | 0.64      | 0.49        | 0.52   |
| 0        | 0.64          | 0.65     | 0.69           | 1.00      | 0.48        | 0.37   |
| 1        | 0.64          | 0.65     | 0.69           | 2.00      | 0.48        | 0.20   |
| 2        | 0.64          | 0.65     | 0.69           | 3.00      | 0.48        | 0.14   |
| 3        | 0.64          | 0.65     | 0.69           | 4.00      | 0.48        | 0.10   |
| 4        | 0.65          | 0.65     | 0.69           | 5.00      | 0.48        | 0.08   |
| 5        | 0.65          | 0.64     | 0.69           | 6.00      | 0.48        | 0.07   |
| 6        | 0.65          | 0.64     | 0.69           | 7.00      | 0.48        | 0.06   |
| 7        | 0.65          | 0.64     | 0.69           | 8.00      | 0.48        | 0.05   |
| 8        | 0.65          | 0.64     | 0.69           | 9.00      | 0.48        | 0.05   |
| 9        | 0.65          | 0.64     | 0.69           | 10.00     | 0.48        | 0.04   |
| 10       | 0.65          | 0.64     | 0.69           | 11.00     | 0.48        | 0.04   |
| 11       | 0.65          | 0.64     | 0.68           | 12.00     | 0.48        | 0.03   |
| 12       | 0.65          | 0.64     | 0.68           | 13.00     | 0.49        | 0.03   |
| 13       | 0.66          | 0.64     | 0.68           | 14.00     | 0.49        | 0.03   |
| 14       | 0.66          | 0.64     | 0.68           | 15.00     | 0.49        | 0.03   |
| 15       | 0.66          | 0.64     | 0.68           | 16.00     | 0.49        | 0.03   |
| 16       | 0.66          | 0.63     | 0.68           | 17.00     | 0.49        | 0.02   |
| 17       | 0.66          | 0.63     | 0.68           | 18.00     | 0.49        | 0.02   |
| 18       | 0.67          | 0.63     | 0.67           | 19.00     | 0.50        | 0.02   |
| 19       | 0.67          | 0.63     | 0.67           | 20.00     | 0.50        | 0.02   |
| 20       | 0.67          | 0.63     | 0.67           | 21.00     | 0.50        | 0.02   |
| 21       | 0.67          | 0.63     | 0.67           | 22.00     | 0.50        | 0.02   |
| 22       | 0.68          | 0.62     | 0.67           | 23.00     | 0.51        | 0.02   |
| 23       | 0.68          | 0.62     | 0.66           | 24.00     | 0.51        | 0.02   |
| 24       | 0.68          | 0.62     | 0.66           | 25.00     | 0.51        | 0.02   |
| 25       | 0.69          | 0.62     | 0.66           | 26.00     | 0.51        | 0.02   |
| 26       | 0.69          | 0.62     | 0.66           | 27.00     | 0.52        | 0.01   |
| 27       | 0.69          | 0.62     | 0.65           | 28.00     | 0.52        | 0.01   |
| 28       | 0.70          | 0.61     | 0.65           | 29.00     | 0.52        | 0.01   |
| 29       | 0.70          | 0.61     | 0.65           | 30.00     | 0.52        | 0.01   |
| 30       | 0.70          | 0.61     | 0.64           | 31.00     | 0.53        | 0.01   |

Continued on next page

| $\alpha$ | $\phi_S^\ell$ | $\phi_S$ | $\varphi^\ell$ | $\varphi$ | $\psi^\ell$ | $\psi$ |
|----------|---------------|----------|----------------|-----------|-------------|--------|
| 31       | 0.71          | 0.61     | 0.64           | 32.00     | 0.53        | 0.01   |
| 32       | 0.71          | 0.60     | 0.64           | 33.00     | 0.53        | 0.01   |
| 33       | 0.71          | 0.60     | 0.63           | 34.00     | 0.54        | 0.01   |
| 34       | 0.72          | 0.60     | 0.63           | 35.00     | 0.54        | 0.01   |
| 35       | 0.72          | 0.59     | 0.63           | 36.00     | 0.55        | 0.01   |
| 36       | 0.73          | 0.59     | 0.62           | 37.00     | 0.55        | 0.01   |
| 37       | 0.73          | 0.59     | 0.62           | 38.00     | 0.55        | 0.01   |
| 38       | 0.74          | 0.58     | 0.61           | 39.00     | 0.56        | 0.01   |
| 39       | 0.74          | 0.58     | 0.61           | 40.00     | 0.56        | 0.01   |
| 40       | 0.74          | 0.57     | 0.60           | 41.00     | 0.57        | 0.01   |
| 41       | 0.75          | 0.57     | 0.60           | 42.00     | 0.57        | 0.01   |
| 42       | 0.75          | 0.56     | 0.60           | 43.00     | 0.57        | 0.01   |
| 43       | 0.76          | 0.56     | 0.59           | 44.00     | 0.58        | 0.01   |
| 44       | 0.76          | 0.55     | 0.59           | 45.00     | 0.58        | 0.01   |
| 45       | 0.77          | 0.55     | 0.58           | 46.00     | 0.59        | 0.01   |
| 46       | 0.77          | 0.54     | 0.57           | 47.00     | 0.59        | 0.01   |
| 47       | 0.78          | 0.54     | 0.57           | 48.00     | 0.60        | 0.01   |
| 48       | 0.78          | 0.53     | 0.56           | 49.00     | 0.60        | 0.01   |
| 49       | 0.79          | 0.53     | 0.56           | 50.00     | 0.61        | 0.01   |
| 50       | 0.79          | 0.52     | 0.55           | 51.00     | 0.61        | 0.01   |
| 51       | 0.80          | 0.51     | 0.54           | 52.00     | 0.62        | 0.01   |
| 52       | 0.80          | 0.51     | 0.54           | 53.00     | 0.62        | 0.01   |
| 53       | 0.81          | 0.50     | 0.53           | 54.00     | 0.63        | 0.01   |
| 54       | 0.81          | 0.49     | 0.52           | 55.00     | 0.64        | 0.01   |
| 55       | 0.82          | 0.48     | 0.52           | 56.00     | 0.64        | 0.01   |
| 56       | 0.82          | 0.48     | 0.51           | 57.00     | 0.65        | 0.01   |
| 57       | 0.83          | 0.47     | 0.50           | 58.00     | 0.65        | 0.01   |
| 58       | 0.83          | 0.46     | 0.49           | 59.00     | 0.66        | 0.00   |
| 59       | 0.84          | 0.45     | 0.49           | 60.00     | 0.67        | 0.00   |
| 60       | 0.84          | 0.44     | 0.48           | 61.00     | 0.67        | 0.00   |
| 61       | 0.85          | 0.43     | 0.47           | 62.00     | 0.68        | 0.00   |
| 62       | 0.85          | 0.42     | 0.46           | 63.00     | 0.69        | 0.00   |

Continued on next page

| $\alpha$ | $\phi_S^\ell$ | $\phi_S$ | $\varphi^\ell$ | $\varphi$ | $\psi^\ell$ | $\psi$ |
|----------|---------------|----------|----------------|-----------|-------------|--------|
| 63       | 0.86          | 0.41     | 0.45           | 64.00     | 0.69        | 0.00   |
| 64       | 0.87          | 0.40     | 0.44           | 65.00     | 0.70        | 0.00   |
| 65       | 0.87          | 0.39     | 0.43           | 66.00     | 0.71        | 0.00   |
| 66       | 0.88          | 0.38     | 0.42           | 67.00     | 0.71        | 0.00   |
| 67       | 0.88          | 0.37     | 0.41           | 68.00     | 0.72        | 0.00   |
| 68       | 0.89          | 0.36     | 0.40           | 69.00     | 0.73        | 0.00   |
| 69       | 0.89          | 0.35     | 0.39           | 70.00     | 0.74        | 0.00   |
| 70       | 0.90          | 0.33     | 0.38           | 71.00     | 0.75        | 0.00   |
| 71       | 0.90          | 0.32     | 0.37           | 72.00     | 0.75        | 0.00   |
| 72       | 0.91          | 0.31     | 0.36           | 73.00     | 0.76        | 0.00   |
| 73       | 0.91          | 0.30     | 0.34           | 74.00     | 0.77        | 0.00   |
| 74       | 0.91          | 0.28     | 0.33           | 75.00     | 0.78        | 0.00   |
| 75       | 0.92          | 0.27     | 0.32           | 76.00     | 0.79        | 0.00   |
| 76       | 0.92          | 0.25     | 0.31           | 77.00     | 0.80        | 0.00   |
| 77       | 0.93          | 0.24     | 0.30           | 78.00     | 0.80        | 0.00   |
| 78       | 0.93          | 0.23     | 0.28           | 79.00     | 0.81        | 0.00   |
| 79       | 0.93          | 0.21     | 0.27           | 80.00     | 0.82        | 0.00   |
| 80       | 0.94          | 0.20     | 0.26           | 81.00     | 0.83        | 0.00   |
| 81       | 0.94          | 0.19     | 0.24           | 82.00     | 0.84        | 0.00   |
| 82       | 0.94          | 0.17     | 0.23           | 83.00     | 0.85        | 0.00   |
| 83       | 0.95          | 0.16     | 0.22           | 84.00     | 0.85        | 0.00   |
| 84       | 0.95          | 0.15     | 0.21           | 85.00     | 0.86        | 0.00   |
| 85       | 0.95          | 0.14     | 0.20           | 86.00     | 0.87        | 0.00   |
| 86       | 0.95          | 0.13     | 0.19           | 87.00     | 0.88        | 0.00   |
| 87       | 0.95          | 0.12     | 0.18           | 88.00     | 0.88        | 0.00   |
| 88       | 0.96          | 0.11     | 0.17           | 89.00     | 0.89        | 0.00   |
| 89       | 0.96          | 0.11     | 0.17           | 90.00     | 0.89        | 0.00   |

Table S110: Reference  $(\phi_S, \varphi, \psi)$  and approached  $(\phi_S^\ell, \varphi^\ell, \psi^\ell)$  values of the topological descriptors for the first excited-state of the pyridinium-phenolate (PP), computed at the LC-wHPBE/6-31G level of theory.  $\alpha$  is the pyridinium-phenolate central twist angle amplitude.

| $\alpha$ | $\phi_S^\ell$ | $\phi_S$ | $\varphi^\ell$ | $\varphi$ | $\psi^\ell$ | $\psi$ |
|----------|---------------|----------|----------------|-----------|-------------|--------|
| 0        | 0.70          | 0.74     | 0.64           | 0.60      | 0.53        | 0.57   |
| 1        | 0.70          | 0.74     | 0.64           | 0.60      | 0.53        | 0.57   |
| 2        | 0.70          | 0.74     | 0.64           | 0.60      | 0.53        | 0.57   |
| 3        | 0.70          | 0.74     | 0.64           | 0.60      | 0.53        | 0.57   |
| 4        | 0.70          | 0.74     | 0.64           | 0.60      | 0.53        | 0.57   |
| 5        | 0.70          | 0.73     | 0.64           | 0.61      | 0.53        | 0.56   |
| 6        | 0.70          | 0.73     | 0.64           | 0.61      | 0.53        | 0.56   |
| 7        | 0.70          | 0.73     | 0.64           | 0.61      | 0.53        | 0.56   |
| 8        | 0.70          | 0.73     | 0.64           | 0.61      | 0.53        | 0.56   |
| 9        | 0.70          | 0.73     | 0.64           | 0.61      | 0.53        | 0.56   |
| 10       | 0.70          | 0.73     | 0.64           | 0.61      | 0.53        | 0.56   |
| 11       | 0.70          | 0.73     | 0.65           | 0.61      | 0.52        | 0.56   |
| 12       | 0.70          | 0.73     | 0.65           | 0.61      | 0.52        | 0.56   |
| 13       | 0.70          | 0.73     | 0.65           | 0.62      | 0.52        | 0.55   |
| 14       | 0.70          | 0.73     | 0.65           | 0.62      | 0.52        | 0.55   |
| 15       | 0.69          | 0.72     | 0.65           | 0.62      | 0.52        | 0.55   |
| 16       | 0.69          | 0.72     | 0.65           | 0.62      | 0.52        | 0.55   |
| 17       | 0.69          | 0.72     | 0.65           | 0.62      | 0.52        | 0.55   |
| 18       | 0.69          | 0.72     | 0.66           | 0.63      | 0.51        | 0.54   |
| 19       | 0.69          | 0.72     | 0.66           | 0.63      | 0.51        | 0.54   |
| 20       | 0.69          | 0.72     | 0.66           | 0.63      | 0.51        | 0.54   |
| 21       | 0.69          | 0.72     | 0.66           | 0.63      | 0.51        | 0.54   |
| 22       | 0.69          | 0.71     | 0.67           | 0.64      | 0.51        | 0.53   |
| 23       | 0.69          | 0.71     | 0.67           | 0.64      | 0.51        | 0.53   |
| 24       | 0.69          | 0.71     | 0.67           | 0.64      | 0.51        | 0.53   |
| 25       | 0.68          | 0.71     | 0.67           | 0.64      | 0.50        | 0.53   |
| 26       | 0.68          | 0.71     | 0.67           | 0.65      | 0.50        | 0.53   |
| 27       | 0.68          | 0.71     | 0.68           | 0.65      | 0.50        | 0.53   |
| 28       | 0.68          | 0.70     | 0.68           | 0.65      | 0.50        | 0.52   |
| 29       | 0.68          | 0.70     | 0.68           | 0.66      | 0.50        | 0.52   |
| 30       | 0.68          | 0.70     | 0.68           | 0.66      | 0.50        | 0.52   |
| 31       | 0.68          | 0.70     | 0.69           | 0.66      | 0.50        | 0.52   |

Continued on next page

| $\alpha$ | $\phi_S^\ell$ | $\phi_S$ | $\varphi^\ell$ | $\varphi$ | $\psi^\ell$ | $\psi$ |
|----------|---------------|----------|----------------|-----------|-------------|--------|
| 32       | 0.68          | 0.69     | 0.69           | 0.67      | 0.50        | 0.51   |
| 33       | 0.67          | 0.69     | 0.69           | 0.67      | 0.49        | 0.51   |
| 34       | 0.67          | 0.69     | 0.70           | 0.67      | 0.49        | 0.51   |
| 35       | 0.67          | 0.69     | 0.70           | 0.68      | 0.49        | 0.50   |
| 36       | 0.67          | 0.68     | 0.70           | 0.68      | 0.49        | 0.50   |
| 37       | 0.67          | 0.68     | 0.70           | 0.68      | 0.49        | 0.50   |
| 38       | 0.66          | 0.68     | 0.71           | 0.69      | 0.48        | 0.50   |
| 39       | 0.66          | 0.68     | 0.71           | 0.69      | 0.48        | 0.50   |
| 40       | 0.66          | 0.67     | 0.72           | 0.69      | 0.47        | 0.49   |
| 41       | 0.66          | 0.67     | 0.72           | 0.70      | 0.47        | 0.49   |
| 42       | 0.65          | 0.67     | 0.72           | 0.70      | 0.47        | 0.49   |
| 43       | 0.65          | 0.66     | 0.73           | 0.71      | 0.46        | 0.48   |
| 44       | 0.65          | 0.66     | 0.73           | 0.71      | 0.46        | 0.48   |
| 45       | 0.64          | 0.65     | 0.74           | 0.71      | 0.45        | 0.47   |
| 46       | 0.64          | 0.65     | 0.74           | 0.72      | 0.45        | 0.47   |
| 47       | 0.63          | 0.65     | 0.74           | 0.72      | 0.45        | 0.47   |
| 48       | 0.63          | 0.64     | 0.75           | 0.73      | 0.44        | 0.46   |
| 49       | 0.63          | 0.64     | 0.75           | 0.73      | 0.44        | 0.46   |
| 50       | 0.62          | 0.63     | 0.76           | 0.74      | 0.44        | 0.45   |
| 51       | 0.62          | 0.63     | 0.76           | 0.74      | 0.44        | 0.45   |
| 52       | 0.61          | 0.62     | 0.77           | 0.74      | 0.43        | 0.44   |
| 53       | 0.61          | 0.62     | 0.77           | 0.75      | 0.43        | 0.44   |
| 54       | 0.60          | 0.61     | 0.77           | 0.75      | 0.42        | 0.43   |
| 55       | 0.60          | 0.61     | 0.78           | 0.76      | 0.42        | 0.43   |
| 56       | 0.59          | 0.60     | 0.78           | 0.76      | 0.41        | 0.43   |
| 57       | 0.59          | 0.60     | 0.79           | 0.77      | 0.41        | 0.42   |
| 58       | 0.58          | 0.59     | 0.79           | 0.77      | 0.40        | 0.42   |
| 59       | 0.57          | 0.59     | 0.80           | 0.78      | 0.39        | 0.41   |
| 60       | 0.57          | 0.58     | 0.80           | 0.78      | 0.39        | 0.41   |
| 61       | 0.56          | 0.57     | 0.81           | 0.79      | 0.39        | 0.40   |
| 62       | 0.55          | 0.57     | 0.82           | 0.79      | 0.38        | 0.40   |
| 63       | 0.55          | 0.56     | 0.82           | 0.80      | 0.38        | 0.39   |

Continued on next page

| $\alpha$ | $\phi_S^\ell$ | $\phi_S$ | $\varphi^\ell$ | $\varphi$ | $\psi^\ell$ | $\psi$ |
|----------|---------------|----------|----------------|-----------|-------------|--------|
| 64       | 0.54          | 0.55     | 0.83           | 0.80      | 0.37        | 0.38   |
| 65       | 0.53          | 0.54     | 0.83           | 0.81      | 0.36        | 0.37   |
| 66       | 0.52          | 0.53     | 0.84           | 0.82      | 0.35        | 0.37   |
| 67       | 0.51          | 0.53     | 0.84           | 0.82      | 0.35        | 0.37   |
| 68       | 0.50          | 0.52     | 0.85           | 0.83      | 0.34        | 0.36   |
| 69       | 0.49          | 0.51     | 0.86           | 0.83      | 0.33        | 0.35   |
| 70       | 0.48          | 0.50     | 0.86           | 0.84      | 0.32        | 0.34   |
| 71       | 0.47          | 0.49     | 0.87           | 0.84      | 0.32        | 0.34   |
| 72       | 0.46          | 0.48     | 0.88           | 0.85      | 0.31        | 0.33   |
| 73       | 0.45          | 0.47     | 0.88           | 0.86      | 0.30        | 0.32   |
| 74       | 0.44          | 0.46     | 0.89           | 0.86      | 0.29        | 0.31   |
| 75       | 0.42          | 0.44     | 0.90           | 0.87      | 0.28        | 0.30   |
| 76       | 0.41          | 0.43     | 0.90           | 0.88      | 0.27        | 0.29   |
| 77       | 0.39          | 0.42     | 0.91           | 0.88      | 0.26        | 0.28   |
| 78       | 0.38          | 0.40     | 0.92           | 0.89      | 0.25        | 0.27   |
| 79       | 0.36          | 0.39     | 0.92           | 0.90      | 0.24        | 0.26   |
| 80       | 0.34          | 0.37     | 0.93           | 0.90      | 0.22        | 0.25   |
| 81       | 0.32          | 0.35     | 0.94           | 0.91      | 0.21        | 0.23   |
| 82       | 0.30          | 0.33     | 0.95           | 0.92      | 0.19        | 0.22   |
| 83       | 0.27          | 0.31     | 0.95           | 0.93      | 0.18        | 0.20   |
| 84       | 0.24          | 0.29     | 0.96           | 0.93      | 0.16        | 0.19   |
| 85       | 0.22          | 0.26     | 0.97           | 0.94      | 0.14        | 0.17   |
| 86       | 0.19          | 0.24     | 0.98           | 0.95      | 0.12        | 0.16   |
| 87       | 0.16          | 0.21     | 0.98           | 0.95      | 0.10        | 0.14   |
| 88       | 0.13          | 0.19     | 0.99           | 0.96      | 0.08        | 0.12   |
| 89       | 0.10          | 0.17     | 0.99           | 0.96      | 0.06        | 0.11   |
| 90       | 0.09          | 0.16     | 0.99           | 0.96      | 0.06        | 0.11   |

Table S111: Reference ( $\phi_S$ ,  $\varphi$ ,  $\psi$ ) and approached ( $\phi_S^\ell$ ,  $\varphi^\ell$ ,  $\psi^\ell$ ) values of the topological descriptors for the first excited-state of the pyridinium-phenolate (PP), computed at the M062X/3-21G level of theory.  $\alpha$  is the pyridinium-phenolate central twist angle amplitude.

| $\alpha$ | $\phi_S^\ell$ | $\phi_S$ | $\varphi^\ell$ | $\varphi$ | $\psi^\ell$ | $\psi$ |
|----------|---------------|----------|----------------|-----------|-------------|--------|
| 0        | 0.66          | 0.71     | 0.66           | 0.63      | 0.50        | 0.54   |
| 1        | 0.66          | 0.71     | 0.66           | 0.63      | 0.50        | 0.54   |
| 2        | 0.66          | 0.71     | 0.66           | 0.63      | 0.50        | 0.54   |
| 3        | 0.66          | 0.71     | 0.66           | 0.63      | 0.50        | 0.54   |
| 4        | 0.66          | 0.71     | 0.66           | 0.63      | 0.50        | 0.54   |
| 5        | 0.66          | 0.71     | 0.66           | 0.63      | 0.50        | 0.54   |
| 6        | 0.66          | 0.70     | 0.66           | 0.63      | 0.50        | 0.53   |
| 7        | 0.66          | 0.70     | 0.66           | 0.63      | 0.50        | 0.53   |
| 8        | 0.66          | 0.70     | 0.66           | 0.63      | 0.50        | 0.53   |
| 9        | 0.66          | 0.70     | 0.67           | 0.63      | 0.50        | 0.53   |
| 10       | 0.66          | 0.70     | 0.67           | 0.63      | 0.50        | 0.53   |
| 11       | 0.66          | 0.70     | 0.67           | 0.64      | 0.50        | 0.53   |
| 12       | 0.66          | 0.70     | 0.67           | 0.64      | 0.50        | 0.53   |
| 13       | 0.65          | 0.70     | 0.67           | 0.64      | 0.49        | 0.53   |
| 14       | 0.65          | 0.70     | 0.67           | 0.64      | 0.49        | 0.53   |
| 15       | 0.65          | 0.70     | 0.67           | 0.64      | 0.49        | 0.53   |
| 16       | 0.65          | 0.69     | 0.68           | 0.65      | 0.49        | 0.52   |
| 17       | 0.65          | 0.69     | 0.68           | 0.65      | 0.49        | 0.52   |
| 18       | 0.65          | 0.69     | 0.68           | 0.65      | 0.49        | 0.52   |
| 19       | 0.65          | 0.69     | 0.68           | 0.65      | 0.49        | 0.52   |
| 20       | 0.65          | 0.69     | 0.68           | 0.65      | 0.49        | 0.52   |
| 21       | 0.65          | 0.69     | 0.69           | 0.66      | 0.48        | 0.51   |
| 22       | 0.64          | 0.68     | 0.69           | 0.66      | 0.48        | 0.51   |
| 23       | 0.64          | 0.68     | 0.69           | 0.66      | 0.48        | 0.51   |
| 24       | 0.64          | 0.68     | 0.69           | 0.66      | 0.48        | 0.51   |
| 25       | 0.64          | 0.68     | 0.70           | 0.67      | 0.47        | 0.50   |
| 26       | 0.64          | 0.68     | 0.70           | 0.67      | 0.47        | 0.50   |
| 27       | 0.64          | 0.67     | 0.70           | 0.67      | 0.47        | 0.50   |
| 28       | 0.63          | 0.67     | 0.71           | 0.68      | 0.46        | 0.50   |
| 29       | 0.63          | 0.67     | 0.71           | 0.68      | 0.46        | 0.50   |
| 30       | 0.63          | 0.67     | 0.71           | 0.68      | 0.46        | 0.50   |
| 31       | 0.63          | 0.66     | 0.72           | 0.69      | 0.46        | 0.49   |

Continued on next page

| $\alpha$ | $\phi_S^\ell$ | $\phi_S$ | $\varphi^\ell$ | $\varphi$ | $\psi^\ell$ | $\psi$ |
|----------|---------------|----------|----------------|-----------|-------------|--------|
| 32       | 0.63          | 0.66     | 0.72           | 0.69      | 0.46        | 0.49   |
| 33       | 0.62          | 0.66     | 0.72           | 0.69      | 0.45        | 0.49   |
| 34       | 0.62          | 0.66     | 0.73           | 0.70      | 0.45        | 0.48   |
| 35       | 0.62          | 0.65     | 0.73           | 0.70      | 0.45        | 0.48   |
| 36       | 0.62          | 0.65     | 0.73           | 0.70      | 0.45        | 0.48   |
| 37       | 0.61          | 0.65     | 0.74           | 0.71      | 0.44        | 0.47   |
| 38       | 0.61          | 0.64     | 0.74           | 0.71      | 0.44        | 0.47   |
| 39       | 0.61          | 0.64     | 0.74           | 0.72      | 0.44        | 0.46   |
| 40       | 0.60          | 0.64     | 0.75           | 0.72      | 0.43        | 0.46   |
| 41       | 0.60          | 0.63     | 0.75           | 0.72      | 0.43        | 0.46   |
| 42       | 0.60          | 0.63     | 0.76           | 0.73      | 0.43        | 0.45   |
| 43       | 0.59          | 0.62     | 0.76           | 0.73      | 0.42        | 0.45   |
| 44       | 0.59          | 0.62     | 0.76           | 0.74      | 0.42        | 0.44   |
| 45       | 0.59          | 0.62     | 0.77           | 0.74      | 0.42        | 0.44   |
| 46       | 0.58          | 0.61     | 0.77           | 0.75      | 0.41        | 0.43   |
| 47       | 0.58          | 0.61     | 0.78           | 0.75      | 0.41        | 0.43   |
| 48       | 0.57          | 0.60     | 0.78           | 0.76      | 0.40        | 0.43   |
| 49       | 0.57          | 0.60     | 0.79           | 0.76      | 0.40        | 0.43   |
| 50       | 0.56          | 0.59     | 0.79           | 0.76      | 0.39        | 0.42   |
| 51       | 0.56          | 0.59     | 0.79           | 0.77      | 0.39        | 0.42   |
| 52       | 0.55          | 0.58     | 0.80           | 0.77      | 0.38        | 0.41   |
| 53       | 0.55          | 0.57     | 0.80           | 0.78      | 0.38        | 0.40   |
| 54       | 0.54          | 0.57     | 0.81           | 0.78      | 0.37        | 0.40   |
| 55       | 0.54          | 0.56     | 0.81           | 0.79      | 0.37        | 0.39   |
| 56       | 0.53          | 0.56     | 0.82           | 0.79      | 0.37        | 0.39   |
| 57       | 0.52          | 0.55     | 0.82           | 0.80      | 0.36        | 0.38   |
| 58       | 0.52          | 0.54     | 0.83           | 0.80      | 0.36        | 0.38   |
| 59       | 0.51          | 0.54     | 0.83           | 0.81      | 0.35        | 0.37   |
| 60       | 0.50          | 0.53     | 0.84           | 0.81      | 0.34        | 0.37   |
| 61       | 0.50          | 0.52     | 0.84           | 0.82      | 0.34        | 0.36   |
| 62       | 0.49          | 0.51     | 0.85           | 0.82      | 0.33        | 0.35   |
| 63       | 0.48          | 0.51     | 0.85           | 0.83      | 0.33        | 0.35   |

Continued on next page



| $\alpha$ | $\phi_S^\ell$ | $\phi_S$ | $\varphi^\ell$ | $\varphi$ | $\psi^\ell$ | $\psi$ |
|----------|---------------|----------|----------------|-----------|-------------|--------|
| 64       | 0.47          | 0.50     | 0.86           | 0.83      | 0.32        | 0.35   |
| 65       | 0.46          | 0.49     | 0.86           | 0.84      | 0.31        | 0.34   |
| 66       | 0.46          | 0.48     | 0.87           | 0.85      | 0.31        | 0.33   |
| 67       | 0.45          | 0.47     | 0.87           | 0.85      | 0.30        | 0.32   |
| 68       | 0.44          | 0.46     | 0.88           | 0.86      | 0.30        | 0.31   |
| 69       | 0.43          | 0.45     | 0.88           | 0.86      | 0.29        | 0.31   |
| 70       | 0.42          | 0.44     | 0.89           | 0.87      | 0.28        | 0.30   |
| 71       | 0.40          | 0.43     | 0.90           | 0.87      | 0.27        | 0.29   |
| 72       | 0.39          | 0.42     | 0.90           | 0.88      | 0.26        | 0.28   |
| 73       | 0.38          | 0.40     | 0.91           | 0.88      | 0.25        | 0.27   |
| 74       | 0.37          | 0.39     | 0.91           | 0.89      | 0.25        | 0.26   |
| 75       | 0.36          | 0.38     | 0.92           | 0.90      | 0.24        | 0.25   |
| 76       | 0.34          | 0.37     | 0.92           | 0.90      | 0.23        | 0.25   |
| 77       | 0.33          | 0.35     | 0.93           | 0.91      | 0.22        | 0.23   |
| 78       | 0.31          | 0.34     | 0.93           | 0.91      | 0.20        | 0.23   |
| 79       | 0.30          | 0.32     | 0.94           | 0.92      | 0.20        | 0.21   |
| 80       | 0.28          | 0.31     | 0.94           | 0.92      | 0.18        | 0.21   |
| 81       | 0.26          | 0.29     | 0.95           | 0.93      | 0.17        | 0.19   |
| 82       | 0.25          | 0.27     | 0.95           | 0.93      | 0.16        | 0.18   |
| 83       | 0.23          | 0.26     | 0.95           | 0.94      | 0.15        | 0.17   |
| 84       | 0.21          | 0.24     | 0.96           | 0.94      | 0.14        | 0.16   |
| 85       | 0.19          | 0.22     | 0.96           | 0.94      | 0.12        | 0.15   |
| 86       | 0.18          | 0.21     | 0.97           | 0.95      | 0.12        | 0.14   |
| 87       | 0.17          | 0.19     | 0.97           | 0.95      | 0.11        | 0.13   |
| 88       | 0.15          | 0.18     | 0.97           | 0.95      | 0.10        | 0.12   |
| 89       | 0.14          | 0.17     | 0.97           | 0.95      | 0.09        | 0.11   |
| 90       | 0.14          | 0.17     | 0.97           | 0.95      | 0.09        | 0.11   |

Table S112: Reference ( $\phi_S$ ,  $\varphi$ ,  $\psi$ ) and approached ( $\phi_S^\ell$ ,  $\varphi^\ell$ ,  $\psi^\ell$ ) values of the topological descriptors for the first excited-state of the pyridinium-phenolate (PP), computed at the M062X/6-311++G(2d,p) level of theory.  $\alpha$  is the pyridinium-phenolate central twist angle amplitude.

| $\alpha$ | $\phi_S^\ell$ | $\phi_S$ | $\varphi^\ell$ | $\varphi$ | $\psi^\ell$ | $\psi$ |
|----------|---------------|----------|----------------|-----------|-------------|--------|
| 0        | 0.66          | 0.71     | 0.66           | 0.62      | 0.50        | 0.54   |
| 1        | 0.66          | 0.71     | 0.66           | 0.62      | 0.50        | 0.54   |
| 2        | 0.66          | 0.71     | 0.66           | 0.62      | 0.50        | 0.54   |
| 3        | 0.66          | 0.71     | 0.66           | 0.62      | 0.50        | 0.54   |
| 4        | 0.66          | 0.71     | 0.66           | 0.63      | 0.50        | 0.54   |
| 5        | 0.66          | 0.71     | 0.66           | 0.63      | 0.50        | 0.54   |
| 6        | 0.66          | 0.71     | 0.66           | 0.63      | 0.50        | 0.54   |
| 7        | 0.66          | 0.71     | 0.66           | 0.63      | 0.50        | 0.54   |
| 8        | 0.66          | 0.71     | 0.66           | 0.63      | 0.50        | 0.54   |
| 9        | 0.66          | 0.70     | 0.66           | 0.63      | 0.50        | 0.53   |
| 10       | 0.66          | 0.70     | 0.66           | 0.63      | 0.50        | 0.53   |
| 11       | 0.65          | 0.70     | 0.67           | 0.63      | 0.49        | 0.53   |
| 12       | 0.65          | 0.70     | 0.67           | 0.64      | 0.49        | 0.53   |
| 13       | 0.65          | 0.70     | 0.67           | 0.64      | 0.49        | 0.53   |
| 14       | 0.65          | 0.70     | 0.67           | 0.64      | 0.49        | 0.53   |
| 15       | 0.65          | 0.70     | 0.67           | 0.64      | 0.49        | 0.53   |
| 16       | 0.65          | 0.70     | 0.67           | 0.64      | 0.49        | 0.53   |
| 17       | 0.65          | 0.69     | 0.68           | 0.65      | 0.49        | 0.52   |
| 18       | 0.65          | 0.69     | 0.68           | 0.65      | 0.49        | 0.52   |
| 19       | 0.65          | 0.69     | 0.68           | 0.65      | 0.49        | 0.52   |
| 20       | 0.65          | 0.69     | 0.68           | 0.65      | 0.49        | 0.52   |
| 21       | 0.65          | 0.69     | 0.69           | 0.66      | 0.48        | 0.51   |
| 22       | 0.64          | 0.69     | 0.69           | 0.66      | 0.48        | 0.51   |
| 23       | 0.64          | 0.68     | 0.69           | 0.66      | 0.48        | 0.51   |
| 24       | 0.64          | 0.68     | 0.69           | 0.66      | 0.48        | 0.51   |
| 25       | 0.64          | 0.68     | 0.70           | 0.67      | 0.47        | 0.50   |
| 26       | 0.64          | 0.68     | 0.70           | 0.67      | 0.47        | 0.50   |
| 27       | 0.64          | 0.68     | 0.70           | 0.67      | 0.47        | 0.50   |
| 28       | 0.64          | 0.67     | 0.70           | 0.68      | 0.47        | 0.50   |
| 29       | 0.63          | 0.67     | 0.71           | 0.68      | 0.46        | 0.50   |
| 30       | 0.63          | 0.67     | 0.71           | 0.68      | 0.46        | 0.50   |
| 31       | 0.63          | 0.67     | 0.71           | 0.69      | 0.46        | 0.49   |

Continued on next page

| $\alpha$ | $\phi_S^\ell$ | $\phi_S$ | $\varphi^\ell$ | $\varphi$ | $\psi^\ell$ | $\psi$ |
|----------|---------------|----------|----------------|-----------|-------------|--------|
| 32       | 0.63          | 0.66     | 0.72           | 0.69      | 0.46        | 0.49   |
| 33       | 0.63          | 0.66     | 0.72           | 0.69      | 0.46        | 0.49   |
| 34       | 0.62          | 0.66     | 0.72           | 0.70      | 0.45        | 0.48   |
| 35       | 0.62          | 0.65     | 0.73           | 0.70      | 0.45        | 0.48   |
| 36       | 0.62          | 0.65     | 0.73           | 0.70      | 0.45        | 0.48   |
| 37       | 0.62          | 0.65     | 0.73           | 0.71      | 0.45        | 0.47   |
| 38       | 0.61          | 0.64     | 0.74           | 0.71      | 0.44        | 0.47   |
| 39       | 0.61          | 0.64     | 0.74           | 0.72      | 0.44        | 0.46   |
| 40       | 0.61          | 0.64     | 0.74           | 0.72      | 0.44        | 0.46   |
| 41       | 0.60          | 0.63     | 0.75           | 0.72      | 0.43        | 0.46   |
| 42       | 0.60          | 0.63     | 0.75           | 0.73      | 0.43        | 0.45   |
| 43       | 0.60          | 0.62     | 0.76           | 0.73      | 0.43        | 0.45   |
| 44       | 0.59          | 0.62     | 0.76           | 0.74      | 0.42        | 0.44   |
| 45       | 0.59          | 0.62     | 0.77           | 0.74      | 0.42        | 0.44   |
| 46       | 0.59          | 0.61     | 0.77           | 0.75      | 0.42        | 0.43   |
| 47       | 0.58          | 0.61     | 0.77           | 0.75      | 0.41        | 0.43   |
| 48       | 0.58          | 0.60     | 0.78           | 0.75      | 0.41        | 0.43   |
| 49       | 0.57          | 0.60     | 0.78           | 0.76      | 0.40        | 0.43   |
| 50       | 0.57          | 0.59     | 0.79           | 0.76      | 0.40        | 0.42   |
| 51       | 0.56          | 0.59     | 0.79           | 0.77      | 0.39        | 0.42   |
| 52       | 0.56          | 0.58     | 0.80           | 0.77      | 0.39        | 0.41   |
| 53       | 0.55          | 0.58     | 0.80           | 0.78      | 0.38        | 0.41   |
| 54       | 0.55          | 0.57     | 0.81           | 0.78      | 0.38        | 0.40   |
| 55       | 0.54          | 0.56     | 0.81           | 0.79      | 0.37        | 0.39   |
| 56       | 0.53          | 0.56     | 0.82           | 0.79      | 0.37        | 0.39   |
| 57       | 0.53          | 0.55     | 0.82           | 0.80      | 0.37        | 0.38   |
| 58       | 0.52          | 0.54     | 0.82           | 0.80      | 0.36        | 0.38   |
| 59       | 0.51          | 0.54     | 0.83           | 0.81      | 0.35        | 0.37   |
| 60       | 0.51          | 0.53     | 0.84           | 0.81      | 0.35        | 0.37   |
| 61       | 0.50          | 0.52     | 0.84           | 0.82      | 0.34        | 0.36   |
| 62       | 0.49          | 0.51     | 0.85           | 0.82      | 0.33        | 0.35   |
| 63       | 0.48          | 0.51     | 0.85           | 0.83      | 0.33        | 0.35   |

Continued on next page

| $\alpha$ | $\phi_S^\ell$ | $\phi_S$ | $\varphi^\ell$ | $\varphi$ | $\psi^\ell$ | $\psi$ |
|----------|---------------|----------|----------------|-----------|-------------|--------|
| 64       | 0.47          | 0.50     | 0.86           | 0.83      | 0.32        | 0.35   |
| 65       | 0.46          | 0.49     | 0.86           | 0.84      | 0.31        | 0.34   |
| 66       | 0.46          | 0.48     | 0.87           | 0.85      | 0.31        | 0.33   |
| 67       | 0.45          | 0.47     | 0.87           | 0.85      | 0.30        | 0.32   |
| 68       | 0.44          | 0.46     | 0.88           | 0.86      | 0.30        | 0.31   |
| 69       | 0.42          | 0.45     | 0.89           | 0.86      | 0.28        | 0.31   |
| 70       | 0.41          | 0.44     | 0.89           | 0.87      | 0.27        | 0.30   |
| 71       | 0.40          | 0.43     | 0.90           | 0.87      | 0.27        | 0.29   |
| 72       | 0.39          | 0.42     | 0.90           | 0.88      | 0.26        | 0.28   |
| 73       | 0.38          | 0.41     | 0.91           | 0.88      | 0.25        | 0.28   |
| 74       | 0.36          | 0.39     | 0.92           | 0.89      | 0.24        | 0.26   |
| 75       | 0.35          | 0.38     | 0.92           | 0.90      | 0.23        | 0.25   |
| 76       | 0.34          | 0.37     | 0.93           | 0.90      | 0.22        | 0.25   |
| 77       | 0.32          | 0.35     | 0.93           | 0.91      | 0.21        | 0.23   |
| 78       | 0.30          | 0.34     | 0.94           | 0.91      | 0.20        | 0.23   |
| 79       | 0.29          | 0.32     | 0.94           | 0.92      | 0.19        | 0.21   |
| 80       | 0.27          | 0.31     | 0.95           | 0.92      | 0.18        | 0.21   |
| 81       | 0.25          | 0.29     | 0.95           | 0.93      | 0.16        | 0.19   |
| 82       | 0.24          | 0.27     | 0.96           | 0.93      | 0.16        | 0.18   |
| 83       | 0.22          | 0.26     | 0.96           | 0.94      | 0.14        | 0.17   |
| 84       | 0.20          | 0.24     | 0.97           | 0.94      | 0.13        | 0.16   |
| 85       | 0.18          | 0.22     | 0.97           | 0.94      | 0.12        | 0.15   |
| 86       | 0.17          | 0.21     | 0.97           | 0.95      | 0.11        | 0.14   |
| 87       | 0.15          | 0.19     | 0.98           | 0.95      | 0.10        | 0.13   |
| 88       | 0.14          | 0.18     | 0.98           | 0.95      | 0.09        | 0.12   |
| 89       | 0.13          | 0.17     | 0.98           | 0.95      | 0.08        | 0.11   |
| 90       | 0.13          | 0.17     | 0.98           | 0.95      | 0.08        | 0.11   |

Table S113: Reference ( $\phi_S$ ,  $\varphi$ ,  $\psi$ ) and approached ( $\phi_S^\ell$ ,  $\varphi^\ell$ ,  $\psi^\ell$ ) values of the topological descriptors for the first excited-state of the pyridinium-phenolate (PP), computed at the M062X/6-311++G(d,p) level of theory.  $\alpha$  is the pyridinium-phenolate central twist angle amplitude.

| $\alpha$ | $\phi_S^\ell$ | $\phi_S$ | $\varphi^\ell$ | $\varphi$ | $\psi^\ell$ | $\psi$ |
|----------|---------------|----------|----------------|-----------|-------------|--------|
| 0        | 0.66          | 0.71     | 0.66           | 0.62      | 0.50        | 0.54   |
| 1        | 0.66          | 0.71     | 0.66           | 0.62      | 0.50        | 0.54   |
| 2        | 0.66          | 0.71     | 0.66           | 0.62      | 0.50        | 0.54   |
| 3        | 0.66          | 0.71     | 0.66           | 0.62      | 0.50        | 0.54   |
| 4        | 0.66          | 0.71     | 0.66           | 0.63      | 0.50        | 0.54   |
| 5        | 0.66          | 0.71     | 0.66           | 0.63      | 0.50        | 0.54   |
| 6        | 0.66          | 0.71     | 0.66           | 0.63      | 0.50        | 0.54   |
| 7        | 0.66          | 0.71     | 0.66           | 0.63      | 0.50        | 0.54   |
| 8        | 0.66          | 0.71     | 0.66           | 0.63      | 0.50        | 0.54   |
| 9        | 0.66          | 0.70     | 0.66           | 0.63      | 0.50        | 0.53   |
| 10       | 0.66          | 0.70     | 0.66           | 0.63      | 0.50        | 0.53   |
| 11       | 0.65          | 0.70     | 0.67           | 0.63      | 0.49        | 0.53   |
| 12       | 0.65          | 0.70     | 0.67           | 0.64      | 0.49        | 0.53   |
| 13       | 0.65          | 0.70     | 0.67           | 0.64      | 0.49        | 0.53   |
| 14       | 0.65          | 0.70     | 0.67           | 0.64      | 0.49        | 0.53   |
| 15       | 0.65          | 0.70     | 0.67           | 0.64      | 0.49        | 0.53   |
| 16       | 0.65          | 0.70     | 0.67           | 0.64      | 0.49        | 0.53   |
| 17       | 0.65          | 0.69     | 0.68           | 0.65      | 0.49        | 0.52   |
| 18       | 0.65          | 0.69     | 0.68           | 0.65      | 0.49        | 0.52   |
| 19       | 0.65          | 0.69     | 0.68           | 0.65      | 0.49        | 0.52   |
| 20       | 0.65          | 0.69     | 0.68           | 0.65      | 0.49        | 0.52   |
| 21       | 0.65          | 0.69     | 0.68           | 0.66      | 0.49        | 0.51   |
| 22       | 0.64          | 0.69     | 0.69           | 0.66      | 0.48        | 0.51   |
| 23       | 0.64          | 0.68     | 0.69           | 0.66      | 0.48        | 0.51   |
| 24       | 0.64          | 0.68     | 0.69           | 0.66      | 0.48        | 0.51   |
| 25       | 0.64          | 0.68     | 0.70           | 0.67      | 0.47        | 0.50   |
| 26       | 0.64          | 0.68     | 0.70           | 0.67      | 0.47        | 0.50   |
| 27       | 0.64          | 0.68     | 0.70           | 0.67      | 0.47        | 0.50   |
| 28       | 0.64          | 0.67     | 0.70           | 0.68      | 0.47        | 0.50   |
| 29       | 0.63          | 0.67     | 0.71           | 0.68      | 0.46        | 0.50   |
| 30       | 0.63          | 0.67     | 0.71           | 0.68      | 0.46        | 0.50   |
| 31       | 0.63          | 0.67     | 0.71           | 0.69      | 0.46        | 0.49   |

Continued on next page

| $\alpha$ | $\phi_S^\ell$ | $\phi_S$ | $\varphi^\ell$ | $\varphi$ | $\psi^\ell$ | $\psi$ |
|----------|---------------|----------|----------------|-----------|-------------|--------|
| 32       | 0.63          | 0.66     | 0.72           | 0.69      | 0.46        | 0.49   |
| 33       | 0.63          | 0.66     | 0.72           | 0.69      | 0.46        | 0.49   |
| 34       | 0.62          | 0.66     | 0.72           | 0.70      | 0.45        | 0.48   |
| 35       | 0.62          | 0.65     | 0.73           | 0.70      | 0.45        | 0.48   |
| 36       | 0.62          | 0.65     | 0.73           | 0.70      | 0.45        | 0.48   |
| 37       | 0.62          | 0.65     | 0.73           | 0.71      | 0.45        | 0.47   |
| 38       | 0.61          | 0.64     | 0.74           | 0.71      | 0.44        | 0.47   |
| 39       | 0.61          | 0.64     | 0.74           | 0.72      | 0.44        | 0.46   |
| 40       | 0.61          | 0.64     | 0.74           | 0.72      | 0.44        | 0.46   |
| 41       | 0.60          | 0.63     | 0.75           | 0.72      | 0.43        | 0.46   |
| 42       | 0.60          | 0.63     | 0.75           | 0.73      | 0.43        | 0.45   |
| 43       | 0.60          | 0.63     | 0.76           | 0.73      | 0.43        | 0.45   |
| 44       | 0.59          | 0.62     | 0.76           | 0.74      | 0.42        | 0.44   |
| 45       | 0.59          | 0.62     | 0.77           | 0.74      | 0.42        | 0.44   |
| 46       | 0.59          | 0.61     | 0.77           | 0.75      | 0.42        | 0.43   |
| 47       | 0.58          | 0.61     | 0.77           | 0.75      | 0.41        | 0.43   |
| 48       | 0.58          | 0.60     | 0.78           | 0.75      | 0.41        | 0.43   |
| 49       | 0.57          | 0.60     | 0.78           | 0.76      | 0.40        | 0.43   |
| 50       | 0.57          | 0.59     | 0.79           | 0.76      | 0.40        | 0.42   |
| 51       | 0.56          | 0.59     | 0.79           | 0.77      | 0.39        | 0.42   |
| 52       | 0.56          | 0.58     | 0.80           | 0.77      | 0.39        | 0.41   |
| 53       | 0.55          | 0.58     | 0.80           | 0.78      | 0.38        | 0.41   |
| 54       | 0.55          | 0.57     | 0.81           | 0.78      | 0.38        | 0.40   |
| 55       | 0.54          | 0.56     | 0.81           | 0.79      | 0.37        | 0.39   |
| 56       | 0.53          | 0.56     | 0.81           | 0.79      | 0.37        | 0.39   |
| 57       | 0.53          | 0.55     | 0.82           | 0.80      | 0.37        | 0.38   |
| 58       | 0.52          | 0.54     | 0.82           | 0.80      | 0.36        | 0.38   |
| 59       | 0.51          | 0.54     | 0.83           | 0.81      | 0.35        | 0.37   |
| 60       | 0.51          | 0.53     | 0.84           | 0.81      | 0.35        | 0.37   |
| 61       | 0.50          | 0.52     | 0.84           | 0.82      | 0.34        | 0.36   |
| 62       | 0.49          | 0.51     | 0.85           | 0.82      | 0.33        | 0.35   |
| 63       | 0.48          | 0.51     | 0.85           | 0.83      | 0.33        | 0.35   |

Continued on next page

| $\alpha$ | $\phi_S^\ell$ | $\phi_S$ | $\varphi^\ell$ | $\varphi$ | $\psi^\ell$ | $\psi$ |
|----------|---------------|----------|----------------|-----------|-------------|--------|
| 64       | 0.47          | 0.50     | 0.86           | 0.83      | 0.32        | 0.35   |
| 65       | 0.46          | 0.49     | 0.86           | 0.84      | 0.31        | 0.34   |
| 66       | 0.46          | 0.48     | 0.87           | 0.85      | 0.31        | 0.33   |
| 67       | 0.45          | 0.47     | 0.87           | 0.85      | 0.30        | 0.32   |
| 68       | 0.44          | 0.46     | 0.88           | 0.86      | 0.30        | 0.31   |
| 69       | 0.42          | 0.45     | 0.89           | 0.86      | 0.28        | 0.31   |
| 70       | 0.41          | 0.44     | 0.89           | 0.87      | 0.27        | 0.30   |
| 71       | 0.40          | 0.43     | 0.90           | 0.87      | 0.27        | 0.29   |
| 72       | 0.39          | 0.42     | 0.90           | 0.88      | 0.26        | 0.28   |
| 73       | 0.38          | 0.41     | 0.91           | 0.88      | 0.25        | 0.28   |
| 74       | 0.36          | 0.39     | 0.92           | 0.89      | 0.24        | 0.26   |
| 75       | 0.35          | 0.38     | 0.92           | 0.90      | 0.23        | 0.25   |
| 76       | 0.34          | 0.37     | 0.93           | 0.90      | 0.22        | 0.25   |
| 77       | 0.32          | 0.35     | 0.93           | 0.91      | 0.21        | 0.23   |
| 78       | 0.31          | 0.34     | 0.94           | 0.91      | 0.20        | 0.23   |
| 79       | 0.29          | 0.32     | 0.94           | 0.92      | 0.19        | 0.21   |
| 80       | 0.27          | 0.31     | 0.95           | 0.92      | 0.18        | 0.21   |
| 81       | 0.25          | 0.29     | 0.95           | 0.93      | 0.16        | 0.19   |
| 82       | 0.24          | 0.27     | 0.96           | 0.93      | 0.16        | 0.18   |
| 83       | 0.22          | 0.26     | 0.96           | 0.94      | 0.14        | 0.17   |
| 84       | 0.20          | 0.24     | 0.97           | 0.94      | 0.13        | 0.16   |
| 85       | 0.19          | 0.22     | 0.97           | 0.94      | 0.12        | 0.15   |
| 86       | 0.17          | 0.21     | 0.97           | 0.95      | 0.11        | 0.14   |
| 87       | 0.16          | 0.19     | 0.98           | 0.95      | 0.10        | 0.13   |
| 88       | 0.14          | 0.18     | 0.98           | 0.95      | 0.09        | 0.12   |
| 89       | 0.13          | 0.17     | 0.98           | 0.95      | 0.08        | 0.11   |
| 90       | 0.13          | 0.17     | 0.98           | 0.95      | 0.08        | 0.11   |

Table S114: Reference ( $\phi_S$ ,  $\varphi$ ,  $\psi$ ) and approached ( $\phi_S^\ell$ ,  $\varphi^\ell$ ,  $\psi^\ell$ ) values of the topological descriptors for the first excited-state of the pyridinium-phenolate (PP), computed at the M062X/6-311+G(d,p) level of theory.  $\alpha$  is the pyridinium-phenolate central twist angle amplitude.

| $\alpha$ | $\phi_S^\ell$ | $\phi_S$ | $\varphi^\ell$ | $\varphi$ | $\psi^\ell$ | $\psi$ |
|----------|---------------|----------|----------------|-----------|-------------|--------|
| 0        | 0.66          | 0.71     | 0.66           | 0.62      | 0.50        | 0.54   |
| 1        | 0.66          | 0.71     | 0.66           | 0.63      | 0.50        | 0.54   |
| 2        | 0.66          | 0.71     | 0.66           | 0.63      | 0.50        | 0.54   |
| 3        | 0.66          | 0.71     | 0.66           | 0.63      | 0.50        | 0.54   |
| 4        | 0.66          | 0.71     | 0.66           | 0.63      | 0.50        | 0.54   |
| 5        | 0.66          | 0.71     | 0.66           | 0.63      | 0.50        | 0.54   |
| 6        | 0.66          | 0.71     | 0.66           | 0.63      | 0.50        | 0.54   |
| 7        | 0.66          | 0.71     | 0.66           | 0.63      | 0.50        | 0.54   |
| 8        | 0.66          | 0.70     | 0.66           | 0.63      | 0.50        | 0.53   |
| 9        | 0.66          | 0.70     | 0.66           | 0.63      | 0.50        | 0.53   |
| 10       | 0.65          | 0.70     | 0.67           | 0.63      | 0.49        | 0.53   |
| 11       | 0.65          | 0.70     | 0.67           | 0.64      | 0.49        | 0.53   |
| 12       | 0.65          | 0.70     | 0.67           | 0.64      | 0.49        | 0.53   |
| 13       | 0.65          | 0.70     | 0.67           | 0.64      | 0.49        | 0.53   |
| 14       | 0.65          | 0.70     | 0.67           | 0.64      | 0.49        | 0.53   |
| 15       | 0.65          | 0.70     | 0.67           | 0.64      | 0.49        | 0.53   |
| 16       | 0.65          | 0.70     | 0.67           | 0.64      | 0.49        | 0.53   |
| 17       | 0.65          | 0.69     | 0.68           | 0.65      | 0.49        | 0.52   |
| 18       | 0.65          | 0.69     | 0.68           | 0.65      | 0.49        | 0.52   |
| 19       | 0.65          | 0.69     | 0.68           | 0.65      | 0.49        | 0.52   |
| 20       | 0.65          | 0.69     | 0.68           | 0.65      | 0.49        | 0.52   |
| 21       | 0.64          | 0.69     | 0.69           | 0.66      | 0.48        | 0.51   |
| 22       | 0.64          | 0.69     | 0.69           | 0.66      | 0.48        | 0.51   |
| 23       | 0.64          | 0.68     | 0.69           | 0.66      | 0.48        | 0.51   |
| 24       | 0.64          | 0.68     | 0.69           | 0.66      | 0.48        | 0.51   |
| 25       | 0.64          | 0.68     | 0.70           | 0.67      | 0.47        | 0.50   |
| 26       | 0.64          | 0.68     | 0.70           | 0.67      | 0.47        | 0.50   |
| 27       | 0.64          | 0.67     | 0.70           | 0.67      | 0.47        | 0.50   |
| 28       | 0.63          | 0.67     | 0.70           | 0.68      | 0.47        | 0.50   |
| 29       | 0.63          | 0.67     | 0.71           | 0.68      | 0.46        | 0.50   |
| 30       | 0.63          | 0.67     | 0.71           | 0.68      | 0.46        | 0.50   |
| 31       | 0.63          | 0.66     | 0.71           | 0.69      | 0.46        | 0.49   |

Continued on next page



| $\alpha$ | $\phi_S^\ell$ | $\phi_S$ | $\varphi^\ell$ | $\varphi$ | $\psi^\ell$ | $\psi$ |
|----------|---------------|----------|----------------|-----------|-------------|--------|
| 32       | 0.63          | 0.66     | 0.72           | 0.69      | 0.46        | 0.49   |
| 33       | 0.63          | 0.66     | 0.72           | 0.69      | 0.46        | 0.49   |
| 34       | 0.62          | 0.66     | 0.72           | 0.70      | 0.45        | 0.48   |
| 35       | 0.62          | 0.65     | 0.73           | 0.70      | 0.45        | 0.48   |
| 36       | 0.62          | 0.65     | 0.73           | 0.71      | 0.45        | 0.47   |
| 37       | 0.62          | 0.65     | 0.73           | 0.71      | 0.45        | 0.47   |
| 38       | 0.61          | 0.64     | 0.74           | 0.71      | 0.44        | 0.47   |
| 39       | 0.61          | 0.64     | 0.74           | 0.72      | 0.44        | 0.46   |
| 40       | 0.61          | 0.64     | 0.75           | 0.72      | 0.43        | 0.46   |
| 41       | 0.60          | 0.63     | 0.75           | 0.72      | 0.43        | 0.46   |
| 42       | 0.60          | 0.63     | 0.75           | 0.73      | 0.43        | 0.45   |
| 43       | 0.60          | 0.62     | 0.76           | 0.73      | 0.43        | 0.45   |
| 44       | 0.59          | 0.62     | 0.76           | 0.74      | 0.42        | 0.44   |
| 45       | 0.59          | 0.62     | 0.77           | 0.74      | 0.42        | 0.44   |
| 46       | 0.58          | 0.61     | 0.77           | 0.75      | 0.41        | 0.43   |
| 47       | 0.58          | 0.61     | 0.78           | 0.75      | 0.41        | 0.43   |
| 48       | 0.58          | 0.60     | 0.78           | 0.76      | 0.41        | 0.43   |
| 49       | 0.57          | 0.60     | 0.78           | 0.76      | 0.40        | 0.43   |
| 50       | 0.57          | 0.59     | 0.79           | 0.76      | 0.40        | 0.42   |
| 51       | 0.56          | 0.59     | 0.79           | 0.77      | 0.39        | 0.42   |
| 52       | 0.56          | 0.58     | 0.80           | 0.77      | 0.39        | 0.41   |
| 53       | 0.55          | 0.57     | 0.80           | 0.78      | 0.38        | 0.40   |
| 54       | 0.54          | 0.57     | 0.81           | 0.78      | 0.37        | 0.40   |
| 55       | 0.54          | 0.56     | 0.81           | 0.79      | 0.37        | 0.39   |
| 56       | 0.53          | 0.56     | 0.82           | 0.79      | 0.37        | 0.39   |
| 57       | 0.53          | 0.55     | 0.82           | 0.80      | 0.37        | 0.38   |
| 58       | 0.52          | 0.54     | 0.83           | 0.80      | 0.36        | 0.38   |
| 59       | 0.51          | 0.54     | 0.83           | 0.81      | 0.35        | 0.37   |
| 60       | 0.51          | 0.53     | 0.84           | 0.81      | 0.35        | 0.37   |
| 61       | 0.50          | 0.52     | 0.84           | 0.82      | 0.34        | 0.36   |
| 62       | 0.49          | 0.51     | 0.85           | 0.82      | 0.33        | 0.35   |
| 63       | 0.48          | 0.51     | 0.85           | 0.83      | 0.33        | 0.35   |

Continued on next page

| $\alpha$ | $\phi_S^\ell$ | $\phi_S$ | $\varphi^\ell$ | $\varphi$ | $\psi^\ell$ | $\psi$ |
|----------|---------------|----------|----------------|-----------|-------------|--------|
| 64       | 0.47          | 0.50     | 0.86           | 0.83      | 0.32        | 0.35   |
| 65       | 0.46          | 0.49     | 0.86           | 0.84      | 0.31        | 0.34   |
| 66       | 0.45          | 0.48     | 0.87           | 0.85      | 0.30        | 0.33   |
| 67       | 0.44          | 0.47     | 0.88           | 0.85      | 0.30        | 0.32   |
| 68       | 0.43          | 0.46     | 0.88           | 0.86      | 0.29        | 0.31   |
| 69       | 0.42          | 0.45     | 0.89           | 0.86      | 0.28        | 0.31   |
| 70       | 0.41          | 0.44     | 0.89           | 0.87      | 0.27        | 0.30   |
| 71       | 0.40          | 0.43     | 0.90           | 0.87      | 0.27        | 0.29   |
| 72       | 0.39          | 0.42     | 0.91           | 0.88      | 0.26        | 0.28   |
| 73       | 0.38          | 0.40     | 0.91           | 0.88      | 0.25        | 0.27   |
| 74       | 0.36          | 0.39     | 0.92           | 0.89      | 0.24        | 0.26   |
| 75       | 0.35          | 0.38     | 0.92           | 0.90      | 0.23        | 0.25   |
| 76       | 0.33          | 0.37     | 0.93           | 0.90      | 0.22        | 0.25   |
| 77       | 0.32          | 0.35     | 0.93           | 0.91      | 0.21        | 0.23   |
| 78       | 0.30          | 0.34     | 0.94           | 0.91      | 0.20        | 0.23   |
| 79       | 0.29          | 0.32     | 0.94           | 0.92      | 0.19        | 0.21   |
| 80       | 0.27          | 0.31     | 0.95           | 0.92      | 0.18        | 0.21   |
| 81       | 0.25          | 0.29     | 0.95           | 0.93      | 0.16        | 0.19   |
| 82       | 0.24          | 0.27     | 0.96           | 0.93      | 0.16        | 0.18   |
| 83       | 0.22          | 0.26     | 0.96           | 0.94      | 0.14        | 0.17   |
| 84       | 0.20          | 0.24     | 0.97           | 0.94      | 0.13        | 0.16   |
| 85       | 0.18          | 0.22     | 0.97           | 0.95      | 0.12        | 0.14   |
| 86       | 0.17          | 0.21     | 0.97           | 0.95      | 0.11        | 0.14   |
| 87       | 0.15          | 0.19     | 0.98           | 0.95      | 0.10        | 0.13   |
| 88       | 0.14          | 0.18     | 0.98           | 0.95      | 0.09        | 0.12   |
| 89       | 0.13          | 0.17     | 0.98           | 0.95      | 0.08        | 0.11   |
| 90       | 0.12          | 0.16     | 0.98           | 0.95      | 0.08        | 0.11   |

Table S115: Reference ( $\phi_S$ ,  $\varphi$ ,  $\psi$ ) and approached ( $\phi_S^\ell$ ,  $\varphi^\ell$ ,  $\psi^\ell$ ) values of the topological descriptors for the first excited-state of the pyridinium-phenolate (PP), computed at the M062X/6-311+G(d) level of theory.  $\alpha$  is the pyridinium-phenolate central twist angle amplitude.

| $\alpha$ | $\phi_S^\ell$ | $\phi_S$ | $\varphi^\ell$ | $\varphi$ | $\psi^\ell$ | $\psi$ |
|----------|---------------|----------|----------------|-----------|-------------|--------|
| 0        | 0.68          | 0.72     | 0.65           | 0.61      | 0.51        | 0.55   |
| 1        | 0.68          | 0.72     | 0.65           | 0.61      | 0.51        | 0.55   |
| 2        | 0.68          | 0.72     | 0.65           | 0.61      | 0.51        | 0.55   |
| 3        | 0.68          | 0.72     | 0.65           | 0.61      | 0.51        | 0.55   |
| 4        | 0.68          | 0.72     | 0.65           | 0.61      | 0.51        | 0.55   |
| 5        | 0.68          | 0.72     | 0.65           | 0.62      | 0.51        | 0.55   |
| 6        | 0.68          | 0.72     | 0.65           | 0.62      | 0.51        | 0.55   |
| 7        | 0.68          | 0.72     | 0.65           | 0.62      | 0.51        | 0.55   |
| 8        | 0.68          | 0.72     | 0.66           | 0.62      | 0.51        | 0.55   |
| 9        | 0.68          | 0.72     | 0.66           | 0.62      | 0.51        | 0.55   |
| 10       | 0.68          | 0.72     | 0.66           | 0.62      | 0.51        | 0.55   |
| 11       | 0.68          | 0.72     | 0.66           | 0.62      | 0.51        | 0.55   |
| 12       | 0.68          | 0.72     | 0.66           | 0.62      | 0.51        | 0.55   |
| 13       | 0.68          | 0.72     | 0.66           | 0.63      | 0.51        | 0.54   |
| 14       | 0.68          | 0.71     | 0.66           | 0.63      | 0.51        | 0.54   |
| 15       | 0.67          | 0.71     | 0.66           | 0.63      | 0.50        | 0.54   |
| 16       | 0.67          | 0.71     | 0.67           | 0.63      | 0.50        | 0.54   |
| 17       | 0.67          | 0.71     | 0.67           | 0.63      | 0.50        | 0.54   |
| 18       | 0.67          | 0.71     | 0.67           | 0.64      | 0.50        | 0.53   |
| 19       | 0.67          | 0.71     | 0.67           | 0.64      | 0.50        | 0.53   |
| 20       | 0.67          | 0.71     | 0.67           | 0.64      | 0.50        | 0.53   |
| 21       | 0.67          | 0.70     | 0.68           | 0.64      | 0.50        | 0.53   |
| 22       | 0.66          | 0.70     | 0.68           | 0.65      | 0.49        | 0.52   |
| 23       | 0.66          | 0.70     | 0.68           | 0.65      | 0.49        | 0.52   |
| 24       | 0.66          | 0.70     | 0.68           | 0.65      | 0.49        | 0.52   |
| 25       | 0.66          | 0.70     | 0.69           | 0.66      | 0.49        | 0.52   |
| 26       | 0.66          | 0.69     | 0.69           | 0.66      | 0.49        | 0.51   |
| 27       | 0.66          | 0.69     | 0.69           | 0.66      | 0.49        | 0.51   |
| 28       | 0.65          | 0.69     | 0.70           | 0.67      | 0.48        | 0.51   |
| 29       | 0.65          | 0.69     | 0.70           | 0.67      | 0.48        | 0.51   |
| 30       | 0.65          | 0.68     | 0.70           | 0.67      | 0.48        | 0.50   |
| 31       | 0.65          | 0.68     | 0.70           | 0.68      | 0.48        | 0.50   |

Continued on next page

| $\alpha$ | $\phi_S^\ell$ | $\phi_S$ | $\varphi^\ell$ | $\varphi$ | $\psi^\ell$ | $\psi$ |
|----------|---------------|----------|----------------|-----------|-------------|--------|
| 32       | 0.65          | 0.68     | 0.71           | 0.68      | 0.47        | 0.50   |
| 33       | 0.65          | 0.67     | 0.71           | 0.68      | 0.47        | 0.50   |
| 34       | 0.64          | 0.67     | 0.71           | 0.69      | 0.47        | 0.49   |
| 35       | 0.64          | 0.67     | 0.72           | 0.69      | 0.46        | 0.49   |
| 36       | 0.64          | 0.67     | 0.72           | 0.69      | 0.46        | 0.49   |
| 37       | 0.64          | 0.66     | 0.72           | 0.70      | 0.46        | 0.48   |
| 38       | 0.63          | 0.66     | 0.73           | 0.70      | 0.45        | 0.48   |
| 39       | 0.63          | 0.65     | 0.73           | 0.71      | 0.45        | 0.47   |
| 40       | 0.63          | 0.65     | 0.74           | 0.71      | 0.45        | 0.47   |
| 41       | 0.62          | 0.65     | 0.74           | 0.71      | 0.44        | 0.47   |
| 42       | 0.62          | 0.64     | 0.75           | 0.72      | 0.44        | 0.46   |
| 43       | 0.62          | 0.64     | 0.75           | 0.72      | 0.44        | 0.46   |
| 44       | 0.61          | 0.64     | 0.75           | 0.73      | 0.43        | 0.46   |
| 45       | 0.61          | 0.63     | 0.76           | 0.73      | 0.43        | 0.45   |
| 46       | 0.60          | 0.63     | 0.76           | 0.74      | 0.43        | 0.45   |
| 47       | 0.60          | 0.62     | 0.77           | 0.74      | 0.42        | 0.44   |
| 48       | 0.60          | 0.62     | 0.77           | 0.75      | 0.42        | 0.44   |
| 49       | 0.59          | 0.61     | 0.78           | 0.75      | 0.41        | 0.43   |
| 50       | 0.59          | 0.61     | 0.78           | 0.75      | 0.41        | 0.43   |
| 51       | 0.58          | 0.60     | 0.78           | 0.76      | 0.41        | 0.43   |
| 52       | 0.58          | 0.60     | 0.79           | 0.76      | 0.40        | 0.43   |
| 53       | 0.57          | 0.59     | 0.79           | 0.77      | 0.40        | 0.42   |
| 54       | 0.56          | 0.58     | 0.80           | 0.77      | 0.39        | 0.41   |
| 55       | 0.56          | 0.58     | 0.80           | 0.78      | 0.39        | 0.41   |
| 56       | 0.55          | 0.57     | 0.81           | 0.78      | 0.38        | 0.40   |
| 57       | 0.55          | 0.57     | 0.81           | 0.79      | 0.38        | 0.40   |
| 58       | 0.54          | 0.56     | 0.82           | 0.79      | 0.37        | 0.39   |
| 59       | 0.53          | 0.55     | 0.82           | 0.80      | 0.37        | 0.38   |
| 60       | 0.53          | 0.55     | 0.83           | 0.80      | 0.36        | 0.38   |
| 61       | 0.52          | 0.54     | 0.83           | 0.81      | 0.36        | 0.37   |
| 62       | 0.51          | 0.53     | 0.84           | 0.81      | 0.35        | 0.37   |
| 63       | 0.50          | 0.52     | 0.84           | 0.82      | 0.34        | 0.36   |

Continued on next page

| $\alpha$ | $\phi_S^\ell$ | $\phi_S$ | $\varphi^\ell$ | $\varphi$ | $\psi^\ell$ | $\psi$ |
|----------|---------------|----------|----------------|-----------|-------------|--------|
| 64       | 0.49          | 0.51     | 0.85           | 0.83      | 0.33        | 0.35   |
| 65       | 0.48          | 0.51     | 0.86           | 0.83      | 0.32        | 0.35   |
| 66       | 0.47          | 0.50     | 0.86           | 0.84      | 0.32        | 0.34   |
| 67       | 0.47          | 0.49     | 0.87           | 0.84      | 0.32        | 0.34   |
| 68       | 0.45          | 0.48     | 0.87           | 0.85      | 0.30        | 0.33   |
| 69       | 0.44          | 0.47     | 0.88           | 0.85      | 0.30        | 0.32   |
| 70       | 0.43          | 0.46     | 0.89           | 0.86      | 0.29        | 0.31   |
| 71       | 0.42          | 0.45     | 0.89           | 0.87      | 0.28        | 0.30   |
| 72       | 0.41          | 0.43     | 0.90           | 0.87      | 0.27        | 0.29   |
| 73       | 0.40          | 0.42     | 0.90           | 0.88      | 0.27        | 0.28   |
| 74       | 0.38          | 0.41     | 0.91           | 0.88      | 0.25        | 0.28   |
| 75       | 0.37          | 0.40     | 0.92           | 0.89      | 0.24        | 0.27   |
| 76       | 0.35          | 0.38     | 0.92           | 0.89      | 0.23        | 0.26   |
| 77       | 0.34          | 0.37     | 0.93           | 0.90      | 0.22        | 0.25   |
| 78       | 0.32          | 0.35     | 0.93           | 0.91      | 0.21        | 0.23   |
| 79       | 0.31          | 0.34     | 0.94           | 0.91      | 0.20        | 0.23   |
| 80       | 0.29          | 0.32     | 0.95           | 0.92      | 0.19        | 0.21   |
| 81       | 0.27          | 0.31     | 0.95           | 0.92      | 0.18        | 0.21   |
| 82       | 0.25          | 0.29     | 0.96           | 0.93      | 0.16        | 0.19   |
| 83       | 0.23          | 0.27     | 0.96           | 0.93      | 0.15        | 0.18   |
| 84       | 0.21          | 0.25     | 0.97           | 0.94      | 0.14        | 0.17   |
| 85       | 0.19          | 0.23     | 0.97           | 0.94      | 0.12        | 0.15   |
| 86       | 0.17          | 0.21     | 0.98           | 0.95      | 0.11        | 0.14   |
| 87       | 0.15          | 0.20     | 0.98           | 0.95      | 0.10        | 0.13   |
| 88       | 0.13          | 0.18     | 0.98           | 0.95      | 0.08        | 0.12   |
| 89       | 0.12          | 0.17     | 0.98           | 0.95      | 0.08        | 0.11   |
| 90       | 0.11          | 0.16     | 0.98           | 0.95      | 0.07        | 0.11   |

Table S116: Reference ( $\phi_S$ ,  $\varphi$ ,  $\psi$ ) and approached ( $\phi_S^\ell$ ,  $\varphi^\ell$ ,  $\psi^\ell$ ) values of the topological descriptors for the first excited-state of the pyridinium-phenolate (PP), computed at the M062X/6-311G(d) level of theory.  $\alpha$  is the pyridinium-phenolate central twist angle amplitude.

| $\alpha$ | $\phi_S^\ell$ | $\phi_S$ | $\varphi^\ell$ | $\varphi$ | $\psi^\ell$ | $\psi$ |
|----------|---------------|----------|----------------|-----------|-------------|--------|
| 0        | 0.66          | 0.71     | 0.66           | 0.63      | 0.50        | 0.54   |
| 1        | 0.66          | 0.71     | 0.66           | 0.63      | 0.50        | 0.54   |
| 2        | 0.66          | 0.71     | 0.66           | 0.63      | 0.50        | 0.54   |
| 3        | 0.66          | 0.71     | 0.66           | 0.63      | 0.50        | 0.54   |
| 4        | 0.66          | 0.70     | 0.66           | 0.63      | 0.50        | 0.53   |
| 5        | 0.66          | 0.70     | 0.66           | 0.63      | 0.50        | 0.53   |
| 6        | 0.66          | 0.70     | 0.66           | 0.63      | 0.50        | 0.53   |
| 7        | 0.66          | 0.70     | 0.66           | 0.63      | 0.50        | 0.53   |
| 8        | 0.66          | 0.70     | 0.66           | 0.63      | 0.50        | 0.53   |
| 9        | 0.66          | 0.70     | 0.66           | 0.64      | 0.50        | 0.53   |
| 10       | 0.66          | 0.70     | 0.66           | 0.64      | 0.50        | 0.53   |
| 11       | 0.66          | 0.70     | 0.66           | 0.64      | 0.50        | 0.53   |
| 12       | 0.66          | 0.70     | 0.67           | 0.64      | 0.50        | 0.53   |
| 13       | 0.66          | 0.70     | 0.67           | 0.64      | 0.50        | 0.53   |
| 14       | 0.66          | 0.69     | 0.67           | 0.64      | 0.50        | 0.52   |
| 15       | 0.66          | 0.69     | 0.67           | 0.65      | 0.50        | 0.52   |
| 16       | 0.65          | 0.69     | 0.67           | 0.65      | 0.49        | 0.52   |
| 17       | 0.65          | 0.69     | 0.67           | 0.65      | 0.49        | 0.52   |
| 18       | 0.65          | 0.69     | 0.68           | 0.65      | 0.49        | 0.52   |
| 19       | 0.65          | 0.69     | 0.68           | 0.65      | 0.49        | 0.52   |
| 20       | 0.65          | 0.69     | 0.68           | 0.66      | 0.49        | 0.51   |
| 21       | 0.65          | 0.68     | 0.68           | 0.66      | 0.49        | 0.51   |
| 22       | 0.65          | 0.68     | 0.69           | 0.66      | 0.48        | 0.51   |
| 23       | 0.65          | 0.68     | 0.69           | 0.66      | 0.48        | 0.51   |
| 24       | 0.65          | 0.68     | 0.69           | 0.67      | 0.48        | 0.50   |
| 25       | 0.64          | 0.68     | 0.69           | 0.67      | 0.48        | 0.50   |
| 26       | 0.64          | 0.67     | 0.70           | 0.67      | 0.47        | 0.50   |
| 27       | 0.64          | 0.67     | 0.70           | 0.68      | 0.47        | 0.50   |
| 28       | 0.64          | 0.67     | 0.70           | 0.68      | 0.47        | 0.50   |
| 29       | 0.64          | 0.67     | 0.70           | 0.68      | 0.47        | 0.50   |
| 30       | 0.64          | 0.67     | 0.71           | 0.69      | 0.47        | 0.49   |
| 31       | 0.64          | 0.66     | 0.71           | 0.69      | 0.47        | 0.49   |

Continued on next page

| $\alpha$ | $\phi_S^\ell$ | $\phi_S$ | $\varphi^\ell$ | $\varphi$ | $\psi^\ell$ | $\psi$ |
|----------|---------------|----------|----------------|-----------|-------------|--------|
| 32       | 0.63          | 0.66     | 0.71           | 0.69      | 0.46        | 0.49   |
| 33       | 0.63          | 0.66     | 0.72           | 0.70      | 0.46        | 0.48   |
| 34       | 0.63          | 0.65     | 0.72           | 0.70      | 0.46        | 0.48   |
| 35       | 0.63          | 0.65     | 0.72           | 0.70      | 0.46        | 0.48   |
| 36       | 0.62          | 0.65     | 0.73           | 0.71      | 0.45        | 0.47   |
| 37       | 0.62          | 0.65     | 0.73           | 0.71      | 0.45        | 0.47   |
| 38       | 0.62          | 0.64     | 0.73           | 0.71      | 0.45        | 0.47   |
| 39       | 0.62          | 0.64     | 0.74           | 0.72      | 0.44        | 0.46   |
| 40       | 0.61          | 0.64     | 0.74           | 0.72      | 0.44        | 0.46   |
| 41       | 0.61          | 0.63     | 0.75           | 0.73      | 0.43        | 0.45   |
| 42       | 0.61          | 0.63     | 0.75           | 0.73      | 0.43        | 0.45   |
| 43       | 0.60          | 0.62     | 0.75           | 0.73      | 0.43        | 0.45   |
| 44       | 0.60          | 0.62     | 0.76           | 0.74      | 0.43        | 0.44   |
| 45       | 0.60          | 0.62     | 0.76           | 0.74      | 0.43        | 0.44   |
| 46       | 0.59          | 0.61     | 0.77           | 0.75      | 0.42        | 0.43   |
| 47       | 0.59          | 0.61     | 0.77           | 0.75      | 0.42        | 0.43   |
| 48       | 0.58          | 0.60     | 0.78           | 0.76      | 0.41        | 0.43   |
| 49       | 0.58          | 0.60     | 0.78           | 0.76      | 0.41        | 0.43   |
| 50       | 0.57          | 0.59     | 0.79           | 0.77      | 0.40        | 0.42   |
| 51       | 0.57          | 0.59     | 0.79           | 0.77      | 0.40        | 0.42   |
| 52       | 0.56          | 0.58     | 0.79           | 0.77      | 0.39        | 0.41   |
| 53       | 0.56          | 0.58     | 0.80           | 0.78      | 0.39        | 0.41   |
| 54       | 0.55          | 0.57     | 0.80           | 0.78      | 0.38        | 0.40   |
| 55       | 0.55          | 0.57     | 0.81           | 0.79      | 0.38        | 0.40   |
| 56       | 0.54          | 0.56     | 0.81           | 0.79      | 0.37        | 0.39   |
| 57       | 0.53          | 0.55     | 0.82           | 0.80      | 0.37        | 0.38   |
| 58       | 0.53          | 0.55     | 0.82           | 0.80      | 0.37        | 0.38   |
| 59       | 0.52          | 0.54     | 0.83           | 0.81      | 0.36        | 0.37   |
| 60       | 0.51          | 0.53     | 0.83           | 0.81      | 0.35        | 0.37   |
| 61       | 0.51          | 0.52     | 0.84           | 0.82      | 0.35        | 0.36   |
| 62       | 0.50          | 0.52     | 0.84           | 0.82      | 0.34        | 0.36   |
| 63       | 0.49          | 0.51     | 0.85           | 0.83      | 0.33        | 0.35   |

Continued on next page

| $\alpha$ | $\phi_S^\ell$ | $\phi_S$ | $\varphi^\ell$ | $\varphi$ | $\psi^\ell$ | $\psi$ |
|----------|---------------|----------|----------------|-----------|-------------|--------|
| 64       | 0.48          | 0.50     | 0.86           | 0.83      | 0.32        | 0.35   |
| 65       | 0.47          | 0.49     | 0.86           | 0.84      | 0.32        | 0.34   |
| 66       | 0.46          | 0.48     | 0.87           | 0.85      | 0.31        | 0.33   |
| 67       | 0.45          | 0.47     | 0.87           | 0.85      | 0.30        | 0.32   |
| 68       | 0.44          | 0.46     | 0.88           | 0.86      | 0.30        | 0.31   |
| 69       | 0.43          | 0.45     | 0.89           | 0.86      | 0.29        | 0.31   |
| 70       | 0.42          | 0.44     | 0.89           | 0.87      | 0.28        | 0.30   |
| 71       | 0.41          | 0.43     | 0.90           | 0.87      | 0.27        | 0.29   |
| 72       | 0.40          | 0.42     | 0.90           | 0.88      | 0.27        | 0.28   |
| 73       | 0.38          | 0.41     | 0.91           | 0.88      | 0.25        | 0.28   |
| 74       | 0.37          | 0.40     | 0.92           | 0.89      | 0.24        | 0.27   |
| 75       | 0.36          | 0.38     | 0.92           | 0.90      | 0.24        | 0.25   |
| 76       | 0.34          | 0.37     | 0.93           | 0.90      | 0.22        | 0.25   |
| 77       | 0.32          | 0.36     | 0.93           | 0.91      | 0.21        | 0.24   |
| 78       | 0.31          | 0.34     | 0.94           | 0.91      | 0.20        | 0.23   |
| 79       | 0.29          | 0.33     | 0.95           | 0.92      | 0.19        | 0.22   |
| 80       | 0.27          | 0.31     | 0.95           | 0.92      | 0.18        | 0.21   |
| 81       | 0.25          | 0.29     | 0.96           | 0.93      | 0.16        | 0.19   |
| 82       | 0.24          | 0.28     | 0.96           | 0.93      | 0.16        | 0.19   |
| 83       | 0.22          | 0.26     | 0.97           | 0.94      | 0.14        | 0.17   |
| 84       | 0.20          | 0.24     | 0.97           | 0.94      | 0.13        | 0.16   |
| 85       | 0.18          | 0.22     | 0.98           | 0.95      | 0.12        | 0.14   |
| 86       | 0.16          | 0.20     | 0.98           | 0.95      | 0.10        | 0.13   |
| 87       | 0.14          | 0.19     | 0.98           | 0.95      | 0.09        | 0.13   |
| 88       | 0.13          | 0.17     | 0.99           | 0.96      | 0.08        | 0.11   |
| 89       | 0.11          | 0.16     | 0.99           | 0.96      | 0.07        | 0.11   |
| 90       | 0.11          | 0.15     | 0.99           | 0.96      | 0.07        | 0.10   |

Table S117: Reference ( $\phi_S$ ,  $\varphi$ ,  $\psi$ ) and approached ( $\phi_S^\ell$ ,  $\varphi^\ell$ ,  $\psi^\ell$ ) values of the topological descriptors for the first excited-state of the pyridinium-phenolate (PP), computed at the M062X/6-311+G level of theory.  $\alpha$  is the pyridinium-phenolate central twist angle amplitude.



| $\alpha$ | $\phi_S^\ell$ | $\phi_S$ | $\varphi^\ell$ | $\varphi$ | $\psi^\ell$ | $\psi$ |
|----------|---------------|----------|----------------|-----------|-------------|--------|
| 0        | 0.69          | 0.72     | 0.65           | 0.62      | 0.52        | 0.55   |
| 1        | 0.69          | 0.72     | 0.65           | 0.62      | 0.52        | 0.55   |
| 2        | 0.69          | 0.72     | 0.65           | 0.62      | 0.52        | 0.55   |
| 3        | 0.69          | 0.72     | 0.65           | 0.62      | 0.52        | 0.55   |
| 4        | 0.69          | 0.72     | 0.65           | 0.62      | 0.52        | 0.55   |
| 5        | 0.69          | 0.72     | 0.65           | 0.62      | 0.52        | 0.55   |
| 6        | 0.69          | 0.72     | 0.65           | 0.62      | 0.52        | 0.55   |
| 7        | 0.69          | 0.72     | 0.65           | 0.62      | 0.52        | 0.55   |
| 8        | 0.68          | 0.72     | 0.65           | 0.62      | 0.51        | 0.55   |
| 9        | 0.68          | 0.72     | 0.65           | 0.62      | 0.51        | 0.55   |
| 10       | 0.68          | 0.72     | 0.66           | 0.63      | 0.51        | 0.54   |
| 11       | 0.68          | 0.71     | 0.66           | 0.63      | 0.51        | 0.54   |
| 12       | 0.68          | 0.71     | 0.66           | 0.63      | 0.51        | 0.54   |
| 13       | 0.68          | 0.71     | 0.66           | 0.63      | 0.51        | 0.54   |
| 14       | 0.68          | 0.71     | 0.66           | 0.63      | 0.51        | 0.54   |
| 15       | 0.68          | 0.71     | 0.66           | 0.63      | 0.51        | 0.54   |
| 16       | 0.68          | 0.71     | 0.66           | 0.64      | 0.51        | 0.53   |
| 17       | 0.68          | 0.71     | 0.67           | 0.64      | 0.50        | 0.53   |
| 18       | 0.67          | 0.71     | 0.67           | 0.64      | 0.50        | 0.53   |
| 19       | 0.67          | 0.70     | 0.67           | 0.64      | 0.50        | 0.53   |
| 20       | 0.67          | 0.70     | 0.67           | 0.65      | 0.50        | 0.52   |
| 21       | 0.67          | 0.70     | 0.67           | 0.65      | 0.50        | 0.52   |
| 22       | 0.67          | 0.70     | 0.68           | 0.65      | 0.50        | 0.52   |
| 23       | 0.67          | 0.70     | 0.68           | 0.65      | 0.50        | 0.52   |
| 24       | 0.67          | 0.69     | 0.68           | 0.66      | 0.50        | 0.51   |
| 25       | 0.66          | 0.69     | 0.69           | 0.66      | 0.49        | 0.51   |
| 26       | 0.66          | 0.69     | 0.69           | 0.66      | 0.49        | 0.51   |
| 27       | 0.66          | 0.69     | 0.69           | 0.67      | 0.49        | 0.51   |
| 28       | 0.66          | 0.69     | 0.69           | 0.67      | 0.49        | 0.51   |
| 29       | 0.66          | 0.68     | 0.70           | 0.67      | 0.48        | 0.50   |
| 30       | 0.66          | 0.68     | 0.70           | 0.68      | 0.48        | 0.50   |
| 31       | 0.66          | 0.68     | 0.70           | 0.68      | 0.48        | 0.50   |

Continued on next page

| $\alpha$ | $\phi_S^\ell$ | $\phi_S$ | $\varphi^\ell$ | $\varphi$ | $\psi^\ell$ | $\psi$ |
|----------|---------------|----------|----------------|-----------|-------------|--------|
| 32       | 0.65          | 0.68     | 0.70           | 0.68      | 0.48        | 0.50   |
| 33       | 0.65          | 0.67     | 0.71           | 0.69      | 0.47        | 0.49   |
| 34       | 0.65          | 0.67     | 0.71           | 0.69      | 0.47        | 0.49   |
| 35       | 0.65          | 0.67     | 0.71           | 0.69      | 0.47        | 0.49   |
| 36       | 0.64          | 0.66     | 0.72           | 0.70      | 0.46        | 0.48   |
| 37       | 0.64          | 0.66     | 0.72           | 0.70      | 0.46        | 0.48   |
| 38       | 0.64          | 0.66     | 0.73           | 0.70      | 0.46        | 0.48   |
| 39       | 0.64          | 0.65     | 0.73           | 0.71      | 0.46        | 0.47   |
| 40       | 0.63          | 0.65     | 0.73           | 0.71      | 0.45        | 0.47   |
| 41       | 0.63          | 0.65     | 0.74           | 0.72      | 0.45        | 0.47   |
| 42       | 0.63          | 0.64     | 0.74           | 0.72      | 0.45        | 0.46   |
| 43       | 0.62          | 0.64     | 0.75           | 0.72      | 0.44        | 0.46   |
| 44       | 0.62          | 0.63     | 0.75           | 0.73      | 0.44        | 0.45   |
| 45       | 0.62          | 0.63     | 0.75           | 0.73      | 0.44        | 0.45   |
| 46       | 0.61          | 0.63     | 0.76           | 0.74      | 0.43        | 0.45   |
| 47       | 0.61          | 0.62     | 0.76           | 0.74      | 0.43        | 0.44   |
| 48       | 0.60          | 0.62     | 0.77           | 0.75      | 0.42        | 0.44   |
| 49       | 0.60          | 0.61     | 0.77           | 0.75      | 0.42        | 0.43   |
| 50       | 0.59          | 0.61     | 0.78           | 0.76      | 0.41        | 0.43   |
| 51       | 0.59          | 0.60     | 0.78           | 0.76      | 0.41        | 0.43   |
| 52       | 0.58          | 0.60     | 0.79           | 0.76      | 0.40        | 0.43   |
| 53       | 0.58          | 0.59     | 0.79           | 0.77      | 0.40        | 0.42   |
| 54       | 0.57          | 0.59     | 0.79           | 0.77      | 0.40        | 0.42   |
| 55       | 0.57          | 0.58     | 0.80           | 0.78      | 0.39        | 0.41   |
| 56       | 0.56          | 0.57     | 0.80           | 0.78      | 0.39        | 0.40   |
| 57       | 0.55          | 0.57     | 0.81           | 0.79      | 0.38        | 0.40   |
| 58       | 0.55          | 0.56     | 0.81           | 0.79      | 0.38        | 0.39   |
| 59       | 0.54          | 0.55     | 0.82           | 0.80      | 0.37        | 0.38   |
| 60       | 0.53          | 0.55     | 0.83           | 0.80      | 0.36        | 0.38   |
| 61       | 0.53          | 0.54     | 0.83           | 0.81      | 0.36        | 0.37   |
| 62       | 0.52          | 0.53     | 0.84           | 0.81      | 0.35        | 0.37   |
| 63       | 0.51          | 0.53     | 0.84           | 0.82      | 0.35        | 0.37   |

Continued on next page

| $\alpha$ | $\phi_S^\ell$ | $\phi_S$ | $\varphi^\ell$ | $\varphi$ | $\psi^\ell$ | $\psi$ |
|----------|---------------|----------|----------------|-----------|-------------|--------|
| 64       | 0.50          | 0.52     | 0.85           | 0.83      | 0.34        | 0.36   |
| 65       | 0.49          | 0.51     | 0.85           | 0.83      | 0.33        | 0.35   |
| 66       | 0.48          | 0.50     | 0.86           | 0.84      | 0.32        | 0.34   |
| 67       | 0.47          | 0.49     | 0.87           | 0.84      | 0.32        | 0.34   |
| 68       | 0.46          | 0.48     | 0.87           | 0.85      | 0.31        | 0.33   |
| 69       | 0.45          | 0.47     | 0.88           | 0.85      | 0.30        | 0.32   |
| 70       | 0.44          | 0.46     | 0.88           | 0.86      | 0.30        | 0.31   |
| 71       | 0.43          | 0.45     | 0.89           | 0.86      | 0.29        | 0.31   |
| 72       | 0.42          | 0.44     | 0.90           | 0.87      | 0.28        | 0.30   |
| 73       | 0.40          | 0.43     | 0.90           | 0.88      | 0.27        | 0.29   |
| 74       | 0.39          | 0.42     | 0.91           | 0.88      | 0.26        | 0.28   |
| 75       | 0.38          | 0.40     | 0.92           | 0.89      | 0.25        | 0.27   |
| 76       | 0.36          | 0.39     | 0.92           | 0.89      | 0.24        | 0.26   |
| 77       | 0.34          | 0.37     | 0.93           | 0.90      | 0.22        | 0.25   |
| 78       | 0.33          | 0.36     | 0.93           | 0.91      | 0.22        | 0.24   |
| 79       | 0.31          | 0.34     | 0.94           | 0.91      | 0.20        | 0.23   |
| 80       | 0.29          | 0.33     | 0.95           | 0.92      | 0.19        | 0.22   |
| 81       | 0.27          | 0.31     | 0.95           | 0.92      | 0.18        | 0.21   |
| 82       | 0.25          | 0.29     | 0.96           | 0.93      | 0.16        | 0.19   |
| 83       | 0.23          | 0.27     | 0.97           | 0.94      | 0.15        | 0.18   |
| 84       | 0.21          | 0.25     | 0.97           | 0.94      | 0.14        | 0.17   |
| 85       | 0.18          | 0.23     | 0.98           | 0.95      | 0.12        | 0.15   |
| 86       | 0.16          | 0.21     | 0.98           | 0.95      | 0.10        | 0.14   |
| 87       | 0.14          | 0.19     | 0.99           | 0.95      | 0.09        | 0.13   |
| 88       | 0.12          | 0.17     | 0.99           | 0.96      | 0.08        | 0.11   |
| 89       | 0.10          | 0.16     | 0.99           | 0.96      | 0.06        | 0.11   |
| 90       | 0.10          | 0.15     | 0.99           | 0.96      | 0.06        | 0.10   |

Table S118: Reference ( $\phi_S$ ,  $\varphi$ ,  $\psi$ ) and approached ( $\phi_S^\ell$ ,  $\varphi^\ell$ ,  $\psi^\ell$ ) values of the topological descriptors for the first excited-state of the pyridinium-phenolate (PP), computed at the M062X/6-311G level of theory.  $\alpha$  is the pyridinium-phenolate central twist angle amplitude.

| $\alpha$ | $\phi_S^\ell$ | $\phi_S$ | $\varphi^\ell$ | $\varphi$ | $\psi^\ell$ | $\psi$ |
|----------|---------------|----------|----------------|-----------|-------------|--------|
| 0        | 0.66          | 0.71     | 0.66           | 0.63      | 0.50        | 0.54   |
| 1        | 0.66          | 0.71     | 0.66           | 0.63      | 0.50        | 0.54   |
| 2        | 0.66          | 0.71     | 0.66           | 0.63      | 0.50        | 0.54   |
| 3        | 0.66          | 0.71     | 0.66           | 0.63      | 0.50        | 0.54   |
| 4        | 0.66          | 0.71     | 0.66           | 0.63      | 0.50        | 0.54   |
| 5        | 0.66          | 0.71     | 0.66           | 0.63      | 0.50        | 0.54   |
| 6        | 0.66          | 0.70     | 0.67           | 0.63      | 0.50        | 0.53   |
| 7        | 0.66          | 0.70     | 0.67           | 0.63      | 0.50        | 0.53   |
| 8        | 0.66          | 0.70     | 0.67           | 0.63      | 0.50        | 0.53   |
| 9        | 0.66          | 0.70     | 0.67           | 0.63      | 0.50        | 0.53   |
| 10       | 0.66          | 0.70     | 0.67           | 0.63      | 0.50        | 0.53   |
| 11       | 0.65          | 0.70     | 0.67           | 0.64      | 0.49        | 0.53   |
| 12       | 0.65          | 0.70     | 0.67           | 0.64      | 0.49        | 0.53   |
| 13       | 0.65          | 0.70     | 0.67           | 0.64      | 0.49        | 0.53   |
| 14       | 0.65          | 0.70     | 0.67           | 0.64      | 0.49        | 0.53   |
| 15       | 0.65          | 0.70     | 0.68           | 0.64      | 0.49        | 0.53   |
| 16       | 0.65          | 0.69     | 0.68           | 0.65      | 0.49        | 0.52   |
| 17       | 0.65          | 0.69     | 0.68           | 0.65      | 0.49        | 0.52   |
| 18       | 0.65          | 0.69     | 0.68           | 0.65      | 0.49        | 0.52   |
| 19       | 0.65          | 0.69     | 0.68           | 0.65      | 0.49        | 0.52   |
| 20       | 0.65          | 0.69     | 0.69           | 0.65      | 0.48        | 0.52   |
| 21       | 0.64          | 0.69     | 0.69           | 0.66      | 0.48        | 0.51   |
| 22       | 0.64          | 0.68     | 0.69           | 0.66      | 0.48        | 0.51   |
| 23       | 0.64          | 0.68     | 0.69           | 0.66      | 0.48        | 0.51   |
| 24       | 0.64          | 0.68     | 0.70           | 0.67      | 0.47        | 0.50   |
| 25       | 0.64          | 0.68     | 0.70           | 0.67      | 0.47        | 0.50   |
| 26       | 0.64          | 0.68     | 0.70           | 0.67      | 0.47        | 0.50   |
| 27       | 0.64          | 0.67     | 0.71           | 0.67      | 0.47        | 0.50   |
| 28       | 0.63          | 0.67     | 0.71           | 0.68      | 0.46        | 0.50   |
| 29       | 0.63          | 0.67     | 0.71           | 0.68      | 0.46        | 0.50   |
| 30       | 0.63          | 0.67     | 0.71           | 0.68      | 0.46        | 0.50   |
| 31       | 0.63          | 0.66     | 0.72           | 0.69      | 0.46        | 0.49   |

Continued on next page

| $\alpha$ | $\phi_S^\ell$ | $\phi_S$ | $\varphi^\ell$ | $\varphi$ | $\psi^\ell$ | $\psi$ |
|----------|---------------|----------|----------------|-----------|-------------|--------|
| 32       | 0.63          | 0.66     | 0.72           | 0.69      | 0.46        | 0.49   |
| 33       | 0.62          | 0.66     | 0.72           | 0.69      | 0.45        | 0.49   |
| 34       | 0.62          | 0.65     | 0.73           | 0.70      | 0.45        | 0.48   |
| 35       | 0.62          | 0.65     | 0.73           | 0.70      | 0.45        | 0.48   |
| 36       | 0.62          | 0.65     | 0.73           | 0.71      | 0.45        | 0.47   |
| 37       | 0.61          | 0.65     | 0.74           | 0.71      | 0.44        | 0.47   |
| 38       | 0.61          | 0.64     | 0.74           | 0.71      | 0.44        | 0.47   |
| 39       | 0.61          | 0.64     | 0.75           | 0.72      | 0.43        | 0.46   |
| 40       | 0.60          | 0.63     | 0.75           | 0.72      | 0.43        | 0.46   |
| 41       | 0.60          | 0.63     | 0.75           | 0.73      | 0.43        | 0.45   |
| 42       | 0.60          | 0.63     | 0.76           | 0.73      | 0.43        | 0.45   |
| 43       | 0.59          | 0.62     | 0.76           | 0.73      | 0.42        | 0.45   |
| 44       | 0.59          | 0.62     | 0.77           | 0.74      | 0.42        | 0.44   |
| 45       | 0.59          | 0.61     | 0.77           | 0.74      | 0.42        | 0.44   |
| 46       | 0.58          | 0.61     | 0.77           | 0.75      | 0.41        | 0.43   |
| 47       | 0.58          | 0.61     | 0.78           | 0.75      | 0.41        | 0.43   |
| 48       | 0.57          | 0.60     | 0.78           | 0.76      | 0.40        | 0.43   |
| 49       | 0.57          | 0.60     | 0.79           | 0.76      | 0.40        | 0.43   |
| 50       | 0.56          | 0.59     | 0.79           | 0.77      | 0.39        | 0.42   |
| 51       | 0.56          | 0.59     | 0.80           | 0.77      | 0.39        | 0.42   |
| 52       | 0.55          | 0.58     | 0.80           | 0.77      | 0.38        | 0.41   |
| 53       | 0.55          | 0.57     | 0.80           | 0.78      | 0.38        | 0.40   |
| 54       | 0.54          | 0.57     | 0.81           | 0.78      | 0.37        | 0.40   |
| 55       | 0.54          | 0.56     | 0.81           | 0.79      | 0.37        | 0.39   |
| 56       | 0.53          | 0.56     | 0.82           | 0.79      | 0.37        | 0.39   |
| 57       | 0.52          | 0.55     | 0.82           | 0.80      | 0.36        | 0.38   |
| 58       | 0.52          | 0.54     | 0.83           | 0.80      | 0.36        | 0.38   |
| 59       | 0.51          | 0.54     | 0.83           | 0.81      | 0.35        | 0.37   |
| 60       | 0.50          | 0.53     | 0.84           | 0.81      | 0.34        | 0.37   |
| 61       | 0.50          | 0.52     | 0.84           | 0.82      | 0.34        | 0.36   |
| 62       | 0.49          | 0.51     | 0.85           | 0.82      | 0.33        | 0.35   |
| 63       | 0.48          | 0.50     | 0.85           | 0.83      | 0.33        | 0.35   |

Continued on next page

| $\alpha$ | $\phi_S^\ell$ | $\phi_S$ | $\varphi^\ell$ | $\varphi$ | $\psi^\ell$ | $\psi$ |
|----------|---------------|----------|----------------|-----------|-------------|--------|
| 64       | 0.47          | 0.50     | 0.86           | 0.84      | 0.32        | 0.34   |
| 65       | 0.46          | 0.49     | 0.86           | 0.84      | 0.31        | 0.34   |
| 66       | 0.46          | 0.48     | 0.87           | 0.85      | 0.31        | 0.33   |
| 67       | 0.45          | 0.47     | 0.88           | 0.85      | 0.30        | 0.32   |
| 68       | 0.44          | 0.46     | 0.88           | 0.86      | 0.30        | 0.31   |
| 69       | 0.43          | 0.45     | 0.89           | 0.86      | 0.29        | 0.31   |
| 70       | 0.42          | 0.44     | 0.89           | 0.87      | 0.28        | 0.30   |
| 71       | 0.40          | 0.43     | 0.90           | 0.87      | 0.27        | 0.29   |
| 72       | 0.39          | 0.42     | 0.90           | 0.88      | 0.26        | 0.28   |
| 73       | 0.38          | 0.40     | 0.91           | 0.88      | 0.25        | 0.27   |
| 74       | 0.37          | 0.39     | 0.91           | 0.89      | 0.25        | 0.26   |
| 75       | 0.35          | 0.38     | 0.92           | 0.90      | 0.23        | 0.25   |
| 76       | 0.34          | 0.37     | 0.92           | 0.90      | 0.23        | 0.25   |
| 77       | 0.33          | 0.35     | 0.93           | 0.91      | 0.22        | 0.23   |
| 78       | 0.31          | 0.34     | 0.93           | 0.91      | 0.20        | 0.23   |
| 79       | 0.29          | 0.32     | 0.94           | 0.92      | 0.19        | 0.21   |
| 80       | 0.28          | 0.31     | 0.94           | 0.92      | 0.18        | 0.21   |
| 81       | 0.26          | 0.29     | 0.95           | 0.93      | 0.17        | 0.19   |
| 82       | 0.24          | 0.27     | 0.95           | 0.93      | 0.16        | 0.18   |
| 83       | 0.22          | 0.26     | 0.96           | 0.94      | 0.14        | 0.17   |
| 84       | 0.21          | 0.24     | 0.96           | 0.94      | 0.14        | 0.16   |
| 85       | 0.19          | 0.22     | 0.96           | 0.94      | 0.12        | 0.15   |
| 86       | 0.17          | 0.21     | 0.97           | 0.95      | 0.11        | 0.14   |
| 87       | 0.16          | 0.19     | 0.97           | 0.95      | 0.10        | 0.13   |
| 88       | 0.15          | 0.18     | 0.97           | 0.95      | 0.10        | 0.12   |
| 89       | 0.14          | 0.17     | 0.97           | 0.95      | 0.09        | 0.11   |
| 90       | 0.13          | 0.17     | 0.97           | 0.95      | 0.08        | 0.11   |

Table S119: Reference ( $\phi_S$ ,  $\varphi$ ,  $\psi$ ) and approached ( $\phi_S^\ell$ ,  $\varphi^\ell$ ,  $\psi^\ell$ ) values of the topological descriptors for the first excited-state of the pyridinium-phenolate (PP), computed at the M062X/6-31++G(2d,p) level of theory.  $\alpha$  is the pyridinium-phenolate central twist angle amplitude.

| $\alpha$ | $\phi_S^\ell$ | $\phi_S$ | $\varphi^\ell$ | $\varphi$ | $\psi^\ell$ | $\psi$ |
|----------|---------------|----------|----------------|-----------|-------------|--------|
| 0        | 0.66          | 0.71     | 0.66           | 0.62      | 0.50        | 0.54   |
| 1        | 0.66          | 0.71     | 0.66           | 0.62      | 0.50        | 0.54   |
| 2        | 0.66          | 0.71     | 0.66           | 0.62      | 0.50        | 0.54   |
| 3        | 0.66          | 0.71     | 0.66           | 0.62      | 0.50        | 0.54   |
| 4        | 0.66          | 0.71     | 0.66           | 0.62      | 0.50        | 0.54   |
| 5        | 0.66          | 0.71     | 0.66           | 0.63      | 0.50        | 0.54   |
| 6        | 0.66          | 0.71     | 0.66           | 0.63      | 0.50        | 0.54   |
| 7        | 0.66          | 0.71     | 0.66           | 0.63      | 0.50        | 0.54   |
| 8        | 0.66          | 0.71     | 0.66           | 0.63      | 0.50        | 0.54   |
| 9        | 0.66          | 0.70     | 0.66           | 0.63      | 0.50        | 0.53   |
| 10       | 0.66          | 0.70     | 0.66           | 0.63      | 0.50        | 0.53   |
| 11       | 0.66          | 0.70     | 0.67           | 0.63      | 0.50        | 0.53   |
| 12       | 0.66          | 0.70     | 0.67           | 0.64      | 0.50        | 0.53   |
| 13       | 0.65          | 0.70     | 0.67           | 0.64      | 0.49        | 0.53   |
| 14       | 0.65          | 0.70     | 0.67           | 0.64      | 0.49        | 0.53   |
| 15       | 0.65          | 0.70     | 0.67           | 0.64      | 0.49        | 0.53   |
| 16       | 0.65          | 0.70     | 0.67           | 0.64      | 0.49        | 0.53   |
| 17       | 0.65          | 0.69     | 0.67           | 0.65      | 0.49        | 0.52   |
| 18       | 0.65          | 0.69     | 0.68           | 0.65      | 0.49        | 0.52   |
| 19       | 0.65          | 0.69     | 0.68           | 0.65      | 0.49        | 0.52   |
| 20       | 0.65          | 0.69     | 0.68           | 0.65      | 0.49        | 0.52   |
| 21       | 0.65          | 0.69     | 0.68           | 0.65      | 0.49        | 0.52   |
| 22       | 0.65          | 0.69     | 0.69           | 0.66      | 0.48        | 0.51   |
| 23       | 0.64          | 0.68     | 0.69           | 0.66      | 0.48        | 0.51   |
| 24       | 0.64          | 0.68     | 0.69           | 0.66      | 0.48        | 0.51   |
| 25       | 0.64          | 0.68     | 0.69           | 0.67      | 0.48        | 0.50   |
| 26       | 0.64          | 0.68     | 0.70           | 0.67      | 0.47        | 0.50   |
| 27       | 0.64          | 0.68     | 0.70           | 0.67      | 0.47        | 0.50   |
| 28       | 0.64          | 0.67     | 0.70           | 0.68      | 0.47        | 0.50   |
| 29       | 0.64          | 0.67     | 0.71           | 0.68      | 0.47        | 0.50   |
| 30       | 0.63          | 0.67     | 0.71           | 0.68      | 0.46        | 0.50   |
| 31       | 0.63          | 0.67     | 0.71           | 0.69      | 0.46        | 0.49   |

Continued on next page

| $\alpha$ | $\phi_S^\ell$ | $\phi_S$ | $\varphi^\ell$ | $\varphi$ | $\psi^\ell$ | $\psi$ |
|----------|---------------|----------|----------------|-----------|-------------|--------|
| 32       | 0.63          | 0.66     | 0.71           | 0.69      | 0.46        | 0.49   |
| 33       | 0.63          | 0.66     | 0.72           | 0.69      | 0.46        | 0.49   |
| 34       | 0.63          | 0.66     | 0.72           | 0.70      | 0.46        | 0.48   |
| 35       | 0.62          | 0.65     | 0.72           | 0.70      | 0.45        | 0.48   |
| 36       | 0.62          | 0.65     | 0.73           | 0.70      | 0.45        | 0.48   |
| 37       | 0.62          | 0.65     | 0.73           | 0.71      | 0.45        | 0.47   |
| 38       | 0.62          | 0.64     | 0.73           | 0.71      | 0.45        | 0.47   |
| 39       | 0.61          | 0.64     | 0.74           | 0.72      | 0.44        | 0.46   |
| 40       | 0.61          | 0.64     | 0.74           | 0.72      | 0.44        | 0.46   |
| 41       | 0.61          | 0.63     | 0.75           | 0.72      | 0.43        | 0.46   |
| 42       | 0.60          | 0.63     | 0.75           | 0.73      | 0.43        | 0.45   |
| 43       | 0.60          | 0.63     | 0.76           | 0.73      | 0.43        | 0.45   |
| 44       | 0.60          | 0.62     | 0.76           | 0.74      | 0.43        | 0.44   |
| 45       | 0.59          | 0.62     | 0.76           | 0.74      | 0.42        | 0.44   |
| 46       | 0.59          | 0.61     | 0.77           | 0.75      | 0.42        | 0.43   |
| 47       | 0.58          | 0.61     | 0.77           | 0.75      | 0.41        | 0.43   |
| 48       | 0.58          | 0.60     | 0.78           | 0.75      | 0.41        | 0.43   |
| 49       | 0.57          | 0.60     | 0.78           | 0.76      | 0.40        | 0.43   |
| 50       | 0.57          | 0.59     | 0.79           | 0.76      | 0.40        | 0.42   |
| 51       | 0.57          | 0.59     | 0.79           | 0.77      | 0.40        | 0.42   |
| 52       | 0.56          | 0.58     | 0.79           | 0.77      | 0.39        | 0.41   |
| 53       | 0.55          | 0.58     | 0.80           | 0.78      | 0.38        | 0.41   |
| 54       | 0.55          | 0.57     | 0.80           | 0.78      | 0.38        | 0.40   |
| 55       | 0.54          | 0.56     | 0.81           | 0.79      | 0.37        | 0.39   |
| 56       | 0.54          | 0.56     | 0.81           | 0.79      | 0.37        | 0.39   |
| 57       | 0.53          | 0.55     | 0.82           | 0.80      | 0.37        | 0.38   |
| 58       | 0.52          | 0.55     | 0.82           | 0.80      | 0.36        | 0.38   |
| 59       | 0.52          | 0.54     | 0.83           | 0.81      | 0.36        | 0.37   |
| 60       | 0.51          | 0.53     | 0.83           | 0.81      | 0.35        | 0.37   |
| 61       | 0.50          | 0.52     | 0.84           | 0.82      | 0.34        | 0.36   |
| 62       | 0.49          | 0.52     | 0.84           | 0.82      | 0.34        | 0.36   |
| 63       | 0.49          | 0.51     | 0.85           | 0.83      | 0.33        | 0.35   |

Continued on next page



| $\alpha$ | $\phi_S^\ell$ | $\phi_S$ | $\varphi^\ell$ | $\varphi$ | $\psi^\ell$ | $\psi$ |
|----------|---------------|----------|----------------|-----------|-------------|--------|
| 64       | 0.48          | 0.50     | 0.85           | 0.83      | 0.33        | 0.35   |
| 65       | 0.47          | 0.49     | 0.86           | 0.84      | 0.32        | 0.34   |
| 66       | 0.46          | 0.48     | 0.87           | 0.84      | 0.31        | 0.33   |
| 67       | 0.45          | 0.47     | 0.87           | 0.85      | 0.30        | 0.32   |
| 68       | 0.44          | 0.46     | 0.88           | 0.86      | 0.30        | 0.31   |
| 69       | 0.43          | 0.45     | 0.88           | 0.86      | 0.29        | 0.31   |
| 70       | 0.42          | 0.44     | 0.89           | 0.87      | 0.28        | 0.30   |
| 71       | 0.41          | 0.43     | 0.89           | 0.87      | 0.27        | 0.29   |
| 72       | 0.40          | 0.42     | 0.90           | 0.88      | 0.27        | 0.28   |
| 73       | 0.38          | 0.41     | 0.91           | 0.88      | 0.25        | 0.28   |
| 74       | 0.37          | 0.40     | 0.91           | 0.89      | 0.25        | 0.27   |
| 75       | 0.36          | 0.38     | 0.92           | 0.89      | 0.24        | 0.26   |
| 76       | 0.34          | 0.37     | 0.92           | 0.90      | 0.23        | 0.25   |
| 77       | 0.33          | 0.35     | 0.93           | 0.91      | 0.22        | 0.23   |
| 78       | 0.31          | 0.34     | 0.93           | 0.91      | 0.20        | 0.23   |
| 79       | 0.29          | 0.32     | 0.94           | 0.92      | 0.19        | 0.21   |
| 80       | 0.28          | 0.31     | 0.94           | 0.92      | 0.18        | 0.21   |
| 81       | 0.26          | 0.29     | 0.95           | 0.93      | 0.17        | 0.19   |
| 82       | 0.24          | 0.28     | 0.95           | 0.93      | 0.16        | 0.19   |
| 83       | 0.22          | 0.26     | 0.96           | 0.94      | 0.14        | 0.17   |
| 84       | 0.20          | 0.24     | 0.96           | 0.94      | 0.13        | 0.16   |
| 85       | 0.19          | 0.22     | 0.97           | 0.94      | 0.12        | 0.15   |
| 86       | 0.17          | 0.21     | 0.97           | 0.95      | 0.11        | 0.14   |
| 87       | 0.16          | 0.19     | 0.97           | 0.95      | 0.10        | 0.13   |
| 88       | 0.14          | 0.18     | 0.97           | 0.95      | 0.09        | 0.12   |
| 89       | 0.13          | 0.17     | 0.98           | 0.95      | 0.08        | 0.11   |
| 90       | 0.13          | 0.16     | 0.98           | 0.95      | 0.08        | 0.11   |

Table S120: Reference ( $\phi_S$ ,  $\varphi$ ,  $\psi$ ) and approached ( $\phi_S^\ell$ ,  $\varphi^\ell$ ,  $\psi^\ell$ ) values of the topological descriptors for the first excited-state of the pyridinium-phenolate (PP), computed at the M062X/6-31++G(d,p) level of theory.  $\alpha$  is the pyridinium-phenolate central twist angle amplitude.

| $\alpha$ | $\phi_S^\ell$ | $\phi_S$ | $\varphi^\ell$ | $\varphi$ | $\psi^\ell$ | $\psi$ |
|----------|---------------|----------|----------------|-----------|-------------|--------|
| 0        | 0.66          | 0.71     | 0.66           | 0.62      | 0.50        | 0.54   |
| 1        | 0.66          | 0.71     | 0.66           | 0.62      | 0.50        | 0.54   |
| 2        | 0.66          | 0.71     | 0.66           | 0.62      | 0.50        | 0.54   |
| 3        | 0.66          | 0.71     | 0.66           | 0.62      | 0.50        | 0.54   |
| 4        | 0.66          | 0.71     | 0.66           | 0.62      | 0.50        | 0.54   |
| 5        | 0.66          | 0.71     | 0.66           | 0.63      | 0.50        | 0.54   |
| 6        | 0.66          | 0.71     | 0.66           | 0.63      | 0.50        | 0.54   |
| 7        | 0.66          | 0.71     | 0.66           | 0.63      | 0.50        | 0.54   |
| 8        | 0.66          | 0.71     | 0.66           | 0.63      | 0.50        | 0.54   |
| 9        | 0.66          | 0.70     | 0.66           | 0.63      | 0.50        | 0.53   |
| 10       | 0.66          | 0.70     | 0.66           | 0.63      | 0.50        | 0.53   |
| 11       | 0.66          | 0.70     | 0.66           | 0.63      | 0.50        | 0.53   |
| 12       | 0.66          | 0.70     | 0.67           | 0.64      | 0.50        | 0.53   |
| 13       | 0.65          | 0.70     | 0.67           | 0.64      | 0.49        | 0.53   |
| 14       | 0.65          | 0.70     | 0.67           | 0.64      | 0.49        | 0.53   |
| 15       | 0.65          | 0.70     | 0.67           | 0.64      | 0.49        | 0.53   |
| 16       | 0.65          | 0.70     | 0.67           | 0.64      | 0.49        | 0.53   |
| 17       | 0.65          | 0.69     | 0.67           | 0.64      | 0.49        | 0.52   |
| 18       | 0.65          | 0.69     | 0.68           | 0.65      | 0.49        | 0.52   |
| 19       | 0.65          | 0.69     | 0.68           | 0.65      | 0.49        | 0.52   |
| 20       | 0.65          | 0.69     | 0.68           | 0.65      | 0.49        | 0.52   |
| 21       | 0.65          | 0.69     | 0.68           | 0.65      | 0.49        | 0.52   |
| 22       | 0.65          | 0.69     | 0.69           | 0.66      | 0.48        | 0.51   |
| 23       | 0.64          | 0.68     | 0.69           | 0.66      | 0.48        | 0.51   |
| 24       | 0.64          | 0.68     | 0.69           | 0.66      | 0.48        | 0.51   |
| 25       | 0.64          | 0.68     | 0.69           | 0.67      | 0.48        | 0.50   |
| 26       | 0.64          | 0.68     | 0.70           | 0.67      | 0.47        | 0.50   |
| 27       | 0.64          | 0.68     | 0.70           | 0.67      | 0.47        | 0.50   |
| 28       | 0.64          | 0.67     | 0.70           | 0.68      | 0.47        | 0.50   |
| 29       | 0.64          | 0.67     | 0.71           | 0.68      | 0.47        | 0.50   |
| 30       | 0.63          | 0.67     | 0.71           | 0.68      | 0.46        | 0.50   |
| 31       | 0.63          | 0.67     | 0.71           | 0.69      | 0.46        | 0.49   |

Continued on next page

| $\alpha$ | $\phi_S^\ell$ | $\phi_S$ | $\varphi^\ell$ | $\varphi$ | $\psi^\ell$ | $\psi$ |
|----------|---------------|----------|----------------|-----------|-------------|--------|
| 32       | 0.63          | 0.66     | 0.71           | 0.69      | 0.46        | 0.49   |
| 33       | 0.63          | 0.66     | 0.72           | 0.69      | 0.46        | 0.49   |
| 34       | 0.63          | 0.66     | 0.72           | 0.70      | 0.46        | 0.48   |
| 35       | 0.62          | 0.65     | 0.72           | 0.70      | 0.45        | 0.48   |
| 36       | 0.62          | 0.65     | 0.73           | 0.70      | 0.45        | 0.48   |
| 37       | 0.62          | 0.65     | 0.73           | 0.71      | 0.45        | 0.47   |
| 38       | 0.62          | 0.64     | 0.73           | 0.71      | 0.45        | 0.47   |
| 39       | 0.61          | 0.64     | 0.74           | 0.72      | 0.44        | 0.46   |
| 40       | 0.61          | 0.64     | 0.74           | 0.72      | 0.44        | 0.46   |
| 41       | 0.61          | 0.63     | 0.75           | 0.72      | 0.43        | 0.46   |
| 42       | 0.60          | 0.63     | 0.75           | 0.73      | 0.43        | 0.45   |
| 43       | 0.60          | 0.63     | 0.76           | 0.73      | 0.43        | 0.45   |
| 44       | 0.60          | 0.62     | 0.76           | 0.74      | 0.43        | 0.44   |
| 45       | 0.59          | 0.62     | 0.76           | 0.74      | 0.42        | 0.44   |
| 46       | 0.59          | 0.61     | 0.77           | 0.75      | 0.42        | 0.43   |
| 47       | 0.58          | 0.61     | 0.77           | 0.75      | 0.41        | 0.43   |
| 48       | 0.58          | 0.60     | 0.78           | 0.75      | 0.41        | 0.43   |
| 49       | 0.57          | 0.60     | 0.78           | 0.76      | 0.40        | 0.43   |
| 50       | 0.57          | 0.59     | 0.79           | 0.76      | 0.40        | 0.42   |
| 51       | 0.57          | 0.59     | 0.79           | 0.77      | 0.40        | 0.42   |
| 52       | 0.56          | 0.58     | 0.79           | 0.77      | 0.39        | 0.41   |
| 53       | 0.55          | 0.58     | 0.80           | 0.78      | 0.38        | 0.41   |
| 54       | 0.55          | 0.57     | 0.80           | 0.78      | 0.38        | 0.40   |
| 55       | 0.54          | 0.56     | 0.81           | 0.79      | 0.37        | 0.39   |
| 56       | 0.54          | 0.56     | 0.81           | 0.79      | 0.37        | 0.39   |
| 57       | 0.53          | 0.55     | 0.82           | 0.80      | 0.37        | 0.38   |
| 58       | 0.52          | 0.55     | 0.82           | 0.80      | 0.36        | 0.38   |
| 59       | 0.52          | 0.54     | 0.83           | 0.81      | 0.36        | 0.37   |
| 60       | 0.51          | 0.53     | 0.83           | 0.81      | 0.35        | 0.37   |
| 61       | 0.50          | 0.52     | 0.84           | 0.82      | 0.34        | 0.36   |
| 62       | 0.49          | 0.52     | 0.84           | 0.82      | 0.34        | 0.36   |
| 63       | 0.49          | 0.51     | 0.85           | 0.83      | 0.33        | 0.35   |

Continued on next page

| $\alpha$ | $\phi_S^\ell$ | $\phi_S$ | $\varphi^\ell$ | $\varphi$ | $\psi^\ell$ | $\psi$ |
|----------|---------------|----------|----------------|-----------|-------------|--------|
| 64       | 0.48          | 0.50     | 0.85           | 0.83      | 0.33        | 0.35   |
| 65       | 0.47          | 0.49     | 0.86           | 0.84      | 0.32        | 0.34   |
| 66       | 0.46          | 0.48     | 0.87           | 0.84      | 0.31        | 0.33   |
| 67       | 0.45          | 0.47     | 0.87           | 0.85      | 0.30        | 0.32   |
| 68       | 0.44          | 0.46     | 0.88           | 0.86      | 0.30        | 0.31   |
| 69       | 0.43          | 0.45     | 0.88           | 0.86      | 0.29        | 0.31   |
| 70       | 0.42          | 0.44     | 0.89           | 0.87      | 0.28        | 0.30   |
| 71       | 0.41          | 0.43     | 0.89           | 0.87      | 0.27        | 0.29   |
| 72       | 0.40          | 0.42     | 0.90           | 0.88      | 0.27        | 0.28   |
| 73       | 0.38          | 0.41     | 0.91           | 0.88      | 0.25        | 0.28   |
| 74       | 0.37          | 0.40     | 0.91           | 0.89      | 0.25        | 0.27   |
| 75       | 0.36          | 0.38     | 0.92           | 0.89      | 0.24        | 0.26   |
| 76       | 0.34          | 0.37     | 0.92           | 0.90      | 0.23        | 0.25   |
| 77       | 0.33          | 0.35     | 0.93           | 0.91      | 0.22        | 0.23   |
| 78       | 0.31          | 0.34     | 0.93           | 0.91      | 0.20        | 0.23   |
| 79       | 0.29          | 0.32     | 0.94           | 0.92      | 0.19        | 0.21   |
| 80       | 0.28          | 0.31     | 0.94           | 0.92      | 0.18        | 0.21   |
| 81       | 0.26          | 0.29     | 0.95           | 0.93      | 0.17        | 0.19   |
| 82       | 0.24          | 0.28     | 0.95           | 0.93      | 0.16        | 0.19   |
| 83       | 0.22          | 0.26     | 0.96           | 0.94      | 0.14        | 0.17   |
| 84       | 0.21          | 0.24     | 0.96           | 0.94      | 0.14        | 0.16   |
| 85       | 0.19          | 0.23     | 0.97           | 0.94      | 0.12        | 0.15   |
| 86       | 0.17          | 0.21     | 0.97           | 0.95      | 0.11        | 0.14   |
| 87       | 0.16          | 0.19     | 0.97           | 0.95      | 0.10        | 0.13   |
| 88       | 0.14          | 0.18     | 0.97           | 0.95      | 0.09        | 0.12   |
| 89       | 0.13          | 0.17     | 0.97           | 0.95      | 0.08        | 0.11   |
| 90       | 0.13          | 0.16     | 0.98           | 0.95      | 0.08        | 0.11   |

Table S121: Reference ( $\phi_S$ ,  $\varphi$ ,  $\psi$ ) and approached ( $\phi_S^\ell$ ,  $\varphi^\ell$ ,  $\psi^\ell$ ) values of the topological descriptors for the first excited-state of the pyridinium-phenolate (PP), computed at the M062X/6-31+G(d,p) level of theory.  $\alpha$  is the pyridinium-phenolate central twist angle amplitude.

| $\alpha$ | $\phi_S^\ell$ | $\phi_S$ | $\varphi^\ell$ | $\varphi$ | $\psi^\ell$ | $\psi$ |
|----------|---------------|----------|----------------|-----------|-------------|--------|
| 0        | 0.66          | 0.71     | 0.66           | 0.62      | 0.50        | 0.54   |
| 1        | 0.66          | 0.71     | 0.66           | 0.62      | 0.50        | 0.54   |
| 2        | 0.66          | 0.71     | 0.66           | 0.62      | 0.50        | 0.54   |
| 3        | 0.66          | 0.71     | 0.66           | 0.62      | 0.50        | 0.54   |
| 4        | 0.66          | 0.71     | 0.66           | 0.63      | 0.50        | 0.54   |
| 5        | 0.66          | 0.71     | 0.66           | 0.63      | 0.50        | 0.54   |
| 6        | 0.66          | 0.71     | 0.66           | 0.63      | 0.50        | 0.54   |
| 7        | 0.66          | 0.71     | 0.66           | 0.63      | 0.50        | 0.54   |
| 8        | 0.66          | 0.71     | 0.66           | 0.63      | 0.50        | 0.54   |
| 9        | 0.66          | 0.70     | 0.66           | 0.63      | 0.50        | 0.53   |
| 10       | 0.66          | 0.70     | 0.66           | 0.63      | 0.50        | 0.53   |
| 11       | 0.66          | 0.70     | 0.67           | 0.63      | 0.50        | 0.53   |
| 12       | 0.66          | 0.70     | 0.67           | 0.64      | 0.50        | 0.53   |
| 13       | 0.65          | 0.70     | 0.67           | 0.64      | 0.49        | 0.53   |
| 14       | 0.65          | 0.70     | 0.67           | 0.64      | 0.49        | 0.53   |
| 15       | 0.65          | 0.70     | 0.67           | 0.64      | 0.49        | 0.53   |
| 16       | 0.65          | 0.70     | 0.67           | 0.64      | 0.49        | 0.53   |
| 17       | 0.65          | 0.69     | 0.67           | 0.65      | 0.49        | 0.52   |
| 18       | 0.65          | 0.69     | 0.68           | 0.65      | 0.49        | 0.52   |
| 19       | 0.65          | 0.69     | 0.68           | 0.65      | 0.49        | 0.52   |
| 20       | 0.65          | 0.69     | 0.68           | 0.65      | 0.49        | 0.52   |
| 21       | 0.65          | 0.69     | 0.68           | 0.66      | 0.49        | 0.51   |
| 22       | 0.65          | 0.69     | 0.69           | 0.66      | 0.48        | 0.51   |
| 23       | 0.64          | 0.68     | 0.69           | 0.66      | 0.48        | 0.51   |
| 24       | 0.64          | 0.68     | 0.69           | 0.66      | 0.48        | 0.51   |
| 25       | 0.64          | 0.68     | 0.69           | 0.67      | 0.48        | 0.50   |
| 26       | 0.64          | 0.68     | 0.70           | 0.67      | 0.47        | 0.50   |
| 27       | 0.64          | 0.68     | 0.70           | 0.67      | 0.47        | 0.50   |
| 28       | 0.64          | 0.67     | 0.70           | 0.68      | 0.47        | 0.50   |
| 29       | 0.64          | 0.67     | 0.71           | 0.68      | 0.47        | 0.50   |
| 30       | 0.63          | 0.67     | 0.71           | 0.68      | 0.46        | 0.50   |
| 31       | 0.63          | 0.67     | 0.71           | 0.69      | 0.46        | 0.49   |

Continued on next page

| $\alpha$ | $\phi_S^\ell$ | $\phi_S$ | $\varphi^\ell$ | $\varphi$ | $\psi^\ell$ | $\psi$ |
|----------|---------------|----------|----------------|-----------|-------------|--------|
| 32       | 0.63          | 0.66     | 0.71           | 0.69      | 0.46        | 0.49   |
| 33       | 0.63          | 0.66     | 0.72           | 0.69      | 0.46        | 0.49   |
| 34       | 0.63          | 0.66     | 0.72           | 0.70      | 0.46        | 0.48   |
| 35       | 0.62          | 0.65     | 0.72           | 0.70      | 0.45        | 0.48   |
| 36       | 0.62          | 0.65     | 0.73           | 0.70      | 0.45        | 0.48   |
| 37       | 0.62          | 0.65     | 0.73           | 0.71      | 0.45        | 0.47   |
| 38       | 0.62          | 0.64     | 0.73           | 0.71      | 0.45        | 0.47   |
| 39       | 0.61          | 0.64     | 0.74           | 0.72      | 0.44        | 0.46   |
| 40       | 0.61          | 0.64     | 0.74           | 0.72      | 0.44        | 0.46   |
| 41       | 0.61          | 0.63     | 0.75           | 0.72      | 0.43        | 0.46   |
| 42       | 0.60          | 0.63     | 0.75           | 0.73      | 0.43        | 0.45   |
| 43       | 0.60          | 0.63     | 0.76           | 0.73      | 0.43        | 0.45   |
| 44       | 0.60          | 0.62     | 0.76           | 0.74      | 0.43        | 0.44   |
| 45       | 0.59          | 0.62     | 0.76           | 0.74      | 0.42        | 0.44   |
| 46       | 0.59          | 0.61     | 0.77           | 0.75      | 0.42        | 0.43   |
| 47       | 0.58          | 0.61     | 0.77           | 0.75      | 0.41        | 0.43   |
| 48       | 0.58          | 0.60     | 0.78           | 0.75      | 0.41        | 0.43   |
| 49       | 0.57          | 0.60     | 0.78           | 0.76      | 0.40        | 0.43   |
| 50       | 0.57          | 0.59     | 0.79           | 0.76      | 0.40        | 0.42   |
| 51       | 0.57          | 0.59     | 0.79           | 0.77      | 0.40        | 0.42   |
| 52       | 0.56          | 0.58     | 0.79           | 0.77      | 0.39        | 0.41   |
| 53       | 0.55          | 0.58     | 0.80           | 0.78      | 0.38        | 0.41   |
| 54       | 0.55          | 0.57     | 0.80           | 0.78      | 0.38        | 0.40   |
| 55       | 0.54          | 0.56     | 0.81           | 0.79      | 0.37        | 0.39   |
| 56       | 0.54          | 0.56     | 0.81           | 0.79      | 0.37        | 0.39   |
| 57       | 0.53          | 0.55     | 0.82           | 0.80      | 0.37        | 0.38   |
| 58       | 0.52          | 0.55     | 0.82           | 0.80      | 0.36        | 0.38   |
| 59       | 0.52          | 0.54     | 0.83           | 0.81      | 0.36        | 0.37   |
| 60       | 0.51          | 0.53     | 0.83           | 0.81      | 0.35        | 0.37   |
| 61       | 0.50          | 0.52     | 0.84           | 0.82      | 0.34        | 0.36   |
| 62       | 0.50          | 0.52     | 0.84           | 0.82      | 0.34        | 0.36   |
| 63       | 0.49          | 0.51     | 0.85           | 0.83      | 0.33        | 0.35   |

Continued on next page

| $\alpha$ | $\phi_S^\ell$ | $\phi_S$ | $\varphi^\ell$ | $\varphi$ | $\psi^\ell$ | $\psi$ |
|----------|---------------|----------|----------------|-----------|-------------|--------|
| 64       | 0.48          | 0.50     | 0.85           | 0.83      | 0.33        | 0.35   |
| 65       | 0.47          | 0.49     | 0.86           | 0.84      | 0.32        | 0.34   |
| 66       | 0.46          | 0.48     | 0.87           | 0.84      | 0.31        | 0.33   |
| 67       | 0.45          | 0.47     | 0.87           | 0.85      | 0.30        | 0.32   |
| 68       | 0.44          | 0.46     | 0.88           | 0.86      | 0.30        | 0.31   |
| 69       | 0.43          | 0.45     | 0.88           | 0.86      | 0.29        | 0.31   |
| 70       | 0.42          | 0.44     | 0.89           | 0.87      | 0.28        | 0.30   |
| 71       | 0.41          | 0.43     | 0.89           | 0.87      | 0.27        | 0.29   |
| 72       | 0.40          | 0.42     | 0.90           | 0.88      | 0.27        | 0.28   |
| 73       | 0.38          | 0.41     | 0.91           | 0.88      | 0.25        | 0.28   |
| 74       | 0.37          | 0.40     | 0.91           | 0.89      | 0.25        | 0.27   |
| 75       | 0.36          | 0.38     | 0.92           | 0.89      | 0.24        | 0.26   |
| 76       | 0.34          | 0.37     | 0.92           | 0.90      | 0.23        | 0.25   |
| 77       | 0.33          | 0.35     | 0.93           | 0.91      | 0.22        | 0.23   |
| 78       | 0.31          | 0.34     | 0.93           | 0.91      | 0.20        | 0.23   |
| 79       | 0.29          | 0.32     | 0.94           | 0.92      | 0.19        | 0.21   |
| 80       | 0.28          | 0.31     | 0.94           | 0.92      | 0.18        | 0.21   |
| 81       | 0.26          | 0.29     | 0.95           | 0.93      | 0.17        | 0.19   |
| 82       | 0.24          | 0.28     | 0.95           | 0.93      | 0.16        | 0.19   |
| 83       | 0.22          | 0.26     | 0.96           | 0.94      | 0.14        | 0.17   |
| 84       | 0.21          | 0.24     | 0.96           | 0.94      | 0.14        | 0.16   |
| 85       | 0.19          | 0.22     | 0.97           | 0.94      | 0.12        | 0.15   |
| 86       | 0.17          | 0.21     | 0.97           | 0.95      | 0.11        | 0.14   |
| 87       | 0.16          | 0.19     | 0.97           | 0.95      | 0.10        | 0.13   |
| 88       | 0.14          | 0.18     | 0.97           | 0.95      | 0.09        | 0.12   |
| 89       | 0.13          | 0.17     | 0.98           | 0.95      | 0.08        | 0.11   |
| 90       | 0.13          | 0.16     | 0.98           | 0.95      | 0.08        | 0.11   |

Table S122: Reference ( $\phi_S$ ,  $\varphi$ ,  $\psi$ ) and approached ( $\phi_S^\ell$ ,  $\varphi^\ell$ ,  $\psi^\ell$ ) values of the topological descriptors for the first excited-state of the pyridinium-phenolate (PP), computed at the M062X/6-31+G(d) level of theory.  $\alpha$  is the pyridinium-phenolate central twist angle amplitude.

| $\alpha$ | $\phi_S^\ell$ | $\phi_S$ | $\varphi^\ell$ | $\varphi$ | $\psi^\ell$ | $\psi$ |
|----------|---------------|----------|----------------|-----------|-------------|--------|
| 0        | 0.69          | 0.73     | 0.65           | 0.61      | 0.52        | 0.56   |
| 1        | 0.69          | 0.73     | 0.65           | 0.61      | 0.52        | 0.56   |
| 2        | 0.69          | 0.73     | 0.65           | 0.61      | 0.52        | 0.56   |
| 3        | 0.69          | 0.73     | 0.65           | 0.61      | 0.52        | 0.56   |
| 4        | 0.69          | 0.73     | 0.65           | 0.61      | 0.52        | 0.56   |
| 5        | 0.69          | 0.73     | 0.65           | 0.61      | 0.52        | 0.56   |
| 6        | 0.69          | 0.73     | 0.65           | 0.61      | 0.52        | 0.56   |
| 7        | 0.69          | 0.73     | 0.65           | 0.61      | 0.52        | 0.56   |
| 8        | 0.69          | 0.73     | 0.65           | 0.61      | 0.52        | 0.56   |
| 9        | 0.69          | 0.73     | 0.65           | 0.62      | 0.52        | 0.55   |
| 10       | 0.69          | 0.72     | 0.65           | 0.62      | 0.52        | 0.55   |
| 11       | 0.69          | 0.72     | 0.65           | 0.62      | 0.52        | 0.55   |
| 12       | 0.69          | 0.72     | 0.66           | 0.62      | 0.51        | 0.55   |
| 13       | 0.68          | 0.72     | 0.66           | 0.62      | 0.51        | 0.55   |
| 14       | 0.68          | 0.72     | 0.66           | 0.62      | 0.51        | 0.55   |
| 15       | 0.68          | 0.72     | 0.66           | 0.63      | 0.51        | 0.54   |
| 16       | 0.68          | 0.72     | 0.66           | 0.63      | 0.51        | 0.54   |
| 17       | 0.68          | 0.72     | 0.66           | 0.63      | 0.51        | 0.54   |
| 18       | 0.68          | 0.71     | 0.67           | 0.63      | 0.50        | 0.54   |
| 19       | 0.68          | 0.71     | 0.67           | 0.63      | 0.50        | 0.54   |
| 20       | 0.68          | 0.71     | 0.67           | 0.64      | 0.50        | 0.53   |
| 21       | 0.68          | 0.71     | 0.67           | 0.64      | 0.50        | 0.53   |
| 22       | 0.67          | 0.71     | 0.67           | 0.64      | 0.50        | 0.53   |
| 23       | 0.67          | 0.71     | 0.68           | 0.64      | 0.50        | 0.53   |
| 24       | 0.67          | 0.70     | 0.68           | 0.65      | 0.50        | 0.52   |
| 25       | 0.67          | 0.70     | 0.68           | 0.65      | 0.50        | 0.52   |
| 26       | 0.67          | 0.70     | 0.68           | 0.65      | 0.50        | 0.52   |
| 27       | 0.67          | 0.70     | 0.69           | 0.66      | 0.49        | 0.52   |
| 28       | 0.67          | 0.69     | 0.69           | 0.66      | 0.49        | 0.51   |
| 29       | 0.66          | 0.69     | 0.69           | 0.66      | 0.49        | 0.51   |
| 30       | 0.66          | 0.69     | 0.70           | 0.67      | 0.48        | 0.51   |
| 31       | 0.66          | 0.69     | 0.70           | 0.67      | 0.48        | 0.51   |

Continued on next page



| $\alpha$ | $\phi_S^\ell$ | $\phi_S$ | $\varphi^\ell$ | $\varphi$ | $\psi^\ell$ | $\psi$ |
|----------|---------------|----------|----------------|-----------|-------------|--------|
| 32       | 0.66          | 0.68     | 0.70           | 0.67      | 0.48        | 0.50   |
| 33       | 0.66          | 0.68     | 0.70           | 0.68      | 0.48        | 0.50   |
| 34       | 0.65          | 0.68     | 0.71           | 0.68      | 0.47        | 0.50   |
| 35       | 0.65          | 0.68     | 0.71           | 0.68      | 0.47        | 0.50   |
| 36       | 0.65          | 0.67     | 0.71           | 0.69      | 0.47        | 0.49   |
| 37       | 0.65          | 0.67     | 0.72           | 0.69      | 0.47        | 0.49   |
| 38       | 0.64          | 0.67     | 0.72           | 0.70      | 0.46        | 0.49   |
| 39       | 0.64          | 0.66     | 0.73           | 0.70      | 0.46        | 0.48   |
| 40       | 0.64          | 0.66     | 0.73           | 0.70      | 0.46        | 0.48   |
| 41       | 0.64          | 0.66     | 0.73           | 0.71      | 0.46        | 0.48   |
| 42       | 0.63          | 0.65     | 0.74           | 0.71      | 0.45        | 0.47   |
| 43       | 0.63          | 0.65     | 0.74           | 0.72      | 0.45        | 0.47   |
| 44       | 0.62          | 0.64     | 0.75           | 0.72      | 0.44        | 0.46   |
| 45       | 0.62          | 0.64     | 0.75           | 0.73      | 0.44        | 0.46   |
| 46       | 0.62          | 0.64     | 0.75           | 0.73      | 0.44        | 0.46   |
| 47       | 0.61          | 0.63     | 0.76           | 0.73      | 0.43        | 0.45   |
| 48       | 0.61          | 0.63     | 0.76           | 0.74      | 0.43        | 0.45   |
| 49       | 0.60          | 0.62     | 0.77           | 0.74      | 0.42        | 0.44   |
| 50       | 0.60          | 0.62     | 0.77           | 0.75      | 0.42        | 0.44   |
| 51       | 0.59          | 0.61     | 0.78           | 0.75      | 0.41        | 0.43   |
| 52       | 0.59          | 0.61     | 0.78           | 0.76      | 0.41        | 0.43   |
| 53       | 0.58          | 0.60     | 0.78           | 0.76      | 0.41        | 0.43   |
| 54       | 0.58          | 0.59     | 0.79           | 0.77      | 0.40        | 0.42   |
| 55       | 0.57          | 0.59     | 0.79           | 0.77      | 0.40        | 0.42   |
| 56       | 0.57          | 0.58     | 0.80           | 0.78      | 0.39        | 0.41   |
| 57       | 0.56          | 0.58     | 0.80           | 0.78      | 0.39        | 0.41   |
| 58       | 0.56          | 0.57     | 0.81           | 0.79      | 0.39        | 0.40   |
| 59       | 0.55          | 0.56     | 0.81           | 0.79      | 0.38        | 0.39   |
| 60       | 0.54          | 0.56     | 0.82           | 0.80      | 0.37        | 0.39   |
| 61       | 0.53          | 0.55     | 0.82           | 0.80      | 0.37        | 0.38   |
| 62       | 0.53          | 0.54     | 0.83           | 0.81      | 0.36        | 0.37   |
| 63       | 0.52          | 0.53     | 0.83           | 0.81      | 0.36        | 0.37   |

Continued on next page

| $\alpha$ | $\phi_S^\ell$ | $\phi_S$ | $\varphi^\ell$ | $\varphi$ | $\psi^\ell$ | $\psi$ |
|----------|---------------|----------|----------------|-----------|-------------|--------|
| 64       | 0.51          | 0.53     | 0.84           | 0.82      | 0.35        | 0.37   |
| 65       | 0.50          | 0.52     | 0.84           | 0.82      | 0.34        | 0.36   |
| 66       | 0.49          | 0.51     | 0.85           | 0.83      | 0.33        | 0.35   |
| 67       | 0.48          | 0.50     | 0.86           | 0.84      | 0.32        | 0.34   |
| 68       | 0.47          | 0.49     | 0.86           | 0.84      | 0.32        | 0.34   |
| 69       | 0.46          | 0.48     | 0.87           | 0.85      | 0.31        | 0.33   |
| 70       | 0.45          | 0.47     | 0.87           | 0.85      | 0.30        | 0.32   |
| 71       | 0.44          | 0.46     | 0.88           | 0.86      | 0.30        | 0.31   |
| 72       | 0.43          | 0.45     | 0.89           | 0.86      | 0.29        | 0.31   |
| 73       | 0.42          | 0.44     | 0.89           | 0.87      | 0.28        | 0.30   |
| 74       | 0.41          | 0.43     | 0.90           | 0.88      | 0.27        | 0.29   |
| 75       | 0.39          | 0.41     | 0.90           | 0.88      | 0.26        | 0.28   |
| 76       | 0.38          | 0.40     | 0.91           | 0.89      | 0.25        | 0.27   |
| 77       | 0.36          | 0.38     | 0.92           | 0.89      | 0.24        | 0.26   |
| 78       | 0.34          | 0.37     | 0.92           | 0.90      | 0.23        | 0.25   |
| 79       | 0.33          | 0.35     | 0.93           | 0.91      | 0.22        | 0.23   |
| 80       | 0.31          | 0.34     | 0.94           | 0.91      | 0.20        | 0.23   |
| 81       | 0.29          | 0.32     | 0.94           | 0.92      | 0.19        | 0.21   |
| 82       | 0.27          | 0.30     | 0.95           | 0.93      | 0.18        | 0.20   |
| 83       | 0.25          | 0.28     | 0.95           | 0.93      | 0.16        | 0.19   |
| 84       | 0.22          | 0.26     | 0.96           | 0.94      | 0.14        | 0.17   |
| 85       | 0.20          | 0.24     | 0.96           | 0.94      | 0.13        | 0.16   |
| 86       | 0.18          | 0.22     | 0.97           | 0.95      | 0.12        | 0.14   |
| 87       | 0.16          | 0.20     | 0.97           | 0.95      | 0.10        | 0.13   |
| 88       | 0.14          | 0.18     | 0.98           | 0.95      | 0.09        | 0.12   |
| 89       | 0.12          | 0.17     | 0.98           | 0.95      | 0.08        | 0.11   |
| 90       | 0.12          | 0.16     | 0.98           | 0.96      | 0.08        | 0.11   |

Table S123: Reference ( $\phi_S$ ,  $\varphi$ ,  $\psi$ ) and approached ( $\phi_S^\ell$ ,  $\varphi^\ell$ ,  $\psi^\ell$ ) values of the topological descriptors for the first excited-state of the pyridinium-phenolate (PP), computed at the M062X/6-31G(d) level of theory.  $\alpha$  is the pyridinium-phenolate central twist angle amplitude.

| $\alpha$ | $\phi_S^\ell$ | $\phi_S$ | $\varphi^\ell$ | $\varphi$ | $\psi^\ell$ | $\psi$ |
|----------|---------------|----------|----------------|-----------|-------------|--------|
| 0        | 0.66          | 0.71     | 0.66           | 0.63      | 0.50        | 0.54   |
| 1        | 0.66          | 0.71     | 0.66           | 0.63      | 0.50        | 0.54   |
| 2        | 0.66          | 0.71     | 0.66           | 0.63      | 0.50        | 0.54   |
| 3        | 0.66          | 0.71     | 0.66           | 0.63      | 0.50        | 0.54   |
| 4        | 0.66          | 0.71     | 0.66           | 0.63      | 0.50        | 0.54   |
| 5        | 0.66          | 0.70     | 0.66           | 0.63      | 0.50        | 0.53   |
| 6        | 0.66          | 0.70     | 0.66           | 0.63      | 0.50        | 0.53   |
| 7        | 0.66          | 0.70     | 0.66           | 0.63      | 0.50        | 0.53   |
| 8        | 0.66          | 0.70     | 0.66           | 0.63      | 0.50        | 0.53   |
| 9        | 0.66          | 0.70     | 0.66           | 0.63      | 0.50        | 0.53   |
| 10       | 0.66          | 0.70     | 0.66           | 0.64      | 0.50        | 0.53   |
| 11       | 0.66          | 0.70     | 0.66           | 0.64      | 0.50        | 0.53   |
| 12       | 0.66          | 0.70     | 0.66           | 0.64      | 0.50        | 0.53   |
| 13       | 0.66          | 0.70     | 0.67           | 0.64      | 0.50        | 0.53   |
| 14       | 0.66          | 0.70     | 0.67           | 0.64      | 0.50        | 0.53   |
| 15       | 0.66          | 0.69     | 0.67           | 0.64      | 0.50        | 0.52   |
| 16       | 0.66          | 0.69     | 0.67           | 0.65      | 0.50        | 0.52   |
| 17       | 0.65          | 0.69     | 0.67           | 0.65      | 0.49        | 0.52   |
| 18       | 0.65          | 0.69     | 0.67           | 0.65      | 0.49        | 0.52   |
| 19       | 0.65          | 0.69     | 0.68           | 0.65      | 0.49        | 0.52   |
| 20       | 0.65          | 0.69     | 0.68           | 0.66      | 0.49        | 0.51   |
| 21       | 0.65          | 0.69     | 0.68           | 0.66      | 0.49        | 0.51   |
| 22       | 0.65          | 0.68     | 0.68           | 0.66      | 0.49        | 0.51   |
| 23       | 0.65          | 0.68     | 0.69           | 0.66      | 0.48        | 0.51   |
| 24       | 0.65          | 0.68     | 0.69           | 0.67      | 0.48        | 0.50   |
| 25       | 0.65          | 0.68     | 0.69           | 0.67      | 0.48        | 0.50   |
| 26       | 0.64          | 0.68     | 0.70           | 0.67      | 0.47        | 0.50   |
| 27       | 0.64          | 0.67     | 0.70           | 0.68      | 0.47        | 0.50   |
| 28       | 0.64          | 0.67     | 0.70           | 0.68      | 0.47        | 0.50   |
| 29       | 0.64          | 0.67     | 0.70           | 0.68      | 0.47        | 0.50   |
| 30       | 0.64          | 0.67     | 0.71           | 0.68      | 0.47        | 0.50   |
| 31       | 0.64          | 0.66     | 0.71           | 0.69      | 0.47        | 0.49   |

Continued on next page

| $\alpha$ | $\phi_S^\ell$ | $\phi_S$ | $\varphi^\ell$ | $\varphi$ | $\psi^\ell$ | $\psi$ |
|----------|---------------|----------|----------------|-----------|-------------|--------|
| 32       | 0.63          | 0.66     | 0.71           | 0.69      | 0.46        | 0.49   |
| 33       | 0.63          | 0.66     | 0.72           | 0.70      | 0.46        | 0.48   |
| 34       | 0.63          | 0.66     | 0.72           | 0.70      | 0.46        | 0.48   |
| 35       | 0.63          | 0.65     | 0.72           | 0.70      | 0.46        | 0.48   |
| 36       | 0.63          | 0.65     | 0.73           | 0.71      | 0.45        | 0.47   |
| 37       | 0.62          | 0.65     | 0.73           | 0.71      | 0.45        | 0.47   |
| 38       | 0.62          | 0.64     | 0.73           | 0.71      | 0.45        | 0.47   |
| 39       | 0.62          | 0.64     | 0.74           | 0.72      | 0.44        | 0.46   |
| 40       | 0.61          | 0.64     | 0.74           | 0.72      | 0.44        | 0.46   |
| 41       | 0.61          | 0.63     | 0.74           | 0.73      | 0.44        | 0.45   |
| 42       | 0.61          | 0.63     | 0.75           | 0.73      | 0.43        | 0.45   |
| 43       | 0.60          | 0.63     | 0.75           | 0.73      | 0.43        | 0.45   |
| 44       | 0.60          | 0.62     | 0.76           | 0.74      | 0.43        | 0.44   |
| 45       | 0.60          | 0.62     | 0.76           | 0.74      | 0.43        | 0.44   |
| 46       | 0.59          | 0.61     | 0.77           | 0.75      | 0.42        | 0.43   |
| 47       | 0.59          | 0.61     | 0.77           | 0.75      | 0.42        | 0.43   |
| 48       | 0.58          | 0.60     | 0.78           | 0.76      | 0.41        | 0.43   |
| 49       | 0.58          | 0.60     | 0.78           | 0.76      | 0.41        | 0.43   |
| 50       | 0.57          | 0.59     | 0.78           | 0.76      | 0.40        | 0.42   |
| 51       | 0.57          | 0.59     | 0.79           | 0.77      | 0.40        | 0.42   |
| 52       | 0.56          | 0.58     | 0.79           | 0.77      | 0.39        | 0.41   |
| 53       | 0.56          | 0.58     | 0.80           | 0.78      | 0.39        | 0.41   |
| 54       | 0.55          | 0.57     | 0.80           | 0.78      | 0.38        | 0.40   |
| 55       | 0.55          | 0.57     | 0.81           | 0.79      | 0.38        | 0.40   |
| 56       | 0.54          | 0.56     | 0.81           | 0.79      | 0.37        | 0.39   |
| 57       | 0.54          | 0.55     | 0.82           | 0.80      | 0.37        | 0.38   |
| 58       | 0.53          | 0.55     | 0.82           | 0.80      | 0.37        | 0.38   |
| 59       | 0.52          | 0.54     | 0.83           | 0.81      | 0.36        | 0.37   |
| 60       | 0.51          | 0.53     | 0.83           | 0.81      | 0.35        | 0.37   |
| 61       | 0.51          | 0.53     | 0.84           | 0.82      | 0.35        | 0.37   |
| 62       | 0.50          | 0.52     | 0.84           | 0.82      | 0.34        | 0.36   |
| 63       | 0.49          | 0.51     | 0.85           | 0.83      | 0.33        | 0.35   |

Continued on next page

| $\alpha$ | $\phi_S^\ell$ | $\phi_S$ | $\varphi^\ell$ | $\varphi$ | $\psi^\ell$ | $\psi$ |
|----------|---------------|----------|----------------|-----------|-------------|--------|
| 64       | 0.48          | 0.50     | 0.85           | 0.83      | 0.33        | 0.35   |
| 65       | 0.47          | 0.49     | 0.86           | 0.84      | 0.32        | 0.34   |
| 66       | 0.46          | 0.49     | 0.87           | 0.84      | 0.31        | 0.34   |
| 67       | 0.45          | 0.48     | 0.87           | 0.85      | 0.30        | 0.33   |
| 68       | 0.44          | 0.47     | 0.88           | 0.86      | 0.30        | 0.32   |
| 69       | 0.43          | 0.46     | 0.88           | 0.86      | 0.29        | 0.31   |
| 70       | 0.42          | 0.45     | 0.89           | 0.87      | 0.28        | 0.30   |
| 71       | 0.41          | 0.44     | 0.90           | 0.87      | 0.27        | 0.30   |
| 72       | 0.40          | 0.42     | 0.90           | 0.88      | 0.27        | 0.28   |
| 73       | 0.39          | 0.41     | 0.91           | 0.88      | 0.26        | 0.28   |
| 74       | 0.37          | 0.40     | 0.91           | 0.89      | 0.25        | 0.27   |
| 75       | 0.36          | 0.39     | 0.92           | 0.90      | 0.24        | 0.26   |
| 76       | 0.34          | 0.37     | 0.93           | 0.90      | 0.22        | 0.25   |
| 77       | 0.33          | 0.36     | 0.93           | 0.91      | 0.22        | 0.24   |
| 78       | 0.31          | 0.34     | 0.94           | 0.91      | 0.20        | 0.23   |
| 79       | 0.29          | 0.33     | 0.94           | 0.92      | 0.19        | 0.22   |
| 80       | 0.28          | 0.31     | 0.95           | 0.92      | 0.18        | 0.21   |
| 81       | 0.26          | 0.30     | 0.95           | 0.93      | 0.17        | 0.20   |
| 82       | 0.24          | 0.28     | 0.96           | 0.93      | 0.16        | 0.19   |
| 83       | 0.22          | 0.26     | 0.97           | 0.94      | 0.14        | 0.17   |
| 84       | 0.20          | 0.24     | 0.97           | 0.94      | 0.13        | 0.16   |
| 85       | 0.18          | 0.22     | 0.98           | 0.95      | 0.12        | 0.14   |
| 86       | 0.16          | 0.20     | 0.98           | 0.95      | 0.10        | 0.13   |
| 87       | 0.15          | 0.19     | 0.98           | 0.95      | 0.10        | 0.13   |
| 88       | 0.13          | 0.17     | 0.98           | 0.96      | 0.08        | 0.11   |
| 89       | 0.12          | 0.16     | 0.99           | 0.96      | 0.08        | 0.11   |
| 90       | 0.11          | 0.15     | 0.99           | 0.96      | 0.07        | 0.10   |

Table S124: Reference ( $\phi_S$ ,  $\varphi$ ,  $\psi$ ) and approached ( $\phi_S^\ell$ ,  $\varphi^\ell$ ,  $\psi^\ell$ ) values of the topological descriptors for the first excited-state of the pyridinium-phenolate (PP), computed at the M062X/6-31+G level of theory.  $\alpha$  is the pyridinium-phenolate central twist angle amplitude.

| $\alpha$ | $\phi_S^\ell$ | $\phi_S$ | $\varphi^\ell$ | $\varphi$ | $\psi^\ell$ | $\psi$ |
|----------|---------------|----------|----------------|-----------|-------------|--------|
| 0        | 0.70          | 0.73     | 0.65           | 0.61      | 0.52        | 0.56   |
| 1        | 0.70          | 0.73     | 0.65           | 0.61      | 0.52        | 0.56   |
| 2        | 0.69          | 0.73     | 0.65           | 0.61      | 0.52        | 0.56   |
| 3        | 0.69          | 0.73     | 0.65           | 0.61      | 0.52        | 0.56   |
| 4        | 0.69          | 0.73     | 0.65           | 0.61      | 0.52        | 0.56   |
| 5        | 0.69          | 0.73     | 0.65           | 0.61      | 0.52        | 0.56   |
| 6        | 0.69          | 0.73     | 0.65           | 0.62      | 0.52        | 0.55   |
| 7        | 0.69          | 0.72     | 0.65           | 0.62      | 0.52        | 0.55   |
| 8        | 0.69          | 0.72     | 0.65           | 0.62      | 0.52        | 0.55   |
| 9        | 0.69          | 0.72     | 0.65           | 0.62      | 0.52        | 0.55   |
| 10       | 0.69          | 0.72     | 0.65           | 0.62      | 0.52        | 0.55   |
| 11       | 0.69          | 0.72     | 0.65           | 0.62      | 0.52        | 0.55   |
| 12       | 0.69          | 0.72     | 0.65           | 0.62      | 0.52        | 0.55   |
| 13       | 0.69          | 0.72     | 0.66           | 0.63      | 0.51        | 0.54   |
| 14       | 0.69          | 0.72     | 0.66           | 0.63      | 0.51        | 0.54   |
| 15       | 0.69          | 0.72     | 0.66           | 0.63      | 0.51        | 0.54   |
| 16       | 0.68          | 0.71     | 0.66           | 0.63      | 0.51        | 0.54   |
| 17       | 0.68          | 0.71     | 0.66           | 0.63      | 0.51        | 0.54   |
| 18       | 0.68          | 0.71     | 0.66           | 0.64      | 0.51        | 0.53   |
| 19       | 0.68          | 0.71     | 0.67           | 0.64      | 0.50        | 0.53   |
| 20       | 0.68          | 0.71     | 0.67           | 0.64      | 0.50        | 0.53   |
| 21       | 0.68          | 0.71     | 0.67           | 0.64      | 0.50        | 0.53   |
| 22       | 0.68          | 0.70     | 0.67           | 0.65      | 0.50        | 0.52   |
| 23       | 0.68          | 0.70     | 0.67           | 0.65      | 0.50        | 0.52   |
| 24       | 0.67          | 0.70     | 0.68           | 0.65      | 0.50        | 0.52   |
| 25       | 0.67          | 0.70     | 0.68           | 0.65      | 0.50        | 0.52   |
| 26       | 0.67          | 0.70     | 0.68           | 0.66      | 0.50        | 0.52   |
| 27       | 0.67          | 0.69     | 0.68           | 0.66      | 0.50        | 0.51   |
| 28       | 0.67          | 0.69     | 0.69           | 0.66      | 0.49        | 0.51   |
| 29       | 0.67          | 0.69     | 0.69           | 0.67      | 0.49        | 0.51   |
| 30       | 0.67          | 0.69     | 0.69           | 0.67      | 0.49        | 0.51   |
| 31       | 0.66          | 0.69     | 0.70           | 0.67      | 0.48        | 0.51   |

Continued on next page

| $\alpha$ | $\phi_S^\ell$ | $\phi_S$ | $\varphi^\ell$ | $\varphi$ | $\psi^\ell$ | $\psi$ |
|----------|---------------|----------|----------------|-----------|-------------|--------|
| 32       | 0.66          | 0.68     | 0.70           | 0.68      | 0.48        | 0.50   |
| 33       | 0.66          | 0.68     | 0.70           | 0.68      | 0.48        | 0.50   |
| 34       | 0.66          | 0.68     | 0.71           | 0.68      | 0.48        | 0.50   |
| 35       | 0.66          | 0.67     | 0.71           | 0.69      | 0.48        | 0.49   |
| 36       | 0.65          | 0.67     | 0.71           | 0.69      | 0.47        | 0.49   |
| 37       | 0.65          | 0.67     | 0.72           | 0.69      | 0.47        | 0.49   |
| 38       | 0.65          | 0.67     | 0.72           | 0.70      | 0.47        | 0.49   |
| 39       | 0.65          | 0.66     | 0.72           | 0.70      | 0.47        | 0.48   |
| 40       | 0.64          | 0.66     | 0.73           | 0.71      | 0.46        | 0.48   |
| 41       | 0.64          | 0.66     | 0.73           | 0.71      | 0.46        | 0.48   |
| 42       | 0.64          | 0.65     | 0.73           | 0.71      | 0.46        | 0.47   |
| 43       | 0.63          | 0.65     | 0.74           | 0.72      | 0.45        | 0.47   |
| 44       | 0.63          | 0.64     | 0.74           | 0.72      | 0.45        | 0.46   |
| 45       | 0.63          | 0.64     | 0.75           | 0.73      | 0.44        | 0.46   |
| 46       | 0.62          | 0.64     | 0.75           | 0.73      | 0.44        | 0.46   |
| 47       | 0.62          | 0.63     | 0.76           | 0.73      | 0.44        | 0.45   |
| 48       | 0.61          | 0.63     | 0.76           | 0.74      | 0.43        | 0.45   |
| 49       | 0.61          | 0.62     | 0.76           | 0.74      | 0.43        | 0.44   |
| 50       | 0.61          | 0.62     | 0.77           | 0.75      | 0.43        | 0.44   |
| 51       | 0.60          | 0.61     | 0.77           | 0.75      | 0.42        | 0.43   |
| 52       | 0.60          | 0.61     | 0.78           | 0.76      | 0.42        | 0.43   |
| 53       | 0.59          | 0.60     | 0.78           | 0.76      | 0.41        | 0.43   |
| 54       | 0.58          | 0.60     | 0.79           | 0.77      | 0.40        | 0.42   |
| 55       | 0.58          | 0.59     | 0.79           | 0.77      | 0.40        | 0.42   |
| 56       | 0.57          | 0.59     | 0.80           | 0.78      | 0.39        | 0.41   |
| 57       | 0.57          | 0.58     | 0.80           | 0.78      | 0.39        | 0.41   |
| 58       | 0.56          | 0.57     | 0.81           | 0.79      | 0.39        | 0.40   |
| 59       | 0.55          | 0.57     | 0.81           | 0.79      | 0.38        | 0.40   |
| 60       | 0.55          | 0.56     | 0.82           | 0.80      | 0.38        | 0.39   |
| 61       | 0.54          | 0.55     | 0.82           | 0.80      | 0.37        | 0.38   |
| 62       | 0.53          | 0.55     | 0.83           | 0.81      | 0.36        | 0.38   |
| 63       | 0.52          | 0.54     | 0.83           | 0.81      | 0.36        | 0.37   |

Continued on next page

| $\alpha$ | $\phi_S^\ell$ | $\phi_S$ | $\varphi^\ell$ | $\varphi$ | $\psi^\ell$ | $\psi$ |
|----------|---------------|----------|----------------|-----------|-------------|--------|
| 64       | 0.52          | 0.53     | 0.84           | 0.82      | 0.35        | 0.37   |
| 65       | 0.51          | 0.52     | 0.84           | 0.82      | 0.35        | 0.36   |
| 66       | 0.50          | 0.51     | 0.85           | 0.83      | 0.34        | 0.35   |
| 67       | 0.49          | 0.51     | 0.86           | 0.83      | 0.33        | 0.35   |
| 68       | 0.48          | 0.50     | 0.86           | 0.84      | 0.32        | 0.34   |
| 69       | 0.47          | 0.49     | 0.87           | 0.85      | 0.32        | 0.33   |
| 70       | 0.46          | 0.48     | 0.87           | 0.85      | 0.31        | 0.33   |
| 71       | 0.45          | 0.47     | 0.88           | 0.86      | 0.30        | 0.32   |
| 72       | 0.44          | 0.46     | 0.89           | 0.86      | 0.29        | 0.31   |
| 73       | 0.42          | 0.44     | 0.89           | 0.87      | 0.28        | 0.30   |
| 74       | 0.41          | 0.43     | 0.90           | 0.88      | 0.27        | 0.29   |
| 75       | 0.40          | 0.42     | 0.91           | 0.88      | 0.26        | 0.28   |
| 76       | 0.38          | 0.41     | 0.91           | 0.89      | 0.25        | 0.27   |
| 77       | 0.36          | 0.39     | 0.92           | 0.89      | 0.24        | 0.26   |
| 78       | 0.35          | 0.38     | 0.93           | 0.90      | 0.23        | 0.25   |
| 79       | 0.33          | 0.36     | 0.93           | 0.91      | 0.22        | 0.24   |
| 80       | 0.31          | 0.34     | 0.94           | 0.91      | 0.20        | 0.23   |
| 81       | 0.29          | 0.33     | 0.95           | 0.92      | 0.19        | 0.22   |
| 82       | 0.27          | 0.31     | 0.95           | 0.93      | 0.18        | 0.20   |
| 83       | 0.25          | 0.29     | 0.96           | 0.93      | 0.16        | 0.19   |
| 84       | 0.22          | 0.27     | 0.97           | 0.94      | 0.14        | 0.18   |
| 85       | 0.20          | 0.24     | 0.97           | 0.94      | 0.13        | 0.16   |
| 86       | 0.17          | 0.22     | 0.98           | 0.95      | 0.11        | 0.14   |
| 87       | 0.15          | 0.20     | 0.98           | 0.95      | 0.10        | 0.13   |
| 88       | 0.13          | 0.18     | 0.99           | 0.96      | 0.08        | 0.12   |
| 89       | 0.11          | 0.16     | 0.99           | 0.96      | 0.07        | 0.11   |
| 90       | 0.10          | 0.15     | 0.99           | 0.96      | 0.06        | 0.10   |

Table S125: Reference ( $\phi_S$ ,  $\varphi$ ,  $\psi$ ) and approached ( $\phi_S^\ell$ ,  $\varphi^\ell$ ,  $\psi^\ell$ ) values of the topological descriptors for the first excited-state of the pyridinium-phenolate (PP), computed at the M062X/6-31G level of theory.  $\alpha$  is the pyridinium-phenolate central twist angle amplitude.



| $\alpha$ | $\phi_S^\ell$ | $\phi_S$ | $\varphi^\ell$ | $\varphi$ | $\psi^\ell$ | $\psi$ |
|----------|---------------|----------|----------------|-----------|-------------|--------|
| 0        | 0.44          | 0.33     | 0.81           | 0.85      | 0.32        | 0.24   |
| 1        | 0.44          | 0.33     | 0.81           | 0.85      | 0.32        | 0.24   |
| 2        | 0.44          | 0.33     | 0.81           | 0.85      | 0.32        | 0.24   |
| 3        | 0.44          | 0.33     | 0.81           | 0.85      | 0.32        | 0.24   |
| 4        | 0.43          | 0.33     | 0.81           | 0.85      | 0.31        | 0.24   |
| 5        | 0.43          | 0.33     | 0.81           | 0.85      | 0.31        | 0.24   |
| 6        | 0.43          | 0.33     | 0.81           | 0.85      | 0.31        | 0.24   |
| 7        | 0.42          | 0.33     | 0.82           | 0.85      | 0.30        | 0.24   |
| 8        | 0.42          | 0.33     | 0.82           | 0.85      | 0.30        | 0.24   |
| 9        | 0.42          | 0.33     | 0.82           | 0.85      | 0.30        | 0.24   |
| 10       | 0.41          | 0.33     | 0.82           | 0.85      | 0.30        | 0.24   |
| 11       | 0.41          | 0.33     | 0.83           | 0.85      | 0.29        | 0.24   |
| 12       | 0.40          | 0.33     | 0.83           | 0.85      | 0.29        | 0.24   |
| 13       | 0.39          | 0.33     | 0.83           | 0.85      | 0.28        | 0.24   |
| 14       | 0.39          | 0.33     | 0.83           | 0.85      | 0.28        | 0.24   |
| 15       | 0.38          | 0.33     | 0.84           | 0.86      | 0.27        | 0.23   |
| 16       | 0.37          | 0.33     | 0.84           | 0.86      | 0.26        | 0.23   |
| 17       | 0.36          | 0.33     | 0.84           | 0.86      | 0.26        | 0.23   |
| 18       | 0.36          | 0.33     | 0.84           | 0.86      | 0.26        | 0.23   |
| 19       | 0.35          | 0.33     | 0.85           | 0.86      | 0.25        | 0.23   |
| 20       | 0.34          | 0.33     | 0.85           | 0.86      | 0.24        | 0.23   |
| 21       | 0.33          | 0.33     | 0.85           | 0.86      | 0.24        | 0.23   |
| 22       | 0.32          | 0.33     | 0.85           | 0.86      | 0.23        | 0.23   |
| 23       | 0.31          | 0.33     | 0.86           | 0.86      | 0.22        | 0.23   |
| 24       | 0.30          | 0.33     | 0.86           | 0.86      | 0.21        | 0.23   |
| 25       | 0.29          | 0.33     | 0.86           | 0.86      | 0.21        | 0.23   |
| 26       | 0.28          | 0.33     | 0.87           | 0.86      | 0.20        | 0.23   |
| 27       | 0.27          | 0.33     | 0.88           | 0.86      | 0.19        | 0.23   |
| 28       | 0.26          | 0.33     | 0.89           | 0.86      | 0.18        | 0.23   |
| 29       | 0.25          | 0.33     | 0.90           | 0.86      | 0.17        | 0.23   |
| 30       | 0.24          | 0.33     | 0.91           | 0.86      | 0.16        | 0.23   |
| 31       | 0.23          | 0.33     | 0.91           | 0.86      | 0.16        | 0.23   |

Continued on next page

| $\alpha$ | $\phi_S^\ell$ | $\phi_S$ | $\varphi^\ell$ | $\varphi$ | $\psi^\ell$ | $\psi$ |
|----------|---------------|----------|----------------|-----------|-------------|--------|
| 32       | 0.22          | 0.32     | 0.92           | 0.86      | 0.15        | 0.23   |
| 33       | 0.20          | 0.32     | 0.93           | 0.87      | 0.13        | 0.22   |
| 34       | 0.19          | 0.32     | 0.94           | 0.87      | 0.13        | 0.22   |
| 35       | 0.18          | 0.32     | 0.95           | 0.87      | 0.12        | 0.22   |
| 36       | 0.17          | 0.32     | 0.95           | 0.87      | 0.11        | 0.22   |
| 37       | 0.16          | 0.32     | 0.96           | 0.87      | 0.11        | 0.22   |
| 38       | 0.15          | 0.32     | 0.96           | 0.87      | 0.10        | 0.22   |
| 39       | 0.14          | 0.32     | 0.97           | 0.87      | 0.09        | 0.22   |
| 40       | 0.13          | 0.31     | 0.97           | 0.87      | 0.08        | 0.22   |
| 41       | 0.12          | 0.31     | 0.98           | 0.87      | 0.08        | 0.22   |
| 42       | 0.11          | 0.31     | 0.98           | 0.87      | 0.07        | 0.22   |
| 43       | 0.11          | 0.31     | 0.98           | 0.88      | 0.07        | 0.22   |
| 44       | 0.10          | 0.31     | 0.98           | 0.88      | 0.06        | 0.22   |
| 45       | 0.09          | 0.30     | 0.98           | 0.88      | 0.06        | 0.21   |
| 46       | 0.09          | 0.30     | 0.98           | 0.88      | 0.06        | 0.21   |
| 47       | 0.09          | 0.30     | 0.98           | 0.88      | 0.06        | 0.21   |
| 48       | 0.10          | 0.30     | 0.98           | 0.88      | 0.06        | 0.21   |
| 49       | 0.11          | 0.30     | 0.98           | 0.88      | 0.07        | 0.21   |
| 50       | 0.12          | 0.29     | 0.98           | 0.88      | 0.08        | 0.20   |
| 51       | 0.13          | 0.29     | 0.98           | 0.89      | 0.08        | 0.20   |
| 52       | 0.14          | 0.29     | 0.97           | 0.89      | 0.09        | 0.20   |
| 53       | 0.15          | 0.29     | 0.97           | 0.89      | 0.10        | 0.20   |
| 54       | 0.16          | 0.29     | 0.96           | 0.89      | 0.11        | 0.20   |
| 55       | 0.17          | 0.28     | 0.96           | 0.89      | 0.11        | 0.19   |
| 56       | 0.18          | 0.28     | 0.95           | 0.89      | 0.12        | 0.19   |
| 57       | 0.19          | 0.28     | 0.95           | 0.89      | 0.13        | 0.19   |
| 58       | 0.20          | 0.28     | 0.94           | 0.90      | 0.13        | 0.19   |
| 59       | 0.21          | 0.27     | 0.93           | 0.90      | 0.14        | 0.19   |
| 60       | 0.22          | 0.27     | 0.92           | 0.90      | 0.15        | 0.19   |
| 61       | 0.22          | 0.27     | 0.91           | 0.90      | 0.15        | 0.19   |
| 62       | 0.23          | 0.26     | 0.90           | 0.90      | 0.16        | 0.18   |
| 63       | 0.24          | 0.26     | 0.90           | 0.90      | 0.17        | 0.18   |

Continued on next page

| $\alpha$ | $\phi_S^\ell$ | $\phi_S$ | $\varphi^\ell$ | $\varphi$ | $\psi^\ell$ | $\psi$ |
|----------|---------------|----------|----------------|-----------|-------------|--------|
| 64       | 0.24          | 0.26     | 0.90           | 0.90      | 0.17        | 0.18   |
| 65       | 0.25          | 0.26     | 0.90           | 0.91      | 0.17        | 0.18   |
| 66       | 0.26          | 0.25     | 0.90           | 0.91      | 0.18        | 0.17   |
| 67       | 0.26          | 0.25     | 0.90           | 0.91      | 0.18        | 0.17   |
| 68       | 0.27          | 0.25     | 0.90           | 0.91      | 0.19        | 0.17   |
| 69       | 0.27          | 0.24     | 0.90           | 0.91      | 0.19        | 0.16   |
| 70       | 0.62          | 0.62     | 0.77           | 0.76      | 0.43        | 0.44   |
| 71       | 0.61          | 0.61     | 0.78           | 0.76      | 0.42        | 0.43   |
| 72       | 0.60          | 0.60     | 0.78           | 0.77      | 0.42        | 0.42   |
| 73       | 0.60          | 0.60     | 0.79           | 0.77      | 0.41        | 0.42   |
| 74       | 0.59          | 0.59     | 0.79           | 0.78      | 0.41        | 0.41   |
| 75       | 0.58          | 0.58     | 0.80           | 0.79      | 0.40        | 0.40   |
| 76       | 0.58          | 0.58     | 0.81           | 0.79      | 0.40        | 0.40   |
| 77       | 0.57          | 0.57     | 0.81           | 0.80      | 0.39        | 0.39   |
| 78       | 0.56          | 0.56     | 0.82           | 0.80      | 0.38        | 0.39   |
| 79       | 0.55          | 0.55     | 0.82           | 0.81      | 0.38        | 0.38   |
| 80       | 0.54          | 0.54     | 0.83           | 0.81      | 0.37        | 0.37   |
| 81       | 0.53          | 0.53     | 0.84           | 0.82      | 0.36        | 0.37   |
| 82       | 0.52          | 0.52     | 0.85           | 0.83      | 0.35        | 0.36   |
| 83       | 0.51          | 0.51     | 0.85           | 0.84      | 0.34        | 0.35   |
| 84       | 0.49          | 0.50     | 0.86           | 0.84      | 0.33        | 0.34   |
| 85       | 0.48          | 0.48     | 0.87           | 0.85      | 0.32        | 0.33   |
| 86       | 0.46          | 0.47     | 0.88           | 0.86      | 0.31        | 0.32   |
| 87       | 0.44          | 0.45     | 0.89           | 0.87      | 0.29        | 0.30   |
| 88       | 0.42          | 0.43     | 0.90           | 0.88      | 0.28        | 0.29   |
| 89       | 0.39          | 0.41     | 0.91           | 0.89      | 0.26        | 0.27   |
| 90       | 0.09          | 0.15     | 0.99           | 0.96      | 0.06        | 0.10   |

Table S126: Reference ( $\phi_S$ ,  $\varphi$ ,  $\psi$ ) and approached ( $\phi_S^\ell$ ,  $\varphi^\ell$ ,  $\psi^\ell$ ) values of the topological descriptors for the first excited-state of the pyridinium-phenolate (PP), computed at the PBE0/3-21G level of theory.  $\alpha$  is the pyridinium-phenolate central twist angle amplitude.

| $\alpha$ | $\phi_S^\ell$ | $\phi_S$ | $\varphi^\ell$ | $\varphi$ | $\psi^\ell$ | $\psi$ |
|----------|---------------|----------|----------------|-----------|-------------|--------|
| 0        | 0.42          | 0.32     | 0.83           | 0.86      | 0.30        | 0.23   |
| 1        | 0.42          | 0.32     | 0.83           | 0.86      | 0.30        | 0.23   |
| 2        | 0.42          | 0.32     | 0.83           | 0.86      | 0.30        | 0.23   |
| 3        | 0.42          | 0.32     | 0.83           | 0.86      | 0.30        | 0.23   |
| 4        | 0.42          | 0.32     | 0.83           | 0.86      | 0.30        | 0.23   |
| 5        | 0.42          | 0.32     | 0.84           | 0.86      | 0.30        | 0.23   |
| 6        | 0.41          | 0.33     | 0.84           | 0.86      | 0.29        | 0.23   |
| 7        | 0.41          | 0.33     | 0.84           | 0.86      | 0.29        | 0.23   |
| 8        | 0.41          | 0.33     | 0.84           | 0.86      | 0.29        | 0.23   |
| 9        | 0.41          | 0.33     | 0.84           | 0.86      | 0.29        | 0.23   |
| 10       | 0.41          | 0.34     | 0.84           | 0.86      | 0.29        | 0.24   |
| 11       | 0.41          | 0.34     | 0.85           | 0.86      | 0.29        | 0.24   |
| 12       | 0.40          | 0.34     | 0.85           | 0.86      | 0.28        | 0.24   |
| 13       | 0.40          | 0.35     | 0.85           | 0.86      | 0.28        | 0.25   |
| 14       | 0.40          | 0.35     | 0.85           | 0.86      | 0.28        | 0.25   |
| 15       | 0.40          | 0.35     | 0.85           | 0.86      | 0.28        | 0.25   |
| 16       | 0.39          | 0.35     | 0.85           | 0.86      | 0.27        | 0.25   |
| 17       | 0.39          | 0.36     | 0.86           | 0.86      | 0.27        | 0.25   |
| 18       | 0.39          | 0.36     | 0.86           | 0.86      | 0.27        | 0.25   |
| 19       | 0.38          | 0.36     | 0.86           | 0.86      | 0.26        | 0.25   |
| 20       | 0.38          | 0.36     | 0.86           | 0.86      | 0.26        | 0.25   |
| 21       | 0.38          | 0.37     | 0.86           | 0.86      | 0.26        | 0.26   |
| 22       | 0.37          | 0.37     | 0.86           | 0.86      | 0.26        | 0.26   |
| 23       | 0.37          | 0.37     | 0.86           | 0.86      | 0.26        | 0.26   |
| 24       | 0.37          | 0.37     | 0.86           | 0.86      | 0.26        | 0.26   |
| 25       | 0.36          | 0.38     | 0.86           | 0.85      | 0.25        | 0.27   |
| 26       | 0.36          | 0.38     | 0.86           | 0.85      | 0.25        | 0.27   |
| 27       | 0.36          | 0.38     | 0.86           | 0.85      | 0.25        | 0.27   |
| 28       | 0.35          | 0.38     | 0.86           | 0.85      | 0.25        | 0.27   |
| 29       | 0.35          | 0.39     | 0.86           | 0.85      | 0.25        | 0.27   |
| 30       | 0.35          | 0.39     | 0.86           | 0.85      | 0.25        | 0.27   |
| 31       | 0.35          | 0.39     | 0.86           | 0.85      | 0.25        | 0.27   |

Continued on next page

| $\alpha$ | $\phi_S^\ell$ | $\phi_S$ | $\varphi^\ell$ | $\varphi$ | $\psi^\ell$ | $\psi$ |
|----------|---------------|----------|----------------|-----------|-------------|--------|
| 32       | 0.35          | 0.40     | 0.85           | 0.85      | 0.25        | 0.28   |
| 33       | 0.35          | 0.40     | 0.85           | 0.85      | 0.25        | 0.28   |
| 34       | 0.35          | 0.40     | 0.85           | 0.85      | 0.25        | 0.28   |
| 35       | 0.35          | 0.41     | 0.84           | 0.85      | 0.25        | 0.29   |
| 36       | 0.35          | 0.42     | 0.84           | 0.84      | 0.25        | 0.30   |
| 37       | 0.36          | 0.42     | 0.83           | 0.84      | 0.26        | 0.30   |
| 38       | 0.36          | 0.43     | 0.83           | 0.84      | 0.26        | 0.30   |
| 39       | 0.37          | 0.44     | 0.83           | 0.83      | 0.27        | 0.31   |
| 40       | 0.38          | 0.45     | 0.82           | 0.83      | 0.28        | 0.32   |
| 41       | 0.39          | 0.46     | 0.82           | 0.82      | 0.28        | 0.33   |
| 42       | 0.41          | 0.48     | 0.81           | 0.82      | 0.30        | 0.34   |
| 43       | 0.43          | 0.49     | 0.81           | 0.81      | 0.31        | 0.35   |
| 44       | 0.46          | 0.51     | 0.80           | 0.80      | 0.33        | 0.36   |
| 45       | 0.48          | 0.53     | 0.79           | 0.78      | 0.35        | 0.38   |
| 46       | 0.51          | 0.55     | 0.78           | 0.77      | 0.37        | 0.39   |
| 47       | 0.54          | 0.57     | 0.77           | 0.76      | 0.39        | 0.41   |
| 48       | 0.56          | 0.59     | 0.76           | 0.75      | 0.40        | 0.42   |
| 49       | 0.58          | 0.60     | 0.76           | 0.74      | 0.41        | 0.43   |
| 50       | 0.60          | 0.61     | 0.75           | 0.74      | 0.43        | 0.44   |
| 51       | 0.61          | 0.62     | 0.75           | 0.74      | 0.43        | 0.44   |
| 52       | 0.61          | 0.63     | 0.75           | 0.74      | 0.43        | 0.45   |
| 53       | 0.61          | 0.63     | 0.75           | 0.74      | 0.43        | 0.45   |
| 54       | 0.61          | 0.63     | 0.75           | 0.74      | 0.43        | 0.45   |
| 55       | 0.61          | 0.63     | 0.76           | 0.74      | 0.43        | 0.45   |
| 56       | 0.61          | 0.63     | 0.76           | 0.74      | 0.43        | 0.45   |
| 57       | 0.61          | 0.62     | 0.76           | 0.75      | 0.43        | 0.44   |
| 58       | 0.61          | 0.62     | 0.77           | 0.75      | 0.43        | 0.44   |
| 59       | 0.60          | 0.62     | 0.77           | 0.75      | 0.42        | 0.44   |
| 60       | 0.60          | 0.61     | 0.77           | 0.76      | 0.42        | 0.43   |
| 61       | 0.60          | 0.61     | 0.78           | 0.76      | 0.42        | 0.43   |
| 62       | 0.59          | 0.60     | 0.78           | 0.77      | 0.41        | 0.42   |
| 63       | 0.59          | 0.60     | 0.79           | 0.77      | 0.41        | 0.42   |

Continued on next page

| $\alpha$ | $\phi_S^\ell$ | $\phi_S$ | $\varphi^\ell$ | $\varphi$ | $\psi^\ell$ | $\psi$ |
|----------|---------------|----------|----------------|-----------|-------------|--------|
| 64       | 0.58          | 0.59     | 0.79           | 0.78      | 0.40        | 0.41   |
| 65       | 0.57          | 0.59     | 0.80           | 0.78      | 0.39        | 0.41   |
| 66       | 0.57          | 0.58     | 0.80           | 0.78      | 0.39        | 0.41   |
| 67       | 0.56          | 0.57     | 0.81           | 0.79      | 0.39        | 0.40   |
| 68       | 0.56          | 0.57     | 0.81           | 0.79      | 0.39        | 0.40   |
| 69       | 0.55          | 0.56     | 0.82           | 0.80      | 0.38        | 0.39   |
| 70       | 0.54          | 0.55     | 0.82           | 0.80      | 0.37        | 0.38   |
| 71       | 0.53          | 0.54     | 0.83           | 0.81      | 0.36        | 0.37   |
| 72       | 0.53          | 0.54     | 0.83           | 0.82      | 0.36        | 0.37   |
| 73       | 0.52          | 0.53     | 0.84           | 0.82      | 0.35        | 0.37   |
| 74       | 0.51          | 0.52     | 0.84           | 0.83      | 0.35        | 0.36   |
| 75       | 0.50          | 0.51     | 0.85           | 0.83      | 0.34        | 0.35   |
| 76       | 0.49          | 0.50     | 0.85           | 0.84      | 0.33        | 0.34   |
| 77       | 0.48          | 0.49     | 0.86           | 0.85      | 0.32        | 0.33   |
| 78       | 0.46          | 0.48     | 0.87           | 0.85      | 0.31        | 0.33   |
| 79       | 0.45          | 0.46     | 0.87           | 0.86      | 0.30        | 0.31   |
| 80       | 0.44          | 0.45     | 0.88           | 0.87      | 0.30        | 0.30   |
| 81       | 0.42          | 0.44     | 0.89           | 0.87      | 0.28        | 0.30   |
| 82       | 0.40          | 0.42     | 0.90           | 0.88      | 0.27        | 0.28   |
| 83       | 0.39          | 0.40     | 0.90           | 0.89      | 0.26        | 0.27   |
| 84       | 0.37          | 0.38     | 0.91           | 0.90      | 0.25        | 0.25   |
| 85       | 0.34          | 0.36     | 0.92           | 0.91      | 0.23        | 0.24   |
| 86       | 0.31          | 0.33     | 0.93           | 0.92      | 0.20        | 0.22   |
| 87       | 0.28          | 0.30     | 0.94           | 0.93      | 0.18        | 0.20   |
| 88       | 0.23          | 0.26     | 0.96           | 0.94      | 0.15        | 0.17   |
| 89       | 0.18          | 0.21     | 0.97           | 0.95      | 0.12        | 0.14   |
| 90       | 0.12          | 0.15     | 0.98           | 0.96      | 0.08        | 0.10   |

Table S127: Reference ( $\phi_S$ ,  $\varphi$ ,  $\psi$ ) and approached ( $\phi_S^\ell$ ,  $\varphi^\ell$ ,  $\psi^\ell$ ) values of the topological descriptors for the first excited-state of the pyridinium-phenolate (PP), computed at the PBE0/6-311++G(2d,p) level of theory.  $\alpha$  is the pyridinium-phenolate central twist angle amplitude.

| $\alpha$ | $\phi_S^\ell$ | $\phi_S$ | $\varphi^\ell$ | $\varphi$ | $\psi^\ell$ | $\psi$ |
|----------|---------------|----------|----------------|-----------|-------------|--------|
| 0        | 0.41          | 0.32     | 0.83           | 0.86      | 0.29        | 0.23   |
| 1        | 0.41          | 0.32     | 0.83           | 0.86      | 0.29        | 0.23   |
| 2        | 0.41          | 0.32     | 0.83           | 0.86      | 0.29        | 0.23   |
| 3        | 0.41          | 0.32     | 0.83           | 0.86      | 0.29        | 0.23   |
| 4        | 0.41          | 0.32     | 0.83           | 0.86      | 0.29        | 0.23   |
| 5        | 0.41          | 0.33     | 0.84           | 0.86      | 0.29        | 0.23   |
| 6        | 0.41          | 0.33     | 0.84           | 0.86      | 0.29        | 0.23   |
| 7        | 0.41          | 0.33     | 0.84           | 0.86      | 0.29        | 0.23   |
| 8        | 0.41          | 0.33     | 0.84           | 0.86      | 0.29        | 0.23   |
| 9        | 0.40          | 0.33     | 0.84           | 0.86      | 0.28        | 0.23   |
| 10       | 0.40          | 0.34     | 0.85           | 0.86      | 0.28        | 0.24   |
| 11       | 0.40          | 0.34     | 0.85           | 0.86      | 0.28        | 0.24   |
| 12       | 0.40          | 0.34     | 0.85           | 0.86      | 0.28        | 0.24   |
| 13       | 0.39          | 0.34     | 0.85           | 0.86      | 0.27        | 0.24   |
| 14       | 0.39          | 0.35     | 0.85           | 0.86      | 0.27        | 0.25   |
| 15       | 0.39          | 0.35     | 0.85           | 0.86      | 0.27        | 0.25   |
| 16       | 0.38          | 0.35     | 0.86           | 0.86      | 0.26        | 0.25   |
| 17       | 0.38          | 0.35     | 0.86           | 0.86      | 0.26        | 0.25   |
| 18       | 0.38          | 0.36     | 0.86           | 0.86      | 0.26        | 0.25   |
| 19       | 0.37          | 0.36     | 0.86           | 0.86      | 0.26        | 0.25   |
| 20       | 0.37          | 0.36     | 0.86           | 0.86      | 0.26        | 0.25   |
| 21       | 0.36          | 0.36     | 0.86           | 0.86      | 0.25        | 0.25   |
| 22       | 0.36          | 0.36     | 0.87           | 0.86      | 0.25        | 0.25   |
| 23       | 0.36          | 0.37     | 0.87           | 0.86      | 0.25        | 0.26   |
| 24       | 0.35          | 0.37     | 0.87           | 0.86      | 0.24        | 0.26   |
| 25       | 0.35          | 0.37     | 0.87           | 0.86      | 0.24        | 0.26   |
| 26       | 0.35          | 0.37     | 0.87           | 0.86      | 0.24        | 0.26   |
| 27       | 0.34          | 0.37     | 0.87           | 0.86      | 0.24        | 0.26   |
| 28       | 0.34          | 0.38     | 0.87           | 0.85      | 0.24        | 0.27   |
| 29       | 0.34          | 0.38     | 0.87           | 0.85      | 0.24        | 0.27   |
| 30       | 0.33          | 0.38     | 0.87           | 0.85      | 0.23        | 0.27   |
| 31       | 0.33          | 0.38     | 0.86           | 0.85      | 0.23        | 0.27   |

Continued on next page

| $\alpha$ | $\phi_S^\ell$ | $\phi_S$ | $\varphi^\ell$ | $\varphi$ | $\psi^\ell$ | $\psi$ |
|----------|---------------|----------|----------------|-----------|-------------|--------|
| 32       | 0.33          | 0.39     | 0.86           | 0.85      | 0.23        | 0.27   |
| 33       | 0.33          | 0.39     | 0.86           | 0.85      | 0.23        | 0.27   |
| 34       | 0.33          | 0.39     | 0.86           | 0.85      | 0.23        | 0.27   |
| 35       | 0.33          | 0.40     | 0.85           | 0.85      | 0.24        | 0.28   |
| 36       | 0.33          | 0.40     | 0.85           | 0.85      | 0.24        | 0.28   |
| 37       | 0.33          | 0.41     | 0.84           | 0.85      | 0.24        | 0.29   |
| 38       | 0.34          | 0.42     | 0.84           | 0.84      | 0.24        | 0.30   |
| 39       | 0.34          | 0.42     | 0.83           | 0.84      | 0.25        | 0.30   |
| 40       | 0.35          | 0.43     | 0.83           | 0.84      | 0.25        | 0.30   |
| 41       | 0.36          | 0.44     | 0.83           | 0.83      | 0.26        | 0.31   |
| 42       | 0.38          | 0.46     | 0.82           | 0.83      | 0.28        | 0.32   |
| 43       | 0.40          | 0.47     | 0.82           | 0.82      | 0.29        | 0.33   |
| 44       | 0.42          | 0.49     | 0.81           | 0.81      | 0.30        | 0.35   |
| 45       | 0.45          | 0.51     | 0.80           | 0.80      | 0.33        | 0.36   |
| 46       | 0.48          | 0.53     | 0.79           | 0.79      | 0.35        | 0.38   |
| 47       | 0.51          | 0.55     | 0.78           | 0.77      | 0.37        | 0.39   |
| 48       | 0.54          | 0.57     | 0.77           | 0.76      | 0.39        | 0.41   |
| 49       | 0.57          | 0.59     | 0.76           | 0.75      | 0.41        | 0.42   |
| 50       | 0.59          | 0.60     | 0.76           | 0.74      | 0.42        | 0.43   |
| 51       | 0.60          | 0.62     | 0.75           | 0.74      | 0.43        | 0.44   |
| 52       | 0.61          | 0.62     | 0.75           | 0.74      | 0.43        | 0.44   |
| 53       | 0.62          | 0.63     | 0.75           | 0.74      | 0.44        | 0.45   |
| 54       | 0.62          | 0.63     | 0.75           | 0.74      | 0.44        | 0.45   |
| 55       | 0.62          | 0.63     | 0.75           | 0.74      | 0.44        | 0.45   |
| 56       | 0.62          | 0.63     | 0.75           | 0.74      | 0.44        | 0.45   |
| 57       | 0.62          | 0.63     | 0.76           | 0.74      | 0.44        | 0.45   |
| 58       | 0.61          | 0.62     | 0.76           | 0.75      | 0.43        | 0.44   |
| 59       | 0.61          | 0.62     | 0.76           | 0.75      | 0.43        | 0.44   |
| 60       | 0.61          | 0.61     | 0.77           | 0.76      | 0.43        | 0.43   |
| 61       | 0.60          | 0.61     | 0.77           | 0.76      | 0.42        | 0.43   |
| 62       | 0.60          | 0.61     | 0.78           | 0.76      | 0.42        | 0.43   |
| 63       | 0.59          | 0.60     | 0.78           | 0.77      | 0.41        | 0.42   |

Continued on next page



| $\alpha$ | $\phi_S^\ell$ | $\phi_S$ | $\varphi^\ell$ | $\varphi$ | $\psi^\ell$ | $\psi$ |
|----------|---------------|----------|----------------|-----------|-------------|--------|
| 64       | 0.59          | 0.59     | 0.79           | 0.77      | 0.41        | 0.42   |
| 65       | 0.58          | 0.59     | 0.79           | 0.78      | 0.40        | 0.41   |
| 66       | 0.57          | 0.58     | 0.80           | 0.78      | 0.39        | 0.41   |
| 67       | 0.57          | 0.58     | 0.80           | 0.79      | 0.39        | 0.40   |
| 68       | 0.56          | 0.57     | 0.81           | 0.79      | 0.39        | 0.40   |
| 69       | 0.55          | 0.56     | 0.81           | 0.80      | 0.38        | 0.39   |
| 70       | 0.55          | 0.56     | 0.82           | 0.80      | 0.38        | 0.39   |
| 71       | 0.54          | 0.55     | 0.82           | 0.81      | 0.37        | 0.38   |
| 72       | 0.53          | 0.54     | 0.83           | 0.81      | 0.36        | 0.37   |
| 73       | 0.52          | 0.53     | 0.84           | 0.82      | 0.35        | 0.37   |
| 74       | 0.51          | 0.52     | 0.84           | 0.82      | 0.35        | 0.36   |
| 75       | 0.50          | 0.51     | 0.85           | 0.83      | 0.34        | 0.35   |
| 76       | 0.49          | 0.50     | 0.85           | 0.84      | 0.33        | 0.34   |
| 77       | 0.48          | 0.49     | 0.86           | 0.84      | 0.32        | 0.34   |
| 78       | 0.47          | 0.48     | 0.87           | 0.85      | 0.32        | 0.33   |
| 79       | 0.46          | 0.47     | 0.87           | 0.86      | 0.31        | 0.32   |
| 80       | 0.44          | 0.46     | 0.88           | 0.86      | 0.30        | 0.31   |
| 81       | 0.43          | 0.44     | 0.89           | 0.87      | 0.29        | 0.30   |
| 82       | 0.41          | 0.43     | 0.90           | 0.88      | 0.27        | 0.29   |
| 83       | 0.39          | 0.41     | 0.91           | 0.89      | 0.26        | 0.27   |
| 84       | 0.37          | 0.39     | 0.92           | 0.90      | 0.24        | 0.26   |
| 85       | 0.34          | 0.37     | 0.93           | 0.90      | 0.22        | 0.25   |
| 86       | 0.32          | 0.34     | 0.94           | 0.91      | 0.21        | 0.23   |
| 87       | 0.28          | 0.31     | 0.95           | 0.93      | 0.18        | 0.20   |
| 88       | 0.24          | 0.27     | 0.96           | 0.94      | 0.16        | 0.18   |
| 89       | 0.17          | 0.22     | 0.98           | 0.95      | 0.11        | 0.14   |
| 90       | 0.11          | 0.15     | 0.99           | 0.96      | 0.07        | 0.10   |

Table S128: Reference ( $\phi_S$ ,  $\varphi$ ,  $\psi$ ) and approached ( $\phi_S^\ell$ ,  $\varphi^\ell$ ,  $\psi^\ell$ ) values of the topological descriptors for the first excited-state of the pyridinium-phenolate (PP), computed at the PBE0/6-311++G(d,p) level of theory.  $\alpha$  is the pyridinium-phenolate central twist angle amplitude.

| $\alpha$ | $\phi_S^\ell$ | $\phi_S$ | $\varphi^\ell$ | $\varphi$ | $\psi^\ell$ | $\psi$ |
|----------|---------------|----------|----------------|-----------|-------------|--------|
| 0        | 0.41          | 0.32     | 0.83           | 0.86      | 0.29        | 0.23   |
| 1        | 0.41          | 0.32     | 0.83           | 0.86      | 0.29        | 0.23   |
| 2        | 0.41          | 0.32     | 0.83           | 0.86      | 0.29        | 0.23   |
| 3        | 0.41          | 0.32     | 0.83           | 0.86      | 0.29        | 0.23   |
| 4        | 0.41          | 0.32     | 0.83           | 0.86      | 0.29        | 0.23   |
| 5        | 0.41          | 0.33     | 0.84           | 0.86      | 0.29        | 0.23   |
| 6        | 0.41          | 0.33     | 0.84           | 0.86      | 0.29        | 0.23   |
| 7        | 0.41          | 0.33     | 0.84           | 0.86      | 0.29        | 0.23   |
| 8        | 0.41          | 0.33     | 0.84           | 0.86      | 0.29        | 0.23   |
| 9        | 0.40          | 0.33     | 0.84           | 0.86      | 0.28        | 0.23   |
| 10       | 0.40          | 0.34     | 0.85           | 0.86      | 0.28        | 0.24   |
| 11       | 0.40          | 0.34     | 0.85           | 0.86      | 0.28        | 0.24   |
| 12       | 0.40          | 0.34     | 0.85           | 0.86      | 0.28        | 0.24   |
| 13       | 0.39          | 0.34     | 0.85           | 0.86      | 0.27        | 0.24   |
| 14       | 0.39          | 0.35     | 0.85           | 0.86      | 0.27        | 0.25   |
| 15       | 0.39          | 0.35     | 0.85           | 0.86      | 0.27        | 0.25   |
| 16       | 0.38          | 0.35     | 0.86           | 0.86      | 0.26        | 0.25   |
| 17       | 0.38          | 0.35     | 0.86           | 0.86      | 0.26        | 0.25   |
| 18       | 0.38          | 0.36     | 0.86           | 0.86      | 0.26        | 0.25   |
| 19       | 0.37          | 0.36     | 0.86           | 0.86      | 0.26        | 0.25   |
| 20       | 0.37          | 0.36     | 0.86           | 0.86      | 0.26        | 0.25   |
| 21       | 0.36          | 0.36     | 0.86           | 0.86      | 0.25        | 0.25   |
| 22       | 0.36          | 0.36     | 0.87           | 0.86      | 0.25        | 0.25   |
| 23       | 0.36          | 0.37     | 0.87           | 0.86      | 0.25        | 0.26   |
| 24       | 0.35          | 0.37     | 0.87           | 0.86      | 0.24        | 0.26   |
| 25       | 0.35          | 0.37     | 0.87           | 0.86      | 0.24        | 0.26   |
| 26       | 0.34          | 0.37     | 0.87           | 0.86      | 0.24        | 0.26   |
| 27       | 0.34          | 0.37     | 0.87           | 0.86      | 0.24        | 0.26   |
| 28       | 0.34          | 0.38     | 0.87           | 0.85      | 0.24        | 0.27   |
| 29       | 0.34          | 0.38     | 0.87           | 0.85      | 0.24        | 0.27   |
| 30       | 0.33          | 0.38     | 0.87           | 0.85      | 0.23        | 0.27   |
| 31       | 0.33          | 0.38     | 0.86           | 0.85      | 0.23        | 0.27   |

Continued on next page

| $\alpha$ | $\phi_S^\ell$ | $\phi_S$ | $\varphi^\ell$ | $\varphi$ | $\psi^\ell$ | $\psi$ |
|----------|---------------|----------|----------------|-----------|-------------|--------|
| 32       | 0.33          | 0.39     | 0.86           | 0.85      | 0.23        | 0.27   |
| 33       | 0.33          | 0.39     | 0.86           | 0.85      | 0.23        | 0.27   |
| 34       | 0.33          | 0.39     | 0.86           | 0.85      | 0.23        | 0.27   |
| 35       | 0.33          | 0.40     | 0.85           | 0.85      | 0.24        | 0.28   |
| 36       | 0.33          | 0.40     | 0.85           | 0.85      | 0.24        | 0.28   |
| 37       | 0.33          | 0.41     | 0.84           | 0.85      | 0.24        | 0.29   |
| 38       | 0.34          | 0.42     | 0.84           | 0.84      | 0.24        | 0.30   |
| 39       | 0.34          | 0.42     | 0.83           | 0.84      | 0.25        | 0.30   |
| 40       | 0.35          | 0.43     | 0.83           | 0.84      | 0.25        | 0.30   |
| 41       | 0.36          | 0.44     | 0.83           | 0.83      | 0.26        | 0.31   |
| 42       | 0.38          | 0.46     | 0.82           | 0.83      | 0.28        | 0.32   |
| 43       | 0.40          | 0.47     | 0.82           | 0.82      | 0.29        | 0.33   |
| 44       | 0.42          | 0.49     | 0.81           | 0.81      | 0.30        | 0.35   |
| 45       | 0.45          | 0.51     | 0.80           | 0.80      | 0.33        | 0.36   |
| 46       | 0.48          | 0.53     | 0.79           | 0.79      | 0.35        | 0.38   |
| 47       | 0.51          | 0.55     | 0.78           | 0.77      | 0.37        | 0.39   |
| 48       | 0.54          | 0.57     | 0.77           | 0.76      | 0.39        | 0.41   |
| 49       | 0.57          | 0.59     | 0.76           | 0.75      | 0.41        | 0.42   |
| 50       | 0.59          | 0.60     | 0.76           | 0.74      | 0.42        | 0.43   |
| 51       | 0.60          | 0.62     | 0.75           | 0.74      | 0.43        | 0.44   |
| 52       | 0.61          | 0.62     | 0.75           | 0.74      | 0.43        | 0.44   |
| 53       | 0.62          | 0.63     | 0.75           | 0.74      | 0.44        | 0.45   |
| 54       | 0.62          | 0.63     | 0.75           | 0.74      | 0.44        | 0.45   |
| 55       | 0.62          | 0.63     | 0.75           | 0.74      | 0.44        | 0.45   |
| 56       | 0.62          | 0.63     | 0.76           | 0.74      | 0.44        | 0.45   |
| 57       | 0.62          | 0.63     | 0.76           | 0.74      | 0.44        | 0.45   |
| 58       | 0.61          | 0.62     | 0.76           | 0.75      | 0.43        | 0.44   |
| 59       | 0.61          | 0.62     | 0.76           | 0.75      | 0.43        | 0.44   |
| 60       | 0.61          | 0.61     | 0.77           | 0.76      | 0.43        | 0.43   |
| 61       | 0.60          | 0.61     | 0.77           | 0.76      | 0.42        | 0.43   |
| 62       | 0.60          | 0.61     | 0.78           | 0.76      | 0.42        | 0.43   |
| 63       | 0.59          | 0.60     | 0.78           | 0.77      | 0.41        | 0.42   |

Continued on next page

| $\alpha$ | $\phi_S^\ell$ | $\phi_S$ | $\varphi^\ell$ | $\varphi$ | $\psi^\ell$ | $\psi$ |
|----------|---------------|----------|----------------|-----------|-------------|--------|
| 64       | 0.59          | 0.59     | 0.79           | 0.77      | 0.41        | 0.42   |
| 65       | 0.58          | 0.59     | 0.79           | 0.78      | 0.40        | 0.41   |
| 66       | 0.57          | 0.58     | 0.80           | 0.78      | 0.39        | 0.41   |
| 67       | 0.57          | 0.58     | 0.80           | 0.79      | 0.39        | 0.40   |
| 68       | 0.56          | 0.57     | 0.81           | 0.79      | 0.39        | 0.40   |
| 69       | 0.55          | 0.56     | 0.81           | 0.80      | 0.38        | 0.39   |
| 70       | 0.55          | 0.56     | 0.82           | 0.80      | 0.38        | 0.39   |
| 71       | 0.54          | 0.55     | 0.82           | 0.81      | 0.37        | 0.38   |
| 72       | 0.53          | 0.54     | 0.83           | 0.81      | 0.36        | 0.37   |
| 73       | 0.52          | 0.53     | 0.84           | 0.82      | 0.35        | 0.37   |
| 74       | 0.51          | 0.52     | 0.84           | 0.82      | 0.35        | 0.36   |
| 75       | 0.50          | 0.51     | 0.85           | 0.83      | 0.34        | 0.35   |
| 76       | 0.49          | 0.50     | 0.85           | 0.84      | 0.33        | 0.34   |
| 77       | 0.48          | 0.49     | 0.86           | 0.84      | 0.32        | 0.34   |
| 78       | 0.47          | 0.48     | 0.87           | 0.85      | 0.32        | 0.33   |
| 79       | 0.46          | 0.47     | 0.87           | 0.86      | 0.31        | 0.32   |
| 80       | 0.44          | 0.46     | 0.88           | 0.86      | 0.30        | 0.31   |
| 81       | 0.43          | 0.44     | 0.89           | 0.87      | 0.29        | 0.30   |
| 82       | 0.41          | 0.43     | 0.90           | 0.88      | 0.27        | 0.29   |
| 83       | 0.39          | 0.41     | 0.91           | 0.89      | 0.26        | 0.27   |
| 84       | 0.37          | 0.39     | 0.92           | 0.90      | 0.24        | 0.26   |
| 85       | 0.34          | 0.37     | 0.93           | 0.90      | 0.22        | 0.25   |
| 86       | 0.32          | 0.34     | 0.94           | 0.91      | 0.21        | 0.23   |
| 87       | 0.28          | 0.31     | 0.95           | 0.93      | 0.18        | 0.20   |
| 88       | 0.24          | 0.27     | 0.96           | 0.94      | 0.16        | 0.18   |
| 89       | 0.18          | 0.22     | 0.97           | 0.95      | 0.12        | 0.14   |
| 90       | 0.11          | 0.15     | 0.99           | 0.96      | 0.07        | 0.10   |

Table S129: Reference ( $\phi_S$ ,  $\varphi$ ,  $\psi$ ) and approached ( $\phi_S^\ell$ ,  $\varphi^\ell$ ,  $\psi^\ell$ ) values of the topological descriptors for the first excited-state of the pyridinium-phenolate (PP), computed at the PBE0/6-311+G(d,p) level of theory.  $\alpha$  is the pyridinium-phenolate central twist angle amplitude.

| $\alpha$ | $\phi_S^\ell$ | $\phi_S$ | $\varphi^\ell$ | $\varphi$ | $\psi^\ell$ | $\psi$ |
|----------|---------------|----------|----------------|-----------|-------------|--------|
| 0        | 0.41          | 0.32     | 0.83           | 0.86      | 0.29        | 0.23   |
| 1        | 0.41          | 0.32     | 0.83           | 0.86      | 0.29        | 0.23   |
| 2        | 0.41          | 0.32     | 0.83           | 0.86      | 0.29        | 0.23   |
| 3        | 0.41          | 0.32     | 0.84           | 0.86      | 0.29        | 0.23   |
| 4        | 0.41          | 0.32     | 0.84           | 0.86      | 0.29        | 0.23   |
| 5        | 0.41          | 0.32     | 0.84           | 0.86      | 0.29        | 0.23   |
| 6        | 0.41          | 0.32     | 0.84           | 0.86      | 0.29        | 0.23   |
| 7        | 0.40          | 0.33     | 0.84           | 0.86      | 0.28        | 0.23   |
| 8        | 0.40          | 0.33     | 0.84           | 0.86      | 0.28        | 0.23   |
| 9        | 0.40          | 0.33     | 0.85           | 0.86      | 0.28        | 0.23   |
| 10       | 0.40          | 0.33     | 0.85           | 0.86      | 0.28        | 0.23   |
| 11       | 0.40          | 0.34     | 0.85           | 0.86      | 0.28        | 0.24   |
| 12       | 0.39          | 0.34     | 0.85           | 0.86      | 0.27        | 0.24   |
| 13       | 0.39          | 0.34     | 0.85           | 0.86      | 0.27        | 0.24   |
| 14       | 0.39          | 0.34     | 0.85           | 0.86      | 0.27        | 0.24   |
| 15       | 0.38          | 0.35     | 0.86           | 0.86      | 0.26        | 0.25   |
| 16       | 0.38          | 0.35     | 0.86           | 0.86      | 0.26        | 0.25   |
| 17       | 0.38          | 0.35     | 0.86           | 0.86      | 0.26        | 0.25   |
| 18       | 0.37          | 0.35     | 0.86           | 0.86      | 0.26        | 0.25   |
| 19       | 0.37          | 0.36     | 0.86           | 0.86      | 0.26        | 0.25   |
| 20       | 0.37          | 0.36     | 0.86           | 0.86      | 0.26        | 0.25   |
| 21       | 0.36          | 0.36     | 0.87           | 0.86      | 0.25        | 0.25   |
| 22       | 0.36          | 0.36     | 0.87           | 0.86      | 0.25        | 0.25   |
| 23       | 0.35          | 0.36     | 0.87           | 0.86      | 0.24        | 0.25   |
| 24       | 0.35          | 0.37     | 0.87           | 0.86      | 0.24        | 0.26   |
| 25       | 0.35          | 0.37     | 0.87           | 0.86      | 0.24        | 0.26   |
| 26       | 0.34          | 0.37     | 0.87           | 0.86      | 0.24        | 0.26   |
| 27       | 0.34          | 0.37     | 0.87           | 0.86      | 0.24        | 0.26   |
| 28       | 0.34          | 0.38     | 0.87           | 0.86      | 0.24        | 0.26   |
| 29       | 0.34          | 0.38     | 0.87           | 0.85      | 0.24        | 0.27   |
| 30       | 0.33          | 0.38     | 0.87           | 0.85      | 0.23        | 0.27   |
| 31       | 0.33          | 0.39     | 0.86           | 0.85      | 0.23        | 0.27   |

Continued on next page

| $\alpha$ | $\phi_S^\ell$ | $\phi_S$ | $\varphi^\ell$ | $\varphi$ | $\psi^\ell$ | $\psi$ |
|----------|---------------|----------|----------------|-----------|-------------|--------|
| 32       | 0.33          | 0.39     | 0.86           | 0.85      | 0.23        | 0.27   |
| 33       | 0.33          | 0.39     | 0.86           | 0.85      | 0.23        | 0.27   |
| 34       | 0.33          | 0.40     | 0.85           | 0.85      | 0.24        | 0.28   |
| 35       | 0.33          | 0.40     | 0.85           | 0.85      | 0.24        | 0.28   |
| 36       | 0.34          | 0.41     | 0.84           | 0.85      | 0.24        | 0.29   |
| 37       | 0.34          | 0.41     | 0.84           | 0.84      | 0.24        | 0.29   |
| 38       | 0.35          | 0.42     | 0.83           | 0.84      | 0.25        | 0.30   |
| 39       | 0.35          | 0.43     | 0.83           | 0.84      | 0.25        | 0.30   |
| 40       | 0.36          | 0.44     | 0.83           | 0.83      | 0.26        | 0.31   |
| 41       | 0.38          | 0.45     | 0.82           | 0.83      | 0.28        | 0.32   |
| 42       | 0.39          | 0.47     | 0.82           | 0.82      | 0.28        | 0.33   |
| 43       | 0.42          | 0.48     | 0.81           | 0.81      | 0.30        | 0.34   |
| 44       | 0.44          | 0.50     | 0.81           | 0.80      | 0.32        | 0.36   |
| 45       | 0.47          | 0.52     | 0.80           | 0.79      | 0.34        | 0.37   |
| 46       | 0.50          | 0.54     | 0.79           | 0.78      | 0.36        | 0.39   |
| 47       | 0.53          | 0.57     | 0.77           | 0.77      | 0.38        | 0.41   |
| 48       | 0.56          | 0.59     | 0.76           | 0.75      | 0.40        | 0.42   |
| 49       | 0.58          | 0.60     | 0.76           | 0.75      | 0.41        | 0.43   |
| 50       | 0.60          | 0.61     | 0.75           | 0.74      | 0.43        | 0.44   |
| 51       | 0.61          | 0.62     | 0.75           | 0.74      | 0.43        | 0.44   |
| 52       | 0.62          | 0.63     | 0.75           | 0.74      | 0.44        | 0.45   |
| 53       | 0.62          | 0.63     | 0.75           | 0.74      | 0.44        | 0.45   |
| 54       | 0.62          | 0.63     | 0.75           | 0.74      | 0.44        | 0.45   |
| 55       | 0.62          | 0.63     | 0.75           | 0.74      | 0.44        | 0.45   |
| 56       | 0.62          | 0.63     | 0.76           | 0.74      | 0.44        | 0.45   |
| 57       | 0.62          | 0.62     | 0.76           | 0.75      | 0.44        | 0.44   |
| 58       | 0.61          | 0.62     | 0.76           | 0.75      | 0.43        | 0.44   |
| 59       | 0.61          | 0.62     | 0.77           | 0.75      | 0.43        | 0.44   |
| 60       | 0.61          | 0.61     | 0.77           | 0.76      | 0.43        | 0.43   |
| 61       | 0.60          | 0.61     | 0.77           | 0.76      | 0.42        | 0.43   |
| 62       | 0.60          | 0.60     | 0.78           | 0.77      | 0.42        | 0.42   |
| 63       | 0.59          | 0.60     | 0.78           | 0.77      | 0.41        | 0.42   |

Continued on next page

| $\alpha$ | $\phi_S^\ell$ | $\phi_S$ | $\varphi^\ell$ | $\varphi$ | $\psi^\ell$ | $\psi$ |
|----------|---------------|----------|----------------|-----------|-------------|--------|
| 64       | 0.58          | 0.59     | 0.79           | 0.77      | 0.40        | 0.42   |
| 65       | 0.58          | 0.59     | 0.79           | 0.78      | 0.40        | 0.41   |
| 66       | 0.57          | 0.58     | 0.80           | 0.78      | 0.39        | 0.41   |
| 67       | 0.57          | 0.58     | 0.80           | 0.79      | 0.39        | 0.40   |
| 68       | 0.56          | 0.57     | 0.81           | 0.79      | 0.39        | 0.40   |
| 69       | 0.55          | 0.56     | 0.81           | 0.80      | 0.38        | 0.39   |
| 70       | 0.54          | 0.55     | 0.82           | 0.80      | 0.37        | 0.38   |
| 71       | 0.54          | 0.55     | 0.83           | 0.81      | 0.37        | 0.38   |
| 72       | 0.53          | 0.54     | 0.83           | 0.81      | 0.36        | 0.37   |
| 73       | 0.52          | 0.53     | 0.84           | 0.82      | 0.35        | 0.37   |
| 74       | 0.51          | 0.52     | 0.84           | 0.83      | 0.35        | 0.36   |
| 75       | 0.50          | 0.51     | 0.85           | 0.83      | 0.34        | 0.35   |
| 76       | 0.49          | 0.50     | 0.86           | 0.84      | 0.33        | 0.34   |
| 77       | 0.48          | 0.49     | 0.86           | 0.84      | 0.32        | 0.34   |
| 78       | 0.47          | 0.48     | 0.87           | 0.85      | 0.32        | 0.33   |
| 79       | 0.45          | 0.47     | 0.88           | 0.86      | 0.30        | 0.32   |
| 80       | 0.44          | 0.45     | 0.88           | 0.87      | 0.30        | 0.30   |
| 81       | 0.42          | 0.44     | 0.89           | 0.87      | 0.28        | 0.30   |
| 82       | 0.41          | 0.42     | 0.90           | 0.88      | 0.27        | 0.28   |
| 83       | 0.39          | 0.41     | 0.91           | 0.89      | 0.26        | 0.27   |
| 84       | 0.37          | 0.39     | 0.92           | 0.90      | 0.24        | 0.26   |
| 85       | 0.34          | 0.36     | 0.93           | 0.91      | 0.22        | 0.24   |
| 86       | 0.31          | 0.34     | 0.94           | 0.92      | 0.20        | 0.23   |
| 87       | 0.28          | 0.31     | 0.95           | 0.93      | 0.18        | 0.20   |
| 88       | 0.23          | 0.27     | 0.96           | 0.94      | 0.15        | 0.18   |
| 89       | 0.17          | 0.21     | 0.98           | 0.95      | 0.11        | 0.14   |
| 90       | 0.11          | 0.15     | 0.99           | 0.96      | 0.07        | 0.10   |

Table S130: Reference ( $\phi_S$ ,  $\varphi$ ,  $\psi$ ) and approached ( $\phi_S^\ell$ ,  $\varphi^\ell$ ,  $\psi^\ell$ ) values of the topological descriptors for the first excited-state of the pyridinium-phenolate (PP), computed at the PBE0/6-311+G(d) level of theory.  $\alpha$  is the pyridinium-phenolate central twist angle amplitude.

| $\alpha$ | $\phi_S^\ell$ | $\phi_S$ | $\varphi^\ell$ | $\varphi$ | $\psi^\ell$ | $\psi$ |
|----------|---------------|----------|----------------|-----------|-------------|--------|
| 0        | 0.42          | 0.32     | 0.83           | 0.86      | 0.30        | 0.23   |
| 1        | 0.42          | 0.32     | 0.83           | 0.86      | 0.30        | 0.23   |
| 2        | 0.42          | 0.32     | 0.83           | 0.86      | 0.30        | 0.23   |
| 3        | 0.42          | 0.32     | 0.83           | 0.86      | 0.30        | 0.23   |
| 4        | 0.42          | 0.32     | 0.83           | 0.86      | 0.30        | 0.23   |
| 5        | 0.41          | 0.32     | 0.83           | 0.86      | 0.29        | 0.23   |
| 6        | 0.41          | 0.32     | 0.83           | 0.86      | 0.29        | 0.23   |
| 7        | 0.41          | 0.33     | 0.83           | 0.86      | 0.29        | 0.23   |
| 8        | 0.41          | 0.33     | 0.84           | 0.86      | 0.29        | 0.23   |
| 9        | 0.40          | 0.33     | 0.84           | 0.86      | 0.28        | 0.23   |
| 10       | 0.40          | 0.33     | 0.84           | 0.86      | 0.28        | 0.23   |
| 11       | 0.39          | 0.33     | 0.84           | 0.86      | 0.28        | 0.23   |
| 12       | 0.39          | 0.33     | 0.84           | 0.86      | 0.28        | 0.23   |
| 13       | 0.39          | 0.33     | 0.85           | 0.86      | 0.27        | 0.23   |
| 14       | 0.38          | 0.33     | 0.85           | 0.86      | 0.27        | 0.23   |
| 15       | 0.37          | 0.33     | 0.85           | 0.86      | 0.26        | 0.23   |
| 16       | 0.37          | 0.33     | 0.85           | 0.86      | 0.26        | 0.23   |
| 17       | 0.36          | 0.33     | 0.86           | 0.86      | 0.25        | 0.23   |
| 18       | 0.36          | 0.34     | 0.86           | 0.86      | 0.25        | 0.24   |
| 19       | 0.35          | 0.34     | 0.86           | 0.86      | 0.25        | 0.24   |
| 20       | 0.34          | 0.34     | 0.86           | 0.86      | 0.24        | 0.24   |
| 21       | 0.34          | 0.34     | 0.86           | 0.86      | 0.24        | 0.24   |
| 22       | 0.33          | 0.34     | 0.87           | 0.86      | 0.23        | 0.24   |
| 23       | 0.32          | 0.34     | 0.87           | 0.86      | 0.22        | 0.24   |
| 24       | 0.31          | 0.34     | 0.87           | 0.86      | 0.22        | 0.24   |
| 25       | 0.31          | 0.34     | 0.87           | 0.86      | 0.22        | 0.24   |
| 26       | 0.30          | 0.34     | 0.87           | 0.86      | 0.21        | 0.24   |
| 27       | 0.29          | 0.34     | 0.87           | 0.86      | 0.20        | 0.24   |
| 28       | 0.28          | 0.34     | 0.88           | 0.86      | 0.20        | 0.24   |
| 29       | 0.28          | 0.34     | 0.88           | 0.86      | 0.20        | 0.24   |
| 30       | 0.27          | 0.34     | 0.88           | 0.87      | 0.19        | 0.24   |
| 31       | 0.26          | 0.34     | 0.89           | 0.87      | 0.18        | 0.24   |

Continued on next page



| $\alpha$ | $\phi_S^\ell$ | $\phi_S$ | $\varphi^\ell$ | $\varphi$ | $\psi^\ell$ | $\psi$ |
|----------|---------------|----------|----------------|-----------|-------------|--------|
| 32       | 0.26          | 0.34     | 0.89           | 0.87      | 0.18        | 0.24   |
| 33       | 0.25          | 0.34     | 0.90           | 0.87      | 0.17        | 0.24   |
| 34       | 0.24          | 0.34     | 0.91           | 0.87      | 0.16        | 0.24   |
| 35       | 0.23          | 0.34     | 0.91           | 0.87      | 0.16        | 0.24   |
| 36       | 0.23          | 0.34     | 0.92           | 0.87      | 0.16        | 0.24   |
| 37       | 0.22          | 0.34     | 0.92           | 0.87      | 0.15        | 0.24   |
| 38       | 0.21          | 0.34     | 0.93           | 0.87      | 0.14        | 0.24   |
| 39       | 0.21          | 0.34     | 0.93           | 0.87      | 0.14        | 0.24   |
| 40       | 0.20          | 0.34     | 0.93           | 0.87      | 0.13        | 0.24   |
| 41       | 0.20          | 0.34     | 0.93           | 0.87      | 0.13        | 0.24   |
| 42       | 0.19          | 0.34     | 0.94           | 0.87      | 0.13        | 0.24   |
| 43       | 0.19          | 0.34     | 0.94           | 0.87      | 0.13        | 0.24   |
| 44       | 0.19          | 0.35     | 0.93           | 0.87      | 0.13        | 0.24   |
| 45       | 0.19          | 0.35     | 0.93           | 0.87      | 0.13        | 0.24   |
| 46       | 0.20          | 0.35     | 0.93           | 0.87      | 0.13        | 0.24   |
| 47       | 0.21          | 0.36     | 0.93           | 0.87      | 0.14        | 0.25   |
| 48       | 0.22          | 0.36     | 0.92           | 0.87      | 0.15        | 0.25   |
| 49       | 0.23          | 0.37     | 0.91           | 0.87      | 0.16        | 0.26   |
| 50       | 0.25          | 0.38     | 0.91           | 0.86      | 0.17        | 0.26   |
| 51       | 0.28          | 0.39     | 0.90           | 0.86      | 0.19        | 0.27   |
| 52       | 0.31          | 0.41     | 0.89           | 0.85      | 0.21        | 0.29   |
| 53       | 0.35          | 0.44     | 0.87           | 0.84      | 0.24        | 0.31   |
| 54       | 0.41          | 0.47     | 0.84           | 0.82      | 0.29        | 0.33   |
| 55       | 0.48          | 0.52     | 0.80           | 0.80      | 0.34        | 0.37   |
| 56       | 0.54          | 0.56     | 0.78           | 0.77      | 0.39        | 0.40   |
| 57       | 0.59          | 0.60     | 0.77           | 0.76      | 0.42        | 0.43   |
| 58       | 0.61          | 0.62     | 0.76           | 0.75      | 0.43        | 0.44   |
| 59       | 0.62          | 0.62     | 0.76           | 0.75      | 0.44        | 0.44   |
| 60       | 0.62          | 0.62     | 0.76           | 0.75      | 0.44        | 0.44   |
| 61       | 0.62          | 0.62     | 0.76           | 0.75      | 0.44        | 0.44   |
| 62       | 0.61          | 0.62     | 0.77           | 0.75      | 0.43        | 0.44   |
| 63       | 0.61          | 0.61     | 0.77           | 0.76      | 0.43        | 0.43   |

Continued on next page

| $\alpha$ | $\phi_S^\ell$ | $\phi_S$ | $\varphi^\ell$ | $\varphi$ | $\psi^\ell$ | $\psi$ |
|----------|---------------|----------|----------------|-----------|-------------|--------|
| 64       | 0.61          | 0.61     | 0.78           | 0.76      | 0.42        | 0.43   |
| 65       | 0.60          | 0.60     | 0.78           | 0.77      | 0.42        | 0.42   |
| 66       | 0.59          | 0.60     | 0.78           | 0.77      | 0.41        | 0.42   |
| 67       | 0.59          | 0.59     | 0.79           | 0.78      | 0.41        | 0.41   |
| 68       | 0.58          | 0.59     | 0.80           | 0.78      | 0.40        | 0.41   |
| 69       | 0.57          | 0.58     | 0.80           | 0.79      | 0.39        | 0.40   |
| 70       | 0.57          | 0.57     | 0.81           | 0.79      | 0.39        | 0.40   |
| 71       | 0.56          | 0.57     | 0.81           | 0.80      | 0.39        | 0.39   |
| 72       | 0.55          | 0.56     | 0.82           | 0.80      | 0.38        | 0.39   |
| 73       | 0.54          | 0.55     | 0.82           | 0.81      | 0.37        | 0.38   |
| 74       | 0.53          | 0.54     | 0.83           | 0.81      | 0.36        | 0.37   |
| 75       | 0.53          | 0.53     | 0.84           | 0.82      | 0.36        | 0.37   |
| 76       | 0.52          | 0.52     | 0.84           | 0.82      | 0.35        | 0.36   |
| 77       | 0.51          | 0.51     | 0.85           | 0.83      | 0.34        | 0.35   |
| 78       | 0.49          | 0.50     | 0.85           | 0.84      | 0.33        | 0.34   |
| 79       | 0.48          | 0.49     | 0.86           | 0.84      | 0.32        | 0.34   |
| 80       | 0.47          | 0.48     | 0.87           | 0.85      | 0.32        | 0.33   |
| 81       | 0.45          | 0.47     | 0.88           | 0.86      | 0.30        | 0.32   |
| 82       | 0.44          | 0.45     | 0.88           | 0.87      | 0.30        | 0.30   |
| 83       | 0.42          | 0.44     | 0.89           | 0.87      | 0.28        | 0.30   |
| 84       | 0.40          | 0.42     | 0.90           | 0.88      | 0.27        | 0.28   |
| 85       | 0.38          | 0.40     | 0.91           | 0.89      | 0.25        | 0.27   |
| 86       | 0.35          | 0.38     | 0.92           | 0.90      | 0.23        | 0.25   |
| 87       | 0.32          | 0.35     | 0.93           | 0.91      | 0.21        | 0.23   |
| 88       | 0.28          | 0.31     | 0.95           | 0.92      | 0.18        | 0.21   |
| 89       | 0.23          | 0.26     | 0.96           | 0.94      | 0.15        | 0.17   |
| 90       | 0.10          | 0.15     | 0.99           | 0.96      | 0.06        | 0.10   |

Table S131: Reference ( $\phi_S$ ,  $\varphi$ ,  $\psi$ ) and approached ( $\phi_S^\ell$ ,  $\varphi^\ell$ ,  $\psi^\ell$ ) values of the topological descriptors for the first excited-state of the pyridinium-phenolate (PP), computed at the PBE0/6-311G(d) level of theory.  $\alpha$  is the pyridinium-phenolate central twist angle amplitude.

| $\alpha$ | $\phi_S^\ell$ | $\phi_S$ | $\varphi^\ell$ | $\varphi$ | $\psi^\ell$ | $\psi$ |
|----------|---------------|----------|----------------|-----------|-------------|--------|
| 0        | 0.42          | 0.32     | 0.83           | 0.86      | 0.30        | 0.23   |
| 1        | 0.42          | 0.32     | 0.83           | 0.86      | 0.30        | 0.23   |
| 2        | 0.41          | 0.32     | 0.83           | 0.86      | 0.29        | 0.23   |
| 3        | 0.41          | 0.32     | 0.83           | 0.86      | 0.29        | 0.23   |
| 4        | 0.41          | 0.32     | 0.83           | 0.86      | 0.29        | 0.23   |
| 5        | 0.41          | 0.32     | 0.83           | 0.86      | 0.29        | 0.23   |
| 6        | 0.41          | 0.33     | 0.83           | 0.86      | 0.29        | 0.23   |
| 7        | 0.41          | 0.33     | 0.84           | 0.86      | 0.29        | 0.23   |
| 8        | 0.40          | 0.33     | 0.84           | 0.86      | 0.28        | 0.23   |
| 9        | 0.40          | 0.33     | 0.84           | 0.86      | 0.28        | 0.23   |
| 10       | 0.40          | 0.33     | 0.84           | 0.86      | 0.28        | 0.23   |
| 11       | 0.40          | 0.34     | 0.85           | 0.86      | 0.28        | 0.24   |
| 12       | 0.39          | 0.34     | 0.85           | 0.86      | 0.27        | 0.24   |
| 13       | 0.39          | 0.34     | 0.85           | 0.86      | 0.27        | 0.24   |
| 14       | 0.39          | 0.34     | 0.85           | 0.86      | 0.27        | 0.24   |
| 15       | 0.38          | 0.34     | 0.85           | 0.86      | 0.27        | 0.24   |
| 16       | 0.38          | 0.35     | 0.86           | 0.86      | 0.26        | 0.25   |
| 17       | 0.38          | 0.35     | 0.86           | 0.86      | 0.26        | 0.25   |
| 18       | 0.37          | 0.35     | 0.86           | 0.86      | 0.26        | 0.25   |
| 19       | 0.37          | 0.35     | 0.86           | 0.86      | 0.26        | 0.25   |
| 20       | 0.36          | 0.35     | 0.86           | 0.86      | 0.25        | 0.25   |
| 21       | 0.36          | 0.36     | 0.86           | 0.86      | 0.25        | 0.25   |
| 22       | 0.35          | 0.36     | 0.86           | 0.86      | 0.25        | 0.25   |
| 23       | 0.35          | 0.36     | 0.87           | 0.86      | 0.24        | 0.25   |
| 24       | 0.34          | 0.36     | 0.87           | 0.86      | 0.24        | 0.25   |
| 25       | 0.34          | 0.36     | 0.87           | 0.86      | 0.24        | 0.25   |
| 26       | 0.34          | 0.36     | 0.87           | 0.86      | 0.24        | 0.25   |
| 27       | 0.33          | 0.37     | 0.87           | 0.86      | 0.23        | 0.26   |
| 28       | 0.33          | 0.37     | 0.87           | 0.86      | 0.23        | 0.26   |
| 29       | 0.33          | 0.37     | 0.87           | 0.86      | 0.23        | 0.26   |
| 30       | 0.32          | 0.37     | 0.87           | 0.86      | 0.22        | 0.26   |
| 31       | 0.32          | 0.38     | 0.87           | 0.86      | 0.22        | 0.26   |

Continued on next page

| $\alpha$ | $\phi_S^\ell$ | $\phi_S$ | $\varphi^\ell$ | $\varphi$ | $\psi^\ell$ | $\psi$ |
|----------|---------------|----------|----------------|-----------|-------------|--------|
| 32       | 0.32          | 0.38     | 0.86           | 0.86      | 0.23        | 0.26   |
| 33       | 0.32          | 0.38     | 0.86           | 0.86      | 0.23        | 0.26   |
| 34       | 0.32          | 0.38     | 0.86           | 0.86      | 0.23        | 0.26   |
| 35       | 0.32          | 0.39     | 0.86           | 0.85      | 0.23        | 0.27   |
| 36       | 0.32          | 0.39     | 0.85           | 0.85      | 0.23        | 0.27   |
| 37       | 0.32          | 0.40     | 0.85           | 0.85      | 0.23        | 0.28   |
| 38       | 0.32          | 0.40     | 0.85           | 0.85      | 0.23        | 0.28   |
| 39       | 0.32          | 0.41     | 0.84           | 0.85      | 0.23        | 0.29   |
| 40       | 0.33          | 0.41     | 0.84           | 0.85      | 0.24        | 0.29   |
| 41       | 0.33          | 0.42     | 0.84           | 0.84      | 0.24        | 0.30   |
| 42       | 0.34          | 0.43     | 0.83           | 0.84      | 0.25        | 0.30   |
| 43       | 0.36          | 0.44     | 0.83           | 0.83      | 0.26        | 0.31   |
| 44       | 0.37          | 0.45     | 0.82           | 0.83      | 0.27        | 0.32   |
| 45       | 0.39          | 0.47     | 0.82           | 0.82      | 0.28        | 0.33   |
| 46       | 0.41          | 0.48     | 0.81           | 0.81      | 0.30        | 0.34   |
| 47       | 0.44          | 0.50     | 0.81           | 0.81      | 0.32        | 0.35   |
| 48       | 0.47          | 0.52     | 0.80           | 0.80      | 0.34        | 0.37   |
| 49       | 0.50          | 0.54     | 0.79           | 0.78      | 0.36        | 0.39   |
| 50       | 0.53          | 0.56     | 0.78           | 0.77      | 0.38        | 0.40   |
| 51       | 0.55          | 0.57     | 0.77           | 0.76      | 0.39        | 0.41   |
| 52       | 0.57          | 0.59     | 0.77           | 0.76      | 0.41        | 0.42   |
| 53       | 0.59          | 0.60     | 0.76           | 0.75      | 0.42        | 0.43   |
| 54       | 0.60          | 0.61     | 0.76           | 0.75      | 0.43        | 0.43   |
| 55       | 0.61          | 0.61     | 0.76           | 0.75      | 0.43        | 0.43   |
| 56       | 0.61          | 0.62     | 0.76           | 0.75      | 0.43        | 0.44   |
| 57       | 0.61          | 0.62     | 0.76           | 0.75      | 0.43        | 0.44   |
| 58       | 0.61          | 0.62     | 0.76           | 0.75      | 0.43        | 0.44   |
| 59       | 0.61          | 0.61     | 0.76           | 0.75      | 0.43        | 0.43   |
| 60       | 0.61          | 0.61     | 0.77           | 0.76      | 0.43        | 0.43   |
| 61       | 0.60          | 0.61     | 0.77           | 0.76      | 0.42        | 0.43   |
| 62       | 0.60          | 0.60     | 0.78           | 0.76      | 0.42        | 0.43   |
| 63       | 0.60          | 0.60     | 0.78           | 0.77      | 0.42        | 0.42   |

Continued on next page

| $\alpha$ | $\phi_S^\ell$ | $\phi_S$ | $\varphi^\ell$ | $\varphi$ | $\psi^\ell$ | $\psi$ |
|----------|---------------|----------|----------------|-----------|-------------|--------|
| 64       | 0.59          | 0.60     | 0.78           | 0.77      | 0.41        | 0.42   |
| 65       | 0.59          | 0.59     | 0.79           | 0.78      | 0.41        | 0.41   |
| 66       | 0.58          | 0.59     | 0.79           | 0.78      | 0.40        | 0.41   |
| 67       | 0.57          | 0.58     | 0.80           | 0.79      | 0.39        | 0.40   |
| 68       | 0.57          | 0.57     | 0.80           | 0.79      | 0.39        | 0.40   |
| 69       | 0.56          | 0.57     | 0.81           | 0.80      | 0.39        | 0.39   |
| 70       | 0.55          | 0.56     | 0.82           | 0.80      | 0.38        | 0.39   |
| 71       | 0.55          | 0.55     | 0.82           | 0.81      | 0.38        | 0.38   |
| 72       | 0.54          | 0.55     | 0.83           | 0.81      | 0.37        | 0.38   |
| 73       | 0.53          | 0.54     | 0.83           | 0.82      | 0.36        | 0.37   |
| 74       | 0.52          | 0.53     | 0.84           | 0.82      | 0.35        | 0.37   |
| 75       | 0.51          | 0.52     | 0.84           | 0.83      | 0.35        | 0.36   |
| 76       | 0.50          | 0.51     | 0.85           | 0.83      | 0.34        | 0.35   |
| 77       | 0.49          | 0.50     | 0.86           | 0.84      | 0.33        | 0.34   |
| 78       | 0.48          | 0.49     | 0.86           | 0.85      | 0.32        | 0.33   |
| 79       | 0.47          | 0.48     | 0.87           | 0.85      | 0.32        | 0.33   |
| 80       | 0.45          | 0.46     | 0.88           | 0.86      | 0.30        | 0.31   |
| 81       | 0.44          | 0.45     | 0.89           | 0.87      | 0.29        | 0.30   |
| 82       | 0.42          | 0.44     | 0.90           | 0.88      | 0.28        | 0.30   |
| 83       | 0.40          | 0.42     | 0.90           | 0.88      | 0.27        | 0.28   |
| 84       | 0.38          | 0.40     | 0.91           | 0.89      | 0.25        | 0.27   |
| 85       | 0.36          | 0.38     | 0.92           | 0.90      | 0.24        | 0.25   |
| 86       | 0.33          | 0.36     | 0.93           | 0.91      | 0.22        | 0.24   |
| 87       | 0.30          | 0.33     | 0.95           | 0.92      | 0.19        | 0.22   |
| 88       | 0.26          | 0.29     | 0.96           | 0.93      | 0.17        | 0.19   |
| 89       | 0.19          | 0.23     | 0.97           | 0.95      | 0.12        | 0.15   |
| 90       | 0.09          | 0.14     | 0.99           | 0.97      | 0.06        | 0.09   |

Table S132: Reference ( $\phi_S$ ,  $\varphi$ ,  $\psi$ ) and approached ( $\phi_S^\ell$ ,  $\varphi^\ell$ ,  $\psi^\ell$ ) values of the topological descriptors for the first excited-state of the pyridinium-phenolate (PP), computed at the PBE0/6-311+G level of theory.  $\alpha$  is the pyridinium-phenolate central twist angle amplitude.

| $\alpha$ | $\phi_S^\ell$ | $\phi_S$ | $\varphi^\ell$ | $\varphi$ | $\psi^\ell$ | $\psi$ |
|----------|---------------|----------|----------------|-----------|-------------|--------|
| 0        | 0.42          | 0.32     | 0.83           | 0.86      | 0.30        | 0.23   |
| 1        | 0.42          | 0.32     | 0.83           | 0.86      | 0.30        | 0.23   |
| 2        | 0.42          | 0.32     | 0.83           | 0.86      | 0.30        | 0.23   |
| 3        | 0.42          | 0.32     | 0.83           | 0.86      | 0.30        | 0.23   |
| 4        | 0.42          | 0.32     | 0.83           | 0.86      | 0.30        | 0.23   |
| 5        | 0.42          | 0.32     | 0.83           | 0.86      | 0.30        | 0.23   |
| 6        | 0.42          | 0.33     | 0.83           | 0.86      | 0.30        | 0.23   |
| 7        | 0.41          | 0.33     | 0.83           | 0.86      | 0.29        | 0.23   |
| 8        | 0.41          | 0.33     | 0.83           | 0.86      | 0.29        | 0.23   |
| 9        | 0.41          | 0.33     | 0.83           | 0.86      | 0.29        | 0.23   |
| 10       | 0.40          | 0.33     | 0.84           | 0.86      | 0.28        | 0.23   |
| 11       | 0.40          | 0.33     | 0.84           | 0.86      | 0.28        | 0.23   |
| 12       | 0.39          | 0.33     | 0.84           | 0.86      | 0.28        | 0.23   |
| 13       | 0.39          | 0.33     | 0.84           | 0.86      | 0.28        | 0.23   |
| 14       | 0.38          | 0.33     | 0.84           | 0.86      | 0.27        | 0.23   |
| 15       | 0.38          | 0.33     | 0.85           | 0.86      | 0.27        | 0.23   |
| 16       | 0.37          | 0.33     | 0.85           | 0.86      | 0.26        | 0.23   |
| 17       | 0.37          | 0.34     | 0.85           | 0.86      | 0.26        | 0.24   |
| 18       | 0.36          | 0.34     | 0.85           | 0.86      | 0.26        | 0.24   |
| 19       | 0.35          | 0.34     | 0.85           | 0.86      | 0.25        | 0.24   |
| 20       | 0.35          | 0.34     | 0.86           | 0.86      | 0.25        | 0.24   |
| 21       | 0.34          | 0.34     | 0.86           | 0.86      | 0.24        | 0.24   |
| 22       | 0.33          | 0.34     | 0.86           | 0.86      | 0.23        | 0.24   |
| 23       | 0.33          | 0.34     | 0.86           | 0.86      | 0.23        | 0.24   |
| 24       | 0.32          | 0.34     | 0.87           | 0.86      | 0.22        | 0.24   |
| 25       | 0.31          | 0.34     | 0.87           | 0.86      | 0.22        | 0.24   |
| 26       | 0.30          | 0.34     | 0.87           | 0.86      | 0.21        | 0.24   |
| 27       | 0.30          | 0.34     | 0.87           | 0.86      | 0.21        | 0.24   |
| 28       | 0.29          | 0.34     | 0.87           | 0.86      | 0.20        | 0.24   |
| 29       | 0.28          | 0.34     | 0.87           | 0.86      | 0.20        | 0.24   |
| 30       | 0.28          | 0.34     | 0.88           | 0.86      | 0.20        | 0.24   |
| 31       | 0.27          | 0.34     | 0.89           | 0.87      | 0.19        | 0.24   |

Continued on next page

| $\alpha$ | $\phi_S^\ell$ | $\phi_S$ | $\varphi^\ell$ | $\varphi$ | $\psi^\ell$ | $\psi$ |
|----------|---------------|----------|----------------|-----------|-------------|--------|
| 32       | 0.26          | 0.34     | 0.89           | 0.87      | 0.18        | 0.24   |
| 33       | 0.26          | 0.34     | 0.89           | 0.87      | 0.18        | 0.24   |
| 34       | 0.25          | 0.34     | 0.90           | 0.87      | 0.17        | 0.24   |
| 35       | 0.24          | 0.35     | 0.91           | 0.87      | 0.16        | 0.24   |
| 36       | 0.24          | 0.35     | 0.91           | 0.87      | 0.16        | 0.24   |
| 37       | 0.23          | 0.35     | 0.91           | 0.87      | 0.16        | 0.24   |
| 38       | 0.23          | 0.35     | 0.92           | 0.87      | 0.16        | 0.24   |
| 39       | 0.22          | 0.35     | 0.92           | 0.87      | 0.15        | 0.24   |
| 40       | 0.22          | 0.35     | 0.92           | 0.87      | 0.15        | 0.24   |
| 41       | 0.21          | 0.35     | 0.92           | 0.87      | 0.14        | 0.24   |
| 42       | 0.21          | 0.35     | 0.93           | 0.87      | 0.14        | 0.24   |
| 43       | 0.21          | 0.35     | 0.93           | 0.87      | 0.14        | 0.24   |
| 44       | 0.21          | 0.35     | 0.92           | 0.87      | 0.14        | 0.24   |
| 45       | 0.21          | 0.36     | 0.92           | 0.87      | 0.14        | 0.25   |
| 46       | 0.21          | 0.36     | 0.92           | 0.87      | 0.14        | 0.25   |
| 47       | 0.22          | 0.37     | 0.91           | 0.87      | 0.15        | 0.26   |
| 48       | 0.24          | 0.37     | 0.91           | 0.87      | 0.16        | 0.26   |
| 49       | 0.25          | 0.38     | 0.91           | 0.86      | 0.17        | 0.26   |
| 50       | 0.27          | 0.39     | 0.90           | 0.86      | 0.19        | 0.27   |
| 51       | 0.29          | 0.40     | 0.90           | 0.86      | 0.20        | 0.28   |
| 52       | 0.32          | 0.41     | 0.89           | 0.85      | 0.22        | 0.29   |
| 53       | 0.35          | 0.43     | 0.87           | 0.84      | 0.24        | 0.30   |
| 54       | 0.39          | 0.45     | 0.85           | 0.83      | 0.27        | 0.32   |
| 55       | 0.43          | 0.48     | 0.83           | 0.82      | 0.30        | 0.34   |
| 56       | 0.48          | 0.51     | 0.80           | 0.80      | 0.34        | 0.36   |
| 57       | 0.52          | 0.55     | 0.79           | 0.79      | 0.37        | 0.39   |
| 58       | 0.56          | 0.57     | 0.78           | 0.77      | 0.40        | 0.41   |
| 59       | 0.59          | 0.59     | 0.77           | 0.76      | 0.42        | 0.42   |
| 60       | 0.60          | 0.60     | 0.77           | 0.76      | 0.42        | 0.43   |
| 61       | 0.61          | 0.61     | 0.76           | 0.76      | 0.43        | 0.43   |
| 62       | 0.61          | 0.61     | 0.77           | 0.76      | 0.43        | 0.43   |
| 63       | 0.61          | 0.61     | 0.77           | 0.76      | 0.43        | 0.43   |

Continued on next page

| $\alpha$ | $\phi_S^\ell$ | $\phi_S$ | $\varphi^\ell$ | $\varphi$ | $\psi^\ell$ | $\psi$ |
|----------|---------------|----------|----------------|-----------|-------------|--------|
| 64       | 0.61          | 0.61     | 0.77           | 0.76      | 0.43        | 0.43   |
| 65       | 0.60          | 0.60     | 0.78           | 0.77      | 0.42        | 0.42   |
| 66       | 0.60          | 0.60     | 0.78           | 0.77      | 0.42        | 0.42   |
| 67       | 0.59          | 0.60     | 0.79           | 0.77      | 0.41        | 0.42   |
| 68       | 0.59          | 0.59     | 0.79           | 0.78      | 0.41        | 0.41   |
| 69       | 0.58          | 0.58     | 0.80           | 0.78      | 0.40        | 0.41   |
| 70       | 0.58          | 0.58     | 0.80           | 0.79      | 0.40        | 0.40   |
| 71       | 0.57          | 0.57     | 0.81           | 0.79      | 0.39        | 0.40   |
| 72       | 0.56          | 0.56     | 0.81           | 0.80      | 0.39        | 0.39   |
| 73       | 0.55          | 0.56     | 0.82           | 0.80      | 0.38        | 0.39   |
| 74       | 0.54          | 0.55     | 0.83           | 0.81      | 0.37        | 0.38   |
| 75       | 0.54          | 0.54     | 0.83           | 0.82      | 0.37        | 0.37   |
| 76       | 0.53          | 0.53     | 0.84           | 0.82      | 0.36        | 0.37   |
| 77       | 0.52          | 0.52     | 0.84           | 0.83      | 0.35        | 0.36   |
| 78       | 0.51          | 0.51     | 0.85           | 0.83      | 0.34        | 0.35   |
| 79       | 0.49          | 0.50     | 0.86           | 0.84      | 0.33        | 0.34   |
| 80       | 0.48          | 0.49     | 0.87           | 0.85      | 0.32        | 0.33   |
| 81       | 0.47          | 0.48     | 0.87           | 0.85      | 0.32        | 0.33   |
| 82       | 0.45          | 0.46     | 0.88           | 0.86      | 0.30        | 0.31   |
| 83       | 0.44          | 0.45     | 0.89           | 0.87      | 0.29        | 0.30   |
| 84       | 0.42          | 0.43     | 0.90           | 0.88      | 0.28        | 0.29   |
| 85       | 0.40          | 0.41     | 0.91           | 0.89      | 0.26        | 0.27   |
| 86       | 0.37          | 0.39     | 0.92           | 0.90      | 0.24        | 0.26   |
| 87       | 0.34          | 0.37     | 0.93           | 0.91      | 0.22        | 0.25   |
| 88       | 0.31          | 0.33     | 0.94           | 0.92      | 0.20        | 0.22   |
| 89       | 0.26          | 0.29     | 0.96           | 0.93      | 0.17        | 0.19   |
| 90       | 0.08          | 0.14     | 0.99           | 0.97      | 0.05        | 0.09   |

Table S133: Reference ( $\phi_S$ ,  $\varphi$ ,  $\psi$ ) and approached ( $\phi_S^\ell$ ,  $\varphi^\ell$ ,  $\psi^\ell$ ) values of the topological descriptors for the first excited-state of the pyridinium-phenolate (PP), computed at the PBE0/6-311G level of theory.  $\alpha$  is the pyridinium-phenolate central twist angle amplitude.



| $\alpha$ | $\phi_S^\ell$ | $\phi_S$ | $\varphi^\ell$ | $\varphi$ | $\psi^\ell$ | $\psi$ |
|----------|---------------|----------|----------------|-----------|-------------|--------|
| 0        | 0.42          | 0.32     | 0.83           | 0.86      | 0.30        | 0.23   |
| 1        | 0.42          | 0.32     | 0.83           | 0.86      | 0.30        | 0.23   |
| 2        | 0.42          | 0.32     | 0.83           | 0.86      | 0.30        | 0.23   |
| 3        | 0.42          | 0.32     | 0.83           | 0.86      | 0.30        | 0.23   |
| 4        | 0.42          | 0.32     | 0.83           | 0.86      | 0.30        | 0.23   |
| 5        | 0.41          | 0.32     | 0.84           | 0.86      | 0.29        | 0.23   |
| 6        | 0.41          | 0.33     | 0.84           | 0.86      | 0.29        | 0.23   |
| 7        | 0.41          | 0.33     | 0.84           | 0.86      | 0.29        | 0.23   |
| 8        | 0.41          | 0.33     | 0.84           | 0.86      | 0.29        | 0.23   |
| 9        | 0.41          | 0.33     | 0.84           | 0.86      | 0.29        | 0.23   |
| 10       | 0.41          | 0.34     | 0.84           | 0.86      | 0.29        | 0.24   |
| 11       | 0.40          | 0.34     | 0.85           | 0.86      | 0.28        | 0.24   |
| 12       | 0.40          | 0.34     | 0.85           | 0.86      | 0.28        | 0.24   |
| 13       | 0.40          | 0.34     | 0.85           | 0.86      | 0.28        | 0.24   |
| 14       | 0.40          | 0.35     | 0.85           | 0.86      | 0.28        | 0.25   |
| 15       | 0.39          | 0.35     | 0.85           | 0.86      | 0.27        | 0.25   |
| 16       | 0.39          | 0.35     | 0.85           | 0.86      | 0.27        | 0.25   |
| 17       | 0.38          | 0.35     | 0.86           | 0.86      | 0.26        | 0.25   |
| 18       | 0.38          | 0.35     | 0.86           | 0.86      | 0.26        | 0.25   |
| 19       | 0.38          | 0.36     | 0.86           | 0.86      | 0.26        | 0.25   |
| 20       | 0.37          | 0.36     | 0.86           | 0.86      | 0.26        | 0.25   |
| 21       | 0.37          | 0.36     | 0.86           | 0.86      | 0.26        | 0.25   |
| 22       | 0.37          | 0.36     | 0.86           | 0.86      | 0.26        | 0.25   |
| 23       | 0.36          | 0.37     | 0.86           | 0.86      | 0.25        | 0.26   |
| 24       | 0.36          | 0.37     | 0.87           | 0.86      | 0.25        | 0.26   |
| 25       | 0.35          | 0.37     | 0.87           | 0.86      | 0.24        | 0.26   |
| 26       | 0.35          | 0.37     | 0.87           | 0.86      | 0.24        | 0.26   |
| 27       | 0.35          | 0.37     | 0.87           | 0.86      | 0.24        | 0.26   |
| 28       | 0.34          | 0.38     | 0.87           | 0.86      | 0.24        | 0.26   |
| 29       | 0.34          | 0.38     | 0.86           | 0.85      | 0.24        | 0.27   |
| 30       | 0.34          | 0.38     | 0.86           | 0.85      | 0.24        | 0.27   |
| 31       | 0.34          | 0.39     | 0.86           | 0.85      | 0.24        | 0.27   |

Continued on next page

| $\alpha$ | $\phi_S^\ell$ | $\phi_S$ | $\varphi^\ell$ | $\varphi$ | $\psi^\ell$ | $\psi$ |
|----------|---------------|----------|----------------|-----------|-------------|--------|
| 32       | 0.34          | 0.39     | 0.86           | 0.85      | 0.24        | 0.27   |
| 33       | 0.33          | 0.39     | 0.86           | 0.85      | 0.23        | 0.27   |
| 34       | 0.33          | 0.40     | 0.85           | 0.85      | 0.24        | 0.28   |
| 35       | 0.34          | 0.40     | 0.85           | 0.85      | 0.24        | 0.28   |
| 36       | 0.34          | 0.41     | 0.84           | 0.85      | 0.24        | 0.29   |
| 37       | 0.34          | 0.41     | 0.84           | 0.84      | 0.24        | 0.29   |
| 38       | 0.35          | 0.42     | 0.83           | 0.84      | 0.25        | 0.30   |
| 39       | 0.35          | 0.43     | 0.83           | 0.84      | 0.25        | 0.30   |
| 40       | 0.36          | 0.44     | 0.83           | 0.83      | 0.26        | 0.31   |
| 41       | 0.38          | 0.45     | 0.83           | 0.83      | 0.27        | 0.32   |
| 42       | 0.39          | 0.46     | 0.82           | 0.82      | 0.28        | 0.33   |
| 43       | 0.41          | 0.48     | 0.82           | 0.81      | 0.30        | 0.34   |
| 44       | 0.44          | 0.50     | 0.81           | 0.80      | 0.32        | 0.36   |
| 45       | 0.46          | 0.52     | 0.80           | 0.79      | 0.33        | 0.37   |
| 46       | 0.50          | 0.54     | 0.79           | 0.78      | 0.36        | 0.39   |
| 47       | 0.53          | 0.56     | 0.78           | 0.77      | 0.38        | 0.40   |
| 48       | 0.55          | 0.58     | 0.77           | 0.76      | 0.39        | 0.41   |
| 49       | 0.58          | 0.60     | 0.76           | 0.75      | 0.41        | 0.43   |
| 50       | 0.59          | 0.61     | 0.76           | 0.74      | 0.42        | 0.44   |
| 51       | 0.60          | 0.62     | 0.75           | 0.74      | 0.43        | 0.44   |
| 52       | 0.61          | 0.62     | 0.75           | 0.74      | 0.43        | 0.44   |
| 53       | 0.61          | 0.63     | 0.75           | 0.74      | 0.43        | 0.45   |
| 54       | 0.61          | 0.63     | 0.76           | 0.74      | 0.43        | 0.45   |
| 55       | 0.61          | 0.63     | 0.76           | 0.74      | 0.43        | 0.45   |
| 56       | 0.61          | 0.62     | 0.76           | 0.74      | 0.43        | 0.44   |
| 57       | 0.61          | 0.62     | 0.76           | 0.75      | 0.43        | 0.44   |
| 58       | 0.61          | 0.62     | 0.77           | 0.75      | 0.43        | 0.44   |
| 59       | 0.60          | 0.62     | 0.77           | 0.75      | 0.42        | 0.44   |
| 60       | 0.60          | 0.61     | 0.78           | 0.76      | 0.42        | 0.43   |
| 61       | 0.59          | 0.61     | 0.78           | 0.76      | 0.41        | 0.43   |
| 62       | 0.59          | 0.60     | 0.78           | 0.77      | 0.41        | 0.42   |
| 63       | 0.58          | 0.60     | 0.79           | 0.77      | 0.40        | 0.42   |

Continued on next page

| $\alpha$ | $\phi_S^\ell$ | $\phi_S$ | $\varphi^\ell$ | $\varphi$ | $\psi^\ell$ | $\psi$ |
|----------|---------------|----------|----------------|-----------|-------------|--------|
| 64       | 0.58          | 0.59     | 0.79           | 0.78      | 0.40        | 0.41   |
| 65       | 0.57          | 0.58     | 0.80           | 0.78      | 0.39        | 0.41   |
| 66       | 0.57          | 0.58     | 0.80           | 0.79      | 0.39        | 0.40   |
| 67       | 0.56          | 0.57     | 0.81           | 0.79      | 0.39        | 0.40   |
| 68       | 0.55          | 0.57     | 0.81           | 0.80      | 0.38        | 0.39   |
| 69       | 0.55          | 0.56     | 0.82           | 0.80      | 0.38        | 0.39   |
| 70       | 0.54          | 0.55     | 0.82           | 0.81      | 0.37        | 0.38   |
| 71       | 0.53          | 0.54     | 0.83           | 0.81      | 0.36        | 0.37   |
| 72       | 0.52          | 0.54     | 0.83           | 0.82      | 0.36        | 0.37   |
| 73       | 0.52          | 0.53     | 0.84           | 0.82      | 0.35        | 0.37   |
| 74       | 0.51          | 0.52     | 0.85           | 0.83      | 0.34        | 0.36   |
| 75       | 0.50          | 0.51     | 0.85           | 0.83      | 0.34        | 0.35   |
| 76       | 0.49          | 0.50     | 0.86           | 0.84      | 0.33        | 0.34   |
| 77       | 0.48          | 0.49     | 0.86           | 0.85      | 0.32        | 0.33   |
| 78       | 0.46          | 0.48     | 0.87           | 0.85      | 0.31        | 0.33   |
| 79       | 0.45          | 0.46     | 0.88           | 0.86      | 0.30        | 0.31   |
| 80       | 0.44          | 0.45     | 0.88           | 0.87      | 0.30        | 0.30   |
| 81       | 0.42          | 0.44     | 0.89           | 0.87      | 0.28        | 0.30   |
| 82       | 0.40          | 0.42     | 0.90           | 0.88      | 0.27        | 0.28   |
| 83       | 0.39          | 0.40     | 0.91           | 0.89      | 0.26        | 0.27   |
| 84       | 0.36          | 0.38     | 0.91           | 0.90      | 0.24        | 0.25   |
| 85       | 0.34          | 0.36     | 0.92           | 0.91      | 0.23        | 0.24   |
| 86       | 0.31          | 0.33     | 0.93           | 0.92      | 0.20        | 0.22   |
| 87       | 0.28          | 0.30     | 0.95           | 0.93      | 0.18        | 0.20   |
| 88       | 0.23          | 0.26     | 0.96           | 0.94      | 0.15        | 0.17   |
| 89       | 0.17          | 0.21     | 0.97           | 0.95      | 0.11        | 0.14   |
| 90       | 0.12          | 0.15     | 0.98           | 0.96      | 0.08        | 0.10   |

Table S134: Reference ( $\phi_S$ ,  $\varphi$ ,  $\psi$ ) and approached ( $\phi_S^\ell$ ,  $\varphi^\ell$ ,  $\psi^\ell$ ) values of the topological descriptors for the first excited-state of the pyridinium-phenolate (PP), computed at the PBE0/6-31++G(2d,p) level of theory.  $\alpha$  is the pyridinium-phenolate central twist angle amplitude.

| $\alpha$ | $\phi_S^\ell$ | $\phi_S$ | $\varphi^\ell$ | $\varphi$ | $\psi^\ell$ | $\psi$ |
|----------|---------------|----------|----------------|-----------|-------------|--------|
| 0        | 0.41          | 0.32     | 0.84           | 0.86      | 0.29        | 0.23   |
| 1        | 0.41          | 0.32     | 0.84           | 0.86      | 0.29        | 0.23   |
| 2        | 0.41          | 0.32     | 0.84           | 0.86      | 0.29        | 0.23   |
| 3        | 0.41          | 0.32     | 0.84           | 0.86      | 0.29        | 0.23   |
| 4        | 0.41          | 0.32     | 0.84           | 0.86      | 0.29        | 0.23   |
| 5        | 0.41          | 0.32     | 0.84           | 0.86      | 0.29        | 0.23   |
| 6        | 0.41          | 0.33     | 0.84           | 0.86      | 0.29        | 0.23   |
| 7        | 0.40          | 0.33     | 0.84           | 0.86      | 0.28        | 0.23   |
| 8        | 0.40          | 0.33     | 0.84           | 0.86      | 0.28        | 0.23   |
| 9        | 0.40          | 0.33     | 0.85           | 0.86      | 0.28        | 0.23   |
| 10       | 0.40          | 0.33     | 0.85           | 0.86      | 0.28        | 0.23   |
| 11       | 0.39          | 0.34     | 0.85           | 0.86      | 0.27        | 0.24   |
| 12       | 0.39          | 0.34     | 0.85           | 0.86      | 0.27        | 0.24   |
| 13       | 0.39          | 0.34     | 0.85           | 0.86      | 0.27        | 0.24   |
| 14       | 0.39          | 0.34     | 0.86           | 0.86      | 0.27        | 0.24   |
| 15       | 0.38          | 0.35     | 0.86           | 0.86      | 0.26        | 0.25   |
| 16       | 0.38          | 0.35     | 0.86           | 0.86      | 0.26        | 0.25   |
| 17       | 0.38          | 0.35     | 0.86           | 0.86      | 0.26        | 0.25   |
| 18       | 0.37          | 0.35     | 0.86           | 0.86      | 0.26        | 0.25   |
| 19       | 0.37          | 0.36     | 0.86           | 0.86      | 0.26        | 0.25   |
| 20       | 0.36          | 0.36     | 0.87           | 0.86      | 0.25        | 0.25   |
| 21       | 0.36          | 0.36     | 0.87           | 0.86      | 0.25        | 0.25   |
| 22       | 0.36          | 0.36     | 0.87           | 0.86      | 0.25        | 0.25   |
| 23       | 0.35          | 0.36     | 0.87           | 0.86      | 0.24        | 0.25   |
| 24       | 0.35          | 0.37     | 0.87           | 0.86      | 0.24        | 0.26   |
| 25       | 0.34          | 0.37     | 0.87           | 0.86      | 0.24        | 0.26   |
| 26       | 0.34          | 0.37     | 0.87           | 0.86      | 0.24        | 0.26   |
| 27       | 0.34          | 0.37     | 0.87           | 0.86      | 0.24        | 0.26   |
| 28       | 0.33          | 0.37     | 0.87           | 0.86      | 0.23        | 0.26   |
| 29       | 0.33          | 0.38     | 0.87           | 0.86      | 0.23        | 0.26   |
| 30       | 0.33          | 0.38     | 0.87           | 0.86      | 0.23        | 0.26   |
| 31       | 0.33          | 0.38     | 0.87           | 0.85      | 0.23        | 0.27   |

Continued on next page

| $\alpha$ | $\phi_S^\ell$ | $\phi_S$ | $\varphi^\ell$ | $\varphi$ | $\psi^\ell$ | $\psi$ |
|----------|---------------|----------|----------------|-----------|-------------|--------|
| 32       | 0.33          | 0.39     | 0.87           | 0.85      | 0.23        | 0.27   |
| 33       | 0.33          | 0.39     | 0.86           | 0.85      | 0.23        | 0.27   |
| 34       | 0.33          | 0.39     | 0.86           | 0.85      | 0.23        | 0.27   |
| 35       | 0.33          | 0.40     | 0.86           | 0.85      | 0.23        | 0.28   |
| 36       | 0.33          | 0.40     | 0.85           | 0.85      | 0.24        | 0.28   |
| 37       | 0.33          | 0.41     | 0.84           | 0.85      | 0.24        | 0.29   |
| 38       | 0.33          | 0.41     | 0.84           | 0.84      | 0.24        | 0.29   |
| 39       | 0.34          | 0.42     | 0.83           | 0.84      | 0.25        | 0.30   |
| 40       | 0.35          | 0.43     | 0.83           | 0.84      | 0.25        | 0.30   |
| 41       | 0.36          | 0.44     | 0.83           | 0.83      | 0.26        | 0.31   |
| 42       | 0.38          | 0.45     | 0.82           | 0.83      | 0.28        | 0.32   |
| 43       | 0.39          | 0.47     | 0.82           | 0.82      | 0.28        | 0.33   |
| 44       | 0.42          | 0.48     | 0.81           | 0.81      | 0.30        | 0.34   |
| 45       | 0.45          | 0.50     | 0.80           | 0.80      | 0.33        | 0.36   |
| 46       | 0.48          | 0.53     | 0.79           | 0.79      | 0.35        | 0.38   |
| 47       | 0.51          | 0.55     | 0.78           | 0.78      | 0.37        | 0.39   |
| 48       | 0.54          | 0.57     | 0.77           | 0.76      | 0.39        | 0.41   |
| 49       | 0.57          | 0.59     | 0.76           | 0.75      | 0.41        | 0.42   |
| 50       | 0.59          | 0.60     | 0.76           | 0.75      | 0.42        | 0.43   |
| 51       | 0.60          | 0.61     | 0.75           | 0.74      | 0.43        | 0.44   |
| 52       | 0.61          | 0.62     | 0.75           | 0.74      | 0.43        | 0.44   |
| 53       | 0.62          | 0.63     | 0.75           | 0.74      | 0.44        | 0.45   |
| 54       | 0.62          | 0.63     | 0.75           | 0.74      | 0.44        | 0.45   |
| 55       | 0.62          | 0.63     | 0.75           | 0.74      | 0.44        | 0.45   |
| 56       | 0.62          | 0.63     | 0.76           | 0.74      | 0.44        | 0.45   |
| 57       | 0.62          | 0.62     | 0.76           | 0.75      | 0.44        | 0.44   |
| 58       | 0.61          | 0.62     | 0.76           | 0.75      | 0.43        | 0.44   |
| 59       | 0.61          | 0.62     | 0.77           | 0.75      | 0.43        | 0.44   |
| 60       | 0.61          | 0.61     | 0.77           | 0.76      | 0.43        | 0.43   |
| 61       | 0.60          | 0.61     | 0.77           | 0.76      | 0.42        | 0.43   |
| 62       | 0.60          | 0.60     | 0.78           | 0.77      | 0.42        | 0.42   |
| 63       | 0.59          | 0.60     | 0.78           | 0.77      | 0.41        | 0.42   |

Continued on next page

| $\alpha$ | $\phi_S^\ell$ | $\phi_S$ | $\varphi^\ell$ | $\varphi$ | $\psi^\ell$ | $\psi$ |
|----------|---------------|----------|----------------|-----------|-------------|--------|
| 64       | 0.59          | 0.59     | 0.79           | 0.77      | 0.41        | 0.42   |
| 65       | 0.58          | 0.59     | 0.79           | 0.78      | 0.40        | 0.41   |
| 66       | 0.58          | 0.58     | 0.80           | 0.78      | 0.40        | 0.41   |
| 67       | 0.57          | 0.58     | 0.80           | 0.79      | 0.39        | 0.40   |
| 68       | 0.56          | 0.57     | 0.81           | 0.79      | 0.39        | 0.40   |
| 69       | 0.56          | 0.56     | 0.81           | 0.80      | 0.39        | 0.39   |
| 70       | 0.55          | 0.55     | 0.82           | 0.80      | 0.38        | 0.38   |
| 71       | 0.54          | 0.55     | 0.82           | 0.81      | 0.37        | 0.38   |
| 72       | 0.53          | 0.54     | 0.83           | 0.81      | 0.36        | 0.37   |
| 73       | 0.52          | 0.53     | 0.83           | 0.82      | 0.36        | 0.37   |
| 74       | 0.51          | 0.52     | 0.84           | 0.83      | 0.35        | 0.36   |
| 75       | 0.50          | 0.51     | 0.85           | 0.83      | 0.34        | 0.35   |
| 76       | 0.49          | 0.50     | 0.85           | 0.84      | 0.33        | 0.34   |
| 77       | 0.48          | 0.49     | 0.86           | 0.84      | 0.32        | 0.34   |
| 78       | 0.47          | 0.48     | 0.87           | 0.85      | 0.32        | 0.33   |
| 79       | 0.46          | 0.47     | 0.87           | 0.86      | 0.31        | 0.32   |
| 80       | 0.44          | 0.45     | 0.88           | 0.86      | 0.30        | 0.31   |
| 81       | 0.43          | 0.44     | 0.89           | 0.87      | 0.29        | 0.30   |
| 82       | 0.41          | 0.42     | 0.90           | 0.88      | 0.27        | 0.28   |
| 83       | 0.39          | 0.41     | 0.90           | 0.89      | 0.26        | 0.27   |
| 84       | 0.37          | 0.39     | 0.91           | 0.90      | 0.25        | 0.26   |
| 85       | 0.35          | 0.37     | 0.92           | 0.91      | 0.23        | 0.25   |
| 86       | 0.32          | 0.34     | 0.93           | 0.92      | 0.21        | 0.23   |
| 87       | 0.28          | 0.31     | 0.94           | 0.93      | 0.18        | 0.20   |
| 88       | 0.24          | 0.27     | 0.96           | 0.94      | 0.16        | 0.18   |
| 89       | 0.18          | 0.21     | 0.97           | 0.95      | 0.12        | 0.14   |
| 90       | 0.11          | 0.15     | 0.98           | 0.96      | 0.07        | 0.10   |

Table S135: Reference  $(\phi_S, \varphi, \psi)$  and approached  $(\phi_S^\ell, \varphi^\ell, \psi^\ell)$  values of the topological descriptors for the first excited-state of the pyridinium-phenolate (PP), computed at the PBE0/6-31++G(d,p) level of theory.  $\alpha$  is the pyridinium-phenolate central twist angle amplitude.

| $\alpha$ | $\phi_S^\ell$ | $\phi_S$ | $\varphi^\ell$ | $\varphi$ | $\psi^\ell$ | $\psi$ |
|----------|---------------|----------|----------------|-----------|-------------|--------|
| 0        | 0.41          | 0.32     | 0.84           | 0.86      | 0.29        | 0.23   |
| 1        | 0.41          | 0.32     | 0.84           | 0.86      | 0.29        | 0.23   |
| 2        | 0.41          | 0.32     | 0.84           | 0.86      | 0.29        | 0.23   |
| 3        | 0.41          | 0.32     | 0.84           | 0.86      | 0.29        | 0.23   |
| 4        | 0.41          | 0.32     | 0.84           | 0.86      | 0.29        | 0.23   |
| 5        | 0.41          | 0.32     | 0.84           | 0.86      | 0.29        | 0.23   |
| 6        | 0.41          | 0.33     | 0.84           | 0.86      | 0.29        | 0.23   |
| 7        | 0.40          | 0.33     | 0.84           | 0.86      | 0.28        | 0.23   |
| 8        | 0.40          | 0.33     | 0.84           | 0.86      | 0.28        | 0.23   |
| 9        | 0.40          | 0.33     | 0.85           | 0.86      | 0.28        | 0.23   |
| 10       | 0.40          | 0.33     | 0.85           | 0.86      | 0.28        | 0.23   |
| 11       | 0.39          | 0.34     | 0.85           | 0.86      | 0.27        | 0.24   |
| 12       | 0.39          | 0.34     | 0.85           | 0.86      | 0.27        | 0.24   |
| 13       | 0.39          | 0.34     | 0.85           | 0.86      | 0.27        | 0.24   |
| 14       | 0.39          | 0.34     | 0.86           | 0.86      | 0.27        | 0.24   |
| 15       | 0.38          | 0.35     | 0.86           | 0.86      | 0.26        | 0.25   |
| 16       | 0.38          | 0.35     | 0.86           | 0.86      | 0.26        | 0.25   |
| 17       | 0.38          | 0.35     | 0.86           | 0.86      | 0.26        | 0.25   |
| 18       | 0.37          | 0.35     | 0.86           | 0.86      | 0.26        | 0.25   |
| 19       | 0.37          | 0.36     | 0.87           | 0.86      | 0.26        | 0.25   |
| 20       | 0.36          | 0.36     | 0.87           | 0.86      | 0.25        | 0.25   |
| 21       | 0.36          | 0.36     | 0.87           | 0.86      | 0.25        | 0.25   |
| 22       | 0.35          | 0.36     | 0.87           | 0.86      | 0.24        | 0.25   |
| 23       | 0.35          | 0.36     | 0.87           | 0.86      | 0.24        | 0.25   |
| 24       | 0.35          | 0.37     | 0.87           | 0.86      | 0.24        | 0.26   |
| 25       | 0.34          | 0.37     | 0.87           | 0.86      | 0.24        | 0.26   |
| 26       | 0.34          | 0.37     | 0.87           | 0.86      | 0.24        | 0.26   |
| 27       | 0.34          | 0.37     | 0.87           | 0.86      | 0.24        | 0.26   |
| 28       | 0.33          | 0.37     | 0.87           | 0.86      | 0.23        | 0.26   |
| 29       | 0.33          | 0.38     | 0.87           | 0.86      | 0.23        | 0.26   |
| 30       | 0.33          | 0.38     | 0.87           | 0.86      | 0.23        | 0.26   |
| 31       | 0.33          | 0.38     | 0.87           | 0.85      | 0.23        | 0.27   |

Continued on next page

| $\alpha$ | $\phi_S^\ell$ | $\phi_S$ | $\varphi^\ell$ | $\varphi$ | $\psi^\ell$ | $\psi$ |
|----------|---------------|----------|----------------|-----------|-------------|--------|
| 32       | 0.33          | 0.39     | 0.87           | 0.85      | 0.23        | 0.27   |
| 33       | 0.33          | 0.39     | 0.86           | 0.85      | 0.23        | 0.27   |
| 34       | 0.32          | 0.39     | 0.86           | 0.85      | 0.23        | 0.27   |
| 35       | 0.33          | 0.40     | 0.86           | 0.85      | 0.23        | 0.28   |
| 36       | 0.33          | 0.40     | 0.85           | 0.85      | 0.24        | 0.28   |
| 37       | 0.33          | 0.41     | 0.84           | 0.85      | 0.24        | 0.29   |
| 38       | 0.33          | 0.41     | 0.84           | 0.84      | 0.24        | 0.29   |
| 39       | 0.34          | 0.42     | 0.83           | 0.84      | 0.25        | 0.30   |
| 40       | 0.35          | 0.43     | 0.83           | 0.84      | 0.25        | 0.30   |
| 41       | 0.36          | 0.44     | 0.83           | 0.83      | 0.26        | 0.31   |
| 42       | 0.38          | 0.45     | 0.82           | 0.83      | 0.28        | 0.32   |
| 43       | 0.40          | 0.47     | 0.82           | 0.82      | 0.29        | 0.33   |
| 44       | 0.42          | 0.49     | 0.81           | 0.81      | 0.30        | 0.35   |
| 45       | 0.45          | 0.50     | 0.80           | 0.80      | 0.33        | 0.36   |
| 46       | 0.48          | 0.53     | 0.79           | 0.79      | 0.35        | 0.38   |
| 47       | 0.51          | 0.55     | 0.78           | 0.78      | 0.37        | 0.39   |
| 48       | 0.54          | 0.57     | 0.77           | 0.76      | 0.39        | 0.41   |
| 49       | 0.57          | 0.59     | 0.76           | 0.75      | 0.41        | 0.42   |
| 50       | 0.59          | 0.60     | 0.76           | 0.75      | 0.42        | 0.43   |
| 51       | 0.60          | 0.61     | 0.75           | 0.74      | 0.43        | 0.44   |
| 52       | 0.61          | 0.62     | 0.75           | 0.74      | 0.43        | 0.44   |
| 53       | 0.62          | 0.63     | 0.75           | 0.74      | 0.44        | 0.45   |
| 54       | 0.62          | 0.63     | 0.75           | 0.74      | 0.44        | 0.45   |
| 55       | 0.62          | 0.63     | 0.75           | 0.74      | 0.44        | 0.45   |
| 56       | 0.62          | 0.63     | 0.76           | 0.74      | 0.44        | 0.45   |
| 57       | 0.62          | 0.62     | 0.76           | 0.75      | 0.44        | 0.44   |
| 58       | 0.61          | 0.62     | 0.76           | 0.75      | 0.43        | 0.44   |
| 59       | 0.61          | 0.62     | 0.77           | 0.75      | 0.43        | 0.44   |
| 60       | 0.61          | 0.61     | 0.77           | 0.76      | 0.43        | 0.43   |
| 61       | 0.60          | 0.61     | 0.77           | 0.76      | 0.42        | 0.43   |
| 62       | 0.60          | 0.60     | 0.78           | 0.77      | 0.42        | 0.42   |
| 63       | 0.59          | 0.60     | 0.78           | 0.77      | 0.41        | 0.42   |

Continued on next page



| $\alpha$ | $\phi_S^\ell$ | $\phi_S$ | $\varphi^\ell$ | $\varphi$ | $\psi^\ell$ | $\psi$ |
|----------|---------------|----------|----------------|-----------|-------------|--------|
| 64       | 0.59          | 0.59     | 0.79           | 0.77      | 0.41        | 0.42   |
| 65       | 0.58          | 0.59     | 0.79           | 0.78      | 0.40        | 0.41   |
| 66       | 0.58          | 0.58     | 0.80           | 0.78      | 0.40        | 0.41   |
| 67       | 0.57          | 0.58     | 0.80           | 0.79      | 0.39        | 0.40   |
| 68       | 0.56          | 0.57     | 0.81           | 0.79      | 0.39        | 0.40   |
| 69       | 0.56          | 0.56     | 0.81           | 0.80      | 0.39        | 0.39   |
| 70       | 0.55          | 0.55     | 0.82           | 0.80      | 0.38        | 0.38   |
| 71       | 0.54          | 0.55     | 0.82           | 0.81      | 0.37        | 0.38   |
| 72       | 0.53          | 0.54     | 0.83           | 0.81      | 0.36        | 0.37   |
| 73       | 0.52          | 0.53     | 0.83           | 0.82      | 0.36        | 0.37   |
| 74       | 0.51          | 0.52     | 0.84           | 0.83      | 0.35        | 0.36   |
| 75       | 0.50          | 0.51     | 0.85           | 0.83      | 0.34        | 0.35   |
| 76       | 0.49          | 0.50     | 0.85           | 0.84      | 0.33        | 0.34   |
| 77       | 0.48          | 0.49     | 0.86           | 0.84      | 0.32        | 0.34   |
| 78       | 0.47          | 0.48     | 0.87           | 0.85      | 0.32        | 0.33   |
| 79       | 0.46          | 0.47     | 0.87           | 0.86      | 0.31        | 0.32   |
| 80       | 0.44          | 0.45     | 0.88           | 0.86      | 0.30        | 0.31   |
| 81       | 0.43          | 0.44     | 0.89           | 0.87      | 0.29        | 0.30   |
| 82       | 0.41          | 0.42     | 0.90           | 0.88      | 0.27        | 0.28   |
| 83       | 0.39          | 0.41     | 0.90           | 0.89      | 0.26        | 0.27   |
| 84       | 0.37          | 0.39     | 0.91           | 0.90      | 0.25        | 0.26   |
| 85       | 0.35          | 0.37     | 0.92           | 0.91      | 0.23        | 0.25   |
| 86       | 0.32          | 0.34     | 0.93           | 0.92      | 0.21        | 0.23   |
| 87       | 0.28          | 0.31     | 0.94           | 0.93      | 0.18        | 0.20   |
| 88       | 0.24          | 0.27     | 0.96           | 0.94      | 0.16        | 0.18   |
| 89       | 0.18          | 0.21     | 0.97           | 0.95      | 0.12        | 0.14   |
| 90       | 0.11          | 0.15     | 0.98           | 0.96      | 0.07        | 0.10   |

Table S136: Reference ( $\phi_S$ ,  $\varphi$ ,  $\psi$ ) and approached ( $\phi_S^\ell$ ,  $\varphi^\ell$ ,  $\psi^\ell$ ) values of the topological descriptors for the first excited-state of the pyridinium-phenolate (PP), computed at the PBE0/6-31+G(d,p) level of theory.  $\alpha$  is the pyridinium-phenolate central twist angle amplitude.

| $\alpha$ | $\phi_S^\ell$ | $\phi_S$ | $\varphi^\ell$ | $\varphi$ | $\psi^\ell$ | $\psi$ |
|----------|---------------|----------|----------------|-----------|-------------|--------|
| 0        | 0.41          | 0.32     | 0.84           | 0.86      | 0.29        | 0.23   |
| 1        | 0.41          | 0.32     | 0.84           | 0.86      | 0.29        | 0.23   |
| 2        | 0.41          | 0.32     | 0.84           | 0.86      | 0.29        | 0.23   |
| 3        | 0.41          | 0.32     | 0.84           | 0.86      | 0.29        | 0.23   |
| 4        | 0.41          | 0.32     | 0.84           | 0.86      | 0.29        | 0.23   |
| 5        | 0.41          | 0.32     | 0.84           | 0.86      | 0.29        | 0.23   |
| 6        | 0.40          | 0.32     | 0.84           | 0.86      | 0.28        | 0.23   |
| 7        | 0.40          | 0.33     | 0.84           | 0.86      | 0.28        | 0.23   |
| 8        | 0.40          | 0.33     | 0.84           | 0.86      | 0.28        | 0.23   |
| 9        | 0.40          | 0.33     | 0.85           | 0.86      | 0.28        | 0.23   |
| 10       | 0.40          | 0.33     | 0.85           | 0.86      | 0.28        | 0.23   |
| 11       | 0.39          | 0.33     | 0.85           | 0.86      | 0.27        | 0.23   |
| 12       | 0.39          | 0.34     | 0.85           | 0.86      | 0.27        | 0.24   |
| 13       | 0.39          | 0.34     | 0.86           | 0.86      | 0.27        | 0.24   |
| 14       | 0.38          | 0.34     | 0.86           | 0.86      | 0.26        | 0.24   |
| 15       | 0.38          | 0.34     | 0.86           | 0.86      | 0.26        | 0.24   |
| 16       | 0.38          | 0.35     | 0.86           | 0.86      | 0.26        | 0.25   |
| 17       | 0.37          | 0.35     | 0.86           | 0.86      | 0.26        | 0.25   |
| 18       | 0.37          | 0.35     | 0.86           | 0.86      | 0.26        | 0.25   |
| 19       | 0.36          | 0.35     | 0.87           | 0.86      | 0.25        | 0.25   |
| 20       | 0.36          | 0.35     | 0.87           | 0.86      | 0.25        | 0.25   |
| 21       | 0.36          | 0.36     | 0.87           | 0.86      | 0.25        | 0.25   |
| 22       | 0.35          | 0.36     | 0.87           | 0.86      | 0.24        | 0.25   |
| 23       | 0.35          | 0.36     | 0.87           | 0.86      | 0.24        | 0.25   |
| 24       | 0.34          | 0.36     | 0.87           | 0.86      | 0.24        | 0.25   |
| 25       | 0.34          | 0.37     | 0.87           | 0.86      | 0.24        | 0.26   |
| 26       | 0.34          | 0.37     | 0.87           | 0.86      | 0.24        | 0.26   |
| 27       | 0.34          | 0.37     | 0.87           | 0.86      | 0.24        | 0.26   |
| 28       | 0.33          | 0.37     | 0.87           | 0.86      | 0.23        | 0.26   |
| 29       | 0.33          | 0.37     | 0.87           | 0.86      | 0.23        | 0.26   |
| 30       | 0.33          | 0.38     | 0.87           | 0.86      | 0.23        | 0.26   |
| 31       | 0.33          | 0.38     | 0.87           | 0.86      | 0.23        | 0.26   |

Continued on next page

| $\alpha$ | $\phi_S^\ell$ | $\phi_S$ | $\varphi^\ell$ | $\varphi$ | $\psi^\ell$ | $\psi$ |
|----------|---------------|----------|----------------|-----------|-------------|--------|
| 32       | 0.32          | 0.38     | 0.87           | 0.85      | 0.22        | 0.27   |
| 33       | 0.32          | 0.39     | 0.86           | 0.85      | 0.23        | 0.27   |
| 34       | 0.32          | 0.39     | 0.86           | 0.85      | 0.23        | 0.27   |
| 35       | 0.32          | 0.40     | 0.86           | 0.85      | 0.23        | 0.28   |
| 36       | 0.33          | 0.40     | 0.85           | 0.85      | 0.24        | 0.28   |
| 37       | 0.33          | 0.41     | 0.84           | 0.85      | 0.24        | 0.29   |
| 38       | 0.33          | 0.41     | 0.84           | 0.84      | 0.24        | 0.29   |
| 39       | 0.34          | 0.42     | 0.83           | 0.84      | 0.25        | 0.30   |
| 40       | 0.35          | 0.43     | 0.83           | 0.84      | 0.25        | 0.30   |
| 41       | 0.36          | 0.44     | 0.83           | 0.83      | 0.26        | 0.31   |
| 42       | 0.38          | 0.45     | 0.82           | 0.83      | 0.28        | 0.32   |
| 43       | 0.40          | 0.47     | 0.82           | 0.82      | 0.29        | 0.33   |
| 44       | 0.42          | 0.49     | 0.81           | 0.81      | 0.30        | 0.35   |
| 45       | 0.45          | 0.51     | 0.80           | 0.80      | 0.33        | 0.36   |
| 46       | 0.49          | 0.53     | 0.79           | 0.79      | 0.35        | 0.38   |
| 47       | 0.52          | 0.55     | 0.78           | 0.77      | 0.37        | 0.39   |
| 48       | 0.55          | 0.58     | 0.77           | 0.76      | 0.39        | 0.41   |
| 49       | 0.58          | 0.59     | 0.76           | 0.75      | 0.41        | 0.42   |
| 50       | 0.59          | 0.61     | 0.75           | 0.74      | 0.42        | 0.44   |
| 51       | 0.61          | 0.62     | 0.75           | 0.74      | 0.43        | 0.44   |
| 52       | 0.61          | 0.62     | 0.75           | 0.74      | 0.43        | 0.44   |
| 53       | 0.62          | 0.63     | 0.75           | 0.74      | 0.44        | 0.45   |
| 54       | 0.62          | 0.63     | 0.75           | 0.74      | 0.44        | 0.45   |
| 55       | 0.62          | 0.63     | 0.75           | 0.74      | 0.44        | 0.45   |
| 56       | 0.62          | 0.63     | 0.76           | 0.74      | 0.44        | 0.45   |
| 57       | 0.62          | 0.62     | 0.76           | 0.75      | 0.44        | 0.44   |
| 58       | 0.61          | 0.62     | 0.76           | 0.75      | 0.43        | 0.44   |
| 59       | 0.61          | 0.62     | 0.77           | 0.75      | 0.43        | 0.44   |
| 60       | 0.61          | 0.61     | 0.77           | 0.76      | 0.43        | 0.43   |
| 61       | 0.60          | 0.61     | 0.77           | 0.76      | 0.42        | 0.43   |
| 62       | 0.60          | 0.60     | 0.78           | 0.77      | 0.42        | 0.42   |
| 63       | 0.59          | 0.60     | 0.78           | 0.77      | 0.41        | 0.42   |

Continued on next page

| $\alpha$ | $\phi_S^\ell$ | $\phi_S$ | $\varphi^\ell$ | $\varphi$ | $\psi^\ell$ | $\psi$ |
|----------|---------------|----------|----------------|-----------|-------------|--------|
| 64       | 0.59          | 0.59     | 0.79           | 0.77      | 0.41        | 0.42   |
| 65       | 0.58          | 0.59     | 0.79           | 0.78      | 0.40        | 0.41   |
| 66       | 0.58          | 0.58     | 0.80           | 0.78      | 0.40        | 0.41   |
| 67       | 0.57          | 0.57     | 0.80           | 0.79      | 0.39        | 0.40   |
| 68       | 0.56          | 0.57     | 0.81           | 0.79      | 0.39        | 0.40   |
| 69       | 0.55          | 0.56     | 0.81           | 0.80      | 0.38        | 0.39   |
| 70       | 0.55          | 0.55     | 0.82           | 0.80      | 0.38        | 0.38   |
| 71       | 0.54          | 0.55     | 0.82           | 0.81      | 0.37        | 0.38   |
| 72       | 0.53          | 0.54     | 0.83           | 0.82      | 0.36        | 0.37   |
| 73       | 0.52          | 0.53     | 0.84           | 0.82      | 0.35        | 0.37   |
| 74       | 0.51          | 0.52     | 0.84           | 0.83      | 0.35        | 0.36   |
| 75       | 0.50          | 0.51     | 0.85           | 0.83      | 0.34        | 0.35   |
| 76       | 0.49          | 0.50     | 0.85           | 0.84      | 0.33        | 0.34   |
| 77       | 0.48          | 0.49     | 0.86           | 0.84      | 0.32        | 0.34   |
| 78       | 0.47          | 0.48     | 0.87           | 0.85      | 0.32        | 0.33   |
| 79       | 0.46          | 0.47     | 0.87           | 0.86      | 0.31        | 0.32   |
| 80       | 0.44          | 0.45     | 0.88           | 0.87      | 0.30        | 0.30   |
| 81       | 0.43          | 0.44     | 0.89           | 0.87      | 0.29        | 0.30   |
| 82       | 0.41          | 0.42     | 0.90           | 0.88      | 0.27        | 0.28   |
| 83       | 0.39          | 0.41     | 0.90           | 0.89      | 0.26        | 0.27   |
| 84       | 0.37          | 0.39     | 0.91           | 0.90      | 0.25        | 0.26   |
| 85       | 0.35          | 0.36     | 0.92           | 0.91      | 0.23        | 0.24   |
| 86       | 0.32          | 0.34     | 0.93           | 0.92      | 0.21        | 0.23   |
| 87       | 0.28          | 0.31     | 0.94           | 0.93      | 0.18        | 0.20   |
| 88       | 0.24          | 0.27     | 0.96           | 0.94      | 0.16        | 0.18   |
| 89       | 0.17          | 0.21     | 0.97           | 0.95      | 0.11        | 0.14   |
| 90       | 0.11          | 0.15     | 0.98           | 0.96      | 0.07        | 0.10   |

Table S137: Reference ( $\phi_S$ ,  $\varphi$ ,  $\psi$ ) and approached ( $\phi_S^\ell$ ,  $\varphi^\ell$ ,  $\psi^\ell$ ) values of the topological descriptors for the first excited-state of the pyridinium-phenolate (PP), computed at the PBE0/6-31+G(d) level of theory.  $\alpha$  is the pyridinium-phenolate central twist angle amplitude.

| $\alpha$ | $\phi_S^\ell$ | $\phi_S$ | $\varphi^\ell$ | $\varphi$ | $\psi^\ell$ | $\psi$ |
|----------|---------------|----------|----------------|-----------|-------------|--------|
| 0        | 0.42          | 0.32     | 0.83           | 0.86      | 0.30        | 0.23   |
| 1        | 0.42          | 0.32     | 0.83           | 0.86      | 0.30        | 0.23   |
| 2        | 0.42          | 0.32     | 0.83           | 0.86      | 0.30        | 0.23   |
| 3        | 0.42          | 0.32     | 0.83           | 0.86      | 0.30        | 0.23   |
| 4        | 0.42          | 0.32     | 0.83           | 0.86      | 0.30        | 0.23   |
| 5        | 0.42          | 0.32     | 0.83           | 0.86      | 0.30        | 0.23   |
| 6        | 0.41          | 0.32     | 0.83           | 0.86      | 0.29        | 0.23   |
| 7        | 0.41          | 0.32     | 0.83           | 0.86      | 0.29        | 0.23   |
| 8        | 0.41          | 0.32     | 0.84           | 0.86      | 0.29        | 0.23   |
| 9        | 0.40          | 0.32     | 0.84           | 0.86      | 0.28        | 0.23   |
| 10       | 0.40          | 0.33     | 0.84           | 0.86      | 0.28        | 0.23   |
| 11       | 0.39          | 0.33     | 0.84           | 0.86      | 0.28        | 0.23   |
| 12       | 0.39          | 0.33     | 0.84           | 0.86      | 0.28        | 0.23   |
| 13       | 0.38          | 0.33     | 0.85           | 0.86      | 0.27        | 0.23   |
| 14       | 0.38          | 0.33     | 0.85           | 0.86      | 0.27        | 0.23   |
| 15       | 0.37          | 0.33     | 0.85           | 0.86      | 0.26        | 0.23   |
| 16       | 0.36          | 0.33     | 0.85           | 0.86      | 0.26        | 0.23   |
| 17       | 0.36          | 0.33     | 0.86           | 0.86      | 0.25        | 0.23   |
| 18       | 0.35          | 0.33     | 0.86           | 0.86      | 0.25        | 0.23   |
| 19       | 0.34          | 0.33     | 0.86           | 0.86      | 0.24        | 0.23   |
| 20       | 0.33          | 0.33     | 0.86           | 0.86      | 0.23        | 0.23   |
| 21       | 0.32          | 0.33     | 0.86           | 0.86      | 0.23        | 0.23   |
| 22       | 0.32          | 0.33     | 0.87           | 0.86      | 0.22        | 0.23   |
| 23       | 0.31          | 0.33     | 0.87           | 0.86      | 0.22        | 0.23   |
| 24       | 0.30          | 0.33     | 0.87           | 0.87      | 0.21        | 0.23   |
| 25       | 0.29          | 0.33     | 0.87           | 0.87      | 0.20        | 0.23   |
| 26       | 0.28          | 0.33     | 0.88           | 0.87      | 0.20        | 0.23   |
| 27       | 0.27          | 0.33     | 0.88           | 0.87      | 0.19        | 0.23   |
| 28       | 0.26          | 0.33     | 0.88           | 0.87      | 0.18        | 0.23   |
| 29       | 0.25          | 0.33     | 0.89           | 0.87      | 0.17        | 0.23   |
| 30       | 0.25          | 0.33     | 0.90           | 0.87      | 0.17        | 0.23   |
| 31       | 0.24          | 0.33     | 0.90           | 0.87      | 0.17        | 0.23   |

Continued on next page

| $\alpha$ | $\phi_S^\ell$ | $\phi_S$ | $\varphi^\ell$ | $\varphi$ | $\psi^\ell$ | $\psi$ |
|----------|---------------|----------|----------------|-----------|-------------|--------|
| 32       | 0.23          | 0.32     | 0.91           | 0.87      | 0.16        | 0.22   |
| 33       | 0.22          | 0.32     | 0.92           | 0.87      | 0.15        | 0.22   |
| 34       | 0.21          | 0.32     | 0.93           | 0.87      | 0.14        | 0.22   |
| 35       | 0.20          | 0.32     | 0.93           | 0.87      | 0.13        | 0.22   |
| 36       | 0.19          | 0.32     | 0.94           | 0.87      | 0.13        | 0.22   |
| 37       | 0.18          | 0.32     | 0.94           | 0.87      | 0.12        | 0.22   |
| 38       | 0.18          | 0.32     | 0.95           | 0.87      | 0.12        | 0.22   |
| 39       | 0.17          | 0.32     | 0.95           | 0.88      | 0.11        | 0.22   |
| 40       | 0.16          | 0.32     | 0.96           | 0.88      | 0.11        | 0.22   |
| 41       | 0.15          | 0.32     | 0.96           | 0.88      | 0.10        | 0.22   |
| 42       | 0.14          | 0.32     | 0.97           | 0.88      | 0.09        | 0.22   |
| 43       | 0.14          | 0.31     | 0.97           | 0.88      | 0.09        | 0.22   |
| 44       | 0.13          | 0.31     | 0.97           | 0.88      | 0.08        | 0.22   |
| 45       | 0.13          | 0.31     | 0.97           | 0.88      | 0.08        | 0.22   |
| 46       | 0.13          | 0.31     | 0.97           | 0.88      | 0.08        | 0.22   |
| 47       | 0.13          | 0.31     | 0.97           | 0.88      | 0.08        | 0.22   |
| 48       | 0.13          | 0.31     | 0.97           | 0.88      | 0.08        | 0.22   |
| 49       | 0.14          | 0.31     | 0.97           | 0.89      | 0.09        | 0.21   |
| 50       | 0.15          | 0.31     | 0.96           | 0.89      | 0.10        | 0.21   |
| 51       | 0.16          | 0.31     | 0.96           | 0.89      | 0.11        | 0.21   |
| 52       | 0.17          | 0.31     | 0.96           | 0.89      | 0.11        | 0.21   |
| 53       | 0.18          | 0.31     | 0.95           | 0.89      | 0.12        | 0.21   |
| 54       | 0.19          | 0.31     | 0.95           | 0.89      | 0.13        | 0.21   |
| 55       | 0.21          | 0.31     | 0.94           | 0.89      | 0.14        | 0.21   |
| 56       | 0.22          | 0.32     | 0.93           | 0.89      | 0.15        | 0.22   |
| 57       | 0.24          | 0.33     | 0.92           | 0.88      | 0.16        | 0.23   |
| 58       | 0.26          | 0.35     | 0.92           | 0.88      | 0.18        | 0.24   |
| 59       | 0.30          | 0.38     | 0.91           | 0.87      | 0.20        | 0.26   |
| 60       | 0.39          | 0.44     | 0.87           | 0.84      | 0.27        | 0.31   |
| 61       | 0.53          | 0.55     | 0.79           | 0.79      | 0.38        | 0.39   |
| 62       | 0.60          | 0.61     | 0.77           | 0.76      | 0.42        | 0.43   |
| 63       | 0.62          | 0.62     | 0.76           | 0.75      | 0.44        | 0.44   |

Continued on next page

| $\alpha$ | $\phi_S^\ell$ | $\phi_S$ | $\varphi^\ell$ | $\varphi$ | $\psi^\ell$ | $\psi$ |
|----------|---------------|----------|----------------|-----------|-------------|--------|
| 64       | 0.62          | 0.62     | 0.77           | 0.76      | 0.43        | 0.44   |
| 65       | 0.61          | 0.61     | 0.77           | 0.76      | 0.43        | 0.43   |
| 66       | 0.61          | 0.61     | 0.77           | 0.76      | 0.43        | 0.43   |
| 67       | 0.60          | 0.60     | 0.78           | 0.77      | 0.42        | 0.42   |
| 68       | 0.60          | 0.60     | 0.78           | 0.77      | 0.42        | 0.42   |
| 69       | 0.59          | 0.59     | 0.79           | 0.78      | 0.41        | 0.41   |
| 70       | 0.58          | 0.59     | 0.80           | 0.78      | 0.40        | 0.41   |
| 71       | 0.58          | 0.58     | 0.80           | 0.79      | 0.40        | 0.40   |
| 72       | 0.57          | 0.57     | 0.81           | 0.79      | 0.39        | 0.40   |
| 73       | 0.56          | 0.56     | 0.81           | 0.80      | 0.39        | 0.39   |
| 74       | 0.55          | 0.56     | 0.82           | 0.80      | 0.38        | 0.39   |
| 75       | 0.54          | 0.55     | 0.82           | 0.81      | 0.37        | 0.38   |
| 76       | 0.54          | 0.54     | 0.83           | 0.82      | 0.37        | 0.37   |
| 77       | 0.53          | 0.53     | 0.84           | 0.82      | 0.36        | 0.37   |
| 78       | 0.52          | 0.52     | 0.84           | 0.83      | 0.35        | 0.36   |
| 79       | 0.50          | 0.51     | 0.85           | 0.83      | 0.34        | 0.35   |
| 80       | 0.49          | 0.50     | 0.86           | 0.84      | 0.33        | 0.34   |
| 81       | 0.48          | 0.49     | 0.86           | 0.85      | 0.32        | 0.33   |
| 82       | 0.47          | 0.47     | 0.87           | 0.86      | 0.32        | 0.32   |
| 83       | 0.45          | 0.46     | 0.88           | 0.86      | 0.30        | 0.31   |
| 84       | 0.43          | 0.44     | 0.89           | 0.87      | 0.29        | 0.30   |
| 85       | 0.41          | 0.42     | 0.90           | 0.88      | 0.27        | 0.28   |
| 86       | 0.39          | 0.40     | 0.91           | 0.89      | 0.26        | 0.27   |
| 87       | 0.36          | 0.38     | 0.92           | 0.90      | 0.24        | 0.25   |
| 88       | 0.33          | 0.35     | 0.93           | 0.91      | 0.22        | 0.23   |
| 89       | 0.28          | 0.31     | 0.95           | 0.93      | 0.18        | 0.20   |
| 90       | 0.11          | 0.15     | 0.98           | 0.96      | 0.07        | 0.10   |

Table S138: Reference ( $\phi_S$ ,  $\varphi$ ,  $\psi$ ) and approached ( $\phi_S^\ell$ ,  $\varphi^\ell$ ,  $\psi^\ell$ ) values of the topological descriptors for the first excited-state of the pyridinium-phenolate (PP), computed at the PBE0/6-31G(d) level of theory.  $\alpha$  is the pyridinium-phenolate central twist angle amplitude.

| $\alpha$ | $\phi_S^\ell$ | $\phi_S$ | $\varphi^\ell$ | $\varphi$ | $\psi^\ell$ | $\psi$ |
|----------|---------------|----------|----------------|-----------|-------------|--------|
| 0        | 0.42          | 0.32     | 0.83           | 0.86      | 0.30        | 0.23   |
| 1        | 0.42          | 0.32     | 0.83           | 0.86      | 0.30        | 0.23   |
| 2        | 0.41          | 0.32     | 0.83           | 0.86      | 0.29        | 0.23   |
| 3        | 0.41          | 0.32     | 0.83           | 0.86      | 0.29        | 0.23   |
| 4        | 0.41          | 0.32     | 0.83           | 0.86      | 0.29        | 0.23   |
| 5        | 0.41          | 0.32     | 0.83           | 0.86      | 0.29        | 0.23   |
| 6        | 0.41          | 0.33     | 0.83           | 0.86      | 0.29        | 0.23   |
| 7        | 0.41          | 0.33     | 0.84           | 0.86      | 0.29        | 0.23   |
| 8        | 0.40          | 0.33     | 0.84           | 0.86      | 0.28        | 0.23   |
| 9        | 0.40          | 0.33     | 0.84           | 0.86      | 0.28        | 0.23   |
| 10       | 0.40          | 0.33     | 0.84           | 0.86      | 0.28        | 0.23   |
| 11       | 0.39          | 0.33     | 0.85           | 0.86      | 0.27        | 0.23   |
| 12       | 0.39          | 0.34     | 0.85           | 0.86      | 0.27        | 0.24   |
| 13       | 0.39          | 0.34     | 0.85           | 0.86      | 0.27        | 0.24   |
| 14       | 0.38          | 0.34     | 0.85           | 0.86      | 0.27        | 0.24   |
| 15       | 0.38          | 0.34     | 0.85           | 0.86      | 0.27        | 0.24   |
| 16       | 0.38          | 0.34     | 0.86           | 0.86      | 0.26        | 0.24   |
| 17       | 0.37          | 0.35     | 0.86           | 0.86      | 0.26        | 0.25   |
| 18       | 0.37          | 0.35     | 0.86           | 0.86      | 0.26        | 0.25   |
| 19       | 0.36          | 0.35     | 0.86           | 0.86      | 0.25        | 0.25   |
| 20       | 0.36          | 0.35     | 0.86           | 0.86      | 0.25        | 0.25   |
| 21       | 0.35          | 0.35     | 0.87           | 0.86      | 0.24        | 0.25   |
| 22       | 0.35          | 0.36     | 0.87           | 0.86      | 0.24        | 0.25   |
| 23       | 0.34          | 0.36     | 0.87           | 0.86      | 0.24        | 0.25   |
| 24       | 0.34          | 0.36     | 0.87           | 0.86      | 0.24        | 0.25   |
| 25       | 0.34          | 0.36     | 0.87           | 0.86      | 0.24        | 0.25   |
| 26       | 0.33          | 0.36     | 0.87           | 0.86      | 0.23        | 0.25   |
| 27       | 0.33          | 0.36     | 0.87           | 0.86      | 0.23        | 0.25   |
| 28       | 0.32          | 0.37     | 0.87           | 0.86      | 0.22        | 0.26   |
| 29       | 0.32          | 0.37     | 0.87           | 0.86      | 0.22        | 0.26   |
| 30       | 0.32          | 0.37     | 0.87           | 0.86      | 0.22        | 0.26   |
| 31       | 0.32          | 0.37     | 0.87           | 0.86      | 0.22        | 0.26   |

Continued on next page



| $\alpha$ | $\phi_S^\ell$ | $\phi_S$ | $\varphi^\ell$ | $\varphi$ | $\psi^\ell$ | $\psi$ |
|----------|---------------|----------|----------------|-----------|-------------|--------|
| 32       | 0.31          | 0.37     | 0.87           | 0.86      | 0.22        | 0.26   |
| 33       | 0.31          | 0.38     | 0.87           | 0.86      | 0.22        | 0.26   |
| 34       | 0.31          | 0.38     | 0.86           | 0.86      | 0.22        | 0.26   |
| 35       | 0.31          | 0.38     | 0.86           | 0.86      | 0.22        | 0.26   |
| 36       | 0.31          | 0.39     | 0.86           | 0.86      | 0.22        | 0.27   |
| 37       | 0.31          | 0.39     | 0.86           | 0.85      | 0.22        | 0.27   |
| 38       | 0.31          | 0.40     | 0.86           | 0.85      | 0.22        | 0.28   |
| 39       | 0.31          | 0.40     | 0.85           | 0.85      | 0.22        | 0.28   |
| 40       | 0.32          | 0.41     | 0.85           | 0.85      | 0.23        | 0.29   |
| 41       | 0.32          | 0.41     | 0.84           | 0.85      | 0.23        | 0.29   |
| 42       | 0.33          | 0.42     | 0.84           | 0.84      | 0.24        | 0.30   |
| 43       | 0.34          | 0.43     | 0.84           | 0.84      | 0.24        | 0.30   |
| 44       | 0.36          | 0.44     | 0.83           | 0.83      | 0.26        | 0.31   |
| 45       | 0.38          | 0.46     | 0.82           | 0.83      | 0.28        | 0.32   |
| 46       | 0.40          | 0.47     | 0.82           | 0.82      | 0.29        | 0.33   |
| 47       | 0.43          | 0.49     | 0.81           | 0.81      | 0.31        | 0.35   |
| 48       | 0.46          | 0.51     | 0.80           | 0.80      | 0.33        | 0.36   |
| 49       | 0.49          | 0.53     | 0.79           | 0.79      | 0.35        | 0.38   |
| 50       | 0.52          | 0.55     | 0.78           | 0.78      | 0.37        | 0.39   |
| 51       | 0.55          | 0.57     | 0.77           | 0.77      | 0.39        | 0.41   |
| 52       | 0.57          | 0.59     | 0.77           | 0.76      | 0.41        | 0.42   |
| 53       | 0.59          | 0.60     | 0.76           | 0.75      | 0.42        | 0.43   |
| 54       | 0.60          | 0.61     | 0.76           | 0.75      | 0.43        | 0.43   |
| 55       | 0.61          | 0.61     | 0.76           | 0.75      | 0.43        | 0.43   |
| 56       | 0.61          | 0.62     | 0.76           | 0.75      | 0.43        | 0.44   |
| 57       | 0.61          | 0.62     | 0.76           | 0.75      | 0.43        | 0.44   |
| 58       | 0.61          | 0.62     | 0.76           | 0.75      | 0.43        | 0.44   |
| 59       | 0.61          | 0.61     | 0.76           | 0.75      | 0.43        | 0.43   |
| 60       | 0.61          | 0.61     | 0.77           | 0.76      | 0.43        | 0.43   |
| 61       | 0.60          | 0.61     | 0.77           | 0.76      | 0.42        | 0.43   |
| 62       | 0.60          | 0.61     | 0.78           | 0.76      | 0.42        | 0.43   |
| 63       | 0.60          | 0.60     | 0.78           | 0.77      | 0.42        | 0.42   |

Continued on next page

| $\alpha$ | $\phi_S^\ell$ | $\phi_S$ | $\varphi^\ell$ | $\varphi$ | $\psi^\ell$ | $\psi$ |
|----------|---------------|----------|----------------|-----------|-------------|--------|
| 64       | 0.59          | 0.60     | 0.78           | 0.77      | 0.41        | 0.42   |
| 65       | 0.59          | 0.59     | 0.79           | 0.78      | 0.41        | 0.41   |
| 66       | 0.58          | 0.59     | 0.79           | 0.78      | 0.40        | 0.41   |
| 67       | 0.57          | 0.58     | 0.80           | 0.79      | 0.39        | 0.40   |
| 68       | 0.57          | 0.57     | 0.80           | 0.79      | 0.39        | 0.40   |
| 69       | 0.56          | 0.57     | 0.81           | 0.80      | 0.39        | 0.39   |
| 70       | 0.55          | 0.56     | 0.82           | 0.80      | 0.38        | 0.39   |
| 71       | 0.55          | 0.55     | 0.82           | 0.81      | 0.38        | 0.38   |
| 72       | 0.54          | 0.55     | 0.83           | 0.81      | 0.37        | 0.38   |
| 73       | 0.53          | 0.54     | 0.83           | 0.82      | 0.36        | 0.37   |
| 74       | 0.52          | 0.53     | 0.84           | 0.82      | 0.35        | 0.37   |
| 75       | 0.51          | 0.52     | 0.84           | 0.83      | 0.35        | 0.36   |
| 76       | 0.50          | 0.51     | 0.85           | 0.83      | 0.34        | 0.35   |
| 77       | 0.49          | 0.50     | 0.86           | 0.84      | 0.33        | 0.34   |
| 78       | 0.48          | 0.49     | 0.86           | 0.85      | 0.32        | 0.33   |
| 79       | 0.47          | 0.48     | 0.87           | 0.85      | 0.32        | 0.33   |
| 80       | 0.45          | 0.46     | 0.88           | 0.86      | 0.30        | 0.31   |
| 81       | 0.44          | 0.45     | 0.89           | 0.87      | 0.29        | 0.30   |
| 82       | 0.42          | 0.44     | 0.90           | 0.88      | 0.28        | 0.30   |
| 83       | 0.40          | 0.42     | 0.90           | 0.88      | 0.27        | 0.28   |
| 84       | 0.38          | 0.40     | 0.91           | 0.89      | 0.25        | 0.27   |
| 85       | 0.36          | 0.38     | 0.92           | 0.90      | 0.24        | 0.25   |
| 86       | 0.33          | 0.36     | 0.93           | 0.91      | 0.22        | 0.24   |
| 87       | 0.30          | 0.33     | 0.94           | 0.92      | 0.20        | 0.22   |
| 88       | 0.26          | 0.29     | 0.96           | 0.93      | 0.17        | 0.19   |
| 89       | 0.19          | 0.24     | 0.97           | 0.95      | 0.12        | 0.16   |
| 90       | 0.09          | 0.14     | 0.99           | 0.96      | 0.06        | 0.09   |

Table S139: Reference ( $\phi_S$ ,  $\varphi$ ,  $\psi$ ) and approached ( $\phi_S^\ell$ ,  $\varphi^\ell$ ,  $\psi^\ell$ ) values of the topological descriptors for the first excited-state of the pyridinium-phenolate (PP), computed at the PBE0/6-31+G level of theory.  $\alpha$  is the pyridinium-phenolate central twist angle amplitude.

| $\alpha$ | $\phi_S^\ell$ | $\phi_S$ | $\varphi^\ell$ | $\varphi$ | $\psi^\ell$ | $\psi$ |
|----------|---------------|----------|----------------|-----------|-------------|--------|
| 0        | 0.43          | 0.32     | 0.82           | 0.86      | 0.31        | 0.23   |
| 1        | 0.43          | 0.32     | 0.82           | 0.86      | 0.31        | 0.23   |
| 2        | 0.43          | 0.32     | 0.82           | 0.86      | 0.31        | 0.23   |
| 3        | 0.42          | 0.32     | 0.82           | 0.86      | 0.30        | 0.23   |
| 4        | 0.42          | 0.33     | 0.82           | 0.86      | 0.30        | 0.23   |
| 5        | 0.42          | 0.33     | 0.82           | 0.86      | 0.30        | 0.23   |
| 6        | 0.42          | 0.33     | 0.82           | 0.86      | 0.30        | 0.23   |
| 7        | 0.41          | 0.33     | 0.83           | 0.86      | 0.29        | 0.23   |
| 8        | 0.41          | 0.33     | 0.83           | 0.86      | 0.29        | 0.23   |
| 9        | 0.41          | 0.33     | 0.83           | 0.86      | 0.29        | 0.23   |
| 10       | 0.40          | 0.33     | 0.83           | 0.86      | 0.29        | 0.23   |
| 11       | 0.40          | 0.33     | 0.84           | 0.86      | 0.28        | 0.23   |
| 12       | 0.39          | 0.33     | 0.84           | 0.86      | 0.28        | 0.23   |
| 13       | 0.39          | 0.33     | 0.84           | 0.86      | 0.28        | 0.23   |
| 14       | 0.38          | 0.33     | 0.84           | 0.86      | 0.27        | 0.23   |
| 15       | 0.37          | 0.33     | 0.85           | 0.86      | 0.26        | 0.23   |
| 16       | 0.37          | 0.33     | 0.85           | 0.86      | 0.26        | 0.23   |
| 17       | 0.36          | 0.33     | 0.85           | 0.86      | 0.26        | 0.23   |
| 18       | 0.35          | 0.33     | 0.85           | 0.86      | 0.25        | 0.23   |
| 19       | 0.35          | 0.33     | 0.85           | 0.86      | 0.25        | 0.23   |
| 20       | 0.34          | 0.33     | 0.86           | 0.86      | 0.24        | 0.23   |
| 21       | 0.33          | 0.33     | 0.86           | 0.86      | 0.23        | 0.23   |
| 22       | 0.32          | 0.33     | 0.86           | 0.86      | 0.23        | 0.23   |
| 23       | 0.31          | 0.33     | 0.86           | 0.86      | 0.22        | 0.23   |
| 24       | 0.30          | 0.33     | 0.87           | 0.86      | 0.21        | 0.23   |
| 25       | 0.30          | 0.33     | 0.87           | 0.86      | 0.21        | 0.23   |
| 26       | 0.29          | 0.33     | 0.87           | 0.86      | 0.20        | 0.23   |
| 27       | 0.28          | 0.33     | 0.87           | 0.86      | 0.20        | 0.23   |
| 28       | 0.27          | 0.33     | 0.88           | 0.87      | 0.19        | 0.23   |
| 29       | 0.26          | 0.33     | 0.89           | 0.87      | 0.18        | 0.23   |
| 30       | 0.25          | 0.33     | 0.89           | 0.87      | 0.17        | 0.23   |
| 31       | 0.24          | 0.33     | 0.90           | 0.87      | 0.17        | 0.23   |

Continued on next page

| $\alpha$ | $\phi_S^\ell$ | $\phi_S$ | $\varphi^\ell$ | $\varphi$ | $\psi^\ell$ | $\psi$ |
|----------|---------------|----------|----------------|-----------|-------------|--------|
| 32       | 0.24          | 0.33     | 0.91           | 0.87      | 0.16        | 0.23   |
| 33       | 0.23          | 0.33     | 0.91           | 0.87      | 0.16        | 0.23   |
| 34       | 0.22          | 0.33     | 0.92           | 0.87      | 0.15        | 0.23   |
| 35       | 0.21          | 0.33     | 0.93           | 0.87      | 0.14        | 0.23   |
| 36       | 0.20          | 0.33     | 0.93           | 0.87      | 0.13        | 0.23   |
| 37       | 0.19          | 0.33     | 0.94           | 0.87      | 0.13        | 0.23   |
| 38       | 0.19          | 0.33     | 0.94           | 0.87      | 0.13        | 0.23   |
| 39       | 0.18          | 0.32     | 0.95           | 0.87      | 0.12        | 0.22   |
| 40       | 0.17          | 0.32     | 0.95           | 0.87      | 0.11        | 0.22   |
| 41       | 0.16          | 0.32     | 0.96           | 0.88      | 0.11        | 0.22   |
| 42       | 0.16          | 0.32     | 0.96           | 0.88      | 0.11        | 0.22   |
| 43       | 0.15          | 0.32     | 0.96           | 0.88      | 0.10        | 0.22   |
| 44       | 0.15          | 0.32     | 0.96           | 0.88      | 0.10        | 0.22   |
| 45       | 0.14          | 0.32     | 0.96           | 0.88      | 0.09        | 0.22   |
| 46       | 0.14          | 0.32     | 0.96           | 0.88      | 0.09        | 0.22   |
| 47       | 0.15          | 0.32     | 0.96           | 0.88      | 0.10        | 0.22   |
| 48       | 0.15          | 0.32     | 0.96           | 0.88      | 0.10        | 0.22   |
| 49       | 0.16          | 0.32     | 0.96           | 0.88      | 0.11        | 0.22   |
| 50       | 0.16          | 0.32     | 0.95           | 0.88      | 0.11        | 0.22   |
| 51       | 0.17          | 0.32     | 0.95           | 0.88      | 0.11        | 0.22   |
| 52       | 0.18          | 0.32     | 0.95           | 0.88      | 0.12        | 0.22   |
| 53       | 0.19          | 0.33     | 0.94           | 0.88      | 0.13        | 0.23   |
| 54       | 0.21          | 0.33     | 0.93           | 0.88      | 0.14        | 0.23   |
| 55       | 0.22          | 0.33     | 0.93           | 0.88      | 0.15        | 0.23   |
| 56       | 0.24          | 0.34     | 0.92           | 0.88      | 0.16        | 0.23   |
| 57       | 0.25          | 0.35     | 0.92           | 0.88      | 0.17        | 0.24   |
| 58       | 0.28          | 0.36     | 0.91           | 0.87      | 0.19        | 0.25   |
| 59       | 0.31          | 0.38     | 0.91           | 0.87      | 0.21        | 0.26   |
| 60       | 0.35          | 0.41     | 0.89           | 0.85      | 0.24        | 0.29   |
| 61       | 0.41          | 0.46     | 0.86           | 0.83      | 0.28        | 0.32   |
| 62       | 0.49          | 0.51     | 0.81           | 0.81      | 0.35        | 0.36   |
| 63       | 0.55          | 0.56     | 0.79           | 0.78      | 0.39        | 0.40   |

Continued on next page

| $\alpha$ | $\phi_S^\ell$ | $\phi_S$ | $\varphi^\ell$ | $\varphi$ | $\psi^\ell$ | $\psi$ |
|----------|---------------|----------|----------------|-----------|-------------|--------|
| 64       | 0.59          | 0.59     | 0.78           | 0.77      | 0.41        | 0.42   |
| 65       | 0.60          | 0.60     | 0.77           | 0.76      | 0.42        | 0.43   |
| 66       | 0.61          | 0.61     | 0.77           | 0.76      | 0.43        | 0.43   |
| 67       | 0.61          | 0.60     | 0.78           | 0.77      | 0.42        | 0.42   |
| 68       | 0.60          | 0.60     | 0.78           | 0.77      | 0.42        | 0.42   |
| 69       | 0.60          | 0.60     | 0.79           | 0.78      | 0.41        | 0.42   |
| 70       | 0.59          | 0.59     | 0.79           | 0.78      | 0.41        | 0.41   |
| 71       | 0.58          | 0.58     | 0.80           | 0.78      | 0.40        | 0.41   |
| 72       | 0.58          | 0.58     | 0.80           | 0.79      | 0.40        | 0.40   |
| 73       | 0.57          | 0.57     | 0.81           | 0.79      | 0.39        | 0.40   |
| 74       | 0.56          | 0.56     | 0.81           | 0.80      | 0.39        | 0.39   |
| 75       | 0.55          | 0.56     | 0.82           | 0.81      | 0.38        | 0.39   |
| 76       | 0.54          | 0.55     | 0.83           | 0.81      | 0.37        | 0.38   |
| 77       | 0.53          | 0.54     | 0.83           | 0.82      | 0.36        | 0.37   |
| 78       | 0.52          | 0.53     | 0.84           | 0.82      | 0.35        | 0.37   |
| 79       | 0.51          | 0.52     | 0.85           | 0.83      | 0.34        | 0.36   |
| 80       | 0.50          | 0.51     | 0.85           | 0.84      | 0.34        | 0.35   |
| 81       | 0.49          | 0.50     | 0.86           | 0.84      | 0.33        | 0.34   |
| 82       | 0.48          | 0.48     | 0.87           | 0.85      | 0.32        | 0.33   |
| 83       | 0.46          | 0.47     | 0.88           | 0.86      | 0.31        | 0.32   |
| 84       | 0.45          | 0.46     | 0.89           | 0.87      | 0.30        | 0.31   |
| 85       | 0.43          | 0.44     | 0.90           | 0.87      | 0.28        | 0.30   |
| 86       | 0.41          | 0.42     | 0.91           | 0.88      | 0.27        | 0.28   |
| 87       | 0.38          | 0.40     | 0.92           | 0.89      | 0.25        | 0.27   |
| 88       | 0.35          | 0.37     | 0.93           | 0.91      | 0.23        | 0.25   |
| 89       | 0.31          | 0.34     | 0.94           | 0.92      | 0.20        | 0.23   |
| 90       | 0.09          | 0.14     | 0.99           | 0.97      | 0.06        | 0.09   |

Table S140: Reference ( $\phi_S$ ,  $\varphi$ ,  $\psi$ ) and approached ( $\phi_S^\ell$ ,  $\varphi^\ell$ ,  $\psi^\ell$ ) values of the topological descriptors for the first excited-state of the pyridinium-phenolate (PP), computed at the PBE0/6-31G level of theory.  $\alpha$  is the pyridinium-phenolate central twist angle amplitude.

| $\alpha$ | $\phi_S^\ell$ | $\phi_S$ | $\varphi^\ell$ | $\varphi$ | $\psi^\ell$ | $\psi$ |
|----------|---------------|----------|----------------|-----------|-------------|--------|
| 0        | 0.63          | 0.68     | 0.70           | 0.66      | 0.47        | 0.51   |
| 1        | 0.63          | 0.68     | 0.70           | 0.66      | 0.47        | 0.51   |
| 2        | 0.63          | 0.68     | 0.70           | 0.66      | 0.47        | 0.51   |
| 3        | 0.63          | 0.68     | 0.70           | 0.66      | 0.47        | 0.51   |
| 4        | 0.63          | 0.68     | 0.70           | 0.66      | 0.47        | 0.51   |
| 5        | 0.63          | 0.68     | 0.70           | 0.66      | 0.47        | 0.51   |
| 6        | 0.63          | 0.68     | 0.70           | 0.67      | 0.47        | 0.50   |
| 7        | 0.63          | 0.67     | 0.70           | 0.67      | 0.47        | 0.50   |
| 8        | 0.63          | 0.67     | 0.70           | 0.67      | 0.47        | 0.50   |
| 9        | 0.63          | 0.67     | 0.71           | 0.67      | 0.46        | 0.50   |
| 10       | 0.62          | 0.67     | 0.71           | 0.67      | 0.46        | 0.50   |
| 11       | 0.62          | 0.67     | 0.71           | 0.67      | 0.46        | 0.50   |
| 12       | 0.62          | 0.67     | 0.71           | 0.67      | 0.46        | 0.50   |
| 13       | 0.62          | 0.67     | 0.71           | 0.67      | 0.46        | 0.50   |
| 14       | 0.62          | 0.67     | 0.71           | 0.68      | 0.46        | 0.50   |
| 15       | 0.62          | 0.66     | 0.71           | 0.68      | 0.46        | 0.49   |
| 16       | 0.62          | 0.66     | 0.72           | 0.68      | 0.45        | 0.49   |
| 17       | 0.62          | 0.66     | 0.72           | 0.68      | 0.45        | 0.49   |
| 18       | 0.61          | 0.66     | 0.72           | 0.69      | 0.45        | 0.49   |
| 19       | 0.61          | 0.66     | 0.72           | 0.69      | 0.45        | 0.49   |
| 20       | 0.61          | 0.65     | 0.73           | 0.69      | 0.44        | 0.48   |
| 21       | 0.61          | 0.65     | 0.73           | 0.69      | 0.44        | 0.48   |
| 22       | 0.60          | 0.65     | 0.73           | 0.70      | 0.44        | 0.48   |
| 23       | 0.60          | 0.65     | 0.73           | 0.70      | 0.44        | 0.48   |
| 24       | 0.60          | 0.64     | 0.74           | 0.70      | 0.43        | 0.47   |
| 25       | 0.60          | 0.64     | 0.74           | 0.71      | 0.43        | 0.47   |
| 26       | 0.59          | 0.64     | 0.74           | 0.71      | 0.43        | 0.47   |
| 27       | 0.59          | 0.63     | 0.75           | 0.71      | 0.42        | 0.46   |
| 28       | 0.59          | 0.63     | 0.75           | 0.72      | 0.42        | 0.46   |
| 29       | 0.59          | 0.63     | 0.75           | 0.72      | 0.42        | 0.46   |
| 30       | 0.58          | 0.62     | 0.76           | 0.72      | 0.41        | 0.45   |
| 31       | 0.58          | 0.62     | 0.76           | 0.73      | 0.41        | 0.45   |

Continued on next page

| $\alpha$ | $\phi_S^\ell$ | $\phi_S$ | $\varphi^\ell$ | $\varphi$ | $\psi^\ell$ | $\psi$ |
|----------|---------------|----------|----------------|-----------|-------------|--------|
| 32       | 0.58          | 0.61     | 0.76           | 0.73      | 0.41        | 0.44   |
| 33       | 0.57          | 0.61     | 0.77           | 0.74      | 0.41        | 0.44   |
| 34       | 0.57          | 0.60     | 0.77           | 0.74      | 0.41        | 0.43   |
| 35       | 0.56          | 0.60     | 0.77           | 0.74      | 0.40        | 0.43   |
| 36       | 0.56          | 0.60     | 0.78           | 0.75      | 0.40        | 0.43   |
| 37       | 0.55          | 0.59     | 0.78           | 0.75      | 0.39        | 0.42   |
| 38       | 0.55          | 0.59     | 0.79           | 0.76      | 0.39        | 0.42   |
| 39       | 0.54          | 0.58     | 0.79           | 0.76      | 0.38        | 0.41   |
| 40       | 0.54          | 0.57     | 0.80           | 0.77      | 0.38        | 0.41   |
| 41       | 0.53          | 0.57     | 0.80           | 0.77      | 0.37        | 0.41   |
| 42       | 0.53          | 0.56     | 0.81           | 0.78      | 0.37        | 0.40   |
| 43       | 0.52          | 0.56     | 0.81           | 0.78      | 0.36        | 0.40   |
| 44       | 0.51          | 0.55     | 0.82           | 0.79      | 0.35        | 0.39   |
| 45       | 0.51          | 0.55     | 0.82           | 0.79      | 0.35        | 0.39   |
| 46       | 0.50          | 0.54     | 0.83           | 0.80      | 0.35        | 0.38   |
| 47       | 0.50          | 0.53     | 0.83           | 0.80      | 0.35        | 0.37   |
| 48       | 0.49          | 0.53     | 0.84           | 0.81      | 0.34        | 0.37   |
| 49       | 0.48          | 0.52     | 0.84           | 0.81      | 0.33        | 0.36   |
| 50       | 0.48          | 0.51     | 0.85           | 0.82      | 0.33        | 0.35   |
| 51       | 0.47          | 0.50     | 0.85           | 0.82      | 0.32        | 0.35   |
| 52       | 0.46          | 0.50     | 0.86           | 0.83      | 0.31        | 0.35   |
| 53       | 0.45          | 0.49     | 0.86           | 0.83      | 0.31        | 0.34   |
| 54       | 0.44          | 0.48     | 0.87           | 0.84      | 0.30        | 0.33   |
| 55       | 0.44          | 0.47     | 0.87           | 0.84      | 0.30        | 0.32   |
| 56       | 0.43          | 0.46     | 0.88           | 0.85      | 0.29        | 0.32   |
| 57       | 0.42          | 0.46     | 0.88           | 0.85      | 0.28        | 0.32   |
| 58       | 0.41          | 0.45     | 0.89           | 0.86      | 0.27        | 0.31   |
| 59       | 0.40          | 0.44     | 0.89           | 0.86      | 0.27        | 0.30   |
| 60       | 0.39          | 0.43     | 0.90           | 0.87      | 0.26        | 0.29   |
| 61       | 0.38          | 0.42     | 0.90           | 0.87      | 0.25        | 0.29   |
| 62       | 0.37          | 0.41     | 0.91           | 0.88      | 0.25        | 0.28   |
| 63       | 0.36          | 0.40     | 0.91           | 0.88      | 0.24        | 0.27   |

Continued on next page

| $\alpha$ | $\phi_S^\ell$ | $\phi_S$ | $\varphi^\ell$ | $\varphi$ | $\psi^\ell$ | $\psi$ |
|----------|---------------|----------|----------------|-----------|-------------|--------|
| 64       | 0.35          | 0.39     | 0.92           | 0.89      | 0.23        | 0.26   |
| 65       | 0.34          | 0.38     | 0.92           | 0.89      | 0.23        | 0.26   |
| 66       | 0.33          | 0.37     | 0.93           | 0.90      | 0.22        | 0.25   |
| 67       | 0.32          | 0.36     | 0.93           | 0.90      | 0.21        | 0.24   |
| 68       | 0.31          | 0.35     | 0.94           | 0.90      | 0.20        | 0.24   |
| 69       | 0.30          | 0.34     | 0.94           | 0.91      | 0.20        | 0.23   |
| 70       | 0.29          | 0.33     | 0.94           | 0.91      | 0.19        | 0.22   |
| 71       | 0.28          | 0.32     | 0.95           | 0.92      | 0.18        | 0.21   |
| 72       | 0.27          | 0.31     | 0.95           | 0.92      | 0.18        | 0.21   |
| 73       | 0.26          | 0.30     | 0.96           | 0.92      | 0.17        | 0.20   |
| 74       | 0.24          | 0.29     | 0.96           | 0.93      | 0.16        | 0.19   |
| 75       | 0.23          | 0.28     | 0.96           | 0.93      | 0.15        | 0.19   |
| 76       | 0.22          | 0.27     | 0.97           | 0.93      | 0.14        | 0.18   |
| 77       | 0.21          | 0.26     | 0.97           | 0.94      | 0.14        | 0.17   |
| 78       | 0.20          | 0.25     | 0.97           | 0.94      | 0.13        | 0.17   |
| 79       | 0.19          | 0.24     | 0.97           | 0.94      | 0.12        | 0.16   |
| 80       | 0.18          | 0.23     | 0.97           | 0.94      | 0.12        | 0.15   |
| 81       | 0.18          | 0.22     | 0.98           | 0.95      | 0.12        | 0.14   |
| 82       | 0.17          | 0.22     | 0.98           | 0.95      | 0.11        | 0.14   |
| 83       | 0.16          | 0.21     | 0.98           | 0.95      | 0.10        | 0.14   |
| 84       | 0.15          | 0.20     | 0.98           | 0.95      | 0.10        | 0.13   |
| 85       | 0.14          | 0.19     | 0.98           | 0.95      | 0.09        | 0.13   |
| 86       | 0.13          | 0.19     | 0.98           | 0.95      | 0.08        | 0.13   |
| 87       | 0.13          | 0.18     | 0.98           | 0.95      | 0.08        | 0.12   |
| 88       | 0.12          | 0.18     | 0.98           | 0.95      | 0.08        | 0.12   |
| 89       | 0.12          | 0.17     | 0.98           | 0.95      | 0.08        | 0.11   |
| 90       | 0.12          | 0.17     | 0.98           | 0.95      | 0.08        | 0.11   |

Table S141: Reference ( $\phi_S$ ,  $\varphi$ ,  $\psi$ ) and approached ( $\phi_S^\ell$ ,  $\varphi^\ell$ ,  $\psi^\ell$ ) values of the topological descriptors for the first excited-state of the pyridinium-phenolate (PP), computed at the TDHF/3-21G level of theory.  $\alpha$  is the pyridinium-phenolate central twist angle amplitude.



| $\alpha$ | $\phi_S^\ell$ | $\phi_S$ | $\varphi^\ell$ | $\varphi$ | $\psi^\ell$ | $\psi$ |
|----------|---------------|----------|----------------|-----------|-------------|--------|
| 0        | 0.63          | 0.67     | 0.69           | 0.66      | 0.47        | 0.50   |
| 1        | 0.63          | 0.67     | 0.69           | 0.66      | 0.47        | 0.50   |
| 2        | 0.63          | 0.67     | 0.69           | 0.66      | 0.47        | 0.50   |
| 3        | 0.63          | 0.67     | 0.69           | 0.66      | 0.47        | 0.50   |
| 4        | 0.63          | 0.67     | 0.69           | 0.66      | 0.47        | 0.50   |
| 5        | 0.63          | 0.67     | 0.69           | 0.66      | 0.47        | 0.50   |
| 6        | 0.62          | 0.66     | 0.69           | 0.66      | 0.47        | 0.50   |
| 7        | 0.62          | 0.66     | 0.69           | 0.67      | 0.47        | 0.50   |
| 8        | 0.62          | 0.66     | 0.69           | 0.67      | 0.47        | 0.50   |
| 9        | 0.62          | 0.66     | 0.69           | 0.67      | 0.47        | 0.50   |
| 10       | 0.62          | 0.66     | 0.69           | 0.67      | 0.47        | 0.50   |
| 11       | 0.62          | 0.66     | 0.69           | 0.67      | 0.47        | 0.50   |
| 12       | 0.62          | 0.66     | 0.70           | 0.67      | 0.46        | 0.50   |
| 13       | 0.62          | 0.66     | 0.70           | 0.67      | 0.46        | 0.50   |
| 14       | 0.62          | 0.65     | 0.70           | 0.68      | 0.46        | 0.49   |
| 15       | 0.61          | 0.65     | 0.70           | 0.68      | 0.46        | 0.49   |
| 16       | 0.61          | 0.65     | 0.70           | 0.68      | 0.46        | 0.49   |
| 17       | 0.61          | 0.65     | 0.71           | 0.68      | 0.45        | 0.49   |
| 18       | 0.61          | 0.65     | 0.71           | 0.68      | 0.45        | 0.49   |
| 19       | 0.61          | 0.64     | 0.71           | 0.69      | 0.45        | 0.48   |
| 20       | 0.60          | 0.64     | 0.71           | 0.69      | 0.45        | 0.48   |
| 21       | 0.60          | 0.64     | 0.72           | 0.69      | 0.44        | 0.48   |
| 22       | 0.60          | 0.64     | 0.72           | 0.69      | 0.44        | 0.48   |
| 23       | 0.60          | 0.63     | 0.72           | 0.70      | 0.44        | 0.47   |
| 24       | 0.59          | 0.63     | 0.73           | 0.70      | 0.43        | 0.47   |
| 25       | 0.59          | 0.63     | 0.73           | 0.70      | 0.43        | 0.47   |
| 26       | 0.59          | 0.63     | 0.73           | 0.71      | 0.43        | 0.46   |
| 27       | 0.58          | 0.62     | 0.74           | 0.71      | 0.42        | 0.46   |
| 28       | 0.58          | 0.62     | 0.74           | 0.71      | 0.42        | 0.46   |
| 29       | 0.58          | 0.61     | 0.74           | 0.72      | 0.42        | 0.45   |
| 30       | 0.57          | 0.61     | 0.75           | 0.72      | 0.41        | 0.45   |
| 31       | 0.57          | 0.61     | 0.75           | 0.73      | 0.41        | 0.44   |

Continued on next page

| $\alpha$ | $\phi_S^\ell$ | $\phi_S$ | $\varphi^\ell$ | $\varphi$ | $\psi^\ell$ | $\psi$ |
|----------|---------------|----------|----------------|-----------|-------------|--------|
| 32       | 0.57          | 0.60     | 0.75           | 0.73      | 0.41        | 0.44   |
| 33       | 0.56          | 0.60     | 0.76           | 0.73      | 0.40        | 0.44   |
| 34       | 0.56          | 0.59     | 0.76           | 0.74      | 0.40        | 0.43   |
| 35       | 0.55          | 0.59     | 0.77           | 0.74      | 0.39        | 0.43   |
| 36       | 0.55          | 0.59     | 0.77           | 0.75      | 0.39        | 0.42   |
| 37       | 0.54          | 0.58     | 0.77           | 0.75      | 0.39        | 0.42   |
| 38       | 0.54          | 0.58     | 0.78           | 0.76      | 0.39        | 0.41   |
| 39       | 0.53          | 0.57     | 0.78           | 0.76      | 0.38        | 0.41   |
| 40       | 0.53          | 0.56     | 0.79           | 0.76      | 0.38        | 0.40   |
| 41       | 0.52          | 0.56     | 0.79           | 0.77      | 0.37        | 0.40   |
| 42       | 0.51          | 0.55     | 0.80           | 0.77      | 0.36        | 0.39   |
| 43       | 0.51          | 0.55     | 0.80           | 0.78      | 0.36        | 0.39   |
| 44       | 0.50          | 0.54     | 0.81           | 0.78      | 0.35        | 0.39   |
| 45       | 0.50          | 0.54     | 0.81           | 0.79      | 0.35        | 0.38   |
| 46       | 0.49          | 0.53     | 0.82           | 0.79      | 0.34        | 0.38   |
| 47       | 0.48          | 0.52     | 0.82           | 0.80      | 0.34        | 0.37   |
| 48       | 0.48          | 0.52     | 0.83           | 0.80      | 0.33        | 0.37   |
| 49       | 0.47          | 0.51     | 0.83           | 0.81      | 0.33        | 0.36   |
| 50       | 0.46          | 0.50     | 0.84           | 0.81      | 0.32        | 0.35   |
| 51       | 0.46          | 0.49     | 0.84           | 0.82      | 0.32        | 0.34   |
| 52       | 0.45          | 0.49     | 0.85           | 0.82      | 0.31        | 0.34   |
| 53       | 0.44          | 0.48     | 0.85           | 0.83      | 0.30        | 0.33   |
| 54       | 0.44          | 0.47     | 0.86           | 0.83      | 0.30        | 0.33   |
| 55       | 0.43          | 0.46     | 0.86           | 0.84      | 0.30        | 0.32   |
| 56       | 0.42          | 0.46     | 0.87           | 0.85      | 0.29        | 0.32   |
| 57       | 0.42          | 0.45     | 0.87           | 0.85      | 0.29        | 0.31   |
| 58       | 0.41          | 0.44     | 0.88           | 0.85      | 0.28        | 0.30   |
| 59       | 0.40          | 0.43     | 0.88           | 0.86      | 0.27        | 0.30   |
| 60       | 0.39          | 0.42     | 0.89           | 0.86      | 0.26        | 0.29   |
| 61       | 0.39          | 0.41     | 0.89           | 0.87      | 0.26        | 0.28   |
| 62       | 0.38          | 0.40     | 0.90           | 0.87      | 0.25        | 0.27   |
| 63       | 0.37          | 0.40     | 0.90           | 0.88      | 0.25        | 0.27   |

Continued on next page

| $\alpha$ | $\phi_S^\ell$ | $\phi_S$ | $\varphi^\ell$ | $\varphi$ | $\psi^\ell$ | $\psi$ |
|----------|---------------|----------|----------------|-----------|-------------|--------|
| 64       | 0.36          | 0.39     | 0.91           | 0.88      | 0.24        | 0.27   |
| 65       | 0.35          | 0.38     | 0.91           | 0.89      | 0.23        | 0.26   |
| 66       | 0.34          | 0.37     | 0.91           | 0.89      | 0.23        | 0.25   |
| 67       | 0.34          | 0.36     | 0.92           | 0.90      | 0.23        | 0.24   |
| 68       | 0.33          | 0.35     | 0.92           | 0.90      | 0.22        | 0.24   |
| 69       | 0.32          | 0.34     | 0.92           | 0.90      | 0.21        | 0.23   |
| 70       | 0.31          | 0.33     | 0.93           | 0.91      | 0.20        | 0.22   |
| 71       | 0.30          | 0.32     | 0.93           | 0.91      | 0.20        | 0.22   |
| 72       | 0.29          | 0.31     | 0.93           | 0.91      | 0.19        | 0.21   |
| 73       | 0.28          | 0.30     | 0.94           | 0.92      | 0.18        | 0.20   |
| 74       | 0.27          | 0.29     | 0.94           | 0.92      | 0.18        | 0.19   |
| 75       | 0.26          | 0.28     | 0.94           | 0.92      | 0.17        | 0.19   |
| 76       | 0.25          | 0.28     | 0.94           | 0.93      | 0.17        | 0.19   |
| 77       | 0.24          | 0.27     | 0.95           | 0.93      | 0.16        | 0.18   |
| 78       | 0.24          | 0.26     | 0.95           | 0.93      | 0.16        | 0.17   |
| 79       | 0.23          | 0.25     | 0.95           | 0.93      | 0.15        | 0.17   |
| 80       | 0.22          | 0.24     | 0.95           | 0.94      | 0.14        | 0.16   |
| 81       | 0.21          | 0.23     | 0.95           | 0.94      | 0.14        | 0.15   |
| 82       | 0.20          | 0.22     | 0.95           | 0.94      | 0.13        | 0.15   |
| 83       | 0.20          | 0.22     | 0.96           | 0.94      | 0.13        | 0.15   |
| 84       | 0.19          | 0.21     | 0.96           | 0.94      | 0.12        | 0.14   |
| 85       | 0.18          | 0.20     | 0.96           | 0.94      | 0.12        | 0.13   |
| 86       | 0.18          | 0.20     | 0.96           | 0.95      | 0.12        | 0.13   |
| 87       | 0.17          | 0.19     | 0.96           | 0.95      | 0.11        | 0.13   |
| 88       | 0.17          | 0.19     | 0.96           | 0.95      | 0.11        | 0.13   |
| 89       | 0.17          | 0.19     | 0.96           | 0.95      | 0.11        | 0.13   |
| 90       | 0.17          | 0.18     | 0.96           | 0.95      | 0.11        | 0.12   |

Table S142: Reference ( $\phi_S$ ,  $\varphi$ ,  $\psi$ ) and approached ( $\phi_S^\ell$ ,  $\varphi^\ell$ ,  $\psi^\ell$ ) values of the topological descriptors for the first excited-state of the pyridinium-phenolate (PP), computed at the TDHF/6-311++G(2d,p) level of theory.  $\alpha$  is the pyridinium-phenolate central twist angle amplitude.

| $\alpha$ | $\phi_S^\ell$ | $\phi_S$ | $\varphi^\ell$ | $\varphi$ | $\psi^\ell$ | $\psi$ |
|----------|---------------|----------|----------------|-----------|-------------|--------|
| 0        | 0.62          | 0.66     | 0.69           | 0.67      | 0.47        | 0.50   |
| 1        | 0.62          | 0.66     | 0.69           | 0.67      | 0.47        | 0.50   |
| 2        | 0.62          | 0.66     | 0.69           | 0.67      | 0.47        | 0.50   |
| 3        | 0.62          | 0.66     | 0.69           | 0.67      | 0.47        | 0.50   |
| 4        | 0.62          | 0.66     | 0.69           | 0.67      | 0.47        | 0.50   |
| 5        | 0.62          | 0.66     | 0.69           | 0.67      | 0.47        | 0.50   |
| 6        | 0.62          | 0.66     | 0.70           | 0.67      | 0.46        | 0.50   |
| 7        | 0.61          | 0.66     | 0.70           | 0.67      | 0.46        | 0.50   |
| 8        | 0.61          | 0.66     | 0.70           | 0.67      | 0.46        | 0.50   |
| 9        | 0.61          | 0.66     | 0.70           | 0.67      | 0.46        | 0.50   |
| 10       | 0.61          | 0.66     | 0.70           | 0.67      | 0.46        | 0.50   |
| 11       | 0.61          | 0.66     | 0.70           | 0.67      | 0.46        | 0.50   |
| 12       | 0.61          | 0.65     | 0.70           | 0.68      | 0.46        | 0.49   |
| 13       | 0.61          | 0.65     | 0.70           | 0.68      | 0.46        | 0.49   |
| 14       | 0.61          | 0.65     | 0.70           | 0.68      | 0.46        | 0.49   |
| 15       | 0.61          | 0.65     | 0.71           | 0.68      | 0.45        | 0.49   |
| 16       | 0.60          | 0.65     | 0.71           | 0.68      | 0.45        | 0.49   |
| 17       | 0.60          | 0.65     | 0.71           | 0.69      | 0.45        | 0.48   |
| 18       | 0.60          | 0.64     | 0.71           | 0.69      | 0.45        | 0.48   |
| 19       | 0.60          | 0.64     | 0.72           | 0.69      | 0.44        | 0.48   |
| 20       | 0.60          | 0.64     | 0.72           | 0.69      | 0.44        | 0.48   |
| 21       | 0.59          | 0.64     | 0.72           | 0.70      | 0.44        | 0.47   |
| 22       | 0.59          | 0.63     | 0.72           | 0.70      | 0.44        | 0.47   |
| 23       | 0.59          | 0.63     | 0.73           | 0.70      | 0.43        | 0.47   |
| 24       | 0.58          | 0.63     | 0.73           | 0.71      | 0.43        | 0.46   |
| 25       | 0.58          | 0.63     | 0.73           | 0.71      | 0.43        | 0.46   |
| 26       | 0.58          | 0.62     | 0.74           | 0.71      | 0.42        | 0.46   |
| 27       | 0.58          | 0.62     | 0.74           | 0.72      | 0.42        | 0.45   |
| 28       | 0.57          | 0.62     | 0.74           | 0.72      | 0.42        | 0.45   |
| 29       | 0.57          | 0.61     | 0.75           | 0.72      | 0.41        | 0.45   |
| 30       | 0.57          | 0.61     | 0.75           | 0.73      | 0.41        | 0.44   |
| 31       | 0.56          | 0.60     | 0.75           | 0.73      | 0.41        | 0.44   |

Continued on next page

| $\alpha$ | $\phi_S^\ell$ | $\phi_S$ | $\varphi^\ell$ | $\varphi$ | $\psi^\ell$ | $\psi$ |
|----------|---------------|----------|----------------|-----------|-------------|--------|
| 32       | 0.56          | 0.60     | 0.76           | 0.73      | 0.40        | 0.44   |
| 33       | 0.55          | 0.60     | 0.76           | 0.74      | 0.40        | 0.43   |
| 34       | 0.55          | 0.59     | 0.77           | 0.74      | 0.39        | 0.43   |
| 35       | 0.55          | 0.59     | 0.77           | 0.75      | 0.39        | 0.42   |
| 36       | 0.54          | 0.58     | 0.77           | 0.75      | 0.39        | 0.42   |
| 37       | 0.54          | 0.58     | 0.78           | 0.75      | 0.39        | 0.42   |
| 38       | 0.53          | 0.57     | 0.78           | 0.76      | 0.38        | 0.41   |
| 39       | 0.52          | 0.57     | 0.79           | 0.76      | 0.37        | 0.41   |
| 40       | 0.52          | 0.56     | 0.79           | 0.77      | 0.37        | 0.40   |
| 41       | 0.51          | 0.56     | 0.80           | 0.77      | 0.36        | 0.40   |
| 42       | 0.51          | 0.55     | 0.80           | 0.78      | 0.36        | 0.39   |
| 43       | 0.50          | 0.54     | 0.81           | 0.78      | 0.35        | 0.39   |
| 44       | 0.50          | 0.54     | 0.81           | 0.79      | 0.35        | 0.38   |
| 45       | 0.49          | 0.53     | 0.82           | 0.79      | 0.34        | 0.38   |
| 46       | 0.48          | 0.53     | 0.82           | 0.80      | 0.34        | 0.37   |
| 47       | 0.48          | 0.52     | 0.83           | 0.80      | 0.33        | 0.37   |
| 48       | 0.47          | 0.51     | 0.83           | 0.81      | 0.33        | 0.36   |
| 49       | 0.46          | 0.51     | 0.84           | 0.81      | 0.32        | 0.36   |
| 50       | 0.46          | 0.50     | 0.84           | 0.82      | 0.32        | 0.35   |
| 51       | 0.45          | 0.49     | 0.85           | 0.82      | 0.31        | 0.34   |
| 52       | 0.44          | 0.48     | 0.85           | 0.83      | 0.30        | 0.33   |
| 53       | 0.44          | 0.48     | 0.85           | 0.83      | 0.30        | 0.33   |
| 54       | 0.43          | 0.47     | 0.86           | 0.84      | 0.30        | 0.32   |
| 55       | 0.42          | 0.46     | 0.86           | 0.84      | 0.29        | 0.32   |
| 56       | 0.41          | 0.45     | 0.87           | 0.85      | 0.28        | 0.31   |
| 57       | 0.41          | 0.44     | 0.88           | 0.85      | 0.28        | 0.30   |
| 58       | 0.40          | 0.44     | 0.88           | 0.86      | 0.27        | 0.30   |
| 59       | 0.39          | 0.43     | 0.89           | 0.86      | 0.26        | 0.30   |
| 60       | 0.38          | 0.42     | 0.89           | 0.87      | 0.26        | 0.29   |
| 61       | 0.37          | 0.41     | 0.90           | 0.87      | 0.25        | 0.28   |
| 62       | 0.37          | 0.40     | 0.90           | 0.88      | 0.25        | 0.27   |
| 63       | 0.36          | 0.39     | 0.91           | 0.88      | 0.24        | 0.27   |

Continued on next page

| $\alpha$ | $\phi_S^\ell$ | $\phi_S$ | $\varphi^\ell$ | $\varphi$ | $\psi^\ell$ | $\psi$ |
|----------|---------------|----------|----------------|-----------|-------------|--------|
| 64       | 0.35          | 0.38     | 0.91           | 0.89      | 0.23        | 0.26   |
| 65       | 0.34          | 0.37     | 0.92           | 0.89      | 0.23        | 0.25   |
| 66       | 0.33          | 0.37     | 0.92           | 0.89      | 0.22        | 0.25   |
| 67       | 0.32          | 0.36     | 0.92           | 0.90      | 0.21        | 0.24   |
| 68       | 0.31          | 0.35     | 0.93           | 0.90      | 0.20        | 0.24   |
| 69       | 0.30          | 0.34     | 0.93           | 0.91      | 0.20        | 0.23   |
| 70       | 0.29          | 0.33     | 0.94           | 0.91      | 0.19        | 0.22   |
| 71       | 0.28          | 0.32     | 0.94           | 0.91      | 0.18        | 0.22   |
| 72       | 0.28          | 0.31     | 0.94           | 0.92      | 0.18        | 0.21   |
| 73       | 0.27          | 0.30     | 0.95           | 0.92      | 0.18        | 0.20   |
| 74       | 0.26          | 0.29     | 0.95           | 0.92      | 0.17        | 0.19   |
| 75       | 0.25          | 0.28     | 0.95           | 0.93      | 0.16        | 0.19   |
| 76       | 0.24          | 0.27     | 0.95           | 0.93      | 0.16        | 0.18   |
| 77       | 0.23          | 0.26     | 0.96           | 0.93      | 0.15        | 0.17   |
| 78       | 0.22          | 0.26     | 0.96           | 0.93      | 0.14        | 0.17   |
| 79       | 0.21          | 0.25     | 0.96           | 0.94      | 0.14        | 0.17   |
| 80       | 0.21          | 0.24     | 0.96           | 0.94      | 0.14        | 0.16   |
| 81       | 0.20          | 0.23     | 0.96           | 0.94      | 0.13        | 0.15   |
| 82       | 0.19          | 0.22     | 0.97           | 0.94      | 0.12        | 0.15   |
| 83       | 0.19          | 0.21     | 0.97           | 0.94      | 0.12        | 0.14   |
| 84       | 0.18          | 0.21     | 0.97           | 0.94      | 0.12        | 0.14   |
| 85       | 0.17          | 0.20     | 0.97           | 0.95      | 0.11        | 0.13   |
| 86       | 0.17          | 0.20     | 0.97           | 0.95      | 0.11        | 0.13   |
| 87       | 0.16          | 0.19     | 0.97           | 0.95      | 0.10        | 0.13   |
| 88       | 0.16          | 0.19     | 0.97           | 0.95      | 0.10        | 0.13   |
| 89       | 0.15          | 0.18     | 0.97           | 0.95      | 0.10        | 0.12   |
| 90       | 0.15          | 0.18     | 0.97           | 0.95      | 0.10        | 0.12   |

Table S143: Reference ( $\phi_S$ ,  $\varphi$ ,  $\psi$ ) and approached ( $\phi_S^\ell$ ,  $\varphi^\ell$ ,  $\psi^\ell$ ) values of the topological descriptors for the first excited-state of the pyridinium-phenolate (PP), computed at the TDHF/6-311++G(d,p) level of theory.  $\alpha$  is the pyridinium-phenolate central twist angle amplitude.

| $\alpha$ | $\phi_S^\ell$ | $\phi_S$ | $\varphi^\ell$ | $\varphi$ | $\psi^\ell$ | $\psi$ |
|----------|---------------|----------|----------------|-----------|-------------|--------|
| 0        | 0.62          | 0.66     | 0.69           | 0.67      | 0.47        | 0.50   |
| 1        | 0.62          | 0.66     | 0.69           | 0.67      | 0.47        | 0.50   |
| 2        | 0.62          | 0.66     | 0.69           | 0.67      | 0.47        | 0.50   |
| 3        | 0.62          | 0.66     | 0.69           | 0.67      | 0.47        | 0.50   |
| 4        | 0.62          | 0.66     | 0.69           | 0.67      | 0.47        | 0.50   |
| 5        | 0.62          | 0.66     | 0.69           | 0.67      | 0.47        | 0.50   |
| 6        | 0.62          | 0.66     | 0.69           | 0.67      | 0.47        | 0.50   |
| 7        | 0.61          | 0.66     | 0.70           | 0.67      | 0.46        | 0.50   |
| 8        | 0.61          | 0.66     | 0.70           | 0.67      | 0.46        | 0.50   |
| 9        | 0.61          | 0.66     | 0.70           | 0.67      | 0.46        | 0.50   |
| 10       | 0.61          | 0.66     | 0.70           | 0.67      | 0.46        | 0.50   |
| 11       | 0.61          | 0.66     | 0.70           | 0.67      | 0.46        | 0.50   |
| 12       | 0.61          | 0.65     | 0.70           | 0.68      | 0.46        | 0.49   |
| 13       | 0.61          | 0.65     | 0.70           | 0.68      | 0.46        | 0.49   |
| 14       | 0.61          | 0.65     | 0.70           | 0.68      | 0.46        | 0.49   |
| 15       | 0.61          | 0.65     | 0.71           | 0.68      | 0.45        | 0.49   |
| 16       | 0.60          | 0.65     | 0.71           | 0.68      | 0.45        | 0.49   |
| 17       | 0.60          | 0.65     | 0.71           | 0.69      | 0.45        | 0.48   |
| 18       | 0.60          | 0.64     | 0.71           | 0.69      | 0.45        | 0.48   |
| 19       | 0.60          | 0.64     | 0.72           | 0.69      | 0.44        | 0.48   |
| 20       | 0.60          | 0.64     | 0.72           | 0.69      | 0.44        | 0.48   |
| 21       | 0.59          | 0.64     | 0.72           | 0.70      | 0.44        | 0.47   |
| 22       | 0.59          | 0.63     | 0.72           | 0.70      | 0.44        | 0.47   |
| 23       | 0.59          | 0.63     | 0.73           | 0.70      | 0.43        | 0.47   |
| 24       | 0.58          | 0.63     | 0.73           | 0.71      | 0.43        | 0.46   |
| 25       | 0.58          | 0.63     | 0.73           | 0.71      | 0.43        | 0.46   |
| 26       | 0.58          | 0.62     | 0.74           | 0.71      | 0.42        | 0.46   |
| 27       | 0.58          | 0.62     | 0.74           | 0.72      | 0.42        | 0.45   |
| 28       | 0.57          | 0.62     | 0.74           | 0.72      | 0.42        | 0.45   |
| 29       | 0.57          | 0.61     | 0.75           | 0.72      | 0.41        | 0.45   |
| 30       | 0.57          | 0.61     | 0.75           | 0.73      | 0.41        | 0.44   |
| 31       | 0.56          | 0.60     | 0.75           | 0.73      | 0.41        | 0.44   |

Continued on next page

| $\alpha$ | $\phi_S^\ell$ | $\phi_S$ | $\varphi^\ell$ | $\varphi$ | $\psi^\ell$ | $\psi$ |
|----------|---------------|----------|----------------|-----------|-------------|--------|
| 32       | 0.56          | 0.60     | 0.76           | 0.73      | 0.40        | 0.44   |
| 33       | 0.55          | 0.60     | 0.76           | 0.74      | 0.40        | 0.43   |
| 34       | 0.55          | 0.59     | 0.77           | 0.74      | 0.39        | 0.43   |
| 35       | 0.55          | 0.59     | 0.77           | 0.75      | 0.39        | 0.42   |
| 36       | 0.54          | 0.58     | 0.77           | 0.75      | 0.39        | 0.42   |
| 37       | 0.54          | 0.58     | 0.78           | 0.75      | 0.39        | 0.42   |
| 38       | 0.53          | 0.57     | 0.78           | 0.76      | 0.38        | 0.41   |
| 39       | 0.53          | 0.57     | 0.79           | 0.76      | 0.38        | 0.41   |
| 40       | 0.52          | 0.56     | 0.79           | 0.77      | 0.37        | 0.40   |
| 41       | 0.51          | 0.56     | 0.80           | 0.77      | 0.36        | 0.40   |
| 42       | 0.51          | 0.55     | 0.80           | 0.78      | 0.36        | 0.39   |
| 43       | 0.50          | 0.54     | 0.81           | 0.78      | 0.35        | 0.39   |
| 44       | 0.50          | 0.54     | 0.81           | 0.79      | 0.35        | 0.38   |
| 45       | 0.49          | 0.53     | 0.82           | 0.79      | 0.34        | 0.38   |
| 46       | 0.48          | 0.53     | 0.82           | 0.80      | 0.34        | 0.37   |
| 47       | 0.48          | 0.52     | 0.83           | 0.80      | 0.33        | 0.37   |
| 48       | 0.47          | 0.51     | 0.83           | 0.81      | 0.33        | 0.36   |
| 49       | 0.46          | 0.51     | 0.84           | 0.81      | 0.32        | 0.36   |
| 50       | 0.46          | 0.50     | 0.84           | 0.82      | 0.32        | 0.35   |
| 51       | 0.45          | 0.49     | 0.85           | 0.82      | 0.31        | 0.34   |
| 52       | 0.44          | 0.48     | 0.85           | 0.83      | 0.30        | 0.33   |
| 53       | 0.44          | 0.48     | 0.85           | 0.83      | 0.30        | 0.33   |
| 54       | 0.43          | 0.47     | 0.86           | 0.84      | 0.30        | 0.32   |
| 55       | 0.42          | 0.46     | 0.86           | 0.84      | 0.29        | 0.32   |
| 56       | 0.42          | 0.45     | 0.87           | 0.85      | 0.29        | 0.31   |
| 57       | 0.41          | 0.44     | 0.88           | 0.85      | 0.28        | 0.30   |
| 58       | 0.40          | 0.44     | 0.88           | 0.86      | 0.27        | 0.30   |
| 59       | 0.39          | 0.43     | 0.89           | 0.86      | 0.26        | 0.30   |
| 60       | 0.38          | 0.42     | 0.89           | 0.87      | 0.26        | 0.29   |
| 61       | 0.38          | 0.41     | 0.90           | 0.87      | 0.25        | 0.28   |
| 62       | 0.37          | 0.40     | 0.90           | 0.88      | 0.25        | 0.27   |
| 63       | 0.36          | 0.39     | 0.91           | 0.88      | 0.24        | 0.27   |

Continued on next page



| $\alpha$ | $\phi_S^\ell$ | $\phi_S$ | $\varphi^\ell$ | $\varphi$ | $\psi^\ell$ | $\psi$ |
|----------|---------------|----------|----------------|-----------|-------------|--------|
| 64       | 0.35          | 0.38     | 0.91           | 0.89      | 0.23        | 0.26   |
| 65       | 0.34          | 0.37     | 0.92           | 0.89      | 0.23        | 0.25   |
| 66       | 0.33          | 0.37     | 0.92           | 0.89      | 0.22        | 0.25   |
| 67       | 0.32          | 0.36     | 0.92           | 0.90      | 0.21        | 0.24   |
| 68       | 0.31          | 0.35     | 0.93           | 0.90      | 0.20        | 0.24   |
| 69       | 0.30          | 0.34     | 0.93           | 0.91      | 0.20        | 0.23   |
| 70       | 0.30          | 0.33     | 0.94           | 0.91      | 0.20        | 0.22   |
| 71       | 0.29          | 0.32     | 0.94           | 0.91      | 0.19        | 0.22   |
| 72       | 0.28          | 0.31     | 0.94           | 0.92      | 0.18        | 0.21   |
| 73       | 0.27          | 0.30     | 0.95           | 0.92      | 0.18        | 0.20   |
| 74       | 0.26          | 0.29     | 0.95           | 0.92      | 0.17        | 0.19   |
| 75       | 0.25          | 0.28     | 0.95           | 0.93      | 0.16        | 0.19   |
| 76       | 0.24          | 0.27     | 0.95           | 0.93      | 0.16        | 0.18   |
| 77       | 0.23          | 0.26     | 0.96           | 0.93      | 0.15        | 0.17   |
| 78       | 0.22          | 0.26     | 0.96           | 0.93      | 0.14        | 0.17   |
| 79       | 0.22          | 0.25     | 0.96           | 0.94      | 0.14        | 0.17   |
| 80       | 0.21          | 0.24     | 0.96           | 0.94      | 0.14        | 0.16   |
| 81       | 0.20          | 0.23     | 0.96           | 0.94      | 0.13        | 0.15   |
| 82       | 0.19          | 0.22     | 0.96           | 0.94      | 0.12        | 0.15   |
| 83       | 0.19          | 0.21     | 0.97           | 0.94      | 0.12        | 0.14   |
| 84       | 0.18          | 0.21     | 0.97           | 0.94      | 0.12        | 0.14   |
| 85       | 0.17          | 0.20     | 0.97           | 0.95      | 0.11        | 0.13   |
| 86       | 0.17          | 0.20     | 0.97           | 0.95      | 0.11        | 0.13   |
| 87       | 0.16          | 0.19     | 0.97           | 0.95      | 0.10        | 0.13   |
| 88       | 0.16          | 0.19     | 0.97           | 0.95      | 0.10        | 0.13   |
| 89       | 0.15          | 0.18     | 0.97           | 0.95      | 0.10        | 0.12   |
| 90       | 0.15          | 0.18     | 0.97           | 0.95      | 0.10        | 0.12   |

Table S144: Reference ( $\phi_S$ ,  $\varphi$ ,  $\psi$ ) and approached ( $\phi_S^\ell$ ,  $\varphi^\ell$ ,  $\psi^\ell$ ) values of the topological descriptors for the first excited-state of the pyridinium-phenolate (PP), computed at the TDHF/6-311+G(d,p) level of theory.  $\alpha$  is the pyridinium-phenolate central twist angle amplitude.

| $\alpha$ | $\phi_S^\ell$ | $\phi_S$ | $\varphi^\ell$ | $\varphi$ | $\psi^\ell$ | $\psi$ |
|----------|---------------|----------|----------------|-----------|-------------|--------|
| 0        | 0.62          | 0.66     | 0.69           | 0.67      | 0.47        | 0.50   |
| 1        | 0.62          | 0.66     | 0.69           | 0.67      | 0.47        | 0.50   |
| 2        | 0.62          | 0.66     | 0.69           | 0.67      | 0.47        | 0.50   |
| 3        | 0.62          | 0.66     | 0.69           | 0.67      | 0.47        | 0.50   |
| 4        | 0.62          | 0.66     | 0.69           | 0.67      | 0.47        | 0.50   |
| 5        | 0.62          | 0.66     | 0.69           | 0.67      | 0.47        | 0.50   |
| 6        | 0.62          | 0.66     | 0.70           | 0.67      | 0.46        | 0.50   |
| 7        | 0.61          | 0.66     | 0.70           | 0.67      | 0.46        | 0.50   |
| 8        | 0.61          | 0.66     | 0.70           | 0.67      | 0.46        | 0.50   |
| 9        | 0.61          | 0.66     | 0.70           | 0.67      | 0.46        | 0.50   |
| 10       | 0.61          | 0.66     | 0.70           | 0.67      | 0.46        | 0.50   |
| 11       | 0.61          | 0.66     | 0.70           | 0.68      | 0.46        | 0.49   |
| 12       | 0.61          | 0.65     | 0.70           | 0.68      | 0.46        | 0.49   |
| 13       | 0.61          | 0.65     | 0.70           | 0.68      | 0.46        | 0.49   |
| 14       | 0.61          | 0.65     | 0.70           | 0.68      | 0.46        | 0.49   |
| 15       | 0.61          | 0.65     | 0.71           | 0.68      | 0.45        | 0.49   |
| 16       | 0.60          | 0.65     | 0.71           | 0.68      | 0.45        | 0.49   |
| 17       | 0.60          | 0.64     | 0.71           | 0.69      | 0.45        | 0.48   |
| 18       | 0.60          | 0.64     | 0.71           | 0.69      | 0.45        | 0.48   |
| 19       | 0.60          | 0.64     | 0.72           | 0.69      | 0.44        | 0.48   |
| 20       | 0.60          | 0.64     | 0.72           | 0.69      | 0.44        | 0.48   |
| 21       | 0.59          | 0.64     | 0.72           | 0.70      | 0.44        | 0.47   |
| 22       | 0.59          | 0.63     | 0.72           | 0.70      | 0.44        | 0.47   |
| 23       | 0.59          | 0.63     | 0.73           | 0.70      | 0.43        | 0.47   |
| 24       | 0.58          | 0.63     | 0.73           | 0.71      | 0.43        | 0.46   |
| 25       | 0.58          | 0.62     | 0.73           | 0.71      | 0.43        | 0.46   |
| 26       | 0.58          | 0.62     | 0.74           | 0.71      | 0.42        | 0.46   |
| 27       | 0.58          | 0.62     | 0.74           | 0.72      | 0.42        | 0.45   |
| 28       | 0.57          | 0.61     | 0.74           | 0.72      | 0.42        | 0.45   |
| 29       | 0.57          | 0.61     | 0.75           | 0.72      | 0.41        | 0.45   |
| 30       | 0.57          | 0.61     | 0.75           | 0.73      | 0.41        | 0.44   |
| 31       | 0.56          | 0.60     | 0.75           | 0.73      | 0.41        | 0.44   |

Continued on next page

| $\alpha$ | $\phi_S^\ell$ | $\phi_S$ | $\varphi^\ell$ | $\varphi$ | $\psi^\ell$ | $\psi$ |
|----------|---------------|----------|----------------|-----------|-------------|--------|
| 32       | 0.56          | 0.60     | 0.76           | 0.73      | 0.40        | 0.44   |
| 33       | 0.55          | 0.59     | 0.76           | 0.74      | 0.40        | 0.43   |
| 34       | 0.55          | 0.59     | 0.77           | 0.74      | 0.39        | 0.43   |
| 35       | 0.54          | 0.59     | 0.77           | 0.75      | 0.39        | 0.42   |
| 36       | 0.54          | 0.58     | 0.77           | 0.75      | 0.39        | 0.42   |
| 37       | 0.53          | 0.58     | 0.78           | 0.76      | 0.38        | 0.41   |
| 38       | 0.53          | 0.57     | 0.78           | 0.76      | 0.38        | 0.41   |
| 39       | 0.52          | 0.57     | 0.79           | 0.76      | 0.37        | 0.41   |
| 40       | 0.52          | 0.56     | 0.79           | 0.77      | 0.37        | 0.40   |
| 41       | 0.51          | 0.56     | 0.80           | 0.77      | 0.36        | 0.40   |
| 42       | 0.51          | 0.55     | 0.80           | 0.78      | 0.36        | 0.39   |
| 43       | 0.50          | 0.54     | 0.81           | 0.78      | 0.35        | 0.39   |
| 44       | 0.49          | 0.54     | 0.81           | 0.79      | 0.35        | 0.38   |
| 45       | 0.49          | 0.53     | 0.82           | 0.79      | 0.34        | 0.38   |
| 46       | 0.48          | 0.53     | 0.82           | 0.80      | 0.34        | 0.37   |
| 47       | 0.48          | 0.52     | 0.83           | 0.80      | 0.33        | 0.37   |
| 48       | 0.47          | 0.51     | 0.83           | 0.81      | 0.33        | 0.36   |
| 49       | 0.46          | 0.51     | 0.84           | 0.81      | 0.32        | 0.36   |
| 50       | 0.46          | 0.50     | 0.84           | 0.82      | 0.32        | 0.35   |
| 51       | 0.45          | 0.49     | 0.85           | 0.82      | 0.31        | 0.34   |
| 52       | 0.44          | 0.48     | 0.85           | 0.83      | 0.30        | 0.33   |
| 53       | 0.44          | 0.48     | 0.86           | 0.83      | 0.30        | 0.33   |
| 54       | 0.43          | 0.47     | 0.86           | 0.84      | 0.30        | 0.32   |
| 55       | 0.42          | 0.46     | 0.87           | 0.84      | 0.29        | 0.32   |
| 56       | 0.41          | 0.45     | 0.87           | 0.85      | 0.28        | 0.31   |
| 57       | 0.41          | 0.44     | 0.88           | 0.85      | 0.28        | 0.30   |
| 58       | 0.40          | 0.44     | 0.88           | 0.86      | 0.27        | 0.30   |
| 59       | 0.39          | 0.43     | 0.89           | 0.86      | 0.26        | 0.30   |
| 60       | 0.38          | 0.42     | 0.89           | 0.87      | 0.26        | 0.29   |
| 61       | 0.38          | 0.41     | 0.90           | 0.87      | 0.25        | 0.28   |
| 62       | 0.37          | 0.40     | 0.90           | 0.88      | 0.25        | 0.27   |
| 63       | 0.36          | 0.39     | 0.91           | 0.88      | 0.24        | 0.27   |

Continued on next page

| $\alpha$ | $\phi_S^\ell$ | $\phi_S$ | $\varphi^\ell$ | $\varphi$ | $\psi^\ell$ | $\psi$ |
|----------|---------------|----------|----------------|-----------|-------------|--------|
| 64       | 0.35          | 0.38     | 0.91           | 0.89      | 0.23        | 0.26   |
| 65       | 0.34          | 0.37     | 0.92           | 0.89      | 0.23        | 0.25   |
| 66       | 0.33          | 0.36     | 0.92           | 0.89      | 0.22        | 0.24   |
| 67       | 0.32          | 0.36     | 0.92           | 0.90      | 0.21        | 0.24   |
| 68       | 0.31          | 0.35     | 0.93           | 0.90      | 0.20        | 0.24   |
| 69       | 0.30          | 0.34     | 0.93           | 0.91      | 0.20        | 0.23   |
| 70       | 0.30          | 0.33     | 0.94           | 0.91      | 0.20        | 0.22   |
| 71       | 0.29          | 0.32     | 0.94           | 0.91      | 0.19        | 0.22   |
| 72       | 0.28          | 0.31     | 0.94           | 0.92      | 0.18        | 0.21   |
| 73       | 0.27          | 0.30     | 0.95           | 0.92      | 0.18        | 0.20   |
| 74       | 0.26          | 0.29     | 0.95           | 0.92      | 0.17        | 0.19   |
| 75       | 0.25          | 0.28     | 0.95           | 0.93      | 0.16        | 0.19   |
| 76       | 0.24          | 0.27     | 0.95           | 0.93      | 0.16        | 0.18   |
| 77       | 0.23          | 0.26     | 0.96           | 0.93      | 0.15        | 0.17   |
| 78       | 0.22          | 0.25     | 0.96           | 0.93      | 0.14        | 0.17   |
| 79       | 0.22          | 0.25     | 0.96           | 0.94      | 0.14        | 0.17   |
| 80       | 0.21          | 0.24     | 0.96           | 0.94      | 0.14        | 0.16   |
| 81       | 0.20          | 0.23     | 0.96           | 0.94      | 0.13        | 0.15   |
| 82       | 0.19          | 0.22     | 0.97           | 0.94      | 0.12        | 0.15   |
| 83       | 0.18          | 0.21     | 0.97           | 0.94      | 0.12        | 0.14   |
| 84       | 0.18          | 0.21     | 0.97           | 0.94      | 0.12        | 0.14   |
| 85       | 0.17          | 0.20     | 0.97           | 0.95      | 0.11        | 0.13   |
| 86       | 0.17          | 0.19     | 0.97           | 0.95      | 0.11        | 0.13   |
| 87       | 0.16          | 0.19     | 0.97           | 0.95      | 0.10        | 0.13   |
| 88       | 0.16          | 0.18     | 0.97           | 0.95      | 0.10        | 0.12   |
| 89       | 0.15          | 0.18     | 0.97           | 0.95      | 0.10        | 0.12   |
| 90       | 0.15          | 0.18     | 0.97           | 0.95      | 0.10        | 0.12   |

Table S145: Reference ( $\phi_S$ ,  $\varphi$ ,  $\psi$ ) and approached ( $\phi_S^\ell$ ,  $\varphi^\ell$ ,  $\psi^\ell$ ) values of the topological descriptors for the first excited-state of the pyridinium-phenolate (PP), computed at the TDHF/6-311+G(d) level of theory.  $\alpha$  is the pyridinium-phenolate central twist angle amplitude.

| $\alpha$ | $\phi_S^\ell$ | $\phi_S$ | $\varphi^\ell$ | $\varphi$ | $\psi^\ell$ | $\psi$ |
|----------|---------------|----------|----------------|-----------|-------------|--------|
| 0        | 0.64          | 0.68     | 0.69           | 0.65      | 0.48        | 0.51   |
| 1        | 0.64          | 0.68     | 0.69           | 0.65      | 0.48        | 0.51   |
| 2        | 0.64          | 0.68     | 0.69           | 0.65      | 0.48        | 0.51   |
| 3        | 0.64          | 0.68     | 0.69           | 0.65      | 0.48        | 0.51   |
| 4        | 0.64          | 0.68     | 0.69           | 0.66      | 0.48        | 0.51   |
| 5        | 0.64          | 0.68     | 0.69           | 0.66      | 0.48        | 0.51   |
| 6        | 0.63          | 0.68     | 0.69           | 0.66      | 0.47        | 0.51   |
| 7        | 0.63          | 0.68     | 0.70           | 0.66      | 0.47        | 0.51   |
| 8        | 0.63          | 0.68     | 0.70           | 0.66      | 0.47        | 0.51   |
| 9        | 0.63          | 0.68     | 0.70           | 0.66      | 0.47        | 0.51   |
| 10       | 0.63          | 0.68     | 0.70           | 0.66      | 0.47        | 0.51   |
| 11       | 0.63          | 0.68     | 0.70           | 0.66      | 0.47        | 0.51   |
| 12       | 0.63          | 0.67     | 0.70           | 0.66      | 0.47        | 0.50   |
| 13       | 0.63          | 0.67     | 0.70           | 0.67      | 0.47        | 0.50   |
| 14       | 0.63          | 0.67     | 0.70           | 0.67      | 0.47        | 0.50   |
| 15       | 0.62          | 0.67     | 0.71           | 0.67      | 0.46        | 0.50   |
| 16       | 0.62          | 0.67     | 0.71           | 0.67      | 0.46        | 0.50   |
| 17       | 0.62          | 0.66     | 0.71           | 0.68      | 0.46        | 0.49   |
| 18       | 0.62          | 0.66     | 0.71           | 0.68      | 0.46        | 0.49   |
| 19       | 0.62          | 0.66     | 0.71           | 0.68      | 0.46        | 0.49   |
| 20       | 0.62          | 0.66     | 0.72           | 0.68      | 0.45        | 0.49   |
| 21       | 0.61          | 0.66     | 0.72           | 0.69      | 0.45        | 0.49   |
| 22       | 0.61          | 0.65     | 0.72           | 0.69      | 0.45        | 0.48   |
| 23       | 0.61          | 0.65     | 0.73           | 0.69      | 0.44        | 0.48   |
| 24       | 0.61          | 0.65     | 0.73           | 0.70      | 0.44        | 0.48   |
| 25       | 0.60          | 0.64     | 0.73           | 0.70      | 0.44        | 0.47   |
| 26       | 0.60          | 0.64     | 0.74           | 0.70      | 0.43        | 0.47   |
| 27       | 0.60          | 0.64     | 0.74           | 0.71      | 0.43        | 0.47   |
| 28       | 0.59          | 0.63     | 0.74           | 0.71      | 0.43        | 0.46   |
| 29       | 0.59          | 0.63     | 0.75           | 0.71      | 0.42        | 0.46   |
| 30       | 0.59          | 0.62     | 0.75           | 0.72      | 0.42        | 0.45   |
| 31       | 0.58          | 0.62     | 0.75           | 0.72      | 0.42        | 0.45   |

Continued on next page

| $\alpha$ | $\phi_S^\ell$ | $\phi_S$ | $\varphi^\ell$ | $\varphi$ | $\psi^\ell$ | $\psi$ |
|----------|---------------|----------|----------------|-----------|-------------|--------|
| 32       | 0.58          | 0.62     | 0.76           | 0.73      | 0.41        | 0.45   |
| 33       | 0.57          | 0.61     | 0.76           | 0.73      | 0.41        | 0.44   |
| 34       | 0.57          | 0.61     | 0.77           | 0.73      | 0.41        | 0.44   |
| 35       | 0.57          | 0.60     | 0.77           | 0.74      | 0.41        | 0.43   |
| 36       | 0.56          | 0.60     | 0.77           | 0.74      | 0.40        | 0.43   |
| 37       | 0.56          | 0.59     | 0.78           | 0.75      | 0.40        | 0.42   |
| 38       | 0.55          | 0.59     | 0.78           | 0.75      | 0.39        | 0.42   |
| 39       | 0.55          | 0.58     | 0.79           | 0.76      | 0.39        | 0.41   |
| 40       | 0.54          | 0.58     | 0.79           | 0.76      | 0.38        | 0.41   |
| 41       | 0.53          | 0.57     | 0.80           | 0.77      | 0.37        | 0.41   |
| 42       | 0.53          | 0.57     | 0.80           | 0.77      | 0.37        | 0.41   |
| 43       | 0.52          | 0.56     | 0.81           | 0.78      | 0.36        | 0.40   |
| 44       | 0.52          | 0.55     | 0.81           | 0.78      | 0.36        | 0.39   |
| 45       | 0.51          | 0.55     | 0.82           | 0.79      | 0.35        | 0.39   |
| 46       | 0.50          | 0.54     | 0.82           | 0.79      | 0.35        | 0.38   |
| 47       | 0.50          | 0.53     | 0.83           | 0.80      | 0.35        | 0.37   |
| 48       | 0.49          | 0.53     | 0.83           | 0.80      | 0.34        | 0.37   |
| 49       | 0.48          | 0.52     | 0.84           | 0.81      | 0.33        | 0.36   |
| 50       | 0.48          | 0.51     | 0.84           | 0.81      | 0.33        | 0.36   |
| 51       | 0.47          | 0.50     | 0.85           | 0.82      | 0.32        | 0.35   |
| 52       | 0.46          | 0.50     | 0.85           | 0.82      | 0.32        | 0.35   |
| 53       | 0.46          | 0.49     | 0.85           | 0.83      | 0.32        | 0.34   |
| 54       | 0.45          | 0.48     | 0.86           | 0.83      | 0.31        | 0.33   |
| 55       | 0.44          | 0.47     | 0.86           | 0.84      | 0.30        | 0.32   |
| 56       | 0.43          | 0.47     | 0.87           | 0.84      | 0.29        | 0.32   |
| 57       | 0.42          | 0.46     | 0.87           | 0.85      | 0.29        | 0.32   |
| 58       | 0.42          | 0.45     | 0.88           | 0.85      | 0.28        | 0.31   |
| 59       | 0.41          | 0.44     | 0.88           | 0.86      | 0.28        | 0.30   |
| 60       | 0.40          | 0.43     | 0.89           | 0.86      | 0.27        | 0.30   |
| 61       | 0.39          | 0.42     | 0.90           | 0.87      | 0.26        | 0.29   |
| 62       | 0.38          | 0.41     | 0.90           | 0.87      | 0.25        | 0.28   |
| 63       | 0.37          | 0.40     | 0.91           | 0.88      | 0.25        | 0.27   |

Continued on next page

| $\alpha$ | $\phi_S^\ell$ | $\phi_S$ | $\varphi^\ell$ | $\varphi$ | $\psi^\ell$ | $\psi$ |
|----------|---------------|----------|----------------|-----------|-------------|--------|
| 64       | 0.36          | 0.39     | 0.91           | 0.88      | 0.24        | 0.27   |
| 65       | 0.35          | 0.38     | 0.92           | 0.89      | 0.23        | 0.26   |
| 66       | 0.34          | 0.38     | 0.92           | 0.89      | 0.23        | 0.26   |
| 67       | 0.33          | 0.37     | 0.93           | 0.90      | 0.22        | 0.25   |
| 68       | 0.32          | 0.36     | 0.93           | 0.90      | 0.21        | 0.24   |
| 69       | 0.31          | 0.35     | 0.93           | 0.90      | 0.20        | 0.24   |
| 70       | 0.30          | 0.34     | 0.94           | 0.91      | 0.20        | 0.23   |
| 71       | 0.29          | 0.33     | 0.94           | 0.91      | 0.19        | 0.22   |
| 72       | 0.28          | 0.32     | 0.95           | 0.91      | 0.18        | 0.22   |
| 73       | 0.27          | 0.31     | 0.95           | 0.92      | 0.18        | 0.21   |
| 74       | 0.26          | 0.30     | 0.95           | 0.92      | 0.17        | 0.20   |
| 75       | 0.25          | 0.29     | 0.95           | 0.92      | 0.16        | 0.19   |
| 76       | 0.24          | 0.28     | 0.96           | 0.93      | 0.16        | 0.19   |
| 77       | 0.23          | 0.27     | 0.96           | 0.93      | 0.15        | 0.18   |
| 78       | 0.22          | 0.26     | 0.96           | 0.93      | 0.14        | 0.17   |
| 79       | 0.21          | 0.25     | 0.96           | 0.94      | 0.14        | 0.17   |
| 80       | 0.20          | 0.24     | 0.97           | 0.94      | 0.13        | 0.16   |
| 81       | 0.19          | 0.23     | 0.97           | 0.94      | 0.12        | 0.15   |
| 82       | 0.18          | 0.23     | 0.97           | 0.94      | 0.12        | 0.15   |
| 83       | 0.17          | 0.22     | 0.97           | 0.94      | 0.11        | 0.15   |
| 84       | 0.17          | 0.21     | 0.97           | 0.94      | 0.11        | 0.14   |
| 85       | 0.16          | 0.20     | 0.97           | 0.95      | 0.10        | 0.13   |
| 86       | 0.15          | 0.20     | 0.97           | 0.95      | 0.10        | 0.13   |
| 87       | 0.14          | 0.19     | 0.97           | 0.95      | 0.09        | 0.13   |
| 88       | 0.14          | 0.19     | 0.98           | 0.95      | 0.09        | 0.13   |
| 89       | 0.14          | 0.18     | 0.98           | 0.95      | 0.09        | 0.12   |
| 90       | 0.14          | 0.18     | 0.98           | 0.95      | 0.09        | 0.12   |

Table S146: Reference  $(\phi_S, \varphi, \psi)$  and approached  $(\phi_S^\ell, \varphi^\ell, \psi^\ell)$  values of the topological descriptors for the first excited-state of the pyridinium-phenolate (PP), computed at the TDHF/6-311G(d) level of theory.  $\alpha$  is the pyridinium-phenolate central twist angle amplitude.

| $\alpha$ | $\phi_S^\ell$ | $\phi_S$ | $\varphi^\ell$ | $\varphi$ | $\psi^\ell$ | $\psi$ |
|----------|---------------|----------|----------------|-----------|-------------|--------|
| 0        | 0.61          | 0.65     | 0.70           | 0.68      | 0.46        | 0.49   |
| 1        | 0.61          | 0.65     | 0.70           | 0.68      | 0.46        | 0.49   |
| 2        | 0.61          | 0.65     | 0.70           | 0.68      | 0.46        | 0.49   |
| 3        | 0.61          | 0.65     | 0.70           | 0.68      | 0.46        | 0.49   |
| 4        | 0.61          | 0.65     | 0.70           | 0.68      | 0.46        | 0.49   |
| 5        | 0.61          | 0.65     | 0.70           | 0.68      | 0.46        | 0.49   |
| 6        | 0.61          | 0.65     | 0.70           | 0.68      | 0.46        | 0.49   |
| 7        | 0.61          | 0.65     | 0.71           | 0.68      | 0.45        | 0.49   |
| 8        | 0.60          | 0.65     | 0.71           | 0.68      | 0.45        | 0.49   |
| 9        | 0.60          | 0.64     | 0.71           | 0.69      | 0.45        | 0.48   |
| 10       | 0.60          | 0.64     | 0.71           | 0.69      | 0.45        | 0.48   |
| 11       | 0.60          | 0.64     | 0.71           | 0.69      | 0.45        | 0.48   |
| 12       | 0.60          | 0.64     | 0.71           | 0.69      | 0.45        | 0.48   |
| 13       | 0.60          | 0.64     | 0.71           | 0.69      | 0.45        | 0.48   |
| 14       | 0.60          | 0.64     | 0.71           | 0.69      | 0.45        | 0.48   |
| 15       | 0.60          | 0.64     | 0.72           | 0.70      | 0.44        | 0.47   |
| 16       | 0.59          | 0.63     | 0.72           | 0.70      | 0.44        | 0.47   |
| 17       | 0.59          | 0.63     | 0.72           | 0.70      | 0.44        | 0.47   |
| 18       | 0.59          | 0.63     | 0.72           | 0.70      | 0.44        | 0.47   |
| 19       | 0.59          | 0.63     | 0.73           | 0.70      | 0.43        | 0.47   |
| 20       | 0.59          | 0.62     | 0.73           | 0.71      | 0.43        | 0.46   |
| 21       | 0.58          | 0.62     | 0.73           | 0.71      | 0.43        | 0.46   |
| 22       | 0.58          | 0.62     | 0.73           | 0.71      | 0.43        | 0.46   |
| 23       | 0.58          | 0.62     | 0.74           | 0.71      | 0.42        | 0.46   |
| 24       | 0.57          | 0.61     | 0.74           | 0.72      | 0.42        | 0.45   |
| 25       | 0.57          | 0.61     | 0.74           | 0.72      | 0.42        | 0.45   |
| 26       | 0.57          | 0.61     | 0.74           | 0.72      | 0.42        | 0.45   |
| 27       | 0.57          | 0.60     | 0.75           | 0.73      | 0.41        | 0.44   |
| 28       | 0.56          | 0.60     | 0.75           | 0.73      | 0.41        | 0.44   |
| 29       | 0.56          | 0.60     | 0.75           | 0.73      | 0.41        | 0.44   |
| 30       | 0.56          | 0.59     | 0.76           | 0.74      | 0.40        | 0.43   |
| 31       | 0.55          | 0.59     | 0.76           | 0.74      | 0.40        | 0.43   |

Continued on next page



| $\alpha$ | $\phi_S^\ell$ | $\phi_S$ | $\varphi^\ell$ | $\varphi$ | $\psi^\ell$ | $\psi$ |
|----------|---------------|----------|----------------|-----------|-------------|--------|
| 32       | 0.55          | 0.59     | 0.77           | 0.75      | 0.39        | 0.42   |
| 33       | 0.54          | 0.58     | 0.77           | 0.75      | 0.39        | 0.42   |
| 34       | 0.54          | 0.58     | 0.77           | 0.75      | 0.39        | 0.42   |
| 35       | 0.54          | 0.57     | 0.78           | 0.76      | 0.39        | 0.41   |
| 36       | 0.53          | 0.57     | 0.78           | 0.76      | 0.38        | 0.41   |
| 37       | 0.53          | 0.56     | 0.79           | 0.77      | 0.38        | 0.40   |
| 38       | 0.52          | 0.56     | 0.79           | 0.77      | 0.37        | 0.40   |
| 39       | 0.52          | 0.55     | 0.79           | 0.77      | 0.37        | 0.39   |
| 40       | 0.51          | 0.55     | 0.80           | 0.78      | 0.36        | 0.39   |
| 41       | 0.50          | 0.54     | 0.80           | 0.78      | 0.36        | 0.39   |
| 42       | 0.50          | 0.54     | 0.81           | 0.79      | 0.35        | 0.38   |
| 43       | 0.49          | 0.53     | 0.81           | 0.79      | 0.35        | 0.38   |
| 44       | 0.49          | 0.52     | 0.82           | 0.80      | 0.34        | 0.37   |
| 45       | 0.48          | 0.52     | 0.82           | 0.80      | 0.34        | 0.37   |
| 46       | 0.47          | 0.51     | 0.83           | 0.81      | 0.33        | 0.36   |
| 47       | 0.47          | 0.51     | 0.83           | 0.81      | 0.33        | 0.36   |
| 48       | 0.46          | 0.50     | 0.84           | 0.82      | 0.32        | 0.35   |
| 49       | 0.45          | 0.49     | 0.84           | 0.82      | 0.31        | 0.34   |
| 50       | 0.45          | 0.49     | 0.85           | 0.83      | 0.31        | 0.34   |
| 51       | 0.44          | 0.48     | 0.85           | 0.83      | 0.30        | 0.33   |
| 52       | 0.43          | 0.47     | 0.86           | 0.84      | 0.30        | 0.32   |
| 53       | 0.43          | 0.46     | 0.86           | 0.84      | 0.30        | 0.32   |
| 54       | 0.42          | 0.46     | 0.87           | 0.85      | 0.29        | 0.32   |
| 55       | 0.41          | 0.45     | 0.87           | 0.85      | 0.28        | 0.31   |
| 56       | 0.41          | 0.44     | 0.88           | 0.86      | 0.28        | 0.30   |
| 57       | 0.40          | 0.43     | 0.88           | 0.86      | 0.27        | 0.30   |
| 58       | 0.39          | 0.42     | 0.89           | 0.87      | 0.26        | 0.29   |
| 59       | 0.38          | 0.42     | 0.89           | 0.87      | 0.26        | 0.29   |
| 60       | 0.37          | 0.41     | 0.90           | 0.87      | 0.25        | 0.28   |
| 61       | 0.36          | 0.40     | 0.90           | 0.88      | 0.24        | 0.27   |
| 62       | 0.36          | 0.39     | 0.91           | 0.88      | 0.24        | 0.27   |
| 63       | 0.35          | 0.38     | 0.91           | 0.89      | 0.23        | 0.26   |

Continued on next page

| $\alpha$ | $\phi_S^\ell$ | $\phi_S$ | $\varphi^\ell$ | $\varphi$ | $\psi^\ell$ | $\psi$ |
|----------|---------------|----------|----------------|-----------|-------------|--------|
| 64       | 0.34          | 0.37     | 0.92           | 0.89      | 0.23        | 0.25   |
| 65       | 0.33          | 0.36     | 0.92           | 0.90      | 0.22        | 0.24   |
| 66       | 0.32          | 0.35     | 0.93           | 0.90      | 0.21        | 0.24   |
| 67       | 0.31          | 0.35     | 0.93           | 0.90      | 0.20        | 0.24   |
| 68       | 0.30          | 0.34     | 0.93           | 0.91      | 0.20        | 0.23   |
| 69       | 0.29          | 0.33     | 0.94           | 0.91      | 0.19        | 0.22   |
| 70       | 0.28          | 0.32     | 0.94           | 0.92      | 0.18        | 0.21   |
| 71       | 0.27          | 0.31     | 0.95           | 0.92      | 0.18        | 0.21   |
| 72       | 0.27          | 0.30     | 0.95           | 0.92      | 0.18        | 0.20   |
| 73       | 0.26          | 0.29     | 0.95           | 0.92      | 0.17        | 0.19   |
| 74       | 0.25          | 0.28     | 0.95           | 0.93      | 0.16        | 0.19   |
| 75       | 0.24          | 0.27     | 0.96           | 0.93      | 0.16        | 0.18   |
| 76       | 0.23          | 0.26     | 0.96           | 0.93      | 0.15        | 0.17   |
| 77       | 0.22          | 0.25     | 0.96           | 0.94      | 0.14        | 0.17   |
| 78       | 0.21          | 0.24     | 0.96           | 0.94      | 0.14        | 0.16   |
| 79       | 0.21          | 0.24     | 0.97           | 0.94      | 0.14        | 0.16   |
| 80       | 0.20          | 0.23     | 0.97           | 0.94      | 0.13        | 0.15   |
| 81       | 0.19          | 0.22     | 0.97           | 0.94      | 0.12        | 0.15   |
| 82       | 0.18          | 0.21     | 0.97           | 0.95      | 0.12        | 0.14   |
| 83       | 0.18          | 0.20     | 0.97           | 0.95      | 0.12        | 0.13   |
| 84       | 0.17          | 0.20     | 0.97           | 0.95      | 0.11        | 0.13   |
| 85       | 0.16          | 0.19     | 0.97           | 0.95      | 0.10        | 0.13   |
| 86       | 0.16          | 0.18     | 0.97           | 0.95      | 0.10        | 0.12   |
| 87       | 0.15          | 0.18     | 0.97           | 0.95      | 0.10        | 0.12   |
| 88       | 0.15          | 0.17     | 0.97           | 0.95      | 0.10        | 0.11   |
| 89       | 0.15          | 0.17     | 0.97           | 0.95      | 0.10        | 0.11   |
| 90       | 0.14          | 0.17     | 0.97           | 0.95      | 0.09        | 0.11   |

Table S147: Reference ( $\phi_S$ ,  $\varphi$ ,  $\psi$ ) and approached ( $\phi_S^\ell$ ,  $\varphi^\ell$ ,  $\psi^\ell$ ) values of the topological descriptors for the first excited-state of the pyridinium-phenolate (PP), computed at the TDHF/6-311+G level of theory.  $\alpha$  is the pyridinium-phenolate central twist angle amplitude.

| $\alpha$ | $\phi_S^\ell$ | $\phi_S$ | $\varphi^\ell$ | $\varphi$ | $\psi^\ell$ | $\psi$ |
|----------|---------------|----------|----------------|-----------|-------------|--------|
| 0        | 0.63          | 0.67     | 0.70           | 0.67      | 0.47        | 0.50   |
| 1        | 0.63          | 0.67     | 0.70           | 0.67      | 0.47        | 0.50   |
| 2        | 0.63          | 0.67     | 0.70           | 0.67      | 0.47        | 0.50   |
| 3        | 0.63          | 0.67     | 0.70           | 0.67      | 0.47        | 0.50   |
| 4        | 0.63          | 0.67     | 0.70           | 0.67      | 0.47        | 0.50   |
| 5        | 0.62          | 0.67     | 0.70           | 0.67      | 0.46        | 0.50   |
| 6        | 0.62          | 0.67     | 0.70           | 0.67      | 0.46        | 0.50   |
| 7        | 0.62          | 0.67     | 0.71           | 0.67      | 0.46        | 0.50   |
| 8        | 0.62          | 0.66     | 0.71           | 0.67      | 0.46        | 0.50   |
| 9        | 0.62          | 0.66     | 0.71           | 0.68      | 0.46        | 0.49   |
| 10       | 0.62          | 0.66     | 0.71           | 0.68      | 0.46        | 0.49   |
| 11       | 0.62          | 0.66     | 0.71           | 0.68      | 0.46        | 0.49   |
| 12       | 0.62          | 0.66     | 0.71           | 0.68      | 0.46        | 0.49   |
| 13       | 0.62          | 0.66     | 0.71           | 0.68      | 0.46        | 0.49   |
| 14       | 0.62          | 0.66     | 0.71           | 0.68      | 0.46        | 0.49   |
| 15       | 0.61          | 0.65     | 0.72           | 0.69      | 0.45        | 0.48   |
| 16       | 0.61          | 0.65     | 0.72           | 0.69      | 0.45        | 0.48   |
| 17       | 0.61          | 0.65     | 0.72           | 0.69      | 0.45        | 0.48   |
| 18       | 0.61          | 0.65     | 0.72           | 0.69      | 0.45        | 0.48   |
| 19       | 0.61          | 0.64     | 0.72           | 0.70      | 0.45        | 0.47   |
| 20       | 0.60          | 0.64     | 0.73           | 0.70      | 0.44        | 0.47   |
| 21       | 0.60          | 0.64     | 0.73           | 0.70      | 0.44        | 0.47   |
| 22       | 0.60          | 0.64     | 0.73           | 0.70      | 0.44        | 0.47   |
| 23       | 0.60          | 0.63     | 0.74           | 0.71      | 0.43        | 0.46   |
| 24       | 0.59          | 0.63     | 0.74           | 0.71      | 0.43        | 0.46   |
| 25       | 0.59          | 0.63     | 0.74           | 0.71      | 0.43        | 0.46   |
| 26       | 0.59          | 0.62     | 0.74           | 0.72      | 0.43        | 0.45   |
| 27       | 0.59          | 0.62     | 0.75           | 0.72      | 0.42        | 0.45   |
| 28       | 0.58          | 0.62     | 0.75           | 0.72      | 0.42        | 0.45   |
| 29       | 0.58          | 0.61     | 0.75           | 0.73      | 0.42        | 0.44   |
| 30       | 0.58          | 0.61     | 0.76           | 0.73      | 0.41        | 0.44   |
| 31       | 0.57          | 0.61     | 0.76           | 0.73      | 0.41        | 0.44   |

Continued on next page

| $\alpha$ | $\phi_S^\ell$ | $\phi_S$ | $\varphi^\ell$ | $\varphi$ | $\psi^\ell$ | $\psi$ |
|----------|---------------|----------|----------------|-----------|-------------|--------|
| 32       | 0.57          | 0.60     | 0.76           | 0.74      | 0.41        | 0.43   |
| 33       | 0.56          | 0.60     | 0.77           | 0.74      | 0.40        | 0.43   |
| 34       | 0.56          | 0.59     | 0.77           | 0.75      | 0.40        | 0.42   |
| 35       | 0.56          | 0.59     | 0.78           | 0.75      | 0.40        | 0.42   |
| 36       | 0.55          | 0.58     | 0.78           | 0.75      | 0.39        | 0.42   |
| 37       | 0.55          | 0.58     | 0.79           | 0.76      | 0.39        | 0.41   |
| 38       | 0.54          | 0.57     | 0.79           | 0.76      | 0.38        | 0.41   |
| 39       | 0.54          | 0.57     | 0.79           | 0.77      | 0.38        | 0.41   |
| 40       | 0.53          | 0.56     | 0.80           | 0.77      | 0.37        | 0.40   |
| 41       | 0.52          | 0.56     | 0.80           | 0.78      | 0.37        | 0.40   |
| 42       | 0.52          | 0.55     | 0.81           | 0.78      | 0.36        | 0.39   |
| 43       | 0.51          | 0.54     | 0.81           | 0.79      | 0.36        | 0.38   |
| 44       | 0.51          | 0.54     | 0.82           | 0.79      | 0.35        | 0.38   |
| 45       | 0.50          | 0.53     | 0.82           | 0.80      | 0.35        | 0.37   |
| 46       | 0.49          | 0.53     | 0.83           | 0.80      | 0.34        | 0.37   |
| 47       | 0.49          | 0.52     | 0.83           | 0.81      | 0.34        | 0.36   |
| 48       | 0.48          | 0.51     | 0.84           | 0.81      | 0.33        | 0.36   |
| 49       | 0.47          | 0.51     | 0.84           | 0.82      | 0.32        | 0.35   |
| 50       | 0.47          | 0.50     | 0.85           | 0.82      | 0.32        | 0.35   |
| 51       | 0.46          | 0.49     | 0.85           | 0.83      | 0.32        | 0.34   |
| 52       | 0.45          | 0.48     | 0.86           | 0.83      | 0.31        | 0.33   |
| 53       | 0.44          | 0.48     | 0.86           | 0.84      | 0.30        | 0.33   |
| 54       | 0.44          | 0.47     | 0.87           | 0.84      | 0.30        | 0.32   |
| 55       | 0.43          | 0.46     | 0.87           | 0.85      | 0.29        | 0.32   |
| 56       | 0.42          | 0.45     | 0.88           | 0.85      | 0.28        | 0.31   |
| 57       | 0.41          | 0.44     | 0.88           | 0.86      | 0.28        | 0.30   |
| 58       | 0.40          | 0.44     | 0.89           | 0.86      | 0.27        | 0.30   |
| 59       | 0.39          | 0.43     | 0.89           | 0.87      | 0.26        | 0.29   |
| 60       | 0.39          | 0.42     | 0.90           | 0.87      | 0.26        | 0.29   |
| 61       | 0.38          | 0.41     | 0.90           | 0.88      | 0.25        | 0.28   |
| 62       | 0.37          | 0.40     | 0.91           | 0.88      | 0.25        | 0.27   |
| 63       | 0.36          | 0.39     | 0.91           | 0.88      | 0.24        | 0.27   |

Continued on next page

| $\alpha$ | $\phi_S^\ell$ | $\phi_S$ | $\varphi^\ell$ | $\varphi$ | $\psi^\ell$ | $\psi$ |
|----------|---------------|----------|----------------|-----------|-------------|--------|
| 64       | 0.35          | 0.38     | 0.92           | 0.89      | 0.23        | 0.26   |
| 65       | 0.34          | 0.37     | 0.92           | 0.89      | 0.23        | 0.25   |
| 66       | 0.33          | 0.36     | 0.93           | 0.90      | 0.22        | 0.24   |
| 67       | 0.32          | 0.35     | 0.93           | 0.90      | 0.21        | 0.24   |
| 68       | 0.31          | 0.34     | 0.94           | 0.91      | 0.20        | 0.23   |
| 69       | 0.30          | 0.33     | 0.94           | 0.91      | 0.20        | 0.22   |
| 70       | 0.29          | 0.32     | 0.94           | 0.91      | 0.19        | 0.22   |
| 71       | 0.28          | 0.32     | 0.95           | 0.92      | 0.18        | 0.21   |
| 72       | 0.27          | 0.31     | 0.95           | 0.92      | 0.18        | 0.21   |
| 73       | 0.26          | 0.30     | 0.96           | 0.92      | 0.17        | 0.20   |
| 74       | 0.24          | 0.29     | 0.96           | 0.93      | 0.16        | 0.19   |
| 75       | 0.23          | 0.28     | 0.96           | 0.93      | 0.15        | 0.19   |
| 76       | 0.22          | 0.27     | 0.96           | 0.93      | 0.14        | 0.18   |
| 77       | 0.21          | 0.26     | 0.97           | 0.94      | 0.14        | 0.17   |
| 78       | 0.20          | 0.25     | 0.97           | 0.94      | 0.13        | 0.17   |
| 79       | 0.20          | 0.24     | 0.97           | 0.94      | 0.13        | 0.16   |
| 80       | 0.19          | 0.23     | 0.97           | 0.94      | 0.12        | 0.15   |
| 81       | 0.18          | 0.22     | 0.97           | 0.94      | 0.12        | 0.15   |
| 82       | 0.17          | 0.21     | 0.98           | 0.95      | 0.11        | 0.14   |
| 83       | 0.16          | 0.21     | 0.98           | 0.95      | 0.10        | 0.14   |
| 84       | 0.16          | 0.20     | 0.98           | 0.95      | 0.10        | 0.13   |
| 85       | 0.15          | 0.19     | 0.98           | 0.95      | 0.10        | 0.13   |
| 86       | 0.14          | 0.19     | 0.98           | 0.95      | 0.09        | 0.13   |
| 87       | 0.14          | 0.18     | 0.98           | 0.95      | 0.09        | 0.12   |
| 88       | 0.13          | 0.18     | 0.98           | 0.95      | 0.08        | 0.12   |
| 89       | 0.13          | 0.17     | 0.98           | 0.95      | 0.08        | 0.11   |
| 90       | 0.13          | 0.17     | 0.98           | 0.95      | 0.08        | 0.11   |

Table S148: Reference ( $\phi_S$ ,  $\varphi$ ,  $\psi$ ) and approached ( $\phi_S^\ell$ ,  $\varphi^\ell$ ,  $\psi^\ell$ ) values of the topological descriptors for the first excited-state of the pyridinium-phenolate (PP), computed at the TDHF/6-311G level of theory.  $\alpha$  is the pyridinium-phenolate central twist angle amplitude.

| $\alpha$ | $\phi_S^\ell$ | $\phi_S$ | $\varphi^\ell$ | $\varphi$ | $\psi^\ell$ | $\psi$ |
|----------|---------------|----------|----------------|-----------|-------------|--------|
| 0        | 0.62          | 0.67     | 0.69           | 0.66      | 0.47        | 0.50   |
| 1        | 0.62          | 0.67     | 0.69           | 0.66      | 0.47        | 0.50   |
| 2        | 0.62          | 0.67     | 0.69           | 0.66      | 0.47        | 0.50   |
| 3        | 0.62          | 0.67     | 0.69           | 0.66      | 0.47        | 0.50   |
| 4        | 0.62          | 0.67     | 0.69           | 0.66      | 0.47        | 0.50   |
| 5        | 0.62          | 0.66     | 0.69           | 0.66      | 0.47        | 0.50   |
| 6        | 0.62          | 0.66     | 0.69           | 0.66      | 0.47        | 0.50   |
| 7        | 0.62          | 0.66     | 0.69           | 0.67      | 0.47        | 0.50   |
| 8        | 0.62          | 0.66     | 0.69           | 0.67      | 0.47        | 0.50   |
| 9        | 0.62          | 0.66     | 0.69           | 0.67      | 0.47        | 0.50   |
| 10       | 0.62          | 0.66     | 0.70           | 0.67      | 0.46        | 0.50   |
| 11       | 0.62          | 0.66     | 0.70           | 0.67      | 0.46        | 0.50   |
| 12       | 0.62          | 0.66     | 0.70           | 0.67      | 0.46        | 0.50   |
| 13       | 0.62          | 0.66     | 0.70           | 0.67      | 0.46        | 0.50   |
| 14       | 0.61          | 0.65     | 0.70           | 0.68      | 0.46        | 0.49   |
| 15       | 0.61          | 0.65     | 0.70           | 0.68      | 0.46        | 0.49   |
| 16       | 0.61          | 0.65     | 0.71           | 0.68      | 0.45        | 0.49   |
| 17       | 0.61          | 0.65     | 0.71           | 0.68      | 0.45        | 0.49   |
| 18       | 0.61          | 0.65     | 0.71           | 0.68      | 0.45        | 0.49   |
| 19       | 0.60          | 0.64     | 0.71           | 0.69      | 0.45        | 0.48   |
| 20       | 0.60          | 0.64     | 0.71           | 0.69      | 0.45        | 0.48   |
| 21       | 0.60          | 0.64     | 0.72           | 0.69      | 0.44        | 0.48   |
| 22       | 0.60          | 0.64     | 0.72           | 0.70      | 0.44        | 0.47   |
| 23       | 0.59          | 0.63     | 0.72           | 0.70      | 0.44        | 0.47   |
| 24       | 0.59          | 0.63     | 0.73           | 0.70      | 0.43        | 0.47   |
| 25       | 0.59          | 0.63     | 0.73           | 0.70      | 0.43        | 0.47   |
| 26       | 0.59          | 0.62     | 0.73           | 0.71      | 0.43        | 0.46   |
| 27       | 0.58          | 0.62     | 0.74           | 0.71      | 0.42        | 0.46   |
| 28       | 0.58          | 0.62     | 0.74           | 0.72      | 0.42        | 0.45   |
| 29       | 0.58          | 0.61     | 0.74           | 0.72      | 0.42        | 0.45   |
| 30       | 0.57          | 0.61     | 0.75           | 0.72      | 0.41        | 0.45   |
| 31       | 0.57          | 0.61     | 0.75           | 0.73      | 0.41        | 0.44   |

Continued on next page

| $\alpha$ | $\phi_S^\ell$ | $\phi_S$ | $\varphi^\ell$ | $\varphi$ | $\psi^\ell$ | $\psi$ |
|----------|---------------|----------|----------------|-----------|-------------|--------|
| 32       | 0.56          | 0.60     | 0.75           | 0.73      | 0.41        | 0.44   |
| 33       | 0.56          | 0.60     | 0.76           | 0.73      | 0.40        | 0.44   |
| 34       | 0.56          | 0.59     | 0.76           | 0.74      | 0.40        | 0.43   |
| 35       | 0.55          | 0.59     | 0.77           | 0.74      | 0.39        | 0.43   |
| 36       | 0.55          | 0.58     | 0.77           | 0.75      | 0.39        | 0.42   |
| 37       | 0.54          | 0.58     | 0.77           | 0.75      | 0.39        | 0.42   |
| 38       | 0.54          | 0.57     | 0.78           | 0.76      | 0.39        | 0.41   |
| 39       | 0.53          | 0.57     | 0.78           | 0.76      | 0.38        | 0.41   |
| 40       | 0.52          | 0.56     | 0.79           | 0.77      | 0.37        | 0.40   |
| 41       | 0.52          | 0.56     | 0.79           | 0.77      | 0.37        | 0.40   |
| 42       | 0.51          | 0.55     | 0.80           | 0.78      | 0.36        | 0.39   |
| 43       | 0.51          | 0.55     | 0.80           | 0.78      | 0.36        | 0.39   |
| 44       | 0.50          | 0.54     | 0.81           | 0.78      | 0.35        | 0.39   |
| 45       | 0.49          | 0.53     | 0.81           | 0.79      | 0.35        | 0.38   |
| 46       | 0.49          | 0.53     | 0.82           | 0.79      | 0.34        | 0.38   |
| 47       | 0.48          | 0.52     | 0.82           | 0.80      | 0.34        | 0.37   |
| 48       | 0.48          | 0.52     | 0.83           | 0.80      | 0.33        | 0.37   |
| 49       | 0.47          | 0.51     | 0.83           | 0.81      | 0.33        | 0.36   |
| 50       | 0.46          | 0.50     | 0.84           | 0.81      | 0.32        | 0.35   |
| 51       | 0.46          | 0.49     | 0.84           | 0.82      | 0.32        | 0.34   |
| 52       | 0.45          | 0.49     | 0.85           | 0.83      | 0.31        | 0.34   |
| 53       | 0.44          | 0.48     | 0.85           | 0.83      | 0.30        | 0.33   |
| 54       | 0.44          | 0.47     | 0.86           | 0.84      | 0.30        | 0.32   |
| 55       | 0.43          | 0.46     | 0.86           | 0.84      | 0.30        | 0.32   |
| 56       | 0.42          | 0.46     | 0.87           | 0.85      | 0.29        | 0.32   |
| 57       | 0.41          | 0.45     | 0.87           | 0.85      | 0.28        | 0.31   |
| 58       | 0.41          | 0.44     | 0.88           | 0.86      | 0.28        | 0.30   |
| 59       | 0.40          | 0.43     | 0.88           | 0.86      | 0.27        | 0.30   |
| 60       | 0.39          | 0.42     | 0.89           | 0.86      | 0.26        | 0.29   |
| 61       | 0.38          | 0.41     | 0.89           | 0.87      | 0.26        | 0.28   |
| 62       | 0.37          | 0.40     | 0.90           | 0.87      | 0.25        | 0.27   |
| 63       | 0.37          | 0.40     | 0.90           | 0.88      | 0.25        | 0.27   |

Continued on next page

| $\alpha$ | $\phi_S^\ell$ | $\phi_S$ | $\varphi^\ell$ | $\varphi$ | $\psi^\ell$ | $\psi$ |
|----------|---------------|----------|----------------|-----------|-------------|--------|
| 64       | 0.36          | 0.39     | 0.91           | 0.88      | 0.24        | 0.27   |
| 65       | 0.35          | 0.38     | 0.91           | 0.89      | 0.23        | 0.26   |
| 66       | 0.34          | 0.37     | 0.92           | 0.89      | 0.23        | 0.25   |
| 67       | 0.33          | 0.36     | 0.92           | 0.90      | 0.22        | 0.24   |
| 68       | 0.32          | 0.35     | 0.92           | 0.90      | 0.21        | 0.24   |
| 69       | 0.31          | 0.34     | 0.93           | 0.90      | 0.20        | 0.23   |
| 70       | 0.30          | 0.33     | 0.93           | 0.91      | 0.20        | 0.22   |
| 71       | 0.29          | 0.32     | 0.93           | 0.91      | 0.19        | 0.22   |
| 72       | 0.28          | 0.31     | 0.94           | 0.91      | 0.18        | 0.21   |
| 73       | 0.28          | 0.30     | 0.94           | 0.92      | 0.18        | 0.20   |
| 74       | 0.27          | 0.29     | 0.94           | 0.92      | 0.18        | 0.19   |
| 75       | 0.26          | 0.28     | 0.94           | 0.92      | 0.17        | 0.19   |
| 76       | 0.25          | 0.28     | 0.95           | 0.93      | 0.16        | 0.19   |
| 77       | 0.24          | 0.27     | 0.95           | 0.93      | 0.16        | 0.18   |
| 78       | 0.23          | 0.26     | 0.95           | 0.93      | 0.15        | 0.17   |
| 79       | 0.22          | 0.25     | 0.95           | 0.93      | 0.14        | 0.17   |
| 80       | 0.21          | 0.24     | 0.95           | 0.94      | 0.14        | 0.16   |
| 81       | 0.21          | 0.23     | 0.96           | 0.94      | 0.14        | 0.15   |
| 82       | 0.20          | 0.23     | 0.96           | 0.94      | 0.13        | 0.15   |
| 83       | 0.19          | 0.22     | 0.96           | 0.94      | 0.12        | 0.15   |
| 84       | 0.19          | 0.21     | 0.96           | 0.94      | 0.12        | 0.14   |
| 85       | 0.18          | 0.20     | 0.96           | 0.94      | 0.12        | 0.13   |
| 86       | 0.17          | 0.20     | 0.96           | 0.95      | 0.11        | 0.13   |
| 87       | 0.17          | 0.19     | 0.96           | 0.95      | 0.11        | 0.13   |
| 88       | 0.16          | 0.19     | 0.96           | 0.95      | 0.11        | 0.13   |
| 89       | 0.16          | 0.19     | 0.96           | 0.95      | 0.11        | 0.13   |
| 90       | 0.16          | 0.18     | 0.96           | 0.95      | 0.11        | 0.12   |

Table S149: Reference ( $\phi_S$ ,  $\varphi$ ,  $\psi$ ) and approached ( $\phi_S^\ell$ ,  $\varphi^\ell$ ,  $\psi^\ell$ ) values of the topological descriptors for the first excited-state of the pyridinium-phenolate (PP), computed at the TDHF/6-31++G(2d,p) level of theory.  $\alpha$  is the pyridinium-phenolate central twist angle amplitude.



| $\alpha$ | $\phi_S^\ell$ | $\phi_S$ | $\varphi^\ell$ | $\varphi$ | $\psi^\ell$ | $\psi$ |
|----------|---------------|----------|----------------|-----------|-------------|--------|
| 0        | 0.62          | 0.66     | 0.69           | 0.67      | 0.47        | 0.50   |
| 1        | 0.62          | 0.66     | 0.69           | 0.67      | 0.47        | 0.50   |
| 2        | 0.62          | 0.66     | 0.69           | 0.67      | 0.47        | 0.50   |
| 3        | 0.62          | 0.66     | 0.69           | 0.67      | 0.47        | 0.50   |
| 4        | 0.62          | 0.66     | 0.69           | 0.67      | 0.47        | 0.50   |
| 5        | 0.62          | 0.66     | 0.69           | 0.67      | 0.47        | 0.50   |
| 6        | 0.62          | 0.66     | 0.69           | 0.67      | 0.47        | 0.50   |
| 7        | 0.61          | 0.66     | 0.70           | 0.67      | 0.46        | 0.50   |
| 8        | 0.61          | 0.66     | 0.70           | 0.67      | 0.46        | 0.50   |
| 9        | 0.61          | 0.66     | 0.70           | 0.67      | 0.46        | 0.50   |
| 10       | 0.61          | 0.66     | 0.70           | 0.67      | 0.46        | 0.50   |
| 11       | 0.61          | 0.66     | 0.70           | 0.68      | 0.46        | 0.49   |
| 12       | 0.61          | 0.65     | 0.70           | 0.68      | 0.46        | 0.49   |
| 13       | 0.61          | 0.65     | 0.70           | 0.68      | 0.46        | 0.49   |
| 14       | 0.61          | 0.65     | 0.70           | 0.68      | 0.46        | 0.49   |
| 15       | 0.61          | 0.65     | 0.71           | 0.68      | 0.45        | 0.49   |
| 16       | 0.60          | 0.65     | 0.71           | 0.68      | 0.45        | 0.49   |
| 17       | 0.60          | 0.64     | 0.71           | 0.69      | 0.45        | 0.48   |
| 18       | 0.60          | 0.64     | 0.71           | 0.69      | 0.45        | 0.48   |
| 19       | 0.60          | 0.64     | 0.71           | 0.69      | 0.45        | 0.48   |
| 20       | 0.60          | 0.64     | 0.72           | 0.69      | 0.44        | 0.48   |
| 21       | 0.59          | 0.64     | 0.72           | 0.70      | 0.44        | 0.47   |
| 22       | 0.59          | 0.63     | 0.72           | 0.70      | 0.44        | 0.47   |
| 23       | 0.59          | 0.63     | 0.73           | 0.70      | 0.43        | 0.47   |
| 24       | 0.59          | 0.63     | 0.73           | 0.71      | 0.43        | 0.46   |
| 25       | 0.58          | 0.62     | 0.73           | 0.71      | 0.43        | 0.46   |
| 26       | 0.58          | 0.62     | 0.74           | 0.71      | 0.42        | 0.46   |
| 27       | 0.58          | 0.62     | 0.74           | 0.72      | 0.42        | 0.45   |
| 28       | 0.57          | 0.61     | 0.74           | 0.72      | 0.42        | 0.45   |
| 29       | 0.57          | 0.61     | 0.75           | 0.72      | 0.41        | 0.45   |
| 30       | 0.57          | 0.61     | 0.75           | 0.73      | 0.41        | 0.44   |
| 31       | 0.56          | 0.60     | 0.75           | 0.73      | 0.41        | 0.44   |

Continued on next page

| $\alpha$ | $\phi_S^\ell$ | $\phi_S$ | $\varphi^\ell$ | $\varphi$ | $\psi^\ell$ | $\psi$ |
|----------|---------------|----------|----------------|-----------|-------------|--------|
| 32       | 0.56          | 0.60     | 0.76           | 0.73      | 0.40        | 0.44   |
| 33       | 0.55          | 0.59     | 0.76           | 0.74      | 0.40        | 0.43   |
| 34       | 0.55          | 0.59     | 0.76           | 0.74      | 0.40        | 0.43   |
| 35       | 0.55          | 0.59     | 0.77           | 0.75      | 0.39        | 0.42   |
| 36       | 0.54          | 0.58     | 0.77           | 0.75      | 0.39        | 0.42   |
| 37       | 0.54          | 0.58     | 0.78           | 0.76      | 0.39        | 0.41   |
| 38       | 0.53          | 0.57     | 0.78           | 0.76      | 0.38        | 0.41   |
| 39       | 0.53          | 0.57     | 0.79           | 0.76      | 0.38        | 0.41   |
| 40       | 0.52          | 0.56     | 0.79           | 0.77      | 0.37        | 0.40   |
| 41       | 0.51          | 0.56     | 0.80           | 0.77      | 0.36        | 0.40   |
| 42       | 0.51          | 0.55     | 0.80           | 0.78      | 0.36        | 0.39   |
| 43       | 0.50          | 0.54     | 0.81           | 0.78      | 0.35        | 0.39   |
| 44       | 0.50          | 0.54     | 0.81           | 0.79      | 0.35        | 0.38   |
| 45       | 0.49          | 0.53     | 0.82           | 0.79      | 0.34        | 0.38   |
| 46       | 0.48          | 0.53     | 0.82           | 0.80      | 0.34        | 0.37   |
| 47       | 0.48          | 0.52     | 0.82           | 0.80      | 0.34        | 0.37   |
| 48       | 0.47          | 0.51     | 0.83           | 0.81      | 0.33        | 0.36   |
| 49       | 0.46          | 0.51     | 0.83           | 0.81      | 0.32        | 0.36   |
| 50       | 0.46          | 0.50     | 0.84           | 0.82      | 0.32        | 0.35   |
| 51       | 0.45          | 0.49     | 0.84           | 0.82      | 0.31        | 0.34   |
| 52       | 0.44          | 0.48     | 0.85           | 0.83      | 0.30        | 0.33   |
| 53       | 0.44          | 0.48     | 0.85           | 0.83      | 0.30        | 0.33   |
| 54       | 0.43          | 0.47     | 0.86           | 0.84      | 0.30        | 0.32   |
| 55       | 0.42          | 0.46     | 0.86           | 0.84      | 0.29        | 0.32   |
| 56       | 0.42          | 0.45     | 0.87           | 0.85      | 0.29        | 0.31   |
| 57       | 0.41          | 0.44     | 0.87           | 0.85      | 0.28        | 0.30   |
| 58       | 0.40          | 0.44     | 0.88           | 0.86      | 0.27        | 0.30   |
| 59       | 0.39          | 0.43     | 0.88           | 0.86      | 0.27        | 0.30   |
| 60       | 0.38          | 0.42     | 0.89           | 0.87      | 0.26        | 0.29   |
| 61       | 0.38          | 0.41     | 0.89           | 0.87      | 0.26        | 0.28   |
| 62       | 0.37          | 0.40     | 0.90           | 0.88      | 0.25        | 0.27   |
| 63       | 0.36          | 0.39     | 0.90           | 0.88      | 0.24        | 0.27   |

Continued on next page

| $\alpha$ | $\phi_S^\ell$ | $\phi_S$ | $\varphi^\ell$ | $\varphi$ | $\psi^\ell$ | $\psi$ |
|----------|---------------|----------|----------------|-----------|-------------|--------|
| 64       | 0.35          | 0.38     | 0.91           | 0.89      | 0.23        | 0.26   |
| 65       | 0.34          | 0.37     | 0.91           | 0.89      | 0.23        | 0.25   |
| 66       | 0.33          | 0.37     | 0.92           | 0.89      | 0.22        | 0.25   |
| 67       | 0.32          | 0.36     | 0.92           | 0.90      | 0.21        | 0.24   |
| 68       | 0.32          | 0.35     | 0.92           | 0.90      | 0.21        | 0.24   |
| 69       | 0.31          | 0.34     | 0.93           | 0.91      | 0.20        | 0.23   |
| 70       | 0.30          | 0.33     | 0.93           | 0.91      | 0.20        | 0.22   |
| 71       | 0.29          | 0.32     | 0.93           | 0.91      | 0.19        | 0.22   |
| 72       | 0.28          | 0.31     | 0.94           | 0.92      | 0.18        | 0.21   |
| 73       | 0.27          | 0.30     | 0.94           | 0.92      | 0.18        | 0.20   |
| 74       | 0.26          | 0.29     | 0.94           | 0.92      | 0.17        | 0.19   |
| 75       | 0.25          | 0.28     | 0.95           | 0.93      | 0.16        | 0.19   |
| 76       | 0.24          | 0.27     | 0.95           | 0.93      | 0.16        | 0.18   |
| 77       | 0.24          | 0.26     | 0.95           | 0.93      | 0.16        | 0.17   |
| 78       | 0.23          | 0.25     | 0.95           | 0.93      | 0.15        | 0.17   |
| 79       | 0.22          | 0.25     | 0.95           | 0.94      | 0.14        | 0.17   |
| 80       | 0.21          | 0.24     | 0.96           | 0.94      | 0.14        | 0.16   |
| 81       | 0.20          | 0.23     | 0.96           | 0.94      | 0.13        | 0.15   |
| 82       | 0.20          | 0.22     | 0.96           | 0.94      | 0.13        | 0.15   |
| 83       | 0.19          | 0.21     | 0.96           | 0.94      | 0.12        | 0.14   |
| 84       | 0.18          | 0.21     | 0.96           | 0.94      | 0.12        | 0.14   |
| 85       | 0.18          | 0.20     | 0.96           | 0.95      | 0.12        | 0.13   |
| 86       | 0.17          | 0.19     | 0.96           | 0.95      | 0.11        | 0.13   |
| 87       | 0.17          | 0.19     | 0.96           | 0.95      | 0.11        | 0.13   |
| 88       | 0.16          | 0.19     | 0.96           | 0.95      | 0.11        | 0.13   |
| 89       | 0.16          | 0.18     | 0.96           | 0.95      | 0.11        | 0.12   |
| 90       | 0.16          | 0.18     | 0.96           | 0.95      | 0.11        | 0.12   |

Table S150: Reference ( $\phi_S$ ,  $\varphi$ ,  $\psi$ ) and approached ( $\phi_S^\ell$ ,  $\varphi^\ell$ ,  $\psi^\ell$ ) values of the topological descriptors for the first excited-state of the pyridinium-phenolate (PP), computed at the TDHF/6-31++G(d,p) level of theory.  $\alpha$  is the pyridinium-phenolate central twist angle amplitude.

| $\alpha$ | $\phi_S^\ell$ | $\phi_S$ | $\varphi^\ell$ | $\varphi$ | $\psi^\ell$ | $\psi$ |
|----------|---------------|----------|----------------|-----------|-------------|--------|
| 0        | 0.62          | 0.66     | 0.69           | 0.67      | 0.47        | 0.50   |
| 1        | 0.62          | 0.66     | 0.69           | 0.67      | 0.47        | 0.50   |
| 2        | 0.62          | 0.66     | 0.69           | 0.67      | 0.47        | 0.50   |
| 3        | 0.62          | 0.66     | 0.69           | 0.67      | 0.47        | 0.50   |
| 4        | 0.62          | 0.66     | 0.69           | 0.67      | 0.47        | 0.50   |
| 5        | 0.62          | 0.66     | 0.69           | 0.67      | 0.47        | 0.50   |
| 6        | 0.62          | 0.66     | 0.69           | 0.67      | 0.47        | 0.50   |
| 7        | 0.61          | 0.66     | 0.70           | 0.67      | 0.46        | 0.50   |
| 8        | 0.61          | 0.66     | 0.70           | 0.67      | 0.46        | 0.50   |
| 9        | 0.61          | 0.66     | 0.70           | 0.67      | 0.46        | 0.50   |
| 10       | 0.61          | 0.66     | 0.70           | 0.67      | 0.46        | 0.50   |
| 11       | 0.61          | 0.66     | 0.70           | 0.68      | 0.46        | 0.49   |
| 12       | 0.61          | 0.65     | 0.70           | 0.68      | 0.46        | 0.49   |
| 13       | 0.61          | 0.65     | 0.70           | 0.68      | 0.46        | 0.49   |
| 14       | 0.61          | 0.65     | 0.70           | 0.68      | 0.46        | 0.49   |
| 15       | 0.61          | 0.65     | 0.71           | 0.68      | 0.45        | 0.49   |
| 16       | 0.60          | 0.65     | 0.71           | 0.68      | 0.45        | 0.49   |
| 17       | 0.60          | 0.65     | 0.71           | 0.69      | 0.45        | 0.48   |
| 18       | 0.60          | 0.64     | 0.71           | 0.69      | 0.45        | 0.48   |
| 19       | 0.60          | 0.64     | 0.71           | 0.69      | 0.45        | 0.48   |
| 20       | 0.60          | 0.64     | 0.72           | 0.69      | 0.44        | 0.48   |
| 21       | 0.59          | 0.64     | 0.72           | 0.70      | 0.44        | 0.47   |
| 22       | 0.59          | 0.63     | 0.72           | 0.70      | 0.44        | 0.47   |
| 23       | 0.59          | 0.63     | 0.73           | 0.70      | 0.43        | 0.47   |
| 24       | 0.59          | 0.63     | 0.73           | 0.71      | 0.43        | 0.46   |
| 25       | 0.58          | 0.62     | 0.73           | 0.71      | 0.43        | 0.46   |
| 26       | 0.58          | 0.62     | 0.74           | 0.71      | 0.42        | 0.46   |
| 27       | 0.58          | 0.62     | 0.74           | 0.72      | 0.42        | 0.45   |
| 28       | 0.57          | 0.61     | 0.74           | 0.72      | 0.42        | 0.45   |
| 29       | 0.57          | 0.61     | 0.75           | 0.72      | 0.41        | 0.45   |
| 30       | 0.57          | 0.61     | 0.75           | 0.73      | 0.41        | 0.44   |
| 31       | 0.56          | 0.60     | 0.75           | 0.73      | 0.41        | 0.44   |

Continued on next page

| $\alpha$ | $\phi_S^\ell$ | $\phi_S$ | $\varphi^\ell$ | $\varphi$ | $\psi^\ell$ | $\psi$ |
|----------|---------------|----------|----------------|-----------|-------------|--------|
| 32       | 0.56          | 0.60     | 0.76           | 0.73      | 0.40        | 0.44   |
| 33       | 0.55          | 0.60     | 0.76           | 0.74      | 0.40        | 0.43   |
| 34       | 0.55          | 0.59     | 0.76           | 0.74      | 0.40        | 0.43   |
| 35       | 0.55          | 0.59     | 0.77           | 0.75      | 0.39        | 0.42   |
| 36       | 0.54          | 0.58     | 0.77           | 0.75      | 0.39        | 0.42   |
| 37       | 0.54          | 0.58     | 0.78           | 0.76      | 0.39        | 0.41   |
| 38       | 0.53          | 0.57     | 0.78           | 0.76      | 0.38        | 0.41   |
| 39       | 0.53          | 0.57     | 0.79           | 0.76      | 0.38        | 0.41   |
| 40       | 0.52          | 0.56     | 0.79           | 0.77      | 0.37        | 0.40   |
| 41       | 0.51          | 0.56     | 0.80           | 0.77      | 0.36        | 0.40   |
| 42       | 0.51          | 0.55     | 0.80           | 0.78      | 0.36        | 0.39   |
| 43       | 0.50          | 0.54     | 0.81           | 0.78      | 0.35        | 0.39   |
| 44       | 0.50          | 0.54     | 0.81           | 0.79      | 0.35        | 0.38   |
| 45       | 0.49          | 0.53     | 0.82           | 0.79      | 0.34        | 0.38   |
| 46       | 0.48          | 0.53     | 0.82           | 0.80      | 0.34        | 0.37   |
| 47       | 0.48          | 0.52     | 0.82           | 0.80      | 0.34        | 0.37   |
| 48       | 0.47          | 0.51     | 0.83           | 0.81      | 0.33        | 0.36   |
| 49       | 0.46          | 0.51     | 0.83           | 0.81      | 0.32        | 0.36   |
| 50       | 0.46          | 0.50     | 0.84           | 0.82      | 0.32        | 0.35   |
| 51       | 0.45          | 0.49     | 0.84           | 0.82      | 0.31        | 0.34   |
| 52       | 0.44          | 0.48     | 0.85           | 0.83      | 0.30        | 0.33   |
| 53       | 0.44          | 0.48     | 0.85           | 0.83      | 0.30        | 0.33   |
| 54       | 0.43          | 0.47     | 0.86           | 0.84      | 0.30        | 0.32   |
| 55       | 0.42          | 0.46     | 0.86           | 0.84      | 0.29        | 0.32   |
| 56       | 0.42          | 0.45     | 0.87           | 0.85      | 0.29        | 0.31   |
| 57       | 0.41          | 0.44     | 0.87           | 0.85      | 0.28        | 0.30   |
| 58       | 0.40          | 0.44     | 0.88           | 0.86      | 0.27        | 0.30   |
| 59       | 0.39          | 0.43     | 0.88           | 0.86      | 0.27        | 0.30   |
| 60       | 0.38          | 0.42     | 0.89           | 0.87      | 0.26        | 0.29   |
| 61       | 0.38          | 0.41     | 0.89           | 0.87      | 0.26        | 0.28   |
| 62       | 0.37          | 0.40     | 0.90           | 0.88      | 0.25        | 0.27   |
| 63       | 0.36          | 0.39     | 0.90           | 0.88      | 0.24        | 0.27   |

Continued on next page

| $\alpha$ | $\phi_S^\ell$ | $\phi_S$ | $\varphi^\ell$ | $\varphi$ | $\psi^\ell$ | $\psi$ |
|----------|---------------|----------|----------------|-----------|-------------|--------|
| 64       | 0.35          | 0.38     | 0.91           | 0.89      | 0.23        | 0.26   |
| 65       | 0.34          | 0.37     | 0.91           | 0.89      | 0.23        | 0.25   |
| 66       | 0.33          | 0.37     | 0.92           | 0.89      | 0.22        | 0.25   |
| 67       | 0.33          | 0.36     | 0.92           | 0.90      | 0.22        | 0.24   |
| 68       | 0.32          | 0.35     | 0.92           | 0.90      | 0.21        | 0.24   |
| 69       | 0.31          | 0.34     | 0.93           | 0.91      | 0.20        | 0.23   |
| 70       | 0.30          | 0.33     | 0.93           | 0.91      | 0.20        | 0.22   |
| 71       | 0.29          | 0.32     | 0.93           | 0.91      | 0.19        | 0.22   |
| 72       | 0.28          | 0.31     | 0.94           | 0.92      | 0.18        | 0.21   |
| 73       | 0.27          | 0.30     | 0.94           | 0.92      | 0.18        | 0.20   |
| 74       | 0.26          | 0.29     | 0.94           | 0.92      | 0.17        | 0.19   |
| 75       | 0.26          | 0.28     | 0.95           | 0.93      | 0.17        | 0.19   |
| 76       | 0.25          | 0.27     | 0.95           | 0.93      | 0.16        | 0.18   |
| 77       | 0.24          | 0.26     | 0.95           | 0.93      | 0.16        | 0.17   |
| 78       | 0.23          | 0.25     | 0.95           | 0.93      | 0.15        | 0.17   |
| 79       | 0.22          | 0.25     | 0.95           | 0.94      | 0.14        | 0.17   |
| 80       | 0.21          | 0.24     | 0.96           | 0.94      | 0.14        | 0.16   |
| 81       | 0.21          | 0.23     | 0.96           | 0.94      | 0.14        | 0.15   |
| 82       | 0.20          | 0.22     | 0.96           | 0.94      | 0.13        | 0.15   |
| 83       | 0.19          | 0.21     | 0.96           | 0.94      | 0.12        | 0.14   |
| 84       | 0.19          | 0.21     | 0.96           | 0.94      | 0.12        | 0.14   |
| 85       | 0.18          | 0.20     | 0.96           | 0.95      | 0.12        | 0.13   |
| 86       | 0.17          | 0.19     | 0.96           | 0.95      | 0.11        | 0.13   |
| 87       | 0.17          | 0.19     | 0.96           | 0.95      | 0.11        | 0.13   |
| 88       | 0.16          | 0.19     | 0.96           | 0.95      | 0.11        | 0.13   |
| 89       | 0.16          | 0.18     | 0.96           | 0.95      | 0.11        | 0.12   |
| 90       | 0.16          | 0.18     | 0.96           | 0.95      | 0.11        | 0.12   |

Table S151: Reference ( $\phi_S$ ,  $\varphi$ ,  $\psi$ ) and approached ( $\phi_S^\ell$ ,  $\varphi^\ell$ ,  $\psi^\ell$ ) values of the topological descriptors for the first excited-state of the pyridinium-phenolate (PP), computed at the TDHF/6-31+G(d,p) level of theory.  $\alpha$  is the pyridinium-phenolate central twist angle amplitude.

| $\alpha$ | $\phi_S^\ell$ | $\phi_S$ | $\varphi^\ell$ | $\varphi$ | $\psi^\ell$ | $\psi$ |
|----------|---------------|----------|----------------|-----------|-------------|--------|
| 0        | 0.62          | 0.66     | 0.69           | 0.67      | 0.47        | 0.50   |
| 1        | 0.62          | 0.66     | 0.69           | 0.67      | 0.47        | 0.50   |
| 2        | 0.62          | 0.66     | 0.69           | 0.67      | 0.47        | 0.50   |
| 3        | 0.62          | 0.66     | 0.69           | 0.67      | 0.47        | 0.50   |
| 4        | 0.62          | 0.66     | 0.69           | 0.67      | 0.47        | 0.50   |
| 5        | 0.62          | 0.66     | 0.69           | 0.67      | 0.47        | 0.50   |
| 6        | 0.62          | 0.66     | 0.69           | 0.67      | 0.47        | 0.50   |
| 7        | 0.61          | 0.66     | 0.70           | 0.67      | 0.46        | 0.50   |
| 8        | 0.61          | 0.66     | 0.70           | 0.67      | 0.46        | 0.50   |
| 9        | 0.61          | 0.66     | 0.70           | 0.67      | 0.46        | 0.50   |
| 10       | 0.61          | 0.66     | 0.70           | 0.67      | 0.46        | 0.50   |
| 11       | 0.61          | 0.66     | 0.70           | 0.68      | 0.46        | 0.49   |
| 12       | 0.61          | 0.65     | 0.70           | 0.68      | 0.46        | 0.49   |
| 13       | 0.61          | 0.65     | 0.70           | 0.68      | 0.46        | 0.49   |
| 14       | 0.61          | 0.65     | 0.70           | 0.68      | 0.46        | 0.49   |
| 15       | 0.61          | 0.65     | 0.71           | 0.68      | 0.45        | 0.49   |
| 16       | 0.60          | 0.65     | 0.71           | 0.68      | 0.45        | 0.49   |
| 17       | 0.60          | 0.64     | 0.71           | 0.69      | 0.45        | 0.48   |
| 18       | 0.60          | 0.64     | 0.71           | 0.69      | 0.45        | 0.48   |
| 19       | 0.60          | 0.64     | 0.71           | 0.69      | 0.45        | 0.48   |
| 20       | 0.60          | 0.64     | 0.72           | 0.69      | 0.44        | 0.48   |
| 21       | 0.59          | 0.64     | 0.72           | 0.70      | 0.44        | 0.47   |
| 22       | 0.59          | 0.63     | 0.72           | 0.70      | 0.44        | 0.47   |
| 23       | 0.59          | 0.63     | 0.73           | 0.70      | 0.43        | 0.47   |
| 24       | 0.59          | 0.63     | 0.73           | 0.71      | 0.43        | 0.46   |
| 25       | 0.58          | 0.62     | 0.73           | 0.71      | 0.43        | 0.46   |
| 26       | 0.58          | 0.62     | 0.74           | 0.71      | 0.42        | 0.46   |
| 27       | 0.58          | 0.62     | 0.74           | 0.72      | 0.42        | 0.45   |
| 28       | 0.57          | 0.61     | 0.74           | 0.72      | 0.42        | 0.45   |
| 29       | 0.57          | 0.61     | 0.75           | 0.72      | 0.41        | 0.45   |
| 30       | 0.57          | 0.61     | 0.75           | 0.73      | 0.41        | 0.44   |
| 31       | 0.56          | 0.60     | 0.75           | 0.73      | 0.41        | 0.44   |

Continued on next page

| $\alpha$ | $\phi_S^\ell$ | $\phi_S$ | $\varphi^\ell$ | $\varphi$ | $\psi^\ell$ | $\psi$ |
|----------|---------------|----------|----------------|-----------|-------------|--------|
| 32       | 0.56          | 0.60     | 0.76           | 0.73      | 0.40        | 0.44   |
| 33       | 0.55          | 0.59     | 0.76           | 0.74      | 0.40        | 0.43   |
| 34       | 0.55          | 0.59     | 0.76           | 0.74      | 0.40        | 0.43   |
| 35       | 0.55          | 0.59     | 0.77           | 0.75      | 0.39        | 0.42   |
| 36       | 0.54          | 0.58     | 0.77           | 0.75      | 0.39        | 0.42   |
| 37       | 0.54          | 0.58     | 0.78           | 0.76      | 0.39        | 0.41   |
| 38       | 0.53          | 0.57     | 0.78           | 0.76      | 0.38        | 0.41   |
| 39       | 0.53          | 0.57     | 0.79           | 0.76      | 0.38        | 0.41   |
| 40       | 0.52          | 0.56     | 0.79           | 0.77      | 0.37        | 0.40   |
| 41       | 0.51          | 0.56     | 0.80           | 0.77      | 0.36        | 0.40   |
| 42       | 0.51          | 0.55     | 0.80           | 0.78      | 0.36        | 0.39   |
| 43       | 0.50          | 0.54     | 0.81           | 0.78      | 0.35        | 0.39   |
| 44       | 0.50          | 0.54     | 0.81           | 0.79      | 0.35        | 0.38   |
| 45       | 0.49          | 0.53     | 0.82           | 0.79      | 0.34        | 0.38   |
| 46       | 0.48          | 0.53     | 0.82           | 0.80      | 0.34        | 0.37   |
| 47       | 0.48          | 0.52     | 0.82           | 0.80      | 0.34        | 0.37   |
| 48       | 0.47          | 0.51     | 0.83           | 0.81      | 0.33        | 0.36   |
| 49       | 0.46          | 0.51     | 0.83           | 0.81      | 0.32        | 0.36   |
| 50       | 0.46          | 0.50     | 0.84           | 0.82      | 0.32        | 0.35   |
| 51       | 0.45          | 0.49     | 0.84           | 0.82      | 0.31        | 0.34   |
| 52       | 0.44          | 0.48     | 0.85           | 0.83      | 0.30        | 0.33   |
| 53       | 0.44          | 0.48     | 0.85           | 0.83      | 0.30        | 0.33   |
| 54       | 0.43          | 0.47     | 0.86           | 0.84      | 0.30        | 0.32   |
| 55       | 0.42          | 0.46     | 0.86           | 0.84      | 0.29        | 0.32   |
| 56       | 0.42          | 0.45     | 0.87           | 0.85      | 0.29        | 0.31   |
| 57       | 0.41          | 0.44     | 0.87           | 0.85      | 0.28        | 0.30   |
| 58       | 0.40          | 0.44     | 0.88           | 0.86      | 0.27        | 0.30   |
| 59       | 0.39          | 0.43     | 0.88           | 0.86      | 0.27        | 0.30   |
| 60       | 0.38          | 0.42     | 0.89           | 0.87      | 0.26        | 0.29   |
| 61       | 0.38          | 0.41     | 0.89           | 0.87      | 0.26        | 0.28   |
| 62       | 0.37          | 0.40     | 0.90           | 0.88      | 0.25        | 0.27   |
| 63       | 0.36          | 0.39     | 0.90           | 0.88      | 0.24        | 0.27   |

Continued on next page



| $\alpha$ | $\phi_S^\ell$ | $\phi_S$ | $\varphi^\ell$ | $\varphi$ | $\psi^\ell$ | $\psi$ |
|----------|---------------|----------|----------------|-----------|-------------|--------|
| 64       | 0.35          | 0.38     | 0.91           | 0.89      | 0.23        | 0.26   |
| 65       | 0.34          | 0.37     | 0.91           | 0.89      | 0.23        | 0.25   |
| 66       | 0.33          | 0.36     | 0.92           | 0.89      | 0.22        | 0.24   |
| 67       | 0.33          | 0.36     | 0.92           | 0.90      | 0.22        | 0.24   |
| 68       | 0.32          | 0.35     | 0.92           | 0.90      | 0.21        | 0.24   |
| 69       | 0.31          | 0.34     | 0.93           | 0.91      | 0.20        | 0.23   |
| 70       | 0.30          | 0.33     | 0.93           | 0.91      | 0.20        | 0.22   |
| 71       | 0.29          | 0.32     | 0.93           | 0.91      | 0.19        | 0.22   |
| 72       | 0.28          | 0.31     | 0.94           | 0.92      | 0.18        | 0.21   |
| 73       | 0.27          | 0.30     | 0.94           | 0.92      | 0.18        | 0.20   |
| 74       | 0.26          | 0.29     | 0.94           | 0.92      | 0.17        | 0.19   |
| 75       | 0.26          | 0.28     | 0.95           | 0.93      | 0.17        | 0.19   |
| 76       | 0.25          | 0.27     | 0.95           | 0.93      | 0.16        | 0.18   |
| 77       | 0.24          | 0.26     | 0.95           | 0.93      | 0.16        | 0.17   |
| 78       | 0.23          | 0.25     | 0.95           | 0.93      | 0.15        | 0.17   |
| 79       | 0.22          | 0.25     | 0.95           | 0.94      | 0.14        | 0.17   |
| 80       | 0.21          | 0.24     | 0.96           | 0.94      | 0.14        | 0.16   |
| 81       | 0.21          | 0.23     | 0.96           | 0.94      | 0.14        | 0.15   |
| 82       | 0.20          | 0.22     | 0.96           | 0.94      | 0.13        | 0.15   |
| 83       | 0.19          | 0.21     | 0.96           | 0.94      | 0.12        | 0.14   |
| 84       | 0.19          | 0.21     | 0.96           | 0.94      | 0.12        | 0.14   |
| 85       | 0.18          | 0.20     | 0.96           | 0.95      | 0.12        | 0.13   |
| 86       | 0.17          | 0.19     | 0.96           | 0.95      | 0.11        | 0.13   |
| 87       | 0.17          | 0.19     | 0.96           | 0.95      | 0.11        | 0.13   |
| 88       | 0.16          | 0.18     | 0.96           | 0.95      | 0.11        | 0.12   |
| 89       | 0.16          | 0.18     | 0.96           | 0.95      | 0.11        | 0.12   |
| 90       | 0.16          | 0.18     | 0.96           | 0.95      | 0.11        | 0.12   |

Table S152: Reference ( $\phi_S$ ,  $\varphi$ ,  $\psi$ ) and approached ( $\phi_S^\ell$ ,  $\varphi^\ell$ ,  $\psi^\ell$ ) values of the topological descriptors for the first excited-state of the pyridinium-phenolate (PP), computed at the TDHF/6-31+G(d) level of theory.  $\alpha$  is the pyridinium-phenolate central twist angle amplitude.

| $\alpha$ | $\phi_S^\ell$ | $\phi_S$ | $\varphi^\ell$ | $\varphi$ | $\psi^\ell$ | $\psi$ |
|----------|---------------|----------|----------------|-----------|-------------|--------|
| 0        | 0.64          | 0.69     | 0.69           | 0.65      | 0.48        | 0.52   |
| 1        | 0.64          | 0.69     | 0.69           | 0.65      | 0.48        | 0.52   |
| 2        | 0.64          | 0.69     | 0.69           | 0.65      | 0.48        | 0.52   |
| 3        | 0.64          | 0.69     | 0.69           | 0.65      | 0.48        | 0.52   |
| 4        | 0.64          | 0.69     | 0.69           | 0.65      | 0.48        | 0.52   |
| 5        | 0.64          | 0.69     | 0.69           | 0.65      | 0.48        | 0.52   |
| 6        | 0.64          | 0.68     | 0.69           | 0.66      | 0.48        | 0.51   |
| 7        | 0.64          | 0.68     | 0.69           | 0.66      | 0.48        | 0.51   |
| 8        | 0.64          | 0.68     | 0.70           | 0.66      | 0.47        | 0.51   |
| 9        | 0.64          | 0.68     | 0.70           | 0.66      | 0.47        | 0.51   |
| 10       | 0.63          | 0.68     | 0.70           | 0.66      | 0.47        | 0.51   |
| 11       | 0.63          | 0.68     | 0.70           | 0.66      | 0.47        | 0.51   |
| 12       | 0.63          | 0.68     | 0.70           | 0.66      | 0.47        | 0.51   |
| 13       | 0.63          | 0.68     | 0.70           | 0.66      | 0.47        | 0.51   |
| 14       | 0.63          | 0.67     | 0.70           | 0.67      | 0.47        | 0.50   |
| 15       | 0.63          | 0.67     | 0.71           | 0.67      | 0.46        | 0.50   |
| 16       | 0.63          | 0.67     | 0.71           | 0.67      | 0.46        | 0.50   |
| 17       | 0.62          | 0.67     | 0.71           | 0.67      | 0.46        | 0.50   |
| 18       | 0.62          | 0.67     | 0.71           | 0.68      | 0.46        | 0.50   |
| 19       | 0.62          | 0.66     | 0.71           | 0.68      | 0.46        | 0.49   |
| 20       | 0.62          | 0.66     | 0.72           | 0.68      | 0.45        | 0.49   |
| 21       | 0.62          | 0.66     | 0.72           | 0.68      | 0.45        | 0.49   |
| 22       | 0.61          | 0.66     | 0.72           | 0.69      | 0.45        | 0.49   |
| 23       | 0.61          | 0.65     | 0.73           | 0.69      | 0.44        | 0.48   |
| 24       | 0.61          | 0.65     | 0.73           | 0.69      | 0.44        | 0.48   |
| 25       | 0.61          | 0.65     | 0.73           | 0.70      | 0.44        | 0.48   |
| 26       | 0.60          | 0.64     | 0.73           | 0.70      | 0.44        | 0.47   |
| 27       | 0.60          | 0.64     | 0.74           | 0.70      | 0.43        | 0.47   |
| 28       | 0.60          | 0.64     | 0.74           | 0.71      | 0.43        | 0.47   |
| 29       | 0.59          | 0.63     | 0.74           | 0.71      | 0.43        | 0.46   |
| 30       | 0.59          | 0.63     | 0.75           | 0.72      | 0.42        | 0.46   |
| 31       | 0.59          | 0.62     | 0.75           | 0.72      | 0.42        | 0.45   |

Continued on next page

| $\alpha$ | $\phi_S^\ell$ | $\phi_S$ | $\varphi^\ell$ | $\varphi$ | $\psi^\ell$ | $\psi$ |
|----------|---------------|----------|----------------|-----------|-------------|--------|
| 32       | 0.58          | 0.62     | 0.76           | 0.72      | 0.41        | 0.45   |
| 33       | 0.58          | 0.62     | 0.76           | 0.73      | 0.41        | 0.45   |
| 34       | 0.57          | 0.61     | 0.76           | 0.73      | 0.41        | 0.44   |
| 35       | 0.57          | 0.61     | 0.77           | 0.74      | 0.41        | 0.44   |
| 36       | 0.57          | 0.60     | 0.77           | 0.74      | 0.41        | 0.43   |
| 37       | 0.56          | 0.60     | 0.78           | 0.75      | 0.40        | 0.43   |
| 38       | 0.56          | 0.59     | 0.78           | 0.75      | 0.40        | 0.42   |
| 39       | 0.55          | 0.59     | 0.79           | 0.75      | 0.39        | 0.42   |
| 40       | 0.54          | 0.58     | 0.79           | 0.76      | 0.38        | 0.41   |
| 41       | 0.54          | 0.57     | 0.80           | 0.76      | 0.38        | 0.41   |
| 42       | 0.53          | 0.57     | 0.80           | 0.77      | 0.37        | 0.41   |
| 43       | 0.53          | 0.56     | 0.81           | 0.77      | 0.37        | 0.40   |
| 44       | 0.52          | 0.56     | 0.81           | 0.78      | 0.36        | 0.40   |
| 45       | 0.51          | 0.55     | 0.82           | 0.78      | 0.35        | 0.39   |
| 46       | 0.51          | 0.54     | 0.82           | 0.79      | 0.35        | 0.38   |
| 47       | 0.50          | 0.54     | 0.82           | 0.79      | 0.35        | 0.38   |
| 48       | 0.50          | 0.53     | 0.83           | 0.80      | 0.35        | 0.37   |
| 49       | 0.49          | 0.52     | 0.83           | 0.81      | 0.34        | 0.36   |
| 50       | 0.48          | 0.52     | 0.84           | 0.81      | 0.33        | 0.36   |
| 51       | 0.47          | 0.51     | 0.84           | 0.82      | 0.32        | 0.35   |
| 52       | 0.47          | 0.50     | 0.85           | 0.82      | 0.32        | 0.35   |
| 53       | 0.46          | 0.49     | 0.85           | 0.83      | 0.32        | 0.34   |
| 54       | 0.45          | 0.48     | 0.86           | 0.83      | 0.31        | 0.33   |
| 55       | 0.44          | 0.48     | 0.86           | 0.84      | 0.30        | 0.33   |
| 56       | 0.44          | 0.47     | 0.87           | 0.84      | 0.30        | 0.32   |
| 57       | 0.43          | 0.46     | 0.87           | 0.85      | 0.29        | 0.32   |
| 58       | 0.42          | 0.45     | 0.88           | 0.85      | 0.28        | 0.31   |
| 59       | 0.41          | 0.44     | 0.88           | 0.86      | 0.28        | 0.30   |
| 60       | 0.40          | 0.43     | 0.89           | 0.86      | 0.27        | 0.30   |
| 61       | 0.39          | 0.42     | 0.89           | 0.87      | 0.26        | 0.29   |
| 62       | 0.39          | 0.41     | 0.90           | 0.87      | 0.26        | 0.28   |
| 63       | 0.38          | 0.41     | 0.90           | 0.88      | 0.25        | 0.28   |

Continued on next page

| $\alpha$ | $\phi_S^\ell$ | $\phi_S$ | $\varphi^\ell$ | $\varphi$ | $\psi^\ell$ | $\psi$ |
|----------|---------------|----------|----------------|-----------|-------------|--------|
| 64       | 0.37          | 0.40     | 0.91           | 0.88      | 0.25        | 0.27   |
| 65       | 0.36          | 0.39     | 0.91           | 0.89      | 0.24        | 0.26   |
| 66       | 0.35          | 0.38     | 0.92           | 0.89      | 0.23        | 0.26   |
| 67       | 0.34          | 0.37     | 0.92           | 0.90      | 0.23        | 0.25   |
| 68       | 0.33          | 0.36     | 0.92           | 0.90      | 0.22        | 0.24   |
| 69       | 0.32          | 0.35     | 0.93           | 0.90      | 0.21        | 0.24   |
| 70       | 0.31          | 0.34     | 0.93           | 0.91      | 0.20        | 0.23   |
| 71       | 0.30          | 0.33     | 0.94           | 0.91      | 0.20        | 0.22   |
| 72       | 0.28          | 0.32     | 0.94           | 0.91      | 0.18        | 0.22   |
| 73       | 0.27          | 0.31     | 0.94           | 0.92      | 0.18        | 0.21   |
| 74       | 0.26          | 0.30     | 0.95           | 0.92      | 0.17        | 0.20   |
| 75       | 0.25          | 0.29     | 0.95           | 0.93      | 0.16        | 0.19   |
| 76       | 0.24          | 0.28     | 0.95           | 0.93      | 0.16        | 0.19   |
| 77       | 0.23          | 0.27     | 0.95           | 0.93      | 0.15        | 0.18   |
| 78       | 0.22          | 0.26     | 0.96           | 0.93      | 0.14        | 0.17   |
| 79       | 0.21          | 0.25     | 0.96           | 0.94      | 0.14        | 0.17   |
| 80       | 0.21          | 0.24     | 0.96           | 0.94      | 0.14        | 0.16   |
| 81       | 0.20          | 0.23     | 0.96           | 0.94      | 0.13        | 0.15   |
| 82       | 0.19          | 0.22     | 0.96           | 0.94      | 0.12        | 0.15   |
| 83       | 0.18          | 0.22     | 0.97           | 0.94      | 0.12        | 0.15   |
| 84       | 0.17          | 0.21     | 0.97           | 0.95      | 0.11        | 0.14   |
| 85       | 0.16          | 0.20     | 0.97           | 0.95      | 0.10        | 0.13   |
| 86       | 0.16          | 0.20     | 0.97           | 0.95      | 0.10        | 0.13   |
| 87       | 0.15          | 0.19     | 0.97           | 0.95      | 0.10        | 0.13   |
| 88       | 0.14          | 0.19     | 0.97           | 0.95      | 0.09        | 0.13   |
| 89       | 0.14          | 0.18     | 0.97           | 0.95      | 0.09        | 0.12   |
| 90       | 0.14          | 0.18     | 0.97           | 0.95      | 0.09        | 0.12   |

Table S153: Reference ( $\phi_S$ ,  $\varphi$ ,  $\psi$ ) and approached ( $\phi_S^\ell$ ,  $\varphi^\ell$ ,  $\psi^\ell$ ) values of the topological descriptors for the first excited-state of the pyridinium-phenolate (PP), computed at the TDHF/6-31G(d) level of theory.  $\alpha$  is the pyridinium-phenolate central twist angle amplitude.

| $\alpha$ | $\phi_S^\ell$ | $\phi_S$ | $\varphi^\ell$ | $\varphi$ | $\psi^\ell$ | $\psi$ |
|----------|---------------|----------|----------------|-----------|-------------|--------|
| 0        | 0.61          | 0.65     | 0.70           | 0.68      | 0.46        | 0.49   |
| 1        | 0.61          | 0.65     | 0.70           | 0.68      | 0.46        | 0.49   |
| 2        | 0.61          | 0.65     | 0.70           | 0.68      | 0.46        | 0.49   |
| 3        | 0.61          | 0.65     | 0.70           | 0.68      | 0.46        | 0.49   |
| 4        | 0.61          | 0.65     | 0.70           | 0.68      | 0.46        | 0.49   |
| 5        | 0.61          | 0.65     | 0.70           | 0.68      | 0.46        | 0.49   |
| 6        | 0.61          | 0.65     | 0.70           | 0.68      | 0.46        | 0.49   |
| 7        | 0.61          | 0.65     | 0.70           | 0.68      | 0.46        | 0.49   |
| 8        | 0.60          | 0.65     | 0.70           | 0.68      | 0.45        | 0.49   |
| 9        | 0.60          | 0.64     | 0.71           | 0.68      | 0.45        | 0.48   |
| 10       | 0.60          | 0.64     | 0.71           | 0.69      | 0.45        | 0.48   |
| 11       | 0.60          | 0.64     | 0.71           | 0.69      | 0.45        | 0.48   |
| 12       | 0.60          | 0.64     | 0.71           | 0.69      | 0.45        | 0.48   |
| 13       | 0.60          | 0.64     | 0.71           | 0.69      | 0.45        | 0.48   |
| 14       | 0.60          | 0.64     | 0.71           | 0.69      | 0.45        | 0.48   |
| 15       | 0.60          | 0.64     | 0.71           | 0.69      | 0.45        | 0.48   |
| 16       | 0.59          | 0.63     | 0.72           | 0.70      | 0.44        | 0.47   |
| 17       | 0.59          | 0.63     | 0.72           | 0.70      | 0.44        | 0.47   |
| 18       | 0.59          | 0.63     | 0.72           | 0.70      | 0.44        | 0.47   |
| 19       | 0.59          | 0.63     | 0.72           | 0.70      | 0.44        | 0.47   |
| 20       | 0.59          | 0.62     | 0.73           | 0.71      | 0.43        | 0.46   |
| 21       | 0.58          | 0.62     | 0.73           | 0.71      | 0.43        | 0.46   |
| 22       | 0.58          | 0.62     | 0.73           | 0.71      | 0.43        | 0.46   |
| 23       | 0.58          | 0.62     | 0.73           | 0.71      | 0.43        | 0.46   |
| 24       | 0.57          | 0.61     | 0.74           | 0.72      | 0.42        | 0.45   |
| 25       | 0.57          | 0.61     | 0.74           | 0.72      | 0.42        | 0.45   |
| 26       | 0.57          | 0.61     | 0.74           | 0.72      | 0.42        | 0.45   |
| 27       | 0.57          | 0.60     | 0.75           | 0.73      | 0.41        | 0.44   |
| 28       | 0.56          | 0.60     | 0.75           | 0.73      | 0.41        | 0.44   |
| 29       | 0.56          | 0.60     | 0.75           | 0.73      | 0.41        | 0.44   |
| 30       | 0.56          | 0.59     | 0.76           | 0.74      | 0.40        | 0.43   |
| 31       | 0.55          | 0.59     | 0.76           | 0.74      | 0.40        | 0.43   |

Continued on next page

| $\alpha$ | $\phi_S^\ell$ | $\phi_S$ | $\varphi^\ell$ | $\varphi$ | $\psi^\ell$ | $\psi$ |
|----------|---------------|----------|----------------|-----------|-------------|--------|
| 32       | 0.55          | 0.59     | 0.76           | 0.75      | 0.40        | 0.42   |
| 33       | 0.54          | 0.58     | 0.77           | 0.75      | 0.39        | 0.42   |
| 34       | 0.54          | 0.58     | 0.77           | 0.75      | 0.39        | 0.42   |
| 35       | 0.53          | 0.57     | 0.78           | 0.76      | 0.38        | 0.41   |
| 36       | 0.53          | 0.57     | 0.78           | 0.76      | 0.38        | 0.41   |
| 37       | 0.52          | 0.56     | 0.78           | 0.77      | 0.37        | 0.40   |
| 38       | 0.52          | 0.56     | 0.79           | 0.77      | 0.37        | 0.40   |
| 39       | 0.51          | 0.55     | 0.79           | 0.77      | 0.36        | 0.39   |
| 40       | 0.51          | 0.55     | 0.80           | 0.78      | 0.36        | 0.39   |
| 41       | 0.50          | 0.54     | 0.80           | 0.78      | 0.36        | 0.39   |
| 42       | 0.50          | 0.54     | 0.81           | 0.79      | 0.35        | 0.38   |
| 43       | 0.49          | 0.53     | 0.81           | 0.79      | 0.35        | 0.38   |
| 44       | 0.48          | 0.52     | 0.82           | 0.80      | 0.34        | 0.37   |
| 45       | 0.48          | 0.52     | 0.82           | 0.80      | 0.34        | 0.37   |
| 46       | 0.47          | 0.51     | 0.83           | 0.81      | 0.33        | 0.36   |
| 47       | 0.47          | 0.51     | 0.83           | 0.81      | 0.33        | 0.36   |
| 48       | 0.46          | 0.50     | 0.84           | 0.82      | 0.32        | 0.35   |
| 49       | 0.45          | 0.49     | 0.84           | 0.82      | 0.31        | 0.34   |
| 50       | 0.45          | 0.49     | 0.85           | 0.83      | 0.31        | 0.34   |
| 51       | 0.44          | 0.48     | 0.85           | 0.83      | 0.30        | 0.33   |
| 52       | 0.43          | 0.47     | 0.86           | 0.84      | 0.30        | 0.32   |
| 53       | 0.43          | 0.46     | 0.86           | 0.84      | 0.30        | 0.32   |
| 54       | 0.42          | 0.46     | 0.86           | 0.85      | 0.29        | 0.32   |
| 55       | 0.41          | 0.45     | 0.87           | 0.85      | 0.28        | 0.31   |
| 56       | 0.40          | 0.44     | 0.87           | 0.86      | 0.27        | 0.30   |
| 57       | 0.40          | 0.43     | 0.88           | 0.86      | 0.27        | 0.30   |
| 58       | 0.39          | 0.42     | 0.89           | 0.87      | 0.26        | 0.29   |
| 59       | 0.38          | 0.42     | 0.89           | 0.87      | 0.26        | 0.29   |
| 60       | 0.37          | 0.41     | 0.90           | 0.87      | 0.25        | 0.28   |
| 61       | 0.36          | 0.40     | 0.90           | 0.88      | 0.24        | 0.27   |
| 62       | 0.35          | 0.39     | 0.91           | 0.88      | 0.23        | 0.27   |
| 63       | 0.35          | 0.38     | 0.91           | 0.89      | 0.23        | 0.26   |

Continued on next page

| $\alpha$ | $\phi_S^\ell$ | $\phi_S$ | $\varphi^\ell$ | $\varphi$ | $\psi^\ell$ | $\psi$ |
|----------|---------------|----------|----------------|-----------|-------------|--------|
| 64       | 0.34          | 0.37     | 0.92           | 0.89      | 0.23        | 0.25   |
| 65       | 0.33          | 0.36     | 0.92           | 0.90      | 0.22        | 0.24   |
| 66       | 0.32          | 0.35     | 0.93           | 0.90      | 0.21        | 0.24   |
| 67       | 0.31          | 0.34     | 0.93           | 0.90      | 0.20        | 0.23   |
| 68       | 0.30          | 0.34     | 0.93           | 0.91      | 0.20        | 0.23   |
| 69       | 0.29          | 0.33     | 0.94           | 0.91      | 0.19        | 0.22   |
| 70       | 0.28          | 0.32     | 0.94           | 0.92      | 0.18        | 0.21   |
| 71       | 0.27          | 0.31     | 0.94           | 0.92      | 0.18        | 0.21   |
| 72       | 0.27          | 0.30     | 0.95           | 0.92      | 0.18        | 0.20   |
| 73       | 0.26          | 0.29     | 0.95           | 0.93      | 0.17        | 0.19   |
| 74       | 0.25          | 0.28     | 0.95           | 0.93      | 0.16        | 0.19   |
| 75       | 0.24          | 0.27     | 0.96           | 0.93      | 0.16        | 0.18   |
| 76       | 0.23          | 0.26     | 0.96           | 0.93      | 0.15        | 0.17   |
| 77       | 0.22          | 0.25     | 0.96           | 0.94      | 0.14        | 0.17   |
| 78       | 0.22          | 0.24     | 0.96           | 0.94      | 0.14        | 0.16   |
| 79       | 0.21          | 0.24     | 0.97           | 0.94      | 0.14        | 0.16   |
| 80       | 0.20          | 0.23     | 0.97           | 0.94      | 0.13        | 0.15   |
| 81       | 0.19          | 0.22     | 0.97           | 0.94      | 0.12        | 0.15   |
| 82       | 0.19          | 0.21     | 0.97           | 0.95      | 0.12        | 0.14   |
| 83       | 0.18          | 0.20     | 0.97           | 0.95      | 0.12        | 0.13   |
| 84       | 0.17          | 0.20     | 0.97           | 0.95      | 0.11        | 0.13   |
| 85       | 0.16          | 0.19     | 0.97           | 0.95      | 0.10        | 0.13   |
| 86       | 0.16          | 0.18     | 0.97           | 0.95      | 0.10        | 0.12   |
| 87       | 0.15          | 0.18     | 0.97           | 0.95      | 0.10        | 0.12   |
| 88       | 0.15          | 0.18     | 0.97           | 0.95      | 0.10        | 0.12   |
| 89       | 0.14          | 0.17     | 0.97           | 0.95      | 0.09        | 0.11   |
| 90       | 0.14          | 0.17     | 0.97           | 0.95      | 0.09        | 0.11   |

Table S154: Reference ( $\phi_S$ ,  $\varphi$ ,  $\psi$ ) and approached ( $\phi_S^\ell$ ,  $\varphi^\ell$ ,  $\psi^\ell$ ) values of the topological descriptors for the first excited-state of the pyridinium-phenolate (PP), computed at the TDHF/6-31+G level of theory.  $\alpha$  is the pyridinium-phenolate central twist angle amplitude.

| $\alpha$ | $\phi_S^\ell$ | $\phi_S$ | $\varphi^\ell$ | $\varphi$ | $\psi^\ell$ | $\psi$ |
|----------|---------------|----------|----------------|-----------|-------------|--------|
| 0        | 0.63          | 0.67     | 0.70           | 0.67      | 0.47        | 0.50   |
| 1        | 0.63          | 0.67     | 0.70           | 0.67      | 0.47        | 0.50   |
| 2        | 0.63          | 0.67     | 0.70           | 0.67      | 0.47        | 0.50   |
| 3        | 0.63          | 0.67     | 0.70           | 0.67      | 0.47        | 0.50   |
| 4        | 0.63          | 0.67     | 0.70           | 0.67      | 0.47        | 0.50   |
| 5        | 0.63          | 0.67     | 0.70           | 0.67      | 0.47        | 0.50   |
| 6        | 0.63          | 0.67     | 0.70           | 0.67      | 0.47        | 0.50   |
| 7        | 0.63          | 0.67     | 0.70           | 0.67      | 0.47        | 0.50   |
| 8        | 0.62          | 0.67     | 0.70           | 0.67      | 0.46        | 0.50   |
| 9        | 0.62          | 0.67     | 0.71           | 0.67      | 0.46        | 0.50   |
| 10       | 0.62          | 0.67     | 0.71           | 0.67      | 0.46        | 0.50   |
| 11       | 0.62          | 0.66     | 0.71           | 0.68      | 0.46        | 0.49   |
| 12       | 0.62          | 0.66     | 0.71           | 0.68      | 0.46        | 0.49   |
| 13       | 0.62          | 0.66     | 0.71           | 0.68      | 0.46        | 0.49   |
| 14       | 0.62          | 0.66     | 0.71           | 0.68      | 0.46        | 0.49   |
| 15       | 0.62          | 0.66     | 0.71           | 0.68      | 0.46        | 0.49   |
| 16       | 0.61          | 0.66     | 0.72           | 0.69      | 0.45        | 0.49   |
| 17       | 0.61          | 0.65     | 0.72           | 0.69      | 0.45        | 0.48   |
| 18       | 0.61          | 0.65     | 0.72           | 0.69      | 0.45        | 0.48   |
| 19       | 0.61          | 0.65     | 0.72           | 0.69      | 0.45        | 0.48   |
| 20       | 0.61          | 0.65     | 0.73           | 0.70      | 0.44        | 0.48   |
| 21       | 0.60          | 0.64     | 0.73           | 0.70      | 0.44        | 0.47   |
| 22       | 0.60          | 0.64     | 0.73           | 0.70      | 0.44        | 0.47   |
| 23       | 0.60          | 0.64     | 0.73           | 0.70      | 0.44        | 0.47   |
| 24       | 0.60          | 0.64     | 0.74           | 0.71      | 0.43        | 0.47   |
| 25       | 0.59          | 0.63     | 0.74           | 0.71      | 0.43        | 0.46   |
| 26       | 0.59          | 0.63     | 0.74           | 0.71      | 0.43        | 0.46   |
| 27       | 0.59          | 0.63     | 0.75           | 0.72      | 0.42        | 0.46   |
| 28       | 0.59          | 0.62     | 0.75           | 0.72      | 0.42        | 0.45   |
| 29       | 0.58          | 0.62     | 0.75           | 0.72      | 0.42        | 0.45   |
| 30       | 0.58          | 0.61     | 0.76           | 0.73      | 0.41        | 0.44   |
| 31       | 0.57          | 0.61     | 0.76           | 0.73      | 0.41        | 0.44   |

Continued on next page



| $\alpha$ | $\phi_S^\ell$ | $\phi_S$ | $\varphi^\ell$ | $\varphi$ | $\psi^\ell$ | $\psi$ |
|----------|---------------|----------|----------------|-----------|-------------|--------|
| 32       | 0.57          | 0.61     | 0.76           | 0.74      | 0.41        | 0.44   |
| 33       | 0.57          | 0.60     | 0.77           | 0.74      | 0.41        | 0.43   |
| 34       | 0.56          | 0.60     | 0.77           | 0.74      | 0.40        | 0.43   |
| 35       | 0.56          | 0.59     | 0.78           | 0.75      | 0.40        | 0.42   |
| 36       | 0.55          | 0.59     | 0.78           | 0.75      | 0.39        | 0.42   |
| 37       | 0.55          | 0.58     | 0.78           | 0.76      | 0.39        | 0.41   |
| 38       | 0.54          | 0.58     | 0.79           | 0.76      | 0.38        | 0.41   |
| 39       | 0.54          | 0.57     | 0.79           | 0.77      | 0.38        | 0.41   |
| 40       | 0.53          | 0.57     | 0.80           | 0.77      | 0.37        | 0.41   |
| 41       | 0.53          | 0.56     | 0.80           | 0.78      | 0.37        | 0.40   |
| 42       | 0.52          | 0.56     | 0.81           | 0.78      | 0.36        | 0.40   |
| 43       | 0.52          | 0.55     | 0.81           | 0.79      | 0.36        | 0.39   |
| 44       | 0.51          | 0.54     | 0.82           | 0.79      | 0.35        | 0.38   |
| 45       | 0.50          | 0.54     | 0.82           | 0.80      | 0.35        | 0.38   |
| 46       | 0.50          | 0.53     | 0.83           | 0.80      | 0.35        | 0.37   |
| 47       | 0.49          | 0.52     | 0.83           | 0.81      | 0.34        | 0.36   |
| 48       | 0.48          | 0.52     | 0.84           | 0.81      | 0.33        | 0.36   |
| 49       | 0.48          | 0.51     | 0.84           | 0.82      | 0.33        | 0.35   |
| 50       | 0.47          | 0.50     | 0.85           | 0.82      | 0.32        | 0.35   |
| 51       | 0.46          | 0.50     | 0.85           | 0.83      | 0.32        | 0.35   |
| 52       | 0.46          | 0.49     | 0.86           | 0.83      | 0.31        | 0.34   |
| 53       | 0.45          | 0.48     | 0.86           | 0.84      | 0.31        | 0.33   |
| 54       | 0.44          | 0.47     | 0.87           | 0.84      | 0.30        | 0.32   |
| 55       | 0.43          | 0.46     | 0.87           | 0.85      | 0.29        | 0.32   |
| 56       | 0.42          | 0.46     | 0.88           | 0.85      | 0.28        | 0.32   |
| 57       | 0.42          | 0.45     | 0.88           | 0.86      | 0.28        | 0.31   |
| 58       | 0.41          | 0.44     | 0.89           | 0.86      | 0.27        | 0.30   |
| 59       | 0.40          | 0.43     | 0.89           | 0.87      | 0.27        | 0.29   |
| 60       | 0.39          | 0.42     | 0.90           | 0.87      | 0.26        | 0.29   |
| 61       | 0.38          | 0.41     | 0.90           | 0.88      | 0.25        | 0.28   |
| 62       | 0.37          | 0.40     | 0.91           | 0.88      | 0.25        | 0.27   |
| 63       | 0.36          | 0.39     | 0.91           | 0.88      | 0.24        | 0.27   |

Continued on next page

| $\alpha$ | $\phi_S^\ell$ | $\phi_S$ | $\varphi^\ell$ | $\varphi$ | $\psi^\ell$ | $\psi$ |
|----------|---------------|----------|----------------|-----------|-------------|--------|
| 64       | 0.35          | 0.38     | 0.92           | 0.89      | 0.23        | 0.26   |
| 65       | 0.34          | 0.37     | 0.92           | 0.89      | 0.23        | 0.25   |
| 66       | 0.33          | 0.37     | 0.93           | 0.90      | 0.22        | 0.25   |
| 67       | 0.32          | 0.36     | 0.93           | 0.90      | 0.21        | 0.24   |
| 68       | 0.31          | 0.35     | 0.94           | 0.91      | 0.20        | 0.23   |
| 69       | 0.30          | 0.34     | 0.94           | 0.91      | 0.20        | 0.23   |
| 70       | 0.29          | 0.33     | 0.94           | 0.91      | 0.19        | 0.22   |
| 71       | 0.28          | 0.32     | 0.95           | 0.92      | 0.18        | 0.21   |
| 72       | 0.27          | 0.31     | 0.95           | 0.92      | 0.18        | 0.21   |
| 73       | 0.26          | 0.30     | 0.96           | 0.92      | 0.17        | 0.20   |
| 74       | 0.25          | 0.29     | 0.96           | 0.93      | 0.16        | 0.19   |
| 75       | 0.23          | 0.28     | 0.96           | 0.93      | 0.15        | 0.19   |
| 76       | 0.22          | 0.27     | 0.96           | 0.93      | 0.14        | 0.18   |
| 77       | 0.22          | 0.26     | 0.97           | 0.94      | 0.14        | 0.17   |
| 78       | 0.21          | 0.25     | 0.97           | 0.94      | 0.14        | 0.17   |
| 79       | 0.20          | 0.24     | 0.97           | 0.94      | 0.13        | 0.16   |
| 80       | 0.19          | 0.23     | 0.97           | 0.94      | 0.12        | 0.15   |
| 81       | 0.18          | 0.22     | 0.98           | 0.95      | 0.12        | 0.14   |
| 82       | 0.17          | 0.21     | 0.98           | 0.95      | 0.11        | 0.14   |
| 83       | 0.16          | 0.21     | 0.98           | 0.95      | 0.10        | 0.14   |
| 84       | 0.16          | 0.20     | 0.98           | 0.95      | 0.10        | 0.13   |
| 85       | 0.15          | 0.19     | 0.98           | 0.95      | 0.10        | 0.13   |
| 86       | 0.14          | 0.18     | 0.98           | 0.95      | 0.09        | 0.12   |
| 87       | 0.13          | 0.18     | 0.98           | 0.95      | 0.08        | 0.12   |
| 88       | 0.13          | 0.17     | 0.98           | 0.95      | 0.08        | 0.11   |
| 89       | 0.12          | 0.17     | 0.98           | 0.95      | 0.08        | 0.11   |
| 90       | 0.12          | 0.17     | 0.98           | 0.95      | 0.08        | 0.11   |

Table S155: Reference ( $\phi_S$ ,  $\varphi$ ,  $\psi$ ) and approached ( $\phi_S^\ell$ ,  $\varphi^\ell$ ,  $\psi^\ell$ ) values of the topological descriptors for the first excited-state of the pyridinium-phenolate (PP), computed at the TDHF/6-31G level of theory.  $\alpha$  is the pyridinium-phenolate central twist angle amplitude.

| $\alpha$ | $\phi_S^\ell$ | $\phi_S$ | $\varphi^\ell$ | $\varphi$ | $\psi^\ell$ | $\psi$ |
|----------|---------------|----------|----------------|-----------|-------------|--------|
| 0        | 0.69          | 0.73     | 0.65           | 0.61      | 0.52        | 0.56   |
| 1        | 0.69          | 0.73     | 0.65           | 0.61      | 0.52        | 0.56   |
| 2        | 0.69          | 0.73     | 0.65           | 0.61      | 0.52        | 0.56   |
| 3        | 0.69          | 0.73     | 0.65           | 0.61      | 0.52        | 0.56   |
| 4        | 0.69          | 0.73     | 0.65           | 0.61      | 0.52        | 0.56   |
| 5        | 0.69          | 0.72     | 0.65           | 0.61      | 0.52        | 0.55   |
| 6        | 0.69          | 0.72     | 0.65           | 0.62      | 0.52        | 0.55   |
| 7        | 0.69          | 0.72     | 0.65           | 0.62      | 0.52        | 0.55   |
| 8        | 0.69          | 0.72     | 0.65           | 0.62      | 0.52        | 0.55   |
| 9        | 0.69          | 0.72     | 0.65           | 0.62      | 0.52        | 0.55   |
| 10       | 0.69          | 0.72     | 0.65           | 0.62      | 0.52        | 0.55   |
| 11       | 0.69          | 0.72     | 0.65           | 0.62      | 0.52        | 0.55   |
| 12       | 0.68          | 0.72     | 0.66           | 0.62      | 0.51        | 0.55   |
| 13       | 0.68          | 0.72     | 0.66           | 0.63      | 0.51        | 0.54   |
| 14       | 0.68          | 0.71     | 0.66           | 0.63      | 0.51        | 0.54   |
| 15       | 0.68          | 0.71     | 0.66           | 0.63      | 0.51        | 0.54   |
| 16       | 0.68          | 0.71     | 0.66           | 0.63      | 0.51        | 0.54   |
| 17       | 0.68          | 0.71     | 0.66           | 0.63      | 0.51        | 0.54   |
| 18       | 0.68          | 0.71     | 0.67           | 0.64      | 0.50        | 0.53   |
| 19       | 0.68          | 0.71     | 0.67           | 0.64      | 0.50        | 0.53   |
| 20       | 0.68          | 0.71     | 0.67           | 0.64      | 0.50        | 0.53   |
| 21       | 0.67          | 0.70     | 0.67           | 0.64      | 0.50        | 0.53   |
| 22       | 0.67          | 0.70     | 0.68           | 0.65      | 0.50        | 0.52   |
| 23       | 0.67          | 0.70     | 0.68           | 0.65      | 0.50        | 0.52   |
| 24       | 0.67          | 0.70     | 0.68           | 0.65      | 0.50        | 0.52   |
| 25       | 0.67          | 0.70     | 0.68           | 0.65      | 0.50        | 0.52   |
| 26       | 0.67          | 0.69     | 0.69           | 0.66      | 0.49        | 0.51   |
| 27       | 0.67          | 0.69     | 0.69           | 0.66      | 0.49        | 0.51   |
| 28       | 0.66          | 0.69     | 0.69           | 0.66      | 0.49        | 0.51   |
| 29       | 0.66          | 0.69     | 0.69           | 0.67      | 0.49        | 0.51   |
| 30       | 0.66          | 0.69     | 0.70           | 0.67      | 0.48        | 0.51   |
| 31       | 0.66          | 0.68     | 0.70           | 0.67      | 0.48        | 0.50   |

Continued on next page

| $\alpha$ | $\phi_S^\ell$ | $\phi_S$ | $\varphi^\ell$ | $\varphi$ | $\psi^\ell$ | $\psi$ |
|----------|---------------|----------|----------------|-----------|-------------|--------|
| 32       | 0.66          | 0.68     | 0.70           | 0.68      | 0.48        | 0.50   |
| 33       | 0.66          | 0.68     | 0.71           | 0.68      | 0.48        | 0.50   |
| 34       | 0.65          | 0.68     | 0.71           | 0.68      | 0.47        | 0.50   |
| 35       | 0.65          | 0.67     | 0.71           | 0.69      | 0.47        | 0.49   |
| 36       | 0.65          | 0.67     | 0.71           | 0.69      | 0.47        | 0.49   |
| 37       | 0.65          | 0.67     | 0.72           | 0.69      | 0.47        | 0.49   |
| 38       | 0.65          | 0.66     | 0.72           | 0.70      | 0.47        | 0.48   |
| 39       | 0.64          | 0.66     | 0.73           | 0.70      | 0.46        | 0.48   |
| 40       | 0.64          | 0.66     | 0.73           | 0.71      | 0.46        | 0.48   |
| 41       | 0.64          | 0.65     | 0.73           | 0.71      | 0.46        | 0.47   |
| 42       | 0.63          | 0.65     | 0.74           | 0.71      | 0.45        | 0.47   |
| 43       | 0.63          | 0.65     | 0.74           | 0.72      | 0.45        | 0.47   |
| 44       | 0.63          | 0.64     | 0.75           | 0.72      | 0.44        | 0.46   |
| 45       | 0.62          | 0.64     | 0.75           | 0.73      | 0.44        | 0.46   |
| 46       | 0.62          | 0.63     | 0.76           | 0.73      | 0.44        | 0.45   |
| 47       | 0.61          | 0.63     | 0.76           | 0.74      | 0.43        | 0.45   |
| 48       | 0.61          | 0.62     | 0.76           | 0.74      | 0.43        | 0.44   |
| 49       | 0.60          | 0.62     | 0.77           | 0.75      | 0.42        | 0.44   |
| 50       | 0.60          | 0.61     | 0.77           | 0.75      | 0.42        | 0.43   |
| 51       | 0.59          | 0.61     | 0.78           | 0.75      | 0.41        | 0.43   |
| 52       | 0.59          | 0.60     | 0.78           | 0.76      | 0.41        | 0.43   |
| 53       | 0.58          | 0.60     | 0.79           | 0.76      | 0.40        | 0.43   |
| 54       | 0.58          | 0.59     | 0.79           | 0.77      | 0.40        | 0.42   |
| 55       | 0.57          | 0.59     | 0.80           | 0.77      | 0.39        | 0.42   |
| 56       | 0.57          | 0.58     | 0.80           | 0.78      | 0.39        | 0.41   |
| 57       | 0.56          | 0.58     | 0.81           | 0.78      | 0.39        | 0.41   |
| 58       | 0.55          | 0.57     | 0.81           | 0.79      | 0.38        | 0.40   |
| 59       | 0.55          | 0.56     | 0.82           | 0.79      | 0.38        | 0.39   |
| 60       | 0.54          | 0.55     | 0.82           | 0.80      | 0.37        | 0.38   |
| 61       | 0.53          | 0.55     | 0.83           | 0.80      | 0.36        | 0.38   |
| 62       | 0.52          | 0.54     | 0.83           | 0.81      | 0.36        | 0.37   |
| 63       | 0.52          | 0.53     | 0.84           | 0.82      | 0.35        | 0.37   |

Continued on next page

| $\alpha$ | $\phi_S^\ell$ | $\phi_S$ | $\varphi^\ell$ | $\varphi$ | $\psi^\ell$ | $\psi$ |
|----------|---------------|----------|----------------|-----------|-------------|--------|
| 64       | 0.51          | 0.52     | 0.84           | 0.82      | 0.35        | 0.36   |
| 65       | 0.50          | 0.52     | 0.85           | 0.83      | 0.34        | 0.36   |
| 66       | 0.49          | 0.51     | 0.86           | 0.83      | 0.33        | 0.35   |
| 67       | 0.48          | 0.50     | 0.86           | 0.84      | 0.32        | 0.34   |
| 68       | 0.47          | 0.49     | 0.87           | 0.84      | 0.32        | 0.34   |
| 69       | 0.46          | 0.48     | 0.87           | 0.85      | 0.31        | 0.33   |
| 70       | 0.45          | 0.47     | 0.88           | 0.86      | 0.30        | 0.32   |
| 71       | 0.44          | 0.46     | 0.89           | 0.86      | 0.29        | 0.31   |
| 72       | 0.42          | 0.45     | 0.89           | 0.87      | 0.28        | 0.30   |
| 73       | 0.41          | 0.43     | 0.90           | 0.87      | 0.27        | 0.29   |
| 74       | 0.40          | 0.42     | 0.91           | 0.88      | 0.26        | 0.28   |
| 75       | 0.38          | 0.41     | 0.91           | 0.89      | 0.25        | 0.27   |
| 76       | 0.37          | 0.39     | 0.92           | 0.89      | 0.24        | 0.26   |
| 77       | 0.35          | 0.38     | 0.93           | 0.90      | 0.23        | 0.25   |
| 78       | 0.33          | 0.36     | 0.93           | 0.90      | 0.22        | 0.24   |
| 79       | 0.32          | 0.35     | 0.94           | 0.91      | 0.21        | 0.23   |
| 80       | 0.30          | 0.33     | 0.95           | 0.92      | 0.19        | 0.22   |
| 81       | 0.27          | 0.31     | 0.95           | 0.92      | 0.18        | 0.21   |
| 82       | 0.25          | 0.30     | 0.96           | 0.93      | 0.16        | 0.20   |
| 83       | 0.23          | 0.28     | 0.97           | 0.94      | 0.15        | 0.18   |
| 84       | 0.20          | 0.26     | 0.97           | 0.94      | 0.13        | 0.17   |
| 85       | 0.18          | 0.23     | 0.98           | 0.95      | 0.12        | 0.15   |
| 86       | 0.16          | 0.21     | 0.98           | 0.95      | 0.10        | 0.14   |
| 87       | 0.13          | 0.19     | 0.99           | 0.95      | 0.08        | 0.13   |
| 88       | 0.11          | 0.17     | 0.99           | 0.96      | 0.07        | 0.11   |
| 89       | 0.10          | 0.16     | 0.99           | 0.96      | 0.06        | 0.11   |
| 90       | 0.09          | 0.15     | 0.99           | 0.96      | 0.06        | 0.10   |

Table S156: Reference ( $\phi_S$ ,  $\varphi$ ,  $\psi$ ) and approached ( $\phi_S^\ell$ ,  $\varphi^\ell$ ,  $\psi^\ell$ ) values of the topological descriptors for the first excited-state of the pyridinium-phenolate (PP), computed at the wB97XD/3-21G level of theory.  $\alpha$  is the pyridinium-phenolate central twist angle amplitude.

| $\alpha$ | $\phi_S^\ell$ | $\phi_S$ | $\varphi^\ell$ | $\varphi$ | $\psi^\ell$ | $\psi$ |
|----------|---------------|----------|----------------|-----------|-------------|--------|
| 0        | 0.65          | 0.70     | 0.67           | 0.64      | 0.49        | 0.53   |
| 1        | 0.65          | 0.70     | 0.67           | 0.64      | 0.49        | 0.53   |
| 2        | 0.65          | 0.70     | 0.67           | 0.64      | 0.49        | 0.53   |
| 3        | 0.65          | 0.70     | 0.67           | 0.64      | 0.49        | 0.53   |
| 4        | 0.65          | 0.70     | 0.67           | 0.64      | 0.49        | 0.53   |
| 5        | 0.65          | 0.70     | 0.67           | 0.64      | 0.49        | 0.53   |
| 6        | 0.65          | 0.69     | 0.67           | 0.64      | 0.49        | 0.52   |
| 7        | 0.65          | 0.69     | 0.68           | 0.64      | 0.49        | 0.52   |
| 8        | 0.65          | 0.69     | 0.68           | 0.64      | 0.49        | 0.52   |
| 9        | 0.65          | 0.69     | 0.68           | 0.64      | 0.49        | 0.52   |
| 10       | 0.65          | 0.69     | 0.68           | 0.65      | 0.49        | 0.52   |
| 11       | 0.64          | 0.69     | 0.68           | 0.65      | 0.48        | 0.52   |
| 12       | 0.64          | 0.69     | 0.68           | 0.65      | 0.48        | 0.52   |
| 13       | 0.64          | 0.69     | 0.68           | 0.65      | 0.48        | 0.52   |
| 14       | 0.64          | 0.69     | 0.68           | 0.65      | 0.48        | 0.52   |
| 15       | 0.64          | 0.69     | 0.69           | 0.65      | 0.48        | 0.52   |
| 16       | 0.64          | 0.68     | 0.69           | 0.66      | 0.48        | 0.51   |
| 17       | 0.64          | 0.68     | 0.69           | 0.66      | 0.48        | 0.51   |
| 18       | 0.64          | 0.68     | 0.69           | 0.66      | 0.48        | 0.51   |
| 19       | 0.63          | 0.68     | 0.69           | 0.66      | 0.47        | 0.51   |
| 20       | 0.63          | 0.68     | 0.70           | 0.66      | 0.47        | 0.51   |
| 21       | 0.63          | 0.67     | 0.70           | 0.67      | 0.47        | 0.50   |
| 22       | 0.63          | 0.67     | 0.70           | 0.67      | 0.47        | 0.50   |
| 23       | 0.63          | 0.67     | 0.70           | 0.67      | 0.47        | 0.50   |
| 24       | 0.63          | 0.67     | 0.71           | 0.68      | 0.46        | 0.50   |
| 25       | 0.62          | 0.67     | 0.71           | 0.68      | 0.46        | 0.50   |
| 26       | 0.62          | 0.66     | 0.71           | 0.68      | 0.46        | 0.49   |
| 27       | 0.62          | 0.66     | 0.72           | 0.69      | 0.45        | 0.49   |
| 28       | 0.62          | 0.66     | 0.72           | 0.69      | 0.45        | 0.49   |
| 29       | 0.62          | 0.66     | 0.72           | 0.69      | 0.45        | 0.49   |
| 30       | 0.61          | 0.65     | 0.73           | 0.70      | 0.44        | 0.48   |
| 31       | 0.61          | 0.65     | 0.73           | 0.70      | 0.44        | 0.48   |

Continued on next page

| $\alpha$ | $\phi_S^\ell$ | $\phi_S$ | $\varphi^\ell$ | $\varphi$ | $\psi^\ell$ | $\psi$ |
|----------|---------------|----------|----------------|-----------|-------------|--------|
| 32       | 0.61          | 0.65     | 0.73           | 0.70      | 0.44        | 0.48   |
| 33       | 0.61          | 0.64     | 0.74           | 0.71      | 0.44        | 0.47   |
| 34       | 0.60          | 0.64     | 0.74           | 0.71      | 0.43        | 0.47   |
| 35       | 0.60          | 0.64     | 0.74           | 0.71      | 0.43        | 0.47   |
| 36       | 0.60          | 0.63     | 0.75           | 0.72      | 0.43        | 0.46   |
| 37       | 0.59          | 0.63     | 0.75           | 0.72      | 0.42        | 0.46   |
| 38       | 0.59          | 0.63     | 0.76           | 0.73      | 0.42        | 0.45   |
| 39       | 0.59          | 0.62     | 0.76           | 0.73      | 0.42        | 0.45   |
| 40       | 0.58          | 0.62     | 0.76           | 0.73      | 0.41        | 0.45   |
| 41       | 0.58          | 0.61     | 0.77           | 0.74      | 0.41        | 0.44   |
| 42       | 0.58          | 0.61     | 0.77           | 0.74      | 0.41        | 0.44   |
| 43       | 0.57          | 0.60     | 0.78           | 0.75      | 0.40        | 0.43   |
| 44       | 0.57          | 0.60     | 0.78           | 0.75      | 0.40        | 0.43   |
| 45       | 0.56          | 0.59     | 0.79           | 0.76      | 0.39        | 0.42   |
| 46       | 0.56          | 0.59     | 0.79           | 0.76      | 0.39        | 0.42   |
| 47       | 0.55          | 0.58     | 0.79           | 0.77      | 0.39        | 0.41   |
| 48       | 0.55          | 0.58     | 0.80           | 0.77      | 0.38        | 0.41   |
| 49       | 0.54          | 0.57     | 0.80           | 0.78      | 0.38        | 0.40   |
| 50       | 0.54          | 0.57     | 0.81           | 0.78      | 0.37        | 0.40   |
| 51       | 0.53          | 0.56     | 0.81           | 0.78      | 0.37        | 0.40   |
| 52       | 0.53          | 0.56     | 0.81           | 0.79      | 0.37        | 0.39   |
| 53       | 0.52          | 0.55     | 0.82           | 0.79      | 0.36        | 0.39   |
| 54       | 0.52          | 0.54     | 0.82           | 0.80      | 0.36        | 0.38   |
| 55       | 0.51          | 0.54     | 0.83           | 0.80      | 0.35        | 0.38   |
| 56       | 0.50          | 0.53     | 0.83           | 0.81      | 0.35        | 0.37   |
| 57       | 0.50          | 0.52     | 0.84           | 0.81      | 0.34        | 0.36   |
| 58       | 0.49          | 0.52     | 0.84           | 0.82      | 0.34        | 0.36   |
| 59       | 0.48          | 0.51     | 0.85           | 0.83      | 0.33        | 0.35   |
| 60       | 0.47          | 0.50     | 0.85           | 0.83      | 0.32        | 0.35   |
| 61       | 0.47          | 0.49     | 0.86           | 0.84      | 0.32        | 0.34   |
| 62       | 0.46          | 0.48     | 0.86           | 0.84      | 0.31        | 0.33   |
| 63       | 0.45          | 0.47     | 0.87           | 0.85      | 0.30        | 0.32   |

Continued on next page

| $\alpha$ | $\phi_S^\ell$ | $\phi_S$ | $\varphi^\ell$ | $\varphi$ | $\psi^\ell$ | $\psi$ |
|----------|---------------|----------|----------------|-----------|-------------|--------|
| 64       | 0.44          | 0.47     | 0.87           | 0.85      | 0.30        | 0.32   |
| 65       | 0.43          | 0.46     | 0.88           | 0.86      | 0.29        | 0.31   |
| 66       | 0.42          | 0.45     | 0.89           | 0.86      | 0.28        | 0.31   |
| 67       | 0.41          | 0.44     | 0.89           | 0.87      | 0.27        | 0.30   |
| 68       | 0.40          | 0.43     | 0.90           | 0.87      | 0.27        | 0.29   |
| 69       | 0.39          | 0.42     | 0.90           | 0.88      | 0.26        | 0.28   |
| 70       | 0.38          | 0.41     | 0.91           | 0.88      | 0.25        | 0.28   |
| 71       | 0.37          | 0.39     | 0.91           | 0.89      | 0.25        | 0.26   |
| 72       | 0.36          | 0.38     | 0.92           | 0.89      | 0.24        | 0.26   |
| 73       | 0.35          | 0.37     | 0.92           | 0.90      | 0.23        | 0.25   |
| 74       | 0.33          | 0.36     | 0.93           | 0.90      | 0.22        | 0.24   |
| 75       | 0.32          | 0.35     | 0.93           | 0.91      | 0.21        | 0.23   |
| 76       | 0.31          | 0.33     | 0.93           | 0.91      | 0.20        | 0.22   |
| 77       | 0.29          | 0.32     | 0.94           | 0.92      | 0.19        | 0.21   |
| 78       | 0.28          | 0.31     | 0.94           | 0.92      | 0.18        | 0.21   |
| 79       | 0.27          | 0.29     | 0.95           | 0.93      | 0.18        | 0.19   |
| 80       | 0.25          | 0.28     | 0.95           | 0.93      | 0.16        | 0.19   |
| 81       | 0.24          | 0.26     | 0.95           | 0.93      | 0.16        | 0.17   |
| 82       | 0.22          | 0.25     | 0.96           | 0.94      | 0.14        | 0.17   |
| 83       | 0.21          | 0.24     | 0.96           | 0.94      | 0.14        | 0.16   |
| 84       | 0.19          | 0.22     | 0.96           | 0.94      | 0.12        | 0.15   |
| 85       | 0.18          | 0.21     | 0.96           | 0.95      | 0.12        | 0.14   |
| 86       | 0.17          | 0.20     | 0.97           | 0.95      | 0.11        | 0.13   |
| 87       | 0.16          | 0.18     | 0.97           | 0.95      | 0.10        | 0.12   |
| 88       | 0.15          | 0.17     | 0.97           | 0.95      | 0.10        | 0.11   |
| 89       | 0.14          | 0.17     | 0.97           | 0.95      | 0.09        | 0.11   |
| 90       | 0.14          | 0.16     | 0.97           | 0.95      | 0.09        | 0.11   |

Table S157: Reference ( $\phi_S$ ,  $\varphi$ ,  $\psi$ ) and approached ( $\phi_S^\ell$ ,  $\varphi^\ell$ ,  $\psi^\ell$ ) values of the topological descriptors for the first excited-state of the pyridinium-phenolate (PP), computed at the wB97XD/6-311++G(2d,p) level of theory.  $\alpha$  is the pyridinium-phenolate central twist angle amplitude.



| $\alpha$ | $\phi_S^\ell$ | $\phi_S$ | $\varphi^\ell$ | $\varphi$ | $\psi^\ell$ | $\psi$ |
|----------|---------------|----------|----------------|-----------|-------------|--------|
| 0        | 0.65          | 0.70     | 0.67           | 0.63      | 0.49        | 0.53   |
| 1        | 0.65          | 0.70     | 0.67           | 0.63      | 0.49        | 0.53   |
| 2        | 0.65          | 0.70     | 0.67           | 0.63      | 0.49        | 0.53   |
| 3        | 0.65          | 0.70     | 0.67           | 0.64      | 0.49        | 0.53   |
| 4        | 0.65          | 0.70     | 0.67           | 0.64      | 0.49        | 0.53   |
| 5        | 0.65          | 0.70     | 0.67           | 0.64      | 0.49        | 0.53   |
| 6        | 0.65          | 0.70     | 0.67           | 0.64      | 0.49        | 0.53   |
| 7        | 0.64          | 0.70     | 0.67           | 0.64      | 0.49        | 0.53   |
| 8        | 0.64          | 0.70     | 0.67           | 0.64      | 0.49        | 0.53   |
| 9        | 0.64          | 0.69     | 0.68           | 0.64      | 0.48        | 0.52   |
| 10       | 0.64          | 0.69     | 0.68           | 0.64      | 0.48        | 0.52   |
| 11       | 0.64          | 0.69     | 0.68           | 0.64      | 0.48        | 0.52   |
| 12       | 0.64          | 0.69     | 0.68           | 0.65      | 0.48        | 0.52   |
| 13       | 0.64          | 0.69     | 0.68           | 0.65      | 0.48        | 0.52   |
| 14       | 0.64          | 0.69     | 0.68           | 0.65      | 0.48        | 0.52   |
| 15       | 0.64          | 0.69     | 0.68           | 0.65      | 0.48        | 0.52   |
| 16       | 0.64          | 0.69     | 0.69           | 0.65      | 0.48        | 0.52   |
| 17       | 0.64          | 0.68     | 0.69           | 0.66      | 0.48        | 0.51   |
| 18       | 0.63          | 0.68     | 0.69           | 0.66      | 0.47        | 0.51   |
| 19       | 0.63          | 0.68     | 0.69           | 0.66      | 0.47        | 0.51   |
| 20       | 0.63          | 0.68     | 0.69           | 0.66      | 0.47        | 0.51   |
| 21       | 0.63          | 0.68     | 0.70           | 0.67      | 0.47        | 0.50   |
| 22       | 0.63          | 0.67     | 0.70           | 0.67      | 0.47        | 0.50   |
| 23       | 0.63          | 0.67     | 0.70           | 0.67      | 0.47        | 0.50   |
| 24       | 0.63          | 0.67     | 0.71           | 0.67      | 0.46        | 0.50   |
| 25       | 0.62          | 0.67     | 0.71           | 0.68      | 0.46        | 0.50   |
| 26       | 0.62          | 0.67     | 0.71           | 0.68      | 0.46        | 0.50   |
| 27       | 0.62          | 0.66     | 0.71           | 0.68      | 0.46        | 0.49   |
| 28       | 0.62          | 0.66     | 0.72           | 0.69      | 0.45        | 0.49   |
| 29       | 0.62          | 0.66     | 0.72           | 0.69      | 0.45        | 0.49   |
| 30       | 0.62          | 0.65     | 0.72           | 0.69      | 0.45        | 0.48   |
| 31       | 0.61          | 0.65     | 0.73           | 0.70      | 0.44        | 0.48   |

Continued on next page

| $\alpha$ | $\phi_S^\ell$ | $\phi_S$ | $\varphi^\ell$ | $\varphi$ | $\psi^\ell$ | $\psi$ |
|----------|---------------|----------|----------------|-----------|-------------|--------|
| 32       | 0.61          | 0.65     | 0.73           | 0.70      | 0.44        | 0.48   |
| 33       | 0.61          | 0.65     | 0.73           | 0.71      | 0.44        | 0.47   |
| 34       | 0.61          | 0.64     | 0.74           | 0.71      | 0.44        | 0.47   |
| 35       | 0.60          | 0.64     | 0.74           | 0.71      | 0.43        | 0.47   |
| 36       | 0.60          | 0.63     | 0.74           | 0.72      | 0.43        | 0.46   |
| 37       | 0.60          | 0.63     | 0.75           | 0.72      | 0.43        | 0.46   |
| 38       | 0.59          | 0.63     | 0.75           | 0.73      | 0.42        | 0.45   |
| 39       | 0.59          | 0.62     | 0.76           | 0.73      | 0.42        | 0.45   |
| 40       | 0.59          | 0.62     | 0.76           | 0.73      | 0.42        | 0.45   |
| 41       | 0.58          | 0.61     | 0.77           | 0.74      | 0.41        | 0.44   |
| 42       | 0.58          | 0.61     | 0.77           | 0.74      | 0.41        | 0.44   |
| 43       | 0.58          | 0.61     | 0.77           | 0.75      | 0.41        | 0.43   |
| 44       | 0.57          | 0.60     | 0.78           | 0.75      | 0.40        | 0.43   |
| 45       | 0.57          | 0.60     | 0.78           | 0.76      | 0.40        | 0.43   |
| 46       | 0.56          | 0.59     | 0.79           | 0.76      | 0.39        | 0.42   |
| 47       | 0.56          | 0.59     | 0.79           | 0.76      | 0.39        | 0.42   |
| 48       | 0.55          | 0.58     | 0.80           | 0.77      | 0.38        | 0.41   |
| 49       | 0.55          | 0.58     | 0.80           | 0.77      | 0.38        | 0.41   |
| 50       | 0.54          | 0.57     | 0.81           | 0.78      | 0.37        | 0.40   |
| 51       | 0.54          | 0.56     | 0.81           | 0.78      | 0.37        | 0.40   |
| 52       | 0.53          | 0.56     | 0.81           | 0.79      | 0.37        | 0.39   |
| 53       | 0.52          | 0.55     | 0.82           | 0.79      | 0.36        | 0.39   |
| 54       | 0.52          | 0.55     | 0.82           | 0.80      | 0.36        | 0.38   |
| 55       | 0.51          | 0.54     | 0.83           | 0.80      | 0.35        | 0.38   |
| 56       | 0.50          | 0.53     | 0.83           | 0.81      | 0.35        | 0.37   |
| 57       | 0.50          | 0.52     | 0.84           | 0.81      | 0.34        | 0.36   |
| 58       | 0.49          | 0.52     | 0.84           | 0.82      | 0.34        | 0.36   |
| 59       | 0.48          | 0.51     | 0.85           | 0.82      | 0.33        | 0.35   |
| 60       | 0.47          | 0.50     | 0.85           | 0.83      | 0.32        | 0.35   |
| 61       | 0.47          | 0.49     | 0.86           | 0.83      | 0.32        | 0.34   |
| 62       | 0.46          | 0.49     | 0.86           | 0.84      | 0.31        | 0.34   |
| 63       | 0.45          | 0.48     | 0.87           | 0.85      | 0.30        | 0.33   |

Continued on next page

| $\alpha$ | $\phi_S^\ell$ | $\phi_S$ | $\varphi^\ell$ | $\varphi$ | $\psi^\ell$ | $\psi$ |
|----------|---------------|----------|----------------|-----------|-------------|--------|
| 64       | 0.44          | 0.47     | 0.88           | 0.85      | 0.30        | 0.32   |
| 65       | 0.43          | 0.46     | 0.88           | 0.86      | 0.29        | 0.31   |
| 66       | 0.42          | 0.45     | 0.89           | 0.86      | 0.28        | 0.31   |
| 67       | 0.41          | 0.44     | 0.89           | 0.87      | 0.27        | 0.30   |
| 68       | 0.40          | 0.43     | 0.90           | 0.87      | 0.27        | 0.29   |
| 69       | 0.39          | 0.42     | 0.90           | 0.88      | 0.26        | 0.28   |
| 70       | 0.38          | 0.41     | 0.91           | 0.88      | 0.25        | 0.28   |
| 71       | 0.37          | 0.40     | 0.91           | 0.89      | 0.25        | 0.27   |
| 72       | 0.35          | 0.38     | 0.92           | 0.89      | 0.23        | 0.26   |
| 73       | 0.34          | 0.37     | 0.93           | 0.90      | 0.22        | 0.25   |
| 74       | 0.33          | 0.36     | 0.93           | 0.90      | 0.22        | 0.24   |
| 75       | 0.31          | 0.35     | 0.94           | 0.91      | 0.20        | 0.23   |
| 76       | 0.30          | 0.33     | 0.94           | 0.91      | 0.20        | 0.22   |
| 77       | 0.29          | 0.32     | 0.94           | 0.92      | 0.19        | 0.21   |
| 78       | 0.27          | 0.31     | 0.95           | 0.92      | 0.18        | 0.21   |
| 79       | 0.26          | 0.29     | 0.95           | 0.93      | 0.17        | 0.19   |
| 80       | 0.24          | 0.28     | 0.96           | 0.93      | 0.16        | 0.19   |
| 81       | 0.22          | 0.26     | 0.96           | 0.93      | 0.14        | 0.17   |
| 82       | 0.21          | 0.25     | 0.97           | 0.94      | 0.14        | 0.17   |
| 83       | 0.19          | 0.24     | 0.97           | 0.94      | 0.12        | 0.16   |
| 84       | 0.18          | 0.22     | 0.97           | 0.94      | 0.12        | 0.15   |
| 85       | 0.17          | 0.21     | 0.97           | 0.95      | 0.11        | 0.14   |
| 86       | 0.16          | 0.20     | 0.98           | 0.95      | 0.10        | 0.13   |
| 87       | 0.14          | 0.18     | 0.98           | 0.95      | 0.09        | 0.12   |
| 88       | 0.13          | 0.17     | 0.98           | 0.95      | 0.08        | 0.11   |
| 89       | 0.13          | 0.17     | 0.98           | 0.95      | 0.08        | 0.11   |
| 90       | 0.12          | 0.16     | 0.98           | 0.95      | 0.08        | 0.11   |

Table S158: Reference ( $\phi_S$ ,  $\varphi$ ,  $\psi$ ) and approached ( $\phi_S^\ell$ ,  $\varphi^\ell$ ,  $\psi^\ell$ ) values of the topological descriptors for the first excited-state of the pyridinium-phenolate (PP), computed at the wB97XD/6-311++G(d,p) level of theory.  $\alpha$  is the pyridinium-phenolate central twist angle amplitude.

| $\alpha$ | $\phi_S^\ell$ | $\phi_S$ | $\varphi^\ell$ | $\varphi$ | $\psi^\ell$ | $\psi$ |
|----------|---------------|----------|----------------|-----------|-------------|--------|
| 0        | 0.65          | 0.70     | 0.67           | 0.63      | 0.49        | 0.53   |
| 1        | 0.65          | 0.70     | 0.67           | 0.63      | 0.49        | 0.53   |
| 2        | 0.65          | 0.70     | 0.67           | 0.64      | 0.49        | 0.53   |
| 3        | 0.65          | 0.70     | 0.67           | 0.64      | 0.49        | 0.53   |
| 4        | 0.65          | 0.70     | 0.67           | 0.64      | 0.49        | 0.53   |
| 5        | 0.65          | 0.70     | 0.67           | 0.64      | 0.49        | 0.53   |
| 6        | 0.65          | 0.70     | 0.67           | 0.64      | 0.49        | 0.53   |
| 7        | 0.64          | 0.70     | 0.67           | 0.64      | 0.49        | 0.53   |
| 8        | 0.64          | 0.70     | 0.67           | 0.64      | 0.49        | 0.53   |
| 9        | 0.64          | 0.69     | 0.68           | 0.64      | 0.48        | 0.52   |
| 10       | 0.64          | 0.69     | 0.68           | 0.64      | 0.48        | 0.52   |
| 11       | 0.64          | 0.69     | 0.68           | 0.64      | 0.48        | 0.52   |
| 12       | 0.64          | 0.69     | 0.68           | 0.65      | 0.48        | 0.52   |
| 13       | 0.64          | 0.69     | 0.68           | 0.65      | 0.48        | 0.52   |
| 14       | 0.64          | 0.69     | 0.68           | 0.65      | 0.48        | 0.52   |
| 15       | 0.64          | 0.69     | 0.68           | 0.65      | 0.48        | 0.52   |
| 16       | 0.64          | 0.69     | 0.69           | 0.65      | 0.48        | 0.52   |
| 17       | 0.64          | 0.68     | 0.69           | 0.66      | 0.48        | 0.51   |
| 18       | 0.64          | 0.68     | 0.69           | 0.66      | 0.48        | 0.51   |
| 19       | 0.63          | 0.68     | 0.69           | 0.66      | 0.47        | 0.51   |
| 20       | 0.63          | 0.68     | 0.69           | 0.66      | 0.47        | 0.51   |
| 21       | 0.63          | 0.68     | 0.70           | 0.67      | 0.47        | 0.50   |
| 22       | 0.63          | 0.67     | 0.70           | 0.67      | 0.47        | 0.50   |
| 23       | 0.63          | 0.67     | 0.70           | 0.67      | 0.47        | 0.50   |
| 24       | 0.63          | 0.67     | 0.71           | 0.67      | 0.46        | 0.50   |
| 25       | 0.63          | 0.67     | 0.71           | 0.68      | 0.46        | 0.50   |
| 26       | 0.62          | 0.67     | 0.71           | 0.68      | 0.46        | 0.50   |
| 27       | 0.62          | 0.66     | 0.71           | 0.68      | 0.46        | 0.49   |
| 28       | 0.62          | 0.66     | 0.72           | 0.69      | 0.45        | 0.49   |
| 29       | 0.62          | 0.66     | 0.72           | 0.69      | 0.45        | 0.49   |
| 30       | 0.62          | 0.65     | 0.72           | 0.69      | 0.45        | 0.48   |
| 31       | 0.61          | 0.65     | 0.73           | 0.70      | 0.44        | 0.48   |

Continued on next page

| $\alpha$ | $\phi_S^\ell$ | $\phi_S$ | $\varphi^\ell$ | $\varphi$ | $\psi^\ell$ | $\psi$ |
|----------|---------------|----------|----------------|-----------|-------------|--------|
| 32       | 0.61          | 0.65     | 0.73           | 0.70      | 0.44        | 0.48   |
| 33       | 0.61          | 0.65     | 0.73           | 0.71      | 0.44        | 0.47   |
| 34       | 0.61          | 0.64     | 0.74           | 0.71      | 0.44        | 0.47   |
| 35       | 0.60          | 0.64     | 0.74           | 0.71      | 0.43        | 0.47   |
| 36       | 0.60          | 0.63     | 0.74           | 0.72      | 0.43        | 0.46   |
| 37       | 0.60          | 0.63     | 0.75           | 0.72      | 0.43        | 0.46   |
| 38       | 0.59          | 0.63     | 0.75           | 0.73      | 0.42        | 0.45   |
| 39       | 0.59          | 0.62     | 0.76           | 0.73      | 0.42        | 0.45   |
| 40       | 0.59          | 0.62     | 0.76           | 0.73      | 0.42        | 0.45   |
| 41       | 0.58          | 0.61     | 0.77           | 0.74      | 0.41        | 0.44   |
| 42       | 0.58          | 0.61     | 0.77           | 0.74      | 0.41        | 0.44   |
| 43       | 0.58          | 0.61     | 0.77           | 0.75      | 0.41        | 0.43   |
| 44       | 0.57          | 0.60     | 0.78           | 0.75      | 0.40        | 0.43   |
| 45       | 0.57          | 0.60     | 0.78           | 0.76      | 0.40        | 0.43   |
| 46       | 0.56          | 0.59     | 0.79           | 0.76      | 0.39        | 0.42   |
| 47       | 0.56          | 0.59     | 0.79           | 0.76      | 0.39        | 0.42   |
| 48       | 0.55          | 0.58     | 0.80           | 0.77      | 0.38        | 0.41   |
| 49       | 0.55          | 0.58     | 0.80           | 0.77      | 0.38        | 0.41   |
| 50       | 0.54          | 0.57     | 0.81           | 0.78      | 0.37        | 0.40   |
| 51       | 0.54          | 0.56     | 0.81           | 0.78      | 0.37        | 0.40   |
| 52       | 0.53          | 0.56     | 0.81           | 0.79      | 0.37        | 0.39   |
| 53       | 0.52          | 0.55     | 0.82           | 0.79      | 0.36        | 0.39   |
| 54       | 0.52          | 0.55     | 0.82           | 0.80      | 0.36        | 0.38   |
| 55       | 0.51          | 0.54     | 0.83           | 0.80      | 0.35        | 0.38   |
| 56       | 0.51          | 0.53     | 0.83           | 0.81      | 0.35        | 0.37   |
| 57       | 0.50          | 0.52     | 0.84           | 0.81      | 0.34        | 0.36   |
| 58       | 0.49          | 0.52     | 0.84           | 0.82      | 0.34        | 0.36   |
| 59       | 0.48          | 0.51     | 0.85           | 0.82      | 0.33        | 0.35   |
| 60       | 0.47          | 0.50     | 0.85           | 0.83      | 0.32        | 0.35   |
| 61       | 0.47          | 0.49     | 0.86           | 0.83      | 0.32        | 0.34   |
| 62       | 0.46          | 0.49     | 0.86           | 0.84      | 0.31        | 0.34   |
| 63       | 0.45          | 0.48     | 0.87           | 0.85      | 0.30        | 0.33   |

Continued on next page

| $\alpha$ | $\phi_S^\ell$ | $\phi_S$ | $\varphi^\ell$ | $\varphi$ | $\psi^\ell$ | $\psi$ |
|----------|---------------|----------|----------------|-----------|-------------|--------|
| 64       | 0.44          | 0.47     | 0.88           | 0.85      | 0.30        | 0.32   |
| 65       | 0.43          | 0.46     | 0.88           | 0.86      | 0.29        | 0.31   |
| 66       | 0.42          | 0.45     | 0.89           | 0.86      | 0.28        | 0.31   |
| 67       | 0.41          | 0.44     | 0.89           | 0.87      | 0.27        | 0.30   |
| 68       | 0.40          | 0.43     | 0.90           | 0.87      | 0.27        | 0.29   |
| 69       | 0.39          | 0.42     | 0.90           | 0.88      | 0.26        | 0.28   |
| 70       | 0.38          | 0.41     | 0.91           | 0.88      | 0.25        | 0.28   |
| 71       | 0.37          | 0.40     | 0.91           | 0.89      | 0.25        | 0.27   |
| 72       | 0.35          | 0.38     | 0.92           | 0.89      | 0.23        | 0.26   |
| 73       | 0.34          | 0.37     | 0.93           | 0.90      | 0.22        | 0.25   |
| 74       | 0.33          | 0.36     | 0.93           | 0.90      | 0.22        | 0.24   |
| 75       | 0.31          | 0.35     | 0.94           | 0.91      | 0.20        | 0.23   |
| 76       | 0.30          | 0.33     | 0.94           | 0.91      | 0.20        | 0.22   |
| 77       | 0.29          | 0.32     | 0.94           | 0.92      | 0.19        | 0.21   |
| 78       | 0.27          | 0.31     | 0.95           | 0.92      | 0.18        | 0.21   |
| 79       | 0.26          | 0.29     | 0.95           | 0.93      | 0.17        | 0.19   |
| 80       | 0.24          | 0.28     | 0.96           | 0.93      | 0.16        | 0.19   |
| 81       | 0.23          | 0.26     | 0.96           | 0.93      | 0.15        | 0.17   |
| 82       | 0.21          | 0.25     | 0.96           | 0.94      | 0.14        | 0.17   |
| 83       | 0.20          | 0.24     | 0.97           | 0.94      | 0.13        | 0.16   |
| 84       | 0.18          | 0.22     | 0.97           | 0.94      | 0.12        | 0.15   |
| 85       | 0.17          | 0.21     | 0.97           | 0.95      | 0.11        | 0.14   |
| 86       | 0.16          | 0.20     | 0.98           | 0.95      | 0.10        | 0.13   |
| 87       | 0.14          | 0.18     | 0.98           | 0.95      | 0.09        | 0.12   |
| 88       | 0.13          | 0.17     | 0.98           | 0.95      | 0.08        | 0.11   |
| 89       | 0.13          | 0.17     | 0.98           | 0.95      | 0.08        | 0.11   |
| 90       | 0.12          | 0.16     | 0.98           | 0.95      | 0.08        | 0.11   |

Table S159: Reference ( $\phi_S$ ,  $\varphi$ ,  $\psi$ ) and approached ( $\phi_S^\ell$ ,  $\varphi^\ell$ ,  $\psi^\ell$ ) values of the topological descriptors for the first excited-state of the pyridinium-phenolate (PP), computed at the wB97XD/6-311+G(d,p) level of theory.  $\alpha$  is the pyridinium-phenolate central twist angle amplitude.

| $\alpha$ | $\phi_S^\ell$ | $\phi_S$ | $\varphi^\ell$ | $\varphi$ | $\psi^\ell$ | $\psi$ |
|----------|---------------|----------|----------------|-----------|-------------|--------|
| 0        | 0.65          | 0.70     | 0.67           | 0.64      | 0.49        | 0.53   |
| 1        | 0.65          | 0.70     | 0.67           | 0.64      | 0.49        | 0.53   |
| 2        | 0.65          | 0.70     | 0.67           | 0.64      | 0.49        | 0.53   |
| 3        | 0.65          | 0.70     | 0.67           | 0.64      | 0.49        | 0.53   |
| 4        | 0.65          | 0.70     | 0.67           | 0.64      | 0.49        | 0.53   |
| 5        | 0.64          | 0.70     | 0.67           | 0.64      | 0.49        | 0.53   |
| 6        | 0.64          | 0.70     | 0.67           | 0.64      | 0.49        | 0.53   |
| 7        | 0.64          | 0.70     | 0.67           | 0.64      | 0.49        | 0.53   |
| 8        | 0.64          | 0.69     | 0.68           | 0.64      | 0.48        | 0.52   |
| 9        | 0.64          | 0.69     | 0.68           | 0.64      | 0.48        | 0.52   |
| 10       | 0.64          | 0.69     | 0.68           | 0.64      | 0.48        | 0.52   |
| 11       | 0.64          | 0.69     | 0.68           | 0.65      | 0.48        | 0.52   |
| 12       | 0.64          | 0.69     | 0.68           | 0.65      | 0.48        | 0.52   |
| 13       | 0.64          | 0.69     | 0.68           | 0.65      | 0.48        | 0.52   |
| 14       | 0.64          | 0.69     | 0.68           | 0.65      | 0.48        | 0.52   |
| 15       | 0.64          | 0.69     | 0.68           | 0.65      | 0.48        | 0.52   |
| 16       | 0.64          | 0.68     | 0.69           | 0.66      | 0.48        | 0.51   |
| 17       | 0.64          | 0.68     | 0.69           | 0.66      | 0.48        | 0.51   |
| 18       | 0.63          | 0.68     | 0.69           | 0.66      | 0.47        | 0.51   |
| 19       | 0.63          | 0.68     | 0.69           | 0.66      | 0.47        | 0.51   |
| 20       | 0.63          | 0.68     | 0.70           | 0.66      | 0.47        | 0.51   |
| 21       | 0.63          | 0.68     | 0.70           | 0.67      | 0.47        | 0.50   |
| 22       | 0.63          | 0.67     | 0.70           | 0.67      | 0.47        | 0.50   |
| 23       | 0.63          | 0.67     | 0.70           | 0.67      | 0.47        | 0.50   |
| 24       | 0.63          | 0.67     | 0.71           | 0.68      | 0.46        | 0.50   |
| 25       | 0.62          | 0.67     | 0.71           | 0.68      | 0.46        | 0.50   |
| 26       | 0.62          | 0.66     | 0.71           | 0.68      | 0.46        | 0.49   |
| 27       | 0.62          | 0.66     | 0.72           | 0.69      | 0.45        | 0.49   |
| 28       | 0.62          | 0.66     | 0.72           | 0.69      | 0.45        | 0.49   |
| 29       | 0.62          | 0.66     | 0.72           | 0.69      | 0.45        | 0.49   |
| 30       | 0.61          | 0.65     | 0.72           | 0.70      | 0.45        | 0.48   |
| 31       | 0.61          | 0.65     | 0.73           | 0.70      | 0.44        | 0.48   |

Continued on next page

| $\alpha$ | $\phi_S^\ell$ | $\phi_S$ | $\varphi^\ell$ | $\varphi$ | $\psi^\ell$ | $\psi$ |
|----------|---------------|----------|----------------|-----------|-------------|--------|
| 32       | 0.61          | 0.65     | 0.73           | 0.70      | 0.44        | 0.48   |
| 33       | 0.61          | 0.64     | 0.73           | 0.71      | 0.44        | 0.47   |
| 34       | 0.60          | 0.64     | 0.74           | 0.71      | 0.43        | 0.47   |
| 35       | 0.60          | 0.64     | 0.74           | 0.71      | 0.43        | 0.47   |
| 36       | 0.60          | 0.63     | 0.75           | 0.72      | 0.43        | 0.46   |
| 37       | 0.60          | 0.63     | 0.75           | 0.72      | 0.43        | 0.46   |
| 38       | 0.59          | 0.63     | 0.75           | 0.73      | 0.42        | 0.45   |
| 39       | 0.59          | 0.62     | 0.76           | 0.73      | 0.42        | 0.45   |
| 40       | 0.59          | 0.62     | 0.76           | 0.73      | 0.42        | 0.45   |
| 41       | 0.58          | 0.61     | 0.77           | 0.74      | 0.41        | 0.44   |
| 42       | 0.58          | 0.61     | 0.77           | 0.74      | 0.41        | 0.44   |
| 43       | 0.57          | 0.60     | 0.78           | 0.75      | 0.40        | 0.43   |
| 44       | 0.57          | 0.60     | 0.78           | 0.75      | 0.40        | 0.43   |
| 45       | 0.56          | 0.60     | 0.78           | 0.76      | 0.40        | 0.43   |
| 46       | 0.56          | 0.59     | 0.79           | 0.76      | 0.39        | 0.42   |
| 47       | 0.56          | 0.59     | 0.79           | 0.77      | 0.39        | 0.42   |
| 48       | 0.55          | 0.58     | 0.80           | 0.77      | 0.38        | 0.41   |
| 49       | 0.55          | 0.57     | 0.80           | 0.78      | 0.38        | 0.40   |
| 50       | 0.54          | 0.57     | 0.81           | 0.78      | 0.37        | 0.40   |
| 51       | 0.53          | 0.56     | 0.81           | 0.79      | 0.37        | 0.39   |
| 52       | 0.53          | 0.56     | 0.82           | 0.79      | 0.37        | 0.39   |
| 53       | 0.52          | 0.55     | 0.82           | 0.79      | 0.36        | 0.39   |
| 54       | 0.52          | 0.54     | 0.82           | 0.80      | 0.36        | 0.38   |
| 55       | 0.51          | 0.54     | 0.83           | 0.80      | 0.35        | 0.38   |
| 56       | 0.50          | 0.53     | 0.83           | 0.81      | 0.35        | 0.37   |
| 57       | 0.50          | 0.52     | 0.84           | 0.82      | 0.34        | 0.36   |
| 58       | 0.49          | 0.52     | 0.84           | 0.82      | 0.34        | 0.36   |
| 59       | 0.48          | 0.51     | 0.85           | 0.83      | 0.33        | 0.35   |
| 60       | 0.47          | 0.50     | 0.85           | 0.83      | 0.32        | 0.35   |
| 61       | 0.47          | 0.49     | 0.86           | 0.84      | 0.32        | 0.34   |
| 62       | 0.46          | 0.48     | 0.87           | 0.84      | 0.31        | 0.33   |
| 63       | 0.45          | 0.48     | 0.87           | 0.85      | 0.30        | 0.33   |

Continued on next page



| $\alpha$ | $\phi_S^\ell$ | $\phi_S$ | $\varphi^\ell$ | $\varphi$ | $\psi^\ell$ | $\psi$ |
|----------|---------------|----------|----------------|-----------|-------------|--------|
| 64       | 0.44          | 0.47     | 0.88           | 0.85      | 0.30        | 0.32   |
| 65       | 0.43          | 0.46     | 0.88           | 0.86      | 0.29        | 0.31   |
| 66       | 0.42          | 0.45     | 0.89           | 0.86      | 0.28        | 0.31   |
| 67       | 0.41          | 0.44     | 0.89           | 0.87      | 0.27        | 0.30   |
| 68       | 0.40          | 0.43     | 0.90           | 0.87      | 0.27        | 0.29   |
| 69       | 0.39          | 0.42     | 0.90           | 0.88      | 0.26        | 0.28   |
| 70       | 0.38          | 0.41     | 0.91           | 0.88      | 0.25        | 0.28   |
| 71       | 0.36          | 0.39     | 0.92           | 0.89      | 0.24        | 0.26   |
| 72       | 0.35          | 0.38     | 0.92           | 0.89      | 0.23        | 0.26   |
| 73       | 0.34          | 0.37     | 0.93           | 0.90      | 0.22        | 0.25   |
| 74       | 0.33          | 0.36     | 0.93           | 0.90      | 0.22        | 0.24   |
| 75       | 0.31          | 0.35     | 0.94           | 0.91      | 0.20        | 0.23   |
| 76       | 0.30          | 0.33     | 0.94           | 0.91      | 0.20        | 0.22   |
| 77       | 0.29          | 0.32     | 0.95           | 0.92      | 0.19        | 0.21   |
| 78       | 0.27          | 0.31     | 0.95           | 0.92      | 0.18        | 0.21   |
| 79       | 0.26          | 0.29     | 0.95           | 0.93      | 0.17        | 0.19   |
| 80       | 0.24          | 0.28     | 0.96           | 0.93      | 0.16        | 0.19   |
| 81       | 0.22          | 0.26     | 0.96           | 0.94      | 0.14        | 0.17   |
| 82       | 0.21          | 0.25     | 0.97           | 0.94      | 0.14        | 0.17   |
| 83       | 0.19          | 0.23     | 0.97           | 0.94      | 0.12        | 0.15   |
| 84       | 0.18          | 0.22     | 0.97           | 0.95      | 0.12        | 0.14   |
| 85       | 0.17          | 0.21     | 0.97           | 0.95      | 0.11        | 0.14   |
| 86       | 0.15          | 0.19     | 0.98           | 0.95      | 0.10        | 0.13   |
| 87       | 0.14          | 0.18     | 0.98           | 0.95      | 0.09        | 0.12   |
| 88       | 0.13          | 0.17     | 0.98           | 0.95      | 0.08        | 0.11   |
| 89       | 0.12          | 0.17     | 0.98           | 0.95      | 0.08        | 0.11   |
| 90       | 0.12          | 0.16     | 0.98           | 0.95      | 0.08        | 0.11   |

Table S160: Reference ( $\phi_S$ ,  $\varphi$ ,  $\psi$ ) and approached ( $\phi_S^\ell$ ,  $\varphi^\ell$ ,  $\psi^\ell$ ) values of the topological descriptors for the first excited-state of the pyridinium-phenolate (PP), computed at the wB97XD/6-311+G(d) level of theory.  $\alpha$  is the pyridinium-phenolate central twist angle amplitude.

| $\alpha$ | $\phi_S^\ell$ | $\phi_S$ | $\varphi^\ell$ | $\varphi$ | $\psi^\ell$ | $\psi$ |
|----------|---------------|----------|----------------|-----------|-------------|--------|
| 0        | 0.67          | 0.71     | 0.66           | 0.62      | 0.50        | 0.54   |
| 1        | 0.67          | 0.71     | 0.66           | 0.62      | 0.50        | 0.54   |
| 2        | 0.67          | 0.71     | 0.66           | 0.62      | 0.50        | 0.54   |
| 3        | 0.67          | 0.71     | 0.66           | 0.63      | 0.50        | 0.54   |
| 4        | 0.67          | 0.71     | 0.66           | 0.63      | 0.50        | 0.54   |
| 5        | 0.67          | 0.71     | 0.67           | 0.63      | 0.50        | 0.54   |
| 6        | 0.67          | 0.71     | 0.67           | 0.63      | 0.50        | 0.54   |
| 7        | 0.67          | 0.71     | 0.67           | 0.63      | 0.50        | 0.54   |
| 8        | 0.67          | 0.71     | 0.67           | 0.63      | 0.50        | 0.54   |
| 9        | 0.66          | 0.71     | 0.67           | 0.63      | 0.50        | 0.54   |
| 10       | 0.66          | 0.71     | 0.67           | 0.63      | 0.50        | 0.54   |
| 11       | 0.66          | 0.71     | 0.67           | 0.63      | 0.50        | 0.54   |
| 12       | 0.66          | 0.71     | 0.67           | 0.64      | 0.50        | 0.53   |
| 13       | 0.66          | 0.70     | 0.67           | 0.64      | 0.50        | 0.53   |
| 14       | 0.66          | 0.70     | 0.67           | 0.64      | 0.50        | 0.53   |
| 15       | 0.66          | 0.70     | 0.68           | 0.64      | 0.49        | 0.53   |
| 16       | 0.66          | 0.70     | 0.68           | 0.64      | 0.49        | 0.53   |
| 17       | 0.66          | 0.70     | 0.68           | 0.65      | 0.49        | 0.52   |
| 18       | 0.65          | 0.70     | 0.68           | 0.65      | 0.49        | 0.52   |
| 19       | 0.65          | 0.69     | 0.68           | 0.65      | 0.49        | 0.52   |
| 20       | 0.65          | 0.69     | 0.69           | 0.65      | 0.48        | 0.52   |
| 21       | 0.65          | 0.69     | 0.69           | 0.66      | 0.48        | 0.51   |
| 22       | 0.65          | 0.69     | 0.69           | 0.66      | 0.48        | 0.51   |
| 23       | 0.65          | 0.69     | 0.69           | 0.66      | 0.48        | 0.51   |
| 24       | 0.64          | 0.68     | 0.70           | 0.66      | 0.47        | 0.51   |
| 25       | 0.64          | 0.68     | 0.70           | 0.67      | 0.47        | 0.50   |
| 26       | 0.64          | 0.68     | 0.70           | 0.67      | 0.47        | 0.50   |
| 27       | 0.64          | 0.68     | 0.71           | 0.67      | 0.47        | 0.50   |
| 28       | 0.64          | 0.67     | 0.71           | 0.68      | 0.47        | 0.50   |
| 29       | 0.64          | 0.67     | 0.71           | 0.68      | 0.47        | 0.50   |
| 30       | 0.63          | 0.67     | 0.72           | 0.68      | 0.46        | 0.50   |
| 31       | 0.63          | 0.67     | 0.72           | 0.69      | 0.46        | 0.49   |

Continued on next page

| $\alpha$ | $\phi_S^\ell$ | $\phi_S$ | $\varphi^\ell$ | $\varphi$ | $\psi^\ell$ | $\psi$ |
|----------|---------------|----------|----------------|-----------|-------------|--------|
| 32       | 0.63          | 0.66     | 0.72           | 0.69      | 0.46        | 0.49   |
| 33       | 0.63          | 0.66     | 0.73           | 0.70      | 0.45        | 0.48   |
| 34       | 0.62          | 0.66     | 0.73           | 0.70      | 0.45        | 0.48   |
| 35       | 0.62          | 0.65     | 0.73           | 0.70      | 0.45        | 0.48   |
| 36       | 0.62          | 0.65     | 0.74           | 0.71      | 0.44        | 0.47   |
| 37       | 0.62          | 0.65     | 0.74           | 0.71      | 0.44        | 0.47   |
| 38       | 0.61          | 0.64     | 0.74           | 0.72      | 0.44        | 0.46   |
| 39       | 0.61          | 0.64     | 0.75           | 0.72      | 0.43        | 0.46   |
| 40       | 0.61          | 0.63     | 0.75           | 0.72      | 0.43        | 0.46   |
| 41       | 0.60          | 0.63     | 0.76           | 0.73      | 0.43        | 0.45   |
| 42       | 0.60          | 0.63     | 0.76           | 0.73      | 0.43        | 0.45   |
| 43       | 0.59          | 0.62     | 0.77           | 0.74      | 0.42        | 0.44   |
| 44       | 0.59          | 0.62     | 0.77           | 0.74      | 0.42        | 0.44   |
| 45       | 0.59          | 0.61     | 0.77           | 0.75      | 0.42        | 0.43   |
| 46       | 0.58          | 0.61     | 0.78           | 0.75      | 0.41        | 0.43   |
| 47       | 0.58          | 0.60     | 0.78           | 0.76      | 0.41        | 0.43   |
| 48       | 0.57          | 0.60     | 0.79           | 0.76      | 0.40        | 0.43   |
| 49       | 0.57          | 0.59     | 0.79           | 0.76      | 0.40        | 0.42   |
| 50       | 0.56          | 0.59     | 0.80           | 0.77      | 0.39        | 0.42   |
| 51       | 0.56          | 0.58     | 0.80           | 0.77      | 0.39        | 0.41   |
| 52       | 0.55          | 0.57     | 0.81           | 0.78      | 0.38        | 0.40   |
| 53       | 0.54          | 0.57     | 0.81           | 0.78      | 0.37        | 0.40   |
| 54       | 0.54          | 0.56     | 0.82           | 0.79      | 0.37        | 0.39   |
| 55       | 0.53          | 0.55     | 0.82           | 0.79      | 0.37        | 0.39   |
| 56       | 0.52          | 0.55     | 0.83           | 0.80      | 0.36        | 0.38   |
| 57       | 0.52          | 0.54     | 0.83           | 0.80      | 0.36        | 0.38   |
| 58       | 0.51          | 0.53     | 0.84           | 0.81      | 0.35        | 0.37   |
| 59       | 0.50          | 0.53     | 0.84           | 0.82      | 0.34        | 0.37   |
| 60       | 0.49          | 0.52     | 0.85           | 0.82      | 0.33        | 0.36   |
| 61       | 0.49          | 0.51     | 0.85           | 0.83      | 0.33        | 0.35   |
| 62       | 0.48          | 0.50     | 0.86           | 0.83      | 0.32        | 0.35   |
| 63       | 0.47          | 0.49     | 0.86           | 0.84      | 0.32        | 0.34   |

Continued on next page

| $\alpha$ | $\phi_S^\ell$ | $\phi_S$ | $\varphi^\ell$ | $\varphi$ | $\psi^\ell$ | $\psi$ |
|----------|---------------|----------|----------------|-----------|-------------|--------|
| 64       | 0.46          | 0.48     | 0.87           | 0.84      | 0.31        | 0.33   |
| 65       | 0.45          | 0.48     | 0.87           | 0.85      | 0.30        | 0.33   |
| 66       | 0.44          | 0.47     | 0.88           | 0.85      | 0.30        | 0.32   |
| 67       | 0.43          | 0.46     | 0.89           | 0.86      | 0.29        | 0.31   |
| 68       | 0.42          | 0.45     | 0.89           | 0.86      | 0.28        | 0.31   |
| 69       | 0.41          | 0.44     | 0.90           | 0.87      | 0.27        | 0.30   |
| 70       | 0.40          | 0.42     | 0.90           | 0.88      | 0.27        | 0.28   |
| 71       | 0.38          | 0.41     | 0.91           | 0.88      | 0.25        | 0.28   |
| 72       | 0.37          | 0.40     | 0.91           | 0.89      | 0.25        | 0.27   |
| 73       | 0.36          | 0.39     | 0.92           | 0.89      | 0.24        | 0.26   |
| 74       | 0.35          | 0.38     | 0.93           | 0.90      | 0.23        | 0.25   |
| 75       | 0.33          | 0.36     | 0.93           | 0.90      | 0.22        | 0.24   |
| 76       | 0.32          | 0.35     | 0.94           | 0.91      | 0.21        | 0.23   |
| 77       | 0.30          | 0.34     | 0.94           | 0.91      | 0.20        | 0.23   |
| 78       | 0.29          | 0.32     | 0.95           | 0.92      | 0.19        | 0.21   |
| 79       | 0.27          | 0.31     | 0.95           | 0.92      | 0.18        | 0.21   |
| 80       | 0.25          | 0.29     | 0.96           | 0.93      | 0.16        | 0.19   |
| 81       | 0.24          | 0.28     | 0.96           | 0.93      | 0.16        | 0.19   |
| 82       | 0.22          | 0.26     | 0.97           | 0.94      | 0.14        | 0.17   |
| 83       | 0.20          | 0.24     | 0.97           | 0.94      | 0.13        | 0.16   |
| 84       | 0.18          | 0.23     | 0.97           | 0.94      | 0.12        | 0.15   |
| 85       | 0.17          | 0.21     | 0.98           | 0.95      | 0.11        | 0.14   |
| 86       | 0.15          | 0.20     | 0.98           | 0.95      | 0.10        | 0.13   |
| 87       | 0.14          | 0.19     | 0.98           | 0.95      | 0.09        | 0.13   |
| 88       | 0.12          | 0.17     | 0.98           | 0.95      | 0.08        | 0.11   |
| 89       | 0.11          | 0.17     | 0.98           | 0.95      | 0.07        | 0.11   |
| 90       | 0.11          | 0.16     | 0.98           | 0.95      | 0.07        | 0.11   |

Table S161: Reference ( $\phi_S$ ,  $\varphi$ ,  $\psi$ ) and approached ( $\phi_S^\ell$ ,  $\varphi^\ell$ ,  $\psi^\ell$ ) values of the topological descriptors for the first excited-state of the pyridinium-phenolate (PP), computed at the wB97XD/6-311G(d) level of theory.  $\alpha$  is the pyridinium-phenolate central twist angle amplitude.

| $\alpha$ | $\phi_S^\ell$ | $\phi_S$ | $\varphi^\ell$ | $\varphi$ | $\psi^\ell$ | $\psi$ |
|----------|---------------|----------|----------------|-----------|-------------|--------|
| 0        | 0.65          | 0.69     | 0.67           | 0.64      | 0.49        | 0.52   |
| 1        | 0.65          | 0.69     | 0.67           | 0.64      | 0.49        | 0.52   |
| 2        | 0.65          | 0.69     | 0.67           | 0.64      | 0.49        | 0.52   |
| 3        | 0.65          | 0.69     | 0.67           | 0.64      | 0.49        | 0.52   |
| 4        | 0.65          | 0.69     | 0.67           | 0.64      | 0.49        | 0.52   |
| 5        | 0.65          | 0.69     | 0.67           | 0.64      | 0.49        | 0.52   |
| 6        | 0.65          | 0.69     | 0.67           | 0.64      | 0.49        | 0.52   |
| 7        | 0.65          | 0.69     | 0.67           | 0.65      | 0.49        | 0.52   |
| 8        | 0.65          | 0.69     | 0.67           | 0.65      | 0.49        | 0.52   |
| 9        | 0.65          | 0.69     | 0.68           | 0.65      | 0.49        | 0.52   |
| 10       | 0.65          | 0.69     | 0.68           | 0.65      | 0.49        | 0.52   |
| 11       | 0.64          | 0.69     | 0.68           | 0.65      | 0.48        | 0.52   |
| 12       | 0.64          | 0.68     | 0.68           | 0.65      | 0.48        | 0.51   |
| 13       | 0.64          | 0.68     | 0.68           | 0.65      | 0.48        | 0.51   |
| 14       | 0.64          | 0.68     | 0.68           | 0.66      | 0.48        | 0.51   |
| 15       | 0.64          | 0.68     | 0.68           | 0.66      | 0.48        | 0.51   |
| 16       | 0.64          | 0.68     | 0.69           | 0.66      | 0.48        | 0.51   |
| 17       | 0.64          | 0.68     | 0.69           | 0.66      | 0.48        | 0.51   |
| 18       | 0.64          | 0.68     | 0.69           | 0.66      | 0.48        | 0.51   |
| 19       | 0.64          | 0.67     | 0.69           | 0.67      | 0.48        | 0.50   |
| 20       | 0.63          | 0.67     | 0.69           | 0.67      | 0.47        | 0.50   |
| 21       | 0.63          | 0.67     | 0.70           | 0.67      | 0.47        | 0.50   |
| 22       | 0.63          | 0.67     | 0.70           | 0.67      | 0.47        | 0.50   |
| 23       | 0.63          | 0.67     | 0.70           | 0.68      | 0.47        | 0.50   |
| 24       | 0.63          | 0.66     | 0.71           | 0.68      | 0.46        | 0.49   |
| 25       | 0.63          | 0.66     | 0.71           | 0.68      | 0.46        | 0.49   |
| 26       | 0.63          | 0.66     | 0.71           | 0.69      | 0.46        | 0.49   |
| 27       | 0.62          | 0.66     | 0.71           | 0.69      | 0.46        | 0.49   |
| 28       | 0.62          | 0.65     | 0.72           | 0.69      | 0.45        | 0.48   |
| 29       | 0.62          | 0.65     | 0.72           | 0.70      | 0.45        | 0.48   |
| 30       | 0.62          | 0.65     | 0.72           | 0.70      | 0.45        | 0.48   |
| 31       | 0.62          | 0.65     | 0.73           | 0.70      | 0.45        | 0.48   |

Continued on next page

| $\alpha$ | $\phi_S^\ell$ | $\phi_S$ | $\varphi^\ell$ | $\varphi$ | $\psi^\ell$ | $\psi$ |
|----------|---------------|----------|----------------|-----------|-------------|--------|
| 32       | 0.61          | 0.64     | 0.73           | 0.71      | 0.44        | 0.47   |
| 33       | 0.61          | 0.64     | 0.73           | 0.71      | 0.44        | 0.47   |
| 34       | 0.61          | 0.64     | 0.74           | 0.71      | 0.44        | 0.47   |
| 35       | 0.61          | 0.63     | 0.74           | 0.72      | 0.44        | 0.46   |
| 36       | 0.60          | 0.63     | 0.74           | 0.72      | 0.43        | 0.46   |
| 37       | 0.60          | 0.63     | 0.75           | 0.73      | 0.43        | 0.45   |
| 38       | 0.60          | 0.62     | 0.75           | 0.73      | 0.43        | 0.45   |
| 39       | 0.59          | 0.62     | 0.76           | 0.73      | 0.42        | 0.45   |
| 40       | 0.59          | 0.62     | 0.76           | 0.74      | 0.42        | 0.44   |
| 41       | 0.59          | 0.61     | 0.76           | 0.74      | 0.42        | 0.44   |
| 42       | 0.58          | 0.61     | 0.77           | 0.75      | 0.41        | 0.43   |
| 43       | 0.58          | 0.60     | 0.77           | 0.75      | 0.41        | 0.43   |
| 44       | 0.57          | 0.60     | 0.78           | 0.76      | 0.40        | 0.43   |
| 45       | 0.57          | 0.59     | 0.78           | 0.76      | 0.40        | 0.42   |
| 46       | 0.56          | 0.59     | 0.79           | 0.76      | 0.39        | 0.42   |
| 47       | 0.56          | 0.58     | 0.79           | 0.77      | 0.39        | 0.41   |
| 48       | 0.56          | 0.58     | 0.80           | 0.77      | 0.39        | 0.41   |
| 49       | 0.55          | 0.57     | 0.80           | 0.78      | 0.38        | 0.40   |
| 50       | 0.54          | 0.57     | 0.80           | 0.78      | 0.38        | 0.40   |
| 51       | 0.54          | 0.56     | 0.81           | 0.79      | 0.37        | 0.39   |
| 52       | 0.53          | 0.56     | 0.81           | 0.79      | 0.37        | 0.39   |
| 53       | 0.53          | 0.55     | 0.82           | 0.80      | 0.37        | 0.38   |
| 54       | 0.52          | 0.54     | 0.82           | 0.80      | 0.36        | 0.38   |
| 55       | 0.51          | 0.54     | 0.83           | 0.81      | 0.35        | 0.37   |
| 56       | 0.51          | 0.53     | 0.83           | 0.81      | 0.35        | 0.37   |
| 57       | 0.50          | 0.52     | 0.84           | 0.82      | 0.34        | 0.36   |
| 58       | 0.49          | 0.52     | 0.84           | 0.82      | 0.34        | 0.36   |
| 59       | 0.49          | 0.51     | 0.85           | 0.83      | 0.33        | 0.35   |
| 60       | 0.48          | 0.50     | 0.85           | 0.83      | 0.33        | 0.35   |
| 61       | 0.47          | 0.49     | 0.86           | 0.84      | 0.32        | 0.34   |
| 62       | 0.46          | 0.48     | 0.86           | 0.84      | 0.31        | 0.33   |
| 63       | 0.45          | 0.48     | 0.87           | 0.85      | 0.30        | 0.33   |

Continued on next page

| $\alpha$ | $\phi_S^\ell$ | $\phi_S$ | $\varphi^\ell$ | $\varphi$ | $\psi^\ell$ | $\psi$ |
|----------|---------------|----------|----------------|-----------|-------------|--------|
| 64       | 0.44          | 0.47     | 0.88           | 0.85      | 0.30        | 0.32   |
| 65       | 0.43          | 0.46     | 0.88           | 0.86      | 0.29        | 0.31   |
| 66       | 0.42          | 0.45     | 0.89           | 0.86      | 0.28        | 0.31   |
| 67       | 0.41          | 0.44     | 0.89           | 0.87      | 0.27        | 0.30   |
| 68       | 0.40          | 0.43     | 0.90           | 0.87      | 0.27        | 0.29   |
| 69       | 0.39          | 0.42     | 0.91           | 0.88      | 0.26        | 0.28   |
| 70       | 0.38          | 0.41     | 0.91           | 0.88      | 0.25        | 0.28   |
| 71       | 0.37          | 0.40     | 0.92           | 0.89      | 0.24        | 0.27   |
| 72       | 0.35          | 0.38     | 0.92           | 0.90      | 0.23        | 0.25   |
| 73       | 0.34          | 0.37     | 0.93           | 0.90      | 0.22        | 0.25   |
| 74       | 0.33          | 0.36     | 0.93           | 0.91      | 0.22        | 0.24   |
| 75       | 0.31          | 0.35     | 0.94           | 0.91      | 0.20        | 0.23   |
| 76       | 0.30          | 0.33     | 0.94           | 0.92      | 0.20        | 0.22   |
| 77       | 0.28          | 0.32     | 0.95           | 0.92      | 0.18        | 0.21   |
| 78       | 0.27          | 0.31     | 0.95           | 0.93      | 0.18        | 0.20   |
| 79       | 0.25          | 0.29     | 0.96           | 0.93      | 0.16        | 0.19   |
| 80       | 0.24          | 0.28     | 0.96           | 0.93      | 0.16        | 0.19   |
| 81       | 0.22          | 0.26     | 0.97           | 0.94      | 0.14        | 0.17   |
| 82       | 0.20          | 0.25     | 0.97           | 0.94      | 0.13        | 0.17   |
| 83       | 0.19          | 0.23     | 0.97           | 0.95      | 0.12        | 0.15   |
| 84       | 0.17          | 0.22     | 0.98           | 0.95      | 0.11        | 0.14   |
| 85       | 0.16          | 0.20     | 0.98           | 0.95      | 0.10        | 0.13   |
| 86       | 0.15          | 0.19     | 0.98           | 0.95      | 0.10        | 0.13   |
| 87       | 0.13          | 0.18     | 0.98           | 0.96      | 0.08        | 0.12   |
| 88       | 0.12          | 0.16     | 0.98           | 0.96      | 0.08        | 0.11   |
| 89       | 0.11          | 0.16     | 0.99           | 0.96      | 0.07        | 0.11   |
| 90       | 0.11          | 0.15     | 0.99           | 0.96      | 0.07        | 0.10   |

Table S162: Reference ( $\phi_S$ ,  $\varphi$ ,  $\psi$ ) and approached ( $\phi_S^\ell$ ,  $\varphi^\ell$ ,  $\psi^\ell$ ) values of the topological descriptors for the first excited-state of the pyridinium-phenolate (PP), computed at the wB97XD/6-311+G level of theory.  $\alpha$  is the pyridinium-phenolate central twist angle amplitude.

| $\alpha$ | $\phi_S^\ell$ | $\phi_S$ | $\varphi^\ell$ | $\varphi$ | $\psi^\ell$ | $\psi$ |
|----------|---------------|----------|----------------|-----------|-------------|--------|
| 0        | 0.67          | 0.71     | 0.66           | 0.63      | 0.50        | 0.54   |
| 1        | 0.67          | 0.71     | 0.66           | 0.63      | 0.50        | 0.54   |
| 2        | 0.67          | 0.71     | 0.66           | 0.63      | 0.50        | 0.54   |
| 3        | 0.67          | 0.71     | 0.66           | 0.63      | 0.50        | 0.54   |
| 4        | 0.67          | 0.71     | 0.66           | 0.63      | 0.50        | 0.54   |
| 5        | 0.67          | 0.71     | 0.66           | 0.63      | 0.50        | 0.54   |
| 6        | 0.67          | 0.71     | 0.66           | 0.63      | 0.50        | 0.54   |
| 7        | 0.67          | 0.70     | 0.67           | 0.63      | 0.50        | 0.53   |
| 8        | 0.67          | 0.70     | 0.67           | 0.64      | 0.50        | 0.53   |
| 9        | 0.67          | 0.70     | 0.67           | 0.64      | 0.50        | 0.53   |
| 10       | 0.67          | 0.70     | 0.67           | 0.64      | 0.50        | 0.53   |
| 11       | 0.67          | 0.70     | 0.67           | 0.64      | 0.50        | 0.53   |
| 12       | 0.66          | 0.70     | 0.67           | 0.64      | 0.50        | 0.53   |
| 13       | 0.66          | 0.70     | 0.67           | 0.64      | 0.50        | 0.53   |
| 14       | 0.66          | 0.70     | 0.67           | 0.64      | 0.50        | 0.53   |
| 15       | 0.66          | 0.70     | 0.68           | 0.65      | 0.49        | 0.52   |
| 16       | 0.66          | 0.69     | 0.68           | 0.65      | 0.49        | 0.52   |
| 17       | 0.66          | 0.69     | 0.68           | 0.65      | 0.49        | 0.52   |
| 18       | 0.66          | 0.69     | 0.68           | 0.65      | 0.49        | 0.52   |
| 19       | 0.66          | 0.69     | 0.68           | 0.66      | 0.49        | 0.51   |
| 20       | 0.65          | 0.69     | 0.69           | 0.66      | 0.48        | 0.51   |
| 21       | 0.65          | 0.69     | 0.69           | 0.66      | 0.48        | 0.51   |
| 22       | 0.65          | 0.68     | 0.69           | 0.66      | 0.48        | 0.51   |
| 23       | 0.65          | 0.68     | 0.69           | 0.67      | 0.48        | 0.50   |
| 24       | 0.65          | 0.68     | 0.70           | 0.67      | 0.48        | 0.50   |
| 25       | 0.65          | 0.68     | 0.70           | 0.67      | 0.48        | 0.50   |
| 26       | 0.64          | 0.67     | 0.70           | 0.68      | 0.47        | 0.50   |
| 27       | 0.64          | 0.67     | 0.71           | 0.68      | 0.47        | 0.50   |
| 28       | 0.64          | 0.67     | 0.71           | 0.68      | 0.47        | 0.50   |
| 29       | 0.64          | 0.67     | 0.71           | 0.69      | 0.47        | 0.49   |
| 30       | 0.64          | 0.66     | 0.71           | 0.69      | 0.47        | 0.49   |
| 31       | 0.63          | 0.66     | 0.72           | 0.69      | 0.46        | 0.49   |

Continued on next page



| $\alpha$ | $\phi_S^\ell$ | $\phi_S$ | $\varphi^\ell$ | $\varphi$ | $\psi^\ell$ | $\psi$ |
|----------|---------------|----------|----------------|-----------|-------------|--------|
| 32       | 0.63          | 0.66     | 0.72           | 0.70      | 0.46        | 0.48   |
| 33       | 0.63          | 0.65     | 0.72           | 0.70      | 0.46        | 0.48   |
| 34       | 0.63          | 0.65     | 0.73           | 0.70      | 0.45        | 0.48   |
| 35       | 0.62          | 0.65     | 0.73           | 0.71      | 0.45        | 0.47   |
| 36       | 0.62          | 0.64     | 0.73           | 0.71      | 0.45        | 0.47   |
| 37       | 0.62          | 0.64     | 0.74           | 0.72      | 0.44        | 0.46   |
| 38       | 0.62          | 0.64     | 0.74           | 0.72      | 0.44        | 0.46   |
| 39       | 0.61          | 0.63     | 0.75           | 0.72      | 0.43        | 0.46   |
| 40       | 0.61          | 0.63     | 0.75           | 0.73      | 0.43        | 0.45   |
| 41       | 0.61          | 0.63     | 0.75           | 0.73      | 0.43        | 0.45   |
| 42       | 0.60          | 0.62     | 0.76           | 0.74      | 0.43        | 0.44   |
| 43       | 0.60          | 0.62     | 0.76           | 0.74      | 0.43        | 0.44   |
| 44       | 0.59          | 0.61     | 0.77           | 0.75      | 0.42        | 0.43   |
| 45       | 0.59          | 0.61     | 0.77           | 0.75      | 0.42        | 0.43   |
| 46       | 0.58          | 0.60     | 0.78           | 0.75      | 0.41        | 0.43   |
| 47       | 0.58          | 0.60     | 0.78           | 0.76      | 0.41        | 0.43   |
| 48       | 0.58          | 0.59     | 0.79           | 0.76      | 0.40        | 0.42   |
| 49       | 0.57          | 0.59     | 0.79           | 0.77      | 0.40        | 0.42   |
| 50       | 0.56          | 0.58     | 0.80           | 0.77      | 0.39        | 0.41   |
| 51       | 0.56          | 0.58     | 0.80           | 0.78      | 0.39        | 0.41   |
| 52       | 0.55          | 0.57     | 0.81           | 0.78      | 0.38        | 0.40   |
| 53       | 0.55          | 0.57     | 0.81           | 0.79      | 0.38        | 0.40   |
| 54       | 0.54          | 0.56     | 0.81           | 0.79      | 0.37        | 0.39   |
| 55       | 0.53          | 0.55     | 0.82           | 0.80      | 0.37        | 0.38   |
| 56       | 0.53          | 0.55     | 0.82           | 0.80      | 0.37        | 0.38   |
| 57       | 0.52          | 0.54     | 0.83           | 0.81      | 0.36        | 0.37   |
| 58       | 0.51          | 0.53     | 0.84           | 0.81      | 0.35        | 0.37   |
| 59       | 0.51          | 0.52     | 0.84           | 0.82      | 0.35        | 0.36   |
| 60       | 0.50          | 0.52     | 0.85           | 0.82      | 0.34        | 0.36   |
| 61       | 0.49          | 0.51     | 0.85           | 0.83      | 0.33        | 0.35   |
| 62       | 0.48          | 0.50     | 0.86           | 0.83      | 0.32        | 0.35   |
| 63       | 0.47          | 0.49     | 0.86           | 0.84      | 0.32        | 0.34   |

Continued on next page

| $\alpha$ | $\phi_S^\ell$ | $\phi_S$ | $\varphi^\ell$ | $\varphi$ | $\psi^\ell$ | $\psi$ |
|----------|---------------|----------|----------------|-----------|-------------|--------|
| 64       | 0.46          | 0.48     | 0.87           | 0.84      | 0.31        | 0.33   |
| 65       | 0.45          | 0.48     | 0.87           | 0.85      | 0.30        | 0.33   |
| 66       | 0.44          | 0.47     | 0.88           | 0.86      | 0.30        | 0.32   |
| 67       | 0.43          | 0.46     | 0.89           | 0.86      | 0.29        | 0.31   |
| 68       | 0.42          | 0.45     | 0.89           | 0.87      | 0.28        | 0.30   |
| 69       | 0.41          | 0.44     | 0.90           | 0.87      | 0.27        | 0.30   |
| 70       | 0.40          | 0.42     | 0.90           | 0.88      | 0.27        | 0.28   |
| 71       | 0.39          | 0.41     | 0.91           | 0.88      | 0.26        | 0.28   |
| 72       | 0.37          | 0.40     | 0.92           | 0.89      | 0.24        | 0.27   |
| 73       | 0.36          | 0.39     | 0.92           | 0.89      | 0.24        | 0.26   |
| 74       | 0.35          | 0.38     | 0.93           | 0.90      | 0.23        | 0.25   |
| 75       | 0.33          | 0.36     | 0.93           | 0.90      | 0.22        | 0.24   |
| 76       | 0.32          | 0.35     | 0.94           | 0.91      | 0.21        | 0.23   |
| 77       | 0.30          | 0.34     | 0.94           | 0.92      | 0.20        | 0.23   |
| 78       | 0.28          | 0.32     | 0.95           | 0.92      | 0.18        | 0.21   |
| 79       | 0.27          | 0.31     | 0.95           | 0.93      | 0.18        | 0.20   |
| 80       | 0.25          | 0.29     | 0.96           | 0.93      | 0.16        | 0.19   |
| 81       | 0.23          | 0.27     | 0.96           | 0.94      | 0.15        | 0.18   |
| 82       | 0.21          | 0.26     | 0.97           | 0.94      | 0.14        | 0.17   |
| 83       | 0.19          | 0.24     | 0.97           | 0.94      | 0.12        | 0.16   |
| 84       | 0.18          | 0.22     | 0.98           | 0.95      | 0.12        | 0.14   |
| 85       | 0.16          | 0.21     | 0.98           | 0.95      | 0.10        | 0.14   |
| 86       | 0.14          | 0.19     | 0.98           | 0.95      | 0.09        | 0.13   |
| 87       | 0.13          | 0.18     | 0.99           | 0.96      | 0.08        | 0.12   |
| 88       | 0.11          | 0.17     | 0.99           | 0.96      | 0.07        | 0.11   |
| 89       | 0.10          | 0.16     | 0.99           | 0.96      | 0.06        | 0.11   |
| 90       | 0.09          | 0.15     | 0.99           | 0.96      | 0.06        | 0.10   |

Table S163: Reference ( $\phi_S$ ,  $\varphi$ ,  $\psi$ ) and approached ( $\phi_S^\ell$ ,  $\varphi^\ell$ ,  $\psi^\ell$ ) values of the topological descriptors for the first excited-state of the pyridinium-phenolate (PP), computed at the wB97XD/6-311G level of theory.  $\alpha$  is the pyridinium-phenolate central twist angle amplitude.

| $\alpha$ | $\phi_S^\ell$ | $\phi_S$ | $\varphi^\ell$ | $\varphi$ | $\psi^\ell$ | $\psi$ |
|----------|---------------|----------|----------------|-----------|-------------|--------|
| 0        | 0.65          | 0.70     | 0.67           | 0.64      | 0.49        | 0.53   |
| 1        | 0.65          | 0.70     | 0.67           | 0.64      | 0.49        | 0.53   |
| 2        | 0.65          | 0.70     | 0.67           | 0.64      | 0.49        | 0.53   |
| 3        | 0.65          | 0.70     | 0.67           | 0.64      | 0.49        | 0.53   |
| 4        | 0.65          | 0.70     | 0.68           | 0.64      | 0.49        | 0.53   |
| 5        | 0.65          | 0.70     | 0.68           | 0.64      | 0.49        | 0.53   |
| 6        | 0.65          | 0.69     | 0.68           | 0.64      | 0.49        | 0.52   |
| 7        | 0.65          | 0.69     | 0.68           | 0.64      | 0.49        | 0.52   |
| 8        | 0.64          | 0.69     | 0.68           | 0.64      | 0.48        | 0.52   |
| 9        | 0.64          | 0.69     | 0.68           | 0.64      | 0.48        | 0.52   |
| 10       | 0.64          | 0.69     | 0.68           | 0.65      | 0.48        | 0.52   |
| 11       | 0.64          | 0.69     | 0.68           | 0.65      | 0.48        | 0.52   |
| 12       | 0.64          | 0.69     | 0.68           | 0.65      | 0.48        | 0.52   |
| 13       | 0.64          | 0.69     | 0.68           | 0.65      | 0.48        | 0.52   |
| 14       | 0.64          | 0.69     | 0.69           | 0.65      | 0.48        | 0.52   |
| 15       | 0.64          | 0.68     | 0.69           | 0.65      | 0.48        | 0.51   |
| 16       | 0.64          | 0.68     | 0.69           | 0.66      | 0.48        | 0.51   |
| 17       | 0.64          | 0.68     | 0.69           | 0.66      | 0.48        | 0.51   |
| 18       | 0.63          | 0.68     | 0.69           | 0.66      | 0.47        | 0.51   |
| 19       | 0.63          | 0.68     | 0.70           | 0.66      | 0.47        | 0.51   |
| 20       | 0.63          | 0.68     | 0.70           | 0.67      | 0.47        | 0.50   |
| 21       | 0.63          | 0.67     | 0.70           | 0.67      | 0.47        | 0.50   |
| 22       | 0.63          | 0.67     | 0.70           | 0.67      | 0.47        | 0.50   |
| 23       | 0.63          | 0.67     | 0.71           | 0.67      | 0.46        | 0.50   |
| 24       | 0.63          | 0.67     | 0.71           | 0.68      | 0.46        | 0.50   |
| 25       | 0.62          | 0.67     | 0.71           | 0.68      | 0.46        | 0.50   |
| 26       | 0.62          | 0.66     | 0.72           | 0.68      | 0.45        | 0.49   |
| 27       | 0.62          | 0.66     | 0.72           | 0.69      | 0.45        | 0.49   |
| 28       | 0.62          | 0.66     | 0.72           | 0.69      | 0.45        | 0.49   |
| 29       | 0.62          | 0.65     | 0.72           | 0.69      | 0.45        | 0.48   |
| 30       | 0.61          | 0.65     | 0.73           | 0.70      | 0.44        | 0.48   |
| 31       | 0.61          | 0.65     | 0.73           | 0.70      | 0.44        | 0.48   |

Continued on next page

| $\alpha$ | $\phi_S^\ell$ | $\phi_S$ | $\varphi^\ell$ | $\varphi$ | $\psi^\ell$ | $\psi$ |
|----------|---------------|----------|----------------|-----------|-------------|--------|
| 32       | 0.61          | 0.65     | 0.73           | 0.70      | 0.44        | 0.48   |
| 33       | 0.61          | 0.64     | 0.74           | 0.71      | 0.44        | 0.47   |
| 34       | 0.60          | 0.64     | 0.74           | 0.71      | 0.43        | 0.47   |
| 35       | 0.60          | 0.64     | 0.74           | 0.71      | 0.43        | 0.47   |
| 36       | 0.60          | 0.63     | 0.75           | 0.72      | 0.43        | 0.46   |
| 37       | 0.59          | 0.63     | 0.75           | 0.72      | 0.42        | 0.46   |
| 38       | 0.59          | 0.62     | 0.76           | 0.73      | 0.42        | 0.45   |
| 39       | 0.59          | 0.62     | 0.76           | 0.73      | 0.42        | 0.45   |
| 40       | 0.58          | 0.62     | 0.76           | 0.74      | 0.41        | 0.44   |
| 41       | 0.58          | 0.61     | 0.77           | 0.74      | 0.41        | 0.44   |
| 42       | 0.58          | 0.61     | 0.77           | 0.74      | 0.41        | 0.44   |
| 43       | 0.57          | 0.60     | 0.78           | 0.75      | 0.40        | 0.43   |
| 44       | 0.57          | 0.60     | 0.78           | 0.75      | 0.40        | 0.43   |
| 45       | 0.56          | 0.59     | 0.79           | 0.76      | 0.39        | 0.42   |
| 46       | 0.56          | 0.59     | 0.79           | 0.76      | 0.39        | 0.42   |
| 47       | 0.55          | 0.58     | 0.80           | 0.77      | 0.38        | 0.41   |
| 48       | 0.55          | 0.58     | 0.80           | 0.77      | 0.38        | 0.41   |
| 49       | 0.54          | 0.57     | 0.80           | 0.78      | 0.38        | 0.40   |
| 50       | 0.54          | 0.57     | 0.81           | 0.78      | 0.37        | 0.40   |
| 51       | 0.53          | 0.56     | 0.81           | 0.79      | 0.37        | 0.39   |
| 52       | 0.53          | 0.56     | 0.82           | 0.79      | 0.37        | 0.39   |
| 53       | 0.52          | 0.55     | 0.82           | 0.80      | 0.36        | 0.38   |
| 54       | 0.52          | 0.54     | 0.83           | 0.80      | 0.36        | 0.38   |
| 55       | 0.51          | 0.54     | 0.83           | 0.81      | 0.35        | 0.37   |
| 56       | 0.50          | 0.53     | 0.84           | 0.81      | 0.34        | 0.37   |
| 57       | 0.50          | 0.52     | 0.84           | 0.82      | 0.34        | 0.36   |
| 58       | 0.49          | 0.51     | 0.85           | 0.82      | 0.33        | 0.35   |
| 59       | 0.48          | 0.51     | 0.85           | 0.83      | 0.33        | 0.35   |
| 60       | 0.47          | 0.50     | 0.86           | 0.83      | 0.32        | 0.35   |
| 61       | 0.47          | 0.49     | 0.86           | 0.84      | 0.32        | 0.34   |
| 62       | 0.46          | 0.48     | 0.87           | 0.84      | 0.31        | 0.33   |
| 63       | 0.45          | 0.47     | 0.87           | 0.85      | 0.30        | 0.32   |

Continued on next page

| $\alpha$ | $\phi_S^\ell$ | $\phi_S$ | $\varphi^\ell$ | $\varphi$ | $\psi^\ell$ | $\psi$ |
|----------|---------------|----------|----------------|-----------|-------------|--------|
| 64       | 0.44          | 0.46     | 0.88           | 0.85      | 0.30        | 0.32   |
| 65       | 0.43          | 0.46     | 0.88           | 0.86      | 0.29        | 0.31   |
| 66       | 0.42          | 0.45     | 0.89           | 0.86      | 0.28        | 0.31   |
| 67       | 0.41          | 0.44     | 0.89           | 0.87      | 0.27        | 0.30   |
| 68       | 0.40          | 0.43     | 0.90           | 0.87      | 0.27        | 0.29   |
| 69       | 0.39          | 0.42     | 0.90           | 0.88      | 0.26        | 0.28   |
| 70       | 0.38          | 0.40     | 0.91           | 0.88      | 0.25        | 0.27   |
| 71       | 0.37          | 0.39     | 0.91           | 0.89      | 0.25        | 0.26   |
| 72       | 0.36          | 0.38     | 0.92           | 0.89      | 0.24        | 0.26   |
| 73       | 0.34          | 0.37     | 0.92           | 0.90      | 0.23        | 0.25   |
| 74       | 0.33          | 0.36     | 0.93           | 0.90      | 0.22        | 0.24   |
| 75       | 0.32          | 0.35     | 0.93           | 0.91      | 0.21        | 0.23   |
| 76       | 0.31          | 0.33     | 0.94           | 0.91      | 0.20        | 0.22   |
| 77       | 0.29          | 0.32     | 0.94           | 0.92      | 0.19        | 0.21   |
| 78       | 0.28          | 0.31     | 0.94           | 0.92      | 0.18        | 0.21   |
| 79       | 0.26          | 0.29     | 0.95           | 0.93      | 0.17        | 0.19   |
| 80       | 0.25          | 0.28     | 0.95           | 0.93      | 0.16        | 0.19   |
| 81       | 0.23          | 0.26     | 0.95           | 0.93      | 0.15        | 0.17   |
| 82       | 0.22          | 0.25     | 0.96           | 0.94      | 0.14        | 0.17   |
| 83       | 0.20          | 0.24     | 0.96           | 0.94      | 0.13        | 0.16   |
| 84       | 0.19          | 0.22     | 0.96           | 0.94      | 0.12        | 0.15   |
| 85       | 0.17          | 0.21     | 0.97           | 0.95      | 0.11        | 0.14   |
| 86       | 0.16          | 0.20     | 0.97           | 0.95      | 0.10        | 0.13   |
| 87       | 0.15          | 0.18     | 0.97           | 0.95      | 0.10        | 0.12   |
| 88       | 0.14          | 0.17     | 0.97           | 0.95      | 0.09        | 0.11   |
| 89       | 0.13          | 0.17     | 0.97           | 0.95      | 0.08        | 0.11   |
| 90       | 0.13          | 0.16     | 0.97           | 0.95      | 0.08        | 0.11   |

Table S164: Reference ( $\phi_S$ ,  $\varphi$ ,  $\psi$ ) and approached ( $\phi_S^\ell$ ,  $\varphi^\ell$ ,  $\psi^\ell$ ) values of the topological descriptors for the first excited-state of the pyridinium-phenolate (PP), computed at the wB97XD/6-31++G(2d,p) level of theory.  $\alpha$  is the pyridinium-phenolate central twist angle amplitude.

| $\alpha$ | $\phi_S^\ell$ | $\phi_S$ | $\varphi^\ell$ | $\varphi$ | $\psi^\ell$ | $\psi$ |
|----------|---------------|----------|----------------|-----------|-------------|--------|
| 0        | 0.65          | 0.70     | 0.67           | 0.64      | 0.49        | 0.53   |
| 1        | 0.65          | 0.70     | 0.67           | 0.64      | 0.49        | 0.53   |
| 2        | 0.65          | 0.70     | 0.67           | 0.64      | 0.49        | 0.53   |
| 3        | 0.65          | 0.70     | 0.67           | 0.64      | 0.49        | 0.53   |
| 4        | 0.65          | 0.70     | 0.67           | 0.64      | 0.49        | 0.53   |
| 5        | 0.65          | 0.70     | 0.67           | 0.64      | 0.49        | 0.53   |
| 6        | 0.65          | 0.70     | 0.67           | 0.64      | 0.49        | 0.53   |
| 7        | 0.64          | 0.70     | 0.67           | 0.64      | 0.49        | 0.53   |
| 8        | 0.64          | 0.69     | 0.67           | 0.64      | 0.49        | 0.52   |
| 9        | 0.64          | 0.69     | 0.68           | 0.64      | 0.48        | 0.52   |
| 10       | 0.64          | 0.69     | 0.68           | 0.64      | 0.48        | 0.52   |
| 11       | 0.64          | 0.69     | 0.68           | 0.65      | 0.48        | 0.52   |
| 12       | 0.64          | 0.69     | 0.68           | 0.65      | 0.48        | 0.52   |
| 13       | 0.64          | 0.69     | 0.68           | 0.65      | 0.48        | 0.52   |
| 14       | 0.64          | 0.69     | 0.68           | 0.65      | 0.48        | 0.52   |
| 15       | 0.64          | 0.69     | 0.68           | 0.65      | 0.48        | 0.52   |
| 16       | 0.64          | 0.68     | 0.69           | 0.65      | 0.48        | 0.51   |
| 17       | 0.64          | 0.68     | 0.69           | 0.66      | 0.48        | 0.51   |
| 18       | 0.64          | 0.68     | 0.69           | 0.66      | 0.48        | 0.51   |
| 19       | 0.63          | 0.68     | 0.69           | 0.66      | 0.47        | 0.51   |
| 20       | 0.63          | 0.68     | 0.69           | 0.66      | 0.47        | 0.51   |
| 21       | 0.63          | 0.68     | 0.70           | 0.67      | 0.47        | 0.50   |
| 22       | 0.63          | 0.67     | 0.70           | 0.67      | 0.47        | 0.50   |
| 23       | 0.63          | 0.67     | 0.70           | 0.67      | 0.47        | 0.50   |
| 24       | 0.63          | 0.67     | 0.71           | 0.68      | 0.46        | 0.50   |
| 25       | 0.63          | 0.67     | 0.71           | 0.68      | 0.46        | 0.50   |
| 26       | 0.62          | 0.66     | 0.71           | 0.68      | 0.46        | 0.49   |
| 27       | 0.62          | 0.66     | 0.71           | 0.69      | 0.46        | 0.49   |
| 28       | 0.62          | 0.66     | 0.72           | 0.69      | 0.45        | 0.49   |
| 29       | 0.62          | 0.66     | 0.72           | 0.69      | 0.45        | 0.49   |
| 30       | 0.62          | 0.65     | 0.72           | 0.70      | 0.45        | 0.48   |
| 31       | 0.61          | 0.65     | 0.73           | 0.70      | 0.44        | 0.48   |

Continued on next page

| $\alpha$ | $\phi_S^\ell$ | $\phi_S$ | $\varphi^\ell$ | $\varphi$ | $\psi^\ell$ | $\psi$ |
|----------|---------------|----------|----------------|-----------|-------------|--------|
| 32       | 0.61          | 0.65     | 0.73           | 0.70      | 0.44        | 0.48   |
| 33       | 0.61          | 0.64     | 0.73           | 0.71      | 0.44        | 0.47   |
| 34       | 0.61          | 0.64     | 0.74           | 0.71      | 0.44        | 0.47   |
| 35       | 0.60          | 0.64     | 0.74           | 0.71      | 0.43        | 0.47   |
| 36       | 0.60          | 0.63     | 0.74           | 0.72      | 0.43        | 0.46   |
| 37       | 0.60          | 0.63     | 0.75           | 0.72      | 0.43        | 0.46   |
| 38       | 0.60          | 0.63     | 0.75           | 0.73      | 0.43        | 0.45   |
| 39       | 0.59          | 0.62     | 0.76           | 0.73      | 0.42        | 0.45   |
| 40       | 0.59          | 0.62     | 0.76           | 0.73      | 0.42        | 0.45   |
| 41       | 0.58          | 0.61     | 0.76           | 0.74      | 0.41        | 0.44   |
| 42       | 0.58          | 0.61     | 0.77           | 0.74      | 0.41        | 0.44   |
| 43       | 0.58          | 0.61     | 0.77           | 0.75      | 0.41        | 0.43   |
| 44       | 0.57          | 0.60     | 0.78           | 0.75      | 0.40        | 0.43   |
| 45       | 0.57          | 0.60     | 0.78           | 0.76      | 0.40        | 0.43   |
| 46       | 0.56          | 0.59     | 0.79           | 0.76      | 0.39        | 0.42   |
| 47       | 0.56          | 0.59     | 0.79           | 0.77      | 0.39        | 0.42   |
| 48       | 0.55          | 0.58     | 0.80           | 0.77      | 0.38        | 0.41   |
| 49       | 0.55          | 0.57     | 0.80           | 0.78      | 0.38        | 0.40   |
| 50       | 0.54          | 0.57     | 0.80           | 0.78      | 0.38        | 0.40   |
| 51       | 0.54          | 0.56     | 0.81           | 0.79      | 0.37        | 0.39   |
| 52       | 0.53          | 0.56     | 0.81           | 0.79      | 0.37        | 0.39   |
| 53       | 0.53          | 0.55     | 0.82           | 0.79      | 0.37        | 0.39   |
| 54       | 0.52          | 0.54     | 0.82           | 0.80      | 0.36        | 0.38   |
| 55       | 0.51          | 0.54     | 0.83           | 0.80      | 0.35        | 0.38   |
| 56       | 0.51          | 0.53     | 0.83           | 0.81      | 0.35        | 0.37   |
| 57       | 0.50          | 0.52     | 0.84           | 0.81      | 0.34        | 0.36   |
| 58       | 0.49          | 0.52     | 0.84           | 0.82      | 0.34        | 0.36   |
| 59       | 0.48          | 0.51     | 0.85           | 0.83      | 0.33        | 0.35   |
| 60       | 0.48          | 0.50     | 0.85           | 0.83      | 0.33        | 0.35   |
| 61       | 0.47          | 0.49     | 0.86           | 0.84      | 0.32        | 0.34   |
| 62       | 0.46          | 0.48     | 0.86           | 0.84      | 0.31        | 0.33   |
| 63       | 0.45          | 0.48     | 0.87           | 0.85      | 0.30        | 0.33   |

Continued on next page

| $\alpha$ | $\phi_S^\ell$ | $\phi_S$ | $\varphi^\ell$ | $\varphi$ | $\psi^\ell$ | $\psi$ |
|----------|---------------|----------|----------------|-----------|-------------|--------|
| 64       | 0.44          | 0.47     | 0.87           | 0.85      | 0.30        | 0.32   |
| 65       | 0.43          | 0.46     | 0.88           | 0.86      | 0.29        | 0.31   |
| 66       | 0.42          | 0.45     | 0.88           | 0.86      | 0.28        | 0.31   |
| 67       | 0.41          | 0.44     | 0.89           | 0.87      | 0.27        | 0.30   |
| 68       | 0.40          | 0.43     | 0.90           | 0.87      | 0.27        | 0.29   |
| 69       | 0.39          | 0.42     | 0.90           | 0.88      | 0.26        | 0.28   |
| 70       | 0.38          | 0.41     | 0.91           | 0.88      | 0.25        | 0.28   |
| 71       | 0.37          | 0.39     | 0.91           | 0.89      | 0.25        | 0.26   |
| 72       | 0.36          | 0.38     | 0.92           | 0.89      | 0.24        | 0.26   |
| 73       | 0.34          | 0.37     | 0.92           | 0.90      | 0.23        | 0.25   |
| 74       | 0.33          | 0.36     | 0.93           | 0.90      | 0.22        | 0.24   |
| 75       | 0.32          | 0.35     | 0.93           | 0.91      | 0.21        | 0.23   |
| 76       | 0.30          | 0.33     | 0.94           | 0.91      | 0.20        | 0.22   |
| 77       | 0.29          | 0.32     | 0.94           | 0.92      | 0.19        | 0.21   |
| 78       | 0.27          | 0.31     | 0.94           | 0.92      | 0.18        | 0.21   |
| 79       | 0.26          | 0.29     | 0.95           | 0.93      | 0.17        | 0.19   |
| 80       | 0.24          | 0.28     | 0.95           | 0.93      | 0.16        | 0.19   |
| 81       | 0.23          | 0.26     | 0.96           | 0.93      | 0.15        | 0.17   |
| 82       | 0.21          | 0.25     | 0.96           | 0.94      | 0.14        | 0.17   |
| 83       | 0.20          | 0.24     | 0.96           | 0.94      | 0.13        | 0.16   |
| 84       | 0.18          | 0.22     | 0.97           | 0.94      | 0.12        | 0.15   |
| 85       | 0.17          | 0.21     | 0.97           | 0.95      | 0.11        | 0.14   |
| 86       | 0.16          | 0.20     | 0.97           | 0.95      | 0.10        | 0.13   |
| 87       | 0.15          | 0.18     | 0.97           | 0.95      | 0.10        | 0.12   |
| 88       | 0.14          | 0.17     | 0.97           | 0.95      | 0.09        | 0.11   |
| 89       | 0.13          | 0.17     | 0.97           | 0.95      | 0.08        | 0.11   |
| 90       | 0.13          | 0.16     | 0.97           | 0.95      | 0.08        | 0.11   |

Table S165: Reference ( $\phi_S$ ,  $\varphi$ ,  $\psi$ ) and approached ( $\phi_S^\ell$ ,  $\varphi^\ell$ ,  $\psi^\ell$ ) values of the topological descriptors for the first excited-state of the pyridinium-phenolate (PP), computed at the wB97XD/6-31++G(d,p) level of theory.  $\alpha$  is the pyridinium-phenolate central twist angle amplitude.



| $\alpha$ | $\phi_S^\ell$ | $\phi_S$ | $\varphi^\ell$ | $\varphi$ | $\psi^\ell$ | $\psi$ |
|----------|---------------|----------|----------------|-----------|-------------|--------|
| 0        | 0.65          | 0.70     | 0.67           | 0.64      | 0.49        | 0.53   |
| 1        | 0.65          | 0.70     | 0.67           | 0.64      | 0.49        | 0.53   |
| 2        | 0.65          | 0.70     | 0.67           | 0.64      | 0.49        | 0.53   |
| 3        | 0.65          | 0.70     | 0.67           | 0.64      | 0.49        | 0.53   |
| 4        | 0.65          | 0.70     | 0.67           | 0.64      | 0.49        | 0.53   |
| 5        | 0.65          | 0.70     | 0.67           | 0.64      | 0.49        | 0.53   |
| 6        | 0.65          | 0.70     | 0.67           | 0.64      | 0.49        | 0.53   |
| 7        | 0.64          | 0.70     | 0.67           | 0.64      | 0.49        | 0.53   |
| 8        | 0.64          | 0.70     | 0.67           | 0.64      | 0.49        | 0.53   |
| 9        | 0.64          | 0.69     | 0.68           | 0.64      | 0.48        | 0.52   |
| 10       | 0.64          | 0.69     | 0.68           | 0.64      | 0.48        | 0.52   |
| 11       | 0.64          | 0.69     | 0.68           | 0.65      | 0.48        | 0.52   |
| 12       | 0.64          | 0.69     | 0.68           | 0.65      | 0.48        | 0.52   |
| 13       | 0.64          | 0.69     | 0.68           | 0.65      | 0.48        | 0.52   |
| 14       | 0.64          | 0.69     | 0.68           | 0.65      | 0.48        | 0.52   |
| 15       | 0.64          | 0.69     | 0.68           | 0.65      | 0.48        | 0.52   |
| 16       | 0.64          | 0.68     | 0.69           | 0.65      | 0.48        | 0.51   |
| 17       | 0.64          | 0.68     | 0.69           | 0.66      | 0.48        | 0.51   |
| 18       | 0.64          | 0.68     | 0.69           | 0.66      | 0.48        | 0.51   |
| 19       | 0.63          | 0.68     | 0.69           | 0.66      | 0.47        | 0.51   |
| 20       | 0.63          | 0.68     | 0.69           | 0.66      | 0.47        | 0.51   |
| 21       | 0.63          | 0.68     | 0.70           | 0.67      | 0.47        | 0.50   |
| 22       | 0.63          | 0.67     | 0.70           | 0.67      | 0.47        | 0.50   |
| 23       | 0.63          | 0.67     | 0.70           | 0.67      | 0.47        | 0.50   |
| 24       | 0.63          | 0.67     | 0.71           | 0.68      | 0.46        | 0.50   |
| 25       | 0.63          | 0.67     | 0.71           | 0.68      | 0.46        | 0.50   |
| 26       | 0.62          | 0.66     | 0.71           | 0.68      | 0.46        | 0.49   |
| 27       | 0.62          | 0.66     | 0.71           | 0.69      | 0.46        | 0.49   |
| 28       | 0.62          | 0.66     | 0.72           | 0.69      | 0.45        | 0.49   |
| 29       | 0.62          | 0.66     | 0.72           | 0.69      | 0.45        | 0.49   |
| 30       | 0.62          | 0.65     | 0.72           | 0.70      | 0.45        | 0.48   |
| 31       | 0.61          | 0.65     | 0.73           | 0.70      | 0.44        | 0.48   |

Continued on next page

| $\alpha$ | $\phi_S^\ell$ | $\phi_S$ | $\varphi^\ell$ | $\varphi$ | $\psi^\ell$ | $\psi$ |
|----------|---------------|----------|----------------|-----------|-------------|--------|
| 32       | 0.61          | 0.65     | 0.73           | 0.70      | 0.44        | 0.48   |
| 33       | 0.61          | 0.64     | 0.73           | 0.71      | 0.44        | 0.47   |
| 34       | 0.61          | 0.64     | 0.74           | 0.71      | 0.44        | 0.47   |
| 35       | 0.60          | 0.64     | 0.74           | 0.71      | 0.43        | 0.47   |
| 36       | 0.60          | 0.63     | 0.74           | 0.72      | 0.43        | 0.46   |
| 37       | 0.60          | 0.63     | 0.75           | 0.72      | 0.43        | 0.46   |
| 38       | 0.60          | 0.63     | 0.75           | 0.73      | 0.43        | 0.45   |
| 39       | 0.59          | 0.62     | 0.76           | 0.73      | 0.42        | 0.45   |
| 40       | 0.59          | 0.62     | 0.76           | 0.73      | 0.42        | 0.45   |
| 41       | 0.58          | 0.61     | 0.76           | 0.74      | 0.41        | 0.44   |
| 42       | 0.58          | 0.61     | 0.77           | 0.74      | 0.41        | 0.44   |
| 43       | 0.58          | 0.61     | 0.77           | 0.75      | 0.41        | 0.43   |
| 44       | 0.57          | 0.60     | 0.78           | 0.75      | 0.40        | 0.43   |
| 45       | 0.57          | 0.60     | 0.78           | 0.76      | 0.40        | 0.43   |
| 46       | 0.56          | 0.59     | 0.79           | 0.76      | 0.39        | 0.42   |
| 47       | 0.56          | 0.59     | 0.79           | 0.77      | 0.39        | 0.42   |
| 48       | 0.55          | 0.58     | 0.80           | 0.77      | 0.38        | 0.41   |
| 49       | 0.55          | 0.57     | 0.80           | 0.78      | 0.38        | 0.40   |
| 50       | 0.54          | 0.57     | 0.80           | 0.78      | 0.38        | 0.40   |
| 51       | 0.54          | 0.56     | 0.81           | 0.78      | 0.37        | 0.40   |
| 52       | 0.53          | 0.56     | 0.81           | 0.79      | 0.37        | 0.39   |
| 53       | 0.53          | 0.55     | 0.82           | 0.79      | 0.37        | 0.39   |
| 54       | 0.52          | 0.54     | 0.82           | 0.80      | 0.36        | 0.38   |
| 55       | 0.51          | 0.54     | 0.83           | 0.80      | 0.35        | 0.38   |
| 56       | 0.51          | 0.53     | 0.83           | 0.81      | 0.35        | 0.37   |
| 57       | 0.50          | 0.52     | 0.84           | 0.81      | 0.34        | 0.36   |
| 58       | 0.49          | 0.52     | 0.84           | 0.82      | 0.34        | 0.36   |
| 59       | 0.48          | 0.51     | 0.85           | 0.83      | 0.33        | 0.35   |
| 60       | 0.48          | 0.50     | 0.85           | 0.83      | 0.33        | 0.35   |
| 61       | 0.47          | 0.49     | 0.86           | 0.84      | 0.32        | 0.34   |
| 62       | 0.46          | 0.48     | 0.86           | 0.84      | 0.31        | 0.33   |
| 63       | 0.45          | 0.48     | 0.87           | 0.85      | 0.30        | 0.33   |

Continued on next page

| $\alpha$ | $\phi_S^\ell$ | $\phi_S$ | $\varphi^\ell$ | $\varphi$ | $\psi^\ell$ | $\psi$ |
|----------|---------------|----------|----------------|-----------|-------------|--------|
| 64       | 0.44          | 0.47     | 0.87           | 0.85      | 0.30        | 0.32   |
| 65       | 0.43          | 0.46     | 0.88           | 0.86      | 0.29        | 0.31   |
| 66       | 0.42          | 0.45     | 0.88           | 0.86      | 0.28        | 0.31   |
| 67       | 0.41          | 0.44     | 0.89           | 0.87      | 0.27        | 0.30   |
| 68       | 0.40          | 0.43     | 0.90           | 0.87      | 0.27        | 0.29   |
| 69       | 0.39          | 0.42     | 0.90           | 0.88      | 0.26        | 0.28   |
| 70       | 0.38          | 0.41     | 0.91           | 0.88      | 0.25        | 0.28   |
| 71       | 0.37          | 0.39     | 0.91           | 0.89      | 0.25        | 0.26   |
| 72       | 0.36          | 0.38     | 0.92           | 0.89      | 0.24        | 0.26   |
| 73       | 0.34          | 0.37     | 0.92           | 0.90      | 0.23        | 0.25   |
| 74       | 0.33          | 0.36     | 0.93           | 0.90      | 0.22        | 0.24   |
| 75       | 0.32          | 0.35     | 0.93           | 0.91      | 0.21        | 0.23   |
| 76       | 0.30          | 0.33     | 0.94           | 0.91      | 0.20        | 0.22   |
| 77       | 0.29          | 0.32     | 0.94           | 0.92      | 0.19        | 0.21   |
| 78       | 0.27          | 0.31     | 0.94           | 0.92      | 0.18        | 0.21   |
| 79       | 0.26          | 0.29     | 0.95           | 0.93      | 0.17        | 0.19   |
| 80       | 0.24          | 0.28     | 0.95           | 0.93      | 0.16        | 0.19   |
| 81       | 0.23          | 0.26     | 0.96           | 0.93      | 0.15        | 0.17   |
| 82       | 0.21          | 0.25     | 0.96           | 0.94      | 0.14        | 0.17   |
| 83       | 0.20          | 0.24     | 0.96           | 0.94      | 0.13        | 0.16   |
| 84       | 0.19          | 0.22     | 0.97           | 0.94      | 0.12        | 0.15   |
| 85       | 0.17          | 0.21     | 0.97           | 0.95      | 0.11        | 0.14   |
| 86       | 0.16          | 0.20     | 0.97           | 0.95      | 0.10        | 0.13   |
| 87       | 0.15          | 0.18     | 0.97           | 0.95      | 0.10        | 0.12   |
| 88       | 0.14          | 0.17     | 0.97           | 0.95      | 0.09        | 0.11   |
| 89       | 0.13          | 0.17     | 0.97           | 0.95      | 0.08        | 0.11   |
| 90       | 0.13          | 0.16     | 0.97           | 0.95      | 0.08        | 0.11   |

Table S166: Reference ( $\phi_S$ ,  $\varphi$ ,  $\psi$ ) and approached ( $\phi_S^\ell$ ,  $\varphi^\ell$ ,  $\psi^\ell$ ) values of the topological descriptors for the first excited-state of the pyridinium-phenolate (PP), computed at the wB97XD/6-31+G(d,p) level of theory.  $\alpha$  is the pyridinium-phenolate central twist angle amplitude.

| $\alpha$ | $\phi_S^\ell$ | $\phi_S$ | $\varphi^\ell$ | $\varphi$ | $\psi^\ell$ | $\psi$ |
|----------|---------------|----------|----------------|-----------|-------------|--------|
| 0        | 0.65          | 0.70     | 0.67           | 0.64      | 0.49        | 0.53   |
| 1        | 0.65          | 0.70     | 0.67           | 0.64      | 0.49        | 0.53   |
| 2        | 0.65          | 0.70     | 0.67           | 0.64      | 0.49        | 0.53   |
| 3        | 0.65          | 0.70     | 0.67           | 0.64      | 0.49        | 0.53   |
| 4        | 0.65          | 0.70     | 0.67           | 0.64      | 0.49        | 0.53   |
| 5        | 0.65          | 0.70     | 0.67           | 0.64      | 0.49        | 0.53   |
| 6        | 0.65          | 0.70     | 0.67           | 0.64      | 0.49        | 0.53   |
| 7        | 0.64          | 0.70     | 0.67           | 0.64      | 0.49        | 0.53   |
| 8        | 0.64          | 0.69     | 0.68           | 0.64      | 0.48        | 0.52   |
| 9        | 0.64          | 0.69     | 0.68           | 0.64      | 0.48        | 0.52   |
| 10       | 0.64          | 0.69     | 0.68           | 0.64      | 0.48        | 0.52   |
| 11       | 0.64          | 0.69     | 0.68           | 0.65      | 0.48        | 0.52   |
| 12       | 0.64          | 0.69     | 0.68           | 0.65      | 0.48        | 0.52   |
| 13       | 0.64          | 0.69     | 0.68           | 0.65      | 0.48        | 0.52   |
| 14       | 0.64          | 0.69     | 0.68           | 0.65      | 0.48        | 0.52   |
| 15       | 0.64          | 0.69     | 0.68           | 0.65      | 0.48        | 0.52   |
| 16       | 0.64          | 0.68     | 0.69           | 0.66      | 0.48        | 0.51   |
| 17       | 0.64          | 0.68     | 0.69           | 0.66      | 0.48        | 0.51   |
| 18       | 0.64          | 0.68     | 0.69           | 0.66      | 0.48        | 0.51   |
| 19       | 0.63          | 0.68     | 0.69           | 0.66      | 0.47        | 0.51   |
| 20       | 0.63          | 0.68     | 0.70           | 0.67      | 0.47        | 0.50   |
| 21       | 0.63          | 0.68     | 0.70           | 0.67      | 0.47        | 0.50   |
| 22       | 0.63          | 0.67     | 0.70           | 0.67      | 0.47        | 0.50   |
| 23       | 0.63          | 0.67     | 0.70           | 0.67      | 0.47        | 0.50   |
| 24       | 0.63          | 0.67     | 0.71           | 0.68      | 0.46        | 0.50   |
| 25       | 0.63          | 0.67     | 0.71           | 0.68      | 0.46        | 0.50   |
| 26       | 0.62          | 0.66     | 0.71           | 0.68      | 0.46        | 0.49   |
| 27       | 0.62          | 0.66     | 0.71           | 0.69      | 0.46        | 0.49   |
| 28       | 0.62          | 0.66     | 0.72           | 0.69      | 0.45        | 0.49   |
| 29       | 0.62          | 0.66     | 0.72           | 0.69      | 0.45        | 0.49   |
| 30       | 0.62          | 0.65     | 0.72           | 0.70      | 0.45        | 0.48   |
| 31       | 0.61          | 0.65     | 0.73           | 0.70      | 0.44        | 0.48   |

Continued on next page

| $\alpha$ | $\phi_S^\ell$ | $\phi_S$ | $\varphi^\ell$ | $\varphi$ | $\psi^\ell$ | $\psi$ |
|----------|---------------|----------|----------------|-----------|-------------|--------|
| 32       | 0.61          | 0.65     | 0.73           | 0.70      | 0.44        | 0.48   |
| 33       | 0.61          | 0.64     | 0.73           | 0.71      | 0.44        | 0.47   |
| 34       | 0.61          | 0.64     | 0.74           | 0.71      | 0.44        | 0.47   |
| 35       | 0.60          | 0.64     | 0.74           | 0.71      | 0.43        | 0.47   |
| 36       | 0.60          | 0.63     | 0.74           | 0.72      | 0.43        | 0.46   |
| 37       | 0.60          | 0.63     | 0.75           | 0.72      | 0.43        | 0.46   |
| 38       | 0.59          | 0.63     | 0.75           | 0.73      | 0.42        | 0.45   |
| 39       | 0.59          | 0.62     | 0.76           | 0.73      | 0.42        | 0.45   |
| 40       | 0.59          | 0.62     | 0.76           | 0.74      | 0.42        | 0.44   |
| 41       | 0.58          | 0.61     | 0.77           | 0.74      | 0.41        | 0.44   |
| 42       | 0.58          | 0.61     | 0.77           | 0.74      | 0.41        | 0.44   |
| 43       | 0.58          | 0.60     | 0.77           | 0.75      | 0.41        | 0.43   |
| 44       | 0.57          | 0.60     | 0.78           | 0.75      | 0.40        | 0.43   |
| 45       | 0.57          | 0.59     | 0.78           | 0.76      | 0.40        | 0.42   |
| 46       | 0.56          | 0.59     | 0.79           | 0.76      | 0.39        | 0.42   |
| 47       | 0.56          | 0.58     | 0.79           | 0.77      | 0.39        | 0.41   |
| 48       | 0.55          | 0.58     | 0.80           | 0.77      | 0.38        | 0.41   |
| 49       | 0.55          | 0.57     | 0.80           | 0.78      | 0.38        | 0.40   |
| 50       | 0.54          | 0.57     | 0.81           | 0.78      | 0.37        | 0.40   |
| 51       | 0.54          | 0.56     | 0.81           | 0.79      | 0.37        | 0.39   |
| 52       | 0.53          | 0.56     | 0.81           | 0.79      | 0.37        | 0.39   |
| 53       | 0.52          | 0.55     | 0.82           | 0.80      | 0.36        | 0.38   |
| 54       | 0.52          | 0.54     | 0.82           | 0.80      | 0.36        | 0.38   |
| 55       | 0.51          | 0.54     | 0.83           | 0.81      | 0.35        | 0.37   |
| 56       | 0.51          | 0.53     | 0.83           | 0.81      | 0.35        | 0.37   |
| 57       | 0.50          | 0.52     | 0.84           | 0.82      | 0.34        | 0.36   |
| 58       | 0.49          | 0.52     | 0.84           | 0.82      | 0.34        | 0.36   |
| 59       | 0.48          | 0.51     | 0.85           | 0.83      | 0.33        | 0.35   |
| 60       | 0.48          | 0.50     | 0.85           | 0.83      | 0.33        | 0.35   |
| 61       | 0.47          | 0.49     | 0.86           | 0.84      | 0.32        | 0.34   |
| 62       | 0.46          | 0.48     | 0.86           | 0.84      | 0.31        | 0.33   |
| 63       | 0.45          | 0.47     | 0.87           | 0.85      | 0.30        | 0.32   |

Continued on next page

| $\alpha$ | $\phi_S^\ell$ | $\phi_S$ | $\varphi^\ell$ | $\varphi$ | $\psi^\ell$ | $\psi$ |
|----------|---------------|----------|----------------|-----------|-------------|--------|
| 64       | 0.44          | 0.47     | 0.87           | 0.85      | 0.30        | 0.32   |
| 65       | 0.43          | 0.46     | 0.88           | 0.86      | 0.29        | 0.31   |
| 66       | 0.42          | 0.45     | 0.88           | 0.86      | 0.28        | 0.31   |
| 67       | 0.41          | 0.44     | 0.89           | 0.87      | 0.27        | 0.30   |
| 68       | 0.40          | 0.43     | 0.90           | 0.87      | 0.27        | 0.29   |
| 69       | 0.39          | 0.42     | 0.90           | 0.88      | 0.26        | 0.28   |
| 70       | 0.38          | 0.41     | 0.91           | 0.88      | 0.25        | 0.28   |
| 71       | 0.37          | 0.39     | 0.91           | 0.89      | 0.25        | 0.26   |
| 72       | 0.36          | 0.38     | 0.92           | 0.89      | 0.24        | 0.26   |
| 73       | 0.34          | 0.37     | 0.92           | 0.90      | 0.23        | 0.25   |
| 74       | 0.33          | 0.36     | 0.93           | 0.90      | 0.22        | 0.24   |
| 75       | 0.32          | 0.35     | 0.93           | 0.91      | 0.21        | 0.23   |
| 76       | 0.30          | 0.33     | 0.94           | 0.91      | 0.20        | 0.22   |
| 77       | 0.29          | 0.32     | 0.94           | 0.92      | 0.19        | 0.21   |
| 78       | 0.27          | 0.31     | 0.94           | 0.92      | 0.18        | 0.21   |
| 79       | 0.26          | 0.29     | 0.95           | 0.93      | 0.17        | 0.19   |
| 80       | 0.24          | 0.28     | 0.95           | 0.93      | 0.16        | 0.19   |
| 81       | 0.23          | 0.26     | 0.96           | 0.93      | 0.15        | 0.17   |
| 82       | 0.21          | 0.25     | 0.96           | 0.94      | 0.14        | 0.17   |
| 83       | 0.20          | 0.23     | 0.96           | 0.94      | 0.13        | 0.15   |
| 84       | 0.18          | 0.22     | 0.97           | 0.95      | 0.12        | 0.14   |
| 85       | 0.17          | 0.21     | 0.97           | 0.95      | 0.11        | 0.14   |
| 86       | 0.16          | 0.19     | 0.97           | 0.95      | 0.10        | 0.13   |
| 87       | 0.15          | 0.18     | 0.97           | 0.95      | 0.10        | 0.12   |
| 88       | 0.14          | 0.17     | 0.97           | 0.95      | 0.09        | 0.11   |
| 89       | 0.13          | 0.17     | 0.97           | 0.95      | 0.08        | 0.11   |
| 90       | 0.13          | 0.16     | 0.97           | 0.95      | 0.08        | 0.11   |

Table S167: Reference ( $\phi_S$ ,  $\varphi$ ,  $\psi$ ) and approached ( $\phi_S^\ell$ ,  $\varphi^\ell$ ,  $\psi^\ell$ ) values of the topological descriptors for the first excited-state of the pyridinium-phenolate (PP), computed at the wB97XD/6-31+G(d) level of theory.  $\alpha$  is the pyridinium-phenolate central twist angle amplitude.

| $\alpha$ | $\phi_S^\ell$ | $\phi_S$ | $\varphi^\ell$ | $\varphi$ | $\psi^\ell$ | $\psi$ |
|----------|---------------|----------|----------------|-----------|-------------|--------|
| 0        | 0.68          | 0.72     | 0.66           | 0.62      | 0.51        | 0.55   |
| 1        | 0.68          | 0.72     | 0.66           | 0.62      | 0.51        | 0.55   |
| 2        | 0.68          | 0.72     | 0.66           | 0.62      | 0.51        | 0.55   |
| 3        | 0.68          | 0.72     | 0.66           | 0.62      | 0.51        | 0.55   |
| 4        | 0.67          | 0.72     | 0.66           | 0.62      | 0.50        | 0.55   |
| 5        | 0.67          | 0.72     | 0.66           | 0.62      | 0.50        | 0.55   |
| 6        | 0.67          | 0.72     | 0.66           | 0.62      | 0.50        | 0.55   |
| 7        | 0.67          | 0.72     | 0.66           | 0.62      | 0.50        | 0.55   |
| 8        | 0.67          | 0.71     | 0.66           | 0.63      | 0.50        | 0.54   |
| 9        | 0.67          | 0.71     | 0.67           | 0.63      | 0.50        | 0.54   |
| 10       | 0.67          | 0.71     | 0.67           | 0.63      | 0.50        | 0.54   |
| 11       | 0.67          | 0.71     | 0.67           | 0.63      | 0.50        | 0.54   |
| 12       | 0.67          | 0.71     | 0.67           | 0.63      | 0.50        | 0.54   |
| 13       | 0.67          | 0.71     | 0.67           | 0.63      | 0.50        | 0.54   |
| 14       | 0.67          | 0.71     | 0.67           | 0.64      | 0.50        | 0.53   |
| 15       | 0.67          | 0.71     | 0.67           | 0.64      | 0.50        | 0.53   |
| 16       | 0.67          | 0.70     | 0.68           | 0.64      | 0.50        | 0.53   |
| 17       | 0.66          | 0.70     | 0.68           | 0.64      | 0.49        | 0.53   |
| 18       | 0.66          | 0.70     | 0.68           | 0.64      | 0.49        | 0.53   |
| 19       | 0.66          | 0.70     | 0.68           | 0.65      | 0.49        | 0.52   |
| 20       | 0.66          | 0.70     | 0.68           | 0.65      | 0.49        | 0.52   |
| 21       | 0.66          | 0.70     | 0.69           | 0.65      | 0.49        | 0.52   |
| 22       | 0.66          | 0.69     | 0.69           | 0.65      | 0.49        | 0.52   |
| 23       | 0.66          | 0.69     | 0.69           | 0.66      | 0.49        | 0.51   |
| 24       | 0.65          | 0.69     | 0.69           | 0.66      | 0.48        | 0.51   |
| 25       | 0.65          | 0.69     | 0.70           | 0.66      | 0.48        | 0.51   |
| 26       | 0.65          | 0.68     | 0.70           | 0.67      | 0.48        | 0.50   |
| 27       | 0.65          | 0.68     | 0.70           | 0.67      | 0.48        | 0.50   |
| 28       | 0.65          | 0.68     | 0.70           | 0.67      | 0.48        | 0.50   |
| 29       | 0.64          | 0.68     | 0.71           | 0.68      | 0.47        | 0.50   |
| 30       | 0.64          | 0.67     | 0.71           | 0.68      | 0.47        | 0.50   |
| 31       | 0.64          | 0.67     | 0.71           | 0.68      | 0.47        | 0.50   |

Continued on next page

| $\alpha$ | $\phi_S^\ell$ | $\phi_S$ | $\varphi^\ell$ | $\varphi$ | $\psi^\ell$ | $\psi$ |
|----------|---------------|----------|----------------|-----------|-------------|--------|
| 32       | 0.64          | 0.67     | 0.72           | 0.69      | 0.46        | 0.49   |
| 33       | 0.64          | 0.67     | 0.72           | 0.69      | 0.46        | 0.49   |
| 34       | 0.63          | 0.66     | 0.72           | 0.70      | 0.46        | 0.48   |
| 35       | 0.63          | 0.66     | 0.73           | 0.70      | 0.45        | 0.48   |
| 36       | 0.63          | 0.66     | 0.73           | 0.70      | 0.45        | 0.48   |
| 37       | 0.63          | 0.65     | 0.73           | 0.71      | 0.45        | 0.47   |
| 38       | 0.62          | 0.65     | 0.74           | 0.71      | 0.44        | 0.47   |
| 39       | 0.62          | 0.64     | 0.74           | 0.72      | 0.44        | 0.46   |
| 40       | 0.62          | 0.64     | 0.75           | 0.72      | 0.44        | 0.46   |
| 41       | 0.61          | 0.64     | 0.75           | 0.72      | 0.43        | 0.46   |
| 42       | 0.61          | 0.63     | 0.76           | 0.73      | 0.43        | 0.45   |
| 43       | 0.60          | 0.63     | 0.76           | 0.73      | 0.43        | 0.45   |
| 44       | 0.60          | 0.62     | 0.76           | 0.74      | 0.43        | 0.44   |
| 45       | 0.60          | 0.62     | 0.77           | 0.74      | 0.42        | 0.44   |
| 46       | 0.59          | 0.61     | 0.77           | 0.75      | 0.42        | 0.43   |
| 47       | 0.59          | 0.61     | 0.78           | 0.75      | 0.41        | 0.43   |
| 48       | 0.58          | 0.60     | 0.78           | 0.76      | 0.41        | 0.43   |
| 49       | 0.58          | 0.60     | 0.79           | 0.76      | 0.40        | 0.43   |
| 50       | 0.57          | 0.59     | 0.79           | 0.76      | 0.40        | 0.42   |
| 51       | 0.57          | 0.59     | 0.80           | 0.77      | 0.39        | 0.42   |
| 52       | 0.56          | 0.58     | 0.80           | 0.77      | 0.39        | 0.41   |
| 53       | 0.56          | 0.58     | 0.80           | 0.78      | 0.39        | 0.41   |
| 54       | 0.55          | 0.57     | 0.81           | 0.78      | 0.38        | 0.40   |
| 55       | 0.54          | 0.56     | 0.81           | 0.79      | 0.37        | 0.39   |
| 56       | 0.54          | 0.56     | 0.82           | 0.79      | 0.37        | 0.39   |
| 57       | 0.53          | 0.55     | 0.82           | 0.80      | 0.37        | 0.38   |
| 58       | 0.52          | 0.54     | 0.83           | 0.81      | 0.36        | 0.37   |
| 59       | 0.52          | 0.54     | 0.83           | 0.81      | 0.36        | 0.37   |
| 60       | 0.51          | 0.53     | 0.84           | 0.82      | 0.35        | 0.37   |
| 61       | 0.50          | 0.52     | 0.84           | 0.82      | 0.34        | 0.36   |
| 62       | 0.49          | 0.51     | 0.85           | 0.83      | 0.33        | 0.35   |
| 63       | 0.48          | 0.50     | 0.85           | 0.83      | 0.33        | 0.35   |

Continued on next page



| $\alpha$ | $\phi_S^\ell$ | $\phi_S$ | $\varphi^\ell$ | $\varphi$ | $\psi^\ell$ | $\psi$ |
|----------|---------------|----------|----------------|-----------|-------------|--------|
| 64       | 0.48          | 0.49     | 0.86           | 0.84      | 0.32        | 0.34   |
| 65       | 0.47          | 0.49     | 0.86           | 0.84      | 0.32        | 0.34   |
| 66       | 0.46          | 0.48     | 0.87           | 0.85      | 0.31        | 0.33   |
| 67       | 0.45          | 0.47     | 0.88           | 0.85      | 0.30        | 0.32   |
| 68       | 0.44          | 0.46     | 0.88           | 0.86      | 0.30        | 0.31   |
| 69       | 0.43          | 0.45     | 0.89           | 0.86      | 0.29        | 0.31   |
| 70       | 0.41          | 0.44     | 0.89           | 0.87      | 0.27        | 0.30   |
| 71       | 0.40          | 0.42     | 0.90           | 0.88      | 0.27        | 0.28   |
| 72       | 0.39          | 0.41     | 0.91           | 0.88      | 0.26        | 0.28   |
| 73       | 0.38          | 0.40     | 0.91           | 0.89      | 0.25        | 0.27   |
| 74       | 0.36          | 0.39     | 0.92           | 0.89      | 0.24        | 0.26   |
| 75       | 0.35          | 0.37     | 0.92           | 0.90      | 0.23        | 0.25   |
| 76       | 0.33          | 0.36     | 0.93           | 0.90      | 0.22        | 0.24   |
| 77       | 0.32          | 0.35     | 0.93           | 0.91      | 0.21        | 0.23   |
| 78       | 0.30          | 0.33     | 0.94           | 0.91      | 0.20        | 0.22   |
| 79       | 0.29          | 0.32     | 0.94           | 0.92      | 0.19        | 0.21   |
| 80       | 0.27          | 0.30     | 0.95           | 0.92      | 0.18        | 0.20   |
| 81       | 0.25          | 0.29     | 0.95           | 0.93      | 0.16        | 0.19   |
| 82       | 0.23          | 0.27     | 0.96           | 0.93      | 0.15        | 0.18   |
| 83       | 0.21          | 0.25     | 0.96           | 0.94      | 0.14        | 0.17   |
| 84       | 0.19          | 0.24     | 0.97           | 0.94      | 0.12        | 0.16   |
| 85       | 0.17          | 0.22     | 0.97           | 0.95      | 0.11        | 0.14   |
| 86       | 0.16          | 0.20     | 0.97           | 0.95      | 0.10        | 0.13   |
| 87       | 0.14          | 0.19     | 0.98           | 0.95      | 0.09        | 0.13   |
| 88       | 0.13          | 0.18     | 0.98           | 0.95      | 0.08        | 0.12   |
| 89       | 0.12          | 0.17     | 0.98           | 0.95      | 0.08        | 0.11   |
| 90       | 0.11          | 0.16     | 0.98           | 0.96      | 0.07        | 0.11   |

Table S168: Reference ( $\phi_S$ ,  $\varphi$ ,  $\psi$ ) and approached ( $\phi_S^\ell$ ,  $\varphi^\ell$ ,  $\psi^\ell$ ) values of the topological descriptors for the first excited-state of the pyridinium-phenolate (PP), computed at the wB97XD/6-31G(d) level of theory.  $\alpha$  is the pyridinium-phenolate central twist angle amplitude.

| $\alpha$ | $\phi_S^\ell$ | $\phi_S$ | $\varphi^\ell$ | $\varphi$ | $\psi^\ell$ | $\psi$ |
|----------|---------------|----------|----------------|-----------|-------------|--------|
| 0        | 0.65          | 0.69     | 0.67           | 0.64      | 0.49        | 0.52   |
| 1        | 0.65          | 0.69     | 0.67           | 0.64      | 0.49        | 0.52   |
| 2        | 0.65          | 0.69     | 0.67           | 0.64      | 0.49        | 0.52   |
| 3        | 0.65          | 0.69     | 0.67           | 0.64      | 0.49        | 0.52   |
| 4        | 0.65          | 0.69     | 0.67           | 0.64      | 0.49        | 0.52   |
| 5        | 0.65          | 0.69     | 0.67           | 0.64      | 0.49        | 0.52   |
| 6        | 0.65          | 0.69     | 0.67           | 0.64      | 0.49        | 0.52   |
| 7        | 0.65          | 0.69     | 0.67           | 0.64      | 0.49        | 0.52   |
| 8        | 0.65          | 0.69     | 0.67           | 0.65      | 0.49        | 0.52   |
| 9        | 0.65          | 0.69     | 0.67           | 0.65      | 0.49        | 0.52   |
| 10       | 0.64          | 0.69     | 0.68           | 0.65      | 0.48        | 0.52   |
| 11       | 0.64          | 0.69     | 0.68           | 0.65      | 0.48        | 0.52   |
| 12       | 0.64          | 0.69     | 0.68           | 0.65      | 0.48        | 0.52   |
| 13       | 0.64          | 0.68     | 0.68           | 0.65      | 0.48        | 0.51   |
| 14       | 0.64          | 0.68     | 0.68           | 0.66      | 0.48        | 0.51   |
| 15       | 0.64          | 0.68     | 0.68           | 0.66      | 0.48        | 0.51   |
| 16       | 0.64          | 0.68     | 0.69           | 0.66      | 0.48        | 0.51   |
| 17       | 0.64          | 0.68     | 0.69           | 0.66      | 0.48        | 0.51   |
| 18       | 0.64          | 0.68     | 0.69           | 0.66      | 0.48        | 0.51   |
| 19       | 0.64          | 0.67     | 0.69           | 0.67      | 0.48        | 0.50   |
| 20       | 0.63          | 0.67     | 0.69           | 0.67      | 0.47        | 0.50   |
| 21       | 0.63          | 0.67     | 0.70           | 0.67      | 0.47        | 0.50   |
| 22       | 0.63          | 0.67     | 0.70           | 0.67      | 0.47        | 0.50   |
| 23       | 0.63          | 0.67     | 0.70           | 0.68      | 0.47        | 0.50   |
| 24       | 0.63          | 0.66     | 0.70           | 0.68      | 0.47        | 0.49   |
| 25       | 0.63          | 0.66     | 0.71           | 0.68      | 0.46        | 0.49   |
| 26       | 0.63          | 0.66     | 0.71           | 0.69      | 0.46        | 0.49   |
| 27       | 0.62          | 0.66     | 0.71           | 0.69      | 0.46        | 0.49   |
| 28       | 0.62          | 0.66     | 0.72           | 0.69      | 0.45        | 0.49   |
| 29       | 0.62          | 0.65     | 0.72           | 0.70      | 0.45        | 0.48   |
| 30       | 0.62          | 0.65     | 0.72           | 0.70      | 0.45        | 0.48   |
| 31       | 0.62          | 0.65     | 0.73           | 0.70      | 0.45        | 0.48   |

Continued on next page

| $\alpha$ | $\phi_S^\ell$ | $\phi_S$ | $\varphi^\ell$ | $\varphi$ | $\psi^\ell$ | $\psi$ |
|----------|---------------|----------|----------------|-----------|-------------|--------|
| 32       | 0.61          | 0.64     | 0.73           | 0.71      | 0.44        | 0.47   |
| 33       | 0.61          | 0.64     | 0.73           | 0.71      | 0.44        | 0.47   |
| 34       | 0.61          | 0.64     | 0.74           | 0.71      | 0.44        | 0.47   |
| 35       | 0.61          | 0.63     | 0.74           | 0.72      | 0.44        | 0.46   |
| 36       | 0.60          | 0.63     | 0.74           | 0.72      | 0.43        | 0.46   |
| 37       | 0.60          | 0.63     | 0.75           | 0.73      | 0.43        | 0.45   |
| 38       | 0.60          | 0.62     | 0.75           | 0.73      | 0.43        | 0.45   |
| 39       | 0.59          | 0.62     | 0.75           | 0.73      | 0.42        | 0.45   |
| 40       | 0.59          | 0.62     | 0.76           | 0.74      | 0.42        | 0.44   |
| 41       | 0.59          | 0.61     | 0.76           | 0.74      | 0.42        | 0.44   |
| 42       | 0.58          | 0.61     | 0.77           | 0.75      | 0.41        | 0.43   |
| 43       | 0.58          | 0.60     | 0.77           | 0.75      | 0.41        | 0.43   |
| 44       | 0.57          | 0.60     | 0.78           | 0.76      | 0.40        | 0.43   |
| 45       | 0.57          | 0.59     | 0.78           | 0.76      | 0.40        | 0.42   |
| 46       | 0.56          | 0.59     | 0.79           | 0.76      | 0.39        | 0.42   |
| 47       | 0.56          | 0.58     | 0.79           | 0.77      | 0.39        | 0.41   |
| 48       | 0.55          | 0.58     | 0.80           | 0.77      | 0.38        | 0.41   |
| 49       | 0.55          | 0.57     | 0.80           | 0.78      | 0.38        | 0.40   |
| 50       | 0.54          | 0.57     | 0.80           | 0.78      | 0.38        | 0.40   |
| 51       | 0.54          | 0.56     | 0.81           | 0.79      | 0.37        | 0.39   |
| 52       | 0.53          | 0.56     | 0.81           | 0.79      | 0.37        | 0.39   |
| 53       | 0.53          | 0.55     | 0.82           | 0.80      | 0.37        | 0.38   |
| 54       | 0.52          | 0.54     | 0.82           | 0.80      | 0.36        | 0.38   |
| 55       | 0.51          | 0.54     | 0.83           | 0.81      | 0.35        | 0.37   |
| 56       | 0.51          | 0.53     | 0.83           | 0.81      | 0.35        | 0.37   |
| 57       | 0.50          | 0.52     | 0.84           | 0.82      | 0.34        | 0.36   |
| 58       | 0.49          | 0.52     | 0.84           | 0.82      | 0.34        | 0.36   |
| 59       | 0.48          | 0.51     | 0.85           | 0.83      | 0.33        | 0.35   |
| 60       | 0.48          | 0.50     | 0.85           | 0.83      | 0.33        | 0.35   |
| 61       | 0.47          | 0.49     | 0.86           | 0.84      | 0.32        | 0.34   |
| 62       | 0.46          | 0.48     | 0.86           | 0.84      | 0.31        | 0.33   |
| 63       | 0.45          | 0.48     | 0.87           | 0.85      | 0.30        | 0.33   |

Continued on next page

| $\alpha$ | $\phi_S^\ell$ | $\phi_S$ | $\varphi^\ell$ | $\varphi$ | $\psi^\ell$ | $\psi$ |
|----------|---------------|----------|----------------|-----------|-------------|--------|
| 64       | 0.44          | 0.47     | 0.88           | 0.85      | 0.30        | 0.32   |
| 65       | 0.43          | 0.46     | 0.88           | 0.86      | 0.29        | 0.31   |
| 66       | 0.42          | 0.45     | 0.89           | 0.86      | 0.28        | 0.31   |
| 67       | 0.41          | 0.44     | 0.89           | 0.87      | 0.27        | 0.30   |
| 68       | 0.40          | 0.43     | 0.90           | 0.87      | 0.27        | 0.29   |
| 69       | 0.39          | 0.42     | 0.90           | 0.88      | 0.26        | 0.28   |
| 70       | 0.38          | 0.41     | 0.91           | 0.88      | 0.25        | 0.28   |
| 71       | 0.36          | 0.40     | 0.92           | 0.89      | 0.24        | 0.27   |
| 72       | 0.35          | 0.38     | 0.92           | 0.90      | 0.23        | 0.25   |
| 73       | 0.34          | 0.37     | 0.93           | 0.90      | 0.22        | 0.25   |
| 74       | 0.33          | 0.36     | 0.93           | 0.91      | 0.22        | 0.24   |
| 75       | 0.31          | 0.35     | 0.94           | 0.91      | 0.20        | 0.23   |
| 76       | 0.30          | 0.33     | 0.94           | 0.92      | 0.20        | 0.22   |
| 77       | 0.28          | 0.32     | 0.95           | 0.92      | 0.18        | 0.21   |
| 78       | 0.27          | 0.31     | 0.95           | 0.93      | 0.18        | 0.20   |
| 79       | 0.25          | 0.29     | 0.96           | 0.93      | 0.16        | 0.19   |
| 80       | 0.24          | 0.28     | 0.96           | 0.93      | 0.16        | 0.19   |
| 81       | 0.22          | 0.26     | 0.97           | 0.94      | 0.14        | 0.17   |
| 82       | 0.20          | 0.25     | 0.97           | 0.94      | 0.13        | 0.17   |
| 83       | 0.19          | 0.23     | 0.97           | 0.95      | 0.12        | 0.15   |
| 84       | 0.17          | 0.22     | 0.98           | 0.95      | 0.11        | 0.14   |
| 85       | 0.16          | 0.20     | 0.98           | 0.95      | 0.10        | 0.13   |
| 86       | 0.15          | 0.19     | 0.98           | 0.95      | 0.10        | 0.13   |
| 87       | 0.13          | 0.18     | 0.98           | 0.96      | 0.08        | 0.12   |
| 88       | 0.12          | 0.16     | 0.98           | 0.96      | 0.08        | 0.11   |
| 89       | 0.11          | 0.16     | 0.98           | 0.96      | 0.07        | 0.11   |
| 90       | 0.11          | 0.15     | 0.99           | 0.96      | 0.07        | 0.10   |

Table S169: Reference ( $\phi_S$ ,  $\varphi$ ,  $\psi$ ) and approached ( $\phi_S^\ell$ ,  $\varphi^\ell$ ,  $\psi^\ell$ ) values of the topological descriptors for the first excited-state of the pyridinium-phenolate (PP), computed at the wB97XD/6-31+G level of theory.  $\alpha$  is the pyridinium-phenolate central twist angle amplitude.

| $\alpha$ | $\phi_S^\ell$ | $\phi_S$ | $\varphi^\ell$ | $\varphi$ | $\psi^\ell$ | $\psi$ |
|----------|---------------|----------|----------------|-----------|-------------|--------|
| 0        | 0.68          | 0.71     | 0.66           | 0.63      | 0.51        | 0.54   |
| 1        | 0.68          | 0.71     | 0.66           | 0.63      | 0.51        | 0.54   |
| 2        | 0.68          | 0.71     | 0.66           | 0.63      | 0.51        | 0.54   |
| 3        | 0.68          | 0.71     | 0.66           | 0.63      | 0.51        | 0.54   |
| 4        | 0.68          | 0.71     | 0.66           | 0.63      | 0.51        | 0.54   |
| 5        | 0.68          | 0.71     | 0.66           | 0.63      | 0.51        | 0.54   |
| 6        | 0.68          | 0.71     | 0.66           | 0.63      | 0.51        | 0.54   |
| 7        | 0.68          | 0.71     | 0.66           | 0.63      | 0.51        | 0.54   |
| 8        | 0.68          | 0.71     | 0.66           | 0.63      | 0.51        | 0.54   |
| 9        | 0.67          | 0.71     | 0.66           | 0.63      | 0.50        | 0.54   |
| 10       | 0.67          | 0.71     | 0.66           | 0.63      | 0.50        | 0.54   |
| 11       | 0.67          | 0.71     | 0.67           | 0.63      | 0.50        | 0.54   |
| 12       | 0.67          | 0.71     | 0.67           | 0.64      | 0.50        | 0.53   |
| 13       | 0.67          | 0.70     | 0.67           | 0.64      | 0.50        | 0.53   |
| 14       | 0.67          | 0.70     | 0.67           | 0.64      | 0.50        | 0.53   |
| 15       | 0.67          | 0.70     | 0.67           | 0.64      | 0.50        | 0.53   |
| 16       | 0.67          | 0.70     | 0.67           | 0.64      | 0.50        | 0.53   |
| 17       | 0.67          | 0.70     | 0.68           | 0.65      | 0.50        | 0.52   |
| 18       | 0.66          | 0.70     | 0.68           | 0.65      | 0.49        | 0.52   |
| 19       | 0.66          | 0.70     | 0.68           | 0.65      | 0.49        | 0.52   |
| 20       | 0.66          | 0.69     | 0.68           | 0.65      | 0.49        | 0.52   |
| 21       | 0.66          | 0.69     | 0.68           | 0.66      | 0.49        | 0.51   |
| 22       | 0.66          | 0.69     | 0.69           | 0.66      | 0.49        | 0.51   |
| 23       | 0.66          | 0.69     | 0.69           | 0.66      | 0.49        | 0.51   |
| 24       | 0.66          | 0.69     | 0.69           | 0.66      | 0.49        | 0.51   |
| 25       | 0.65          | 0.68     | 0.69           | 0.67      | 0.48        | 0.50   |
| 26       | 0.65          | 0.68     | 0.70           | 0.67      | 0.48        | 0.50   |
| 27       | 0.65          | 0.68     | 0.70           | 0.67      | 0.48        | 0.50   |
| 28       | 0.65          | 0.68     | 0.70           | 0.68      | 0.48        | 0.50   |
| 29       | 0.65          | 0.67     | 0.71           | 0.68      | 0.47        | 0.50   |
| 30       | 0.65          | 0.67     | 0.71           | 0.68      | 0.47        | 0.50   |
| 31       | 0.64          | 0.67     | 0.71           | 0.69      | 0.47        | 0.49   |

Continued on next page

| $\alpha$ | $\phi_S^\ell$ | $\phi_S$ | $\varphi^\ell$ | $\varphi$ | $\psi^\ell$ | $\psi$ |
|----------|---------------|----------|----------------|-----------|-------------|--------|
| 32       | 0.64          | 0.67     | 0.72           | 0.69      | 0.46        | 0.49   |
| 33       | 0.64          | 0.66     | 0.72           | 0.69      | 0.46        | 0.49   |
| 34       | 0.64          | 0.66     | 0.72           | 0.70      | 0.46        | 0.48   |
| 35       | 0.63          | 0.66     | 0.73           | 0.70      | 0.45        | 0.48   |
| 36       | 0.63          | 0.65     | 0.73           | 0.71      | 0.45        | 0.47   |
| 37       | 0.63          | 0.65     | 0.73           | 0.71      | 0.45        | 0.47   |
| 38       | 0.63          | 0.65     | 0.74           | 0.71      | 0.45        | 0.47   |
| 39       | 0.62          | 0.64     | 0.74           | 0.72      | 0.44        | 0.46   |
| 40       | 0.62          | 0.64     | 0.74           | 0.72      | 0.44        | 0.46   |
| 41       | 0.62          | 0.63     | 0.75           | 0.73      | 0.44        | 0.45   |
| 42       | 0.61          | 0.63     | 0.75           | 0.73      | 0.43        | 0.45   |
| 43       | 0.61          | 0.63     | 0.76           | 0.73      | 0.43        | 0.45   |
| 44       | 0.60          | 0.62     | 0.76           | 0.74      | 0.43        | 0.44   |
| 45       | 0.60          | 0.62     | 0.77           | 0.74      | 0.42        | 0.44   |
| 46       | 0.60          | 0.61     | 0.77           | 0.75      | 0.42        | 0.43   |
| 47       | 0.59          | 0.61     | 0.78           | 0.75      | 0.41        | 0.43   |
| 48       | 0.59          | 0.60     | 0.78           | 0.76      | 0.41        | 0.43   |
| 49       | 0.58          | 0.60     | 0.78           | 0.76      | 0.41        | 0.43   |
| 50       | 0.58          | 0.59     | 0.79           | 0.77      | 0.40        | 0.42   |
| 51       | 0.57          | 0.59     | 0.79           | 0.77      | 0.40        | 0.42   |
| 52       | 0.57          | 0.58     | 0.80           | 0.78      | 0.39        | 0.41   |
| 53       | 0.56          | 0.58     | 0.80           | 0.78      | 0.39        | 0.41   |
| 54       | 0.55          | 0.57     | 0.81           | 0.79      | 0.38        | 0.40   |
| 55       | 0.55          | 0.56     | 0.81           | 0.79      | 0.38        | 0.39   |
| 56       | 0.54          | 0.56     | 0.82           | 0.80      | 0.37        | 0.39   |
| 57       | 0.53          | 0.55     | 0.82           | 0.80      | 0.37        | 0.38   |
| 58       | 0.53          | 0.54     | 0.83           | 0.81      | 0.36        | 0.37   |
| 59       | 0.52          | 0.54     | 0.83           | 0.81      | 0.36        | 0.37   |
| 60       | 0.51          | 0.53     | 0.84           | 0.82      | 0.35        | 0.37   |
| 61       | 0.50          | 0.52     | 0.84           | 0.82      | 0.34        | 0.36   |
| 62       | 0.50          | 0.51     | 0.85           | 0.83      | 0.34        | 0.35   |
| 63       | 0.49          | 0.51     | 0.86           | 0.83      | 0.33        | 0.35   |

Continued on next page

| $\alpha$ | $\phi_S^\ell$ | $\phi_S$ | $\varphi^\ell$ | $\varphi$ | $\psi^\ell$ | $\psi$ |
|----------|---------------|----------|----------------|-----------|-------------|--------|
| 64       | 0.48          | 0.50     | 0.86           | 0.84      | 0.32        | 0.34   |
| 65       | 0.47          | 0.49     | 0.87           | 0.84      | 0.32        | 0.34   |
| 66       | 0.46          | 0.48     | 0.87           | 0.85      | 0.31        | 0.33   |
| 67       | 0.45          | 0.47     | 0.88           | 0.85      | 0.30        | 0.32   |
| 68       | 0.44          | 0.46     | 0.88           | 0.86      | 0.30        | 0.31   |
| 69       | 0.43          | 0.45     | 0.89           | 0.87      | 0.29        | 0.30   |
| 70       | 0.41          | 0.44     | 0.90           | 0.87      | 0.27        | 0.30   |
| 71       | 0.40          | 0.43     | 0.90           | 0.88      | 0.27        | 0.29   |
| 72       | 0.39          | 0.42     | 0.91           | 0.88      | 0.26        | 0.28   |
| 73       | 0.38          | 0.40     | 0.92           | 0.89      | 0.25        | 0.27   |
| 74       | 0.36          | 0.39     | 0.92           | 0.89      | 0.24        | 0.26   |
| 75       | 0.35          | 0.38     | 0.93           | 0.90      | 0.23        | 0.25   |
| 76       | 0.33          | 0.36     | 0.93           | 0.91      | 0.22        | 0.24   |
| 77       | 0.32          | 0.35     | 0.94           | 0.91      | 0.21        | 0.23   |
| 78       | 0.30          | 0.33     | 0.94           | 0.92      | 0.20        | 0.22   |
| 79       | 0.28          | 0.32     | 0.95           | 0.92      | 0.18        | 0.21   |
| 80       | 0.26          | 0.30     | 0.96           | 0.93      | 0.17        | 0.20   |
| 81       | 0.24          | 0.29     | 0.96           | 0.93      | 0.16        | 0.19   |
| 82       | 0.22          | 0.27     | 0.97           | 0.94      | 0.14        | 0.18   |
| 83       | 0.20          | 0.25     | 0.97           | 0.94      | 0.13        | 0.17   |
| 84       | 0.18          | 0.23     | 0.98           | 0.95      | 0.12        | 0.15   |
| 85       | 0.17          | 0.22     | 0.98           | 0.95      | 0.11        | 0.14   |
| 86       | 0.15          | 0.20     | 0.98           | 0.95      | 0.10        | 0.13   |
| 87       | 0.13          | 0.18     | 0.99           | 0.96      | 0.08        | 0.12   |
| 88       | 0.11          | 0.17     | 0.99           | 0.96      | 0.07        | 0.11   |
| 89       | 0.10          | 0.16     | 0.99           | 0.96      | 0.06        | 0.11   |
| 90       | 0.10          | 0.15     | 0.99           | 0.96      | 0.06        | 0.10   |

Table S170: Reference ( $\phi_S$ ,  $\varphi$ ,  $\psi$ ) and approached ( $\phi_S^\ell$ ,  $\varphi^\ell$ ,  $\psi^\ell$ ) values of the topological descriptors for the first excited-state of the pyridinium-phenolate (PP), computed at the wB97XD/6-31G level of theory.  $\alpha$  is the pyridinium-phenolate central twist angle amplitude.

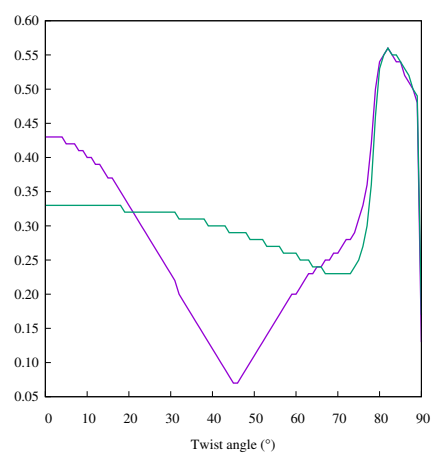

Figure S3: Reference (green) and approached (purple)  $\phi_S$  plots for the PP first excited-state computed at the B3LYP/3-21G level of theory. The descriptors values are reported with respect to the pyridinium-phenolate twist angle amplitude.

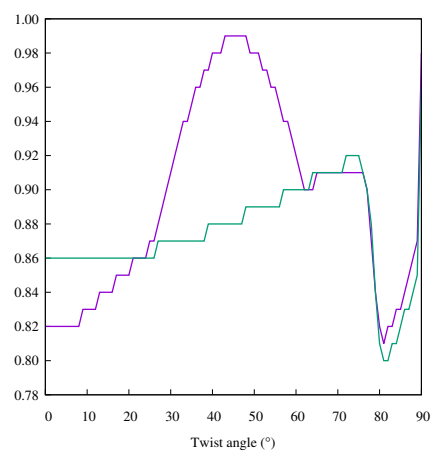

Figure S4: Reference (green) and approached (purple)  $\varphi$  plots for the PP first excited-state computed at the B3LYP/3-21G level of theory. The descriptors values are reported with respect to the pyridinium-phenolate twist angle amplitude.



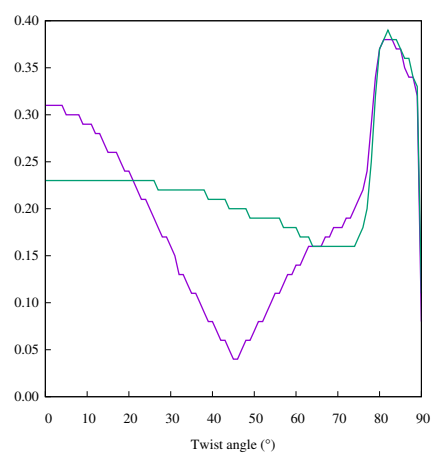

Figure S5: Reference (green) and approached (purple)  $\psi$  plots for the PP first excited-state computed at the B3LYP/3-21G level of theory. The descriptors values are reported with respect to the pyridinium-phenolate twist angle amplitude.

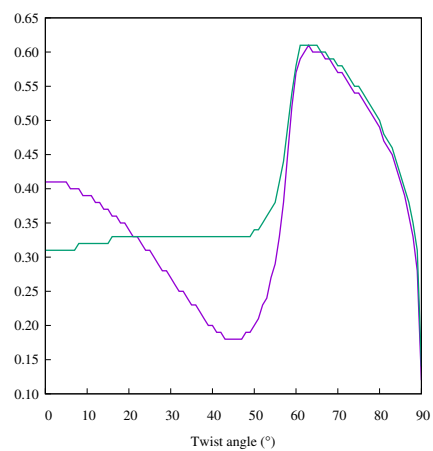

Figure S6: Reference (green) and approached (purple)  $\phi_S$  plots for the PP first excited-state computed at the B3LYP/6-311++G(2d,p) level of theory. The descriptors values are reported with respect to the pyridinium-phenolate twist angle amplitude.

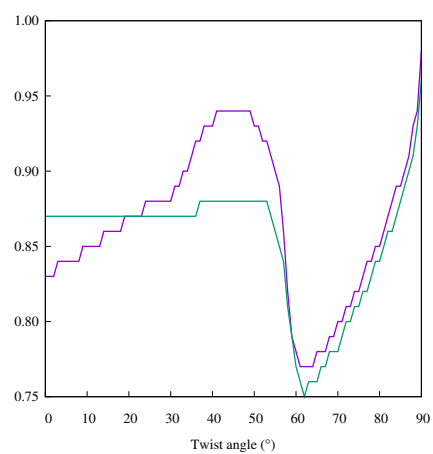

Figure S7: Reference (green) and approached (purple)  $\varphi$  plots for the PP first excited-state computed at the B3LYP/6-311++G(2d,p) level of theory. The descriptors values are reported with respect to the pyridinium-phenolate twist angle amplitude.

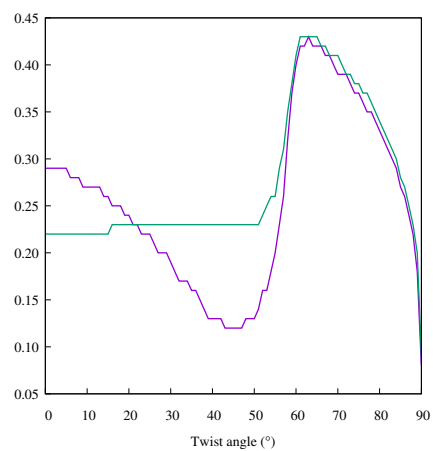

Figure S8: Reference (green) and approached (purple)  $\psi$  plots for the PP first excited-state computed at the B3LYP/6-311++G(2d,p) level of theory. The descriptors values are reported with respect to the pyridinium-phenolate twist angle amplitude.

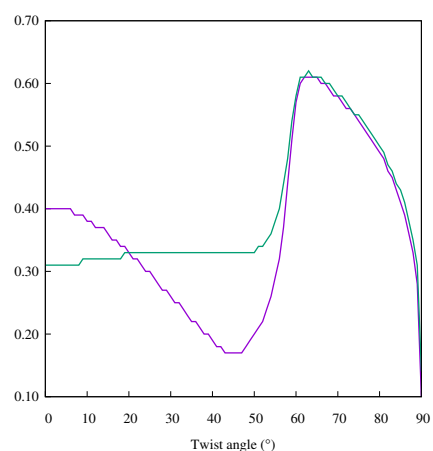

Figure S9: Reference (green) and approached (purple)  $\phi_S$  plots for the PP first excited-state computed at the B3LYP/6-311+G(d) level of theory. The descriptors values are reported with respect to the pyridinium-phenolate twist angle amplitude.

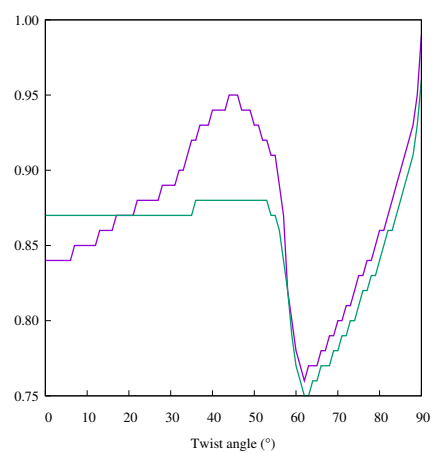

Figure S10: Reference (green) and approached (purple)  $\varphi$  plots for the PP first excited-state computed at the B3LYP/6-311+G(d) level of theory. The descriptors values are reported with respect to the pyridinium-phenolate twist angle amplitude.

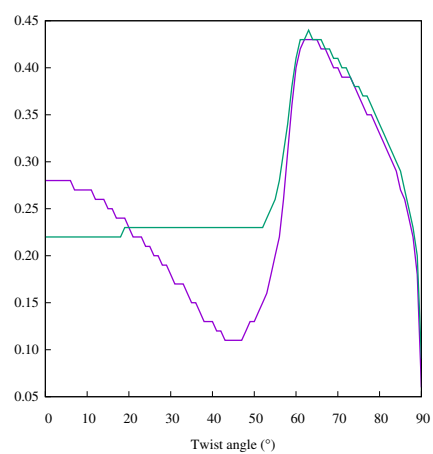

Figure S11: Reference (green) and approached (purple)  $\psi$  plots for the PP first excited-state computed at the B3LYP/6-311+G(d) level of theory. The descriptors values are reported with respect to the pyridinium-phenolate twist angle amplitude.

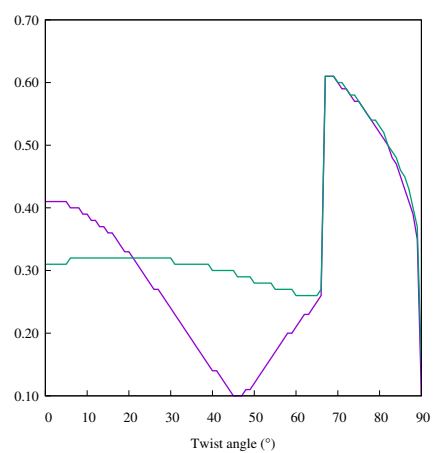

Figure S12: Reference (green) and approached (purple)  $\phi_S$  plots for the PP first excited-state computed at the B3LYP/6-311G(d) level of theory. The descriptors values are reported with respect to the pyridinium-phenolate twist angle amplitude.

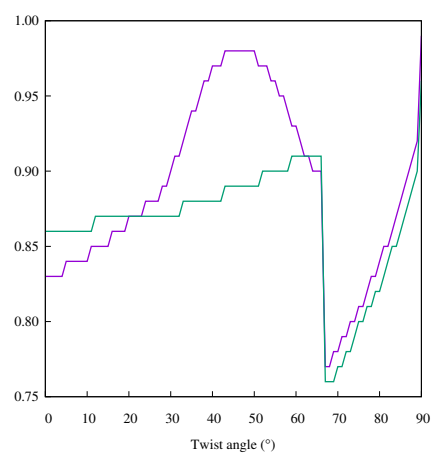

Figure S13: Reference (green) and approached (purple)  $\varphi$  plots for the PP first excited-state computed at the B3LYP/6-311G(d) level of theory. The descriptors values are reported with respect to the pyridinium-phenolate twist angle amplitude.

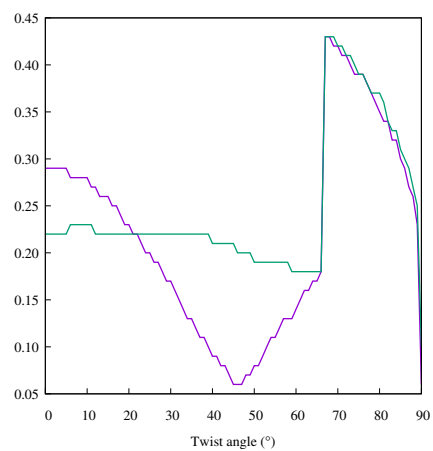

Figure S14: Reference (green) and approached (purple)  $\psi$  plots for the PP first excited-state computed at the B3LYP/6-311G(d) level of theory. The descriptors values are reported with respect to the pyridinium-phenolate twist angle amplitude.

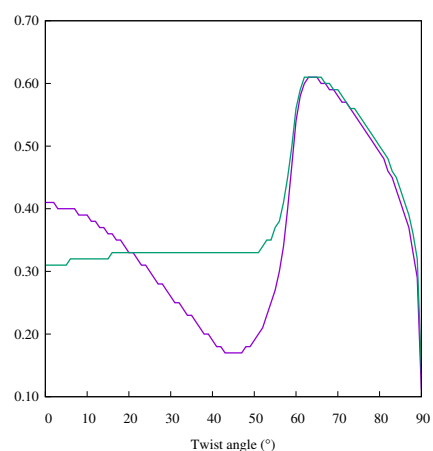

Figure S15: Reference (green) and approached (purple)  $\phi_S$  plots for the PP first excited-state computed at the B3LYP/6-311++G(d,p) level of theory. The descriptors values are reported with respect to the pyridinium-phenolate twist angle amplitude.

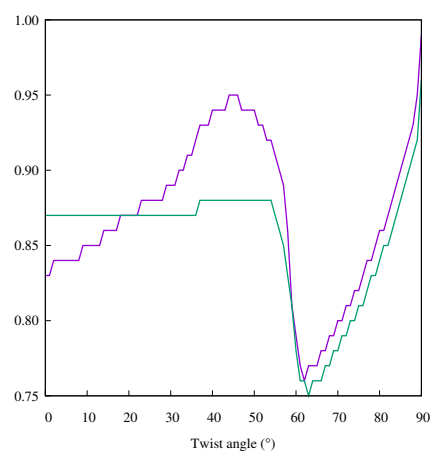

Figure S16: Reference (green) and approached (purple)  $\varphi$  plots for the PP first excited-state computed at the B3LYP/6-311++G(d,p) level of theory. The descriptors values are reported with respect to the pyridinium-phenolate twist angle amplitude.

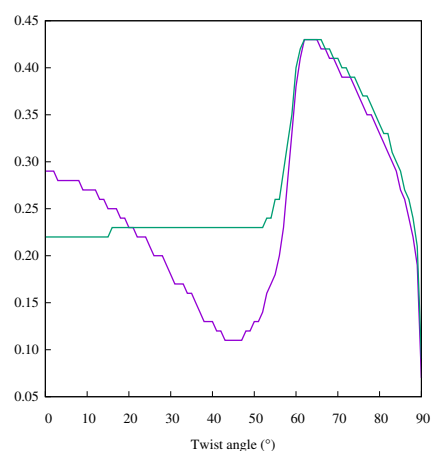

Figure S17: Reference (green) and approached (purple)  $\psi$  plots for the PP first excited-state computed at the B3LYP/6-311++G(d,p) level of theory. The descriptors values are reported with respect to the pyridinium-phenolate twist angle amplitude.

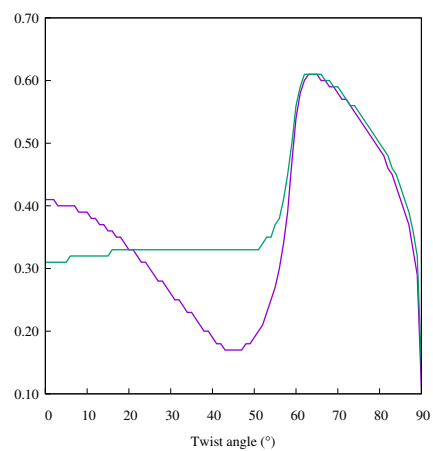

Figure S18: Reference (green) and approached (purple)  $\phi_S$  plots for the PP first excited-state computed at the B3LYP/6-311++G(d,p) level of theory. The descriptors values are reported with respect to the pyridinium-phenolate twist angle amplitude.

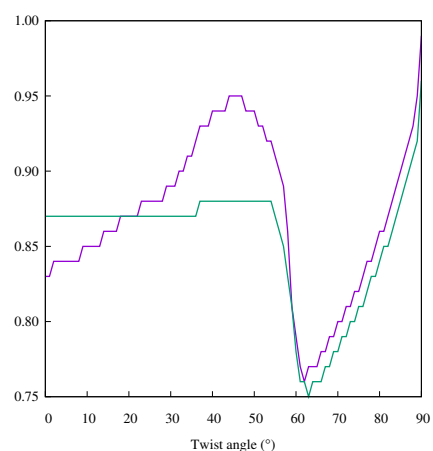

Figure S19: Reference (green) and approached (purple)  $\varphi$  plots for the PP first excited-state computed at the B3LYP/6-311+G(d,p) level of theory. The descriptors values are reported with respect to the pyridinium-phenolate twist angle amplitude.

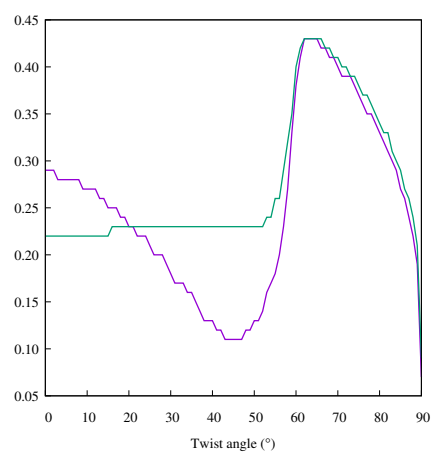

Figure S20: Reference (green) and approached (purple)  $\psi$  plots for the PP first excited-state computed at the B3LYP/6-311+G(d,p) level of theory. The descriptors values are reported with respect to the pyridinium-phenolate twist angle amplitude.



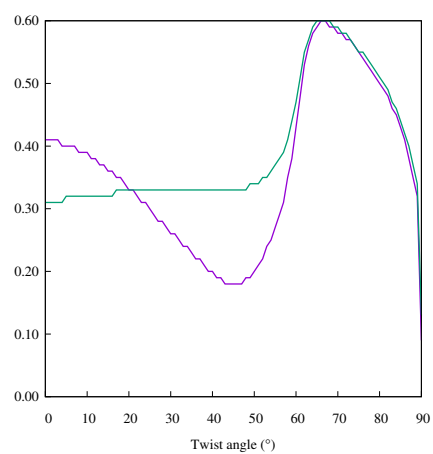

Figure S21: Reference (green) and approached (purple)  $\phi_S$  plots for the PP first excited-state computed at the B3LYP/6-311+G level of theory. The descriptors values are reported with respect to the pyridinium-phenolate twist angle amplitude.

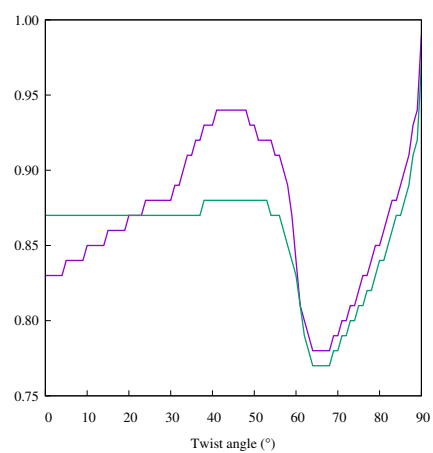

Figure S22: Reference (green) and approached (purple)  $\varphi$  plots for the PP first excited-state computed at the B3LYP/6-311+G level of theory. The descriptors values are reported with respect to the pyridinium-phenolate twist angle amplitude.

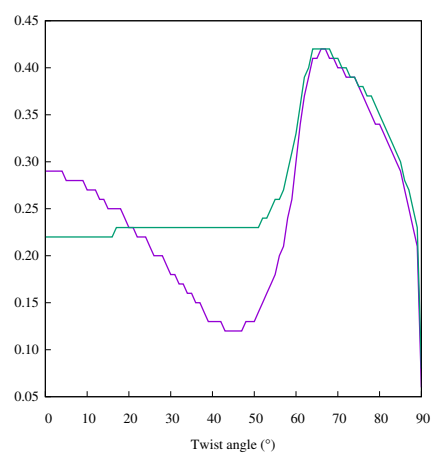

Figure S23: Reference (green) and approached (purple)  $\psi$  plots for the PP first excited-state computed at the B3LYP/6-311+G level of theory. The descriptors values are reported with respect to the pyridinium-phenolate twist angle amplitude.

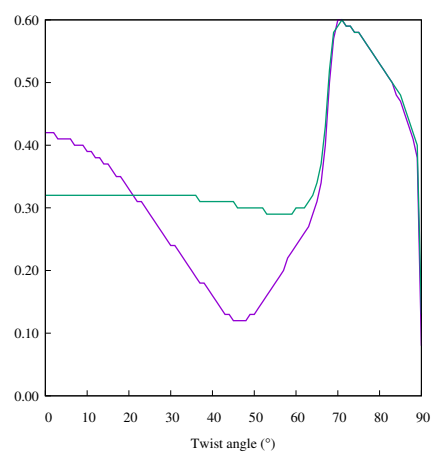

Figure S24: Reference (green) and approached (purple)  $\phi_S$  plots for the PP first excited-state computed at the B3LYP/6-311G level of theory. The descriptors values are reported with respect to the pyridinium-phenolate twist angle amplitude.

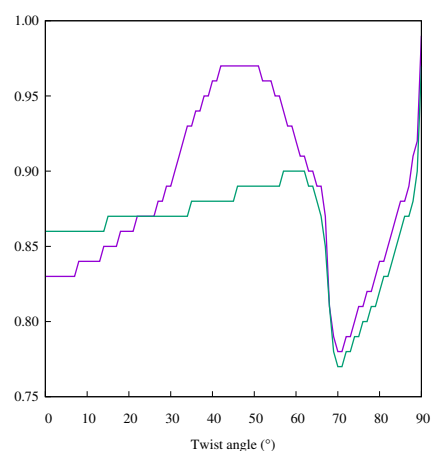

Figure S25: Reference (green) and approached (purple)  $\varphi$  plots for the PP first excited-state computed at the B3LYP/6-311G level of theory. The descriptors values are reported with respect to the pyridinium-phenolate twist angle amplitude.

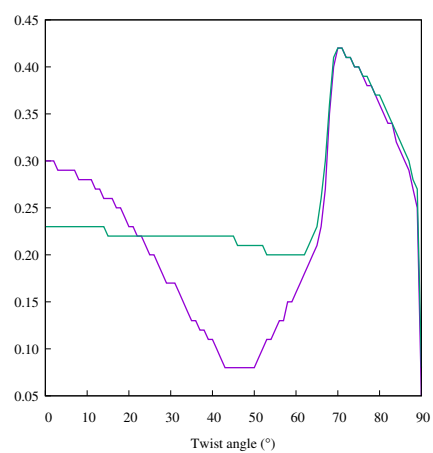

Figure S26: Reference (green) and approached (purple)  $\psi$  plots for the PP first excited-state computed at the B3LYP/6-311G level of theory. The descriptors values are reported with respect to the pyridinium-phenolate twist angle amplitude.

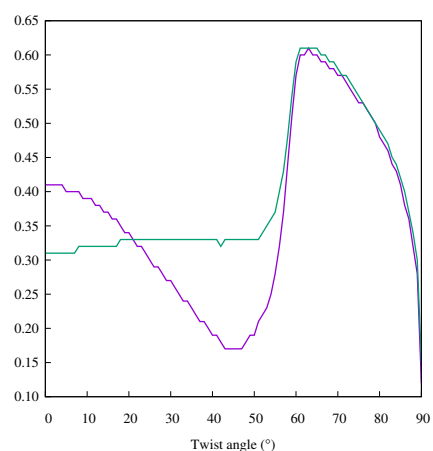

Figure S27: Reference (green) and approached (purple)  $\phi_S$  plots for the PP first excited-state computed at the B3LYP/6-31++G(2d,p) level of theory. The descriptors values are reported with respect to the pyridinium-phenolate twist angle amplitude.

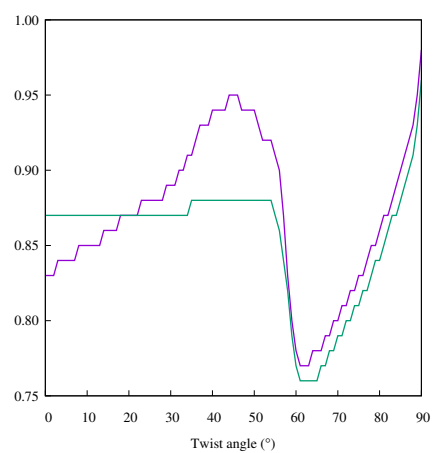

Figure S28: Reference (green) and approached (purple)  $\varphi$  plots for the PP first excited-state computed at the B3LYP/6-31++G(2d,p) level of theory. The descriptors values are reported with respect to the pyridinium-phenolate twist angle amplitude.

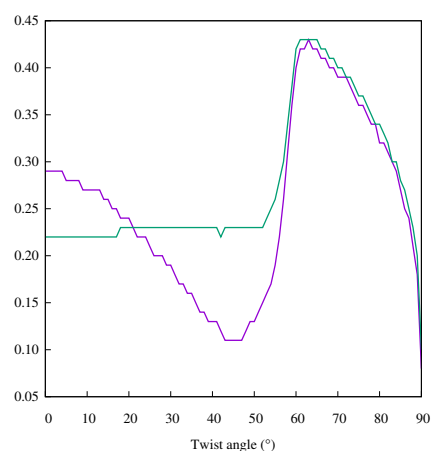

Figure S29: Reference (green) and approached (purple)  $\psi$  plots for the PP first excited-state computed at the B3LYP/6-31++G(2d,p) level of theory. The descriptors values are reported with respect to the pyridinium-phenolate twist angle amplitude.

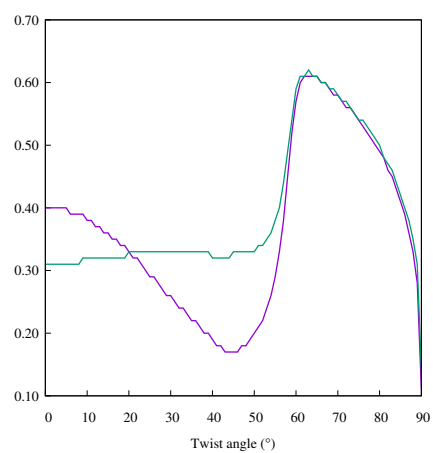

Figure S30: Reference (green) and approached (purple)  $\phi_S$  plots for the PP first excited-state computed at the B3LYP/6-31+G(d) level of theory. The descriptors values are reported with respect to the pyridinium-phenolate twist angle amplitude.

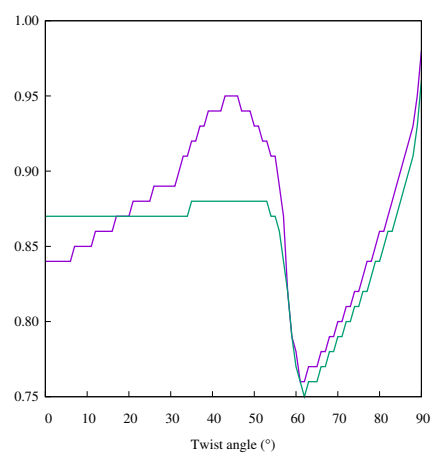

Figure S31: Reference (green) and approached (purple)  $\varphi$  plots for the PP first excited-state computed at the B3LYP/6-31+G(d) level of theory. The descriptors values are reported with respect to the pyridinium-phenolate twist angle amplitude.

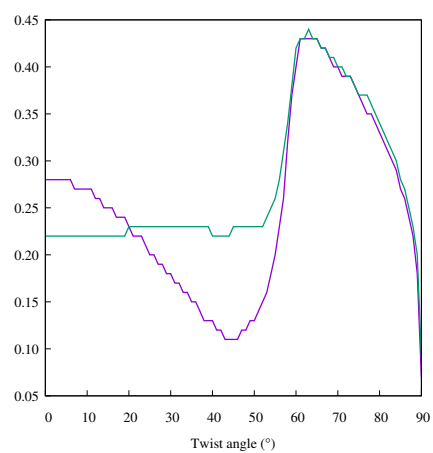

Figure S32: Reference (green) and approached (purple)  $\psi$  plots for the PP first excited-state computed at the B3LYP/6-31+G(d) level of theory. The descriptors values are reported with respect to the pyridinium-phenolate twist angle amplitude.

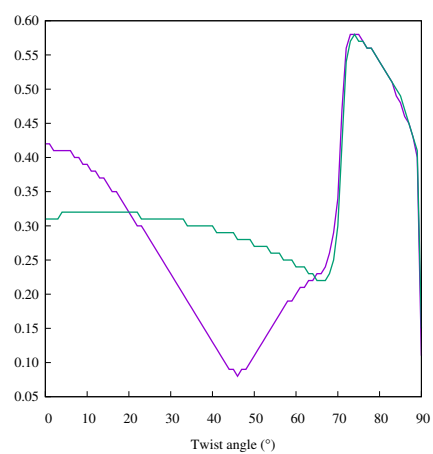

Figure S33: Reference (green) and approached (purple)  $\phi_S$  plots for the PP first excited-state computed at the B3LYP/6-31G(d) level of theory. The descriptors values are reported with respect to the pyridinium-phenolate twist angle amplitude.

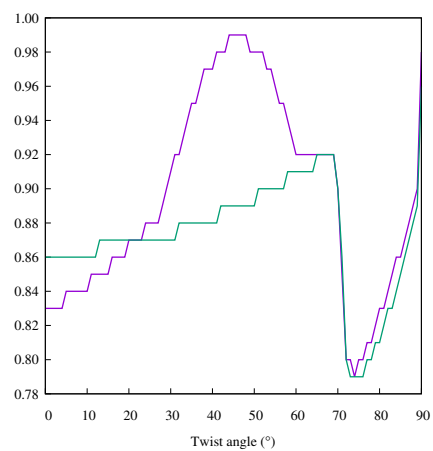

Figure S34: Reference (green) and approached (purple)  $\varphi$  plots for the PP first excited-state computed at the B3LYP/6-31G(d) level of theory. The descriptors values are reported with respect to the pyridinium-phenolate twist angle amplitude.

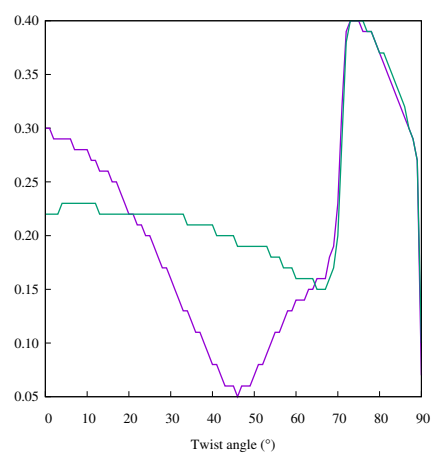

Figure S35: Reference (green) and approached (purple)  $\psi$  plots for the PP first excited-state computed at the B3LYP/6-31G(d) level of theory. The descriptors values are reported with respect to the pyridinium-phenolate twist angle amplitude.

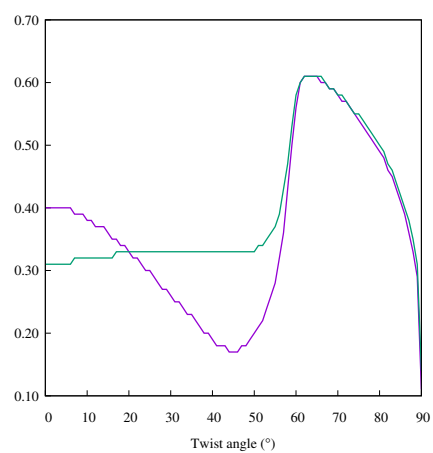

Figure S36: Reference (green) and approached (purple)  $\phi_S$  plots for the PP first excited-state computed at the B3LYP/6-31++G(d,p) level of theory. The descriptors values are reported with respect to the pyridinium-phenolate twist angle amplitude.



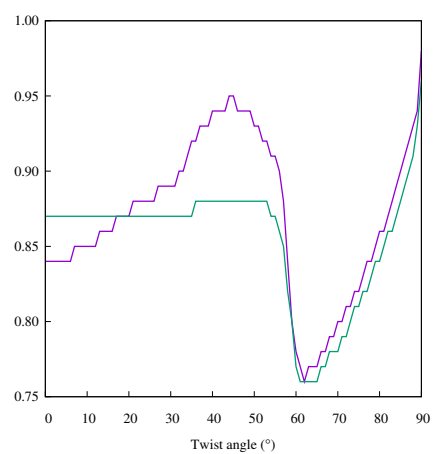

Figure S37: Reference (green) and approached (purple)  $\varphi$  plots for the PP first excited-state computed at the B3LYP/6-31++G(d,p) level of theory. The descriptors values are reported with respect to the pyridinium-phenolate twist angle amplitude.

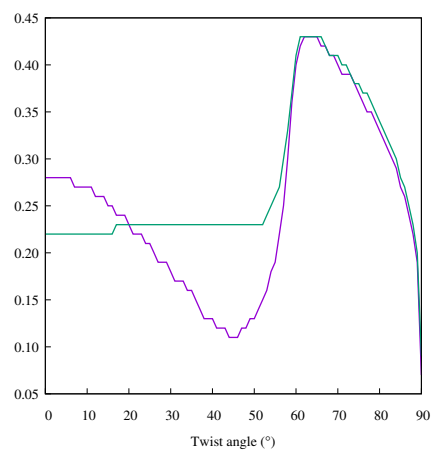

Figure S38: Reference (green) and approached (purple)  $\psi$  plots for the PP first excited-state computed at the B3LYP/6-31++G(d,p) level of theory. The descriptors values are reported with respect to the pyridinium-phenolate twist angle amplitude.

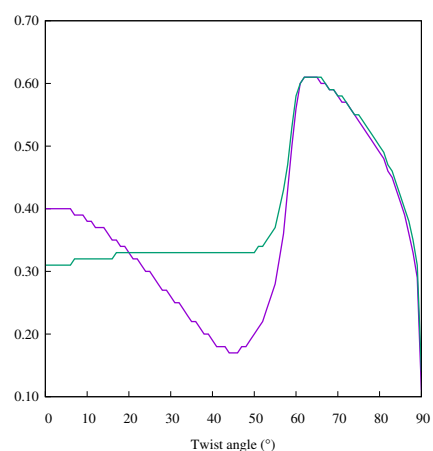

Figure S39: Reference (green) and approached (purple)  $\phi_S$  plots for the PP first excited-state computed at the B3LYP/6-31+G(d,p) level of theory. The descriptors values are reported with respect to the pyridinium-phenolate twist angle amplitude.

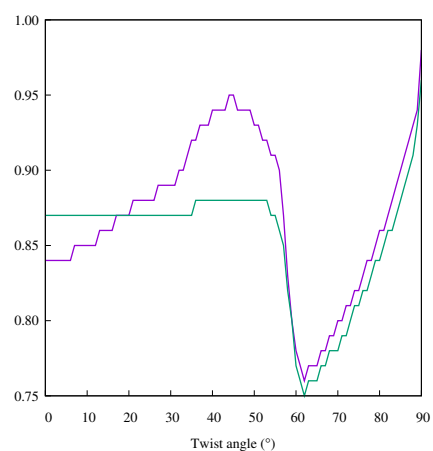

Figure S40: Reference (green) and approached (purple)  $\varphi$  plots for the PP first excited-state computed at the B3LYP/6-31+G(d,p) level of theory. The descriptors values are reported with respect to the pyridinium-phenolate twist angle amplitude.

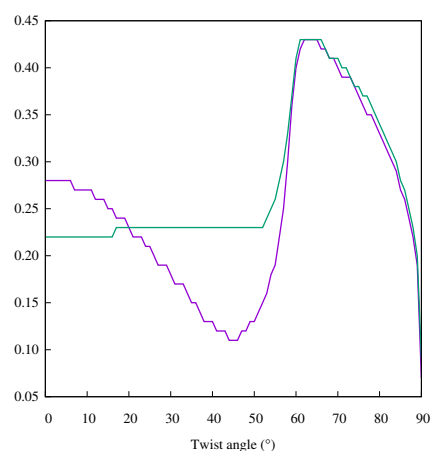

Figure S41: Reference (green) and approached (purple)  $\psi$  plots for the PP first excited-state computed at the B3LYP/6-31+G(d,p) level of theory. The descriptors values are reported with respect to the pyridinium-phenolate twist angle amplitude.

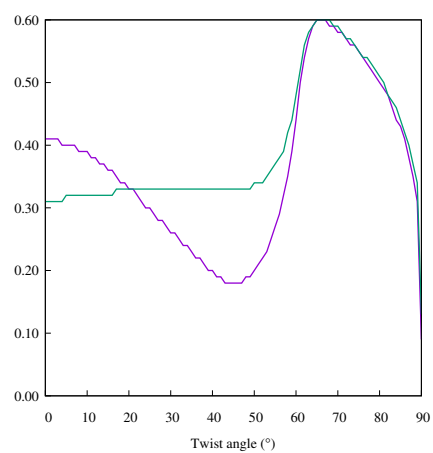

Figure S42: Reference (green) and approached (purple)  $\phi_S$  plots for the PP first excited-state computed at the B3LYP/6-31+G level of theory. The descriptors values are reported with respect to the pyridinium-phenolate twist angle amplitude.

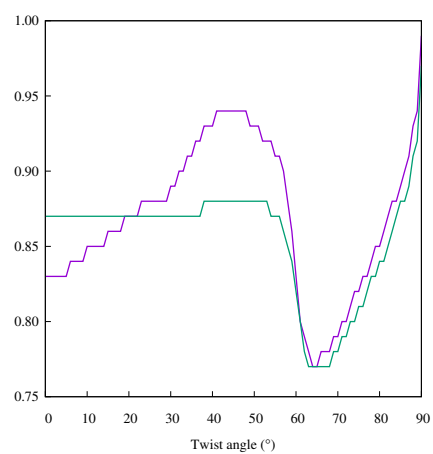

Figure S43: Reference (green) and approached (purple)  $\varphi$  plots for the PP first excited-state computed at the B3LYP/6-31+G level of theory. The descriptors values are reported with respect to the pyridinium-phenolate twist angle amplitude.

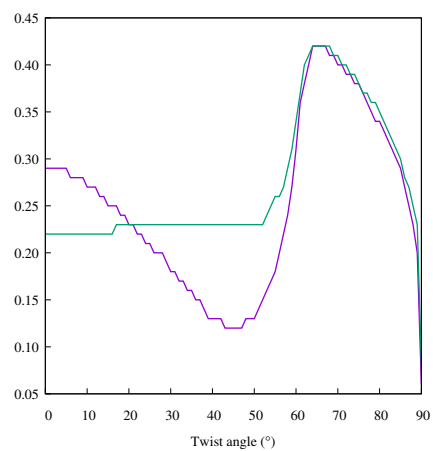

Figure S44: Reference (green) and approached (purple)  $\psi$  plots for the PP first excited-state computed at the B3LYP/6-31+G level of theory. The descriptors values are reported with respect to the pyridinium-phenolate twist angle amplitude.

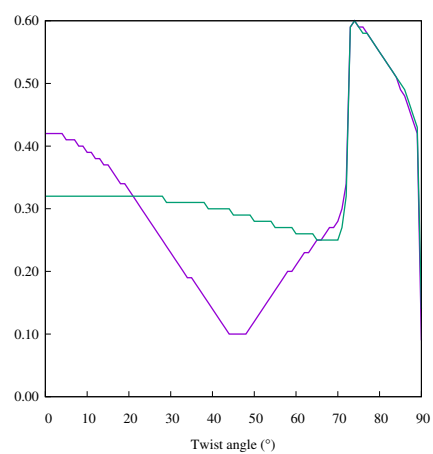

Figure S45: Reference (green) and approached (purple)  $\phi_S$  plots for the PP first excited-state computed at the B3LYP/6-31G level of theory. The descriptors values are reported with respect to the pyridinium-phenolate twist angle amplitude.

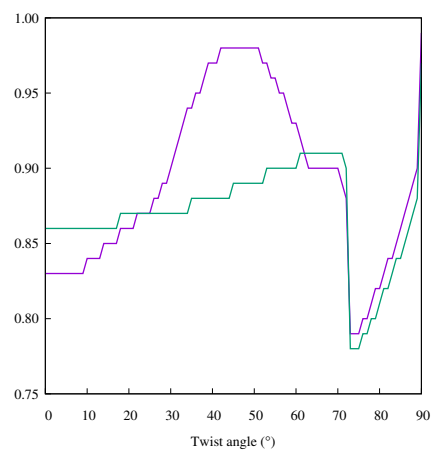

Figure S46: Reference (green) and approached (purple)  $\varphi$  plots for the PP first excited-state computed at the B3LYP/6-31G level of theory. The descriptors values are reported with respect to the pyridinium-phenolate twist angle amplitude.

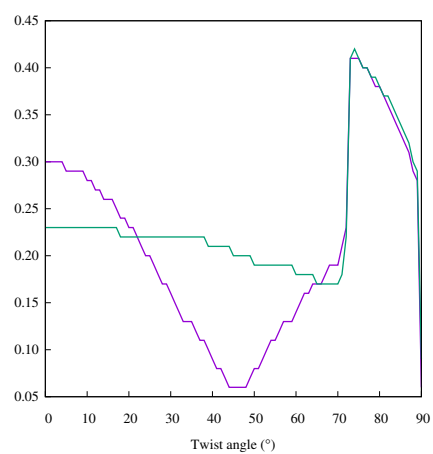

Figure S47: Reference (green) and approached (purple)  $\psi$  plots for the PP first excited-state computed at the B3LYP/6-31G level of theory. The descriptors values are reported with respect to the pyridinium-phenolate twist angle amplitude.

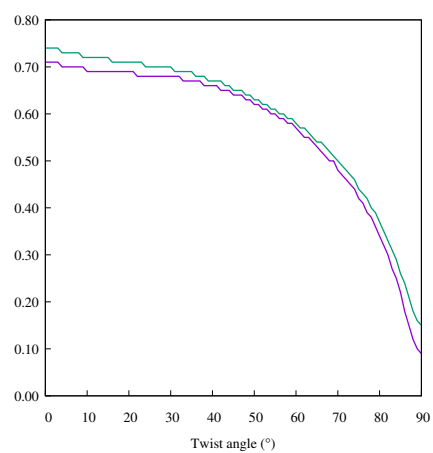

Figure S48: Reference (green) and approached (purple)  $\phi_S$  plots for the PP first excited-state computed at the CAM-B3LYP/3-21G level of theory. The descriptors values are reported with respect to the pyridinium-phenolate twist angle amplitude.

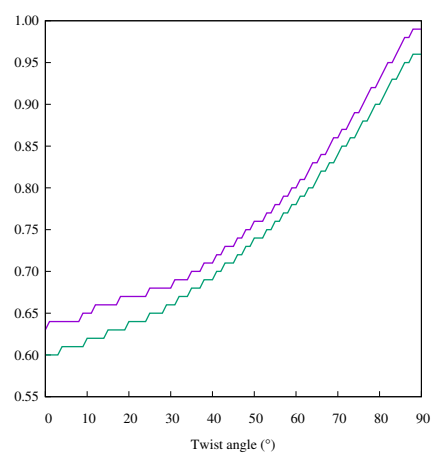

Figure S49: Reference (green) and approached (purple)  $\phi$  plots for the PP first excited-state computed at the CAM-B3LYP/3-21G level of theory. The descriptors values are reported with respect to the pyridinium-phenolate twist angle amplitude.

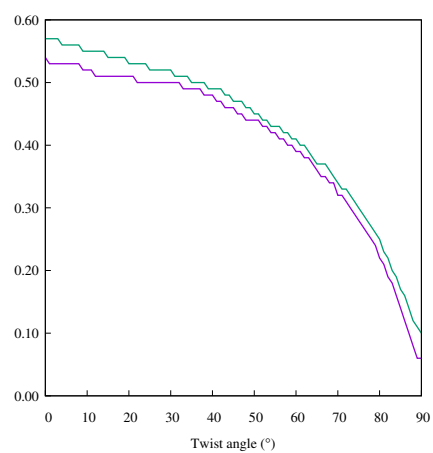

Figure S50: Reference (green) and approached (purple)  $\psi$  plots for the PP first excited-state computed at the CAM-B3LYP/3-21G level of theory. The descriptors values are reported with respect to the pyridinium-phenolate twist angle amplitude.

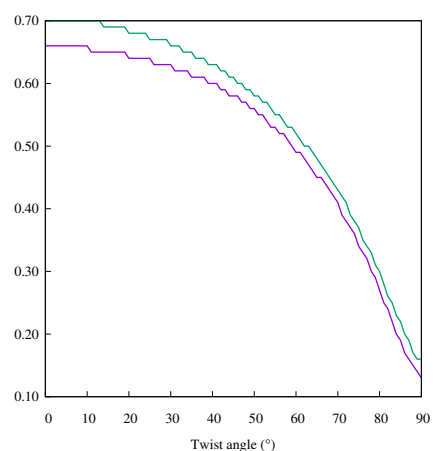

Figure S51: Reference (green) and approached (purple)  $\phi_S$  plots for the PP first excited-state computed at the CAM-B3LYP/6-311++G(2d,p) level of theory. The descriptors values are reported with respect to the pyridinium-phenolate twist angle amplitude.

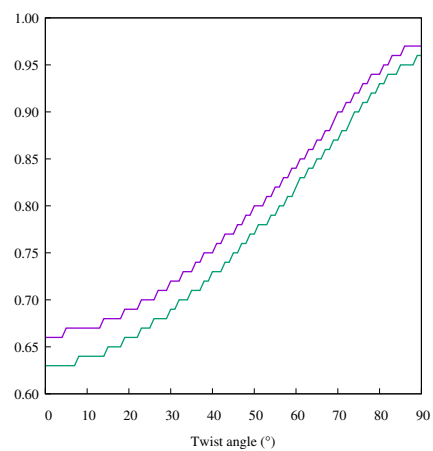

Figure S52: Reference (green) and approached (purple)  $\varphi$  plots for the PP first excited-state computed at the CAM-B3LYP/6-311++G(2d,p) level of theory. The descriptors values are reported with respect to the pyridinium-phenolate twist angle amplitude.



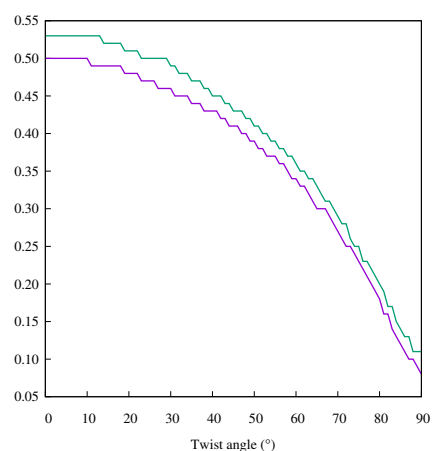

Figure S53: Reference (green) and approached (purple)  $\psi$  plots for the PP first excited-state computed at the CAM-B3LYP/6-311++G(2d,p) level of theory. The descriptors values are reported with respect to the pyridinium-phenolate twist angle amplitude.

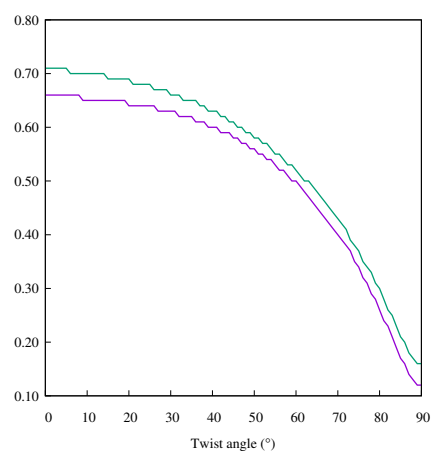

Figure S54: Reference (green) and approached (purple)  $\phi_S$  plots for the PP first excited-state computed at the CAM-B3LYP/6-311+G(d) level of theory. The descriptors values are reported with respect to the pyridinium-phenolate twist angle amplitude.

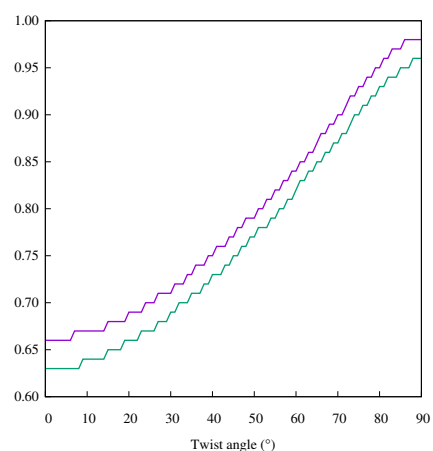

Figure S55: Reference (green) and approached (purple)  $\varphi$  plots for the PP first excited-state computed at the CAM-B3LYP/6-311+G(d) level of theory. The descriptors values are reported with respect to the pyridinium-phenolate twist angle amplitude.

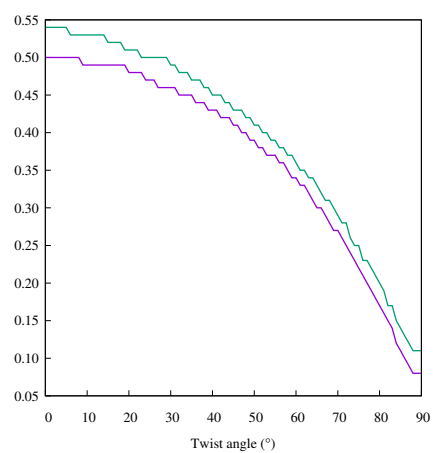

Figure S56: Reference (green) and approached (purple)  $\psi$  plots for the PP first excited-state computed at the CAM-B3LYP/6-311+G(d) level of theory. The descriptors values are reported with respect to the pyridinium-phenolate twist angle amplitude.

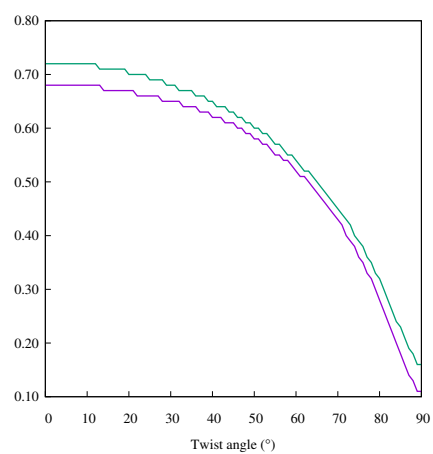

Figure S57: Reference (green) and approached (purple)  $\phi_S$  plots for the PP first excited-state computed at the CAM-B3LYP/6-311G(d) level of theory. The descriptors values are reported with respect to the pyridinium-phenolate twist angle amplitude.

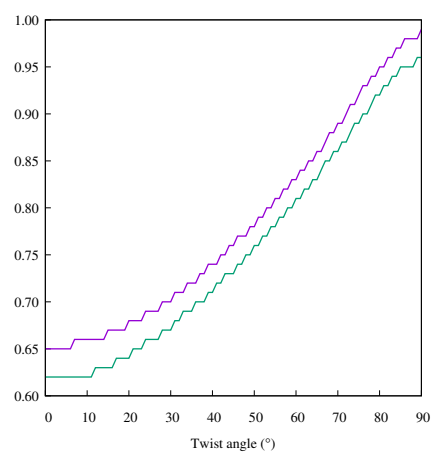

Figure S58: Reference (green) and approached (purple)  $\varphi$  plots for the PP first excited-state computed at the CAM-B3LYP/6-311G(d) level of theory. The descriptors values are reported with respect to the pyridinium-phenolate twist angle amplitude.

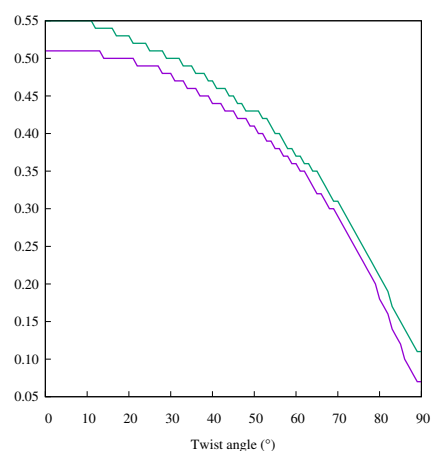

Figure S59: Reference (green) and approached (purple)  $\psi$  plots for the PP first excited-state computed at the CAM-B3LYP/6-311G(d) level of theory. The descriptors values are reported with respect to the pyridinium-phenolate twist angle amplitude.

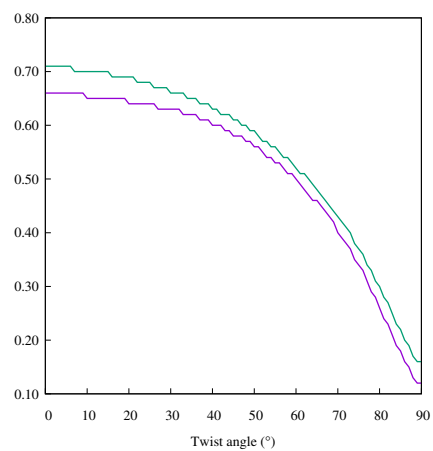

Figure S60: Reference (green) and approached (purple)  $\phi_S$  plots for the PP first excited-state computed at the CAM-B3LYP/6-311++G(d,p) level of theory. The descriptors values are reported with respect to the pyridinium-phenolate twist angle amplitude.

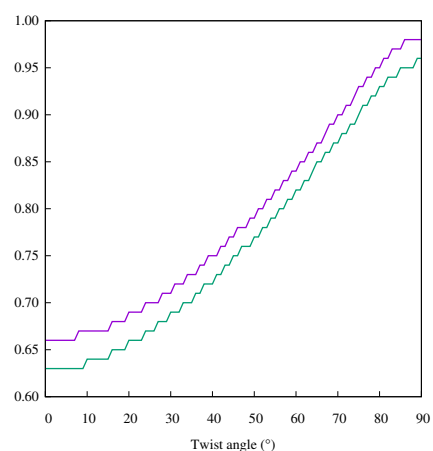

Figure S61: Reference (green) and approached (purple)  $\varphi$  plots for the PP first excited-state computed at the CAM-B3LYP/6-311++G(d,p) level of theory. The descriptors values are reported with respect to the pyridinium-phenolate twist angle amplitude.

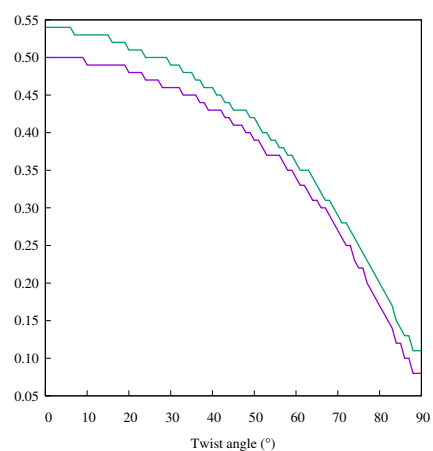

Figure S62: Reference (green) and approached (purple)  $\psi$  plots for the PP first excited-state computed at the CAM-B3LYP/6-311++G(d,p) level of theory. The descriptors values are reported with respect to the pyridinium-phenolate twist angle amplitude.

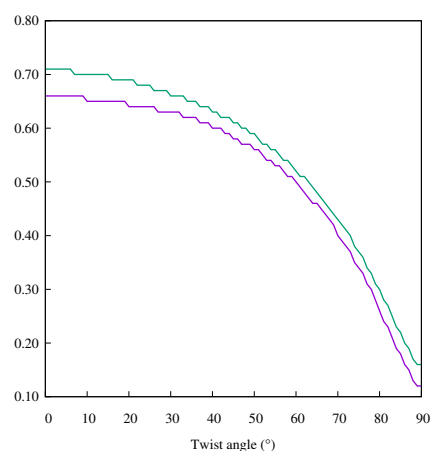

Figure S63: Reference (green) and approached (purple)  $\phi_S$  plots for the PP first excited-state computed at the CAM-B3LYP/6-311+G(d,p) level of theory. The descriptors values are reported with respect to the pyridinium-phenolate twist angle amplitude.

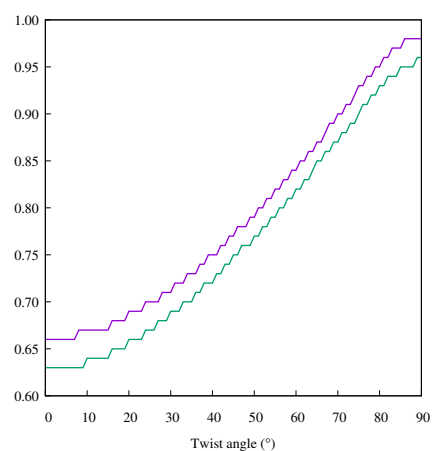

Figure S64: Reference (green) and approached (purple)  $\varphi$  plots for the PP first excited-state computed at the CAM-B3LYP/6-311+G(d,p) level of theory. The descriptors values are reported with respect to the pyridinium-phenolate twist angle amplitude.

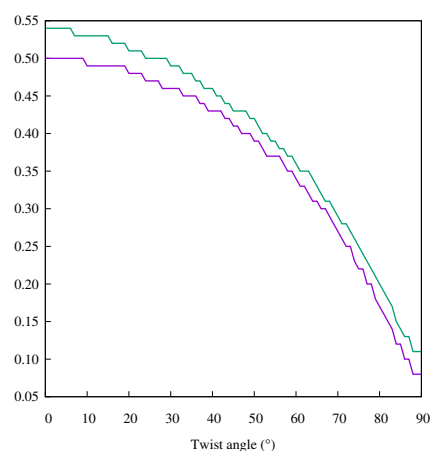

Figure S65: Reference (green) and approached (purple)  $\psi$  plots for the PP first excited-state computed at the CAM-B3LYP/6-311+G(d,p) level of theory. The descriptors values are reported with respect to the pyridinium-phenolate twist angle amplitude.

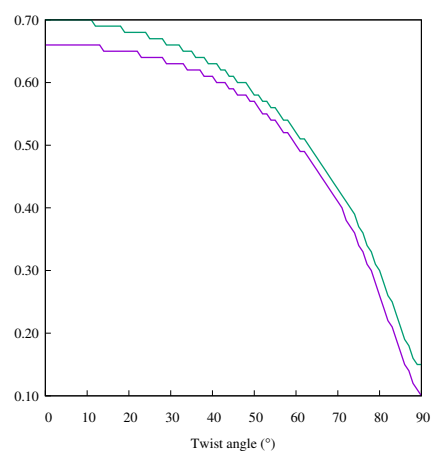

Figure S66: Reference (green) and approached (purple)  $\phi_S$  plots for the PP first excited-state computed at the CAM-B3LYP/6-311+G level of theory. The descriptors values are reported with respect to the pyridinium-phenolate twist angle amplitude.

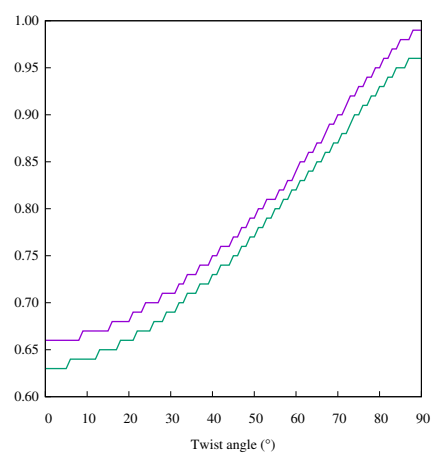

Figure S67: Reference (green) and approached (purple)  $\varphi$  plots for the PP first excited-state computed at the CAM-B3LYP/6-311+G level of theory. The descriptors values are reported with respect to the pyridinium-phenolate twist angle amplitude.

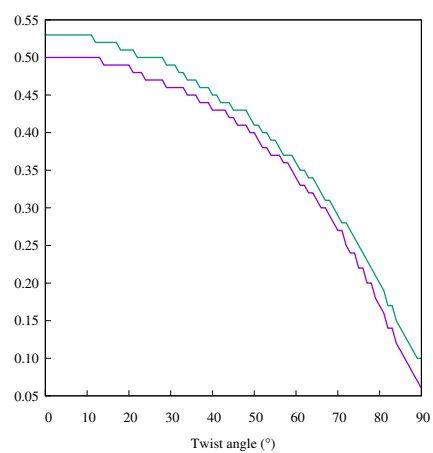

Figure S68: Reference (green) and approached (purple)  $\psi$  plots for the PP first excited-state computed at the CAM-B3LYP/6-311+G level of theory. The descriptors values are reported with respect to the pyridinium-phenolate twist angle amplitude.



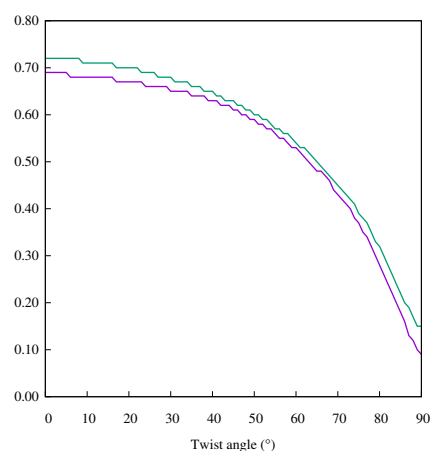

Figure S69: Reference (green) and approached (purple)  $\phi_S$  plots for the PP first excited-state computed at the CAM-B3LYP/6-311G level of theory. The descriptors values are reported with respect to the pyridinium-phenolate twist angle amplitude.

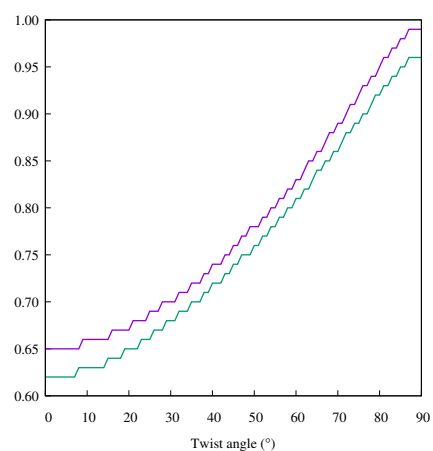

Figure S70: Reference (green) and approached (purple)  $\varphi$  plots for the PP first excited-state computed at the CAM-B3LYP/6-311G level of theory. The descriptors values are reported with respect to the pyridinium-phenolate twist angle amplitude.

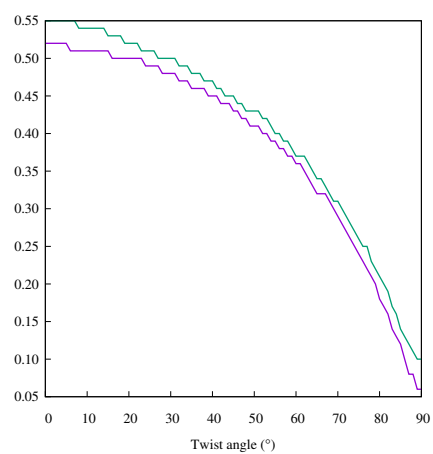

Figure S71: Reference (green) and approached (purple)  $\psi$  plots for the PP first excited-state computed at the CAM-B3LYP/6-311G level of theory. The descriptors values are reported with respect to the pyridinium-phenolate twist angle amplitude.

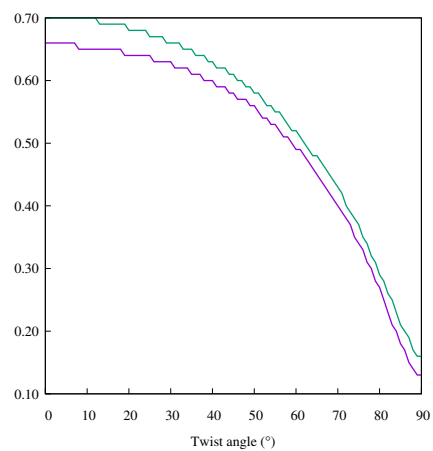

Figure S72: Reference (green) and approached (purple)  $\phi_S$  plots for the PP first excited-state computed at the CAM-B3LYP/6-31++G(2d,p) level of theory. The descriptors values are reported with respect to the pyridinium-phenolate twist angle amplitude.

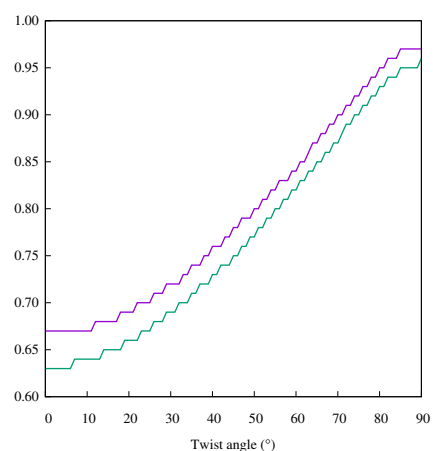

Figure S73: Reference (green) and approached (purple)  $\varphi$  plots for the PP first excited-state computed at the CAM-B3LYP/6-31++G(2d,p) level of theory. The descriptors values are reported with respect to the pyridinium-phenolate twist angle amplitude.

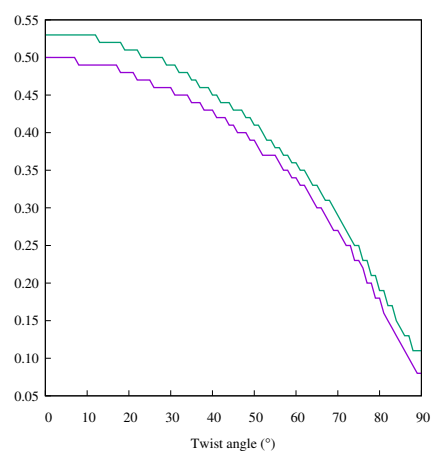

Figure S74: Reference (green) and approached (purple)  $\psi$  plots for the PP first excited-state computed at the CAM-B3LYP/6-31++G(2d,p) level of theory. The descriptors values are reported with respect to the pyridinium-phenolate twist angle amplitude.

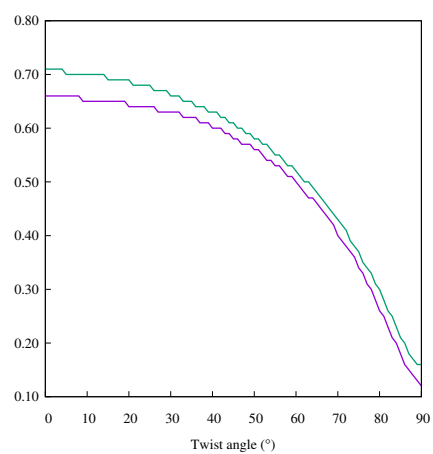

Figure S75: Reference (green) and approached (purple)  $\phi_S$  plots for the PP first excited-state computed at the CAM-B3LYP/6-31+G(d) level of theory. The descriptors values are reported with respect to the pyridinium-phenolate twist angle amplitude.

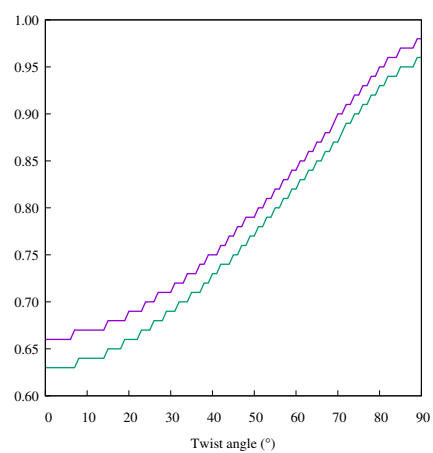

Figure S76: Reference (green) and approached (purple)  $\varphi$  plots for the PP first excited-state computed at the CAM-B3LYP/6-31+G(d) level of theory. The descriptors values are reported with respect to the pyridinium-phenolate twist angle amplitude.

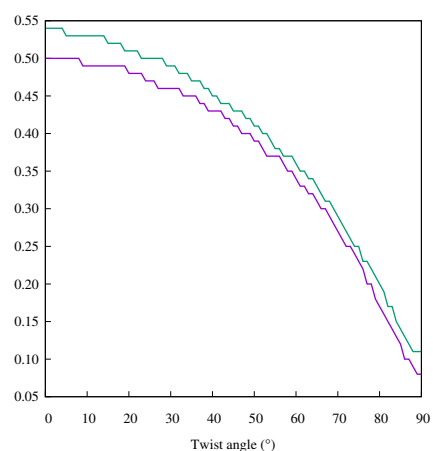

Figure S77: Reference (green) and approached (purple)  $\psi$  plots for the PP first excited-state computed at the CAM-B3LYP/6-31+G(d) level of theory. The descriptors values are reported with respect to the pyridinium-phenolate twist angle amplitude.

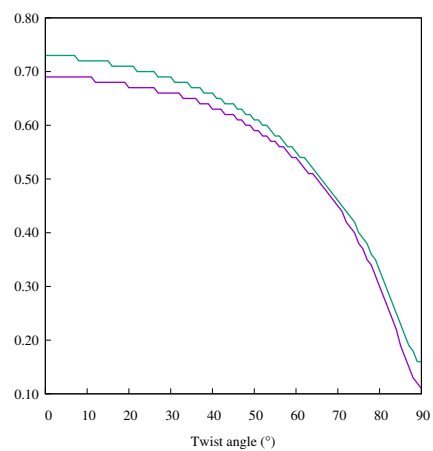

Figure S78: Reference (green) and approached (purple)  $\phi_S$  plots for the PP first excited-state computed at the CAM-B3LYP/6-31G(d) level of theory. The descriptors values are reported with respect to the pyridinium-phenolate twist angle amplitude.

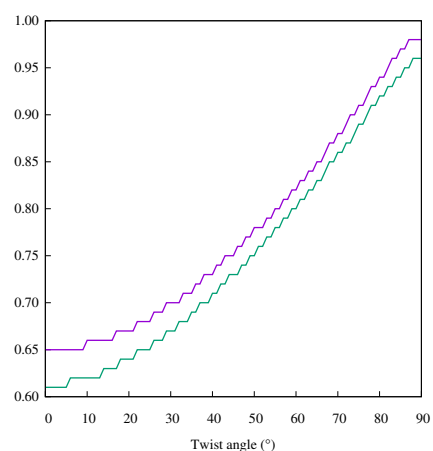

Figure S79: Reference (green) and approached (purple)  $\varphi$  plots for the PP first excited-state computed at the CAM-B3LYP/6-31G(d) level of theory. The descriptors values are reported with respect to the pyridinium-phenolate twist angle amplitude.

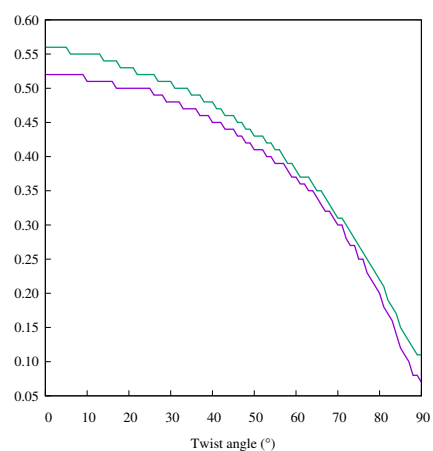

Figure S80: Reference (green) and approached (purple)  $\psi$  plots for the PP first excited-state computed at the CAM-B3LYP/6-31G(d) level of theory. The descriptors values are reported with respect to the pyridinium-phenolate twist angle amplitude.

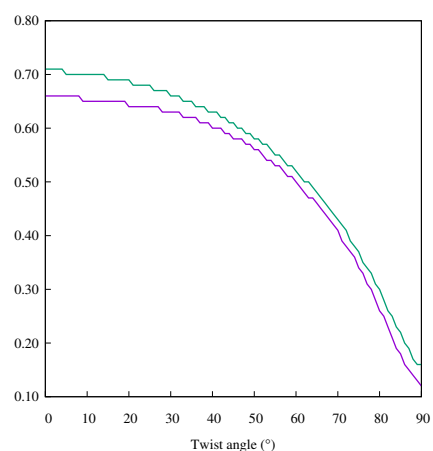

Figure S81: Reference (green) and approached (purple)  $\phi_S$  plots for the PP first excited-state computed at the CAM-B3LYP/6-31++G(d,p) level of theory. The descriptors values are reported with respect to the pyridinium-phenolate twist angle amplitude.

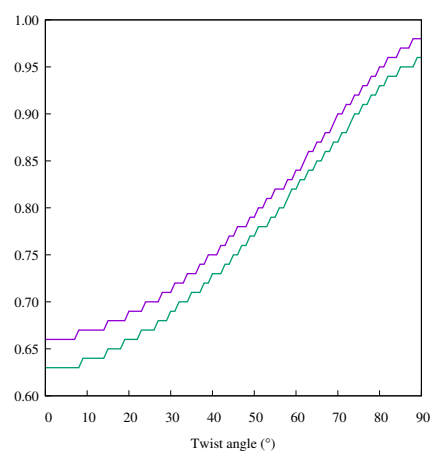

Figure S82: Reference (green) and approached (purple)  $\varphi$  plots for the PP first excited-state computed at the CAM-B3LYP/6-31++G(d,p) level of theory. The descriptors values are reported with respect to the pyridinium-phenolate twist angle amplitude.

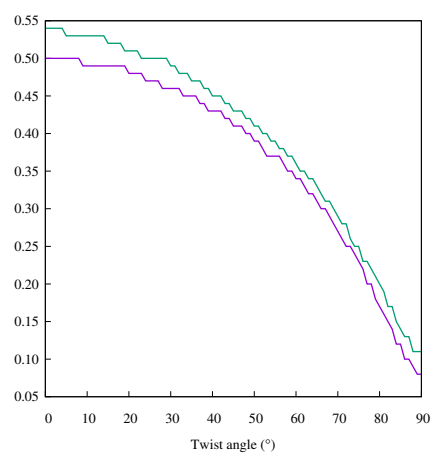

Figure S83: Reference (green) and approached (purple)  $\psi$  plots for the PP first excited-state computed at the CAM-B3LYP/6-31++G(d,p) level of theory. The descriptors values are reported with respect to the pyridinium-phenolate twist angle amplitude.

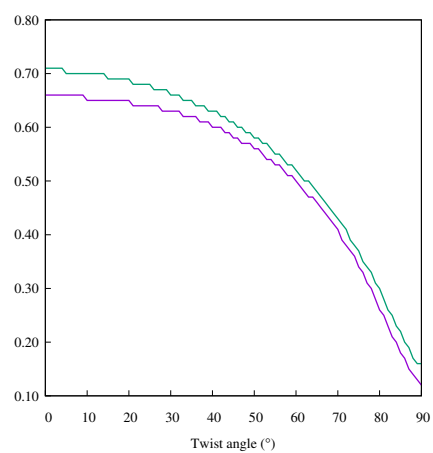

Figure S84: Reference (green) and approached (purple)  $\phi_S$  plots for the PP first excited-state computed at the CAM-B3LYP/6-31+G(d,p) level of theory. The descriptors values are reported with respect to the pyridinium-phenolate twist angle amplitude.



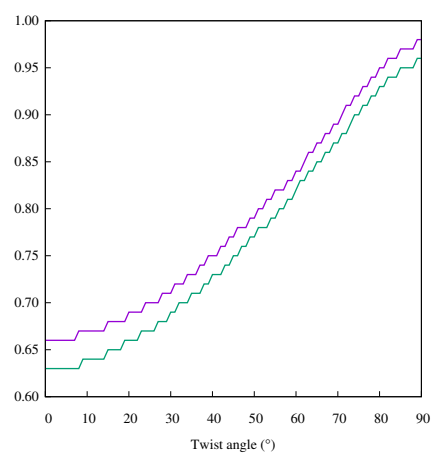

Figure S85: Reference (green) and approached (purple)  $\varphi$  plots for the PP first excited-state computed at the CAM-B3LYP/6-31+G(d,p) level of theory. The descriptors values are reported with respect to the pyridinium-phenolate twist angle amplitude.

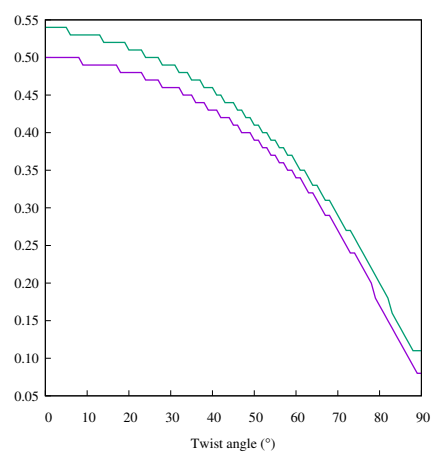

Figure S86: Reference (green) and approached (purple)  $\psi$  plots for the PP first excited-state computed at the CAM-B3LYP/6-31+G(d,p) level of theory. The descriptors values are reported with respect to the pyridinium-phenolate twist angle amplitude.

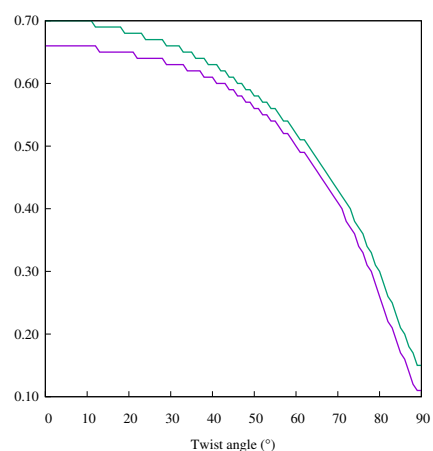

Figure S87: Reference (green) and approached (purple)  $\phi_S$  plots for the PP first excited-state computed at the CAM-B3LYP/6-31+G level of theory. The descriptors values are reported with respect to the pyridinium-phenolate twist angle amplitude.

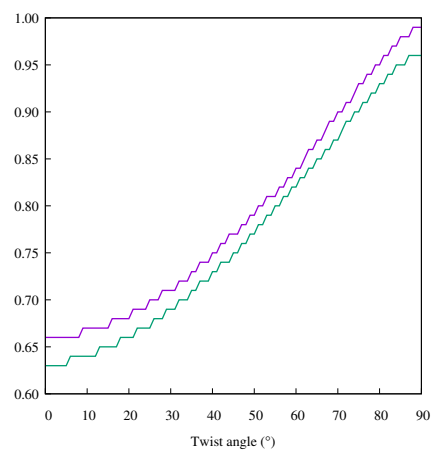

Figure S88: Reference (green) and approached (purple)  $\varphi$  plots for the PP first excited-state computed at the CAM-B3LYP/6-31+G level of theory. The descriptors values are reported with respect to the pyridinium-phenolate twist angle amplitude.

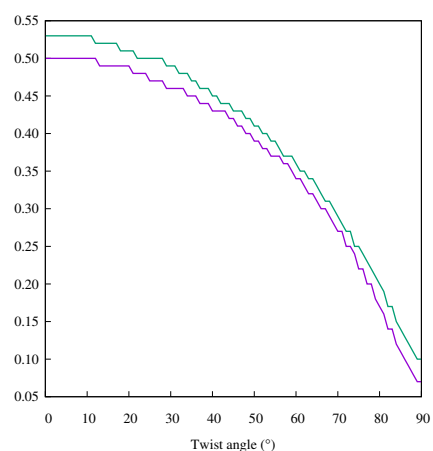

Figure S89: Reference (green) and approached (purple)  $\psi$  plots for the PP first excited-state computed at the CAM-B3LYP/6-31+G level of theory. The descriptors values are reported with respect to the pyridinium-phenolate twist angle amplitude.

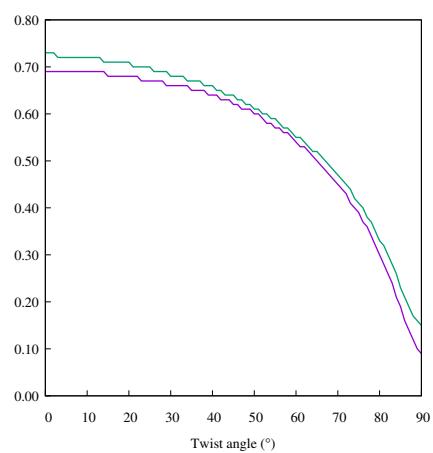

Figure S90: Reference (green) and approached (purple)  $\phi_S$  plots for the PP first excited-state computed at the CAM-B3LYP/6-31G level of theory. The descriptors values are reported with respect to the pyridinium-phenolate twist angle amplitude.

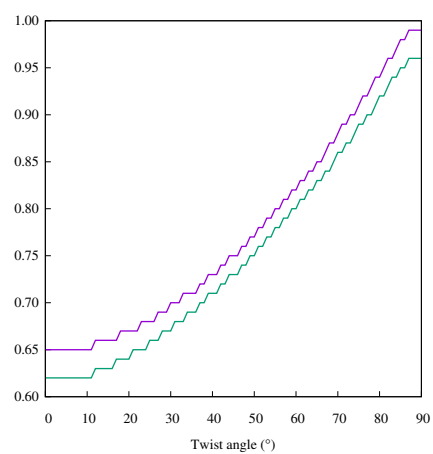

Figure S91: Reference (green) and approached (purple)  $\varphi$  plots for the PP first excited-state computed at the CAM-B3LYP/6-31G level of theory. The descriptors values are reported with respect to the pyridinium-phenolate twist angle amplitude.

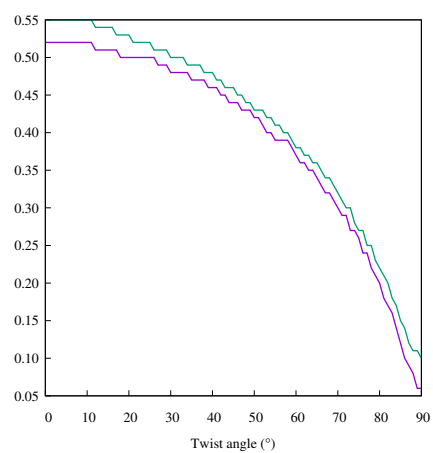

Figure S92: Reference (green) and approached (purple)  $\psi$  plots for the PP first excited-state computed at the CAM-B3LYP/6-31G level of theory. The descriptors values are reported with respect to the pyridinium-phenolate twist angle amplitude.

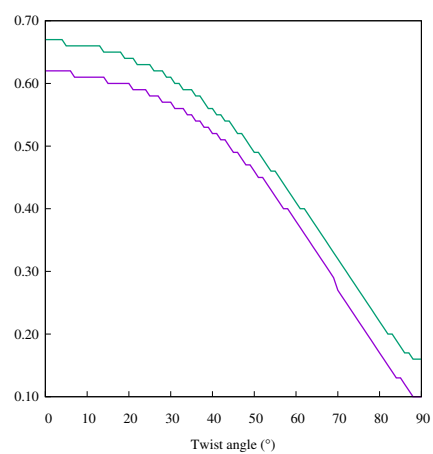

Figure S93: Reference (green) and approached (purple)  $\phi_S$  plots for the PP first excited-state computed at the CIS/3-21G level of theory. The descriptors values are reported with respect to the pyridinium-phenolate twist angle amplitude.

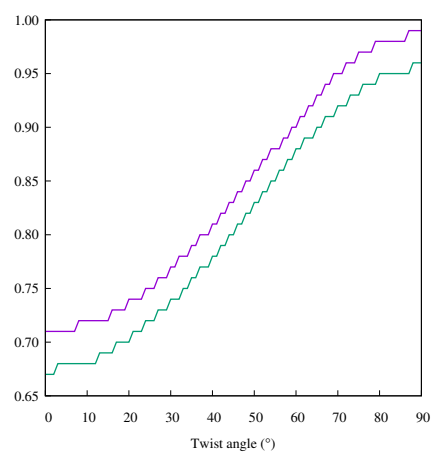

Figure S94: Reference (green) and approached (purple)  $\varphi$  plots for the PP first excited-state computed at the CIS/3-21G level of theory. The descriptors values are reported with respect to the pyridinium-phenolate twist angle amplitude.

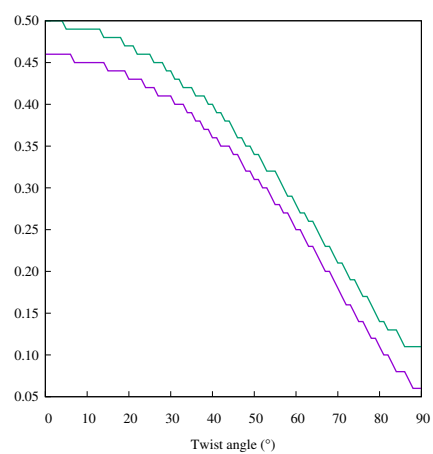

Figure S95: Reference (green) and approached (purple)  $\psi$  plots for the PP first excited-state computed at the CIS/3-21G level of theory. The descriptors values are reported with respect to the pyridinium-phenolate twist angle amplitude.

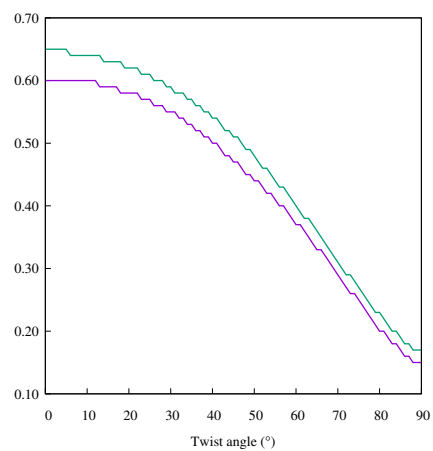

Figure S96: Reference (green) and approached (purple)  $\phi_S$  plots for the PP first excited-state computed at the CIS/6-311++G(2d,p) level of theory. The descriptors values are reported with respect to the pyridinium-phenolate twist angle amplitude.

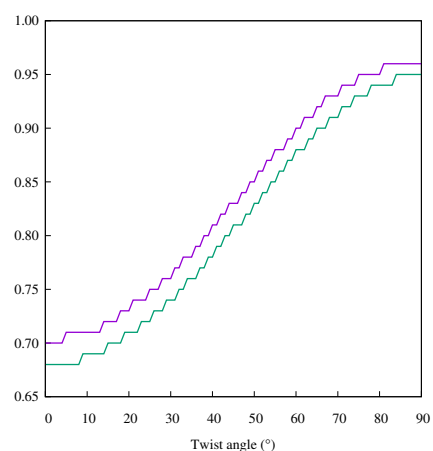

Figure S97: Reference (green) and approached (purple)  $\phi$  plots for the PP first excited-state computed at the CIS/6-311++G(2d,p) level of theory. The descriptors values are reported with respect to the pyridinium-phenolate twist angle amplitude.

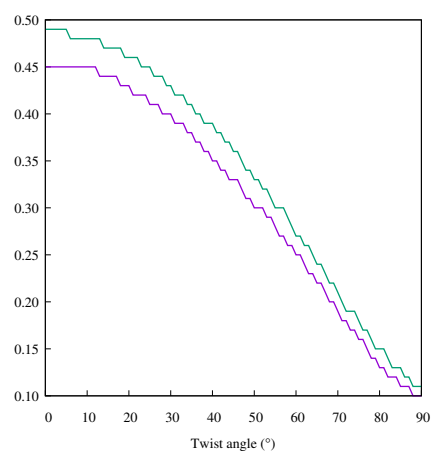

Figure S98: Reference (green) and approached (purple)  $\psi$  plots for the PP first excited-state computed at the CIS/6-311++G(2d,p) level of theory. The descriptors values are reported with respect to the pyridinium-phenolate twist angle amplitude.

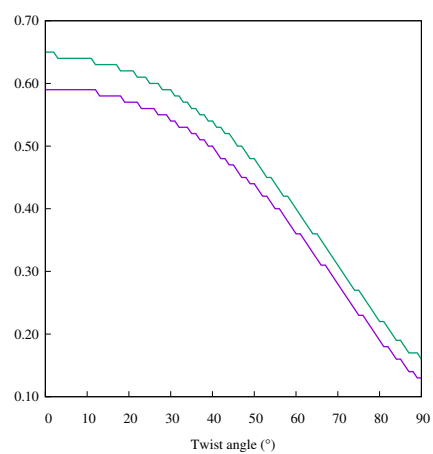

Figure S99: Reference (green) and approached (purple)  $\phi_S$  plots for the PP first excited-state computed at the CIS/6-311+G(d) level of theory. The descriptors values are reported with respect to the pyridinium-phenolate twist angle amplitude.

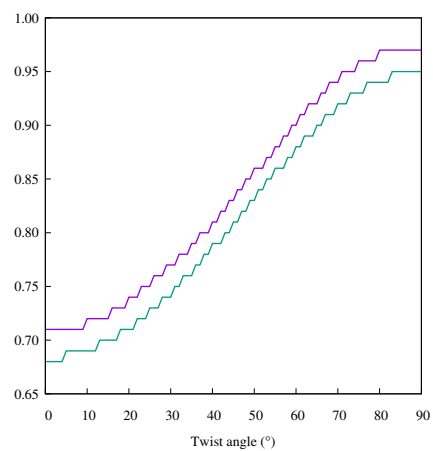

Figure S100: Reference (green) and approached (purple)  $\varphi$  plots for the PP first excited-state computed at the CIS/6-311+G(d) level of theory. The descriptors values are reported with respect to the pyridinium-phenolate twist angle amplitude.



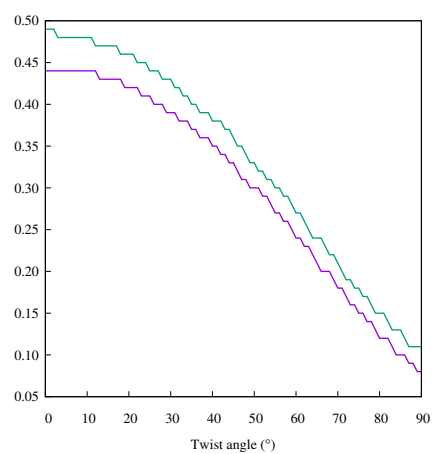

Figure S101: Reference (green) and approached (purple)  $\psi$  plots for the PP first excited-state computed at the CIS/6-311+G(d) level of theory. The descriptors values are reported with respect to the pyridinium-phenolate twist angle amplitude.

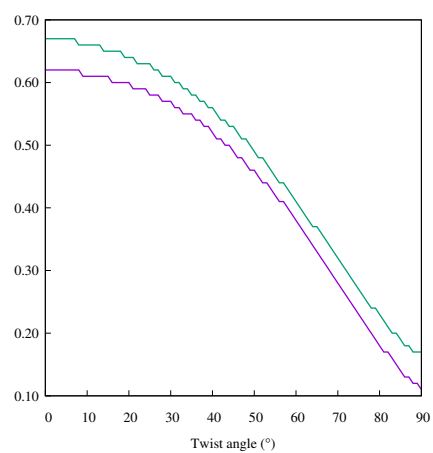

Figure S102: Reference (green) and approached (purple)  $\phi_S$  plots for the PP first excited-state computed at the CIS/6-311G(d) level of theory. The descriptors values are reported with respect to the pyridinium-phenolate twist angle amplitude.

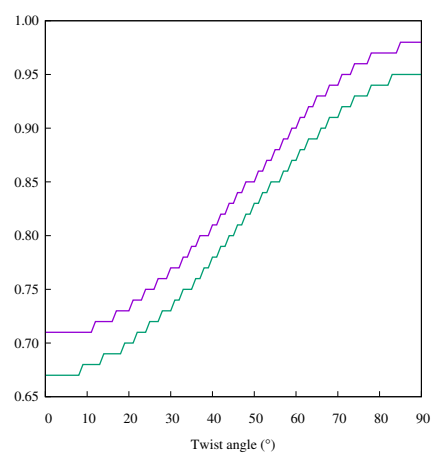

Figure S103: Reference (green) and approached (purple)  $\varphi$  plots for the PP first excited-state computed at the CIS/6-311G(d) level of theory. The descriptors values are reported with respect to the pyridinium-phenolate twist angle amplitude.

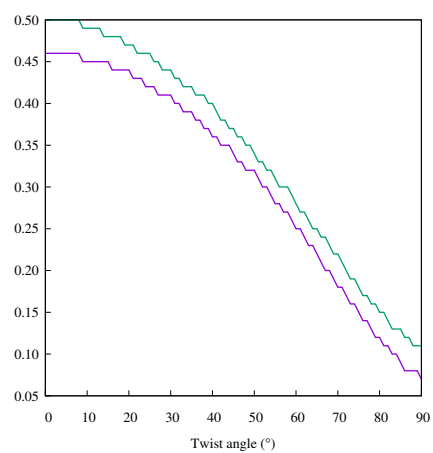

Figure S104: Reference (green) and approached (purple)  $\psi$  plots for the PP first excited-state computed at the CIS/6-311G(d) level of theory. The descriptors values are reported with respect to the pyridinium-phenolate twist angle amplitude.

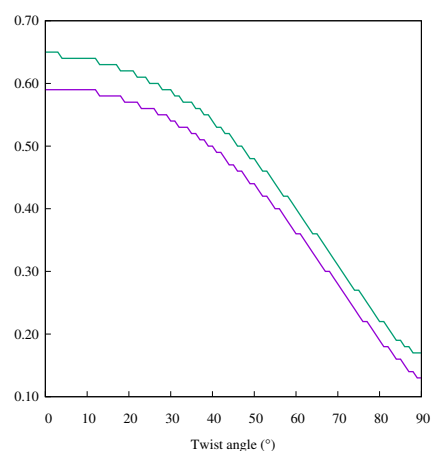

Figure S105: Reference (green) and approached (purple)  $\phi_S$  plots for the PP first excited-state computed at the CIS/6-311++G(d,p) level of theory. The descriptors values are reported with respect to the pyridinium-phenolate twist angle amplitude.

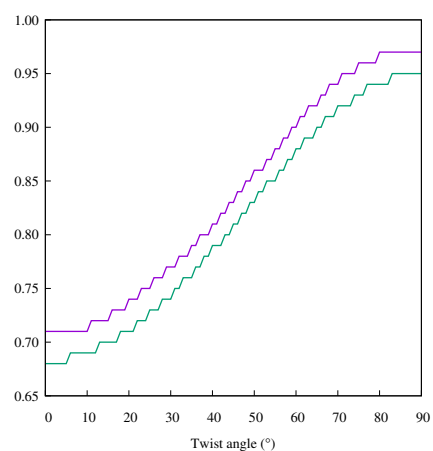

Figure S106: Reference (green) and approached (purple)  $\varphi$  plots for the PP first excited-state computed at the CIS/6-311++G(d,p) level of theory. The descriptors values are reported with respect to the pyridinium-phenolate twist angle amplitude.

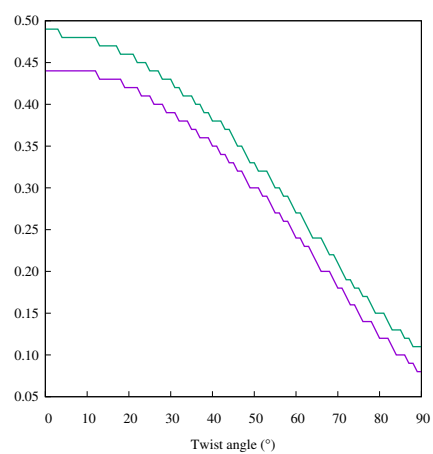

Figure S107: Reference (green) and approached (purple)  $\psi$  plots for the PP first excited-state computed at the CIS/6-311++G(d,p) level of theory. The descriptors values are reported with respect to the pyridinium-phenolate twist angle amplitude.

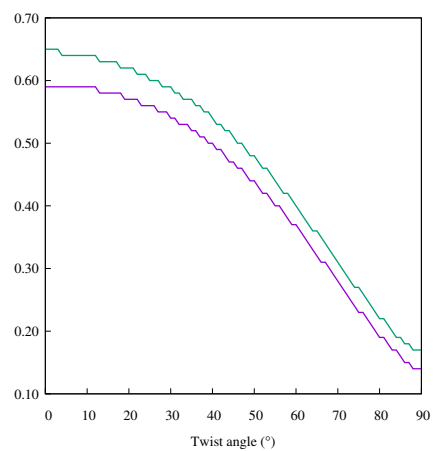

Figure S108: Reference (green) and approached (purple)  $\phi_S$  plots for the PP first excited-state computed at the CIS/6-311++G(d,p) level of theory. The descriptors values are reported with respect to the pyridinium-phenolate twist angle amplitude.

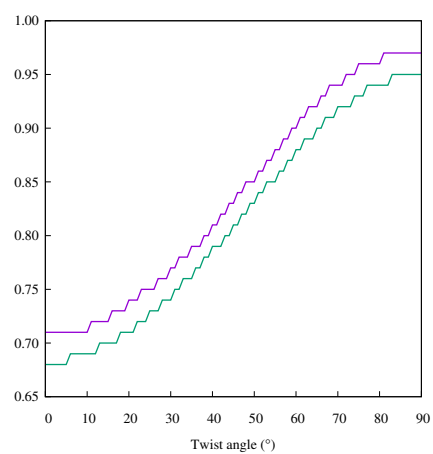

Figure S109: Reference (green) and approached (purple)  $\varphi$  plots for the PP first excited-state computed at the CIS/6-311+G(d,p) level of theory. The descriptors values are reported with respect to the pyridinium-phenolate twist angle amplitude.

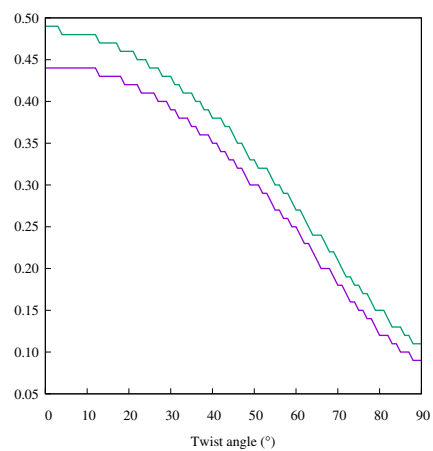

Figure S110: Reference (green) and approached (purple)  $\psi$  plots for the PP first excited-state computed at the CIS/6-311+G(d,p) level of theory. The descriptors values are reported with respect to the pyridinium-phenolate twist angle amplitude.

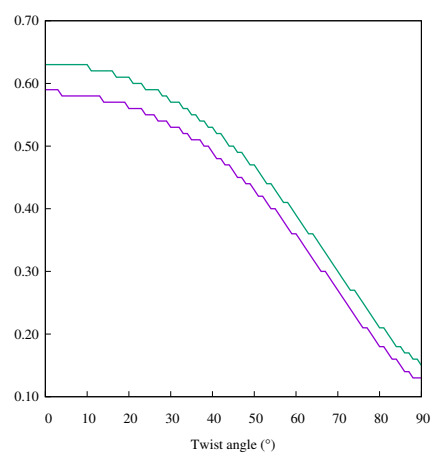

Figure S111: Reference (green) and approached (purple)  $\phi_S$  plots for the PP first excited-state computed at the CIS/6-311+G level of theory. The descriptors values are reported with respect to the pyridinium-phenolate twist angle amplitude.

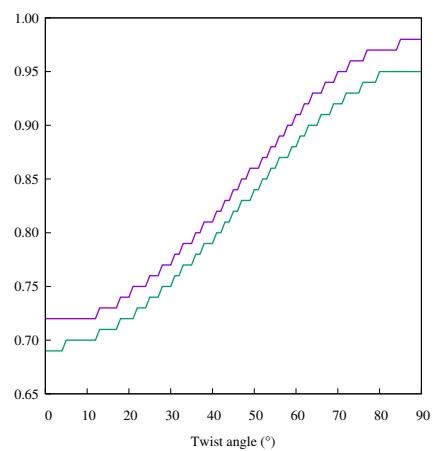

Figure S112: Reference (green) and approached (purple)  $\varphi$  plots for the PP first excited-state computed at the CIS/6-311+G level of theory. The descriptors values are reported with respect to the pyridinium-phenolate twist angle amplitude.

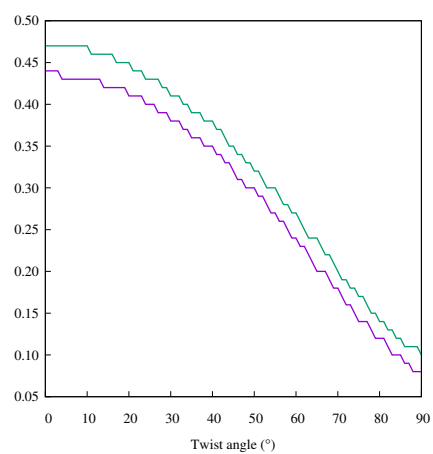

Figure S113: Reference (green) and approached (purple)  $\psi$  plots for the PP first excited-state computed at the CIS/6-311+G level of theory. The descriptors values are reported with respect to the pyridinium-phenolate twist angle amplitude.

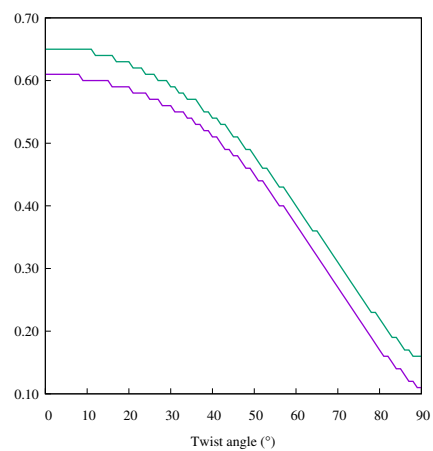

Figure S114: Reference (green) and approached (purple)  $\phi_S$  plots for the PP first excited-state computed at the CIS/6-311G level of theory. The descriptors values are reported with respect to the pyridinium-phenolate twist angle amplitude.

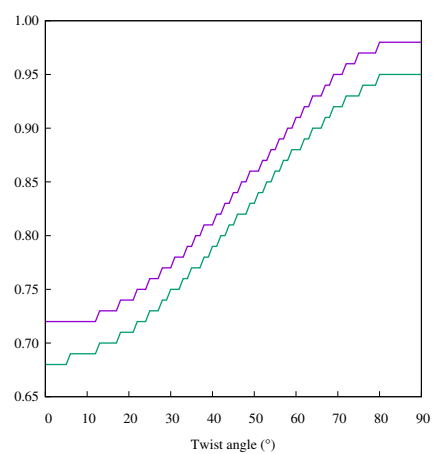

Figure S115: Reference (green) and approached (purple)  $\varphi$  plots for the PP first excited-state computed at the CIS/6-311G level of theory. The descriptors values are reported with respect to the pyridinium-phenolate twist angle amplitude.

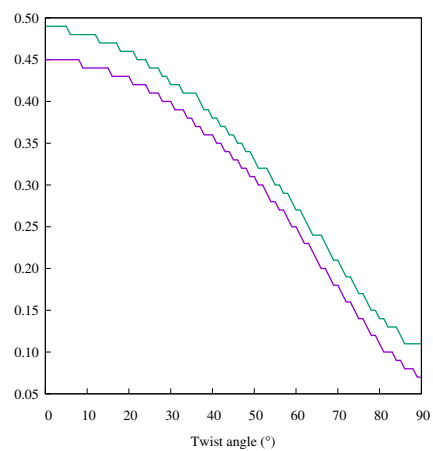

Figure S116: Reference (green) and approached (purple)  $\psi$  plots for the PP first excited-state computed at the CIS/6-311G level of theory. The descriptors values are reported with respect to the pyridinium-phenolate twist angle amplitude.



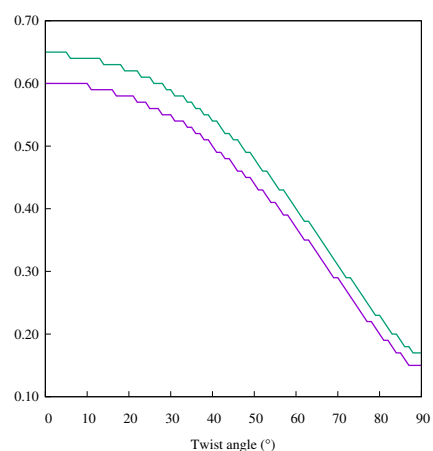

Figure S117: Reference (green) and approached (purple)  $\phi_S$  plots for the PP first excited-state computed at the CIS/6-31++G(2d,p) level of theory. The descriptors values are reported with respect to the pyridinium-phenolate twist angle amplitude.

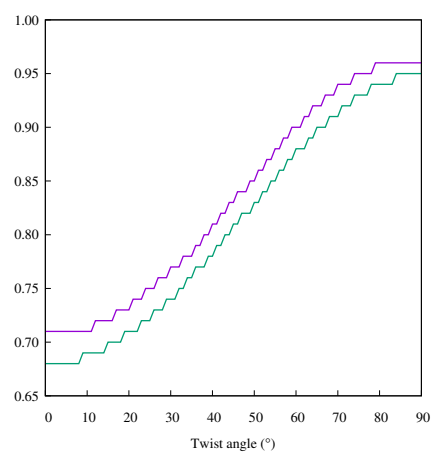

Figure S118: Reference (green) and approached (purple)  $\varphi$  plots for the PP first excited-state computed at the CIS/6-31++G(2d,p) level of theory. The descriptors values are reported with respect to the pyridinium-phenolate twist angle amplitude.

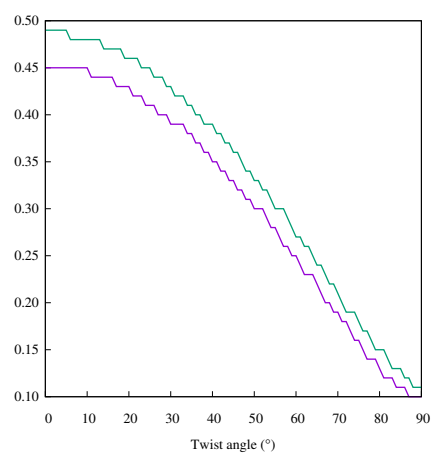

Figure S119: Reference (green) and approached (purple)  $\psi$  plots for the PP first excited-state computed at the CIS/6-31++G(2d,p) level of theory. The descriptors values are reported with respect to the pyridinium-phenolate twist angle amplitude.

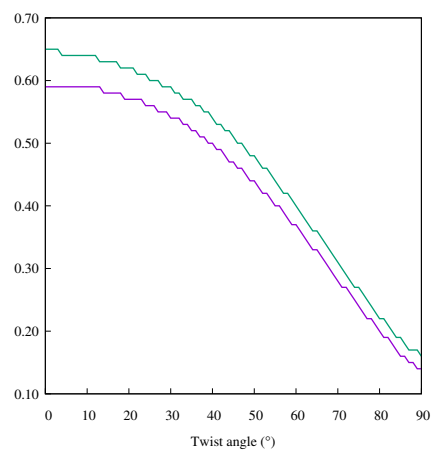

Figure S120: Reference (green) and approached (purple)  $\phi_S$  plots for the PP first excited-state computed at the CIS/6-31+G(d) level of theory. The descriptors values are reported with respect to the pyridinium-phenolate twist angle amplitude.

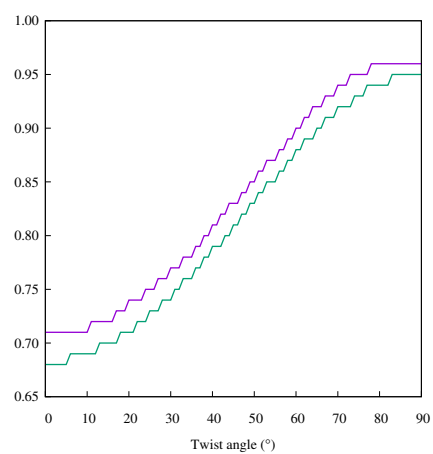

Figure S121: Reference (green) and approached (purple)  $\varphi$  plots for the PP first excited-state computed at the CIS/6-31+G(d) level of theory. The descriptors values are reported with respect to the pyridinium-phenolate twist angle amplitude.

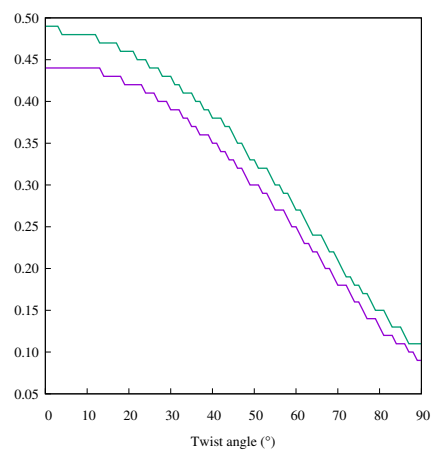

Figure S122: Reference (green) and approached (purple)  $\psi$  plots for the PP first excited-state computed at the CIS/6-31+G(d) level of theory. The descriptors values are reported with respect to the pyridinium-phenolate twist angle amplitude.

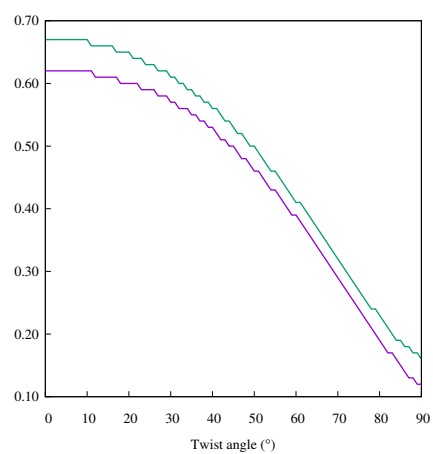

Figure S123: Reference (green) and approached (purple)  $\phi_S$  plots for the PP first excited-state computed at the CIS/6-31G(d) level of theory. The descriptors values are reported with respect to the pyridinium-phenolate twist angle amplitude.

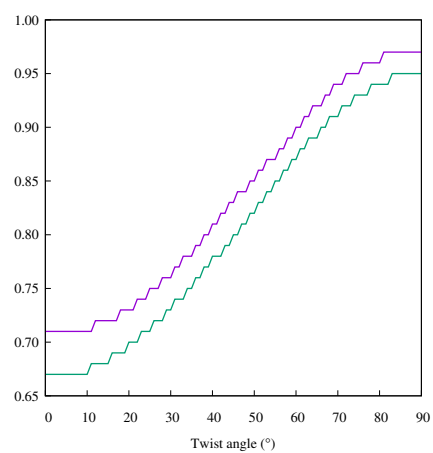

Figure S124: Reference (green) and approached (purple)  $\varphi$  plots for the PP first excited-state computed at the CIS/6-31G(d) level of theory. The descriptors values are reported with respect to the pyridinium-phenolate twist angle amplitude.

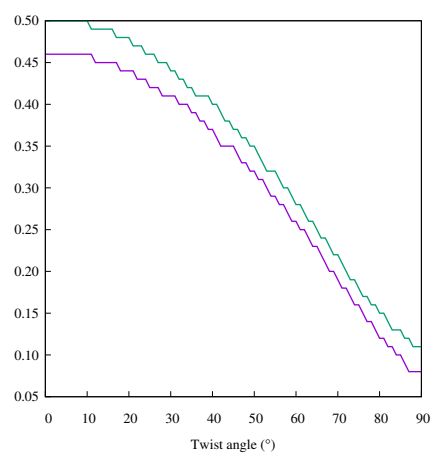

Figure S125: Reference (green) and approached (purple)  $\psi$  plots for the PP first excited-state computed at the CIS/6-31Gd level of theory. The descriptors values are reported with respect to the pyridinium-phenolate twist angle amplitude.

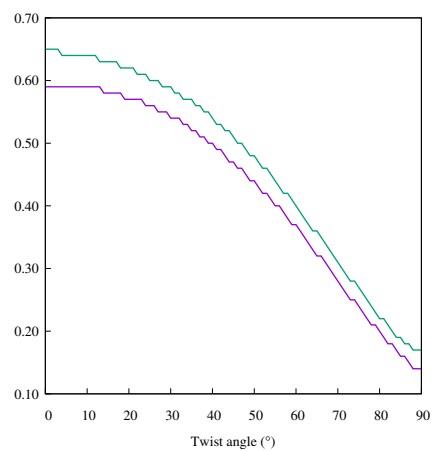

Figure S126: Reference (green) and approached (purple)  $\phi_S$  plots for the PP first excited-state computed at the CIS/6-31++G(d,p) level of theory. The descriptors values are reported with respect to the pyridinium-phenolate twist angle amplitude.

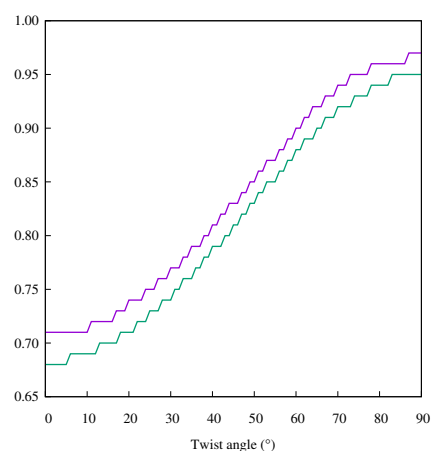

Figure S127: Reference (green) and approached (purple)  $\varphi$  plots for the PP first excited-state computed at the CIS/6-31++G(d,p) level of theory. The descriptors values are reported with respect to the pyridinium-phenolate twist angle amplitude.

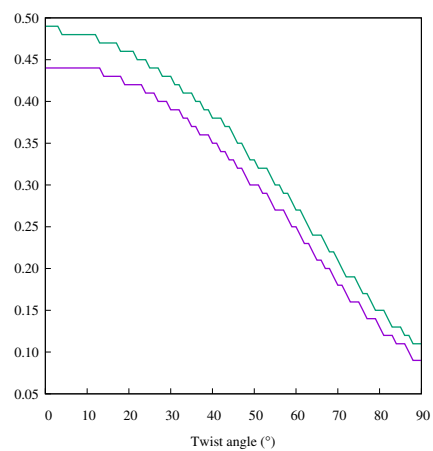

Figure S128: Reference (green) and approached (purple)  $\psi$  plots for the PP first excited-state computed at the CIS/6-31++G(d,p) level of theory. The descriptors values are reported with respect to the pyridinium-phenolate twist angle amplitude.

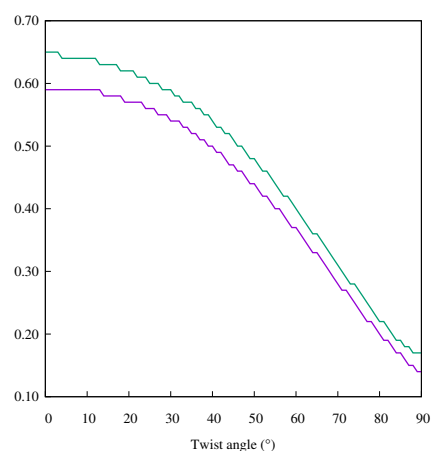

Figure S129: Reference (green) and approached (purple)  $\phi_S$  plots for the PP first excited-state computed at the CIS/6-31+G(d,p) level of theory. The descriptors values are reported with respect to the pyridinium-phenolate twist angle amplitude.

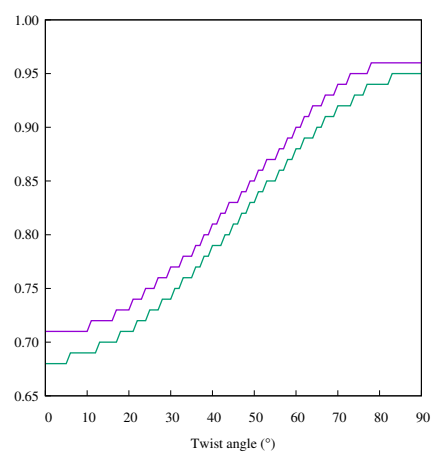

Figure S130: Reference (green) and approached (purple)  $\varphi$  plots for the PP first excited-state computed at the CIS/6-31+G(d,p) level of theory. The descriptors values are reported with respect to the pyridinium-phenolate twist angle amplitude.

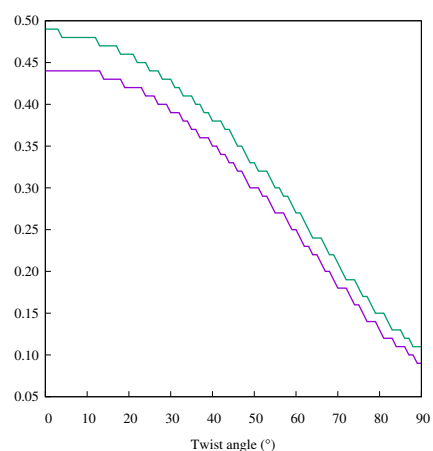

Figure S131: Reference (green) and approached (purple)  $\psi$  plots for the PP first excited-state computed at the CIS/6-31+G(d,p) level of theory. The descriptors values are reported with respect to the pyridinium-phenolate twist angle amplitude.

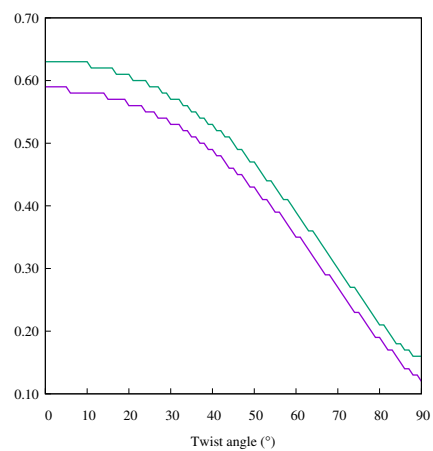

Figure S132: Reference (green) and approached (purple)  $\phi_S$  plots for the PP first excited-state computed at the CIS/6-31+G level of theory. The descriptors values are reported with respect to the pyridinium-phenolate twist angle amplitude.



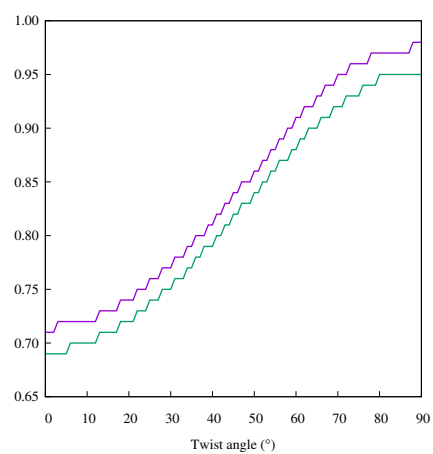

Figure S133: Reference (green) and approached (purple)  $\varphi$  plots for the PP first excited-state computed at the CIS/6-31+G level of theory. The descriptors values are reported with respect to the pyridinium-phenolate twist angle amplitude.

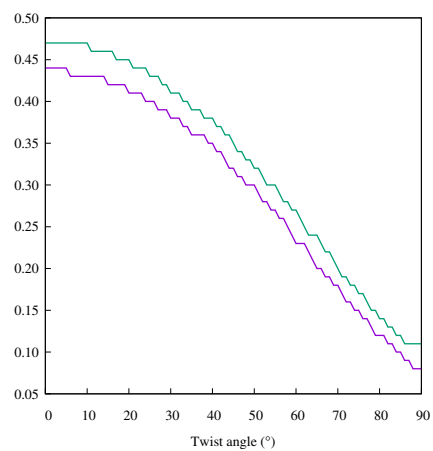

Figure S134: Reference (green) and approached (purple)  $\psi$  plots for the PP first excited-state computed at the CIS/6-31+G level of theory. The descriptors values are reported with respect to the pyridinium-phenolate twist angle amplitude.

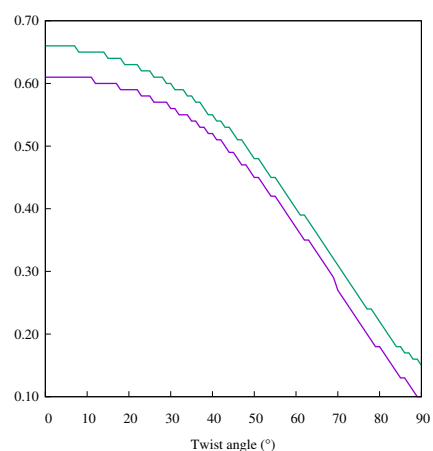

Figure S135: Reference (green) and approached (purple)  $\phi_S$  plots for the PP first excited-state computed at the CIS/6-31G level of theory. The descriptors values are reported with respect to the pyridinium-phenolate twist angle amplitude.

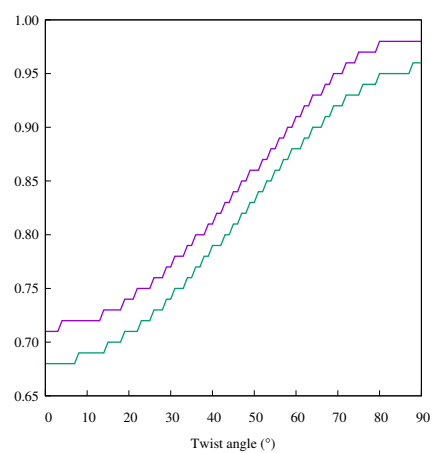

Figure S136: Reference (green) and approached (purple)  $\varphi$  plots for the PP first excited-state computed at the CIS/6-31G level of theory. The descriptors values are reported with respect to the pyridinium-phenolate twist angle amplitude.

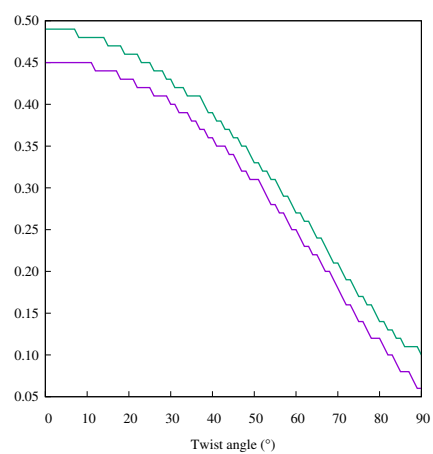

Figure S137: Reference (green) and approached (purple)  $\psi$  plots for the PP first excited-state computed at the CIS/6-31G level of theory. The descriptors values are reported with respect to the pyridinium-phenolate twist angle amplitude.

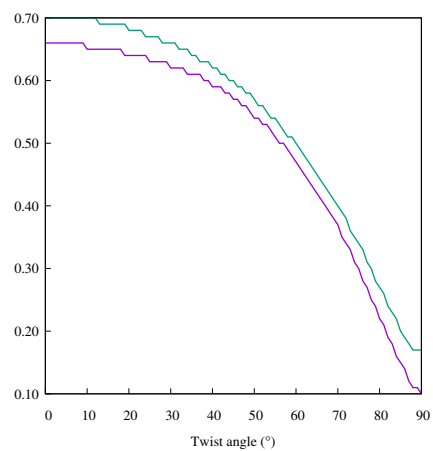

Figure S138: Reference (green) and approached (purple)  $\phi_S$  plots for the PP first excited-state computed at the LC-wHPBE/3-21G level of theory. The descriptors values are reported with respect to the pyridinium-phenolate twist angle amplitude.

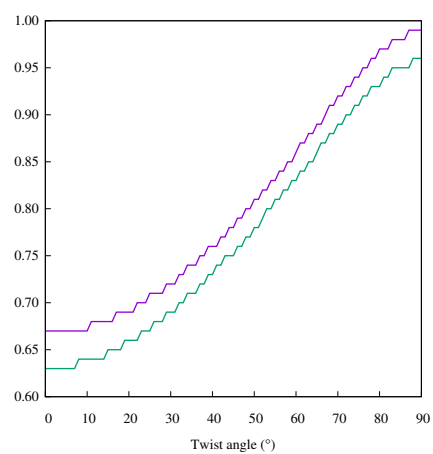

Figure S139: Reference (green) and approached (purple)  $\varphi$  plots for the PP first excited-state computed at the LC-wHPBE/3-21G level of theory. The descriptors values are reported with respect to the pyridinium-phenolate twist angle amplitude.

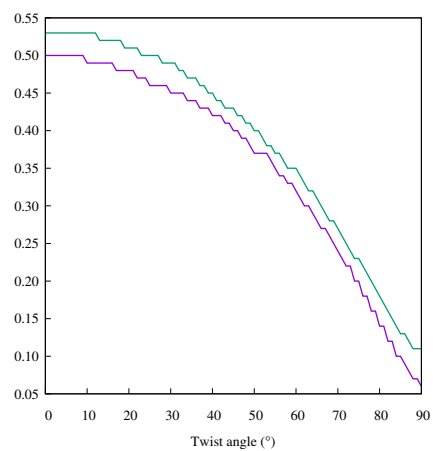

Figure S140: Reference (green) and approached (purple)  $\psi$  plots for the PP first excited-state computed at the LC-wHPBE/3-21G level of theory. The descriptors values are reported with respect to the pyridinium-phenolate twist angle amplitude.

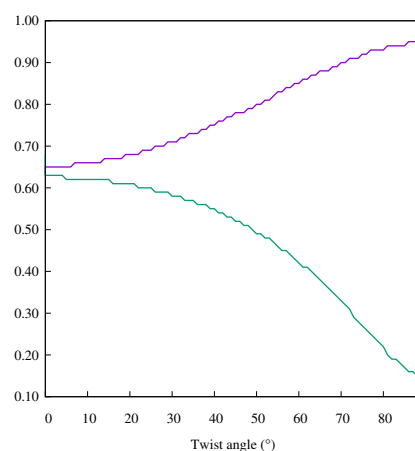

Figure S141: Reference (green) and approached (purple)  $\phi_S$  plots for the PP first excited-state computed at the LC-wHPBE/6-311++G(2d,p) level of theory. The descriptors values are reported with respect to the pyridinium-phenolate twist angle amplitude.

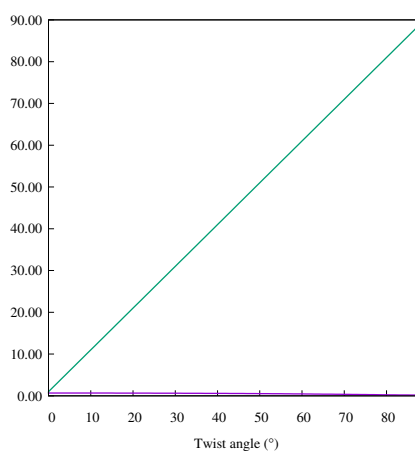

Figure S142: Reference (green) and approached (purple)  $\varphi$  plots for the PP first excited-state computed at the LC-wHPBE/6-311++G(2d,p) level of theory. The descriptors values are reported with respect to the pyridinium-phenolate twist angle amplitude.

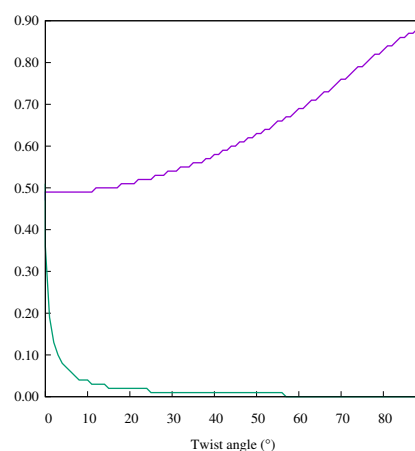

Figure S143: Reference (green) and approached (purple)  $\psi$  plots for the PP first excited-state computed at the LC-wHPBE/6-311++G(2d,p) level of theory. The descriptors values are reported with respect to the pyridinium-phenolate twist angle amplitude.

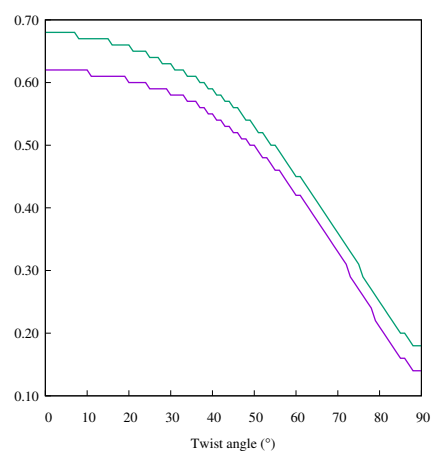

Figure S144: Reference (green) and approached (purple)  $\phi_S$  plots for the PP first excited-state computed at the LC-wHPBE/6-311+G(d) level of theory. The descriptors values are reported with respect to the pyridinium-phenolate twist angle amplitude.

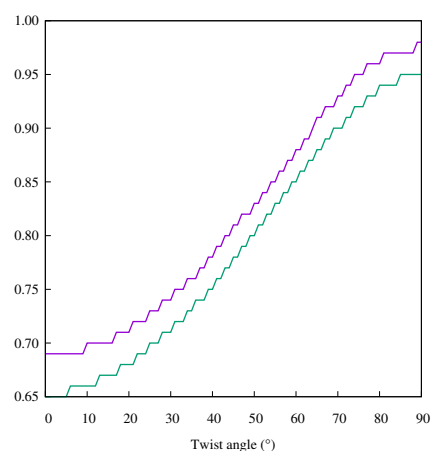

Figure S145: Reference (green) and approached (purple)  $\varphi$  plots for the PP first excited-state computed at the LC-wHPBE/6-311+G(d) level of theory. The descriptors values are reported with respect to the pyridinium-phenolate twist angle amplitude.

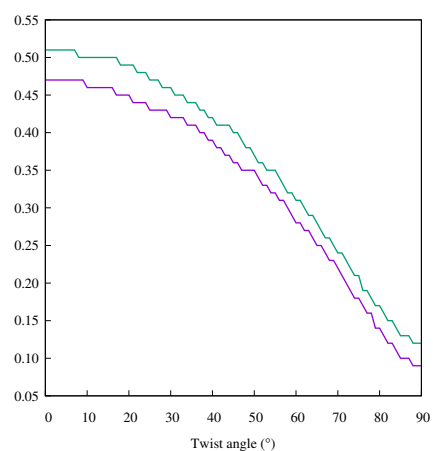

Figure S146: Reference (green) and approached (purple)  $\psi$  plots for the PP first excited-state computed at the LC-wHPBE/6-311+G(d) level of theory. The descriptors values are reported with respect to the pyridinium-phenolate twist angle amplitude.

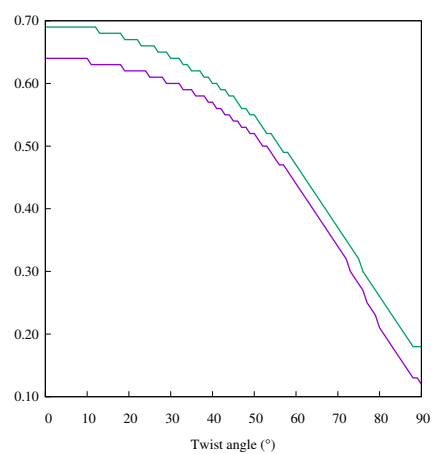

Figure S147: Reference (green) and approached (purple)  $\phi_S$  plots for the PP first excited-state computed at the LC-wHPBE/6-311G(d) level of theory. The descriptors values are reported with respect to the pyridinium-phenolate twist angle amplitude.

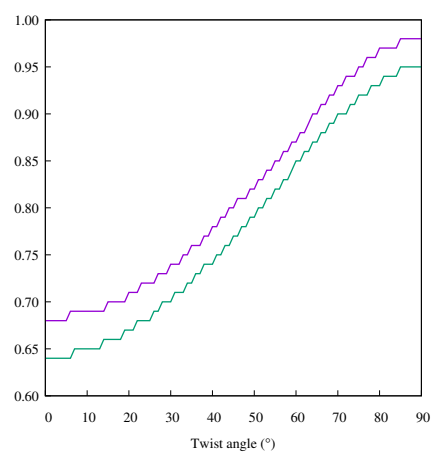

Figure S148: Reference (green) and approached (purple)  $\varphi$  plots for the PP first excited-state computed at the LC-wHPBE/6-311G(d) level of theory. The descriptors values are reported with respect to the pyridinium-phenolate twist angle amplitude.



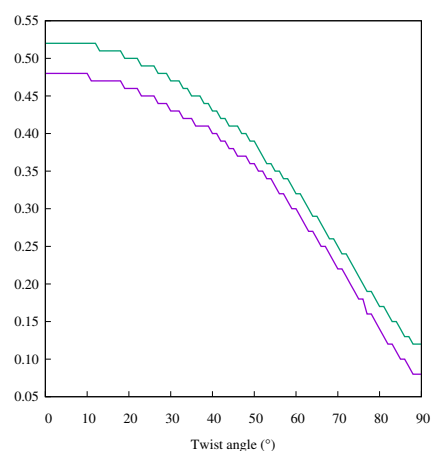

Figure S149: Reference (green) and approached (purple)  $\psi$  plots for the PP first excited-state computed at the LC-wHPBE/6-311G(d) level of theory. The descriptors values are reported with respect to the pyridinium-phenolate twist angle amplitude.

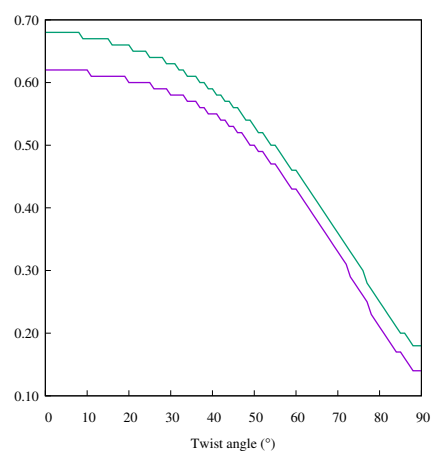

Figure S150: Reference (green) and approached (purple)  $\phi_S$  plots for the PP first excited-state computed at the LC-wHPBE/6-311++G(d,p) level of theory. The descriptors values are reported with respect to the pyridinium-phenolate twist angle amplitude.

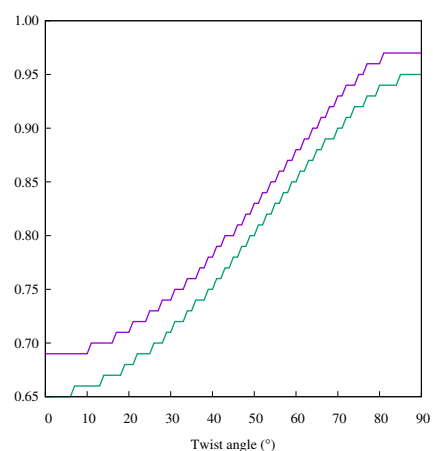

Figure S151: Reference (green) and approached (purple)  $\varphi$  plots for the PP first excited-state computed at the LC-wHPBE/6-311++G(d,p) level of theory. The descriptors values are reported with respect to the pyridinium-phenolate twist angle amplitude.

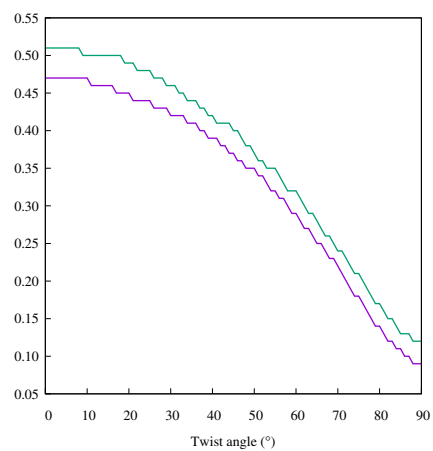

Figure S152: Reference (green) and approached (purple)  $\psi$  plots for the PP first excited-state computed at the LC-wHPBE/6-311++G(d,p) level of theory. The descriptors values are reported with respect to the pyridinium-phenolate twist angle amplitude.

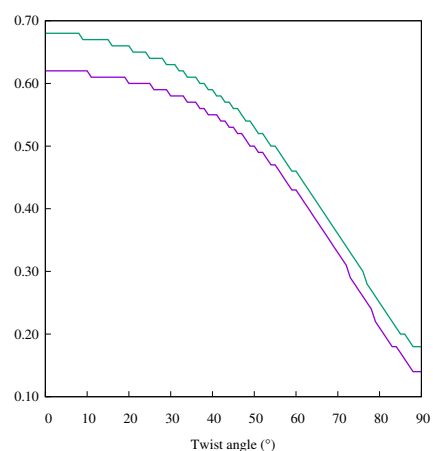

Figure S153: Reference (green) and approached (purple)  $\phi_S$  plots for the PP first excited-state computed at the LC-wHPBE/6-311+G(d,p) level of theory. The descriptors values are reported with respect to the pyridinium-phenolate twist angle amplitude.

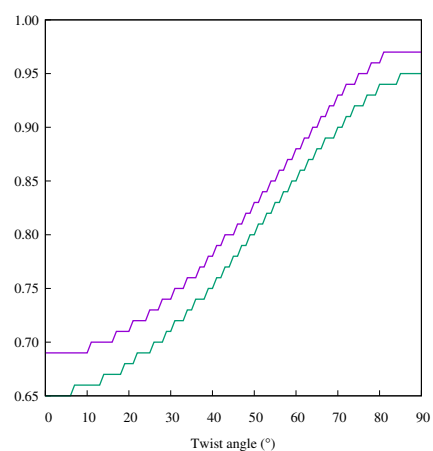

Figure S154: Reference (green) and approached (purple)  $\phi$  plots for the PP first excited-state computed at the LC-wHPBE/6-311+G(d,p) level of theory. The descriptors values are reported with respect to the pyridinium-phenolate twist angle amplitude.

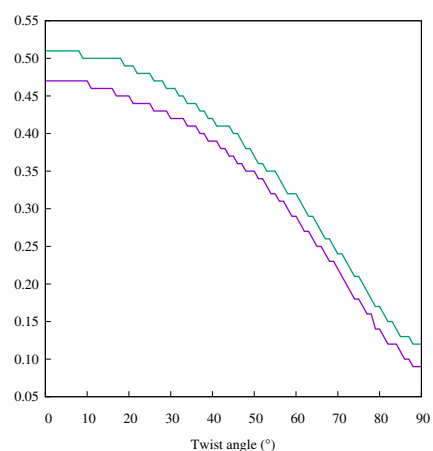

Figure S155: Reference (green) and approached (purple)  $\psi$  plots for the PP first excited-state computed at the LC-wHPBE/6-311+G(d,p) level of theory. The descriptors values are reported with respect to the pyridinium-phenolate twist angle amplitude.

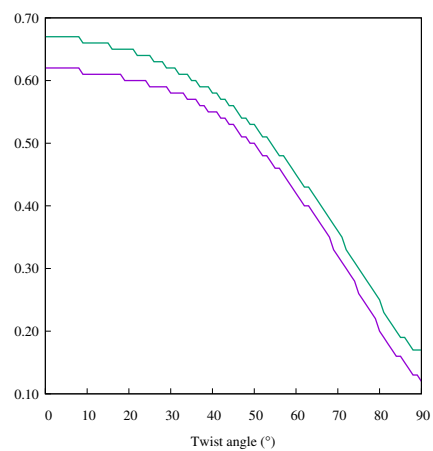

Figure S156: Reference (green) and approached (purple)  $\phi_S$  plots for the PP first excited-state computed at the LC-wHPBE/6-311+G level of theory. The descriptors values are reported with respect to the pyridinium-phenolate twist angle amplitude.

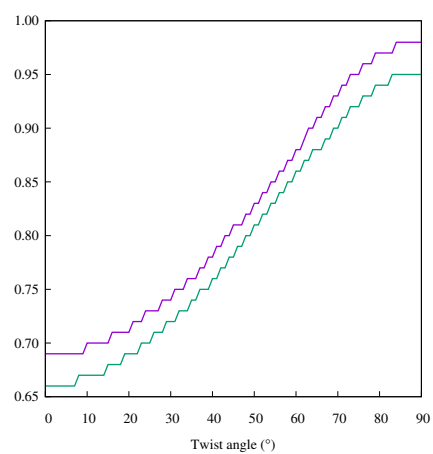

Figure S157: Reference (green) and approached (purple)  $\varphi$  plots for the PP first excited-state computed at the LC-wHPBE/6-311+G level of theory. The descriptors values are reported with respect to the pyridinium-phenolate twist angle amplitude.

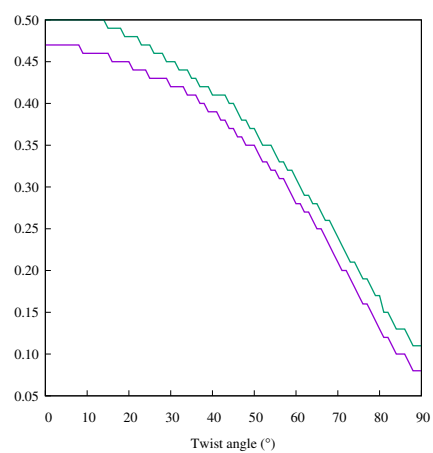

Figure S158: Reference (green) and approached (purple)  $\psi$  plots for the PP first excited-state computed at the LC-wHPBE/6-311+G level of theory. The descriptors values are reported with respect to the pyridinium-phenolate twist angle amplitude.

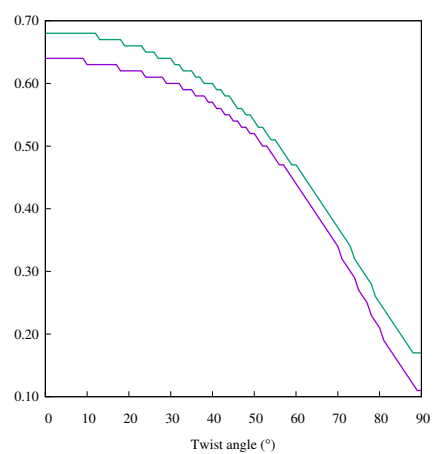

Figure S159: Reference (green) and approached (purple)  $\phi_S$  plots for the PP first excited-state computed at the LC-wHPBE/6-311G level of theory. The descriptors values are reported with respect to the pyridinium-phenolate twist angle amplitude.

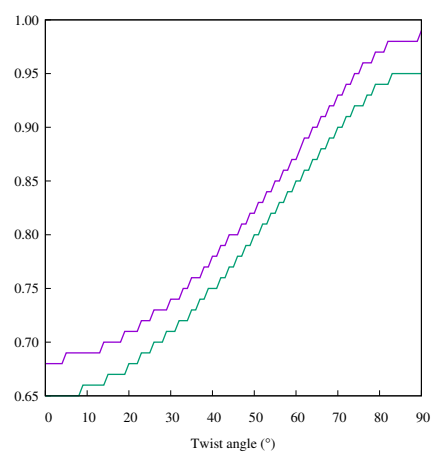

Figure S160: Reference (green) and approached (purple)  $\varphi$  plots for the PP first excited-state computed at the LC-wHPBE/6-311G level of theory. The descriptors values are reported with respect to the pyridinium-phenolate twist angle amplitude.

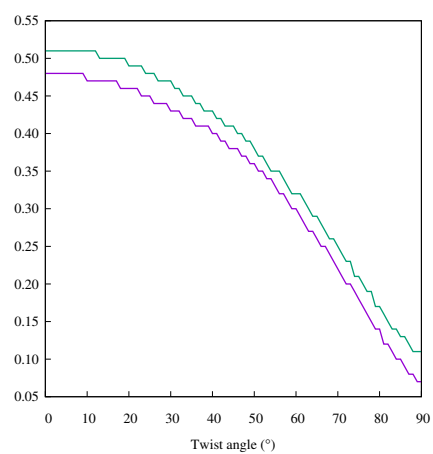

Figure S161: Reference (green) and approached (purple)  $\psi$  plots for the PP first excited-state computed at the LC-wHPBE/6-311G level of theory. The descriptors values are reported with respect to the pyridinium-phenolate twist angle amplitude.

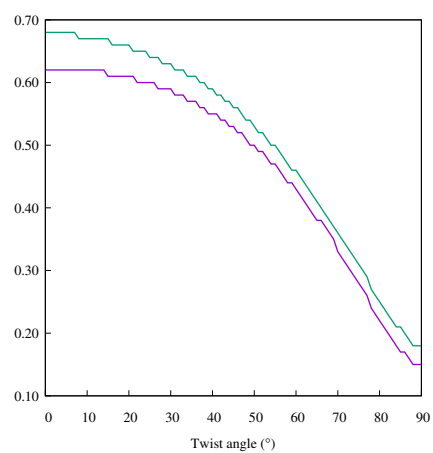

Figure S162: Reference (green) and approached (purple)  $\phi_S$  plots for the PP first excited-state computed at the LC-wHPBE/6-31++G(2d,p) level of theory. The descriptors values are reported with respect to the pyridinium-phenolate twist angle amplitude.

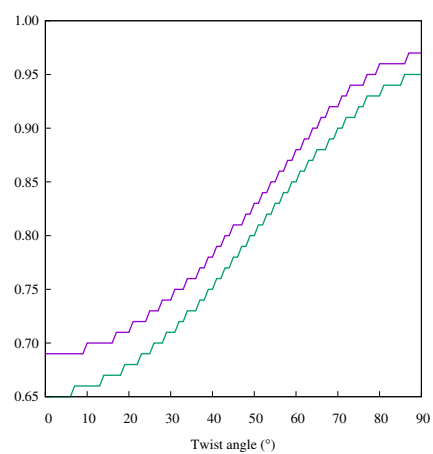

Figure S163: Reference (green) and approached (purple)  $\varphi$  plots for the PP first excited-state computed at the LC-wHPBE/6-31++G(2d,p) level of theory. The descriptors values are reported with respect to the pyridinium-phenolate twist angle amplitude.

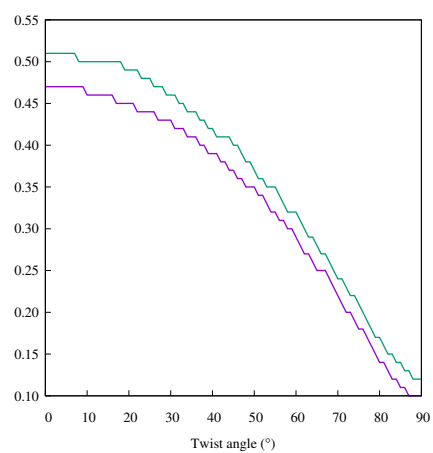

Figure S164: Reference (green) and approached (purple)  $\psi$  plots for the PP first excited-state computed at the LC-wHPBE/6-31++G(2d,p) level of theory. The descriptors values are reported with respect to the pyridinium-phenolate twist angle amplitude.



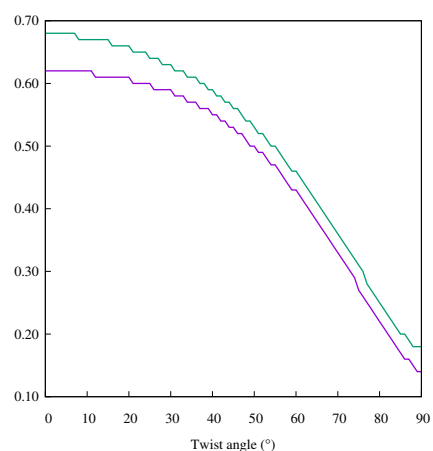

Figure S165: Reference (green) and approached (purple)  $\phi_S$  plots for the PP first excited-state computed at the LC-wHPBE/6-31+G(d) level of theory. The descriptors values are reported with respect to the pyridinium-phenolate twist angle amplitude.

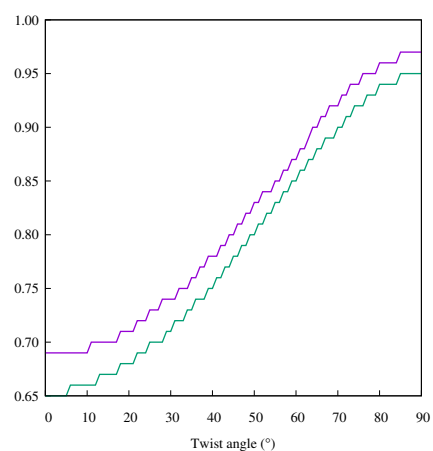

Figure S166: Reference (green) and approached (purple)  $\varphi$  plots for the PP first excited-state computed at the LC-wHPBE/6-31+G(d) level of theory. The descriptors values are reported with respect to the pyridinium-phenolate twist angle amplitude.

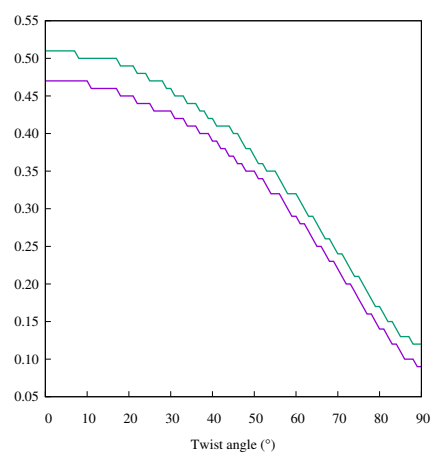

Figure S167: Reference (green) and approached (purple)  $\psi$  plots for the PP first excited-state computed at the LC-wHPBE/6-31+G(d) level of theory. The descriptors values are reported with respect to the pyridinium-phenolate twist angle amplitude.

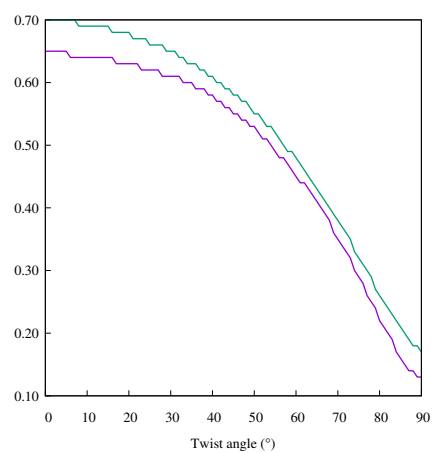

Figure S168: Reference (green) and approached (purple)  $\phi_S$  plots for the PP first excited-state computed at the LC-wHPBE/6-31G(d) level of theory. The descriptors values are reported with respect to the pyridinium-phenolate twist angle amplitude.

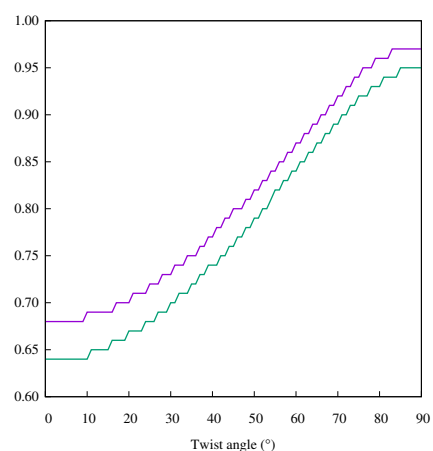

Figure S169: Reference (green) and approached (purple)  $\varphi$  plots for the PP first excited-state computed at the LC-wHPBE/6-31G(d) level of theory. The descriptors values are reported with respect to the pyridinium-phenolate twist angle amplitude.

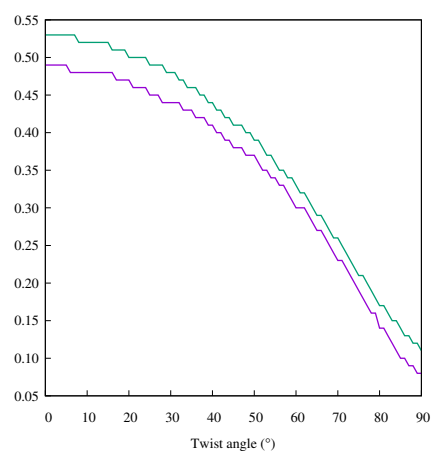

Figure S170: Reference (green) and approached (purple)  $\psi$  plots for the PP first excited-state computed at the LC-wHPBE/6-31G(d) level of theory. The descriptors values are reported with respect to the pyridinium-phenolate twist angle amplitude.

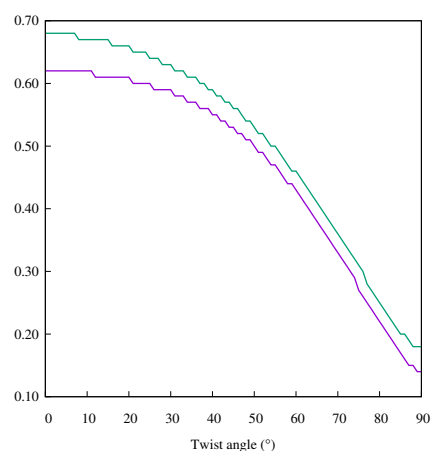

Figure S171: Reference (green) and approached (purple)  $\phi_S$  plots for the PP first excited-state computed at the LC-wHPBE/6-31++G(d,p) level of theory. The descriptors values are reported with respect to the pyridinium-phenolate twist angle amplitude.

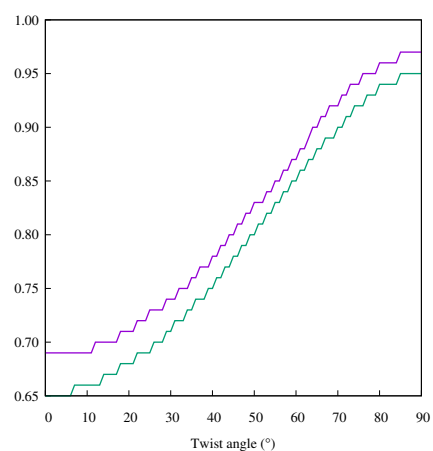

Figure S172: Reference (green) and approached (purple)  $\phi$  plots for the PP first excited-state computed at the LC-wHPBE/6-31++G(d,p) level of theory. The descriptors values are reported with respect to the pyridinium-phenolate twist angle amplitude.

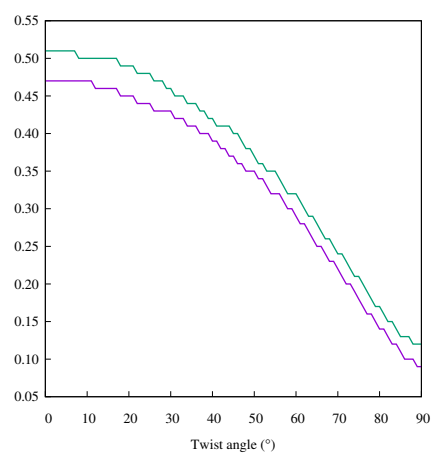

Figure S173: Reference (green) and approached (purple)  $\psi$  plots for the PP first excited-state computed at the LC-wHPBE/6-31++G(d,p) level of theory. The descriptors values are reported with respect to the pyridinium-phenolate twist angle amplitude.

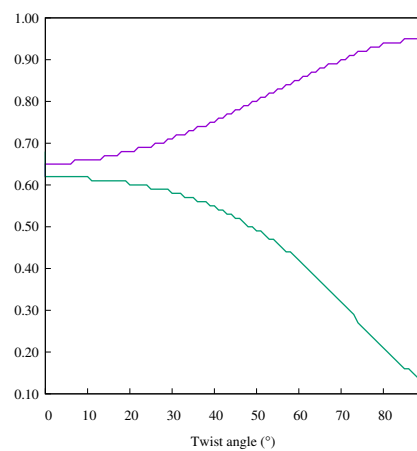

Figure S174: Reference (green) and approached (purple)  $\phi_S$  plots for the PP first excited-state computed at the LC-wHPBE/6-31+G(d,p) level of theory. The descriptors values are reported with respect to the pyridinium-phenolate twist angle amplitude.

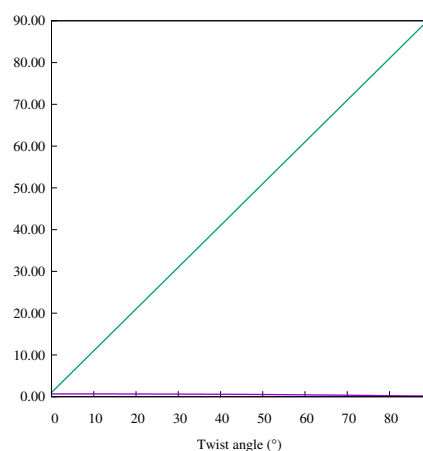

Figure S175: Reference (green) and approached (purple)  $\varphi$  plots for the PP first excited-state computed at the LC-wHPBE/6-31+G(d,p) level of theory. The descriptors values are reported with respect to the pyridinium-phenolate twist angle amplitude.

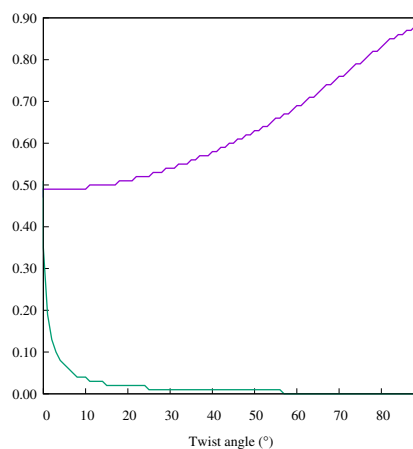

Figure S176: Reference (green) and approached (purple)  $\psi$  plots for the PP first excited-state computed at the LC-wHPBE/6-31+G(d,p) level of theory. The descriptors values are reported with respect to the pyridinium-phenolate twist angle amplitude.

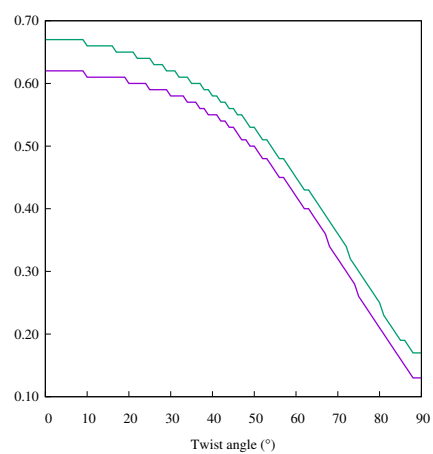

Figure S177: Reference (green) and approached (purple)  $\phi_S$  plots for the PP first excited-state computed at the LC-wHPBE/6-31+G level of theory. The descriptors values are reported with respect to the pyridinium-phenolate twist angle amplitude.

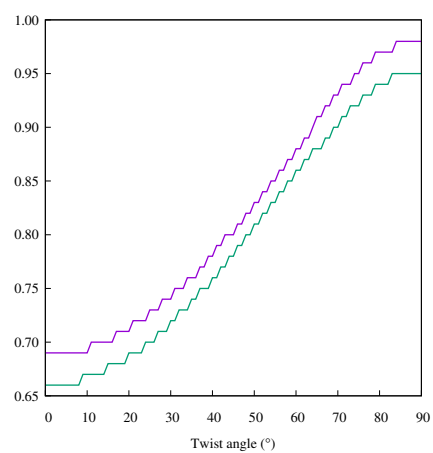

Figure S178: Reference (green) and approached (purple)  $\varphi$  plots for the PP first excited-state computed at the LC-wHPBE/6-31+G level of theory. The descriptors values are reported with respect to the pyridinium-phenolate twist angle amplitude.

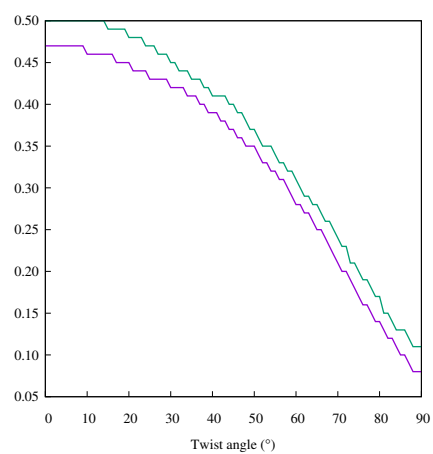

Figure S179: Reference (green) and approached (purple)  $\psi$  plots for the PP first excited-state computed at the LC-wHPBE/6-31+G level of theory. The descriptors values are reported with respect to the pyridinium-phenolate twist angle amplitude.

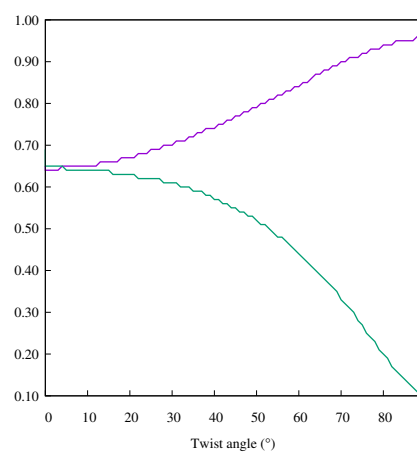

Figure S180: Reference (green) and approached (purple)  $\phi_S$  plots for the PP first excited-state computed at the LC-wHPBE/6-31G level of theory. The descriptors values are reported with respect to the pyridinium-phenolate twist angle amplitude.



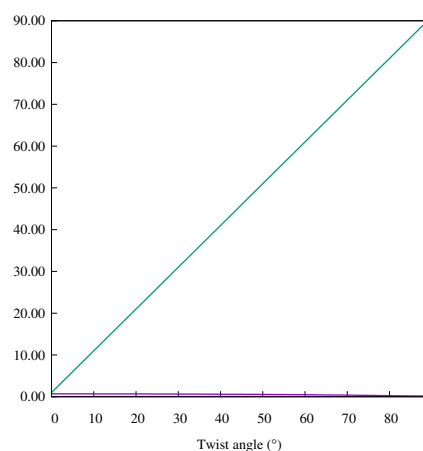

Figure S181: Reference (green) and approached (purple)  $\varphi$  plots for the PP first excited-state computed at the LC-wHPBE/6-31G level of theory. The descriptors values are reported with respect to the pyridinium-phenolate twist angle amplitude.

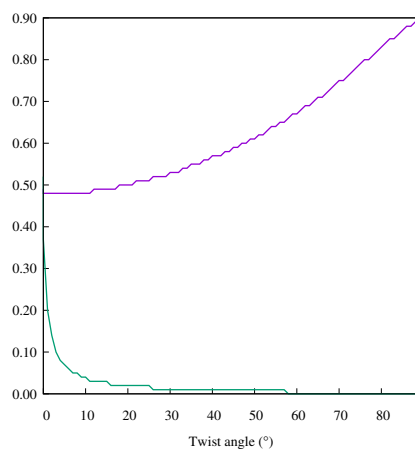

Figure S182: Reference (green) and approached (purple)  $\psi$  plots for the PP first excited-state computed at the LC-wHPBE/6-31G level of theory. The descriptors values are reported with respect to the pyridinium-phenolate twist angle amplitude.

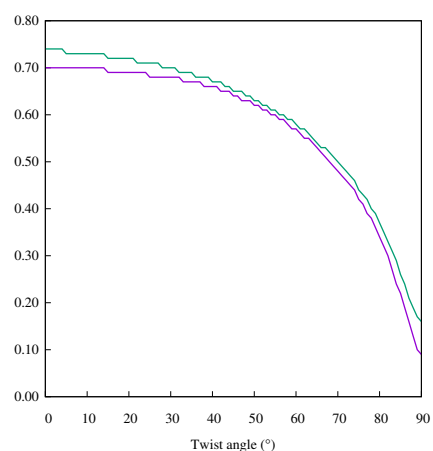

Figure S183: Reference (green) and approached (purple)  $\phi_S$  plots for the PP first excited-state computed at the M062X/3-21G level of theory. The descriptors values are reported with respect to the pyridinium-phenolate twist angle amplitude.

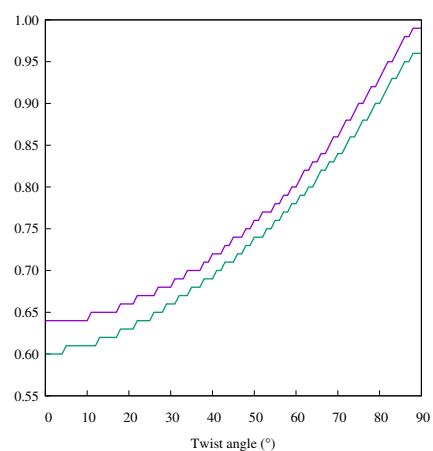

Figure S184: Reference (green) and approached (purple)  $\varphi$  plots for the PP first excited-state computed at the M062X/3-21G level of theory. The descriptors values are reported with respect to the pyridinium-phenolate twist angle amplitude.

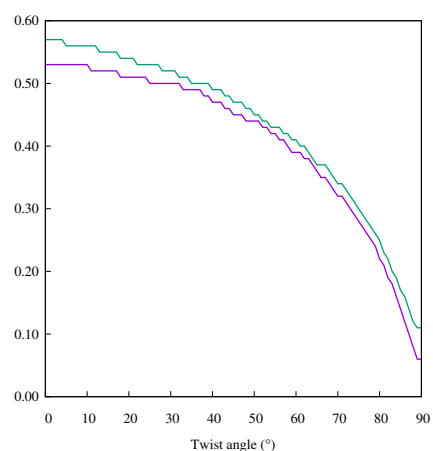

Figure S185: Reference (green) and approached (purple)  $\psi$  plots for the PP first excited-state computed at the M062X/3-21G level of theory. The descriptors values are reported with respect to the pyridinium-phenolate twist angle amplitude.

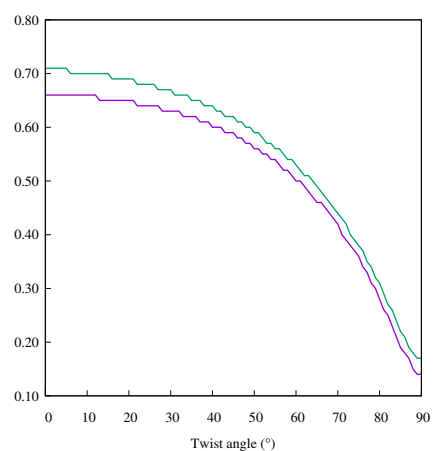

Figure S186: Reference (green) and approached (purple)  $\phi_S$  plots for the PP first excited-state computed at the M062X/6-311++G(2d,p) level of theory. The descriptors values are reported with respect to the pyridinium-phenolate twist angle amplitude.

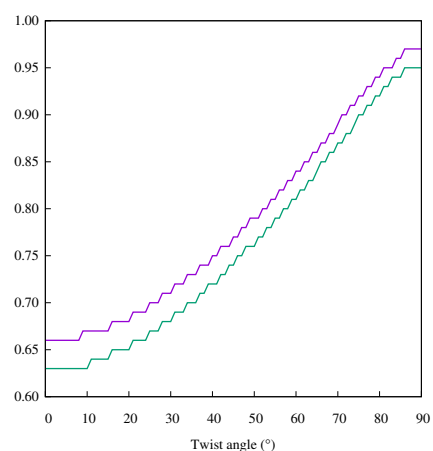

Figure S187: Reference (green) and approached (purple)  $\varphi$  plots for the PP first excited-state computed at the M062X/6-311++G(2d,p) level of theory. The descriptors values are reported with respect to the pyridinium-phenolate twist angle amplitude.

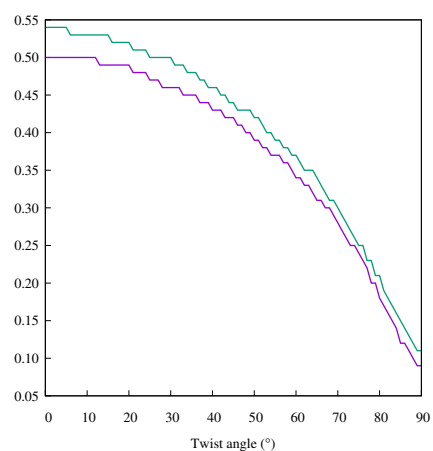

Figure S188: Reference (green) and approached (purple)  $\psi$  plots for the PP first excited-state computed at the M062X/6-311++G(2d,p) level of theory. The descriptors values are reported with respect to the pyridinium-phenolate twist angle amplitude.

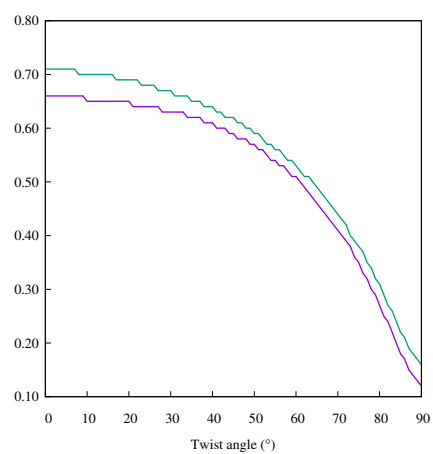

Figure S189: Reference (green) and approached (purple)  $\phi_S$  plots for the PP first excited-state computed at the M062X/6-311+G(d) level of theory. The descriptors values are reported with respect to the pyridinium-phenolate twist angle amplitude.

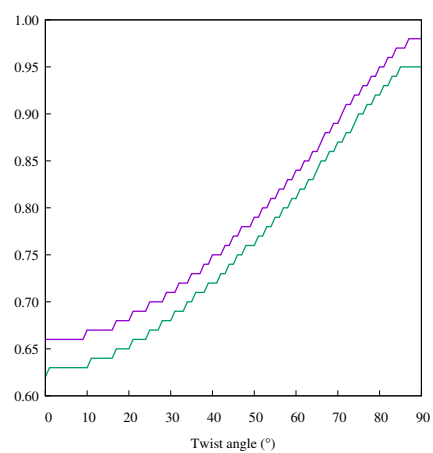

Figure S190: Reference (green) and approached (purple)  $\varphi$  plots for the PP first excited-state computed at the M062X/6-311+G(d) level of theory. The descriptors values are reported with respect to the pyridinium-phenolate twist angle amplitude.

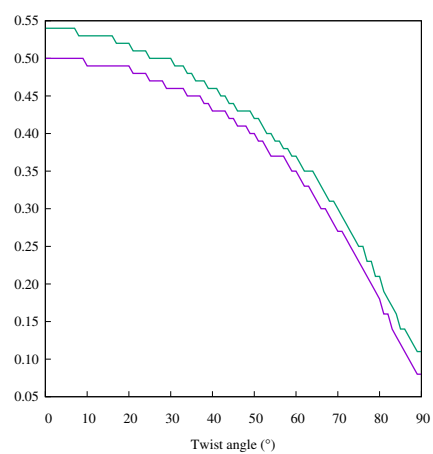

Figure S191: Reference (green) and approached (purple)  $\psi$  plots for the PP first excited-state computed at the M062X/6-311+G(d) level of theory. The descriptors values are reported with respect to the pyridinium-phenolate twist angle amplitude.

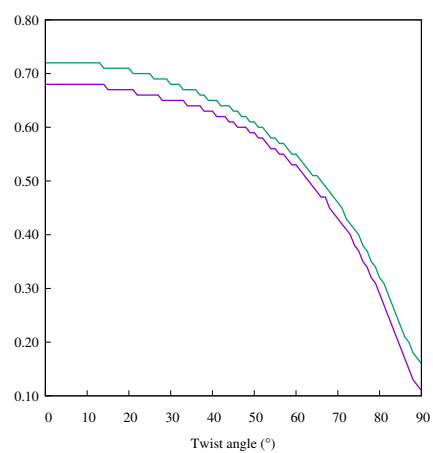

Figure S192: Reference (green) and approached (purple)  $\phi_S$  plots for the PP first excited-state computed at the M062X/6-311G(d) level of theory. The descriptors values are reported with respect to the pyridinium-phenolate twist angle amplitude.

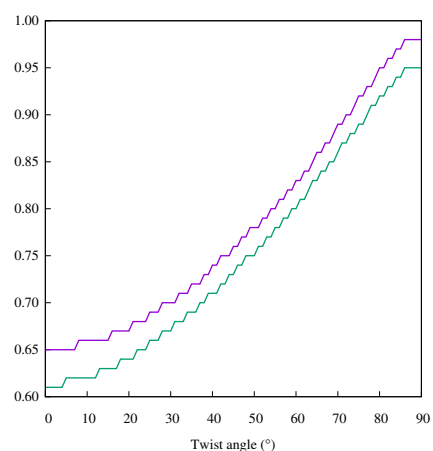

Figure S193: Reference (green) and approached (purple)  $\varphi$  plots for the PP first excited-state computed at the M062X/6-311G(d) level of theory. The descriptors values are reported with respect to the pyridinium-phenolate twist angle amplitude.

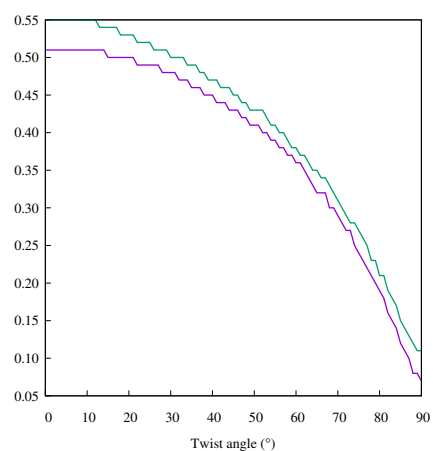

Figure S194: Reference (green) and approached (purple)  $\psi$  plots for the PP first excited-state computed at the M062X/6-311G(d) level of theory. The descriptors values are reported with respect to the pyridinium-phenolate twist angle amplitude.

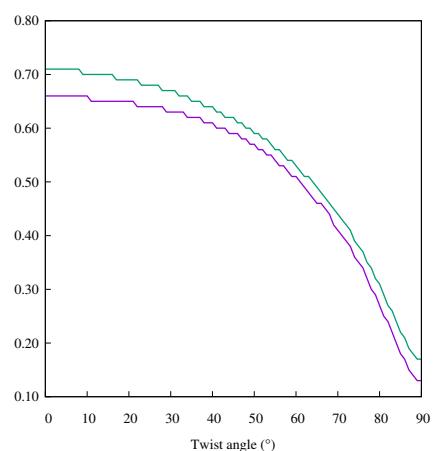

Figure S195: Reference (green) and approached (purple)  $\phi_S$  plots for the PP first excited-state computed at the M062X/6-311++G(d,p) level of theory. The descriptors values are reported with respect to the pyridinium-phenolate twist angle amplitude.

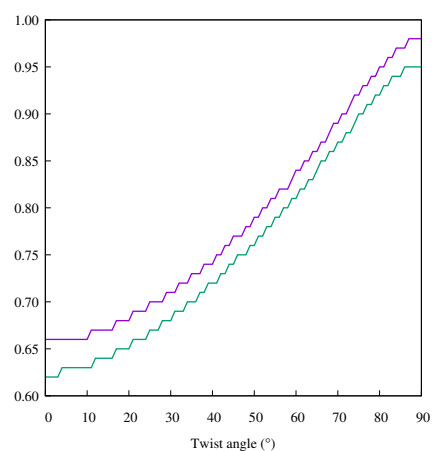

Figure S196: Reference (green) and approached (purple)  $\varphi$  plots for the PP first excited-state computed at the M062X/6-311++G(d,p) level of theory. The descriptors values are reported with respect to the pyridinium-phenolate twist angle amplitude.



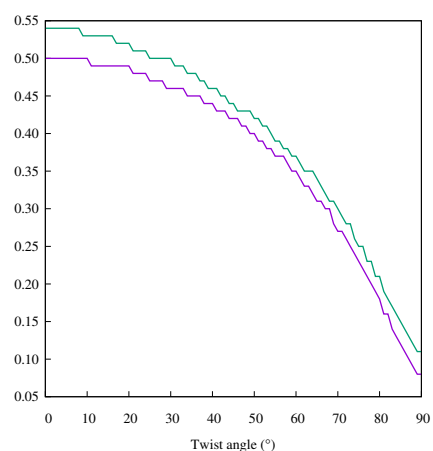

Figure S197: Reference (green) and approached (purple)  $\psi$  plots for the PP first excited-state computed at the M062X/6-311++G(d,p) level of theory. The descriptors values are reported with respect to the pyridinium-phenolate twist angle amplitude.

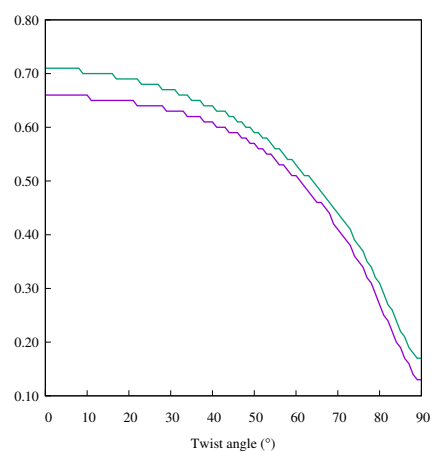

Figure S198: Reference (green) and approached (purple)  $\phi_S$  plots for the PP first excited-state computed at the M062X/6-311+G(d,p) level of theory. The descriptors values are reported with respect to the pyridinium-phenolate twist angle amplitude.

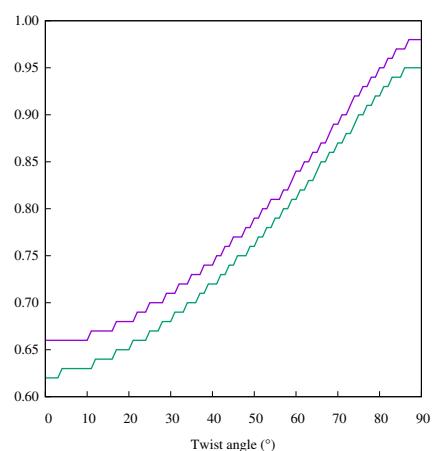

Figure S199: Reference (green) and approached (purple)  $\varphi$  plots for the PP first excited-state computed at the M062X/6-311+G(d,p) level of theory. The descriptors values are reported with respect to the pyridinium-phenolate twist angle amplitude.

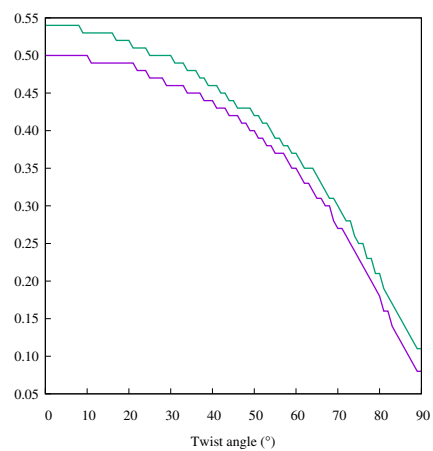

Figure S200: Reference (green) and approached (purple)  $\psi$  plots for the PP first excited-state computed at the M062X/6-311+G(d,p) level of theory. The descriptors values are reported with respect to the pyridinium-phenolate twist angle amplitude.

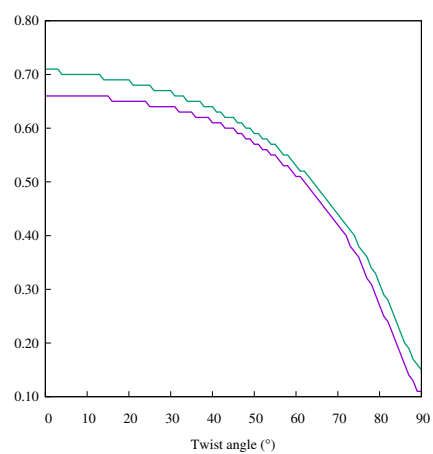

Figure S201: Reference (green) and approached (purple)  $\phi_S$  plots for the PP first excited-state computed at the M062X/6-311+G level of theory. The descriptors values are reported with respect to the pyridinium-phenolate twist angle amplitude.

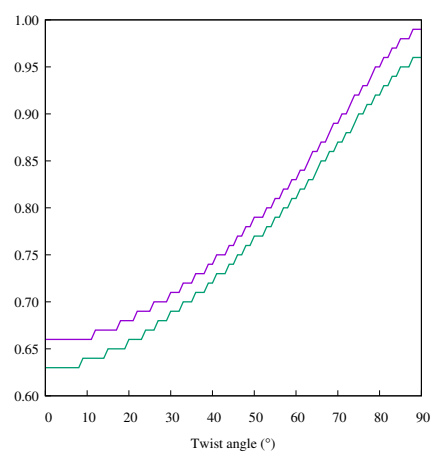

Figure S202: Reference (green) and approached (purple)  $\varphi$  plots for the PP first excited-state computed at the M062X/6-311+G level of theory. The descriptors values are reported with respect to the pyridinium-phenolate twist angle amplitude.

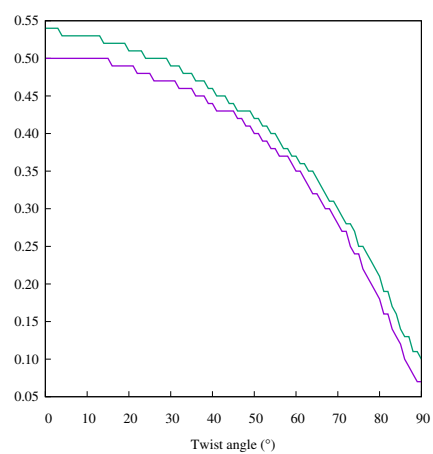

Figure S203: Reference (green) and approached (purple)  $\psi$  plots for the PP first excited-state computed at the M062X/6-311+G level of theory. The descriptors values are reported with respect to the pyridinium-phenolate twist angle amplitude.

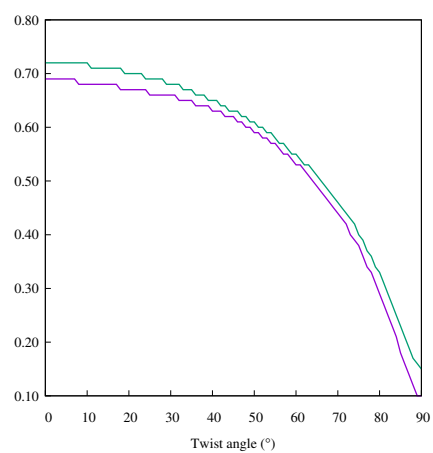

Figure S204: Reference (green) and approached (purple)  $\phi_S$  plots for the PP first excited-state computed at the M062X/6-311G level of theory. The descriptors values are reported with respect to the pyridinium-phenolate twist angle amplitude.

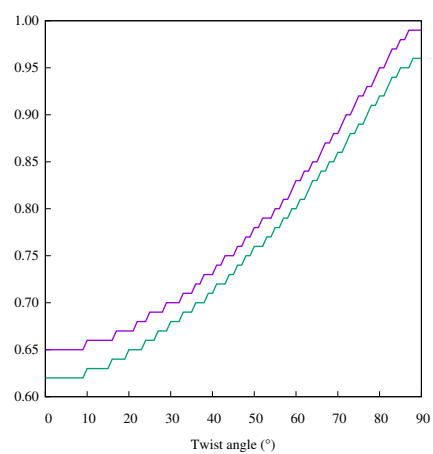

Figure S205: Reference (green) and approached (purple)  $\varphi$  plots for the PP first excited-state computed at the M062X/6-311G level of theory. The descriptors values are reported with respect to the pyridinium-phenolate twist angle amplitude.

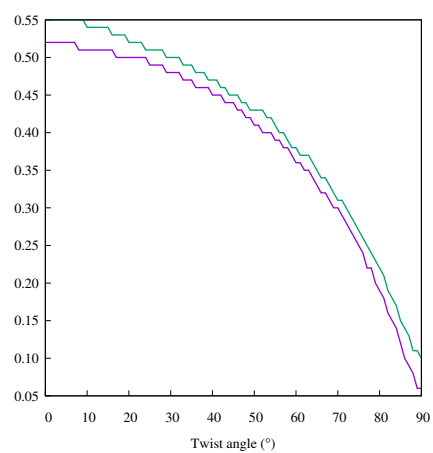

Figure S206: Reference (green) and approached (purple)  $\psi$  plots for the PP first excited-state computed at the M062X/6-311G level of theory. The descriptors values are reported with respect to the pyridinium-phenolate twist angle amplitude.

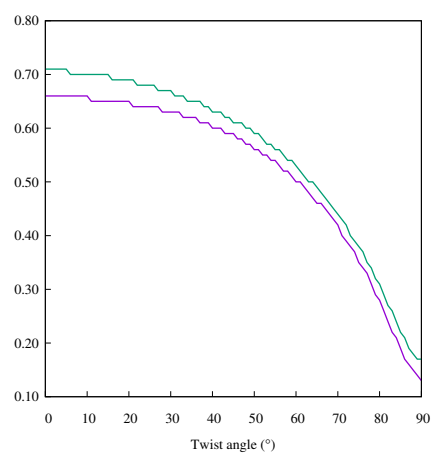

Figure S207: Reference (green) and approached (purple)  $\phi_S$  plots for the PP first excited-state computed at the M062X/6-31++G(2d,p) level of theory. The descriptors values are reported with respect to the pyridinium-phenolate twist angle amplitude.

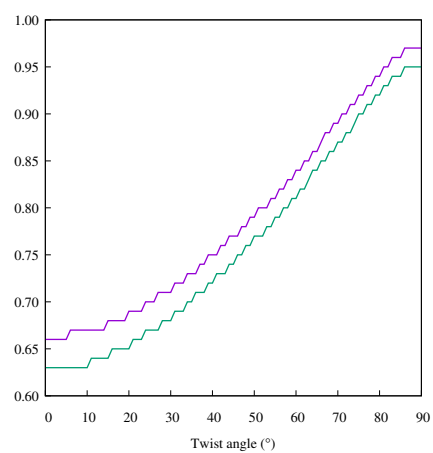

Figure S208: Reference (green) and approached (purple)  $\varphi$  plots for the PP first excited-state computed at the M062X/6-31++G(2d,p) level of theory. The descriptors values are reported with respect to the pyridinium-phenolate twist angle amplitude.

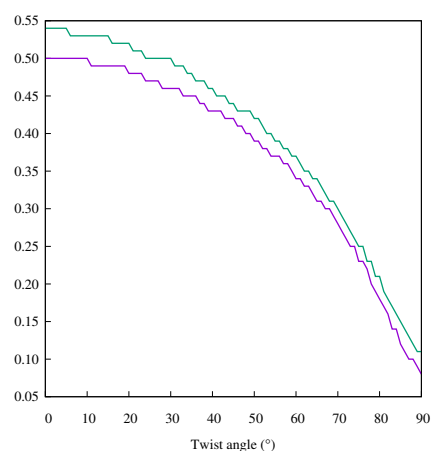

Figure S209: Reference (green) and approached (purple)  $\psi$  plots for the PP first excited-state computed at the M062X/6-31++G(2d,p) level of theory. The descriptors values are reported with respect to the pyridinium-phenolate twist angle amplitude.

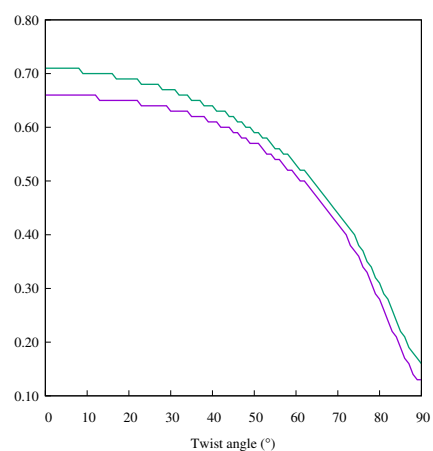

Figure S210: Reference (green) and approached (purple)  $\phi_S$  plots for the PP first excited-state computed at the M062X/6-31+G(d) level of theory. The descriptors values are reported with respect to the pyridinium-phenolate twist angle amplitude.

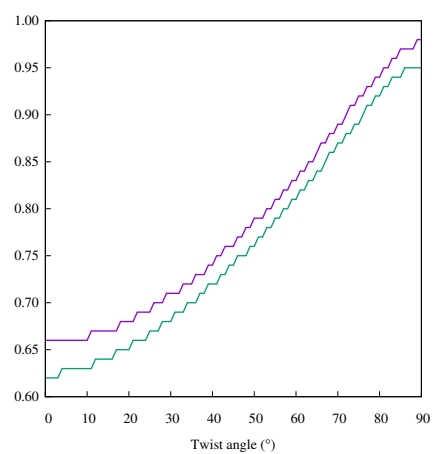

Figure S211: Reference (green) and approached (purple)  $\varphi$  plots for the PP first excited-state computed at the M062X/6-31+G(d) level of theory. The descriptors values are reported with respect to the pyridinium-phenolate twist angle amplitude.

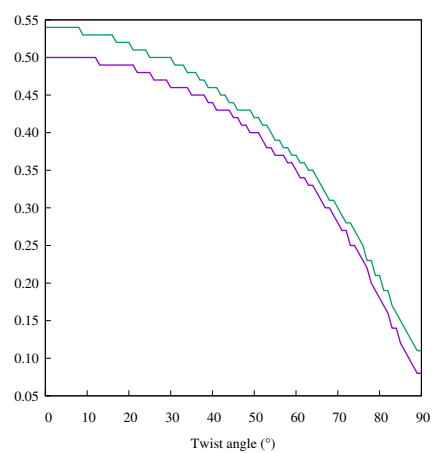

Figure S212: Reference (green) and approached (purple)  $\psi$  plots for the PP first excited-state computed at the M062X/6-31+G(d) level of theory. The descriptors values are reported with respect to the pyridinium-phenolate twist angle amplitude.



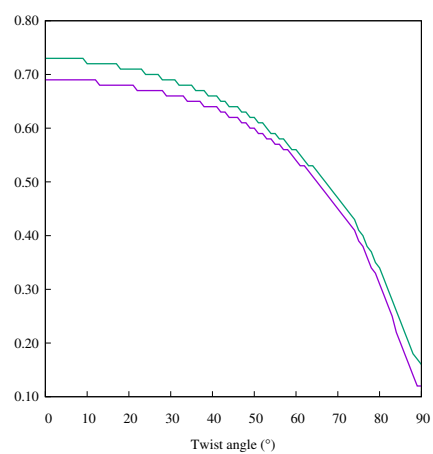

Figure S213: Reference (green) and approached (purple)  $\phi_S$  plots for the PP first excited-state computed at the M062X/6-31G(d) level of theory. The descriptors values are reported with respect to the pyridinium-phenolate twist angle amplitude.

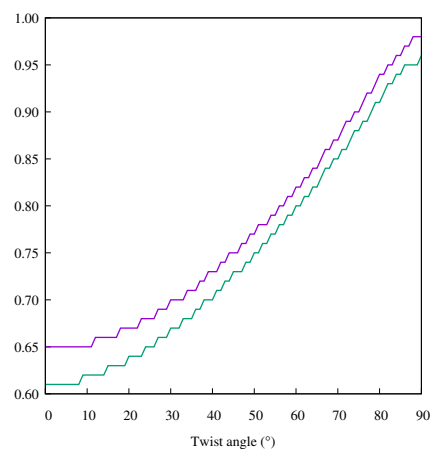

Figure S214: Reference (green) and approached (purple)  $\varphi$  plots for the PP first excited-state computed at the M062X/6-31G(d) level of theory. The descriptors values are reported with respect to the pyridinium-phenolate twist angle amplitude.

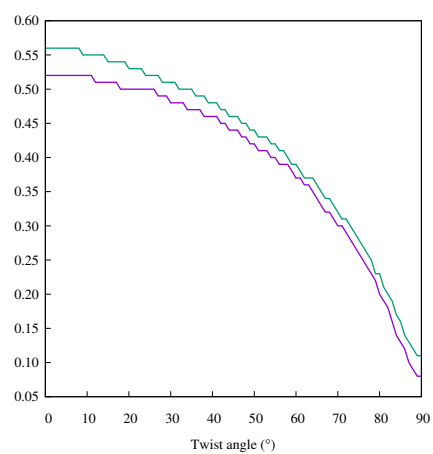

Figure S215: Reference (green) and approached (purple)  $\psi$  plots for the PP first excited-state computed at the M062X/6-31G(d) level of theory. The descriptors values are reported with respect to the pyridinium-phenolate twist angle amplitude.

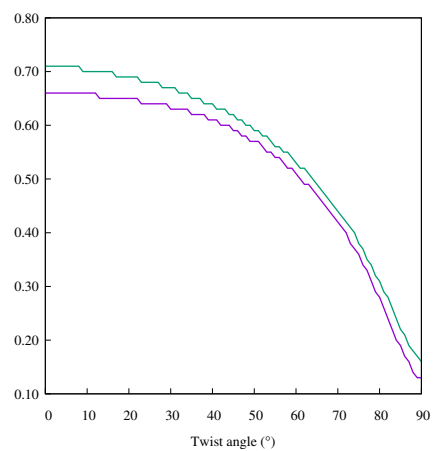

Figure S216: Reference (green) and approached (purple)  $\phi_S$  plots for the PP first excited-state computed at the M062X/6-31++G(d,p) level of theory. The descriptors values are reported with respect to the pyridinium-phenolate twist angle amplitude.

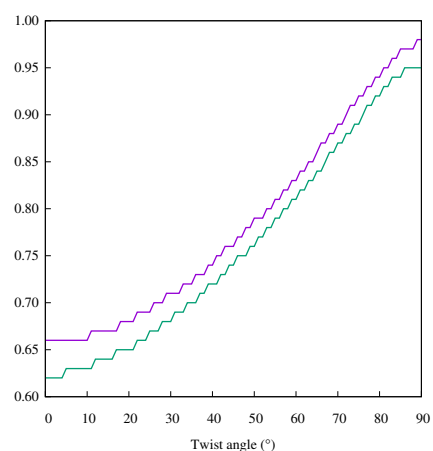

Figure S217: Reference (green) and approached (purple)  $\varphi$  plots for the PP first excited-state computed at the M062X/6-31++G(d,p) level of theory. The descriptors values are reported with respect to the pyridinium-phenolate twist angle amplitude.

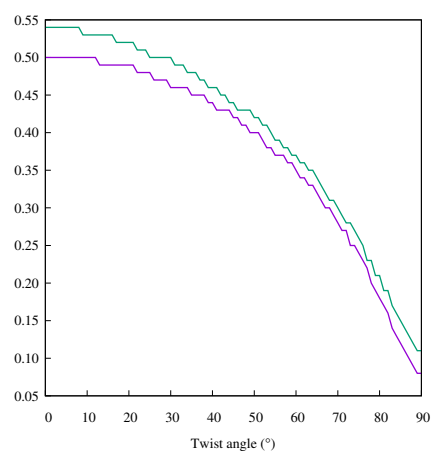

Figure S218: Reference (green) and approached (purple)  $\psi$  plots for the PP first excited-state computed at the M062X/6-31++G(d,p) level of theory. The descriptors values are reported with respect to the pyridinium-phenolate twist angle amplitude.

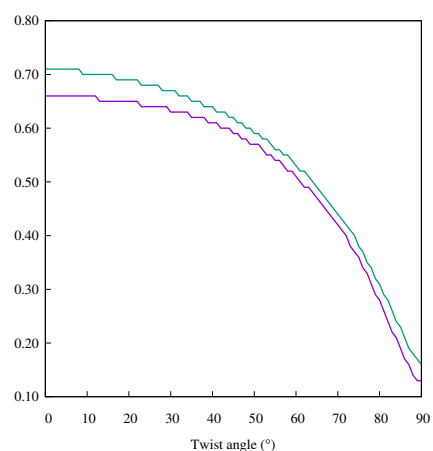

Figure S219: Reference (green) and approached (purple)  $\phi_S$  plots for the PP first excited-state computed at the M062X/6-31+G(d,p) level of theory. The descriptors values are reported with respect to the pyridinium-phenolate twist angle amplitude.

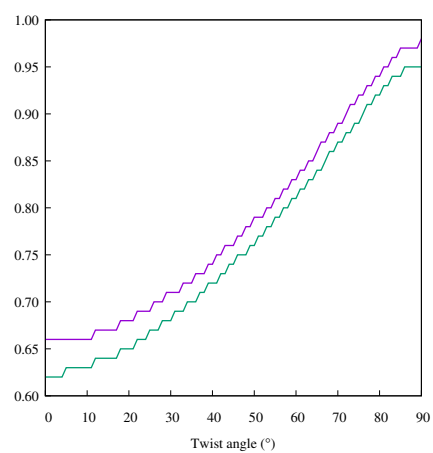

Figure S220: Reference (green) and approached (purple)  $\varphi$  plots for the PP first excited-state computed at the M062X/6-31+G(d,p) level of theory. The descriptors values are reported with respect to the pyridinium-phenolate twist angle amplitude.

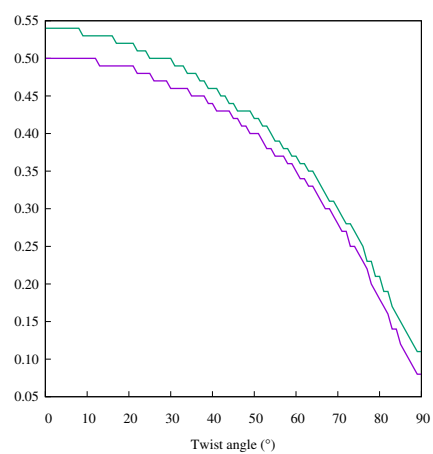

Figure S221: Reference (green) and approached (purple)  $\psi$  plots for the PP first excited-state computed at the M062X/6-31+G(d,p) level of theory. The descriptors values are reported with respect to the pyridinium-phenolate twist angle amplitude.

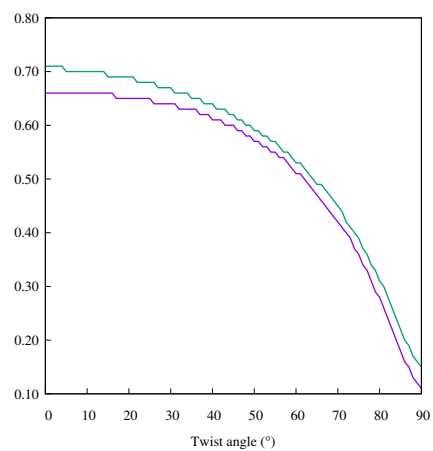

Figure S222: Reference (green) and approached (purple)  $\phi_S$  plots for the PP first excited-state computed at the M062X/6-31+G level of theory. The descriptors values are reported with respect to the pyridinium-phenolate twist angle amplitude.

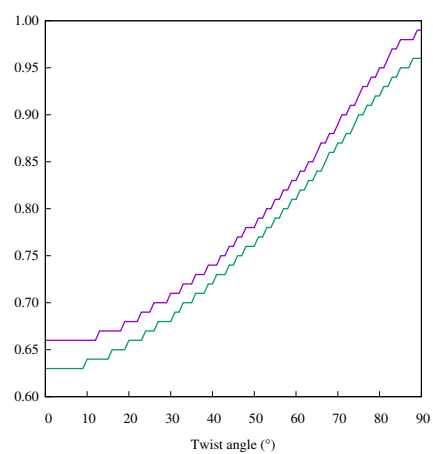

Figure S223: Reference (green) and approached (purple)  $\varphi$  plots for the PP first excited-state computed at the M062X/6-31+G level of theory. The descriptors values are reported with respect to the pyridinium-phenolate twist angle amplitude.

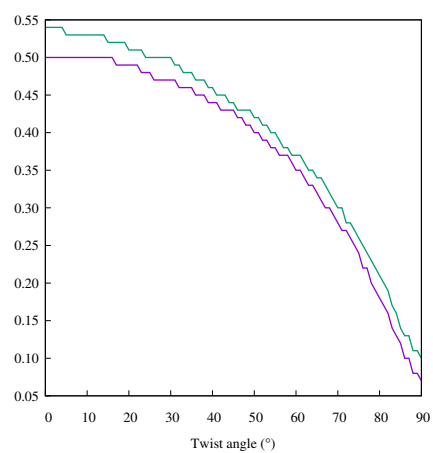

Figure S224: Reference (green) and approached (purple)  $\psi$  plots for the PP first excited-state computed at the M062X/6-31+G level of theory. The descriptors values are reported with respect to the pyridinium-phenolate twist angle amplitude.

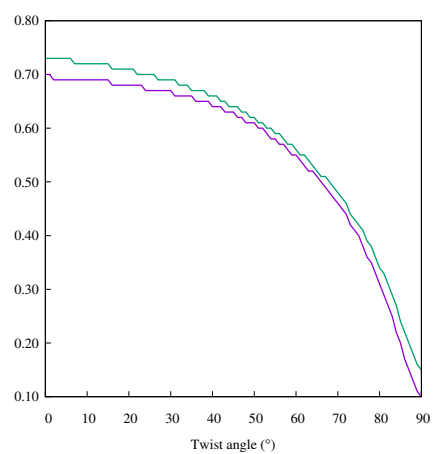

Figure S225: Reference (green) and approached (purple)  $\phi_S$  plots for the PP first excited-state computed at the M062X/6-31G level of theory. The descriptors values are reported with respect to the pyridinium-phenolate twist angle amplitude.

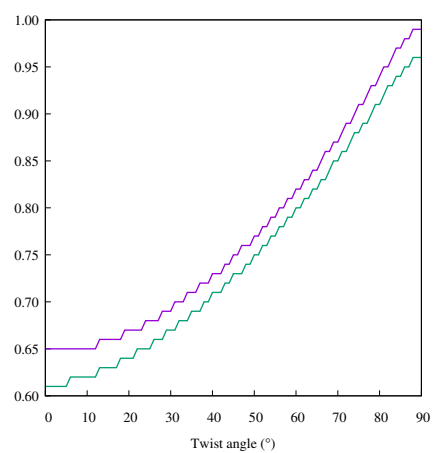

Figure S226: Reference (green) and approached (purple)  $\varphi$  plots for the PP first excited-state computed at the M062X/6-31G level of theory. The descriptors values are reported with respect to the pyridinium-phenolate twist angle amplitude.

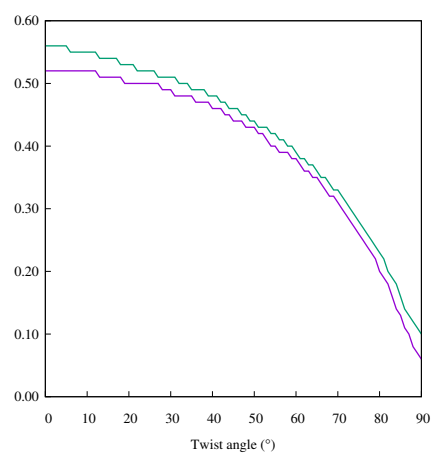

Figure S227: Reference (green) and approached (purple)  $\psi$  plots for the PP first excited-state computed at the M062X/6-31G level of theory. The descriptors values are reported with respect to the pyridinium-phenolate twist angle amplitude.

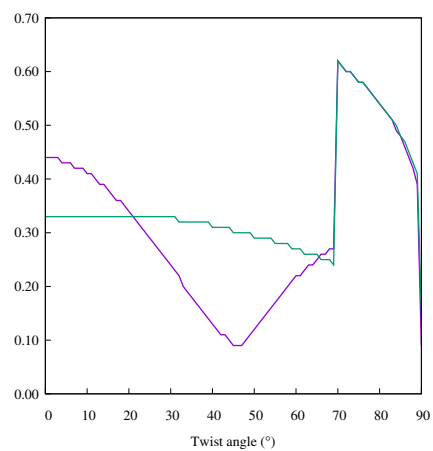

Figure S228: Reference (green) and approached (purple)  $\phi_S$  plots for the PP first excited-state computed at the PBE0/3-21G level of theory. The descriptors values are reported with respect to the pyridinium-phenolate twist angle amplitude.



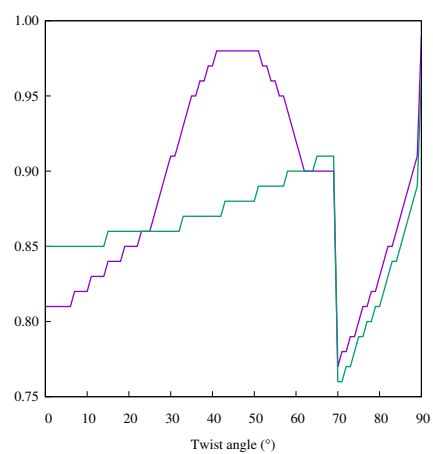

Figure S229: Reference (green) and approached (purple)  $\varphi$  plots for the PP first excited-state computed at the PBE0/3-21G level of theory. The descriptors values are reported with respect to the pyridinium-phenolate twist angle amplitude.

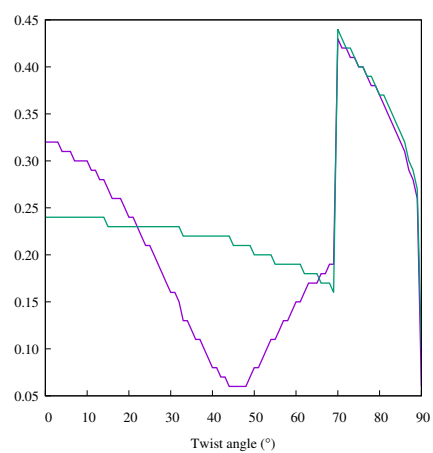

Figure S230: Reference (green) and approached (purple)  $\psi$  plots for the PP first excited-state computed at the PBE0/3-21G level of theory. The descriptors values are reported with respect to the pyridinium-phenolate twist angle amplitude.

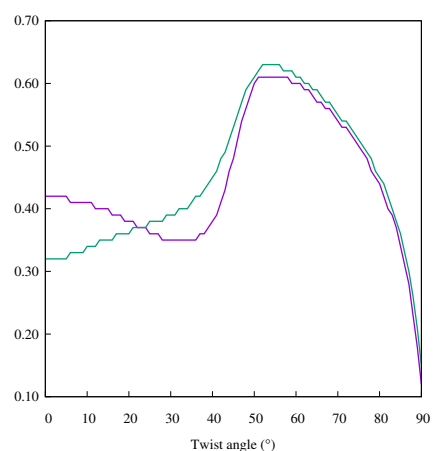

Figure S231: Reference (green) and approached (purple)  $\phi_S$  plots for the PP first excited-state computed at the PBE0/6-311++G(2d,p) level of theory. The descriptors values are reported with respect to the pyridinium-phenolate twist angle amplitude.

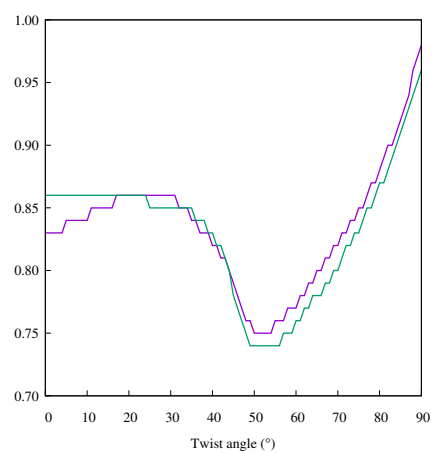

Figure S232: Reference (green) and approached (purple)  $\phi$  plots for the PP first excited-state computed at the PBE0/6-311++G(2d,p) level of theory. The descriptors values are reported with respect to the pyridinium-phenolate twist angle amplitude.

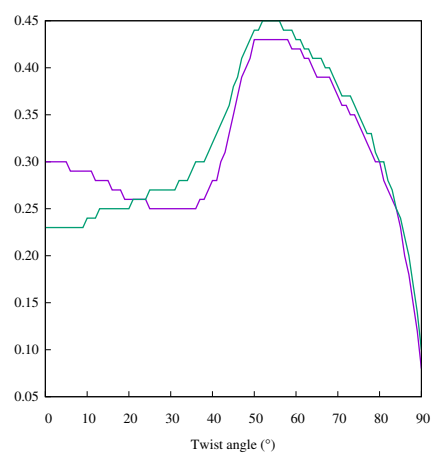

Figure S233: Reference (green) and approached (purple)  $\psi$  plots for the PP first excited-state computed at the PBE0/6-311++G(2d,p) level of theory. The descriptors values are reported with respect to the pyridinium-phenolate twist angle amplitude.

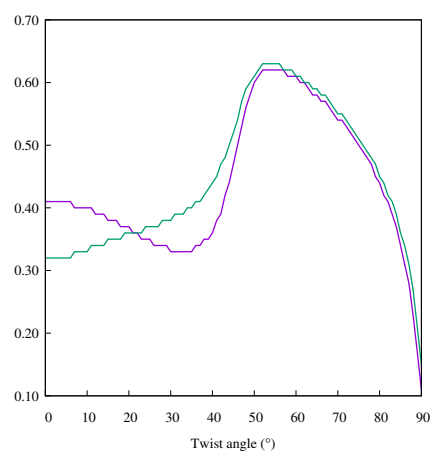

Figure S234: Reference (green) and approached (purple)  $\phi_S$  plots for the PP first excited-state computed at the PBE0/6-311+G(d) level of theory. The descriptors values are reported with respect to the pyridinium-phenolate twist angle amplitude.

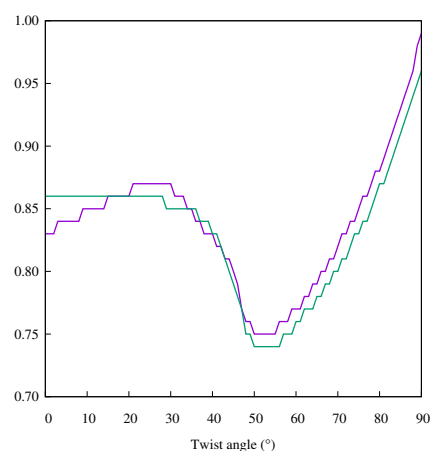

Figure S235: Reference (green) and approached (purple)  $\varphi$  plots for the PP first excited-state computed at the PBE0/6-311+G(d) level of theory. The descriptors values are reported with respect to the pyridinium-phenolate twist angle amplitude.

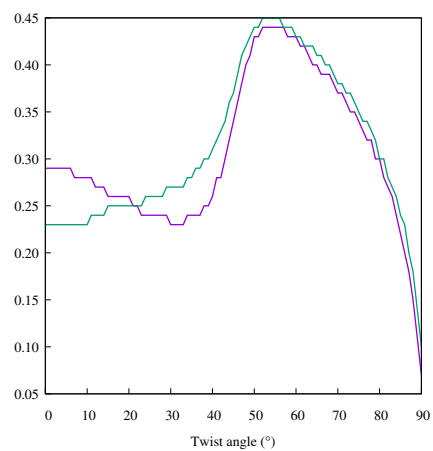

Figure S236: Reference (green) and approached (purple)  $\psi$  plots for the PP first excited-state computed at the PBE0/6-311+G(d) level of theory. The descriptors values are reported with respect to the pyridinium-phenolate twist angle amplitude.

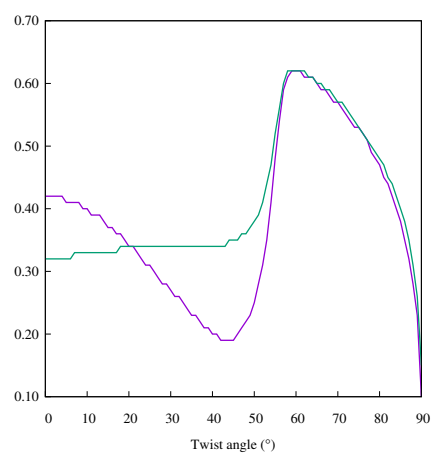

Figure S237: Reference (green) and approached (purple)  $\phi_S$  plots for the PP first excited-state computed at the PBE0/6-311G(d) level of theory. The descriptors values are reported with respect to the pyridinium-phenolate twist angle amplitude.

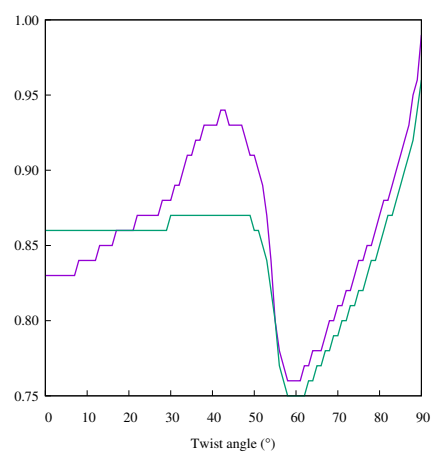

Figure S238: Reference (green) and approached (purple)  $\varphi$  plots for the PP first excited-state computed at the PBE0/6-311G(d) level of theory. The descriptors values are reported with respect to the pyridinium-phenolate twist angle amplitude.

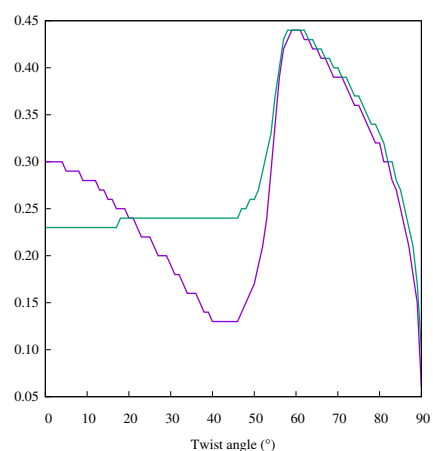

Figure S239: Reference (green) and approached (purple)  $\psi$  plots for the PP first excited-state computed at the PBE0/6-311G(d) level of theory. The descriptors values are reported with respect to the pyridinium-phenolate twist angle amplitude.

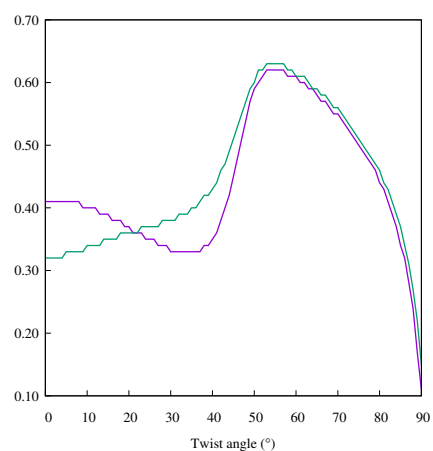

Figure S240: Reference (green) and approached (purple)  $\phi_S$  plots for the PP first excited-state computed at the PBE0/6-311++Gdp level of theory. The descriptors values are reported with respect to the pyridinium-phenolate twist angle amplitude.

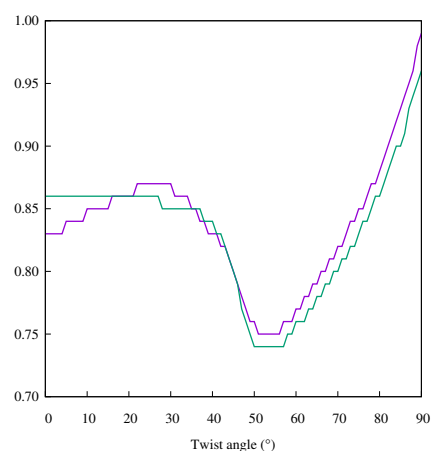

Figure S241: Reference (green) and approached (purple)  $\varphi$  plots for the PP first excited-state computed at the PBE0/6-311++G(d,p) level of theory. The descriptors values are reported with respect to the pyridinium-phenolate twist angle amplitude.

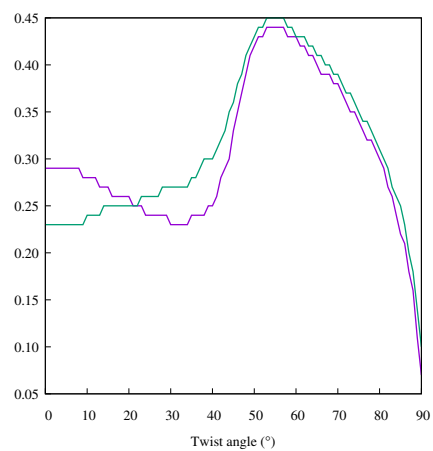

Figure S242: Reference (green) and approached (purple)  $\psi$  plots for the PP first excited-state computed at the PBE0/6-311++G(d,p) level of theory. The descriptors values are reported with respect to the pyridinium-phenolate twist angle amplitude.

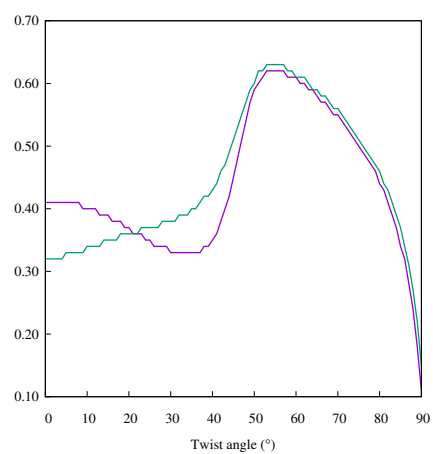

Figure S243: Reference (green) and approached (purple)  $\phi_S$  plots for the PP first excited-state computed at the PBE0/6-311+G(d,p) level of theory. The descriptors values are reported with respect to the pyridinium-phenolate twist angle amplitude.

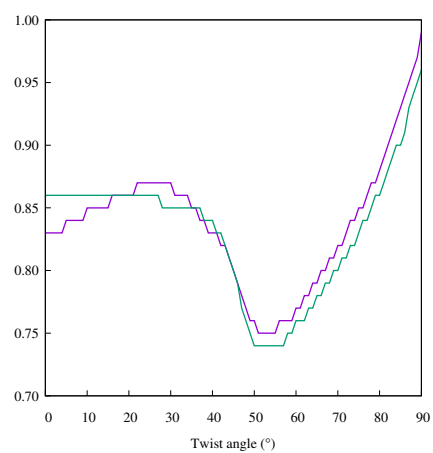

Figure S244: Reference (green) and approached (purple)  $\varphi$  plots for the PP first excited-state computed at the PBE0/6-311+G(d,p) level of theory. The descriptors values are reported with respect to the pyridinium-phenolate twist angle amplitude.



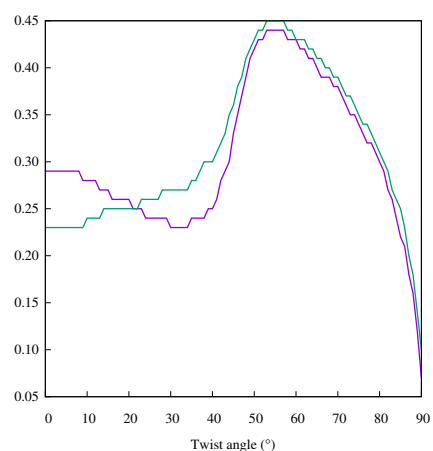

Figure S245: Reference (green) and approached (purple)  $\psi$  plots for the PP first excited-state computed at the PBE0/6-311+G(d,p) level of theory. The descriptors values are reported with respect to the pyridinium-phenolate twist angle amplitude.

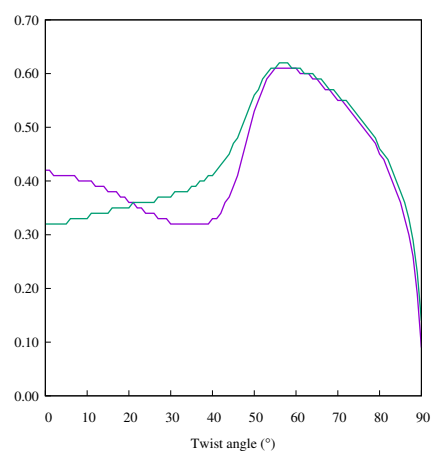

Figure S246: Reference (green) and approached (purple)  $\phi_S$  plots for the PP first excited-state computed at the PBE0/6-311+G level of theory. The descriptors values are reported with respect to the pyridinium-phenolate twist angle amplitude.

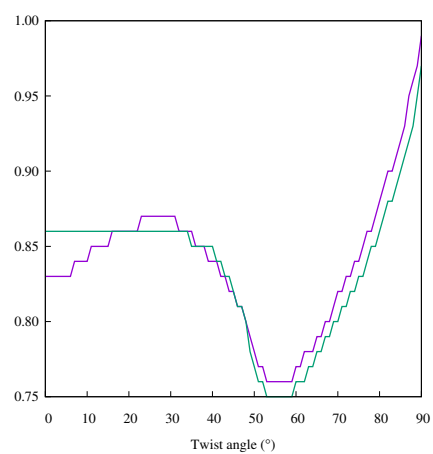

Figure S247: Reference (green) and approached (purple)  $\varphi$  plots for the PP first excited-state computed at the PBE0/6-311+G level of theory. The descriptors values are reported with respect to the pyridinium-phenolate twist angle amplitude.

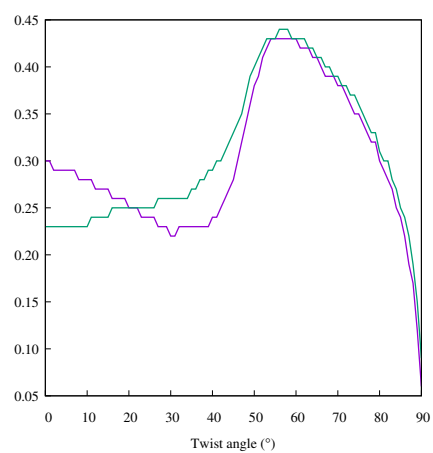

Figure S248: Reference (green) and approached (purple)  $\psi$  plots for the PP first excited-state computed at the PBE0/6-311+G level of theory. The descriptors values are reported with respect to the pyridinium-phenolate twist angle amplitude.

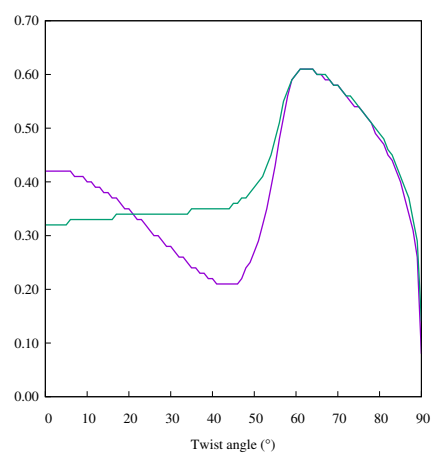

Figure S249: Reference (green) and approached (purple)  $\phi_S$  plots for the PP first excited-state computed at the PBE0/6-311G level of theory. The descriptors values are reported with respect to the pyridinium-phenolate twist angle amplitude.

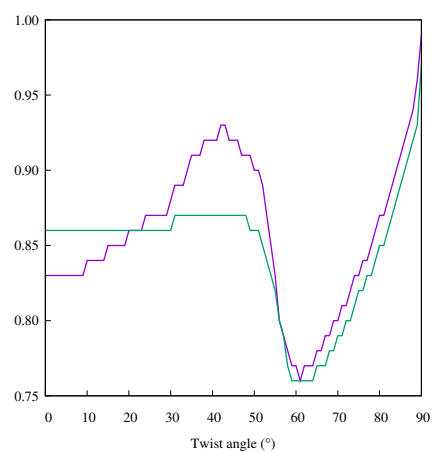

Figure S250: Reference (green) and approached (purple)  $\varphi$  plots for the PP first excited-state computed at the PBE0/6-311G level of theory. The descriptors values are reported with respect to the pyridinium-phenolate twist angle amplitude.

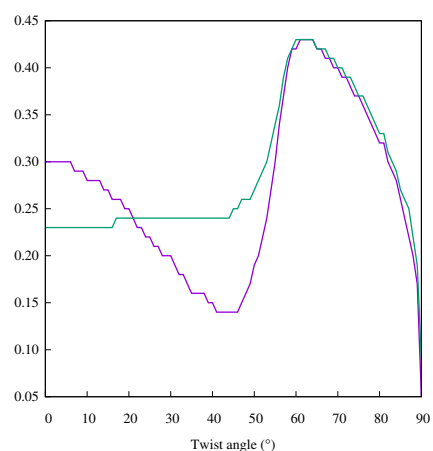

Figure S251: Reference (green) and approached (purple)  $\psi$  plots for the PP first excited-state computed at the PBE0/6-311G level of theory. The descriptors values are reported with respect to the pyridinium-phenolate twist angle amplitude.

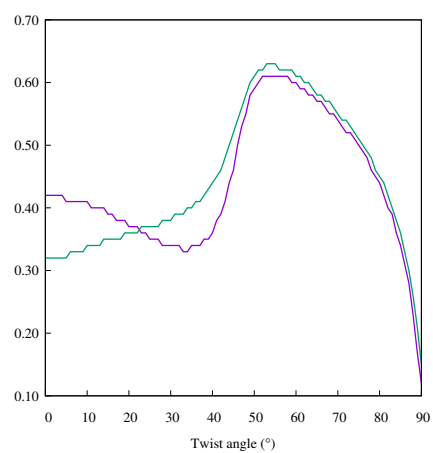

Figure S252: Reference (green) and approached (purple)  $\phi_S$  plots for the PP first excited-state computed at the PBE0/6-31++G(2d,p) level of theory. The descriptors values are reported with respect to the pyridinium-phenolate twist angle amplitude.

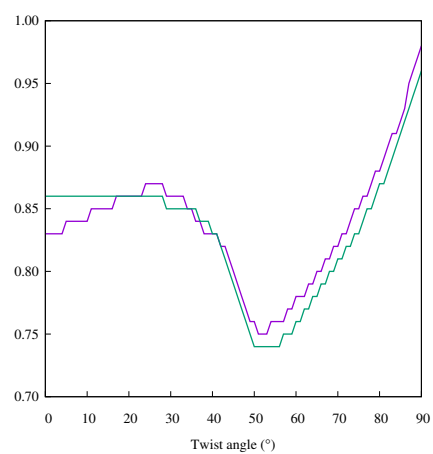

Figure S253: Reference (green) and approached (purple)  $\varphi$  plots for the PP first excited-state computed at the PBE0/6-31++G(2d,p) level of theory. The descriptors values are reported with respect to the pyridinium-phenolate twist angle amplitude.

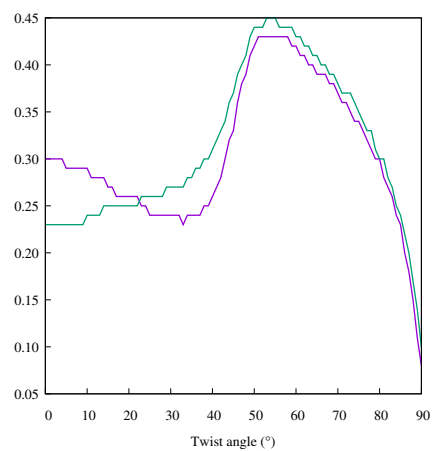

Figure S254: Reference (green) and approached (purple)  $\psi$  plots for the PP first excited-state computed at the PBE0/6-31++G(2d,p) level of theory. The descriptors values are reported with respect to the pyridinium-phenolate twist angle amplitude.

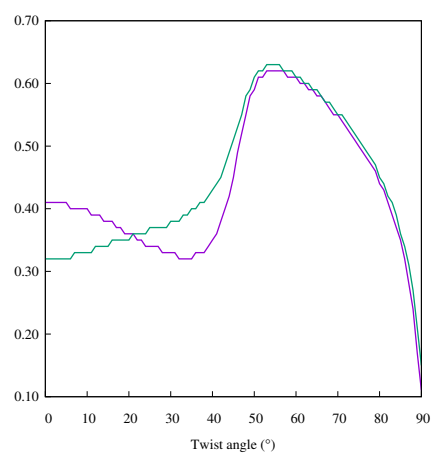

Figure S255: Reference (green) and approached (purple)  $\phi_S$  plots for the PP first excited-state computed at the PBE0/6-31+G(d) level of theory. The descriptors values are reported with respect to the pyridinium-phenolate twist angle amplitude.

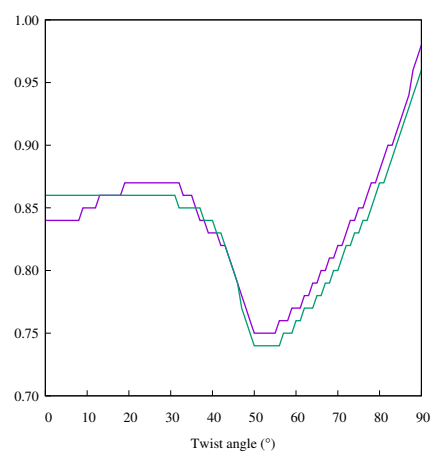

Figure S256: Reference (green) and approached (purple)  $\varphi$  plots for the PP first excited-state computed at the PBE0/6-31+G(d) level of theory. The descriptors values are reported with respect to the pyridinium-phenolate twist angle amplitude.

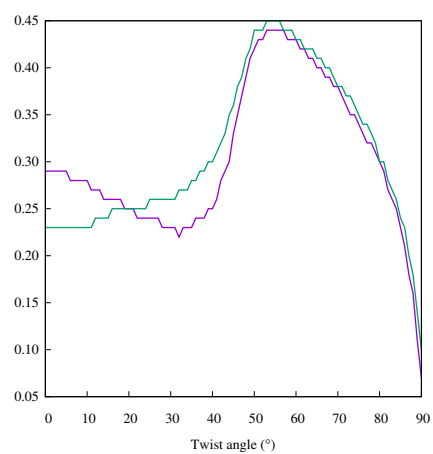

Figure S257: Reference (green) and approached (purple)  $\psi$  plots for the PP first excited-state computed at the PBE0/6-31+G(d) level of theory. The descriptors values are reported with respect to the pyridinium-phenolate twist angle amplitude.

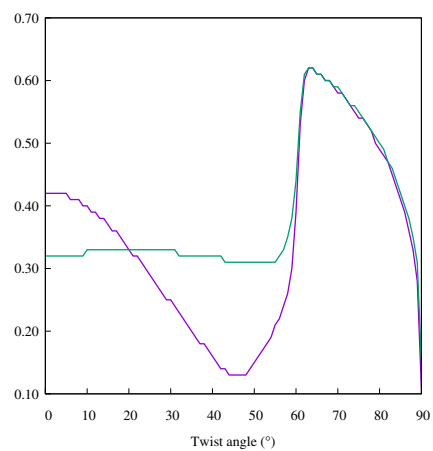

Figure S258: Reference (green) and approached (purple)  $\phi_S$  plots for the PP first excited-state computed at the PBE0/6-31G(d) level of theory. The descriptors values are reported with respect to the pyridinium-phenolate twist angle amplitude.

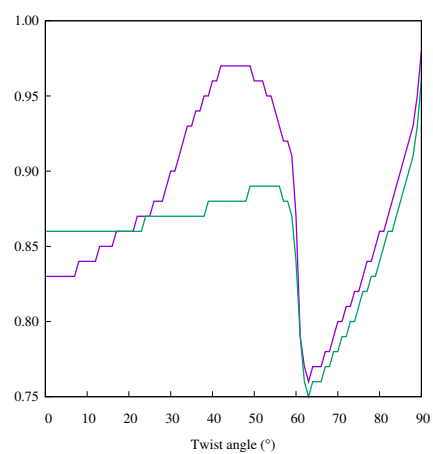

Figure S259: Reference (green) and approached (purple)  $\varphi$  plots for the PP first excited-state computed at the PBE0/6-31G(d) level of theory. The descriptors values are reported with respect to the pyridinium-phenolate twist angle amplitude.

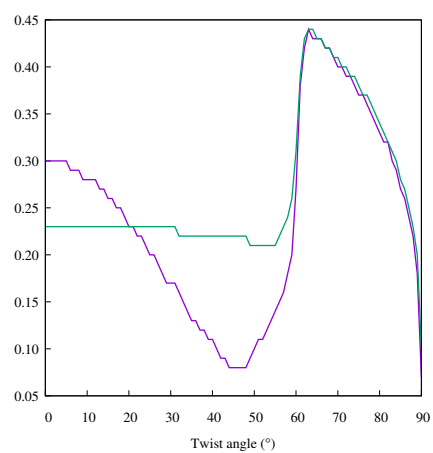

Figure S260: Reference (green) and approached (purple)  $\psi$  plots for the PP first excited-state computed at the PBE0/6-31G(d) level of theory. The descriptors values are reported with respect to the pyridinium-phenolate twist angle amplitude.



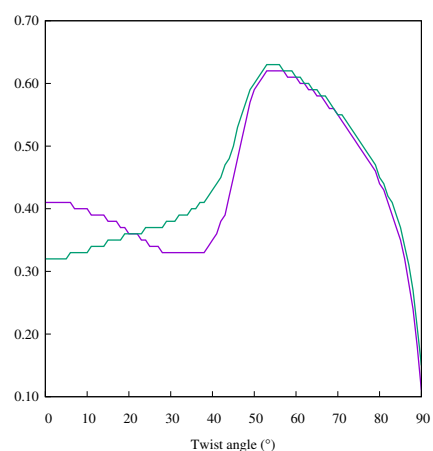

Figure S261: Reference (green) and approached (purple)  $\phi_S$  plots for the PP first excited-state computed at the PBE0/6-31++G(d,p) level of theory. The descriptors values are reported with respect to the pyridinium-phenolate twist angle amplitude.

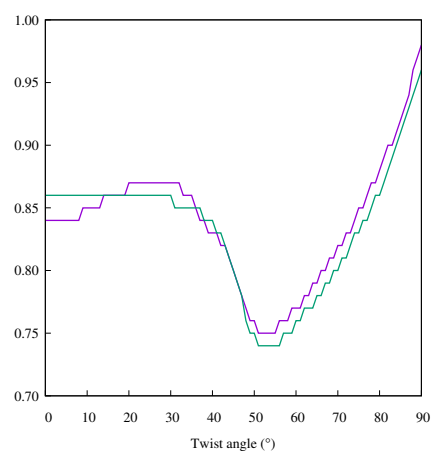

Figure S262: Reference (green) and approached (purple)  $\phi$  plots for the PP first excited-state computed at the PBE0/6-31++G(d,p) level of theory. The descriptors values are reported with respect to the pyridinium-phenolate twist angle amplitude.

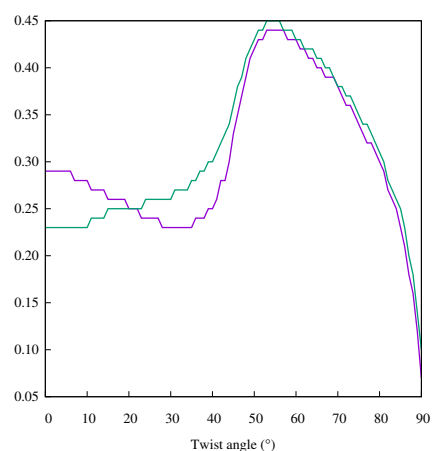

Figure S263: Reference (green) and approached (purple)  $\psi$  plots for the PP first excited-state computed at the PBE0/6-31++G(d,p) level of theory. The descriptors values are reported with respect to the pyridinium-phenolate twist angle amplitude.

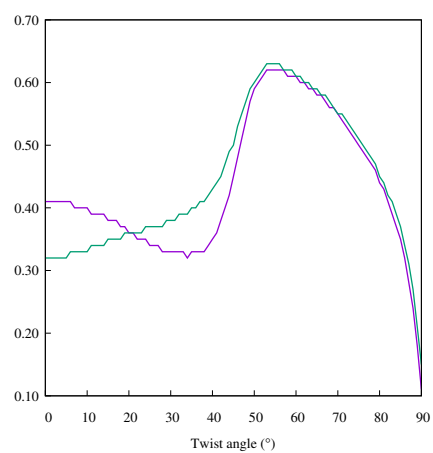

Figure S264: Reference (green) and approached (purple)  $\phi_S$  plots for the PP first excited-state computed at the PBE0/6-31+G(d,p) level of theory. The descriptors values are reported with respect to the pyridinium-phenolate twist angle amplitude.

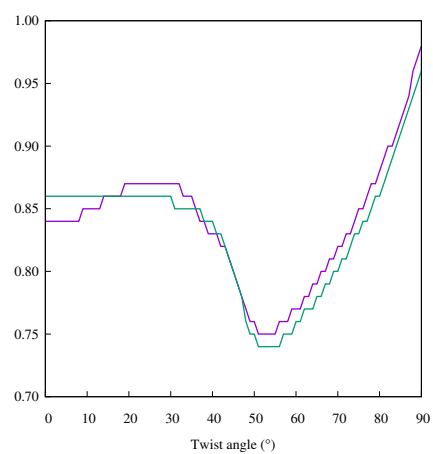

Figure S265: Reference (green) and approached (purple)  $\varphi$  plots for the PP first excited-state computed at the PBE0/6-31+G(d,p) level of theory. The descriptors values are reported with respect to the pyridinium-phenolate twist angle amplitude.

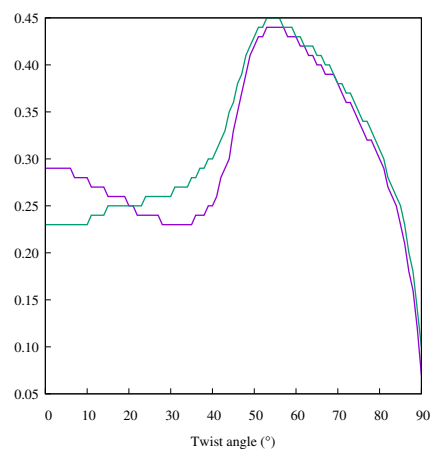

Figure S266: Reference (green) and approached (purple)  $\psi$  plots for the PP first excited-state computed at the PBE0/6-31+G(d,p) level of theory. The descriptors values are reported with respect to the pyridinium-phenolate twist angle amplitude.

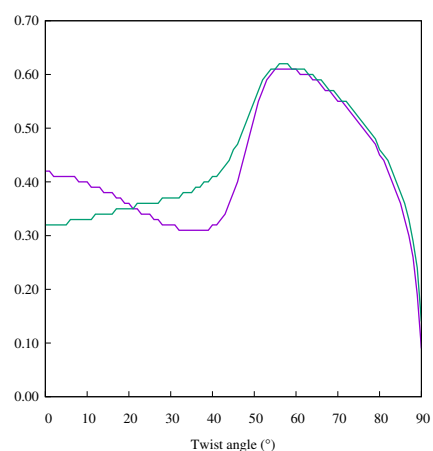

Figure S267: Reference (green) and approached (purple)  $\phi_S$  plots for the PP first excited-state computed at the PBE0/6-31+G level of theory. The descriptors values are reported with respect to the pyridinium-phenolate twist angle amplitude.

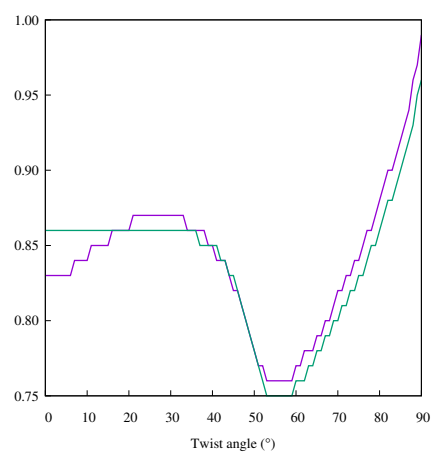

Figure S268: Reference (green) and approached (purple)  $\phi$  plots for the PP first excited-state computed at the PBE0/6-31+G level of theory. The descriptors values are reported with respect to the pyridinium-phenolate twist angle amplitude.

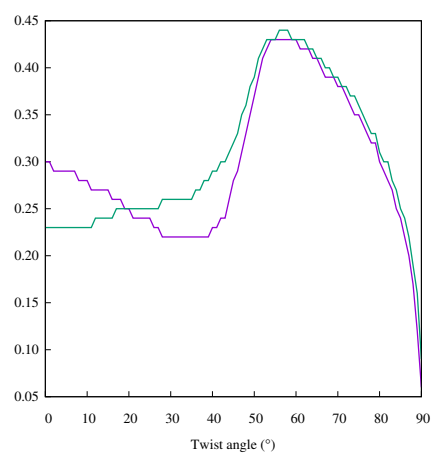

Figure S269: Reference (green) and approached (purple)  $\psi$  plots for the PP first excited-state computed at the PBE0/6-31+G level of theory. The descriptors values are reported with respect to the pyridinium-phenolate twist angle amplitude.

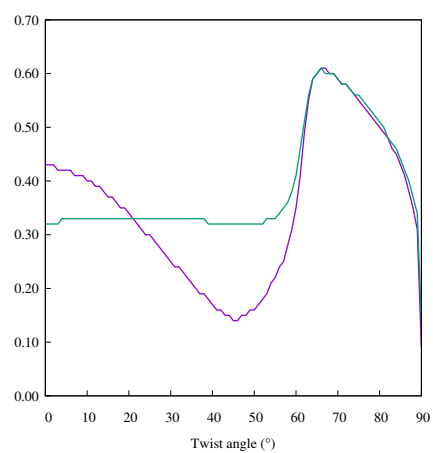

Figure S270: Reference (green) and approached (purple)  $\phi_S$  plots for the PP first excited-state computed at the PBE0/6-31G level of theory. The descriptors values are reported with respect to the pyridinium-phenolate twist angle amplitude.

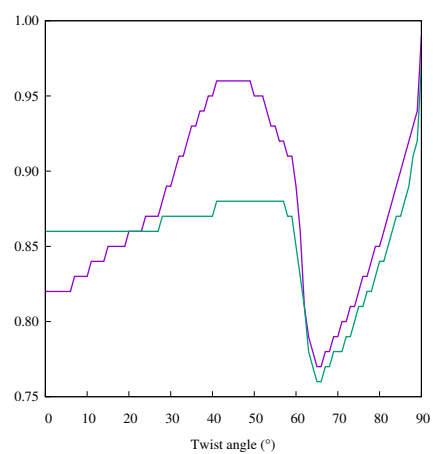

Figure S271: Reference (green) and approached (purple)  $\varphi$  plots for the PP first excited-state computed at the PBE0/6-31G level of theory. The descriptors values are reported with respect to the pyridinium-phenolate twist angle amplitude.

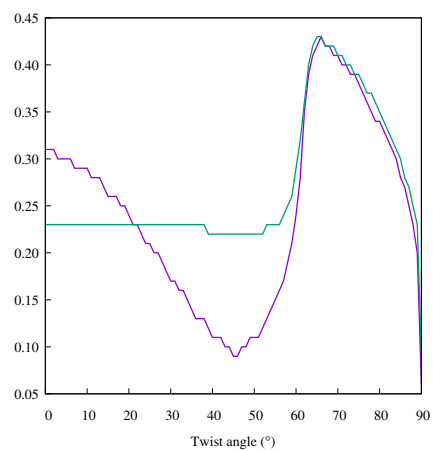

Figure S272: Reference (green) and approached (purple)  $\psi$  plots for the PP first excited-state computed at the PBE0/6-31G level of theory. The descriptors values are reported with respect to the pyridinium-phenolate twist angle amplitude.

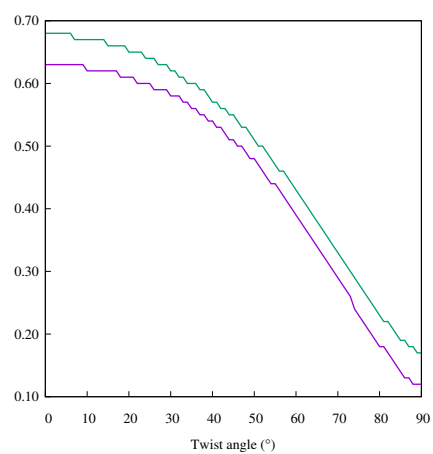

Figure S273: Reference (green) and approached (purple)  $\phi_S$  plots for the PP first excited-state computed at the TDHF/3-21G level of theory. The descriptors values are reported with respect to the pyridinium-phenolate twist angle amplitude.

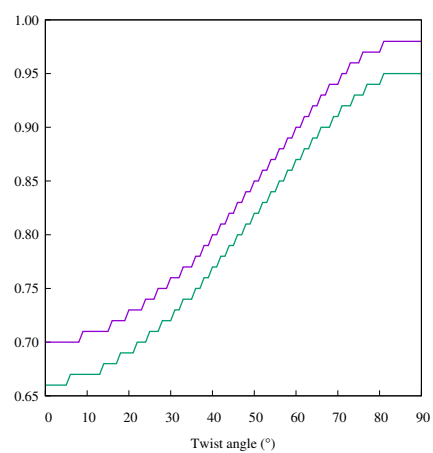

Figure S274: Reference (green) and approached (purple)  $\varphi$  plots for the PP first excited-state computed at the TDHF/3-21G level of theory. The descriptors values are reported with respect to the pyridinium-phenolate twist angle amplitude.

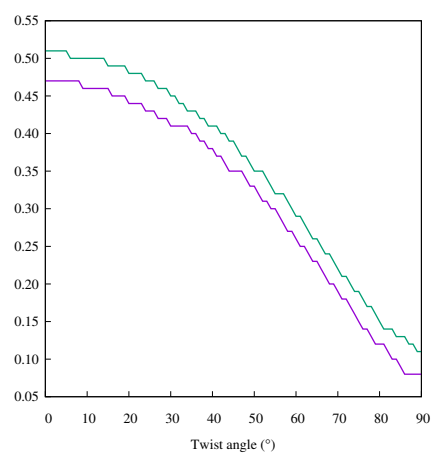

Figure S275: Reference (green) and approached (purple)  $\psi$  plots for the PP first excited-state computed at the TDHF/3-21G level of theory. The descriptors values are reported with respect to the pyridinium-phenolate twist angle amplitude.

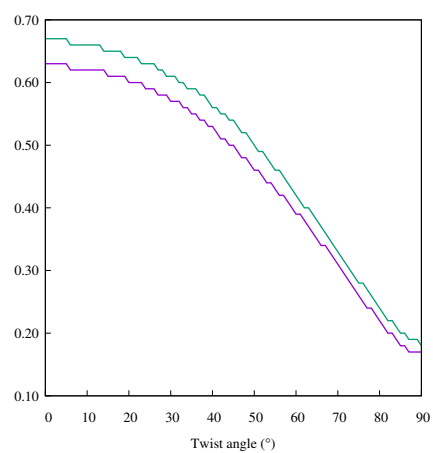

Figure S276: Reference (green) and approached (purple)  $\phi_S$  plots for the PP first excited-state computed at the TDHF/6-311++G(2d,p) level of theory. The descriptors values are reported with respect to the pyridinium-phenolate twist angle amplitude.



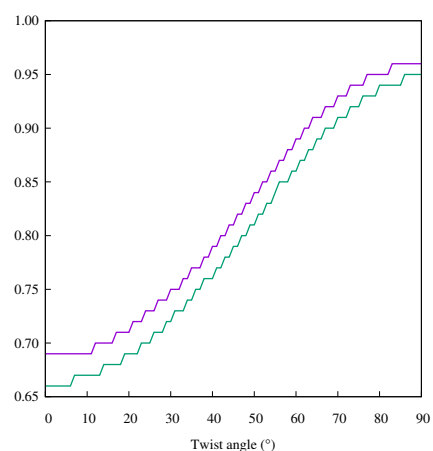

Figure S277: Reference (green) and approached (purple)  $\varphi$  plots for the PP first excited-state computed at the TDHF/6-311++G(2d,p) level of theory. The descriptors values are reported with respect to the pyridinium-phenolate twist angle amplitude.

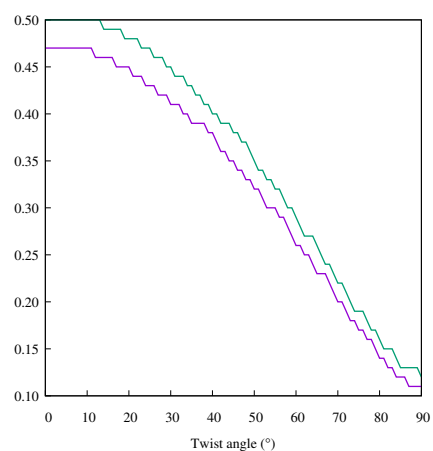

Figure S278: Reference (green) and approached (purple)  $\psi$  plots for the PP first excited-state computed at the TDHF/6-311++G(2d,p) level of theory. The descriptors values are reported with respect to the pyridinium-phenolate twist angle amplitude.

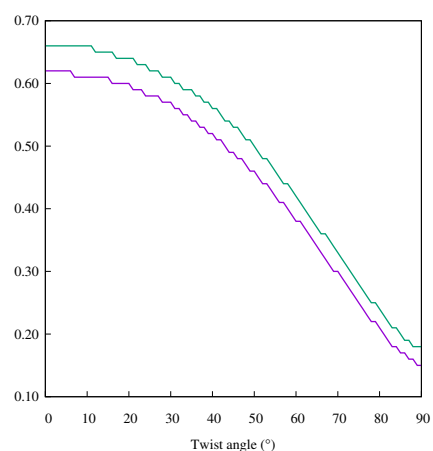

Figure S279: Reference (green) and approached (purple)  $\phi_S$  plots for the PP first excited-state computed at the TDHF/6-311+G(d) level of theory. The descriptors values are reported with respect to the pyridinium-phenolate twist angle amplitude.

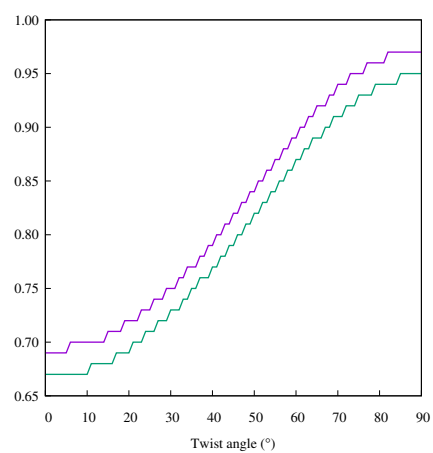

Figure S280: Reference (green) and approached (purple)  $\varphi$  plots for the PP first excited-state computed at the TDHF/6-311+G(d) level of theory. The descriptors values are reported with respect to the pyridinium-phenolate twist angle amplitude.

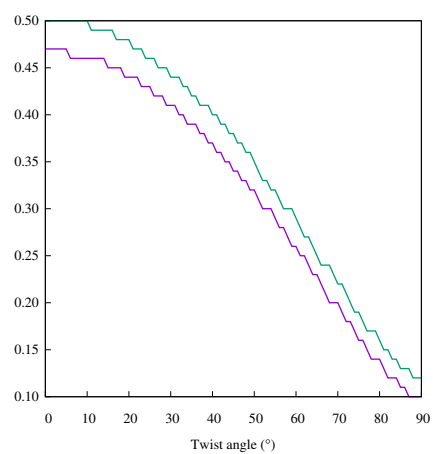

Figure S281: Reference (green) and approached (purple)  $\psi$  plots for the PP first excited-state computed at the TDHF/6-311+G(d) level of theory. The descriptors values are reported with respect to the pyridinium-phenolate twist angle amplitude.

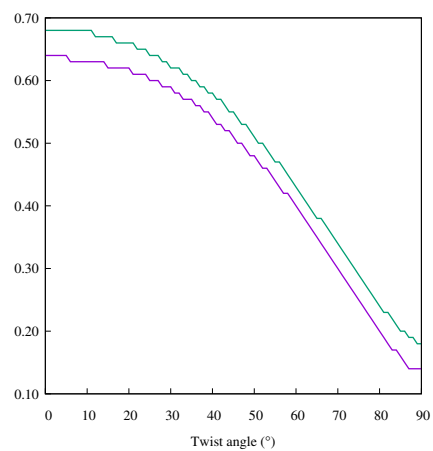

Figure S282: Reference (green) and approached (purple)  $\phi_S$  plots for the PP first excited-state computed at the TDHF/6-311G(d) level of theory. The descriptors values are reported with respect to the pyridinium-phenolate twist angle amplitude.

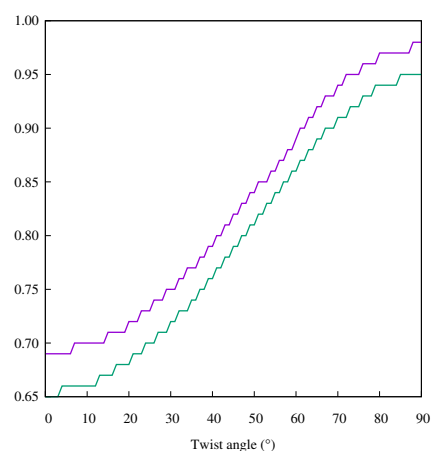

Figure S283: Reference (green) and approached (purple)  $\varphi$  plots for the PP first excited-state computed at the TDHF/6-311G(d) level of theory. The descriptors values are reported with respect to the pyridinium-phenolate twist angle amplitude.

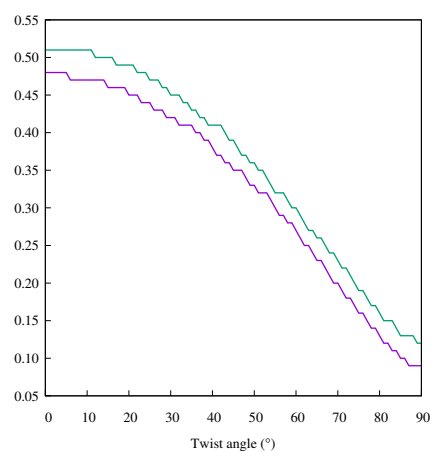

Figure S284: Reference (green) and approached (purple)  $\psi$  plots for the PP first excited-state computed at the TDHF/6-311G(d) level of theory. The descriptors values are reported with respect to the pyridinium-phenolate twist angle amplitude.

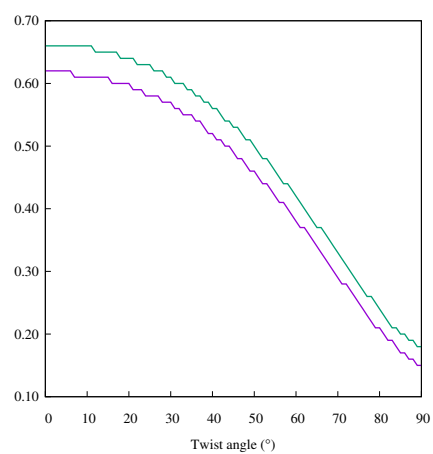

Figure S285: Reference (green) and approached (purple)  $\phi_S$  plots for the PP first excited-state computed at the TDHF/6-311++G(d,p) level of theory. The descriptors values are reported with respect to the pyridinium-phenolate twist angle amplitude.

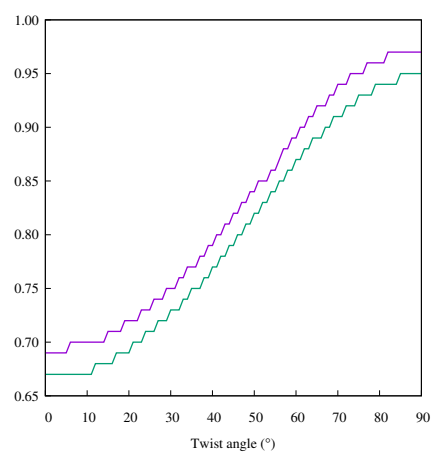

Figure S286: Reference (green) and approached (purple)  $\varphi$  plots for the PP first excited-state computed at the TDHF/6-311++G(d,p) level of theory. The descriptors values are reported with respect to the pyridinium-phenolate twist angle amplitude.

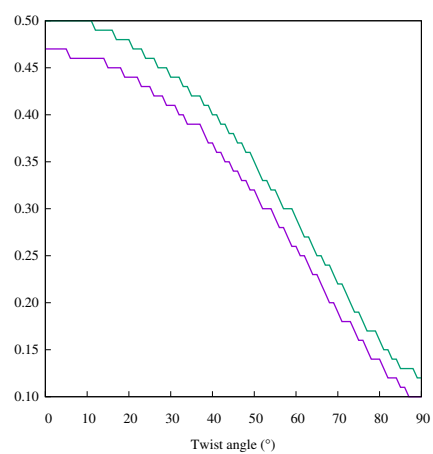

Figure S287: Reference (green) and approached (purple)  $\psi$  plots for the PP first excited-state computed at the TDHF/6-311++G(d,p) level of theory. The descriptors values are reported with respect to the pyridinium-phenolate twist angle amplitude.

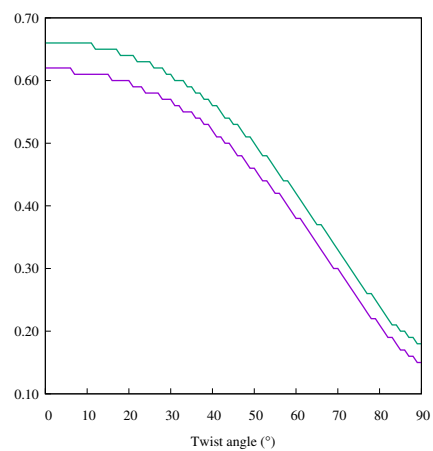

Figure S288: Reference (green) and approached (purple)  $\phi_S$  plots for the PP first excited-state computed at the TDHF/6-311+G(d,p) level of theory. The descriptors values are reported with respect to the pyridinium-phenolate twist angle amplitude.

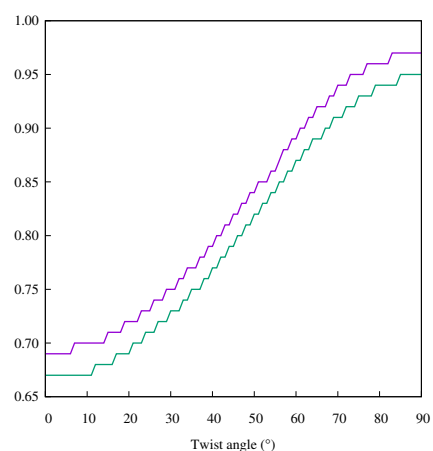

Figure S289: Reference (green) and approached (purple)  $\varphi$  plots for the PP first excited-state computed at the TDHF/6-311+G(d,p) level of theory. The descriptors values are reported with respect to the pyridinium-phenolate twist angle amplitude.

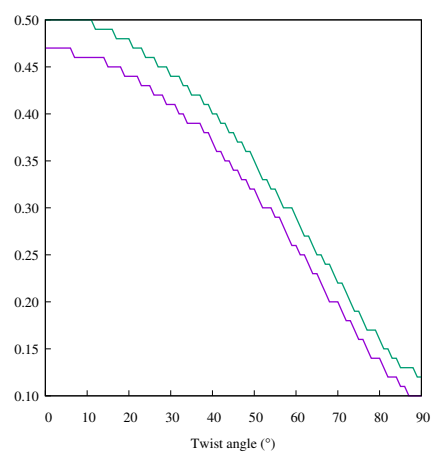

Figure S290: Reference (green) and approached (purple)  $\psi$  plots for the PP first excited-state computed at the TDHF/6-311+G(d,p) level of theory. The descriptors values are reported with respect to the pyridinium-phenolate twist angle amplitude.

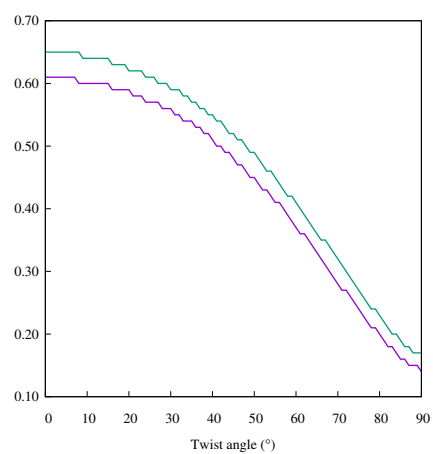

Figure S291: Reference (green) and approached (purple)  $\phi_S$  plots for the PP first excited-state computed at the TDHF/6-311+G level of theory. The descriptors values are reported with respect to the pyridinium-phenolate twist angle amplitude.

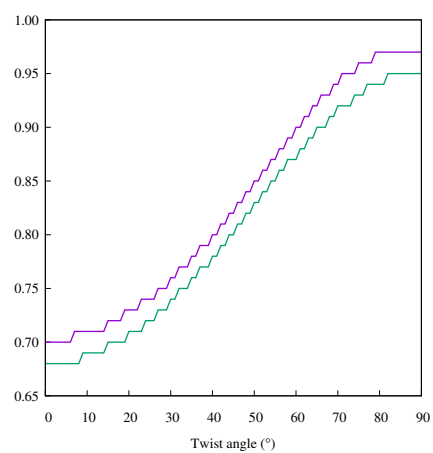

Figure S292: Reference (green) and approached (purple)  $\varphi$  plots for the PP first excited-state computed at the TDHF/6-311+G level of theory. The descriptors values are reported with respect to the pyridinium-phenolate twist angle amplitude.



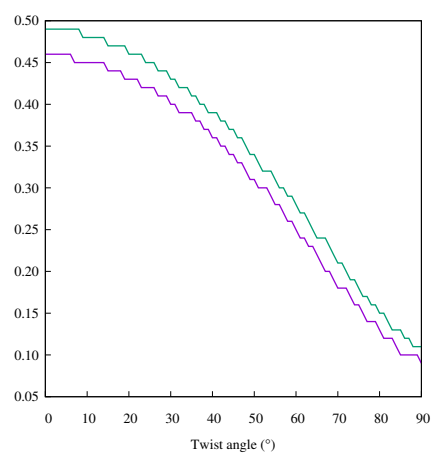

Figure S293: Reference (green) and approached (purple)  $\psi$  plots for the PP first excited-state computed at the TDHF/6-311+G level of theory. The descriptors values are reported with respect to the pyridinium-phenolate twist angle amplitude.

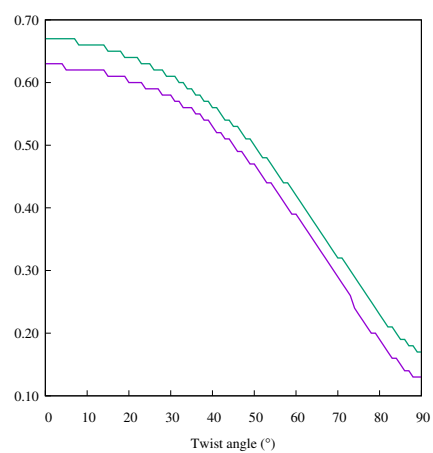

Figure S294: Reference (green) and approached (purple)  $\phi_S$  plots for the PP first excited-state computed at the TDHF/6-311G level of theory. The descriptors values are reported with respect to the pyridinium-phenolate twist angle amplitude.

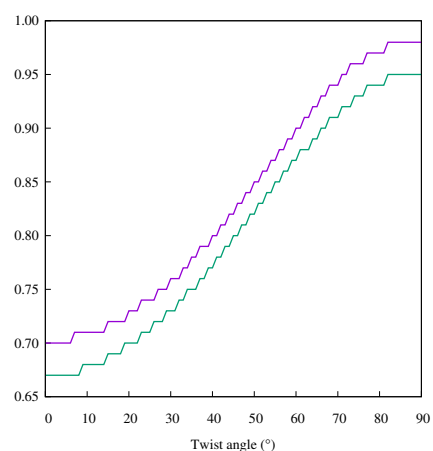

Figure S295: Reference (green) and approached (purple)  $\varphi$  plots for the PP first excited-state computed at the TDHF/6-311G level of theory. The descriptors values are reported with respect to the pyridinium-phenolate twist angle amplitude.

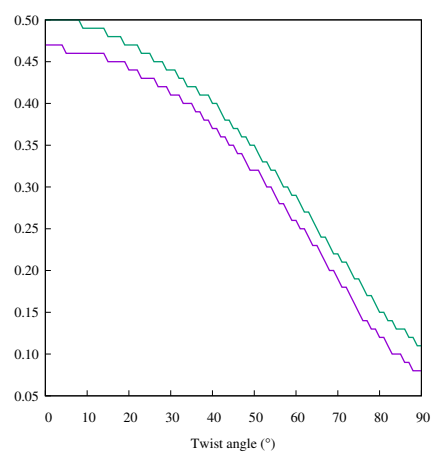

Figure S296: Reference (green) and approached (purple)  $\psi$  plots for the PP first excited-state computed at the TDHF/6-311G level of theory. The descriptors values are reported with respect to the pyridinium-phenolate twist angle amplitude.

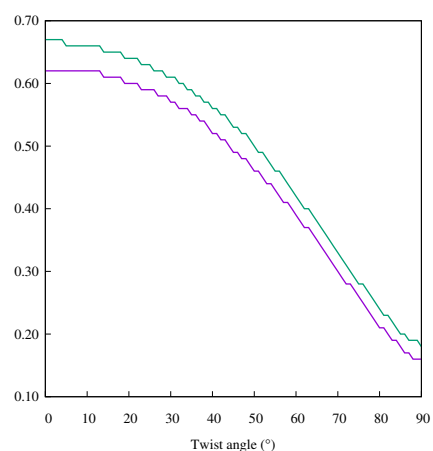

Figure S297: Reference (green) and approached (purple)  $\phi_S$  plots for the PP first excited-state computed at the TDHF/6-31++G(2d,p) level of theory. The descriptors values are reported with respect to the pyridinium-phenolate twist angle amplitude.

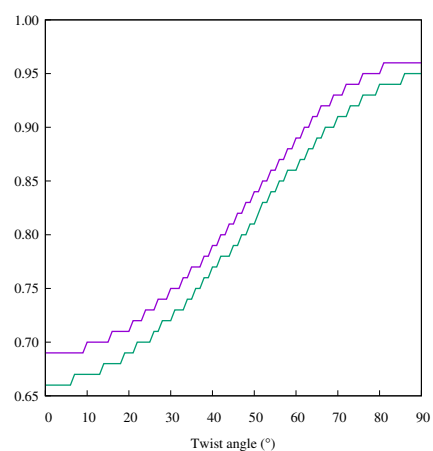

Figure S298: Reference (green) and approached (purple)  $\varphi$  plots for the PP first excited-state computed at the TDHF/6-31++G(2d,p) level of theory. The descriptors values are reported with respect to the pyridinium-phenolate twist angle amplitude.

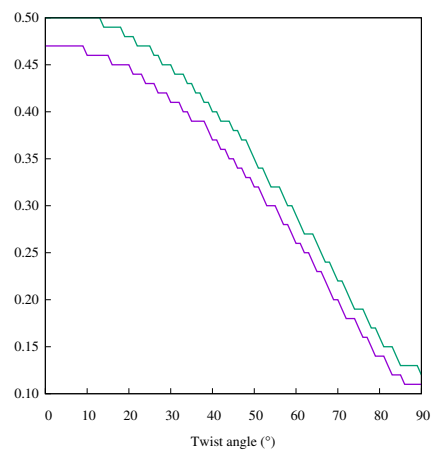

Figure S299: Reference (green) and approached (purple)  $\psi$  plots for the PP first excited-state computed at the TDHF/6-31++G(2d,p) level of theory. The descriptors values are reported with respect to the pyridinium-phenolate twist angle amplitude.

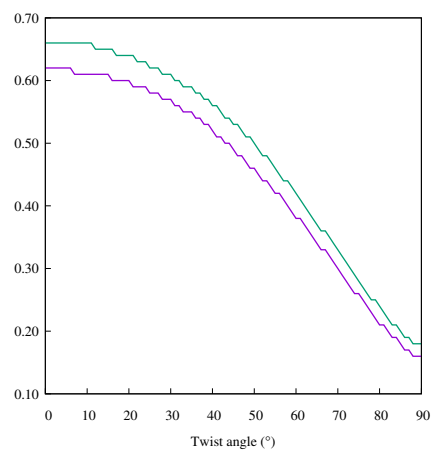

Figure S300: Reference (green) and approached (purple)  $\phi_S$  plots for the PP first excited-state computed at the TDHF/6-31+G(d) level of theory. The descriptors values are reported with respect to the pyridinium-phenolate twist angle amplitude.

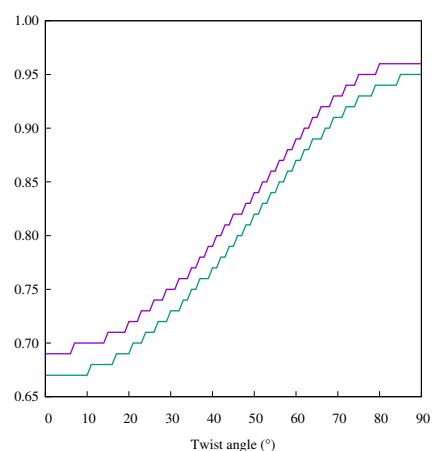

Figure S301: Reference (green) and approached (purple)  $\varphi$  plots for the PP first excited-state computed at the TDHF/6-31+G(d) level of theory. The descriptors values are reported with respect to the pyridinium-phenolate twist angle amplitude.

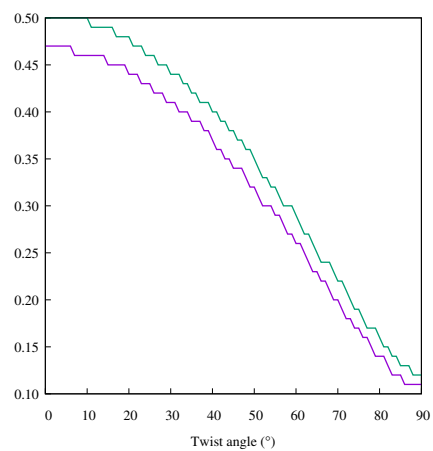

Figure S302: Reference (green) and approached (purple)  $\psi$  plots for the PP first excited-state computed at the TDHF/6-31+G(d) level of theory. The descriptors values are reported with respect to the pyridinium-phenolate twist angle amplitude.

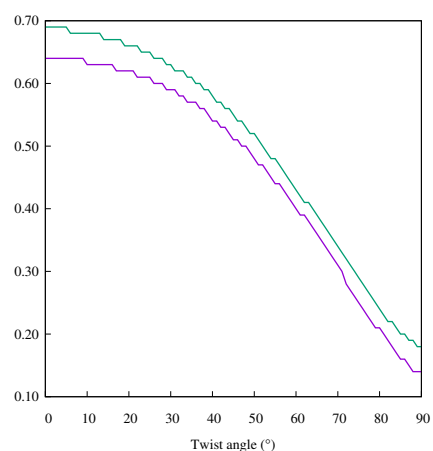

Figure S303: Reference (green) and approached (purple)  $\phi_S$  plots for the PP first excited-state computed at the TDHF/6-31G(d) level of theory. The descriptors values are reported with respect to the pyridinium-phenolate twist angle amplitude.

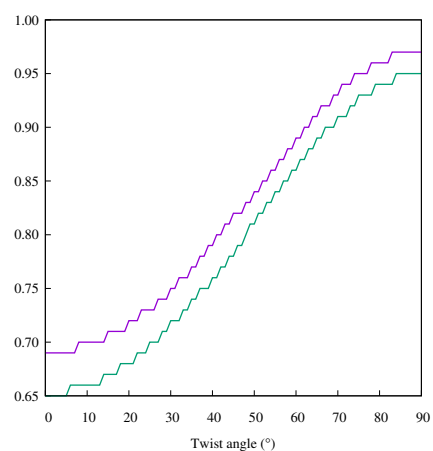

Figure S304: Reference (green) and approached (purple)  $\varphi$  plots for the PP first excited-state computed at the TDHF/6-31G(d) level of theory. The descriptors values are reported with respect to the pyridinium-phenolate twist angle amplitude.

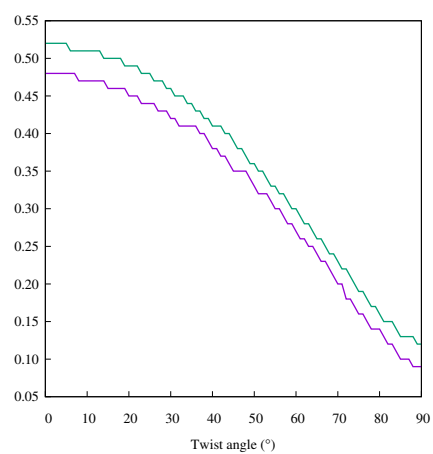

Figure S305: Reference (green) and approached (purple)  $\psi$  plots for the PP first excited-state computed at the TDHF/6-31G(d) level of theory. The descriptors values are reported with respect to the pyridinium-phenolate twist angle amplitude.

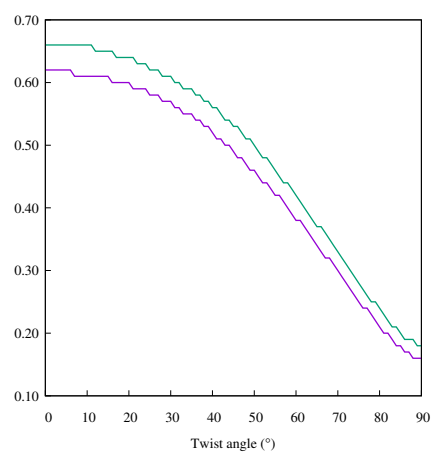

Figure S306: Reference (green) and approached (purple)  $\phi_S$  plots for the PP first excited-state computed at the TDHF/6-31++G(d,p) level of theory. The descriptors values are reported with respect to the pyridinium-phenolate twist angle amplitude.

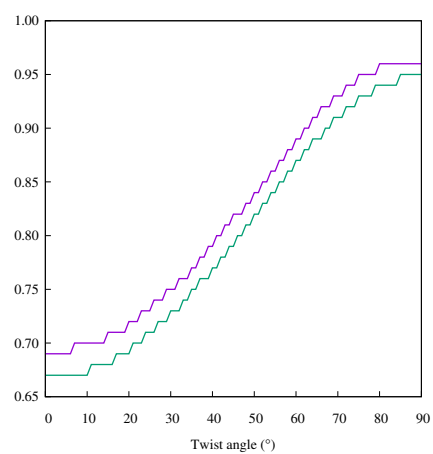

Figure S307: Reference (green) and approached (purple)  $\varphi$  plots for the PP first excited-state computed at the TDHF/6-31++G(d,p) level of theory. The descriptors values are reported with respect to the pyridinium-phenolate twist angle amplitude.

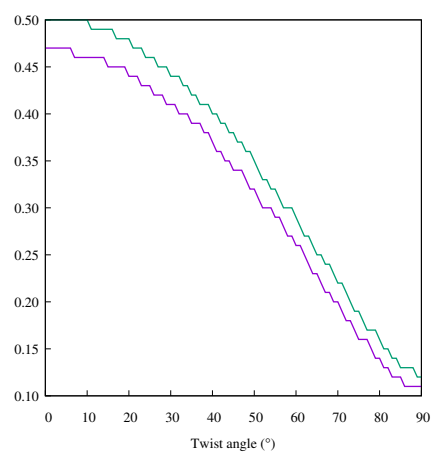

Figure S308: Reference (green) and approached (purple)  $\psi$  plots for the PP first excited-state computed at the TDHF/6-31++G(d,p) level of theory. The descriptors values are reported with respect to the pyridinium-phenolate twist angle amplitude.



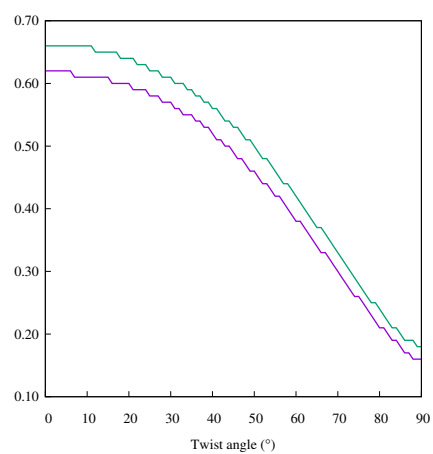

Figure S309: Reference (green) and approached (purple)  $\phi_S$  plots for the PP first excited-state computed at the TDHF/6-31+G(d,p) level of theory. The descriptors values are reported with respect to the pyridinium-phenolate twist angle amplitude.

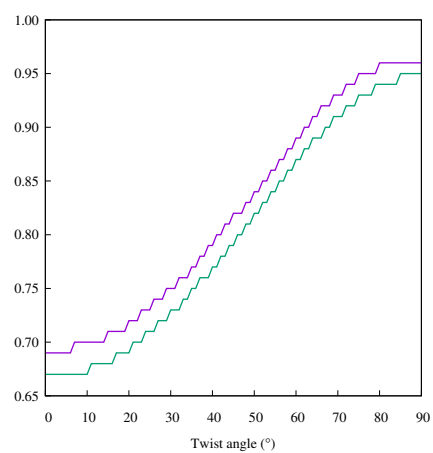

Figure S310: Reference (green) and approached (purple)  $\varphi$  plots for the PP first excited-state computed at the TDHF/6-31+G(d,p) level of theory. The descriptors values are reported with respect to the pyridinium-phenolate twist angle amplitude.

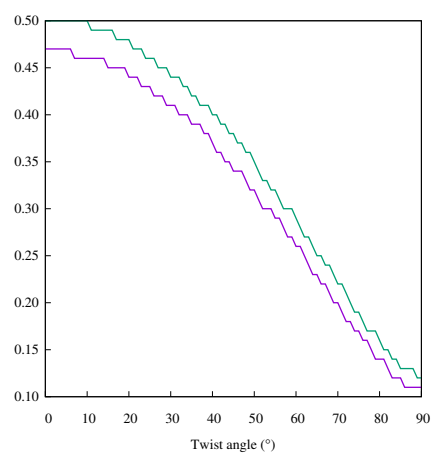

Figure S311: Reference (green) and approached (purple)  $\psi$  plots for the PP first excited-state computed at the TDHF/6-31+G(d,p) level of theory. The descriptors values are reported with respect to the pyridinium-phenolate twist angle amplitude.

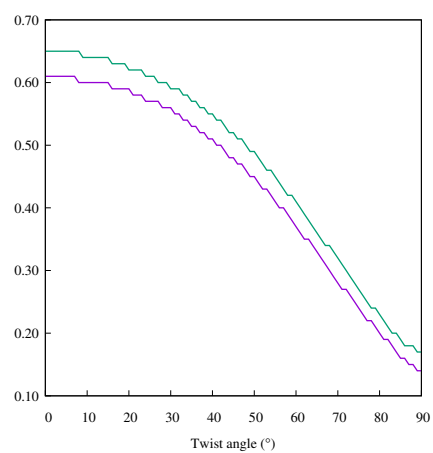

Figure S312: Reference (green) and approached (purple)  $\phi_S$  plots for the PP first excited-state computed at the TDHF/6-31+G level of theory. The descriptors values are reported with respect to the pyridinium-phenolate twist angle amplitude.

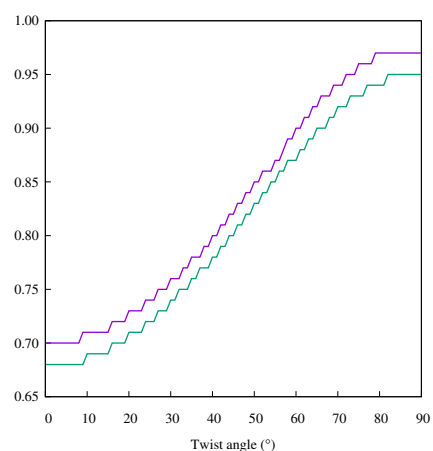

Figure S313: Reference (green) and approached (purple)  $\varphi$  plots for the PP first excited-state computed at the TDHF/6-31+G level of theory. The descriptors values are reported with respect to the pyridinium-phenolate twist angle amplitude.

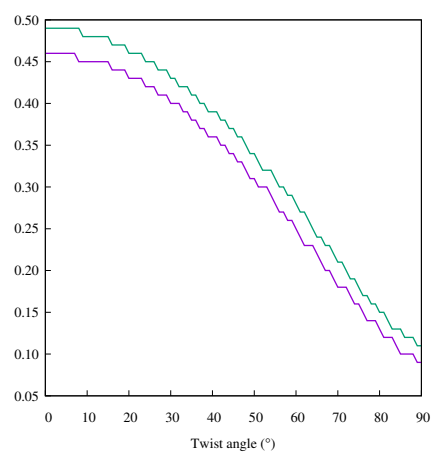

Figure S314: Reference (green) and approached (purple)  $\psi$  plots for the PP first excited-state computed at the TDHF/6-31+G level of theory. The descriptors values are reported with respect to the pyridinium-phenolate twist angle amplitude.

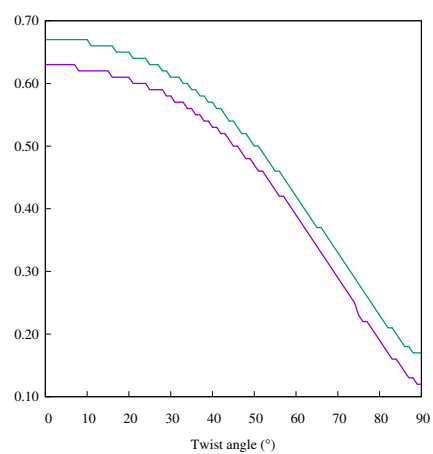

Figure S315: Reference (green) and approached (purple)  $\phi_S$  plots for the PP first excited-state computed at the TDHF/6-31G level of theory. The descriptors values are reported with respect to the pyridinium-phenolate twist angle amplitude.

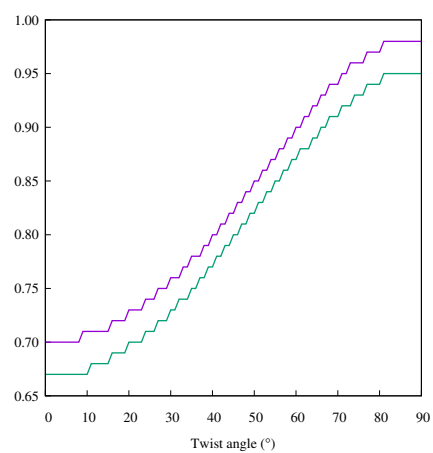

Figure S316: Reference (green) and approached (purple)  $\varphi$  plots for the PP first excited-state computed at the TDHF/6-31G level of theory. The descriptors values are reported with respect to the pyridinium-phenolate twist angle amplitude.

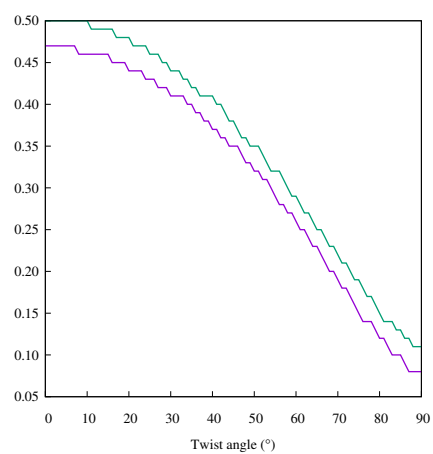

Figure S317: Reference (green) and approached (purple)  $\psi$  plots for the PP first excited-state computed at the TDHF/6-31G level of theory. The descriptors values are reported with respect to the pyridinium-phenolate twist angle amplitude.

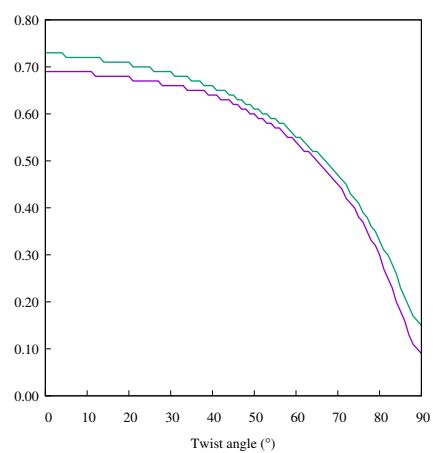

Figure S318: Reference (green) and approached (purple)  $\phi_S$  plots for the PP first excited-state computed at the wB97XD/3-21G level of theory. The descriptors values are reported with respect to the pyridinium-phenolate twist angle amplitude.

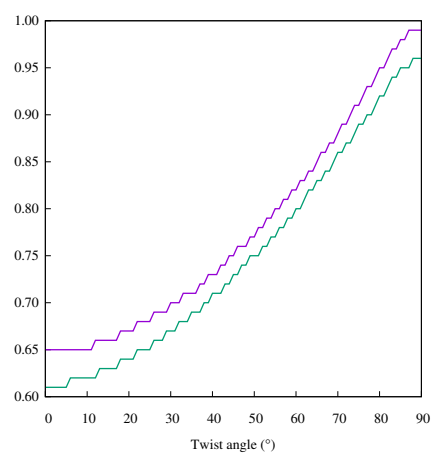

Figure S319: Reference (green) and approached (purple)  $\varphi$  plots for the PP first excited-state computed at the wB97XD/3-21G level of theory. The descriptors values are reported with respect to the pyridinium-phenolate twist angle amplitude.

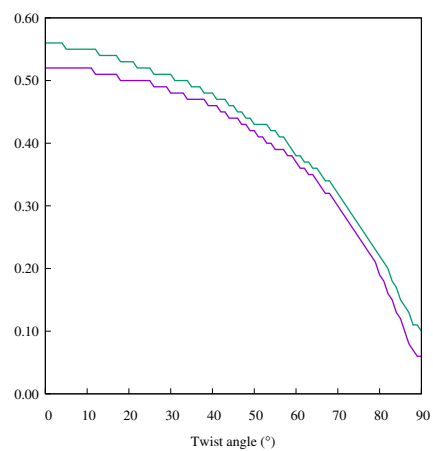

Figure S320: Reference (green) and approached (purple)  $\psi$  plots for the PP first excited-state computed at the wB97XD/3-21G level of theory. The descriptors values are reported with respect to the pyridinium-phenolate twist angle amplitude.

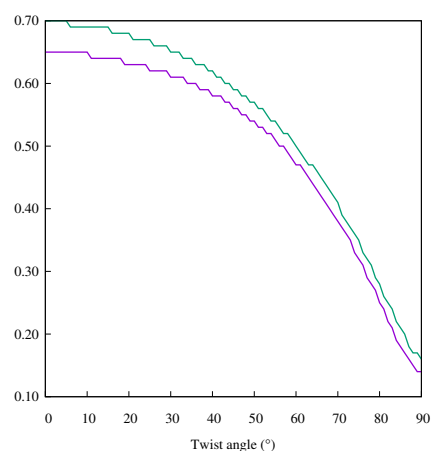

Figure S321: Reference (green) and approached (purple)  $\phi_S$  plots for the PP first excited-state computed at the wB97XD/6-311++G(2d,p) level of theory. The descriptors values are reported with respect to the pyridinium-phenolate twist angle amplitude.

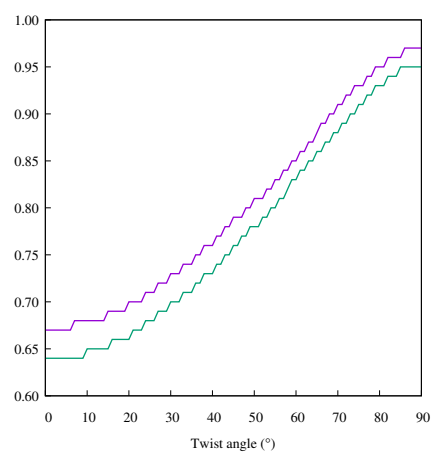

Figure S322: Reference (green) and approached (purple)  $\phi$  plots for the PP first excited-state computed at the wB97XD/6-311++G(2d,p) level of theory. The descriptors values are reported with respect to the pyridinium-phenolate twist angle amplitude.

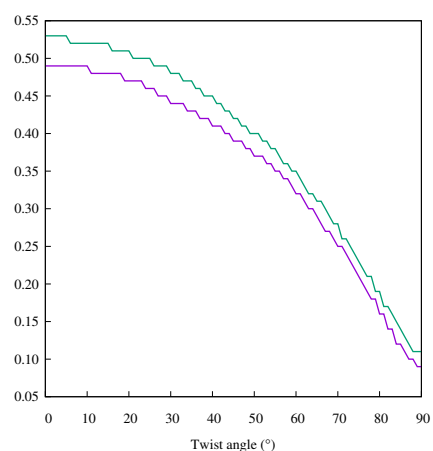

Figure S323: Reference (green) and approached (purple)  $\psi$  plots for the PP first excited-state computed at the wB97XD/6-311++G(2d,p) level of theory. The descriptors values are reported with respect to the pyridinium-phenolate twist angle amplitude.

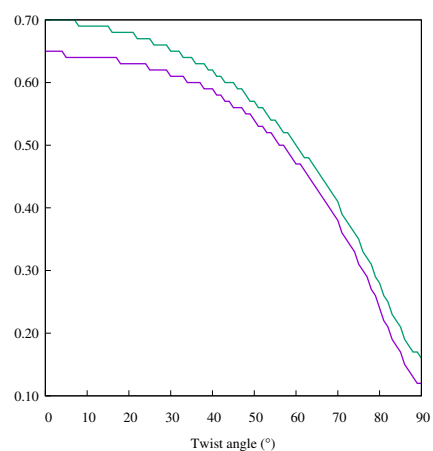

Figure S324: Reference (green) and approached (purple)  $\phi_S$  plots for the PP first excited-state computed at the wB97XD/6-311+G(d) level of theory. The descriptors values are reported with respect to the pyridinium-phenolate twist angle amplitude.



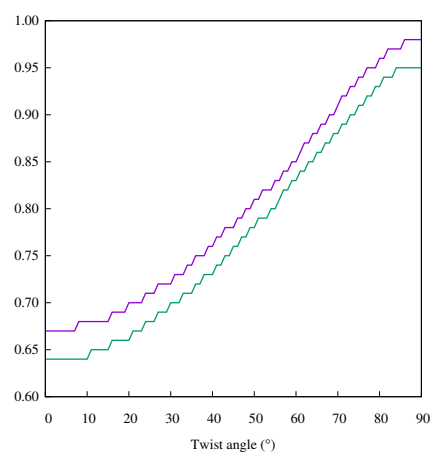

Figure S325: Reference (green) and approached (purple)  $\varphi$  plots for the PP first excited-state computed at the wB97XD/6-311+G(d) level of theory. The descriptors values are reported with respect to the pyridinium-phenolate twist angle amplitude.

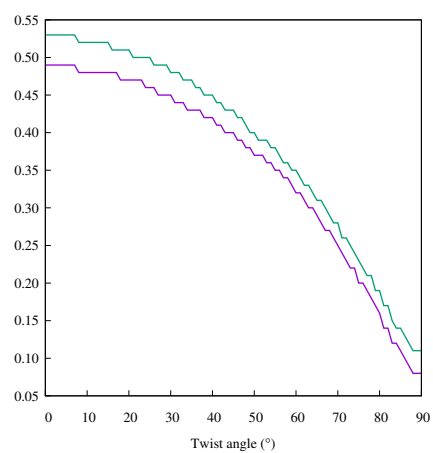

Figure S326: Reference (green) and approached (purple)  $\psi$  plots for the PP first excited-state computed at the wB97XD/6-311+G(d) level of theory. The descriptors values are reported with respect to the pyridinium-phenolate twist angle amplitude.

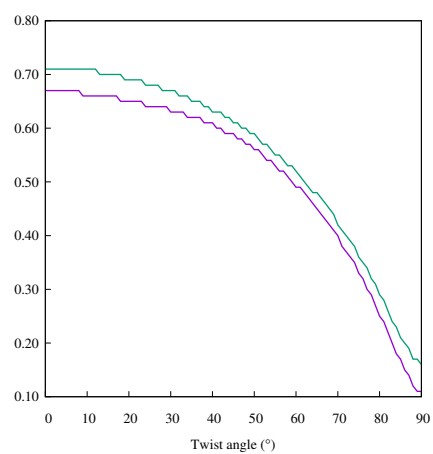

Figure S327: Reference (green) and approached (purple)  $\phi_S$  plots for the PP first excited-state computed at the wB97XD/6-311G(d) level of theory. The descriptors values are reported with respect to the pyridinium-phenolate twist angle amplitude.

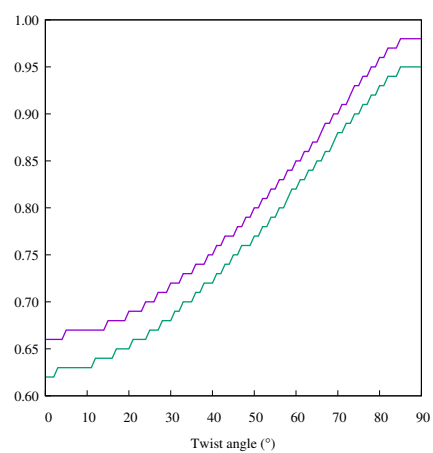

Figure S328: Reference (green) and approached (purple)  $\varphi$  plots for the PP first excited-state computed at the wB97XD/6-311G(d) level of theory. The descriptors values are reported with respect to the pyridinium-phenolate twist angle amplitude.

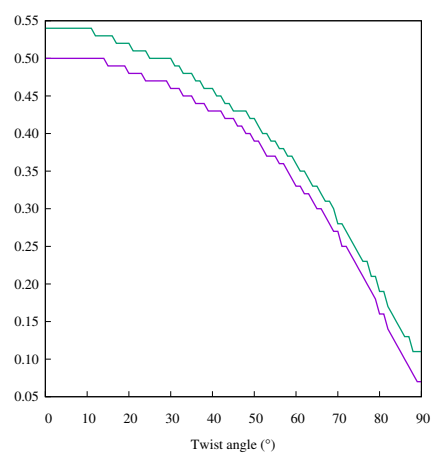

Figure S329: Reference (green) and approached (purple)  $\psi$  plots for the PP first excited-state computed at the wB97XD/6-311G(d) level of theory. The descriptors values are reported with respect to the pyridinium-phenolate twist angle amplitude.

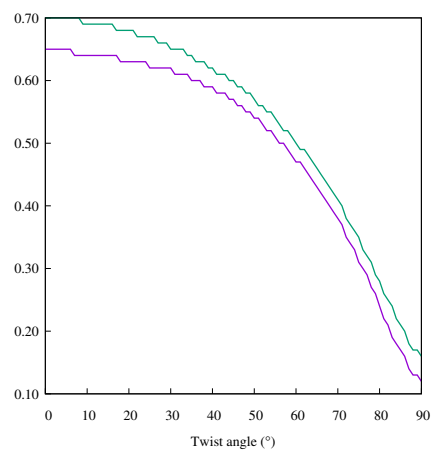

Figure S330: Reference (green) and approached (purple)  $\phi_S$  plots for the PP first excited-state computed at the wB97XD/6-311++G(d,p) level of theory. The descriptors values are reported with respect to the pyridinium-phenolate twist angle amplitude.

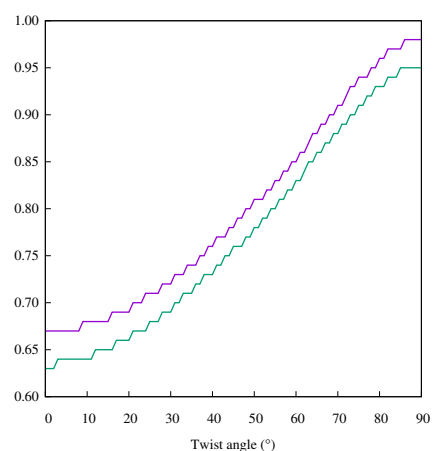

Figure S331: Reference (green) and approached (purple)  $\varphi$  plots for the PP first excited-state computed at the wB97XD/6-311++G(d,p) level of theory. The descriptors values are reported with respect to the pyridinium-phenolate twist angle amplitude.

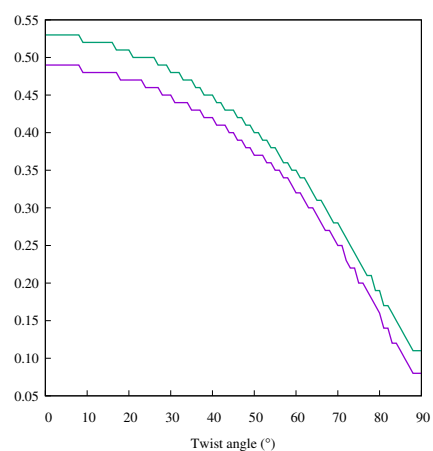

Figure S332: Reference (green) and approached (purple)  $\psi$  plots for the PP first excited-state computed at the wB97XD/6-311++G(d,p) level of theory. The descriptors values are reported with respect to the pyridinium-phenolate twist angle amplitude.

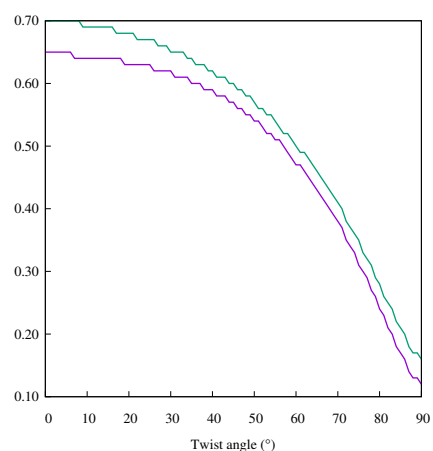

Figure S333: Reference (green) and approached (purple)  $\phi_S$  plots for the PP first excited-state computed at the wB97XD/6-311+G(d,p) level of theory. The descriptors values are reported with respect to the pyridinium-phenolate twist angle amplitude.

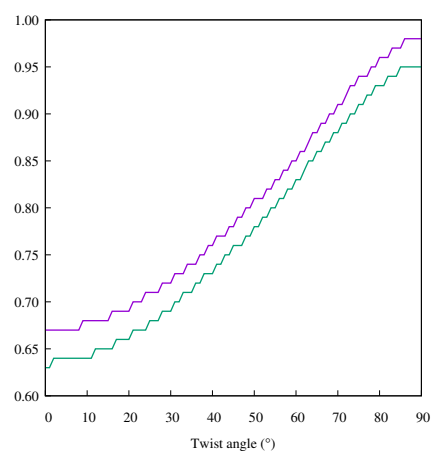

Figure S334: Reference (green) and approached (purple)  $\varphi$  plots for the PP first excited-state computed at the wB97XD/6-311+G(d,p) level of theory. The descriptors values are reported with respect to the pyridinium-phenolate twist angle amplitude.

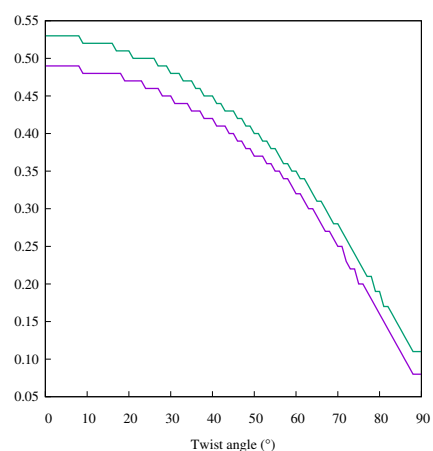

Figure S335: Reference (green) and approached (purple)  $\psi$  plots for the PP first excited-state computed at the wB97XD/6-311+G(d,p) level of theory. The descriptors values are reported with respect to the pyridinium-phenolate twist angle amplitude.

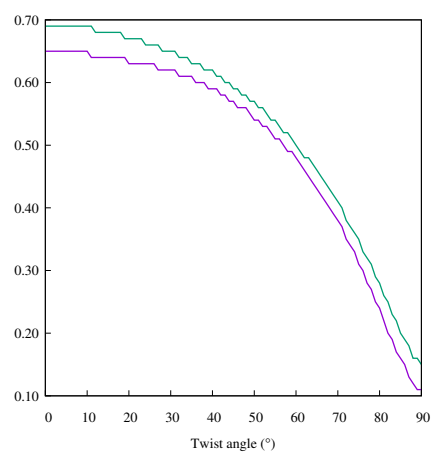

Figure S336: Reference (green) and approached (purple)  $\phi_S$  plots for the PP first excited-state computed at the wB97XD/6-311+G level of theory. The descriptors values are reported with respect to the pyridinium-phenolate twist angle amplitude.

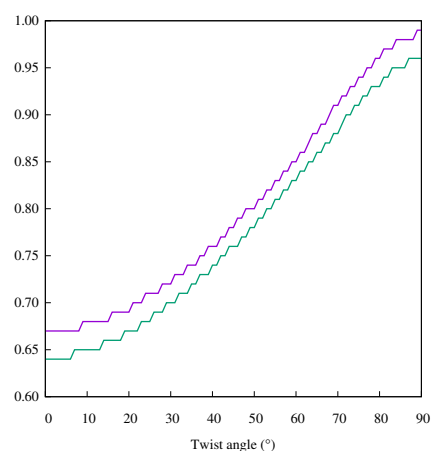

Figure S337: Reference (green) and approached (purple)  $\varphi$  plots for the PP first excited-state computed at the wB97XD/6-311+G level of theory. The descriptors values are reported with respect to the pyridinium-phenolate twist angle amplitude.

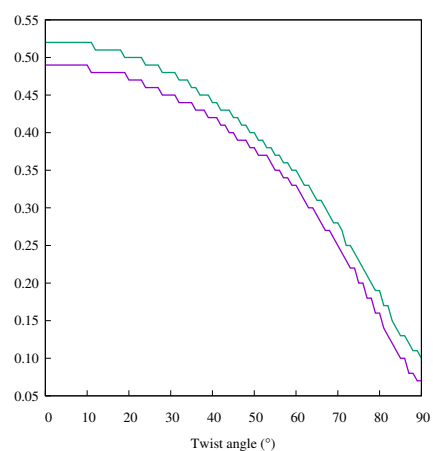

Figure S338: Reference (green) and approached (purple)  $\psi$  plots for the PP first excited-state computed at the wB97XD/6-311+G level of theory. The descriptors values are reported with respect to the pyridinium-phenolate twist angle amplitude.

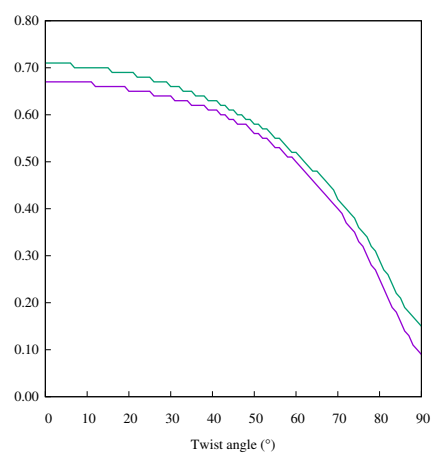

Figure S339: Reference (green) and approached (purple)  $\phi_S$  plots for the PP first excited-state computed at the wB97XD/6-311G level of theory. The descriptors values are reported with respect to the pyridinium-phenolate twist angle amplitude.

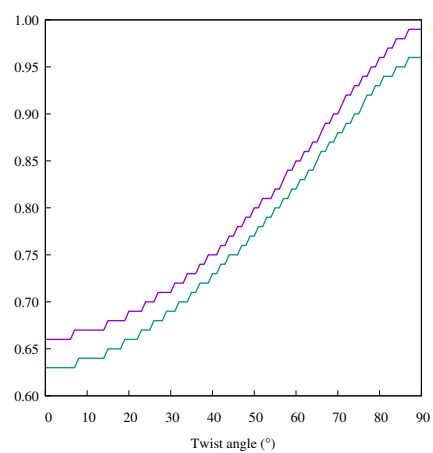

Figure S340: Reference (green) and approached (purple)  $\varphi$  plots for the PP first excited-state computed at the wB97XD/6-311G level of theory. The descriptors values are reported with respect to the pyridinium-phenolate twist angle amplitude.



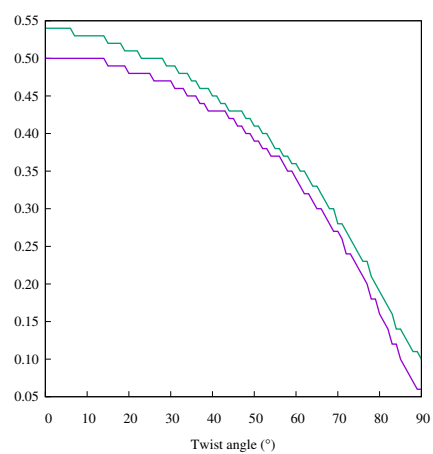

Figure S341: Reference (green) and approached (purple)  $\psi$  plots for the PP first excited-state computed at the wB97XD/6-311G level of theory. The descriptors values are reported with respect to the pyridinium-phenolate twist angle amplitude.

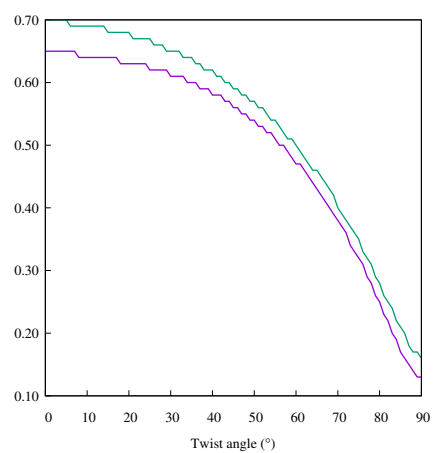

Figure S342: Reference (green) and approached (purple)  $\phi_S$  plots for the PP first excited-state computed at the wB97XD/6-31++G(2d,p) level of theory. The descriptors values are reported with respect to the pyridinium-phenolate twist angle amplitude.

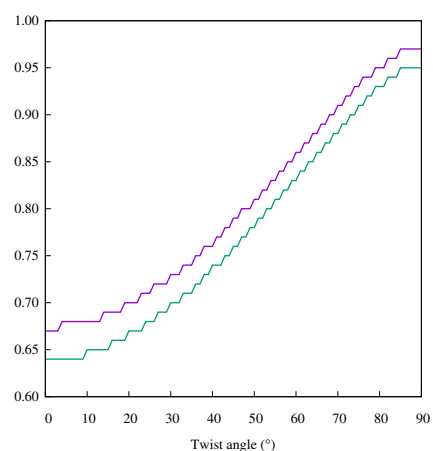

Figure S343: Reference (green) and approached (purple)  $\varphi$  plots for the PP first excited-state computed at the wB97XD/6-31++G(2d,p) level of theory. The descriptors values are reported with respect to the pyridinium-phenolate twist angle amplitude.

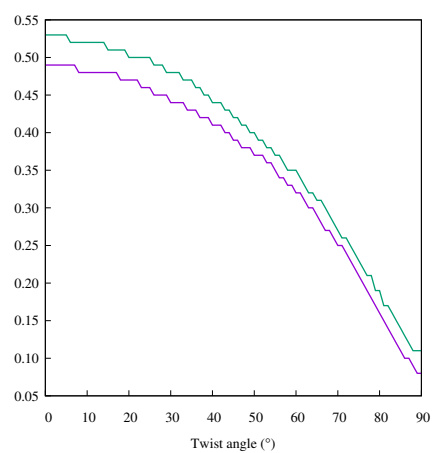

Figure S344: Reference (green) and approached (purple)  $\psi$  plots for the PP first excited-state computed at the wB97XD/6-31++G(2d,p) level of theory. The descriptors values are reported with respect to the pyridinium-phenolate twist angle amplitude.

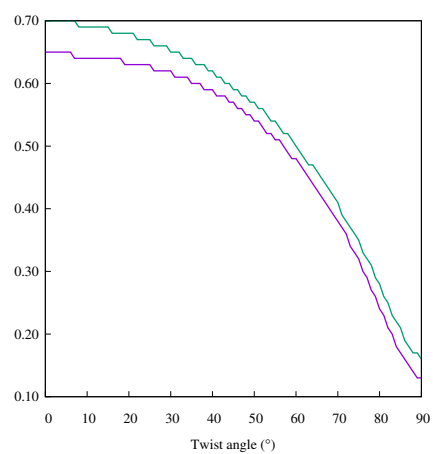

Figure S345: Reference (green) and approached (purple)  $\phi_S$  plots for the PP first excited-state computed at the wB97XD/6-31+G(d) level of theory. The descriptors values are reported with respect to the pyridinium-phenolate twist angle amplitude.

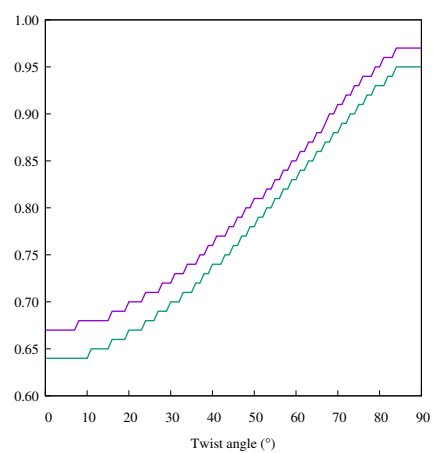

Figure S346: Reference (green) and approached (purple)  $\varphi$  plots for the PP first excited-state computed at the wB97XD/6-31+G(d) level of theory. The descriptors values are reported with respect to the pyridinium-phenolate twist angle amplitude.

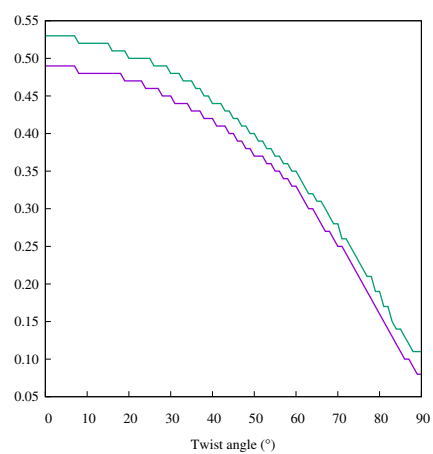

Figure S347: Reference (green) and approached (purple)  $\psi$  plots for the PP first excited-state computed at the wB97XD/6-31+G(d) level of theory. The descriptors values are reported with respect to the pyridinium-phenolate twist angle amplitude.

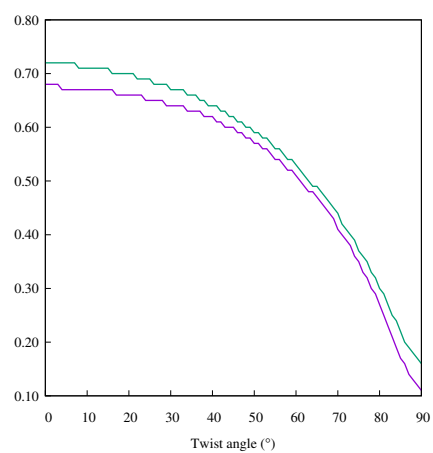

Figure S348: Reference (green) and approached (purple)  $\phi_S$  plots for the PP first excited-state computed at the wB97XD/6-31G(d) level of theory. The descriptors values are reported with respect to the pyridinium-phenolate twist angle amplitude.

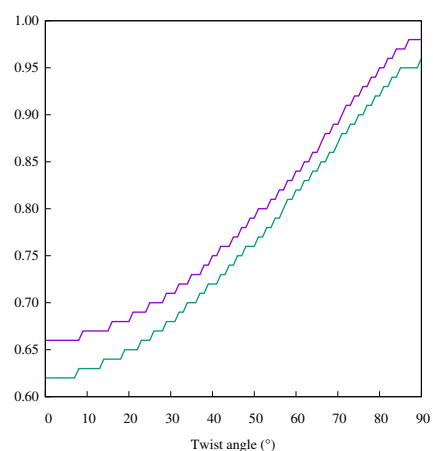

Figure S349: Reference (green) and approached (purple)  $\varphi$  plots for the PP first excited-state computed at the wB97XD/6-31G(d) level of theory. The descriptors values are reported with respect to the pyridinium-phenolate twist angle amplitude.

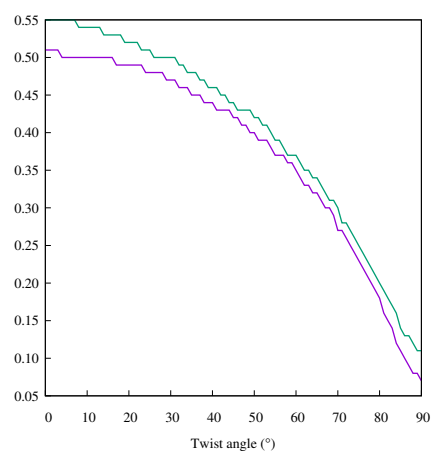

Figure S350: Reference (green) and approached (purple)  $\psi$  plots for the PP first excited-state computed at the wB97XD/6-31G(d) level of theory. The descriptors values are reported with respect to the pyridinium-phenolate twist angle amplitude.

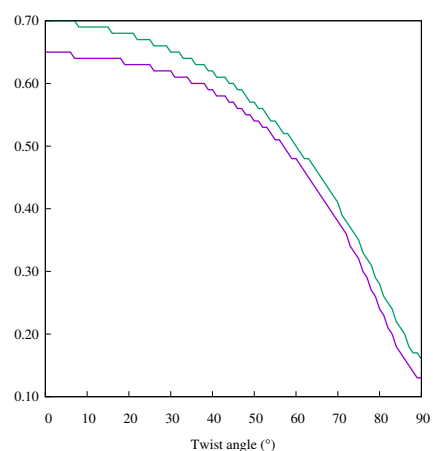

Figure S351: Reference (green) and approached (purple)  $\phi_S$  plots for the PP first excited-state computed at the wB97XD/6-31++G(d,p) level of theory. The descriptors values are reported with respect to the pyridinium-phenolate twist angle amplitude.

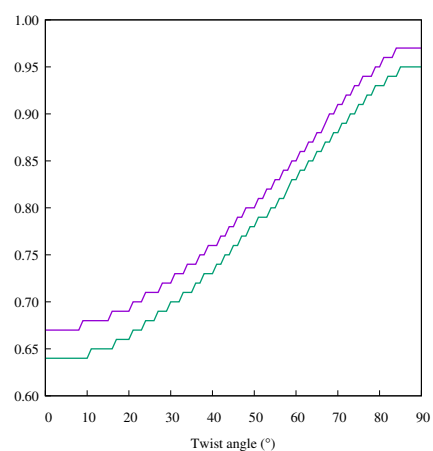

Figure S352: Reference (green) and approached (purple)  $\varphi$  plots for the PP first excited-state computed at the wB97XD/6-31++G(d,p) level of theory. The descriptors values are reported with respect to the pyridinium-phenolate twist angle amplitude.

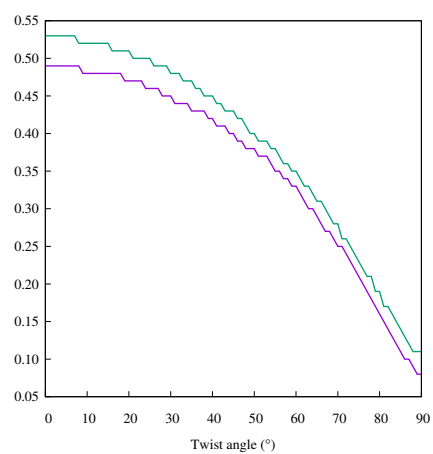

Figure S353: Reference (green) and approached (purple)  $\psi$  plots for the PP first excited-state computed at the wB97XD/6-31++G(d,p) level of theory. The descriptors values are reported with respect to the pyridinium-phenolate twist angle amplitude.

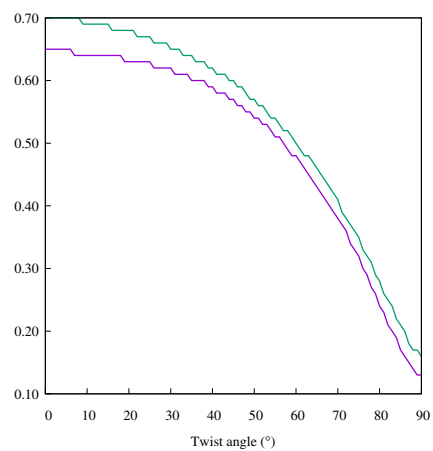

Figure S354: Reference (green) and approached (purple)  $\phi_S$  plots for the PP first excited-state computed at the wB97XD/6-31+G(d,p) level of theory. The descriptors values are reported with respect to the pyridinium-phenolate twist angle amplitude.

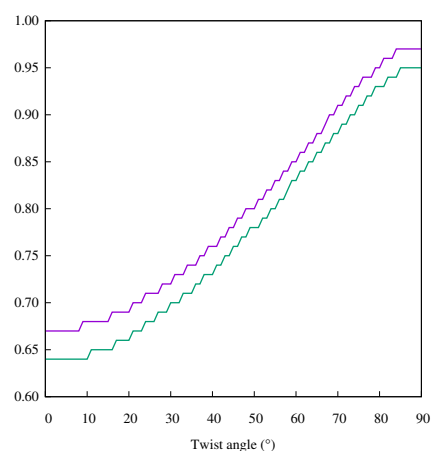

Figure S355: Reference (green) and approached (purple)  $\varphi$  plots for the PP first excited-state computed at the wB97XD/6-31+G(d,p) level of theory. The descriptors values are reported with respect to the pyridinium-phenolate twist angle amplitude.

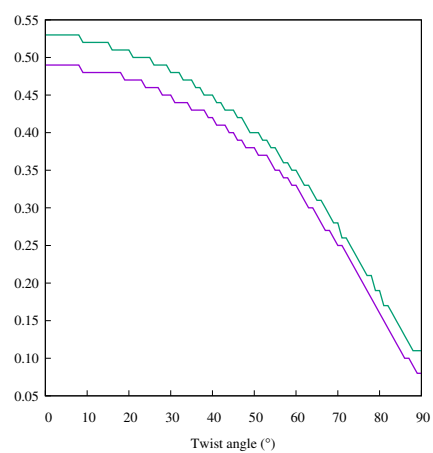

Figure S356: Reference (green) and approached (purple)  $\psi$  plots for the PP first excited-state computed at the wB97XD/6-31+G(d,p) level of theory. The descriptors values are reported with respect to the pyridinium-phenolate twist angle amplitude.



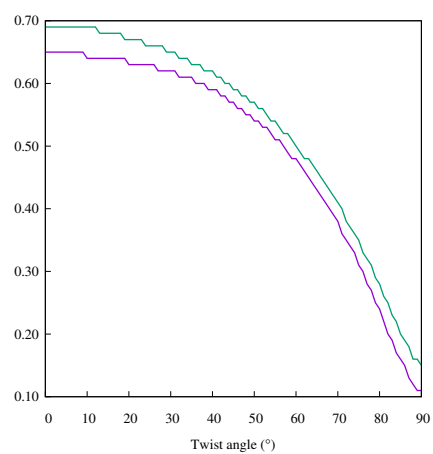

Figure S357: Reference (green) and approached (purple)  $\phi_S$  plots for the PP first excited-state computed at the wB97XD/6-31+G level of theory. The descriptors values are reported with respect to the pyridinium-phenolate twist angle amplitude.

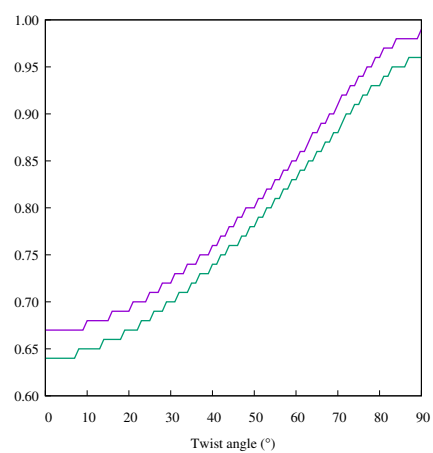

Figure S358: Reference (green) and approached (purple)  $\varphi$  plots for the PP first excited-state computed at the wB97XD/6-31+G level of theory. The descriptors values are reported with respect to the pyridinium-phenolate twist angle amplitude.

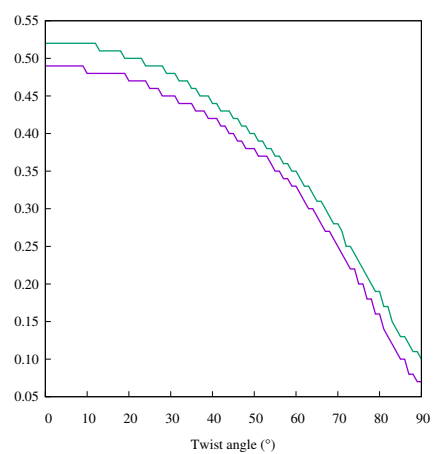

Figure S359: Reference (green) and approached (purple)  $\psi$  plots for the PP first excited-state computed at the wB97XD/6-31+G level of theory. The descriptors values are reported with respect to the pyridinium-phenolate twist angle amplitude.

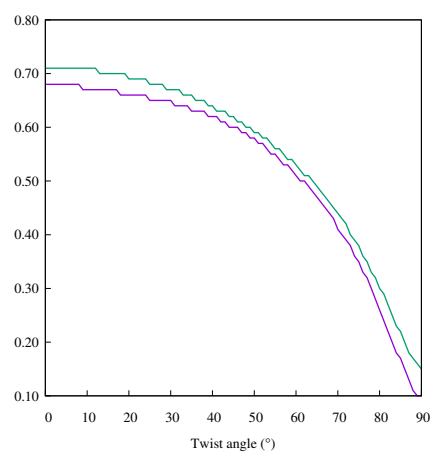

Figure S360: Reference (green) and approached (purple)  $\phi_S$  plots for the PP first excited-state computed at the wB97XD/6-31G level of theory. The descriptors values are reported with respect to the pyridinium-phenolate twist angle amplitude.

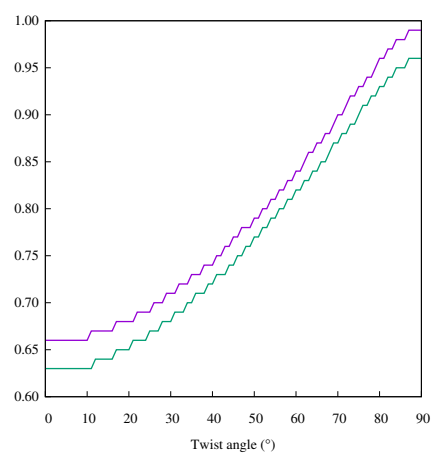

Figure S361: Reference (green) and approached (purple)  $\varphi$  plots for the PP first excited-state computed at the wB97XD/6-31G level of theory. The descriptors values are reported with respect to the pyridinium-phenolate twist angle amplitude.

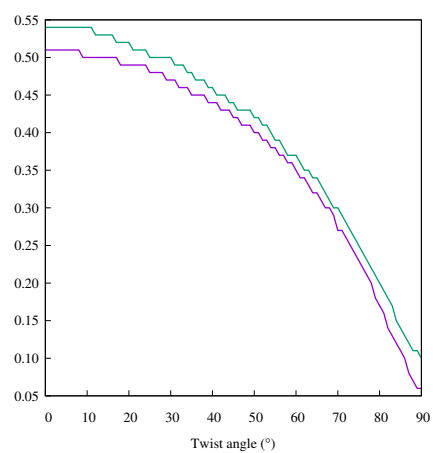

Figure S362: Reference (green) and approached (purple)  $\psi$  plots for the PP first excited-state computed at the wB97XD/6-31G level of theory. The descriptors values are reported with respect to the pyridinium-phenolate twist angle amplitude.

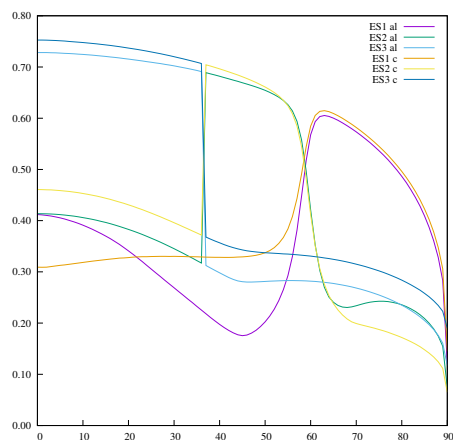

Figure S363: Reference (c) and approached (al)  $\phi_S$  plots for the first three excited-states (ES) of the PP molecule computed at the B3LYP/6-311++G(2d,p) level of theory, reported with respect to the central twist angle amplitude ( $^{\circ}$ )

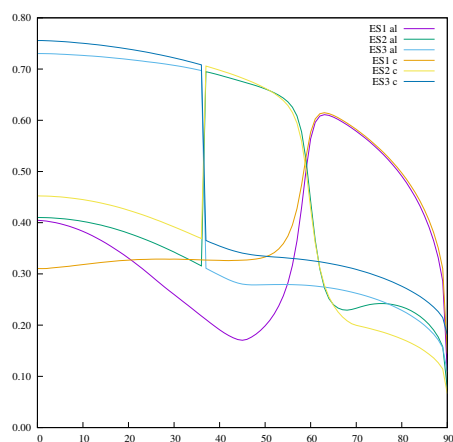

Figure S364: Reference (c) and approached (al)  $\phi_S$  plots for the first three excited-states (ES) of the PP molecule computed at the B3LYP/6-31+G(d,p) level of theory, reported with respect to the central twist angle amplitude ( $^{\circ}$ )

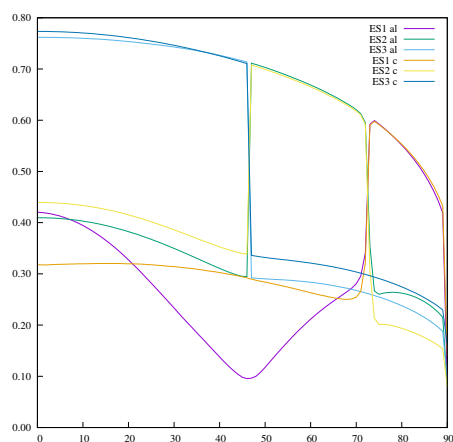

Figure S363: Reference (c) and approached (al)  $\phi_S$  plots for the first three excited-states (ES) of the PP molecule computed at the B3LYP/6-31G level of theory, reported with respect to the central twist angle amplitude ( $^\circ$ )

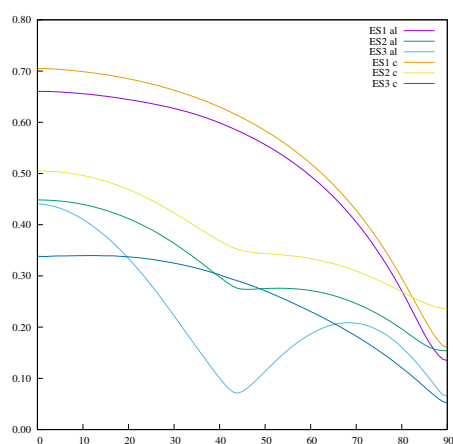

Figure S365: Reference (c) and approached (al)  $\phi_S$  plots for the first three excited-states (ES) of the PP molecule computed at the CAM-B3LYP/6-311++G(2d,p) level of theory, reported with respect to the central twist angle amplitude ( $^\circ$ )

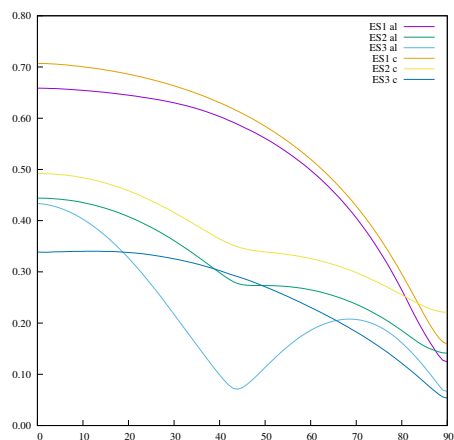

Figure S366: Reference (c) and approached (al)  $\phi_S$  plots for the first three excited-states (ES) of the PP molecule computed at the CAM-B3LYP/6-31+G(d,p) level of theory, reported with respect to the central twist angle amplitude ( $^\circ$ )

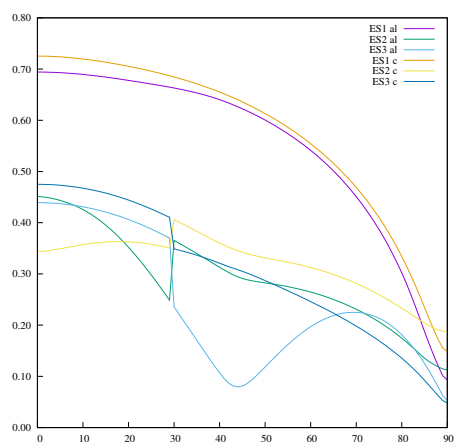

Figure S367: Reference (c) and approached (al)  $\phi_S$  plots for the first three excited-states (ES) of the PP molecule computed at the CAM-B3LYP/6-31G level of theory, reported with respect to the central twist angle amplitude ( $^\circ$ )

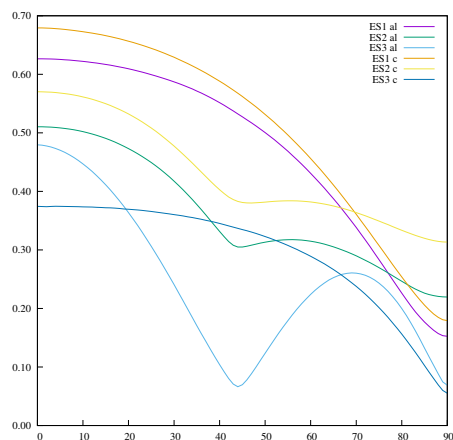

Figure S368: Reference (c) and approached (al)  $\phi_S$  plots for the first three excited-states (ES) of the PP molecule computed at the LC-wHPBE/6-311++G(2d,p) level of theory, reported with respect to the central twist angle amplitude ( $^\circ$ )

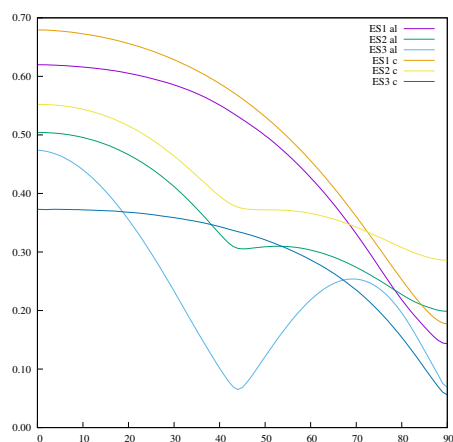

Figure S369: Reference (c) and approached (al)  $\phi_S$  plots for the first three excited-states (ES) of the PP molecule computed at the LC-wHPBE/6-31+G(d,p) level of theory, reported with respect to the central twist angle amplitude ( $^\circ$ )

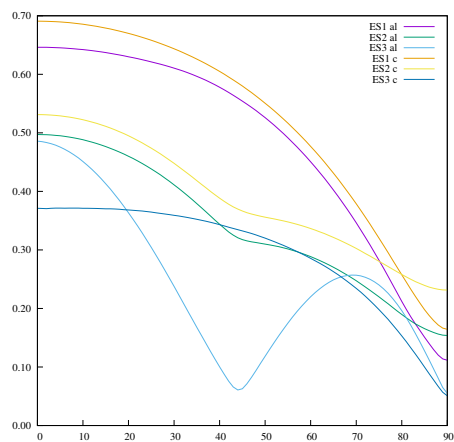

Figure S370: Reference (c) and approached (al)  $\phi_S$  plots for the first three excited-states (ES) of the PP molecule computed at the LC-wHPBE/6-31G level of theory, reported with respect to the central twist angle amplitude ( $^\circ$ )

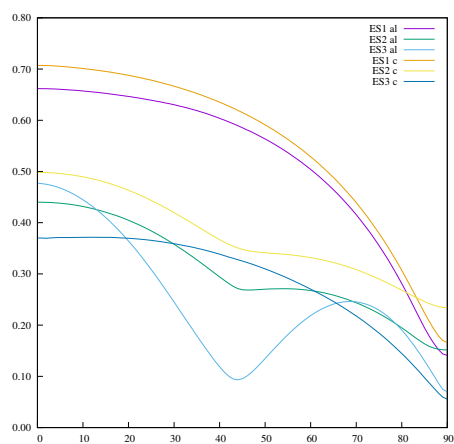

Figure S371: Reference (c) and approached (al)  $\phi_S$  plots for the first three excited-states (ES) of the PP molecule computed at the M062X/6-311++G(2d,p) level of theory, reported with respect to the central twist angle amplitude ( $^\circ$ )



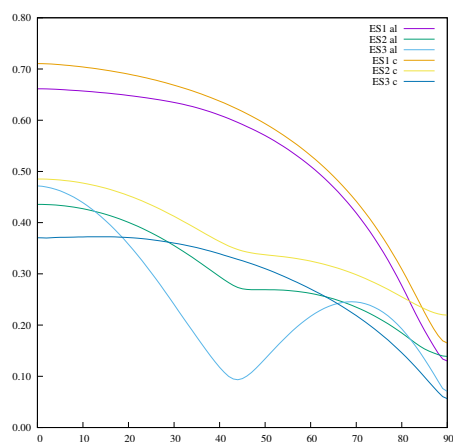

Figure S372: Reference (c) and approached (al)  $\phi_S$  plots for the first three excited-states (ES) of the PP molecule computed at the M062X/6-31+G(d,p) level of theory, reported with respect to the central twist angle amplitude ( $^\circ$ )

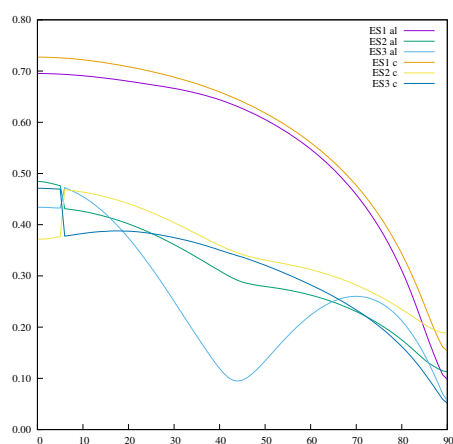

Figure S373: Reference (c) and approached (al)  $\phi_S$  plots for the first three excited-states (ES) of the PP molecule computed at the M062X/6-31G level of theory, reported with respect to the central twist angle amplitude ( $^\circ$ )

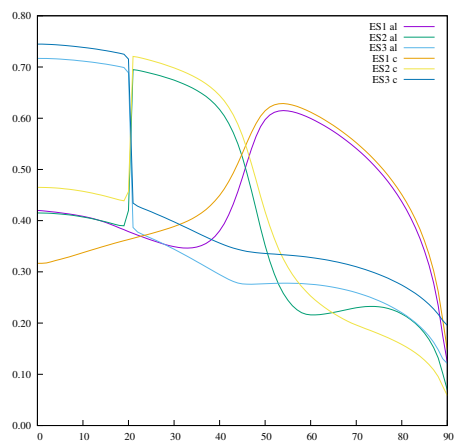

Figure S374: Reference (c) and approached (al)  $\phi_S$  plots for the first three excited-states (ES) of the PP molecule computed at the PBE0/6-311++G(2d,p) level of theory, reported with respect to the central twist angle amplitude ( $^{\circ}$ )

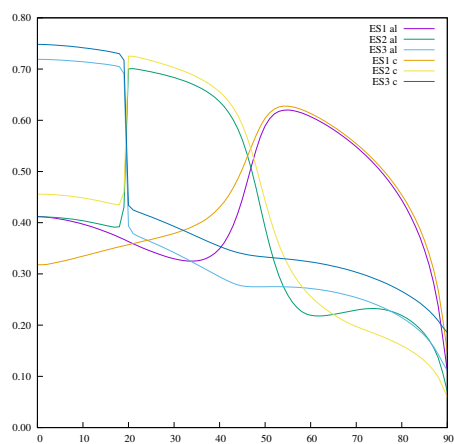

Figure S375: Reference (c) and approached (al)  $\phi_S$  plots for the first three excited-states (ES) of the PP molecule computed at the PBE0/6-31+G(d,p) level of theory, reported with respect to the central twist angle amplitude ( $^{\circ}$ )

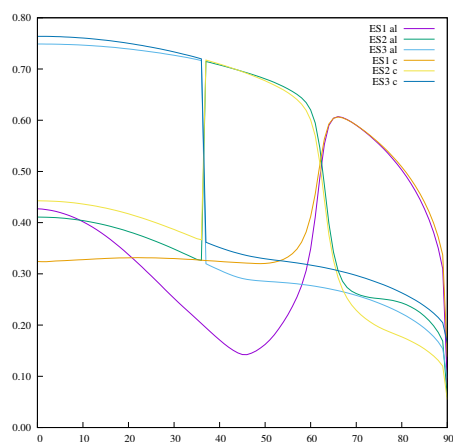

Figure S363: Reference (c) and approached (al)  $\phi_S$  plots for the first three excited-states (ES) of the PP molecule computed at the PBE0/6-31G level of theory, reported with respect to the central twist angle amplitude ( $^\circ$ )

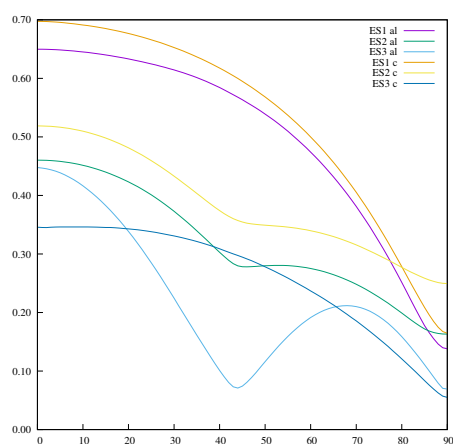

Figure S376: Reference (c) and approached (al)  $\phi_S$  plots for the first three excited-states (ES) of the PP molecule computed at the wb97XD/6-311++G(2d,p) level of theory, reported with respect to the central twist angle amplitude ( $^\circ$ )

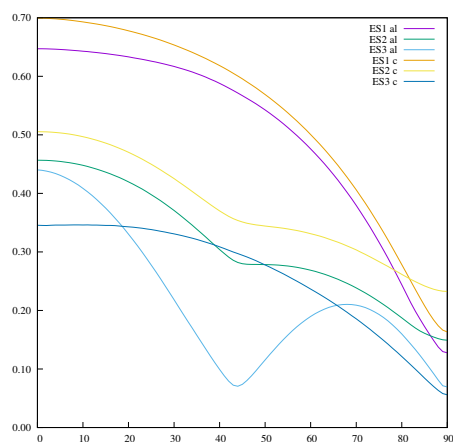

Figure S377: Reference (c) and approached (al)  $\phi_S$  plots for the first three excited-states (ES) of the PP molecule computed at the wB97XD/6-31+G(d,p) level of theory, reported with respect to the central twist angle amplitude ( $^\circ$ )

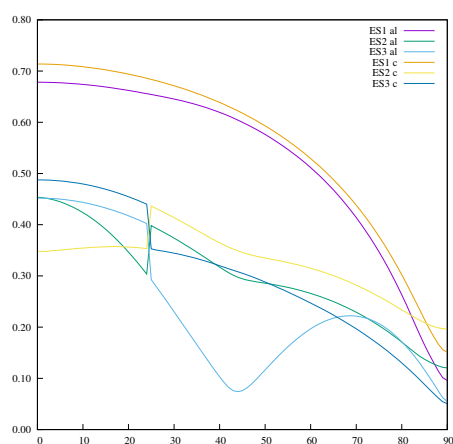

Figure S378: Reference (c) and approached (al)  $\phi_S$  plots for the first three excited-states (ES) of the PP molecule computed at the wB97XD/6-31G level of theory, reported with respect to the central twist angle amplitude ( $^\circ$ )
